# Supplementary material for: Review of AdS/CFT Integrability: An Overview
Source: arXiv:1012.3982 ancillary file (2012-02-21)
Supplement: Supplementary file 1 [file IntAdS.pdf]

# Review of AdS/CFT Integrability

This is a collection of article preprints that have appeared as a review of AdS/CFT integrability.

The following table lists the review chapters contained in this document. Refereed content is marked. The attached chapters are preprints taken from arXiv.org. The table lists the arXiv identifier, the reproduced version number and the arXiv submission date.

All chapters have been refereed and published in the journal “Letters in Mathematical Physics”, volume 99 (2012). For each chapter we list the journal page numbers together with the submission date of the accepted article.

| chapter | page | ref | arXiv id  | ver | date     | LMP pp.       | date                 |
|---------|------|-----|-----------|-----|----------|---------------|----------------------|
| 0       | 3    | ✓   | 1012.3982 | v5  | 21.02.12 | 1– 2<br>3– 32 | 04.07.11<br>04.07.11 |
| I.1     | 35   | ✓   | 1012.3983 | v3  | 15.07.11 | 33– 58        | 10.07.11             |
| I.2     | 61   | ✓   | 1012.3984 | v3  | 06.12.11 | 59– 84        | 25.04.11             |
| I.3     | 87   | ✓   | 1012.3985 | v3  | 30.11.11 | 85–102        | 05.05.11             |
| II.1    | 105  | ✓   | 1012.3986 | v3  | 22.01.11 | 103–125       | 22.01.11             |
| II.2    | 129  | –   | 1012.3987 | v2  | 20.12.10 | 127–148       | 03.05.11             |
| II.3    | 149  | ✓   | 1012.3988 | v3  | 01.03.11 | 149–167       | 17.02.11             |
| II.4    | 167  | ✓   | 1012.3989 | v3  | 26.09.11 | 169–190       | 09.08.11             |
| III.1   | 189  | ✓   | 1012.3990 | v3  | 24.11.11 | 191–208       | 27.02.11             |
| III.2   | 207  | ✓   | 1012.3991 | v3  | 11.02.11 | 209–229       | 11.02.11             |
| III.3   | 229  | –   | 1012.3992 | v2  | 20.12.10 | 231–253       | 23.02.11             |
| III.4   | 251  | ✓   | 1012.3993 | v4  | 04.11.11 | 255–276       | 11.02.11             |
| III.5   | 273  | ✓   | 1012.3994 | v4  | 18.08.11 | 277–297       | 26.03.11             |
| III.6   | 293  | ✓   | 1012.3995 | v3  | 18.07.11 | 299–320       | 09.02.11             |
| III.7   | 315  | –   | 1012.3996 | v2  | 20.12.10 | 321–347       | 25.04.11             |
| IV.1    | 339  | ✓   | 1012.3997 | v4  | 28.11.11 | 349–374       | 30.03.11             |
| IV.2    | 363  | ✓   | 1012.3998 | v4  | 29.08.11 | 375–400       | 18.04.11             |
| IV.3    | 387  | ✓   | 1012.3999 | v4  | 06.01.12 | 401–423       | 11.05.11             |
| IV.4    | 409  | –   | 1012.4000 | v2  | 20.12.10 | 425–453       | 05.05.11             |
| V.1     | 437  | –   | 1012.4001 | v2  | 20.12.10 | 455–479       | 11.04.11             |
| V.2     | 461  | –   | 1012.4002 | v3  | 18.01.11 | 481–505       | 16.05.11             |
| V.3     | 485  | ✓   | 1012.4003 | v3  | 14.12.11 | 507–528       | 25.04.11             |
| VI.1    | 507  | ✓   | 1012.4004 | v4  | 20.03.11 | 529–545       | 17.02.11             |
| VI.2    | 523  | ✓   | 1012.4005 | v5  | 07.11.11 | 547–565       | 25.02.11             |



## Review of AdS/CFT Integrability: An Overview

NIKLAS BEISERT<sup>†,1</sup>, CHANGRIM AHN<sup>2</sup>, LUIS F. ALDAY<sup>3,4</sup>, ZOLTÁN BAJNOK<sup>5</sup>,  
JAMES M. DRUMMOND<sup>6,7</sup>, LISA FREYHULT<sup>8</sup>, NIKOLAY GROMOV<sup>9,10</sup>,  
ROMUALD A. JANIK<sup>11</sup>, VLADIMIR KAZAKOV<sup>12,13</sup>, THOMAS KLOSE<sup>8,14</sup>,  
GREGORY P. KORCHEMSKY<sup>15</sup>, CHARLOTTE KRISTJANSEN<sup>16</sup>, MARC MAGRO<sup>17,1</sup>,  
TRISTAN MCLOUGHLIN<sup>1</sup>, JOSEPH A. MINAHAN<sup>8</sup>, RAFAEL I. NEPOMECHIE<sup>18</sup>,  
ADAM REJ<sup>19</sup>, RADU ROIBAN<sup>20</sup>, SAKURA SCHÄFER-NAMEKI<sup>9,21</sup>,  
CHRISTOPH SIEG<sup>22,23</sup>, MATTHIAS STAUDACHER<sup>22,1</sup>, ALESSANDRO TORRIELLI<sup>24,25</sup>,  
ARKADY A. TSEYTLIN<sup>19</sup>, PEDRO VIEIRA<sup>26</sup>, DMYTRO VOLIN<sup>20</sup> AND  
KONSTANTINOS ZOUBOS<sup>16</sup>

<sup>†</sup>corresponding author, e-mail address: nbeisert@aei.mpg.de

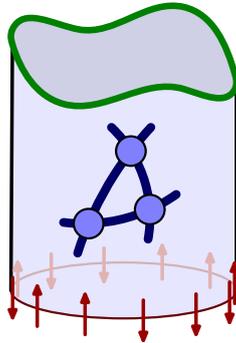

**Abstract:** This is the introductory chapter of a review collection on integrability in the context of the AdS/CFT correspondence. In the collection we present an overview of the achievements and the status of this subject as of the year 2010.

**Addresses:**

- <sup>1</sup> *Max-Planck-Institut für Gravitationsphysik, Albert-Einstein-Institut  
Am Mühlenberg 1, 14476 Potsdam, Germany*
- <sup>2</sup> *Department of Physics and Institute for the Early Universe  
Ewha Womans University, Seoul 120-750, South Korea*
- <sup>3</sup> *Mathematical Institute, University of Oxford  
24-29 St. Giles', Oxford OX1 3LB, U.K.*
- <sup>4</sup> *School of Natural Sciences, Institute for Advanced Study, Princeton, NJ 08540, USA*
- <sup>5</sup> *Theoretical Physics Research Group of the Hungarian Academy of Sciences  
1117 Pázmány s. 1/A, Budapest, Hungary*
- <sup>6</sup> *PH-TH Division, CERN, Geneva, Switzerland*
- <sup>7</sup> *LAPTH, Université de Savoie, CNRS  
B.P. 110, 74941 Annecy-le-Vieux Cedex, France*
- <sup>8</sup> *Department of Physics and Astronomy, Division for Theoretical Physics  
Uppsala University, Box 516, SE-751 08 Uppsala, Sweden*
- <sup>9</sup> *Department of Mathematics, King's College, The Strand, London, WC2R 2LS, U.K.*
- <sup>10</sup> *PNPI, Gatchina, Leningrad District, 188300 St. Petersburg, Russia*
- <sup>11</sup> *Institute of Physics, Jagiellonian University  
ul. Reymonta 4, 30-059 Kraków, Poland*
- <sup>12</sup> *LPT, Ecole Normale Supérieure, 24 rue Lhomond, 75231 Paris Cedex 05, France*
- <sup>13</sup> *Université Pierre et Marie Curie (Paris-VI), 4 Place Jussieu, 75252 Paris Cedex 05, France*
- <sup>14</sup> *Princeton Center for Theoretical Science  
Princeton University, Princeton, NJ 08544, USA*
- <sup>15</sup> *Institut de Physique Théorique, CEA Saclay  
91191 Gif-sur-Yvette Cedex, France*
- <sup>16</sup> *The Niels Bohr Institute, Blegdamsvej 17, 2100 Copenhagen, Denmark*
- <sup>17</sup> *Université de Lyon, Laboratoire de Physique, ENS Lyon et CNRS UMR 5672,  
46 allée d'Italie, 69364 Lyon CEDEX 07, France*
- <sup>18</sup> *Physics Department, P.O. Box 248046, University of Miami  
Coral Gables, FL 33124, USA*
- <sup>19</sup> *Blackett Laboratory, Imperial College London, SW7 2AZ, U.K.*
- <sup>20</sup> *Department of Physics, The Pennsylvania State University  
University Park, PA 16802, USA*
- <sup>21</sup> *Kavli Institute for Theoretical Physics, University of California,  
Santa Barbara, CA 93106, USA*
- <sup>22</sup> *Institut für Mathematik und Institut für Physik, Humboldt-Universität zu Berlin  
Johann von Neumann-Haus, Rudower Chaussee 25, 12489 Berlin, Germany*
- <sup>23</sup> *Niels Bohr International Academy, Niels Bohr Institute  
Blegdamsvej 17, 2100 Copenhagen, Denmark*
- <sup>24</sup> *Department of Mathematics, University of York  
Heslington, York, YO10 5DD, U.K.*
- <sup>25</sup> *Institute for Theoretical Physics, Utrecht University  
Leuvenlaan 4, 3584 CE Utrecht, The Netherlands*
- <sup>26</sup> *Perimeter Institute for Theoretical Physics,  
Waterloo, Ontario N2L 2Y5, Canada*

## Preface

Since late 2002 tremendous and rapid progress has been made in exploring planar  $\mathcal{N} = 4$  super Yang–Mills theory and free IIB superstrings on the  $AdS_5 \times S^5$  background. These two models are claimed to be exactly dual by the AdS/CFT correspondence, and the novel results give full support to the duality. The key to this progress lies in the integrability of the free/planar sector of the AdS/CFT pair of models.

Many reviews of integrability in the context of the AdS/CFT correspondence are available in the literature. They cover selected branches of the subject which have appeared over the years. Still it becomes increasingly difficult to maintain an overview of the entire subject, even for experts. Already for several years there has been a clear demand for an up-to-date review to present a global view and summary of the subject, its motivation, techniques, results and implications.

Such a review appears to be a daunting task: With around 8 years of development and perhaps up to 1000 scientific articles written, the preparation would represent a major burden on the prospective authors. Therefore, our idea was to prepare a coordinated review collection to fill the gap of a missing global review for AdS/CFT integrability. Coordination consisted in carefully splitting up the subject into a number of coherent topics. These cover most aspects of the subject without overlapping too much. Each topic is reviewed by someone who has made important contributions to it. The collection is aimed at beginning students and at scientists working on different subjects, but also at experts who would like to (re)acquire an overview. Special care was taken to keep the chapters brief (around 20 pages), focused and self-contained in order to enable the interested reader to absorb a selected topic in one go.

As the individual chapters will not convey an overview of the subject as a whole, the purpose of the introductory chapter is to assemble the pieces of the puzzle into a bigger picture. It consists of two parts: The first part is a general review of AdS/CFT integrability. It concentrates on setting the scene, outlining the achievements and putting them into context. It tries to provide a qualitative understanding of what integrability is good for and how and why it works. The second part maps out how the topics/chapters fit together and make up the subject. It also contains sketches of the contents of each chapter. This part helps the reader in identifying the chapters (s)he is most interested in.

There are reasons for and against combining all the contributions into one article or book. Practical issues however make it advisable to have the chapters appear as autonomous review articles. After all, they are the works of individuals. They are merely tied together by the introductory chapter on which all the contributors have signed as coauthors. If you wish to refer to this review on AdS/CFT integrability as a whole, we suggest that you cite (only) the introductory chapter:

N. Beisert et al.,  
*“Review of AdS/CFT Integrability: An Overview”*,  
 Lett. Math. Phys. 99, 3 (2012), arXiv:1012.3982.

If your work refers to a particular topic of the review, we encourage you to cite the corresponding specialised chapter(s) (instead/in addition), e.g.

## Chapter 0: An Overview

J. A. Minahan,

*“Review of AdS/CFT Integrability, Chapter I.1: Spin Chains in  $\mathcal{N} = 4$  SYM”*,  
Lett. Math. Phys. 99, 33 (2012), arXiv:1012.3983.

Finally, I would like to thank my coauthors for their collaboration on this project. In particular, I am grateful to Pedro Vieira who set up a website for internal discussions which facilitated the coordination greatly: Drafts and outlines of the chapters were uploaded to this forum. Here, the contributors to the collection gave helpful comments and suggestions on the other chapters. It is fair to say that the forum improved the quality and completeness of the articles and how they fit together before they first appeared in public. Also managing the final production stage would not have been nearly as efficient without it. Thanks for all your help and prompt availability during the last week!

*Niklas Beisert*      Potsdam, December 2010

## Introduction

An old dream of Quantum Field Theory (QFT) is to derive a quantitative description of the mass spectrum of hadronic particles and their excitations. Ideally, one would be able to express the masses of particles such as protons and neutrons as functions of the parameters of the theory

$$m_p = f_1(\alpha_s, \alpha, \mu_{\text{reg}}, \dots), \quad m_n = f_2(\alpha_s, \alpha, \mu_{\text{reg}}, \dots), \quad \dots$$

They might be combinations of elementary functions, solutions to differential or integral equations or something that can be evaluated effortlessly on a present-day computer. For the energy levels of the hydrogen atom analogous functions are known and they work to a high accuracy. However, it has become clear that an elementary analytical understanding of the hadron spectrum will remain a dream. There are many reasons why this is more than can be expected; just to mention a few: At low energies, the coupling constant  $\alpha_s$  is too large for meaningful approximations. In particular, non-perturbative contributions dominate such that the standard loop expansion simply does not apply. Self-interactions of the chromodynamic field lead to a non-linear and highly complex problem. Clearly, confinement obscures the nature of fundamental particles in Quantum Chromodynamics (QCD) at low energies. Of course there are non-perturbative methods to arrive at reasonable approximations for the spectrum, but these are typically based on effective field theory or elaborate numerical simulations instead of elementary analytical QCD.

**Spectrum of Scaling Dimensions.** We shall use the above hadronic spectrum as an analog to explain the progress in applying methods of integrability to the spectrum of planar  $\mathcal{N} = 4$  super Yang–Mills (SYM) theory.<sup>1</sup> The analogy does not go all the way, certainly not at a technical level, but it is still useful for a qualitative understanding of the achievements.

First of all,  $\mathcal{N} = 4$  SYM is a cousin of QCD and of the Standard Model of particle physics. It is based on the same types of fundamental particles and interactions — it is a renormalisable gauge field theory on four-dimensional Minkowski space — but the details of the models are different. Importantly,  $\mathcal{N} = 4$  SYM has a much richer set of symmetries: supersymmetry and conformal symmetry. In particular, the latter implies that there are no massive particles whose spectrum we might wish to compute. Nevertheless, composite particles and their mass spectrum have an analogue in conformal field theories: These are called *local operators*. They are composed from the fundamental fields, all residing at a common point in spacetime. As in QCD, the colour charges are balanced out making the composites gauge-invariant objects. Last but not least, there is a characteristic quantity to replace the mass, the so-called *scaling dimension*. Classically, it equals the sum of the constituent dimensions, and, like the mass, it does receive quantum corrections (the so-called *anomalous dimensions*) from interactions between the constituents.

---

<sup>1</sup>Please note that, here and below, references to the original literature can be found in the chapters of this review collection where the underlying models are introduced.

In the planar  $\mathcal{N} = 4$  SYM model and for scaling dimensions of local operators the particle physicist's dream is coming true. We know how to express the scaling dimension  $D_O$  of some local operator  $O$  as a function of the coupling constant  $\lambda$

$$D_O = f(\lambda).$$

In general this function is given as the solution of a set of integral equations.<sup>2</sup> What is more, in particular cases the equations have been solved numerically for a wide range of  $\lambda$ 's! These equations follow from the so-called Thermodynamic Bethe Ansatz (TBA) or related techniques (Y-system). In a certain limit, the equations simplify to a set of algebraic equations, the so-called asymptotic Bethe equations. It is also becoming clear that not only the spectrum, but many other observables can be determined in this way. Thus it appears that planar  $\mathcal{N} = 4$  SYM can be *solved* exactly.

**Integrability.** With the new methods at hand we can now compute observables which were previously inaccessible by all practical means. By studying the observables and the solution, we hope to get novel insights, not only into this particular model, but also into quantum gauge field theory in general. What is it that makes planar  $\mathcal{N} = 4$  SYM calculable and other models not? Is its behaviour generic or very special? Can we for instance use the solution as a starting point or first approximation for other models? On the one hand one may view  $\mathcal{N} = 4$  SYM as a very special QFT. On the other hand, any other four-dimensional gauge theory can be viewed as  $\mathcal{N} = 4$  SYM with some particles and interactions added or removed: For instance, several quantities show a universal behaviour throughout the class of four-dimensional gauge theories (e.g. highest “transcendentality” part, tree-level gluon scattering). Moreover this behaviour is dictated by  $\mathcal{N} = 4$  SYM acting as a representative model. Thus, indeed, selected results obtained in  $\mathcal{N} = 4$  SYM can be carried over to general gauge theories. Nevertheless it is obvious that we cannot make direct predictions along these lines for most observables, such as the hadron spectrum.

The miracle which leads to the solution of planar  $\mathcal{N} = 4$  SYM described above is generally called *integrability*. Integrability is a phenomenon which is typically confined to two-dimensional models (of Euclidean or Minkowski signature). Oddly, here it helps in solving a four-dimensional QFT.

**AdS/CFT Correspondence.** A more intuitive understanding of why there is integrability comes from the *AdS/CFT correspondence* [1], see also the reviews [2] and [3]. The latter is a duality relation between certain pairs of models. One partner is a conformal field theory, i.e. a QFT with exact conformal spacetime symmetry. The other partner is a string theory where the strings propagate on a background which contains an Anti-de-Sitter spacetime (AdS) as a factor. The boundary of an  $AdS_{d+1}$  spacetime is a conformally flat  $d$ -dimensional spacetime on which the CFT is formulated. The AdS/CFT duality relates the string partition function with sources  $\phi$  for string vertex

---

<sup>2</sup>As a matter of fact, the system of equations is not yet in a form which enables easy evaluation. E.g. there are infinitely many equations for infinitely many quantities. It is however common belief that one can, as in similar cases, reduce the system to a finite set of Non-Linear Integral Equations (NLIE).

operators fixed to value  $J$  at the boundary of  $AdS_{d+1}$  to the  $CFT_d$  partition function with sources  $J$  for local operators

$$Z_{\text{str}}[\phi|_{\partial AdS} = J] = Z_{\text{CFT}}[J].$$

More colloquially: For every string observable at the boundary of  $AdS_{d+1}$  there is a corresponding observable in the  $CFT_d$  (and vice versa) whose values are expected to match. This is a remarkable statement because it relates two rather different types of models on spacetimes of different dimensionalities. From it we gain novel insights into one model through established results from the other model. For example, we can hope to learn about the long-standing problem of quantum gravity (gravity being a fundamental part of every string theory) through studying a more conventional QFT. However, this transfer of results requires a leap of faith as long as the duality lacks a formal proof.

Most attempts at testing the predictions of the AdS/CFT duality have focused on its most symmetric setting: The CFT partner is the gauge theory featured above,  $\mathcal{N} = 4$  SYM. The string partner is IIB superstring theory on the  $AdS_5 \times S^5$  background. This pair is an ideal testing ground because the large amount of supersymmetry leads to simplifications and even allows for exact statements about both models. In this context, we can also understand the miraculous appearance of integrability in planar  $\mathcal{N} = 4$  SYM better: By means of the AdS/CFT duality it translates to integrability of the string worldsheet model. The latter is a two-dimensional non-linear sigma model on a symmetric coset space for which integrability is a common phenomenon. Consequently, integrability has become an important tool to perform exact calculations in both models. Full agreement between both sides of the duality has been observed in all considered cases. Therefore, integrability has added substantially to the credibility of the AdS/CFT correspondence.

**String/Gauge Duality.** Another important aspect of the AdS/CFT duality is that in many cases it relates a string theory to a gauge theory. In fact, the insight regarding the similarities between these two types of models is as old as string theory: It is well-known that the hadron spectrum organises into so-called Regge trajectories. These represent an approximate linear relationship with universal slope between the mass squared of hadronic resonances and their spin. This is precisely what a string theory on flat space predicts, hence string theory was for some time considered a candidate model of the strong interactions. For various reasons this idea did not work out. Instead, it was found that a gauge theory, namely QCD, provides an accurate and self-consistent description of the strong interactions. Altogether it implies that string theory, under some conditions, can be a useful approximation to gauge theory phenomena. A manifestation of stringy behaviour in gauge theory is the occurrence of flux tubes of the chromodynamic field. Flux tubes form between two quarks when they are pulled apart. To some approximation they can be viewed as one-dimensional objects with constant tension, i.e. strings. The AdS/CFT correspondence goes even further. It proposes that in some cases a gauge theory is exactly dual to a string theory. By studying those cases, we hope to gain more insights into string/gauge duality in general, perhaps even for QCD.

A milestone of string/gauge duality was the discovery of the planar limit [4], see Fig. 1. This is a limit for models with gauge group  $SU(N_c)$ ,  $SO(N_c)$  or  $Sp(N_c)$ . It



**Parameter Space.** Let us now discuss the progress due to integrability based on a map of the parameter space of our gauge and string theory, see Fig. 2. Typically there are two relevant parameters for a gauge theory, the 't Hooft coupling  $\lambda = g_{\text{YM}}^2 N_c$  and the number of colours  $N_c$  as a measure of the rank of the gauge group. In a string theory we have the effective string tension  $T = R^2/2\pi\alpha'$  (composed from the inverse string tension  $\alpha'$  and the  $AdS_5/S^5$  radius  $R$ ) and the string coupling  $g_{\text{str}}$ . The AdS/CFT correspondence relates them as follows

$$\lambda = 4\pi^2 T^2, \quad \frac{1}{N_c} = \frac{g_{\text{str}}}{4\pi^2 T^2}.$$

The region of parameter space where  $\lambda$  is small is generally called the *weak coupling* regime. This is where perturbative gauge theory in terms of Feynman diagrams provides reliable results. By adding more loop orders to the series expansion one can obtain more accurate estimates towards the centre of the parameter space (up to non-perturbative effects). Unfortunately, conventional methods in combination with computer algebra only allow evaluating the first few coefficients of the series in practice. Thus we cannot probe the parameter space far away from the weak coupling regime. However,  $N_c$  can be finite in practice, therefore the regime of perturbative gauge theory extends along the line  $\lambda = 0$ .

The region around the point  $\lambda = \infty$ ,  $g_{\text{str}} = 0$  is where perturbative string theory applies. Here, strings are weakly coupled, but the region is nevertheless called the *strong coupling* regime referring to the gauge theory parameter  $\lambda$ . String theory provides a double expansion around this point. The accuracy towards finite  $\lambda$  is increased by adding quantum corrections to the worldsheet sigma model (curvature expansion, “worldsheet loops”). Finite- $g_{\text{str}}$  corrections correspond to adding handles to the string worldsheet (genus expansion, “string loops”). As before, both expansions are far from trivial, and typically only the first few coefficients can be computed in practice. Consequently, series expansions do not give reliable approximations far away from the point  $\lambda = \infty$ ,  $g_{\text{str}} = 0$ .

Here we can see the weak/strong dilemma of the AdS/CFT duality, see also Fig. 3: The perturbative regimes of the two models do not overlap. On the one hand AdS/CFT provides novel insights into both models. On the other hand, we cannot really be sure of them until there is a general proof of the duality. Conventional perturbative expansions are of limited use in verifying, and tests had been possible only for a few special observables (cf. [5] for example).

This is where integrability comes to help. As explained above, it provides novel computational means in *planar*  $\mathcal{N} = 4$  SYM at arbitrary coupling  $\lambda$ . The AdS/CFT correspondence relates this regime to free ( $g_{\text{str}} = 0$ ) IIB superstrings on  $AdS_5 \times S^5$  at arbitrary tension  $T$ . It connects the regime of perturbative gauge theory with the regime of perturbative string theory. Integrability predicts the spectrum of planar scaling dimensions for local operators as a function of  $\lambda$ , cf. Fig. 3. In string theory this is dual to the energy spectrum of free string states (strings which neither break apart nor join with others). We find that integrability makes coincident predictions for both models. At weak coupling one can compare to results obtained by conventional perturbative means in gauge theory, and one finds agreement. Analogous agreement with perturbative strings

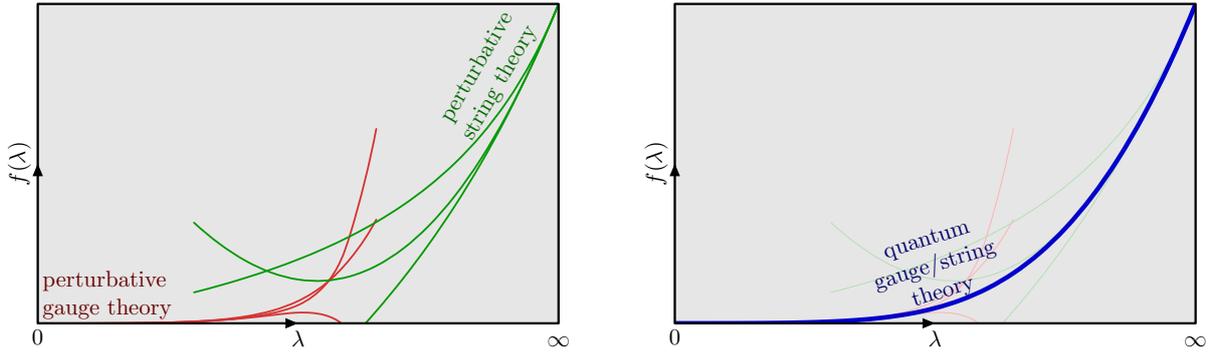

**Figure 3:** Weak coupling (3, 5, 7 loops) and strong coupling (0, 1, 2 loops) expansions (left) and numerically exact evaluation (right) of some interpolating function  $f(\lambda)$ .

is found at strong coupling. And for intermediate coupling the spectrum apparently interpolates smoothly between the two perturbative regimes.

Methods of integrability provide us with reliable data over the complete range of couplings. We can investigate in practice a gauge theory at strong coupling. There it behaves like a weakly coupled string theory. Likewise a string theory on a highly curved background (equivalent to low tension) behaves like a weakly coupled gauge theory. At intermediate coupling, the results are reminiscent of neither model or of both; this is merely a matter of taste and depends crucially on whether one's intuition is based on classical or quantum physics. In any case, integrability can give us valuable insights into a truly quantum gauge and/or string theory at intermediate coupling strength.

**Solving a Theory.** In conclusion, we claim that integrability solves the planar sector of a particular pair of gauge and string theories. We should be clear about the actual meaning of this statement: It certainly does not mean that the spectrum is given by a simple formula as in the case of a harmonic oscillator, the (idealised) hydrogen atom or strings in flat space (essentially a collection of harmonic oscillators)<sup>3</sup>

$$E_{\text{HO}} = \omega(n + \frac{1}{2}), \quad E_{\text{hyd}} = -\frac{m_e \alpha^2}{n^2}, \quad m_{\text{flat}}^2 = m_0^2 + \frac{1}{\alpha'} \sum_{k=-\infty}^{\infty} n_k |k|.$$

It would be too much to hope for such a simplistic behaviour in our models: For instance, the one-loop corrections to scaling dimensions are typically algebraic numbers. Therefore the best we can expect is to find a system of algebraic equations whose solutions determine the spectrum. This is what methods of integrability provide more or less directly. Integrability vastly reduces the complexity of the spectral problem by bypassing almost all steps of standard QFT methods: There we first need to compute all the entries of the matrix of scaling dimensions. Each entry requires a full-fledged computation of higher loop Feynman graphs involving sophisticated combinatorics and demanding loop integrals. The naively evaluated matrix contains infinities calling for proper regularisation

<sup>3</sup>In fact, these systems are also integrable, but of an even simpler kind.

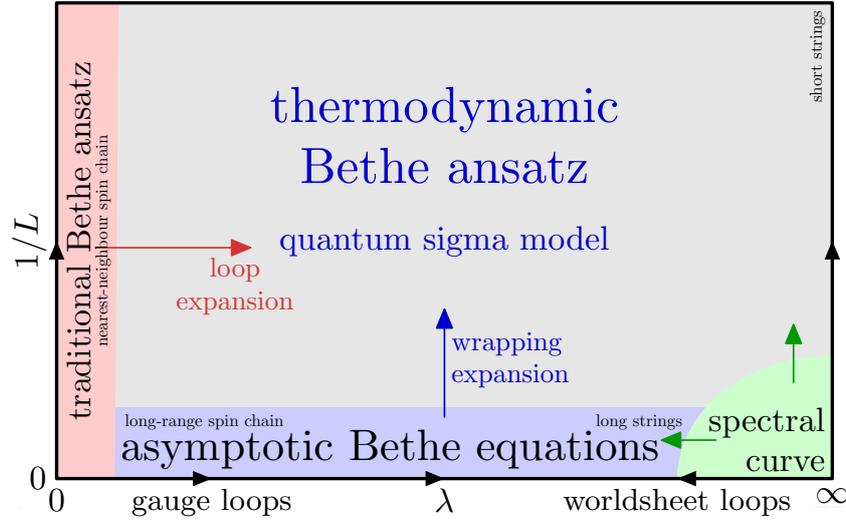

**Figure 4:** Phase diagram of local operators in planar  $\mathcal{N} = 4$  SYM mapped with respect to coupling  $\lambda$  vs. “size”  $L$ . Also indicated are the integrability methods that describe the spectrum accurately.

and renormalisation. The final step consists in diagonalising this (potentially large) matrix. This is why scaling dimensions are solutions of algebraic equations. In comparison, the integrable approach directly predicts the algebraic equations determining the scaling dimension  $D$

$$f(D, \lambda) = 0.$$

This is what we call a *solution* of the spectral problem.

A crucial benefit of integrability is that the spectral equations include the coupling constant  $\lambda$  in functional form. Whereas standard methods produce an expansion whose higher loop coefficients are exponentially or even factorially hard to compute, here we can directly work at intermediate coupling strength.

What is more, integrability gives us easy access to composite objects with a large number of constituents. Generally, there is an enormous phase space for such objects growing exponentially with their size. Standard methods would require computing the complete matrix of scaling dimensions and then filter out the desired eigenvalue. Clearly this procedure is prohibitive for large sizes. Conversely, the integrable approach is formulated in terms of physically meaningful quantities. This allows us to assume a certain coherent behaviour for the constituents of the object we are interested in, and then approach the *thermodynamic limit*. Consequently we obtain a set of equations for the energy of just this object. Moreover, the thermodynamic limit is typically much simpler than the finite-size equations. The size of the object can be viewed as a quantum parameter, where infinite vs. finite size corresponds to classical vs. quantum physics. In fact, in many cases it does map to classical vs. quantum strings! In Fig. 4 we present a phase space for local operators in planar  $\mathcal{N} = 4$  SYM. On it we indicate the respective integrability methods to be described in detail in the overview section and in the chapters.

As already mentioned, a strength of the integrable system approach is that objects

are often represented through their physical parameters. This is not just an appealing feature, but also a reason for the efficiency: The framework of quantum mechanics and QFT is heavily based on equivalence classes. Explicit calculations usually work with representatives. Choosing a particular representative in a class introduces further auxiliary degrees of freedom into the system. These degrees of freedom are carried along the intermediate steps of the calculation, and it is reasonable to expect them to be a source of added difficulty because there is no physical principle to constrain their contributions. In particular, they are the habitat of the notorious infinities of QFT. At the end of the day, all of their contributions miraculously<sup>4</sup> vanish into thin air. Hence a substantial amount of efforts typically go into calculating contributions which one is actually not interested in. Conversely, one may view integrable methods as working directly in terms of the physical equivalence classes instead of their representatives. The observables are then computed without intermediate steps or complications. The fact that such a shortcut exists for some models is a true miracle; it is called *integrability*.

So far we have discussed solving the spectrum of our planar model(s). A large amount of evidence has now accumulated that this is indeed possible, and, more importantly, we understand how to do it in practice. Solving the theory, however, requires much more; we should be able to compute *all of its observables*. For a gauge theory they include not only the spectrum of scaling dimensions, but also correlation functions, scattering amplitudes, expectation values of Wilson loops, surface operators and other extended objects, as well as combinations of these (loops with insertions, form factors, . . .), if not more. For several of these, in particular for scattering amplitudes, it is becoming clear that integrability provides tools to substantially simplify their computation. Hence it is plausible to expect that the planar limit can be solved.

Can we also solve the models away from the planar limit? There are many indications that integrability breaks down for finite number of colours  $N_c$ . Nevertheless, this alone does not imply that we should become dispirited. Integrability may still prove useful, not in the sense of an exact solution, but as a means to perform an expansion in terms of genus, i.e. in powers of  $1/N_c \sim g_{\text{str}}$ . This might give us a new handle to approach the centre of parameter space in Fig. 2 coming from below. The centre will, with all due optimism, most likely remain a tough nut to crack.

In conclusion, methods of integrability have already brought and will continue to bring novel insights into the gauge and string models. Having many concrete results at hand helps in particular to understand their duality better. In particular we can confirm and complete the AdS/CFT *dictionary* which relates objects and observables between the two models.

**Integrability as a Symmetry.** Above we have argued that the success of integrability is based on the strict reduction to the physical degrees of freedom. Another important point of view is that integrability is a hidden symmetry. Symmetries have always been a key towards a better understanding in particle physics and QFT. Here the hidden symmetry is in fact so powerful that it not only relates selected quantities to others, but,

---

<sup>4</sup>Of course, the miracle is consistency of the model paired with failing to make mistakes in the calculation (often used as a convenient cross check of the result).

in some sense, anything to everything else. The extended symmetry thus predicts the outcome of every measurement, at least in principle. Conventionally one would expect the resulting model to be trivial, just like a harmonic oscillator, but there are important interesting and highly non-trivial cases.

Integrability finds a natural mathematical implementation in the field of *quantum algebra*. More concretely, the type of quantum integrable system that we encounter is usually formulated in terms of deformed universal enveloping algebras of affine Lie algebras. The theory of such quasi-triangular Hopf algebras is in general highly developed. It provides the objects and their relations for the solution of the physical system. Curiously, our gauge/string theory integrable model appears to be based on some unconventional or exceptional superalgebra which largely remains to be understood. It is not even clear whether quasi-triangular Hopf algebras are a sufficient framework for a complete mathematical implementation of the system.

**Relations to Other Subjects.** An aspect which makes the topic of this review a particularly attractive one to work on is its relation to diverse subjects of theoretical physics and mathematics. Let us collect a few here, including those mentioned above, together with references to the chapters of this review where the relations are discussed in more detail:

- Most obviously, the topic of the review itself belongs to *four-dimensional QFT*, more specifically, *gauge theory* and/or *CFT*, but also to *string theory on curved backgrounds*.
- Recalling the discussion from a few lines above, the mathematical framework for the kind of integrable models that we encounter is *quantum algebra*, see Chapter VI.2.
- As mentioned earlier, string theory always contains a self-consistent formulation of quantum gravity. By gaining a deeper understanding of string theory models, we hope to learn more about *quantum gravity* as such. Furthermore, by means of the string-related Kawai–Lewellen–Tye [6] and Bern–Carrasco–Johansson relations [7], there is a connection between scattering amplitudes in  $\mathcal{N} = 4$  SYM and  $\mathcal{N} = 8$  *supergravity*, which stands a chance of being free of perturbative divergencies.<sup>5</sup> These aspects are not part of the review. In fact, it would be highly desirable to explore the use of integrability results in this context.
- Prior to the discoveries related to the AdS/CFT correspondence, integrability in four-dimensional gauge theories was already observed in the context of *high-energy scattering* and the BFKL equations, and for *deep inelastic scattering* and the DGLAP equations, see Chapter IV.4 and [8]. Note that the *twist states* discussed in Chapters III.4 play a prominent role in deep inelastic scattering.
- There are also rather distinct applications of integrability in supersymmetric gauge theories: There is the famous Seiberg–Witten solution [9] for the BPS masses in  $D = 4$ ,  $\mathcal{N} = 2$  gauge theories. Furthermore, supersymmetric vacua in  $D = 2$ ,

---

<sup>5</sup>One should point out that these relations are essentially non-planar.

$\mathcal{N} = 4$  gauge theories with matter can be described by Bethe ansätze [10]. It remains to be seen whether there are connections to the subject of the present review.

- There are further links to general *four-dimensional gauge theories*: On a qualitative level we might hope to learn about QCD strings from novel results in the AdS/CFT correspondence at finite coupling. On a practical level, the leading-order results in  $\mathcal{N} = 4$  SYM can be carried over to general gauge theories essentially because  $\mathcal{N} = 4$  SYM contains all types of particles and interactions allowed in a renormalisable QFT. Chapter IV.4 is most closely related to this topic.
- Along the same lines, the BFKL dynamics in leading logarithmic approximation is universal to all four-dimensional gauge theories. The analytic expressions derived in  $\mathcal{N} = 4$  SYM may allow us to clarify the nature of the most interesting Regge singularity, *the pomeron* (see [11]), which is the most interesting object for perturbative QCD and for its applications to particle collider physics.<sup>6</sup>
- A certain class of composite states, but also loop integrals in QFT, often involve generalised harmonic sums, generalised polylogarithms and multiple zeta values. The exploration of such *special functions* is an active topic of mathematics. See Chapters I.2, III.4 and V.2.
- Local operators of the gauge theory are equivalent to states of a quantum spin chain. Spin chain models come to use in connection with *magnetic properties* in *solid state physics*. Also in gauge theory, ferromagnetic and anti-ferromagnetic states play an important role, see Chapters I.1 and III.4.
- More elaborate spin chains — such as the one-dimensional Hubbard model (cf. [12]) — are considered in connection to *electron transport*. Curiously, this rather exceptional Hubbard chain makes an appearance in the gauge theory context, in at least two distinct ways, see Chapters I.3 and III.2.
- And there are many more avenues left to be explored.

---

<sup>6</sup>We thank L. Lipatov for pointing out this application.

## Outline

The review collection consists of the above introduction and 23 chapters grouped into 6 major subjects. Each chapter reviews a particular topic in a self-contained manner. The following overview gives a brief summary of each part and each chapter, and is meant to tie the whole collection together. It can be understood as an extensive table of contents.

Where possible, we have put the chapters into a natural and meaningful order with regards to content. A chapter builds upon insights and results presented in the earlier chapters and begins roughly where the previous one ended. In many cases this reflects the historical developments, but we have tried to pull loops straight. Our aim was to prepare a pedagogical and generally accessible introduction to the subject of AdS/CFT integrability rather than a historically accurate account.

While the topics were fixed, the design and presentation of each chapter was largely the responsibility of its authors. The only guideline was to discuss an instructive example in detail while presenting the majority of results more briefly. Furthermore, the chapters give a guide to the literature relevant to the topic where more details can be found. Open problems are also discussed in the chapters. Note that we did not enforce uniform conventions for naming, use of **alphabets**, normalisations, and so on. This merely reflects a reality of the literature. However, each chapter is meant to be self-consistent.

Before we begin with the overview, we would like to point out existing reviews on AdS/CFT integrability and related subjects which cover specific aspects in more detail. We can recommend several reviews dedicated to the subject [13]. Also a number of PhD theses are available which at least contain a general review as the introduction [14]. It is also worthwhile to read some of the very brief accounts of the subject in the form of news items [15]. Last but not least, we would like to refer the reader to prefaces of special issues dedicated to AdS/CFT integrability [16] and closely related subjects [17].

## Table of Contents

page numbers refer to Lett. Math. Phys. 99 (2012), numbers 1210.0392–0405 are arxiv.org identifiers.

### I $\mathcal{N} = 4$ Super Yang–Mills Theory

- I.1 J. A. Minahan, “*Spin Chains in  $\mathcal{N} = 4$  SYM*”, pp. 33, 1012.3983.
- I.2 C. Sieg, “*The spectrum from perturbative gauge theory*”, pp. 59, 1012.3984.
- I.3 A. Rej, “*Long-range spin chains*”, pp. 85, 1012.3985.

### II IIB Superstrings on $AdS_5 \times S^5$

- II.1 A. Tseytlin, “*Classical  $AdS_5 \times S^5$  string solutions*”, pp. 103, 1012.3986.
- II.2 T. McLoughlin, “*Quantum Strings in  $AdS_5 \times S^5$* ”, pp. 127, arxiv:1012.3987.
- II.3 M. Magro, “*Sigma Model, Gauge Fixing*”, pp. 149, 1012.3988.
- II.4 S. Schäfer-Nameki, “*The Spectral Curve*”, pp. 169, 1012.3989.

### III Solving the AdS/CFT Spectrum

- III.1 M. Staudacher, “*Bethe Ansätze and the R-Matrix Formalism*”, pp. 191, 1012.3990.
- III.2 C. Ahn and R. I. Nepomechie, “*Exact world-sheet S-matrix*”, pp. 209, 1012.3991.
- III.3 P. Vieira and D. Volin, “*The dressing factor*”, pp. 231, 1012.3992.
- III.4 L. Freyhult, “*Twist states and the cusp anomalous dimension*”, pp. 255, 1012.3993.
- III.5 R. Janik, “*Lüscher corrections*”, pp. 277, 1012.3994.
- III.6 Z. Bajnok, “*Thermodynamic Bethe Ansatz*”, pp. 299, 1012.3995.
- III.7 V. Kazakov and N. Gromov, “*Hirota Dynamics for Quantum Integrability*”, pp. 321, 1012.3996.

### IV Further Applications of Integrability

- IV.1 C. Kristjansen, “*Aspects of Non-planarity*”, pp. 349, 1012.3997.
- IV.2 K. Zoubos, “*Deformations, Orbifolds and Open Boundaries*”, pp. 375, 1012.3998.
- IV.3 T. Klose, “ *$\mathcal{N} = 6$  Chern-Simons and Strings on  $AdS_4 \times CP^3$* ”, pp. 401, 1012.3999.
- IV.4 G. Korchemsky, “*Integrability in QCD and  $\mathcal{N} < 4$  SYM*”, pp. 425, 1012.4000.

### V Scattering Amplitudes

- V.1 R. Roiban, “*Scattering Amplitudes – a Brief Introduction*”, pp. 455, 1012.4001.
- V.2 J. M. Drummond, “*Dual Superconformal Symmetry*”, pp. 481, 1012.4002.
- V.3 L. F. Alday, “*Scattering Amplitudes at Strong Coupling*”, pp. 507, 1012.4003.

### VI Algebraic Aspects of Integrability

- VI.1 N. Beisert, “*Superconformal Algebra*”, pp. 529, 1012.4004.
- VI.2 A. Torrielli, “*Yangian Algebra*”, pp. 547, 1012.4005.

## Overview

The chapters are grouped into six parts representing the major topics and activities of this subject, see Fig. 5. In the first two Parts I and II we start by outlining the perturbative gauge and string theory setup. Here we focus on down-to-earth quantum field theory calculations which yield the solid foundation in spectral data of local operators. In the following Part III we review the construction of the spectrum by integrable methods. More than merely reproducing the previously obtained data, this goes far beyond what could possibly be computed by conventional methods: It can apparently predict the exact spectrum. The next Part IV summarises applications of these methods to similar problems, beyond the spectrum, beyond planarity, beyond  $\mathcal{N} = 4$  SYM or strings on  $AdS_5 \times S^5$ . Among these avenues is the application of integrability to scattering amplitudes; as this topic has grown into a larger subject we shall devote Part V to it. The final Part VI reviews classical and quantum algebraic aspects of the models and of integrability.

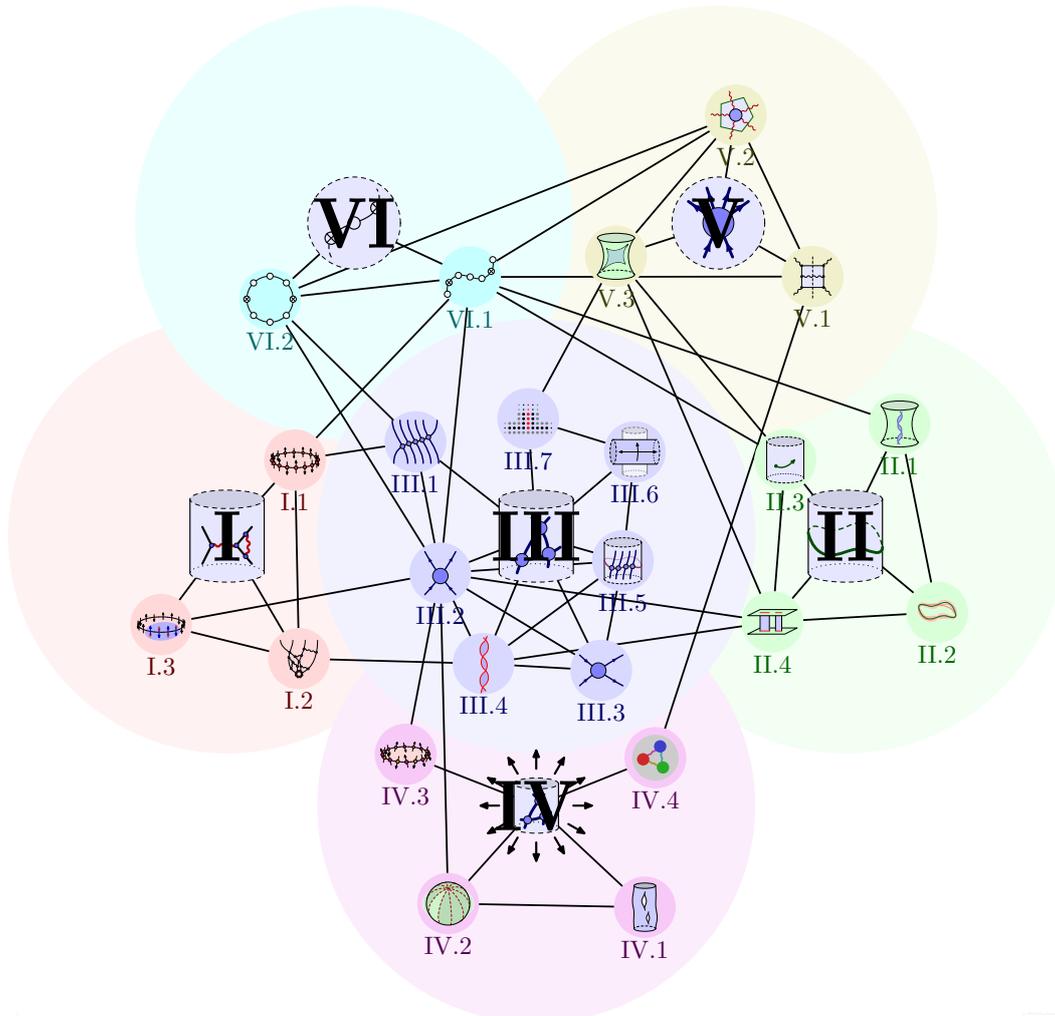

**Figure 5:** Suggested order of study.

# I $\mathcal{N} = 4$ Super Yang–Mills Theory

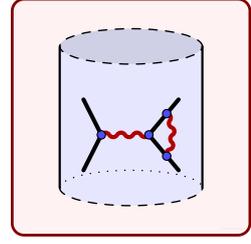

This part deals with the maximally supersymmetric Yang–Mills ( $\mathcal{N} = 4$  SYM) theory in four spacetime dimensions. This model is a straightforward quantum field theory. It uses the same types of particles and interactions that come to play in the Standard Model of particle physics. However, the particle spectrum and the interactions are delicately balanced granting the model a host of unusual and unexpected features. The best-known of these is exact (super)conformal symmetry at the quantum level. A far less apparent feature is what this review collection is all about: integrability.

In this part we focus on the perturbative field theory, typically expressed through Feynman diagrams. The calculations are honest and reliable but they become tough as soon as one goes to higher loop orders. Integrability will only be discussed as far as it directly concerns the gauge theory setup, i.e. in the sense of conserved operators acting on a spin chain. The full power of integrability will show up only in Part III.

## I.1 Spin Chains in $\mathcal{N} = 4$ SYM

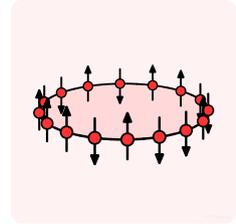

Chapter I.1 introduces the gauge theory, its local operators, and outlines how to compute the spectrum of their planar one-loop anomalous dimensions. It is explained how to map one-to-one local operators to states of a certain quantum spin chain. The operator which measures the planar, one-loop anomalous dimensions corresponds to the spin chain Hamiltonian in this picture. Importantly, this Hamiltonian is of the integrable kind, and the planar model can be viewed as a generalisation of the Heisenberg spin chain. This implies that its spectrum is solved efficiently by the corresponding Bethe ansatz. E.g. a set of one-loop planar anomalous dimensions  $\delta D$  is encoded in the solutions of the following set of Bethe equations for the variables  $u_k \in \mathbb{C}$  ( $k = 1, \dots, M$ )

$$\left( \frac{u_k + \frac{i}{2}}{u_k - \frac{i}{2}} \right)^L = \prod_{\substack{j=1 \\ j \neq k}}^M \frac{u_k - u_j + i}{u_k - u_j - i}, \quad 1 = \prod_{j=1}^M \frac{u_j + \frac{i}{2}}{u_j - \frac{i}{2}}, \quad \delta D = \frac{\lambda}{8\pi^2} \sum_{j=1}^M \frac{1}{u_j^2 + \frac{1}{4}}.$$

Finally the Chapter presents applications of the Bethe ansatz to sample problems.

## I.2 The spectrum from perturbative gauge theory

The following Chapter I.2 reviews the computation of the spectrum of anomalous dimensions at higher loops in perturbative gauge theory. The calculation in terms of Feynman diagrams is firmly established, but just a handful orders takes you to the limit of what is generally possible. Computer algebra and superspace techniques push the limit by a few orders.

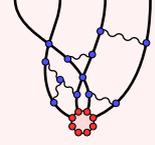

In our case the results provide a valuable set of irrefutable data which the integrable model approach must be able to reproduce to show its viability. This comprises not only explicit energy eigenvalues, but also crucial data for the integrable system, such as the magnon dispersion relation and scattering matrix. Importantly, also the leading finite-size terms are accessible in this approach, e.g. the four-loop anomalous dimension to the simplest non-trivial local operator reads (cf. the above Bethe equation with  $L = 4, M = 2$ )

$$\delta D = \frac{3\lambda}{4\pi^2} - \frac{3\lambda^2}{16\pi^4} + \frac{21\lambda^3}{256\pi^6} - \frac{(78 - 18\zeta(3) + 45\zeta(5))\lambda^4}{2048\pi^8} + \dots$$

## I.3 Long-range spin chains

The final Chapter I.3 of this part reviews spin chain Hamiltonians originating in planar gauge theory at higher loops. The one-loop Hamiltonian describes interactions between two neighbouring spins. At higher loops the Hamiltonian is deformed by interactions between several neighbouring spins, e.g.

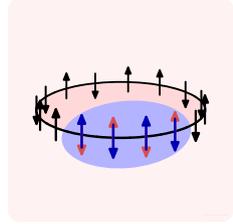

$$H = \sum_{j=1}^L \left( \frac{\lambda}{8\pi^2} (1 - P_{j,j+1}) + \frac{\lambda^2}{128\pi^4} (-3 + 4P_{j,j+1} - P_{j,j+2}) + \dots \right).$$

Moreover, the Hamiltonian can dynamically add or remove spin sites! While integrable nearest-neighbour Hamiltonians have been studied in detail for a long time, a better general understanding of long-range deformations was developed only recently. Curiously, several well-known integrable spin chain models make an appearance in this context, in particular, the Haldane–Shastry, Inozemtsev and Hubbard models.

## II IIB Superstrings on $AdS_5 \times S^5$

This part concerns IIB string theory on the maximally supersymmetric  $AdS_5 \times S^5$  background. The string worldsheet model is a two-dimensional UV-finite quantum field theory. It is of the non-linear sigma model kind with target space  $AdS_5 \times S^5$  and further possesses worldsheet diffeomorphisms. Also this model has a number of exceptional features, such as kappa symmetry, which make it a viable string theory on a stable background. Somewhat less surprising than in gauge theory, this model is also integrable, a property shared by many two-dimensional sigma models on coset spaces.

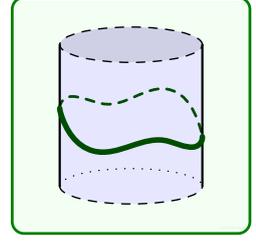

We outline how to extract spectral data from classical string solutions with quantum corrections. There are many complications, such as non-linearity of the classical equations of motion, lack of manifest supersymmetry and presence of constraints. Again, integrability will help tremendously; here we focus on string-specific aspects, and leave the more general applications to Part III.

### II.1 Classical $AdS_5 \times S^5$ string solutions

The first Chapter II.1 of this part introduces the Green–Schwarz string on the curved spacetime  $AdS_5 \times S^5$ . For the classical spectrum only the bosonic fields are relevant. To find exact solutions of the non-linear equations of motions, one typically makes an ansatz for the shape of the string. Taking inspiration from spinning strings in flat space, one can for instance assume a geodesic rod spinning around some orthogonal axes. The equations of motion together with the Virasoro constraints dictate the local evolution, while boundary conditions quantise the string modes. Next, the target space isometries give rise to conserved charges, such as angular momenta and energy. These can be expressed in terms of the parameters of the string solution. E.g., a particular class of spinning strings on  $AdS_3 \times S^1 \subset AdS_5 \times S^5$  obeys the following relation ( $K, E$  are elliptic integrals)

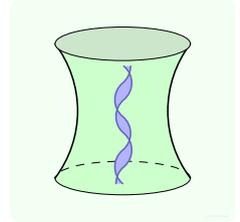

$$\frac{S^2}{(K(m) - E(m))^2} - \frac{J^2}{K(m)^2} = 16n^2T^2(1 - m), \quad \frac{J^2}{K(m)^2} - \frac{E^2}{E(m)^2} = 16n^2T^2m.$$

Such relations can be used to express the energy  $E$  as a function of the angular momenta  $J, S$ , the string modes  $n$  and the string tension  $T$ .<sup>7</sup>

<sup>7</sup>Note that complicated classes of solutions will require further internal parameters in addition to  $m$ .

## II.2 Quantum Strings in $AdS_5 \times S^5$

Chapter II.2 continues with semiclassical quantisation of strings. Here, one distinguishes between point-like and extended strings.

Quantisation around point-like strings is the direct analogue of what is commonly done in flat space. The various modes of the string can be excited in quantised amounts, and the string spectrum takes the form

$$E - J = \sum_{k=1}^M N_k \sqrt{1 + \lambda n_k^2 / J^2} + \dots, \quad \sum_{k=1}^M N_k n_k = 0.$$

The main difference with flat space is that the modes interact, adding non-trivial corrections to the spectrum. These corrections can be computed in terms of a scattering problem on the worldsheet.

Quantisation around extended string solutions is far less trivial: The spectrum of fluctuations now crucially depends on the classical solution. Another effect is that the energy of the classical string receives quantum corrections due to vacuum energies of the string modes.

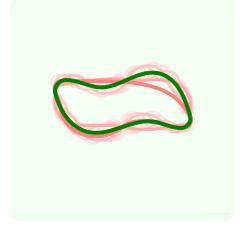

## II.3 Sigma Model, Gauge Fixing

Spheres and anti-de-Sitter spacetimes are symmetric cosets. Chapter II.3 presents the formulation of the string worldsheet as a two-dimensional coset space sigma model of the target space isometry supergroup. In particular, integrability finds a simple formulation in a family of flat connections  $A(z)$  on the worldsheet and its holonomy  $M(z)$  around the closed worldsheet

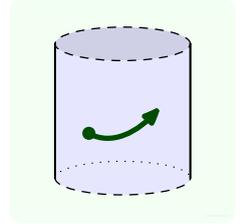

$$dA(z) + A(z) \wedge A(z) = 0, \quad M(z) = \text{P exp} \oint A(z).$$

Series expansion of  $M(z)$  in the spectral parameter  $z$  leads to an infinite tower of charges extending the isometries to an infinite-dimensional algebra.

Proper treatment of symmetries and integrability towards a canonical quantisation requires a Hamiltonian formulation. Here the major complications are the presence of first and second class constraints due to worldsheet diffeomorphisms and kappa symmetry. Finally, one encounters notorious ambiguities in deriving the algebra of conserved charges.

## II.4 The Spectral Curve

In the final Chapter II.4 on strings, the flat connection is applied to the construction of the (semi)classical string spectrum. The eigenvalues  $e^{ip_k(z)}$  of the monodromy  $M(z)$  are integrals of motion. As functions of complex  $z$  they define a spectral curve for each classical solution. Instead of studying explicit classical solutions we can now study abstract spectral curves. Besides containing all the spectral information, they offer a neat physical picture: String modes correspond to handles of the Riemann surface, and each handle has two associated moduli: the mode number  $n_k$  and an amplitude  $\alpha_k$ . They can be extracted easily as periods of the curve

$$\oint_{A_k} dp = 0, \quad \frac{1}{2\pi} \oint_{B_k} dp = n_k, \quad \frac{\sqrt{\lambda}}{4\pi^2 i} \oint_{A_k} \frac{1+z^4}{1-z^4} dp = N_k.$$

Note that quantisation replaces the amplitude by an integer excitation number  $N_k$  thus providing access to the semiclassical spectrum of fluctuation modes.

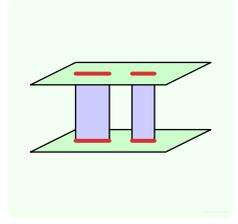

## III Solving the AdS/CFT Spectrum

Armed with some basic knowledge of the relevant structures in gauge and string theory (as well as an unconditional belief in the applicability of integrable structures to this problem) we aim to solve the planar spectrum in this part.

The starting point is that in both models there is a one-dimensional space (spin chain, string) on which some particles (magnons, excitations) can propagate. By virtue of symmetry and integrability one can derive how they scatter, at all couplings and in all directions. Taking periodicity into account properly, one arrives at a complete and exact description of the spectrum. For certain states this program was carried out, and all results are in complete agreement with explicit calculations in perturbative gauge or string theory (as far as they are available). Yet, the results from the integrable system approach go far beyond what is otherwise possible in QFT: They provide a window to finite coupling  $\lambda$ !

There are several proposals of how to formulate these equations — through an algebraic system or through integral equations. However, it is commonly believed that a reasonably simple and generally usable form for such equations has not yet been found (let alone proved).

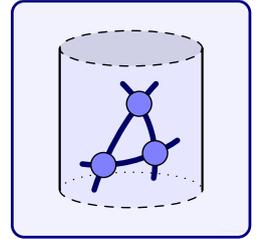

### III.1 Bethe Ansätze and the R-Matrix Formalism

As a warm-up exercise and to gather experience, Chapter III.1 solves one of the oldest quantum mechanical systems — the Heisenberg spin chain. This is done along the lines of Bethe’s original work, using a factorised magnon scattering picture, but also in several variants of the Bethe ansatz. This introduces us to ubiquitous concepts of integrable systems such as R-matrices, transfer matrices and the famous Yang–Baxter equation

$$R_{12}R_{13}R_{23} = R_{23}R_{13}R_{12}.$$

The chapter ends by sketching a promising novel method for constructing the so-called Baxter Q-operators, allowing to surpass the Bethe ansatz technique.

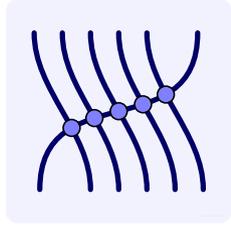

### III.2 Exact world-sheet S-matrix

Even though little is known about gauge or string theory at finite coupling, the magnon scattering pictures and symmetries qualitatively agree for weak and strong coupling. Under the assumption that they remain valid at intermediate couplings, Chapter III.2 describes how to make use of symmetry to determine all the relevant quantities: Both, the magnon dispersion relation

$$e(p) = \sqrt{1 + \frac{\lambda}{\pi^2} \sin^2(\frac{1}{2}p)}$$

and the 16-flavour scattering matrix are almost completely determined through representation theory of an extended  $\mathfrak{psu}(2|2)$  superalgebra. Integrability then ensures factorised scattering, and determines the spectrum on sufficiently long chains or strings through the asymptotic Bethe equations.

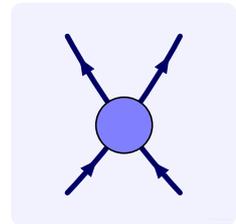

### III.3 The dressing factor

Symmetry alone cannot predict an overall phase factor of the scattering matrix which is nevertheless crucial for the spectrum. Several other desirable properties of factorised scattering systems, such as unitarity, crossing and fusion, constrain its form

$$S_{12}^0 S_{12}^0 = f_{12}.$$

Chapter III.3 presents this crossing equation and its solution – the so-called dressing phase. It has a host of interesting analytic properties relating to the physics of the model under discussion.

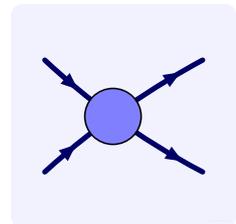

### III.4 Twist states and the cusp anomalous dimension

The asymptotic Bethe equations predict the spectrum up to finite-size corrections. In Chapter III.4 we apply them to the interesting class of twist states. These are ideally suited for testing purposes because a lot of solid spectral data are known from perturbative gauge and string theory. They also have an interesting dependence on their spin  $j$ , in terms of generalised harmonic sums of fixed degree.

Importantly, in the large spin limit, finite-size corrections turn out to be suppressed. The Bethe equations reduce to an integral equation to predict the exact cusp dimension (and generalisations). The latter turns out to interpolate smoothly between weak and strong coupling in full agreement with perturbative data

$$D_{\text{cusp}} = \frac{\lambda}{2\pi^2} - \frac{\lambda^2}{96\pi^2} + \frac{11\lambda^3}{23040\pi^2} + \dots = \frac{\sqrt{\lambda}}{\pi} - \frac{3 \log 2}{\pi} - \frac{\beta(2)}{\pi\sqrt{\lambda}} + \dots$$

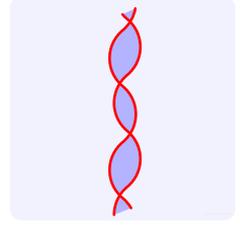

### III.5 Lüscher corrections

For generic states, however, finite-size corrections are required to get agreement with gauge and string theory. Chapter III.5 explains how to apply Lüscher terms to determine these: On a closed worldsheet there are virtual particles propagating in the spatial direction in non-trivial loops around the string. When they interact with physical excitations, they give rise to non-trivial energy shifts ( $q_j$  and  $p_k$  are virtual and real particle momenta, respectively)

$$\delta E = - \sum_j \int \frac{dq_j}{2\pi} e^{-L\tilde{e}_j(q_j)} \text{STr}_j \prod_k S_{jk}(q_j, p_k).$$

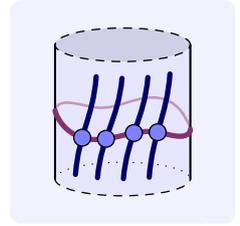

### III.6 Thermodynamic Bethe Ansatz

Although finite-size corrections appear under control, it is clearly desirable to find equations to determine the exact spectrum in one go. Chapter III.6 describes the thermodynamic Bethe ansatz approach based on the following idea: Consider the string worldsheet at finite temperature with Wick rotated time. It has the topology of a torus of radius  $R$  and time period  $L$ . We are primarily interested in the zero temperature limit where time is decompactified. Now the torus partition function can be evaluated in the mirror theory where the periods are exchanged

$$Z(R, L) = \tilde{Z}(L, R).$$

Then, instead of time, we can decompactify the radius. Conveniently, the asymptotic Bethe equations become exact, and eventually predict the finite-size spectrum.

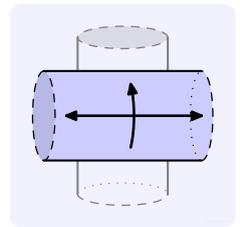

### III.7 Hirota Dynamics for Quantum Integrability

Chapter III.7 presents an equivalent proposal for the finite-size spectrum based on the conserved charges of an integrable model. The latter are typically packaged into transfer matrix eigenvalues  $T(u)$ . These exist in various instances which obey intricate relations, such as the discrete Hirota equation (also known as the Y-system for equivalent quantities  $Y_{a,s}(u)$ )

$$T_{a,s}(u + \frac{i}{2})T_{a,s}(u - \frac{i}{2}) = T_{a+1,s}(u)T_{a-1,s}(u) + T_{a,s+1}(u)T_{a,s-1}(u).$$

Similarly to Chapter II.4, one can start from these equations, subject to suitable boundary conditions, and predict the spectrum at finite coupling.

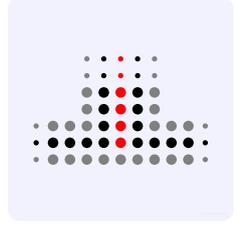

## IV Further Applications of Integrability

For the sake of a clear presentation the previous parts focused on one particular application of integrability in AdS/CFT: Solving the exact planar spectrum of  $\mathcal{N} = 4$  supersymmetric Yang–Mills theory or equivalently of IIB string theory on  $AdS_5 \times S^5$ . While this topic has been at the centre of attention, many investigations have dealt with extending the applications of integrability to other observables beyond the planar spectrum and to more general models. This part and the following try to give an overview of these developments.

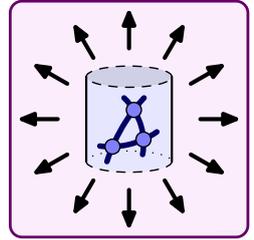

### IV.1 Aspects of Non-planarity

Integrability predicts the planar spectrum accurately and with minimum effort. It would be desirable to extend the applications of integrability to non-planar corrections because, e.g., in QCD  $N_c = 3$  rather than  $N_c = \infty$ . For the spectrum, these are interactions where the spin chain or the string splits up and recombines

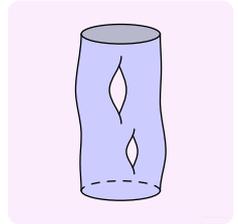

$$H = H_0 + \frac{1}{N_c} (H_+ + H_-) + \dots$$

They result in a string worldsheet of higher genus or with more than two punctures.

Chapter IV.1 reviews the available results on higher-genus corrections, higher-point functions as well as supersymmetric Wilson loops in the AdS/CFT context. It is shown that most of the basic constructions of integrability do not work in the non-planar setup.

## IV.2 Deformations, Orbifolds and Open Boundaries

There exist many deformations of  $\mathcal{N} = 4$  SYM which preserve some or the other property, e.g. by deforming the ( $\mathcal{N} = 1$ ) superpotential

$$\int d^4x d^4\theta \operatorname{Tr} (e^{i\beta} XYZ - e^{-i\beta} ZYX).$$

It is natural to find out under which conditions integrability can survive. Chapter IV.2 reviews such superconformal deformations of  $\mathcal{N} = 4$  SYM and shows how the methods of integrability can be adjusted to these cases. It turns out that these merely deform the boundary conditions of the integrable model by introducing additional phases into the Bethe equations (in the spin chain context this has a similar effect as turning on a magnetic field). Different boundary conditions can also arise from looking at other corners of the spectrum or at different observables; this is another topic of the present chapter.

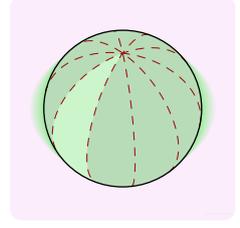

## IV.3 $\mathcal{N} = 6$ Chern-Simons and Strings on $AdS_4 \times CP^3$

Recently a quantum field theory in three dimensions was discovered which behaves in many respects like  $\mathcal{N} = 4$  SYM —  $\mathcal{N} = 6$  supersymmetric Chern–Simons–matter theory

$$S = \frac{k}{4\pi} \int \operatorname{Tr} (A \wedge dA + \frac{2}{3} A \wedge A \wedge A + \dots).$$

It is exactly superconformal at the quantum level, and there is an AdS/CFT dual string theory — IIA superstrings on the  $AdS_4 \times CP^3$  background. Importantly, there exists a large- $N_c$  limit, in which the model becomes integrable. Chapter IV.3 reviews integrability in this  $AdS_4/CFT_3$  correspondence. While being largely analogous to the constructions in the previous parts, there are several noteworthy differences in the application of integrable methods: For instance, here the spin representation alternates between the sites.

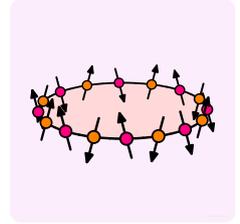

## IV.4 Integrability in QCD and $\mathcal{N} < 4$ SYM

Similar integrable structures were known to exist in more general gauge theories long before the exploitation of integrability in  $\mathcal{N} = 4$  SYM. Chapter IV.4 introduces evolution equations for high-energy scattering (BFKL) and scaling of quasi-partonic operators in connection to deep inelastic scattering (DGLAP). To some extent these take the form of integrable Hamiltonians with  $sl(2|\mathcal{N})$  symmetry ( $J_{12}$  is the two-particle spin operator and  $\Psi$  is the digamma function)

$$H_{12} \simeq \Psi(J_{12}) - \Psi(1).$$

Its eigenvalues determine the scaling of certain hadronic structure functions and control the energy dependence of scattering amplitudes in the high-energy (Regge) limit.

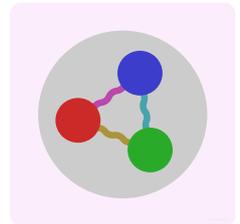

## V Integrability for Scattering Amplitudes

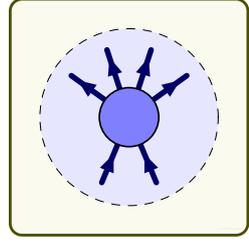

The most conservative application of quantum field theories is to compute scattering cross sections (to be compared to particle scattering experiments). With old blades sharpened and new ones developed, the charted territory of tree and loop scattering amplitudes in  $\mathcal{N} = 4$  SYM has increased dramatically, see e.g. the recent reviews [18] and the special issue [19]. It was soon noticed that something special was going on in the planar limit which makes amplitudes much simpler than originally thought. It does not take much imagination to conjecture a connection to integrability. This part reviews scattering amplitudes and what integrability implies in this context. This topic is under active investigation, many advances have been and are being made, but a lot remains to be understood. Here, one can expect that integrability will enable a similarly simple solution as in the case of the planar spectrum.

### V.1 Scattering Amplitudes – a Brief Introduction

Chapter V.1 gives an introduction into the topic of scattering amplitudes in  $\mathcal{N} = 4$  SYM. First of all, the spinor-helicity formalism and colour-ordering scheme strips the combinatorial structure and leaves plain functions. For instance, an essential part of an  $n$ -particle amplitude simply reads  $\langle\langle kj \rangle\rangle$  is a Lorentz-invariant  $\delta$  constructed from the momenta of particles  $k$  and  $j$ )

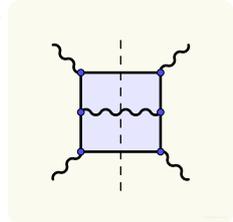

$$A_n^{\text{MHV}} = \frac{\delta^4(P) \delta^8(Q)}{\langle 12 \rangle \langle 23 \rangle \cdots \langle n1 \rangle}.$$

The S-matrix displays a host of useful analyticity properties related to unitarity. These can be used to reconstruct tree and loop amplitudes from scratch, which is typically far more efficient than using Feynman diagrams following from the Lagrangian description.

### V.2 Dual Superconformal Symmetry

Chapter V.2 reviews simplifications found in planar scattering. It turns out that the underlying scalar integrals are of a special form which hints at conformal symmetry in a dual space. Indeed, the amplitudes obey a dual superconformal symmetry in addition to the conventional one. The two sets of conformal symmetries close onto an infinite-dimensional algebra which is at the heart of integrability — the Yangian.

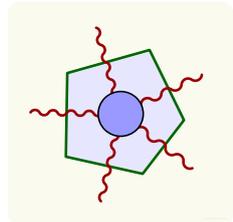

This symmetry helps to determine all (tree) amplitudes, by means of recursion or through a Grassmannian integral ( $C$  is a  $k \times n$  matrix,  $M_j$  are its  $k \times k$  minors of consecutive columns, and  $Z$  are  $4|4$  twistors encoding the momenta of the  $n$  legs)

$$A_{n,k}^{\text{tree}}(Z) = \int \frac{d^{k(n-k)} C \delta^{k(4|4)}(CZ)}{M_1 \cdots M_n}.$$

### V.3 Scattering Amplitudes at Strong Coupling

Chapter V.3 discusses the string dual of scattering amplitudes. Here it makes sense to transform particle momenta to distances by means of a T-duality. At strong coupling an amplitude is then dominated by the minimal area of a string worldsheet ending on a light-like polygonal contour on the  $AdS_5$  boundary (the previous Chapter V.2 provides evidence in favour of a general relation between amplitudes and light-like polygonal Wilson loops). Such minimal areas can be computed efficiently by integrable means bypassing the determination of the complicated shape of the worldsheet (cf. Chapter III.5)

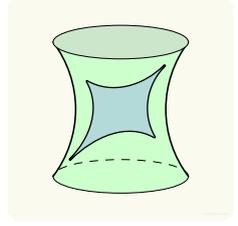

$$A_{\text{reg}} = \sum_k \int \frac{d\theta m_k \cosh \theta}{2\pi} \log(1 + Y_k(\theta)).$$

## VI Algebraic Aspects of Integrability

Integrability can be viewed as a symmetry. In most cases it enhances an obvious, finite-dimensional symmetry of a physical system to a hidden, infinite-dimensional algebra. The extended symmetry then imposes a large number of constraints onto the system which determine the dynamics (almost) completely, but without making it trivial. Many of the properties and methods that come to use in integrable systems find a mathematical formulation in terms of quantum algebra. Often this does not help immediately in computing particular physical observables, one of the main objectives of the previous parts. Rather, it can give a deeper understanding of how the model's integrability works, with a view to finding rigorous proofs for the applicability of the (well-tested) proposals.

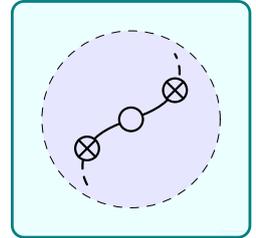

This final part of the review presents the symmetries relevant to our gauge and string theory problem. These are the Lie supergroup  $PSU(2, 2|4)$  as the obvious symmetry and its Yangian algebra to encode integrability.

### VI.1 Superconformal Algebra

The Lie superalgebra  $\mathfrak{psu}(2, 2|4)$  is generated by  $8 \times 8$  supermatrices (in  $2|4|2$  grading)

$$J = \left( \begin{array}{c|c|c} L & -iQ & P \\ \hline S & R & \bar{Q} \\ \hline K & -i\bar{S} & \bar{L} \end{array} \right),$$

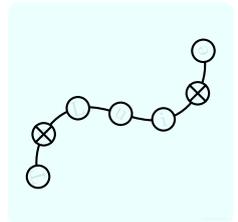

subject to suitable constraints, projections and hermiticity conditions. It serves as the spacetime superconformal symmetry in gauge theory as well as the target space isometries of the dual string theory.

Chapter VI.1 summarises some well-known facts and results for this algebra. It also explains how the algebra applies to the gauge and string theory setup. The chapter is not so much related to integrability itself, it can rather be understood as an appendix to many of the other chapters when it comes to the basics of symmetry.

## VI.2 Yangian Algebra

In physics one is used to the concept of locally and homogeneously acting symmetries. Chapter VI.2 introduces the Yangian algebra whose non-local action is encoded by the coproduct

$$\Delta(Y^A) = Y^A \otimes 1 + 1 \otimes Y^A + f_{BC}^A J^B \otimes J^C.$$

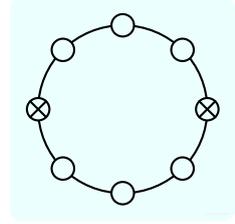

For instance, such a non-local action permits a scattering matrix which is fully determined by the algebra while still being non-trivial. The scattering matrix becomes a natural intertwining object of the Yangian, its R-matrix. It enjoys a host of useful properties which eventually make the physical system tractable.

## Acknowledgements

N. Beisert thanks T. Bargheer, M. de Leeuw and L. Lipatov for helpful comments on the manuscript.

The work of C. Ahn was supported in part by KRF-2007-313-C00150 and WCU grant R32-2008-000-10130-0 (CA). R. Janik was supported in part by Polish science funds as a research project N N202 105136 (2009–2011). The work of C. Kristjansen and K. Zoubos was supported by FNU through grant number 272-08-0329. The work of R. I. Nepomechie was supported in part by the National Science Foundation under Grants PHY-0554821 and PHY-0854366 (RN). The work of A. Torrielli has been partially supported by EPSRC through the grant no. EP/H000054/1.

## References

- [1] J. M. Maldacena, “*The large  $N$  limit of superconformal field theories and supergravity*”, *Adv. Theor. Math. Phys.* 2, 231 (1998), [hep-th/9711200](#). • S. S. Gubser, I. R. Klebanov and A. M. Polyakov, “*Gauge theory correlators from non-critical string theory*”, *Phys. Lett. B* 428, 105 (1998), [hep-th/9802109](#). • E. Witten, “*Anti-de Sitter space and holography*”, *Adv. Theor. Math. Phys.* 2, 253 (1998), [hep-th/9802150](#).
- [2] S. Kovacs, “ *$N=4$  supersymmetric Yang-Mills theory and the AdS/SCFT correspondence*”, [hep-th/9908171](#). • O. Aharony, S. S. Gubser, J. M. Maldacena, H. Ooguri and Y. Oz, “*Large  $N$  field theories, string theory and gravity*”, *Phys. Rept.* 323, 183 (2000), [hep-th/9905111](#). • E. D’Hoker and D. Z. Freedman, “*Supersymmetric gauge theories and the AdS/CFT correspondence*”, [hep-th/0201253](#). • J. M. Maldacena, “*Lectures on AdS/CFT*”, [hep-th/0309246](#). • H. Nastase, “*Introduction to AdS-CFT*”, [arxiv:0712.0689](#). • J. Polchinski, “*Introduction to Gauge/Gravity Duality*”, [arxiv:1010.6134](#).
- [3] M. K. Benna and I. R. Klebanov, “*Gauge-String Dualities and Some Applications*”, [arxiv:0803.1315](#). • I. R. Klebanov and J. M. Maldacena, “*Solving quantum field theories via curved spacetimes*”, *Phys. Today* 62, 28 (2009).
- [4] G. ’t Hooft, “*A Planar Diagram Theory for Strong Interactions*”, *Nucl. Phys. B* 72, 461 (1974).

- [5] G. T. Horowitz and J. Polchinski, “*Gauge / gravity duality*”, [gr-qc/0602037](#).
- [6] H. Kawai, D. C. Lewellen and S.-H. H. Tye, “*A relation between tree amplitudes of closed and open strings*”, *Nucl. Phys. B*269, 1 (1986).
- [7] Z. Bern, J. J. M. Carrasco and H. Johansson, “*New Relations for Gauge-Theory Amplitudes*”, *Phys. Rev. D*78, 085011 (2008), [arxiv:0805.3993](#). • Z. Bern, J. J. M. Carrasco and H. Johansson, “*Perturbative Quantum Gravity as a Double Copy of Gauge Theory*”, *Phys. Rev. Lett.* 105, 061602 (2010), [arxiv:1004.0476](#).
- [8] B. L. Ioffe, V. S. Fadin and L. N. Lipatov, (eds.), “*Quantum chromodynamics: Perturbative and nonperturbative aspects*”, Cambridge University Press (2010), Cambridge, UK.
- [9] N. Seiberg and E. Witten, “*Monopole Condensation, And Confinement In  $\mathcal{N} = 2$  Supersymmetric Yang-Mills Theory*”, *Nucl. Phys. B*426, 19 (1994), [hep-th/9407087](#). • N. Seiberg and E. Witten, “*Monopoles, duality and chiral symmetry breaking in  $\mathcal{N} = 2$  supersymmetric QCD*”, *Nucl. Phys. B*431, 484 (1994), [hep-th/9408099](#).
- [10] N. A. Nekrasov and S. L. Shatashvili, “*Supersymmetric vacua and Bethe ansatz*”, *Nucl. Phys. Proc. Suppl.* 192-193, 91 (2009), [arxiv:0901.4744](#). • N. A. Nekrasov and S. L. Shatashvili, “*Quantum integrability and supersymmetric vacua*”, *Prog. Theor. Phys. Suppl.* 177, 105 (2009), [arxiv:0901.4748](#).
- [11] H. Lotter, “*Phenomenology of the BFKL pomeron and unitarity corrections at low  $x$* ”, [hep-ph/9705288](#). • J. R. Forshaw and D. A. Ross, “*Quantum chromodynamics and the pomeron*”, Cambridge University Press (1997), Cambridge, UK. • S. Donnachie, G. Dosch, P. Landshoff and O. Nachtmann, “*Pomeron Physics and QCD*”, Cambridge University Press (2002), Cambridge, UK.
- [12] F. H. L. Essler, H. Frahm, F. Göhmann, A. Klümper and V. E. Korepin, “*The one-dimensional Hubbard model*”, Cambridge University Press (2005), Cambridge, UK.
- [13] J. Plefka, “*Spinning strings and integrable spin chains in the AdS/CFT correspondence*”, *Living Rev. Rel.* 8, 9 (2005), [hep-th/0507136](#). • J. A. Minahan, “*A brief introduction to the Bethe ansatz in  $\mathcal{N} = 4$  super-Yang-Mills*”, *J. Phys. A*39, 12657 (2006). • N. Dorey, “*Notes on integrability in gauge theory and string theory*”, *J. Phys. A*42, 254001 (2009). • G. Arutyunov and S. Frolov, “*Foundations of the AdS<sub>5</sub> × S<sup>5</sup> Superstring. Part I*”, *J. Phys. A*42, 254003 (2009), [arxiv:0901.4937](#). • B. Basso and G. P. Korchemsky, “*Nonperturbative scales in AdS/CFT*”, *J. Phys. A*42, 254005 (2009), [arxiv:0901.4945](#). • L. F. Alday, “*Scattering amplitudes and the AdS/CFT correspondence*”, *J. Phys. A*42, 254006 (2009). • D. Serban, “*Integrability and the AdS/CFT correspondence*”, *J. Phys. A*44, 124001 (2011), [arxiv:1003.4214](#). • F. Fiamberti, A. Santambrogio and C. Sieg, “*Superspace methods for the computation of wrapping effects in the standard and beta-deformed  $\mathcal{N} = 4$  SYM*”, [arxiv:1006.3475](#).
- [14] N. Beisert, “*The dilatation operator of  $\mathcal{N} = 4$  super Yang-Mills theory and integrability*”, *Phys. Rept.* 405, 1 (2005), [hep-th/0407277](#). • I. Swanson, “*A review of integrable deformations in AdS/CFT*”, *Mod. Phys. Lett. A*22, 915 (2007), [arxiv:0705.2844](#). • K. Okamura, “*Aspects of Integrability in AdS/CFT Duality*”, [arxiv:0803.3999](#). • B. Vicedo, “*Finite- $g$  Strings*”, *J. Phys. A* 44, 124002 (2011), [arxiv:0810.3402](#). • A. Rejz, “*Integrability and the AdS/CFT correspondence*”, *J. Phys. A*42, 254002 (2009), [arxiv:0907.3468](#). • N. Gromov, “*Integrability in AdS/CFT correspondence:*

- Quasi-classical analysis*”, J. Phys. A42, 254004 (2009). • D. Volin, “*Quantum integrability and functional equations*”, J. Phys. A44, 124003 (2011), arxiv:1003.4725. • V. G. M. Puletti, “*On string integrability. A journey through the two-dimensional hidden symmetries in the AdS/CFT dualities*”, Adv. High Energy Phys. 2010, 471238 (2010), arxiv:1006.3494. • M. de Leeuw, “*The S-matrix of the AdS<sub>5</sub> × S<sup>5</sup> superstring*”, arxiv:1007.4931.
- [15] S. Schäfer-Nameki, “*Strings and super-Yang-Mills theory: The integrable story*”, J. Stat. Mech. 0612, N001 (2006). • H. Nicolai, “*String theory: Back to basics*”, Nature 449, 797 (2007).
- [16] C. Kristjansen, M. Staudacher and A. Tseytlin, (eds.), “*Gauge-string duality and integrability: Progress and outlook*”, J. Phys. A42, 250301 (2009). • P. Dorey, J. Minahan and A. Tseytlin, (eds.), “*Quantum integrable models and gauge-string duality*”, J. Phys. A44, 120301 (2011).
- [17] P. Dorey, G. Dunne and J. Feinberg, (eds.), “*Recent Advances in Low-Dimensional Quantum Field Theories*”, J. Phys. A39, issue 41 editorial (2006). • F. Alcaraz, O. Babelon, J. de Gier and O. Foda, (eds.), “*The 75th Anniversary of the Bethe Ansatz*”, topical articles in J. Stat. Mech., <http://iopscience.iop.org/1742-5468/focus/extra.topical2>.
- [18] L. J. Dixon, “*Gluon scattering in  $\mathcal{N} = 4$  super-Yang-Mills theory from weak to strong coupling*”, PoS RADCOR2007, 056 (2007), arxiv:0803.2475. • L. F. Alday and R. Roiban, “*Scattering Amplitudes, Wilson Loops and the String/Gauge Theory Correspondence*”, Phys. Rept. 468, 153 (2008), arxiv:0807.1889. • J. M. Henn, “*Duality between Wilson loops and gluon amplitudes*”, Fortsch. Phys. 57, 729 (2009), arxiv:0903.0522. • M. Wolf, “*A First Course on Twistors, Integrability and Gluon Scattering Amplitudes*”, J. Phys. A43, 393001 (2010), arxiv:1001.3871. • J. M. Drummond, “*Hidden Simplicity of Gauge Theory Amplitudes*”, Class. Quant. Grav. 27, 214001 (2010), arxiv:1010.2418.
- [19] R. Roiban, M. Spradlin and A. Volovich, (eds.), “*Scattering Amplitudes in Gauge Theories: Progress and Outlook*”, J. Phys. A 44, 450301 (2011).



# Review of AdS/CFT Integrability, Chapter I.1: Spin Chains in $\mathcal{N} = 4$ Super Yang-Mills

JOSEPH A. MINAHAN

*Department of Physics and Astronomy, Uppsala University  
SE-751 20 Uppsala, Sweden*

joseph.minahan@fysast.uu.se

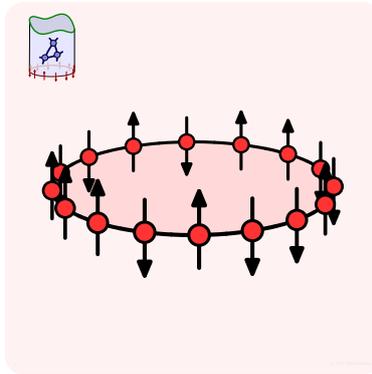

**Abstract:** In this chapter of *Review of AdS/CFT Integrability* we introduce  $\mathcal{N} = 4$  Super Yang-Mills. We discuss the global superalgebra  $PSU(2,2|4)$  and its action on gauge invariant operators. We then discuss the computation of the correlators of certain gauge invariant operators, the so-called single trace operators in the large  $N$  limit. We show that interactions in the gauge theory lead to mixing of the operators. We compute this mixing at the one-loop level and show that the problem maps to a one-dimensional spin chain with nearest neighbor interactions. For operators in the  $SU(2)$  sector we show that the spin chain is the ferromagnetic Heisenberg spin chain whose eigenvalues are determined by the Bethe equations.

# 1 Introduction and summary

In this chapter of *Review of AdS/CFT Integrability* [1], we introduce  $\mathcal{N} = 4$  super Yang-Mills (SYM), a gauge theory with the maximal amount of supersymmetry <sup>1</sup>.  $\mathcal{N} = 4$  SYM was first considered by Brink, Scherk and Schwarz [3], who explicitly constructed its Lagrangian by dimensionally reducing SYM from 10 to 4 dimensions. One of the remarkable properties of  $\mathcal{N} = 4$  SYM is that it is conformal [4], meaning that it has no inherent mass scale in the theory. Many theories are classically conformal, namely any theory with only massless fields and marginal couplings. But  $\mathcal{N} = 4$  stays conformal even at the quantum level. In particular its  $\beta$ -function is zero to all orders in perturbation theory, as was first conjectured in [5] when studying open string loop amplitudes which reduce to ten dimensional SYM in the infinite string tension limit.

In a theory such as QCD which has a running coupling constant, there is a natural mass scale at the crossover point from weak to strong coupling. In QCD this is roughly where confinement sets in and is responsible for the proton mass. Since  $\mathcal{N} = 4$  SYM is conformal it cannot be confining, meaning that there are no mesons and hadrons, the physical particles in QCD. Why then should we study it?

There are several reasons. First, its large amount of symmetry leads to an underlying integrability, making many physical quantities analytically calculable, as many of the chapters in this review will explain. Second, the AdS/CFT correspondence [6] conjectures that  $\mathcal{N} = 4$  Super Yang-Mills is equivalent to type IIB string theory on  $AdS_5 \times S^5$ . This correspondence is a strong/weak duality which is normally very difficult to confirm because when one theory is computationally under control the other is not. However, the integrability allows us to plow forward and calculate at strong coupling, thus testing many consequences of the conjecture. Third, while QCD is not conformal, it is asymptotically free. Hence at high energies it is close to being conformal. Many essential features of high energy gluon scattering, which is relevant for the LHC, can be learned by studying gauge boson amplitudes in  $\mathcal{N} = 4$  SYM.

There are other reasons for studying  $\mathcal{N} = 4$  SYM, including its conjectured invariance under  $SL(2, Z)$  duality transformations [7], but they are less relevant for integrability. Nevertheless, the three reasons stated here are hopefully enough motivation to press on.

In the following sections we will first describe the fields that make up  $\mathcal{N} = 4$  SYM, showing that they lead to a vanishing one-loop  $\beta$ -function. We then discuss the symmetry algebra of  $\mathcal{N} = 4$ . Here we define a class of operators called chiral primaries whose dimensions are protected from quantum corrections. We next describe a particular set of gauge invariant operators, single trace operators, which are of significant importance in the large  $N$  limit. We find how the fields transform under the symmetry algebra and from there find the chiral primaries in the single trace operators. Using supersymmetry arguments we then show that the gauge coupling  $g_{\text{YM}}$  is fixed under rescalings and so the theory is conformal, even at the quantum level.

We then compute the one-loop anomalous dimensions for a general set of single trace operators composed of scalar fields. We show that in the large  $N$  limit where the contributions to the anomalous dimensions are dominated by planar graphs, the problem

---

<sup>1</sup>This chapter is a substantial extension of an earlier review [2].

is identical to computing the energies of a certain spin-chain with nearest neighbor interactions. We then describe how the spin-chain can be generalized to all single trace operators. Finally, we discuss the solutions for this spin-chain in a particular sector called the  $SU(2)$  sector, where one finds the famous Bethe equations.

The full description of these spin chains, including their higher loop generalizations and their solutions are deferred to later chapters of the review.

## 2 The field content and the vanishing $\beta$ -function

The fields contained in  $\mathcal{N} = 4$  SYM are the gauge bosons  $\mathcal{A}_\mu$ , six massless real scalar fields  $\phi^I$ ,  $I = 1 \dots 6$ , four chiral fermions  $\psi_\alpha^a$  and four anti-chiral fermions  $\bar{\psi}_{\dot{\alpha}a}$ , with  $a = 1 \dots 4$ . The indices  $\alpha, \dot{\alpha} = 1, 2$  are the spinor indices of the two independent  $SU(2)$  algebras that make up the 4 dimensional Lorentz algebra. All fields transform in the adjoint representation of the  $SU(N)$  gauge group. There is a global  $SU(4) \simeq SO(6)$  symmetry, called an  $R$ -symmetry, with the scalars transforming in the  $\mathbf{6}$ ,  $\psi_\alpha^a$  in the  $\mathbf{4}$  (raised  $a$  index) and  $\bar{\psi}_{\dot{\alpha}a}$  in the  $\bar{\mathbf{4}}$  (lowered  $a$  index) representations of the  $R$ -symmetry algebra.

Let us use the information about the field content to rapidly show that the one-loop  $\beta$ -function is zero. For any  $SU(N)$  gauge theory, the one-loop  $\beta$ -function for the gauge coupling  $g_{\text{YM}}$  is given by [8]

$$\beta_1(g_{\text{YM}}) \equiv \mu \frac{\partial g_{\text{YM}}}{\partial \mu} = -\frac{g_{\text{YM}}^3}{16\pi^2} \left( \frac{11}{3} N - \frac{1}{6} \sum_i C_i - \frac{1}{3} \sum_j \tilde{C}_j \right), \quad (2.1)$$

where the first sum is over all real scalars with quadratic casimir  $C_i$  and the second sum is over all Weyl fermions with quadratic casimir  $\tilde{C}_j$ . All fields in  $\mathcal{N} = 4$  SYM are in the adjoint, hence all casimirs are  $N$ . One can then quickly see that with six real scalars and eight Weyl fermions that  $\beta_1(g_{\text{YM}}) = 0$ .

Going beyond one-loop, the  $\beta$ -function for  $\mathcal{N} = 4$  SYM was shown to be zero up to three loops using superspace arguments [9]. Subsequently it was argued using light cone gauge that the  $\beta$ -function is zero to all loops [10]. In a later section we will present a different argument for why the  $\beta$ -function is zero to all orders.

## 3 The superconformal algebra

The conformal symmetry, the supersymmetry and the  $R$ -symmetry of  $\mathcal{N} = 4$  SYM are part of a larger symmetry group. This group is known as the  $\mathcal{N} = 4$  superconformal group, or more formally as  $PSU(2, 2|4)$ . This symmetry group is unbroken by quantum corrections and thus serves as a powerful tool by putting significant constraints on the theory. In this section we will review the  $PSU(2, 2|4)$  algebra and its consequences. A more detailed description is given in [11].

$PSU(2, 2|4)$  has the bosonic subalgebra  $SU(2, 2) \times SU(4)$ . The  $SU(2, 2) \simeq SO(2, 4)$  is the four dimensional conformal algebra while the  $SU(4) \simeq SO(6)$  is the  $R$ -symmetry. The conformal algebra has 15 generators: ten generators belong to the Poincaré algebra

which itself contains four generators of space-time translations,  $P_\mu$  and six generators of the  $SO(1,3) \equiv SU(2) \times SU(2)$  Lorentz transformations,  $M_{\mu\nu}$ . The other generators of the conformal algebra are the four generators of special conformal transformations,  $K_\mu$  and one generator of dilatations,  $D$ . These generators then satisfy the commutation relations

$$\begin{aligned} [D, P_\mu] &= -iP_\mu & [D, M_{\mu\nu}] &= 0 & [D, K_\mu] &= +iK_\mu \\ [M_{\mu\nu}, P_\lambda] &= -i(\eta_{\mu\lambda}P_\nu - \eta_{\lambda\nu}P_\mu) & [M_{\mu\nu}, K_\lambda] &= -i(\eta_{\mu\lambda}K_\nu - \eta_{\lambda\nu}K_\mu) \\ [P_\mu, K_\nu] &= 2i(M_{\mu\nu} - \eta_{\mu\nu}D). \end{aligned} \quad (3.1)$$

Let  $\mathcal{O}(x)$  be a local operator in the field theory with dimension  $\Delta$ . This signifies that under the rescaling  $x \rightarrow \lambda x$ ,  $\mathcal{O}(x)$  scales as  $\mathcal{O}(x) \rightarrow \lambda^{-\Delta}\mathcal{O}(\lambda x)$ .  $D$  is the generator of these scalings, by which we mean that  $\mathcal{O}(x) \rightarrow \lambda^{-iD}\mathcal{O}(x)\lambda^{iD}$ . Thus, its action on  $\mathcal{O}(x)$  is

$$[D, \mathcal{O}(x)] = i \left( -\Delta + x \frac{\partial}{\partial x} \right) \mathcal{O}(x). \quad (3.2)$$

Next, we let  $D$  act on  $[K_\mu, \mathcal{O}(0)]$ , where we find using the Jacobi identity

$$\begin{aligned} [D, [K_\mu, \mathcal{O}(0)]] &= [[D, K_\mu], \mathcal{O}(0)] + [K_\mu, [D, \mathcal{O}(0)]] \\ &= i[K_\mu, \mathcal{O}(0)] - i\Delta[K_\mu, \mathcal{O}(0)]. \end{aligned} \quad (3.3)$$

Thus,  $K_\mu$  creates a new local operator from  $\mathcal{O}$  with its dimension lowered by 1. Aside from the identity operator, the local operators in a unitary quantum field theory must have positive dimension. Therefore, if we keep creating new lower dimensional operators by commuting with the special conformal generators, we must eventually reach a barrier where we can go no further. Hence the last operator in this chain,  $\tilde{\mathcal{O}}(x)$  must satisfy

$$[K_\mu, \tilde{\mathcal{O}}(0)] = 0. \quad (3.4)$$

for all  $K_\mu$ . The operator  $\tilde{\mathcal{O}}(x)$  is called *primary*<sup>2</sup>. Starting with  $\tilde{\mathcal{O}}$ , we can build new operators with the same dimension or higher by commuting it with the other generators of the conformal algebra. The higher dimensional operators are called *descendants*<sup>3</sup> of  $\tilde{\mathcal{O}}$ .

The conformal algebra can be combined with supersymmetry to make a superconformal algebra. In four dimensions one can have gauge theories with  $\mathcal{N} = 1$ ,  $\mathcal{N} = 2$  or  $\mathcal{N} = 4$  supersymmetry, and all of these cases can be combined with the conformal symmetries to make an  $\mathcal{N} = 1$ ,  $\mathcal{N} = 2$  or  $\mathcal{N} = 4$  superconformal algebra. Here, we only consider the  $\mathcal{N} = 4$  case.

The generators of supersymmetry transformations are fermionic and are called *supercharges*. For  $\mathcal{N} = 4$  supersymmetry there are 16 separate supercharges,  $Q_{\alpha a}$  and

<sup>2</sup>The primary condition (3.4) is defined at  $x = 0$  where the space-time position is a fixed point of the dilatation. If the local operator were at a different space-time point then it would commute with a different combination of the conformal generators.

<sup>3</sup>Peradventure they should have been called *ascendants*.

$\tilde{Q}_{\dot{\alpha}}^a$ , where  $\alpha, \dot{\alpha} = 1, 2$  and  $a = 1..4$  are the same spinor and  $R$ -symmetry indices that label the Weyl fields, except here the  $\alpha$  indices are paired with the  $\bar{4}$  and the  $\dot{\alpha}$  indices are paired with the  $4$ . The supersymmetry algebra is a graded Lie algebra which combines the generators of the Poincaré algebra with the supercharges and contains the commutation and anti-commutation relations

$$\begin{aligned} \{Q_{\alpha a}, \tilde{Q}_{\dot{\alpha}}^b\} &= \gamma_{\alpha\dot{\alpha}}^\mu \delta_a^b P_\mu, & \{Q_{\alpha a}, Q_{\alpha b}\} &= \{\tilde{Q}_{\dot{\alpha}}^a, \tilde{Q}_{\dot{\alpha}}^b\} = 0 \\ [P_\mu, Q_{\alpha a}] &= [P_\mu, \tilde{Q}_{\dot{\alpha}}^b] = 0 \\ [M^{\mu\nu}, Q_{\alpha a}] &= i\gamma_{\alpha\beta}^{\mu\nu} \epsilon^{\beta\gamma} Q_{\gamma a}, & [M^{\mu\nu}, \tilde{Q}_{\dot{\alpha}}^a] &= i\gamma_{\dot{\alpha}\dot{\beta}}^{\mu\nu} \epsilon^{\dot{\beta}\dot{\gamma}} \tilde{Q}_{\dot{\gamma}}^a, \end{aligned} \quad (3.5)$$

where  $\gamma_{\alpha\beta}^{\mu\nu} = \gamma_{\alpha\dot{\alpha}}^{[\mu} \gamma_{\dot{\beta}\beta}^{\nu]}$ . Simple dimension counting within the algebra shows that  $Q_{\alpha a}$  and  $\tilde{Q}_{\dot{\alpha}}^a$  have dimension  $1/2$  and so their commutators with  $D$  is

$$[D, Q_{\alpha a}] = -\frac{i}{2} Q_{\alpha a} \quad [D, \tilde{Q}_{\dot{\alpha}}^a] = -\frac{i}{2} \tilde{Q}_{\dot{\alpha}}^a. \quad (3.6)$$

By including the special conformal generators we generate a new set of supercharges by commuting  $K_\mu$  with  $Q_{\alpha a}$  and  $\tilde{Q}_{\dot{\alpha}}^a$ ,

$$[K^\mu, Q_{\alpha a}] = \gamma_{\alpha\dot{\alpha}}^\mu \epsilon^{\dot{\alpha}\dot{\beta}} \tilde{S}_{\dot{\beta} a} \quad [K^\mu, \tilde{Q}_{\dot{\alpha}}^a] = \gamma_{\alpha\dot{\alpha}}^\mu \epsilon^{\alpha\beta} S_\beta^a. \quad (3.7)$$

The operators  $S_\alpha^a$  and  $\tilde{S}_{\dot{\alpha} a}$  have dimension  $-1/2$  and are known as the special conformal supercharges, or the superconformal charges. Their  $R$ -charge representations are reversed from the supercharges and combine with the regular supercharges to give 32 supercharges in total. The superconformal generators have anticommutation relations that mirror the anticommutation relations of the supercharges,

$$\begin{aligned} \{S_\alpha^a, \tilde{S}_{\dot{\alpha} b}\} &= \gamma_{\alpha\dot{\alpha}}^\mu \delta_a^b K_\mu & \{S_\alpha^a, S_\alpha^b\} &= \{\tilde{S}_{\dot{\alpha} a}, \tilde{S}_{\dot{\alpha} b}\} = 0 \\ [K_\mu, S_\alpha^a] &= [K_\mu, \tilde{S}_{\dot{\alpha} a}] = 0. \end{aligned} \quad (3.8)$$

Nonzero anticommutation relations between the supercharges and the superconformal charges complete the algebra,

$$\begin{aligned} \{Q_{\alpha a}, S_\beta^b\} &= -i\varepsilon_{\alpha\beta} \sigma^{IJ} \delta_a^b R_{IJ} + \gamma_{\alpha\beta}^{\mu\nu} \delta_a^b M_{\mu\nu} - \frac{1}{2} \varepsilon_{\alpha\beta} \delta_a^b D \\ \{\tilde{Q}_{\dot{\alpha}}^a, \tilde{S}_{\dot{\beta} b}\} &= +i\varepsilon_{\dot{\alpha}\dot{\beta}} \sigma^{IJ} \delta_a^b R_{IJ} + \gamma_{\dot{\alpha}\dot{\beta}}^{\mu\nu} \delta_a^b M_{\mu\nu} - \frac{1}{2} \varepsilon_{\dot{\alpha}\dot{\beta}} \delta_a^b D \\ \{Q_{\alpha a}, \tilde{S}_{\dot{\beta} b}\} &= \{\tilde{Q}_{\dot{\alpha}}^a, S_\beta^b\} = 0. \end{aligned} \quad (3.9)$$

On the righthand side of (3.9) one has in addition to the Lorentz and dilatation generators the  $SU(4) \simeq SO(6)$   $R$ -symmetry generators  $R_{IJ}$ , where  $I, J = 1 \dots 6$ . The supercharges transform under the two spinor representations of  $SO(6)$ , while all generators of the conformal algebra commute with  $R_{IJ}$ .

Let us now return to the primary operator  $\tilde{\mathcal{O}}(x)$ . Commuting the superconformal charges with a local operator  $\mathcal{O}(0)$  lowers the dimension by  $1/2$ . A lower bound on the dimension must still exist, so we assume that  $\tilde{\mathcal{O}}(0)$  satisfies

$$[S_\alpha^a, \tilde{\mathcal{O}}(0)] = [\tilde{S}_{\dot{\alpha} a}, \tilde{\mathcal{O}}(0)] = 0 \quad \text{for all } \alpha, \dot{\alpha}, a. \quad (3.10)$$

$\tilde{\mathcal{O}}(x)$  is clearly primary since the anticommutation relations in (3.8) directly lead to (3.4). The descendants of  $\tilde{\mathcal{O}}(0)$  are constructed from the rest of the algebra.

The primary operator and its descendants make up an irreducible representation of  $PSU(2, 2|4)$ , with the primary as the highest weight of the representation.  $PSU(2, 2|4)$  is noncompact, so the representation is infinite dimensional<sup>4</sup>. For example, one can act with  $P_\mu$  on  $\tilde{\mathcal{O}}(x)$  an arbitrary number of times, where  $[P_\mu, \mathcal{O}(x)] = -i\partial_\mu \mathcal{O}(x)$ , making a new local operator with one higher dimension. Using the supercharges we can also make new operators with 1/2 higher dimension.

We will be particularly interested in a class of highest weight representations which, while still infinite dimensional, are smaller because there are fewer independent operators at each half-step in dimension. In order for this to occur,  $\tilde{\mathcal{O}}(0)$  must commute with some of the supercharges. Let us then place the further restriction on  $\tilde{\mathcal{O}}(x)$  that

$$[Q_\alpha^a, \tilde{\mathcal{O}}(0)] = 0 \quad \text{for some } \alpha, a. \quad (3.11)$$

It then follows from the anticommutation relations in (3.9) that

$$[\{Q_{\alpha a}, S_\beta^b\}, \tilde{\mathcal{O}}(0)] = [-i\varepsilon_{\alpha\beta}\sigma^{IJ}{}_a{}^b R_{IJ} - \varepsilon_{\alpha\beta}\delta_a{}^b D + \sigma_{\alpha\beta}^{\mu\nu}\delta_a{}^b M_{\mu\nu}, \tilde{\mathcal{O}}(0)] = 0. \quad (3.12)$$

We assume that  $\tilde{\mathcal{O}}(x)$  is a scalar, therefore  $\tilde{\mathcal{O}}(0)$  commutes with the Lorentz generators  $M_{\mu\nu}$ . What remains is a simple relation between the action of the  $R$ -symmetry and the dimension  $\Delta$  of  $\tilde{\mathcal{O}}(x)$ ,

$$\sigma^{IJ}{}_a{}^b [R_{IJ}, \tilde{\mathcal{O}}(0)] = \Delta \delta_a{}^b \tilde{\mathcal{O}}(0). \quad (3.13)$$

To help us find operators that can satisfy the relation in (3.13) we consider the Cartan subalgebra of  $SO(6)$ .  $SO(6)$  is a rank 3 group and thus has three commuting generators in its Cartan subalgebra. We choose these generators to be  $R_{12}$ ,  $R_{34}$  and  $R_{56}$  and write the corresponding charges as  $(J_1, J_2, J_3)$ . The  $\sigma^{IJ}{}_a{}^b$  are the generators in the  $SU(4)$  fundamental representation, with

$$\sigma^{12} = \begin{pmatrix} 1 & 0 & 0 & 0 \\ 0 & 1 & 0 & 0 \\ 0 & 0 & -1 & 0 \\ 0 & 0 & 0 & -1 \end{pmatrix} \quad \sigma^{34} = \begin{pmatrix} 1 & 0 & 0 & 0 \\ 0 & -1 & 0 & 0 \\ 0 & 0 & 1 & 0 \\ 0 & 0 & 0 & -1 \end{pmatrix} \quad \sigma^{56} = \begin{pmatrix} 1 & 0 & 0 & 0 \\ 0 & -1 & 0 & 0 \\ 0 & 0 & -1 & 0 \\ 0 & 0 & 0 & 1 \end{pmatrix}, \quad (3.14)$$

as a consistent choice of Cartan generators. Hence, a primary operator with  $R$ -charges  $(J_1, 0, 0)$  is annihilated by  $Q_{\alpha 1}$  and  $Q_{\alpha 2}$  if  $\Delta = J_1$ . The anticommutation relations in (3.9) indicate that such operators are also annihilated by  $\tilde{Q}_\alpha^3$  and  $\tilde{Q}_\alpha^4$ . Hence, an operator of this type commutes with half of the supercharges. Such operators are called chiral primary or BPS operators. By the same logic an operator with  $(0, J_2, 0)$  and dimension  $\Delta = J_2$  is also a chiral primary. But such a state is in the same  $SO(6)$  representation as the  $(J_2, 0, 0)$  operator, and hence is in the same  $PSU(2, 2|4)$  representation. Therefore, it is only necessary to consider the scalar operators with charges  $(J, 0, 0)$  and  $\Delta = J$ .

In general the dimension of an operator will depend on the Yang-Mills coupling  $g_{\text{YM}}$ . The dimension at zero coupling is known as the bare dimension. The correction to

<sup>4</sup>Except for the trivial representation which only contains the identity operator.

the bare dimension is the anomalous dimension. From our discussion so far we learn two important facts. First, the anomalous dimensions within the same  $PSU(2, 2|4)$  representation are equal. This is because the generators can only change the dimension in  $1/2$  integer steps. Second, and more strikingly, the chiral primaries and their descendants cannot have an anomalous dimension. This is because the chiral primaries commute with half the supercharges no matter what the coupling. If they did not commute then there would have to be extra operators at each level. But the number of independent operators with a given dimension is a finite integer which cannot change by varying a continuous parameter such as the coupling. Hence, the relation in (3.13) continues to hold. Since the  $R$ -charges are integers that stay fixed, then the dimensions must also stay fixed.

## 4 Gauge invariant operators in $\mathcal{N} = 4$ SYM

We now apply our discussion in the previous section to the actual operators that one encounters in  $\mathcal{N} = 4$  SYM. The physical observables in a gauge theory must be gauge invariant. In  $\mathcal{N} = 4$  SYM, the local gauge invariant operators are made up of products of traces of the fields that transform covariantly under the gauge group. This includes the scalars  $\phi^I$ , the fermions  $\psi_\alpha^a$ ,  $\bar{\psi}_{\dot{\alpha}a}$  and the field strengths  $\mathcal{F}_{\mu\nu}$ . Since these fields all lie in the adjoint representation, their transformation under a gauge transformation is

$$\chi(x) \rightarrow \chi(x) + [\varepsilon(x), \chi(x)] \quad (4.1)$$

where  $\chi(x)$  is one of the covariant fields and  $\varepsilon(x)$  is a generator of gauge transformations. We have explicitly included the space-time dependence of the fields to emphasize that this is a local transformation. From a covariant field  $\chi(x)$  we can make other covariant fields  $\mathcal{D}_\mu\chi(x)$ , where  $\mathcal{D}_\mu$  is the covariant derivative

$$\mathcal{D}_\mu\chi(x) \equiv \partial_\mu\chi(x) - [\mathcal{A}_\mu(x), \chi(x)]. \quad (4.2)$$

The gauge connection  $\mathcal{A}_\mu(x)$  does not transform covariantly, but instead transforms as

$$\mathcal{A}_\mu(x) \rightarrow \mathcal{A}_\mu(x) + \partial_\mu\varepsilon(x) + [\varepsilon(x), \mathcal{A}_\mu(x)]. \quad (4.3)$$

It is then clear that the single trace local operator

$$\mathcal{O}(x) = \text{Tr}[\chi_1(x)\chi_2(x)\dots\chi_L(x)], \quad (4.4)$$

where  $\chi_i(x)$  refers to one of the above covariant fields with or without covariant derivatives, is gauge invariant. We can also build other local gauge invariant operators by taking products of traces. Later on we will take the limit where the number of colors  $N$  is large. In this limit the dimension of the product of single trace operators is equal to the sum of their dimensions, so all information about the spectrum of local operators comes from the single trace operators.

Because  $[\mathcal{D}_\mu, \mathcal{D}_\nu] = -\mathcal{F}_{\mu\nu}(x)$ , any antisymmetric combination of covariant derivatives can always be replaced with a field strength. Hence, it is only necessary to consider symmetric products of  $\mathcal{D}_\mu$  acting on any field  $\chi$ . Furthermore, we can use the equations

of motion and the Bianchi identities to get rid of certain combinations of covariant derivatives. As an example, the equations of motion for the scalar fields are schematically

$$\mathcal{D}^\mu \mathcal{D}_\mu \phi^I = \dots \quad (4.5)$$

The right hand side of (4.5) contains cubic scalar terms as well as fermion bilinears, but otherwise has no derivatives. Therefore, inside a trace we can always replace two contracted derivatives on a scalar with nonderivative terms.

With these rules we can build all single trace operators. We first construct the single trace chiral primaries, from which we can systematically assemble the other operators. The  $SU(2, 2) \times SU(4)$  bosonic subgroup of  $PSU(2, 2|4)$  is rank six and so an operator will have a sextuplet of charges,  $(\Delta, S_1, S_2; J_1, J_2, J_3)$ . The  $J_i$  are the  $R$ -charges discussed in the last section,  $\Delta$  is the dimension, and  $S_1$  and  $S_2$  are the two charges of the  $SO(1, 3)$  Lorentz group (*i.e.* the spins). In this subsection we will only consider the gauge theory at zero coupling, in which case the dimension can be replaced with the bare dimension  $\Delta_0$  and all dimensions are additive.

The six adjoint scalars  $\phi^I$  can be expressed as three complex fields,  $Z = \frac{1}{\sqrt{2}}(\phi^1 + i\phi^2)$ ,  $W = \frac{1}{\sqrt{2}}(\phi^3 + i\phi^4)$   $X = \frac{1}{\sqrt{2}}(\phi^5 + i\phi^6)$ , along with their conjugates. Scalars in 4 dimensions have bare dimension 1 and are of course spinless, thus the charges for  $Z$ ,  $W$  and  $X$  are given by  $(1, 0, 0; 1, 0, 0)$ ,  $(1, 0, 0; 0, 1, 0)$ , and  $(1, 0, 0; 0, 0, 1)$  respectively. Their conjugates,  $\bar{Z}$ ,  $\bar{W}$  and  $\bar{X}$  have reversed  $R$ -charges. The sixteen fermions  $\psi_\alpha^a$  and  $\bar{\psi}_{\dot{\alpha}a}$  have charges  $(\frac{3}{2}, \pm\frac{1}{2}, 0; \pm\frac{1}{2}, \pm\frac{1}{2}, \pm\frac{1}{2})$  and  $(\frac{3}{2}, 0, \pm\frac{1}{2}; \pm\frac{1}{2}, \pm\frac{1}{2}, \pm\frac{1}{2})$  where the number of negative signs for the  $SU(4)$  charges is even for the first set and odd for the second. The field strengths have six independent components and naturally split into their even and odd self-duals, where  $\mathcal{F}_\pm^{\mu\nu} = \pm\frac{1}{2}\varepsilon^{\mu\nu\rho\sigma}\mathcal{F}_{\pm\rho\sigma}$ . In terms of the  $SO(1, 3) \simeq SU(2) \times SU(2)$  Lorentz group, the even and odd self-duals fall into the  $(3, 1) \oplus (1, 3)$  representation. It is thus convenient to write the components using the  $SU(2) \times SU(2)$  spinor indices, where we define

$$\mathcal{F}_{+\alpha\beta} \equiv \frac{1}{2}(\gamma^{\mu\nu})_{\alpha\beta}\mathcal{F}_{+\mu\nu} = \mathcal{F}_{+\beta\alpha}, \quad \mathcal{F}_{-\dot{\alpha}\dot{\beta}} \equiv \frac{1}{2}(\gamma^{\mu\nu})_{\dot{\alpha}\dot{\beta}}\mathcal{F}_{-\mu\nu} = \mathcal{F}_{-\dot{\beta}\dot{\alpha}}. \quad (4.6)$$

From this we readily see that the  $\mathcal{F}_+$  have charges  $(2, m, 0; 0, 0, 0)$  and the  $\mathcal{F}_-$  have charges  $(2, 0, m; 0, 0, 0)$  where  $m = +1, 0, -1$ . It is also useful to write the covariant derivatives as a bispinor  $\mathcal{D}_{\alpha\dot{\beta}} \equiv (\gamma^\mu)_{\alpha\dot{\beta}}\mathcal{D}_\mu$ . Then  $\mathcal{D}_{\alpha\dot{\beta}}$  acting on a field adds the charges  $(1, \pm\frac{1}{2}, \pm\frac{1}{2}; 0, 0, 0)$  to the charges of the operator.

Let us now consider the gauge invariant operator  $\Psi_L \equiv \text{Tr}[Z^L]$ , with  $L \geq 2$  ( $\text{Tr}Z = 0$ ). The charges of  $\Psi_L$  are  $(L, 0, 0; L, 0, 0)$ , which satisfies  $\Delta_0 = J_1$ . Therefore,  $\Psi_L$  is a chiral primary and  $\Delta = \Delta_0$ , even after the coupling is turned on.  $\Psi_L$  is the highest weight element of the  $L$ -fold symmetric traceless representation of  $SO(6)$ . Hence, any operator of the form

$$\chi_{I_1 I_2 \dots I_L} \text{Tr}(\phi^{I_1} \phi^{I_2} \dots \phi^{I_L}),$$

where  $\chi_{I_1 I_2 \dots I_L}$  is completely symmetric in its indices and the trace of any two indices is zero, is a chiral primary with its dimension protected from quantum corrections. Notice further that if we change one of the  $Z$  fields in  $\Psi_L$  to any other scalar field, aside from  $\bar{Z}$ , then the resulting operator is automatically symmetric and traceless because of the

cyclicity of the trace. To make a non-BPS operator strictly out of scalars will require at least one  $\overline{Z}$  or two other scalar fields that are not  $Z$  or  $\overline{Z}$ .

A very convenient way to classify the single trace operators is to use bosonic and fermionic creation operators [12–14] (see also [11]). To this end we note that the vector representation of the  $SO(6)$   $R$ -symmetry group is equivalent to the antisymmetric representation of  $SU(4)$ . Hence, the scalar fields can be written in  $SU(4)$  notation as  $\phi^{ab}$  with the indices antisymmetrized. Likewise, the fermions in the antifundamental representation can have its  $SU(4)$  index raised to three antisymmetric indices,  $\overline{\psi}_{\dot{\alpha}}^{abc} \equiv \varepsilon^{abcd}\overline{\psi}_{\dot{\alpha}d}$ . Thus all fields have their fundamental  $SU(4)$  indices antisymmetrized. Furthermore, the field strengths come with symmetrized spinor indices, the combination  $\varepsilon^{\alpha\beta}\mathcal{D}_{\alpha\dot{\alpha}}\psi_{\dot{\beta}}^a$  can always be replaced by a nonderivative term by the equations of motion, and all covariant derivatives are symmetrized. Hence, all indices in either of the  $SU(2)$ 's of the Lorentz group are symmetrized for any field, including those with covariant derivatives.

Therefore, we will build the fields at each site within the trace with two sets of bosonic creation operators  $A_{\alpha}^{\dagger}$ ,  $B_{\dot{\alpha}}^{\dagger}$ , and a set of fermionic creation operators  $C^{a\dagger}$ . The adjoints of these fields are  $A^{\alpha}$ ,  $B^{\dot{\alpha}}$  and  $C_a$  and we have the usual set of commutation or anticommutation relations

$$[A^{\alpha}, A_{\beta}^{\dagger}] = \delta^{\alpha}_{\beta}, \quad [B^{\dot{\alpha}}, B_{\dot{\beta}}^{\dagger}] = \delta^{\dot{\alpha}}_{\dot{\beta}}, \quad \{C_a, C^{b\dagger}\} = \delta_a^b. \quad (4.7)$$

One starts with a ground state  $|0\rangle$  for each site and defines the operator

$$\mathcal{C} = A_{\alpha}^{\dagger}A^{\alpha} - B_{\dot{\alpha}}^{\dagger}B^{\dot{\alpha}} + C^{a\dagger}C_a - 2. \quad (4.8)$$

Then the states that correspond to the actual fields are those states  $|\chi\rangle$  in the oscillator Fock space where  $\mathcal{C}|\chi\rangle = 0$ . We denote this projected Fock space by  $\mathcal{V}$ . The states satisfying the  $\mathcal{C} = 0$  condition and the fields they correspond to are

$$\begin{aligned} (A^{\dagger})^{k+2}(B^{\dagger})^k|0\rangle &\Rightarrow \mathcal{D}^k\mathcal{F}_+ \\ (A^{\dagger})^{k+1}(B^{\dagger})^kC^{a\dagger}|0\rangle &\Rightarrow \mathcal{D}^k\psi^a \\ (A^{\dagger})^k(B^{\dagger})^kC^{a\dagger}C^{b\dagger}|0\rangle &\Rightarrow \mathcal{D}^k\phi^{ab} \\ (A^{\dagger})^k(B^{\dagger})^{k+1}C^{a\dagger}C^{b\dagger}C^{c\dagger}|0\rangle &\Rightarrow \mathcal{D}^k\overline{\psi}^{abc} \\ (A^{\dagger})^k(B^{\dagger})^{k+2}C^{a\dagger}C^{b\dagger}C^{c\dagger}C^{d\dagger}|0\rangle &\Rightarrow \mathcal{D}^k\mathcal{F}_-, \end{aligned} \quad (4.9)$$

where we have suppressed all Lorentz indices.

The elements of  $PSU(2, 2|4)$  can also be nicely represented by the oscillators. In particular we have that

$$\begin{aligned} P_{\alpha\dot{\beta}} &= A_{\alpha}^{\dagger}B_{\dot{\beta}}^{\dagger} & K_{\alpha\dot{\beta}} &= -\varepsilon_{\alpha\gamma}\varepsilon_{\dot{\beta}\dot{\delta}}A^{\gamma}B^{\dot{\delta}} \\ Q_{\alpha a} &= A_{\alpha}^{\dagger}C_a & \widetilde{Q}_{\dot{\alpha}}^a &= B_{\dot{\alpha}}^{\dagger}C^{a\dagger} & S_{\alpha}^a &= -i\varepsilon_{\alpha\beta}A^{\alpha}C^{a\dagger} & \widetilde{S}_{\dot{\alpha} a} &= -i\varepsilon_{\dot{\alpha}\dot{\beta}}B^{\dot{\beta}}C_a \\ R^a_b &= C^{a\dagger}C_b - \frac{1}{4}\delta^a_b C^{c\dagger}C_c & D &= -\frac{i}{2}\left(A_{\alpha}^{\dagger}A^{\alpha} + B_{\dot{\alpha}}^{\dagger}B^{\dot{\alpha}} + 2\right) \\ M_{\alpha}^{\beta} &= A_{\alpha}^{\dagger}A^{\beta} - \frac{1}{2}\delta_{\alpha}^{\beta}A_{\gamma}^{\dagger}A^{\gamma} & \widetilde{M}_{\dot{\alpha}}^{\dot{\beta}} &= B_{\dot{\alpha}}^{\dagger}B^{\dot{\beta}} - \frac{1}{2}\delta_{\dot{\alpha}}^{\dot{\beta}}B_{\dot{\gamma}}^{\dagger}B^{\dot{\gamma}}, \end{aligned} \quad (4.10)$$

where we have expressed the  $R$ -symmetry generators in  $SU(4)$  notation and the Lorentz generators in  $SU(2) \times SU(2)$  notation<sup>5</sup>. The oscillator representation of the algebra is also useful when applied to  $\mathcal{N} = \text{SYM}$  scattering amplitudes [15]. Notice that all generators commute with  $\mathcal{C}$ , hence  $\mathcal{C}$  is a centralizer of the algebra. Thus, the elements of the algebra acting on the above states preserve the  $\mathcal{C} = 0$  condition. In fact the “ $P$ ” in front of  $PSU(2, 2|4)$  stands for “projective” and corresponds to the projection we have made onto the  $\mathcal{C} = 0$  states. This projection is necessary in order for (4.10) to give the relations in (3.9).

The set of projected states in this Fock space (4.9) form an irreducible representation of  $PSU(2, 2|4)$  called the “singleton” representation [16]<sup>6</sup>. However, it cannot correspond to a representation of gauge invariant operators since all of the fields are traceless. Hence we will need  $L \geq 2$  fields inside the trace, leading to tensor products of the singleton representations.

$$\mathcal{V}_1 \otimes \mathcal{V}_2 \otimes \cdots \otimes \mathcal{V}_L. \quad (4.11)$$

The various generators of  $PSU(2, 2|4)$  on the tensor product have the general form

$$\mathcal{T} = \sum_{\ell=1}^L \oplus \mathcal{T}_\ell, \quad (4.12)$$

where  $\mathcal{T}_\ell$  is the generator at site  $\ell$ . We can also define  $\mathcal{C}$  in this way, however the projection is still carried out at each site, *i.e.*  $\mathcal{C}_\ell = 0$ . A gauge invariant operator is then mapped to a state in the tensor product, but because of the cyclicity of the trace must be projected onto only those states that are invariant under the shift,

$$\mathcal{V}_1 \otimes \mathcal{V}_2 \otimes \cdots \otimes \mathcal{V}_L \rightarrow \mathcal{V}_L \otimes \mathcal{V}_1 \otimes \cdots \otimes \mathcal{V}_{L-1}. \quad (4.13)$$

Let us now concentrate on the operator

$$\mathcal{O}^{abcd} = \text{Tr} \phi^{ab} \phi^{cd} - \frac{1}{4!} \varepsilon^{abcd} \varepsilon_{a'b'c'd'} \text{Tr} \phi^{a'b} \phi^{c'd'}, \quad (4.14)$$

which is part of the same  $SU(4)$  representation as  $\text{Tr} Z^2$  and so is a chiral primary. We then act with four supercharges in the following manner:

$$\frac{1}{4!} \varepsilon^{\alpha\gamma} \varepsilon^{\beta\delta} \{Q_{\alpha a}, [Q_{\beta b}, \{Q_{\gamma c}, [Q_{\delta d}, \mathcal{O}^{abcd}]]\}] = \varepsilon^{\alpha\gamma} \varepsilon^{\beta\delta} \text{Tr} \mathcal{F}_{+\alpha\beta} F_{+\gamma\delta}. \quad (4.15)$$

Likewise, letting  $\mathcal{O}_{abcd} = \text{Tr} \phi_{ab} \phi_{cd} - \frac{1}{4!} \varepsilon_{abcd} \varepsilon^{a'b'c'd'} \text{Tr} \phi_{a'b} \phi_{c'd'}$  and acting with the other four supercharges we find

$$\frac{1}{4!} \varepsilon^{\dot{\alpha}\dot{\gamma}} \varepsilon^{\dot{\beta}\dot{\delta}} \{\tilde{Q}_{\dot{\alpha}}^a, [\tilde{Q}_{\dot{\beta}}^b, \{\tilde{Q}_{\dot{\gamma}}^c, [\tilde{Q}_{\dot{\delta}}^d, \mathcal{O}_{abcd}]]\}] = \varepsilon^{\alpha\gamma} \varepsilon^{\beta\delta} \text{Tr} \mathcal{F}_{-\alpha\beta} F_{-\gamma\delta}. \quad (4.16)$$

<sup>5</sup>Strictly speaking, one should use the conformal Hamiltonian,  $H = iD$ , instead of  $D$  as an  $SU(2, 2)$  generator. See [11] for a further discussion on this point.

<sup>6</sup>Some authors call this representation a “doubleton” (*cf.* [13]). Another name is the fundamental representation.

Therefore,  $\text{Tr}\mathcal{F}_+F_+$  and  $\text{Tr}\mathcal{F}_-\mathcal{F}_-$  are in the same supermultiplet as the chiral primary and thus their dimensions are protected from quantum corrections, meaning that they have dimension 4 no matter what the coupling. These terms appear in the Lagrangian under the combination

$$-i(\tau \text{Tr}\mathcal{F}_+F_+ - \bar{\tau} \text{Tr}\mathcal{F}_-\mathcal{F}_-), \quad (4.17)$$

where  $\tau = \frac{4\pi i}{g_{\text{YM}}^2} + \frac{\theta}{2\pi}$  with the  $\theta$ -angle included. Since  $\text{Tr}\mathcal{F}_+F_+$  and  $\text{Tr}\mathcal{F}_-\mathcal{F}_-$  are dimension 4 and the Lagrangian must also be dimension 4, we see that  $\tau$ , and hence  $g_{\text{YM}}$  is invariant under rescaling. From this argument we learn that the  $\beta$ -function is zero.

## 5 One loop anomalous dimensions and the relation to spin chains

In this section we compute the one-loop anomalous dimensions for operators composed of scalar fields with no covariant derivatives [17]. This computation is complicated by the problem of operator mixing. However, the mixing can often be restricted to operators within certain ‘‘closed’’ sectors.

To find the anomalous dimension of an operator, one considers the two-point correlator of the operator with itself. In particular, one finds that

$$\langle \mathcal{O}(x)\bar{\mathcal{O}}(y) \rangle \approx \frac{1}{|x-y|^{2\Delta}}, \quad (5.1)$$

where the dimension  $\Delta = \Delta_0 + \gamma$ , with  $\Delta_0$  being the bare dimension and  $\gamma$  being the anomalous dimension arising from quantum corrections. For operators made up only of scalar fields with no covariant derivatives, all fields have bare dimension 1 and the bare dimension of the operator is  $L$ , the number of scalar fields inside the trace.

If  $g_{\text{YM}}$  is small, then  $\gamma \ll \Delta_0$ , in which case we can approximate the correlator in (5.1) as

$$\langle \mathcal{O}(x)\bar{\mathcal{O}}(y) \rangle \approx \frac{1}{|x-y|^{2\Delta_0}}(1 - \gamma \ln \Lambda^2|x-y|^2), \quad (5.2)$$

where  $\Lambda$  is cutoff scale. The leading contribution to this correlator is called the tree-level contribution.

Let us now investigate what happens as we let  $N \rightarrow \infty$ . For example, let us consider the chiral primary operator  $\Psi_L$ , rescaled to

$$\Psi_L = \frac{(4\pi^2)^{L/2}}{\sqrt{L}N^{L/2}} \text{Tr}Z^L = \frac{(4\pi^2)^{L/2}}{\sqrt{L}N^{L/2}} Z^A{}_B Z^B{}_C \dots Z^{\dots}{}_A \quad A, B, C = 1..N, \quad (5.3)$$

where we have explicitly put in the color indices. The prefactors are for normalization purposes. At tree level, the correlator of a  $Z$  field and its conjugate  $\bar{Z}$  is<sup>7</sup>

$$\langle Z^A{}_B(x)\bar{Z}^C{}_D(y) \rangle_{\text{tree}} = \frac{\delta^A{}_D \delta_B^C}{4\pi^2|x-y|^2}, \quad (5.4)$$

<sup>7</sup>We have ignored the fact that  $Z^A{}_A = 0$ , which is justifiable when we take the large  $N$  limit.

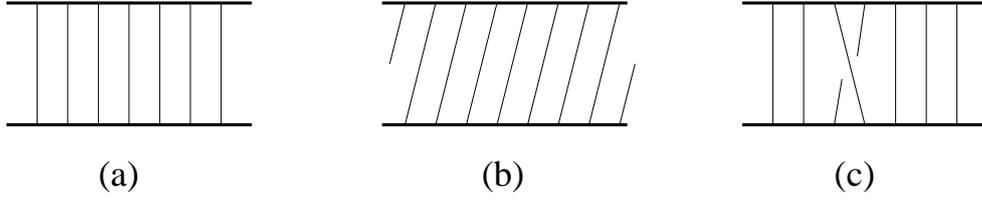

**Figure 1:** Contractions of fields. The horizontal lines represent the operators and the ordered vertical lines the contractions between the two operators of the individual fields inside the trace. (a) and (b) are planar while (c) is nonplanar.

where we have ignored the fact that  $Z^A_A = 0$  which is justified in the large  $N$  limit. If we now contract  $\Psi_L$  with its conjugate  $\bar{\Psi}_L$ , then the leading contribution to the correlator comes from contracting the individual fields in order, as shown in figure 1 (a) and (b). The contribution of all such ordered contractions is

$$\langle \Psi_L(x) \bar{\Psi}_L(y) \rangle_{\text{ordered}} = \frac{LN^L}{(\sqrt{L}N^{L/2})^2 |x-y|^{2L}} = \frac{1}{|x-y|^{2L}}. \quad (5.5)$$

The factor of  $N^L$  comes from  $L$  factors of  $\delta^{A'}_A \delta^A_{A'} = N$ , where each double set of delta functions are from contractions of neighboring fields. The factor of  $L$  comes from the  $L$  ways of contracting the fields in the plane, of which (a) and (b) are two examples of this.

Figure 1 (c) is an example of a nonplanar graph, a graph where the lines connecting the fields cannot be drawn in the plane without cutting other lines. To avoid such cuttings one must lift at least one connecting line out of the plane. The figure in (c) differs from (a) by two field contractions. Whereas in (a) we would have had a factor of

$$\dots \delta^{A'}_A \delta^A_{A'} \delta^{B'}_B \delta^B_{B'} \delta^{C'}_C \delta^C_{C'} \dots = \dots N^3 \dots, \quad (5.6)$$

in (c) we have the factor

$$\dots \delta^{A'}_A \delta^A_{B'} \delta^{C'}_B \delta^B_{A'} \delta^{B'}_C \delta^C_{C'} \dots = \dots N \dots, \quad (5.7)$$

where the dots represent contractions that are the same in both cases. Hence, the nonplanar graph in (c) is suppressed by a factor of  $1/N^2$  from that in (a). In the limit where  $N \rightarrow \infty$  we can thus ignore this contribution compared to the one in (a) or (b).

All nonplanar graphs will be suppressed by powers of  $1/N^2$ , where the power depends on the topology of the graph. Actually, this analysis is valid only if  $L \ll N$ . If  $L$  were on the order of  $N$  then the suppression coming from the  $1/N$  factors is swamped by the huge number of nonplanar diagrams compared to the number of planar diagrams. (There are  $L!$  total tree level diagrams of which only  $L$  are planar.)

Generalizing the tree-level correlator in (5.5) to any scalar operator of the form

$$\mathcal{O}_{I_1, I_2 \dots I_L}(x) = \frac{(4\pi^2)^{L/2}}{\sqrt{C_{I_1, I_2 \dots I_L}} N^{L/2}} \text{Tr}(\phi_{I_1}(x) \phi_{I_2}(x) \dots \phi_{I_L}(x)), \quad (5.8)$$

where  $C_{I_1, I_2 \dots I_L}$  is a symmetry factor (which is  $n$  if the indices are invariant when shifting by  $L/n$ ), one finds

$$\langle \mathcal{O}_{I_1, I_2 \dots I_L}(x) \overline{\mathcal{O}}^{J_1, J_2 \dots J_L}(y) \rangle_{\text{tree}} = \frac{1}{C_{I_1, I_2 \dots I_L}} (\delta_{I_1}^{J_1} \delta_{I_2}^{J_2} \dots \delta_{I_L}^{J_L} + \text{cycles}) \frac{1}{|x - y|^{2L}}, \quad (5.9)$$

where ‘‘cycles’’ refers to the  $L - 1$  cyclic shifts of the  $J_i$  indices.

We next consider the one-loop contribution to the two-point correlator. Since we are only considering scalar operators, we only need to consider the bosonic part of the  $\mathcal{N} = 4$  action<sup>8</sup> which is given by

$$S = \frac{1}{2g_{\text{YM}}^2} \int d^4x \left\{ -\frac{1}{2} \text{Tr} \mathcal{F}^2 + \text{Tr} \mathcal{D}_\mu \phi_I \mathcal{D}^\mu \phi^I - \sum_{I < J} \text{Tr} [\phi_I, \phi_J]^2 \right\}. \quad (5.10)$$

This action contains a quartic interaction term for the scalars as well as interaction terms between the scalars and the gauge bosons coming from the covariant derivatives. Hence there will be several types of Feynman graphs that can contribute to the anomalous dimension. But because of the robustness of the superconformal algebra, it is sufficient to only consider Feynman graphs containing the scalar vertex. Graphs containing gauge bosons do affect the anomalous dimension, but their contribution can be determined by insisting that chiral primaries have zero anomalous dimension.

If we absorb a factor of  $g_{\text{YM}}$  into the fields so that their kinetic terms are canonical, then the quartic term can be written as

$$\frac{g_{\text{YM}}^2}{4} \sum_{I, J} \left( \text{Tr} \phi_I \phi_I \phi_J \phi_J - \text{Tr} \phi_I \phi_J \phi_I \phi_J \right). \quad (5.11)$$

This vertex should then be inserted in the correlator and be Wick contracted with two neighboring fields in the incoming operator and two neighboring fields in the outgoing operator so that the resulting Feynman graph is planar. This is shown in figure 2. In particular, we should consider the subcorrelator from (5.9),

$$\begin{aligned} & \left\langle (\phi_{I_k} \phi_{I_{k+1}})^A{}_C(x) \left( \frac{i g_{\text{YM}}^2}{4} \int d^4z \sum_{I, J} (\text{Tr} \phi_I \phi_I \phi_J \phi_J(z) - \text{Tr} \phi_I \phi_J \phi_I \phi_J(z)) \right) \right. \\ & \quad \left. \times (\phi^{J_{k+1}} \phi^{J_k})^{C'}{}_{A'}(y) \right\rangle \\ &= i \frac{N}{(4\pi^2)^2} \delta^A{}_{A'} \delta_C{}^{C'} \frac{g_{\text{YM}}^2 N}{64 \pi^4} (2\delta_{I_k}^{J_k} \delta_{I_{k+1}}^{J_{k+1}} + 2\delta_{I_k I_{k+1}} \delta^{J_k J_{k+1}} - 4\delta_{I_k}^{J_{k+1}} \delta_{I_{k+1}}^{J_k}) \\ & \quad \times \int \frac{d^4z}{|z - x|^4 |z - y|^4}. \end{aligned} \quad (5.12)$$

The set of delta functions for the flavor indices arise from the two terms in (5.11). There are four planar ways to contract the indices in (5.11) with the incoming and outgoing

<sup>8</sup>Other parts of the action will contribute at one-loop, but we will show that we can compute their contribution by using an indirect method.

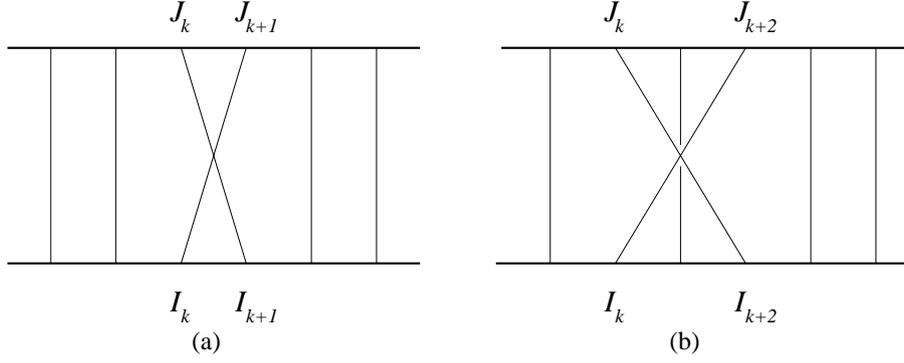

**Figure 2:** Quartic interaction inserted into the correlator, connecting (a) two neighboring fields (b) nonneighboring fields. Case (b) is nonplanar. Notice that the interaction has added a loop to the diagrams.

fields. The first term either contracts the incoming indices with the outgoing indices in order, or it contracts incoming to incoming and outgoing to outgoing. The second term in (5.11) always contracts the indices between the incoming and outgoing fields in reverse order. Note that there are two factors of  $N$  in (5.12), coming from sums over color factors, while the correlator  $\langle (\phi_{I_k} \phi_{I_{k+1}})^A_C(x) (\phi^{J_{k+1}} \phi^{J_k})^{C'}_{A'}(y) \rangle$  has only one such factor. In fact, it is not difficult to see that for all planar graphs, every factor of  $g_{\text{YM}}^2$  comes with a factor of  $N$ . Hence, it is convenient to define the 't Hooft coupling,  $\lambda \equiv g_{\text{YM}}^2 N$ , as a new expansion parameter.

The integral in (5.12) has a logarithmic divergence as  $z \rightarrow x$  and  $z \rightarrow y$ , hence it is necessary to add a UV cutoff  $\Lambda$ . There is no IR divergence since the integral is well behaved as  $z \rightarrow \infty$ . The integral over  $z$  is in Minkowski space, but it can be Wick rotated to Euclidean space such that  $d^4 z \rightarrow id^4 z_E$ . With the UV cutoff the integral is restricted to the region where  $|z_E - x| \geq \Lambda^{-1}$  and  $|z_E - y| \geq \Lambda^{-1}$ . The integral is then dominated by the regions near the cutoff and can be approximated to

$$i \int \frac{d^4 z_E}{|z - x|^4 |z - y|^4} \approx \frac{2i}{|x - y|^4} \int_{\Lambda^{-1}}^{|x-y|} \frac{d\xi d\Omega_3}{\xi} = \frac{2\pi^2 i}{|x - y|^4} \ln(\Lambda^2 |x - y|^2). \quad (5.13)$$

Therefore the subcorrelator in (5.12) becomes

$$\frac{N \delta^A_{A'} \delta_C^{C'}}{(4\pi^2)^2 |x - y|^4} \frac{\lambda}{16\pi^2} (2\delta_{I_k I_{k+1}} \delta^{J_k J_{k+1}} - \delta_{I_k}^{J_{k+1}} \delta_{I_{k+1}}^{J_k} - \delta_{I_k}^{J_k} \delta_{I_{k+1}}^{J_{k+1}}) \ln(\Lambda^2 |x - y|^2). \quad (5.14)$$

Normally one does loop integrals in momentum space. We could have done that here as well, but for these particular one-loop calculations it is easier to do things in coordinate space. This is mainly because the operators are local so all fields within the operator are at the same coordinate position, simplifying the calculation.

There will also be other one-loop contributions to the correlators. Figure 3 shows some examples of these. These can come from gluon exchange between scalar fields or self energy diagrams. We could compute these contributions explicitly, but we will soon

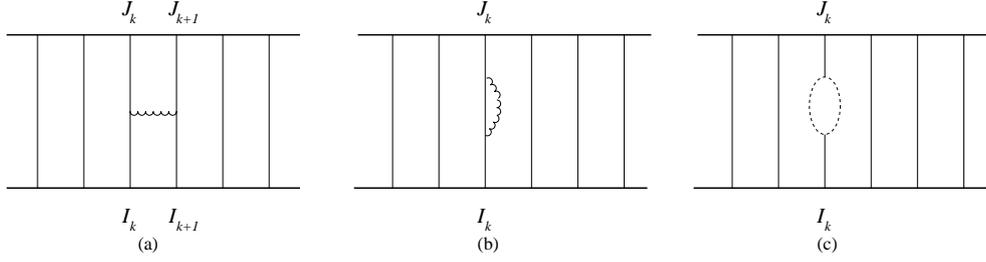

**Figure 3:** One-loop planar graphs that do not affect the flavor structures. (a) A gluon exchange between neighboring scalars. The gluon carries no  $R$ -charge, so the flavor indices are unchanged. (b) Scalar self-energy from a gluon. (c) Scalar self-energy from a fermion loop.  $R$ -charge conservation and the fact that only one scalar line is involved means that (b) and (c) leave the flavor indices unchanged.

show that we do not actually need to do this. At this point we note that since the  $R$ -charge is conserved and since gluons have no  $R$ -charge, then these types of diagrams will only lead to terms where all incoming indices are contracted sequentially with the outgoing indices, giving the same flavor structure as the planar tree-level graphs.

Applying these arguments to the correlator in (5.9), we find the one-loop result

$$\begin{aligned} & \langle \mathcal{O}_{I_1, I_2, \dots, I_L}(x) \overline{\mathcal{O}}^{J_1, J_2, \dots, J_L}(y) \rangle_{\text{one-loop}} \\ &= \frac{\lambda}{16\pi^2} \frac{\ln(\Lambda^2|x-y|^2)}{|x-y|^{2L}} \sum_{\ell=1}^L (2P_{\ell, \ell+1} - K_{\ell, \ell+1} - 1 + C) \frac{1}{\sqrt{C_{I_1, \dots, I_L} C_{J_1, \dots, J_L}}} \delta_{I_1}^{J_1} \delta_{I_2}^{J_2} \dots \delta_{I_L}^{J_L} \\ & \quad + \text{cycles} . \end{aligned} \quad (5.15)$$

There is a sum over  $\ell$  because the diagram in figure 2(a) can have the interaction between any of the  $L$  pairs of neighboring fields. The constant  $C$  comes from the diagrams in figure 3. ‘‘Cycles’’ again refers to the  $L - 1$  uniform shifts of the  $J_k$  indices.

$P_{\ell, \ell+1}$  is the exchange operator, and as its name implies it exchanges the flavor indices of the  $\ell$  and the  $\ell + 1$  sites inside the trace. Its action on the  $\delta$ -functions in (5.15) is

$$P_{\ell, \ell+1} \delta_{I_1}^{J_1} \dots \delta_{I_\ell}^{J_\ell} \delta_{I_{\ell+1}}^{J_{\ell+1}} \dots \delta_{I_L}^{J_L} = \delta_{I_1}^{J_1} \dots \delta_{I_\ell}^{J_{\ell+1}} \delta_{I_{\ell+1}}^{J_\ell} \dots \delta_{I_L}^{J_L} . \quad (5.16)$$

$K_{\ell, \ell+1}$  is the trace operator which contracts the flavor indices of neighboring fields. Its action on the  $\delta$ -functions is

$$K_{\ell, \ell+1} \delta_{I_1}^{J_1} \dots \delta_{I_\ell}^{J_\ell} \delta_{I_{\ell+1}}^{J_{\ell+1}} \dots \delta_{I_L}^{J_L} = \delta_{I_1}^{J_1} \dots \delta_{I_\ell I_{\ell+1}}^{J_\ell J_{\ell+1}} \dots \delta_{I_L}^{J_L} . \quad (5.17)$$

Because of the  $P_{\ell, \ell+1}$  and  $K_{\ell, \ell+1}$  there is operator mixing at the one-loop level.

Adding the one-loop correlator to the tree level correlator in (5.9) we get the expression

$$\begin{aligned} & \langle \mathcal{O}_{I_1, I_2, \dots, I_L}(x) \overline{\mathcal{O}}^{J_1, J_2, \dots, J_L}(y) \rangle = \\ & \frac{1}{|x-y|^{2L}} \left( 1 - \frac{\lambda}{16\pi^2} \ln(\Lambda^2|x-y|^2) \sum_{\ell=1}^L (C - 1 - 2P_{\ell, \ell+1} + K_{\ell, \ell+1}) \right) \delta^{j_1}_{i_1} \dots \delta^{j_L}_{i_L} \\ & \quad + \text{cycles} . \end{aligned} \quad (5.18)$$

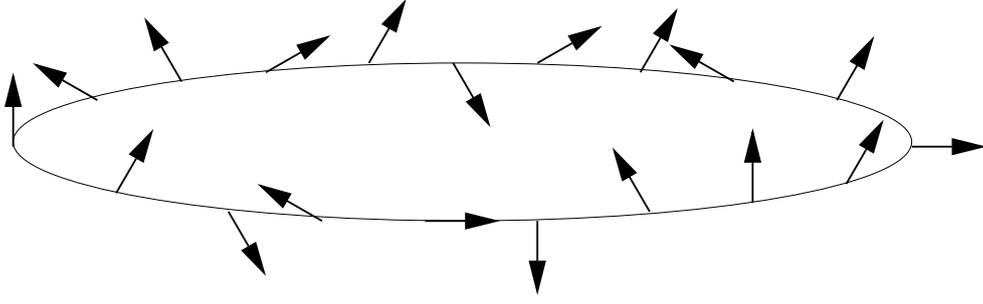

**Figure 4:** A spin-chain with  $SO(6)$  vector sites.

If we compare this result to (5.2), we see that because of the operator mixing the anomalous dimension  $\gamma$  should be replaced with an operator,  $\Gamma$ , where

$$\Gamma = \frac{\lambda}{16\pi^2} \sum_{\ell=1}^L (1 - C - 2P_{\ell,\ell+1} + K_{\ell,\ell+1}). \quad (5.19)$$

The possible one-loop anomalous dimensions are then found by diagonalizing  $\Gamma$ .

The entire class of scalar single trace operators of length  $L$  can be mapped to a Hilbert space which itself is a tensor product of finite dimensional Hilbert spaces

$$\mathcal{V}_1 \otimes \mathcal{V}_2 \cdots \otimes \mathcal{V}_\ell \otimes \cdots \otimes \mathcal{V}_L. \quad (5.20)$$

Each  $\mathcal{V}_\ell$  is the Hilbert space for an  $SO(6)$  vector representation, *i.e.*  $CP^5$ . The tensor product is the same Hilbert space as that of a one-dimensional spin-chain with  $L$  sites, where at each site there is an  $SO(6)$  vector “spin” (see figure 4). Because of the cyclicity property of the trace, we should include the further restriction that the Hilbert space be invariant under the shift

$$\mathcal{V}_1 \otimes \mathcal{V}_2 \cdots \otimes \mathcal{V}_\ell \otimes \cdots \otimes \mathcal{V}_L \rightarrow \mathcal{V}_L \otimes \mathcal{V}_1 \cdots \otimes \mathcal{V}_{\ell-1} \otimes \cdots \otimes \mathcal{V}_{L-1}. \quad (5.21)$$

The operator  $\Gamma$  in (5.19) acts linearly on this space:

$$\Gamma : \mathcal{V}_1 \otimes \mathcal{V}_2 \cdots \otimes \mathcal{V}_\ell \otimes \cdots \otimes \mathcal{V}_L \rightarrow \mathcal{V}_1 \otimes \mathcal{V}_2 \cdots \otimes \mathcal{V}_\ell \otimes \cdots \otimes \mathcal{V}_L. \quad (5.22)$$

Furthermore, it is Hermitian and commutes with the shift in (5.21). Thus, we can treat  $\Gamma$  as a Hamiltonian on the spin-chain. The energy eigenstates then correspond to the possible anomalous dimensions for the scalar operators. Since the Hamiltonian commutes with the shift, it is also consistent to project onto eigenstates that are invariant under the shift. Because  $P_{\ell,\ell+1}$  and  $K_{\ell,\ell+1}$  act on neighboring fields, the spin-chain Hamiltonian only has nearest neighbor interactions between the spins.

One particular eigenstate of  $\Gamma$  corresponds to the chiral primary  $\Psi_L$  in (5.3).  $\Psi_L$  is symmetric under the exchange of any field, hence  $P_{\ell,\ell+1}\Psi_L = \Psi_L$  for any  $\ell$ . Furthermore,  $\Psi_L$  has only  $Z$  fields and not  $\bar{Z}$  fields, thus  $K_{\ell,\ell+1}\Psi_L = 0$ . This generalizes to any chiral primary, which is in the  $L^{\text{th}}$  symmetric traceless representation of  $SO(6)$ . Therefore,

$$\Gamma \Psi_L = \frac{\lambda}{16\pi^2} \sum_{\ell=1}^L (1 - C - 2)\Psi_L \quad (5.23)$$

However, the dimension of  $\Psi_L$  is protected, meaning that its anomalous dimension is zero. Hence, we find that  $C = -1$  and  $\Gamma$  becomes [17]

$$\Gamma = \frac{\lambda}{8\pi^2} \sum_{\ell=1}^L \left( 1 - P_{\ell,\ell+1} + \frac{1}{2} K_{\ell,\ell+1} \right). \quad (5.24)$$

Another useful way to write  $\Gamma$  is in terms of projectors. The tensor product of two  $SO(6)$  vector representations is reducible into the traceless symmetric, the antisymmetric, and the singlet representations. The operators that project  $\mathcal{V}_\ell \otimes \mathcal{V}_{\ell+1}$  onto these three representations are

$$\Pi_{\ell,\ell+1}^{\text{sym}} = \frac{1}{2}(1 + P_{\ell,\ell+1}) - \frac{1}{6}K_{\ell,\ell+1}, \quad \Pi_{\ell,\ell+1}^{\text{as}} = \frac{1}{2}(1 - P_{\ell,\ell+1}), \quad \Pi_{\ell,\ell+1}^{\text{sing}} = \frac{1}{6}K_{\ell,\ell+1}. \quad (5.25)$$

We can then write  $\Gamma$  as

$$\Gamma = \frac{\lambda}{8\pi^2} \sum_{\ell=1}^L \left( 0 \Pi_{\ell,\ell+1}^{\text{sym}} + 2 \Pi_{\ell,\ell+1}^{\text{as}} + 3 \Pi_{\ell,\ell+1}^{\text{sing}} \right), \quad (5.26)$$

with only two of the three projectors contributing to  $\Gamma$ .

Although we will not show it here, the Hamiltonian that corresponds to  $\Gamma$  for the spin-chain is integrable [17]. There is a precise meaning for what this means which will be explained in later chapters of the review (see [18,19]). For us it means that the system is solvable, at least in principle. We will give a taste of this in the next section where we consider a certain subset of scalar operators.

Going beyond one-loop, one finds that the  $n$ -loop contribution to the anomalous dimension can involve up to  $n$  neighboring fields in an effective Hamiltonian [20] (see [21]). Therefore, as  $\lambda$  becomes larger these longer range interactions become more and more important, such that at strong coupling the spin-chain is effectively long range. In this case the Hamiltonian is not known above the first few loop orders [20,22].

## 6 One-loop generalization to all single trace operators

In this subsection we describe the generalization of  $\Gamma$  to all single trace operators. We do not give a derivation here, but instead refer the reader to the references.

In the general case the ‘‘spins’’ at each site of the chain are made up of the elements of the singleton representation enumerated in (4.9). The Hilbert space is then the tensor product in (4.11) projected onto states invariant under the shift in (4.13). The one-loop anomalous dimension is then described by a Hamiltonian with nearest neighbor interactions. Unlike the scalar case where the spins are in a finite dimensional representation, the singleton representation is infinite dimensional. However, there is still a beautiful way to write the Hamiltonian in terms of projectors [23,24].

The various  $PSU(2,2|4)$  representations can be expressed in terms of their highest weights which are given by the six charges of the  $PSU(2,2|4)$  Cartan subalgebra. The

singleton is then labeled by  $(1, 0, 0; 1, 0, 0)$ , where the highest weight in the representation belongs to the  $Z$  field. The Hamiltonian will involve the tensor product of two singleton representations which decomposes as

$$\mathcal{V} \otimes \mathcal{V} = \sum_{j=0}^{\infty} \mathcal{V}_j. \quad (6.1)$$

The first two representations in this decomposition are different from the others and have the highest weights

$$\mathcal{V}_0 : (2, 0, 0; 2, 0, 0) \quad \mathcal{V}_1 : (2, 0, 0; 1, 1, 0). \quad (6.2)$$

The other representations have highest weights

$$\mathcal{V}_j : (j, j - 2, j - 2; 0, 0, 0) \quad j \geq 2. \quad (6.3)$$

Notice that if we limit ourselves to scalar fields with no Lorentz charges then the only representations in play are  $\mathcal{V}_0$ ,  $\mathcal{V}_1$  and  $\mathcal{V}_2$ , whose decompositions under the  $SO(6)$  subgroup contain the symmetric traceless, the antisymmetric, and singlet representations respectively.

The Hamiltonian for the complete spin-chain has the compact form [23, 24]

$$\Gamma = \frac{\lambda}{8\pi^2} \sum_{\ell=1}^L \sum_{j=0}^{\infty} 2h(j) \Pi_{\ell, \ell+1}^{(j)}, \quad (6.4)$$

where  $\Pi_{\ell, \ell+1}^{(j)}$  projects  $\mathcal{V}_\ell \otimes \mathcal{V}_{\ell+1}$  onto  $\mathcal{V}_j$  and  $h(j)$  is the harmonic sum defined by<sup>9</sup>

$$h(j) \equiv \sum_{k=1}^j \frac{1}{k}. \quad (6.5)$$

Examining the expression for  $\Gamma$  in (5.26) we see that it has the form in (6.4) when only  $j = 0, 1, 2$  contribute.

## 7 Closed sectors

Since we have operator mixing, the alert reader could very well be concerned that scalar field operators will mix with operators that contain non-scalar fields. It turns out that generally this can happen, but not at the one-loop level.

Operator mixing preserves the total charges of the  $PSU(2, 2|4)$  symmetry group. This is because the anomalous dimension matrix is the dilatation operator  $D$  minus the bare dimension. To see why this matters consider the complete dilatation operator, which can be expressed as an expansion in  $\lambda$  of the form

$$D = \sum_{n=0}^{\infty} \lambda^n D^{(2n)}. \quad (7.1)$$

---

<sup>9</sup>In [25] Lipatov remarked that harmonic sums would appear in the anomalous dimension matrix for  $\mathcal{N} = 4$  SYM, leading him to predict that the theory would be solvable.

$D^{(0)}$  gives the bare dimension of the operator while  $D^{(2)}$  is the one-loop anomalous dimension operator  $\Gamma$  in (5.24) for scalar single trace operators or (6.4) for the most general single trace operators. The dilation operator commutes with the Lorentz generators and the  $R$ -symmetry generators. Since this is true for any value of  $\lambda$ , it must be true that all  $D^{(2n)}$  commute with these generators. Hence, the Lorentz and  $R$ -charges are preserved by the mixing. Furthermore, each of the  $D^{(2n)}$  commutes with  $D^{(0)}$ , which can be established by power counting in the graphs. Therefore, mixing only occurs between operators with the same  $R$ -charges, Lorentz charges, and bare dimensions.

We can use this information to show the existence of closed sectors. One such sector are operators made up of two types of scalar fields, say,  $Z$  and  $W$ , which have the charges  $(1, 0, 0; 1, 0, 0)$  and  $(1, 0, 0; 0, 1, 0)$  respectively. Hence, the total charges of a single trace operator made up of  $L - M$   $Z$  fields and  $M$   $W$  fields is  $(L, 0, 0; L - M, M, 0)$ . The mixing must preserve these charges and the only way to do this is to mix with operators having the same number of  $Z$  and  $W$  fields with possible rearrangements to their order, as one can verify by checking the charges for the other fields. This closed sector is called the  $SU(2)$  sector, since  $Z$  and  $W$  make up a doublet of an  $SU(2)$  subgroup of the  $R$ -symmetry group.

If we now include a third type of scalar field  $X$ , then the combination  $ZWX$  which has charges  $(3, 0, 0; 1, 1, 1)$  can mix with two fermions with individual charges  $(\frac{3}{2}, \frac{1}{2}, 0; \frac{1}{2}, \frac{1}{2}, \frac{1}{2})$  and  $(\frac{3}{2}, -\frac{1}{2}, 0; \frac{1}{2}, \frac{1}{2}, \frac{1}{2})$  but is otherwise closed [26]. This closed sector is the  $SU(2|3)$  sector containing an  $SU(3)$  subgroup of the  $R$ -symmetry and an  $SU(2)$  subgroup of the Lorentz group. The scalars make up a triplet of the  $SU(3)$  and are singlets under the  $SU(2)$  while the fermions are singlets under the  $SU(3)$  and make up a doublet of the  $SU(2)$ . Notice that this sort of mixing changes the number of fields in the trace. Such mixing is called dynamical [26].

We call the full set of scalar operators the  $SO(6)$  sector since the fields form a representation of the full  $R$ -symmetry group but are singlets under the Lorentz group. However, this cannot be a closed sector, since not even an  $SU(3)$  subsector is closed to mixing with fields with non-zero Lorentz charges. In fact, the  $SO(6)$  sector can mix into operators containing any one of the fields so the smallest closed sector containing  $SO(6)$  is the full  $PSU(2, 2|4)$ . However, the mixing outside of the  $SO(6)$  sector is dynamical, but dynamical mixing cannot occur until the two-loop level [26]. Hence the  $SO(6)$  sector is closed at one-loop.

Both  $SU(2)$  and  $SU(2|3)$  are compact groups and so the fields in these closed sectors are part of a finite dimensional representation of the group. There is another important closed sector where this is not the case. This is the  $SU(1, 1)$  sector (also called the  $SL(2)$  sector) [24]. In this sector we only have one type of scalar field, say  $Z$ , and covariant derivatives with one type of polarization, say  $\mathcal{D}_{++}$  which has charges  $(1, \frac{1}{2}, \frac{1}{2}; 0, 0, 0)$ . A typical single trace operator in this sector could have  $L$  scalar fields and  $M$  covariant derivatives. The mixing occurs by redistributing the  $M$  covariant derivatives among the  $L$  fields. Notice that this sector is nondynamical. Notice further that the fields fall into an infinite dimensional representation of  $SU(1, 1)$  since we can have an arbitrary number of covariant derivatives on any  $Z$  field. In fact the  $SU(1, 1)$  sector even appears in QCD [27] (see [28]).

## 8 The $SU(2)$ sector and the Heisenberg spin-chain

Let us now restrict our single trace operators to the  $SU(2)$  closed sector. The two independent fields transform under a doublet of  $SU(2)$ , hence we can label the  $Z$  field as spin up ( $\uparrow$ ) and the  $W$  field as spin down ( $\downarrow$ ). There is no contribution from  $K_{\ell,\ell+1}$  in (5.24) since the operators only have  $Z$  and  $W$  fields and not their conjugates. Thus, the  $SU(2)$  sector has the Hamiltonian

$$\Gamma_{SU(2)} = \frac{\lambda}{8\pi^2} \sum_{\ell=1}^L (1 - P_{\ell,\ell+1}). \quad (8.1)$$

In terms of spin operators the Hamiltonian can be rewritten as

$$\Gamma_{SU(2)} = \frac{\lambda}{8\pi^2} \sum_{\ell=1}^L \left( \frac{1}{2} - 2 \vec{S}_{\ell} \cdot \vec{S}_{\ell+1} \right). \quad (8.2)$$

Remarkably,  $\Gamma_{SU(2)}$  is the Hamiltonian of the Heisenberg spin-chain with  $L$  lattice sites. The total spin  $\vec{S} = \sum_{\ell} \vec{S}_{\ell}$  commutes with  $\Gamma$  so the energy eigenstates are simultaneously total spin eigenstates. This should not be surprising since we have already established that the dilatation operator commutes with the  $R$ -symmetry and the spin here is one of its subgroups.

Because of the sign of the  $\vec{S}_{\ell} \cdot \vec{S}_{\ell+1}$  term the spin-chain is ferromagnetic and the ground state has all spins aligned, with total spin  $L/2$ . This is the symmetric representation, which corresponds to the chiral primary operator. A quick check of the Hamiltonian in (8.2) shows that its energy is zero. The operators which are not chiral primaries correspond to excitations about the ground state. They have total spin that is less than  $L/2$ . A full description on how to find these other states is given in [17]. Here we give a partial description based on an  $S$ -matrix approach (see [18]).

Let us start with a ground state which we write as  $|\uparrow\uparrow\uparrow \dots \uparrow\uparrow\rangle$ . This corresponds to the chiral primary  $\Psi_L$  described in an earlier section. Let us now consider the states where one spin is down. In this case the Hamiltonian in (8.1) acts like a constant plus a hopping term, moving the down spin either one site to the left or the right. In particular, the action on a state with a down spin at a particular position  $\ell$  is

$$\begin{aligned} \Gamma_{SU(2)} |\uparrow \dots \uparrow \downarrow \uparrow \dots \uparrow\rangle \\ = \frac{\lambda}{8\pi^2} \left( 2 |\uparrow \dots \uparrow \downarrow \uparrow \dots \uparrow\rangle - |\uparrow \dots \downarrow \uparrow \uparrow \dots \uparrow\rangle - |\uparrow \dots \uparrow \uparrow \downarrow \dots \uparrow\rangle \right). \end{aligned} \quad (8.3)$$

From this it is easy to see that the eigenstates are

$$|p\rangle \equiv \frac{1}{\sqrt{L}} \sum_{\ell=1}^L e^{ip\ell} |\uparrow \dots \downarrow \dots \uparrow\rangle \quad (8.4)$$

where

$$\Gamma_{SU(2)} |p\rangle = \varepsilon(p) |p\rangle, \quad \varepsilon(p) = \frac{\lambda}{2\pi^2} \sin^2 \frac{p}{2}. \quad (8.5)$$

The state  $|p\rangle$  is called a single magnon state with momentum  $p$ . The dispersion is  $\varepsilon(p)$  and the magnon momentum  $p$  must be quantized so that the state is invariant under the shift  $\ell \rightarrow \ell + L$ , therefore  $p = 2\pi n/L$ . If  $n = 0$  then this is the symmetric state and so this has total spin  $L/2$ . All other cases have total spin  $L/2 - 1$ . This is fine for an ordinary spin chain, but we must remember that our states need to be invariant under the shift  $\ell \rightarrow \ell + 1$  since the single trace operators are invariant if we shift all fields over by one position. Hence, the only allowed state is the  $p = 0$  state and we find no operators that are not chiral primaries with only a single  $W$  field.

The first nontrivial case occurs with two down spins, since here it will be possible to satisfy the trace condition but not be in the symmetric representation. We will construct these states using an argument that goes back to Yang and Yang [29]. Instead of a closed chain of length  $L$  let us suppose we have a chain of infinite length. Consider the unnormalized two magnon state

$$|p_1, p_2\rangle = \sum_{\ell_1 < \ell_2} e^{ip_1\ell_1 + ip_2\ell_2} |\dots \downarrow^{\ell_1} \dots \downarrow^{\ell_2} \dots\rangle + e^{i\phi} \sum_{\ell_1 > \ell_2} e^{ip_1\ell_1 + ip_2\ell_2} |\dots \downarrow^{\ell_2} \dots \downarrow^{\ell_1} \dots\rangle, \quad (8.6)$$

where we assume that  $p_1 > p_2$ . We can think of  $|p_1, p_2\rangle$  as the scattering state for two magnons. The first term is the incoming part while the second term is the outgoing part. The phase  $e^{i\phi}$  is then the  $S$ -matrix  $S_{12}$  for the scattering. It is clear that if  $|p_1, p_2\rangle$  is to be an eigenstate of  $\Gamma_{SU(2)}$  then the eigenvalue will be the sum of the eigenvalues of two single magnon states with magnon momenta  $p_1$  and  $p_2$  respectively, since for  $|\ell_1 - \ell_2| \gg 1$  the two magnons cannot be interacting with each other. The subtlety occurs when the two down spins are next to each other, because the Hamiltonian cannot hop a down spin on top of another down spin. However, by adjusting the phase  $e^{i\phi}$  we can ensure that  $|p_1, p_2\rangle$  is an eigenstate. If we concentrate on all the ways the Hamiltonian puts the two down spins next to each other at sites  $\ell$  and  $\ell + 1$  we find that in order to have an eigenstate we must satisfy the equation

$$\begin{aligned} e^{ip_2} (2 - e^{-ip_1} - e^{ip_2}) + e^{ip_1} (2 - e^{ip_1} - e^{-ip_2}) e^{i\phi} \\ = (4 - e^{-ip_1} - e^{ip_1} - e^{-ip_2} - e^{ip_2}) (e^{ip_2} + e^{ip_1} e^{i\phi}), \end{aligned} \quad (8.7)$$

which has the solution

$$e^{i\phi} = S_{12} = -\frac{e^{ip_1 + ip_2} - 2e^{ip_2} + 1}{e^{ip_1 + ip_2} - 2e^{ip_1} + 1} \quad (8.8)$$

Now let us put the two magnons back on a cyclic spin chain of length  $L$ . The trace condition enforces the total momentum to be  $p_1 + p_2 = 0$ . The quantization condition for  $p_1$  works as follows. If we transport the magnon once around the circle the state is invariant. However, the transport brings the first magnon past the second one, so it also picks up a phase  $e^{i\phi}$ . Hence we have that  $e^{ip_1 L} e^{i\phi} = 1$ . With  $p_2 = -p_1$  we readily see that  $e^{i\phi} = e^{-ip_1}$ . Thus the allowed values for  $p_1$  are  $p_1 = 2\pi n/(L - 1)$  and the possible eigenvalues for the two magnon state are

$$\gamma = \frac{\lambda}{\pi^2} \sin^2 \frac{\pi n}{L - 1}.$$

The case where  $n = 0$  is the symmetric state with spin  $L/2$ . All other choices have spin  $L/2 - 2$ .

To go even further, it is convenient to define the rapidity variable  $u$ , where  $e^{ip} = \frac{u+i/2}{u-i/2}$ . The dispersion relation is then

$$\varepsilon(u) = \frac{\lambda}{8\pi^2} \frac{1}{u^2 + 1/4}, \quad (8.9)$$

while the  $S$ -matrix in (8.8) for magnons with rapidity variables  $u_j$  and  $u_k$  is

$$S_{jk} = \frac{u_j - u_k - i}{u_j - u_k + i}. \quad (8.10)$$

For  $M$  magnons one then sets up a state

$$|p_1, p_2, \dots, p_M\rangle = \sum_{\ell_1 < \ell_2 < \dots < \ell_M} e^{ip_1\ell_1 + ip_2\ell_2 + \dots + ip_M\ell_M} |\dots \downarrow^{\ell_1} \dots \downarrow^{\ell_2} \dots \dots \downarrow^{\ell_M} \dots\rangle + \dots \quad (8.11)$$

with  $p_1 > p_2 > \dots > p_M$  and where the last set of dots refers to the other possible orderings for the magnons, with appropriate phase factors. One can show that the phase factors are products of the two-particle  $S$ -matrices, which makes the system integrable. Putting the magnons on a circle with  $L$  sites we then find the quantization condition for the  $j^{\text{th}}$  magnon

$$\left(\frac{u_j + i/2}{u_j - i/2}\right)^L = \prod_{k \neq j}^M \frac{u_j - u_k + i}{u_j - u_k - i}. \quad (8.12)$$

The energy of the state is

$$\gamma = \sum_{j=1}^M \varepsilon(u_j), \quad (8.13)$$

where  $\varepsilon(u_j)$  is given by (8.9). The trace condition for the total momentum is

$$\prod_{j=1}^M \frac{u_j + i/2}{u_j - i/2} = 1 \quad (8.14)$$

The equations in (8.12) were first derived by Bethe many years ago [30] and are called the Bethe equations for the Heisenberg spin chain. Further solutions to these equations can be found in [17, 31]. Their generalization to other sectors including the full  $PSU(2, 2|4)$  long-range spin chain [32] are discussed in [33]

**Acknowledgments:** This work was supported in part by Vetenskapsrådet.

## References

- [1] N. Beisert et al., “*Review of AdS/CFT Integrability: An Overview*”, [arxiv:1012.3982](https://arxiv.org/abs/1012.3982).

- [2] J. A. Minahan, “*A Brief Introduction to the Bethe Ansatz in  $\mathcal{N} = 4$  Super- Yang-Mills*”, J. Phys. A39, 12657 (2006).
- [3] L. Brink, J. H. Schwarz and J. Scherk, “*Supersymmetric Yang-Mills Theories*”, Nucl. Phys. B121, 77 (1977).
- [4] M. F. Sohnius and P. C. West, “*Conformal Invariance in  $\mathcal{N} = 4$  Supersymmetric Yang-Mills Theory*”, Phys. Lett. B100, 245 (1981).
- [5] M. B. Green, J. H. Schwarz and L. Brink, “ *$\mathcal{N} = 4$  Yang-Mills and  $\mathcal{N} = 8$  Supergravity as Limits of String Theories*”, Nucl. Phys. B198, 474 (1982).
- [6] J. M. Maldacena, “*The large  $N$  limit of superconformal field theories and supergravity*”, Adv. Theor. Math. Phys. 2, 231 (1998), hep-th/9711200. • S. S. Gubser, I. R. Klebanov and A. M. Polyakov, “*Gauge theory correlators from non-critical string theory*”, Phys. Lett. B428, 105 (1998), hep-th/9802109. • E. Witten, “*Anti-de Sitter space and holography*”, Adv. Theor. Math. Phys. 2, 253 (1998), hep-th/9802150.
- [7] C. Montonen and D. I. Olive, “*Magnetic Monopoles as Gauge Particles?*”, Phys. Lett. B72, 117 (1977). • H. Osborn, “*Topological Charges for  $\mathcal{N} = 4$  Supersymmetric Gauge Theories and Monopoles of Spin 1*”, Phys. Lett. B83, 321 (1979). • L. Girardello, A. Giveon, M. Porrati and A. Zaffaroni, “*S Duality in  $\mathcal{N} = 4$  Yang-Mills Theories with General Gauge Groups*”, Nucl. Phys. B448, 127 (1995), hep-th/9502057. • C. Vafa and E. Witten, “*A Strong Coupling Test of S Duality*”, Nucl. Phys. B431, 3 (1994), hep-th/9408074.
- [8] D. J. Gross and F. Wilczek, “*Asymptotically Free Gauge Theories. 1*”, Phys. Rev. D8, 3633 (1973).
- [9] M. T. Grisaru, M. Roček and W. Siegel, “*Zero Three Loop Beta Function in  $\mathcal{N} = 4$  Superyang-Mills Theory*”, Phys. Rev. Lett. 45, 1063 (1980).
- [10] S. Mandelstam, “*Light Cone Superspace and the Ultraviolet Finiteness of the  $\mathcal{N} = 4$  Model*”, Nucl. Phys. B213, 149 (1983). • L. Brink, O. Lindgren and B. E. W. Nilsson, “*The Ultraviolet Finiteness of the  $\mathcal{N} = 4$  Yang-Mills Theory*”, Phys. Lett. B123, 323 (1983).
- [11] N. Beisert, “*Review of AdS/CFT Integrability, Chapter VI.1: Superconformal Algebra*”, arxiv:1012.4004.
- [12] M. Günaydin and C. Saclioglu, “*Oscillator Like Unitary Representations of Noncompact Groups with a Jordan Structure and the Noncompact Groups of Supergravity*”, Commun. Math. Phys. 87, 159 (1982). • M. Günaydin and N. Marcus, “*The Spectrum of the  $S^5$  Compactification of the Chiral  $\mathcal{N} = 2, D=10$  Supergravity and the Unitary Supermultiplets of  $U(2, 2/4)$* ”, Class. Quant. Grav. 2, L11 (1985).
- [13] M. Günaydin, D. Minic and M. Zagermann, “*4D Doubleton Conformal Theories, CPT and II B String on  $AdS_5 \times S^5$* ”, Nucl. Phys. B534, 96 (1998), hep-th/9806042.
- [14] M. Günaydin, D. Minic and M. Zagermann, “*Novel Supermultiplets of  $SU(2,2-4)$  and the  $AdS_5/CFT(4)$  Duality*”, Nucl. Phys. B544, 737 (1999), hep-th/9810226.
- [15] J. M. Drummond, “*Review of AdS/CFT Integrability, Chapter V.2: Dual Superconformal Symmetry*”, arxiv:1012.4002.
- [16] S. Ferrara, C. Fronsdal and A. Zaffaroni, “*On  $\mathcal{N} = 8$  Supergravity on  $AdS_5$  and  $\mathcal{N} = 4$  Superconformal Yang-Mills Theory*”, Nucl. Phys. B532, 153 (1998), hep-th/9802203.

- [17] J. A. Minahan and K. Zarembo, “*The Bethe-ansatz for  $\mathcal{N} = 4$  super Yang-Mills*”, JHEP 0303, 013 (2003), [hep-th/0212208](#).
- [18] M. Staudacher, “*Review of AdS/CFT Integrability, Chapter III.1: Bethe Ansatz and the R-Matrix Formalism*”, [arxiv:1012.3990](#). • C. Ahn and R. I. Nepomechie, “*Review of AdS/CFT Integrability, Chapter III.2: Exact world-sheet S-matrix*”, [arxiv:1012.3991](#).
- [19] A. Torrielli, “*Review of AdS/CFT Integrability, Chapter VI.2: Yangian Algebra*”, [arxiv:1012.4005](#).
- [20] N. Beisert, C. Kristjansen and M. Staudacher, “*The dilatation operator of  $\mathcal{N} = 4$  conformal super Yang-Mills theory*”, Nucl. Phys. B664, 131 (2003), [hep-th/0303060](#). • N. Beisert, “*The Dilatation Operator of  $\mathcal{N} = 4$  Super Yang-Mills Theory and Integrability*”, Phys. Rept. 405, 1 (2005), [hep-th/0407277](#).
- [21] C. Sieg, “*Review of AdS/CFT Integrability, Chapter I.2: The spectrum from perturbative gauge theory*”, [arxiv:1012.3984](#).
- [22] C. Sieg, “*Superspace computation of the three-loop dilatation operator of  $\mathcal{N} = 4$  SYM theory*”, [arxiv:1008.3351](#).
- [23] N. Beisert, “*The complete one-loop dilatation operator of  $\mathcal{N} = 4$  super Yang-Mills theory*”, Nucl. Phys. B676, 3 (2004), [hep-th/0307015](#).
- [24] N. Beisert and M. Staudacher, “*The  $\mathcal{N} = 4$  SYM Integrable Super Spin Chain*”, Nucl. Phys. B670, 439 (2003), [hep-th/0307042](#).
- [25] L. N. Lipatov, “*Evolution Equations in QCD*”, Prepared for ICTP Conference on Perspectives in Hadronic Physics, Trieste, Italy, 12-16 May 1997.
- [26] N. Beisert, “*The  $su(2|3)$  dynamic spin chain*”, Nucl. Phys. B682, 487 (2004), [hep-th/0310252](#).
- [27] L. N. Lipatov, “*High-Energy Asymptotics of Multicolor QCD and Exactly Solvable Lattice Models*”, [hep-th/9311037](#). • L. D. Faddeev and G. P. Korchemsky, “*High-Energy QCD as a Completely Integrable Model*”, Phys. Lett. B342, 311 (1995), [hep-th/9404173](#).
- [28] G. Korchemsky, “*Review of AdS/CFT Integrability, Chapter IV.4: Integrability in QCD and  $\mathcal{N} < 4$  SYM*”, [arxiv:1012.4000](#).
- [29] C. N. Yang and C. P. Yang, “*One-Dimensional Chain of Anisotropic Spin-Spin Interactions. I: Proof of Bethe’s Hypothesis for Ground State in a Finite System*”, Phys. Rev. 150, 321 (1966).
- [30] H. Bethe, “*On the Theory of Metals. 1. Eigenvalues and Eigenfunctions for the Linear Atomic Chain*”, Z. Phys. 71, 205 (1931).
- [31] N. Beisert, J. A. Minahan, M. Staudacher and K. Zarembo, “*Stringing spins and spinning strings*”, JHEP 0309, 010 (2003), [hep-th/0306139](#). • N. Beisert, S. Frolov, M. Staudacher and A. A. Tseytlin, “*Precision Spectroscopy of AdS/CFT*”, JHEP 0310, 037 (2003), [hep-th/0308117](#).
- [32] N. Beisert and M. Staudacher, “*Long-range PSU(2,2|4) Bethe ansatz for gauge theory and strings*”, Nucl. Phys. B727, 1 (2005), [hep-th/0504190](#).
- [33] A. Rej, “*Review of AdS/CFT Integrability, Chapter I.3: Long-range spin chains*”, [arxiv:1012.3985](#). • S. Schäfer-Nameki, “*Review of AdS/CFT Integrability, Chapter*

Chapter I.1: Spin Chains in  $\mathcal{N} = 4$  Super Yang-Mills

*II.4: The Spectral Curve*, [arxiv:1012.3989](#). • P. Vieira and D. Volin, “*Review of AdS/CFT Integrability, Chapter III.3: The dressing factor*”, [arxiv:1012.3992](#).



# Review of AdS/CFT Integrability, Chapter I.2: The spectrum from perturbative gauge theory

C. SIEG

*Institut für Mathematik und Institut für Physik, Humboldt-Universität zu Berlin  
Johann von Neumann Haus, Rudower Chaussee 25, 12489 Berlin, Germany*

*Niels Bohr International Academy, Niels Bohr Institute  
Blegdamsvej 17, 2100 Copenhagen, Denmark*

csieg@math.hu-berlin.de

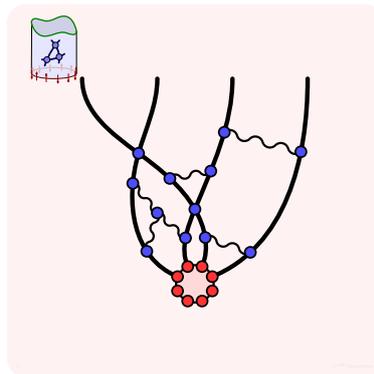

**Abstract:** We review the constructions and tests of the dilatation operator and of the spectrum of composite operators in the flavour  $SU(2)$  subsector of  $\mathcal{N} = 4$  SYM in the planar limit by explicit Feynman graph calculations with emphasis on analyses beyond one loop. From four loops on, the dilatation operator determines the spectrum only in the asymptotic regime, i.e. to a loop order which is strictly smaller than the number of elementary fields of the composite operators. We review also the calculations which take a first step beyond this limitation by including the leading wrapping corrections.

# 1 Introduction

In the context of the AdS/CFT correspondence [1], the discovery of integrability is a key ingredient towards finding the exact spectrum of strings in  $\text{AdS}_5 \times \text{S}^5$  and of composite operators in  $\mathcal{N} = 4$  SYM theory with gauge group  $SU(N)$  in the planar limit, i.e. for  $N \rightarrow \infty$ . As reviewed in chapters [II.1] and [II.2], on the string side of the duality the spectrum is accessible order by order as a strong coupling expansion in terms of the 't Hooft coupling by a (semi)classical analysis of string states with large quantized charges. It is also described in terms of respective string Bethe ansätze which are reviewed in chapter [III.1].

In the  $\mathcal{N} = 4$  SYM theory, the weak coupling expansion of the planar spectrum, i.e. the conformal dimensions of composite operators, can be obtained by direct perturbative calculations of various correlation functions. The appearance of UV divergences requires renormalization, which then leads to a mixing among operators with the same bare conformal dimension. The eigenvalues of the new eigenstates under conformal rescalings are given as the sum of the bare scaling dimension and an individual anomalous dimension. The operator mixing can be extracted, e.g. from the correlation functions involving two composite operators. Alternatively, one can directly calculate the diagrams which contribute to the renormalization of these operators. This directly allows one to obtain an expression for the dilatation operator, whose eigenvalues are the anomalous dimensions.

Perturbative calculations become very cumbersome at high loop orders and can be avoided, if the observed integrability at one loop, which is reviewed in chapter [I.1], also persists to higher loop orders. The dilatation operator can then be determined, using some very general structural information from the underlying Feynman graphs only and some data from the gauge Bethe ansätze. The details of this approach are reviewed in chapter [I.3]. Direct Feynman graph calculations of the dilatation operator in the flavour  $SU(2)$  subsector to three loops and of some of its eigenvalues and of parts of the Bethe ansätze also to higher loops provide important checks for the assumed integrability.

Even if integrability holds to all loop orders, the respective Bethe ansätze and planar dilatation operator allow us to compute the anomalous dimensions only in the asymptotic regime. In this regime, the loop order of the result is constrained to be strictly smaller than the length (the number of elementary fields) of the shortest composite operator involved. At loop orders which are equal to or exceed this number, the so-called wrapping interactions [2,3] have to be considered. They are corrections due to the finite size of the composite operators and have their origin in the neglected higher genus contributions to the dilatation operator [4]. In the dual string theory the counterparts of the wrapping interactions are corrections due to the finite circumference of the closed string worldsheet cylinder [5]. Their analyses are reviewed in chapters [III.5] and [III.6].

In this chapter we review the explicit Feynman graph calculations in  $\mathcal{N} = 4$  SYM theory in the planar limit beyond one loop. It is organized as follows:

In Section 2 we give a short summary of how composite operators are renormalized, and how the dilatation operator is defined in terms of the renormalization constants.

In Section 3 we then review the explicit calculations and tests of the dilatation oper-

ator with particular focus on calculations beyond the first order in perturbation theory.<sup>1</sup> Only the flavour  $SU(2)$  subsector will be considered, since most higher loop calculations are performed within this subsector. As examples we recalculate in detail the respective one- and two-loop dilatation operator in  $\mathcal{N} = 1$  superfield formalism. This approach is much more efficient than the originally used formalism without manifest supersymmetries, and it yields more direct relations between the dilatation operator and the underlying Feynman graphs. We then display the result of a three-loop calculation and also summarize the existing checks of the magnon dispersion relation, of the structure of the dilatation operator and of some of its eigenvalues in the asymptotic regime at three and higher loops.

In Section 4, we review the perturbative calculations which consider the first wrapping corrections and hence yield results beyond the asymptotic regime. The general strategy of these calculations will be explained. In this way, the four-loop anomalous dimension for the length four Konishi descendant in the flavour  $SU(2)$  subsector could be determined. Further results for different operators and for the terms of highest transcendentality are then summarized briefly.

In Section 5 we give a concluding summary, and in two appendices we present the explicit D-algebra manipulations for the one- and two-loop calculation and the expressions for the relevant integrals.

## 2 Renormalization of composite operators

The dilatation operator and anomalous dimensions can be obtained from a perturbative calculation of the correlation functions which involve the composite operators  $\mathcal{O}_a$ , where  $a$  labels the different operators. The encountered UV divergences require a renormalization of the composite operators as

$$\mathcal{O}_{a,\text{ren}}(\phi_{i,\text{ren}}) = \mathcal{Z}_a^b(\lambda, \varepsilon) \mathcal{O}_{b,\text{bare}}(\phi_{i,\text{bare}}), \quad \phi_{i,\text{ren}} = \mathcal{Z}_i^{1/2} \phi_{i,\text{bare}}, \quad (2.1)$$

where in an appropriate basis  $\mathcal{Z} = \mathbf{1} + \delta\mathcal{Z}$ , and the matrix  $\delta\mathcal{Z}$  is of order  $\mathcal{O}(\lambda)$  in the renormalized coupling constant  $\lambda$ . It also depends on the regulator  $\varepsilon$  and is in general non-diagonal and thus leads to mixing between the different composite operators. The matrix element  $\delta\mathcal{Z}_a^b$  is given by the negative of the sum of the overall UV divergences of the Feynman diagrams in which the vertices of the theory lead to interactions between the elementary fields of operator  $\mathcal{O}_b$ , such that the resulting external field flavour and ordering coincide with the ones of the operator  $\mathcal{O}_a$ . One also has to consider contributions from wave function renormalization of the elementary fields  $\phi_i$  the operators are composed of. Respective factors  $\mathcal{Z}_i^{1/2}$  are included within  $\mathcal{Z}$ .

$\mathcal{N} = 4$  SYM theory can be regularized by supersymmetric dimensional reduction [6] in  $D = 4 - 2\varepsilon$  dimensions. The coupling constant  $g_{\text{YM}}$  is then accompanied by the 't Hooft mass  $\mu$  in the combination  $g_{\text{YM}}\mu^\varepsilon$  to restore the mass dimension of the loop integrals. Thereby,  $g_{\text{YM}}$  is not renormalized and hence itself does not depend on  $\mu$ , such that superconformal invariance is preserved. This was explicitly found to three loops by

---

<sup>1</sup>The one-loop results are reviewed in chapter [I.1].

computing the vanishing of the  $\beta$ -function in an  $\mathcal{N} = 1$  superfield formulation [7]. The finiteness of  $\mathcal{N} = 4$  SYM theory was then later shown to all orders [8]. A first argument was given in [9]. In particular, the self-energy of the superfields is finite, i.e.  $\mathcal{Z}_i^{1/2}$  is trivial.<sup>2</sup> In the planar limit, where the coupling constant is  $\lambda = g_{\text{YM}}^2 N$ , the dilatation operator is then extracted from the renormalization constant of the composite operators in (2.1) as

$$\mathcal{D} = \mu \frac{d}{d\mu} \ln \mathcal{Z}(\lambda \mu^{2\varepsilon}, \varepsilon) = \lim_{\varepsilon \rightarrow 0} \left[ 2\varepsilon \lambda \frac{d}{d\lambda} \ln \mathcal{Z}(\lambda, \varepsilon) \right]. \quad (2.2)$$

The logarithm of  $\mathcal{Z} = 1 + \delta\mathcal{Z}$  has to be understood as a formal series in powers of  $\delta\mathcal{Z}$ . All poles of higher order in  $\varepsilon$  must cancel in  $\ln \mathcal{Z}$ , such that it only contains simple  $\frac{1}{\varepsilon}$  poles. In effect, the above description extracts the coefficient of the  $\frac{1}{\varepsilon}$  pole of  $\mathcal{Z}$ , and at a given loop order  $K$  multiplies it by a factor  $2K$ . This then yields the dilatation operator as a power series

$$\mathcal{D} = \sum_{k \geq 1} g^{2k} \mathcal{D}_k, \quad g = \frac{\sqrt{\lambda}}{4\pi}, \quad (2.3)$$

where for later convenience we have absorbed powers of  $4\pi$  into the definition of a new coupling constant  $g$ .

### 3 Dilatation operator in the $SU(2)$ subsector

$\mathcal{N} = 4$  SYM theory contains six real scalar fields, four complex Weyl fermions and a gauge field that all transform in the adjoint representation of the gauge group  $SU(N)$ . In the following we denote these fields as component fields, since in a superspace formalism they appear as components of superfields. In order to build the  $\mathcal{N} = 1$  superfields, the real scalar component fields are complexified and combined together each with one fermion or with its complex conjugate into three chiral superfields  $\phi_i$ ,  $i = 1, 2, 3$  or respectively anti-chiral ones  $\bar{\phi}_i$ . The three field flavours are transformed into each other by an  $SU(3)$  subgroup of the  $SU(4)$  R-symmetry group. The remaining gauge field and fermions are combined together into an  $\mathcal{N} = 1$  vector superfield  $V$ . An explicit expression of the  $\mathcal{N} = 4$  SYM action in terms of  $\mathcal{N} = 1$  superfields and the respective Feynman rules in which the Wick rotation is included can be found, e.g. in [10]. The superspace conventions are as in [11], where also an introduction to the D-algebra is given. The latter is required to reduce the supergraphs, i.e. the Feynman diagrams in superspace, to ordinary spacetime objects that are located at a single point in the fermionic coordinates of superspace.

#### 3.1 Operator mixing in the $SU(2)$ subsector

In the following, we denote the three chiral field flavours of  $\mathcal{N} = 4$  SYM theory by  $\phi_i = (\phi, \psi, Z)$ . The flavour  $SU(2)$  subsector contains operators which are composed of only two different types of these fields, e.g.  $\phi$  and  $Z$ . Their color indices are all contracted

---

<sup>2</sup>This holds apart from gauge artefacts that are not relevant here.

with each other to yield a gauge invariant object. In general, the gauge contractions form several cycles, and one obtains a multi-trace operator. Such an operator is a normal-ordered product of single-trace operators, i.e. of operators each of which only contains a single cycle of gauge contractions.

Mixing only occurs between those operators that have the same numbers of both types of fields  $\phi$  and  $Z$ . Then, it suffices to consider operators which contain a number of fields  $\phi$  that does not exceed the number of fields  $Z$ , since the results for the remaining operators follow immediately by an exchange of the role of the two fields. Usually, the fields  $\phi$  are denoted as impurities which appear between fields of type  $Z$  within the traces over the gauge group. Furthermore, in the planar limit that we exclusively consider from now on,<sup>3</sup> the Feynman diagrams that alter the gauge trace structure of the composite operators are suppressed. The renormalization of multi-trace operators then follows immediately from the one of their single-trace constituents. We can therefore restrict the analysis to single-trace operators. In this case, the planar Feynman diagrams can only affect the ordering of the two different types of fields inside the single trace, but they cannot alter their multiplicities and in particular the length  $L$  of the composite operators that is defined as the total number of constituent fields. Flavour contractions cannot appear, since the composite operators of the  $SU(2)$  subsector do not contain the complex conjugate fields  $(\bar{\phi}, \bar{\psi}, \bar{Z})$ . The  $SU(2)$  subsector is closed under renormalization, at least perturbatively [12]. The operators

$$\text{tr}(Z^L), \quad \text{tr}(\phi Z^{L-1}) \quad (3.1)$$

which are the ground state and a state with a single impurity are protected and do not acquire anomalous dimensions. Operators which contain more than a single impurity  $\phi$  undergo non-trivial mixing.

Since the aforementioned operator mixing only occurs within subsets of single-trace operators that only differ by permutations of their field content, the renormalization constant  $\mathcal{Z}$  and hence also the dilatation operator  $\mathcal{D}$  can be expressed in terms of flavour permutations that act on the constituent fields of these composite operators. The flavour permutations themselves can be written as products of permutations acting on nearest neighbour sites. For composite operators of fixed length  $L$  they are given by [13]

$$\{a_1, \dots, a_n\} = \sum_{r=0}^{L-1} P_{a_1+r \ a_1+r+1} \cdots P_{a_n+r \ a_n+r+1} \quad (3.2)$$

and by the identity  $\{\}$  in flavour space that measures the length  $L$  of the composite operator it is applied to. The structures consider the insertion of the Feynman subdiagrams in which elementary fields interact at all possible positions within the single trace of the composite operator by the summation. Periodicity with period  $L$  is thereby understood. No other insertions have to be considered here, since in the planar limit the interactions have to occur between adjacent fields.

The permutation structures (3.2) admit a definition of the range of the interaction in flavour space obtained from their lists of arguments as

$$\kappa = \max_{a_1, \dots, a_n} - \min_{a_1, \dots, a_n} + 2. \quad (3.3)$$

---

<sup>3</sup>See chapter [IV.1] for a review concerning effects of non-planarity.

The range  $\kappa$  and hence also the possible arguments  $a_1, \dots, a_n$  of the permutation structures are subject to constraints from the underlying Feynman diagrams. In order to find the restrictions for those structures that can appear in the expression of the dilatation operator, we focus on Feynman diagrams in which the elementary interactions occur in a single region that is simply connected also when the composite operator is removed from the diagram. These diagrams may have overall UV divergences that contribute with simple  $\frac{1}{\varepsilon}$  poles to the renormalization constant  $\mathcal{Z}$  and hence according to (2.2) also to the dilatation operator. The remaining diagrams, in which the elementary interactions occur in several non simply-connected regions after the removal of the composite operator, cannot contribute with simple  $\frac{1}{\varepsilon}$  poles. Their calculation is only required if one wants to determine  $\mathcal{Z}$  itself completely, for example in order to check explicitly that in  $\ln \mathcal{Z}$  all higher order poles in  $\varepsilon$  cancel. Here, we will not consider them further and only focus on the diagrams that can contribute to the dilatation operator. The interaction range  $R$  of a diagram of the latter type is defined as the number of adjacent elementary fields of the composite operator that enter the single simply connected interaction region. It can only yield contributions with permutation structures (3.2) that obey the following conditions:

$$n \leq K, \quad \kappa \leq R, \quad R \leq K + 1, \quad (3.4)$$

where  $K$  denotes the number of loops inside the diagram. The first inequality considers that each nearest-neighbour permutation is associated with at least one loop. The second condition ensures that the range of the interaction in flavour space does not exceed the interaction range  $R$  of the Feynman diagram. In a third inequality  $R$  itself is bounded from above by the loop order, since each interaction between nearest neighbour fields of the composite operator generates at least one loop. We denote the diagrams that saturate this bound, i.e. the ones with interaction range  $R = K + 1$  as maximum range diagrams. Since the summation in (3.2) runs over all insertion points with periodicity  $L$ , the smallest integer entry can always be fixed, e.g. to 1 by shifting all  $a_i$  by a common integer. According to (3.4) the biggest integer can then be at most  $K$ . Further relations between the structures (3.2) can be found in [14]. The independent permutation structures which obey (3.4) then form a basis in which the  $K$ -loop dilatation operator can be written down.

The basis with elements (3.2) is not the best choice in order to express the result of an explicit Feynman diagram calculation, since the different flavour arrangements within a single Feynman diagram generate linear combinations of several permutation structures (3.2) with fixed relative coefficients. If, instead, the generated combinations themselves are used as basis elements, each Feynman diagram is associated with only one of them [15, 16]. The basis elements obtained from supergraphs are called chiral functions and are defined as

$$\chi(a_1, \dots, a_n) = \{a_1, \dots, a_n\} \Big|_{\mathbb{P} \rightarrow \mathbb{P} - \mathbb{1}}, \quad (3.5)$$

where  $\mathbb{P} \rightarrow \mathbb{P} - \mathbb{1}$  denotes a replacement of all permutations in (3.2) by the fixed combination of permutation and identity. The expansion of the resulting products yields  $\chi$  in terms of linear combinations of permutation structures. For each  $\chi$  we define the range of the interaction in flavour space by applying the definition (3.3) to its list of

arguments. The chiral functions capture the structure of the chiral and anti-chiral superfield lines of the underlying supergraphs. Hence, all supergraphs which only differ by the arrangement of the flavour-neutral vector fields generate contributions with the same chiral function. In particular, at loop order  $K$  the chiral functions  $\chi(a_1, \dots, a_n)$  with  $n = K$  are associated each with a single Feynman graph since they do not contain any vector fields. We denote the respective graphs as chiral graphs.

Except of the identity  $\chi() = \{\}$ , all chiral functions (3.5) yield zero when they are applied to one of the protected states in (3.1). The expression of the dilatation operator in terms of chiral functions should hence not explicitly depend on  $\chi()$ . We will come back to this statement at the end of Section 3.5.2.

### 3.2 One-loop dilatation operator

The one-loop calculation in the  $SU(2)$  subsector was addressed by Berenstein, Maldacena and Nastase in [17]. They used component fields to compute the term involving the permutation structure  $\{1\}$ , which permutes the flavour of two neighbouring fields. It is the maximum shuffling term at one loop, since it shifts the position of the impurity by the maximum number of one site at this loop order. Its generalization to higher loops will be discussed in Section 3.5.1. The remaining Feynman diagrams all contribute to the identity operation  $\{\}$  in flavour space and were not computed explicitly. Instead, their contribution was reconstructed from the fact that the eigenvalue for the ground state in (3.1) should be zero. Furthermore, the contributions in which two neighbouring impurities interact with each other were neglected.

Using  $\mathcal{N} = 1$  superfields instead of component fields for the one-loop calculation, only a single Feynman diagram contains a UV divergence and hence contributes to the renormalization constant in (2.1). It is evaluated as

$$\begin{array}{c} \cup \\ | \\ \cup \end{array} = +\lambda I_1 \chi(1) , \tag{3.6}$$

where the bold horizontal line represents the composite operator of arbitrary length  $L \geq 2$ , thereby omitting its  $L-2$  elementary field lines that do not participate in the local interaction. The D-algebra manipulations are trivial in this case as explicitly displayed in Appendix A. The resulting loop integral is given in Appendix B. The further one-loop diagram of gluon exchange is finite, and the one-loop wave function renormalization vanishes. This is different from their behaviour in component formalism, where they have to be considered. According to the description (2.2), the one-loop dilatation operator follows from (3.6) as

$$\mathcal{D}_1 = -2\chi(1) . \tag{3.7}$$

Including also the contributions to the trace operator in flavour space, which extends the result to the flavour  $SO(6)$  subsector,<sup>4</sup> the full one-loop calculation in component fields was performed in [18], and the result was recognized as the Hamiltonian of a respective integrable Heisenberg spin chain.

<sup>4</sup>The flavor  $SO(6)$  subsector is only closed to one loop.

|             | $R = 1$                                                                           | $R = 2$                                                                           | $R = 3$                                                                            |
|-------------|-----------------------------------------------------------------------------------|-----------------------------------------------------------------------------------|------------------------------------------------------------------------------------|
| $\chi()$    | 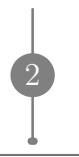 | 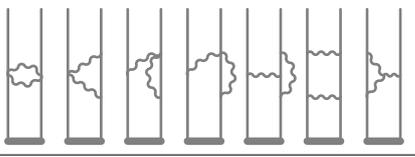 | 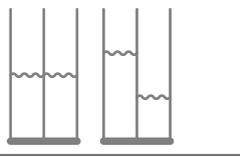 |
| $\chi(1)$   | —                                                                                 | 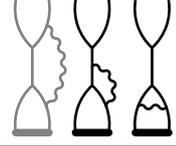 | 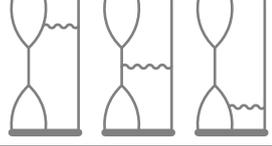 |
| $\chi(1,2)$ | —                                                                                 | —                                                                                 | 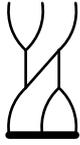 |

**Table 1:** Diagrams in  $\mathcal{N} = 1$  superfields (apart from eventual reflections) which can in principle contribute to the two-loop dilatation operator. Graphs which contain the vanishing one-loop self-energies are not drawn. It turns out that all diagrams depicted in gray are also irrelevant. The two-loop chiral self-energy is finite, and the remaining range  $R \geq 2$  diagrams are irrelevant due to generalized finiteness conditions [10].

### 3.3 Two-loop dilatation operator

A two-loop renormalization of composite operators in the  $SU(2)$  subsector was performed in [19] in component formalism. As in the one-loop case [17] only the diagrams which contribute to genuine flavour permutations were explicitly calculated, and the coefficient of the identity operation was determined by the condition of a vanishing eigenvalue of the ground state (3.1). Furthermore, the contributions in which impurities interact with each other were neglected.

The relevant diagrams for the complete two-loop calculation of the dilatation operator in terms of  $\mathcal{N} = 1$  superfields are given in Table 1. The chiral self-energy is identically zero at one loop and finite at higher loops. According to the generalized finiteness conditions derived in [10], all range  $R \geq 2$  diagrams, in which all vertices appear in loops are also finite. This concerns all remaining diagrams in the first line and in the second line the respective first diagram in the second and third columns. The pole parts of the last two diagrams in this line in the third column cancel against each other [15, 16]. This cancellation is based on the fact that, in order to obtain contributions with overall UV divergences, a sufficient number of spinor derivatives  $D_\alpha$  and  $\bar{D}_{\dot{\alpha}}$  has to remain inside the loops in order to be transformed into spacetime derivatives. This yields constraints on the D-algebra manipulations that amount to the formulation of generalized finiteness conditions in [10]. All diagrams that are irrelevant due to these conditions are depicted in gray. We only have to compute the remaining diagrams and consider also their reflections where necessary. The substructures in the relevant range  $R = 2$  diagrams with chiral function  $\chi(1)$  combine into the one-loop chiral vertex correction that is explicitly given

in (A.2). We then find

$$\begin{aligned}
 \text{Diagram 1} &= \text{Diagram 2} + \text{Diagram 3} + \text{Diagram 4} = -2\lambda^2 I_2 \chi(1) , & \text{Diagram 5} &= +\lambda^2 I_2 \chi(1, 2) , & (3.8)
 \end{aligned}$$

where we have to consider also the reflection of the last diagram which contributes with chiral function  $\chi(2, 1)$ . According to the description (2.2), the two-loop dilatation operator is then obtained by extracting the  $\frac{1}{\varepsilon}$  pole of the sum of these diagrams and multiplying it by  $-4$ . With the pole part of the respective integral  $I_2$  given in (B.4) this then yields

$$\mathcal{D}_2 = 4\chi(1) - 2[\chi(1, 2) + \chi(2, 1)] . \quad (3.9)$$

An explicit demonstration of the cancellation of the double poles in  $\ln \mathcal{Z}$  as mentioned after (2.2) can be found in [10], where the one- and two-loop calculations were presented as a demonstration for the efficiency of the used approach.

### 3.4 Three-loop dilatation operator

At three-loop order a calculation of the dilatation operator directly from Feynman graphs of  $\mathcal{N} = 1$  superfields was recently performed in [10]. The result reads

$$\begin{aligned}
 \mathcal{D}_3 &= -4(\chi(1, 2, 3) + \chi(3, 2, 1)) + 2(\chi(2, 1, 3) - \chi(1, 3, 2)) - 4\chi(1, 3) \\
 &\quad + 16(\chi(1, 2) + \chi(2, 1)) - 16\chi(1) - 4(\chi(1, 2, 1) + \chi(2, 1, 2)) . & (3.10)
 \end{aligned}$$

It determines the planar spectrum in the  $SU(2)$  subsector to three loops and hence goes beyond an earlier test of two eigenvalues [20], which employs Anselmi's trick [21] to reduce the calculation to two loops. The three-loop results confirm the prediction from integrability in [13]. Earlier checks of some of the three-loop eigenvalues are summarized in Section 3.5.3.

### 3.5 Partial tests at higher loops

To three-loop order and also beyond, certain parts of the respective Bethe ansatz and dilatation operator have been checked by direct Feynman diagram calculations. This concerns the so-called maximum shuffling terms, which contribute to the dispersion relation of the Bethe ansatz. Further terms in the higher loop expressions of the dilatation operator have also been tested explicitly.

#### 3.5.1 Tests of the magnon dispersion relation

Even if with the assumed integrability the  $SU(2)$  dilatation operator itself has been determined only to the first few loop orders (see chapter [I.3] for a review), the magnon dispersion relation of the Bethe ansatz is an all-order expression and directly related to certain Feynman diagrams. For a single magnon of momentum  $p$  it is given by [3]

$$E(p) = \sqrt{1 + 16g^2 \sin^2 \frac{p}{2}} - 1 , \quad (3.11)$$

and it is fixed by the underlying symmetry algebra up to an unknown function of the coupling constant [22], which in the  $\mathcal{N} = 4$  SYM case essentially appears to be given by  $g^2$  itself and has already been substituted accordingly.<sup>5</sup>

At a fixed loop order  $K$  in the expansion of the above relation, the momentum dependence can be expressed as linear combination of the elements  $\cos(k-1)p \sin^2 \frac{p}{2}$  with  $1 \leq k \leq K$ . In particular, the term with  $k = K$  is generated by the so-called maximum shuffling diagrams, which include shifts of the position of a single impurity (which is a magnon in the spin chain notation) by the maximum number of  $K$  neighbouring sites. The relevant diagrams are given by

$$\rightarrow \lambda^K I_K \chi(1, 2, \dots, K-1, K) \quad (3.12)$$

and by its reflection. When the sum of these two diagrams is applied to the eigenstate of a single magnon with momentum  $p$ , it yields the eigenvalue

$$\lambda^K I_K [\chi(1, 2, \dots, K) + \chi(K, \dots, 2, 1)] \rightarrow -8\lambda^K I_K \cos(K-1)p \sin^2 \frac{p}{2}. \quad (3.13)$$

According to the description (2.2), the  $\frac{1}{\epsilon}$  pole of this expression has to be multiplied by  $-2K$  to obtain its contribution to the magnon dispersion relation. A comparison with the respective term in the expansion of (3.11), thereby taking into account the relation (2.3) between the couplings, then makes a prediction for the  $\frac{1}{\epsilon}$  pole of the integral  $I_K$  as

$$\text{Res}_0(\text{KR}(I_K)) = \frac{1}{(4\pi)^{2K}} \frac{(2K-2)!}{(K-1)!K!} \frac{1}{K}. \quad (3.14)$$

The explicit expressions for the poles of  $I_K$  for some  $K$  are listed in (B.4). They are consistent with this result.

In [23] it was shown that at generic loop order the pole structure of the maximum shuffling diagrams in component fields is in accord with the BMN square root formula [17]. The latter was proposed as an all-order expression for the anomalous dimensions in the so-called BMN limit, where the length  $L$  of the operators and the coupling  $g$  become infinite  $L, g \rightarrow \infty$ , thereby keeping fixed the numbers of impurities inside the operators and also the effective coupling constant  $g' = \frac{g}{L}$ . For magnon momenta  $p_j = \frac{2\pi n_j}{L} \ll 1$  the dispersion relation (3.11) yields the individual contributions of each magnon  $j$  with mode number  $n_j$  to the BMN square root formula. Since the scattering of magnons is neglected, their momenta  $p_j$  assume a simple form and are solutions of the originally proposed Bethe equations [3] with a magnon S-matrix that becomes trivial in the BMN limit. However, these Bethe equations do not yield the anomalous dimensions of  $\mathcal{N} = 4$  SYM theory since the S-matrix is incomplete. One has to consider the so-called dressing phase [24] that first appeared at strong coupling [25] but is important also at weak coupling [24, 26], where it alters the magnon momenta at order  $\mathcal{O}(g^6)$ .<sup>6</sup> Due to the dressing phase, the

<sup>5</sup>The explicit Feynman diagram calculation in [10] confirms that this is correct to three loops. It is non-trivial in the AdS<sub>4</sub>/CFT<sub>3</sub> correspondence that is reviewed in chapter [IV.3].

<sup>6</sup>The dressing phase is reviewed in chapter [III.3].

S-matrix violates perturbative BMN scaling, i.e. its perturbative expansion diverges if after the replacement  $g \rightarrow g'L$  the limit  $L \rightarrow \infty$  is taken, thereby keeping  $g'$  fixed and small. The Bethe equations involving this S-matrix then yield anomalous dimensions that violate perturbative BMN scaling from four loops on. However, the BMN square root formula obeys this scaling, and hence it cannot describe the anomalous dimensions of operators with two or more impurities beyond three loops.<sup>7</sup> Since the dressing phase only affects the scattering of magnons, all tests and derivations of the BMN square root formula that rely on the calculation of phase shifts of a single magnon are insensitive to this failure and succeed. This concerns the previously mentioned all-order test of the maximum shuffling terms [23] and also an all order derivation employing the  $\mathcal{N} = 1$  superfield formalism [27]. It would be more appropriate to say that in these calculations the magnon dispersion relation in the BMN limit is obtained.

The magnon dispersion relation (3.11) describes the free propagation of one magnon. It is thus built up from all Feynman diagrams with chiral functions that do not yield a vanishing result when applied to the single magnon momentum eigenstate. The number of impurities of the composite operator sets an upper bound on the number of bubbles formed by two neighbouring lines of the composite operator inside the Feynman diagrams. Such a bubble appears for example in the lower right corner of the graph in (3.12), and it vanishes unless the two involved field flavours are different. The diagrams contributing to the magnon dispersion relation hence must not contain more than one of these bubbles. This restricts their chiral functions to  $\chi(1, \dots, k)$  and  $\chi(k, \dots, 1)$  after the identities for the permutation structures (3.2) found in [14] have been used to simplify the chiral functions, e.g. as  $\chi(1, 2, 1) = \chi(2, 1, 2) = \chi(1)$  in the three loop result (3.10). All-order expressions for the coefficients of these terms in the dilatation operator then follow directly from the magnon dispersion relation (3.11) and can be found in [10]. It should be stressed that the aforementioned contributions also yield non-vanishing results when additional magnons are present outside of the  $k + 1$  interacting legs. They therefore also contribute to the magnon S-matrix.

### 3.5.2 Tests of magnon scattering

The Feynman diagrams that vanish for a single magnon state, but are non-vanishing if two or more magnons are present within their respective interaction ranges, should exclusively be associated with the magnon S-matrix. Their contributions appear together with the ones of the aforementioned maximum and non-maximum shuffling terms in the dilatation operator. In the  $SU(2)$  subsector they first show up at three-loops as the contribution with chiral function  $\chi(1, 3)$  in (3.10).<sup>8</sup> The further chiral functions  $\chi(2, 1, 3)$ ,  $\chi(1, 3, 2)$  are also associated with magnon scattering, but they only appear in a combination that is associated with a similarity transformation, i.e. a change in the basis of operators [13, 14], that does not affect the eigenvalues.

As a more complicated example, we consider the four-loop dilatation operator. It

---

<sup>7</sup>This breakdown is independent of the general restriction of the Bethe ansatz to the asymptotic regime that requires a termination of the expansion at a loop order  $K \leq L - 1$  to avoid the wrapping corrections.

<sup>8</sup>A two-loop test of the S-matrix of the  $SL(2)$  subsector can be found in [28].

can be determined from the underlying integrability as reviewed in chapter [I.3]. In the basis of the chiral functions (3.5) it reads

$$\begin{aligned}
 \mathcal{D}_4 = & + 200\chi(1) - 150[\chi(1, 2) + \chi(2, 1)] + 8(10 + \epsilon_{3a})\chi(1, 3) - 4\chi(1, 4) \\
 & + 60[\chi(1, 2, 3) + \chi(3, 2, 1)] \\
 & + (8 + 2\beta + 4\epsilon_{3a} - 4i\epsilon_{3b} + 2i\epsilon_{3c} - 4i\epsilon_{3d})\chi(1, 3, 2) \\
 & + (8 + 2\beta + 4\epsilon_{3a} + 4i\epsilon_{3b} - 2i\epsilon_{3c} + 4i\epsilon_{3d})\chi(2, 1, 3) \\
 & - (4 + 4i\epsilon_{3b} + 2i\epsilon_{3c})[\chi(1, 2, 4) + \chi(1, 4, 3)] \\
 & - (4 - 4i\epsilon_{3b} - 2i\epsilon_{3c})[\chi(1, 3, 4) + \chi(2, 1, 4)] \\
 & - (12 + 2\beta + 4\epsilon_{3a})\chi(2, 1, 3, 2) \\
 & + (18 + 4\epsilon_{3a})[\chi(1, 3, 2, 4) + \chi(2, 1, 4, 3)] \\
 & - (8 + 2\epsilon_{3a} + 2i\epsilon_{3b})[\chi(1, 2, 4, 3) + \chi(1, 4, 3, 2)] \\
 & - (8 + 2\epsilon_{3a} - 2i\epsilon_{3b})[\chi(2, 1, 3, 4) + \chi(3, 2, 1, 4)] \\
 & - 10[\chi(1, 2, 3, 4) + \chi(4, 3, 2, 1)] .
 \end{aligned} \tag{3.15}$$

The coefficients  $\epsilon_i$ ,  $i = 3a, 3b, 3c, 3d$  in the above result are not fixed by the construction and parameterize the previously mentioned similarity transformations. The coefficient  $\beta$  is the leading term of the previously mentioned dressing phase. The magnon dispersion relation is encoded in the first two terms in the first line, the second line and the last line. The further contributions should be associated with magnon scattering. As the contributions from the maximum shuffling diagrams (3.12) in the last line, also the other terms in the last four lines have chiral functions that saturate all the bounds in (3.4). Hence, the underlying Feynman diagrams are chiral and of maximum range and their contributions can be calculated as easily as the one of the maximum shuffling terms (3.12).

The term in (3.15) with chiral function  $\chi(2, 1, 3, 2)$  only satisfies the first bound in (3.4), i.e. the underlying Feynman diagram is chiral but it is not of maximum range. It involves the leading coefficient  $\beta$  of the dressing phase, which can be determined from an evaluation of the respective diagram

$$\begin{array}{c} \text{Diagram} \end{array} \rightarrow \lambda^4 I_\beta \chi(2, 1, 3, 2) \tag{3.16}$$

if the coefficient  $\epsilon_{3a}$  of the similarity transformations is known. One finds  $\epsilon_{3a} = -4$  for example by computing the diagram which generates  $\chi(1, 3, 2, 4)$  or  $\chi(2, 1, 4, 3)$ . With the pole part of the integral  $I_\beta$  given in (B.5), the leading coefficient of the dressing phase is then determined as  $\beta = 4\zeta(3)$ . The result was obtained in [29], using component formalism. It agrees with one of the proposals in [24] and with the result extracted from a four-loop calculation of a four-point amplitude in [26].

It is also relatively easy to compute the terms with chiral functions which only saturate the second and third bound in (3.4), i.e. all terms in (3.15) with chiral functions that contain 1 and 4 in their lists of arguments and hence only stem from Feynman diagrams

of maximum range  $R = 5$ . This calculation was performed in [15, 16] in  $\mathcal{N} = 1$  superfield formalism in the context of calculating the first wrapping correction to be discussed below. The results yield an overdetermined system of equations that uniquely fixes the coefficients  $\epsilon_i$  and provides non-trivial checks of the remaining coefficients that are fixed by the underlying integrability. The analogous calculation of the  $R = 6$  diagrams at five loops can be found in [30].

The expressions (3.7), (3.9), (3.10) and (3.15) do not depend on the identity  $\chi()$ . This guarantees that the anomalous dimension of the BPS operators (3.1) are zero. The generalized finiteness conditions in [10] predict this to all orders and relate it to the finiteness of the chiral self-energy, i.e. to the preservation of conformal invariance.

### 3.5.3 Checks of eigenvalues

To three loops the results (3.7), (3.9) and (3.10) for the dilatation operator have been obtained by direct Feynman diagram calculations. At higher loops, only the terms that saturate at least one of the bounds in (3.4) have been tested as described above. Further checks concern the eigenvalues of the dilatation operator for some composite operators. They should match with the anomalous dimensions obtained in direct Feynman diagram calculations.

Of particular interest is thereby the Konishi supermultiplet. As superconformal primary it contains the  $\mathcal{N} = 1$  Konishi operator [31] that has bare scaling dimension  $\Delta_0 = 2$  and reads

$$\mathcal{K} = \text{tr} \left( e^{-g_{\text{YM}} V} \bar{\phi}_i e^{g_{\text{YM}} V} \phi^i \right). \quad (3.17)$$

This operator is not chiral, and hence all its superfield components lie beyond the  $SU(2)$  subsector. However, the Konishi supermultiplet also contains an operator of this subsector. In order to find it, one has to select the level four descendant of bare dimension  $\Delta_0 = 4$  that is chiral and pick out the relevant  $SU(4)$  R-symmetry component given by

$$\text{tr} \left( [\phi, Z] [\phi, Z] \right). \quad (3.18)$$

It contains as lowest superfield component the respective operator built out of the two scalar fields of the flavour  $SU(2)$  subsector.

All members of a superconformal multiplet acquire the same anomalous dimension. For the Konishi multiplet it is given to four loops in (4.1). The one- and two-loop contributions were obtained by explicit Feynman diagram calculations in [32] and [33], and then also by an OPE analysis in [34], see also [35]. These results are also found for a twist-two operator with conformal spin  $S = 2$  that appears within another level four descendant of the Konishi multiplet. It belongs to the closed  $SL(2)$  subsector that contains certain operators with general twist and conformal spin  $S$ . For twist-two operators with generic  $S$ , the result to two loops has been obtained from Feynman diagrams in [36]. At three loops it could be extracted [37] as the terms with highest transcendentality, i.e. with highest degrees of the harmonic sums, from the NNLO QCD result for the non-singlet splitting functions of QCD [38]. The truncation of the QCD result is based on the observation [39] that due to special properties of the DGLAP and BFKL equations in  $\mathcal{N} = 4$  SYM theory a mixing between functions of different transcendentality degrees does not

occur. Specializing to  $S = 2$ , the extracted result agrees with the three-loop contribution in (4.1). When the dilatation operator given in (3.7), (3.9) and (3.10) is applied to the state (3.18), it also correctly yields the result in (4.1).<sup>9</sup> In fact, the three-loop term was first predicted in [13], where the dilatation operator was constructed from integrability. Later, an explicit Feynman diagram calculation [20], which employs Anselmi's trick [21] to reduce the calculation to two loops, led to the same result. The calculation in [10] also confirms the result and furthermore fixes the planar three-loop spectrum of all composite single-trace operators of the flavour  $SU(2)$  subsector from field theory by a direct Feynman diagram calculation of the dilatation operator.

The previously mentioned twist-two operators of the  $SL(2)$  sector are very important for tests of the AdS/CFT correspondence and the underlying integrability. These tests are reviewed in chapter [III.4]. In particular, the results in the strict  $S \rightarrow \infty$  limit are not modified by wrapping interactions. At finite  $S$  such modifications occur. The simplest example is  $S = 2$ , i.e. the operator which appears in the Konishi multiplet. Its anomalous dimension is affected by wrapping interactions at four loops and beyond.

## 4 Wrapping interactions

In the following we briefly summarize the calculations of the previously mentioned wrapping interactions. A more detailed review is given by [40].

The Bethe ansätze or the dilatation operator yield reliable results for the anomalous dimensions in the asymptotic limit only. The origin and precise form of this restriction can be understood by recalling the construction from Feynman diagrams. In Section 3 it was argued that at a given loop order  $K$  the dilatation operator is determined from Feynman diagrams with range  $R \leq K + 1$ , which lead to flavour permutations with range  $\kappa \leq R$ . For the construction of the diagrams, it is thereby implicitly assumed that the length  $L$  of the involved composite operators is at least as big as the maximal interaction range  $K + 1$ . Therefore, an application of the dilatation operator to composite operators of length  $L$  can in general only yield the correct anomalous dimensions in the asymptotic limit, i.e. to a loop order  $K \leq L - 1$ . At  $K \geq L$  loops, the assumption of a sufficient length of the involved composite operators becomes invalid, and therefore contributions from diagrams with interaction range  $R > L$  should be removed from the dilatation operator. Instead, there are contributions from new diagrams that are built with the operators of the respective lower length  $L$ . The new diagrams are called wrapping diagrams since, due to the insufficient length of the composite operators, the interactions wrap around them. Two examples of such diagrams are depicted in Figure 1. Beyond the asymptotic limit, the dilatation operator explicitly depends on the length  $L$  of the composite operators it is applied to. More precisely, the coefficients of the chiral functions in the expression of the dilatation operator become functions of  $L$  at loop orders  $K \geq L$ , while in the asymptotic limit they are constants, and the dilatation operator depends on the length only via the permutation structures (3.2).

---

<sup>9</sup>At four and higher loops this is no longer the case since the wrapping interactions have to be considered. This will be discussed in Section 4.

The appearance of wrapping interactions is closely connected to the truncation of the genus  $h$  expansion of the dilatation operator beyond the planar  $h = 0$  contribution [4]. If in a planar wrapping diagram the composite operator is replaced by a longer operator, the additional fields lines cannot leave the diagram without crossing any other lines, i.e. it becomes a diagram of genus  $h = 1$ . The appearing wrapping diagrams hence come from certain genus  $h = 1$  contributions to the dilatation operator, which become planar when it is applied to a sufficiently short composite operator. Wrapping diagrams appear at all orders in the genus expansion of the dilatation operator. They are of genus  $h + 1$  in the asymptotic regime and encode the finite size effects at genus  $h$ . The planar wrapping diagrams are special since they can be projected out of all genus one contributions by introducing spectator fields [4]. While in general for higher genus diagrams the notion of the range of the interaction is not meaningful, it is still well defined for the subset of genus one diagrams when they become the planar wrapping diagrams. Integrability seems to persist, even if in general at higher genus its breakdown is expected [13].<sup>10</sup>

In order to obtain the anomalous dimensions beyond the asymptotic regime, one should not abandon the dilatation operator as obtained from the underlying integrability at loop orders  $K \geq 4$  and compute all Feynman diagrams. Instead, the considerations at the beginning of this section imply that the dilatation operator is still useful, since it can be corrected for an application to composite operators of shorter length  $L$ . First, at each loop order  $K$  all contributions from Feynman graphs of longer range  $K + 1 \geq R > L$  have to be removed. Then, contributions from the wrapping interactions have to be added.

This procedure is particularly powerful at the critical order  $K = L$  where wrapping arises for the first time, since only relatively few Feynman diagrams of restricted topology have to be computed explicitly. Most diagrams are captured automatically by those terms in the dilatation operator that are not removed in the modification process. Also, the only contributions that one has to remove from the dilatation operator are the ones that come from Feynman diagrams with maximum range  $R = K + 1$ . It is convenient to divide these diagrams according to their range of interaction in flavour space  $\kappa$  into two classes. The first class contains diagrams with  $\kappa = R = K + 1$ , i.e. according to the definition of  $\kappa$  in (3.3) their range  $R$  is encoded within the list of arguments of their chiral functions. The second class collects all the remaining diagrams with  $\kappa < R = K + 1$ . Such Feynman diagrams contain a chiral structure with interaction range  $\kappa$ , and the remaining  $R - \kappa$  neighbouring field lines are connected with it and with each other only by vector fields. Since the latter are flavour neutral, the range  $R$  of these diagrams is not captured by the chiral functions. It was shown in [16] in the  $\mathcal{N} = 1$  superfield formalism that the diagrams of the second class do not contribute to the dilatation operator: either they are finite or their overall UV divergences cancel against each other. This is also an implication of the generalized finiteness conditions derived in [10]. In Section 3.3 we have already used the results when we disregarded the two-loop diagrams with  $R = 3$  but  $\kappa < 3$  in the first two rows of the last column of Table 1. The diagrams of the first class that have  $\kappa = R = K + 1$  are the only maximum range diagrams that contribute with their overall UV divergences. These contributions can be easily identified and removed from the expression of the dilatation operator, since their chiral functions are of maximum

---

<sup>10</sup>In chapter [IV.1] the analyses of higher genus contributions are reviewed.

range. The subtraction procedure becomes almost trivial: one just has to remove all contributions with chiral functions that have 1 and  $K$  within their list of arguments. This does not require the calculation of any Feynman diagrams. For example, in the four-loop expression (3.15) one removes the last contribution in the first line and the ones in the fifth, sixth and the last four lines. The eigenvalues of the subtracted dilatation operator are no longer independent of the scheme coefficients  $\epsilon_i$ , which have to be fixed by calculating at least some of the diagrams with range  $R = K + 1$ . If one could compute the wrapping interactions that have to be added to the subtracted dilatation operator also as functions of  $\epsilon_i$ , the eigenvalues of the resulting operator should not depend on the  $\epsilon_i$ . However, the calculation of the wrapping interactions takes place in a scheme fixed by the use of  $\mathcal{N} = 1$  supergraphs, and therefore the  $\epsilon_i$  in the subtracted dilatation operator have to assume the respective values. Finally, it is important to remark that the simplicity of the subtraction procedure is only guaranteed if chiral functions (3.5) are used as basis elements. If, instead, the basis of permutation structures (3.2) is used, the subtraction of the contribution from a Feynman diagram with  $R = K + 1$  affects the coefficients of several permutation structures also with different flavour interaction ranges  $\kappa \leq R$  in the dilatation operator.<sup>11</sup>

The aforementioned method was first introduced and used in [15], with the details given in [16], in the case  $K = L = 4$ , i.e. for the four-loop anomalous dimension of the Konishi operator. In  $\mathcal{N} = 4$  SYM theory it is the simplest case where wrapping arises. The calculation starts from the four-loop asymptotic dilatation operator (3.15) and modifies it for an application to the length four Konishi descendant of the flavour  $SU(2)$  subsector (3.18) in order to determine the correct eigenvalue [15, 16]. Including also the lower orders, the anomalous dimension of the Konishi operator to four-loops was then determined as

$$\gamma = 12g^2 - 48g^4 + 336g^6 + (-2496 + 576\zeta(3) - 1440\zeta(5))g^8, \quad (4.1)$$

where the full conformal dimension is obtained as  $\Delta = \Delta_0 + \gamma$  with the bare scaling dimension  $\Delta_0$  as described in Section 3.5.3. The four-loop contribution has also been obtained from a generalized Lüscher formula [42]. This approach is reviewed in chapter [III.5]. Furthermore, it was later also found in a computer-based calculation in component formalism [43]. The matching of the Feynman diagram and Lüscher based calculations provides the first test of AdS/CFT and the underlying integrability beyond the asymptotic limit. It is also reproduced by the recently proposed  $Y$ -system [44], which is derived from the thermodynamic Bethe ansatz (TBA) [45] and is a candidate to capture the full planar spectrum of  $\mathcal{N} = 4$  SYM theory. The TBA and  $Y$ -system are reviewed, respectively, in chapters [III.6] and [III.7]. Earlier attempts to describe the wrapping effects in terms of integrable systems are included in chapter [I.3].

In [46] the result (4.1) which also holds for the earlier mentioned twist-two operator with conformal spin  $S = 2$  has been generalized to arbitrary  $S$ . When analytically continued to  $S = -1$ , it yields the correct pole structure as predicted from the BFKL equation.

---

<sup>11</sup>In the context of the BMN matrix model a subtraction attempt was made in [41]. It does not lead to the correct result, since the necessary modifications of the contributions with permutation structures of lower range and the addition of the wrapping diagrams was not performed.

A result for the five-loop anomalous dimension of the Konishi operator has been obtained in impressive calculations on the basis of the generalized Lüscher formula [47] and the TBA [48]. Also this result has been generalized to arbitrary spin  $S$ , and it is in accord with the pole structure from the BFKL equation [49]. To obtain the five-loop result for the Konishi multiplet from a Feynman diagram calculation is very difficult, even with the universal cancellation mechanisms discovered in [10]. Instead, a five-loop result for the  $L = 5$  operator  $\text{tr}([\phi, Z][\phi, Z]Z)$  which is in the same supermultiplet as certain twist-three operators has been computed [30], and it agrees with the result from the generalized Lüscher formula [50]. The six-loop results for the twist-three operators with generic conformal spin  $S$  has recently become available [51].

Beyond the asymptotic limit, the contributions of highest transcendentality, i.e. which contain the  $\zeta$ -function with biggest argument, are generated entirely by the wrapping interactions. In the four-loop result in (4.1) this is the term with  $\zeta(5)$ . Its generalization to twist-two operators with generic conformal spin  $S$  has been obtained from a Feynman diagram calculation in component formalism in [52]. At generic loop and critical wrapping order  $K = L$  the highest transcendentality degree of the wrapping diagrams is  $2K - 3$  compared to  $2K - 5$  of the dressing phase in the asymptotic Bethe ansatz. A clean setup that allows one to study the transcendentality structure without admixtures from the dressing phase is provided by single-impurity operators in the  $\beta$ -deformed  $\mathcal{N} = 4$  SYM theory.<sup>12</sup> The leading wrapping corrections have been calculated up to 11 loops in [53] and were confirmed in [54]. A clear pattern emerges also for the terms of lower transcendentality. The diagrams in Figure 1 are responsible for the highest transcen-

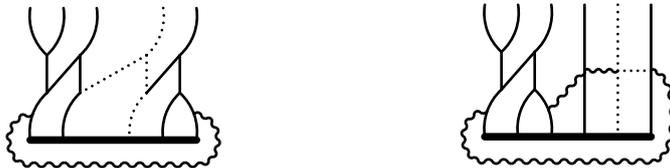

**Figure 1:** Wrapping diagrams that generate contributions of highest transcendentality at leading wrapping order.

dency contribution involving  $\zeta(2K - 3)$ . The respective term can be traced back to a component  $\frac{1}{2}P_K$  in the decomposition of the integrals, where  $P_K$  is the  $K$ -loop cake integral given in (B.6).

## 5 Conclusions

We have reviewed the explicit Feynman diagram calculations which at small 't Hooft coupling determine the planar spectrum of composite operators in the flavour  $SU(2)$  subsector of  $\mathcal{N} = 4$  SYM theory and test the underlying integrability. We have presented the calculations up to two loops in detail and summarized the calculations and partial checks at higher loops. The use of  $\mathcal{N} = 1$  superspace techniques and of chiral functions as operators in flavour space allowed us to directly interpret the Feynman diagrams in terms

<sup>12</sup>Among other deformations the  $\beta$ -deformation is reviewed in chapter [IV.2].

of the dispersion relation and the scattering matrix that appear in the integrability-based Bethe ansatz.

Then, we reviewed how anomalous dimensions beyond the asymptotic limit can be obtained by computing the leading wrapping corrections and which properties and interpretation these interactions have. The existing tests in these setups have been summarized.

## Acknowledgements

I am very grateful to Francesco Fiamberti and Alberto Santambrogio for reading parts of the manuscript. I also want to thank Francesco Fiamberti, Matias Leoni, Andrea Mauri, Joseph Minahan, Alberto Santambrogio, Olof Ohlsson Sax, Gabriele Tartaglino-Mazzucchelli, Alessandro Torielli and Daniela Zanon for very pleasant collaborations on some of the papers reviewed here and in other chapters of this review.

## A D-algebra

The propagators and vertices of superfields depend not only on the bosonic, but also on the fermionic coordinates  $\theta^\alpha, \bar{\theta}^{\dot{\alpha}}$ , of superspace and carry covariant spinor derivatives  $D_\alpha, \bar{D}_{\dot{\alpha}}$ . By the D-algebra manipulation which consists of transfers, partial integrations and the use of (anti)-commutation relations for products of these spinor derivatives, the underlying expression is transformed into the final result that is localized at a single point in the coordinates  $\theta^\alpha, \bar{\theta}^{\dot{\alpha}}$ . We refer the reader to [11] for an introduction to the  $\mathcal{N} = 1$  superfield formalism in the adopted conventions and to [10] for an explicit presentation of the relevant Feynman rules. Here, we only recall that two  $D_\alpha$  and two  $\bar{D}_{\dot{\alpha}}$  have to remain in each loop in order to obtain a non-vanishing result. The loop is then localized in the fermionic coordinates. We indicate this by filling it grey. Also, we recall two simple relations,  $D^2 \bar{D}^2 D^2 = \square D^2$  and  $\bar{D}^2 D^2 \bar{D}^2 = \square \bar{D}^2$ , which transform spinor derivatives into spacetime derivatives  $\square = \partial^\mu \partial_\mu$ .

The one-loop diagram (3.6) requires no D-algebra manipulations, and one directly obtains

$$\begin{array}{c}
 \begin{array}{c} \bar{D}^2 \quad \bar{D}^2 \\ \text{---} \quad \text{---} \\ \text{---} \quad \text{---} \\ \bar{D}^2 \quad \bar{D}^2 \end{array} \\
 = \\
 \begin{array}{c} \bar{D}^2 \quad \bar{D}^2 \\ \text{---} \quad \text{---} \\ \text{---} \quad \text{---} \\ \bar{D}^2 \quad \bar{D}^2 \end{array} \\
 \rightarrow -I_1,
 \end{array} \tag{A.1}$$

where the loop integral  $I_1$ , given in (B.2) for  $K = 1$ , is the one extracted from the grey-scaled region. Its UV pole is listed in (B.4). There appears an additional factor  $-1$  in front of  $I_1$ : we have to transform the full fermionic measure in the algebraic expression of

the diagram into the chiral measure of the term that adds the chiral composite operator with a chiral source to the action. This means, we replace  $d^4\theta \rightarrow d^2\bar{D}^2$  and combine the extra derivatives  $\bar{D}^2$  with the remaining  $D^2$  in the above diagram to  $\square$ , such that the propagator that connects the chiral and anti-chiral cubic vertex is cancelled, thereby yielding the factor  $-1$ . In the result we have not considered any other non-trivial prefactors of the propagators and vertices. They are contained within the color- and flavour factors (chiral functions) of the complete result given in (3.6).

The one-loop correction to the chiral vertex that enters (3.8) is easily evaluated

$$\begin{aligned}
 \text{Diagram} &= \bar{D}^2 \left( \text{Diagram 1} + \dots \right) = \left( \text{Diagram 2} + \dots \right) i\lambda g_{\text{YM}} \epsilon_{ijk} \text{tr} (T^a [T^b, T^c]) , \\
 & \tag{A.2}
 \end{aligned}$$

where the ellipsis denote the remaining two diagrams obtained by cyclic permutations of the external legs, and we have included the color and flavour factors. Also in this case, the  $\square$  is produced after reducing the full fermionic measure to the chiral measure as mentioned above. When  $\square$  cancels the propagator a factor  $-1$  is produced.

The D-algebra manipulations for the diagrams (3.8) contributing to the two-loop dilatation operator are

$$\begin{aligned}
 & \text{Diagram 1} \parallel \text{Diagram 2} + \text{Diagram 3} + \text{Diagram 4} = 2 \text{Diagram 5} \rightarrow 2I_2 , \\
 & \text{Diagram 6} \parallel \text{Diagram 7} \rightarrow I_2 , \\
 & \tag{A.3}
 \end{aligned}$$

where equalities hold up to disregarded finite contributions, and the final expressions in terms of the integral  $I_2$  consider the aforementioned factor  $-1$ .

## B Integrals

Using the scalar  $G$ -function defined as

$$G(\alpha, \beta) = \frac{\Gamma(\frac{D}{2} - \alpha)\Gamma(\frac{D}{2} - \beta)\Gamma(\alpha + \beta - \frac{D}{2})}{(4\pi)^{\frac{D}{2}}\Gamma(\alpha)\Gamma(\beta)\Gamma(D - \alpha - \beta)}, \quad (\text{B.1})$$

in  $D$ -dimensional Euclidean space, the following integrals can be found exactly to all loop orders

$$I_K = \begin{array}{c} \text{Diagram: A triangle with vertices 1, 2, 3. Vertex 1 is top-left, 2 is top-right, 3 is right. A curved line connects 1 and 2. A dashed line connects 3 and K-1. A solid line connects K and K-1.} \\ \text{Diagram: A triangle with vertices 1, 2, 3. Vertex 1 is top-left, 2 is top-right, 3 is right. A curved line connects 1 and 2. A dashed line connects 3 and K-1. A solid line connects K and K-1.} \end{array} = \prod_{k=0}^{K-1} G(1 - (\frac{D}{2} - 2)k, 1). \quad (\text{B.2})$$

They are logarithmically divergent in  $D = 4 - 2\varepsilon$  dimensions, and their overall UV divergence is obtained with the operations K to extract the pole part and R to subtract subdivergences as

$$\text{KR}(I_K) = \text{K} \left( I_K - \sum_{k=1}^{K-1} \text{KR}(I_k) I_{K-k} \right). \quad (\text{B.3})$$

To the first few loop orders, one finds

$$\begin{aligned} \text{KR}(I_1) &= \frac{1}{(4\pi)^2} \frac{1}{\varepsilon}, \\ \text{KR}(I_2) &= \frac{1}{(4\pi)^4} \left( -\frac{1}{2\varepsilon^2} + \frac{1}{2\varepsilon} \right), \\ \text{KR}(I_3) &= \frac{1}{(4\pi)^6} \left( \frac{1}{6\varepsilon^3} - \frac{1}{2\varepsilon^2} + \frac{2}{3\varepsilon} \right), \\ \text{KR}(I_4) &= \frac{1}{(4\pi)^8} \left( -\frac{1}{24\varepsilon^4} + \frac{1}{4\varepsilon^3} - \frac{19}{24\varepsilon^2} + \frac{5}{4\varepsilon} \right), \\ \text{KR}(I_5) &= \frac{1}{(4\pi)^{10}} \left( \frac{1}{120\varepsilon^5} - \frac{1}{12\varepsilon^4} + \frac{11}{24\varepsilon^3} - \frac{19}{12\varepsilon^2} + \frac{14}{5\varepsilon} \right), \\ \text{KR}(I_6) &= \frac{1}{(4\pi)^{12}} \left( -\frac{1}{720\varepsilon^6} + \frac{1}{48\varepsilon^5} - \frac{25}{144\varepsilon^4} + \frac{47}{48\varepsilon^3} - \frac{1313}{360\varepsilon^2} + \frac{7}{\varepsilon} \right). \end{aligned} \quad (\text{B.4})$$

The pole parts of the integrals that appear in the calculations of the four-loop dressing phase or of the wrapping interactions at critical wrapping order can very efficiently be computed by using a modified and extended version of the Gegenbauer polynomial  $x$ -space technique [55, 16]. The integral of the simplest contribution that allows us to determine the leading four-loop coefficient of the dressing phase reads

$$I_\beta = \begin{array}{c} \text{Diagram: A lens-shaped region bounded by two circular arcs meeting at two points.} \end{array}, \quad \text{KR}(I_\beta) = \frac{1}{(4\pi)^8} \left( -\frac{1}{12\varepsilon^4} + \frac{1}{3\varepsilon^3} - \frac{5}{12\varepsilon^2} - \frac{1}{\varepsilon} \left( \frac{1}{2} - \zeta(3) \right) \right). \quad (\text{B.5})$$

The terms of highest transcendentality from wrapping corrections at critical order are determined by the cake integral. This integral is logarithmically divergent for  $K \geq 3$

loops and reads

$$P_K = \kappa \left( \begin{array}{c} 1 \quad 2 \\ \diagdown \quad \diagup \\ \text{---} \quad \text{---} \\ \diagup \quad \diagdown \\ \kappa-1 \quad 4 \end{array} \right), \quad \mathbb{K}(P_K) = \frac{1}{(4\pi)^{2K}} \frac{1}{\varepsilon} \frac{2}{K} \binom{2K-3}{K-1} \zeta(2K-3), \quad (\text{B.6})$$

where the pole part has been obtained in [56] at generic loop order.

## References

- [I.1] J. Minahan, “*Review of AdS/CFT Integrability, Chapter I.1: Spin Chains in  $\mathcal{N} = 4$  SYM*”, [arxiv:1012.3983](#).
  - [I.3] A. Rej, “*Review of AdS/CFT Integrability, Chapter I.3: Long-range spin chains*”, [arxiv:1012.3985](#).
  - [II.1] A. Tseytlin, “*Review of AdS/CFT Integrability, Chapter II.1: Classical  $AdS_5 \times S^5$  string solutions*”, [arxiv:1012.3986](#).
  - [II.2] T. McLoughlin, “*Review of AdS/CFT Integrability, Chapter II.2: Quantum Strings in  $AdS_5 \times S^5$* ”, [arxiv:1012.3987](#).
  - [III.1] M. Staudacher, “*Review of AdS/CFT Integrability, Chapter III.1: Bethe Ansätze and the R-Matrix Formalism*”, [arxiv:1012.3990](#).
  - [III.3] P. Vieira and D. Volin, “*Review of AdS/CFT Integrability, Chapter III.3: The dressing factor*”, [arxiv:1012.3992](#).
  - [III.4] L. Freyhult, “*Review of AdS/CFT Integrability, Chapter III.4: Twist states and the cusp anomalous dimension*”, [arxiv:1012.3993](#).
  - [III.5] R. Janik, “*Review of AdS/CFT Integrability, Chapter III.5: Lüscher corrections*”, [arxiv:1012.3994](#).
  - [III.6] Z. Bajnok, “*Review of AdS/CFT Integrability, Chapter III.6: Thermodynamic Bethe Ansatz*”, [arxiv:1012.3995](#).
  - [III.7] V. Kazakov and N. Gromov, “*Review of AdS/CFT Integrability, Chapter III.7: Hirota Dynamics for Quantum Integrability*”, [arxiv:1012.3996](#).
  - [IV.1] C. Kristjansen, “*Review of AdS/CFT Integrability, Chapter IV.1: Aspects of Non-planarity*”, [arxiv:1012.3997](#).
  - [IV.2] K. Zoubos, “*Review of AdS/CFT Integrability, Chapter IV.2: Deformations, Orbifolds and Open Boundaries*”, [arxiv:1012.3998](#).
  - [IV.3] T. Klohe, “*Review of AdS/CFT Integrability, Chapter IV.3:  $\mathcal{N} = 6$  Chern-Simons and Strings on  $AdS_4 \times CP^3$* ”, [arxiv:1012.3999](#).
- [1] J. M. Maldacena, “*The large  $N$  limit of superconformal field theories and supergravity*”, *Adv. Theor. Math. Phys.* 2, 231 (1998), [hep-th/9711200](#). • S. S. Gubser, I. R. Klebanov and A. M. Polyakov, “*Gauge theory correlators from non-critical string theory*”, *Phys. Lett.* B428, 105 (1998), [hep-th/9802109](#). • E. Witten, “*Anti-de Sitter space and holography*”, *Adv. Theor. Math. Phys.* 2, 253 (1998), [hep-th/9802150](#).

- [2] D. Serban and M. Staudacher, “*Planar  $\mathcal{N} = 4$  gauge theory and the Inozemtsev long range spin chain*”, JHEP 0406, 001 (2004), [hep-th/0401057](#).
- [3] N. Beisert, V. Dippel and M. Staudacher, “*A novel long range spin chain and planar  $\mathcal{N} = 4$  super Yang-Mills*”, JHEP 0407, 075 (2004), [hep-th/0405001](#).
- [4] C. Sieg and A. Torrielli, “*Wrapping interactions and the genus expansion of the 2-point function of composite operators*”, Nucl. Phys. B723, 3 (2005), [hep-th/0505071](#).
- [5] J. Ambjorn, R. A. Janik and C. Kristjansen, “*Wrapping interactions and a new source of corrections to the spin-chain / string duality*”, Nucl. Phys. B736, 288 (2006), [hep-th/0510171](#).
- [6] W. Siegel, “*Supersymmetric Dimensional Regularization via Dimensional Reduction*”, Phys. Lett. B84, 193 (1979).
- [7] M. T. Grisaru, M. Rocek and W. Siegel, “*Superloops 3, beta 0: A Calculation in  $\mathcal{N} = 4$  Yang-Mills Theory*”, Nucl. Phys. B183, 141 (1981). • M. T. Grisaru, M. Rocek and W. Siegel, “*Zero Three Loop beta Function in  $\mathcal{N} = 4$  Superyang-Mills Theory*”, Phys. Rev. Lett. 45, 1063 (1980). • W. E. Caswell and D. Zanon, “*Vanishing Three Loop beta Function in  $\mathcal{N} = 4$  Supersymmetric Yang-Mills Theory*”, Phys. Lett. B100, 152 (1981). • W. E. Caswell and D. Zanon, “*Zero Three Loop beta Function in the  $\mathcal{N} = 4$  Supersymmetric Yang-Mills Theory*”, Nucl. Phys. B182, 125 (1981).
- [8] S. Mandelstam, “*Light Cone Superspace and the Ultraviolet Finiteness of the  $\mathcal{N} = 4$  Model*”, Nucl. Phys. B213, 149 (1983). • L. Brink, O. Lindgren and B. E. W. Nilsson, “*The Ultraviolet Finiteness of the  $\mathcal{N} = 4$  Yang-Mills Theory*”, Phys. Lett. B123, 323 (1983). • P. S. Howe, K. S. Stelle and P. K. Townsend, “*The Relaxed Hypermultiplet: An Unconstrained  $\mathcal{N} = 2$  Superfield Theory*”, Nucl. Phys. B214, 519 (1983). • P. S. Howe, K. S. Stelle and P. K. Townsend, “*Miraculous Ultraviolet Cancellations in Supersymmetry Made Manifest*”, Nucl. Phys. B236, 125 (1984).
- [9] S. Ferrara and B. Zumino, “*Supergauge Invariant Yang-Mills Theories*”, Nucl. Phys. B79, 413 (1974).
- [10] C. Sieg, “*Superspace calculation of the three-loop dilatation operator of  $\mathcal{N} = 4$  SYM theory*”, [arxiv:1008.3351](#).
- [11] S. J. Gates, M. T. Grisaru, M. Rocek and W. Siegel, “*Superspace, or one thousand and one lessons in supersymmetry*”, Front. Phys. 58, 1 (1983), [hep-th/0108200](#).
- [12] J. A. Minahan, “*The  $SU(2)$  sector in AdS/CFT*”, Fortsch. Phys. 53, 828 (2005), [hep-th/0503143](#).
- [13] N. Beisert, C. Kristjansen and M. Staudacher, “*The dilatation operator of  $\mathcal{N} = 4$  super Yang-Mills theory*”, Nucl. Phys. B664, 131 (2003), [hep-th/0303060](#).
- [14] N. Beisert and T. Klose, “*Long-range  $gl(n)$  integrable spin chains and plane-wave matrix theory*”, J. Stat. Mech. 0607, P006 (2006), [hep-th/0510124](#).
- [15] F. Fiamberti, A. Santambrogio, C. Sieg and D. Zanon, “*Wrapping at four loops in  $\mathcal{N} = 4$  SYM*”, Phys. Lett. B666, 100 (2008), [arxiv:0712.3522](#).

- [16] F. Fiamberti, A. Santambrogio, C. Sieg and D. Zanon, “*Anomalous dimension with wrapping at four loops in  $\mathcal{N} = 4$  SYM*”, Nucl. Phys. B805, 231 (2008), arxiv:0806.2095.
- [17] D. E. Berenstein, J. M. Maldacena and H. S. Nastase, “*Strings in flat space and pp waves from  $\mathcal{N} = 4$  super Yang Mills*”, JHEP 0204, 013 (2002), hep-th/0202021.
- [18] J. A. Minahan and K. Zarembo, “*The Bethe-ansatz for  $\mathcal{N} = 4$  super Yang-Mills*”, JHEP 0303, 013 (2003), hep-th/0212208.
- [19] D. J. Gross, A. Mikhailov and R. Roiban, “*A calculation of the plane wave string Hamiltonian from  $\mathcal{N} = 4$  super-Yang-Mills theory*”, JHEP 0305, 025 (2003), hep-th/0208231.
- [20] B. Eden, C. Jarczak and E. Sokatchev, “*A three-loop test of the dilatation operator in  $\mathcal{N} = 4$  SYM*”, Nucl. Phys. B712, 157 (2005), hep-th/0409009.
- [21] D. Anselmi, “*The  $\mathcal{N} = 4$  quantum conformal algebra*”, Nucl. Phys. B541, 369 (1999), hep-th/9809192.
- [22] N. Beisert, “*The  $su(2|2)$  dynamic  $S$ -matrix*”, Adv. Theor. Math. Phys. 12, 945 (2008), hep-th/0511082.
- [23] D. J. Gross, A. Mikhailov and R. Roiban, “*Operators with large  $R$  charge in  $\mathcal{N} = 4$  Yang-Mills theory*”, Annals Phys. 301, 31 (2002), hep-th/0205066.
- [24] N. Beisert, B. Eden and M. Staudacher, “*Transcendentality and crossing*”, J. Stat. Mech. 0701, P021 (2007), hep-th/0610251.
- [25] G. Arutyunov, S. Frolov and M. Staudacher, “*Bethe ansatz for quantum strings*”, JHEP 0410, 016 (2004), hep-th/0406256. • R. Hernandez and E. Lopez, “*Quantum corrections to the string Bethe ansatz*”, JHEP 0607, 004 (2006), hep-th/0603204.
- [26] Z. Bern, M. Czakon, L. J. Dixon, D. A. Kosower and V. A. Smirnov, “*The Four-Loop Planar Amplitude and Cusp Anomalous Dimension in Maximally Supersymmetric Yang-Mills Theory*”, Phys. Rev. D75, 085010 (2007), hep-th/0610248.
- [27] A. Santambrogio and D. Zanon, “*Exact anomalous dimensions of  $\mathcal{N} = 4$  Yang-Mills operators with large  $R$  charge*”, Phys. Lett. B545, 425 (2002), hep-th/0206079.
- [28] B. Eden, “*A two-loop test for the factorised  $S$ -matrix of planar  $\mathcal{N} = 4$* ”, Nucl. Phys. B738, 409 (2006), hep-th/0501234.
- [29] N. Beisert, T. McLoughlin and R. Roiban, “*The Four-Loop Dressing Phase of  $\mathcal{N} = 4$  SYM*”, Phys. Rev. D76, 046002 (2007), arxiv:0705.0321.
- [30] F. Fiamberti, A. Santambrogio and C. Sieg, “*Five-loop anomalous dimension at critical wrapping order in  $\mathcal{N} = 4$  SYM*”, arxiv:0908.0234.
- [31] K. Konishi, “*Anomalous Supersymmetry Transformation of Some Composite Operators in SQCD*”, Phys. Lett. B135, 439 (1984).
- [32] D. Anselmi, M. T. Grisaru and A. Johansen, “*A Critical Behaviour of Anomalous Currents, Electric- Magnetic Universality and  $CFT_4$* ”, Nucl. Phys. B491, 221 (1997), hep-th/9601023. • D. Anselmi, D. Z. Freedman, M. T. Grisaru and A. A. Johansen, “*Universality of the operator product expansions of  $SCFT(4)$* ”, Phys. Lett. B394, 329 (1997), hep-th/9608125.

- [33] M. Bianchi, S. Kovacs, G. Rossi and Y. S. Stanev, “*On the logarithmic behavior in  $\mathcal{N} = 4$  SYM theory*”, JHEP 9908, 020 (1999), [hep-th/9906188](#). • M. Bianchi, S. Kovacs, G. Rossi and Y. S. Stanev, “*Anomalous dimensions in  $\mathcal{N} = 4$  SYM theory at order  $g^{*4}$* ”, Nucl. Phys. B584, 216 (2000), [hep-th/0003203](#).
- [34] G. Arutyunov, B. Eden, A. C. Petkou and E. Sokatchev, “*Exceptional non-renormalization properties and OPE analysis of chiral four-point functions in  $\mathcal{N} = 4$  SYM(4)*”, Nucl. Phys. B620, 380 (2002), [hep-th/0103230](#).
- [35] M. Bianchi, S. Kovacs, G. Rossi and Y. S. Stanev, “*Properties of the Konishi multiplet in  $\mathcal{N} = 4$  SYM theory*”, JHEP 0105, 042 (2001), [hep-th/0104016](#).
- [36] A. V. Kotikov, L. N. Lipatov and V. N. Velizhanin, “*Anomalous dimensions of Wilson operators in  $\mathcal{N} = 4$  SYM theory*”, Phys. Lett. B557, 114 (2003), [hep-ph/0301021](#).
- [37] A. V. Kotikov, L. N. Lipatov, A. I. Onishchenko and V. N. Velizhanin, “*Three-loop universal anomalous dimension of the Wilson operators in  $\mathcal{N} = 4$  SUSY Yang-Mills model*”, Phys. Lett. B595, 521 (2004), [hep-th/0404092](#).
- [38] S. Moch, J. A. M. Vermaseren and A. Vogt, “*The three-loop splitting functions in QCD: The non-singlet case*”, Nucl. Phys. B688, 101 (2004), [hep-ph/0403192](#).
- [39] A. V. Kotikov and L. N. Lipatov, “*DGLAP and BFKL evolution equations in the  $\mathcal{N} = 4$  supersymmetric gauge theory*”, Nucl. Phys. B661, 19 (2003), [hep-ph/0208220](#).
- [40] F. Fiamberti, A. Santambrogio and C. Sieg, “*Superspace methods for the computation of wrapping effects in the standard and beta-deformed  $\mathcal{N} = 4$  SYM*”, [arxiv:1006.3475](#).
- [41] T. Fischbacher, T. Klose and J. Plefka, “*Planar plane-wave matrix theory at the four loop order: Integrability without BMN scaling*”, JHEP 0502, 039 (2005), [hep-th/0412331](#).
- [42] Z. Bajnok and R. A. Janik, “*Four-loop perturbative Konishi from strings and finite size effects for multiparticle states*”, Nucl. Phys. B807, 625 (2009), [arxiv:0807.0399](#).
- [43] V. N. Velizhanin, “*The Four-Loop Konishi in  $\mathcal{N} = 4$  SYM*”, [arxiv:0808.3832](#).
- [44] N. Gromov, V. Kazakov, A. Kozak and P. Vieira, “*Integrability for the Full Spectrum of Planar AdS/CFT II*”, [arxiv:0902.4458](#). • N. Gromov, V. Kazakov and P. Vieira, “*Exact Spectrum of Anomalous Dimensions of Planar  $\mathcal{N} = 4$  Supersymmetric Yang-Mills Theory*”, Phys. Rev. Lett. 103, 131601 (2009), [arxiv:0901.3753](#).
- [45] D. Bombardelli, D. Fioravanti and R. Tateo, “*Thermodynamic Bethe Ansatz for planar AdS/CFT: a proposal*”, J. Phys. A42, 375401 (2009), [arxiv:0902.3930](#). • G. Arutyunov and S. Frolov, “*On String S-matrix, Bound States and TBA*”, JHEP 0712, 024 (2007), [arxiv:0710.1568](#). • G. Arutyunov and S. Frolov, “*String hypothesis for the  $AdS_5 \times S^5$  mirror*”, JHEP 0903, 152 (2009), [arxiv:0901.1417](#).
- [46] Z. Bajnok, R. A. Janik and T. Lukowski, “*Four loop twist two, BFKL, wrapping and strings*”, Nucl. Phys. B816, 376 (2009), [arxiv:0811.4448](#).
- [47] Z. Bajnok, A. Hegedus, R. A. Janik and T. Lukowski, “*Five loop Konishi from AdS/CFT*”, Nucl. Phys. B827, 426 (2010), [arxiv:0906.4062](#).
- [48] G. Arutyunov, S. Frolov and R. Suzuki, “*Five-loop Konishi from the Mirror TBA*”, JHEP 1004, 069 (2010), [arxiv:1002.1711](#). • J. Balog and A. Hegedus, “*5-loop*

- Konishi from linearized TBA and the XXX magnet*”, JHEP 1006, 080 (2010), [arxiv:1002.4142](#).
- [49] T. Lukowski, A. Rej and V. N. Velizhanin, “*Five-Loop Anomalous Dimension of Twist-Two Operators*”, Nucl. Phys. B831, 105 (2010), [arxiv:0912.1624](#).
- [50] M. Beccaria, V. Forini, T. Lukowski and S. Zieme, “*Twist-three at five loops, Bethe Ansatz and wrapping*”, JHEP 0903, 129 (2009), [arxiv:0901.4864](#).
- [51] V. N. Velizhanin, “*Six-Loop Anomalous Dimension of Twist-Three Operators in  $\mathcal{N} = 4$  SYM*”, [arxiv:1003.4717](#).
- [52] V. N. Velizhanin, “*Leading transcendentality contributions to the four-loop universal anomalous dimension in  $\mathcal{N} = 4$  SYM*”, [arxiv:0811.0607](#).
- [53] F. Fiamberti, A. Santambrogio, C. Sieg and D. Zanon, “*Finite-size effects in the superconformal beta-deformed  $\mathcal{N} = 4$  SYM*”, JHEP 0808, 057 (2008), [arxiv:0806.2103](#). • F. Fiamberti, A. Santambrogio, C. Sieg and D. Zanon, “*Single impurity operators at critical wrapping order in the beta-deformed  $\mathcal{N} = 4$  SYM*”, JHEP 0908, 034 (2009), [arxiv:0811.4594](#).
- [54] M. Beccaria and G. F. De Angelis, “*On the wrapping correction to single magnon energy in twisted  $\mathcal{N}=4$  SYM*”, Int. J. Mod. Phys. A24 5803 (2009) [arxiv:0903.0778](#). • N. Gromov and F. Levkovich-Maslyuk, “*Y-system and beta-deformed  $\mathcal{N} = 4$  Super-Yang-Mills*”, [arxiv:1006.5438](#). • G. Arutyunov, M. de Leeuw and S. J. van Tongeren, “*Twisting the Mirror TBA*”, JHEP 1102 025 (2011), [arxiv:1009.4118](#).
- [55] K. G. Chetyrkin, A. L. Kataev and F. V. Tkachov, “*New Approach to Evaluation of Multiloop Feynman Integrals: The Gegenbauer Polynomial  $x$  Space Technique*”, Nucl. Phys. B174, 345 (1980). • A. V. Kotikov, “*The Gegenbauer Polynomial Technique: the evaluation of a class of Feynman diagrams*”, Phys. Lett. B375, 240 (1996), [hep-ph/9512270](#).
- [56] D. J. Broadhurst, “*Evaluation of a class of Feynman diagrams for all numbers of loops and dimensions*”, Phys. Lett. B164, 356 (1985).



# Review of AdS/CFT Integrability, Chapter I.3: Long-range spin chains

ADAM REJ

*Blackett Laboratory, Imperial College, London SW7 2AZ, U.K.*

a.rej@imperial.ac.uk

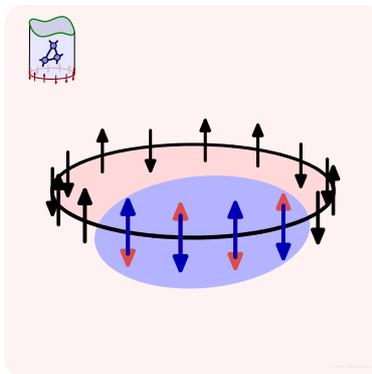

**Abstract:** In this contribution we review long-range integrable spin chains that originate from the recently discovered integrability in the planar AdS/CFT correspondence. We also briefly summarise the theory of generic integrable perturbatively long-range spin chains.

# 1 Introduction

The appearance of integrability in the planar AdS/CFT [1] is a rather unexpected occurrence. The unravelling of the integrable structures on the gauge theory side of the duality began with the ground-breaking work [2], where the one-loop dilatation operator in the  $\mathfrak{so}(6)$  sub-sector has been derived and identified with the Hamiltonian of an integrable  $\mathfrak{so}(6)$  spin chain. This was subsequently generalised to the full interaction sector of the theory  $\mathfrak{psu}(2, 2|4)$  in [3]. At one-loop order the dilatation operator is of the nearest-neighbour type and thus resembles Hamiltonians of other integrable spin chains. At higher orders in perturbation theory, however, this is not the case anymore. The first higher-loop corrections to the dilatation operator were first studied in the  $\mathfrak{su}(2)$  sub-sector, see [4], and the two-loop correction found therein has been shown to be integrable as well. Conjecturing the integrability to hold at higher loops and with help of further assumptions, also the three- and four-loop corrections have been found<sup>1</sup>. This has furnished first evidence that the integrability might be an all-loop feature of the dilatation operator of  $\mathcal{N} = 4$  SYM theory. The higher-rank sectors were first studied in [6], where the two- and three-loop corrections to the dilatation operator in the maximal compact sub-sector of the theory  $\mathfrak{su}(2|3)$  have been determined and their integrability has been verified. The generalisation to the full theory has turned out to be very intricate, nevertheless higher corrections for the non-compact  $\mathfrak{su}(1, 1|2)$  sub-sector have been derived in [7] and [8]. These developments were paralleled by the formulation of the corresponding one-loop and higher-loop Bethe ansätze, as well as a host of discoveries of integrable structures on the string theory side. Integrable structures have also been found in the context of the  $AdS_4/CFT_3$  and  $AdS_3/CFT_2$  correspondences. Please refer to other reviews of this series for further details and references.

The perturbative corrections to the dilatation operator have been found assuming that wrapping interactions may be neglected. These interactions wrap around the chain and thus account for highly non-local interactions between the spins. Since an interaction between two neighbouring spins contributes a factor  $\mathcal{O}(\lambda)$ , first wrapping interactions may in general appear at the order  $\mathcal{O}(\lambda^L)$ , where  $L$  is the length of the system. Please refer to [9] for further discussion of these non-local interactions. In what follows we will always assume that the order of perturbation theory  $\ell$  is smaller than the length of the system, i.e.  $\ell < L$ .

The higher-loop corrections to the dilatation operator exhibit *novel* features when compared with Hamiltonians of the vast majority of integrable spin chains. Firstly, the range of the interactions increases with the loop order. Secondly, beyond the one-loop level operators with the same classical dimension but different lengths are mixed together. The simplest example of such process furnishes the mixing of three scalar fields with two fermions

$$\text{tr} \left( \dots \underbrace{\mathcal{X}\mathcal{Y}\mathcal{Z}}_{\Delta_0=3, L=3} \dots \right) \leftrightarrow \text{tr} \left( \dots \underbrace{\mathcal{U}\mathcal{V}}_{\Delta_0=3, L=2} \dots \right). \quad (1.1)$$

Integrable long-range spin chains with these properties have not been hitherto inves-

<sup>1</sup>The four-loop contribution was only determined up to a single coefficient, which was then uniquely fixed in [5].

tigated. They should be distinguished from the long-range spin chains considered before in the literature, as they are defined as long-range deformations of nearest-neighbour models. There is a host of evidence that these unusual features do not hinder the integrability. This suggests that integrable perturbatively long-range spin chains should be well-defined and could constitute an interesting class of models not studied in the literature. The Inozemtsev model, see [10], an important intrinsically long-range spin chain and its connection to perturbatively long-range spin chains will be briefly discussed in section 4.3. Unless stated otherwise, throughout this review by long-range spin chains we will mean perturbative long-range spin chains.

The investigation of generic closed integrable long-range spin chains has been initiated in [11], where the underlying symmetry algebra was assumed to be  $\mathfrak{gl}(n)$ . It has been found that integrable long-range spin chains are characterised by four infinite families of parameters and thus span a very large class. However, it turns out that only two families of the parameters influence the Bethe equations. The two others correspond to rotations of the higher conserved charges and to similarity transformations. The latter do not influence the spectrum. These findings were subsequently generalised to arbitrary Lie (super)algebra in [12]. Moreover, a novel recursion relation has been proposed, which allows to lift an integrable nearest-neighbour spin chain to its long-range counterpart, see also [13]. This has laid solid foundations for the theory of perturbative long-range systems.

This review is structured as follows. In section 2 we will briefly discuss the perturbative corrections to the dilatation operator in the  $\mathfrak{su}(2)$  sub-sector of the planar  $\mathcal{N} = 4$  gauge theory. The higher-rank sectors  $\mathfrak{su}(2|3)$  and  $\mathfrak{su}(1, 1|2)$  are the subject of section 3. In section 4 we will review the general theory of perturbative long-range integrable spin chains. Finally, in section 5 we will explain an interesting relation between the Hubbard model and long-range spin chains. In this article we assume that the reader is familiar with the rudiments of integrable spin chains and their application to AdS/CFT correspondence presented in [14].

## 2 The $\mathfrak{su}(2)$ sub-sector

The  $\mathfrak{su}(2)$  sector is one of the simplest dynamical sectors. It has been proven in [4] that this sector is closed, i.e. there is no mixing with other types of the operators. It consists of two types of scalar  $\mathcal{X}$  and  $\mathcal{Z}$

$$\mathrm{tr} (\mathcal{X}^M \mathcal{Z}^{L-M}) + \dots \quad (2.1)$$

In the spin chain picture one identifies the  $\mathcal{X}$  fields with say up spins  $\uparrow$  and the  $\mathcal{Z}$  fields with down spins  $\downarrow$

$$\mathrm{tr} (\mathcal{X}^M \mathcal{Z}^{L-M}) + \dots \longleftrightarrow \underbrace{|\uparrow\uparrow \dots \uparrow}_{M} \underbrace{\downarrow\downarrow \dots \downarrow}_{L-M} + \dots \quad (2.2)$$

The cyclicity of the trace imposes closed periodic boundary conditions on the spin chain. Up to now this is merely a change in the notation. The advantage of the spin chain

reinterpretation becomes apparent when one considers the one-loop dilatation operator in this sector, which may be extracted from the one-loop  $\mathfrak{so}(6)$  dilatation operator found in [2] by restricting to the case of two scalar fields. Introducing the notation

$$\{n_1, n_2, \dots, n_l\} = \sum_{k=1}^L P_{k+n_1, k+n_1+1} P_{k+n_2, k+n_2+1} \dots P_{k+n_l, k+n_l+1}, \quad (2.3)$$

where  $P_{a,b}$  permutes the spins at site  $a$  and  $b$  in the chain, the one-loop dilatation operator may be written as

$$D_2 = 2(\{\} - \{0\}). \quad (2.4)$$

Thus  $D_2$  is proportional to the Hamiltonian of the  $XXX$  spin chain! The computation of higher-loop corrections with diagrammatic methods becomes very involved beyond the leading order. A novel method of determining the higher-loop corrections has been introduced in [4]. The authors have analysed and classified the two-loop Green functions corresponding to the operators (2.2). They have advocated that only certain types of interactions are permitted, which in the spin chain picture correspond to permutations of the neighbouring sites. Furthermore, it has been argued that at two-loop order only interactions permuting at most three consecutive spins are allowed. One can thus assume that a subclass of (2.3) consisting of all permutations of at most three nearest-neighbours span the basis for the two-loop dilatation operators  $D_4$ . The coefficients of the linear combinations may be fixed using additional constraints. The simplest one follows from the fact that the scaling dimension of the half-BPS operators  $\text{tr } \mathcal{Z}^L$  is protected and does not receive any radiative corrections. Consequently,

$$D_4(\text{tr } \mathcal{Z}^L) = 0, \quad (2.5)$$

for any  $L$ . Further constraints follow from the so-called BMN scaling. It has been argued in [15] that the  $\ell$ -loop anomalous dimension of the operators  $\text{tr } \mathcal{X}^M \mathcal{Z}^J$  should scale as

$$\gamma_{2\ell} \sim (\lambda')^\ell (1 + \mathcal{O}(1/J)), \quad \lambda' = \frac{g^2}{J^2}, \quad (2.6)$$

for  $M = \text{fixed}$  and  $J \rightarrow \infty$ . Moreover, the leading coefficient should match the string theory prediction

$$\Delta = J + \sum_{k=1}^M \sqrt{1 + 4\pi\lambda' n_k^2}. \quad (2.7)$$

The mode numbers  $n_k$  are subjected to the level matching condition  $\sum_{k=1}^M n_k = 0$ . While it is now known that BMN scaling *breaks down* at the four-loop order, see the discussion in [16], it has played a major role in the development of the subject. At the two-loop order these both requirements uniquely fix  $D_4$  to

$$D_4 = 2(-4\{\} + 6\{0\} - (\{0, 1\} + \{1, 0\})). \quad (2.8)$$

One of the very few manifestations of the integrability at the level of the spectrum are the so-called parity pairs, i.e. pairs of operators with opposite parity and equal energies.

Please see review by Charlotte Kristjansen [17] for the definition of parity and further discussion of parity pairs. The existence of such pairs hints at the presence of higher conserved charges which commute with the dilatation operator, but anticommute with the parity operator. At one-loop order the simplest of these charges is

$$Q_3^{(2)} = 4(\{1, 0\} - \{0, 1\}). \quad (2.9)$$

It should be stressed that it is rather a non-trivial task to find explicitly the higher conserved charges for an integrable spin chain. The situation is facilitated to a great extent if the so-called boost operator is known, see [18] and [19]. Interestingly, as argued in [20], the mere existence of  $Q^{(3)}$  seems to guarantee the existence of all higher charges.

The authors of [4] have discovered that the first higher charge may also be determined at the two-loop order such that  $[D(\lambda), Q_3(\lambda)] = 0$  holds up to  $\mathcal{O}(\lambda^3)$ , i.e.

$$\left[ D_4, Q_3^{(2)} \right] + \left[ D_2, Q_3^{(4)} \right] = 0. \quad (2.10)$$

This guarantees the degeneracy of the spectrum at two-loop order. It is thus plausible to assume that integrability will be present at higher loops. More generally, if the higher charges are determined to a given loop order  $\ell$  and commute with each other up to  $\mathcal{O}(\lambda^{\ell+1})$ , the system is said to be perturbatively integrable up to  $\ell$ -th order.

There is strong evidence that the  $\mathfrak{su}(2)$  sector is perturbatively integrable at least up to three-loop order. The three-loop dilatation operator may be again found [4] by imposing the degeneracy for the paired operators (i.e. imposing the presence of the parity pairs) in conjunction with the constraints discussed above

$$D_6 = 4(15\{\} - 26\{0\} + 6(\{0, 1\} + \{1, 0\}) + \{0, 2\} - (\{0, 1, 2\} + \{2, 1, 0\})). \quad (2.11)$$

Also the corresponding three-loop correction to the first higher charge satisfying the perturbative integrability condition at three-loop order may be found. The same set of conditions allowed to constrain the form of the four-loop correction to the dilatation operator up to two coefficients [4]. Moreover, it has been found that one of these unknowns does not affect the spectrum since it can be eliminated by a similarity transformation

$$D' = J(\lambda) D J(\lambda)^{-1}. \quad (2.12)$$

In [5] the remaining constant has been fixed by a more careful analysis of the implications of the BMN limit. This analysis has been further extended to the five-loop order in [21]. In [22] it has been argued that the BMN limit is sufficient to determine the all-loop two-spin interaction part of the dilatation operator. One should however note that it is *incorrect* to assume the BMN limit at and beyond four-loop order and the corrections found with help of this constraint need to be modified. It has been proposed in [23] to use instead the form of the one-magnon dispersion relation together with the two-magnon scattering matrix derived in [24]. This allowed to determine the four-loop correction up to an unknown constant  $\beta_{2,3}^{(4)}$  and parameters related to the similarity transformations, cf. (2.12). It turns out that the constant  $\beta_{2,3}^{(4)}$  multiplies a term with four permutations that reshuffle only four consecutive spins and thus may be determined by evaluating only

a sub-class of the Feynman diagrams. These diagrams have been calculated in [23] and the remaining coefficient could have been fixed to  $\beta_{2,3}^{(4)} = 4\zeta(3)$ . This is the first evidence of the so-called dressing phase introduced in section 4. For a discussion of the dressing factor of the AdS/CFT correspondence the reader should refer to the review by Pedro Vieira and Dmytro Volin [25].

### 3 Higher-rank sectors : $\mathfrak{su}(2|3)$ and $\mathfrak{su}(1, 1|2)$

In this section we will discuss higher-order corrections to the dilatation operator beyond the  $\mathfrak{su}(2)$  sub-sector. The novel feature, when compared with the previous case, is the central role played by the symmetry algebra. The higher-loop corrections to the symmetry generators are strongly constrained by the algebra relations

$$[J^A(\lambda), J^B(\lambda)] = f_C^{AB} J^C(\lambda). \quad (3.1)$$

The structure constants  $f_C^{AB}$  do not receive quantum corrections. In what follows we will discuss two particular examples:  $\mathfrak{su}(2|3)$  and  $\mathfrak{su}(1, 1|2)$  sub-sectors.

#### 3.1 The maximal compact sub-sector $\mathfrak{su}(2|3)$

The  $\mathfrak{su}(2|3)$  sector consists of three scalars and two fermionic fields and can be schematically represented by

$$\text{tr} (\mathcal{X}^{M_1} \mathcal{Y}^{M_2} \mathcal{U}^{M_3} \mathcal{V}^{M_4} \mathcal{Z}^{L-M}) + \dots, \quad (3.2)$$

where  $M = M_1 + M_2 + M_3 + M_4$ . Please note that in view of the mixing processes (1.1) the length  $L$  is not conserved beyond the one-loop order. A generic state of the  $\mathcal{N} = 4$  SYM theory is characterised by the classical dimension  $\Delta_0$ , the  $\mathfrak{su}(2)^2$  labels  $[s_1, s_2]$ , the  $\mathfrak{su}(4)$  Dynkin labels  $[q_1, p, q_2]$ , the  $\mathfrak{u}(1)$  hypercharge  $B$  and the length  $L$ . Please refer to [14] for details. The truncation to the  $\mathfrak{su}(2|3)$  sector is obtained by restricting to the states with

$$\Delta_0 = p + \frac{1}{2}q_1 + \frac{3}{2}q_2. \quad (3.3)$$

This also implies certain relations on some of the generators, see [6]. The full symmetry algebra  $\mathfrak{psu}(2, 2|4)$  thus effectively reduces to  $\mathfrak{su}(2|3)$ . It consists of the generators

$$J = \{L^\alpha_\beta, R^a_b, D, \delta D | Q^a_\alpha, S^a_\alpha\}. \quad (3.4)$$

The  $\mathfrak{su}(2)$  and  $\mathfrak{su}(3)$  generators  $L^\alpha_\beta$  and  $R^a_b$  are traceless. The corresponding commutation relations are as follows

$$[L^\alpha_\beta, J_\gamma] = \delta^\alpha_\gamma J_\beta - \frac{1}{2}\delta^\alpha_\beta J_\gamma, \quad [L^\alpha_\beta, J^\gamma] = -\delta^\gamma_\beta J^\alpha + \frac{1}{2}\delta^\alpha_\beta J^\gamma, \quad (3.5)$$

$$[R^a_b, J_c] = \delta^a_c J_b - \frac{1}{3}\delta^a_b J_c, \quad [R^a_b, J^c] = -\delta^c_b J^a + \frac{1}{3}\delta^a_b J^c. \quad (3.6)$$

The commutators of the dilatation operator and its anomalous part are given by

$$[D, J] = \text{eng}(J)J, \quad [\delta D, J] = 0, \quad (3.7)$$

with  $\text{eng}(Q) = -\text{eng}(S) = \frac{1}{2}$ . The supercharges  $Q^a_\alpha$  and  $S^a_\alpha$  anticommute <sup>2</sup>

$$\{S^a_\alpha, Q^b_\beta\} = \delta^b_a L^\alpha_\beta + \delta^\alpha_\beta R^b_a + \frac{1}{6} \delta^b_a \delta^\alpha_\beta (2D + \delta D). \quad (3.8)$$

The symmetry generators act on (3.2) by reshuffling the operators in the trace and changing the labels  $M_1, M_2, M_3, M_4$  and  $L$ . An interaction replacing the sequence of fields  $A_1, \dots, A_n$  within the state  $|C_1 \dots C_L\rangle = (-1)^{(C_1 \dots C_i)(C_{i+1} \dots C_L)} |C_{i+1} \dots C_L C_1 \dots C_i\rangle$  by  $B_1, \dots, B_m$  will be denoted as

$$\begin{aligned} & \left\{ \begin{matrix} A_1 \dots A_n \\ B_1 \dots B_m \end{matrix} \right\} |C_1 \dots C_L\rangle = \\ & \sum_{i=0}^{L-1} (-1)^{(C_1 \dots C_i)(C_{i+1} \dots C_L)} \delta_{C_{i+1}}^{A_1} \dots \delta_{C_{i+n}}^{A_n} |B_1 \dots B_m C_{i+n+1} \dots C_L C_1 \dots C_i\rangle. \end{aligned} \quad (3.9)$$

Here  $(-1)^{XY}$  equals  $-1$  if both  $X$  and  $Y$  are fermionic and  $+1$  otherwise.

The key observation of [6] is that the algebra relation (3.5)-(3.8) *largely* constrain the form of the generators. For example, at tree-level one expects the following general  $\mathfrak{su}(3) \times \mathfrak{su}(2)$  invariant form of the generators

$$R^a_b = c_1 \left\{ \begin{matrix} a \\ b \end{matrix} \right\} + c_2 \delta^a_b \left\{ \begin{matrix} c \\ c \end{matrix} \right\}, \quad (3.10)$$

$$L^\alpha_\beta = c_3 \left\{ \begin{matrix} \alpha \\ \beta \end{matrix} \right\} + c_4 \delta^\alpha_\beta \left\{ \begin{matrix} \gamma \\ \gamma \end{matrix} \right\}, \quad (3.11)$$

$$D_0 = c_5 \left\{ \begin{matrix} a \\ a \end{matrix} \right\} + c_6 \left\{ \begin{matrix} \alpha \\ \alpha \end{matrix} \right\}, \quad (3.12)$$

$$(Q_0)_\alpha^a = c_7 \left\{ \begin{matrix} a \\ \alpha \end{matrix} \right\}, \quad (3.13)$$

$$(S_0)_a^\alpha = c_8 \left\{ \begin{matrix} \alpha \\ a \end{matrix} \right\}. \quad (3.14)$$

Please note that the generators  $R^a_b$  and  $L^\alpha_\beta$  are not influenced by radiative corrections and the formulas (3.10) and (3.11) will be thus valid to all orders. The non-trivial solution to (3.5)-(3.8) is furnished by

$$c_1 = c_3 = c_5 = 1, \quad c_2 = -\frac{1}{3}, \quad c_4 = -\frac{1}{2}, \quad c_6 = \frac{3}{2}, \quad c_7 = e^{i\beta}, \quad c_8 = e^{-i\beta}. \quad (3.15)$$

Moreover, the parameter  $\beta$  corresponds to the similarity transformation

$$J_0 \rightarrow e^{2i\beta D_0} J_0 e^{-2i\beta D_0}. \quad (3.16)$$

Thus, the commutation relations allowed to unambiguously determine the form of the generators! A similar method has been applied in [6] to determine corrections to the generators  $Q$  and  $S$  up to the order  $\mathcal{O}(\lambda^2)$  and up to the order  $\mathcal{O}(\lambda^3)$  for the dilatation generator  $D$ . Please note that since the perturbative expansion of  $\delta D$  starts at  $\mathcal{O}(\lambda)$  and in view of (3.7) the  $k$ -th order contribution to  $\delta D$  may be constrained through the perturbative expansion of the remaining generators up to the order  $\mathcal{O}(\lambda^{(k-1)})$ . At higher orders, however, the relations (3.5)-(3.8) *do not* determine all physical coefficients and further assumptions must be made. Up to the three-loop order it is sufficient to

---

<sup>2</sup>The supersymmetry generator  $Q^a_\alpha$  should not be confused with the higher conserved charges  $Q_r$ . Even though the same symbol is used to denote both charges, it will become clear from the context which quantity is referred to.

exploit constraints following from the topology of the Feynman diagrams together with the absence of the radiative corrections for the half-BPS states and impose the BMN limit, see [6]. The two- and three-loop corrections to the dilatation operator found in this way preserve the maximum amount of parity pairs and the dilatation operator was conjectured to be perturbatively integrable up to three-loop order [6]. The next conserved charge  $Q_3$  has been constructed in [26] up to the order  $\mathcal{O}(\lambda^2)$ .

In [27] it has been proposed how to reformulate the description of the  $\mathfrak{su}(2|3)$  spin-chain in order to eliminate the length-changing processes (1.1). The underlying idea is to “freeze out” the dynamic effects by choosing one of the bosonic fields, say  $\phi^3 := \mathcal{Z}$  as the background field. The other fields in the sector are then redefined as follows

$$\{\phi^1, \phi^2, \psi^1, \psi^2\} \ni \mathcal{F} \mapsto \mathcal{F}_n := \mathcal{F} \underbrace{\mathcal{Z} \dots \mathcal{Z}}_n. \quad (3.17)$$

In this way the dynamic effects are traded for infinitely many spin degrees of freedom labelled by  $n$  and the spin chain becomes static. This reformulation may be useful to make the dynamic spin chains accessible to an algebraic treatment.

### 3.2 The non-compact $\mathfrak{su}(1, 1|2)$ sub-sector

The constraints following from algebra relations become particularly important in the non-compact sectors, where the modules are infinite-dimensional. Any diagrammatic calculations in this case are only realistic at low loop order, as for example at the two-loop level in the fermionic  $\mathfrak{sl}(2)$  sub-sector [28]. The algebraic approach in non-compact sectors has been advocated in [7] and the complete  $\mathcal{O}(\lambda^{3/2})$  symmetry algebra in the  $\mathfrak{su}(1, 1|2)$  sub-sector as well as the two-loop correction to the dilatation operator have been found. The  $\mathfrak{su}(1, 1|2)$  sub-sector consists of two scalar fields, two fermions and derivatives

$$\mathcal{D}^k \mathcal{Z}, \quad \mathcal{D}^k \mathcal{X}, \quad \mathcal{D}^k \mathcal{U}, \quad \mathcal{D}^k \dot{\mathcal{U}}. \quad (3.18)$$

Formally, the truncation of the full symmetry algebra to the  $\mathfrak{su}(1, 1|2)$  sub-sector is achieved by setting the classical dimensions of states simultaneously equal to the following linear combination of the eigenvalues of the Cartan generators of the  $\mathfrak{psu}(2, 2|4)$  algebra

$$D_0 = s_1 + \frac{1}{2}q_2 + p + \frac{3}{2}q_1 = s_2 + \frac{1}{2}q_1 + p + \frac{3}{2}q_2. \quad (3.19)$$

Interestingly, the residual symmetry is larger than expected and consists of a tensor product  $\mathfrak{psu}(1, 1|2) \times (\mathfrak{psu}(1|1))^2$ . The anomalous part of the dilatation operator  $\delta D$  is a central charge for both components of the product. The full set of commutation relations may be found in [7].

By invoking constraints from Feynman rules, imposing the algebra relations (3.1) and using representation theory, it has been found in [7] that the next-to-leading corrections<sup>3</sup> to the  $\mathfrak{psu}(1, 1|2)$  algebra generators satisfy

$$J_{\text{NLO}} = \pm [J_{\text{LO}}, X]. \quad (3.20)$$

<sup>3</sup>The generators of  $\mathfrak{psu}(1, 1|2)$  have an expansion in  $g^2 \sim \lambda$ , while the expansion parameter of the  $\mathfrak{psu}(1|1)$  generators is  $g \sim \sqrt{\lambda}$ .

The sign in front of the commutator is different for generators corresponding to positive and negative algebra roots. The generator  $X$  may be expressed through the  $\mathfrak{psu}(1|1)^2$  supercharges  $T^\pm$  and  $\bar{T}^\pm$  together with an auxiliary generator  $h$

$$X = \frac{1}{2} (\{\bar{T}^-, [\bar{T}^+, h]\} - \{T^+, [T^-, h]\}) . \quad (3.21)$$

The generator  $h$  at the leading order is a one-site generator of the harmonic numbers  $H(j)$

$$\begin{aligned} h |\mathcal{D}^k \mathcal{Z}\rangle &= H(k) |\mathcal{D}^k \mathcal{Z}\rangle, & h |\mathcal{D}^k \mathcal{X}\rangle &= H(k) |\mathcal{D}^k \mathcal{X}\rangle \\ h |\mathcal{D}^k \mathcal{U}\rangle &= H(k+1) |\mathcal{D}^k \mathcal{U}\rangle, & h |\mathcal{D}^k \dot{\mathcal{U}}\rangle &= H(k+1) |\mathcal{D}^k \dot{\mathcal{U}}\rangle. \end{aligned} \quad (3.22)$$

The higher corrections to  $h$  may be found recursively [7]. Also the  $\mathcal{O}(\lambda^{3/2})$  corrections to the fermionic generators of the two copies of  $\mathfrak{psu}(1|1)$ , that is  $T^\pm$  and  $\bar{T}^\pm$ , could have been determined in a compact form. Since the classical action of these generators is trivial, this is enough to determine the two-loop dilatation generator

$$\delta D_4^{\mathfrak{su}(1,1|2)} = 2 \{\bar{T}^+, \bar{T}^-\}_4 = 2 \{T^+, T^-\}_4 = 2 \{T_3^+, T_1^-\} + 2 \{T_1^+, T_3^-\} . \quad (3.23)$$

The two-loop correction determined in this way was found to reproduce correctly the two-loop anomalous dimension in the  $\mathfrak{sl}(2)$  and  $\mathfrak{su}(1|1)$  sub-sectors, at least for the states considered [7]. It has been argued in [8] that the relation (3.20) has a very simple generalisation at higher orders

$$\frac{\partial}{\partial \lambda} J(\lambda) = \pm [J(\lambda), X(\lambda)] . \quad (3.24)$$

In other words,  $X(\lambda)$  generates translations in  $\lambda$  for symmetry generators. The leading order result (3.21) is lifted to higher orders in the simplest possible way

$$X(\lambda) = \frac{1}{2} (\{\bar{T}^-(\lambda), [\bar{T}^+(\lambda), h(\lambda)]\} - \{T^+(\lambda), [T^-(\lambda), h(\lambda)]\}) . \quad (3.25)$$

The function  $h(\lambda)$  may be recursively determined from the corresponding Serre-like relations, see [8] for further details. The equation (3.24) allowed to determine the dilatation operator in this sector up to three-loop order, which was subsequently subject to numerous spectral tests (see [7] and [8]) and appears to be perturbatively integrable.

## 4 Generic integrable long-range spin chains

The  $\mathfrak{su}(2)$ ,  $\mathfrak{su}(2|3)$  and  $\mathfrak{su}(1,1|2)$  spin chains discussed above furnish examples of novel long-range integrable spin chains. The integrability of any spin chain is based on the existence of an infinite set of independent hermitian commuting charges  $Q_r$

$$[Q_r, Q_s] = 0 . \quad (4.1)$$

The  $Q_2$  charge is usually associated with the Hamiltonian, while the total momentum operator is usually identified with  $\exp(i Q_1)$ . It is an interesting question what are the

generic long-range spin chains satisfying (4.1). In this section we will discuss the recent progress in the theory of such systems.

In this section we will assume that the spin chain charges admit perturbative expansion

$$Q_r(\lambda) = \sum_{k=0}^{\infty} \left(\frac{\lambda}{16\pi^2}\right)^k Q_r^{(k)}. \quad (4.2)$$

Furthermore, we will assume that the maximal range of  $Q_r^{(k)}$  is  $r+k$ , i.e.  $Q_r^{(k)}$  acts locally on  $r+k$  adjacent sites in the spin chain. Please note that for finite values of  $\lambda$  the range of interactions becomes formally infinite.

## 4.1 Closed long-range spin chains with $\mathfrak{gl}(n)$ symmetry algebra

Generic spin chains with the underlying symmetry algebra  $\mathfrak{gl}(n)$  have been investigated in [11]. It has been proposed that the  $\mathfrak{gl}(n)$ -invariant long-range interactions may be expanded in the basis (2.3). The range of an interaction  $\{n_1, \dots, n_l\}$  is given by  $R = \max\{n_i\} - \min\{n_i\} + 2$ . Consequently, the basis for the  $k$ -loop correction to the charge  $Q_r$  is spanned by (2.3) with  $R \leq r+k$ . The number of all permutations up to range  $R$  is given by  $R! - (R-1)! + 1$ . Please note that at the  $k$ -loop order the relation (4.1) amounts to

$$\sum_{j=0}^k [Q_r^{(j)}, Q_s^{(k-j)}] = 0, \quad (4.3)$$

so that the procedure is recursive. The authors of [11] have applied this method to  $Q_2$  and  $Q_3$  charges up to and including four-loop order. Interestingly, it is enough to consider solely commutation relations between  $Q_2$  and  $Q_3$  since the commutators with higher charges *do not* lead to further restrictions. The relation (4.3) does not fix all the coefficients of the basis. For example, the  $Q_2$  charge up to two-loop order is presented in Table 1. The free parameters appearing at any loop order can be divided into three classes, which we will discuss in what follows.

The first class constitute the moduli  $\alpha_l(\lambda)$  and  $\beta_{r,s}(\lambda)$ . They govern propagation and scattering of the spins and differ for different models. They enter directly into the Bethe equations and dispersion relation. It has been conjectured in [11] that only the main equation out of the set of Bethe equations corresponding to the nearest-neighbour integrable  $\mathfrak{gl}(n)$  spin chain needs to be modified. Explicitly, the main Bethe equations take the following form

$$1 = \left(\frac{x(u_k - \frac{i}{2})}{x(u_k + \frac{i}{2})}\right)^L \prod_{j=1, j \neq k}^{K_u} \frac{u_k - u_j + i}{u_k - u_j - i} \exp(2i\theta(u_k, u_j)) \prod_{l=1}^{K_v} \frac{u_k - v_l - \frac{i}{2}}{u_k - v_l + \frac{i}{2}}. \quad (4.4)$$

The reader might find it useful to refer to [29] and [30] for a pedagogical discussion of single-level and nested Bethe equations. Here, the main Bethe roots are labelled by  $u_k$ , while the auxiliary Bethe roots coupling to the main roots are denoted by  $v_j$ . The difference to the Bethe equations of the nearest-neighbour spin chain is twofold.

Firstly, the function  $x(u)$ , the so-called rapidity map, determines the momentum-rapidity relation of a single magnon

$$\exp(ip(u)) = \frac{x(u + \frac{i}{2})}{x(u - \frac{i}{2})}. \quad (4.5)$$

The rapidity map depends on the  $\alpha_l(\lambda)$  parameters through the relation

$$u(x) = x + \sum_{l=0}^{\infty} \frac{\alpha_l(\lambda)}{x^{l+1}}, \quad (4.6)$$

which needs to be solved for  $x$ . Secondly, the additional piece of the scattering matrix,  $\exp(2i\theta(u, v))$ , known in the literature as the dressing factor, is determined by the  $\beta_{r,s}(\lambda)$  parameters

$$\theta(u, v) = \sum_{r=2}^{\infty} \sum_{s=r+1}^{\infty} \beta_{r,s}(\lambda) (q_r(u) q_s(v) - q_s(u) q_r(v)). \quad (4.7)$$

The  $\beta_{r,s}(\lambda)$  coefficients start at order  $\mathcal{O}(\lambda^{s-1})$

$$\beta_{r,s}(\lambda) = \sum_{k=s-1}^{\infty} \left(\frac{\lambda}{16\pi^2}\right)^k \beta_{r,s}^{(k)}. \quad (4.8)$$

The parity conservation requires  $\beta_{r,s} = 0$  for all even  $r + s$ . The quantities  $q_r(u)$  are the elementary magnon charges and are given by

$$q_r(u) = \frac{i}{r-1} \left( \frac{1}{x(u + \frac{i}{2})^{r-1}} - \frac{1}{x(u - \frac{i}{2})^{r-1}} \right). \quad (4.9)$$

Clearly, the distinct character of the  $\alpha_l(\lambda)$  and  $\beta_{r,s}(\lambda)$  moduli parameters becomes apparent. The  $\alpha_l(\lambda)$  parameters specify the one-magnon state, while the  $\beta_{r,s}(\lambda)$  “dress” the scalar part of the scattering matrix of two magnons. Thanks to integrability these pieces of information are enough to fully describe the system.

The second class of parameters  $\gamma_{r,s}(\lambda)$  are elements of the normalisation matrix of the charges. Upon introducing the normalised charges, for which the eigenvalues are given by a sum over the charge densities  $\tilde{Q}_s := \sum_{k=1}^{K_u} q_s(u_k)$ , the  $[\gamma(\lambda)]_{r,s}$  matrix simply acts as a rotation matrix

$$Q_r = \gamma_{r,0}(\lambda) L + \sum_{s=2}^{\infty} \gamma_{r,s}(\lambda) \tilde{Q}_s. \quad (4.10)$$

This transformation readily preserves the commutation relations (4.1).

Finally, the last class is spanned by the parameters  $\epsilon_{k,l}(\lambda)$ , which merely influence the eigenvectors and correspond to similarity transformations. They are thus unphysical.

The authors of [11] have only analysed  $Q_2$  and  $Q_3$  charges. Although it seems very plausible that all charges may be constructed in this way, it was still rather a hypothesis. The integrability of the long-range spin chains with the  $\mathfrak{gl}(n)$  symmetry algebra has been first confirmed in [31] by constructing the corresponding Yangian algebra up to and including three-loop order. Please refer to [32] for details on Yangians and their relation to integrability.

## 4.2 Generic integrable long-range spin chains

A method for constructing integrable closed long-range spin chains with generic Lie (super)algebras and spin representations has been introduced in [12, 13] inspired by the findings of [33]. Interestingly, it is a bottom-up approach. The starting point provides an integrable nearest-neighbour spin chain with a symmetry (super)algebra  $\mathcal{A}$  and a given spin representation. It has been proposed that the higher-loop deformations of the conserved charges are governed by a generating equation similar to (3.24)

$$\frac{d}{d\lambda} Q_r(\lambda) = i [X(\lambda), Q_r(\lambda)] + \sum_{s=2}^{\infty} \gamma_{r,s}(\lambda) Q_s(\lambda). \quad (4.11)$$

Here,  $X(\lambda)$  is some operator with well-defined commutation relations with all conserved charges. It is straightforward to check that the deformations generated by (4.11) preserve the commutation relations (4.1). Substituting the expansion (4.2) into (4.11) one can order by order “boost” an integrable nearest-neighbour spin chain to its long-range counterpart. The freedom encountered in the previous sub-section while determining the generic form of the higher-loop corrections corresponds to freedom in choosing the  $X(\lambda)$  operator. It has been advocated in [12, 13] that there are three different admissible classes of such operators: boost charges, bi-local charges and local charges. The first two act inhomogeneously on the spin chain and are parametrised by  $\alpha_r(\lambda)$  and  $\beta_{r,s}(\lambda)$  respectively. The local operators, on the other hand, do not influence the spectrum and thus may be associated with the  $\epsilon_{k,l}(\lambda)$  degrees of freedom. The Bethe equation diagonalising spin chains constructed in such way are similar to those presented in sub-section 4.1

$$1 = \left( \frac{x(u_k - \frac{i}{2} t_a)}{x(u_k + \frac{i}{2} t_a)} \right)^L \prod_{b=1}^r \prod_{\substack{j=1 \\ (b,j) \neq (a,k)}}^{K_b} \frac{u_{a,k} - u_{b,j} + \frac{i}{2} C_{ab}}{u_{a,k} - u_{b,j} - \frac{i}{2} C_{ab}} \exp(2i \theta^{\{t\}}(u_{a,k}, u_{b,j})). \quad (4.12)$$

The number of levels of the Bethe equations  $r$  coincides with the rank of the Lie (super)algebra  $\mathcal{A}$ . The Dynkin labels of the spin representation are denoted by  $t_a$ ,  $a = 1, \dots, r$  and the symmetric Cartan matrix is represented by  $C_{ab}$ . The dressing phase  $\theta^{\{t\}}$  is indexed with  $t$  to remind that the elementary magnon charges are also influenced by the spin representation

$$q_r(t, u) = \frac{i}{r-1} \left( \frac{1}{x(u + \frac{i}{2} t)} - \frac{1}{x(u - \frac{i}{2} t)} \right). \quad (4.13)$$

These results were obtained by applying asymptotic Bethe ansatz techniques to the chain constructed by means of (4.11). Equation (4.11) thus plays a central role in the theory of closed long-range integrable spin chains.

In [33] the most general perturbatively long-range integrable spin chains in the fundamental representation of the  $\mathfrak{gl}(n)$  symmetry algebra and with open boundary conditions have been studied. For open spin chains any excitation returns back to its initial position after being shifted  $2L$  times. On its way it is reflected at the two boundaries, each of

them giving rise to a boundary scattering phase. Moreover, in general, the momentum after reflection is not equal to reversed incoming momentum and the relation between those two momenta needs to be specified via the reflection map. This is due to the fact that the Hamiltonian will generically not preserve parity. Thus the corresponding Bethe equations differ structurally from the Bethe equations for the closed chains. A set of such Bethe equations for arbitrary boundary scattering phase has been formulated in [33].

### 4.3 Examples: Inozemtsev spin chain

In [34] the first attempt has been made to embed the novel perturbative long-range integrability in the framework of well-studied integrable models. It was found that up to three-loop order the dilatation operator in the  $\mathfrak{su}(2)$  sector may be constructed from the conserved charges of the Inozemtsev model [10].

The Inozemtsev model furnishes one of the few known examples of integrable long-range spin chains which are not defined as a deformations of nearest-neighbour models. The Hamiltonian of this model is given by

$$H = \sum_{j=1}^L \sum_{n=1}^{L-1} f_{L,\kappa}(n)(1 - P_{j,j+n}), \quad (4.14)$$

where  $P_{a,b}$ , as before, denotes the permutation of sites  $a$  and  $b$ . The spin chain is assumed to be in the fundamental representation of the  $\mathfrak{su}(2)$  symmetry algebra. The interaction strength  $f_{L,\kappa}(n)$  is given by the elliptic Weierstrass function

$$f_{L,\kappa}(z) = \frac{1}{z^2} + \sum'_{m,n=-\infty}^{\infty} \left( \frac{1}{(z - mL - in\pi/\kappa)^2} - \frac{1}{(mL + in\pi/\kappa)^2} \right), \quad (4.15)$$

where the prime means that the term  $m = n = 0$  should be omitted. A detailed study of the Hamiltonian (4.14), see [10], gave compelling evidence in favour of its integrability. In particular, the corresponding Lax pair has been found. In the limit  $\kappa \rightarrow 0$  the interaction interpolates smoothly to the Haldane-Shastry interaction [35]- [36], which is another known example of an integrable long-range spin chain.

The authors of [34] have found that simple linear combinations of the higher conserved charges of the Inozemtsev model allow to reconstruct the dilatation operator in the  $\mathfrak{su}(2)$  model up to three-loop order. It is necessary to invoke the higher charges since the Hamiltonian (4.14) only involves two spin interactions, while already at three-loop order the  $\mathfrak{su}(2)$  dilatation operator acts on three sites simultaneously. Under a suitable identification of the coupling constant

$$\frac{\lambda}{16\pi^2} = \sum_{n>0} \frac{1}{4 \sinh^2(n\kappa)} \quad (4.16)$$

and keeping  $\frac{\lambda}{16\pi^2}$  perturbatively small, the Inozemtsev model turns into long-range model of the type discussed in 4.1. Up to four-loop order

$$\alpha_l = \lambda \delta_{l,0} + \lambda^3 + \mathcal{O}(\lambda^4), \quad \beta_{r,s} = 0 + \mathcal{O}(\lambda^4), \quad (4.17)$$

$$\gamma_{2,r} = (2 + 6\lambda - 20\lambda^2 + 120\lambda^3)\delta_{r,2} + (6\lambda^2 - 30\lambda^3)\delta_{r,4} + \mathcal{O}(\lambda^4). \quad (4.18)$$

It would be interesting to find higher-loop corrections to the above formulas.

## 5 Hubbard model

In this section we will discuss an intriguing relation between a short-range dynamical model of electrons, the Hubbard model, and the long-range spin chains discussed before.

The Hubbard model is a dynamical, short-range model of  $N$  electrons on  $L$  lattice sites. Due to Pauli's exclusion principle, there are four possible states on each lattice site: no particle, spin-up electron, spin down electron and double occupied state with spin-up and spin-down electrons. In what follows, we will consider the half-filled case  $N = L$ . The Hamiltonian of the Hubbard model consists of the kinetic part that forces the electrons to jump between different sites and the potential part, which according to the value of  $U$  corresponds to repulsive or attractive force

$$\hat{H}_{\text{Hubbard}} = -t \sum_{i=1}^L \sum_{\sigma=\uparrow,\downarrow} \left( c_{i,\sigma}^\dagger c_{i+1,\sigma} + c_{i+1,\sigma}^\dagger c_{i,\sigma} \right) + tU \sum_{i=1}^L c_{i,\uparrow}^\dagger c_{i,\uparrow} c_{i,\downarrow}^\dagger c_{i,\downarrow}. \quad (5.1)$$

The operators  $c_{i,\sigma}^\dagger$  and  $c_{i,\sigma}$  are canonical Fermi operators obeying standard anticommutation relations. We assume the system to be closed and thus we identify  $c_{L+1,\sigma} = c_{1,\sigma}$  and  $c_{L+1,\sigma}^\dagger = c_{1,\sigma}^\dagger$ . The Hamiltonian is invariant with respect to the  $\mathfrak{su}(2)$  transformations

$$[\hat{H}_{\text{Hubbard}}, \hat{S}^a] = 0, \quad a = +, -, z, \quad (5.2)$$

with  $\hat{S}^a = \sum_{i=1}^L \hat{S}_i^a$ . This allows to classify the spectrum according to the eigenvalues of the total spin and its  $z$  component. The integrability of this model has been shown in [37].

It has been shown in [38] that upon the following identification of the parameters

$$t = -\frac{2\pi}{\sqrt{\lambda}}, \quad U = \frac{4\pi}{\sqrt{\lambda}}, \quad (5.3)$$

this short range model may be identified with the BDS spin chain [21]. Please note that with the identification (5.3) and in the limit  $\lambda \rightarrow 0$  the potential part of the Hamiltonian is dominating and perturbation theory around the states with minimal potential energy may be applied. This allowed to show that the effective Hamiltonian acting on the ground state space of the potential part coincides at one-, two- and three-loop order with the corresponding dilatation operator in the  $\mathfrak{su}(2)$  sub-sector, *cf.* formulas (2.4), (2.8) and (2.11). The reader should note that the ground space of the potential part of the Hamiltonian (5.1) is identical with the Hilbert space of a  $\mathfrak{su}(2)$  spin chain. Please refer to [38] for detailed description of this procedure. Moreover, the spectral equations of the Hubbard model (Lieb-Wu equations [37]) have been shown to reproduce to any perturbative order the Bethe equations of the long-range spin chain with the  $\mathfrak{su}(2)$  symmetry algebra and the following moduli parameters

$$\alpha_l = \lambda \delta_{l,0}, \quad \beta_{r,s} = 0. \quad (5.4)$$

Even though this choice *disagrees* with the asymptotic Bethe equations of the  $\mathfrak{su}(2)$  subsector of  $\mathcal{N} = \text{SYM}$  at four-loop order and beyond, see [25], it may suggest that generic long-range spin chains as well as the asymptotic integrability in the  $\mathcal{N} = 4$  SYM theory may be intimately related to yet-to-be-discovered integrable short-range models.

## 6 Conclusions

Integrable long-range spin chains are a natural and very non-trivial extension of the nearest-neighbour spin chains, a prime example in the literature on integrable models. The complexity of the long-range interactions gives evidence that even seemingly very complicated models may exhibit integrability, which is often indispensable to understand the dynamics of a system. There is a host of evidence that planar AdS/CFT correspondence may be one such system and several long-range spin chains have found applications in this string/gauge theory duality. This has already allowed to study many non-perturbative aspects of the duality, see [39]. Moreover, methods based on integrability have allowed to conjecture the spectral equations of the planar AdS/CFT correspondence, see [40].

## Acknowledgements

I would like to thank Till Bargheer, Niklas Beisert, Marc Magro and Christoph Sieg for pointing out some shortcomings in the initial manuscript. The author is supported by a STFC postdoctoral fellowship.

## A Three-Loop Hamiltonian of a generic long-range spin chain with $\mathfrak{gl}(n)$ symmetry algebra

$$\begin{aligned}
 Q_2(\lambda) = & (\{\} - \{0\}) \\
 & + \alpha_0(\lambda) (-3\{\} + 4\{0\} - \{0, 1, 0\}) \\
 & + \alpha_0(\lambda)^2 (20\{\} - 29\{0\} + 10\{0, 1, 0\} - \{0, 1, 2\} - \{2, 1, 0\} + \{0, 2, 1\} + \{1, 0, 2\} \\
 & \quad - \{0, 1, 2, 1, 0\}) \\
 & + \frac{i}{2}\alpha_1(\lambda) (-6\{0, 1\} + 6\{1, 0\} + \{0, 1, 2, 1\} - \{1, 2, 1, 0\} + \{0, 1, 0, 2\} - \{0, 2, 1, 0\}) \\
 & + \frac{1}{2}\beta_{2,3}(\lambda) (-4\{\} + 8\{0\} - 2\{0, 1\} - 2\{1, 0\} - 2\{0, 2\} \\
 & \quad - 2\{0, 1, 2\} - 2\{2, 1, 0\} + 2\{0, 2, 1\} + 2\{1, 0, 2\} \\
 & \quad + \{0, 1, 2, 1\} + \{1, 2, 1, 0\} + \{0, 1, 0, 2\} + \{0, 2, 1, 0\} - 2\{1, 0, 2, 1\}) \\
 & + i\epsilon_{2,1}(\lambda) (\{1, 0, 2\} - \{0, 2, 1\}) \\
 & + i\epsilon_{2,2}(\lambda) (-\{0, 1, 2, 1\} + \{1, 2, 1, 0\} + \{0, 1, 0, 2\} - \{0, 2, 1, 0\}) \\
 & + \mathcal{O}\{\lambda^3\}
 \end{aligned}$$

**Table 1:** Normalised Hamiltonian up to third order.

## References

- [1] J. M. Maldacena, “*The large  $N$  limit of superconformal field theories and supergravity*”, *Adv. Theor. Math. Phys.* 2, 231 (1998), [hep-th/9711200](#).
- [2] J. A. Minahan and K. Zarembo, “*The Bethe-ansatz for  $N = 4$  super Yang-Mills*”, *JHEP* 0303, 013 (2003), [hep-th/0212208](#).
- [3] N. Beisert, “*The complete one-loop dilatation operator of  $N = 4$  super Yang-Mills theory*”, *Nucl. Phys.* B676, 3 (2004), [hep-th/0307015](#).
- [4] N. Beisert, C. Kristjansen and M. Staudacher, “*The dilatation operator of  $N = 4$  super Yang-Mills theory*”, *Nucl. Phys.* B664, 131 (2003), [hep-th/0303060](#).
- [5] N. Beisert, “*Higher loops, integrability and the near BMN limit*”, *JHEP* 0309, 062 (2003), [hep-th/0308074](#).
- [6] N. Beisert, “*The  $su(2|3)$  dynamic spin chain*”, *Nucl. Phys.* B682, 487 (2004), [hep-th/0310252](#).
- [7] B. I. Zwiebel, “ *$N = 4$  SYM to two loops: Compact expressions for the non-compact symmetry algebra of the  $su(1,1|2)$  sector*”, *JHEP* 0602, 055 (2006), [hep-th/0511109](#).
- [8] B. I. Zwiebel, “*Iterative Structure of the  $N=4$  SYM Spin Chain*”, *JHEP* 0807, 114 (2008), [arxiv:0806.1786](#).

- [9] C. Sieg, “*Review of AdS/CFT Integrability, Chapter I.2: The spectrum from perturbative gauge theory*”, [arxiv:1012.3984](#).
- [10] V. I. Inozemtsev, “*On the connection between the one-dimensional  $s = 1/2$  Heisenberg chain and Haldane-Shastry model*”, *J. Stat. Phys.* 59, 1143 (1990).
- [11] N. Beisert and T. Klose, “*Long-range  $gl(n)$  integrable spin chains and plane-wave matrix theory*”, *J. Stat. Mech.* 0607, P006 (2006), [hep-th/0510124](#).
- [12] T. Bargheer, N. Beisert and F. Loebbert, “*Boosting Nearest-Neighbour to Long-Range Integrable Spin Chains*”, *J. Stat. Mech.* 0811, L11001 (2008), [arxiv:0807.5081](#).
- [13] T. Bargheer, N. Beisert and F. Loebbert, “*Long-Range Deformations for Integrable Spin Chains*”, *J. Phys. A* 42, 285205 (2009), [arxiv:0902.0956](#).
- [14] J. A. Minahan, “*Review of AdS/CFT Integrability, Chapter I.1: Spin Chains in  $\mathcal{N} = 4$  SYM*”, [arxiv:1012.3983](#).
- [15] D. E. Berenstein, J. M. Maldacena and H. S. Nastase, “*Strings in flat space and pp waves from  $N = 4$  super Yang Mills*”, *JHEP* 0204, 013 (2002), [hep-th/0202021](#).
- [16] B. Eden and M. Staudacher, “*Integrability and transcendentality*”, *J. Stat. Mech.* 0611, P014 (2006), [hep-th/0603157](#).
- [17] C. Kristjansen, “*Review of AdS/CFT Integrability, Chapter IV.1: Aspects of Non-planarity*”, [arxiv:1012.3997](#).
- [18] M. Tetelman, *Sov. Phys. JETP* 55, 306 (1981).
- [19] K. Sogo and M. Wadati, “*Boost Operator and Its Application to Quantum Gelfand-Levitan Equation for Heisenberg-Ising Chain with Spin One-Half*”, *Prog. Theor. Phys.* 69 No.2, 431 (1983).
- [20] M. Grabowski and P. Mathieu, “*Integrability test for spin chains*”, *J.Phys.A* A28, 4777 (1995), [hep-th/9412039](#).
- [21] N. Beisert, V. Dippel and M. Staudacher, “*A novel long range spin chain and planar  $N = 4$  super Yang- Mills*”, *JHEP* 0407, 075 (2004), [hep-th/0405001](#).
- [22] A. V. Ryzhov and A. A. Tseytlin, “*Towards the exact dilatation operator of  $N = 4$  super Yang- Mills theory*”, *Nucl. Phys. B* 698, 132 (2004), [hep-th/0404215](#).
- [23] N. Beisert, T. McLoughlin and R. Roiban, “*The Four-Loop Dressing Phase of  $N=4$  SYM*”, *Phys. Rev. D* 76, 046002 (2007), [arxiv:0705.0321](#).
- [24] N. Beisert, “*The  $su(2|2)$  dynamic  $S$ -matrix*”, *Adv. Theor. Math. Phys.* 12, 945 (2008), [hep-th/0511082](#).
- [25] P. Vieira and D. Volin, “*Review of AdS/CFT Integrability, Chapter III.3: The dressing factor*”, [arxiv:1012.3992](#).
- [26] A. Agarwal and G. Ferretti, “*Higher charges in dynamical spin chains for SYM theory*”, *JHEP* 0510, 051 (2005), [hep-th/0508138](#).
- [27] N. Beisert, “*The  $su(2|3)$  Undynamic Spin Chain*”, *Prog. Theor. Phys. Suppl.* 177, 1 (2009), [arxiv:0807.0099](#).
- [28] A. V. Belitsky, G. P. Korchemsky and D. Mueller, “*Integrability of two-loop dilatation operator in gauge theories*”, *Nucl. Phys. B* 735, 17 (2006), [hep-th/0509121](#).

- [29] M. Staudacher, “*Review of AdS/CFT Integrability, Chapter III.1: Bethe Ansatz and the R-Matrix Formalism*”, [arxiv:1012.3990](#).
- [30] C. Ahn and R. I. Nepomechie, “*Review of AdS/CFT Integrability, Chapter III.2: Exact world-sheet S-matrix*”, [arxiv:1012.3991](#).
- [31] N. Beisert and D. Erkal, “*Yangian Symmetry of Long-Range  $gl(N)$  Integrable Spin Chains*”, *J. Stat. Mech.* 0803, P03001 (2008), [arxiv:0711.4813](#).
- [32] A. Torrielli, “*Review of AdS/CFT Integrability, Chapter VI.2: Yangian Algebra*”, [arxiv:1012.4005](#).
- [33] N. Beisert and F. Loebbert, “*Open Perturbatively Long-Range Integrable  $gl(N)$  Spin Chains*”, *Adv. Sci. Lett.* 2, 261 (2009), [arxiv:0805.3260](#).
- [34] D. Serban and M. Staudacher, “*Planar  $N = 4$  gauge theory and the Inozemtsev long range spin chain*”, *JHEP* 0406, 001 (2004), [hep-th/0401057](#).
- [35] F. D. M. Haldane, “*Exact Jastrow-Gutzwiller resonating valence bond ground state of the spin 1/2 antiferromagnetic Heisenberg chain with  $1/r^{*2}$  exchange*”, *Phys. Rev. Lett.* 60, 635 (1988).
- [36] B. Sriram Shastry, “*Exact solution of an  $S = 1/2$  Heisenberg antiferromagnetic chain with long ranged interactions*”, *Phys. Rev. Lett.* 60, 639 (1988).
- [37] E. H. Lieb and F. Y. Wu, “*Absence of Mott transition in an exact solution of the short-range, one-band model in one dimension*”, *Phys. Rev. Lett.* 20, 1445 (1968).
- [38] A. Rej, D. Serban and M. Staudacher, “*Planar  $N = 4$  gauge theory and the Hubbard model*”, *JHEP* 0603, 018 (2006), [hep-th/0512077](#).
- [39] L. Freyhult, “*Review of AdS/CFT Integrability, Chapter III.4: Twist states and the cusp anomalous dimension*”, [arxiv:1012.3993](#).
- [40] V. Kazakov and N. Gromov, “*Review of AdS/CFT Integrability, Chapter III.7: Hirota Dynamics for Quantum Integrability*”, [arxiv:1012.3996](#).

# Review of AdS/CFT Integrability, Chapter II.1: Classical $AdS_5 \times S^5$ string solutions

A.A. TSEYTLIN\*

*Blackett Laboratory, Imperial College London, SW7 2AZ, U.K.*

tseytlin@imperial.ac.uk

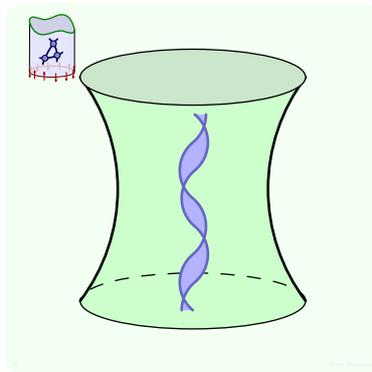

**Abstract:** We review basic examples of classical string solutions in  $AdS_5 \times S^5$ . We concentrate on simplest rigid closed string solutions of circular or folded type described by integrable 1-d Neumann system but mention also various generalizations and related open-string solutions.

---

\*Also at Lebedev Institute, Moscow.

## 1 Introduction

$AdS_5 \times S^5$  space plays a special role in superstring theory [1]. This space (supported by a 5-form flux) is one of the three maximally supersymmetric “vacua” of type IIB 10-d supergravity [2], along with its limits – the flat Minkowski space and the plane-wave background [3]. It appears as a “near-horizon” region of the solitonic D3-brane background [4]; that explains its central role in the AdS/CFT duality [5] (see [6] for a review). The duality states that certain “observables” in  $\mathcal{N} = 4$  supersymmetric  $SU(N)$  4-d gauge theory have direct counterparts in the type IIB superstring theory in  $AdS_5 \times S^5$  space, and vice versa.

The type IIB superstring theory in a curved space with a 5-form Ramond-Ramond (RR) background is defined by the Green-Schwarz [7] action ( $T_0 = \frac{1}{2\pi\alpha'}$ )

$$I = I_B + I_F, \quad I_B = \frac{1}{2}T_0 \int d^2\sigma \sqrt{-g}g^{ab}G_{\mu\nu}(x)\partial_a x^\mu \partial_b x^\nu, \quad (1.1)$$

$$I_F = iT_0 \int d^2\sigma(\sqrt{-g}g^{ab}\delta^{IJ} - \epsilon^{ab}s^{IJ})\bar{\theta}^I \rho_a D_b \theta^J + O(\theta^4). \quad (1.2)$$

Here  $x^\mu$  ( $\mu = 0, 1, \dots, 9$ ) are the bosonic string coordinates,  $\theta^I$  ( $I = 1, 2$ ) are two Majorana-Weyl spinor fields,  $g_{ab}$  ( $a, b = 0, 1$ ) is an independent 2-d metric,  $\rho_a$  are projections of the 10-d Dirac matrices,  $\rho_a \equiv \Gamma_A E_\mu^A \partial_a x^\mu$ ,  $E_\mu^A$  is the vielbein of the target space metric,  $G_{\mu\nu} = E_\mu^A E_\nu^B \eta_{AB}$ .  $\epsilon^{ab}$  is antisymmetric 2-d tensor and  $s^{IJ} = \text{diag}(1, -1)$ .  $D_a$  is the projection of the 10-d covariant derivative  $D_\mu$ . The latter is given by  $D_\mu = \partial_\mu + \frac{1}{4}\omega_\mu^{AB}\Gamma_{AB} - \frac{1}{8 \cdot 5!}\Gamma^{\mu_1 \dots \mu_5}\Gamma_\mu F_{\mu_1 \dots \mu_5}$ , where  $\omega_\mu^{AB}$  is the Lorentz connection and  $F_{\mu_1 \dots \mu_5}$  is the RR 5-form field. Here  $G_{\mu\nu}$  and  $F_{\mu_1 \dots \mu_5}$  should be related so that the 2-d Weyl and kappa-symmetry anomalies cancel.

In the case of the  $AdS_5 \times S^5$  background the explicit form of the superstring action can be found using the supercoset construction [8]. The group of super-isometries (Killing vectors and Killing spinors or solutions of  $D_\mu \epsilon^I = 0$ ) of this background is  $PSU(2, 2|4)$ , i.e. the same as  $\mathcal{N} = 4$  super-extension of the 4-d conformal group  $SO(2, 4)$ . Using that  $AdS_5 = SO(2, 4)/SO(1, 4)$  and  $S^5 = SO(6)/SO(5)$  the superstring action can be constructed in terms of the components of  $PSU(2, 2|4)$  current restricted to the coset  $PSU(2, 2|4)/[SO(1, 4) \times SO(5)]$  (see [9] for details).

Since the metric of  $AdS_5 \times S^5$  has direct product structure, the bosonic part of the action (1.1) is a sum of the actions for the  $AdS_5$  and  $S^5$  sigma models. The two sets of bosons are coupled through their interaction with the fermions. The latter fact is crucial for the UV finiteness of the superstring model [8, 10, 11] (see also [12]).

Below we shall consider classical bosonic solutions of the  $AdS_5 \times S^5$  string action. The study of classical string solutions and their semiclassical quantization initiated in [13–16] is an important tool for investigating the structure of the AdS/CFT correspondence (for reviews see, e.g., [17–20]). The AdS energy of a closed string solution expressed in terms of other conserved charges and string tension gives the strong coupling limit of the scaling dimension of the corresponding gauge-theory operator. Classical solutions for open strings ending at the boundary of  $AdS_5$  describe the strong coupling limit of the associated Wilson loops and gluon scattering amplitudes (see [21] and [22–24]).

Coset space sigma models are known to be classically integrable [25, 26] and this integrability extends [27] also to the full kappa-invariant  $AdS_5 \times S^5$  superstring action. The integrability allows one to describe, in particular, large class of (finite gap [28]) classical string solutions in terms of the associated spectral curve [29, 30] (see [31]).

This description is, however, formal and obscures somewhat the physical interpretation of the solutions. It is very useful to complement it with a study of specific examples of solutions that can be constructed directly from the sigma model equations of motion by starting with certain natural ansatze. This will be our aim below.

We shall mostly concentrate on the simplest spinning ‘‘rigid’’ closed string solutions for which the shape of the string does not change with time (extra oscillations increase the energy for given spins). We shall consider several types of solutions and their limits that reveal different patterns of dependence of the energy on the string tension and the spins. This provides an important information about the strong ‘t Hooft coupling limit of the corresponding gauge theory anomalous dimensions and thus aids one in understanding the underlying description of the string/gauge theory spectrum valid for all values of the string tension or ‘t Hooft coupling.

## 2 Bosonic string in $AdS_5 \times S^5$

At the classical level (with fermion fields vanishing) the  $AdS_5$  and  $S^5$  parts of the string action are still effectively coupled through their interaction with 2-d metric  $g_{ab}$ . If one solves for  $g_{ab}$  one gets a non-linear Nambu-Goto type action containing interactions between the  $AdS_5$  and  $S^5$  coordinates. In the conformal gauge  $\sqrt{-g}g^{ab} = \eta^{ab}$  the classical equations for the  $AdS_5$  and  $S^5$  parts are decoupled, but there is a constraint on their initial data from the equation for  $g_{ab}$ , i.e. that the 2-d stress tensor should vanish (the Virasoro conditions). We shall study the corresponding solutions below but let us start with the definition of the  $AdS_n$  space and the explicit form of the  $AdS_5 \times S^5$  bosonic string action.

### 2.1 $AdS_5 \times S^5$ space

Just like the  $d$ -dimensional sphere  $S^d$  can be represented as a surface in  $R^{d+1}$

$$X_M X_M = X_1^2 + \dots + X_{d+1}^2 = 1 \quad (2.1)$$

the  $d = n + 1$  dimensional anti - de Sitter space  $AdS_d$  can be represented as a hyperboloid (a constant negative curvature quadric)

$$-\eta_{PQ} Y^P Y^Q = Y_0^2 - Y_1^2 - \dots - Y_n^2 + Y_{n+1}^2 = 1 \quad (2.2)$$

in  $R^{2,d-1}$  with the metric

$$ds^2 = \eta_{PQ} dY^P dY^Q, \quad \eta_{PQ} = (-1, +1, \dots, +1, -1). \quad (2.3)$$

We set the radius of the sphere and the hyperboloid to 1. In what follows we will be interested in the case of  $d = 5$ .

It is often useful to solve (2.2),(2.1) by choosing an explicit parametrization of  $Y_P$  and  $X_M$  in terms of 5+5 independent “global” coordinates

$$\begin{aligned} Y_1 &\equiv Y_1 + iY_2 = \sinh \rho \cos \theta e^{i\phi_1}, & Y_2 &\equiv Y_3 + iY_4 = \sinh \rho \sin \theta e^{i\phi_2}, \\ Y_0 &\equiv Y_5 + iY_0 = \cosh \rho e^{it}, & X_3 &\equiv X_5 + iX_6 = \cos \gamma e^{i\varphi_3}, \\ X_1 &\equiv X_1 + iX_2 = \sin \gamma \cos \psi e^{i\varphi_1}, & X_2 &\equiv X_3 + iX_4 = \sin \gamma \sin \psi e^{i\varphi_2}. \end{aligned} \quad (2.4)$$

Then the corresponding metrics are

$$(ds^2)_{AdS_5} = d\rho^2 - \cosh^2 \rho dt^2 + \sinh^2 \rho (d\theta^2 + \cos^2 \theta d\phi_1^2 + \sin^2 \theta d\phi_2^2), \quad (2.5)$$

$$(ds^2)_{S^5} = d\gamma^2 + \cos^2 \gamma d\varphi_3^2 + \sin^2 \gamma (d\psi^2 + \cos^2 \psi d\varphi_1^2 + \sin^2 \psi d\varphi_2^2), \quad (2.6)$$

and they are obviously related by an analytic continuation.

Note that choosing  $\rho > 0$  and  $0 < t \leq 2\pi$  (and standard periodicities for the  $S^3$  angles  $\theta, \phi_1, \phi_2$ ) already covers the hyperboloid once. Near “the center”  $\rho = 0$  the  $AdS_5$  metric is that of  $S^1 \times R^4$  while near its boundary  $\rho \rightarrow \infty$  it is that of  $S^1 \times S^3$ . To avoid closed time-like curves and to relate the corresponding theory to gauge theory in  $R \times S^3$  it is standard to decompactify the  $t$  direction, i.e. to assume  $-\infty < t < \infty$ . Thus in all discussions of AdS/CFT and in what follows by  $AdS_5$  we shall understand its universal cover (in particular, we will ignore the possibility of string winding in global AdS time direction). In the case of  $AdS_2$  plotted as a hyperboloid in  $R^{2,1}$  that corresponds to going around the circular dimension infinite number of times or “cutting it open”. We present images of  $S^2$  and of a universal cover of  $AdS_2$  in Figure 1.<sup>†</sup> Another useful image of the universal cover of the  $AdS_3$  space is a body of 2-cylinder with  $R_t \times S^1$  as a boundary and  $\rho$  as a radial coordinate.

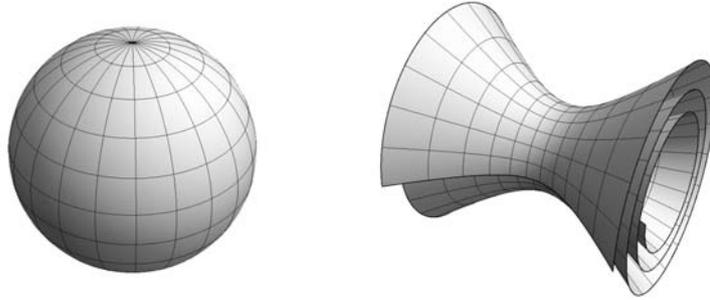

**Figure 1:** Images of a sphere and of a universal cover of AdS space

Let us mention also another choice of  $AdS_5 \times S^5$  coordinates – the Poincaré coordinates – that cover only part of  $AdS_5$  (for more details see, e.g., [6]):

$$\begin{aligned} Y_0 = \frac{x_0}{z} &= \cosh \rho \sin t, & Y_5 = \frac{1}{2z}(1 + z^2 - x_0^2 + x_i^2) &= \cosh \rho \cos t, \\ Y_i = \frac{x_i}{z} &= n_i \sinh \rho, & Y_4 = \frac{1}{2z}(-1 + z^2 - x_0^2 + x_i^2) &= n_4 \sinh \rho, \end{aligned} \quad (2.7)$$

<sup>†</sup>We thank N. Beisert for sending us these figures.

Here  $n_i^2 + n_4^2 = 1$  ( $i = 1, 2, 3$ ) parametrizes the 3-sphere in (2.5):  $dn_k dn_k = d\Omega_3(\theta, \phi_1, \phi_2)$ . Then the  $AdS_5$  metric (2.5) takes the form ( $m, n = 0, 1, 2, 3$ )

$$(ds^2)_{AdS_5} = \frac{1}{z^2}(dx^m dx_m + dz^2), \quad x_m = \eta_{mn} x^n. \quad (2.8)$$

The full  $AdS_5 \times S^5$  metric may be written also in the conformally-flat form as

$$(ds^2)_{AdS_5 \times S^5} = \frac{1}{z^2}(dx^m dx_m + dz_M dz_M), \quad z^2 = z_M z_M, \quad M = 1, \dots, 6, \quad (2.9)$$

where  $dz_M dz_M = dz^2 + z^2 d\Omega_5(\gamma, \psi, \varphi_1, \varphi_2, \varphi_3)$ . The Poincaré coordinates are useful for the discussion of solutions representing open strings ending at the AdS boundary (see [22–24]).

## 2.2 String action, equations of motion and conserved angular momenta

The bosonic part of the  $AdS_5 \times S^5$  action (1.1) in the conformal gauge is

$$I_B = \frac{1}{2}T \int d\tau \int_0^{2\pi} d\sigma (L_{AdS} + L_S), \quad T = \frac{R^2}{2\pi\alpha'} = \frac{\sqrt{\lambda}}{2\pi}, \quad (2.10)$$

where  $\sqrt{\lambda} \equiv \frac{R^2}{\alpha'}$  ( $\lambda$  corresponds to ‘t Hooft coupling on the  $\mathcal{N}=4$  super Yang-Mills side),  $R$  is the (same) radius of  $AdS_5$  and  $S^5$  and

$$L_{AdS} = -\partial_a Y_P \partial^a Y^P - \tilde{\Lambda}(Y_P Y^P + 1), \quad L_S = -\partial_a X_M \partial^a X_M + \Lambda(X_M X_M - 1) \quad (2.11)$$

Here  $X_M$ ,  $M = 1, \dots, 6$  and  $Y_P$ ,  $P = 0, \dots, 5$  are the embedding coordinates of  $R^6$  with the Euclidean metric  $\delta_{MN}$  in  $L_S$  and of  $R^{2,4}$  with  $\eta_{PQ} = (-1, +1, +1, +1, +1, -1)$  in  $L_{AdS}$ , respectively ( $Y_P = \eta_{PQ} Y^Q$ ).  $\Lambda$  and  $\tilde{\Lambda}$  are the Lagrange multipliers imposing the two hypersurface conditions. The classical equations for (2.10) are

$$\partial^a \partial_a Y_P - \tilde{\Lambda} Y_P = 0, \quad \tilde{\Lambda} = \partial^a Y_P \partial_a Y^P, \quad Y_P Y^P = -1, \quad (2.12)$$

$$\partial^a \partial_a X_M + \Lambda X_M = 0, \quad \Lambda = \partial^a X_M \partial_a X_M, \quad X_M X_M = 1. \quad (2.13)$$

The action (2.10) is to be supplemented with the conformal gauge constraints

$$\dot{Y}_P \dot{Y}^P + Y'_P Y'^P + \dot{X}_M \dot{X}_M + X'_M X'_M = 0, \quad \dot{Y}_P Y'^P + \dot{X}_M X'_M = 0. \quad (2.14)$$

We will be interested in the closed string solutions with the world sheet as a cylinder, i.e. will impose the periodicity conditions

$$Y_P(\tau, \sigma + 2\pi) = Y_P(\tau, \sigma), \quad X_M(\tau, \sigma + 2\pi) = X_M(\tau, \sigma). \quad (2.15)$$

The action (2.10) is invariant under the  $SO(2, 4)$  and  $SO(6)$  rotations with the conserved (on-shell) charges

$$S_{PQ} = \sqrt{\lambda} \int_0^{2\pi} \frac{d\sigma}{2\pi} (Y_P \dot{Y}_Q - Y_Q \dot{Y}_P), \quad J_{MN} = \sqrt{\lambda} \int_0^{2\pi} \frac{d\sigma}{2\pi} (X_M \dot{X}_N - X_N \dot{X}_M) \quad (2.16)$$

There is a natural choice of the 3+3 Cartan generators of  $SO(2, 4) \times SO(6)$  corresponding to the 3+3 linear isometries of the  $AdS_5 \times S^5$  metric (2.5),(2.6), i.e. to the translations in the time  $t$ , in the 2 angles  $\phi_a$  and the 3 angles  $\varphi_i$ :

$$S_0 \equiv S_{50} \equiv E = \sqrt{\lambda} E, \quad S_1 \equiv S_{12} = \sqrt{\lambda} S_1, \quad S_2 \equiv S_{34} = \sqrt{\lambda} S_2, \quad (2.17)$$

$$J_1 \equiv J_{12} = \sqrt{\lambda} J_1, \quad J_2 \equiv J_{34} = \sqrt{\lambda} J_2, \quad J_3 \equiv J_{56} = \sqrt{\lambda} J_3. \quad (2.18)$$

### 2.3 Classical solutions: geodesics

We will be interested in classical solutions that have finite values of the AdS energy  $E$  and the spins  $S_r, J_i$  ( $r = 1, 2; i = 1, 2, 3$ ). The Virasoro condition will give a relation between the 6 charges in (2.17),(2.18) allowing one to express the energy in terms of the other 5, i.e.  $E = \sqrt{\lambda} E(S_r, J_i; k_s) = \sqrt{\lambda} E(\frac{S_r}{\sqrt{\lambda}}, \frac{J_i}{\sqrt{\lambda}}; k_s)$ . Here  $k_s$  stands for other (hidden) conserved charges, like ‘‘topological’’ numbers determining particular shape of the string (e.g., number of folds, spikes, winding numbers, etc).<sup>‡</sup>

For a solution to have a consistent semiclassical interpretation, it should correspond to a state of a quantum Hamiltonian which carries the same quantum numbers (and should thus be associated to a particular SYM operator with definite scaling dimension). It should represent a ‘‘highest-weight’’ state of a symmetry algebra, i.e. all other non-Cartan (non-commuting) components of the symmetry generators (2.16) should vanish; other members of the multiplet can be obtained by applying rotations to a ‘‘highest-weight’’ solution.<sup>§</sup>

Let us start with point-like strings, for which  $Y_P = Y_P(\tau)$ ,  $X_M = X_M(\tau)$  in (2.12)–(2.14), i.e. with massless geodesics in  $AdS_5 \times S^5$ . Then  $\Lambda, \tilde{\Lambda} = \text{const}$  (as follows directly from (2.12),(2.13)) and (2.14) implies that  $\Lambda = -\tilde{\Lambda} > 0$ . The generic massless geodesic in  $AdS_5 \times S^5$  can be of two ‘‘irreducible’’ types (up to a global  $SO(2, 4) \times SO(6)$  transformation): (i) massless geodesic that stays entirely within  $AdS_5$ ; (ii) a geodesic that runs along the time direction in  $AdS_5$  and wraps a big circle of  $S^5$ . In the latter case the angular motion in  $S^5$  provides an effective mass to a particle in  $AdS_5$ , i.e. the corresponding geodesic in  $AdS_5$  is a massive one,

$$Y_5 + iY_0 = e^{i\kappa\tau}, \quad X_5 + iX_6 = e^{i\kappa\tau}, \quad \kappa = \sqrt{\Lambda}, \quad Y_{1,2,3,4} = X_{1,2,3,4} = 0. \quad (2.19)$$

The only non-vanishing integrals of motion are  $E = J_3 = \sqrt{\lambda} \kappa$ , representing the energy and the  $SO(6)$  spin of this BPS state, corresponding to the BMN ‘‘vacuum’’ operator  $\text{tr}(Z^{J_3})$  in the SYM theory [13] (see also [12]).

The solution for a massless geodesic in  $AdS_5$  is a straight line in  $R^{2,4}$ ,  $Y_P(\tau) = A_P + B_P\tau$  with  $B_P B^P = A_P B^P = 0$ ,  $A_P A^P = -1$ . The  $SO(2, 4)$  angular momentum tensor in (2.16) is  $S_{PQ} = \sqrt{\lambda} (A_P B_Q - A_Q B_P)$ . It always has non-vanishing non-Cartan components [18], e.g., if  $Y_5 + iY_0 = 1 + ip\tau$ ,  $Y_3 = p\tau$ ,  $Y_{1,2,4} = 0$  we get

<sup>‡</sup>A simple example of an infinite-energy solution is an infinitely stretched string in  $AdS_2$  described (in conformal gauge) by  $t = \kappa\tau$ ,  $\rho = \rho(\sigma)$ ,  $\rho'^2 - \kappa^2 \cosh^2 \rho = 0$ , i.e.  $\cosh \rho = |\cos(\kappa\sigma)|^{-1}$ . It is formally  $2\pi$  periodic if  $\kappa = 1$ . In the Poincare patch the corresponding solution is  $z = \frac{\cos \kappa\sigma}{\cos \kappa\tau - \sin \kappa\sigma}$ ,  $x_0 = \frac{\sin \kappa\tau}{\cos \kappa\tau - \sin \kappa\sigma}$ .

<sup>§</sup>For a discussion of the relation of the above  $SO(2, 4)$  charges to the standard conformal group generators in the boundary theory and a relation between  $SO(2, 4)$  representations labelled by the AdS energy  $E = S_{50}$  and the dilatation operator  $D = S_{54}$  see [18] and refs. there.

$S_{50} = S_{53} = \sqrt{\lambda} p$ . This geodesic thus does not represent a “highest-weight” semiclassical state. In terms of Poincare coordinates (2.8) the massless geodesic is represented by  $x_0 = x_3 = p\tau$ ,  $z = a = \text{const}$ , i.e. it runs parallel to the boundary (reaching the boundary at spatial infinity where Poincare patch ends – that follows from its description in global coordinates).

Below we shall consider examples of extended ( $\sigma$ -dependent) solitonic string solutions of the equations (2.12),(2.13) subject to the constraints (2.14),(2.15) that have finite AdS energy and spins. The aim will be to find the expression for the energy  $E$  in terms of other charges.<sup>¶</sup> In general, a string all points of which can move fast in  $S^5$  will admit a “fast string” (BMN-type) limit in which  $E$  will have an analytic dependence on the square of string tension or on  $\lambda$  when expressed in terms of  $S_r$  and  $J_i$  and expanded in large total spin of  $S^5$  [15, 16]. At the same time, the energy of a string whose center is at rest or which moves only within the  $AdS_5$  will depend explicitly on  $\sqrt{\lambda}$  (i.e. will be non-analytic in  $\lambda$ ) [14, 16, 40].

### 3 Simplest rigid string solutions

Here we shall consider few simple explicit closed-string solutions of the non-linear equations (2.12),(2.13) which are “rigid”, i.e. for which the shape of the string does not change with time. These may be interpreted as examples of non-topological solitons of the  $AdS_5 \times S^5$  conformal-gauge string sigma model (2.10) on a 2-d cylinder  $(\tau, \sigma)$ .

#### 3.1 Examples of string solutions in flat space

Let us start with recalling several examples of string solutions in flat space. The flat-space string action and equations of motion in the conformal gauge are ( $\sqrt{-g}g^{ab} = \eta^{ab}$ ,  $x_\mu = \eta_{\mu\nu}x^\nu$ ,  $\eta_{\mu\nu} = \text{diag}(-1, 1, \dots, 1)$ )

$$I_B = \frac{1}{2}T_0 \int d^2\sigma \partial_a x_\mu \partial^a x^\mu, \quad \partial_+ \partial_- x^\mu = 0, \quad \partial_\pm x^\mu \partial_\pm x_\mu = 0. \quad (3.1)$$

The general solution of free equations  $x^\mu = x_0^\mu + p^\mu \tau + f_+^\mu(\sigma + \tau) + f_-^\mu(\sigma - \tau)$  subject to the closed string periodicity condition  $x^\mu(\tau, \sigma) = x^\mu(\tau, \sigma + 2\pi)$  is parametrized by constants,  $f_\pm^\mu(\sigma \pm \tau) = \sum_n (a_{(\pm)n}^\mu \cos[n(\sigma \pm \tau)] + b_{(\pm)n}^\mu \sin[n(\sigma \pm \tau)])$ , which are constrained by the Virasoro conditions. Simple explicit solutions representing semiclassical (coherent) states corresponding to particular quantum states in the string spectrum have only finite number of the Fourier modes excited. The Virasoro condition then implies a relation between the energy of the string  $E = T_0 \int d\sigma \partial_\tau x^0$  and its linear momenta, spins, oscillation numbers, etc. Some explicit examples are:

---

<sup>¶</sup>Early discussions of semiclassical strings in de Sitter and Anti de Sitter spaces appeared, e.g., in [32, 33]. The fact that in AdS space the string mass scales linearly with large quantum numbers (as opposed to square root Regge relation in flat space) was first observed in [33].

**Folded string rotating on a plane:**

$$x^0 = \kappa\tau, \quad x_1 + ix_2 = a \sin \sigma e^{i\tau}, \quad (3.2)$$

$$E = 2\pi T_0 \kappa = \sqrt{\frac{2}{\alpha'}} J, \quad J = \frac{a^2}{2\alpha'}. \quad (3.3)$$

**Spiky string rotating on a plane:**

$$x^0 = \kappa\tau, \quad x_1 + ix_2 = \frac{1}{2}a [e^{im(\tau+\sigma)} + me^{i(\tau-\sigma)}], \quad (3.4)$$

$$E = \sqrt{\frac{4m}{(m+1)\alpha'}} J, \quad \kappa = am, \quad J = \frac{a^2 m(m+1)}{4\alpha'}. \quad (3.5)$$

Here  $m+1$  is the number of spikes, i.e.  $m=1$  is the case of the folded string.<sup>||</sup>

**Circular string rotating in two orthogonal planes of  $R^4$ :**

$$x^0 = \kappa\tau, \quad x_1 + ix_2 = a e^{i(\tau+\sigma)}, \quad x_3 + ix_4 = a e^{i(\tau-\sigma)} \quad (3.6)$$

$$E = \frac{\kappa}{\alpha'} = \sqrt{\frac{4}{\alpha'}} J, \quad J_1 = J_2 = J = \frac{a^2}{\alpha'}. \quad (3.7)$$

Here  $J_1 = J_{12}$ ,  $J_2 = J_{34}$  are the values of the orbital momentum.

**Circular string pulsating in one plane:**

$$x^0 = \kappa\tau, \quad x_1 + ix_2 = a \sin \tau e^{i\sigma}, \quad (3.8)$$

$$E = 2\pi T_0 \kappa = \sqrt{\frac{2}{\alpha'}} N, \quad N = \frac{a^2}{2\alpha'}. \quad (3.9)$$

Here  $N$  is the oscillation number (an adiabatic invariant). This solution is formally not rigid but is very similar – the shape of the string remains circular, only its radius changes with time. An example of a non-rigid solution is a “kinky string” [34] for which the string has a shape of a quadrangle at the initial moment in time, then shrinks to diagonal due to the tension, then expands back, etc.

### 3.2 Circular rotating strings: rational solutions

A simple subclass of “rational” solutions of the  $AdS_5 \times S^5$  equations (2.12),(2.13) is found by assuming that  $\Lambda, \tilde{\Lambda} = \text{const}$  [16, 35]. In this case  $Y_P$  and  $X_M$  are given by simple trigonometric solutions of the linear 2-d massive scalar equation and one is just to make sure that the constant parameters are such that all the constraints in (2.12)–(2.15) are satisfied. An example is a circular string solution in  $R_t \times S^5$  part of  $AdS_5 \times S^5$  which is a direct analog of the circular 2-spin solution (3.6) [16] (see (2.4))

$$Y_0 = e^{i\kappa\tau}, \quad X_1 = \frac{a}{\sqrt{2}} e^{im(\tau+\sigma)}, \quad X_2 = \frac{a}{\sqrt{2}} e^{im(\tau-\sigma)}, \quad X_3 = \sqrt{1-a^2}, \quad (3.10)$$

$$J_1 = J_2 \equiv J = \frac{ma^2}{2} = \frac{\kappa^2}{4m}, \quad E = \sqrt{\lambda} \kappa = \sqrt{4m\sqrt{\lambda}} J. \quad (3.11)$$

Here  $m$  is a winding number,  $\tilde{\Lambda} = \kappa^2$ ,  $\Lambda = 0$ , i.e. the  $S^5$  part of the solution is essentially the same as in flat space: the string rotates on  $S^3$  of radius  $a \leq 1$  inside  $S^5$  of radius

<sup>||</sup>The relation between (3.4) and (3.2) for  $m=1$  involves  $\sigma \rightarrow \sigma + \frac{\pi}{2}$ .

1. The semiclassical spin parameter  $J$  is bounded from above, i.e. the fast-string BMN-type limit ( $J \rightarrow \infty$ ) cannot be realised. Instead, there is a smooth small spin ( $J \rightarrow 0$ ) or “small-string” limit ( $a \rightarrow 0$ ) in which the Regge form of the energy is to be expected. Remarkably, the exact expression for the classical string energy has the same “Regge” form as in flat space (3.7) with  $\frac{1}{\alpha'} \rightarrow \sqrt{\lambda}$ . This solution is thus a semiclassical analog [36] of a “short” quantum string for which the energy should scale (for fixed charges) as  $E \sim \sqrt{\sqrt{\lambda}}$  [37]. The solution (3.10) has an obvious generalization to the case of the 3-rd non-zero spin in  $S^5$  [16]: one needs to consider a non-zero  $X_3 = \sqrt{1 - a^2} e^{i w' \tau}$ .

There is a different solution (with  $\Lambda = w^2 - m^2$ ) describing a circular string with two equal spins moving on a “big”  $S^3 \subset S^5$  [16]

$$Y_0 = e^{i\kappa\tau}, \quad X_1 = \frac{1}{\sqrt{2}} e^{i(w\tau+m\sigma)}, \quad X_2 = \frac{1}{\sqrt{2}} e^{i(w\tau-m\sigma)}, \quad X_3 = 0, \quad (3.12)$$

$$J_1 = J_2 \equiv J = \frac{1}{2}w, \quad \kappa^2 = w^2 + m^2, \quad E = \sqrt{(2J)^2 + \lambda m^2}. \quad (3.13)$$

The two solutions coincide when  $a = 1$  in (3.10) and  $w = m$  in (3.12). This solution admits the fast-string limit in which ( $J \gg 1$ )

$$E = 2J + \frac{\lambda m^2}{4J} - \frac{\lambda^2 m^4}{64J^3} + O\left(\frac{\lambda^3}{J^5}\right), \quad (3.14)$$

but it does not have a small-string limit as here the radius of the string is always 1: even though  $J$  may become small, the energy does not go to zero due to string winding around big circle of  $S^5$ . In contrast to (3.10), this solution is unstable under small perturbations [16, 38].

There is another counterpart of the flat-space solution (3.6) in  $AdS_5 \times S^5$  when the circular string rotates solely in  $AdS_5$  [16, 35] (here we choose the winding number to be  $m = 1$ )

$$Y_0 = \sqrt{1 + 2r^2} e^{i\kappa\tau}, \quad Y_1 = r e^{i(w\tau+\sigma)}, \quad Y_2 = r e^{i(w\tau-\sigma)}. \quad (3.15)$$

Here  $r = \sinh \rho_0 = \frac{1}{2}\kappa$ ,  $w^2 = \kappa^2 + 1$  and the energy  $E = \sqrt{\lambda}E$ . The two equal spins  $S_1 = S_2 = \frac{1}{2}S = \sqrt{\lambda}S$  and the energy are related by the parametric equations  $S = \frac{1}{4}\kappa^2\sqrt{\kappa^2 + 1}$ ,  $E = \kappa + \frac{1}{2}\kappa^3$ . This solution again admits a “small-string” limit ( $S \rightarrow 0$ ) in which it represents a small circular string rotating around its c.o.m. in the two orthogonal planes in the central ( $\rho \approx 0$  or “near-flat”, see (2.5)) region of  $AdS_5$ . In the small spin limit  $S \ll 1$  [36]

$$E = \sqrt{4\sqrt{\lambda}S} \left[ 1 + \frac{S}{\sqrt{\lambda}} - \frac{3S^2}{2\lambda} + O\left(\frac{S^3}{\lambda^{3/2}}\right) \right]. \quad (3.16)$$

Here in contrast to the  $J_1 = J_2$  solution (3.10) the classical energy contains non-trivial “curvature” corrections which modify the leading-order flat-space Regge behavior. In the opposite large spin limit  $S \gg 1$  we get [16, 35, 40]

$$E = 2S + \frac{3}{4}(4\lambda S)^{1/3} + O(S^{-1/3}). \quad (3.17)$$

Yet another  $AdS_5 \times S^5$  counterpart of the flat-space solution (3.6) is found by having a circular string rotating both in  $AdS_5$  and in  $S^5$  (we choose again the winding numbers in  $\sigma$  to be 1)

$$Y_0 = \sqrt{1+r^2} e^{i\kappa\tau}, \quad Y_1 = r e^{i(w\tau+\sigma)}, \quad X_1 = a e^{i(\tau-\sigma)}, \quad X_2 = \sqrt{1-a^2} \quad (3.18)$$

Here  $w^2 = \kappa^2 + 1$  and  $r = \sinh \rho_0$  and  $a = \sin \gamma_0$  determine the size of the string in  $AdS_5$  and  $S^5$  respectively (cf. (2.5),(2.6)). The conformal gauge conditions (2.14) imply  $(1+r^2)\kappa^2 = r^2(w^2+1) + 2a^2$ ,  $r^2w = a^2$  and thus for this solution one has  $S = r^2w = J = a^2 \leq 1$ , i.e.  $S = J \leq \sqrt{\lambda}$ . Also,  $E = (1+r^2)\kappa = \kappa + \frac{S\kappa}{\sqrt{\kappa^2+1}}$ , where  $\kappa$  satisfies  $\kappa^2 = \frac{2S}{\sqrt{\kappa^2+1}} + 2S$  which is readily solved. In the small  $S$  limit one finds (cf. (3.16))

$$E = \sqrt{4\sqrt{\lambda}S} \left[ 1 + \frac{S}{2\sqrt{\lambda}} - \frac{5S^2}{8\lambda} + O\left(\frac{S^3}{\lambda^{3/2}}\right) \right]. \quad (3.19)$$

In the small-size or  $S = J \rightarrow 0$  limit (when  $w \rightarrow 1$ ,  $r \rightarrow a \rightarrow 0$ ) this solution reduces to the flat-space one (3.6) with the energy taking the form (3.7).

At the  $S = J = 1$  point (where  $a = 1$ ,  $\kappa = \sqrt{3}$ ,  $w = 2$ ,  $r = \sqrt{2}$ ) this ‘‘small-string’’  $S = J$  solution coincides with the ‘‘large-string’’  $S = J$  solution discussed in [35, 41]

$$Y_0 = \sqrt{1+r^2} e^{i\kappa\tau}, \quad Y_1 = r e^{i(w\tau+\sigma)}, \quad X_1 = e^{i(\omega\tau-\sigma)}, \quad (3.20)$$

$$w^2 = \kappa^2 + 1, \quad S = r^2w = \omega = J. \quad (3.21)$$

Then  $E = \kappa + \frac{S\kappa}{\sqrt{\kappa^2+1}}$ , where  $\kappa(S)$  satisfies  $\kappa^2 = \frac{2S}{\sqrt{\kappa^2+1}} + S^2 + 1$ . The cubic equation for  $\kappa^2$  admits two real solutions  $\kappa^{(1,2)} = \sqrt{1 + \frac{1}{2}S^2 \pm \frac{1}{2}S\sqrt{8 + S^2}}$ . The first solution is defined for any  $S \geq -1$  and the corresponding energy [36]

$$E = \sqrt{1 + \frac{1}{2}S^2 + \frac{1}{2}S\sqrt{8 + S^2}} \left[ 1 + \frac{S}{\sqrt{2 + \frac{1}{2}S^2 + \frac{1}{2}S\sqrt{8 + S^2}}} \right] \quad (3.22)$$

admits a regular large  $S$  expansion as in (3.14) [35, 41]:

$$E = 2S + \frac{\lambda}{S} - \frac{5\lambda^2}{4S^3} + O\left(\frac{\lambda^3}{S^5}\right). \quad (3.23)$$

In the small  $S$  expansion we get  $E = \sqrt{\lambda} + \sqrt{2} S + \frac{S^2}{4\sqrt{\lambda}} + \dots$ , i.e. this solution does not have the flat-space Regge asymptotics; this is not surprising since here the string is wrapped on a big circle of  $S^5$  and its tension gives a large contribution to the energy even for small spin.

The above examples illustrate possible patterns of behaviour of the classical string energy on the string tension and conserved spins in different limits. They should be reproducible from the exact results for the string spectrum in appropriate semiclassical string limits.

### 3.3 Rigid string ansatz: reduction to 1-d Neumann system

The above examples of solutions in  $AdS_5 \times S^5$  are special cases of a rigid string ansatz for which the shape of the string does not change with time  $\tau$  or the AdS time  $t$ . Making such an ansatz and substituting it into the equations (2.12),(2.13) one finds that they can be obtained from a 1-d integrable action describing an oscillator on a sphere – the Neumann model [42, 35, 16]. Along with the integrability of the equations describing geodesics in  $AdS_5 \times S^5$  this reduction of the  $AdS_5 \times S^5$  string sigma model to an integrable 1-d system is a simple illustration of the *integrability* of this 2-d theory.

The general solution of the resulting equations can then be written in terms of hyper-elliptic (genus 2 surface) functions, with the rational solutions discussed above and the elliptic solutions described below in the next section being the important special cases. The general rigid string ansatz may be written as (see (2.4))

$$Y_r = z_r(\sigma) e^{i\omega_r\tau} \quad (r = 0, 1, 2) ; \quad X_i = z_i(\sigma) e^{iw_i\tau} \quad (i = 1, 2, 3) \quad (3.24)$$

Here  $\omega_{1,2}$  and  $w_i$  are rotation frequencies and  $z_r$  and  $z_i$  (which are, in general, complex) satisfy

$$z_r = r_r e^{i\beta_r}, \quad \eta^{rs} r_r r_s = -1, \quad z_i = r_i e^{i\alpha_i}, \quad r^i r_i = 1, \quad (3.25)$$

$$r_r(\sigma + 2\pi) = r_r(\sigma), \quad \beta_r(\sigma + 2\pi) = \beta_r(\sigma) + 2\pi k_r, \quad (3.26)$$

$$r_i(\sigma + 2\pi) = r_i(\sigma), \quad \alpha_i(\sigma + 2\pi) = \alpha_i(\sigma) + 2\pi m_i. \quad (3.27)$$

Here  $\eta_{rs} = (-1, 1, 1)$ ,  $k_r$  and  $m_i$  (which are the “winding numbers” for the corresponding isometric angles in (2.4)) are integers. We assume that  $\beta_0 = 0$ ,  $k_0 = 0$ ,  $\omega_0 \equiv \kappa$ . The corresponding Cartan charges are (cf. (2.16),(2.17),(2.18))\*\*  $S_r = \omega_r \int_0^{2\pi} \frac{d\sigma}{2\pi} r_r^2(\sigma)$ ,  $J_i = w_i \int_0^{2\pi} \frac{d\sigma}{2\pi} r_i^2(\sigma)$ . The equations for the remaining “dynamical” variables  $r_r$  and  $r_i$  can be derived from the following 1-d “mechanical” Lagrangian

$$L = \eta^{rs} (z'_r z'_s{}^* - \omega_r^2 z_r z_s^*) - \tilde{\Lambda} (\eta^{rs} z_r z_s^* + 1) + z'_i z'_i{}^* - w_i^2 z_i z_i^* + \Lambda (z_i z_i^* - 1). \quad (3.28)$$

The trajectory of this effective “particle” belonging to a product of a 2-hyperboloid ( $r_r$ ) and 2-sphere ( $r_i$ ) gives the profile of the string. The angular parts of  $z_r$  and  $z_i$  can be easily separated leading to an effective Lagrangian for a particle on a constant curvature surface with an “ $r^2 + r^{-2}$ ” potential or to a special case of a 1-d integrable Neumann system – the Neumann-Rosochatius system [35]. The corresponding 2+2 integrals of motion can be explicitly written down [42, 35]. The resulting solutions represent, in particular, folded or circular bended wound rotating rigid strings.

For example, such closed string solutions in  $AdS^5$  will be parametrised by the frequencies  $\omega_0 = \kappa, \omega_i = (\omega_1, \omega_2)$  as well by two integrals of motion  $b_k$ .  $(\omega_i, b_k)$  may be viewed as independent coordinates on the moduli space of these solitons. The closed string periodicity condition implies that the solutions will be classified by two integer “winding numbers”  $n_i$  related to  $\omega_r$  and  $b_i$ . In general, the energy  $E$  will be a function

---

\*\*Here  $E = S_0$ . All other components of the conserved angular momentum tensors in (2.16) vanish automatically if all the frequencies are different [42], but their vanishing should be checked if 2 of the 3 frequencies are equal.

not only of  $S_1, S_2$  but also of  $n_i$ . Depending on the values of these parameters the string's shape may be of the two types: (i) “folded”, i.e. having a shape of an interval, or (ii) “circular”, i.e. having a shape of a circle. A folded string may be straight as in the one-spin case [14] or bent [42,43]. A “circular” string may be a round circle as in [16] or may have a more general “bent circle” shape. Some of such solutions will be discussed explicitly below.

## 4 Spinning rigid strings in $AdS_5 \times S^5$ : elliptic solutions

In this section we shall consider an important example of a non-trivial rigid string solution describing a folded spinning string in  $AdS_3$  part of  $AdS_5$  [44,14]. We shall then discuss some of its generalizations and similar solutions described in terms of elliptic functions.

### 4.1 Folded spinning string in $AdS_3$

Let us consider a rigid string moving in  $AdS_3$  part  $ds^2 = -\cosh^2 \rho dt^2 + d\rho^2 + \sinh^2 \rho d\phi^2$  of  $AdS_5$  (2.5), i.e.  $Y_0 = \cosh \rho(\sigma) e^{i\kappa\tau}$ ,  $Y_1 = \sinh \rho(\sigma) e^{i\omega\tau}$ , or

$$t = \kappa \tau, \quad \phi = \omega \tau, \quad \rho = \rho(\sigma) = \rho(\sigma + 2\pi) . \quad (4.1)$$

This ansatz satisfies the equations for  $t$  and  $\phi$  while for  $\rho$  we get 1-d sinh-Gordon equation  $\rho'' = \frac{1}{2}(\kappa^2 - \omega^2) \sinh(2\rho)$ . Its first integral satisfying the Virasoro condition (2.14) leads to the following solution

$$\rho'^2 = \kappa^2 \cosh^2 \rho - \omega^2 \sinh^2 \rho, \quad (4.2)$$

$$\sinh \rho(\sigma) = \frac{k}{\sqrt{1-k^2}} \operatorname{cn}(\omega \sigma + \mathbf{K} | k^2), \quad k \equiv \frac{\kappa}{\omega} . \quad (4.3)$$

Here we assumed that  $\rho(0) = 0$ ;  $\operatorname{cn}$  is the standard elliptic function and  $\mathbf{K} \equiv \mathbf{K}(k^2) = \int_0^{\pi/2} du (1 - k^2 \sin^2 u)^{-1/2}$  is the complete elliptic integral of the first kind. This solution describes a folded closed string rotating around its center of mass and generalizes the flat-space solution (3.2) (for  $\sigma \rightarrow 0$  we get  $\sinh \rho \rightarrow a \sin \sigma$ ,  $a = \frac{k}{\sqrt{1-k^2}}$ ). In (4.3)  $\sigma$  varies from 0 to  $\frac{\pi}{2}$  with  $\rho$  changing from 0 to its maximal value  $\rho_0$ ,  $\coth \rho_0 = \frac{\omega}{\kappa} = k^{-1}$ . The full ( $2\pi$  periodic) folded closed string solution is found by gluing together four such functions  $\rho(\sigma)$  on  $\frac{\pi}{2}$  intervals to cover the full  $0 \leq \sigma \leq 2\pi$  interval. The periodicity condition  $2\pi = \int_0^{2\pi} d\sigma = 4 \int_0^{\rho_0} \frac{d\rho}{\sqrt{\kappa^2 \cosh^2 \rho - \omega^2 \sinh^2 \rho}}$  implies a relation between the parameters  $\kappa$  and  $\omega$ , i.e.  $\kappa = \frac{2k}{\pi} \mathbf{K}$ ,  $\omega = \frac{2}{\pi} \mathbf{K}$ . The classical energy  $E = \sqrt{\lambda} \mathbf{E}$  and the spin  $S = \sqrt{\lambda} \mathbf{S}$  are expressed in terms of the complete elliptic integrals  $\mathbf{K} = \mathbf{K}(k^2)$  and  $\mathbf{E} = \mathbf{E}(k^2) = \int_0^{\pi/2} du (1 - k^2 \sin^2 u)^{1/2}$

$$\mathbf{E} = \frac{2}{\pi} \frac{k}{1-k^2} \mathbf{E}, \quad \mathbf{S} = \frac{2}{\pi} \left( \frac{1}{1-k^2} \mathbf{E} - \mathbf{K} \right) . \quad (4.4)$$

Solving for  $k$  gives the relation  $E = E(S)$ . The expression for  $E(S)$  can be easily found in the two limiting cases: (i) large spin or long string limit:  $\rho_0 \rightarrow \infty$ , i.e.  $k \rightarrow 1$ , and (ii) small spin or short string limit:  $\rho_0 \rightarrow 0$ , i.e.  $k \rightarrow 0$ . In the first limit the string's ends are close to the boundary of  $AdS_5$  and one obtains [14, 15, 45]

$$E = S + \frac{\sqrt{\lambda}}{\pi} \left[ \ln\left(\frac{8\pi}{\sqrt{\lambda}} S\right) - 1 \right] + \frac{\lambda}{2\pi^2} \frac{\ln\left(\frac{8\pi}{\sqrt{\lambda}} S\right) - 1}{S} + O\left(\frac{\ln^2 S}{S^2}\right), \quad S \gg 1. \quad (4.5)$$

The coefficient of the  $\ln S$  term [14] is governed by the strong-coupling limit of the so-called ‘‘scaling function’’ (cusp anomaly) and the subleading terms can be shown to obey non-trivial reciprocity relations [46, 45] (see [47]). The leading  $S$  term in (4.5) [44] may be interpreted as being due to the fold points of the string moving (in the strict  $S = \infty$  limit) along null lines at the boundary while the  $\ln S$  term [14] is due to the stretching of the string (this term is string length times its tension). Indeed, in the large spin limit or  $\kappa, \omega \gg 1$  the solution (4.3) with  $\sigma \in (0, \frac{\pi}{2})$  simplifies to [15, 48]<sup>††</sup>

$$t = \kappa \tau, \quad \phi = \omega \tau, \quad \rho = \kappa \sigma, \quad \kappa = \omega \gg 1. \quad (4.6)$$

This very simple form of the asymptotic large spin solution allows one to compute quantum 1-loop [15] and 2-loop [11] corrections to the energy (see [12, 31]).

Let us mention also that the asymptotic solution (4.6) with  $\kappa \rightarrow \infty$  describing infinite string with folds reaching the AdS boundary and capturing the coefficient of the  $\ln S$  term in  $E - S$  (4.5) is closely related to the ‘‘null cusp’’ open string solution [50] describing an open string (euclidean) world surface ending on the two orthogonal null lines at the boundary of  $AdS_5$  in Poincare coordinates,  $z = \sqrt{2x^+x^-}$ ,  $x^\pm = x_0 \pm x_1$  (see (2.8)). In the conformal gauge

$$z = \sqrt{2} e^{\sqrt{2}\tau}, \quad x^+ = e^{\sqrt{2}(\tau+\sigma)}, \quad x^- = e^{\sqrt{2}(\tau-\sigma)}. \quad (4.7)$$

This solution written in the embedding coordinates (2.7) is then equivalent to (4.6) after a euclidean continuation ( $\tau \rightarrow i\tau$ ) and an  $SO(2, 4)$  coordinate transformation [51]. This explains (from strong-coupling or semiclassical string perspective) why the coefficient of the  $\ln S$  term in (4.5) can be interpreted as a cusp anomalous dimension (a dimension of a Wilson loop defined by null cusp, see also [47, 22]).

In the small spin or ‘‘short string’’ limit, when the string is rotating in the central ( $\rho = 0$ ) region of  $AdS_3$  we get the same flat-space (3.3) Regge type asymptotics [14, 15, 49] as in the circular string cases in (3.16), (3.19)

$$E = \sqrt{2\sqrt{\lambda}} S \left[ 1 + \frac{3S}{8\sqrt{\lambda}} + O(S^2) \right], \quad S \ll 1. \quad (4.8)$$

## 4.2 Some generalizations and similar solutions

The above  $AdS_3$  solution is special having minimal energy for given spin. It has several generalizations. One may consider a similar solution of circular shape with several spikes

<sup>††</sup>This is readily seen directly from (4.2) in the limit when  $\kappa \rightarrow \omega$ .

[52] that is the analog of the spiky string in flat space (3.4).<sup>‡‡</sup> For the spiky string in AdS the large spin limit of the energy is (cf. (4.5))

$E = S + \frac{\sqrt{\lambda}}{2\pi} \left( \ln \frac{16\pi S}{\sqrt{\lambda} n} - 1 + \ln \sin \frac{\pi}{n} \right) + \dots$ , where  $n$  is the number of spikes ( $n = 2$  is the folded string case). The large-spin asymptotic solution consists of  $n$  segments each of which is conformally equivalent to the limit (4.6) of the folded string [53].

One may also find similar rigid string solutions with  $\ln S$  scaling of  $E - S$  at large spin with two non-zero spins  $S_1, S_2$ , i.e. moving in the whole  $AdS_5$  [16, 42, 54, 55, 43] subject to the rigid string ansatz (3.24), i.e.  $t = \kappa\tau$ ,  $\rho = \rho(\sigma)$ ,  $\theta = \theta(\sigma)$ ,  $\phi_1 = \omega_1\tau$ ,  $\phi_2 = \omega_2\tau$ . The simplest circular solution of that type is a round string [16] with  $\rho = \rho_0 = \text{const}$ ,  $\theta = \frac{\pi}{4}$ ,  $\omega_1 = \omega_2$  and thus with  $S_1 = S_2$  already discussed above in (3.15)-(3.17). It does not, however, represent a state with a minimal energy for given values of the spins. To get a stable lower-energy solution with  $S_1 = S_2$  one is to relax the  $\rho = \text{const}$  condition, allowing the string to develop, in the large spin limit, long arcs stretching to infinity (i.e. to the boundary of  $AdS_5$ ) and carrying most of the energy. Then for a particular  $S_1 = S_2 = S$  string of circular shape with with 3 cusps described by an elliptic function limit of a general hyperelliptic solution of the Neumann model (3.28) one finds for its energy [54, 43]:  $E = 2S + \frac{3}{2} \times \frac{\sqrt{\lambda}}{\pi} \ln S + \dots$ . Similar open-string solutions were discussed in [56].

Another important generalization of the folded spinning string in  $AdS_3$  is found by adding an angular momentum  $J$  in  $S^5$ , i.e. by assuming in addition to (4.1) that the string orbits a big circle in  $S^5$ ,  $\varphi = \nu\tau$  [15]. The  $AdS_5$  and  $S^5$  parameters are coupled via the Virasoro constraint (4.2) which is modified to  $\rho'^2 = (\kappa^2 - \nu^2) \cosh^2 \rho - (\omega^2 - \nu^2) \sinh^2 \rho$  so that the relations (4.3)-(4.4) have straightforward generalizations. The resulting expression for the energy  $E = \sqrt{\lambda} E(S, J)$  (with  $J = \nu$ ) can be expanded in several limits. In the short string limit with  $J \ll 1$ ,  $S \ll 1$  one finds [15]

$$E = \sqrt{J^2 + 2\sqrt{\lambda} S} + \dots \quad (4.9)$$

This limit probes the  $\rho \approx 0$  region of  $AdS_5$  where the energy spectrum should thus be as in flat space, i.e. should be just a relativistic expression for the energy of a string moving with momentum  $J$  and rotating around its c.o.m. with spin  $S$ , i.e.  $E^2 - J^2 = 2\sqrt{\lambda} S + \dots$ . If the boost energy is smaller than the rotational one,  $J^2 \ll S$ , then  $E \approx \sqrt{2\sqrt{\lambda} S} + O(\frac{J^2}{\sqrt{S}})$ . For strings with  $J \gg 1$  and  $\frac{J}{S} = \text{fixed}$  we get a regular “fast-string” expansion as in (3.14),(3.23),  $E = J + S + \frac{\lambda S}{2J^2} + \dots$ . In the limit when  $S$  is large the string can become very long and its ends approach the boundary of  $AdS_5$ . The analog of the asymptotic solution (4.6) is

$$\rho = \mu\sigma, \quad \kappa = \omega, \quad \mu^2 = \kappa^2 - \nu^2, \quad \kappa, \mu, \nu \gg 1. \quad (4.10)$$

The spin  $S$  and  $\mu$  are related by  $\mu \approx \frac{1}{\pi} \ln S + \dots$  so in the limit when  $\kappa, \omega, \mu, \nu$  are large with their ratios fixed, i.e.  $S \gg 1$  with  $\ell \equiv \frac{\pi J}{\ln S} = \text{fixed}$  we get [57, 48, 58]

$$E = S + \sqrt{J^2 + \frac{\lambda}{\pi^2} \ln^2 S} + \dots = S + \frac{\sqrt{\lambda}}{\pi} f_0(\ell) \ln S + \dots, \quad (4.11)$$

<sup>‡‡</sup>The spiky string is described (in conformal gauge) by a generalization of the ansatz in (3.24) discussed below.

where  $f_0(\ell) = \sqrt{1 + \ell^2}$ . Again, the fast-string expansion in the limit when  $\ln S \ll J$  (i.e.  $\ell \gg 1$ ) gives a regular series in  $\lambda$  [15],  $E = S + J + \frac{\lambda}{2\pi^2 J} \ln^2 \frac{S}{J} + \dots$ . This solution has also a generalization to the case of winding along  $S^1$  in  $S^5$  [59, 61].

There is also an analog of the folded spinning string in  $S^5$  [14], where the string is spinning on  $S^2$  with its center at rest. The corresponding ansatz is  $X_1 + iX_2 = \sin \psi(s) e^{iw\tau}$ ,  $X_3 = \cos \psi(s)$  where  $\psi$  solves the 1-d sine-Gordon equation. The short string (small spin) limit here gives again the flat-space Regge behaviour,  $E = \sqrt{2\sqrt{\lambda}J} \left(1 + \frac{J}{8\sqrt{\lambda}} + \dots\right)$ . For large spin  $E = J + 2\frac{\sqrt{\lambda}}{\pi} + O(J^{-1})$ .

There is a  $(J_1, J_2)$  generalization of this solution discussed in [39, 60]. The AdS spiky string of [52] also admits a generalization to the case of non-zero  $J$  or/and winding in  $S^1$  of  $S^5$  [62]; in this case the spikes are rounded up.

Among other elliptic solutions let us mention also pulsating strings in  $AdS_5 \times S^5$  that generalize the flat space solution (3.8) [14, 63, 64, 40]; here the role of the spin is played by the adiabatic invariant – the oscillation number  $N = \frac{\sqrt{\lambda}}{2\pi} \int d\theta p_\theta$ . It is interesting to compare the large/small spin expansions of the classical string energy in the equations (3.14), (3.16), (3.17), (3.19), (3.23) and (4.5), (4.8) with what one finds for pulsating string solutions in  $AdS_3$  [63, 40] ( $N = \frac{N}{\sqrt{\lambda}}$ )

$$E = N + c_1 \sqrt{\sqrt{\lambda} N} + O(N^0), \quad N \gg 1, \quad c_1 = 0.7622\dots \quad (4.12)$$

$$E = \sqrt{2\sqrt{\lambda} N} \left[1 + \frac{5N}{8\sqrt{\lambda}} + O(N^2)\right], \quad N \ll 1, \quad (4.13)$$

and  $R \times S^2$  [63, 64]

$$E = N + \frac{\lambda}{4N} + O(N^{-2}), \quad N \gg 1, \quad (4.14)$$

$$E = \sqrt{2\sqrt{\lambda} N} \left[1 - \frac{N}{8\sqrt{\lambda}} + O(N^2)\right], \quad N \ll 1. \quad (4.15)$$

### 4.3 Spiky strings and giant magnons in $S^5$

An important class of rigid strings that are described by a slight generalization of the ansatz in (3.24) are strings with spikes [52, 65] and (bound states of) giant magnons [66–68] with several non-zero angular momenta. Both the spiky strings in  $S^5$  and the giant magnons can be described [69] by a generalization of the rigid string ansatz (3.24) of [42, 35]. It is possible to show that the giant magnon solutions are a particular limit of the spiky string solutions and that a giant magnon with two angular momenta can be interpreted as a superposition of two magnons moving with the same speed. Consider strings moving in  $R_t \times S^5$  part of  $AdS_5 \times S^5$  and described by the following generalization of the rigid string ansatz in (3.24) [69]

$$t = \kappa\tau, \quad X_i = z_i(\xi) e^{iw_i\tau}, \quad \xi \equiv \sigma + b\tau, \quad (4.16)$$

where  $z_i = r_i e^{i\alpha_i}$ ,  $z_i(\xi + 2\pi) = z_i(\xi)$ . Here  $b$  is a new parameter. The 1-d mechanical system for the functions  $z_i$  that follows from (2.13) is an integrable model: a generalization of the Neumann-Rosochatius one where a particle on a sphere is coupled also to a

constant magnetic field. This ansatz describes the  $S^5$  analog of the  $AdS_5$  spiky string of [52] with extra angular momenta [69]. The spiky string is built out of several arcs; in the limit when  $J_1 \rightarrow \infty$  with  $E - J_1 = \text{finite}$  the single arc is the giant magnon of [66] with an extra momentum  $J_2$  [68] (see also [70, 71]). In this limit  $\kappa \rightarrow \infty$  and it is natural to rescale  $\xi$  so that it takes values on an infinite line (a single arc is an open rather than a closed string). Then

$$E - J_1 = \sqrt{J_2^2 + \frac{\lambda}{\pi^2} \sin^2 \frac{p}{2}}, \quad (4.17)$$

where  $p$  is related to the length of the arc and may be interpreted as a momentum of the giant magnon [66]. The giant magnon may be viewed as a strong-coupling “image” of the elementary spin-chain magnon on the gauge-theory side.

One may also find a generalization of the giant magnon with two finite angular momenta  $J_2, J_3$  [69]. A single-spin folded string in  $S^2$  [14] in the limit when the folds approach the equator can be interpreted [66] as a superposition of two magnons with  $p = \pi$  and  $J_2 = 0$ . A generalization to the case of  $J_2, J_3 \neq 0$  is  $E - J_1 = \sqrt{J_2^2 + \frac{\lambda}{\pi^2}} + \sqrt{J_3^2 + \frac{\lambda}{\pi^2}}$ . When  $J_2 = J_3 = 0$ , one recovers the expression for the energy of two giant magnons with  $p = \pi$ , i.e.  $E - J_1 = 2\frac{\sqrt{\lambda}}{\pi}$  or the leading term in the folded spinning string energy in the limit  $J_1 \rightarrow \infty$ . Spiky strings with several spins were discussed also in [72–74].

Let us mention also some related rigid string elliptic solutions. A “helical” string solution interpolating between the folded or circular spinning string and the giant magnon with spin was constructed in [75]. Refs. [76, 77] found an “inverted” single-spike string wrapping the equator of  $S^2$  in  $S^5$  (see also [78]). Ref. [79] (see also [80] for a review) discussed a general family of “helical” string solutions in  $R_t \times S^3$  (which are most general elliptic solutions on  $R_t \times S^3$ ) interpolating between pulsating and single-spike strings which was obtained from the helical string of [75] by interchanging  $\tau$  and  $\sigma$  in  $S^3$  coordinates (this maps a string with large spin into a pulsating string with large winding number).

#### 4.4 Other approaches to constructing solutions

The integrability of the sigma model equations (2.12),(2.13) implies that one is able to construct large relevant class of solutions – “finite gap” solutions in terms of theta-functions [81]. Also one can construct new non-trivial solutions from given ones using “dressing” [82] or Bäcklund transformations [83]. Using the dressing method one may generate non-trivial solutions from simple ones, e.g., non-rigid or non-stationary (scattering) solutions from rigid string ones. Examples are scattering and bound states of giant magnons with several spins and arbitrary momenta [72, 84] or the single-spike solution of [76] from a static wrapped string and solutions with multiple spikes describing their scattering [77]. Similar methods can be applied also in the open-string (Wilson loop) setting [21] to find generalizations of the null cusp solution (4.7) [85].

An alternative approach to constructing explicit  $AdS_5 \times S^5$  string solutions of (2.12)–(2.14) is based on the Pohlmeyer reduction [25, 32, 33, 18, 66, 68, 75, 86–89]. The basic idea is to solve the Virasoro conditions (2.14) explicitly by introducing, instead of the string

coordinates  $(Y_P, X_M)$ , a new set of “current”-type variables. Then (2.12)–(2.14) become equivalent to a generalized sine-Gordon (non-abelian Toda) 2-d integrable system. Given a solitonic solution of this system one can then reconstruct the corresponding string solution by solving linear equations for  $(Y_P, X_M)$  with  $\tilde{\Lambda}$  and  $\Lambda$  in (2.12),(2.13) being given functions of  $(\tau, \sigma)$ . For example, in the case of a string on  $R_t \times S^2$  one may set  $t = \kappa\tau$  and then the three 3-vectors  $X_i, \partial_+ X_i, \partial_- X_i$  ( $i = 1, 2, 3$ ) will have only one non-trivial scalar product  $\partial_+ X_i \partial_- X_i \equiv \kappa^2 \cos 2\alpha = -\Lambda$ . The remaining dynamical equation takes the SG form:  $\partial_+ \partial_- \alpha + \frac{\kappa^2}{2} \sin 2\alpha = 0$ . The Pohlmeyer-reduced model for a string on  $R_t \times S^3$  is the complex SG model, while strings moving in  $AdS_5$  are related to generalized sinh-Gordon-type models. The giant magnon corresponds to the SG soliton [66] while its  $J_2 \neq 0$  generalization – to charged soliton of the complex SG model [68]. Various examples of solutions (multi giant magnons, spikes, etc.) obtained using this method can be found in [75, 88–90]. The approach based on the Pohlmeyer reduction was recently applied also to constructing open-string surfaces ending on null segments which generalize the null cusp solution [91, 92].

## References

- [1] M. B. Green and J. H. Schwarz, “Supersymmetrical String Theories,” *Phys. Lett. B* **109**, 444 (1982).
- [2] J. H. Schwarz, “Covariant Field Equations Of Chiral N=2 D=10 Supergravity,” *Nucl. Phys. B* **226**, 269 (1983).
- [3] M. Blau, J. M. Figueroa-O’Farrill, C. Hull and G. Papadopoulos, “A new maximally supersymmetric background of IIB superstring theory,” *JHEP* **0201**, 047 (2002) [arXiv:hep-th/0110242].
- [4] G. T. Horowitz and A. Strominger, “Black strings and P-branes,” *Nucl. Phys. B* **360**, 197 (1991). M. J. Duff and J. X. Lu, “The Selfdual Type IIB Superthreebrane,” *Phys. Lett. B* **273**, 409 (1991).
- [5] J. M. Maldacena, “The large N limit of superconformal field theories and supergravity,” *Adv. Theor. Math. Phys.* **2**, 231 (1998) [arXiv:hep-th/9711200].
- [6] O. Aharony, S. S. Gubser, J. M. Maldacena, H. Ooguri and Y. Oz, “Large N field theories, string theory and gravity,” *Phys. Rept.* **323**, 183 (2000) [arXiv:hep-th/9905111].
- [7] M. B. Green and J. H. Schwarz, “Covariant Description Of Superstrings,” *Phys. Lett. B* **136**, 367 (1984).
- [8] R. R. Metsaev and A. A. Tseytlin, “Type IIB superstring action in AdS(5) x S(5) background,” *Nucl. Phys. B* **533**, 109 (1998) [arXiv:hep-th/9805028].
- [9] M. Magro, “Review of AdS/CFT Integrability, Chapter II.3: Sigma Model, Gauge Fixing”, arXiv:1012.3988 [hep-th].
- [10] N. Drukker, D. J. Gross and A. A. Tseytlin, “Green-Schwarz string in AdS(5) x S(5): Semiclassical partition function,” *JHEP* **0004**, 021 (2000) [arXiv:hep-th/0001204].

- [11] R. Roiban, A. Tirziu and A. A. Tseytlin, “Two-loop world-sheet corrections in  $AdS_5 \times S^5$  superstring,” JHEP **0707**, 056 (2007) [arXiv:0704.3638]. R. Roiban and A. A. Tseytlin, “Strong-coupling expansion of cusp anomaly from quantum superstring,” JHEP **0711**, 016 (2007) [arXiv:0709.0681].
- [12] T. McLoughlin, “Review of AdS/CFT Integrability, Chapter II.2: Quantum Strings in  $AdS_5 \times S^5$ ”, arXiv:1012.3987 [hep-th].
- [13] D. E. Berenstein, J. M. Maldacena and H. S. Nastase, “Strings in flat space and pp waves from  $N = 4$  super Yang Mills,” JHEP **0204**, 013 (2002) [arXiv:hep-th/0202021].
- [14] S.S. Gubser, I.R. Klebanov and A.M. Polyakov, “A semi-classical limit of the gauge/string correspondence,” Nucl. Phys. B **636**, 99 (2002) [hep-th/0204051].
- [15] S. Frolov and A. A. Tseytlin, “Semiclassical quantization of rotating superstring in  $AdS(5) \times S(5)$ ,” JHEP **0206**, 007 (2002) [arXiv:hep-th/0204226].
- [16] S. Frolov and A. A. Tseytlin, “Multi-spin string solutions in  $AdS(5) \times S^5$ ,” Nucl. Phys. B **668**, 77 (2003) [arXiv:hep-th/0304255].
- [17] A. A. Tseytlin, “Semiclassical quantization of superstrings:  $AdS(5) \times S(5)$  and beyond,” Int. J. Mod. Phys. A **18**, 981 (2003) [arXiv:hep-th/0209116]. “Semiclassical strings and AdS/CFT,” in “Cargese 2004, String theory: From gauge interactions to cosmology”, 265-290 [arXiv:hep-th/0409296].
- [18] A. A. Tseytlin, “Spinning strings and AdS/CFT duality,” in “From Fields to Strings: Circumnavigating Theoretical Physics”, M. Shifman et al, eds. (World Scientific, 2004). vol. 2, 1648-1707. [arXiv:hep-th/0311139].
- [19] J. Plefka, “Spinning strings and integrable spin chains in the AdS/CFT correspondence,” Living Rev. Rel. **8**, 9 (2005) [arXiv:hep-th/0507136].
- [20] A. A. Tseytlin, “Quantum strings in  $AdS_5 \times S^5$  and AdS/CFT duality,” in: “Crossing the Boundaries: Gauge Dynamics at Strong Coupling: Honoring the 60th birthday of M. Shifman”, Minneapolis, 14-17 May 2009. Int. J. Mod. Phys. A **25**, 319 (2010) [arXiv:0907.3238 [hep-th]].
- [21] J. M. Maldacena, “Wilson loops in large  $N$  field theories,” Phys. Rev. Lett. **80**, 4859 (1998) [arXiv:hep-th/9803002]. L. F. Alday and J. M. Maldacena, “Gluon scattering amplitudes at strong coupling,” JHEP **0706**, 064 (2007) [arXiv:0705.0303].
- [22] R. Roiban, “Review of AdS/CFT Integrability, Chapter V.1: Scattering Amplitudes – a Brief Introduction”, arXiv:1012.4001 [hep-th].
- [23] J. Drummond, “Review of AdS/CFT Integrability, Chapter V.2: Dual Superconformal Symmetry”, arXiv:1012.4002 [hep-th].
- [24] L. F. Alday, “Review of AdS/CFT Integrability, Chapter V.3: Scattering Amplitudes at Strong Coupling”, arXiv:1012.4003 [hep-th].
- [25] K. Pohlmeyer, “Integrable hamiltonian systems and interactions through quadratic constraints,” Commun. Math. Phys. **46**, 207 (1976).

- [26] M. Luscher and K. Pohlmeyer, “Scattering Of massless lumps and nonlocal charges in the two-dimensional classical nonlinear sigma model,” Nucl. Phys. B **137**, 46 (1978).  
H. Eichenherr and M. Forger, “On The Dual Symmetry Of The Nonlinear Sigma Models,” Nucl. Phys. B **155**, 381 (1979).
- [27] I. Bena, J. Polchinski and R. Roiban, “Hidden symmetries of the AdS(5) x S5 superstring,” Phys. Rev. D **69**, 046002 (2004) [arXiv:hep-th/0305116].
- [28] S. Novikov, S.V. Manakov, L.P. Pitaevsky and V.E. Zakharov, “Theory of Solitons.The Inverse Scattering Method”. Consultants Bureau (1984), New York, USA, 276p.
- [29] V. A. Kazakov, A. Marshakov, J. A. Minahan and K. Zarembo, “Classical / quantum integrability in AdS/CFT,” JHEP **0405**, 024 (2004) [arXiv:hep-th/0402207]. N. Beisert, V. A. Kazakov, K. Sakai and K. Zarembo, “The algebraic curve of classical superstrings on AdS(5) x S5,” Commun. Math. Phys. **263**, 659 (2006) [arXiv:hep-th/0502226]. B. Vicedo, “Finite-g Strings,” arXiv:0810.3402 .
- [30] N. Gromov, “Integrability in AdS/CFT correspondence: Quasi-classical analysis,” J. Phys. A **42**, 254004 (2009).
- [31] S. Schäfer-Nameki, “Review of AdS/CFT Integrability, Chapter II.4: The Spectral Curve”, arXiv:1012.3989 [hep-th].
- [32] B.M. Barbashov and V.V. Nesterenko, “Relativistic String Model In A Space-Time Of A Constant Curvature, Commun. Math. Phys. **78**, 499 (1981).
- [33] H. J. De Vega and N. Sanchez, “Exact integrability of strings in D-Dimensional De Sitter space-time,” Phys. Rev. **D47**, 3394 (1993). H. J. de Vega, A. L. Larsen and N. G. Sanchez, “Semiclassical Quantization Of Circular Strings In De Sitter And Anti-De Sitter Space-Times,” Phys. Rev. D **51**, 6917 (1995) [arXiv:hep-th/9410219].
- [34] T. McLoughlin and X. Wu, “Kinky strings in AdS(5) x S5,” JHEP **0608**, 063 (2006) [arXiv:hep-th/0604193].
- [35] G. Arutyunov, J. Russo and A. A. Tseytlin, “Spinning strings in AdS(5) x S5: New integrable system relations,” Phys. Rev. D **69**, 086009 (2004) [arXiv:hep-th/0311004].
- [36] R. Roiban and A. A. Tseytlin, “Quantum strings in  $AdS_5 \times S^5$  : strong-coupling corrections to dimension of Konishi operator,” JHEP **0911**, 013 (2009) [arXiv:0906.4294].
- [37] S. S. Gubser, I. R. Klebanov and A. M. Polyakov, “Gauge theory correlators from non-critical string theory,” Phys. Lett. B **428**, 105 (1998) [arXiv:hep-th/9802109].
- [38] S. Frolov and A. A. Tseytlin, “Quantizing three-spin string solution in AdS(5) x S5,” JHEP **0307**, 016 (2003) [arXiv:hep-th/0306130].
- [39] S. Frolov and A. A. Tseytlin, “Rotating string solutions: AdS/CFT duality in non-supersymmetric sectors,” Phys. Lett. B **570**, 96 (2003) [arXiv:hep-th/0306143].
- [40] I. Y. Park, A. Tirziu and A. A. Tseytlin, “Semiclassical circular strings in AdS(5) and ‘long’ gauge field strength operators,” Phys. Rev. D **71**, 126008 (2005) [arXiv:hep-th/0505130].

- [41] I. Y. Park, A. Tirziu and A. A. Tseytlin, “Spinning strings in  $AdS(5) \times S^5$ : One-loop correction to energy in  $SL(2)$  sector,” *JHEP* **0503**, 013 (2005) [arXiv:hep-th/0501203].
- [42] G. Arutyunov, S. Frolov, J. Russo and A. A. Tseytlin, “Spinning strings in  $AdS(5) \times S^5$  and integrable systems,” *Nucl. Phys. B* **671**, 3 (2003) [arXiv:hep-th/0307191].
- [43] A. Tirziu and A. A. Tseytlin, “Semiclassical rigid strings with two spins in  $AdS_5$ ,” *Phys. Rev. D* **81**, 026006 (2010) [arXiv:0911.2417 [hep-th]].
- [44] H. J. de Vega and I. L. Egusquiza, “Planetoid String Solutions in 3 + 1 Axisymmetric Spacetimes,” *Phys. Rev. D* **54**, 7513 (1996) [arXiv:hep-th/9607056].
- [45] M. Beccaria, V. Forini, A. Tirziu and A. A. Tseytlin, “Structure of large spin expansion of anomalous dimensions at strong coupling,” *Nucl. Phys. B* **812**, 144 (2009) [arXiv:0809.5234].
- [46] B. Basso and G. P. Korchemsky, “Anomalous dimensions of high-spin operators beyond the leading order,” *Nucl. Phys. B* **775**, 1 (2007) [arXiv:hep-th/0612247].
- [47] L. Freyhult, “Review of  $AdS/CFT$  Integrability, Chapter III.4: Twist states and the cusp anomalous dimension”, arXiv:1012.3993 [hep-th].
- [48] S. Frolov, A. Tirziu and A. A. Tseytlin, “Logarithmic corrections to higher twist scaling at strong coupling from  $AdS/CFT$ ,” *Nucl. Phys. B* **766**, 232 (2007) [arXiv:hep-th/0611269].
- [49] A. Tirziu and A. A. Tseytlin, “Quantum corrections to energy of short spinning string in  $AdS_5$ ,” *Phys. Rev. D* **78**, 066002 (2008) [arXiv:0806.4758].
- [50] M. Kruczenski, “A note on twist two operators in  $N = 4$  SYM and Wilson loops in Minkowski signature,” *JHEP* **0212**, 024 (2002) [arXiv:hep-th/0210115].
- [51] M. Kruczenski, R. Roiban, A. Tirziu and A. A. Tseytlin, “Strong-coupling expansion of cusp anomaly and gluon amplitudes from quantum open strings in  $AdS_5 \times S^5$ ,” *Nucl. Phys. B* **791**, 93 (2008) [arXiv:0707.4254].
- [52] M. Kruczenski, “Spiky strings and single trace operators in gauge theories,” *JHEP* **0508**, 014 (2005) [arXiv:hep-th/0410226].
- [53] M. Kruczenski and A. A. Tseytlin, “Spiky strings, light-like Wilson loops and pp-wave anomaly,” *Phys. Rev. D* **77**, 126005 (2008) [arXiv:0802.2039].
- [54] A.L. Larsen and A. Khan, “Novel explicit multi spin string solitons in  $AdS(5)$ ,” *Nucl. Phys. B* **686**, 75 (2004) [arXiv:hep-th/0312184].
- [55] S. Ryang, “Folded three-spin string solutions in  $AdS(5) \times S^5$ ,” *JHEP* **0404**, 053 (2004) [arXiv:hep-th/0403180].
- [56] A. Irrgang and M. Kruczenski, “Double-helix Wilson loops: case of two angular momenta,” *JHEP* **0912**, 014 (2009) [arXiv:0908.3020].
- [57] A. V. Belitsky, A. S. Gorsky and G. P. Korchemsky, “Logarithmic scaling in gauge / string correspondence,” *Nucl. Phys. B* **748**, 24 (2006) [arXiv:hep-th/0601112].

- [58] J. G. Russo, “Anomalous dimensions in gauge theories from rotating strings in  $AdS(5) \times S(5)$ ,” JHEP **0206**, 038 (2002) [arXiv:hep-th/0205244].
- [59] S. Giombi, R. Ricci, R. Roiban, A. A. Tseytlin and C. Vergu, “Generalized scaling function from light-cone gauge  $AdS_5 \times S^5$  superstring,” JHEP **1006**, 060 (2010) [arXiv:1002.0018].
- [60] N. Beisert, S. Frolov, M. Staudacher and A. A. Tseytlin, “Precision spectroscopy of AdS/CFT,” JHEP **0310**, 037 (2003) [arXiv:hep-th/0308117].
- [61] M. Kruczenski and A. Tirziu, “Spiky strings in Bethe Ansatz at strong coupling,” Phys. Rev. D **81**, 106004 (2010) [arXiv:1002.4843].
- [62] R. Ishizeki, M. Kruczenski, A. Tirziu and A. A. Tseytlin, “Spiky strings in  $AdS_3 \times S^1$  and their AdS-pp-wave limits,” Phys. Rev. D **79**, 026006 (2009) [arXiv:0812.2431].
- [63] J. A. Minahan, “Circular semiclassical string solutions on  $AdS(5) \times S^5$ ,” Nucl. Phys. B **648**, 203 (2003) [arXiv:hep-th/0209047]. J. Engquist, J. A. Minahan and K. Zarembo, “Yang-Mills duals for semiclassical strings on  $AdS(5) \times S^5$ ,” JHEP **0311**, 063 (2003) [arXiv:hep-th/0310188].
- [64] M. Kruczenski and A. A. Tseytlin, “Semiclassical relativistic strings in  $S^5$  and long coherent operators in  $N = 4$  SYM theory,” JHEP **0409**, 038 (2004) [arXiv:hep-th/0406189].
- [65] S. Ryang, “Wound and rotating strings in  $AdS(5) \times S^5$ ,” JHEP **0508**, 047 (2005) [arXiv:hep-th/0503239].
- [66] D. M. Hofman and J. M. Maldacena, “Giant magnons,” J. Phys. A **39**, 13095 (2006) [arXiv:hep-th/0604135].
- [67] N. Dorey, “Magnon bound states and the AdS/CFT correspondence,” J. Phys. A **39**, 13119 (2006) [arXiv:hep-th/0604175].
- [68] H. Y. Chen, N. Dorey and K. Okamura, “Dyonic giant magnons,” JHEP **0609**, 024 (2006) [arXiv:hep-th/0605155].
- [69] M. Kruczenski, J. Russo and A. A. Tseytlin, “Spiky strings and giant magnons on  $S^5$ ,” JHEP **0610**, 002 (2006) [arXiv:hep-th/0607044].
- [70] G. Arutyunov, S. Frolov and M. Zamaklar, “Finite-size effects from giant magnons,” Nucl. Phys. B **778**, 1 (2007) [arXiv:hep-th/0606126].
- [71] J. A. Minahan, A. Tirziu and A. A. Tseytlin, “Infinite spin limit of semiclassical string states,” JHEP **0608**, 049 (2006) [arXiv:hep-th/0606145].
- [72] M. Spradlin and A. Volovich, “Dressing the giant magnon,” JHEP **0610**, 012 (2006) [arXiv:hep-th/0607009].
- [73] N. P. Bobev and R. C. Rashkov, “Multispin giant magnons,” Phys. Rev. D **74**, 046011 (2006) [arXiv:hep-th/0607018].
- [74] S. Ryang, “Three-spin giant magnons in  $AdS(5) \times S^5$ ,” JHEP **0612**, 043 (2006) [arXiv:hep-th/0610037].

- [75] K. Okamura and R. Suzuki, “A perspective on classical strings from complex sine-Gordon solitons,” *Phys. Rev. D* **75**, 046001 (2007) [arXiv:hep-th/0609026].
- [76] R. Ishizeki and M. Kruczenski, “Single spike solutions for strings on  $S^2$  and  $S^3$ ,” *Phys. Rev. D* **76**, 126006 (2007) [arXiv:0705.2429]. A. E. Mosaffa and B. Safarzadeh, “Dual Spikes: New Spiky String Solutions,” *JHEP* **0708**, 017 (2007) [arXiv:0705.3131].
- [77] R. Ishizeki, M. Kruczenski, M. Spradlin and A. Volovich, “Scattering of single spikes,” *JHEP* **0802**, 009 (2008) [arXiv:0710.2300].
- [78] M. C. Abbott and I. V. Aniceto, “Vibrating giant spikes and the large-winding sector,” *JHEP* **0806**, 088 (2008) [arXiv:0803.4222]. C. Ahn and P. Bozhilov, “Finite-size Effects for Single Spike,” *JHEP* **0807**, 105 (2008) [arXiv:0806.1085]. S. Ryang, “Conformal  $SO(2,4)$  Transformations for the Helical AdS String Solution,” *JHEP* **0805**, 021 (2008) [arXiv:0803.3855].
- [79] H. Hayashi, K. Okamura, R. Suzuki and B. Vicedo, “Large Winding Sector of AdS/CFT,” *JHEP* **0711**, 033 (2007) [arXiv:0709.4033].
- [80] K. Okamura, “Aspects of Integrability in AdS/CFT Duality,” arXiv:0803.3999. K. Okamura, “Giant Spinons,” arXiv:0911.1528.
- [81] N. Dorey, B. Vicedo, “On the dynamics of finite-gap solutions in classical string theory,” *JHEP* **0607**, 014 (2006). [hep-th/0601194].
- [82] V. E. Zakharov and A. V. Mikhailov, “Relativistically Invariant Two-Dimensional Models In Field Theory Integrable By The Inverse Problem Technique.” *Sov. Phys. JETP* **47**, 1017 (1978) [*Zh. Eksp. Teor. Fiz.* **74**, 1953 (1978)]. “On The Integrability Of Classical Spinor Models In Two-Dimensional Space-Time,” *Commun. Math. Phys.* **74**, 21 (1980).
- [83] A. T. Ogielski, M. K. Prasad, A. Sinha and L. L. Wang, “Backlund Transformations And Local Conservation Laws For Principal Chiral Fields,” *Phys. Lett. B* **91**, 387 (1980). J. P. Harnad, Y. Saint Aubin and S. Shnider, “Backlund Transformations For Nonlinear Sigma Models With Values In Riemannian Symmetric Spaces,” *Commun. Math. Phys.* **92**, 329 (1984). G. Arutyunov and M. Staudacher, “Matching higher conserved charges for strings and spins,” *JHEP* **0403**, 004 (2004) [arXiv:hep-th/0310182].
- [84] C. Kalousios, M. Spradlin and A. Volovich, “Dressing the giant magnon. II,” *JHEP* **0703**, 020 (2007) [arXiv:hep-th/0611033].
- [85] A. Jevicki, C. Kalousios, M. Spradlin and A. Volovich, “Dressing the Giant Gluon,” *JHEP* **0712**, 047 (2007) [arXiv:0708.0818].
- [86] M. Grigoriev and A. A. Tseytlin, “Pohlmeyer reduction of  $AdS_5 \times S^5$  superstring sigma model,” *Nucl. Phys. B* **800**, 450 (2008) [arXiv:0711.0155]. “On reduced models for superstrings on  $AdS_n \times S^n$ ,” *Int. J. Mod. Phys. A* **23**, 2107 (2008) [arXiv:0806.2623]. B. Hoare, Y. Iwashita and A. A. Tseytlin, “Pohlmeyer-reduced form of string theory in  $AdS_5 \times S^5$  : semiclassical expansion,” *J. Phys. A* **42**, 375204 (2009) [arXiv:0906.3800]. Y. Iwashita, “One-loop corrections to  $AdS_5 \times S^5$  superstring partition function via Pohlmeyer reduction,” *J. Phys. A* **43**, 345403 (2010) [arXiv:1005.4386].

- [87] A. Mikhailov and S. Schafer-Nameki, “Sine-Gordon-like action for the Superstring in  $AdS(5) \times S(5)$ ,” *JHEP* **0805**, 075 (2008) [arXiv:0711.0195].
- [88] J. L. Miramontes, “Pohlmeyer reduction revisited,” *JHEP* **0810**, 087 (2008) [arXiv:0808.3365]. T. J. Hollowood and J. L. Miramontes, “Magnons, their Solitonic Avatars and the Pohlmeyer Reduction,” *JHEP* **0904**, 060 (2009) [arXiv:0902.2405].
- [89] A. Jevicki, K. Jin, C. Kalousios and A. Volovich, “Generating AdS String Solutions,” *JHEP* **0803**, 032 (2008) [arXiv:0712.1193]. A. Jevicki and K. Jin, “Solitons and AdS String Solutions,” *Int. J. Mod. Phys. A* **23**, 2289 (2008) [arXiv:0804.0412]. “Moduli Dynamics of AdS3 Strings,” *JHEP* **0906**, 064 (2009) [arXiv:0903.3389].
- [90] I. Aniceto and A. Jevicki, “N-body Dynamics of Giant Magnons in  $R \times S^2$ ,” arXiv:0810.4548
- [91] L. F. Alday and J. Maldacena, “Minimal surfaces in AdS and the eight-gluon scattering amplitude at strong coupling,” arXiv:0903.4707 . “Null polygonal Wilson loops and minimal surfaces in Anti-de-Sitter space,” *JHEP* **0911**, 082 (2009) [arXiv:0904.0663]. L. F. Alday, D. Gaiotto and J. Maldacena, “Thermodynamic Bubble Ansatz,” arXiv:0911.4708 . L. F. Alday, J. Maldacena, A. Sever and P. Vieira, “Y-system for Scattering Amplitudes,” arXiv:1002.2459
- [92] H. Dorn, G. Jorjadze and S. Wuttke, “On spacelike and timelike minimal surfaces in  $AdS_n$ ,” arXiv:0903.0977 . K. Sakai and Y. Satoh, “A note on string solutions in AdS3,” *JHEP* **0910**, 001 (2009) [arXiv:0907.5259]. S. Ryang, “Asymptotic AdS String Solutions for Null Polygonal Wilson Loops in  $R^{1,2}$ ,” arXiv:0910.4796 . H. Dorn, N. Drukker, G. Jorjadze and C. Kalousios, “Space-like minimal surfaces in  $AdS \times S$ ,” arXiv:0912.3829 . A. Jevicki and K. Jin, “Series Solution and Minimal Surfaces in AdS,” arXiv:0911.1107. B. A. Burrington and P. Gao, “Minimal surfaces in AdS space and Integrable systems,” arXiv:0911.4551 .



# Review of AdS/CFT Integrability, Chapter II.2: Quantum Strings in $\text{AdS}_5 \times \text{S}^5$

TRISTAN MCLOUGHLIN

*Max-Planck-Institut für Gravitationsphysik,  
Albert-Einstein-Institut,  
Am Mühlenberg 1, D-14476 Potsdam, Germany*

tmcclough@aei.mpg.de

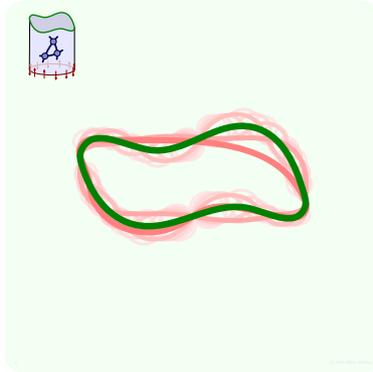

**Abstract:** We review the semiclassical analysis of strings in  $\text{AdS}_5 \times \text{S}^5$  with a focus on the relationship to the underlying integrable structures. We discuss the perturbative calculation of energies for strings with large charges, using the folded string spinning in  $\text{AdS}_3 \subset \text{AdS}_5$  as our main example. Furthermore, we review the perturbative light-cone quantization of the string theory and the calculation of the worldsheet S-matrix.

# 1 Introduction

The semiclassical study of strings in  $AdS_5 \times S^5$  has played a key role in extending our understanding of the AdS/CFT correspondence beyond the supergravity approximation. The analysis of quantum corrections to the energies of strings with large charges has gone hand-in-hand with the discovery and application of the integrable structures present in the duality. In particular, it has been important for comparison with the Bethe ansatz predictions for the anomalous dimensions of long operators and to understand the finite size corrections of short operators.

Due to the presence of Ramond-Ramond fields one must make use of the Green-Schwarz formalism for the string action, adapted to the  $AdS_5 \times S^5$  geometry [1] (see [2] for a brief introduction),<sup>1</sup> which to quadratic order in fermionic fields is

$$I = -\frac{\sqrt{\lambda}}{4\pi} \int d^2\sigma h^{ab} G_{\mu\nu} \partial_a x^\mu \partial_b x^\nu - i \frac{\sqrt{\lambda}}{2\pi} \int d^2\sigma (h^{ab} \delta^{IJ} - \epsilon^{ab} s^{IJ}) \bar{\theta}^I \varrho_a D_b \theta^J. \quad (1.1)$$

Here we have used the rescaled worldsheet metric  $h^{ab} = \sqrt{-g} g^{ab}$ , the induced Dirac matrices  $\varrho_a = \partial_a x^\mu E_\mu^A \Gamma_A$  and the covariant derivative

$$D_a \theta^I = \left( \partial_a + \frac{1}{4} \partial_a x^\mu \omega_\mu^{AB} \Gamma_{AB} \right) \theta^I + \frac{1}{2} \varrho_a \Gamma_{01234} \epsilon^{IJ} \theta^J. \quad (1.2)$$

Directly quantizing this action is beyond current methods and one must take a perturbative approach, expanding about a given classical solution in powers of the effective string tension,  $\sqrt{\lambda}$ . A classical solution is characterised by the conserved charges corresponding to the AdS energy,  $E$ , two AdS spins,  $S_i$ , and three angular momenta of the sphere,  $J_s$ , in addition to any parameters specifying further properties of the string such as non-trivial winding. The Virasoro conditions provide a constraint on these parameters and for the solutions we are interested in we can express the string energy as a function of the remaining charges:  $E = E(S_i, J_s; k_r)$ . In the semiclassical approach one takes a string solution where one or more of the rescaled charges are finite,  $S_i = \frac{S_i}{\sqrt{\lambda}}$  or  $J_s = \frac{J_s}{\sqrt{\lambda}}$ , and computes the worldsheet loop corrections to the energy as an expansion in large tension,

$$E = \sqrt{\lambda} \left[ E_0(S_i, J_s; k_r) + \frac{1}{\sqrt{\lambda}} E_1(S_i, J_s; k_r) + \frac{1}{\lambda} E_2(S_i, J_s; k_r) + \dots \right]. \quad (1.3)$$

In general, calculating these corrections involves gauge-fixing the diffeomorphism and kappa gauge invariance, and studying the fluctuations of the fields – bosonic, fermionic and conformal ghosts from gauge fixing – about the classical solution. An important point is that all UV divergences of the worldsheet theory cancel and, relatedly, the conformal anomaly vanishes once the contribution from the path integral measure is accounted for; thus the semiclassical expansion is well defined. On general grounds this is expected as the string theory is of critical dimension and it was explicitly shown at

---

<sup>1</sup>One can also study strings in different backgrounds,  $AdS_4 \times CP^3$  is of particular interest where many results parallel the  $AdS_5 \times S^5$  case. See [3].

one-loop in [4] and [5].<sup>2</sup> A solution which has played a particularly important role in our quantitative understanding of the AdS/CFT duality is the spinning folded string in  $AdS_5$ , introduced in [6] and whose semiclassical analysis was initiated in [5]. In the large spin limit [6–8], the difference between its energy  $E$  and spin  $S$  scales like  $\ln S$  with the coefficient being the universal scaling function,  $f(\lambda)$ . This function provided the first example of a result interpolating between weak and strong coupling which can be calculated from the all-order asymptotic Bethe ansatz (ABA) [9, 10] (see [11, 12] for a review of the all-order ABA). The one and two-loop semiclassical calculations [5, 13–15] have been shown to match the predictions of the string ABA [16–18] using the one-loop phase factor [19–21] and its all-order generalisation [22, 10] in a very non-trivial test of the duality and its quantum integrability (see [23] for a review of the ABA calculation and references). We will discuss this solution, its generalisations and related solutions in Sec. 2.3. While for the most part we focus on closed strings, similar semiclassical analysis has also been applied to open strings: duals to cuspy Wilson loops, to Wilson loops describing “quark–anti-quark” systems, [4, 24], to Wilson loops describing high energy scattering [25] and more recently, dimensionally reduced amplitudes [26].

Another solution which has played a crucial role in our understanding of the quantum string in  $AdS_5 \times S^5$  is the BMN string, [27] [6] see also [2], which is the BPS solution dual to the ferromagnetic vacuum of the spin chain description of the gauge theory. This solution is the natural vacuum state in the light-cone quantization of the worldsheet theory where the physical Hamiltonian,  $H_{l.c.}$ , is proportional to  $P_- = E - J$ , with  $J$  one of the sphere angular momenta.<sup>3</sup> Finding quantum string energies,  $E$ , corresponds to computing the spectrum of the  $H_{l.c.}$ . Unfortunately the exact light-cone Hamiltonian has a non-polynomial form [30, 34] and is not a suitable starting point for “first-principles” quantization. One can, however, solve for the spectrum perturbatively. At leading order the theory is simply that of free massive fields [27, 35] while at subleading orders [36, 29, 30, 37, 32] the interactions are somewhat more complicated and, due to the gauge fixing, do not respect worldsheet Lorentz invariance. Alternatively, as the worldsheet theory is integrable, it is possible to find the spectrum of the decompactified theory, via the ABA, by calculating the worldsheet S-matrix [17], [16, 18]. A review of the exact form of this S-matrix and its properties can be found [12], in this review we will restrict ourselves to briefly describing its perturbative calculation (for a more thorough review see [38]).

## 2 Quantum spinning strings

We will, as an illustrative example, consider the the folded spinning string [6], [5], see also [2]. This solution describes a string extended and rotating with spin,  $S$ , in an  $AdS_3$

---

<sup>2</sup> Particular care must be taken with the fermionic fields. Importantly, they couple to the worldsheet metric rather than the zweibein and so contribute to the conformal anomaly four times the usual 2-d Majorana fermion amount.

<sup>3</sup>There are essentially two ways to fix the light-cone gauge in  $AdS_5 \times S^5$ , which differ by picking inequivalent light-cone geodesics. In one case, which is possible only in the Poincaré patch, the light-cone directions lie entirely in  $AdS_5$  [28]. In our case the light-cone is shared between  $AdS_5$  and  $S^5$

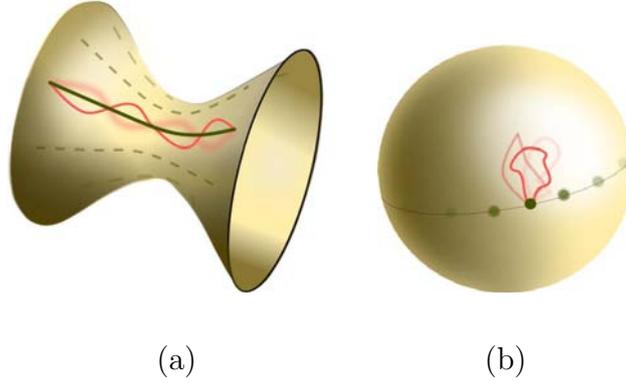

**Figure 1:** In (a) we show the classical folded spinning string moving in  $AdS_3 \subset AdS_5$  at a certain time (dark solid line) and earlier/later times (dashed lines). The quantum fluctuations, corresponding to oscillations transverse (light wavy lines) to the classical solution, acquire mass due to the background curvature. In (b) we show the motion of the string on the sphere, essentially a point moving along a great circle, with its fluctuations again seeing more of the geometry.

subspace of  $AdS_5$  while additionally moving along a great circle of the  $S^5$  with angular momentum  $J$  (see Fig. 1). In terms of the global coordinates

$$ds_{AdS_5}^2 = -\cosh^2 \rho dt^2 + d\rho^2 + \sinh^2 \rho (d\theta^2 + \cos^2 \theta d\phi_1^2 + \sin^2 \theta d\phi_2^2) , \quad (2.1)$$

$$ds_{S^5}^2 = +\cos^2 \gamma d\varphi_3^2 + d\gamma^2 + \sin^2 \gamma (d\psi^2 + \cos^2 \psi d\varphi_1^2 + \sin^2 \psi d\varphi_2^2) , \quad (2.2)$$

the string solution is given by  $\theta = \gamma = \psi = \frac{\pi}{2}$ ,

$$t = \kappa\tau , \quad \phi_2 = \omega\tau , \quad \rho = \rho(\sigma) = \rho(\sigma + 2\pi) , \quad \varphi_2 = \nu\tau . \quad (2.3)$$

The equations of motion and the conformal constraints are satisfied provided

$$\rho'' = (\kappa^2 - \omega^2) \sinh \rho \cosh \rho , \quad \rho'^2 = \kappa^2 \cosh^2 \rho - \omega^2 \sinh^2 \rho - \nu^2 , \quad (2.4)$$

and the other fields are zero. This string can be thought of as four segments: the first, for  $0 \leq \sigma \leq \frac{\pi}{2}$ , extends from the origin of the  $AdS_5$  space along the radial direction to a maximum  $\rho(\frac{\pi}{2}) = \rho_0$  i.e.  $\rho'(\frac{\pi}{2}) = 0$ . The string then turns and runs back along itself to the origin, this then repeats before the string closes on itself. In fact, this solution is generically rather complicated however, in various limits it simplifies dramatically.

## 2.1 Quantum corrections

It is possible to extract the one-loop correction to the energy by various means though, of course, all give identical results. The most direct method is to fix a physical gauge, such as light-cone, solve the resulting constraints and quantise the remaining degrees of freedom; the correction to the AdS energy of the string is the correction to the two-dimensional energy of the vacuum state. However, for many purposes, and particularly for more

---

e.g. [29–33].

complicated solutions at higher orders, the most convenient method, introduced in this context by [14, 26, 13] and most completely described in [39, 40], is to relate the correction to the energy to the calculation of the worldsheet effective action. <sup>4</sup>As in standard QFT, and in analogy with the thermodynamic Gibbs free energy, in the presence of a non-trivial background solution,  $\varphi_c(x)$ , the expectation value of the conjugate source,  $J(x)$ , is given by the functional derivative of the effective action,  $\Gamma[\varphi_c(x)]$ , which is simply the Legendre transform of the vacuum energy functional. For the theory we are interested in the sources are simply the conserved charge densities, such as  $E$ ,  $S$  and  $J$ . These are conjugate to time derivatives of the fields and so the background is specified by the constant parameters e.g.  $\kappa$ ,  $\omega$ , and  $\nu$ . Thus

$$\frac{1}{T}\Gamma(\kappa, \omega, \nu) = -\frac{i}{T} \ln \langle e^{iH_{2d}T} \rangle + \kappa \langle E \rangle - \omega \langle S \rangle - \nu \langle J \rangle \quad (2.5)$$

where  $T \rightarrow \infty$  is the worldsheet time interval. Due to the classical Virasoro constraints not all parameters are independent e.g.  $\kappa = \kappa(\omega, \nu)$ . Furthermore, the energy functional vanishes as  $\langle H_{2d} \rangle = 0$  due to the quantum conformal constraint. The charges are thus found from the effective action by e.g.

$$\frac{1}{T} \frac{\partial \Gamma(\omega, \nu)}{\partial \nu} = \frac{\partial \kappa(\omega, \nu)}{\partial \nu} \langle E \rangle - \langle J \rangle. \quad (2.6)$$

Hence, we need only calculate the worldsheet effective action to determine the corrections to the string charges. In general, the leading quantum correction to the effective action,  $\Gamma_1$ , is found by expanding the Lagrangian,  $L$ , about a classical solution,  $\varphi = \varphi_c + \tilde{\varphi}$ , and performing the Gaussian integral

$$\Gamma_1 = \frac{i}{2} \log \det \left[ -\frac{\delta^2 L}{\delta \tilde{\varphi} \delta \tilde{\varphi}} \right] = \frac{i}{2} \text{Tr} \log \left[ -\frac{\delta^2 L}{\delta \tilde{\varphi} \delta \tilde{\varphi}} \right]. \quad (2.7)$$

For the string theory we must include not only the bosonic fluctuations but also those of the fermionic and the ghost fields which give inverses of determinants.

In general the effective action is an extrinsic quantity. <sup>5</sup> This can be seen by considering the simple case where the quadratic fluctuation operator is given by  $K = -\partial^2 + m^2$  with constant masses,  $m$ . Fourier transformed this is  $\tilde{K} = -\omega^2 + n^2 + m^2$ , and so

$$\Gamma_1 = \frac{iT}{2} \int \frac{d\omega}{2\pi} \sum_n \log(-\omega^2 + n^2 + m^2) = \frac{lT}{2} \int \frac{d^2 p_E}{(2\pi)^2} \log(p_E^2 + m^2) \quad (2.8)$$

where in the last identity we have Wick rotated to Euclidean signature and taken the extent of the spatial direction,  $l$ , to also be large. Note that by performing the integration over  $\omega$  in this constant mass case, or in fact for any stationary solution, one recovers the sum over fluctuation frequencies which gives the more common expression for the correction to the string energy c.f. appendix A [5]. <sup>6</sup>

<sup>4</sup>There is yet another method, essentially a generalisation of the WKB formula, for finding the leading quantum correction to periodic solutions due to Daschen, Hasslacher and Neveu [41]. Such methods were applied to the semiclassical quantization of the giant magnon [42] in [43]

<sup>5</sup>Strictly speaking all our considerations are only valid in the large volume limit and under the assumption that interactions are local.

<sup>6</sup>It is also possible to make use of the integrable structure and extract the fluctuation frequencies

## 2.2 Point-like BMN string

If we consider the case  $\omega = 0$ ,  $\kappa = \nu$ , for (2.3), this forces  $\rho_0 = 0$  and so corresponds to the point-like BMN string rotating only in the  $S^5$  (see Fig. 1 (b)). As mentioned in the introduction, this solution plays a fundamental role in our understanding the quantum string. Here we merely calculate the one-loop correction to its classical AdS energy  $E_0 = J = \sqrt{\lambda}\kappa$ .

It is convenient to switch to Cartesian coordinates:  $(\rho, \theta, \phi_1, \phi_2) \rightarrow z_k$ ,  $k = 1, \dots, 4$  and  $(\gamma, \psi, \varphi_1, \varphi_3) \rightarrow y_s$ ,  $s = 1, \dots, 4$  such that

$$ds^2 = -\frac{(1 + \frac{1}{4}z^2)^2}{(1 - \frac{1}{4}z^2)^2} dt^2 + \frac{dz_k dz_k}{(1 - \frac{1}{4}z^2)^2} + \frac{(1 - \frac{1}{4}y^2)^2}{(1 + \frac{1}{4}y^2)^2} d\varphi_3^2 + \frac{dy_s dy_s}{(1 + \frac{1}{4}y^2)^2}. \quad (2.9)$$

Now, expanding near  $z_k = y_s = 0$ ,

$$t = \nu\tau + \frac{\tilde{t}}{\lambda^{1/4}}, \quad z_k = \frac{\tilde{z}_k}{\lambda^{1/4}}, \quad \varphi_3 = \nu\tau + \frac{\tilde{\varphi}}{\lambda^{1/4}}, \quad y_s = \frac{\tilde{y}_s}{\lambda^{1/4}}, \quad (2.10)$$

the bosonic terms of the action (1.1), in conformal gauge, give the quadratic term <sup>7</sup>

$$I_B = -\frac{1}{4\pi} \int d^2\sigma \left[ -\partial_a \tilde{t} \partial^a \tilde{t} + \partial_a \tilde{\varphi} \partial^a \tilde{\varphi} + \nu^2 (\tilde{z}^2 + \tilde{y}^2) + \partial_a \tilde{z}_k \partial^a \tilde{z}_k + \partial_a \tilde{y}_s \partial^a \tilde{y}_s \right]. \quad (2.11)$$

This action corresponds to two massless longitudinal fluctuations  $\tilde{t}$  and  $\tilde{\varphi}$ , plus eight free, massive scalars, with mass  $m = \nu$ . For the fermions we find for the induced Dirac matrices  $\varrho_0 = \kappa \Gamma^-$  and  $\varrho_1 = 0$  so that the action becomes

$$I_F = \frac{i\nu}{2\pi} \int d^2\sigma \left[ \bar{\theta}^1 \Gamma^- \partial_+ \theta^1 + \bar{\theta}^2 \Gamma^- \partial_- \theta^2 - 2\nu \bar{\theta}^1 \Gamma^- \Pi \theta^2 \right] \quad (2.12)$$

where we have defined  $\partial_{\pm} = \partial_0 \pm \partial_1$ ,  $\Gamma^{\pm} = \mp \Gamma_0 + \Gamma_9$  and  $\Pi = \Gamma_{1234}$ . Furthermore because of the form of the fermionic kinetic operator it was natural to choose the kappa-gauge fixing  $\Gamma^+ \theta^I = 0$  which simplified the mass term. This action corresponds to eight free, massive fermionic excitations, with  $m = \pm\nu$ . Finally, one must include contributions from the conformal bosonic ghosts, however for the cases in which we are interested, as was shown in [4, 5], the ghost contribution is essentially trivial. Their only effect is to cancel the two massless longitudinal bosonic fluctuations.

As the masses of the transverse bosons and physical fermions are equal one immediately sees that the ratio of fluctuation determinants cancels and the one-loop effective action is zero. Thus the correction to the AdS energy, (2.5),  $\langle E - J \rangle = \frac{1}{\kappa T} \Gamma$  is zero which is exactly as expected as this state is BPS. As we will see later, it provides a sensible vacuum about which to study fluctuation interactions.

---

from the string algebraic curve. While this powerful method is widely used in the calculation of quantum corrections we will not discuss it here, but simply refer the reader to [44] for a review and references.

<sup>7</sup>We note that this is essentially the same action as that found by expanding the action for a string in the plane-wave geometry, [35],  $ds^2 = dx^+ dx^- + \frac{1}{4} x^2 dx^+ dx^+ + dx^i dx^i$  about the solution  $x^+ = 2\nu\tau$  [27,35].

### 2.3 Spinning folded string

While for the BPS solution we find zero correction to the string energy, a generic spinning string solution spontaneously breaks supersymmetry and we expect to find a non-trivial correction at one-loop. We will consider the so-called “semi-classical scaling” or long-string limit of the spinning string solutions, see [7, 8] and also [39],

$$S \gg J \gg 1, \quad \text{with} \quad \ell \equiv \frac{J}{2 \ln S}. \quad (2.13)$$

As discussed at length in [8, 39], upon taking  $\omega = \kappa$  the solution simplifies dramatically becoming homogeneous so that  $\rho(\sigma) = \mu\sigma$ . The conformal gauge condition becomes  $\kappa = \sqrt{\mu^2 + \nu^2}$  and in this limit of large spin,  $\mu = \frac{1}{\pi} \ln S$  and  $\ell = \frac{\nu}{\mu}$ .

As  $\mu$  is thus very large, by rescaling the worldsheet coordinate  $\sigma$  such that  $\rho = \sigma$ , we find the string length  $l = 2\pi\mu$  becomes infinite. The folded string becomes two overlapping, infinite, open strings. One can further expand in small  $\ell$ , the so called “slow long string limit”, [8, 39]. In this further limit the quantum string energy is given by

$$E - S = \frac{\sqrt{\lambda}}{\pi} f(\lambda) \ln S, \quad (2.14)$$

where  $f(\lambda)$  is the universal scaling function. At leading order this can be checked by expanding the classical energy which is given by  $E_0 - S = \mu\sqrt{1 + \ell^2}$ . We will see this form persists at subleading orders in the semiclassical expansion, i.e. there are no  $\ln^k S$  terms, and furthermore we can calculate the numerical coefficients [5, 8, 13, 39]

$$f(\sqrt{\lambda}) = 1 - \frac{3 \ln 2}{\sqrt{\lambda}} - \frac{K}{\lambda} + \dots \quad (2.15)$$

where  $K$  is the Catalan constant.

To calculate these coefficients we expand about the homogeneous,  $J = 0$  solution,  $\hat{t} = \kappa\tau$ ,  $\hat{\rho} = \kappa\sigma$ ,  $\hat{\theta} = \frac{\pi}{2}$ ,  $\hat{\phi}_2 = \kappa\tau$ , and (following [5] closely, where full details can be found) we again consider the conformal gauge action.

**Bosons** The bosonic action (1.1) to quadratic order in fluctuations (using coordinates (2.1) for the  $AdS_5$  space but (2.9) for the sphere) is

$$I_B = -\frac{1}{4\pi} \int d^2\sigma \left[ -\cosh^2 \hat{\rho} (\partial \tilde{t})^2 + \sinh^2 \hat{\rho} (\partial \tilde{\phi}_2)^2 + 2\kappa \sinh \hat{\rho} \tilde{\rho} (\partial_0 \tilde{t} - \partial_0 \tilde{\phi}_2) \right. \\ \left. + (\partial \tilde{\rho})^2 + \sinh^2 \hat{\rho} ((\partial \tilde{\theta})^2 + \tilde{\theta}^2 (\partial \phi_1)^2 + \kappa^2 \tilde{\theta}^2) + (\partial \tilde{\phi}_3)^2 + \sum_s (\partial \tilde{y}_s)^2 \right] \quad (2.16)$$

where e.g.  $(\partial t)^2 = \partial_a t \partial^a t$ . In this expression the coefficients depend on the worldsheet coordinates, however by making the field redefinitions

$$\bar{\chi} = \frac{1}{2} \sinh 2\hat{\rho} (\tilde{\phi}_2 - \tilde{t}), \quad \bar{\xi} = -\sinh^2 \hat{\rho} \tilde{\phi}_2 + \cosh^2 \hat{\rho} \tilde{t}, \quad \bar{\theta} = \sinh \hat{\rho} \tilde{\theta}, \\ \bar{\rho} = \tilde{\rho}, \quad \bar{x}_1 = \tilde{\theta} \cos \phi_1, \quad \bar{x}_2 = \tilde{\theta} \sin \phi_1, \quad (2.17)$$

this can be put in the form

$$I_B = -\frac{1}{4\pi} \int d^2\sigma \left[ (\partial\bar{\chi})^2 - (\partial\bar{\xi})^2 + (\partial\bar{\rho})^2 + 4\kappa(\partial_1\bar{\chi})\bar{\xi} - 4\kappa(\partial_0\bar{\chi})\bar{\rho} \right. \\ \left. + \sum_i ((\partial\bar{x}_i)^2 + 2\kappa^2 x_i^2) + (\partial\tilde{\phi}_3)^2 + \sum_s (\partial\tilde{y}_s)^2 \right]. \quad (2.18)$$

It is now straightforward to calculate the determinant of the fluctuation operator

$$\det K_B = -(\partial^2)^7 (\partial^2 + 2\kappa^2)^2 (\partial + 4\kappa^2) \quad (2.19)$$

corresponding to two scalars with mass  $\sqrt{2}\kappa$ , one with mass  $2\kappa$  and seven massless scalars – two from the AdS space, five from the sphere.

**Fermions** Substituting the classical solution in the expressions for the induced Dirac matrices we find (where the flat index 0 is the homologue of  $t$ , 1 corresponds to  $\rho$ , and 2 to  $\phi_2$ )

$$\varrho_0 = \kappa \Gamma_0 (\cosh \hat{\rho} - \sinh \hat{\rho} \Gamma_{02}) , \quad \varrho_1 = \kappa \Gamma_1 . \quad (2.20)$$

Using the expression for the quadratic action (1.1), we again find that the dependence on the worldsheet coordinates can be removed by a field redefinition

$$\theta^I = S\Psi^I, \quad \text{with} \quad S = \exp\left(\frac{\kappa\sigma}{2}\Gamma_{02}\right) , \quad (2.21)$$

such that the corresponding transformations of the induced Dirac matrices are

$$\tau_0 = S^{-1}\varrho_0 S = \kappa \Gamma_0 , \quad \text{and} \quad \tau_1 = S^{-1}\varrho_1 S = \kappa \Gamma_1 . \quad (2.22)$$

Making use of the relevant terms of the spin connection,  $\omega_t^{01} = \sinh \rho$  and  $\omega_{\phi_2}^{41} = \cosh \rho \cos \theta$ , one can show that the portion of the covariant derivative that couples to the background curvature,  $D_a = \partial_a + \frac{1}{4}\omega_a^{AB}\Gamma_{AB}$ , essentially becomes trivial:  $S^{-1}D_a S = \partial_a + B_a$  where  $\eta^{ab}\tau_a B_b = \epsilon^{ab}\tau_a B_b = 0$ . Thus the fermionic action can be written as

$$I_F = \frac{i\sqrt{\lambda}}{2\pi} \int d^2\sigma (\eta^{ab}\delta^{IJ} - \epsilon^{ab}s^{IJ})(\bar{\Psi}^I \tau_a \partial_b \Psi^J + \frac{1}{2}\epsilon^{JK}\bar{\Psi}^I \tau_a \Gamma_{01234}\tau_b \Psi^K) . \quad (2.23)$$

As can be seen from the form of the kinetic operator one can fix the fermionic kappa-symmetry by imposing  $\Psi^1 = \Psi^2 = \Psi$  resulting in the fermion action <sup>8</sup>

$$I_F = \frac{i\sqrt{\lambda}}{\pi} \int d^2\sigma \bar{\Psi}^I (\tau^a \partial_a + iM)\Psi , \quad \text{where} \quad M = i\kappa^2 \Gamma_{234} . \quad (2.24)$$

Of the eight physical fermions four have mass  $\kappa$  and four have  $-\kappa$ , thus

$$\det K_F = (\partial^2 + \kappa^2)^8 . \quad (2.25)$$

---

<sup>8</sup>While it is not relevant for the case at hand in general one must be careful with the boundary conditions imposed on the fermions which can be subtle. See [45] for a discussion.

**Energy Correction** To determine the correction to the energy we must evaluate the sum over momenta. As we are interested in the leading term in the large  $\kappa$  expansion we can treat the worldsheet, after rescaling by  $\kappa$ , as having infinite extent and so the worldsheet momenta are continuous. In momentum space the one-loop effective action is (having taken into account the conformal ghosts which cancel two massless bosons)

$$\Gamma_1 = \frac{1}{2}V_2 \int \frac{d^2p}{(2\pi)^2} \left[ \ln(p^2 + 4) + 2 \ln(p^2 + 2) + 5 \ln p^2 - 8 \ln(p^2 + 1) \right] \quad (2.26)$$

where we recall that two-dimensional volume is given by  $V_2 = 2\pi\kappa^2 T$ . While the complete expression is finite the individual terms are divergent so we introduce a cut-off at intermediate stages to perform the integration. The quadratic and logarithmic divergences cancel and the finite result is

$$\langle E - S \rangle |_{\text{one-loop}} = \frac{1}{\kappa T} \Gamma_1 = -\frac{3 \ln 2}{\pi} \ln S \quad (2.27)$$

which is the leading correction to the universal scaling function. We note that the  $\ln S$  dependence arises from the fact that the effective action is proportional to the worldsheet volume as, in the scaling limit, we can completely remove  $\kappa$  from the action. This remains true at all orders.

**Generalisations** The two-loop calculation of the universal scaling function was carried out in [13–15]. The equivalence [26] of the spinning folded string, in the  $l \rightarrow \infty$  limit, to the null cusp Wilson loop solution [46] plays a key role in these calculations; as does a form of the action with particularly simple fermions [47]. One can obviously include the effects of non-zero  $J$  by keeping finite  $\nu$ , or equivalently  $\ell$ , dependence. The generalised one-loop calculation in the “long string” limit was performed in [8] and the two-loop analysis in [39, 40, 48]. Here, it is necessary to take into account the quantum corrections to the Virasoro condition and to the relations between solution parameters and charges as described in Sec. 2.1. Furthermore, the calculation is simplified by using a light-cone gauge [28] adapted to a geodesic entirely in the  $AdS_5$  space. These results match those found from the ABA [49]. These calculations thus provide vigorous checks of the two-loop finiteness of the worldsheet theory and the underlying quantum integrability.

## 2.4 Circular spinning strings

While the energies of spinning folded strings have provided stringent checks of ABA the relationship is slightly complicated. It is a separate class of solutions, rigid circular spinning strings (see [2] for a review and further references), whose energies are most transparently related to the strong coupling expression for the S-matrix entering the ABA. The simplest circular strings come in two types: the so-called  $\mathfrak{su}(2)$  circular strings moving on a  $S^3 \subset S^5$ , [50], and the  $\mathfrak{sl}(2)$  circular strings lying in  $AdS_3 \times S^1 \subset AdS_5 \times S^5$  [51].

The computation of the one-loop correction to the energies of the  $\mathfrak{su}(2)$  [52, 53] and  $\mathfrak{sl}(2)$  [54, 19, 55, 56] strings<sup>9</sup> played a key part in discovering the presence of the one-loop

<sup>9</sup>An early semiclassical analysis of circular strings in AdS was performed in [57].

term [20] in the phase in the strong-coupling (or “string”) form of the Bethe Ansatz [16–18].

The  $(S, J)$  string solution of [51] has a spiral-like shape, with projection to  $AdS_3$  being a constant radius circle (with winding number  $k$ ), and projection to  $S^5$  – a big circle (with winding number  $m$ ). The corresponding spins are, respectively,  $S$  and  $J$  with the Virasoro condition implying that  $u \equiv \frac{S}{J} = -\frac{m}{k}$ . Expanding the classical energy in large semiclassical parameters  $S$  and  $J$  with fixed  $k$  and  $u$  [51, 54] we have

$$E_0 = S + J + \frac{\lambda}{J} e_1(u, k) + \frac{\lambda^2}{J^3} e_3(u, k) + \frac{\lambda^2}{J^5} e_5(u, k) + \dots \quad (2.28)$$

For circular strings the expressions for the fluctuation frequencies are sufficiently complicated that they must be expanded in  $J$  to be evaluated and subsequently summing over modes becomes slightly subtle [54, 58, 53, 59, 19, 55, 60, 56]. The correct procedure, given in [19] for the  $\mathfrak{sl}(2)$  case (see also [56] for the  $\mathfrak{su}(2)$  case), gives two types of terms for the one-loop correction,  $E_1 = E_1^{\text{even}} + E_1^{\text{odd}}$ , where

$$E_1^{\text{even}} = \frac{\lambda}{J^2} g_2(u, k) + \frac{\lambda^2}{J^4} g_4(u, k) + \dots, \quad E_1^{\text{odd}} = \frac{\lambda^{5/2}}{J^5} g_5(u, k) + \dots \quad (2.29)$$

The absence of the  $\frac{1}{J}$  and  $\frac{1}{J^3}$  terms suggests that the two leading  $\frac{\lambda}{J}$  and  $\frac{\lambda^2}{J^3}$  terms receive no quantum corrections and their coefficients should directly match weak coupling gauge theory results. Indeed, the coefficient  $g_2$  of the “even”  $\frac{1}{J^2}$  term in (2.29) can be reproduced as a leading  $\frac{1}{J}$  (finite spin chain length) correction from the one-loop gauge theory Bethe Ansatz [53, 58]. At the same time, the presence of the non-analytic term  $\frac{\lambda^{5/2}}{J^5}$  in (2.29) implies that a similar  $\frac{1}{J^5}$  term in the classical energy (2.28) is not protected so that its coefficient cannot be directly compared to three-loop result on the gauge theory side which implies [19] that the corresponding “string” Bethe Ansatz [16] should be modified to contain a non-trivial one-loop correction to the phase. This phase was determined by directly matching to higher orders in this expansion [20, 21].

## 2.5 Finite size effects and short operators

Semiclassical analysis can also be applied to strings of finite length and even, to a certain degree, short strings. For the folded spinning string, Sec. 2.3, the large  $S$  corrections to the one-loop calculation were analysed in [61] and the exact one-loop expression for the fluctuation determinants was found in [62] (for two-loop results see [48]). The one-loop correction to the small spin or short string limit of the string were calculated in [63] and the generalisation with non-zero  $J$  in [64]. Short, excited strings dual to operators in the Konishi multiplet are particularly important in testing the conjectured exact results for the spectrum at finite volume. The correction to their energies at strong coupling was calculated semiclassically, with caveats regarding the validity of these methods in this regime, in [65]. For the circular spinning strings, in addition to the energy correction (2.29), a careful analysis shows the presence of exponential corrections,  $\mathcal{O}(e^{-J})$  [55, 56, 66]. Similar exponential corrections are found for quantum corrections to finite-sized giant-magnons calculated using algebraic curve methods (see [44]). Such corrections cannot

be accounted for by modifying the phase in the BA but rather arise from finite volume effects. See [67] for reviews and references.

### 3 Perturbative light-cone quantization

As we saw in Sec. 2.2, the string action expanded about the BMN string is particularly simple and is exactly solvable to quadratic order in fluctuations. This string solution provides a sensible vacuum about which to perturbatively quantize the  $AdS_5 \times S^5$  Green-Schwarz string [36, 29, 30, 32, 68]. In this context it is natural to make use of light-cone gauge, introducing the coordinates and momenta,  $p_\mu = h^{0a} G_{\mu\nu} \partial_a x^\nu$ ,

$$x^+ = \frac{1}{2}(t + \phi), \quad x^- = \phi - t, \quad p_- = \frac{1}{2}(p_\phi - p_t), \quad p_+ = p_\phi + p_t \quad (3.1)$$

where we focus on the bosonic fields for simplicity. The Hamiltonian density  $\mathcal{H} = p_\mu \dot{x}^\mu - \mathcal{L}$  is given by

$$\mathcal{H} = -\frac{h^{\tau\sigma}}{h^{\tau\tau}}(x'^\mu p_\mu) + \frac{1}{2h^{\tau\tau}}(p_\mu G^{\mu\nu} p_\nu + x'^\mu G_{\mu\nu} x'^\nu), \quad (3.2)$$

with the notation  $x' = \partial_\sigma x$  and  $\dot{x} = \partial_\tau x$ . As is usual in theories with general coordinate invariance, the Hamiltonian is a sum of constraints times Lagrange multipliers.

To impose light-cone gauge one sets  $x^+ = \tau$  and  $p_- = \text{const}$ . The metric coefficients  $1/h^{\tau\tau}$  and  $h^{\tau\sigma}/h^{\tau\tau}$  act as Lagrange multipliers, generating delta functions that impose two constraints which determine  $x^-$  and  $p_+$  in terms of the transverse variables (and the constant  $p_-$ ).<sup>10</sup> The transverse coordinates and momenta  $x^A$ ,  $p_A$   $A = 1, \dots, 8$  will then have dynamics which follow from the light-cone Hamiltonian  $-p_+ = \mathcal{H}_{lc}$ . The first constraint, or level-matching constraint, yields  $x'^- = -x'^A p_A / p_-$ . While solving the quadratic constraint equation for  $p_+$  we obtain the somewhat dispiriting result

$$-\mathcal{H}_{lc} = \frac{p_- G_{+-}}{G_{--}} + \frac{p_- \sqrt{G}}{G_{--}} \sqrt{1 + \frac{G_{--}}{p_-^2} (p_A G^{AB} p_B + x'^A G_{AB} x'^B) + \frac{G_{--}^2}{p_-^4} (x'^A p_A)^2}, \quad (3.3)$$

with  $G \equiv G_{+-}^2 - G_{++} G_{--}$ .<sup>11</sup> Using the relation between the canonical momenta and the target space charges we have

$$E - J = -P_+ = \frac{\sqrt{\lambda}}{2\pi} \int_0^{2\pi} d\sigma \mathcal{H}_{lc}, \quad \frac{1}{2}(E + J) = P_- = \frac{\sqrt{\lambda}}{2\pi} \int_0^{2\pi} d\sigma p_- . \quad (3.4)$$

**Perturbative expansion** To make progress we perform the large tension expansion: rescaling the transverse fields by  $\lambda^{-1/4}$  and expanding in large  $\sqrt{\lambda}$ , or equivalently  $P_- =$

<sup>10</sup>In fact, the constraints determine the derivatives of  $x^-$  and so  $x^-$  itself is non-local in this gauge. This has important consequences for the ‘‘off-shell’’ symmetry algebra.

<sup>11</sup>We have made use of the fact that the  $AdS_5 \times S^5$  metric, (2.9), rewritten in light-cone coordinates, (3.1), has no  $G_{+A}$  or  $G_{-A}$  components.

$\sqrt{\lambda}p_- \sim J$ , while keeping  $-P_+ = E - J$  fixed. Being careful with the expansion of the  $G_{--}$  terms, see e.g. [30], one finds the first two orders,

$$\begin{aligned} \mathcal{H}_{lc}^{pp} &= \frac{1}{2p_-} \left[ (\dot{p}^A)^2 + (x'^A)^2 + p_-^2 (x^A)^2 \right] \\ &+ \frac{1}{4\sqrt{\lambda}p_-} \left( z^2(p_y^2 + y'^2) - y^2(p_z^2 + z'^2) + 2z^2z'^2 - 2y^2y'^2 \right), \end{aligned} \quad (3.5)$$

where beyond leading order the eight transverse fields split into two sets of four,  $x^A = (z^i, y^s)$ . One can remove the dependence on the density  $p_-$  by rescaling the worldsheet coordinates, and thus we see that we are taking the large charge limit but keeping the worldsheet compact.

The leading order term is simply the plane-wave Hamiltonian whose spectrum consists of an infinite tower of non-interacting massive oscillators,

$$x^A(\sigma, \tau) = \sum_{n=-\infty}^{\infty} x_n^A(\tau) e^{-in\sigma}, \quad x_n^A(\tau) = \frac{i}{\sqrt{2\omega_n}} (a_n^A e^{-i\omega_n\tau} - a_{-n}^{A\dagger} e^{i\omega_n\tau}), \quad (3.6)$$

where  $n \in \mathbb{Z}$ ,  $\omega_n = \sqrt{p_-^2 + n^2}$ , and the raising and lowering operators obey the usual commutation relations. One can straightforwardly include the fermions, though the subleading interaction terms become somewhat involved [29,30,32]. At leading order one again gets massive oscillators,  $b_n^\alpha$ ,  $\alpha = 1, \dots, 8$  and thus the full plane-wave Hamiltonian,  $H_{pp}$ , is

$$H_{pp} = \frac{1}{p_-} \sum_{n=-\infty}^{\infty} \omega_n \left( a_n^{A\dagger} a_n^A + b_n^{\alpha\dagger} b_n^\alpha \right), \quad (3.7)$$

where one can immediately see that the energy of the vacuum state,  $|\text{Vac}\rangle$ , corresponding to a string with charge  $P_-$  vanishes.

**Near-BMN energy spectrum** The quartic terms give rise to corrections of order  $\mathcal{O}(1/J)$ , the effects of which can be perturbatively included in the spectrum. In the simple case where we consider a single complex boson from the sphere  $y = y^1 + iy^2$ , the leading correction to the two excitation state  $a_n^\dagger a_{-n}^\dagger |P_-\rangle$  is

$$E - J = 2\sqrt{1 + \lambda'n^2} - 2\frac{\lambda'n^2}{J} + \frac{N_B(n^2)}{J} \quad (3.8)$$

with  $\lambda' = \lambda/J^2$  an effective coupling. Due to the form of the interactions there is a normal ordering ambiguity, here characterised by the arbitrary function  $N_B(n^2)$ . There are related functions in the correction to all energies and they are fixed by demanding that the full spectrum possess the underlying global  $\mathfrak{psu}(2, 2|4)$  symmetry. This implies, for example,  $N_B = 0$ . Equivalently, they could be fixed by demanding that the algebra of generators, including the Hamiltonian, is satisfied at this order. These expressions for string energies can be compared to the string ABA [37, 31, 32, 68] and were one of the first pieces of evidence for a non-trivial dressing phase interpolating between strong and weak coupling.

### 3.1 Worldsheet S-matrix

As the theory in light-cone gauge has only massive particles, we can study the interactions by calculating the worldsheet S-matrix. Modulo issues of gauge dependence<sup>12</sup> this object should match the spin chain S-matrix introduced in [17], see [12] for reviews. The perturbative study of the worldsheet S-matrix was initiated in [70] while its symmetries and many properties were analysed in [71, 72] (see [38] for an extensive review). To define the S-matrix one must consider the theory on the plane: this corresponds to scaling  $p_-$  out of the action and taking the decompactification limit  $p_- \rightarrow \infty$ . In order to define free, asymptotic states for generic momentum one relaxes the level matching condition and then studies the interactions in powers of  $\sqrt{\lambda}$  or equivalently in a small (worldsheet) momentum expansion.

**Asymptotic states** Of the global group, the light-cone gauge preserves a subset  $PSU(2|2)_L \times PSU(2|2)_R \subset PSU(2, 2|4)$ . The bosonic subgroup of each  $PSU(2|2)$  factor consists of two  $SU(2)$  groups and it is useful to introduce a bispinor notation for the physical bosons  $Z_{\alpha\dot{\alpha}} = (\sigma_i)_{\alpha\dot{\alpha}} z^i$ ,  $Y_{a\dot{a}} = (\sigma_s)_{a\dot{a}} y^s$  and fermions,  $\Psi_{a\dot{\alpha}}, \Upsilon_{\alpha\dot{a}}$ , which are charged under different combinations of the  $SU(2)$ 's. One may define superindices  $A = (a|\alpha)$  and  $\dot{A} = (\dot{a}|\dot{\alpha})$  combining all asymptotic fields creating incoming or outgoing particles into a single bi-fundamental supermultiplet of which we will denote by  $\Phi_{A\dot{A}}^{(in/out)}$ .

**The S-matrix.** The two-particle S-matrix is a unitary operator relating *in*- and *out*-states. In the basis  $\Phi_{A\dot{A}}(p)$ , so that  $|\Phi_{A\dot{A}}(p)\Phi_{B\dot{B}}(p')\rangle^{(in)} = \Phi_{A\dot{A}}^{(in)}(p)\Phi_{B\dot{B}}^{(in)}(p')|\text{Vac}\rangle$ , its matrix representation is

$$\mathbb{S} |\Phi_{A\dot{A}}(p)\Phi_{B\dot{B}}(p')\rangle^{(in)} = |\Phi_{C\dot{C}}(p)\Phi_{D\dot{D}}(p')\rangle^{(out)} \mathbb{S}_{A\dot{A}B\dot{B}}^{C\dot{C}D\dot{D}}(p, p') . \quad (3.9)$$

Before gauge fixing the worldsheet theory is classically integrable [73]; since fixing light-cone may be interpreted as expanding about the BMN solution and solving some of the equations of motion, the gauge-fixed theory is also expected to be integrable at the classical level. In such an integrable theory, the S-matrix, invariant under a non-simple product group, must be a tensor product of S-matrices for each of the factors (see e.g. [74])<sup>13</sup>

$$\mathbb{S} = \mathbf{S} \otimes \mathbf{S} \quad , \quad \mathbb{S}_{A\dot{A}B\dot{B}}^{C\dot{C}D\dot{D}}(p, p') = \mathbf{S}_{AB}^{CD}(p, p') \mathbf{S}_{\dot{A}\dot{B}}^{\dot{C}\dot{D}}(p, p') . \quad (3.10)$$

It is important to note that a factorised tensor structure does not follow solely from the  $PSU(2|2) \times PSU(2|2)$  symmetry considerations; confirming group factorisation is thus an important test of integrability.

<sup>12</sup>The S-matrix is gauge-dependent, since unlike the spectrum it is not a physical object with a clear target-space interpretation. The differences between gauges can be attributed to the definition of the string length [17]. The difference in the definition of length and the gauge-dependence of the S-matrix, mutually cancel in the Bethe equations [32, 69].

<sup>13</sup>This can be understood as a requirement that the Faddeev-Zamolodchikov algebra is also a direct product: the field  $\Phi_{A\dot{A}}$  is represented by a bilinear in oscillators:  $\Phi_{A\dot{A}} \sim z_A z_{\dot{A}}$  each transforming under one of the  $PSU(2|2)$  factors [72]. The two sets of oscillators mutually commute. The braiding relations for each of these sets are determined by an  $PSU(2|2)$ -invariant S-matrix  $\mathbf{S}$  consistent with the Lagrangian of the theory.

The first nontrivial order in the expansion of the S-matrix in the coupling constant  $2\pi/\sqrt{\lambda}$  defines the T-matrix

$$\mathbb{S} = \mathbb{I} + \frac{2\pi i}{\sqrt{\lambda}} \mathbb{T} + \mathcal{O}\left(\frac{1}{\lambda}\right). \quad (3.11)$$

which inherits the factorised form  $\mathbb{T} = \mathbb{I} \otimes \mathbb{T} + \mathbb{T} \otimes \mathbb{I}$  from the S-matrix. Furthermore, since  $SU(2) \times SU(2) \subset PSU(2|2)$  is a manifest symmetry of the gauge-fixed worldsheet theory,  $\mathbb{T}$  may be parametrised in terms of ten unknown functions of the momenta  $p$  and  $p'$ . These functions, to leading order in  $1/\sqrt{\lambda}$ , can be easily extracted from the matrix elements of quartic terms of the light-cone Hamiltonian (3.5) (see [70] where explicit expressions for  $\mathbb{T}$  can be found). Equivalently one can Legendre transform with respect to the transverse fields to find the light-cone Lagrangian and then use the usual LSZ reduction to calculate the worldsheet scattering amplitudes perturbatively.

### Properties of the S-matrix

- The explicit perturbative calculation does indeed show that the two-body S-matrix has the factorised form (3.10). Furthermore, it can be explicitly checked to leading order that the ten functions in the T-matrix agree with the corresponding functions in the strong coupling BA S-matrix. It can be shown explicitly that there is no two-to-four particle scattering [70].
- In calculating the S-matrix we relax the level-matching constraint. In this “off-shell” formulation of the theory the symmetries become extended by two additional central charges related to the worldsheet momentum [71] (the same as found in the spin chain [75]). Furthermore, as the supersymmetry generators,  $Q \sim \int e^{ix^-} \Omega(Z, Y, \Upsilon, \Psi)$ , depend on the zero mode of the longitudinal coordinate,  $x^- \sim \int d\sigma \partial_\sigma x^-$ , there is a mild non-locality in the action of the symmetries which thus satisfy a Hopf algebra [70, 72].
- The integrable structures of the perturbative string S-matrix have been further studied including the construction of the classical r-matrix e.g. [76]. Furthermore, assuming the quantum integrability of the full worldsheet theory, and using the global symmetries, the worldsheet S-matrix was uniquely determined up to an overall phase. We refer the reader to [12, 77] for a more complete discussion of these and other exact properties of the worldsheet S-matrix.

## 3.2 Simplifying Limits

Due to the complexity of the world sheet theory, going beyond the leading perturbative term is challenging. One simplifying limit which has proved useful is the “near-flat limit” [78]. This limit corresponds to studying the worldsheet near a constant density solution boosted with rapidity  $\lambda^{1/4}$  in the worldsheet light-cone direction,  $\sigma^-$ . The left- and right-moving excitations on the worldsheet scale differently and the right movers essentially decouple. The resulting theory has only quartic interactions and is much

more tractable. The one-loop and two-loop [79] corrections to the S-matrix have been calculated and shown to match the all-order conjecture [22]; furthermore factorization at one-loop was explicitly shown. In the two-loop calculation radiative corrections induce a correction to the relativistic dispersion relation which corresponds to the expansion of the sine function, natural from a spin chain perspective, which appears in the exact dispersion relation [75].

Another interesting formulation of the theory is found via a generalisation of the Pohlmeyer reduction [80] which is used to relate, at a classical level, the string theory on  $AdS_5 \times S^5$  to a massive, Lorentz invariant theory which only involves the physical fields. Applied to strings on  $\mathbb{R} \times S^3$  this method consists of gauge fixing and solving the Virasoro constraints so that the remaining degree of freedom satisfies the sine-Gordon equation of motion [81]. Generalised to the full superstring [82] the reduced theory is a massive deformation of a gauged WZW model with an integrable potential. The resulting model has been explicitly shown to be UV finite to two-loops and there is evidence that the equivalence to the standard formulation persists at the quantum level [83]. The two-particle S-matrix was calculated in this formalism in [84] where it was shown that it has the appropriate group factorisation properties. Being manifestly Lorentz invariant this formalism may provide a better basis for understanding the quantum theory.

**Acknowledgements:** It is a pleasure to thank N. Beisert, T. Klose, M. Magro and A. Tseytlin for useful comments on the manuscript.

## References

- [1] R. R. Metsaev and A. A. Tseytlin, “*Type IIB superstring action in  $AdS_5 \times S^5$  background*”, Nucl. Phys. B533, 109 (1998), [hep-th/9805028](#).
- [2] A. Tseytlin, “*Review of AdS/CFT Integrability, Chapter II.1: Classical  $AdS_5 \times S^5$  string solutions*”, [arxiv:1012.3986](#).
- [3] T. Klose, “*Review of AdS/CFT Integrability, Chapter IV.3:  $\mathcal{N} = 6$  Chern-Simons and Strings on  $AdS_4 \times CP^3$* ”, [arxiv:1012.3999](#).
- [4] N. Drukker, D. J. Gross and A. A. Tseytlin, “*Green-Schwarz string in  $AdS_5 \times S^5$ : Semiclassical partition function*”, JHEP 0004, 021 (2000), [hep-th/0001204](#).
- [5] S. Frolov and A. A. Tseytlin, “*Semiclassical quantization of rotating superstring in  $AdS_5 \times S^5$* ”, JHEP 0206, 007 (2002), [hep-th/0204226](#).
- [6] S. S. Gubser, I. R. Klebanov and A. M. Polyakov, “*A semi-classical limit of the gauge/string correspondence*”, Nucl. Phys. B636, 99 (2002), [hep-th/0204051](#).
- [7] A. V. Belitsky, A. S. Gorsky and G. P. Korchemsky, “*Logarithmic scaling in gauge / string correspondence*”, Nucl. Phys. B748, 24 (2006), [hep-th/0601112](#).
- [8] S. Frolov, A. Tirziu and A. A. Tseytlin, “*Logarithmic corrections to higher twist scaling at strong coupling from AdS/CFT*”, Nucl. Phys. B766, 232 (2007), [hep-th/0611269](#).
- [9] B. Eden and M. Staudacher, “*Integrability and transcendentality*”, J. Stat. Mech. 0611, P014 (2006), [hep-th/0603157](#).

- [10] N. Beisert, B. Eden and M. Staudacher, “*Transcendentality and crossing*”, J. Stat. Mech. 0701, P021 (2007), [hep-th/0610251](#).
- [11] M. Staudacher, “*Review of AdS/CFT Integrability, Chapter III.1: Bethe Ansatz and the R-Matrix Formalism*”, [arxiv:1012.3990](#).
- [12] C. Ahn and R. I. Nepomechie, “*Review of AdS/CFT Integrability, Chapter III.2: Exact world-sheet S-matrix*”, [arxiv:1012.3991](#). • P. Vieira and D. Volin, “*Review of AdS/CFT Integrability, Chapter III.3: The dressing factor*”, [arxiv:1012.3992](#).
- [13] R. Roiban and A. A. Tseytlin, “*Strong-coupling expansion of cusp anomaly from quantum superstring*”, JHEP 0711, 016 (2007), [arxiv:0709.0681](#).
- [14] R. Roiban, A. Tirziu and A. A. Tseytlin, “*Two-loop world-sheet corrections in  $AdS_5 \times S^5$  superstring*”, JHEP 0707, 056 (2007), [arxiv:0704.3638](#).
- [15] S. Giombi, R. Ricci, R. Roiban, A. A. Tseytlin and C. Vergu, “*Quantum  $AdS_5 \times S^5$  superstring in the AdS light-cone gauge*”, [arxiv:0912.5105](#).
- [16] G. Arutyunov, S. Frolov and M. Staudacher, “*Bethe ansatz for quantum strings*”, JHEP 0410, 016 (2004), [hep-th/0406256](#).
- [17] M. Staudacher, “*The factorized S-matrix of CFT/AdS*”, JHEP 0505, 054 (2005), [hep-th/0412188](#).
- [18] N. Beisert and M. Staudacher, “*Long-range PSU(2,2/4) Bethe ansatz for gauge theory and strings*”, Nucl. Phys. B727, 1 (2005), [hep-th/0504190](#).
- [19] N. Beisert and A. A. Tseytlin, “*On quantum corrections to spinning strings and Bethe equations*”, Phys. Lett. B629, 102 (2005), [hep-th/0509084](#).
- [20] R. Hernandez and E. Lopez, “*Quantum corrections to the string Bethe ansatz*”, JHEP 0607, 004 (2006), [hep-th/0603204](#).
- [21] L. Freyhult and C. Kristjansen, “*A universality test of the quantum string Bethe ansatz*”, Phys. Lett. B638, 258 (2006), [hep-th/0604069](#).
- [22] N. Beisert, R. Hernandez and E. Lopez, “*A crossing-symmetric phase for  $AdS_5 \times S^5$  strings*”, JHEP 0611, 070 (2006), [hep-th/0609044](#).
- [23] L. Freyhult, “*Review of AdS/CFT Integrability, Chapter III.4: Twist states and the cusp anomalous dimension*”, [arxiv:1012.3993](#).
- [24] S. Forste, D. Ghoshal and S. Theisen, “*Stringy corrections to the Wilson loop in  $N = 4$  super Yang-Mills theory*”, JHEP 9908, 013 (1999), [hep-th/9903042](#). • J. Sonnenschein, “*Wilson loops from supergravity and string theory*”, Class. Quant. Grav. 17, 1257 (2000), [hep-th/9910089](#). • Y. Kinar, E. Schreiber, J. Sonnenschein and N. Weiss, “*Quantum fluctuations of Wilson loops from string models*”, Nucl. Phys. B583, 76 (2000), [hep-th/9911123](#). • V. Forini, “*Quark-antiquark potential in AdS at one loop*”, JHEP 1011, 079 (2010), [arxiv:1009.3939](#).
- [25] R. A. Janik, “*String fluctuations, AdS/CFT and the soft pomeron intercept*”, Phys. Lett. B500, 118 (2001), [hep-th/0010069](#). • L. A. Pando Zayas, J. Sonnenschein and D. Vaman, “*Regge trajectories revisited in the gauge / string correspondence*”, Nucl. Phys. B682, 3 (2004), [hep-th/0311190](#).
- [26] M. Kruczenski, R. Roiban, A. Tirziu and A. A. Tseytlin, “*Strong-coupling expansion of cusp anomaly and gluon amplitudes from quantum open strings in  $AdS_5 \times S^5$* ”, Nucl. Phys. B791, 93 (2008), [arxiv:0707.4254](#).

- [27] D. E. Berenstein, J. M. Maldacena and H. S. Nastase, “*Strings in flat space and pp waves from  $N = 4$  super Yang Mills*”, JHEP 0204, 013 (2002), [hep-th/0202021](#).
- [28] R. R. Metsaev and A. A. Tseytlin, “*Superstring action in  $AdS(5) \times S(5)$ : kappa-symmetry light cone gauge*”, Phys. Rev. D63, 046002 (2001), [hep-th/0007036](#). • R. R. Metsaev, C. B. Thorn and A. A. Tseytlin, “*Light-cone superstring in  $AdS$  space-time*”, Nucl. Phys. B596, 151 (2001), [hep-th/0009171](#).
- [29] C. G. Callan, Jr., H. K. Lee, T. McLoughlin, J. H. Schwarz, I. Swanson and X. Wu, “*Quantizing string theory in  $AdS_5 \times S^5$ : Beyond the pp-wave*”, Nucl. Phys. B673, 3 (2003), [hep-th/0307032](#).
- [30] C. G. Callan, Jr., T. McLoughlin and I. Swanson, “*Holography beyond the Penrose limit*”, Nucl. Phys. B694, 115 (2004), [hep-th/0404007](#).
- [31] G. Arutyunov and S. Frolov, “*Uniform light-cone gauge for strings in  $AdS_5 \times S^5$ : Solving  $su(1/1)$  sector*”, JHEP 0601, 055 (2006), [hep-th/0510208](#).
- [32] S. Frolov, J. Plefka and M. Zamaklar, “*The  $AdS_5 \times S^5$  superstring in light-cone gauge and its Bethe equations*”, J. Phys. A39, 13037 (2006), [hep-th/0603008](#).
- [33] G. Arutyunov, S. Frolov and M. Zamaklar, “*Finite-size effects from giant magnons*”, Nucl. Phys. B778, 1 (2007), [hep-th/0606126](#).
- [34] G. Arutyunov and S. Frolov, “*Integrable Hamiltonian for classical strings on  $AdS_5 \times S^5$* ”, JHEP 0502, 059 (2005), [hep-th/0411089](#).
- [35] R. R. Metsaev, “*Type IIB Green-Schwarz superstring in plane wave Ramond- Ramond background*”, Nucl. Phys. B625, 70 (2002), [hep-th/0112044](#). • R. R. Metsaev and A. A. Tseytlin, “*Exactly solvable model of superstring in plane wave Ramond-Ramond background*”, Phys. Rev. D65, 126004 (2002), [hep-th/0202109](#).
- [36] A. Parnachev and A. V. Ryzhov, “*Strings in the near plane wave background and  $AdS/CFT$* ”, JHEP 0210, 066 (2002), [hep-th/0208010](#).
- [37] C. G. Callan, Jr., T. McLoughlin and I. Swanson, “*Higher impurity  $AdS/CFT$  correspondence in the near-BMN limit*”, Nucl. Phys. B700, 271 (2004), [hep-th/0405153](#). • T. McLoughlin and I. Swanson, “ *$N$ -impurity superstring spectra near the pp-wave limit*”, Nucl. Phys. B702, 86 (2004), [hep-th/0407240](#).
- [38] G. Arutyunov and S. Frolov, “*Foundations of the  $AdS_5 \times S^5$  Superstring. Part I*”, J. Phys. A42, 254003 (2009), [arxiv:0901.4937](#).
- [39] R. Roiban and A. A. Tseytlin, “*Spinning superstrings at two loops: strong-coupling corrections to dimensions of large-twist SYM operators*”, Phys. Rev. D77, 066006 (2008), [arxiv:0712.2479](#).
- [40] S. Giombi, R. Ricci, R. Roiban, A. A. Tseytlin and C. Vergu, “*Generalized scaling function from light-cone gauge  $AdS_5 \times S^5$  superstring*”, [arxiv:1002.0018](#).
- [41] R. F. Dashen, B. Hasslacher and A. Neveu, “*The Particle Spectrum in Model Field Theories from Semiclassical Functional Integral Techniques*”, Phys. Rev. D11, 3424 (1975).
- [42] D. M. Hofman and J. M. Maldacena, “*Giant magnons*”, J. Phys. A39, 13095 (2006), [hep-th/0604135](#).

- [43] J. A. Minahan, “Zero modes for the giant magnon”, JHEP 0702, 048 (2007), [hep-th/0701005](#). • G. Papathanasiou and M. Spradlin, “Semiclassical Quantization of the Giant Magnon”, JHEP 0706, 032 (2007), [arxiv:0704.2389](#). • H.-Y. Chen, N. Dorey and R. F. Lima Matos, “Quantum Scattering of Giant Magnons”, JHEP 0709, 106 (2007), [arxiv:0707.0668](#).
- [44] S. Schäfer-Nameki, “Review of AdS/CFT Integrability, Chapter II.4: The Spectral Curve”, [arxiv:1012.3989](#).
- [45] V. Mikhaylov, “On the Fermionic Frequencies of Circular Strings”, [arxiv:1002.1831](#).
- [46] M. Kruczenski, “A note on twist two operators in  $N = 4$  SYM and Wilson loops in Minkowski signature”, JHEP 0212, 024 (2002), [hep-th/0210115](#).
- [47] R. Kallosh and A. A. Tseytlin, “Simplifying superstring action on  $AdS_5 \times S^5$ ”, JHEP 9810, 016 (1998), [hep-th/9808088](#).
- [48] S. Giombi, R. Ricci, R. Roiban and A. Tseytlin, “Two-loop  $AdS_5 \times S^5$  superstring: testing asymptotic Bethe ansatz and finite size corrections”, [arxiv:1010.4594](#), \* Temporary entry \*.
- [49] P. Y. Casteill and C. Kristjansen, “The Strong Coupling Limit of the Scaling Function from the Quantum String Bethe Ansatz”, Nucl. Phys. B785, 1 (2007), [arxiv:0705.0890](#). • N. Gromov, “Generalized Scaling Function at Strong Coupling”, JHEP 0811, 085 (2008), [arxiv:0805.4615](#). • Z. Bajnok, J. Balog, B. Basso, G. P. Korchemsky and L. Palla, “Scaling function in AdS/CFT from the  $O(6)$  sigma model”, Nucl. Phys. B811, 438 (2009), [arxiv:0809.4952](#).
- [50] S. Frolov and A. A. Tseytlin, “Multi-spin string solutions in  $AdS_5 \times S^5$ ”, Nucl. Phys. B668, 77 (2003), [hep-th/0304255](#).
- [51] G. Arutyunov, J. Russo and A. A. Tseytlin, “Spinning strings in  $AdS_5 \times S^5$ : New integrable system relations”, Phys. Rev. D69, 086009 (2004), [hep-th/0311004](#).
- [52] S. Frolov and A. A. Tseytlin, “Quantizing three-spin string solution in  $AdS_5 \times S^5$ ”, JHEP 0307, 016 (2003), [hep-th/0306130](#). • S. A. Frolov, I. Y. Park and A. A. Tseytlin, “On one-loop correction to energy of spinning strings in  $S^5$ ”, Phys. Rev. D71, 026006 (2005), [hep-th/0408187](#).
- [53] N. Beisert, A. A. Tseytlin and K. Zarembo, “Matching quantum strings to quantum spins: One-loop vs. finite-size corrections”, Nucl. Phys. B715, 190 (2005), [hep-th/0502173](#).
- [54] I. Y. Park, A. Tirziu and A. A. Tseytlin, “Spinning strings in  $AdS_5 \times S^5$ : One-loop correction to energy in  $SL(2)$  sector”, JHEP 0503, 013 (2005), [hep-th/0501203](#).
- [55] S. Schafer-Nameki and M. Zamaklar, “Stringy sums and corrections to the quantum string Bethe ansatz”, JHEP 0510, 044 (2005), [hep-th/0509096](#).
- [56] S. Schafer-Nameki, “Exact expressions for quantum corrections to spinning strings”, Phys. Lett. B639, 571 (2006), [hep-th/0602214](#).
- [57] H. J. de Vega, A. L. Larsen and N. G. Sanchez, “Semiclassical quantization of circular strings in de Sitter and anti-de Sitter space-times”, Phys. Rev. D51, 6917 (1995), [hep-th/9410219](#).

- [58] R. Hernandez, E. Lopez, A. Perianez and G. Sierra, “*Finite size effects in ferromagnetic spin chains and quantum corrections to classical strings*”, JHEP 0506, 011 (2005), [hep-th/0502188](#).
- [59] S. Schafer-Nameki, M. Zamaklar and K. Zarembo, “*Quantum corrections to spinning strings in  $AdS_5 \times S^5$  and Bethe ansatz: A comparative study*”, JHEP 0509, 051 (2005), [hep-th/0507189](#).
- [60] J. A. Minahan, A. Tirziu and A. A. Tseytlin, “ *$1/J^2$  corrections to BMN energies from the quantum long range Landau-Lifshitz model*”, JHEP 0511, 031 (2005), [hep-th/0510080](#).
- [61] M. Beccaria, V. Forini, A. Tirziu and A. A. Tseytlin, “*Structure of large spin expansion of anomalous dimensions at strong coupling*”, Nucl. Phys. B812, 144 (2009), [arxiv:0809.5234](#).
- [62] M. Beccaria, G. V. Dunne, V. Forini, M. Pawellek and A. A. Tseytlin, “*Exact computation of one-loop correction to energy of spinning folded string in  $AdS_5 \times S^5$* ”, J. Phys. A 43, 165402 (2010), [arxiv:1001.4018](#).
- [63] A. Tirziu and A. A. Tseytlin, “*Quantum corrections to energy of short spinning string in  $AdS_5$* ”, Phys. Rev. D78, 066002 (2008), [arxiv:0806.4758](#).
- [64] M. Beccaria and A. Tirziu, “*On the short string limit of the folded spinning string in  $AdS_5 \times S^5$* ”, [arxiv:0810.4127](#).
- [65] R. Roiban and A. A. Tseytlin, “*Quantum strings in  $AdS_5 \times S^5$ : strong-coupling corrections to dimension of Konishi operator*”, [arxiv:0906.4294](#).
- [66] S. Schafer-Nameki, M. Zamaklar and K. Zarembo, “*How accurate is the quantum string Bethe ansatz?*”, JHEP 0612, 020 (2006), [hep-th/0610250](#).
- [67] V. Kazakov and N. Gromov, “*Review of AdS/CFT Integrability, Chapter III.7: Hirota Dynamics for Quantum Integrability*”, [arxiv:1012.3996](#). • Z. Bajnok, “*Review of AdS/CFT Integrability, Chapter III.6: Thermodynamic Bethe Ansatz*”, [arxiv:1012.3995](#).
- [68] A. Hentschel, J. Plefka and P. Sundin, “*Testing the nested light-cone Bethe equations of the  $AdS_5 \times S^5$  superstring*”, JHEP 0705, 021 (2007), [hep-th/0703187](#).
- [69] G. Arutyunov and S. Frolov, “*On  $AdS_5 \times S^5$  string S-matrix*”, Phys. Lett. B639, 378 (2006), [hep-th/0604043](#).
- [70] T. Klose, T. McLoughlin, R. Roiban and K. Zarembo, “*Worldsheet scattering in  $AdS_5 \times S^5$* ”, JHEP 0703, 094 (2007), [hep-th/0611169](#).
- [71] G. Arutyunov, S. Frolov, J. Plefka and M. Zamaklar, “*The off-shell symmetry algebra of the light-cone  $AdS_5 \times S^5$  superstring*”, J. Phys. A40, 3583 (2007), [hep-th/0609157](#).
- [72] G. Arutyunov, S. Frolov and M. Zamaklar, “*The Zamolodchikov-Faddeev algebra for  $AdS_5 \times S^5$  superstring*”, JHEP 0704, 002 (2007), [hep-th/0612229](#).
- [73] I. Bena, J. Polchinski and R. Roiban, “*Hidden symmetries of the  $AdS_5 \times S^5$  superstring*”, Phys. Rev. D69, 046002 (2004), [hep-th/0305116](#).
- [74] E. Ogievetsky, P. Wiegmann and N. Reshetikhin, “*The Principal Chiral Field in Two-Dimensions on Classical Lie Algebras: The Bethe Ansatz Solution and Factorized Theory of Scattering*”, Nucl. Phys. B280, 45 (1987).

- [75] N. Beisert, “*The  $su(2/2)$  dynamic  $S$ -matrix*”, Adv. Theor. Math. Phys. 12, 945 (2008), [hep-th/0511082](#).
- [76] N. Beisert and F. Spill, “*The Classical  $r$ -matrix of  $AdS/CFT$  and its Lie Bialgebra Structure*”, Commun. Math. Phys. 285, 537 (2009), [arxiv:0708.1762](#).
- [77] A. Torrielli, “*Review of  $AdS/CFT$  Integrability, Chapter VI.2: Yangian Algebra*”, [arxiv:1012.4005](#).
- [78] J. M. Maldacena and I. Swanson, “*Connecting giant magnons to the pp-wave: An interpolating limit of  $AdS_5 \times S^5$* ”, Phys. Rev. D76, 026002 (2007), [hep-th/0612079](#).
- [79] T. Klose and K. Zarembo, “*Reduced sigma-model on  $AdS_5 \times S^5$ : one-loop scattering amplitudes*”, JHEP 0702, 071 (2007), [hep-th/0701240](#). • T. Klose, T. McLoughlin, J. A. Minahan and K. Zarembo, “*World-sheet scattering in  $AdS_5 \times S^5$  at two loops*”, JHEP 0708, 051 (2007), [arxiv:0704.3891](#). • V. Giangreco Marotta Puletti, T. Klose and O. Ohlsson Sax, “*Factorized world-sheet scattering in near-flat  $AdS_5 \times S^5$* ”, Nucl. Phys. B792, 228 (2008), [arxiv:0707.2082](#).
- [80] K. Pohlmeyer, “*Integrable Hamiltonian Systems and Interactions Through Quadratic Constraints*”, Commun. Math. Phys. 46, 207 (1976).
- [81] A. A. Tseytlin, “*Spinning strings and  $AdS/CFT$  duality*”, [hep-th/0311139](#). • A. Mikhailov, “*An action variable of the sine-Gordon model*”, J. Geom. Phys. 56, 2429 (2006), [hep-th/0504035](#).
- [82] M. Grigoriev and A. A. Tseytlin, “*Pohlmeyer reduction of  $AdS_5 \times S^5$  superstring sigma model*”, Nucl. Phys. B800, 450 (2008), [arxiv:0711.0155](#). • A. Mikhailov and S. Schafer-Nameki, “*Sine-Gordon-like action for the Superstring in  $AdS(5) \times S(5)$* ”, JHEP 0805, 075 (2008), [arxiv:0711.0195](#). • M. Grigoriev and A. A. Tseytlin, “*On reduced models for superstrings on  $AdS_n \times S^n$* ”, Int. J. Mod. Phys. A23, 2107 (2008), [arxiv:0806.2623](#). • J. L. Miramontes, “*Pohlmeyer reduction revisited*”, JHEP 0810, 087 (2008), [arxiv:0808.3365](#).
- [83] R. Roiban and A. A. Tseytlin, “*UV finiteness of Pohlmeyer-reduced form of the  $AdS_5 \times S^5$  superstring theory*”, JHEP 0904, 078 (2009), [arxiv:0902.2489](#). • B. Hoare, Y. Iwashita and A. A. Tseytlin, “*Pohlmeyer-reduced form of string theory in  $AdS_5 \times S^5$ : semiclassical expansion*”, [arxiv:0906.3800](#).
- [84] B. Hoare and A. A. Tseytlin, “*Tree-level  $S$ -matrix of Pohlmeyer reduced form of  $AdS_5 \times S^5$  superstring theory*”, JHEP 1002, 094 (2010), [arxiv:0912.2958](#). • B. Hoare and A. Tseytlin, “*On the perturbative  $S$ -matrix of generalized sine-Gordon models*”, JHEP 1011, 111 (2010), [arxiv:1008.4914](#).

# Review of AdS/CFT Integrability, Chapter II.3: Sigma Model, Gauge Fixing

MARC MAGRO

*Université de Lyon, Laboratoire de Physique, ENS Lyon et CNRS UMR 5672,  
46 allée d'Italie, 69364 Lyon CEDEX 07, France*

*and*

*Max-Planck-Institut für Gravitationsphysik  
Albert-Einstein-Institut  
Am Mühlenberg 1, 14476 Potsdam, Germany*

Marc.Magro@ens-lyon.fr

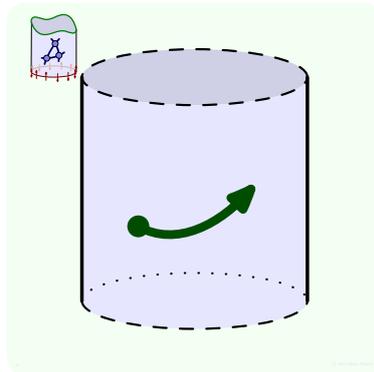

**Abstract:** This review is devoted to the classical integrability of the  $\text{AdS}_5 \times \text{S}^5$  superstring theory. It starts with a reminder of the corresponding action as a coset model. The symmetries of this action are then reviewed. The classical integrability is then considered from the lagrangian and hamiltonian points of view. The second part of this review deals with the gauge fixing of this theory. Finally, some aspects of the pure spinor formulation are also briefly reviewed.

# 1 Introduction

The list of topics reviewed in this chapter is the following. First, we review the classical action of  $AdS_5 \times S^5$  superstring theory as a supercoset model and its symmetries. The next topic concerns the integrability of that model and two important objects related to it, the Lax pair and the monodromy matrix. For all these aspects, a key role is played by a  $\mathbb{Z}_4$  grading of the superalgebra  $\mathfrak{psu}(2, 2|4)$ . The integrability property is then discussed from a Hamiltonian point of view. More precisely, it is recalled how to prove that an infinite number of conserved quantities are in involution. The first part of this chapter ends by recalling how factorized scattering theory is used in the quantum case. The second part of the review deals with gauge fixing, in particular with the so called uniform light-cone gauge, which is adapted to apply factorized scattering theory and to test the AdS/CFT conjecture. This chapter ends with some aspects related to the pure spinor formulation.

**Note** The topics reviewed here are restricted on purpose. The main references related to these topics are indicated in the last section.

## 2 Classical integrability

### 2.1 Action as a coset model and its symmetries

**Metsaev-Tseytlin Action** The action is of the sigma-model type on the coset super-space<sup>1</sup>

$$G/H = PSU(2, 2|4) / [SO(4, 1) \times SO(5)], \quad (2.1)$$

together with a Wess-Zumino term [2]. This is therefore a generalization of the situation encountered in the flat case [3]. The bosonic part of the coset defined by (2.1) is  $SO(4, 2)/SO(4, 1) \times SO(6)/SO(5)$  which corresponds to  $AdS_5 \times S^5$ . The Lie superalgebra  $\mathfrak{su}(2, 2|4)$  is a non-compact real form of  $\mathfrak{sl}(4|4)$ , which can itself be spanned by the  $8 \times 8$  matrices written in  $4 \times 4$  blocks and whose supertrace (Str) vanishes. Here  $\text{Str } M = \text{Tr } A - \text{Tr } D$  where  $A$  and  $D$  are the top and bottom diagonal  $4 \times 4$  blocks of the matrix  $M$ . The superalgebra  $\mathfrak{g} = \mathfrak{psu}(2, 2|4)$  is then obtained by quotienting  $\mathfrak{su}(2, 2|4)$  over the  $\mathfrak{u}(1)$  factor corresponding to the identity. In the following,  $\{t_A\}$  denotes a corresponding basis of  $\mathfrak{g}$ ,  $\eta_{AB} = \text{Str}(t_A t_B)$  and  $\eta^{AB}$  its inverse.

The coset (2.1) is associated with an automorphism  $\Omega$  of order 4 of  $\mathfrak{g}$ . This means that  $\mathfrak{g}$  admits a  $\mathbb{Z}_4$  grading:

$$\mathfrak{g} = \mathfrak{g}^{(0)} \oplus \mathfrak{g}^{(1)} \oplus \mathfrak{g}^{(2)} \oplus \mathfrak{g}^{(3)} \quad (2.2)$$

with  $\mathfrak{g}^{(0)} = \mathfrak{h} = \mathfrak{so}(4, 1) \oplus \mathfrak{so}(5)$  and  $[\mathfrak{g}^{(m)}, \mathfrak{g}^{(n)}] \subset \mathfrak{g}^{(p)}$  with  $p = m + n \pmod{4}$ . The generators of  $\mathfrak{g}^{(0)}$  and  $\mathfrak{g}^{(2)}$  are even while those of  $\mathfrak{g}^{(1)}$  and  $\mathfrak{g}^{(3)}$  are odd. The supertrace

<sup>1</sup>More precisely, one needs to consider the universal cover as the physical space  $AdS_5$  is a universal cover, see [1].

is compatible with the  $\mathbb{Z}_4$  grading, which means that  $\text{Str}(M_m M_n) = 0$  for  $M_m \in \mathfrak{g}^{(m)}$ ,  $M_n \in \mathfrak{g}^{(n)}$  and  $m + n \neq 0 \pmod{4}$ .

Let  $(\sigma, \tau)$  be coordinates on the world-sheet and  $g(\sigma, \tau)$  a periodic function,  $g(\sigma + \ell, \tau) = g(\sigma, \tau)$ , taking values in  $G$ . The Lagrangian is written in terms of the left-invariant current  $A_\alpha = -g^{-1} \partial_\alpha g$ :

$$L = -\frac{\sqrt{\lambda}}{4\pi} \text{Str} \left[ \gamma^{\alpha\beta} A_\alpha^{(2)} A_\beta^{(2)} + \kappa \epsilon^{\alpha\beta} A_\alpha^{(1)} A_\beta^{(3)} \right]. \quad (2.3)$$

Here,  $\epsilon^{\alpha\beta}$  is antisymmetric with  $\epsilon^{\tau\sigma} = 1$ ;  $\gamma^{\alpha\beta}$  is the Weyl-invariant combination of the world-sheet metric with  $\det \gamma = -1$ . For convenience, the coefficient in front of the Lagrangian has been written in terms of the t'Hooft coupling constant  $\lambda$ , with the AdS/CFT correspondence  $\sqrt{\lambda} \leftrightarrow (R^2/\alpha')$ , where  $R$  is the common radius of  $S^5$  and  $AdS_5$  and  $\alpha'$  the string slope.

The first term of the action corresponds simply to a non-linear sigma model on  $AdS_5 \times S^5$ . The second term is like a Wess-Zumino term which relies on the  $\mathbb{Z}_4$  decomposition of  $\mathfrak{g}$ . This comes from the property<sup>2</sup> [4]

$$2 \text{Str}(A^{(2)} \wedge A^{(3)} \wedge A^{(3)} - A^{(2)} \wedge A^{(1)} \wedge A^{(1)}) = d \text{Str}(A^{(1)} \wedge A^{(3)})$$

which shows that the l.h.s. is a closed and exact 3-form and explains the 2d expression of the Wess-Zumino term. The coefficient  $\kappa$  in front of this Wess-Zumino term is in fact equal to  $\pm 1$  in order to have  $\kappa$ -symmetry (see below).

**Equations of motion and global  $PSU(2, 2|4)$  symmetry** By varying the action with respect to  $g$ , one finds the following equation of motion:

$$\partial_\alpha S^\alpha - [A_\alpha, S^\alpha] = 0 \quad (2.4)$$

where  $S^\alpha = \gamma^{\alpha\beta} A_\beta^{(2)} - \frac{1}{2} \epsilon^{\alpha\beta} (A_\beta^{(1)} - A_\beta^{(3)})$ . By definition, the current  $A_\alpha$  is also a solution of the Maurer-Cartan equation

$$\partial_0 A_1 - \partial_1 A_0 - [A_0, A_1] = 0. \quad (2.5)$$

$A_\alpha$  being the left-invariant current, the action corresponding to (2.3) is invariant under the global transformation  $g(\sigma, \tau) \rightarrow \tilde{g}g(\sigma, \tau)$  with  $\tilde{g} \in PSU(2, 2|4)$ . The equation of motion (2.4) is identical to the equation of conservation of the Noether current  $(\sqrt{\lambda}/2\pi)gS^\alpha g^{-1}$  associated with that symmetry. The corresponding Noether charge and its projection onto an element  $M \in \mathfrak{psu}(2, 2|4)$  are respectively

$$Q = \frac{\sqrt{\lambda}}{2\pi} \int_0^\ell d\sigma g S^0 g^{-1} \quad \text{and} \quad Q_M = \text{Str}(QM). \quad (2.6)$$

**$SO(4, 1) \times SO(5)$  gauge symmetry** Under a local right multiplication  $g(\sigma, \tau) \rightarrow g(\sigma, \tau)h(\sigma, \tau)$  with  $h(\sigma, \tau) \in H$ , the components  $A_\alpha^{(1,2,3)}$  of the current transform as  $A_\alpha^{(1,2,3)} \rightarrow h^{-1} A_\alpha^{(1,2,3)} h$ . This shows that the action is invariant under these  $SO(4, 1) \times SO(5)$  gauge transformations.

---

<sup>2</sup>Using form notations.

**Virasoro constraints and reparametrization** Varying the action with respect to the metric gives the Virasoro constraints

$$\text{Str}(A_\alpha^{(2)} A_\beta^{(2)}) - \frac{1}{2} \gamma_{\alpha\beta} \gamma^{\rho\sigma} \text{Str}(A_\rho^{(2)} A_\sigma^{(2)}) = 0 \quad (2.7)$$

which reflect the two-dimensional reparameterization invariance of the action.

**$\kappa$ -symmetry** This symmetry is a key property of the Green-Schwarz formulation of superstring theories as it enables the reduction of the fermionic degrees of freedom to the physical ones. It acts on both the group element  $g$  and the world-sheet metric  $\gamma^{\alpha\beta}$ . Its action on  $g$  can be viewed as a particular local right multiplication that depends on fermionic parameters [5]. More precisely, at the infinitesimal level, it corresponds to  $\delta g = g(\epsilon^{(1)} + \epsilon^{(3)})$  with<sup>3</sup>

$$\epsilon^{(1)} = iA_{\alpha,+}^{(2)} \kappa_-^{(1)\alpha} + i\kappa_-^{(1)\alpha} A_{\alpha,+}^{(2)} \quad \text{and} \quad \epsilon^{(3)} = iA_{\alpha,-}^{(2)} \kappa_+^{(3)\alpha} + i\kappa_+^{(3)\alpha} A_{\alpha,-}^{(2)}.$$

In these equations,  $V_\pm^\alpha \equiv \frac{1}{2}(\gamma^{\alpha\beta} \mp \epsilon^{\alpha\beta})V_\beta$ ,  $\kappa_+^{(1)} = 0$  and  $\kappa_-^{(3)} = 0$ . The corresponding transformation of the metric can be written as:

$$\delta\gamma^{\alpha\beta} = -\frac{1}{2} \text{Str} \left( W \left( [i\kappa_-^{(1)\alpha}, A_-^{(1)\beta}] + [i\kappa_+^{(3)\alpha}, A_+^{(3)\beta}] \right) \right)$$

where  $W$  is the diagonal matrix  $(1, \dots, 1, -1, \dots, -1)$ .

## 2.2 Lagrangian integrability

**Lax pair and monodromy** The requirement for classical integrability is the existence of an infinite number of conserved quantities. This is ensured when the equations of motion are equivalent to a zero curvature equation

$$\partial_\alpha L_\beta - \partial_\beta L_\alpha - [L_\alpha, L_\beta] = 0 \quad (2.8)$$

associated with a Lax connection  $L_\alpha(\sigma, \tau, z)$  depending on the dynamical fields and on a complex spectral parameter  $z$ . Indeed, a consequence of this equation is that the monodromy

$$T(\tau, z) = \overleftarrow{\text{exp}} \int_0^\ell d\sigma L_\sigma(\sigma, \tau, z) \quad (2.9)$$

satisfies the equation

$$\partial_\tau T(\tau, z) = [L_\tau(0, \tau, z), T(\tau, z)].$$

Therefore, its eigenvalues, which depend on the complex spectral parameter  $z$ , form an infinite set of conserved quantities. Let us remark that for an integrable model defined on the 2d plane rather than on the cylinder, the time evolution of the corresponding monodromy matrix obeys the equation

$$\partial_\tau T(\tau, z) = L_\tau(+\infty, \tau, z)T(\tau, z) - T(\tau, z)L_\tau(-\infty, \tau, z).$$

<sup>3</sup>See §6.1 of [6] or §1.2.3 of [7] for more details.

However, to have configurations of finite energy, one has typically  $L_\tau(\sigma, \tau, z) \rightarrow 0$  when  $\sigma \rightarrow \pm\infty$ . If it is the case, then the whole monodromy is conserved.

A Lax connection is not unique and one can construct other Lax connections by making a formal gauge transformation<sup>4</sup>

$$L_\alpha \rightarrow UL_\alpha U^{-1} + \partial_\alpha U U^{-1} \quad (2.10)$$

where  $U(\sigma + \ell, \tau) = U(\sigma, \tau)$ . The eigenvalues of  $T(\tau, z)$  are invariant under such transformations.

The fact that  $AdS_5 \times S^5$  superstring theory is integrable is not the sole peculiarity of this theory. It originates in the existence of the associated  $\mathbb{Z}_4$  grading and is a generalization of the situation encountered in the bosonic case for a symmetric coset corresponding to a  $\mathbb{Z}_2$  grading. To prove the existence of a Lax connection, one can start with an ansatz for  $L_\alpha(z)$  generalizing the situation for the symmetric spaces<sup>5</sup>,

$$L(z) = a_1(z)A^{(0)} + a_2(z)A^{(2)} + a_3(z) * A^{(2)} + a_4(z)A^{(1)} + a_5(z)A^{(3)},$$

and determine the conditions on the coefficients  $a_i(z)$  in order the flatness condition (2.8) to reproduce the Maurer-Cartan equations (2.5) and the equation of motion (2.4). Proceeding like that, one can show that the quantity

$$L(z) = A^{(0)} + z^{-1}A^{(1)} + \frac{1}{2}(z^2 + z^{-2})A^{(2)} + \frac{1}{2}(z^2 - z^{-2}) * A^{(2)} + zA^{(3)} \quad (2.11)$$

is a Lax connection [8].

**$\kappa$ -symmetry and integrability** As previously mentioned, the theory is invariant under  $\kappa$ -symmetry transformations only when the parameter  $\kappa$  in front of the Wess-Zumino term equals  $\pm 1$ . The existence of a Lax connection or, in other words, the integrability of the theory, is only valid for the same values of  $\kappa$ . One rough way to understand this fact is that the corresponding bosonic coset model is integrable. This integrability property is thus extended to the full Green-Schwarz action, via the  $\kappa$ -symmetry, which relates bosons to fermions. It is also possible to prove that under a  $\kappa$ -symmetry transformation, and using the Virasoro constraints (2.7), the Lax connection (2.11) undergoes a formal gauge transformation (2.10). This shows that the eigenvalues of the monodromy matrix are  $\kappa$ -symmetry invariant. Note that it is also clear that these eigenvalues are invariant under a  $SO(4, 1) \times SO(5)$  gauge transformation.

**Local and non-local conserved charges** The conserved charges are both local and non-local. Typically, they can be obtained by expansion around some particular value of the spectral parameter. One can obtain for instance a sequence of local charges. Another possible sequence starts with the Noether charges (2.6) and goes on with multi-local charges. This discussion is closely related to the study of the algebraic curve [9], which is associated with the eigenvalues of  $T(z)$ . It is also related to the construction of the Yangian charges. We refer to [10], [11] and more generally to [12].

<sup>4</sup>In the present case,  $U \in PSU(2, 2|4)$ .

<sup>5</sup>We use here form notations and  $*$  designates the Hodge star on the worldsheet.

## 2.3 Hamiltonian integrability

**Canonical analysis** At the Hamiltonian level, a "conservative" definition of integrability requires a further condition. There must be an infinite number of conserved quantities that are in involution, which means that their Poisson brackets (P.B.) vanish. For finite dimensional systems, this condition is necessary in order to apply Liouville's theorem. The proof that such a property holds for string theory on  $AdS_5 \times S^5$  is rather technical and therefore only intermediate steps will be reviewed here.

The first step is to do a canonical analysis by considering the current  $A_\alpha$  as a dynamical variable rather than the group element  $g$  itself. Due to this choice and to the gauge invariances of the action, there are constraints on the phase space. Applying the Dirac procedure for constrained systems, one finds that the theory can be described by the spatial component  $A_\sigma(\sigma, \tau)$  of this current and its conjugate momentum  $\Pi(\sigma, \tau)$  with four types of constraints. First the Virasoro constraints. Then a bosonic constraint,  $\mathcal{C}^{(0)}$ , associated with the  $SO(4, 1) \times SO(5)$  gauge invariance. Finally, two fermionic constraints  $(\mathcal{C}^{(1)}, \mathcal{C}^{(3)})$ . It is possible to extract from each of the fermionic constraints two constraints,  $(\mathcal{K}^{(1)}, \mathcal{K}^{(3)})$ , which are first-class<sup>6</sup> and generate the  $\kappa$ -symmetry transformations. However, as usual with  $\kappa$ -symmetry, it is not possible to separate covariantly  $(\mathcal{C}^{(1)}, \mathcal{C}^{(3)})$  into  $(\mathcal{K}^{(1)}, \mathcal{K}^{(3)})$  and a complementary set of second-class constraints.

Rather than  $\Pi$  itself, the interesting quantity is in fact  $(\nabla_\sigma \Pi)$  where  $\nabla_\sigma = \partial_\sigma - [A_\sigma, \cdot]$ . In the case of the principal chiral model, this can be understood as  $(\nabla_\sigma \Pi)$  coincides with the time component  $A_\tau$  of the current. The result of this analysis is that the P.B. of  $A_\sigma$  and  $(\nabla_\sigma \Pi)$  take the same form as in the principal chiral model. The most convenient way to write these P.B. is to use tensorial notation and to define for any quantity  $M \in \mathfrak{g}$ ,  $M_{\underline{1}} = M \otimes 1$  and  $M_{\underline{2}} = 1 \otimes M$ . Then, we have<sup>7</sup>,

$$\begin{aligned} \{A_{\sigma\underline{1}}(\sigma), A_{\sigma\underline{2}}(\sigma')\} &= 0, \\ \{(\nabla_\sigma \Pi)_{\underline{1}}(\sigma), A_{\sigma\underline{2}}(\sigma')\} &= [C_{\underline{1}\underline{2}}, A_{\sigma\underline{2}}] \delta_{\sigma\sigma'} - C_{\underline{1}\underline{2}} \partial_\sigma \delta_{\sigma\sigma'}, \\ \{(\nabla_\sigma \Pi)_{\underline{1}}(\sigma), (\nabla_\sigma \Pi)_{\underline{2}}(\sigma')\} &= [C_{\underline{1}\underline{2}}, (\nabla_\sigma \Pi)_{\underline{2}}] \delta_{\sigma\sigma'}. \end{aligned}$$

The quadratic Casimir is defined by:

$$C_{\underline{1}\underline{2}} = \eta^{AB} t_A \otimes t_B = C_{\underline{1}\underline{2}}^{(00)} + C_{\underline{1}\underline{2}}^{(13)} + C_{\underline{1}\underline{2}}^{(22)} + C_{\underline{1}\underline{2}}^{(31)},$$

where in the last equality we have projected into the different gradings. The important characteristic of these P.B. is the presence of a non-ultra local term, proportional to  $\delta'$ .

**Hamiltonian Lax Connection** The next step is to mimic the procedure recalled above for the Lagrangian analysis. One can start with a general expression for an Hamiltonian Lax connection as a linear combination of  $A_\sigma^{(i)}$  and  $(\nabla_\sigma \Pi)^{(j)}$ . However, this does not fix completely the Lax connection and leads to many different possibilities, that differ from each other by terms proportional to the constraints. It is nevertheless possible to determine a unique linear combination that satisfies the two following conditions.

<sup>6</sup>Which means that their P.B. with all the other constraints vanish on the constraint surface.

<sup>7</sup>The time dependence is not indicated in the P.B. as they are equal-time P.B.

Firstly, that the zero curvature condition holds on the whole phase space, which means even without using the constraints. Secondly, that the conserved quantities  $\text{Str}[T^n(z)]$  obtained from the monodromy matrix associated with this particular Lax connection are first-class, or, in other words, gauge-invariant. It is possible to show that the corresponding  $L_\alpha^H(z)$  differs from the corresponding Lagrangian expression (2.11) by terms proportional to the constraints.

**Poisson brackets of  $L_\sigma^H(z)$**  The goal is to compute the Poisson brackets of the monodromy matrix associated with  $L_\sigma^H(z)$ . This requires first to compute the Poisson brackets of two spatial Lax components. This computation is straightforward. However, organizing the result in a specific algebraic form is much more difficult. Denoting  $\mathcal{L}(\sigma, z) \equiv L_\sigma^H(\sigma, \tau; z)$ , the result of this analysis is

$$\{\mathcal{L}_1(\sigma, z_1), \mathcal{L}_2(\sigma', z_2)\} = [r_{\underline{12}}^-(z_1, z_2), \mathcal{L}_1(\sigma, z_1)]\delta_{\sigma\sigma'} + [r_{\underline{12}}^+(z_1, z_2), \mathcal{L}_2(\sigma, z_2)]\delta_{\sigma\sigma'} - (r_{\underline{12}}^+(z_1, z_2) - r_{\underline{12}}^-(z_1, z_2))\partial_\sigma\delta_{\sigma\sigma'}. \quad (2.12)$$

The matrices  $r_{\underline{12}}^\pm$  have the following expression:

$$r_{\underline{12}}^-(z_1, z_2) = \frac{2 \sum_{j=0}^3 z_1^j z_2^{4-j} C_{\underline{12}}^{(j \ 4-j)}}{\phi(z_2)(z_2^4 - z_1^4)}, \quad r_{\underline{12}}^+(z_1, z_2) = \frac{2 \sum_{j=0}^3 z_1^{4-j} z_2^j C_{\underline{12}}^{(4-j \ j)}}{\phi(z_1)(z_2^4 - z_1^4)}$$

with  $\phi(z) = z(du/dz)$  where

$$u(z) = 2 \frac{1 + z^4}{1 - z^4} \quad (2.13)$$

is the Zhukovsky map. The form (2.12) of the P.B. is exactly similar to the one appearing in the principal chiral model [13], [14]. It is again non ultra-local due to the presence of the  $\delta'$  term. The Jacobi identity for the Poisson bracket (2.12) is ensured by the following property

$$[r_{\underline{12}}^-, r_{\underline{13}}^-] + [r_{\underline{12}}^-, r_{\underline{23}}^-] + [r_{\underline{32}}^-, r_{\underline{13}}^-] = 0 \quad (2.14)$$

satisfied by  $r_{\underline{12}}^-$ .

**Algebraic interpretation and the Zhukovsky map** As usual with integrable models, it is also possible and instructive to start the story from a purely algebraic point of view. In this framework, the approach corresponds to the so-called  $R$ -matrix one. This means to construct first the  $r_{\underline{12}}^\pm$  matrices independently of the model considered i.e. without any reference to phase-space variables. The realization in terms of phase space variables is then achieved at the end *via* the matrix  $\mathcal{L}(\sigma, z)$ .

Starting from  $\mathfrak{g} = \mathfrak{psu}(2, 2|4)$ , one considers its loop algebra<sup>8</sup>  $\mathfrak{Lg} = \mathfrak{g}[[z, z^{-1}]]$ . Any  $X(z) \in \mathfrak{Lg}$  can be decomposed into its pole part,  $\pi_-(X)$  and its regular part  $\pi_+(X)$ . This splitting of  $\mathfrak{Lg}$  enables one to define a  $R$ -matrix on  $\text{End } \mathfrak{Lg}$ . It is simply given by  $R = \pi_+ - \pi_-$  and satisfies the modified classical Yang-Baxter equation:

$$[R(X), R(Y)] - R([R(X), Y] + [X, R(Y)]) = -[X, Y]. \quad (2.15)$$

<sup>8</sup>More precisely, it is necessary to consider its twisted loop algebra  $\mathfrak{Lg}^\Omega$ , where the twist is induced by the  $\mathbb{Z}_4$ -grading  $\Omega$  of  $\mathfrak{g}$ .

Let  $(\cdot, \cdot)$  be an inner-product on  $\mathfrak{Lg}$ . This inner product has a natural extension on  $\mathfrak{Lg} \otimes \mathfrak{Lg}$ . One can then associate to any operator  $\mathfrak{D} \in \text{End } \mathfrak{Lg}$  its kernel  $\mathfrak{D}_{\underline{12}} \in \mathfrak{Lg} \otimes \mathfrak{Lg}$  through the relation

$$\forall X, Y \in \mathfrak{Lg}, \quad (\mathfrak{D}(X), Y) = (\mathfrak{D}_{\underline{12}}, Y \otimes X).$$

An important property is that the kernel of  $\mathfrak{D}^*$  is simply<sup>9</sup>  $\mathfrak{D}_{\underline{21}}$ . The eq.(2.15) can then be rewritten successively as

$$\begin{aligned} [R_{\underline{12}}, R_{\underline{13}}] + [R_{\underline{12}}, R_{\underline{23}}] + [R_{\underline{32}}, R_{\underline{13}}] &= -\widehat{\omega}_{\underline{123}}, \\ [R_{\underline{12}}, R_{\underline{13}}] + [R_{\underline{12}}, R_{\underline{23}}] - [R_{\underline{13}}, R_{\underline{23}}^*] &= -\widehat{\omega}_{\underline{123}}. \end{aligned} \quad (2.16)$$

For simplicity the expression of  $\widehat{\omega}$  is not reproduced here (see [15]).

The key point is the following: if we take the inner product

$$(X, Y)_u = \oint \frac{du}{2\pi i} \text{Str}(X(z)Y(z))$$

with  $u(z)$  given by (2.13), then  $R^* \neq -R$ . This means that the eq.(2.16) does not correspond to the classical Yang-Baxter equation but to<sup>10</sup> the eq.(2.14) with  $R_{\underline{12}} = r_{\underline{12}}^-$  and  $R_{\underline{12}}^* = -r_{\underline{12}}^+$ . Therefore, the integrable structure of the  $AdS_5 \times S^5$  superstring fits precisely into the general  $R$ -matrix approach. The specifics of this model are encoded in its hamiltonian Lax matrix which can be formally written as

$$\mathcal{L}(\sigma, z) = 4\phi(z)^{-1} \sum_{k=1}^{\infty} z^k \left( kA_1^{(k)} + 2(\nabla_\sigma \Pi)^{(k)} \right).$$

**Involution of the conserved quantities** The last step, which is the computation of the P.B. of the monodromy matrix (2.9) from the result (2.12) is delicate. Indeed, the non ultra-local term in (2.12) leads to ambiguities for the P.B. of the monodromy. The way to proceed is the following. Consider the transition matrices

$$T(\sigma_1, \sigma_2, \tau, z) = \overleftarrow{\exp} \int_{\sigma_2}^{\sigma_1} d\sigma \mathcal{L}(\sigma, z).$$

The P.B. of two transition matrices with all different points are well defined. However, there are ambiguities whenever two points coincide. A simple argument to understand this property is the following. To compute the P.B. of  $T(\sigma_1, \sigma_2, \tau, z)$  with  $T(\sigma'_1, \sigma'_2, \tau, z')$ , we have, schematically, to twice integrate a  $\delta'$  term multiplied by some smooth function. Omitting for brevity the function, we have to evaluate

$$\int_{\sigma_2}^{\sigma_1} d\sigma \int_{\sigma'_2}^{\sigma'_1} d\sigma' \partial_\sigma \delta_{\sigma\sigma'} = \chi(\sigma_1; [\sigma'_2, \sigma'_1]) - \chi(\sigma_2; [\sigma'_2, \sigma'_1]),$$

<sup>9</sup>  $\mathfrak{D}_{\underline{21}} = P(\mathfrak{D}_{\underline{12}})$  with  $P(A \otimes B) = B \otimes A$ .

<sup>10</sup>The r.h.s.  $-\widehat{\omega}$  is a contact term proportional to  $\delta(z_1 - z_2)\delta(z_2 - z_3)$  and is absent in eq.(2.14).

where  $\chi(\sigma; [\sigma', \sigma''])$  is the characteristic function of the interval  $[\sigma', \sigma'']$ . But this function is undefined when two points coincide. Therefore the P.B. of the monodromy matrices  $T(\tau, z) = T(\ell, 0, \tau, z)$  and  $T(\tau, z')$  is not well defined. However, it has been proved in [14] that one can give a meaning to the limit of coinciding points if one imposes that the P.B. of the monodromy matrix satisfies the antisymmetry and the derivation rules. This leads to a regularization which consists in point splitting and in applying a symmetric limit procedure. This regularization is equivalent to taking  $\theta(0) = 1/2$  where  $\theta$  is the Heaviside function. This procedure leads to the following result for the P.B. of the monodromy matrix:

$$\{T_{\underline{1}}, T_{\underline{2}}\} = \frac{1}{2}[r_{\underline{1}\underline{2}}^+ + r_{\underline{1}\underline{2}}^-, T_{\underline{1}}T_{\underline{2}}] + \frac{1}{2}T_{\underline{1}}(r_{\underline{1}\underline{2}}^+ - r_{\underline{1}\underline{2}}^-)T_{\underline{2}} - \frac{1}{2}T_{\underline{2}}(r_{\underline{1}\underline{2}}^+ - r_{\underline{1}\underline{2}}^-)T_{\underline{1}}, \quad (2.17)$$

where  $T_{\underline{1}} = T(\tau, z_1) \otimes \text{Id}$  and  $T_{\underline{2}} = \text{Id} \otimes T(\tau, z_2)$ . This P.B. is called the classical exchange algebra. Taking the supertrace on both spaces  $\underline{1}$  and  $\underline{2}$ , one finds that the conserved quantities  $\text{Str}[T^n(z_1)]$  and  $\text{Str}[T^m(z_2)]$  are in involution. Let us however insist that contrary to what happens for the monodromy, the P.B. of  $\text{Str}[T^n(z_1)]$  and  $\text{Str}[T^m(z_2)]$  has no ambiguity. In other words, its vanishing is independent of the choice of regularization.

**What is the quantum exchange algebra ?** The quantum analogue of the exchange algebra (2.17) is not known. This is in fact a long-standing problem for non ultra-local integrable models. The reason is that the P.B. (2.17) does not satisfy completely the Jacobi identity. This means that the P.B.  $\{T_{\underline{1}}, \{T_{\underline{2}}, \{\dots, \dots\}, T_{\underline{n}}\}\}$  with  $n$  occurrences of  $T$  must be separately defined for each  $n$ . This is clearly an obstruction for the determination of the quantum exchange algebra.

There are however integrable models for which the quantum exchange algebra is known. The simplest ones are of course ultra-local models. In that case  $r_{\underline{1}\underline{2}}^+ = r_{\underline{1}\underline{2}}^-$  is an antisymmetric  $r$ -matrix, solution of the classical Yang-Baxter equation

$$[r_{\underline{1}\underline{2}}, r_{\underline{1}\underline{3}}] + [r_{\underline{1}\underline{2}}, r_{\underline{2}\underline{3}}] + [r_{\underline{1}\underline{3}}, r_{\underline{2}\underline{3}}] = 0. \quad (2.18)$$

The quantum exchange algebra is then simply  $R_{\underline{1}\underline{2}}T_{\underline{1}}T_{\underline{2}} = T_{\underline{2}}T_{\underline{1}}R_{\underline{1}\underline{2}}$  with  $R_{\underline{1}\underline{2}} = 1 + \hbar r_{\underline{1}\underline{2}} + \dots$  a solution of the quantum Yang-Baxter equation  $R_{\underline{1}\underline{2}}R_{\underline{1}\underline{3}}R_{\underline{2}\underline{3}} = R_{\underline{2}\underline{3}}R_{\underline{1}\underline{3}}R_{\underline{1}\underline{2}}$ . The interest of such a relation is that one can discretize the model and apply Bethe Ansatz techniques.

Another possibility, this time for some specific non ultra-local models, is when the matrices  $r_{\underline{1}\underline{2}}^\pm$  are such that  $r_{\underline{1}\underline{2}} = (1/2)(r_{\underline{1}\underline{2}}^+ + r_{\underline{1}\underline{2}}^-)$  satisfies the classical Yang-Baxter equation (2.18). Denoting  $s_{\underline{1}\underline{2}} = (1/2)(r_{\underline{1}\underline{2}}^+ - r_{\underline{1}\underline{2}}^-)$ , the quantum analogue of (2.17) for these models is [16], [17]:

$$R_{\underline{1}\underline{2}}T_{\underline{1}}S_{\underline{1}\underline{2}}T_{\underline{2}} = T_{\underline{2}}S_{\underline{1}\underline{2}}T_{\underline{1}}R_{\underline{1}\underline{2}}.$$

with  $S_{\underline{1}\underline{2}} = 1 + \hbar s_{\underline{1}\underline{2}} + \dots$  and similarly for  $R$  and  $r$ . However, for both the principal chiral model and the superstring on  $AdS_5 \times S^5$ , the corresponding matrix  $r_{\underline{1}\underline{2}}$  does not satisfy the classical Yang-Baxter equation.

For  $AdS_5 \times S^5$  superstring theory, the only available results so far consist in the approach developed in [18] within the pure spinor formulation (see section 4) and the

subsequent conjecture made there. Some interesting results have however been obtained very recently in [19] for conformal models on supergroups.

At this point, the results obtained in [20], [21] for the bosonic subsector  $\mathbb{R} \times S^3$  of the full theory have to be mentioned. For this subsector, one has a similar P.B. as in eq.(2.17). However, on the space of finite-gap solutions, it is possible to show that some variables form a set of action-angle variables if one computes their P.B. from the expression (2.17). Such a result is interesting because it confirms the correctness of the expression for the action variables obtained from the algebraic curve.

## 2.4 Quantum integrability and factorized scattering theory

In order to compute the spectrum at the quantum level, one has therefore to follow another road. The idea is then to apply the methods of factorized scattering theory [22]. The prerequisites are the following. As usual for quantization within the Green-Schwarz formulation, the first step is to go to a light-cone gauge<sup>11</sup>. In such a gauge, the theory has a massive spectrum. The idea is then to study first the decompactification limit by considering the theory on a plane instead of a cylinder. Since the theory has a massive spectrum, it makes sense to talk about a world-sheet  $S$ -matrix in that limit. Note however that the light-cone gauge action is not Lorentz invariant and therefore some properties must be adapted and extended to the case at hand. The key hypothesis is to suppose that the theory remains integrable at the quantum level. This assumption means that the  $n \rightarrow n$   $S$ -matrix factorizes into a product of  $2 \rightarrow 2$   $S$ -matrices. Let us insist here that it is in fact not necessary to have an infinite number of conserved quantities (see [24] for a review). The next step is then to determine the dispersion relation and the two-body  $S$ -matrix from the symmetries<sup>12</sup> of the light-cone gauged action in the decompactification limit. Thus, an important question related to that program is to determine these symmetries. Once all these steps are completed, finite size effects can be considered. Here we review the first steps of this procedure.

# 3 Gauge Fixing

## 3.1 Motivation and choice of gauges

In this review, we will mainly focus on the light-cone gauge that is most adapted to the program detailed above with the further requirement that it is suited for the comparison between the energy of string states and the conformal dimension of the dual  $\mathcal{N} = 4$  Yang-Mills operators.

Let us begin by recalling a few things about light-cone gauges. Consider first the purely bosonic case. In flat space, light-cone gauge fixing is realized in two steps. The first one consists in going to the conformal gauge  $\gamma^{\alpha\beta} = \eta^{\alpha\beta}$ . The second one is to fix the

---

<sup>11</sup>Another possibility developed in [6], [23] and subsequent articles for the full  $AdS_5 \times S^5$  theory is to go to a conformal gauge and to make a Pohlmeyer reduction. This has the advantage of keeping manifest the 2d Lorentz invariance.

<sup>12</sup>More precisely the "off-shell" symmetries, see below.

residual conformal diffeomorphism symmetry by imposing  $x_+(\sigma, \tau) = \tau$ . Another way to implement these gauge fixing conditions is to use the first-order formulation [25] and to impose  $x_+ = \tau$  and to fix  $p_+$ , the momentum conjugate of  $x_-$ , to a constant. If these two ways to proceed are equivalent in flat space, this is no more the case for a curved space. Furthermore, it is impossible to apply the first procedure in the case of  $AdS_5 \times S^5$ , in particular because its null Killing vectors are not covariantly constant [26]. Therefore, the bosonic light-cone gauge conditions are imposed within the first-order formulation.

As recalled in [27], there are two inequivalent sets of null geodesics in  $AdS_5 \times S^5$ : for the first set, the geodesic stays entirely in  $AdS_5$ , for the second one it wraps a big circle of  $S^5$ . These two possibilities correspond to two types of light-cone gauges. In the case of superstrings, the  $\kappa$ -symmetry invariance must be also fixed and this leads again to different possibilities. Using the Poincaré coordinates patch, and viewing  $\mathfrak{psu}(2, 2|4)$  as the four-dimensional  $\mathcal{N} = 4$  super-conformal algebra, one possibility to fix  $\kappa$ -symmetry is to set the fermions associated with the 16 superboost generators to zero. This gauge is called the S-gauge. It has been used in particular in [28] for the study of the 2d duality of  $AdS_5 \times S^5$  related to the dual superconformal symmetry of scattering amplitudes in  $\mathcal{N} = 4$  super-Yang-Mills theory [29], [30] (see [31]). Another possibility is to put to zero half of these fermions and half of the fermions associated with the supersymmetry generators. Combined to the AdS light-cone gauge, this leads to the action in [32] which is at most quartic in the fermions.

### 3.2 Uniform light-cone gauge

The gauge we will review leads to much more complicated action than the AdS light-cone gauge but is well suited for the AdS/CFT correspondence. Indeed, to test this conjecture, one needs to compare the space-time energy  $E$  of a string state with the conformal dimension of the dual operator. One feature of the uniform light-cone gauge is precisely that the corresponding world-sheet Hamiltonian is simply related to  $E$ . We only review here the main steps for the bosonic string on  $AdS_5 \times S^5$  and refer to the literature for the complete treatment and for some subtleties omitted here.

**Bosonic case** (i) Consider first the metric in global coordinates

$$ds^2 = R^2 \left[ - \left( \frac{1 + z^2/4}{1 - z^2/4} \right)^2 dt^2 + \frac{dz_i^2}{(1 - z^2/4)^2} + \left( \frac{1 - y^2/4}{1 + y^2/4} \right)^2 d\phi^2 + \frac{dy_i^2}{(1 + y^2/4)^2} \right]$$

with  $i = 1, \dots, 4$  and where  $(t, z_i)$  describe  $AdS_5$ , with  $t$  the global time of  $AdS_5$ , while  $(\phi, y_i)$  describe  $S^5$ , with  $\phi$  an angle parameterizing the equator of  $S^5$ . The conserved charges associated with shifts in  $t$  and  $\phi$  are respectively the space-time energy  $E = - \int_0^\ell d\sigma p_t$  and the angular momentum  $J = \int_0^\ell d\sigma p_\phi$  where  $p_t$  and  $p_\phi$  are the conjugate momenta respectively of  $t$  and  $\phi$ . Define then  $x_- = \phi - t$  and  $x_+ = (1/2)(\phi + t)$ , such that  $p_- = (p_\phi + p_t)$  and  $p_+ = (1/2)(p_\phi - p_t)$ . The corresponding conserved charges associated with these densities are

$$P_- = J - E \quad \text{and} \quad P_+ = (1/2)(J + E). \quad (3.1)$$

(ii) The light-cone gauge conditions are

$$x_+ = \tau \quad \text{and} \quad p_+ = 1.$$

As a consequence of the last condition, the charge  $P_+$  is identical to  $\ell$ .

(iii) The next step is to solve the Virasoro constraints. One of them gives  $p_-$  in terms of a square root of the transverse coordinates<sup>13</sup>  $(x_M, p_M)$  while the other constraint together with the periodicity of the fields imply the following result for the world-sheet momentum  $p_{WS}$  of the string:

$$p_{WS} = - \int_0^\ell d\sigma p_M x'^M = \int_0^\ell d\sigma x'_- = 0.$$

This condition is called the level-matching condition. In the dual picture, it corresponds to the vanishing of the total momentum of multi-magnon configurations.

(iv) The Virasoro conditions being solved, the gauge-fixed Lagrangian is

$$p_M \dot{x}^M + p_+ \dot{x}_- + p_-.$$

Since  $p_+ = 1$ , the second term in the r.h.s. is a total derivative, which means that the light-cone gauged action is of the form  $\int (p_M \dot{x}^M - h)$  with the light-cone Hamiltonian density  $h = -p_-(x_M, x'_M, p_M)$ . Together with the relation (3.1), this means that the light-cone Hamiltonian  $H$  is identical to

$$H = -P_- = E - J. \tag{3.2}$$

This is the relation announced above between the space-time energy  $E$ , the light-cone Hamiltonian  $H$  and the angular momentum  $J$ .

(v) The way to deal with the level-matching condition is to impose it on the states. In the dual picture, this means for instance that double-magnon excitations can be considered. However, to correspond to a physical state, the two magnons should have opposite momenta. When the level-matching condition is imposed (respectively relaxed), one refers to the on-(off-)shell theory.

**Full theory** This short reminder does not reflect at all the difficulty when fermions are included ! In particular, some of the steps that need to be completed include choosing an adequate coset representative (which is such that all the fermions are neutral under the isometries generated by shifts of  $t$  and  $\phi$ ), fixing the  $\kappa$ -symmetry gauge invariance and developing the first-order formulation for the complete Metsaev - Tseytlin action.

**Decompactification limit** As discussed above, in order to make use of the factorized scattering theory, the first step is to consider the decompactification limit, which means to go from the cylinder to the plane. As  $\ell$  corresponds to  $P_+$  this limit is obtained by letting  $P_+ \rightarrow \infty$  while keeping  $\lambda$  fixed. Since the energies of the states are finite, the relations (3.1) imply that  $J$  goes to infinity in this limit.

---

<sup>13</sup>Formed by  $z_i, y_i$  and their conjugate momenta.

**Symmetry** Let us first consider the case  $P_+$  finite. It is clear from the results (3.2) and (3.1) that the light-cone Hamiltonian and  $P_+$  correspond to particular charges of the form (2.6). More precisely, we have

$$H = -\frac{i}{2}Q_{\Sigma_+} \quad \text{and} \quad P_+ = \frac{i}{4}Q_{\Sigma_-}$$

for some  $\Sigma_{\pm} \in \mathfrak{psu}(2, 2|4)$ . As  $x_+ = \tau$ , all the charges  $Q_M$  that are independent of  $x_+$  and commute with  $H$  are conserved. However, we have a general result

$$\{H, Q_M\} = -\frac{i}{2}\{Q_{\Sigma_+}, Q_M\} = -\frac{i}{2}Q_{[\Sigma_+, M]}. \quad (3.3)$$

Therefore, all the elements  $M \in \mathfrak{psu}(2, 2|4)$  that commute with  $\Sigma_+$  give conserved charges. It can be shown that these elements correspond to

$$\mathfrak{psu}(2|2) \oplus \mathfrak{psu}(2|2) \oplus \Sigma_+ \oplus \Sigma_-,$$

the two last elements being associated with  $H$  and  $P_+$ .

We need now first to go to the decompactification limit and then off-shell. In the decompactification limit, we are left a priori with  $\mathfrak{psu}(2|2) \oplus \mathfrak{psu}(2|2)$  together with a central charge that corresponds to the Hamiltonian. However, this is not the final answer for the off-shell theory. The reason is that for odd elements  $M_1$  and  $M_2$ , central charges may appear in the Poisson bracket  $\{Q_{M_1}, Q_{M_2}\}$ . This means that this P.B. is only equal to  $Q_{[M_1, M_2]}$  up to some central charges. An explicit computation enables one to determine these central charges and shows that the symmetry is  $\mathfrak{psu}(2|2) \oplus \mathfrak{psu}(2|2)$  extended by three central charges  $H$ ,  $C$  and  $C^\dagger$  with

$$C = \frac{i\sqrt{\lambda}}{4\pi}(e^{ip_{ws}} - 1).$$

As it should be,  $C$  vanishes when  $p_{ws} = 0$ . The determination of the off-shell symmetry algebra is the starting point needed to apply factorized scattering theory.

## 4 Pure spinor formulation

In this section, we mention some results that have been obtained for the pure spinor (P.S.) formulation and that are directly related to the aspects treated in this review for the Green-Schwarz (G.S.) formulation.

The Lagrangian can be written as<sup>14</sup> [33]

$$L = \frac{1}{2}A^{(2)}\bar{A}^{(2)} + \frac{1}{4}A^{(1)}\bar{A}^{(3)} + \frac{3}{4}A^{(3)}\bar{A}^{(1)} + w\bar{\partial}\lambda + \bar{w}\partial\bar{\lambda} - N\bar{A}^{(0)} - \bar{N}A^{(0)} - N\bar{N}.$$

It is written in conformal gauge. Here,  $A = -g^{-1}\partial g$  with  $\partial = \partial_0 + \partial_1$  while  $\bar{A} = -g^{-1}\bar{\partial}g$  with  $\bar{\partial} = \partial_0 - \partial_1$ . The fields  $\lambda$  and  $\bar{\lambda}$  are bosonic ghosts taking values in  $\mathfrak{g}^{(1)}$  and  $\mathfrak{g}^{(3)}$  respectively. They satisfy the pure spinor conditions:

$$[\lambda, \lambda]_+ = 0 \quad \text{and} \quad [\bar{\lambda}, \bar{\lambda}]_+ = 0.$$

---

<sup>14</sup>Taking the supertrace is understood.

$w$  and  $\bar{w}$ , are the conjugate momenta respectively of  $\lambda$  and  $\bar{\lambda}$  and take values respectively in  $\mathfrak{g}^{(3)}$  and  $\mathfrak{g}^{(1)}$ . Finally,  $N$  and  $\bar{N}$  are the pure spinor currents defined by:

$$N = -[w, \lambda]_+ = -w\lambda - \lambda w \quad \text{and} \quad \bar{N} = -[\bar{w}, \bar{\lambda}]_+ = -\bar{w}\bar{\lambda} - \bar{\lambda}\bar{w}.$$

They take values in  $\mathfrak{g}^{(0)}$ . There are a  $SO(4, 1) \times SO(5)$  gauge invariance and a global  $PSU(2, 2|4)$  invariance. However,  $\kappa$ -symmetry is not present but there is an invariance under a BRST symmetry  $Q = \int \text{Str}(dz\lambda A_3 + d\bar{z}\bar{\lambda}\bar{A}_1)$ .

The equations of motion can again be rewritten as a zero curvature equation  $\partial\bar{\mathcal{L}} - \partial\bar{\mathcal{L}} - [\bar{\mathcal{L}}, \mathcal{L}] = 0$  for the Lax connection [34]

$$\begin{aligned} \mathcal{L}(z) &= (A^{(0)} + N - z^4 N) + zA^{(1)} + z^2 A^{(2)} + z^3 A^{(3)}, \\ \bar{\mathcal{L}}(z) &= (\bar{A}^{(0)} + \bar{N} - z^{-4} \bar{N}) + z^{-3} \bar{A}^{(1)} + z^{-2} \bar{A}^{(2)} + z^{-1} \bar{A}^{(3)}, \end{aligned}$$

which means that the theory is classically integrable. In the G.S. formulation, the eigenvalues of the monodromy matrix are  $\kappa$ -symmetry invariant. The corresponding statement in the P.S. formulation is that they are BRST invariant. When putting the ghosts to zero, the Lagrangian Lax pair is different from the one in (2.11). However, it is possible again to determine an Hamiltonian Lax connection for the P.S. formulation. This connection agrees with the Hamiltonian one of the G.S. formulation up to terms proportional to the ghosts. As a consequence, the P.S. classical exchange algebra is the same as in the G.S. formulation and this property remains true when the contribution of the ghosts to the P.B. is included. This classical exchange algebra has been first obtained in<sup>15</sup> [18].

As this review focuses on the classical case, we just indicate briefly some results related to the quantum case and which are directly relevant to the framework of this review. Contrary to the G.S. formulation where going to a light-cone gauge breaks the global  $PSU(2, 2|4)$  symmetry and the conformal invariance, the quantization of the P.S. action is done within the framework of a 2d conformal field theory with an unbroken  $PSU(2, 2|4)$  invariance. It has been proved that at the quantum level this theory is conformally and BRST invariant [35], [36]. Furthermore, the classically conserved non-local currents can be made BRST invariant at the quantum level [37]. The one-loop corrections to the tree level OPE [38] [39] [40] of the left-invariant currents have been studied in [41] and it has been explicitly demonstrated in [38] that the monodromy matrix is not renormalized at one loop.

## 5 References

First of all, for many aspects treated in this chapter, the reader is referred to the extended pedagogical review [7]. The reference [42] presents a systematic discussion of other string backgrounds that share the properties reviewed in §2.1. A general reference on integrable models is the book [12]. The classical exchange algebra was first obtained within the pure spinor formulation in [18]. It was rederived within that formulation and within the

<sup>15</sup>There is a subtlety in the actual comparison with the result (2.12) due to the fact that the observables considered in [18] are gauge-invariant.

Green-Schwarz formulation in [43]. The analysis to fix the Hamiltonian Lax connection has been presented in [44]. The algebraic origin and interpretation of the Hamiltonian Lax connection and of the  $r_{\mathbf{12}}^{\pm}$  matrices have been put forward in [15]. General references about the  $R$ -matrix approach can be found in the bibliography of the latter. For earlier attempts to compute the classical exchange algebra, see [45], [46], [47], and [48], [49] in AdS light-cone gauge. For the problem of non ultra-local terms we recommend the thesis [50]. For the AdS light-cone gauge, we refer to the proceedings [51], to the original references [52], [32] and to [53] for the integrability of the theory in that gauge. For the uniform light-cone gauge, the references for the topics reviewed here are [54], [55], [56] and more specifically [57], [58] and, once again, the review [7]. Further references are indicated in [59]. Finally, the references [60] and [61] contain a pedagogical introduction to the P.S. formulation of  $AdS_5 \times S^5$  superstring theory.

**Acknowledgments** I thank F. Delduc and B. Vicedo for their comments. This review was written when visiting the Albert-Einstein-Institut. I thank this Institute for its kind hospitality. This work is also partially supported by Agence Nationale de la Recherche under the contract ANR-07-CEXC-010.

## References

- [1] N. Beisert, “*Review of AdS/CFT Integrability, Chapter VI.1: Superconformal Algebra*”, arxiv:1012.4004.
- [2] R. R. Metsaev and A. A. Tseytlin, “*Type IIB superstring action in  $AdS_5 \times S^5$  background*”, Nucl. Phys. B533, 109 (1998), hep-th/9805028.
- [3] M. Henneaux and L. Mezincescu, “*A Sigma Model Interpretation of Green-Schwarz Covariant Superstring Action*”, Phys. Lett. B152, 340 (1985).
- [4] N. Berkovits, M. Bershadsky, T. Hauer, S. Zhukov and B. Zwiebach, “*Superstring theory on  $AdS_2 \times S^2$  as a coset supermanifold*”, Nucl. Phys. B567, 61 (2000), hep-th/9907200.
- [5] I. N. McArthur, “*Kappa-symmetry of Green-Schwarz actions in coset superspaces*”, Nucl. Phys. B573, 811 (2000), hep-th/9908045.
- [6] M. Grigoriev and A. A. Tseytlin, “*Pohlmeyer reduction of  $AdS_5 \times S^5$  superstring sigma model*”, Nucl. Phys. B800, 450 (2008), arxiv:0711.0155.
- [7] G. Arutyunov and S. Frolov, “*Foundations of the  $AdS_5 \times S^5$  Superstring. Part I*”, J. Phys. A42, 254003 (2009), arxiv:0901.4937.
- [8] I. Bena, J. Polchinski and R. Roiban, “*Hidden symmetries of the  $AdS_5 \times S^5$  superstring*”, Phys. Rev. D69, 046002 (2004), hep-th/0305116.
- [9] N. Beisert, V. A. Kazakov, K. Sakai and K. Zarembo, “*The algebraic curve of classical superstrings on  $AdS_5 \times S^5$* ”, Commun. Math. Phys. 263, 659 (2006), hep-th/0502226.
- [10] S. Schäfer-Nameki, “*Review of AdS/CFT Integrability, Chapter II.4: The Spectral Curve*”, arxiv:1012.3989.
- [11] A. Torrielli, “*Review of AdS/CFT Integrability, Chapter VI.2: Yangian Algebra*”, arxiv:1012.4005.

- [12] O. Babelon, D. Bernard and M. Talon, “*Introduction to Classical Integrable Models*”, Cambridge University Press (2003).
- [13] J. M. Maillet, “*Kac-Moody algebra and extended Yang-baxter relations in the  $O(N)$  non-linear sigma model*”, Phys. Lett. B162, 137 (1985).
- [14] J. M. Maillet, “*New integrable canonical structures in two-dimensional models*”, Nucl. Phys. B269, 54 (1986).
- [15] B. Vicedo, “*The classical R-matrix of AdS/CFT and its Lie dialgebra structure*”, arxiv:1003.1192.
- [16] L. Freidel and J. M. Maillet, “*Quadratic algebras and integrable systems*”, Phys. Lett. B262, 278 (1991).
- [17] L. Freidel and J. M. Maillet, “*On classical and quantum integrable field theories associated to Kac-Moody current algebras*”, Phys. Lett. B263, 403 (1991).
- [18] A. Mikhailov and S. Schäfer-Nameki, “*Algebra of transfer-matrices and Yang-Baxter equations on the string worldsheet in  $AdS_5 \times S^5$* ”, Nucl. Phys. B802, 1 (2008), arxiv:0712.4278.
- [19] R. Benichou, “*Fusion of line operators in conformal sigma-models on supergroups, and the Hirota equation*”, arxiv:1011.3158.
- [20] N. Dorey and B. Vicedo, “*A symplectic structure for string theory on integrable backgrounds*”, JHEP 0703, 045 (2007), hep-th/0606287.
- [21] B. Vicedo, “*Semiclassical Quantisation of Finite-Gap Strings*”, JHEP 0806, 086 (2008), arxiv:0803.1605.
- [22] A. B. Zamolodchikov and A. B. Zamolodchikov, “*Factorized S-matrices in two dimensions as the exact solutions of certain relativistic quantum field models*”, Annals Phys. 120, 253 (1979).
- [23] A. Mikhailov and S. Schäfer-Nameki, “*Sine-Gordon-like action for the Superstring in  $AdS(5) \times S(5)$* ”, JHEP 0805, 075 (2008), arxiv:0711.0195.
- [24] P. Dorey, “*Exact S matrices*”, hep-th/9810026, Proceedings of the Eotvos Summer School in Physics: Conformal field theories and integrable models.
- [25] P. Goddard, J. Goldstone, C. Rebbi and C. B. Thorn, “*Quantum dynamics of a massless relativistic string*”, Nucl. Phys. B56, 109 (1973).
- [26] G. T. Horowitz and A. R. Steif, “*Strings in strong gravitational fields*”, Phys. Rev. D42, 1950 (1990).
- [27] A. Tseytlin, “*Review of AdS/CFT Integrability, Chapter II.1: Classical  $AdS_5 \times S^5$  string solutions*”, arxiv:1012.3986.
- [28] N. Beisert, R. Ricci, A. A. Tseytlin and M. Wolf, “*Dual Superconformal Symmetry from  $AdS_5 \times S^5$  Superstring Integrability*”, Phys. Rev. D78, 126004 (2008), arxiv:0807.3228.
- [29] J. M. Drummond, J. Henn, V. A. Smirnov and E. Sokatchev, “*Magic identities for conformal four-point integrals*”, JHEP 0701, 064 (2007), hep-th/0607160.
- [30] J. M. Drummond, J. Henn, G. P. Korchemsky and E. Sokatchev, “*Dual superconformal symmetry of scattering amplitudes in  $\mathcal{N} = 4$  super-Yang-Mills theory*”, arxiv:0807.1095.

- [31] J. Drummond, “*Review of AdS/CFT Integrability, Chapter V.2: Dual Superconformal Symmetry*”, [arxiv:1012.4002](#).
- [32] R. R. Metsaev and A. A. Tseytlin, “*Superstring action in  $AdS_5 \times S^5$ : kappa-symmetry light cone gauge*”, *Phys. Rev. D* **63**, 046002 (2001), [hep-th/0007036](#).
- [33] N. Berkovits, “*Super-Poincare covariant quantization of the superstring*”, *JHEP* **0004**, 018 (2000), [hep-th/0001035](#).
- [34] B. C. Vallilo, “*Flat currents in the classical  $AdS_5 \times S^5$  pure spinor superstring*”, *JHEP* **0403**, 037 (2004), [hep-th/0307018](#).
- [35] N. Berkovits, “*Quantum consistency of the superstring in  $AdS_5 \times S^5$  background*”, *JHEP* **0503**, 041 (2005), [hep-th/0411170](#).
- [36] B. C. Vallilo, “*One loop conformal invariance of the superstring in an  $AdS_5 \times S^5$  background*”, *JHEP* **0212**, 042 (2002), [hep-th/0210064](#).
- [37] N. Berkovits, “*BRST cohomology and nonlocal conserved charges*”, *JHEP* **0502**, 060 (2005), [hep-th/0409159](#).
- [38] A. Mikhailov and S. Schäfer-Nameki, “*Perturbative study of the transfer matrix on the string worldsheet in  $AdS_5 \times S^5$* ”, [arxiv:0706.1525](#).
- [39] V. G. M. Puletti, “*Operator product expansion for pure spinor superstring on  $AdS_5 \times S^5$* ”, *JHEP* **0610**, 057 (2006), [hep-th/0607076](#).
- [40] M. Bianchi and J. Kluson, “*Current algebra of the pure spinor superstring in  $AdS_5 \times S^5$* ”, *JHEP* **0608**, 030 (2006), [hep-th/0606188](#).
- [41] O. A. Bedoya, D. Z. Marchioro, D. L. Nedel and B. C. Vallilo, “*Quantum Current Algebra for the  $AdS_5 \times S^5$  Superstring*”, [arxiv:1003.0701](#).
- [42] K. Zarembo, “*Strings on Semisymmetric Superspaces*”, [arxiv:1003.0465](#).
- [43] M. Magro, “*The Classical Exchange Algebra of  $AdS_5 \times S^5$  String Theory*”, *JHEP* **0901**, 021 (2009), [arxiv:0810.4136](#).
- [44] B. Vicedo, “*Hamiltonian dynamics and the hidden symmetries of the  $AdS_5 \times S^5$  superstring*”, [arxiv:0910.0221](#).
- [45] A. K. Das, J. Maharana, A. Melikyan and M. Sato, “*The algebra of transition matrices for the  $AdS_5 \times S^5$  superstring*”, *JHEP* **0412**, 055 (2004), [hep-th/0411200](#).
- [46] A. Mikhailov, “*Bihamiltonian structure of the classical superstring in  $AdS_5 \times S^5$* ”, [hep-th/0609108](#).
- [47] J. Kluson, “*Reduced Sigma-Model on  $O(N)$ : Hamiltonian Analysis and Poisson Bracket of Lax Connection*”, *JHEP* **0709**, 100 (2007), [arxiv:0707.3264](#).
- [48] A. K. Das, A. Melikyan and M. Sato, “*The algebra of flat currents for the string on  $AdS_5 \times S^5$  in the light-cone gauge*”, *JHEP* **0511**, 015 (2005), [hep-th/0508183](#).
- [49] S. Aoyama, “*Classical Exchange Algebra of the Superstring on  $S^5$  with the AdS-time*”, [arxiv:0709.3911](#).
- [50] B. Vicedo, “*Finite-g Strings*”, [arxiv:0810.3402](#).
- [51] A. A. Tseytlin, “*Light cone superstrings in AdS space*”, *Int. J. Mod. Phys. A* **16**, 900 (2001), [hep-th/0009226](#).

- [52] R. R. Metsaev, C. B. Thorn and A. A. Tseytlin, “*Light-cone superstring in AdS space-time*”, Nucl. Phys. B596, 151 (2001), [hep-th/0009171](#).
- [53] L. F. Alday, G. Arutyunov and A. A. Tseytlin, “*On integrability of classical superstrings in  $AdS_5 \times S^5$* ”, JHEP 0507, 002 (2005), [hep-th/0502240](#).
- [54] G. Arutyunov and S. Frolov, “*Integrable Hamiltonian for classical strings on  $AdS_5 \times S^5$* ”, JHEP 0502, 059 (2005), [hep-th/0411089](#).
- [55] G. Arutyunov and S. Frolov, “*Uniform light-cone gauge for strings in  $AdS_5 \times S^5$ : Solving  $su(1/1)$  sector*”, JHEP 0601, 055 (2006), [hep-th/0510208](#).
- [56] G. Arutyunov, S. Frolov and M. Zamaklar, “*Finite-size effects from giant magnons*”, Nucl. Phys. B778, 1 (2007), [hep-th/0606126](#).
- [57] S. Frolov, J. Plefka and M. Zamaklar, “*The  $AdS_5 \times S^5$  superstring in light-cone gauge and its Bethe equations*”, J. Phys. A39, 13037 (2006), [hep-th/0603008](#).
- [58] G. Arutyunov, S. Frolov, J. Plefka and M. Zamaklar, “*The off-shell symmetry algebra of the light-cone  $AdS_5 \times S^5$  superstring*”, J. Phys. A40, 3583 (2007), [hep-th/0609157](#).
- [59] T. McLoughlin, “*Review of AdS/CFT Integrability, Chapter II.2: Quantum Strings in  $AdS_5 \times S^5$* ”, [arxiv:1012.3987](#).
- [60] I. Adam, A. Dekel, L. Mazzucato and Y. Oz, “*Integrability of type II superstrings on Ramond-Ramond backgrounds in various dimensions*”, JHEP 0706, 085 (2007), [hep-th/0702083](#).
- [61] V. G. M. Puletti, “*On string integrability. A journey through the two- dimensional hidden symmetries in the AdS/CFT dualities*”, Adv. High Energy Phys. 2010, 471238 (2010), [arxiv:1006.3494](#).

# Review of AdS/CFT Integrability, Chapter II.4: The Spectral Curve

SAKURA SCHÄFER-NAMEKI

*Kavli Institute for Theoretical Physics, University of California,  
Santa Barbara, CA 93106, USA*

*and*

*Department of Mathematics, King's College,  
The Strand, London, WC2R 2LS, UK*

ss299 theory.caltech.edu

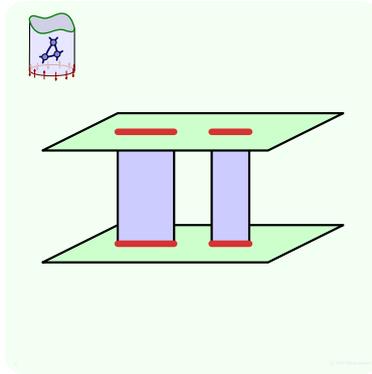

**Abstract:** We review the spectral curve for the classical string in  $AdS_5 \times S^5$ . Classical integrability of the  $AdS_5 \times S^5$  string implies the existence of a flat connection, whose monodromies generate an infinite set of conserved charges. The spectral curve is constructed out of the quasi-momenta, which are eigenvalues of the monodromy matrix, and each finite-gap classical solution can be characterized in terms of such a curve. This provides a concise and powerful description of the classical solution space. In addition, semi-classical quantization of the string can be performed in terms of the quasi-momenta. We review the general frame-work of the semi-classical quantization in this context and exemplify it with the circular string solution which is supported on  $\mathbb{R} \times S^3 \subset AdS_5 \times S^5$ .

# Contents

|                                                                          |            |
|--------------------------------------------------------------------------|------------|
| <b>Title</b>                                                             | <b>167</b> |
| <b>1 Introduction and Outlook</b>                                        | <b>168</b> |
| <b>2 Classical Integrability and Spectral Curve</b>                      | <b>170</b> |
| 2.1 Lax connection and monodromy matrix for $AdS_5 \times S^5$ . . . . . | 170        |
| 2.2 Spectral Curves: Generalities . . . . .                              | 171        |
| 2.3 Algebraic Curve for $AdS_5 \times S^5$ . . . . .                     | 171        |
| 2.4 Characterization of Solutions by Quasi-momenta . . . . .             | 172        |
| 2.5 Example: Circular String . . . . .                                   | 174        |
| <b>3 The Algebraic Curve of <math>\mathcal{N} = 4</math> SYM</b>         | <b>175</b> |
| 3.1 Bethe Ansatz Equations . . . . .                                     | 175        |
| 3.2 Thermodynamic Limit and Algebraic Curve . . . . .                    | 176        |
| <b>4 Semi-classical Quantization of the Spectral Curve</b>               | <b>177</b> |
| 4.1 Perturbing the Spectral Curve . . . . .                              | 178        |
| 4.2 General expression of one-loop energy shift . . . . .                | 180        |
| 4.2.1 Off-shell Fluctuation Frequencies . . . . .                        | 180        |
| 4.2.2 Frequencies from inversion symmetry . . . . .                      | 180        |
| 4.2.3 Basis of fluctuation energies . . . . .                            | 181        |
| 4.2.4 Final result . . . . .                                             | 182        |
| 4.2.5 Exampe: Circular String . . . . .                                  | 183        |
| <b>References</b>                                                        | <b>185</b> |

## 1 Introduction and Outlook

The integrability of the classical superstring in  $AdS_5 \times S^5$  follows from the existence of an infinite set of conserved charges [1]. In principle this allows for a complete classical solution of the theory, albeit in practice finding explicit classical solutions may be limited to simple field configurations. However, in the context of the spectral AdS/CFT correspondence, where the main objective is to map the spectrum of string energies in  $AdS_5 \times S^5$  to the spectrum of anomalous dimensions of four-dimensional  $\mathcal{N} = 4$  Super-Yang Mills (SYM), finding explicit solutions is not of primary interest. Indeed, it is much more important to find a way to directly characterize the spectrum. On the SYM theory side, this was achieved by noting that certain Bethe ansätze compute the spectrum of the dilatation operator. For the dual classical and semi-classical string theory in  $AdS_5 \times S^5$  this role is played by the spectral curve.

More specifically, using the classical Lax connection [1] and the monodromy matrix obtained by parallel transporting the connection around the worldsheet, it is possible to setup an elegant framework, which allows to characterize all finite gap solutions in terms of complex algebraic curves. In this geometric description, finite-gap translates into

finite genus of the curve. The conserved charges, such as the energy, can in this way be computed without having to solve the equations of motion. Furthermore, semi-classical quantization can be described in this framework, and allows for a concise description of the one-loop energy shifts presented in the part of the review [2].

The seminal paper [3] was the first to point out the importance of the spectral curves for the integrable systems that arise in the AdS/CFT correspondence. The algebraic curves for the classical string in the  $\mathbb{R} \times S^3$  subspace and the corresponding subsector of one-loop planar  $\mathcal{N} = 4$  SYM were shown to agree by some simple identifications. On the gauge theory side, the spectral curve emerges in the thermodynamic limit of the ferromagnetic Heisenberg-spin chain, that diagonalizes the one-loop dilatation operator in the  $\mathfrak{su}(2)$  subsector. Subsequently, this analysis was generalized to the  $\mathfrak{sl}(2)$  subsector or  $AdS_3 \times S^1$  string solutions [4], the  $\mathfrak{su}(4)$  subsector [5] and finally to the complete  $\mathfrak{psu}(2, 2|4)$  symmetric one-loop Heisenberg spin-chain [6, 7] and the  $AdS_5 \times S^5$  superstring [8].

Apart from providing a nice geometric description of classical solutions to the superstring, or in the dual theory, Bethe root configurations in the thermodynamic limit, the spectral curve is a very powerful tool to compute quantum corrections to classical string solutions. This was first advocated in the papers [9] and then applied to the classical string spectral curve in [10–15], in particular allowing a test of the asymptotics Bethe ansatz [16] and an explicit formula for the one-loop energy shift for a large class of solutions.

There are various interesting questions where spectral curves should either be useful or give a more elegant description, in the context of the AdS/CFT correspondence. Albeit, applications to higher order  $\alpha'$  corrections seem to be difficult to describe. Both conceptually and computationally, it would be very important to find a suitable all-loop quantization of the algebraic curve. To an extent, the Bethe ansatz, and more recently the characterization of the complete finite-size spectrum in terms of a Y-system (see the chapter [17] of this review) serve that purpose. However, a direct derivation of the Y-system from a quantum monodromy matrix is still unknown.

A brief comment on other formulations of the superstring in  $AdS_5 \times S^5$  is in place. In the pure spinor string, it is possible to find a flat connection that confirms the classical integrability and an associated algebraic curve [18]. It has been argued based on BRST-cohomology that the charges generated from the monodromy matrix of this flat connection exists to all orders in the  $\alpha'$  expansion [19], which has been confirmed to subleading order in [20].

The outline of this part of the review is as follows: we begin in section 2 by reviewing the Lax connection and monodromy matrix of the  $AdS_5 \times S^5$  string. We then define the algebraic curve in terms of the quasi-momenta (which are essentially the eigenvalues of the monodromy matrix). In section 2.4 we give a characterization of the quasi-momenta in terms of their asymptotics, poles structure etc. The example of the circular string in  $S^3$  is rephrased in terms of the algebraic curve in section 2.5. In section 3 we briefly discuss the algebraic curve of the dual  $\mathcal{N} = 4$  SYM theory at one-loop. In section 4 the general procedure for the semi-classical quantization is presented, and a general expression for the one-loop energy shift is derived from the algebraic curve. We furthermore show, that from this general analysis it is straightforward to compute the energy shift for the

circular string of section 2.5.

Relation to other parts of the review:

The relevant superstring action for the  $AdS_5 \times S^5$  string was described in [21]. The Lax connection and monodromy matrix were already introduced in [22]. Classical finite-gap solutions and their semi-classical quantization from the sigma-model point of view was discussed in [2]. The present part of the review gives an alternative point of view on the material in [2], which manifestly relies on the integrable structure of the theory.

## 2 Classical Integrability and Spectral Curve

### 2.1 Lax connection and monodromy matrix for $AdS_5 \times S^5$

Recall that a classical sigma-model is integrable if its equation of motion can be put into zero-curvature form, with a Lax connection  $L_\alpha(\sigma, \tau, z)$  depending on the spectral parameter  $z$ , where  $\alpha = \sigma, \tau$  denotes the world-sheet coordinates:

$$\partial_\alpha L_\beta - \partial_\beta L_\alpha - [L_\alpha, L_\beta] = 0. \quad (2.1)$$

From the Lax connection we can form the monodromy matrix, by parallel transport along the  $\sigma$  direction of the world-sheet, along some path  $\gamma$

$$\Omega(z) = \mathcal{P} \exp \left( \int_0^{2\pi} L_\sigma(\sigma, \tau, z) \right). \quad (2.2)$$

The classical superstring on  $AdS_5 \times S^5$  is described in terms of the Green-Schwarz action by Metsaev and Tseytlin (see also [21]) as a sigma-model into the supercoset space

$$\frac{PSU(2, 2|4)}{SO(4, 1) \times SO(5)} \supset AdS_5 \times S^5. \quad (2.3)$$

A useful description of the superstring action is in terms of the supercurrents for the map from the world-sheet into the supergroup  $g : \Sigma \rightarrow PSU(2, 2|4)$  which is gauged by the left-action

$$g \rightarrow gH, \quad H \in SO(4, 1) \times SO(5). \quad (2.4)$$

Define the currents as

$$J = -g^{-1}dg \in \mathfrak{psu}(2, 2|4), \quad (2.5)$$

which is flat  $dJ - J \wedge J = 0$  and transforms as  $J \rightarrow H^{-1}JH$ .

The superalgebra  $\mathfrak{psu}(2, 2|4)$  has a  $\mathbb{Z}_4$  grading

$$\mathfrak{psu}(2, 2|4) = \mathfrak{g}^{(0)} \oplus \mathfrak{g}^{(1)} \oplus \mathfrak{g}^{(2)} \oplus \mathfrak{g}^{(3)}, \quad (2.6)$$

and we shall decompose the currents accordingly as

$$J = J^{(0)} + J^{(1)} + J^{(2)} + J^{(3)}. \quad (2.7)$$

The action for the superstring in  $AdS_5 \times S^5$  then takes the form

$$S = \frac{\sqrt{\lambda}}{4\pi} \int \text{STr} (J^{(2)} \wedge *J^{(2)} - J^{(1)} \wedge J^{(3)} + \Lambda \wedge J^{(2)}), \quad (2.8)$$

where the Lagrange multiplier  $\Lambda$  in the last term ensures the super-tracelessness of  $J^{(2)}$ , as is required for  $PSU(2, 2|4)$ .

## 2.2 Spectral Curves: Generalities

Before discussing the curve for  $AdS_5 \times S^5$  we should first elaborate on spectral curves for classical integrable systems more generally, and point out important aspects. Consider a classical integrable system, described by a Lax connection  $L(x)$  and monodromy matrix  $\Omega(x)$ . The spectral curve is a complex curve defined defined by the eigenvalue equation for  $\Omega(x)$

$$\text{SDet}(y \text{Id} - \Omega(x)) = 0. \quad (2.9)$$

It is generically not an algebraic curve and may have essential singularities and infinite genus. A useful subclass of configurations, the so-called “finite gap” solutions, are such that the spectral curve is of finite genus, in this instance referred to then as “algebraic curve”. These curves may still have singular points, which however can be desingularized by standard algebraic geometric methods, e.g. by small resolutions, and we shall now distinguish these two birationally equivalent curves in the following. Naturally, the curve defined by (2.9) can be written in terms of the eigenvalues  $\lambda_i(x)$  of  $\Omega(x)$ . However, these will exhibit essential singularities in the spectral parameter, and it is more convenient to study the so-called quasi-momenta,  $p_i$ , where  $\lambda_i(x) = e^{ip_i(x)}$ . In what follows, we shall specify the curve entirely in terms of the properties of the quasi-momenta. For more details on e.g. the maps between the various descriptions, see [23].

## 2.3 Algebraic Curve for $AdS_5 \times S^5$

In [1] it was demonstrated that the classical equations of motion for this action are equivalent to the flatness of a one-parameter family of connections (Lax connection), thus establishing the classical integrability of the theory. The Lax connection depends on the spectral parameter, which will be denoted by  $x \in \mathbb{C}$  and is given as

$$L(x) = J^{(0)} + \frac{x^2 + 1}{x^2 - 1} J^{(2)} - \frac{2x}{x^2 - 1} (*J^{(2)} - \Lambda) + \sqrt{\frac{x+1}{x-1}} J^{(1)} + \sqrt{\frac{x-1}{x+1}} J^{(3)}. \quad (2.10)$$

For all  $x$  this is a flat connection  $dL(x) - L(x) \wedge L(x) = 0$ . As in (2.2) we can define the corresponding monodromy matrix by parallel transport along a closed path  $\gamma$ , encircling the compact world-sheet direction

$$\Omega(x) = \mathcal{P} \exp \left( \int_{\gamma} L(x) \right). \quad (2.11)$$

Super-tracelessness of  $L(x)$  implies unimodularity  $\text{SDet} \Omega(x) = 1$ . We can diagonalize  $\Omega(x)$  and denote the eigenvalues by  $e^{ip(x)}$ , where  $p(x)$  are the *quasi-momenta*. More specifically, we obtain

$$\Omega(x) \sim \text{Diag} \left( e^{i\hat{p}_1(x)}, e^{i\hat{p}_2(x)}, e^{i\hat{p}_3(x)}, e^{i\hat{p}_4(x)} | e^{i\tilde{p}_1(x)}, e^{i\tilde{p}_2(x)}, e^{i\tilde{p}_3(x)}, e^{i\tilde{p}_4(x)} \right), \quad (2.12)$$

where  $\hat{p}$  denotes the eigenvalues corresponding to  $AdS_5$  and  $\tilde{p}$  to  $S^5$ . From unimodularity of  $\Omega(x)$  it follows that<sup>1</sup>.

$$\sum_{i=1}^4 \hat{p}_i(x) - \tilde{p}_i(x) = 2\pi k, \quad k \in \mathbb{Z}. \quad (2.13)$$

By definition, the eigenvalues  $e^{ip(x)}$  are the zeroes of the characteristic polynomial of  $\Omega(x)$ , and as we shall define in the next section, the quasi-momenta  $p(x)$  define the spectral curve. More precisely, the equation (2.13) entails that  $p$  is a multivalued function of  $x$ , or alternatively, it is a single-valued function of a cover of the complex  $x$ -plane, which defines the spectral curve. In the next section we will give a characterization of the quasi-momenta and of the resulting curve. The degree of the characteristic polynomial specifies the number of sheets of the cover, which in the case of the  $AdS_5 \times S^5$  string is eight.

The key insight of [3] was that classical solutions can be equivalently characterized in terms of this algebraic curve, or alternatively, the quasi-momenta.

## 2.4 Characterization of Solutions by Quasi-momenta

In this section we will give a hands-on description of how classical solutions are encoded in terms of the quasi-momenta. This will be exemplified in the next subsection.

Classical solutions with global conserved charges  $(S_1, S_2, J_1, J_2, J_3)$  and energy  $E$  will be encoded in terms of quasi-momenta. Here  $(E, S_1, S_2)$  labels weights of the  $SO(4, 2)$  and  $(J_1, J_2, J_3)$  of the  $SO(6)$  isometry groups of  $AdS_5 \times S^5$ . Rather than solving an equivalent of the classical equations of motion, we lay out constraints, that will fully characterize the quasi-momenta in terms of asymptotics (which will be fixed by the global charges), behaviour at poles (which arise due to the pole in the Lax connection), symmetries (from the automorphism of the Lie-superalgebra  $\mathfrak{psu}(2, 2|4)$ ), and finally the so-called filling fractions. We will now discuss all these points in detail:

- The eight sheets are connected by cuts. Each of these connects two sheets, e.g.  $i$  and  $j$ , and will be denoted by  $\mathcal{C}^{ij}$ . The quasi-momenta will have discontinuities along these branch-cuts

$$p_i(x + i\epsilon) - p_j(x - i\epsilon) = 2\pi n_{ij}, \quad x \in \mathcal{C}_n^{ij} \quad (2.14)$$

for the combination of sheets

$$i \in \{\tilde{1}, \tilde{2}, \hat{2}, \hat{2}\}, \quad j \in \{\tilde{3}, \tilde{4}, \hat{3}, \hat{4}\}. \quad (2.15)$$

Note that these cuts arise from the diagonalization of  $\Omega$ , and are thus intrinsic to the spectral data. The classical curve only depends on the branch-points, however, in the quantum theory, the cuts become meaningful. This will become clear, in the

---

<sup>1</sup>The Lagrange multiplier  $\Lambda$ , cf. (2.8), would correspond to an unphysical, overall shift, and will be ignored from now on [8].

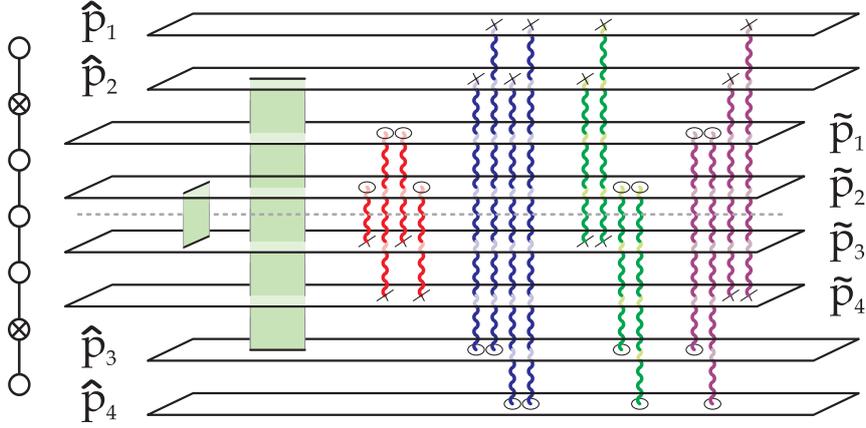

**Figure 1:** The spectral curve for classical superstrings on  $AdS_5 \times S^5$ . The sheets are connected by cuts (green), which characterize classical solutions. The left most cut alone, e.g. corresponds to a one-cut solution in the  $S^3 \times \mathbb{R}$  subspace, whereas the second cut is supported in  $AdS_3 \times S^1$ . The remaining part of the graph depicts all polarization of physical fluctuations. Red: bosonic fluctuations in the  $S^5$  direction. Blue: bosonic fluctuations in the  $AdS_5$  direction. Green and purple: fermionic fluctuations.

section on spin-chain spectral curves, where the cuts are shown to be condensates of Bethe roots.

More specifically, we can associate with cuts stretching between sheets of various types a "polarization". These correspond precisely to the sixteen physical polarization of the superstring in  $AdS_5 \times S^5$  and are identified in the algebraic curve in terms of cuts connecting the following pairs of sheets:

$$\begin{aligned}
 S^5 &: (\tilde{1}, \tilde{3}), (\tilde{1}, \tilde{4}), (\tilde{2}, \tilde{3}), (\tilde{2}, \tilde{4}) \\
 AdS_5 &: (\hat{1}, \hat{3}), (\hat{1}, \hat{4}), (\hat{2}, \hat{3}), (\hat{2}, \hat{4}) \\
 \text{Fermions} &: (\tilde{1}, \hat{3}), (\tilde{1}, \hat{4}), (\tilde{2}, \hat{3}), (\tilde{2}, \hat{4}) \\
 &: (\hat{1}, \tilde{3}), (\hat{1}, \tilde{4}), (\hat{2}, \tilde{3}), (\hat{2}, \tilde{4}).
 \end{aligned} \tag{2.16}$$

The situation is depicted in figure 1, where both macroscopic cuts, that correspond to a classical solution are shown, as well as all the physical excitations from (2.16).

- The quasi-momenta have poles in the  $x$ -plane at  $x = \pm 1$  – which can be readily seen from the Lax connection, which has poles at  $x = \pm 1$  – with residues that are correlated due to the Virasoro constraint

$$\{\hat{p}_1, \hat{p}_2, \hat{p}_3, \hat{p}_4 | \tilde{p}_1, \tilde{p}_2, \tilde{p}_3, \tilde{p}_4\} = \frac{\{\alpha_{\pm}, \alpha_{\pm}, \beta_{\pm}, \beta_{\pm} | \alpha_{\pm}, \alpha_{\pm}, \beta_{\pm}, \beta_{\pm}\}}{x \pm 1} + O(1). \tag{2.17}$$

- Global charges of the classical solution determine the asymptotics of the quasi-momenta for  $x \rightarrow \infty$ . This follows simply from the fact that in this limit, the Lax

connection  $L(x)$  reduces to the Noether current. It is useful to rescale the global  $\mathfrak{psu}(2, 2|4)$  charges by  $1/\sqrt{\lambda}$  and define  $\mathcal{Q} = Q/\sqrt{\lambda}$ . Then the asymptotics of the quasi-momenta are

$$\begin{pmatrix} \hat{p}_1 \\ \hat{p}_2 \\ \hat{p}_3 \\ \frac{\hat{p}_4}{\tilde{p}_1} \\ \tilde{p}_2 \\ \tilde{p}_3 \\ \tilde{p}_4 \end{pmatrix} = \frac{2\pi}{x} \begin{pmatrix} +\mathcal{E} - \mathcal{S}_1 + \mathcal{S}_2 \\ +\mathcal{E} + \mathcal{S}_1 - \mathcal{S}_2 \\ -\mathcal{E} - \mathcal{S}_1 - \mathcal{S}_2 \\ \frac{-\mathcal{E} + \mathcal{S}_1 + \mathcal{S}_2}{+\mathcal{J}_1 + \mathcal{J}_2 - \mathcal{J}_3} \\ +\mathcal{J}_1 - \mathcal{J}_2 + \mathcal{J}_3 \\ -\mathcal{J}_1 + \mathcal{J}_2 + \mathcal{J}_3 \\ -\mathcal{J}_1 - \mathcal{J}_2 - \mathcal{J}_3 \end{pmatrix} + O\left(\frac{1}{x^2}\right). \quad (2.18)$$

For the spectral problem it is in particular of interest to note that the energy  $\mathcal{E} = E/\sqrt{\lambda}$  can be extracted from these asymptotics

$$E = \frac{\sqrt{\lambda}}{4\pi} \lim_{x \rightarrow \infty} x(\hat{p}_1(x) + \hat{p}_2(x)). \quad (2.19)$$

We will see later, how this is done in practice.

- The quasi-momenta are furthermore restricted by an automorphism of the algebra  $\mathfrak{psu}(2, 2|4)$ , which imposes the following relations for the quasi-momenta

$$\begin{aligned} \tilde{p}_{1,2}(x) &= -\tilde{p}_{2,1}(1/x) - 2\pi m \\ \tilde{p}_{3,4}(x) &= -\tilde{p}_{4,3}(1/x) + 2\pi m \\ \hat{p}_{1,2,3,4}(x) &= -\hat{p}_{2,1,4,3}(1/x). \end{aligned} \quad (2.20)$$

This inversion symmetry allows us to determine the quasi-momenta inside the region  $|x| < 1$ .

- Finally, for each cut, we define the filling fraction

$$S_{ij} = \pm \frac{\sqrt{\lambda}}{8\pi^2 i} \oint_{\mathcal{C}_{ij}} \left(1 - \frac{1}{x^2}\right) p_i(x) dx. \quad (2.21)$$

These are the action angle variables for the theory [24]. These curve data specify precisely a macroscopic excitations of the string with  $S_{ij}$  quanta of mode number  $n$ .

## 2.5 Example: Circular String

To illustrate the spectral curve method, we now describe the circular string solution with support in  $S^3 \times \mathbb{R}$  [25, 10]. We restrict to the case, when all  $\mathfrak{su}(4)$  spins  $J_i$  are equal, and parametrize the solution by one spin  $J = \sqrt{\lambda}\mathcal{J}$ . We furthermore restrict to the case of a single cut. Since this solution has trivial support in the  $AdS_5$  direction, the corresponding quasi-momenta are determined simply in terms of trivial asymptotics at

infinity and the correct pole structure at  $\pm 1$ . The poles are correlated as required by (2.17) and determine the quasi-momenta as

$$\hat{p}_1 = \hat{p}_2 = -\hat{p}_3 = -\hat{p}_4 = \frac{2\pi\kappa x}{x^2 - 1}. \quad (2.22)$$

The quasi-momenta associated to the  $S^5$  directions will have cuts, and have to be consistent with the inversion symmetry. In [10] these were determined as

$$\begin{pmatrix} \tilde{p}_1 \\ \tilde{p}_2 \\ \tilde{p}_3 \\ \tilde{p}_4 \end{pmatrix} = \begin{pmatrix} \frac{x}{x^2-1}K(1/x) \\ \frac{x}{x^2-1}K(x) - m \\ \frac{x}{1-x^2}K(x) + m \\ \frac{x}{1-x^2}K(1/x) \end{pmatrix} \quad (2.23)$$

where  $K(x) = \sqrt{m^2x^2 + \mathcal{J}}$ . The cut extends along the imaginary axis and from the various constraints

$$\mathcal{E} = \kappa = \sqrt{\mathcal{J}^2 + m^2}. \quad (2.24)$$

It is in general not so easy to reverse-engineer the solution from the quasi-momenta. However, for many aspects, in particular computing the spectrum, it is a particularly powerful way to describe solutions.

### 3 The Algebraic Curve of $\mathcal{N} = 4$ SYM

So far our discussion of the spectral curve was focused on the classical  $AdS_5 \times S^5$  string. However, there is a spectral curve also for the dual  $\mathcal{N} = 4$  SYM theory. At one-loop it was shown that the eigenvalues of the dilatation operator can be equivalently computed from a ferro-magnetic Heisenberg spin chain with  $\mathfrak{psu}(2, 2|4)$  symmetry, which can be diagonalized using a Bethe ansatz [26–28]. In the thermodynamic limit Bethe roots condense and form cuts. The resulting structure is precisely an algebraic curve, which intriguingly resembles the curve for the superstring [4–8]. We will now briefly summarize the construction of the SYM curve. For details of the Bethe ansatz see the other contributions [29, 30].

#### 3.1 Bethe Ansatz Equations

The one-loop dilatation operator can be diagonalized by a Bethe ansatz for a super-spin chain with symmetry  $\mathfrak{psu}(2, 2|4)$  and  $\mathbf{4|4}$  representation at each spin-chain site [27]. The Bethe roots are  $u_i^{(k)}$ ,  $k = 1, \dots, r = 7$  and  $i = 1, \dots, J_k$ , where  $J_k$  denotes the excitation number for the  $k$ th root. Further, define  $J = \sum J_k$  as the total excitation number,  $L$  be the length of the spin chain, and denote the Cartan matrix<sup>2</sup> of  $\mathfrak{psu}(2, 2|4)$  by  $M$  and the weight of the representation by  $V$ . Then the Bethe Ansatz equations for the nearest neighbour spin-chain are

$$\left( \frac{u_i^{(k)} - \frac{i}{2}V_k}{u_i^{(k)} + \frac{i}{2}V_k} \right)^L = \prod_{l=1}^r \prod_{j=1}^{J_l} \frac{u_i^{(k)} - u_j^{(l)} - \frac{i}{2}M_{kl}}{u_i^{(k)} - u_j^{(l)} + \frac{i}{2}M_{kl}}. \quad (3.1)$$

<sup>2</sup>This is modulo signs that are discussed in [30].

Translational invariance along the spin chain implies further that

$$1 = \prod_{k=1}^r \prod_{i=1}^{J_k} \frac{u_i^{(k)} + \frac{i}{2}V_k}{u_i^{(k)} - \frac{i}{2}V_k} = e^{iP}, \quad (3.2)$$

where  $P$  is the total momentum. Solving these algebraic equations for the Bethe roots determines the values of the conserved charges, in particular the energy of the spin-chain Hamiltonian, and thus the Dilatation operator at one-loop

$$Q_n = \frac{i}{n-1} \sum_{l=1}^n \sum_{j=1}^{J_n} \left( \frac{1}{(u_j^{(l)} + \frac{i}{2}V_l)^{n-1}} - \frac{1}{(u_j^{(l)} - \frac{i}{2}V_l)^{n-1}} \right). \quad (3.3)$$

In particular, the energy  $E$  of the state is read off from  $Q_2$  as

$$E = cg^2 Q_2, \quad (3.4)$$

for some constant  $c$ .

### 3.2 Thermodynamic Limit and Algebraic Curve

As in the case of the superstring, the main interest is in determining the values of  $Q_r$ , and not in solving an auxiliary set of equations – the classical equations of motion in the case of the superstring, or the Bethe ansatz equations in the SYM theory. There is an analog of the spectral curve in the SYM that arises in the limit of large number of Bethe roots. More precisely, the algebraic curve of the above system arises in the thermodynamic limit  $L \rightarrow \infty$ . Taking the logarithm of (3.1) yields

$$L \log \left( \frac{u_i^{(k)} - \frac{i}{2}V_k}{u_i^{(k)} + \frac{i}{2}V_k} \right) = \sum_{l=1}^r \sum_{j=1, j \neq i}^{J_l} \log \left( \frac{u_i^{(k)} - u_j^{(l)} - \frac{i}{2}M_{kl}}{u_i^{(k)} - u_j^{(l)} + \frac{i}{2}M_{kl}} \right) - 2\pi i n_i^{(k)}, \quad (3.5)$$

where  $n_i^{(k)} \in \mathbb{Z}$  are the mode numbers, arising due to taking the logarithm. We now rescale the Bethe roots by  $1/L$  to  $x_i^{(k)} = u_i^{(k)}/L$  and take  $L, J \rightarrow \infty$ , while keeping  $n_i^{(k)}$  fixed

$$-\frac{V_k}{x_i^{(k)}} = \sum_{l=1}^r \frac{1}{J_l} \sum_{j=1, j \neq i}^{J_l} \frac{M_{kl}}{x_i^{(k)} - x_j^{(l)}} - 2\pi n_i^{(k)}. \quad (3.6)$$

It is useful to introduce a density of Bethe roots and a resolvent for their distribution

$$\begin{aligned} \rho_k(x) &= \sum_{j=1}^{J_k} \delta(x - x_j^{(k)}) \\ G_k(x) &= \frac{1}{J_k} \sum_{j=1}^{J_k} \frac{1}{x - x_j^{(k)}}. \end{aligned} \quad (3.7)$$

In the limit, the Bethe roots condense into cuts  $\mathcal{C}_k$ , and the Bethe equations take the continuum form

$$\oint_{\mathcal{C}} dv \frac{\rho_k(v) M_{kf(v)}}{v-u} = -\frac{V_k}{u} + 2\pi n_i^{(k)}, \quad u \in \mathcal{C}_i^{(k)}, \quad (3.8)$$

where  $\mathcal{C} = \cup_k \mathcal{C}_k$  and each of the curves  $\mathcal{C}_k$  associated to simple roots is on the other hand  $\mathcal{C}_k = \cup_j \mathcal{C}_j^{(k)}$ . This can equivalently be written in terms of the resolvent  $G_k(u)$  in the continuum limit

$$M_{kk} \mathcal{G}_k(u) + \sum_{l \neq k} M_{kl} G_l(u) = -\frac{V_k}{u} + 2\pi n_i^{(k)}, \quad u \in \mathcal{C}_i^{(k)}. \quad (3.9)$$

Slashes denote principal values. This equation can be put into a more familiar form by writing them in terms of the singular resolvents  $\tilde{G}$ , where the poles in  $1/u$  have been absorbed into the definition of the resolvent, and furthermore taking linear combinations (the quasi-momenta)  $p_i \sim \pm(\tilde{G}_{i-1} - \tilde{G}_i)$  (for details see [6]) so that we arrive at

$$M_{kk} \tilde{\mathcal{G}}_k + \sum_{j \neq k} M_{kj} \tilde{G}_j(u) = \not{p}_k(u) - \not{p}_{k+1}(u) = 2\pi n_j^{(k)}, \quad u \in \mathcal{C}_j^{(k)}. \quad (3.10)$$

This is precisely the type of equation that characterizes the spectral curve in the superstring case. Again, the asymptotics of the resolvent/quasi-momenta encode the relation to the global charges

$$G_k(u) = -\frac{1}{u} \int_{\mathcal{C}_k} dv \rho_k(v) + O\left(\frac{1}{u^2}\right) = -\frac{J_k}{u} + O\left(\frac{1}{u^2}\right). \quad (3.11)$$

A precise comparison of the SYM curve [6, 7] and string curve [8] can be found in [7]. The main features are, that the asymptotics and constraints on the quasi-momenta agree up to a redefinition of the spectral parameter and modulo pole structure, and thus, also the algebraic curves are in agreement.

## 4 Semi-classical Quantization of the Spectral Curve

Apart from giving a general, concise description of classical solutions, the spectral curve is a powerful means to compute quantum fluctuations. In part [2] of the review, the quantization around classical solutions with large spins, was already described from the point of view of the sigma-model: a classical field configuration is perturbed and the fluctuations quadratically quantized. The sum of the fluctuation frequencies make up the energy shift at one-loop (in  $\alpha'$ , or equivalently  $1/\sqrt{\lambda}$ ). We will not give an alternative approach, based on the algebraic curve, and present a general expression for the one-loop shift for general solutions.

## 4.1 Perturbing the Spectral Curve

A classical configuration can be viewed as a continuous collection of poles which have condensed into the cuts  $\mathcal{C}^{ij}$ . This intuition is particularly transparent in the comparison with the algebraic curve of the Yang-Mill theory, as discussed in section 3, where indeed, the cuts arose from condensation of Bethe roots. From this point of view, semi-classical quantization naturally corresponds to adding small fluctuations, or poles, to the classical configuration. Naturally, these fluctuations will have polarizations, labeled by  $(ij)$ , and amount to shifting the quasi-momenta

$$p_i(x) \rightarrow p_i(x) + \delta^{ij} p_i(x). \quad (4.1)$$

The energy shift is then obtained as the sum over all fluctuation frequencies. The shifts in the quasi-momenta  $\delta^{ij} p_i(x)$  are constrained by the asymptotics etc of the quasi-momenta, outlined in section 2.4:

- The perturbed quasi-momenta will have to continue to satisfy the relation (2.14). First we need to determine the position of the new pole  $x_n^{ij}$

$$p_i(x_n^{ij}) - p_j(x_n^{ij}) = 2\pi n_{ij}. \quad (4.2)$$

The physical poles correspond to solutions of this equation with  $|x_n^{ij}| > 1$ .<sup>3</sup> The fluctuation  $\delta_n^{ij} p_i$  will have to add a pole at  $x_n^{ij}$  with residue,  $\alpha(x_n^{ij})$ , such that it changes the filling fraction  $S_{ij}$  (2.21) by one, i.e.

$$\delta_n^{ij} p_i = \pm \frac{\alpha(x_n^{ij})}{x - x_n^{ij}}, \quad (4.3)$$

with

$$\alpha(x) = \frac{4\pi}{\sqrt{\lambda}} \frac{x^2}{x^2 - 1}. \quad (4.4)$$

The total shifted quasi-momentum is obtained by summing over all fluctuations with all relevant polarizations in (2.16)

$$\delta p_i \sim \sum_{(ij)} \delta^{(ij)} p_i(x) = \sum_{(ij)} \epsilon_i N_n^{ij} \frac{\alpha(x_n^{ij})}{x - x_n^{ij}}, \quad (4.5)$$

where  $N_n^{ij}$  label the excitations with mode number  $n$  and polarization  $(ij)$ , and the signs are

$$1 = \epsilon_1 = \epsilon_2 = -\epsilon_3 = -\epsilon_4 = -\epsilon_{\bar{1}} = -\epsilon_{\bar{2}} = \epsilon_{\bar{3}} = \epsilon_{\bar{4}}. \quad (4.6)$$

From (2.14) it furthermore follows that

$$\delta p_i(x + i\epsilon) - \delta p_j(x - i\epsilon) = 0, \quad x \in \mathcal{C}_n^{ij}. \quad (4.7)$$

---

<sup>3</sup> The inversion symmetry maps the region  $|x| > 1$  maps to  $|x| < 1$ , so that considering one of these regions (the physical region) is sufficient to describe the curve. Without loss of generality the region  $|x| > 1$  is chosen to be the physical region.

- As in the classical case, the poles at  $x = \pm 1$  have to be correlated due to the Virasoro constraint

$$\begin{aligned} & \{\delta\hat{p}_1, \delta\hat{p}_2, \delta\hat{p}_3, \delta\hat{p}_4 | \delta\tilde{p}_1, \delta\tilde{p}_2, \delta\tilde{p}_3, \delta\tilde{p}_4\} \\ &= \frac{\{\delta\alpha_{\pm}, \delta\alpha_{\pm}, \delta\beta_{\pm}, \delta\beta_{\pm} | \delta\alpha_{\pm}, \delta\alpha_{\pm}, \delta\beta_{\pm}, \delta\beta_{\pm}\}}{x \pm 1} + O(1). \end{aligned} \quad (4.8)$$

- The asymptotics at infinity (2.18) of the  $\delta^{ij}p_i$  can be easily read off

$$\begin{pmatrix} \delta\hat{p}_1 \\ \delta\hat{p}_2 \\ \delta\hat{p}_3 \\ \delta\hat{p}_4 \\ \delta\tilde{p}_1 \\ \delta\tilde{p}_2 \\ \delta\tilde{p}_3 \\ \delta\tilde{p}_4 \end{pmatrix} = \frac{4\pi}{x\sqrt{\lambda}} \begin{pmatrix} +\delta\Delta/2 & +N_{\hat{1}\hat{4}} + N_{\hat{1}\hat{3}} & +N_{\hat{1}\hat{3}} + N_{\hat{1}\hat{4}} \\ +\delta\Delta/2 & +N_{\hat{2}\hat{3}} + N_{\hat{2}\hat{4}} & +N_{\hat{2}\hat{4}} + N_{\hat{2}\hat{3}} \\ -\delta\Delta/2 & -N_{\hat{2}\hat{3}} - N_{\hat{1}\hat{3}} & -N_{\hat{1}\hat{3}} - N_{\hat{2}\hat{3}} \\ -\delta\Delta/2 & -N_{\hat{1}\hat{4}} - N_{\hat{2}\hat{4}} & -N_{\hat{2}\hat{4}} - N_{\hat{1}\hat{4}} \\ -N_{\hat{1}\hat{4}} - N_{\hat{1}\hat{3}} & -N_{\hat{1}\hat{3}} - N_{\hat{1}\hat{4}} & \\ -N_{\hat{2}\hat{3}} - N_{\hat{2}\hat{4}} & -N_{\hat{2}\hat{4}} - N_{\hat{2}\hat{3}} & \\ +N_{\hat{2}\hat{3}} + N_{\hat{1}\hat{3}} & +N_{\hat{1}\hat{3}} + N_{\hat{2}\hat{3}} & \\ +N_{\hat{1}\hat{4}} + N_{\hat{2}\hat{4}} & +N_{\hat{2}\hat{4}} + N_{\hat{1}\hat{4}} & \end{pmatrix} + O\left(\frac{1}{x^2}\right), \quad (4.9)$$

where  $\delta\Delta$  parametrizes the shift in the energy  $\mathcal{E}$ . From these asymptotics we can also determine the fluctuation frequencies  $\Omega_n^{ij}$  that are familiar from the direct semi-classical quantization by

$$\Omega_n^{ij} = -2\delta_{i,\hat{1}} + \frac{\sqrt{\lambda}}{2\pi} \lim_{x \rightarrow \infty} x \delta_n^{ij} p_i(x). \quad (4.10)$$

The energy shift then takes the usual form, as sum over fluctuation frequencies

$$\delta\Delta = \sum_{ij,n} N_{ij}^n \Omega_n^{ij}. \quad (4.11)$$

- Finally, the inversion symmetries extend trivially to the shifted quasi-momenta. These rather inconspicuous transformations, however, turn out to be rather powerful in determining the energy shifts. We shall see in section 4.2 how one can derive a closed expression for the one-loop energy shift, by invoking the asymptotics, pole structure, and inversion symmetry.

So far we covered all the constraints that follow from the asymptotics of the classical quasi-momenta. In addition, the fluctuations will backreact upon the classical cuts and close to the branch-points (or cut-endpoints) we impose for  $p_i \sim \sqrt{(x-a)}$  close to the branch-point  $x = a$

$$\delta p_i \sim \frac{d}{dx} p_i. \quad (4.12)$$

Solving these constraints in particular fixes  $\delta E$ , which is the desired one-loop energy shift.

## 4.2 General expression of one-loop energy shift

Rather than presenting examples of computations of energy shifts using the algebraic curve, which can e.g. be found for a plentitude of solutions (BMN, spinning string solutions, giant magnon) in the literature listed in the introduction, it is perhaps more interesting to point out that using general properties of the quasi-momenta constrain the energy shift such that closed expressions can be obtained for fairly general solutions (for any number of cuts) [12]. We then apply it to the circular string solution of section 2.5. This will be essentially a trivial step, once the general energy shift has been derived, and hopefully exemplifies that the algebraic curve approach is indeed very powerful for computing these effects.

### 4.2.1 Off-shell Fluctuation Frequencies

The key idea is to introduce the concept of an *off-shell fluctuation* (also sometimes referred to as quasi-energies), which means, defining the fluctuation as a function of the spectral parameter  $x$  and a variable  $y$ , such that the following holds

$$\delta_n^{ij} p_k(x) = \delta^{ij} p_k(x; y) \Big|_{y=x_n^{ij}} . \quad (4.13)$$

This off-shell fluctuation  $\delta^{ij} p_k(x; y)$  is fixed by the same asymptotics as the *on-shell* shift of quasimomenta  $\delta_n^{ij} p_k(x)$  except that the position of the pole is left unfixed. In the same way, we can then define off-shell fluctuation energies, by applying the same reasoning to (4.10)

$$\Omega_n^{ij} = \Omega^{ij}(y) \Big|_{y=x_n^{ij}} . \quad (4.14)$$

The off-shell frequency is related for the particular case of the  $SU(2)$  principal chiral model to the quasi-energy introduced in [14].

It is simple to reconstruct the off-shell frequency from a given on-shell one  $\Omega_n^{ij}$ . We know that the mode number  $n$  is determined precisely by the requirement  $p_i(x_n^{ij}) - p_j(x_n^{ij}) = 2\pi n$ , so that reverting this relation, treating  $n$  now as a function of  $p_l(y)$  we obtain

$$\Omega^{ij}(y) = \Omega_n^{ij} \Big|_{n \rightarrow \frac{p_i(y) - p_j(y)}{2\pi}} . \quad (4.15)$$

We will now explain how, using the inversion symmetry (2.20), we can relate many off-shell fluctuation energies. In this way we will find a powerful reduction algorithm for the computation of the fluctuation energies and thus the one loop energy shift

$$\delta \Delta^{1-loop} = \frac{1}{2} \sum_{ij,n} (-1)^{F_{ij}} \Omega_n^{ij} , \quad (4.16)$$

around a generic classical solution.

### 4.2.2 Frequencies from inversion symmetry

An important property of the quasi-momenta, which follows from the  $\mathbb{Z}_4$ -grading of the  $\mathfrak{psu}(2, 2|4)$  superalgebra, is the inversion symmetry (2.20) under  $x \rightarrow 1/x$ , which exchanges the quasi-momenta  $p_{\bar{1},\bar{4}} \leftrightarrow p_{\bar{2},\bar{3}}$  and likewise for the  $AdS$  hatted quasi-momenta.

Thereby, a pole connecting the sheets  $(\tilde{2}, \tilde{3})$  at position  $y$ , always comes with an image pole at position  $1/y$  connecting the sheets  $(\tilde{1}, \tilde{4})$ . We can obtain a physical frequency  $\Omega^{\hat{1}\hat{4}}(y)$ , by analytically continuing the off-shell frequency  $\Omega^{\tilde{2}\tilde{3}}(y)$ , inside the unit circle. This is because when we cross the unit-circle, the physical pole for  $(\tilde{2}\tilde{3})$  becomes unphysical, thereby rendering its image, which lies now outside the unit-circle, a physical pole for  $(\tilde{1}\tilde{4})$ . More precisely, it was shown in [12], that with this kind of reasoning we can compute the  $(\hat{1}\hat{4})$  fluctuation in terms of the  $(\hat{2}\hat{3})$  one. For the  $AdS$  fluctuations, indeed, the relation is

$$\Omega^{\hat{1}\hat{4}}(y) = -\Omega^{\hat{2}\hat{3}}(1/y) - 2. \quad (4.17)$$

This follows by invoking the general pole/asymptotics of the quasi-momenta and in the inversion symmetry.

Similarly we can proceed for the  $S^5$  frequencies and relate  $\Omega^{\tilde{2}\tilde{3}}(y)$  with  $\Omega^{\tilde{1}\tilde{4}}(y)$ . It is clear that  $\Omega^{\tilde{1}\tilde{4}}(y) = -\Omega^{\tilde{2}\tilde{3}}(1/y) + \text{constant}$ , which can be fixed from  $\Omega^{\tilde{1}\tilde{4}}(\infty) = 0$ . Thus, the relation is similar to (4.17), except that the constant term differs:

$$\Omega^{\tilde{1}\tilde{4}}(y) = -\Omega^{\tilde{2}\tilde{3}}(1/y) + \Omega^{\tilde{2}\tilde{3}}(0). \quad (4.18)$$

For the purpose of computing the one-loop shift these constants are irrelevant and can be shown to cancel in the sum over frequencies<sup>4</sup>.

So far we have obtained the frequencies (14) from (23). In the next subsection we will show how to derive all remaining frequencies. For a very large class of classical solutions we will be able to extract all fluctuation energies, including the fermionic ones, from the knowledge of a single  $S^3$  and a single  $AdS_3$  fluctuation energy.

### 4.2.3 Basis of fluctuation energies

For simplicity we consider only symmetric classical configurations that have pairwise symmetric quasi-momenta

$$p_{\hat{1},\hat{2},\hat{1},\hat{2}} = -p_{\hat{4},\hat{3},\hat{4},\hat{3}}, \quad (4.19)$$

This is in particular the case for all rank one solutions, i.e.  $\mathfrak{su}(2)$  and  $\mathfrak{sl}(2)$ , however, a generalization to other cases should not be difficult.

Consider e.g. the fermionic frequency  $\Omega^{\hat{2}\hat{3}}(y)$ . This energy can be thought of as a linear combination of the physical fluctuation  $\Omega^{\tilde{2}\tilde{3}}(y)$  and an unphysical fluctuation  $\Omega^{\hat{2}\hat{2}}(y)$  (it is unphysical, as it is not one of the fluctuations in (2.16)) momentum-carrying polarisations

$$\Omega^{\hat{2}\hat{3}}(y) = \Omega^{\tilde{2}\tilde{3}}(y) + \Omega^{\hat{2}\hat{2}}(y). \quad (4.20)$$

Since we are considering symmetric configurations, this unphysical fluctuation energy is identical to  $\Omega^{\hat{3}\hat{3}}(y)$ , i.e.

$$\Omega^{\hat{2}\hat{2}}(y) = \Omega^{\hat{3}\hat{3}}(y). \quad (4.21)$$

As in (4.20), these unphysical fluctuations can be linearly combined in terms of physical fluctuations

$$\Omega^{\hat{2}\hat{3}}(y) = \Omega^{\hat{2}\hat{2}}(y) + \Omega^{\tilde{2}\tilde{3}}(y) + \Omega^{\hat{3}\hat{3}}(y). \quad (4.22)$$

---

<sup>4</sup>Note, that in the case of  $AdS_4 \times \mathbb{CP}^3$  these constants play an important role.

Combining all these relations we obtain

$$\Omega^{\hat{2}\tilde{3}}(y) = \frac{1}{2} \left( \Omega^{\tilde{2}\tilde{3}}(y) + \Omega^{\hat{2}\hat{3}}(y) \right). \quad (4.23)$$

Proceeding in a similar fashion all frequencies can be obtained as linear combinations of  $\Omega^{\tilde{2}\tilde{3}}(y)$  and  $\Omega^{\hat{2}\hat{3}}(y)$ .

#### 4.2.4 Final result

The physical frequencies are labeled by the eight bosonic and eight fermionic polarizations (2.16), so we can label them by

$$\Omega^{ij}, \quad \text{where } i = (\hat{1}, \hat{2}, \tilde{1}, \tilde{2}) \quad j = (\hat{3}, \hat{4}, \tilde{3}, \tilde{4}). \quad (4.24)$$

To construct the complete set of off-shell frequencies for a symmetric solution (4.19) in terms of the two fundamental  $S^3$  and  $AdS_3$  ones  $\Omega^{\tilde{2}\tilde{3}}(y)$  and  $\Omega^{\hat{2}\hat{3}}(y)$  and their images under  $y \rightarrow 1/y$ , we first construct by inversion

$$\begin{aligned} \Omega^{\tilde{1}\tilde{4}}(y) &= -\Omega^{\tilde{2}\tilde{3}}(1/y) + \Omega^{\tilde{2}\tilde{3}}(0) \\ \Omega^{\hat{1}\hat{4}}(y) &= -\Omega^{\hat{2}\hat{3}}(1/y) - 2. \end{aligned} \quad (4.25)$$

The remaining frequencies are then obtained by linear combination of these four fluctuation frequencies. In this way we obtain the following concise form for all off-shell frequencies

$$\Omega^{ij}(y) = \frac{1}{2} \left( \Omega^{i'j'}(y) + \Omega^{j'j}(y) \right), \quad (4.26)$$

where

$$(\hat{1}, \hat{2}, \tilde{1}, \tilde{2}, \hat{3}, \hat{4}, \tilde{3}, \tilde{4})' = (\hat{4}, \hat{3}, \tilde{4}, \tilde{3}, \hat{2}, \hat{1}, \tilde{2}, \tilde{1}). \quad (4.27)$$

To finally, make the point, that these are indeed written in terms of the basis frequencies  $\Omega^{\tilde{2}\tilde{3}}(y)$  and  $\Omega^{\hat{2}\hat{3}}(y)$ , we present the complete set of frequencies

$$\begin{aligned} \Omega^{\tilde{1}\tilde{4}}(y) &= -\Omega^{\tilde{2}\tilde{3}}(1/y) + \Omega^{\tilde{2}\tilde{3}}(0) \\ \Omega^{\tilde{2}\tilde{4}}(y) &= \Omega^{\tilde{1}\tilde{3}}(y) = \frac{1}{2} \left( \Omega^{\tilde{2}\tilde{3}}(y) + \Omega^{\tilde{1}\tilde{4}}(y) \right) = \frac{1}{2} \left( \Omega^{\tilde{2}\tilde{3}}(y) - \Omega^{\tilde{2}\tilde{3}}(1/y) + \Omega^{\tilde{2}\tilde{3}}(0) \right) \\ \Omega^{\hat{1}\hat{4}}(y) &= -\Omega^{\hat{2}\hat{3}}(1/y) - 2 \\ \Omega^{\hat{2}\hat{4}}(y) &= \Omega^{\hat{1}\hat{3}}(y) = \frac{1}{2} \left( \Omega^{\hat{2}\hat{3}}(y) + \Omega^{\hat{1}\hat{4}}(y) \right) = \frac{1}{2} \left( \Omega^{\hat{2}\hat{3}}(y) - \Omega^{\hat{2}\hat{3}}(1/y) \right) - 1 \\ \Omega^{\tilde{2}\hat{4}}(y) &= \Omega^{\tilde{1}\hat{3}}(y) = \frac{1}{2} \left( \Omega^{\tilde{2}\tilde{3}}(y) + \Omega^{\tilde{1}\hat{4}}(y) \right) = \frac{1}{2} \left( \Omega^{\tilde{2}\tilde{3}}(y) - \Omega^{\tilde{2}\tilde{3}}(1/y) + \Omega^{\tilde{2}\tilde{3}}(0) \right) \\ \Omega^{\tilde{2}\hat{4}}(y) &= \Omega^{\tilde{1}\hat{3}}(y) = \frac{1}{2} \left( \Omega^{\tilde{2}\tilde{3}}(y) + \Omega^{\tilde{1}\hat{4}}(y) \right) = \frac{1}{2} \left( \Omega^{\tilde{2}\tilde{3}}(y) - \Omega^{\tilde{2}\tilde{3}}(1/y) \right) - 1 \\ \Omega^{\tilde{1}\hat{4}}(y) &= \Omega^{\hat{1}\tilde{4}}(y) = \frac{1}{2} \left( \Omega^{\tilde{1}\hat{4}}(y) + \Omega^{\hat{1}\tilde{4}}(y) \right) = \frac{1}{2} \left( -\Omega^{\tilde{2}\tilde{3}}(1/y) - \Omega^{\hat{2}\hat{3}}(1/y) + \Omega^{\tilde{2}\tilde{3}}(0) \right) - 1 \\ \Omega^{\hat{2}\tilde{3}}(y) &= \Omega^{\tilde{2}\hat{3}}(y) = \frac{1}{2} \left( \Omega^{\tilde{2}\tilde{3}}(y) + \Omega^{\hat{2}\hat{3}}(y) \right). \end{aligned} \quad (4.28)$$

In the complete one-loop energy shift (4.16) the constant terms in (4.28) will drop out and thus do not need to be computed. This is in particular clear, when performing the graded sum over  $\Omega^{ij}(x_n^{ij})$  with the explicit frequencies in (4.28).

For the general case of not symmetric solutions, we can repeat the above analysis, however the minimal set of required off-shell fluctuation frequencies will generically be larger than two.

#### 4.2.5 Exampe: Circular String

We shall now specialize to the case of  $\mathfrak{su}(2)$  solutions, and then apply these results to the circular string discussed in section 2.5. For  $\mathfrak{su}(2)$  solutions, only  $\tilde{p}_2$  (and  $\tilde{p}_3$ ) will be connected by square root cuts (outside the unit circle) and

$$\tilde{p}_2 = -\tilde{p}_3, \quad \tilde{p}_1 = -\tilde{p}_4 \quad \text{and} \quad \hat{p}_1 = \hat{p}_2 = -\hat{p}_3 = -\hat{p}_4, \quad (4.29)$$

so that we will generically have 6 different frequencies, namely:

1. One internal fluctuation corresponding to a pole shared by  $\tilde{p}_2$  and  $\tilde{p}_3$  which we denote by

$$\Omega_S(y) = \Omega^{\tilde{2}\tilde{3}}(y) \quad (4.30)$$

2. Another  $S^3$  fluctuation connecting  $\tilde{p}_1$  and  $\tilde{p}_4$

$$\Omega_{\bar{S}}(y) = \Omega^{\tilde{1}\tilde{4}}(y) \quad (4.31)$$

3. Two fluctuations which live in  $S^5$  but are orthogonal to the ones in  $S^3$ ,

$$\Omega_{S_\perp}(y) = \Omega^{\tilde{1}\tilde{3}}(y) = \Omega^{\tilde{1}\tilde{4}}(y) \quad (4.32)$$

4. Four  $AdS_5$  fluctuations

$$\Omega_A(y) = \Omega^{\hat{1}\hat{3}}(y) = \Omega^{\hat{1}\hat{4}}(y) = \Omega^{\hat{2}\hat{3}}(y) = \Omega^{\hat{2}\hat{4}}(y) \quad (4.33)$$

5. Four fermionic excitations which end on either  $p_2$  or  $p_3$  (which are the sheets where there are cuts outside the unit circle)

$$\Omega_F(y) = \Omega^{\hat{1}\hat{3}}(y) = \Omega^{\hat{2}\hat{3}}(y) = \Omega^{\hat{2}\hat{3}}(y) = \Omega^{\hat{2}\hat{4}}(y) \quad (4.34)$$

6. Four fermionic poles which end on either  $p_1$  or  $p_4$  (which are the sheets where there are cuts inside the unit circle)

$$\Omega_{\bar{F}}(y) = \Omega^{\hat{1}\hat{4}}(y) = \Omega^{\hat{2}\hat{4}}(y) = \Omega^{\hat{1}\hat{3}}(y) = \Omega^{\hat{1}\hat{4}}(y). \quad (4.35)$$

These expressions apply to any  $\mathfrak{su}(2)$  solution, where the cuts are symmetrically arranged (as commented earlier, the more general case follows trivially but may require more "basis fluctuations"). They also apply to higher cut solutions, as exemplified in [12].

We now apply these expressions to the circular string of section 2.5. Recall, the quasi-momenta for the circular string in  $S^3 \times \mathbb{R}$  depend on the following parameters of the solution, which are the spin  $J$  and winding  $m$  repackaged as  $\mathcal{J} = J/\sqrt{\lambda}$ ,  $\kappa = \sqrt{\mathcal{J}^2 + m^2}$ . The classical energy is

$$\mathcal{E} = \frac{E}{\sqrt{\lambda}} = \sqrt{\mathcal{J}^2 + m^2}. \quad (4.36)$$

The classical solution is determined by the quasi-momenta 2.23. The fluctuations were first determined from the sigma-model point of view in [31], the exact expansion in terms of  $1/\mathcal{J}$  as provided in [32] and a derivation of the fluctuation frequencies using the algebraic curve was done in [10]. Here we will argue that we only need two frequencies, namely the so-called "internal fluctuations" within the  $S^3$  and one  $AdS$ -fluctuation (which is trivial to obtain).

The off-shell frequencies in the  $(\tilde{2}, \tilde{3})$  and  $(\hat{2}, \hat{3})$  directions are

$$\begin{aligned} \Omega^{\tilde{2}\tilde{3}}(y) &= \frac{2m + n_{\tilde{2}\tilde{3}}}{\kappa y} = \frac{2m + \frac{p_{\tilde{2}} - p_{\tilde{3}}}{2\pi}}{\kappa y} = \frac{2\sqrt{m^2 y^2 + \mathcal{J}^2}}{(y^2 - 1)\sqrt{m^2 + \mathcal{J}^2}} \\ \Omega^{\hat{2}\hat{3}}(y) &= \frac{2}{y^2 - 1}. \end{aligned} \quad (4.37)$$

This will be our only input. We will now demonstrate that the remaining  $\mathfrak{su}(2)$  frequencies can be obtained with the methods outlined in the last section.

The AdS-frequencies are all given by generalizations of (4.17)

$$\begin{aligned} \Omega^{\hat{1}\hat{4}}(y) &= -\Omega^{\hat{2}\hat{3}}(1/y) - 2 = \frac{2}{y^2 - 1} \\ \Omega^{\hat{2}\hat{4}}(y) &= \frac{1}{2} \left( \Omega^{\hat{2}\hat{3}} + \Omega^{\hat{1}\hat{4}} \right) = \frac{2}{y^2 - 1} \\ \Omega^{\hat{1}\hat{3}}(y) &= -\Omega^{\hat{2}\hat{4}}(1/y) - 2 = \frac{2}{y^2 - 1}. \end{aligned} \quad (4.38)$$

Thus showing the expected agreement of all AdS fluctuation energies.

Let us move to the less trivial  $S^5$  fluctuations. From (4.28) we know

$$\Omega^{\bar{1}\bar{4}}(y) = -\Omega^{\tilde{2}\tilde{3}}(1/y) + \Omega^{\tilde{2}\tilde{3}}(0). \quad (4.39)$$

Applied to (4.37) we get

$$\Omega^{\bar{1}\bar{4}}(y) = \frac{2 \left( -\mathcal{J} y^2 + y \sqrt{m^2 + y^2 \mathcal{J}^2} + \mathcal{J} \right)}{(y^2 - 1) \sqrt{m^2 + \mathcal{J}^2}} = \frac{n_{\bar{1}\bar{4}} y - 2\mathcal{J}}{\kappa}, \quad (4.40)$$

by recalling that  $n_{\bar{1}\bar{4}} = \frac{p_{\bar{1}}(y) - p_{\bar{4}}}{2\pi}$ . The remaining frequencies are obtained by linear combination and inversion

$$\begin{aligned}\Omega^{\bar{1}\bar{3}}(y) &= \frac{1}{2} \left( \Omega^{\bar{1}\bar{4}} + \Omega^{\bar{2}\bar{3}} \right) = \frac{y(m + n_{\bar{1}\bar{3}}) - \mathcal{J} - \sqrt{m^2 y^2 + \mathcal{J}^2}}{\kappa} \\ \Omega^{\bar{2}\bar{4}}(y) &= -\Omega^{\bar{1}\bar{3}}(1/y) - 2 \frac{\partial \mathcal{E}}{\partial \mathcal{J}} = \frac{y(m + n_{\bar{2}\bar{4}}) - \mathcal{J} - \sqrt{m^2 y^2 + \mathcal{J}^2}}{\kappa}.\end{aligned}\tag{4.41}$$

Finally we compute the fermion frequencies, which are simply linear combinations

$$\begin{aligned}\Omega^{\hat{1}\bar{4}}(y) &= \Omega^{\bar{1}\bar{4}}(y) + \Omega^{\hat{1}\bar{1}}(y) = \frac{n_{\hat{1}\bar{4}} y - \mathcal{J} - \kappa}{\kappa} \\ \Omega^{\bar{1}\hat{3}}(y) &= \Omega^{\bar{1}\bar{4}}(y) + \Omega^{\bar{4}\hat{3}}(y) = \frac{n_{\hat{1}\bar{4}} y - \mathcal{J} - \kappa}{\kappa}.\end{aligned}\tag{4.42}$$

Similarly one can check the other fermionic frequencies

$$\Omega_{\hat{1}\bar{3}}(y) = \frac{1}{2} (\Omega_{\bar{2}\bar{3}}(y) + \Omega_{\hat{1}\bar{4}}(y)) = \frac{m + n_{\hat{1}\bar{3}}}{y\kappa}.\tag{4.43}$$

The complete 1-loop energy shift is obtained by

$$\delta E = \frac{1}{2} \sum_{n \in \mathbb{Z}} \sum_{(ij)} (-1)^{F_{ij}} \Omega^{ij}(x_n^{ij}),\tag{4.44}$$

where  $\Omega^{ij}(x_n^{ij})$  are of course now the on-shell frequencies, obtained by evaluating the off-shell frequencies at the position of the poles  $x_n^{ij}$ . Note that the sum can be converted into a contour integral in the  $n$ -plane (see e.g. [32, 10]), which simplifies the evaluation of the energy shift. This is in complete agreement with [31, 10].

## Acknowledgements

I thank Niklas Beisert for comments on the manuscript and for making this review happening. I would also like to thank the Caltech Theory Group for their generous hospitality.

## References

- [1] I. Bena, J. Polchinski and R. Roiban, “*Hidden symmetries of the  $AdS_5 \times S^5$  superstring*”, Phys. Rev. D69, 046002 (2004), [hep-th/0305116](#).
- [2] T. McLoughlin, “*Review of AdS/CFT Integrability, Chapter II.2: Quantum Strings in  $AdS_5 \times S^5$* ”, [arxiv:1012.3987](#).
- [3] V. A. Kazakov, A. Marshakov, J. A. Minahan and K. Zarembo, “*Classical / quantum integrability in AdS/CFT*”, JHEP 0405, 024 (2004), [hep-th/0402207](#).
- [4] V. A. Kazakov and K. Zarembo, “*Classical / quantum integrability in non-compact sector of AdS/CFT*”, JHEP 0410, 060 (2004), [hep-th/0410105](#).

- [5] N. Beisert, V. A. Kazakov and K. Sakai, “Algebraic curve for the  $SO(6)$  sector of  $AdS/CFT$ ”, *Commun. Math. Phys.* 263, 611 (2006), [hep-th/0410253](#).
- [6] S. Schäfer-Nameki, “The algebraic curve of 1-loop planar  $\mathcal{N} = 4$  SYM”, *Nucl. Phys.* B714, 3 (2005), [hep-th/0412254](#).
- [7] N. Beisert, V. A. Kazakov, K. Sakai and K. Zarembo, “Complete spectrum of long operators in  $\mathcal{N} = 4$  SYM at one loop”, *JHEP* 0507, 030 (2005), [hep-th/0503200](#).
- [8] N. Beisert, V. A. Kazakov, K. Sakai and K. Zarembo, “The algebraic curve of classical superstrings on  $AdS_5 \times S^5$ ”, *Commun. Math. Phys.* 263, 659 (2006), [hep-th/0502226](#).
- [9] N. Beisert, S. Frolov, M. Staudacher and A. A. Tseytlin, “Precision spectroscopy of  $AdS/CFT$ ”, *JHEP* 0310, 037 (2003), [hep-th/0308117](#). • N. Beisert, J. A. Minahan, M. Staudacher and K. Zarembo, “Stringing spins and spinning strings”, *JHEP* 0309, 010 (2003), [hep-th/0306139](#). • N. Beisert and L. Freyhult, “Fluctuations and energy shifts in the Bethe ansatz”, *Phys. Lett.* B622, 343 (2005), [hep-th/0506243](#).
- [10] N. Gromov and P. Vieira, “The  $AdS_5 \times S^5$  superstring quantum spectrum from the algebraic curve”, *Nucl. Phys.* B789, 175 (2008), [hep-th/0703191](#).
- [11] N. Gromov and P. Vieira, “Constructing the  $AdS/CFT$  dressing factor”, *Nucl. Phys.* B790, 72 (2008), [hep-th/0703266](#). • N. Gromov and P. Vieira, “Complete 1-loop test of  $AdS/CFT$ ”, *JHEP* 0804, 046 (2008), [arxiv:0709.3487](#).
- [12] N. Gromov, S. Schäfer-Nameki and P. Vieira, “Efficient precision quantization in  $AdS/CFT$ ”, *JHEP* 0812, 013 (2008), [arxiv:0807.4752](#).
- [13] N. Gromov, S. Schäfer-Nameki and P. Vieira, “Quantum Wrapped Giant Magnon”, *Phys. Rev.* D78, 026006 (2008), [arxiv:0801.3671](#). • N. Gromov, “Generalized Scaling Function at Strong Coupling”, *JHEP* 0811, 085 (2008), [arxiv:0805.4615](#).
- [14] B. Vicedo, “Semiclassical Quantisation of Finite-Gap Strings”, *JHEP* 0806, 086 (2008), [arxiv:0803.1605](#).
- [15] N. Gromov, “Integrability in  $AdS/CFT$  correspondence: Quasi-classical analysis”, *J. Phys.* A42, 254004 (2009).
- [16] N. Beisert, B. Eden and M. Staudacher, “Transcendentality and crossing”, *J. Stat. Mech.* 0701, P021 (2007), [hep-th/0610251](#). • N. Beisert, R. Hernandez and E. Lopez, “A crossing-symmetric phase for  $AdS_5 \times S^5$  strings”, *JHEP* 0611, 070 (2006), [hep-th/0609044](#).
- [17] Z. Bajnok, “Review of  $AdS/CFT$  Integrability, Chapter III.6: Thermodynamic Bethe Ansatz”, [arxiv:1012.3995](#).
- [18] B. C. Vallilo, “Flat currents in the classical  $AdS_5 \times S^5$  pure spinor superstring”, *JHEP* 0403, 037 (2004), [hep-th/0307018](#). • N. Berkovits, “BRST cohomology and nonlocal conserved charges”, *JHEP* 0502, 060 (2005), [hep-th/0409159](#).
- [19] N. Berkovits, “Quantum consistency of the superstring in  $AdS_5 \times S^5$  background”, *JHEP* 0503, 041 (2005), [hep-th/0411170](#).
- [20] A. Mikhailov and S. Schäfer-Nameki, “Perturbative study of the transfer matrix on the string worldsheet in  $AdS_5 \times S^5$ ”, [arxiv:0706.1525](#).
- [21] A. Tseytlin, “Review of  $AdS/CFT$  Integrability, Chapter II.1: Classical  $AdS_5 \times S^5$  string solutions”, [arxiv:1012.3986](#).

- [22] M. Magro, “*Review of AdS/CFT Integrability, Chapter II.3: Sigma Model, Gauge Fixing*”, arxiv:1012.3988.
- [23] O. Babelon, D. Bernard and M. Talon, “*Introduction to Classical Integrable Systems*”, Cambridge University Press (2003), Cambridge, UK. • B. Vicedo, “*Finite-g Strings*”, arxiv:0810.3402.
- [24] N. Dorey and B. Vicedo, “*A symplectic structure for string theory on integrable backgrounds*”, JHEP 0703, 045 (2007), hep-th/0606287.
- [25] S. Frolov and A. A. Tseytlin, “*Multi-spin string solutions in  $AdS_5 \times S^5$* ”, Nucl. Phys. B668, 77 (2003), hep-th/0304255.
- [26] J. A. Minahan and K. Zarembo, “*The Bethe-ansatz for  $\mathcal{N} = 4$  super Yang-Mills*”, JHEP 0303, 013 (2003), hep-th/0212208. • N. Beisert, “*The dilatation operator of  $\mathcal{N} = 4$  super Yang-Mills theory and integrability*”, Phys. Rept. 405, 1 (2005), hep-th/0407277. • N. Beisert, “*The complete one-loop dilatation operator of  $\mathcal{N} = 4$  super Yang-Mills theory*”, Nucl. Phys. B676, 3 (2004), hep-th/0307015.
- [27] N. Beisert and M. Staudacher, “*The  $\mathcal{N} = 4$  SYM Integrable Super Spin Chain*”, Nucl. Phys. B670, 439 (2003), hep-th/0307042.
- [28] N. Beisert and M. Staudacher, “*Long-range  $PSU(2,2/4)$  Bethe ansatz for gauge theory and strings*”, Nucl. Phys. B727, 1 (2005), hep-th/0504190.
- [29] J. A. Minahan, “*Review of AdS/CFT Integrability, Chapter I.1: Spin Chains in  $\mathcal{N} = 4$  SYM*”, arxiv:1012.3983.
- [30] M. Staudacher, “*Review of AdS/CFT Integrability, Chapter III.1: Bethe Ansatz and the R-Matrix Formalism*”, arxiv:1012.3990.
- [31] S. Frolov and A. A. Tseytlin, “*Quantizing three-spin string solution in  $AdS_5 \times S^5$* ”, JHEP 0307, 016 (2003), hep-th/0306130. • S. A. Frolov, I. Y. Park and A. A. Tseytlin, “*On one-loop correction to energy of spinning strings in  $S^5$* ”, Phys. Rev. D71, 026006 (2005), hep-th/0408187.
- [32] S. Schäfer-Nameki, “*Exact expressions for quantum corrections to spinning strings*”, Phys. Lett. B639, 571 (2006), hep-th/0602214.



# Review of AdS/CFT Integrability, Chapter III.1: Bethe Ansätze and the R-Matrix Formalism

MATTHIAS STAUDACHER

*Institut für Mathematik und Institut für Physik, Humboldt-Universität zu Berlin  
Johann von Neumann-Haus, Rudower Chaussee 25, 12489 Berlin, Germany  
and*

*Max-Planck-Institut für Gravitationsphysik, Albert-Einstein-Institut  
Am Mühlenberg 1, 14476 Potsdam, Germany*

matthias@aei.mpg.de

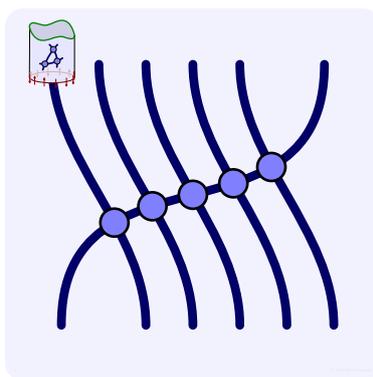

**Abstract:** The one-dimensional Heisenberg XXX spin chain appears in a special limit of the AdS/CFT integrable system. We review various ways of proving its integrability, and discuss the associated methods of solution. In particular, we outline the coordinate and the algebraic Bethe ansatz, giving reference to literature suitable for learning these techniques. Finally, we speculate which of the methods might lift to the exact solution of the AdS/CFT system, and sketch a promising method for constructing the Baxter Q-operator of the XXX chain. It allows to find the spectrum of the model using certain algebraic techniques, while entirely avoiding Bethe's ansatz.

# 1 Introduction

Quantum integrability was discovered in 1931 by young postdoc Hans Bethe during a research stay in Rome. Interestingly, this happened while the general formalism of non-relativistic quantum mechanics was still being developed. Bethe took a look at a one-dimensional model for a metal, the so-called Heisenberg spin chain, whose Hamiltonian reads

$$\mathbf{H} = 4 \sum_{l=1}^L \left( \frac{1}{4} - \vec{S}_l \cdot \vec{S}_{l+1} \right) \quad \text{with} \quad \vec{S}_l = \frac{1}{2} \vec{\sigma}_l, \quad (1.1)$$

where  $\vec{\sigma}_l$  are the three Pauli matrices, i.e. each  $\vec{S}_l$  is a separate spin- $\frac{1}{2}$  representation of  $\mathfrak{su}(2)$ . He managed to find, in a sense to be explained below, the *exact* solution of this model by making a clever educated guess for the “wave function”  $|\psi\rangle$  of the spin chain system, that is for the eigenstates of the spectral problem

$$\mathbf{H} \cdot |\psi\rangle = E |\psi\rangle, \quad (1.2)$$

where  $E$  are the energy eigenvalues. His original paper is still very readable today, and easily accessible either in its original German version [1], or its English translation, which is easily available on the internet. The last sentence of this masterpiece, just before the acknowledgements to Enrico Fermi and the sponsor of his visit, the Rockefeller foundation, indicates that Bethe was not quite aware how lucky he had been discovering quantum integrability in one dimension: He states with confidence that he was intending to generalize his method to the solution of higher dimensional lattices in a follow-up paper. We now know that this was bound to fail.

Bethe’s discovery of the exact solution of the spectral problem (1.2) is of timeless beauty and extraordinary importance for condensed matter theory and mathematical physics. The method continued and continues to be relevant to a multitude of widely differing problems. The maybe latest reincarnation occurred in the context of integrability in AdS/CFT, which is the focus of this review. As explained in the articles of part I of this volume, the Hamiltonian (1.1) appears in  $\mathcal{N} = 4$  Yang-Mills theory in the scalar field subsector, where  $\vec{S} \in \mathfrak{su}(2) \subset \mathfrak{su}(4) \subset \mathfrak{psu}(2, 2|4)$ , as the one-loop approximation of the conformal dilatation generator  $\mathbf{D} \in \mathfrak{su}(2, 2) \subset \mathfrak{psu}(2, 2|4)$

$$\mathbf{D} = L + g^2 \mathbf{H} + \mathcal{O}(g^4). \quad (1.3)$$

To understand the meaning of these Lie algebras in the AdS/CFT context, please refer to the article [2]. Here  $g^2$  is related to the ‘t Hooft coupling constant  $\lambda$  by  $g^2 = \frac{\lambda}{16\pi^2}$ . Note that we did not yet fully define the Hamiltonian in (1.1), since we so far did not state how to interpret  $\vec{S}_{L+1}$ . In other words, we need to specify the *boundary conditions* of the chain. For  $\mathcal{N} = 4$  we need periodic boundary conditions

$$\vec{S}_{L+1} := \vec{S}_1, \quad (1.4)$$

which is also the case originally solved by Bethe. It is relatively easy to see that  $\mathbf{H}$  in (1.1) with (1.4) is rotationally invariant, i.e. commutes with the total spin operator  $\vec{S}$ :

$$[\mathbf{H}, \vec{S}] = 0 \quad \text{where} \quad \vec{S} = \sum_{l=1}^L \vec{S}_l. \quad (1.5)$$

## 1.1 Understanding the problem

Let us first understand the problem, before contemplating its solution. The first thing to grasp is that the  $\mathbf{H}$  in (1.1) is just a simple matrix of size  $2^L \times 2^L$ . Why? Because the spin chain is composed of  $L$  Pauli spins, each of which can be pointing either up  $\uparrow$  or down  $\downarrow$ . Or, as in Bethe's paper,<sup>1</sup> left  $\leftarrow$  or right  $\rightarrow$ . In the AdS/CFT context, the two spin orientations correspond to two of the three possible complex scalar matter fields, say  $Z$  and  $X$ , and the spin chain is a local composite single trace operator. A basis for the configuration space of the chain is of size  $2^L$ . The eigenstates  $|\psi\rangle$  must then be the appropriate linear combinations of these  $2^L$  basis vectors. The proper mathematical concept to describe this set-up is the tensor product. Let us denote the state space of a single spin by  $\mathbb{C}^2$ . Then a basis of this two-dimensional complex (as quantum mechanics demands) vector space is

$$|\uparrow\rangle = Z = \begin{pmatrix} 1 \\ 0 \end{pmatrix}, \quad |\downarrow\rangle = X = \begin{pmatrix} 0 \\ 1 \end{pmatrix}. \quad (1.6)$$

The full state space of the quantum spin chain is then

$$\underbrace{\mathbb{C}^2 \otimes \mathbb{C}^2 \otimes \dots \otimes \mathbb{C}^2}_{L\text{-times}}, \quad (1.7)$$

and  $\vec{S}_l$  in (1.1) means that this operator acts like the  $2 \times 2$  identity matrix  $\mathbb{I}_2$  on each copy of  $\mathbb{C}^2$ , except for the  $l$ -th one, where it acts as  $\frac{1}{2}\vec{\sigma}$ . Tensor products can be confusing, and I recommend the very pedagogical introduction [3] for a transparent and detailed explanation in the same context. To illustrate, let us study the simplest non-trivial example of this, the  $L = 2$  spin chain. In the basis

$$\left\{ |\uparrow\rangle \otimes |\uparrow\rangle, |\uparrow\rangle \otimes |\downarrow\rangle, |\downarrow\rangle \otimes |\uparrow\rangle, |\downarrow\rangle \otimes |\downarrow\rangle \right\}, \quad (1.8)$$

or short

$$\left\{ |\uparrow\uparrow\rangle, |\uparrow\downarrow\rangle, |\downarrow\uparrow\rangle, |\downarrow\downarrow\rangle \right\}, \quad (1.9)$$

we have from (1.1) (the reader may have to play a bit with Pauli's matrices to see this)

$$\mathbf{H} = \begin{pmatrix} 0 & 0 & 0 & 0 \\ 0 & +4 & -4 & 0 \\ 0 & -4 & +4 & 0 \\ 0 & 0 & 0 & 0 \end{pmatrix}. \quad (1.10)$$

In this simplest case, it is of course trivial to find the eigensystem of the matrix  $\mathbf{H}$ . The (not fully normalized) eigenvectors are

$$\left\{ |\uparrow\uparrow\rangle, |\uparrow\downarrow\rangle + |\downarrow\uparrow\rangle, |\uparrow\downarrow\rangle - |\downarrow\uparrow\rangle, |\downarrow\downarrow\rangle \right\}, \quad (1.11)$$

---

<sup>1</sup>An interesting historical question is why Bethe's left-right convention lost out to up-down.

and in this basis the diagonalized Hamiltonian reads

$$\begin{pmatrix} 0 & 0 & 0 & 0 \\ 0 & 0 & 0 & 0 \\ 0 & 0 & 8 & 0 \\ 0 & 0 & 0 & 0 \end{pmatrix}. \quad (1.12)$$

It is useful to reorder the basis to

$$\left\{ |\uparrow\uparrow\rangle, |\uparrow\downarrow\rangle + |\downarrow\uparrow\rangle, |\downarrow\downarrow\rangle, |\uparrow\downarrow\rangle - |\downarrow\uparrow\rangle \right\}, \quad (1.13)$$

such that the diagonalized Hamiltonian becomes

$$\begin{pmatrix} 0 & 0 & 0 & 0 \\ 0 & 0 & 0 & 0 \\ 0 & 0 & 0 & 0 \\ 0 & 0 & 0 & 8 \end{pmatrix}. \quad (1.14)$$

In view of (1.2) we see that we have two distinct energy eigenvalues, namely a triply degenerate value  $E = 0$  with eigenstates  $|\uparrow\uparrow\rangle, |\uparrow\downarrow\rangle + |\downarrow\uparrow\rangle, |\downarrow\downarrow\rangle$ , as well as a non-degenerate eigenvalue  $E = 8$  with eigenstate  $|\uparrow\downarrow\rangle - |\downarrow\uparrow\rangle$ . Group theoretically this is to be expected, as we have a  $\mathfrak{su}(2)$  invariant chain, and in the tensor product of two (since  $L = 2$ ) spin- $\frac{1}{2}$  representations we have one spin-1 triplet and one spin-0 singlet:  $\frac{1}{2} \otimes \frac{1}{2} = 1 \oplus 0$ . Recall that the Hamiltonian  $\mathbf{H}$  commutes with the total spin, therefore, as remarked below (1.4), the energy eigenvalues in each  $\mathfrak{su}(2)$  multiplet must be identical.

Let us introduce two further important operators. The first is the *permutation operator*  $\mathbb{P}_{l,l+1}$ , which permutes the spins at site  $l$  and  $l + 1$ . In our simplest length  $L = 2$  example, we clearly have, in the basis (1.8),

$$\mathbb{P}_{1,2} = \begin{pmatrix} 1 & 0 & 0 & 0 \\ 0 & 0 & 1 & 0 \\ 0 & 1 & 0 & 0 \\ 0 & 0 & 0 & 1 \end{pmatrix}. \quad (1.15)$$

If we denote by  $\mathbb{I}_{1,2}$  the four-dimensional unit matrix, we can obviously rewrite the Hamiltonian matrix (1.10) as  $\mathbf{H} = 2(\mathbb{I}_{1,2} - \mathbb{P}_{1,2}) + 2(\mathbb{I}_{2,1} - \mathbb{P}_{2,1})$ . Since the interaction in the Hamiltonian (1.1) for general  $L$  is nearest-neighbor and pairwise, we can immediately lift this result from 2 to  $L$  and find that

$$\mathbf{H} = 2 \sum_{l=1}^L (\mathbb{I}_{l,l+1} - \mathbb{P}_{l,l+1}). \quad (1.16)$$

It is a nice exercise with tensor products to alternatively deduce this result directly from (1.1) by using the explicit form of the three Pauli matrices. For the solution of this exercise, see again [3].

The other important operator is the *shift operator*, defined as  $\mathbf{U} = \mathbb{P}_{1,2} \dots \mathbb{P}_{L-1,L}$ . We invite the reader to playfully act with it on a general spin chain state, and its name

will immediately become obvious. Strictly speaking, we could define a left-shift and a right-shift operator, but this distinction will not be needed here. Now it is easy to see that because of the periodic boundary conditions the shift operator commutes with the Hamiltonian:  $[\mathbf{U}, \mathbf{H}] = 0$ , as well as with the total spin operator:  $[\mathbf{U}, \vec{S}] = 0$ . Therefore each eigenstate  $|\psi\rangle$  in (1.2) must also carry a definite shift eigenvalue  $U$ :  $\mathbf{U} \cdot |\psi\rangle = U |\psi\rangle$ . Furthermore, it should be obvious that  $\mathbf{U}^L = \mathbb{I}$ , since shifting by  $L$  sites returns us to the original configuration. Therefore, all eigenvalues of  $\mathbf{U}$  have to satisfy  $U^L = 1$ , and we conclude that they are quantized in units of  $1/L$ , i.e.  $U = e^{2\pi i n/L}$  with the quantum number  $n = 0, 1, \dots, L-1$ . In our nearly trivial  $L = 2$  example we have  $\mathbf{U} = \mathbb{P}_{1,2}$  as in (1.15), while the shift operator becomes diagonal in the basis (1.13) where it reads

$$\begin{pmatrix} +1 & 0 & 0 & 0 \\ 0 & +1 & 0 & 0 \\ 0 & 0 & +1 & 0 \\ 0 & 0 & 0 & -1 \end{pmatrix}. \quad (1.17)$$

So the triplet state has shift quantum number  $n = 0$ , and the singlet  $n = 1$ . The shift operator plays a crucial role in the  $\mathcal{N} = 4$  gauge theory context: Because of gauge invariance, all planar local composite operators are single trace operators, see part I of this review. The trace leads to *two distinct* consequences for the spin chain interpretation of these operators. The *first* is that the “first” field (spin chain site  $l = 1$ ) inside the trace gets “hooked” to the “last field” (site  $l = L$ ). This is just the periodic boundary condition (1.4). The *second* is that because of trace cyclicity only the eigenvalue  $U = 1$  is allowed, all states with  $n \neq 0$  are actually identically zero in gauge theory. So if we interpret our  $L = 2$  eigenstates in (1.13) via (1.6) in gauge theory, we find, using trace cyclicity,

$$\left\{ \text{Tr } Z^2, \text{Tr } ZX + \text{Tr } XZ, \text{Tr } X^2, \text{Tr } ZX - \text{Tr } XZ \right\} = \left\{ \text{Tr } Z^2, 2 \text{Tr } ZX, \text{Tr } X^2, 0 \right\}. \quad (1.18)$$

So as concerns the triplet,  $\text{Tr } ZX$  and  $\text{Tr } X^2$  are some  $\mathfrak{su}(2)$  descendents of the BPS primary state  $\text{Tr } Z^2$  (cf. part Va) with anomalous dimension  $E = 0$ , but the  $L = 2$  Heisenberg chain’s singlet simply disappears (or maybe better to say: is projected out) in gauge theory! So the energy  $E = 8$  of this state has no interpretation in gauge theory, at least not in the maximally supersymmetric  $\mathcal{N} = 4$  case.

## 1.2 Understanding the solution of the problem

As we just explained, the Hamiltonian is just a  $2^L \times 2^L$  matrix, so what is the problem? The quick answer is that Hans Bethe neither had a laptop nor Mathematica or Maple (and even if he had had one, he would have quickly run into problems for sizes  $L \geq 10$  or so). So he derived the equations which carry his name. Let us assume that we have a number  $M$  of down spins in a chain of length  $L$ . While the Hamiltonian clearly shifts around those down spins, it certainly does not change  $M$ , as is easily seen from (1.16). In fact, this follows from (1.5), which says, in particular, that the z-component of spin commutes with  $\mathbf{H}$ :  $[\mathbf{H}, S^z] = 0$ : For all-spins-up, the eigenvalue of  $S^z$  is  $\frac{1}{2}L$ , and reversing

one spin lowers the total spin by 1 (*not* by  $\frac{1}{2}$ , think about it!) so we have for  $M$  reversed spins  $\frac{1}{2}(L - 2M)$ . Since  $S^z$  and  $L$  are conserved, so is  $M$ . So the  $2^L \times 2^L$  matrix is block-diagonal, with  $L + 1$  blocks ( $M = 0, \dots, L$ ), and the  $M$ -th block is a  $\binom{L}{M} \times \binom{L}{M}$  matrix. In order to nicely write down the eigenvalues of the  $M$ -th block, Bethe introduced  $M$  complex numbers  $u_1, \dots, u_M$ . To be honest, he probably first introduced them as real numbers, but quickly found that they needed to be complex for his solution to work in general. According to him, the eigenvalues of the Hamiltonian  $\mathbf{H}$  (the energies) are then given by

$$E = 2 \sum_{k=1}^M \frac{1}{u_k^2 + \frac{1}{4}}, \quad (1.19)$$

and the eigenvalues of the shift operator  $\mathbf{U}$  are

$$U = \prod_{k=1}^M \frac{u_k + \frac{i}{2}}{u_k - \frac{i}{2}}. \quad (1.20)$$

So, instead of diagonalizing a  $\binom{L}{M} \times \binom{L}{M}$  matrix, we have to find the correct sets of *distinct*<sup>2</sup> numbers  $\{u_1, \dots, u_M\}$ . They are fittingly called Bethe roots, and are determined from a system of  $M$  algebraic equations for these  $M$  variables:

$$\left( \frac{u_k + \frac{i}{2}}{u_k - \frac{i}{2}} \right)^L = \prod_{\substack{j=1 \\ j \neq k}}^M \frac{u_k - u_j + i}{u_k - u_j - i}, \quad \text{where } k = 1, \dots, M. \quad (1.21)$$

So what are the solutions of these equations? Let us see how to reproduce our results for the  $L = 2$  chain from the previous section. There are three blocks of  $\mathbf{H}$ , corresponding to  $M = 0, 1, 2$  (look back at (1.10)). The  $M = 0$  block is  $1 \times 1$ , there are no Bethe roots, so the sum in (1.19) is empty and indeed gives  $E = 0$ . The  $M = 1$  block is of size  $2 \times 2$ . Solving (1.21), there is just one *finite* Bethe root, which is easily found to be  $u_1 = 0$ . This indeed gives from (1.19)  $E=8$  and from (1.20)  $U=-1$ . The reader can also try the final  $1 \times 1$  block with  $M = 2$ , she will, however, not find finite, distinct Bethe roots  $u_1, u_2$  corresponding to the eigenvalue  $E = 0$  for  $|\downarrow\downarrow\rangle$ .

This was a partial success, we did encounter the correct energies  $E = 0, 8$  which appear at  $L = 2$ , but the multiplicities do not seem right. Why did we only find two instead of four states for the  $L = 2$  chain? The answer is pretty tricky, and best understood by manipulating the periodic boundary conditions (1.4), replacing them by

$$S_{L+1}^3 := S_1^3, \quad S_{L+1}^\pm := e^{\mp i\phi} S_1^\pm, \quad (1.22)$$

where  $\phi$  is some phase, and  $S_l^\pm = S_l^1 \pm i S_l^2$  are the usual  $\mathfrak{su}(2)$  ladder operators. For  $\phi = 0$  we obviously recover (1.4). Let us denote (1.1) with (1.22) instead of (1.4) by  $\mathbf{H}_\phi$ . The length  $L = 2$  Hamiltonian matrix (1.10) is then modified to

$$\mathbf{H}_\phi = \begin{pmatrix} 0 & 0 & 0 & 0 \\ 0 & +2 & -2 & 0 \\ 0 & -2 & +2 & 0 \\ 0 & 0 & 0 & 0 \end{pmatrix} + \begin{pmatrix} 0 & 0 & 0 & 0 \\ 0 & +2 & -2e^{+i\phi} & 0 \\ 0 & -2e^{-i\phi} & +2 & 0 \\ 0 & 0 & 0 & 0 \end{pmatrix}. \quad (1.23)$$

<sup>2</sup>We will see in the next subsection why the Bethe roots must all be distinct.

The basis (1.13) is modified to

$$\left\{ |\uparrow\uparrow\rangle, e^{-i\frac{\phi}{4}}|\uparrow\downarrow\rangle + e^{+i\frac{\phi}{4}}|\downarrow\uparrow\rangle, |\downarrow\downarrow\rangle, e^{-i\frac{\phi}{4}}|\uparrow\downarrow\rangle - e^{+i\frac{\phi}{4}}|\downarrow\uparrow\rangle \right\}, \quad (1.24)$$

and the diagonalized Hamiltonian now reads in generalization of (1.14)

$$\begin{pmatrix} 0 & 0 & 0 & 0 \\ 0 & 8 \sin^2 \frac{\phi}{4} & 0 & 0 \\ 0 & 0 & 0 & 0 \\ 0 & 0 & 0 & 8 \cos^2 \frac{\phi}{4} \end{pmatrix}. \quad (1.25)$$

We see that the degeneracy of the triplet is (partially) lifted, as the “middle state” now has energy  $E = 8 \sin^2 \frac{\phi}{4}$  while  $|\uparrow\uparrow\rangle$  and  $|\downarrow\downarrow\rangle$  remain at  $E = 0$ . Therefore the  $\mathfrak{su}(2)$  invariance must be broken<sup>3</sup> for generic  $\phi$ , and we indeed now have  $[\mathbf{H}_\phi, \vec{S}] \neq 0$ .

Bethe’s equations still work with minor modifications. In fact, they work much better! The formula for the energy (1.19) remains unaffected, but (1.21) are modified to

$$\left( \frac{u_k + \frac{i}{2}}{u_k - \frac{i}{2}} \right)^L e^{i\phi} = \prod_{\substack{j=1 \\ j \neq k}}^M \frac{u_k - u_j + i}{u_k - u_j - i}, \quad \text{where } k = 1, \dots, M. \quad (1.26)$$

Let’s redo the  $L = 2$  case (confer the discussion just after (1.21)). There are still three blocks of  $\mathbf{H}$ , corresponding to  $M = 0, 1, 2$ . As before, the  $M = 0$  block is  $1 \times 1$ , there are no Bethe roots, and thus  $E = 0$ . The  $M = 1$  block is of size  $2 \times 2$ . However, this time around, solving (1.26) yields not one but *two* finite Bethe roots. They are easily found to be  $u_1 = -\frac{1}{2} \cot \frac{\phi}{4}$  or  $u_1 = \frac{1}{2} \tan \frac{\phi}{4}$ . From (1.19) this gives, respectively,  $E = 8 \sin^2 \frac{\phi}{4}$  and  $E = 8 \cos^2 \frac{\phi}{4}$ . Finally, for the  $1 \times 1$  block with  $M = 2$  we find  $u_{1,2} = -\frac{1}{2} \cot \frac{\phi}{2} \pm \frac{i}{2 \sin \frac{\phi}{2}}$ . Curiously, this leads from (1.19) for arbitrary  $\phi$  to the correct energy  $E = 0$ , showing that “non-trivial” Bethe roots can lead to trivial energies. Let us now take the  $\phi \rightarrow 0$  limit. We observe that the Bethe root  $u_1 = -\frac{1}{2} \cot \frac{\phi}{4}$  of the  $M = 1$  descendent  $|\uparrow\downarrow\rangle + |\downarrow\uparrow\rangle$  of the  $\mathfrak{su}(2)$  highest weight state  $|\uparrow\uparrow\rangle$  *diverges*, while the root  $u_1 = \frac{1}{2} \tan \frac{\phi}{4}$  of the singlet state  $|\uparrow\downarrow\rangle - |\downarrow\uparrow\rangle$  returns to its correct untwisted value  $u_1 = 0$ . Likewise, the two Bethe roots  $u_{1,2} = -\frac{1}{2} \cot \frac{\phi}{2} \pm \frac{i}{2 \sin \frac{\phi}{2}}$  of the  $M = 2$  descendent  $|\downarrow\downarrow\rangle$  also both diverge. So this is the answer to our multiplicity puzzle: The untwisted Bethe ansatz equations (1.21) only yield the highest weight states,<sup>4</sup> i.e. those states which are annihilated by the total  $S^+$ . The descendents of these formally correspond to adding roots at infinity! Note that each “step” down the multiplet adds one further such infinite root.<sup>5</sup> This is an artifact resulting from the  $\mathfrak{su}(2)$  invariance, if we break the latter by the twist field  $\phi$ , the Bethe equations (1.26) yield the correct energies and all states are nicely described by finite sets of Bethe roots.

<sup>3</sup>We still have  $[\mathbf{H}_\phi, S^z] = 0$ , so the number  $M$  of down-spins is still conserved.

<sup>4</sup>It may be proved that the eigenvectors are highest weight states and, therefore, in (1.21)  $M$  should in fact be restricted to values  $M \leq L/2$ .

<sup>5</sup>Note that if we allow roots at infinity, we have to *ad hoc* relax the restriction that all Bethe roots must be distinct, since we need  $n$  of these for level  $n$  descendents.

The attentive reader might wonder what is the advantage of this reformulation of the matrix diagonalization problem (1.2) by (1.21) with (1.19) (or their generalization (1.26) with (1.19)). The system of equations (1.26) is increasingly tricky to solve, even using numerical techniques, as  $L$  and  $M$  increase from the nearly trivial values we just discussed. Nevertheless there are huge advantages as compared to brute force diagonalization of the  $2^L \times 2^L$  Hamiltonian. In fact, in order to understand this statement, we invite the serious reader to take Mathematica or Maple, and to find the complete spectrum of the  $L = 3, 4$  and maybe the  $L = 5$  chain by finding all states both from (1.26) as well as directly from (1.1) with “quasiperiodic” boundary conditions (1.22). For sure, as  $L$  increases, direct diagonalization becomes impossible even with the help of a powerful computer due to the exponential growth of the matrix size. With a “metal” where the number of atoms in a unit volume is  $L^3 \sim \mathcal{O}(10^{23})$  this is clearly impossible. On the other hand, the system of equations (1.26) actually tends to enormously simplify for large values of  $L$ : One often is able to derive neat linear integral equations in this thermodynamic limit. For one example within this review series, see [4]. Furthermore, the reformulation of a matrix diagonalization problem to an entirely algebraic problem is conceptually very interesting and useful. Note that this algebraic reformulation is quite different from working out the characteristic polynomial  $\det(E \mathbb{I} - \mathbf{H})$  of the Hamiltonian matrix, where we first need to compute a large  $2^L \times 2^L$  determinant. In fact, numerically it is a particularly bad idea to compute the characteristic polynomial and to then determine its eigenvalues, since it wildly oscillates. It is much better to obtain the spectrum by different methods starting from the original matrix.

### 1.3 Understanding how to arrive at the solution, and AdS/CFT

So far we just tried to explain how Bethe’s solution of the diagonalization problem of the Heisenberg chain works. But how to find his equations (1.19), (1.26)? If an exact solution to some problem exists, there are usually many ways to find it. The Heisenberg chain is no exception. In the following, we will briefly sketch a number of rather distinct, interesting solution methods, referring for details to various excellent pedagogical presentations already existing in the literature. We will begin in Section 2 with Bethe’s original method, nowadays called “coordinate Bethe ansatz”. We then move on to a more “modern” approach termed “algebraic Bethe ansatz” in Section 3. In Section 4 we briefly discuss how these techniques are related to AdS/CFT, as well as to other articles in this review collection. We end in Section 5 with yet another method of solution pioneered a long time ago by Baxter. Curiously, it was only very recently properly applied to the Heisenberg magnet. This author believes that this method will prove to be very powerful in the AdS/CFT context.

## 2 Coordinate Bethe Ansatz

“Ansatz” is a German word for a procedure which means “make a guess for the solution, and check whether it works”. Bethe made an inspired guess for the form of the eigenvector  $|\psi\rangle$  in (1.2), and then constructively proved that his ansatz is correct if certain conditions,

the *Bethe equations*, are satisfied. As a by-product, the energy eigenvalues  $E$  are found.

Clearly  $|\psi\rangle$  may be written for a given number of down spins  $M$  as

$$|\psi\rangle = \sum \psi(l_1, l_2, \dots, l_M) S_{l_1}^- S_{l_2}^- \dots S_{l_M}^- |0\rangle, \quad (2.1)$$

where  $|0\rangle = |\uparrow\uparrow\dots\uparrow\rangle$  is the *vacuum* state where all  $L$  spins point up, and the (local)  $\mathfrak{su}(2)$  lowering operator  $S_{l_k}^-$  flips the spin from up to down at position  $l_k$ . We can think of  $\psi(l_1, l_2, \dots, l_M)$  as the position space wave function of the spin chain, where the positions  $l_k$  live on the lattice numbered by  $1, \dots, L$ . The sum in (2.1) is over all orderings  $1 \leq l_1 < l_2 < \dots < l_M \leq L$ , in order to avoid overcounting of states. The  $<$  stems from the fact that we can only lower each up-spin once, since each lattice site is in a spin  $\frac{1}{2}$  representation. Of course we could have just as well started from  $|0\rangle = |\downarrow\downarrow\dots\downarrow\rangle$ , and then used  $S_{l_k}^+$  instead of  $S_{l_k}^-$  in (2.1). But as in real life, one is often forced to make a choice in order to proceed.

So far so good, there is nothing ‘‘Bethe’’ yet. Here is his ansatz:

$$\psi(l_1, l_2, \dots, l_M) = \sum_{\{\tau\}} A(\tau) e^{i p_{\tau_1} l_1 + \dots + i p_{\tau_M} l_M}. \quad (2.2)$$

The sum runs over the set  $\{\tau\}$  of all  $M!$  permutations  $\tau$  of the  $M$  downspins, so  $\tau = \{\tau_1, \dots, \tau_M\}$  is a permutation of the  $M$  labels  $1, \dots, M$ . This looks like a clever linear superposition of  $M!$  plane wave factors, where each factor is multiplied with an amplitude  $A(\tau)$  dependent on the permutations  $\tau$ , but *not* on the positions  $l_k$ . We can also think of this as a kind of generalization of a Fourier transform, which usually solves translation-invariant free systems. Our system is not free, however! This picture is nevertheless useful, as it leads to the interpretation of the set of numbers  $\{p_1, \dots, p_M\}$  as the lattice *momenta* of the  $M$  down-spins in the background of the up-spin vacuum.

The next step is to check whether (2.2) really works. So, with some effort we can just plug this expression into (2.1), and check that we indeed have a solution (i.e. (1.2) holds) iff the momenta  $\{p_1, \dots, p_M\}$  satisfy for  $k = 1, \dots, M$  the constraints<sup>6</sup>

$$e^{i p_k L} e^{i \phi} = \prod_{\substack{j=1 \\ j \neq k}}^M S(p_k, p_j), \quad \text{where} \quad S(p_k, p_j) = -\frac{e^{i p_k + i p_j} - 2 e^{i p_k} + 1}{e^{i p_k + i p_j} - 2 e^{i p_j} + 1}. \quad (2.3)$$

In this case, the amplitudes  $A(\tau)$  in the wavefunction (2.2) are given by

$$A(\tau) = \text{sign}(\tau) \prod_{j < k} (e^{i p_k + i p_j} - 2 e^{i p_k} + 1), \quad (2.4)$$

where  $\text{sign}(\tau)$  is the signature of the permutation, while the energy eigenvalue is found to be

$$E = \sum_{k=1}^M 8 \sin^2 \left( \frac{p_k}{2} \right). \quad (2.5)$$

---

<sup>6</sup>It is technically easier to first try  $M = 1$ , which trivially works, then  $M = 2$ , where we find the nice formula for  $S(p_k, p_j)$ , and then go about proving it for general  $M$ .

Comparing, respectively, the expressions (2.5) and (2.3) to (1.19) and (1.21), even the hasty reader will recognize their similarity. These are the same equations, once we identify for all  $k = 1, \dots, M$

$$e^{ip_k} = \frac{u_k + \frac{i}{2}}{u_k - \frac{i}{2}} \iff u_k = \frac{1}{2} \cot \frac{p_k}{2}. \quad (2.6)$$

So the Bethe roots are nothing but specially parametrized lattice momenta of the down-spin “particles”, which are often called magnons.

The nice thing about the Bethe ansatz is that it not only yields the spectrum, but also the (unnormalized) wavefunctions<sup>7</sup>. It is easy to see that the latter are fully antisymmetric under exchange of any two momenta and, therefore, any two Bethe roots. This is the reason, mentioned already just before (1.21), why we need to discard solutions with coinciding roots, as in this case the eigenvector  $|\psi\rangle$  of (1.2) vanishes, which is of course disallowed by elementary linear algebra.

We recommend to the serious student to study the solution we just sketched in much more detail. Apart from Bethe’s quite readable original paper [1], a very pedagogical presentation of the coordinate Bethe ansatz may be found in [6]. Chapter 2.1 of [7] might also be helpful. Insightful and artfully written accounts by B. Sutherland are found in [8] and in his book [9].

### 3 Algebraic Bethe Ansatz

The coordinate Bethe ansatz is very “physical”, and widely applicable. However, one disadvantage is that it totally obscures *why* a given Hamiltonian is integrable. A beautiful general method originates in work of Baxter in the early 1970’s, and was systematized and generalized in the late 1970’s and early 1980’s within the so-called “quantum inverse scattering program” initiated by the “Leningrad school” around Ludvig Faddeev. Its main advantage is that it allows to find in a rather systematic way very general classes of integrable models. For example, it is easy to generalize the XXX Heisenberg Hamiltonian to more general representations of the spin, and to symmetry algebras larger than  $\mathfrak{su}(2)$  while preserving integrability.

Let us panoramically sketch its key features. I certainly cannot improve the brilliant presentation in [10]. If this is too hard upon initial reading, please first study [3]. Some important complementary information is in [11], and the presentation in the very recent notes [12] as well as in the initial review part of the article [13] is also very nice.

The starting point is not the Hamiltonian (1.1), but instead a “generating object” [10], the quantum Lax operator. It admittedly falls a bit from the sky; I do not know a very good way to motivate it. Then again, one has to start with *something*<sup>8</sup> (mathematicians call it axiom). In the case of the Heisenberg chain, this operator reads

$$\mathcal{L}_{a,l}(u) = \begin{pmatrix} u + i S_l^3 & i S_l^- \\ i S_l^+ & u - i S_l^3 \end{pmatrix}_a, \quad (3.1)$$

<sup>7</sup>The normalization may also be found, see e.g. [5].

<sup>8</sup>In the case of AdS/CFT, we neither know the Hamiltonian nor a good “generating object”.

which is a  $2 \times 2$  matrix in some *auxiliary space*  $\mathbb{C}^2$  indexed by  $a$ . Each of its four matrix elements is also a  $2 \times 2$  matrix expressed through the site- $l$  spin operators we introduced in (1.1). It also depends on a complex variable  $u$ , the *spectral parameter*. A *monodromy matrix* is then built as<sup>9</sup>

$$\mathcal{M}_a(u) = \begin{pmatrix} e^{i\frac{\phi}{2}} & 0 \\ 0 & e^{-i\frac{\phi}{2}} \end{pmatrix} \cdot \mathcal{L}_{a,L}(u) \cdot \mathcal{L}_{a,L-1}(u) \cdot \dots \cdot \mathcal{L}_{a,2}(u) \cdot \mathcal{L}_{a,1}(u). \quad (3.2)$$

One next takes the trace  $\text{Tr}_a$  over the two-dimensional auxiliary space  $a$

$$\mathbf{T}(u) = \text{Tr}_a \mathcal{M}_a(u), \quad (3.3)$$

and thereby constructs the *transfer matrix* as an operator on the quantum space (1.7), which also depends on  $u$ . Now take *two* different auxiliary spaces  $a$  and  $b$  instead of just one, while concentrating on a single spin chain site  $l$ . Then you can (and should, at least once in your life) check by direct computation that the *Yang-Baxter equation* holds on the triple tensor product of our three spaces  $a, b, l$ :

$$\mathcal{R}_{a,b}(u - u') \mathcal{L}_{a,l}(u) \mathcal{L}_{b,l}(u') = \mathcal{L}_{b,l}(u') \mathcal{L}_{a,l}(u) \mathcal{R}_{a,b}(u - u'). \quad (3.4)$$

The *R-matrix*  $\mathcal{R}$  is essentially, in hopefully obvious notation, the same thing as (3.1)

$$\mathcal{R}_{a,b}(u) = \begin{pmatrix} u + \frac{i}{2} + i S_a^3 & i S_a^- \\ i S_a^+ & u + \frac{i}{2} - i S_a^3 \end{pmatrix}_b = \begin{pmatrix} u + \frac{i}{2} + i S_b^3 & i S_b^- \\ i S_b^+ & u + \frac{i}{2} - i S_b^3 \end{pmatrix}_a. \quad (3.5)$$

Using the notation of Section 1, there are further instructive ways to write this

$$\mathcal{R}_{a,b}(u) = \left( u + \frac{i}{2} \right) \mathbb{I}_{a,b} + 2i S_a^3 S_b^3 + i S_a^+ S_b^- + i S_a^- S_b^+ = u + \frac{i}{2} + 2i \vec{S}_a \cdot \vec{S}_b, \quad (3.6)$$

the most important form being

$$\mathcal{R}_{a,b}(u) = u \mathbb{I}_{a,b} + i \mathbb{P}_{a,b}. \quad (3.7)$$

You should also learn the beautiful graphical way (the so-called “train arguments”) to depict (3.4), which allows to trivialize many proofs (this is one of the things very nicely explained in the earlier Faddeev lecture [11]). For example this one,

$$\mathcal{R}_{a,b}(u - u') \mathcal{M}_a(u) \mathcal{M}_b(u') = \mathcal{M}_b(u') \mathcal{M}_a(u) \mathcal{R}_{a,b}(u - u'), \quad (3.8)$$

where  $\mathcal{M}_a$  and  $\mathcal{M}_b$  are built as in (3.2), using (3.1). Then taking the doubletrace  $\text{Tr}_a \text{Tr}_b$  of (3.8) over the two auxiliary spaces  $a, b$  the matrix  $\mathcal{R}_{a,b}$  drops out, and we derive

$$\mathbf{T}(u) \mathbf{T}(u') = \mathbf{T}(u') \mathbf{T}(u), \quad \text{i.e.} \quad [\mathbf{T}(u), \mathbf{T}(u')] = 0. \quad (3.9)$$

---

<sup>9</sup>Here  $\cdot$  denotes  $2 \times 2$  matrix multiplication in the auxiliary space. The entries of this  $2 \times 2$  matrix act on (1.7). Therefore, the whole thing  $\mathcal{M}_a(u)$  acts on the tensor product of (1.7) and the auxiliary space  $a$ .

The transfer matrix operator commutes with itself at different values of the spectral parameter  $u$ ! What does all this formal stuff have to do with our earlier discussion, though? The point is that we can expand  $\mathbf{T}(u)$ , or actually more naturally  $\log \mathbf{T}(u)$  in a power series around any point  $u_0$  of the complex  $u$ -plane, thereby generating a set of linearly independent operators acting on the quantum space (1.7). Because of (3.9), these all commute with each other (or, to express this in fancier way, “are in involution”). This formally proves the integrability, since for the special point  $u_0 = \frac{i}{2}$  one of these charges is our Hamiltonian (1.1) with boundary conditions (1.22):

$$\mathbf{H}_\phi = 2L - 2i \frac{d}{du} \log \mathbf{T}(u) \Big|_{u=\frac{i}{2}}. \quad (3.10)$$

What is more, we may also obtain the Bethe equations within this formalism, even though it is somewhat tedious (see chapter 4 of [10]). The basic idea is quite nice and simple though. First, introduce the following notation for the monodromy (3.2)

$$\mathcal{M}_a(u) = \begin{pmatrix} \mathbf{A}(u) & \mathbf{B}(u) \\ \mathbf{C}(u) & \mathbf{D}(u) \end{pmatrix}, \quad (3.11)$$

where again the  $2 \times 2$  matrix acts on the auxiliary space  $a$ , and in consequence  $\mathbf{A}, \mathbf{B}, \mathbf{C}, \mathbf{D}$  are operators on (1.7). If one is just interested in the transfer matrix operator  $\mathbf{T}(u) = \mathbf{A}(u) + \mathbf{D}(u)$  the off-diagonal components  $\mathbf{C}(u)$  and  $\mathbf{B}(u)$  may be ignored. They are, however, very useful for the construction of the Bethe states. Let us use the same “ferromagnetic” vacuum state  $|0\rangle = |\uparrow\uparrow \dots \uparrow\rangle$  as for the coordinate Bethe ansatz, c.f. (2.1). One immediately sees from (3.1),(3.2) that  $\mathbf{C}(u)|0\rangle = 0$ . Now the algebraic Bethe ansatz is simply the following “trial wavefunction”

$$|\psi\rangle = \mathbf{B}(u_1) \mathbf{B}(u_2) \dots \mathbf{B}(u_M) |0\rangle, \quad (3.12)$$

which should be compared to (2.1),(2.2). The next step is again to check whether (3.12) really works. What does that mean here? Well, this time around we have to check whether the state (3.12) is an eigenstate of the transfer matrix *operator*  $\mathbf{T}(u)$ , i.e. that

$$\mathbf{T}(u) \cdot |\psi\rangle = T(u) |\psi\rangle, \quad (3.13)$$

where  $T(u)$  is the eigenvalue. Then we will have killed (=diagonalized)  $L$  birds (=commuting charges) with one stone, and thus will have also solved (1.2) (because of (3.10)). The tedious part is to check this, where one proceeds again from (3.8). The upshot is that it actually does not work (i.e. the state  $|\psi\rangle$  in (3.12) is not an eigenstate) *unless* the set of variables  $\{u_1, u_2, \dots, u_M\}$  in (3.12) satisfies the Bethe equations (1.26). In fact, they follow from eliminating the “unwanted terms” ruining (3.13). Pretty cool!

## 4 Extensions, Deformations, and AdS/CFT

We just sketched two methods (coordinate and algebraic Bethe ansätze) for solving the one-dimensional Heisenberg magnet. The latter reemerged some 80 years after its

invention in the special  $\mathfrak{su}(2)$  sector of AdS/CFT, in the one-loop approximation (1.3) to the dilatation operator. We found it convenient to discuss a further parameter, the angle  $\phi$  breaking the periodic boundary conditions (1.22) while preserving integrability. In fact, this angle naturally appears in a certain deformation of the original AdS/CFT set-up, see the article [14] by Konstantinos Zoubos.

Let us now discuss what needs to be done to apply the Bethe ansatz to AdS/CFT. The first step is to extend the set of allowed operators from the  $\mathfrak{su}(2)$  sector of  $X$  and  $Z$  fields (1.6) to the full, infinite set of “spins”. The full one-loop magnet (see the article [15] by Joe Minahan) with  $\mathfrak{psu}(2, 2|4)$  symmetry is also integrable, the Hamiltonian is known, and the Bethe equations may be derived. The main new feature is, due to the extra components, the need for the so-called *nested* Bethe ansatz technique. E.g. in a magnet with  $\mathfrak{su}(n)$  symmetry, one needs  $n - 1$  Bethe ansatz *levels*. It again exists in both versions, coordinate and algebraic. The basic idea is beautiful, but the details are rather gruesome, and will not be discussed here. If you want to learn it, the best article I know is a lecture course by Sutherland [16]. It is worth going through for other reasons as well, as the article’s main topic is the Hubbard model, which is closely related to the AdS/CFT system. You can also try his original article [17], or again his book [9], and in particular Appendix B.8 therein.

The second, much more difficult step is to extend the integrable spin chain beyond the one-loop level, and to connect the resulting equations to the string sigma model, cf. the articles of section II of the review. Adding radiative corrections to the dilatation operator, see (1.3) leads to *long-range* spin chains, see the article [18] by Adam Rej, which do not fit well into the standard framework of the quantum inverse scattering method. No equally nice general theory along the lines of the nearest neighbor spin chains exists. It should be stressed that taking into account a *finite* number of corrections to (1.3) does not lead to an integrable model. Once we go beyond one-loop, we have to deal with the all-orders system, including the notoriously difficult wrapping interactions (see [19], and [20]). The biggest impediment to applying the two techniques we discussed to the full model is that we *neither* know the exact dilatation operator  $\mathbf{D}$  in order to apply the coordinate Bethe ansatz, *nor* the generating Lax operator of the model in order to apply the algebraic Bethe ansatz. It somewhat contradicts the idea of making an ansatz for  $|\psi\rangle$ , if we do not know which operator equation (see (1.2) or (3.13)) is to be diagonalized.

That does not mean, however, that progress is impossible, as this review collection proves. We only briefly hinted at the beautiful picture behind the coordinate Bethe ansatz, where the down-spins are considered nearly free particles in the background of the up-spin vacuum. When one takes any one particle (= “magnon”) with momentum  $p_k$  around the chain, the standard phase factor  $e^{ip_k L}$  of a would-be free particle gets modified by strictly pairwise (= “factorized scattering”) collisions with all other particles carrying momentum  $p_j$ , modifying the phase with a two-body *S-matrix* element  $S(p_k, p_j)$ : Please take another look at (2.3). This idea works beautifully for AdS/CFT, and leads to the so-called *asymptotic Bethe ansatz*, see [21] and [22], as well as the detailed discussion, using both coordinate and algebraic Bethe ansatz formalism, in the Ph.D. thesis of Marius de Leeuw [23]. The way it works is that one just assumes the existence of an integrable all-loop Hamiltonian, without actually knowing it exactly, and then fixes all S-matrix elements by symmetry, as well as further considerations such as crossing invariance. Note

that “ansatz” is now used in a slightly different fashion. The new principle is to “make a guess for the solution, check self-consistency, and hope that it works”. And it actually only works up to the already mentioned wrapping interactions. The way around it are the somewhat empirical and arcane techniques discussed in [20] by Romuald Janik, [24] by Volodya Kazakov and Kolja Gromov, and [25] by Zoltan Bajnok of this collection. However, according to the thinking of this author, the following question remains open: Is there a non-asymptotic, *exact* Bethe ansatz for the AdS/CFT system?

## 5 Bethe Equations without Ansatz: Q-Operator

Somewhat ironically, this author wrote this review on the Bethe ansatz technique even though he no longer believes it to be the most elegant and powerful technique to solve a given quantum integrable model. Certain deformations of the XXX chain exist, where the matrix elements of the Lax operator are replaced by functions periodic (trigonometric XXZ, or 6-vertex model) model or double-periodic (elliptic XYZ, or 8-vertex model) in the spectral parameter.<sup>10</sup> The XYZ model was first solved in the early seventies by Baxter, introducing what is now known as the *Q-operator*. The limit of his construction back to the XXX case is very subtle. In fact, the Q-operator for the XXX chain with compact spin- $\frac{1}{2}$  representation (our illustrative example of this review) was only explicitly constructed very recently in [26]. The main difference to Bethe’s approach is that *no ansatz* is required to solve the model. To conclude this review, let us, therefore, just hint at the elegant and powerful way to derive the Bethe equations (1.26) using this method. Here the starting point is neither the Hamiltonian (1.1) as for the coordinate Bethe ansatz nor the Lax operator (3.1) for the algebraic Bethe ansatz, but the “generating objects” are two novel Lax-operators

$$L_l^-(u) = \begin{pmatrix} 1 & \mathbf{a}_-^\dagger \\ i\mathbf{a}_- & u + i\mathbf{a}_-^\dagger\mathbf{a}_- \end{pmatrix}_l, \quad \text{and} \quad L_l^+(u) = \begin{pmatrix} u - i\mathbf{a}_+^\dagger\mathbf{a}_+ & i\mathbf{a}_+^\dagger \\ -\mathbf{a}_+ & 1 \end{pmatrix}_l, \quad (5.1)$$

which also satisfy various Yang-Baxter equations. Here the  $2 \times 2$  matrices act on some spin chain site  $l$ , the operators  $\mathbf{a}_\pm, \mathbf{a}_\pm^\dagger$  are however not  $\mathfrak{su}(2)$  Lie-algebra generators, but *harmonic oscillator* operators:  $[\mathbf{a}_\pm, \mathbf{a}_\pm^\dagger] = 1$ . Then one may prove that, in a sense made precise in [26], Faddeev’s Lax operator in (3.1) factors into  $\mathcal{L}_{a,l}(u) \sim L_l^-(u) L_l^+(u)$ , where now the auxiliary space  $a$  is given by the tensor product  $\mathcal{F}_+ \times \mathcal{F}_-$  of the two copies of harmonic oscillators. The Baxter operators are then constructed in analogy with the transfer matrix operator of (3.3),(3.2) as the trace in these Fock spaces of a monodromy matrix built from (5.1) (with  $h_\pm = \mathbf{a}_\pm^\dagger\mathbf{a}_\pm$ )

$$\mathbf{Q}_\pm(u) \equiv \frac{e^{\pm\frac{\phi}{2}u}}{\text{Tr}_{\mathcal{F}_\pm}(e^{-i\phi h_\pm})} \text{Tr}_{\mathcal{F}_\pm} (e^{-i\phi h_\pm} L_L^\pm(u) \otimes \cdots \otimes L_1^\pm(u)). \quad (5.2)$$

They are operators on the spin chain space (1.7). To illustrate it let us return once more to the discussion of the  $L = 2$  chain of Section 1. It is easy to use (5.2) with (5.1) to

---

<sup>10</sup>To date these do not seem to play a major role in some AdS/CFT setting.

compute, say,  $\mathbf{Q}_-(u; \phi)$  in the spin chain basis (1.8):

$$e^{-\frac{\phi}{2}u} \begin{pmatrix} 1 & 0 & 0 & 0 \\ 0 & u + \frac{1}{2} \cot \frac{\phi}{2} & \frac{1}{2} \cot \frac{\phi}{2} + \frac{i}{2} & 0 \\ 0 & \frac{1}{2} \cot \frac{\phi}{2} - \frac{i}{2} & u + \frac{1}{2} \cot \frac{\phi}{2} & 0 \\ 0 & 0 & 0 & u^2 + u \cot \frac{\phi}{2} + \frac{1}{2 \sin^2 \frac{\phi}{2}} - \frac{1}{4} \end{pmatrix} \quad (5.3)$$

Diagonalizing this operator by going to the basis (1.24), we find

$$e^{-\frac{\phi}{2}u} \begin{pmatrix} 1 & 0 & 0 & 0 \\ 0 & u + \frac{1}{2} \cot \frac{\phi}{4} & 0 & 0 \\ 0 & 0 & u^2 + u \cot \frac{\phi}{2} + \frac{1}{2 \sin^2 \frac{\phi}{2}} - \frac{1}{4} & 0 \\ 0 & 0 & 0 & u - \frac{1}{2} \tan \frac{\phi}{4} \end{pmatrix} \quad (5.4)$$

We see that the eigenvalues  $Q_-(u)$  of the  $\mathbf{Q}_-$ -operators take the form “exponential times polynomial”, and the same is true for  $Q_+(u)$ :

$$Q_-(u) = e^{-\frac{\phi}{2}u} \prod_{k=1}^M (u - u_k), \quad Q_+(u) = e^{+\frac{\phi}{2}u} \prod_{k=1}^{L-M} (u - u_k). \quad (5.5)$$

The roots of the polynomials are precisely the ones we found in the course of the discussion of the  $L = 2$  solutions of the twisted Bethe equations! See (1.26) and the discussion just below. And indeed, using the two  $\mathbf{Q}$ -operators it is easy to solve the XXX model in an entirely algebraic fashion, as one may derive the following *operator equations*:

$$2i \sin \frac{\phi}{2} u^L = \mathbf{Q}_+(u + \frac{i}{2}) \mathbf{Q}_-(u - \frac{i}{2}) - \mathbf{Q}_+(u - \frac{i}{2}) \mathbf{Q}_-(u + \frac{i}{2}), \quad (5.6)$$

$$2i \sin \frac{\phi}{2} \mathbf{T}(u) = \mathbf{Q}_+(u + i) \mathbf{Q}_-(u - i) - \mathbf{Q}_+(u - i) \mathbf{Q}_-(u + i). \quad (5.7)$$

It is straightforward to prove (no ansatz here!) that the eigenvalues of the  $\mathbf{Q}_\pm$ -operators must always be of the form (5.5). Then it is an easy exercise to derive the Bethe equations (1.26) from (5.6). Furthermore, the transfer matrix and, therefore, through (3.10) the Hamiltonian of the Heisenberg chain, follow from (5.7). Nice, no?

This entirely algebraic methodology generalizes to spin chains with  $\mathfrak{su}(n)$  [27] as well as  $\mathfrak{su}(n|m)$  symmetry [28], thereby bypassing the rather tedious nested Bethe ansatz technique. It will be interesting to see how to describe the eigenstates in this language. In any case I hope the method will also lift to the full AdS/CFT system.

## References

- [1] H. Bethe, “Zur Theorie der Metalle. I. Eigenwerte und Eigenfunktionen der linearen Atomkette,” *Z. Phys.* **71** (1931) 205–226.
- [2] N. Beisert, “Review of AdS/CFT Integrability, Chapter VI.1: Superconformal Algebra,” arXiv:1012.4004 [hep-th].

- [3] R. I. Nepomechie, “*A Spin Chain Primer*,” Int. J. Mod. Phys. **B13** (1999) 2973–2986, [arXiv:hep-th/9810032](#).
- [4] S. Schäfer-Nameki, “*Review of AdS/CFT Integrability, Chapter II.4: The Spectral Curve*,” [arXiv:1012.3989 \[hep-th\]](#).
- [5] V. Korepin, N. Bogoliubov, and A. Izergin, *Quantum Inverse Scattering Method and Correlation Functions*. Cambridge University Press, 1993.
- [6] M. Karbach and G. Müller, “*Introduction to the Bethe ansatz I*,” Computers in Physics **11** (1997) 36, [arXiv:cond-mat/9809162](#).
- [7] M. Staudacher, “*The factorized S-matrix of CFT/AdS*,” JHEP **05** (2005) 054, [arXiv:hep-th/0412188](#).
- [8] B. Sutherland, “*A brief history of the quantum soliton with new results on the quantization of the Toda lattice*,” Rocky Mtn. J. of Math. **8** (1978) 431.
- [9] B. Sutherland, *Beautiful Models: 70 Years of Exactly Solved Quantum Many-Body Problems*. World Scientific, 2004.
- [10] L. D. Faddeev, “*How Algebraic Bethe Ansatz works for integrable model*,” [arXiv:hep-th/9605187](#).
- [11] L. D. Faddeev, “*Algebraic aspects of Bethe Ansatz*,” Int. J. Mod. Phys. **A10** (1995) 1845–1878, [arXiv:hep-th/9404013](#).
- [12] A. Doikou, S. Evangelisti, G. Feverati, and N. Karaiskos, “*Introduction to Quantum Integrability*,” [arXiv:0912.3350 \[math-ph\]](#).
- [13] J. Escobedo, N. Gromov, A. Sever, and P. Vieira, “*Tailoring Three-Point Functions and Integrability*,” [arXiv:1012.2475 \[hep-th\]](#).
- [14] K. Zoubos, “*Review of AdS/CFT Integrability, Chapter IV.2: Deformations, Orbifolds and Open Boundaries*,” [arXiv:1012.3998 \[hep-th\]](#).
- [15] J. A. Minahan, “*Review of AdS/CFT Integrability, Chapter I.1: Spin Chains in  $\mathcal{N} = 4$  SYM*,” [arXiv:1012.3983 \[hep-th\]](#).
- [16] B. Sutherland, *Exactly Solvable Problems in Condensed Matter and Relativistic Field Theory*. Lecture Notes in Physics 242. Springer, Berlin, Germany, 1985.
- [17] B. Sutherland, “*A General Model for Multicomponent Quantum Systems*,” Phys. Rev. **B12** (1975) 3795–3805.
- [18] A. Rej, “*Review of AdS/CFT Integrability, Chapter I.3: Long-range spin chains*,” [arXiv:1012.3985 \[hep-th\]](#).
- [19] C. Sieg, “*Review of AdS/CFT Integrability, Chapter I.2: The spectrum from perturbative gauge theory*,” [arXiv:1012.3984 \[hep-th\]](#).

- [20] R. Janik, “*Review of AdS/CFT Integrability, Chapter III.5: Lüscher corrections,*” arXiv:1012.3994 [hep-th].
- [21] C. Ahn and R. I. Nepomechie, “*Review of AdS/CFT Integrability, Chapter III.2: Exact world-sheet S-matrix,*” arXiv:1012.3991 [hep-th].
- [22] P. Vieira and D. Volin, “*Review of AdS/CFT Integrability, Chapter III.3: The dressing factor,*” arXiv:1012.3992 [hep-th].
- [23] M. de Leeuw, “*The S-matrix of the  $AdS_5 \times S^5$  superstring,*” arXiv:1007.4931 [hep-th].
- [24] V. Kazakov and N. Gromov, “*Review of AdS/CFT Integrability, Chapter III.7: Hirota Dynamics for Quantum Integrability,*” arXiv:1012.3996 [hep-th].
- [25] Z. Bajnok, “*Review of AdS/CFT Integrability, Chapter III.6: Thermodynamic Bethe Ansatz,*” arXiv:1012.3995 [hep-th].
- [26] V. V. Bazhanov, T. Lukowski, C. Meneghelli, and M. Staudacher, “*A Shortcut to the Q-Operator,*” J. Stat. Mech. **1011** (2010) P11002, arXiv:1005.3261 [hep-th].
- [27] V. V. Bazhanov, R. Frassek, T. Lukowski, C. Meneghelli, and M. Staudacher, “*Baxter Q-Operators and Representations of Yangians,*” arXiv:1010.3699 [math-ph].
- [28] R. Frassek, T. Lukowski, C. Meneghelli, and M. Staudacher, “*Oscillator Construction of  $su(n-m)$  Q-Operators,*” arXiv:1012.6021 [math-ph].



# Review of AdS/CFT Integrability, Chapter III.2: Exact world-sheet $S$ -matrix

CHANGRIM AHN <sup>1</sup> AND RAFAEL I. NEPOMECHIE <sup>2</sup>

<sup>1</sup> *Department of Physics and Institute for the Early Universe, Ewha Womans University, Seoul 120-750, South Korea*

<sup>2</sup> *Physics Department, P.O. Box 248046, University of Miami, Coral Gables, FL 33124 USA*

ahn@ewha.ac.kr; nepomechie@physics.miami.edu

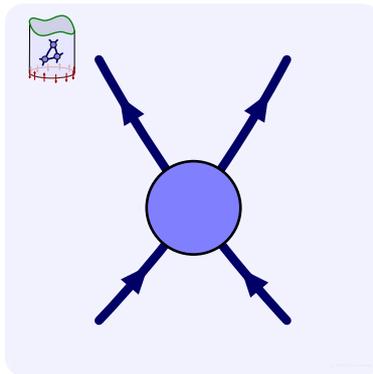

**Abstract:** We review the derivation of the  $S$ -matrix for planar  $\mathcal{N} = 4$  supersymmetric Yang-Mills theory and type IIB superstring theory on an  $AdS_5 \times S^5$  background. After deriving the  $S$ -matrix for the  $su(2)$  and  $su(3)$  sectors at the one-loop level based on coordinate Bethe ansatz, we show how  $su(2|2)$  symmetry leads to the exact asymptotic  $S$ -matrix up to an overall scalar function. We then briefly review the spectrum of bound states by relating these states to simple poles of the  $S$ -matrix. Finally, we review the derivation of the asymptotic Bethe equations, which can be used to determine the asymptotic multiparticle spectrum.

# 1 Introduction

$S$ -matrices are quantum mechanical probability amplitudes between incoming and outgoing on-shell particle states. Exact factorized  $S$ -matrices have played a key role in the development of integrable models [1]. Indeed, starting from an exact  $S$ -matrix, it is in principle possible to compute the asymptotic spectrum, finite-size effects (Lüscher corrections, thermodynamic Bethe ansatz), form factors, and correlation functions non-perturbatively.

As reviewed in many articles in this volume, planar four-dimensional  $\mathcal{N} = 4$  supersymmetric Yang-Mills (SYM) theory and its holographic dual, type IIB superstring theory on  $AdS_5 \times S^5$ , are believed to be quantum integrable. The world-sheet and spin-chain  $S$ -matrix have been derived based on an  $su(2|2)^2$  symmetry in [2]- [9] and will be reviewed here. This  $S$ -matrix has been confirmed by various checks. One of these checks is that the all-loop asymptotic Bethe ansatz equations (BAEs) [10] can be derived from the exact factorized  $S$ -matrix using either nested Bethe ansatz or algebraic Bethe ansatz methods [3, 4, 11, 12]. As a warm up, we first review the computation of the one-loop  $S$ -matrix in the  $su(2)$  and  $su(3)$  sectors, based on a direct coordinate Bethe ansatz, using integrable spin-chain Hamiltonians whose eigenvalues are the anomalous dimensions of scalar operators in planar  $\mathcal{N} = 4$  SYM. Using the  $S$ -matrices, we show how the bound-state spectrum can be constructed. Finally, we show how imposing periodicity on the asymptotic multiparticle wavefunction leads to the asymptotic Bethe equations, which can be used to determine the asymptotic multiparticle spectrum.

The outline of this chapter is as follows. In Sec. 2 we review the derivation of the exact  $\mathcal{N} = 4$  SYM  $S$ -matrix, first by coordinate Bethe ansatz for one-loop order, and then by utilizing  $su(2|2)$  symmetry for all-loop order. We also discuss the spectrum of bound states. In Sec. 3 we review the derivation of the asymptotic Bethe equations, first for the  $su(2)$  and  $su(3)$  sectors, and then for the full theory.

## 2 Exact S-matrix

### 2.1 Coordinate Bethe ansatz

For the planar  $\mathcal{N} = 4$  SYM theory, we are interested in SYM composite operators,

$$\text{Tr} [\mathcal{O}_1 \mathcal{O}_2 \cdots \mathcal{O}_L], \quad \mathcal{O}_i \in \{D^n \Phi, D^n \Psi, D^n F\}, \quad (2.1)$$

where all operators are at the same spacetime point. It is useful to associate the composite operators with state vectors of a quantum spin chain. The BPS operator  $\text{Tr}[Z^L]$ , where  $Z$  is one of the scalars  $\Phi$ , is the vacuum state  $|0\rangle$ . This choice of vacuum breaks the global  $psu(2, 2|4)$  symmetry down to  $su(2|2) \otimes su(2|2)$ . Other composite operators which are obtained by replacing some  $Z$ 's with certain other SYM fields (“impurities”) are mapped to excited states over the vacuum:

$$|\downarrow^1 \cdots Z \downarrow^{x_1} \chi Z \cdots Z \downarrow^{x_2} \chi' Z \cdots Z \downarrow^{x_M} \chi'' Z \cdots \downarrow^L Z\rangle \equiv \text{Tr} [Z^{x_1-1} \chi Z^{x_2-x_1-1} \chi' \cdots \chi'' \cdots], \quad (2.2)$$

where

$$\chi, \chi', \chi'', \dots \in \{\Phi_{a\dot{a}}, \Psi_{\dot{a}\alpha}, \bar{\Psi}_{a\dot{\alpha}}, D_{\alpha\dot{\alpha}}Z\}, \quad a, \dot{a} = 1, 2, \quad \alpha, \dot{\alpha} = 3, 4. \quad (2.3)$$

All other orientations for the operators  $\mathcal{O}_i$  should be regarded as multiple excitations  $\chi$  coincident at a single site.<sup>1</sup> Due to the cyclic property of the trace, the state (2.2) should be invariant under a uniform translation  $x_k \rightarrow x_k + 1$ . These excitation states belong to a bifundamental representation of a centrally extended  $su(2|2)_L \otimes su(2|2)_R$ , which should also be a symmetry of the  $S$ -matrix. The same structure can be discovered on the string world-sheet action in the light-cone gauge [13, 14].

For the  $S$ -matrix, we focus on a particular class of states, namely asymptotic states, where the distances between the impurities  $\chi, \chi', \dots$ , are very large:

$$1 \ll x_1 \ll x_2 \ll \dots \ll x_M \ll L \rightarrow \infty. \quad (2.4)$$

The  $S$ -matrices are defined as amplitudes between two such asymptotic states.

To illustrate this, we derive the two-particle  $S$ -matrix directly from the spin chain using coordinate Bethe ansatz. For simplicity, we will first consider composite operators in the  $su(2)$  sector where the impurities are a complex scalar field  $X$ .

The one-loop anomalous dimensions of the  $su(2)$  sector are given by the Hamiltonian of the spin-1/2 ferromagnetic  $su(2)$ -invariant (“XXX”) Heisenberg quantum spin-chain model [15]

$$\Gamma = \frac{\lambda}{8\pi^2} H, \quad H = \sum_{l=1}^L (1 - \mathcal{P}_{l,l+1}), \quad (2.5)$$

where  $\lambda = g_{YM}^2 N$  is the 't Hooft coupling, and  $\mathcal{P}$  is the permutation operator on  $\mathcal{C}^2 \otimes \mathcal{C}^2$ . We also need to impose a periodic boundary condition by identifying  $L + 1 \equiv 1$ .

It is obvious that the vacuum state  $|0\rangle$  is an eigenstate of  $H$  with zero energy. Since  $[H, S^z] = 0$ , the energy eigenstates can be classified according to the number of impurities (“magnons”). One-particle excited states with momentum  $p$  are given by<sup>2</sup>

$$|\psi(p)\rangle = \sum_{x=1}^L e^{ipx} \left| \overset{\downarrow}{Z} \cdots \overset{\downarrow}{X} \cdots \overset{\downarrow}{Z} \right\rangle. \quad (2.6)$$

One can easily check that (2.6) is an eigenstate of  $H$  with eigenvalue  $E = \epsilon(p)$ , where

$$\epsilon(p) = 4 \sin^2(p/2). \quad (2.7)$$

<sup>1</sup>For example,  $D\Phi$  is a superposition of  $\Phi$  and  $DZ$ . More precisely, the excitations are  $Z \mapsto DZ$  and  $Z \mapsto \Phi$ ; combining these, one obtains  $Z \mapsto DZ \mapsto D\Phi$ , or equivalently  $Z \mapsto \Phi \mapsto D\Phi$ .

<sup>2</sup>The invariance of states by a shift of one site (noted earlier) implies that the total momentum should vanish. Therefore, a one-particle state with nonvanishing momentum is not allowed in a strict sense. The one- or two-particle states which we consider here can be thought of as part of an infinitely long chain where these particles are asymptotically separated from other particles.

Two-particle eigenstate can be written as

$$|\psi(p_1, p_2)\rangle = A_{XX}(12)|X(p_1)X(p_2)\rangle + A_{XX}(21)|X(p_2)X(p_1)\rangle, \quad (2.8)$$

$$|X(p_i)X(p_j)\rangle = \sum_{x_1 < x_2} e^{i(p_i x_1 + p_j x_2)} | \overset{\downarrow 1}{Z} \cdots \overset{\downarrow x_1}{X} \cdots \overset{\downarrow x_2}{X} \cdots \overset{\downarrow L}{Z} \rangle. \quad (2.9)$$

Now we impose that these states satisfy

$$H|\psi\rangle = E(p_1, p_2)|\psi\rangle \quad (2.10)$$

and find that

$$E = \epsilon(p_1) + \epsilon(p_2), \quad (2.11)$$

where  $\epsilon(p)$  is given by (2.7). This leads to the  $X - X$  scattering amplitude given by

$$A_{XX}(21) = S(p_2, p_1)A_{XX}(12), \quad (2.12)$$

$$S(p_2, p_1) = \frac{u_2 - u_1 + i}{u_2 - u_1 - i}, \quad (2.13)$$

where  $u_j = u(p_j)$  and

$$u(p) = \frac{1}{2} \cot(p/2). \quad (2.14)$$

We now consider the more complicated case where there are two different types of complex scalar fields, namely,  $X$  and  $Y$ . This is the so-called  $su(3)$  sector, which is closed only at one loop. The ( $su(3)$ -invariant) Hamiltonian is again given by (2.5), except now  $\mathcal{P}$  is the permutation operator on  $\mathcal{C}^3 \otimes \mathcal{C}^3$ . The two-particle eigenstates with one particle of each type are of the form

$$\begin{aligned} |\psi\rangle &= A_{XY}(12)|X(p_1)Y(p_2)\rangle + A_{XY}(21)|X(p_2)Y(p_1)\rangle \\ &+ A_{YX}(12)|Y(p_1)X(p_2)\rangle + A_{YX}(21)|Y(p_2)X(p_1)\rangle, \end{aligned} \quad (2.15)$$

$$|\phi_1(p_i)\phi_2(p_j)\rangle = \sum_{x_1 < x_2} e^{i(p_i x_1 + p_j x_2)} | \overset{\downarrow 1}{Z} \cdots \overset{\downarrow x_1}{\phi_1} \cdots \overset{\downarrow x_2}{\phi_2} \cdots \overset{\downarrow L}{Z} \rangle. \quad (2.16)$$

Applying the Hamiltonian on  $|\psi\rangle$  and imposing the condition (2.10), one finds that the amplitudes should be related by (see e.g. [16])

$$\begin{pmatrix} A_{XY}(21) \\ A_{YX}(21) \end{pmatrix} = \begin{pmatrix} R(p_2, p_1) & T(p_2, p_1) \\ T(p_2, p_1) & R(p_2, p_1) \end{pmatrix} \begin{pmatrix} A_{XY}(12) \\ A_{YX}(12) \end{pmatrix}, \quad (2.17)$$

where the transmission and reflection amplitudes are given by

$$T(p_2, p_1) = \frac{u_2 - u_1}{u_2 - u_1 - i}, \quad R(p_2, p_1) = \frac{i}{u_2 - u_1 - i}, \quad (2.18)$$

respectively. Combining Eqs.(2.13) and (2.17), one can construct an  $su(2)$ -invariant  $S$ -matrix which connects two amplitudes related by momentum exchange as follows:

$$\begin{pmatrix} A_{XX}(21) \\ A_{XY}(21) \\ A_{YX}(21) \\ A_{YY}(21) \end{pmatrix} = \mathbf{S} \cdot \begin{pmatrix} A_{XX}(12) \\ A_{YX}(12) \\ A_{XY}(12) \\ A_{YY}(12) \end{pmatrix} = \begin{pmatrix} S & & & \\ & T & R & \\ & R & T & \\ & & & S \end{pmatrix} \begin{pmatrix} A_{XX}(12) \\ A_{YX}(12) \\ A_{XY}(12) \\ A_{YY}(12) \end{pmatrix}. \quad (2.19)$$

At higher loops, the  $su(2)$  sector remains closed, but the Hamiltonian becomes longer ranged. Integrability persists, but only in a perturbative sense [17]. Correspondingly, one must introduce a perturbative asymptotic Bethe ansatz, and in particular, an asymptotic  $S$ -matrix [2, 18]. That is, in contrast to the one-loop case (XXX model) where the  $S$ -matrix is “local,” for higher loops the  $S$ -matrix is only asymptotic: it applies only to in-going and out-going particles which are widely separated.

## 2.2 Yang-Baxter equation and ZF algebra

It is not practical to extend the above approach to all loops and to all sectors of planar  $\mathcal{N} = 4$  SYM. Fortunately, there is an alternative approach – based on symmetry – to derive an exact asymptotic  $S$ -matrix which is valid for any value of ‘t Hooft coupling constant. To this end, it is convenient to introduce Zamolodchikov-Faddeev (ZF) operators [1, 19] to define particle states. Using the ZF operators one can reformulate the derivation of the  $S$ -matrix into an algebraic problem. In Eq.(2.16), we have introduced an asymptotic two-particle state as a superposition of plane waves. Now we express these states in terms of creation (ZF) operators acting on the vacuum state as follows:

$$|\phi_1(p_i)\phi_2(p_j)\rangle \equiv A_{\phi_1}^\dagger(p_i)A_{\phi_2}^\dagger(p_j)|0\rangle. \quad (2.20)$$

As can be noticed in (2.1), the ZF operators corresponding to the elementary fields of  $\mathcal{N} = 4$  SYM can be denoted by  $A_{ii}^\dagger$ , where the index  $i = (a, \alpha) = 1, 2, 3, 4$  and similarly for  $\dot{i}$ . A very remarkable feature of the AdS/CFT  $S$ -matrix is that it is factorized into a tensor product of two identical  $S$ -matrices, one acting on the index  $i$  and the other on  $\dot{i}$ :

$$\mathbb{S} = S \otimes \dot{S}. \quad (2.21)$$

A natural way to describe the factorized  $S$ -matrix is to introduce “quark” ZF operators  $A_i^\dagger$  and identify  $A_{ii}^\dagger$  with the tensor product of the quark ZF operators by

$$A_{ii}^\dagger(p) = A_i^\dagger(p) \otimes A_i^\dagger(p). \quad (2.22)$$

By the factorization property, it is enough now to consider only  $A_i^\dagger$  sector for our discussion.

The bulk  $S$ -matrix elements  $S_{ij}^{i'j'}(p_1, p_2)$  define the ZF algebra relation

$$A_i^\dagger(p_1) A_j^\dagger(p_2) = S_{ij}^{i'j'}(p_1, p_2) A_{j'}^\dagger(p_2) A_{i'}^\dagger(p_1), \quad (2.23)$$

where summation over repeated indices is always understood. It is convenient to arrange these matrix elements into a  $16 \times 16$  matrix  $S$  as follows,

$$S = S_{ij}^{i'j'} e_{ii'} \otimes e_{jj'}, \quad (2.24)$$

where  $e_{ij}$  is the usual elementary  $4 \times 4$  matrix whose  $(i, j)$  matrix element is 1, and all others are zero.

As is well known [1], starting from  $A_i^\dagger(p_1) A_j^\dagger(p_2) A_k^\dagger(p_3)$ , one can arrive at linear combinations of  $A_{k''}^\dagger(p_3) A_{j''}^\dagger(p_2) A_{i''}^\dagger(p_1)$  by applying the relation (2.23) three times, in two different ways. The consistency condition is the Yang-Baxter equation,

$$S_{12}(p_1, p_2) S_{13}(p_1, p_3) S_{23}(p_2, p_3) = S_{23}(p_2, p_3) S_{13}(p_1, p_3) S_{12}(p_1, p_2). \quad (2.25)$$

We use the standard convention  $S_{12} = S \otimes \mathbb{I}$ ,  $S_{23} = \mathbb{I} \otimes S$ , and  $S_{13} = \mathcal{P}_{12} S_{23} \mathcal{P}_{12}$ , where  $\mathcal{P}_{12} = \mathcal{P} \otimes \mathbb{I}$ ,  $\mathcal{P} = e_{ij} \otimes e_{ji}$  is the permutation matrix, and  $\mathbb{I}$  is the four-dimensional identity matrix. The ZF algebra (2.23) also implies the bulk unitarity equation

$$S_{12}(p_1, p_2) S_{21}(p_2, p_1) = \mathbb{I}, \quad (2.26)$$

where  $S_{21} = \mathcal{P}_{12} S_{12} \mathcal{P}_{12}$ .

Solving the Yang-Baxter equation can be complicated. Fortunately, as we shall see below,  $su(2|2)$  symmetry suffices to determine the AdS/CFT  $S$ -matrix (in the fundamental representation) – there is no need to solve the Yang-Baxter equation, as it is automatically satisfied.

### 2.3 Centrally extended $su(2|2)$

The centrally extended  $su(2|2)$  algebra consists of the rotation generators  $\mathbb{L}_a^b$ ,  $\mathbb{R}_\alpha^\beta$ , the supersymmetry generators  $\mathbb{Q}_\alpha^a$ ,  $\mathbb{Q}_a^{\dagger\alpha}$ , and the central elements  $\mathbb{C}$ ,  $\mathbb{C}^\dagger$ ,  $\mathbb{H}$ .<sup>3</sup> Latin indices  $a, b, \dots$  take values  $\{1, 2\}$ , while Greek indices  $\alpha, \beta, \dots$  take values  $\{3, 4\}$ . These generators have the following nontrivial commutation relations [3, 4, 9]

$$\begin{aligned} [\mathbb{L}_a^b, \mathbb{J}_c] &= \delta_c^b \mathbb{J}_a - \frac{1}{2} \delta_a^b \mathbb{J}_c, & [\mathbb{R}_\alpha^\beta, \mathbb{J}_\gamma] &= \delta_\gamma^\beta \mathbb{J}_\alpha - \frac{1}{2} \delta_\alpha^\beta \mathbb{J}_\gamma, \\ [\mathbb{L}_a^b, \mathbb{J}^c] &= -\delta_a^c \mathbb{J}^b + \frac{1}{2} \delta_a^b \mathbb{J}^c, & [\mathbb{R}_\alpha^\beta, \mathbb{J}^\gamma] &= -\delta_\alpha^\gamma \mathbb{J}^\beta + \frac{1}{2} \delta_\alpha^\beta \mathbb{J}^\gamma, \\ \{\mathbb{Q}_\alpha^a, \mathbb{Q}_\beta^b\} &= \epsilon_{\alpha\beta} \epsilon^{ab} \mathbb{C}, & \{\mathbb{Q}_a^{\dagger\alpha}, \mathbb{Q}_b^{\dagger\beta}\} &= \epsilon^{\alpha\beta} \epsilon_{ab} \mathbb{C}^\dagger, \\ \{\mathbb{Q}_\alpha^a, \mathbb{Q}_b^{\dagger\beta}\} &= \delta_b^a \mathbb{R}_\alpha^\beta + \delta_\alpha^\beta \mathbb{L}_b^a + \frac{1}{2} \delta_b^a \delta_\alpha^\beta \mathbb{H}, \end{aligned} \quad (2.27)$$

where  $\mathbb{J}_i$  ( $\mathbb{J}^i$ ) denotes any lower (upper) index of a generator, respectively.

<sup>3</sup>The central charge  $\mathbb{H}$  is identified as the world-sheet Hamiltonian. The additional central charges  $\mathbb{C}$  and  $\mathbb{C}^\dagger$ , which are necessary for having momentum-dependent representations with the appropriate energy, also appear in the off-shell symmetry algebra of the gauge-fixed sigma model [14].

The action of the bosonic generators on the ZF operators is given by

$$\begin{aligned} [\mathbb{L}_a^b, A_c^\dagger(p)] &= (\delta_c^b \delta_a^d - \frac{1}{2} \delta_a^b \delta_c^d) A_d^\dagger(p), \quad [\mathbb{L}_a^b, A_\gamma^\dagger(p)] = 0, \\ [\mathbb{R}_\alpha^\beta, A_\gamma^\dagger(p)] &= (\delta_\gamma^\beta \delta_\alpha^\delta - \frac{1}{2} \delta_\alpha^\beta \delta_\gamma^\delta) A_\delta^\dagger(p), \quad [\mathbb{R}_\alpha^\beta, A_c^\dagger(p)] = 0. \end{aligned} \quad (2.28)$$

The operator relations for supersymmetry generators<sup>4</sup>

$$\begin{aligned} \mathbb{Q}_\alpha^a A_b^\dagger(p) &= e^{-ip/2} \left[ a(p) \delta_b^a A_\alpha^\dagger(p) + A_b^\dagger(p) \mathbb{Q}_\alpha^a \right], \\ \mathbb{Q}_\alpha^a A_\beta^\dagger(p) &= e^{-ip/2} \left[ b(p) \epsilon_{\alpha\beta} \epsilon^{ab} A_b^\dagger(p) - A_\beta^\dagger(p) \mathbb{Q}_\alpha^a \right], \\ \mathbb{Q}_a^{\dagger\alpha} A_b^\dagger(p) &= e^{ip/2} \left[ c(p) \epsilon_{ab} \epsilon^{\alpha\beta} A_\beta^\dagger(p) + A_b^\dagger(p) \mathbb{Q}_a^{\dagger\alpha} \right], \\ \mathbb{Q}_a^{\dagger\alpha} A_\beta^\dagger(p) &= e^{ip/2} \left[ d(p) \delta_\beta^\alpha A_a^\dagger(p) - A_\beta^\dagger(p) \mathbb{Q}_a^{\dagger\alpha} \right], \end{aligned} \quad (2.29)$$

and the central charges

$$\begin{aligned} \mathbb{C} A_i^\dagger(p) &= e^{-ip} \left[ a(p) b(p) A_i^\dagger(p) + A_i^\dagger(p) \mathbb{C} \right], \\ \mathbb{C}^\dagger A_i^\dagger(p) &= e^{ip} \left[ c(p) d(p) A_i^\dagger(p) + A_i^\dagger(p) \mathbb{C}^\dagger \right], \\ \mathbb{H} A_i^\dagger(p) &= [a(p) d(p) + b(p) c(p)] A_i^\dagger(p) + A_i^\dagger(p) \mathbb{H}, \end{aligned} \quad (2.30)$$

can be used to act with the generators on multiparticle states. The ZF operators form a representation of the symmetry algebra provided  $ad - bc = 1$ . The representation is also unitary provided  $d = a^*, c = b^*$ . Acting with  $\mathbb{C}$  on both sides of Eq.(2.23) applied to the vacuum state, one can deduce the further constraint

$$e^{-ip_1} a(p_1) b(p_1) + e^{-i(p_1+p_2)} a(p_2) b(p_2) = e^{-ip_2} a(p_2) b(p_2) + e^{-i(p_1+p_2)} a(p_1) b(p_1), \quad (2.31)$$

which leads to the relation  $a(p)b(p) = ig(e^{ip} - 1)$ , where  $g$  is a constant. It follows that the parameters can be chosen as follows [3, 9, 20]

$$a = \sqrt{g}\eta, \quad b = \sqrt{g} \frac{i}{\eta} \left( \frac{x^+}{x^-} - 1 \right), \quad c = -\sqrt{g} \frac{\eta}{x^+}, \quad d = \sqrt{g} \frac{x^+}{i\eta} \left( 1 - \frac{x^-}{x^+} \right), \quad (2.32)$$

where

$$x^+ + \frac{1}{x^+} - x^- - \frac{1}{x^-} = \frac{i}{g}, \quad \frac{x^+}{x^-} = e^{ip}, \quad \eta = e^{ip/4} \sqrt{i(x^- - x^+)}. \quad (2.33)$$

Hence, for a one-particle state,

$$\mathbb{H} = -ig \left( x^+ - \frac{1}{x^+} - x^- + \frac{1}{x^-} \right) = \sqrt{1 + 16g^2 \sin^2 \frac{p}{2}}. \quad (2.34)$$

<sup>4</sup>Such momentum-dependent braiding relations, which are typical for nonlocal (fractional-spin) integrals of motion, have long been used to determine  $S$ -matrices in certain integrable models, see e.g. [21–23].

The anomalous dimension  $\mathbb{H} - 1$  matches with the weak-coupling result given by (2.5) and (2.7), provided we make the identification  $g = \sqrt{\lambda}/(4\pi)$ . That is, the symmetry determines the exact dispersion relation, except for the dependence on the coupling constant. See also [24].

The  $S$ -matrix can be determined (up to a phase) by demanding that it commute with the symmetry generators. That is, starting from  $\mathbb{J} A_i^\dagger(p_1) A_j^\dagger(p_2)|0\rangle$  where  $\mathbb{J}$  is a symmetry generator, and assuming that  $\mathbb{J}$  annihilates the vacuum state, one can arrive at linear combinations of  $A_{j'}^\dagger(p_2) A_{i'}^\dagger(p_1)|0\rangle$  in two different ways, by applying the ZF relation (2.23) and the symmetry relations (2.28), (2.29) in different orders. The consistency condition is a system of linear equations for the  $S$ -matrix elements. The result for the nonzero matrix elements  $S_{ij}^{i'j'}(p_1, p_2)$  is [3, 9]

$$\begin{aligned}
 S_{aa}^{aa} &= A, & S_{\alpha\alpha}^{\alpha\alpha} &= D, \\
 S_{ab}^{ab} &= \frac{1}{2}(A - B), & S_{ab}^{ba} &= \frac{1}{2}(A + B), \\
 S_{\alpha\beta}^{\alpha\beta} &= \frac{1}{2}(D - E), & S_{\alpha\beta}^{\beta\alpha} &= \frac{1}{2}(D + E), \\
 S_{ab}^{\alpha\beta} &= -\frac{1}{2}\epsilon_{ab}\epsilon^{\alpha\beta} C, & S_{\alpha\beta}^{ab} &= -\frac{1}{2}\epsilon^{ab}\epsilon_{\alpha\beta} F, \\
 S_{\alpha\alpha}^{aa} &= G, & S_{\alpha\alpha}^{a\alpha} &= H, & S_{\alpha\alpha}^{a\alpha} &= K, & S_{\alpha\alpha}^{\alpha a} &= L,
 \end{aligned} \tag{2.35}$$

where  $a, b \in \{1, 2\}$  with  $a \neq b$ ;  $\alpha, \beta \in \{3, 4\}$  with  $\alpha \neq \beta$ ; and

$$\begin{aligned}
 A &= S_0 \frac{x_2^- - x_1^+ \eta_1 \eta_2}{x_2^+ - x_1^- \tilde{\eta}_1 \tilde{\eta}_2}, \\
 B &= -S_0 \left[ \frac{x_2^- - x_1^+}{x_2^+ - x_1^-} + 2 \frac{(x_1^- - x_1^+)(x_2^- - x_2^+)(x_2^- + x_1^+)}{(x_1^- - x_2^+)(x_1^- x_2^- - x_1^+ x_2^+)} \right] \frac{\eta_1 \eta_2}{\tilde{\eta}_1 \tilde{\eta}_2}, \\
 C &= S_0 \frac{2ix_1^- x_2^- (x_1^+ - x_2^+) \eta_1 \eta_2}{x_1^+ x_2^+ (x_1^- - x_2^+) (1 - x_1^- x_2^-)}, & D &= -S_0, \\
 E &= S_0 \left[ 1 - 2 \frac{(x_1^- - x_1^+)(x_2^- - x_2^+)(x_1^- + x_2^+)}{(x_1^- - x_2^+)(x_1^- x_2^- - x_1^+ x_2^+)} \right], \\
 F &= S_0 \frac{2i(x_1^- - x_1^+)(x_2^- - x_2^+)(x_1^+ - x_2^+)}{(x_1^- - x_2^+)(1 - x_1^- x_2^-) \tilde{\eta}_1 \tilde{\eta}_2}, \\
 G &= S_0 \frac{(x_2^- - x_1^-) \eta_1}{(x_2^+ - x_1^-) \tilde{\eta}_1}, & H &= S_0 \frac{(x_2^+ - x_2^-) \eta_1}{(x_1^- - x_2^+) \tilde{\eta}_2}, \\
 K &= S_0 \frac{(x_1^+ - x_1^-) \eta_2}{(x_1^- - x_2^+) \tilde{\eta}_1}, & L &= S_0 \frac{(x_1^+ - x_2^+) \eta_2}{(x_1^- - x_2^+) \tilde{\eta}_2},
 \end{aligned} \tag{2.36}$$

where  $x_i^\pm = x^\pm(p_i)$  and

$$\eta_1 = \eta(p_1) e^{ip_2/2}, \quad \eta_2 = \eta(p_2), \quad \tilde{\eta}_1 = \eta(p_1), \quad \tilde{\eta}_2 = \eta(p_2) e^{ip_1/2}, \tag{2.37}$$

where  $\eta(p)$  is given in (2.33). This  $S$ -matrix satisfies the standard Yang-Baxter equation (2.25). It also satisfies the unitarity equation (2.26), provided that the scalar factor obeys

$$S_0(p_1, p_2) S_0(p_2, p_1) = 1. \tag{2.38}$$

In order to determine  $S_0$ , one should impose on the full  $S$ -matrix (2.21) crossing symmetry and other physical requirements, which will be explained in the next chapter of this volume [25]. The final result is given by

$$S_0(p_1, p_2)^2 = \frac{x_1^- - x_2^+}{x_1^+ - x_2^-} \frac{1 - \frac{1}{x_1^+ x_2^-}}{1 - \frac{1}{x_1^- x_2^+}} \sigma(p_1, p_2)^2, \quad (2.39)$$

where the dressing factor  $\sigma(p_1, p_2)$  is called the BES/BHL phase factor [7, 8].

We remark that the above  $S$ -matrix is in fact in the “string frame” (or “basis”) [9]. Starting from the spin chain one obtains the  $S$ -matrix instead in the “spin-chain frame,” where (2.37) is replaced by

$$\eta_1 = \eta(p_1), \quad \eta_2 = \eta(p_2), \quad \tilde{\eta}_1 = \eta(p_1), \quad \tilde{\eta}_2 = \eta(p_2). \quad (2.40)$$

The  $S$ -matrix in the spin-chain frame satisfies a “twisted” version of the Yang-Baxter equation, rather than (2.25).

We also remark that the  $su(2|2)$   $S$ -matrix is closely related [4, 11] to Shastry’s  $R$ -matrix [26, 27] for the Hubbard model.

## 2.4 Bound states

So far we have considered two-particle asymptotic scattering states. The two particles carrying real momenta can be widely separated. Another interesting case occurs when the two particles are closely localized and behave as a single particle. This kind of localized state is the bound state [28, 29].

As a first example, let us consider again the  $su(2)$  sector at one loop. In terms of

$$x = \frac{x_1 + x_2}{2}, \quad r = x_2 - x_1, \quad p_{1,2} = \frac{p}{2} \pm k, \quad (2.41)$$

we can reexpress the two-particle state (2.8) as

$$|\psi\rangle = \sum_{x, r} e^{ipx} (A_{XX}(12)e^{-ikr} + A_{XX}(21)e^{ikr}) |Z \cdots \overbrace{XZ \cdots ZX}^r \cdots Z\rangle. \quad (2.42)$$

Notice that  $r > 0$  by definition. To have a localized wave, the amplitude should decay exponentially as the distance  $r$  increases. This can be satisfied if we take  $k = iq$  ( $q > 0$ ) and  $A_{XX}(12) = 0$ . From Eq.(2.12) this leads to a condition that  $S(p_2, p_1)$  should have a pole. In other words, a simple pole of the  $S$ -matrix corresponds to a bound state. In terms of  $u$ -variables, this condition is satisfied by  $u_{2,1} = u \pm i/2$  as one can see from (2.13). This is an example of a so-called string solution, of size 2. Following a similar procedure, one can find that the higher bound-state poles of the  $S$ -matrices can be obtained when the particles carry momenta

$$u_j^{(n)} = u + i \frac{2j - n - 1}{2}, \quad j = 1, \dots, n. \quad (2.43)$$

This is a string of size  $n$ . The energy of this particle can be obtained from (2.7)

$$\epsilon_n(u) = \frac{n}{u^2 + n^2/4}. \quad (2.44)$$

Now consider the more complicated case of the  $su(3)$  sector, for which the two-particle eigenstates are given by (2.15) and (2.16). By the same argument as above, the localized state is possible when  $u_2 - u_1 = i$ . This leads to  $A_{XY}(12) = A_{YX}(12) = 0$  from (2.17) and  $A_{XY}(21) = A_{YX}(21)$  because the residues of  $T$  and  $R$  in (2.18) are the same. Therefore, the localized state can be written as

$$|\psi\rangle \sim \sum_{x, r} e^{ipx} e^{ikr} \left[ |Z \cdots \overbrace{XZ \cdots ZY}^r \cdots Z\rangle + |Z \cdots \overbrace{YZ \cdots ZX}^r \cdots Z\rangle \right], \quad (2.45)$$

where  $X$  and  $Y$  appear symmetrically.

The bound states for generic value of 't Hooft coupling constant can be constructed in a similar way. Combining two factors of the amplitude  $A$  (2.36) with (2.39), the  $S$ -matrix of the  $su(2)$  sector (in the spin-chain frame) is given by

$$S(p_1, p_2) = \frac{x_1^+ - x_2^-}{x_1^- - x_2^+} \frac{1 - \frac{1}{x_1^+ x_2^-}}{1 - \frac{1}{x_1^- x_2^+}} \sigma(p_1, p_2)^2. \quad (2.46)$$

This amplitude has two simple poles at  $x_1^- = x_2^+$  and  $x_1^- = 1/x_2^+$ . Let us consider first the former case for general higher-order bound states where simple poles appear

$$x_1^- = x_2^+, \quad x_2^- = x_3^+, \quad \cdots, \quad x_{n-1}^- = x_n^+. \quad (2.47)$$

With these bound-state conditions, one can easily show that the momentum ( $p$ ) and energy ( $\mathbb{H}$ ) are given by

$$\frac{X^+}{X^-} = e^{ip}, \quad X^+ + \frac{1}{X^+} - X^- - \frac{1}{X^-} = \frac{in}{g} \quad (2.48)$$

$$\mathbb{H} = -ig \left( X^+ - \frac{1}{X^+} - X^- + \frac{1}{X^-} \right) = \sqrt{n^2 + 16g^2 \sin^2 \frac{p}{2}}, \quad (2.49)$$

and satisfy the BPS (shortening) condition in (2.48) if we identify

$$X^- \equiv x_n^-, \quad \text{and} \quad X^+ \equiv x_1^+. \quad (2.50)$$

The other pole at  $x_1^- = 1/x_2^+$  cannot satisfy this condition and leads to non-BPS states.

The situation for the full  $su(2|2)$   $S$ -matrix is more complicated even though the locations of poles are the same as in the  $su(2)$  sector. The  $M$ -particle bound states belong to an atypical totally symmetric representation of the centrally extended  $su(2|2)$  algebra. This representation has dimension  $2M|2M$  and can be realized on the graded vector space where the basis is given by

- $M + 1$  bosonic states: symmetric in  $a_i$ :  $|e_{a_1 \dots a_M}\rangle$ , where  $a_i = 1, 2$  are bosonic indices.

- $M-1$  bosonic states: symmetric in  $a_i$ :  $|e_{a_1 \dots a_{M-2} \alpha_1 \alpha_2}\rangle$ , where  $\alpha_i = 3, 4$  are fermionic indices.
- $2M$  fermionic states: symmetric in  $a_i$ :  $|e_{a_1 \dots a_{M-1} \alpha}\rangle$ , where  $\alpha = 3, 4$ .

An efficient realization of this representation is to introduce [20] a vector space of analytic functions of two bosonic variables  $w_a$  and two fermionic variables  $\theta_\alpha$ . For example, the 8-dimensional states for  $M = 2$  can be given by

$$\begin{aligned} |e_1\rangle &= \frac{w_1 w_1}{\sqrt{2}}, & |e_2\rangle &= w_1 w_2, & |e_3\rangle &= \frac{w_2 w_2}{\sqrt{2}}, & |e_4\rangle &= \theta_3 \theta_4, \\ |e_5\rangle &= w_1 \theta_3, & |e_6\rangle &= w_1 \theta_4, & |e_7\rangle &= w_2 \theta_3, & |e_8\rangle &= w_2 \theta_4. \end{aligned} \quad (2.51)$$

The  $su(2|2)$  generators can be represented by differential operators on this vector space as follows:

$$\begin{aligned} \mathbb{L}_a^b &= w_a \frac{\partial}{\partial w_b} - \frac{1}{2} \delta_a^b w_c \frac{\partial}{\partial w_c}, & \mathbb{R}_\alpha^\beta &= \theta_\alpha \frac{\partial}{\partial \theta_\beta} - \frac{1}{2} \delta_\alpha^\beta \theta_\gamma \frac{\partial}{\partial \theta_\gamma}, \\ \mathbb{Q}_\alpha^a &= a \theta_\alpha \frac{\partial}{\partial w_a} + b \epsilon^{ab} \epsilon_{\alpha\beta} w_b \frac{\partial}{\partial \theta_\beta}, & \mathbb{Q}_a^{\dagger\alpha} &= d w_a \frac{\partial}{\partial \theta_\alpha} + c \epsilon_{ab} \epsilon^{\alpha\beta} \theta_\beta \frac{\partial}{\partial w_b}, \\ \mathbb{C} &= ab \left( w_a \frac{\partial}{\partial w_a} + \theta_\alpha \frac{\partial}{\partial \theta_\alpha} \right), & \mathbb{C}^\dagger &= cd \left( w_a \frac{\partial}{\partial w_a} + \theta_\alpha \frac{\partial}{\partial \theta_\alpha} \right), \\ \mathbb{H} &= (ad + bc) \left( w_a \frac{\partial}{\partial w_a} + \theta_\alpha \frac{\partial}{\partial \theta_\alpha} \right). \end{aligned} \quad (2.52)$$

From this, it is straightforward to evaluate how the generators act on the bound states.

In contrast with the case of the fundamental representation reviewed in the previous subsection, the  $su(2|2)$  symmetry is not enough to determine the bound-state  $S$ -matrix completely. A very important observation is that the fundamental bulk  $S$ -matrix (2.35) has a remarkable Yangian symmetry  $Y(su(2|2))$  [30,31] which can be used to completely determine the two-particle [20,32] and general  $l$ -particle bound state bulk  $S$ -matrices [33]. It is fortunate that such a general way of generating higher-dimensional  $S$ -matrices has been found, since the fusion procedure does not seem to work for AdS/CFT  $S$ -matrices [20].

### 3 Asymptotic Bethe equations

For a system of  $N$  *free* particles on a ring of length  $L$ , the quantized momenta, and therefore the exact spectrum, are trivially determined. For particles which are not free but instead have *integrable* interactions, the problem of determining the spectrum is much more difficult, but nevertheless is still tractable. Indeed, if one knows the (asymptotic)  $S$ -matrix which satisfies the Yang-Baxter equations, then in principle it is possible to derive a set of (asymptotic) Bethe equations which determine the (asymptotic) quantized momenta, and therefore, the (asymptotic) multiparticle spectrum. These (asymptotic) Bethe equations are obtained by imposing periodicity on the (asymptotic) multiparticle wavefunction. In the AdS/CFT case, this task is technically difficult due to the matrix structure of the  $S$ -matrix and the complicated functional dependence of its matrix elements. Before addressing this problem, it is helpful to consider some simpler examples.

### 3.1 The S-matrix is a phase

As a first warm-up exercise, let us consider the simple case of a two-body (asymptotic) S-matrix which is a phase rather than a matrix.<sup>5</sup> An example is the magnon-magnon S-matrix in the  $su(2)$  sector at one loop, which is given by (2.13), (2.14). The ZF operator  $A^\dagger(p)$  does not have an internal index, and satisfies (cf., (2.23))

$$A^\dagger(p_1) A^\dagger(p_2) = S(p_1, p_2) A^\dagger(p_2) A^\dagger(p_1). \quad (3.1)$$

Integrability of the model implies that the multiparticle wavefunction is of the Bethe type. That is, the (asymptotic) eigenstates can be expressed as

$$|\psi\rangle = \sum_{1 \leq x_{Q_1} \ll \dots \ll x_{Q_N} \leq L} \Psi^{(Q)}(x_1, \dots, x_N) \left| \begin{array}{cccc} \downarrow 1 & & \downarrow x_{Q_1} & \downarrow x_{Q_N} \\ \downarrow Z & \dots & \downarrow X & \dots & \downarrow X & \dots & \downarrow Z \\ \end{array} \right\rangle, \quad (3.2)$$

where the (asymptotic)  $N$ -particle wavefunction in the sector  $Q = (Q_1, \dots, Q_N)$  such that  $x_{Q_1} \ll \dots \ll x_{Q_N}$  is given by

$$\Psi^{(Q)}(x_1, \dots, x_N) = \sum_P A^P e^{ip_P \cdot x_Q}. \quad (3.3)$$

The sum is over all permutations of  $P = (P_1, \dots, P_N)$ , and  $p_P \cdot x_Q = \sum_{k=1}^N p_{P_k} x_{Q_k}$ . Also, the coordinate-independent amplitudes  $A^P$  are related to each other according to

$$A^P \sim A^\dagger(p_{P_1}) \dots A^\dagger(p_{P_N}). \quad (3.4)$$

For example, for  $N = 2$ , the wavefunction in the sector  $x_1 \ll x_2$  is given by

$$\Psi^{(12)}(x_1, x_2) = A^{12} e^{i(p_1 x_1 + p_2 x_2)} + A^{21} e^{i(p_2 x_1 + p_1 x_2)}, \quad x_1 \ll x_2. \quad (3.5)$$

Since

$$A^{21} \sim A^\dagger(p_2) A^\dagger(p_1) = S(p_2, p_1) A^\dagger(p_1) A^\dagger(p_2) \sim S(p_2, p_1) A^{12}, \quad (3.6)$$

we recover the previous results (2.8), (2.9), (2.12) upon identifying

$$A_{XX}(12) = A^{12}, \quad A_{XX}(21) = A^{21}. \quad (3.7)$$

We consider a system of  $N$  widely-separated particles on a ring of length  $L$ . Periodicity of the wavefunction  $\Psi(x_1, \dots, x_N)$  in (say) the first coordinate,

$$\Psi(1, x_2, \dots, x_N) = \Psi(L + 1, x_2, \dots, x_N), \quad (3.8)$$

implies a relationship between the wavefunctions in the sectors  $x_1 \ll \dots \ll x_N$  and  $x_2 \ll \dots \ll x_N \ll x_1$ :

$$\Psi^{(1\dots N)}(1, x_2, \dots, x_N) = \Psi^{(2\dots N1)}(L + 1, x_2, \dots, x_N). \quad (3.9)$$

---

<sup>5</sup>In this case, the Yang-Baxter equations are trivially satisfied by the S-matrix.

According to (3.3), the wavefunctions in these two sectors are given by

$$\begin{aligned}\Psi^{(1\dots N)}(1, x_2, \dots, x_N) &= A^{1\dots N} e^{i(p_1 + p_2 x_2 + \dots + p_N x_N)} + \dots, \\ \Psi^{(2\dots N1)}(L+1, x_2, \dots, x_N) &= A^{2\dots N1} e^{i(p_1 L + p_1 + p_2 x_2 + \dots + p_N x_N)} + \dots,\end{aligned}\quad (3.10)$$

where we have displayed only the terms which depend on the particular combination  $p_2 x_2 + \dots + p_N x_N$ . In view of the periodicity condition (3.9), the coefficients  $A^{1\dots N}$  and  $A^{2\dots N1}$  in (3.10) must be related as follows

$$A^{1\dots N} = A^{2\dots N1} e^{ip_1 L}. \quad (3.11)$$

There is another relation between the coefficients  $A^{1\dots N}$  and  $A^{2\dots N1}$  which follows from (3.4). Indeed, it is easy to see that

$$\begin{aligned}A^{1\dots N} &\sim A^\dagger(p_1) A^\dagger(p_2) \dots A^\dagger(p_N) \\ &= \prod_{j=2}^N S(p_1, p_j) A^\dagger(p_2) \dots A^\dagger(p_N) A^\dagger(p_1) \sim \prod_{j=2}^N S(p_1, p_j) A^{2\dots N1},\end{aligned}\quad (3.12)$$

where we have used (3.1) to move  $A^\dagger(p_1)$  to the right successively past all the other ZF operators. The two relations (3.11) and (3.12) imply that

$$\prod_{j=2}^N S(p_1, p_j) = e^{ip_1 L}. \quad (3.13)$$

Examining the terms in the ellipsis in (3.10) similarly leads to the (asymptotic) Bethe equations for all the momenta,

$$\prod_{\substack{j=1 \\ j \neq k}}^N S(p_k, p_j) = e^{ip_k L}, \quad k = 1, \dots, N. \quad (3.14)$$

For a ‘‘local’’  $S$ -matrix such as the one for the spin-1/2 ferromagnetic Heisenberg chain, these equations are exact for finite  $L$ ; at least in principle one can solve these equations for the momenta and therefore compute the exact finite- $L$  spectrum,

$$\mathbf{P} = \sum_{k=1}^N p_k, \quad \mathbf{E} = \sum_{k=1}^N \epsilon(p_k), \quad (3.15)$$

where  $\epsilon(p)$  is the one-particle dispersion relation (see, e.g. (2.7)). For an asymptotic  $S$ -matrix such as the one for AdS/CFT, the asymptotic Bethe equations can be used to determine the spectrum only asymptotically.<sup>6</sup>

<sup>6</sup>Nevertheless, it is possible to obtain at least a part of the exact spectrum by other means [34].

### 3.2 The S-matrix is a $4 \times 4$ matrix

As a second warm-up exercise, we consider a solution of the Yang-Baxter equations which is a  $4 \times 4$  matrix. For simplicity, we further restrict the  $S$ -matrix to be  $su(2)$ -invariant. Hence, we take

$$S_{jk}^{j'k'}(p_1, p_2) = \frac{1}{u_1 - u_2 - i} \left[ (u_1 - u_2) \delta_j^{j'} \delta_k^{k'} + i \delta_j^{k'} \delta_k^{j'} \right], \quad (3.16)$$

where again  $u_j = u(p_j)$  and  $u(p)$  is given by (2.14). This is in fact the magnon-magnon  $S$ -matrix in the  $su(3)$  sector which we discussed earlier (2.19). The ZF operator now has an internal index which can take the values 1 and 2, and satisfies (2.23). As we shall see, the analysis is similar to the one in Sec. 3.1. The new feature is the internal symmetry, which is handled neatly by introducing the transfer matrix (3.25).

The (asymptotic) eigenstates can now be expressed as

$$|\psi\rangle = \sum_{1 \leq x_{Q_1} \ll \dots \ll x_{Q_N} \leq L} \sum_{i_1, \dots, i_N=1}^2 \Psi_{i_1 \dots i_N}^{(Q)}(x_1, \dots, x_N) \left| \overset{1}{\downarrow} Z \cdots \overset{x_{Q_1}}{\downarrow} \phi_{i_1} \cdots \overset{x_{Q_N}}{\downarrow} \phi_{i_N} \cdots \overset{L}{\downarrow} Z \right\rangle, \quad (3.17)$$

where the (asymptotic)  $N$ -particle wavefunction in the sector  $Q = (Q_1, \dots, Q_N)$  is given by <sup>7</sup>

$$\Psi_{i_1 \dots i_N}^{(Q)}(x_1, \dots, x_N) = \sum_P A_{i_1 \dots i_N}^{P|Q} e^{ip_P \cdot x_Q} \quad (3.18)$$

and

$$A_{i_1 \dots i_N}^{P|Q} \sim A_{i_{Q_1}}^\dagger(p_{P_1}) \cdots A_{i_{Q_N}}^\dagger(p_{P_N}), \quad (3.19)$$

cf. (3.2)-(3.4). For  $N = 2$  in the sector  $x_1 \ll x_2$ , upon identifying

$$A_{\phi_i \phi_j}(12) = A_{ij}^{12|12}, \quad A_{\phi_i \phi_j}(21) = A_{ij}^{21|12} \quad (3.20)$$

where  $\phi_1 = X, \phi_2 = Y$ , we recover the previous results (2.15)-(2.19). <sup>8</sup>

Proceeding as before, we see that the periodicity of the wavefunction in the first coordinate,

$$\Psi_{i_1 \dots i_N}(1, x_2, \dots, x_N) = \Psi_{i_1 \dots i_N}(L+1, x_2, \dots, x_N) \quad (3.21)$$

<sup>7</sup>The original papers include [35]- [38]. Here we follow the appendix in [39].

<sup>8</sup>For example,

$$\begin{aligned} A_{XY}(21) &= A_{12}^{21|12} \sim A_1^\dagger(p_2) A_2^\dagger(p_1) = S_{12}^{12} A_2^\dagger(p_1) A_1^\dagger(p_2) + S_{12}^{21} A_1^\dagger(p_1) A_2^\dagger(p_2) \\ &\sim S_{12}^{12} A_{21}^{12|12} + S_{12}^{21} A_{12}^{12|12} = T A_{YX}(12) + R A_{XY}(12), \end{aligned}$$

which is in agreement with (2.17). Here the arguments  $(p_2, p_1)$  of all the  $S$ -matrix elements have been suppressed for brevity.

implies a relationship between the wavefunctions in the sectors  $x_1 \ll \dots \ll x_N$  and  $x_2 \ll \dots \ll x_N \ll x_1$ :

$$\Psi_{i_1 \dots i_N}^{(1 \dots N)}(1, x_2, \dots, x_N) = \Psi_{i_1 \dots i_N}^{(2 \dots N1)}(L+1, x_2, \dots, x_N). \quad (3.22)$$

This leads to the following relationship between coefficients

$$A_{i_1 \dots i_N}^{1 \dots N | 1 \dots N} = A_{i_1 \dots i_N}^{2 \dots N1 | 2 \dots N1} e^{ip_1 L}. \quad (3.23)$$

We now proceed to generate from (3.19) another relation between these two coefficients. Using (2.23) to move  $A_{i_1}^\dagger(p_1)$  to the right successively past all the other ZF operators, we obtain

$$\begin{aligned} A_{i_1 \dots i_N}^{1 \dots N | 1 \dots N} &\sim A_{i_1}^\dagger(p_1) A_{i_2}^\dagger(p_2) \dots A_{i_N}^\dagger(p_N) \\ &= S_{i_1 i_2}^{a_2 i_2'}(p_1, p_2) S_{a_2 i_3}^{a_3 i_3'}(p_1, p_3) \dots S_{a_{N-1} i_N}^{i_1' i_N'}(p_1, p_N) A_{i_2'}^\dagger(p_2) \dots A_{i_N'}^\dagger(p_N) A_{i_1'}^\dagger(p_1) \\ &\sim S_{i_1 i_2}^{a_2 i_2'}(p_1, p_2) S_{a_2 i_3}^{a_3 i_3'}(p_1, p_3) \dots S_{a_{N-1} i_N}^{i_1' i_N'}(p_1, p_N) A_{i_1' \dots i_N'}^{2 \dots N1 | 2 \dots N1}. \end{aligned} \quad (3.24)$$

It is very convenient to introduce the so-called (inhomogeneous) transfer matrix

$$t_{i_1 \dots i_N}^{i_1' \dots i_N'}(p; p_1, \dots, p_N) \equiv S_{a_N i_1}^{a_1 i_1'}(p, p_1) S_{a_1 i_2}^{a_2 i_2'}(p, p_2) \dots S_{a_{N-1} i_N}^{a_N i_N'}(p, p_N). \quad (3.25)$$

Its value at  $p = p_1$  is proportional to the coefficient of  $A_{i_1' \dots i_N'}^{2 \dots N1 | 2 \dots N1}$  in (3.24),

$$t_{i_1 \dots i_N}^{i_1' \dots i_N'}(p_1; p_1, \dots, p_N) = -S_{i_1 i_2}^{a_2 i_2'}(p_1, p_2) S_{a_2 i_3}^{a_3 i_3'}(p_1, p_3) \dots S_{a_{N-1} i_N}^{i_1' i_N'}(p_1, p_N), \quad (3.26)$$

since  $S_{ij}^{i'j'}(p, p) = -\delta_i^{j'} \delta_j^{i'}$ , as one can see from (3.16).

We demand that  $A_{i_1' \dots i_N'}^{2 \dots N1 | 2 \dots N1}$  be an eigenvector of the transfer matrix,<sup>9</sup>

$$t_{i_1 \dots i_N}^{i_1' \dots i_N'}(p; p_1, \dots, p_N) A_{i_1' \dots i_N'}^{2 \dots N1 | 2 \dots N1} = \Lambda(p; p_1, \dots, p_N) A_{i_1' \dots i_N'}^{2 \dots N1 | 2 \dots N1}, \quad (3.27)$$

where  $\Lambda(p; p_1, \dots, p_N)$  is the corresponding eigenvalue. It follows from Eqs. (3.23), (3.24), (3.26), (3.27) that

$$\Lambda(p_1; p_1, \dots, p_N) = -e^{ip_1 L}; \quad (3.28)$$

and more generally

$$\Lambda(p_k; p_1, \dots, p_N) = -e^{ip_k L}, \quad k = 1, \dots, N. \quad (3.29)$$

To summarize so far: imposing periodic boundary conditions on the multiparticle wavefunction has led to the important relations (3.29). However, in order to obtain

<sup>9</sup>This is necessary in order to be able to satisfy (3.23). We note that the transfer matrix has the commutativity property

$$[t(p; p_1, \dots, p_N), t(p'; p_1, \dots, p_N)] = 0$$

by virtue of the fact that the  $S$ -matrix satisfies the Yang-Baxter equation. (See, eg. [40]- [42].) Hence, the corresponding eigenvectors do not depend on the value of  $p$ .

more explicit equations for the momenta, we need the eigenvalues  $\Lambda(p; p_1, \dots, p_N)$  of the transfer matrix (3.25). For the case of the  $S$ -matrix (3.16), the result is well known [40]–[42],

$$\Lambda(p; p_1, \dots, p_N) = \frac{1}{\prod_{l=1}^N (u - u_l - i)} \left\{ \prod_{l=1}^N (u - u_l + i) \prod_{l=1}^m \left( \frac{u - \lambda_l - \frac{i}{2}}{u - \lambda_l + \frac{i}{2}} \right) + \prod_{l=1}^N (u - u_l) \prod_{l=1}^m \left( \frac{u - \lambda_l + \frac{3i}{2}}{u - \lambda_l + \frac{i}{2}} \right) \right\}, \quad (3.30)$$

where the “auxiliary” Bethe roots  $\lambda_1, \dots, \lambda_m$  satisfy the Bethe ansatz equations

$$\prod_{l=1}^N \frac{\lambda_k - u_l + \frac{i}{2}}{\lambda_k - u_l - \frac{i}{2}} = \prod_{\substack{j=1 \\ j \neq k}}^m \frac{\lambda_k - \lambda_j + i}{\lambda_k - \lambda_j - i}, \quad k = 1, \dots, m. \quad (3.31)$$

Finally, substituting the result (3.30) into (3.29), we obtain

$$\prod_{l=1}^N \frac{u_k - u_l + i}{u_k - u_l - i} \prod_{l=1}^m \frac{u_k - \lambda_l - \frac{i}{2}}{u_k - \lambda_l + \frac{i}{2}} = -e^{ip_k L}, \quad k = 1, \dots, N. \quad (3.32)$$

The coupled set of equations (3.31) and (3.32) are the sought-after (asymptotic) Bethe equations for a system of  $N$  particles on a ring of length  $L$  with the two-particle (asymptotic)  $S$ -matrix (3.16).

### 3.3 AdS/CFT

We are finally ready to address the AdS/CFT case, albeit only sketchily. The arguments of Sec. 3.2 leading to (3.29) carry through essentially unchanged.<sup>10</sup> The difficult step is determining the eigenvalues of the transfer matrix. Whereas for the  $4 \times 4$   $S$ -matrix (3.16) the result (3.30) is easily obtained by algebraic Bethe ansatz, for the larger AdS/CFT  $S$ -matrix (2.35), (2.36) a more general procedure (namely, *nested* algebraic Bethe ansatz) is required [11]. Alternatively, the result can be obtained by nested coordinate Bethe ansatz [3, 12] or by analytic Bethe ansatz [4]. In this way, one can derive the  $AdS_5/CFT_4$  asymptotic Bethe equations which were first conjectured in [10]. In terms of the compact notation introduced in [43], these equations are given by

$$U_0 = 1, \quad U_j(x_{j,k}) \prod_{\substack{j'=1 \\ (j',k') \neq (j,k)}}^7 \prod_{k'=1}^{K_{j'}} \frac{u_{j,k} - u_{j',k'} + \frac{i}{2} M_{j,j'}}{u_{j,k} - u_{j',k'} - \frac{i}{2} M_{j,j'}} = 1, \quad j = 1, \dots, 7, \quad (3.33)$$

<sup>10</sup>It is convenient to work in a graded formalism, where certain minus signs appear. [11]



and finite-size effects via thermodynamic Bethe ansatz (reviewed in [46]). A certain Drinfeld twist of this  $S$ -matrix, together with  $c$ -number diagonal twists of the boundary conditions, lead [47] to the deformed Bethe equations of Beisert and Roiban [43, 48].

The  $su(2|2)$   $S$ -matrix of  $AdS_5/CFT_4$  also plays an important role in determining the  $S$ -matrix of  $AdS_4/CFT_3$  [44] (see also [49]). Indeed, the scattering matrices for the two types of particles (“solitons” and “antisolitons”) again have the same  $su(2|2)$  matrix structure; the main difference with respect to the  $AdS_5/CFT_4$  case is in the scalar factors, which satisfy new crossing relations. As already noted, this  $S$ -matrix leads to the all-loop BAEs conjectured in [45].

## Acknowledgments

We thank N. Beisert for his helpful comments. This work was supported in part by KRF-2007-313-C00150 and WCU grant R32-2008-000-10130-0 (CA), and by the National Science Foundation under Grants PHY-0554821 and PHY-0854366 (RN).

## References

- [1] A. B. Zamolodchikov and Al. B. Zamolodchikov, “Factorized  $S$  matrices in two-dimensions as the exact solutions of certain relativistic quantum field models,” *Ann. Phys.* **120**, 253 (1979).
- [2] M. Staudacher, “The factorized  $S$ -matrix of CFT/AdS,” *JHEP* **0505**, 054 (2005) [arXiv:hep-th/0412188].
- [3] N. Beisert, “The  $su(2|2)$  dynamic  $S$ -matrix,” *Adv. Theor. Math. Phys.* **12**, 945 (2008) [arXiv:hep-th/0511082].
- [4] N. Beisert, “The Analytic Bethe Ansatz for a Chain with Centrally Extended  $su(2|2)$  Symmetry,” *J. Stat. Mech.* **0701**, P017 (2007) [arXiv:nlin/0610017].
- [5] R. A. Janik, “The  $AdS_5 \times S^5$  superstring worldsheet  $S$ -matrix and crossing symmetry,” *Phys. Rev.* **D73**, 086006 (2006) [arXiv:hep-th/0603038].
- [6] G. Arutyunov and S. Frolov, “On  $AdS_5 \times S^5$  string  $S$ -matrix,” *Phys. Lett.* **B639**, 378 (2006) [arXiv:hep-th/0604043].
- [7] N. Beisert, R. Hernandez and E. Lopez, “A crossing-symmetric phase for  $AdS_5 \times S^5$  strings,” *JHEP* **0611**, 070 (2006) [arXiv:hep-th/0609044].
- [8] N. Beisert, B. Eden and M. Staudacher, “Transcendentality and crossing,” *J. Stat. Mech.* **0701**, P021 (2007) [arXiv:hep-th/0610251].
- [9] G. Arutyunov, S. Frolov and M. Zamaklar, “The Zamolodchikov-Faddeev algebra for  $AdS_5 \times S^5$  superstring,” *JHEP* **0704**, 002 (2007) [arXiv:hep-th/0612229].

- [10] N. Beisert and M. Staudacher, “Long-range  $PSU(2, 2|4)$  Bethe ansätze for gauge theory and strings,” *Nucl. Phys.* **B727**, 1 (2005) [arXiv:hep-th/0504190].
- [11] M. J. Martins and C.S. Melo, “The Bethe ansatz approach for factorizable centrally extended  $S$ -matrices,” *Nucl. Phys.* **B785**, 246 (2007) [arXiv:hep-th/0703086].
- [12] M. de Leeuw, “Coordinate Bethe Ansatz for the String  $S$ -Matrix,” *J. Phys.* **A40**, 14413 (2007) [arXiv:0705.2369].
- [13] T. McLoughlin, “Review of AdS/CFT Integrability, Chapter II.2: Quantum Strings in  $AdS_5 \times S^5$ ,” arXiv:1012.3987 [hep-th].
- [14] M. Magro, “Review of AdS/CFT Integrability, Chapter II.3: Sigma Model, Gauge Fixing,” arXiv:1012.3988 [hep-th].
- [15] J. A. Minahan and K. Zarembo, “The Bethe-Ansatz for  $\mathcal{N} = 4$  Super Yang-Mills,” *JHEP* **0303**, 013 (2003) [arXiv:hep-th/0212208].
- [16] D. Berenstein and S. E. Vázquez, “Integrable open spin chains from giant gravitons,” *JHEP* **0506**, 059 (2005) [arXiv:hep-th/0501078].
- [17] A. Rej, “Review of AdS/CFT Integrability, Chapter I.3: Long-range spin chains,” arXiv:1012.3985 [hep-th].
- [18] B. Sutherland, “A brief history of the quantum soliton with new results on the quantization of the Toda lattice,” *Rocky Mtn. J. Math.* **8**, 431 (1978).
- [19] L.D. Faddeev, “Quantum completely integral models of field theory,” *Sov. Sci. Rev.* **C1**, 107 (1980).
- [20] G. Arutyunov and S. Frolov, “The  $S$ -matrix of String Bound States,” *Nucl. Phys. B* **804**, 90 (2008) [arXiv:0803.4323 [hep-th]].
- [21] P.P. Kulish and N.Yu. Reshetikhin, “Quantum linear problem for the sine-Gordon equation and higher representation,” *J. Sov. Math.* **23**, 2435 (1983).
- [22] A.B. Zamolodchikov, “Fractional-spin integrals of motion in perturbed conformal field theory,” in *Fields, Strings and Quantum Gravity*, eds. H. Guo, Z. Qiu and H. Tye, (Gordon and Breach, 1989).
- [23] D. Bernard and A. Leclair, “Quantum group symmetries and nonlocal currents in 2-D QFT,” *Commun. Math. Phys.* **142**, 99 (1991).
- [24] A. Santambrogio and D. Zanon, “Exact anomalous dimensions of  $N = 4$  Yang-Mills operators with large R charge,” *Phys. Lett. B* **545**, 425 (2002) [arXiv:hep-th/0206079].
- [25] P. Vieira and D. Volin, “Review of AdS/CFT Integrability, Chapter III.3: The dressing factor,” arXiv:1012.3992 [hep-th].

- [26] B. S. Shastry, “Exact Integrability of the One-Dimensional Hubbard Model,” *Phys. Rev. Lett.* **56**, 2453 (1986).
- [27] B. S. Shastry, “Decorated star-triangle relations and exact integrability of the one-dimensional Hubbard model,” *J. Stat. Phys.* **50**, 57 (1988).
- [28] N. Dorey, “Magnon bound states and the AdS/CFT correspondence,” *J. Phys.* **A39**, 13119 (2006) [arXiv:hep-th/0604175].
- [29] H.Y. Chen, N. Dorey and K.Okamura, “On the scattering of magnon boundstates,” *JHEP* **0611**, 035 (2006) [arXiv:hep-th/0608047].
- [30] N. Beisert, “The  $S$ -Matrix of AdS/CFT and Yangian Symmetry,” *PoS(SOLVAY)* **002** (2006) [arXiv:0704.0400].
- [31] A. Torrielli, “Review of AdS/CFT Integrability, Chapter VI.2: Yangian Algebra,” arXiv:1012.4005 [hep-th].
- [32] M. de Leeuw, “Bound States, Yangian Symmetry and Classical r-matrix for the  $AdS_5 \times S^5$  Superstring,” *JHEP* **0806**, 085 (2008) [arXiv:0804.1047 [hep-th]].
- [33] G. Arutyunov, M. de Leeuw and A. Torrielli, “The Bound State  $S$ -Matrix for  $AdS_5 \times S^5$  Superstring,” *Nucl. Phys. B* **819**, 319 (2009) [arXiv:0902.0183 [hep-th]].
- [34] R.A. Janik, “Review of AdS/CFT Integrability, Chapter III.5: Lüscher corrections,” arXiv:1012.3994 [hep-th].
- [35] C.N. Yang, “Some exact results for the many body problems in one dimension with repulsive delta function interaction,” *Phys. Rev. Lett.* **19**, 1312 (1967).
- [36] M. Gaudin, “Un système à une dimension de fermions en interaction ,” *Phys. Lett.* **A24**, 55 (1967).
- [37] M. Gaudin, *La fonction d'onde de Bethe* (Masson, 1983).
- [38] N. Andrei, K. Furuya and J. H. Lowenstein, “Solution Of The Kondo Problem,” *Rev. Mod. Phys.* **55**, 331 (1983).
- [39] G. Arutyunov and S. Frolov, “On String S-matrix, Bound States and TBA,” *JHEP* **0712**, 024 (2007) [arXiv:0710.1568 [hep-th]].
- [40] L. D. Faddeev, “How Algebraic Bethe Ansatz works for integrable model,” [arXiv:hep-th/9605187].
- [41] R. I. Nepomechie, “A Spin Chain Primer,” *Int. J. Mod. Phys. B* **13**, 2973 (1999) [arXiv:hep-th/9810032].
- [42] M. Staudacher, “Review of AdS/CFT Integrability, Chapter III.1: Bethe Ansätze and the R-Matrix Formalism,” arXiv:1012.3990 [hep-th].

- [43] N. Beisert and R. Roiban, “Beauty and the twist: The Bethe ansatz for twisted  $\mathcal{N} = 4$  SYM,” *JHEP* **0508**, 039 (2005) [arXiv:hep-th/0505187].
- [44] C. Ahn and R.I. Nepomechie, “ $\mathcal{N} = 6$  super Chern-Simons theory  $S$ -matrix and all-loop Bethe ansatz equations,” *JHEP* **0809**, 010 (2008) [arXiv:0807.1924 [hep-th]].
- [45] N. Gromov and P. Vieira, “The all loop AdS4/CFT3 Bethe ansatz,” *JHEP* **0901**, 016 (2009) [arXiv:0807.0777 [hep-th]].
- [46] Z. Bajnok, “Review of AdS/CFT Integrability, Chapter III.6: Thermodynamic Bethe Ansatz,” arXiv:1012.3995 [hep-th].
- [47] C. Ahn, Z. Bajnok, D. Bombardelli and R. I. Nepomechie, “Twisted Bethe equations from a twisted S-matrix,” [arXiv:1010.3229 [hep-th]].
- [48] K. Zoubos, “Review of AdS/CFT Integrability, Chapter IV.2: Deformations, Orbifolds and Open Boundaries,” arXiv:1012.3998 [hep-th].
- [49] T. Klose, “Review of AdS/CFT Integrability, Chapter IV.3:  $\mathcal{N} = 6$  Chern-Simons and Strings on  $AdS_4 \times CP^3$ ,” arXiv:1012.3999 [hep-th].



# Review of AdS/CFT Integrability, Chapter III.3: The dressing factor

PEDRO VIEIRA<sup>a</sup>, DMYTRO VOLIN<sup>b</sup>

<sup>a</sup> *Perimeter Institute for Theoretical Physics,  
Waterloo, Ontario N2L 2Y5 , Canada*

<sup>b</sup> *Department of Physics, The Pennsylvania State University,  
University Park, PA 16802, USA*

pedrovieira AT gmail.com , dvolin AT psu.edu

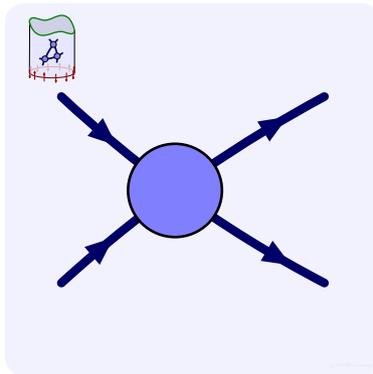

**Abstract:** We review the construction of the AdS/CFT dressing factor, its analytic properties and several checks of its validity.

## 1 Introduction

The two-body S-matrix is the main figure in the solution of 1+1 dimensional integrable theories. *In principle*, given this object there is a more or less well defined route to compute the asymptotic and even the finite-size spectrum of the theory.

Typically, particles have polarizations and therefore the S-matrix has a nontrivial matrix structure. The various ratios of the S-matrix elements give us the relative weights of different scattering processes in the same theory. These ratios are mostly kinematic and highly constrained by the symmetries of the system. For integrable models, symmetry together with the condition of factorized scattering is usually enough to constraint completely the matrix structure of the S-matrix up to an overall scalar factor called *dressing factor*. This factor contains much more dynamical information and is therefore considerably harder to derive. Usually, to find the correct dressing factor, one needs to consider unitarity and crossing equations supplemented by the knowledge of the exact bound state spectrum.

In this review we will study the dressing factor for a very interesting integrable model which appears in the spectrum problem of planar AdS/CFT [1, 2].

We start by considering (section 2) a warm-up toy model, the  $O(4)$  sigma model, which will be quite instructive. Then we move to the AdS/CFT system (sections 3 and 4). Our logical flow will be roughly the opposite of the chronological one. We will start by solving directly the crossing relation in section 3. Then, in section 4, we will consider several rewritings and expansions of the dressing factor, including the Beisert-Eden-Staudacher solution [3, 4] and several weak and strong coupling expansions. Along the way we will describe analytical properties and remarkable checks of the AdS/CFT dressing factor which established its correctness beyond reasonable doubt. In section 5 we present some concluding remarks.

## 2 Dressing factor in the $O(4)$ sigma model

The  $O(4)$  sigma model in two dimensions is an integrable relativistic model where particles have energy and momentum given by

$$\epsilon(\theta) = m \cosh(\pi\theta) , \quad p(\theta) = m \sinh(\pi\theta) , \quad (2.1)$$

where  $\theta$  is the so called rapidity. Lorentz boosts amount to simple translations in  $\theta$ . Hence, the  $O(4)$  Lorentz invariant two-body S-matrix must be a function of the difference of rapidities  $\theta = \theta_1 - \theta_2$  of the two particles being scattered,  $\hat{S}_{2 \rightarrow 2}(\theta_1, \theta_2) = \hat{S}(\theta)$ . The hat emphasizes that this object is a *matrix* since the scattered particles have isotopic degrees of freedom. Since the model is integrable the matrix structure of the S-matrix can be fixed from the symmetry of the problem together with the Yang-Baxter triangular relation [5]. One finds

$$\left[ \hat{S}(\theta) \right]_{hk}^{jl} = \sigma^2(\theta) \left( \frac{i\theta}{(\theta - i)^2} \delta_{hk} \delta_{jl} + \frac{\theta}{\theta - i} \delta_{hj} \delta_{lk} - \frac{i}{\theta - i} \delta_{hl} \delta_{jk} \right) . \quad (2.2)$$

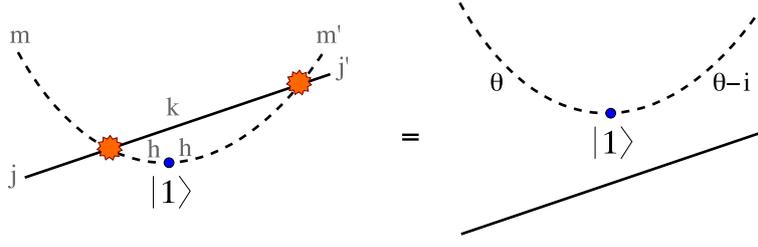

**Figure 1:** Scattering of a physical particle (solid line) with a composite of particle/antiparticle of zero total zero charges (dashed line) should be inconsequential [6]. This picture translates into formula (2.4).

The overall *dressing factor*  $\sigma^2(\theta)$  is however left undetermined since it drops out of Yang-Baxter. This *function* is constrained by imposing extra physical conditions: crossing symmetry and unitarity. Let us adapt a nice argument by Beisert [6] to derive the implications of crossing symmetry. We construct a composite singlet state with one particle and one antiparticle,

$$|1\rangle \propto \sum_{h=1}^4 |\{h, \theta\}, \{h, \theta - i\}\rangle. \quad (2.3)$$

The second particle has the same color as the first particle and the opposite energy and momenta since  $\theta \rightarrow \theta - i$  flips these two quantities. The singlet state (2.3) is therefore a spurious state which has zero color, momentum and energy. Physically we think of it as a virtual pair of particle and anti-particle created by a vacuum fluctuation. Scattering of a physical particle through this bound state should be inessential, see figure 1. Algebraically, the condition depicted in this figure translates into

$$\sum_{h=1}^4 \sum_{k=1}^4 [\hat{S}(\theta)]_{jh}^{km} [\hat{S}(\theta - i)]_{kh}^{j'm'} = \delta_j^{j'} \delta_{mm'}. \quad (2.4)$$

This condition then implies  $\sigma^2(\theta)\sigma^2(\theta - i)\theta^2/(\theta + i)^2 = 1$  or

$$\sigma(\theta + i/2)\sigma(\theta - i/2) = \frac{\theta - i/2}{\theta + i/2}. \quad (2.5)$$

This is the crossing relation [5]. We will now provide two derivations of the so-called *minimal solution* to the equation (2.5).

### First derivation

We start by taking the logarithm and derivative of the crossing relation (2.5):

$$K^+ + K^- = \frac{1}{2\pi i} \left( \frac{1}{\theta - i/2} - \frac{1}{\theta + i/2} \right), \quad (2.6)$$

where  $K \equiv \frac{1}{2\pi i} \frac{d}{d\theta} \log \sigma(\theta)$  and  $f^\pm = f(\theta \pm i/2)$ . Next we go to Fourier space,

$$\mathcal{F}(K^\pm)(\omega) = \int_{-\infty}^{\infty} d\theta e^{i\theta\omega} K(\theta \pm i/2) = e^{\pm\omega/2} \int_{-\infty \pm i/2}^{\infty \pm i/2} d\theta e^{i\theta\omega} K(\theta). \quad (2.7)$$

At this point we need some physical input about the particle content of the  $O(4)$  sigma model [5]. Since there are no bound states,  $\sigma(\theta)$  should not have poles in the strip  $-1/2 < \text{Im}(\theta) < 1/2$ . Unitarity  $\hat{S}(\theta)\hat{S}(-\theta) = \mathbb{I}$  yields  $\sigma^2(\theta)\sigma^2(-\theta) = 1$  which implies the absence of zeros in the same strip. The absence of poles and zeros in this strip is often called the *minimality condition*.

Assuming this condition to hold we can solve (2.5) uniquely. Indeed, since  $K(\theta)$  has no singularities in the strip  $-1/2 < \text{Im}(\theta) < 1/2$  we can deform the integral contour (2.7) back to the real axis and conclude that  $\mathcal{F}(K^\pm)(\omega) = e^{\pm\omega/2} \mathcal{F}(K)(\omega)$ . The Fourier transform of (2.6) then yields

$$\mathcal{F}(K)(\omega) = \frac{e^{-|\omega|/2}}{2 \cosh(\omega/2)}. \quad (2.8)$$

The Kernel  $K(\theta)$  is now trivially computed as

$$K(\theta) = \mathcal{F}^{-1} \left[ \frac{e^{-|\omega|/2}}{2 \cosh(\omega/2)} \right] = \frac{1}{2\pi i} \frac{d}{d\theta} \log \left[ \frac{1 \Gamma(1 - \frac{\theta}{2i}) \Gamma(\frac{1}{2} + \frac{\theta}{2i})}{i \Gamma(1 + \frac{\theta}{2i}) \Gamma(\frac{1}{2} - \frac{\theta}{2i})} \right]. \quad (2.9)$$

The quantity inside the logarithm can then be identified with the dressing factor  $\sigma(\theta)$ . To fix the constant of integration we imposed the condition

$$\sigma^2(0) = -1. \quad (2.10)$$

This constraint simply states that there cannot be two identical particles in the theory, which is indeed the case for the  $O(4)$  sigma model.

## Second derivation

Let us redo the above derivation avoiding passing to Fourier space. The argumentation now will be admittedly more involved but it is also the most useful for the analogy with solving the AdS/CFT crossing equation. First, the crossing equation (2.5) can be re-written as

$$\sigma^{D+D^{-1}} = \theta^{-(D-D^{-1})}, \quad (2.11)$$

where  $D = e^{\frac{i}{2}\partial_\theta}$  is the shift operator,  $Df(\theta) \equiv f(\theta + i/2)$ , and  $f^{\mathcal{O}[D]} \equiv \exp(\mathcal{O}[D] \log f)$ . Formally we might be tempted to solve (2.11) as

$$\sigma(\theta) = \theta^{f[D]} \quad \text{where} \quad f[D] = -\frac{D - D^{-1}}{D + D^{-1}}. \quad (2.12)$$

However, we have to interpret this expression with care. E.g. if we naively expand  $f[D] = 1 + 2 \sum_{n=1}^{\infty} (-1)^n D^{2n}$  we see that  $\sigma^2(0) = 0$ . Similarly, if we expand this operator at *large*  $D$  as  $f[D] = -1 - 2 \sum_{n=1}^{\infty} (-1)^n D^{-2n}$  we get  $1/\sigma^2(0) = 0$ . In both cases we face an obvious contradiction with the minimality condition. The only possible interpretation of (2.12) which is consistent with the minimality condition and (2.10) is

$$f[D] = \frac{D^{-2}}{1 + D^{-2}} - \frac{D^2}{1 + D^2} \equiv \sum_{n=1}^{\infty} (-1)^n D^{2n} - \sum_{n=1}^{\infty} (-1)^n D^{-2n}, \quad (2.13)$$

so that

$$\begin{aligned} \sigma(\theta) &= \exp \left( \sum_{n=1}^{\infty} (-1)^n D^{2n} \log(\theta) - \sum_{n=1}^{\infty} (-1)^n D^{-2n} \log(\theta) \right) \\ &= c_{reg} \prod_{n=0}^{\infty} \frac{(\theta + 2ni)(\theta - (2n+1)i)}{(\theta - 2ni)(\theta + (2n+1)i)} = -c_{reg} \frac{\Gamma(1 - \frac{\theta}{2i}) \Gamma(\frac{1}{2} + \frac{\theta}{2i})}{\Gamma(1 + \frac{\theta}{2i}) \Gamma(\frac{1}{2} - \frac{\theta}{2i})}. \end{aligned} \quad (2.14)$$

The sums in the exponent in (2.14) are divergent and therefore need to be regularized. The simplest way to do regularization is by computing the derivative of these sums and then integrating back. This procedure introduces an unknown constant of integration:  $c_{reg}$ . Using (2.10) we fix it to  $c_{reg} = i$ . We recover precisely what we derived before in (2.9).

This derivation of the dressing factor is almost the same as the first one. Indeed, in both cases, to obtain regular expressions we need to take a derivative of the logarithm of the crossing equation. More importantly, the shift operator  $D = e^{\frac{i}{2}\partial_\theta}$  is Fourier transformed to  $\mathcal{F}(\mathcal{D}) = e^{-\frac{i}{2}\omega}$ . However, one advantage of using the second derivation is that (2.14) explicitly highlights the analytic structure of the solution, in particular by looking at its zeros and poles we immediately recognize the ratio of gamma functions. In the case of the AdS/CFT, when the analytical structure is more involved, use of shift operators instead of their Fourier transforms is even more preferable.

Let us comment on a trivial feature of the above derivations. The (logarithm of the) dressing factor is singular for  $\theta = \pm i$ . This means that for practical purposes, it was a good idea to shift from the original functional equation  $\sigma(\theta)\sigma(\theta - i) = \dots$  to the relation (2.5) of the form  $\sigma(\theta + i/2)\sigma(\theta - i/2) = \dots$ . It avoids the burden of carrying around several  $i0$ 's in the above derivations.

### 3 Crossing equation

The AdS/CFT system is considerably more complicated than the  $O(4)$  sigma model described above. However many features have a clear analogue in both models. The energy and momenta of the particle excitations, which are also called magnons, are now given by [7, 8, 6]

$$e^{ip} = \frac{x^+}{x^-}, \quad E = ig \left( x^- - \frac{1}{x^-} - x^+ + \frac{1}{x^+} \right), \quad (3.1)$$

where  $x^\pm \equiv x(u \pm i/2)$ ,  $u/g \equiv x(u) + 1/x(u)$  and  $g \equiv \sqrt{\lambda}/4\pi$ . The variable  $u$  is the Bethe rapidity and is the direct analogue of  $\theta$  in the  $O(4)$  sigma model;  $x(u)$  is the so called Zhukovsky variable. Unless otherwise stated, we choose the branch of the Zhukovsky variables such that  $|x^\pm(u)| > 1$ . This is the so called physical region, the one with a good  $g \rightarrow 0$  limit. We represent the cuts of the functions  $x^\pm(u)$  as uniting the corresponding branch-points horizontally in the complex  $u$  plane, see figure 2.

The two-body scattering matrix of the AdS/CFT system,  $\hat{S} = \hat{S}_0 \times \sigma^{-2}$ , depends on the rapidities of the particles being scattered and on the 't Hooft coupling. As in the previous example, we have a matrix part  $\hat{S}_0$  which can be fixed by symmetry and Yang-Baxter – see review [2] and references therein – and a scalar *dressing factor*  $\sigma^2$  which is the main focus of this review.

To avoid possible ambiguities let us mention that we use a definition of  $\sigma$  such that the Beisert-Staudacher Bethe equations [9, 6] in the  $SU(2)$  sector read  $e^{ip_k L} = \prod_{j \neq k} \frac{u_k - u_j + i}{u_k - u_j - i} \sigma(u_k, u_j)^2$ .

In contradistinction with the  $O(4)$  sigma model, the AdS/CFT integrable system *does* have infinitely many bound states. The  $n$ -th bound state is a composite state of  $n$  elementary magnons with rapidities [10]

$$u + ij, \quad \text{with} \quad j = -\frac{n-1}{2}, \dots, \frac{n-1}{2}, \quad (3.2)$$

separated by  $i$  and with real part  $u$ . The energy and momentum of the bound state are the sum of energies and momenta of the individual constituents with the rapidities (3.2). The result is again (3.1) but with  $x^\pm$  replaced by  $x(u \pm in/2)$ . The existence of bound states is reflected in a simple pole of the scattering matrix at the point  $u = v - i$ . By convention, this pole is included in  $\hat{S}_0$ . Hence  $\sigma^2(u, v)$  should be regular at this point.

As usual in integrable models, the most powerful tool to fix  $\sigma^2(u, v)$  is by using crossing symmetry. The AdS/CFT generalized crossing equation was first proposed by Janik [11] and is presented in (3.4) below. As discussed in section 2, one can motivate this relation by finding a singlet particle/antiparticle state  $|1\rangle$  with zero charges and imposing trivial scattering of this object with physical particles [6]. Yet another derivation of crossing is [12].

To be able to discuss the crossing equation we need to explain what the *particle*  $\rightarrow$  *antiparticle* transformation is for the AdS/CFT system. This transformation should be understood as the following monodromy in  $u$ . We start with some  $x^\pm$  at real  $u$ . The energy and momentum following from (3.1) are then real. Next, we take  $u$  into the complex plane: first we cross the cut of  $x^+(u)$  (in the lower half plane), then the cut of  $x^-(u)$  (in the upper half plane) and finally we come back to the original value of  $u$ , see figure 2.<sup>1</sup> Of course, since we crossed cuts we are now at some other sheet; to stress the difference let us denote the point on the different sheet by  $\mathbf{u}$ . Since we crossed the cuts of  $x^\pm$  we have  $x^\pm(\mathbf{u}) = 1/x^\pm(u)$  and therefore  $E(\mathbf{u}), p(\mathbf{u}) = -E(u), -p(u)$  as expected

<sup>1</sup>Another interesting transformation can be considered when we only cross the  $x^-$  cut. If we now compute the energy and momenta from (3.1) at real  $u$  we see that they are purely imaginary. This is the so called mirror kinematics where we should identify  $p_{mirror} = iE$  and  $E_{mirror} = ip$ , see [13, 14] and review [15] for more details.

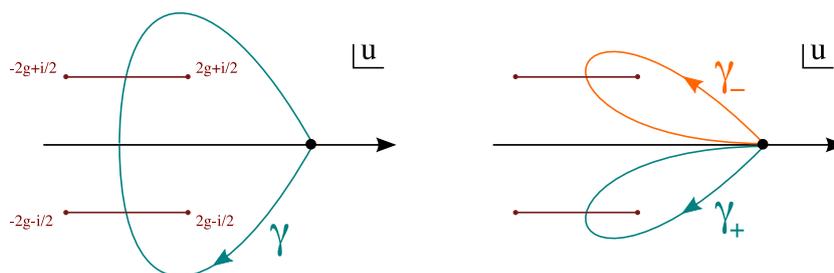

**Figure 2:** Analytical continuation contours used in the crossing equation. The horizontal segments corresponds to the choice of branch-cuts for  $x^\pm(u) = x(u \pm i/2)$  such that  $|x(u)| > 1$ . The upper (lower) cut is the cut of  $x^-$  ( $x^+$ ).

for a particle to antiparticle transformation. In sum, we have,

$$x_{\text{antiparticle}}^\pm = \frac{1}{x_{\text{particle}}^\pm}. \quad (3.3)$$

Note however that it is important to specify the path  $\gamma$  under which  $x^\pm \rightarrow 1/x^\pm$  to properly define this transformation. The crossing relation then reads

$$\sigma(u, v) \sigma^\gamma(u, v) = \frac{1 - \frac{1}{x^+ y^+}}{1 - \frac{x^-}{y^-}} \frac{1 - \frac{x^-}{y^+}}{1 - \frac{1}{x^+ y^-}}, \quad (3.4)$$

where  $\sigma^\gamma(u, v)$  means the analytical continuation of  $\sigma(u, v)$  in the  $u$  variable over the contour  $\gamma$ . We will use  $x^\pm \equiv x^\pm(u)$  and  $y^\pm \equiv x^\pm(v)$  in this review.

### Assumptions on the analytical structure

The crossing equation (3.4) admits infinitely many solutions. To single out the correct one we need additional physically motivated constraints on the analytical structure of the dressing factor. This is the analogue of the minimality condition for the  $O(4)$  case discussed in section 2.

1. **Bound states and simple poles/zeros.** The position of simple poles in the S-matrix should correctly reproduce the structure of bound states. The only bound states in the AdS/CFT system are the (3.2) described above. These states are already accounted for by the simple pole of  $\hat{S}_0$ . We therefore require that  $\sigma^2(u, v)$  does not have simple poles. Unitarity then excludes simple zeros as well.<sup>2</sup>
2. **Poles/zeros of higher degree.** An exceptional feature of  $1 + 1d$  theories is that the S-matrix can contain poles of higher degree associated with multiparticle exchanges. In [16] Dorey, Hofman, and Maldacena showed that the exchange of pairs of composite states should lead to double poles in the AdS/CFT scattering

<sup>2</sup>In the  $O(4)$  case we only required the absence of poles and zeros in the physical strip due to the periodicity properties of  $p$  as a function of  $\theta$ . In the AdS/CFT case there is no such periodicity and we should require the absence of poles everywhere.

matrix at  $u - v = im$  for integer  $m$ <sup>3</sup>. Since the matrix factor  $\hat{S}_0$  does not contain such double poles we should allow for their presence in the dressing factor. These should be, however, the only poles of  $\sigma^2(u, v)$ . Using unitarity, we see that the zeros of  $\sigma^2(u, v)$  are double zeros located at  $u - v = -im$ . These double poles (and zeros) are called DHM poles (and zeros). Note that DHM poles will inevitably appear in the solution of crossing. Therefore we can reformulate our requirement as a demand to pick up solution with the simplest possible pole/zero structure.

3. **Branch points.** In the  $O(4)$  sigma model, the S-matrix, when thought of as a function of the kinematic invariants, has branch cut singularities at particle creation thresholds. The rapidity  $\theta$  uniformizes the  $S$ -matrix rendering it meromorphic. In the AdS/CFT system we are not able to introduce such uniformizing variable. The best we can do is to require that the structure of branch points is as simple as possible: only the branch points which are explicitly required by crossing equations are allowed in  $\sigma(u, v)$ . We will see that this criterium leads to infinitely many square-root branch points at the points  $u = \pm 2g \pm in$  for half-integer  $n$ , i.e. when  $x(u \mp in) = \pm 1$ .
4.  **$\chi$ -decomposition** The dressing factor  $\sigma(u, v) = e^{i\theta(u, v)}$  can be decomposed as

$$\theta(u, v) = \chi(x^+, y^-) - \chi(x^-, y^-) - \chi(x^+, y^+) + \chi(x^-, y^+), \quad (3.5)$$

where  $\chi(x, y)$  is antisymmetric,  $\chi(x, y) = -\chi(y, x)$ , and  $\theta(u, v)$  is the *phase shift*. This form is the most general expression we should expect for long-range integrable spin chains [18]. Hence, from the  $\mathcal{N} = 4$  point of view it is perfectly justified. More precisely this form is a direct consequence of the decomposition of  $\theta(u, v)$  in terms of higher conserved charges (4.2) which will be reviewed in more detail in section 4. The higher charge decomposition property was realized in [17, 18], while the representation (3.5) appeared in [41]. Further evidence for this decomposition comes from considering the scattering of bound-states, see point 6 below.

5. **Asymptotics at infinity.** As  $x \rightarrow \infty$  we expect  $\chi(x, y)$  to approach some constant value. Since infinite  $x$  corresponds to zero momenta this will ensure that  $\sigma^2(p = 0, p') \rightarrow 1$ , i.e. particles scatter trivially with zero momentum particles. This should be imposed since excitations with zero momenta correspond to global symmetry transformations of the state and should therefore have an irrelevant effect.
6. **Analyticity of  $\chi(x, y)$  in the physical domain  $|x| > 1$ .** In points 2 and 3 above we anticipated the existence of DHM poles and of square root singularities at  $u = v + in$  and  $u = \pm 2g \pm in$  respectively. So, what we want to argue in this point is that these singularities should not be present in the physical sheet  $|x(u)| > 1$ . This is the trickiest point and requires a somehow more involved argument. The basic idea is that if these singularities would be present for  $|x| > 1$  then they would lead to unphysical singularities in the description of the scattering of bound states.

---

<sup>3</sup>The possible values of  $m$  are in general restricted depending on what Riemann sheets of  $\sigma(u, v)$  we are located [16]. We do not need this restriction; it will naturally come out.

To show this we have to consider the phase shift when scattering a  $n$ -th with a  $m$ -th bound state with real rapidities  $u$  and  $v$ . The total phase shift is the sum of the phase shifts acquired by each of the  $n$  constituents of the first bound state when scattered through each of the  $m$  constituents of the second bound state. I.e.  $\theta_{n,m}(u, v) = \sum_{j=-\frac{n-1}{2}}^{\frac{n-1}{2}} \sum_{k=-\frac{m-1}{2}}^{\frac{m-1}{2}} \theta(u + ij, u + ik)$ . Using (3.5) we simplify this sum to [19]<sup>4</sup>

$$\begin{aligned} \theta_{n,m}(u, v) &= \chi(x(u + in/2), x(v + im/2)) - \chi(x(u - in/2), x(v + im/2)) \\ &\quad - \chi(x(u + in/2), x(v - im/2)) + \chi(x(u - in/2), x(v - im/2)). \end{aligned} \quad (3.6)$$

The scattering matrix  $\hat{S}(u, v)$  should be analytic for real  $u$  and  $v$  provided we are in the physical domain  $|x(u \pm in/2)| > 1$ . If the square root cuts or the DHM poles were present in the physical region of  $\chi(x, y)$  they would clearly lead to singularities in the real axis for some  $n$ -th bound states (of even  $n$ ). Hence they must be absent.

### Solution

In this derivation we follow [20] closely. The crossing relation (3.4) is valid on the infinite genus Riemann surface [4] where  $u$  lives. Instead of evaluating it at a real  $u$  in the physical sheet where  $|x^\pm(u)| > 1$  let us cross the cut of  $x^-(u)$  and return back to the real  $u$  axis. This means that we should flip  $x^- \rightarrow 1/x^-$  in the right hand side of (3.4) which becomes<sup>5</sup>

$$\sigma^{\gamma^-}(u, v)\sigma^{\gamma^+}(u, v) = \frac{1 - \frac{1}{x^+y^+}}{1 - \frac{1}{x^-y^-}} \frac{1 - \frac{1}{x^-y^+}}{1 - \frac{1}{x^+y^-}}, \quad (3.7)$$

where  $\sigma^{\gamma^\pm}(u, v)$  is the analytical continuation of  $\sigma(u, v)$  through the  $u$  contour which crosses the cut of  $x^\pm$  so that  $x^\pm \rightarrow 1/x^\pm$  respectively, see figure 2. Of course, the contour  $\gamma$  described above (3.4) is nothing but  $\gamma = \gamma^+ + (\gamma^-)^{-1}$ . Next we notice that  $\sigma^{\gamma^-} = \frac{\sigma_1(x^+, v)}{\sigma_1(1/x^-, v)}$  and  $\sigma^{\gamma^+} = \frac{\sigma_1(1/x^+, v)}{\sigma_1(x^-, v)}$  where  $\sigma_1(x, v) \equiv e^{i\chi(x, y^-) - i\chi(x, y^+)}$ , see decomposition (3.5). By plugging these expressions into the crossing relations we get

$$\frac{\sigma_1(x^+, v)\sigma_1(1/x^+, v)}{\sigma_1(x^-, v)\sigma_1(1/x^-, v)} = \frac{1 - \frac{1}{x^+y^+}}{1 - \frac{1}{x^-y^-}} \frac{1 - \frac{1}{x^-y^+}}{1 - \frac{1}{x^+y^-}}. \quad (3.8)$$

As in the  $O(4)$  sigma model, it is useful to manipulate expressions by using the shift operator  $D = e^{\frac{i}{2}\partial_u}$ . The shorthand notation for (3.8) reads

$$(\sigma_1(x, v)\sigma_1(1/x, v))^{D-D^{-1}} = \left( \frac{x - \frac{1}{y^+}}{x - \frac{1}{y^-}} \right)^{D+D^{-1}}. \quad (3.9)$$

<sup>4</sup>The nice fusion properties of the dressing factor can be seen as further evidence in favor of the composition (3.5)

<sup>5</sup>This more symmetric form of crossing is the analogue of (2.5) where we evaluate the dressing factors at  $\theta \pm i/2$ , see comment at the end of section 2. Similarly to what happens in the  $O(4)$  model, the derivation also simplifies when we consider this more symmetric form.

The use of shift operators in the AdS/CFT system is potentially dangerous due to the presence of the branch points so let us analyse expression (3.9) with care. The right hand side of (3.9) is uniquely defined in the region  $|\operatorname{Re}(u)| > 2g$  if we use the physical choice of cuts for  $x(u)$ , see figure 2. The reason is that if  $|\operatorname{Re}(u)| > 2g$  we never cross the cuts of  $x^+(u)$  or  $x^-(u)$ . Interestingly, the left hand side of (3.9) is not ambiguous at all in the whole strip  $|\operatorname{Im}(u)| < 1/2$ , and in particular on the real axis. Indeed, when we cross the cut of  $x(u)$ , the two terms in the product  $\sigma_1(x, v)\sigma_1(1/x, v)$  become just exchanged, so this product does not have the cut of  $x(u)$ .<sup>6</sup> We conclude that it is safe to use the shift operator for the expression (3.9) at least in the intersection of two domains  $|\operatorname{Re}(u)| > 2g$  and  $|\operatorname{Im}(u)| < 1/2$ . We therefore consider (3.9) in this intersection, solve it, and then analytically continue the solution everywhere.

Formally we can solve (3.9) by<sup>7</sup>

$$\sigma_1(x, v)\sigma_1(1/x, v) = \left( \frac{x - \frac{1}{y^+}}{x - \frac{1}{y^-}} \right)^{f[D]}, \quad (3.10)$$

where

$$f[D] = \frac{D + D^{-1}}{D - D^{-1}}. \quad (3.11)$$

However, to interpret this expression we must give a meaning to this operator.<sup>8</sup> For example, a naive expansion in powers of  $D$  or  $1/D$  leads to  $f[D] = -1 + \mathcal{O}(D)$  or  $f[D] = +1 + \mathcal{O}(1/D)$  respectively. Both expansions must be discarded, because of the  $\mp 1$  terms: the presence of such terms would mean that  $\sigma_1(x, v)\sigma_1(1/x, v)$  has the branch-cuts of  $x(u)$ , however this should not be the case as explained above. The proper interpretation of  $f[D]$  which leads to a function  $\sigma_1(x, v)\sigma_1(1/x, v)$  without a branch cut for  $u \in [-2g, 2g]$  is given by<sup>9</sup>

$$f[D] = \frac{D^{-2}}{1 - D^{-2}} - \frac{D^2}{1 - D^2} \equiv \sum_{n=1}^{\infty} D^{-2n} - \sum_{n=1}^{\infty} D^{2n}. \quad (3.12)$$

The reason is of course the absence of  $D^0$  terms in this expansion. Plugging the definition

<sup>6</sup>Of course, this product might still have cuts of  $x(u + in)$  with nonzero integer  $n$  and this is why we restrict ourselves to the strip  $|\operatorname{Im}(u)| < 1/2$  to be on the safe side.

<sup>7</sup>A priori we could imagine multiplying the right hand side of (3.10) by a zero mode of  $D - D^{-1}$ , i.e. a function  $g(u)$  periodic in  $u$  with period  $i$ . Such functions must however always have poles or zeros. As explained in the previous section, the only allowed poles (zeros) are the DHM poles (zeros). Suppose that  $g(u)$  contains any of DHM poles. Then by periodicity it contains poles at  $u = i\mathbb{Z}$ . But due to unitarity it contains also zeroes in the same positions. Hence  $g(u)$  is a constant which can be set to 1 due to (3.5). Hence (3.10).

<sup>8</sup>This can be almost xeroxed from the discussion of the dressing factor in the  $O(4)$  sigma model in section 2 where we needed to regularize a very similar expression, see (2.14).

<sup>9</sup>Strictly speaking, the expression (3.10) with  $f[D]$  given by (3.12) still needs to be regularized to have a precise meaning. For instance, instead of  $f[D]$  we might consider  $\partial_u^2 f[D]$  and then integrate back. However, the terms that depend on the regularization are canceled out when computing the dressing factor  $\sigma(u, v)$  because of the anti-symmetrization (3.5) over the several  $\chi$  factors.

of  $\sigma_1(x, v)$  in terms of  $\chi(x, y)$  in (3.10) we see that it can be further factorized into

$$e^{i\chi(x,y)+i\chi(1/x,y)} = \left( \frac{x - \frac{1}{y}}{\sqrt{x}} \right)^{-f[D]}. \quad (3.13)$$

The factor  $1/\sqrt{x}$  is irrelevant for  $\sigma_1$  but we insert it to ensure the antisymmetry of  $\chi(x, y)$  with respect to the interchange  $x \leftrightarrow y$ . A direct calculation yields<sup>10</sup>

$$e^{i\chi(x,y)+i\chi(1/x,y)+i\chi(x,1/y)+i\chi(1/x,1/y)} = (u - v)^{-f[D]} = \frac{\Gamma(1 + iu - iv)}{\Gamma(1 - iu + iv)}. \quad (3.14)$$

Now, if we take  $u$  on top of the cut of  $x(u)$  we have  $x(u-i0) = 1/x(u+i0)$ . Similarly for  $v$ . Hence, with an harmless abuse of notation, we can think of (3.14) as a Riemann-Hilbert problem:

$$\chi(u+i0, v+i0)+\chi(u-i0, v+i0)+\chi(u+i0, v-i0)+\chi(u-i0, v-i0) = \frac{1}{i} \log \frac{\Gamma(1 + iu - iv)}{\Gamma(1 - iu + iv)}. \quad (3.15)$$

Needless to say, Riemann-Hilbert problems are much simpler than generic functional equations – such as the original crossing equation – and can be solved by standard methods. In our case the solution is given by

$$\chi(x, y) = \frac{1}{i} K_u \star K_v \star \log \frac{\Gamma(1 + iu - iv)}{\Gamma(1 - iu + iv)}, \quad (3.16)$$

with the kernel  $K$  defined as<sup>11</sup>

$$K_u \star F \equiv \int_{-2g+i0}^{2g+i0} \frac{dw}{2\pi i} \frac{x(u) - \frac{1}{x(u)}}{x(w) - \frac{1}{x(w)}} \frac{1}{w - u} F(w). \quad (3.17)$$

The kernel is engineered to satisfy the following equation<sup>12</sup>:

$$(K_u \star F)(u + i0) + (K_u \star F)(u - i0) = F(u), \quad |u| < 2g. \quad (3.18)$$

The solution (3.16) was chosen among the other possible solutions by the requirement that  $\chi(x, y)$  should be analytic for  $|x| > 1$  and  $\chi(x, y) \rightarrow \text{const}$  as  $x \rightarrow \infty$ . The expression (3.16) can be rewritten in the form proposed in [16] if we rewrite the action of the kernels as an integral in the Zhukovsky plane,

$$(K_u \star F)(u) = \oint_{|z|=1} \frac{dz}{2\pi i} \frac{1}{x - z} F(g(z + 1/z)) - \frac{1}{g} \int_{-2g+i0}^{2g+i0} \frac{dv}{2\pi i} \frac{1}{x(v) - \frac{1}{x(v)}} F(v), \quad (3.19)$$

<sup>10</sup>the logarithm of the right hand side is antisymmetric with respect to  $u \leftrightarrow v$  as it should.

<sup>11</sup>Note that  $x(u) - 1/x(u) = g^{-1}\sqrt{u^2 - 4g^2}$ , so  $K_u$  is the typical kernel used to solve Riemann-Hilbert problems of the form (3.18).

<sup>12</sup>This kernel coincides, after an analytical transformation [21], with the inverse Fourier transform of the sum  $K_0 + K_1$  of the magic kernels in [3]. The relevance of Riemann-Hilbert problem for  $K_u$  was recognized in [21].

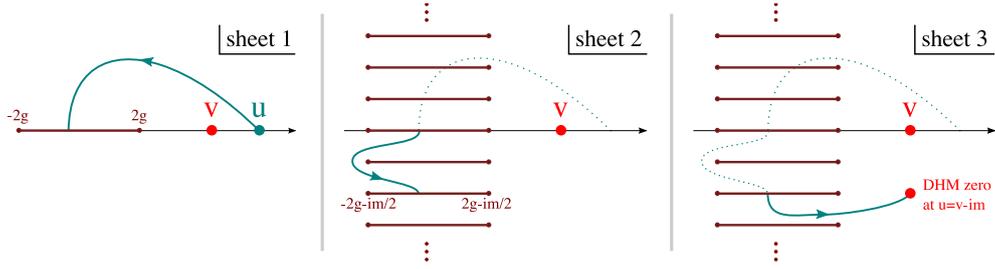

**Figure 3:** Analytical structure of  $e^{i\chi(x,y)}$  as a function of  $u$ .

and notice that the second term does not contribute to the dressing phase once we anti-symmetrize in (3.5). Dropping it, we obtain the DHM representation

$$\chi(x, y) = -i \oint_{|z|=1} \frac{dz}{2\pi i} \oint_{|z'|=1} \frac{dz'}{2\pi i} \frac{1}{x-z} \frac{1}{y-z'} \log \frac{\Gamma[1 + ig(z + \frac{1}{z} - z' - \frac{1}{z'})]}{\Gamma[1 - ig(z + \frac{1}{z} - z' - \frac{1}{z'})]}. \quad (3.20)$$

### Analytical structure at finite coupling

To investigate the analytical structure of  $\chi(x(u), x(v))$  as a function of  $u$  we will use (3.12) to write<sup>13</sup>:

$$i\chi(x(u), x(v)) = \sum_{n \neq 0} \text{sign}(n) K_u \star D^{2n} K_u \star \log(u - v) \quad (3.21)$$

which is valid in the physical domain  $|x(u)| > 1$ . To go to  $|x(u)| < 1$  we must cross the cut  $u \in [-2g, 2g]$ . Using (3.18) to go through this cut, we obtain

$$\chi(x(u), x(v)) = i \sum_{n \neq 0} \text{sign}(n) K_u \star D^{2n} K_u \star \log(u - v) - i \sum_{n \neq 0} \text{sign}(n) D^{2n} K_u \star \log(u - v). \quad (3.22)$$

Since the only cut we crossed was the cut of  $x(u)$ , this expression is valid in the domain where  $|x(u)| < 1$  while  $|x[u + in]| > 1$  for  $n \neq 0$ . By crossing the cut of  $x(u)$  we moved into a different Riemann sheet. On this new sheet  $\chi(x(u), x(v))$  has all the cuts of  $x(u + in)$  for  $n \in \mathbb{Z}$  as depicted in figure 3. We could now decide to go through one of the new cuts, e.g.  $|x(u + im)| = 1$  with  $m \neq 0$ . This will bring us to a third Riemann sheet which is now defined by  $|x(u)| < 1$  and  $|x(u + im)| < 1$  with all other  $|x(u + in)| > 1$ . When going through the cut of  $|x[u + im]|$  we pick an extra contribution from the second term in (3.22) so that

$$\begin{aligned} i\chi(x(u), x(v)) = & - \sum_{n \neq 0} \text{sign}(n) K_u \star D^{2n} K_u \star \log(u - v) + \sum_{n \neq 0, m} \text{sign}(n) D^{2n} K_u \star \log(u - v) \\ & - \text{sign}(m) D^{2m} K_u \star \log(u - v) + \text{sign}(m) \log(u - v + im). \end{aligned} \quad (3.23)$$

When constructing  $\sigma^2$  the last term leads to double poles or double zeros (depending on the sign of  $m$ ). These are precisely the DHM poles/zeros mentioned above. This is a very nontrivial *finite coupling* check of the dressing factor.

<sup>13</sup>The sharp reader will have noticed that  $K_v$  was replaced by  $K_u$ . Such replacements are allowed since the difference between both expressions cancels out in the anti-symmetrization (3.5). The (derivative of the logarithm of the) representation (3.21) for the dressing phase was proposed in [22].

## 4 Useful representations and expansions

A particularly useful alternative way of expressing  $\chi(x, y)$  is through its large  $x$  and  $y$  expansion,

$$\chi(x, y) = - \sum_{r,s=1}^{\infty} \frac{c_{r,s}(g)}{x^r y^s}, \quad (4.1)$$

where  $c_{r,s} = -c_{s,r}$  are a set of functions of the 't Hooft coupling only. For the dressing factor this translates into an expansion in terms of magnon higher conserved charges:

$$\frac{1}{i} \log \sigma(u, v) = \sum_{r,s=1}^{\infty} c_{r,s}(g) q_{r+1}(u) q_{s+1}(v), \quad q_r(u) \equiv \frac{1}{(x^+)^{r-1}} - \frac{1}{(x^-)^{r-1}}. \quad (4.2)$$

The higher conserved charges  $q_r(u)$  were initially written in [8] and the expansion (4.2) was proposed in [17] (up to minor modifications). This proposal found further support in [18] where Beisert and Klose argued that generic  $gl(r)$  symmetric long-ranged integrable spin chain models give rise to (4.2).<sup>14</sup> Expanding (3.20) at large  $x$  and  $y$  and parameterizing  $z, z' = e^\phi, e^{\phi'}$ , we find

$$c_{r,s}(g) = i \int_0^{2\pi} \frac{d\phi}{2\pi} \int_0^{2\pi} \frac{d\phi'}{2\pi} \exp(ir\phi + is\phi') \log \frac{\Gamma[1 + 2ig(\cos \phi - \cos \phi')]}{\Gamma[1 - 2ig(\cos \phi - \cos \phi')]}. \quad (4.3)$$

The logarithm of gamma functions in this expression has an integral representation as  $-2i \operatorname{Im} \int_0^\infty \frac{dt}{t} \left[ \frac{e^{2igt(\cos \phi - \cos \phi')} - 1}{e^t - 1} - 2ig(\cos \phi - \cos \phi') e^{-t} \right]$ . Only the exponential term survives after the  $\phi$  and  $\phi'$  integration. Furthermore, these angular integrals yield integral representations of Bessel functions. Hence,

$$c_{r,s}(g) = 2 \sin\left(\frac{\pi}{2}(r-s)\right) \int_0^\infty dt \frac{J_r(2gt) J_s(2gt)}{t(e^t - 1)}. \quad (4.4)$$

Our logical flow was pretty much the exact opposite of the chronological one. The dressing factor was first guessed by Beisert-Eden-Staudacher [3] in the form (4.1),(4.4) based on the string analysis of Beisert-Hernandez-Lopez [4] and on transcendentality considerations [24]. Dorey-Hofman-Maldacena [16] derived (4.3) from (4.4) and resummed (4.1) to derive the integral representation (3.20). Only later the dressing factor was shown to satisfy the crossing equation in [25] and explicitly derived in [20].

### Weak coupling expansion

The constants  $c_{r,s}(g)$  admit a convergent weak coupling expansion as

$$c_{r,s}(g) = \sum_{n=0}^{\infty} c_{r,s}^{(n)} g^{r+s+2n} \quad (4.5)$$

<sup>14</sup>For more recent discussions of general integrable long range Hamiltonians see [23].

where [3]

$$c_{r,s}^{(n)} = 2(-1)^n \sin\left(\frac{\pi}{2}(r-s)\right) \frac{(2n+r+s-1)!(2n+r+s)!}{n!(n+r)!(n+s)!(n+r+s)!} \zeta(2n+r+s). \quad (4.6)$$

The convergence radius of this expansion is  $g_c = 1/4$ , see figure 4. A simple explanation for this radius of convergence is that at  $g = i/4$  the branch points of the dressing factor collide in pairs. As one can see from (4.6), the constants  $c_{r,s}(g)$  behave at weak coupling as

$$c_{r,s}(g) = \mathcal{O}(g^{r+s}). \quad (4.7)$$

This was predicted in [18] as the generic behavior of the constants  $c_{r,s}(g)$  for spin chain arising from perturbative computations in gauge theories in the planar limit. It is therefore a very important check of the solution (3.20).

The leading weak coupling term is  $c_{1,2} = -c_{2,1} = -2g^3\zeta(3)$ . For rapidities  $u, v = \mathcal{O}(1)$  it leads to

$$\sigma^2(u, v) = 1 + 256 \zeta(3) g^6 \frac{(u-v)(4uv-1)}{(1+4u^2)^2(1+4v^2)^2} + \mathcal{O}(g^8). \quad (4.8)$$

This means that the effect of the dressing factor only affects the rapidities of the particles at order  $g^6$ . The energy of a multi-particle state is given by a sum of dispersion relations  $\sum_j \epsilon(u_j)$  where  $\epsilon(u_j) = \mathcal{O}(g^2)$  which means that the dressing factor only affect the anomalous dimensions of single trace operators at order  $g^8$ , i.e. at 4 loops! It is therefore no surprise that it was originally thought that such factor was absent all together [8].

The cusp anomalous dimension<sup>15</sup>, for example, can be computed using the dressing factor derived above [26, 3]. One finds

$$\begin{aligned} f(g) = & 8g^2 - \frac{8\pi^2}{3}g^4 + \frac{88\pi^4}{45}g^2 - \left(\frac{315\pi^6}{584} + 64\zeta(3)^2\right)g^8 \\ & + \left(\frac{28384\pi^8}{14175} + \frac{128\pi^2\zeta(3)^2}{3} + 1280\zeta(3)\zeta(5)\right)g^{10} - \dots \end{aligned} \quad (4.9)$$

This expansion deserves a couple of comments. First notice that the degree of transcendently of each term is correlated to the corresponding order of perturbation theory. This is in perfect agreement with the Kotikov-Lipatov transcendentality conjecture [24]. The zeta functions in (4.6) are precisely of the required degree not to spoil this nice property! Second, if we were to compute the cusp anomalous dimension using  $\sigma^2(u, v) = 1$ , we would find *exactly the same result (4.9) with the replacement  $\zeta(2n+1) \rightarrow i\zeta(2n+1)$* ! Quite mysteriously, the constants  $c_{r,s}^{(n)}$  are *uniquely* fixed to (4.6) provided (a) we assume (4.7) and (b) require that the presence of the dressing factor simply amounts to  $\zeta(2n+1) \rightarrow i\zeta(2n+1)$  in the cusp anomalous dimension computed without any dressing factor.

---

<sup>15</sup>Operators of the form  $\text{Tr}(ZD^S Z)$ +permutations have an anomalous dimension  $\Delta(S, g) \simeq f(g) \log S$  at large  $S$ . The cusp anomalous dimension is  $f(g)/2$ .

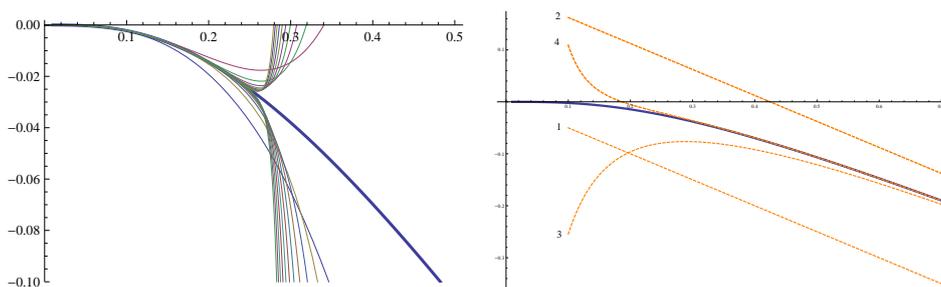

**Figure 4:** **Left:**  $c_{1,2}(g)$  as given by (4.3) or (4.4) can be evaluated for any  $g$ : thick line. The weak coupling Taylor expansion (4.5) has a finite radius of convergence. The several thin lines plotted in this figure are several truncations of this expansion (from 1 to 20 terms); the more terms are included the more they approach the real curve for  $g < 1/4$ , the radius of convergence. **Right:**  $c_{1,2}(g)$  (blue line) compared with its strong coupling expansion (dotted orange lines). 1 is the AFS result, 2 is AFS plus HL, 3 already includes the two loop correction and 4 contains the first four non-trivial terms. We see that the fit with four terms is perfect even for relatively small  $g$ ! This fast convergence was also observed in numerical computations of dimensions, see e.g. [27].

The cusp anomalous dimension turns out to be a very important quantity in the study of gluon scattering amplitudes in  $\mathcal{N} = 4$  SYM [28]. It governs the IR divergent part of these amplitudes. The cusp anomalous dimension has been computed analytically up to three loops [29] and numerically at four loops [30]. Thus the first line in (4.9) can be checked: it matches precisely the perturbative calculations!

Let us mention two more remarkable weak coupling checks of the dressing factor. At weak coupling it is convenient to think of operators

$$O(x) = \text{Tr} (Z \dots ZXZ \dots Z\Psi Z \dots ZDZ \dots Z) (x) + \text{permutations} \quad (4.10)$$

as spin excitations  $X, \Psi, D, \dots$  around a ferromagnetic spin chain vacuum  $\text{Tr} Z^L$ . In this language the anomalous dimension matrix can be thought of as a spin chain Hamiltonian [31]. At four loops we have a Hamiltonian of range four explicitly computed in [32]. At this loop order some coefficients of this Hamiltonian get  $\zeta(3)$  factors. These lead precisely to the dressing factor (4.8)!

Other impressive weak coupling checks concerns the computation of the anomalous dimension of short operators such as the Konishi operator. At four loops the range of interaction of the Hamiltonian is as large as the operator itself and the scattering picture breaks down [33]. Still, using the Luscher formalism, this correction can be computed [34]. This prediction was checked against a tour de force computation [35] and agreement was found. Other remarkable four and five loop checks concern the behavior of general twist two operators as predicted from the AdS/CFT system with the predictions of BFKL, see reviews [36] and [34] for details.

### Strong coupling

The dressing factor can also be expanded at strong coupling. However, contrary to the expansion at weak coupling which was convergent, at strong coupling the expansion is merely asymptotic, albeit Borel summable. We have  $c_{r,s}(g) = \sum_{n=0}^{\infty} d_{r,s}^{(n)} g^{1-n}$  where [4]

$$d_{r,s}^{(n)} = \frac{\zeta(n) ((-1)^{r+s} - 1) \Gamma\left(\frac{1}{2}(n - r + s - 1)\right) \Gamma\left(\frac{1}{2}(n + r + s - 3)\right)}{2(-2\pi)^n \Gamma(n-1) \Gamma\left(\frac{1}{2}(-n - r + s + 3)\right) \Gamma\left(\frac{1}{2}(-n + r + s + 1)\right)}. \quad (4.11)$$

The leading order coefficients at strong coupling are given by

$$d_{r,s}^{(0)} = \frac{\delta_{s,r-1} - \delta_{s,r+1}}{sr}, \quad d_{r,s}^{(1)} = \frac{(-1)^{r+s} - 1}{\pi} \frac{1}{r^2 - s^2}. \quad (4.12)$$

The simplest way to compute the leading order expression for the dressing factor at strong coupling is to resum (4.1) with  $c_{r,s}(g) \simeq g d_{r,s}^{(0)}$ . The result is

$$\chi^{(0)}(x, y) = (x + 1/x - y - 1/y) \log(1 - 1/xy) - 1/x + 1/y. \quad (4.13)$$

The last two terms in (4.13) cancel out when constructing the dressing factor as in (3.5) while the first term yields

$$\sigma(u, v) \simeq \frac{1 - \frac{1}{x^- y^+}}{1 - \frac{1}{x^+ y^-}} \left( \frac{1 - \frac{1}{x^- y^-}}{1 - \frac{1}{x^- y^+}} \frac{1 - \frac{1}{x^+ y^+}}{1 - \frac{1}{x^+ y^-}} \right)^{i(v-u)}. \quad (4.14)$$

This is the so called AFS dressing factor. It was engineered by Arutyunov, Frolov, and Staudacher [17] to match the strong coupling Bethe Ansatz equations with the KMMZ integral equations [37] describing classical string solutions. Historically, this work was the first solid indication that  $\sigma^2(u, v) \neq 1$ .

To compute the subleading term at strong coupling, and also the next-to-subleading etc, it is convenient to use the DHM representation (3.20) and

$$\frac{1}{i} \log \frac{\Gamma(1 + ix)}{\Gamma(1 - ix)} = -x \log(x/e)^2 - \frac{\pi}{2} \text{sign}(x) + \sum_{n>0, \text{ odd}}^{\infty} \frac{2\zeta(-n)}{n} \frac{1}{x^n} \quad (4.15)$$

which is valid for real  $x$ . When using this expansion in (3.20) we see that the first term yields the AFS dressing factor (4.14). The second term, gives us the leading quantum correction, known as the Hernandez-Lopez phase [40]. The sum in (4.15) yields all other subleading quantum corrections.

Let us now discuss the leading quantum correction. The sign term in (4.15) simply constrains the limits of integration in (3.20). This leads to

$$\chi^{(1)}(x, y) = \frac{1}{4\pi} \int_{-1}^1 \frac{dz'}{y - z'} \int_{1/z'}^{z'} \frac{dz}{x - z} - (x \leftrightarrow y), \quad (4.16)$$

which can be directly computed in terms of dilogarithms. In this way we obtain the resummation of (4.8) using  $d_{r,s}^{(1)}$ , performed in [41], see also [4]. The Hernandez-Lopez

phase is a 1-loop effect in the world-sheet strong coupling expansion and can be derived using only (quasi) classical considerations [42]. This was done in [43,40] using particularly simple circular string solutions [43], checked to be consistent with more complicated solutions in [44], and derived in full generality in [39] using the algebraic curve method [45].

It is fun to notice that the leading and subleading strong coupling terms in the expansion of  $\chi(x, y)$  are by far the hardest to compute. All other subleading corrections come from using the last sum in (4.15) in (3.20). They lead to rational integrands in  $z$  and  $z'$  so that the integrals can be trivially computed by residues.

Another curious feature of the AdS/CFT dressing factor is the following: the strong and weak coupling coefficients (4.6) and (4.11) are related by [3]  $c_{r,s}^{(n)} = d_{r,s}^{(-2n-r-s+1)}$ . This relation is further discussed in [46].

We end this section with the discussion of some other strong coupling checks of the dressing factor. Explicit perturbative computations of the full S-matrix  $\hat{S}$  were done up to 2 loops [47] in the near-flat space limit [48]. Finite size corrections around the giant-magnon solutions were performed and probe the dressing factor to all loop orders [34]. The strong coupling asymptotic expansion of the cusp anomalous dimension was found analytically at any loop order [50, 21]. The two loop coefficient was checked through a direct string computation [51]. The reproduction of the  $O(6)$  sigma model [52] from the BES/FRS equation [55] in the Alday-Maldacena limit [56], see also [53, 54]. This probes the dressing phase at all-loop order. The match of the generalized scaling function computed at one [49] and two [57] loops with a direct string theory prediction at one [58] and two [59] loops. This is a very nontrivial check since it amounts to matching a non-trivial functional dependence. Last three checks emerged from the exhaustive study of anomalous dimensions for twist operators. For more references and a review of twist operators see [36].

## 5 Concluding remarks

The dressing factor of the AdS/CFT system is a remarkable object with a very non-trivial dependence on the momenta of the scattered particles and on the 't Hooft coupling. It has been impressively scrutinized with remarkable success. Still, there are some challenges to be addressed.

Perhaps the most obvious one is the lack of an independent derivation of the dressing factor purely from gauge theory, without recurring to AdS/CFT. The most significant advantage of the string language is the existence of the notion of Wick rotation which allows us to argue in favor of the crossing relation [11, 6, 12]. On the gauge side the situation is much worse since there is no known meaning for the cross channel at all. This lack of interpretation on the gauge side is present also in the computation of the spectrum at finite volume. The finite volume computation is based on the Wick rotation trick of Zamolodchikov [60] which was implemented for the AdS/CFT case in [13, 14]. There is no interpretation of the Wick rotation from the gauge theory side, and therefore there is no derivation of the  $Y$ -system [61, 15] which does not rely on the light-cone world-sheet description.

Another interesting puzzle concerns the involved structure of the dressing factor. It motivates us to search for an underlying simpler system. For instance, the  $O(4)$  sigma model dressing factor can be interpreted as an effective interaction between spin wave excitations in a very simple antiferromagnet [62]. There has been some interesting progress in this direction in the AdS/CFT context [38]. The difference in signs in the denominators of (2.13) and (3.12) might be telling us to look for noncompact spin chains.

## Acknowledgments

Research at the Perimeter Institute is supported in part by the Government of Canada through NSERC and by the Province of Ontario through MRI. The work of D.V. is supported by the US Department of Energy under contracts DE-FG02-201390ER40577. D.V. would also thank for the hospitality of the Perimeter Institute, where the part of this work was done. This work was partially funded by the research grants PTDC/FIS/099293/2008 and CERN/FP/109306/2009.

## References

- [1] N. Beisert et al., "Review of AdS/CFT Integrability: An Overview", arXiv:1012.3982 [hep-th].
- [2] C. Ahn and R. Nepomechie, "Review of AdS/CFT Integrability, Chapter III.2: Exact world-sheet S-matrix", arXiv:1012.3991 [hep-th].
- [3] N. Beisert, B. Eden and M. Staudacher, *J. Stat. Mech.* **0701** (2007) P021 [hep-th/0610251].
- [4] N. Beisert, R. Hernandez and E. Lopez, *JHEP* **0611**, 070 (2006) [arXiv:hep-th/0609044].
- [5] A. B. Zamolodchikov and A. B. Zamolodchikov, *Nucl. Phys. B* **133**, 525 (1978) [*JETP Lett.* **26**, 457 (1977)].
- [6] N. Beisert, "The  $su(2|2)$  dynamic S-matrix," *Adv. Theor. Math. Phys.* **12** (2008) 945 [arXiv:hep-th/0511082]. • N. Beisert, *J. Stat. Mech.* **0701** (2007) P017 [arXiv:nlin/0610017].
- [7] A. Santambrogio and D. Zanon, *Phys. Lett. B* **545** (2002) 425 [arXiv:hep-th/0206079].
- [8] N. Beisert, V. Dippel and M. Staudacher, *JHEP* **0407**, 075 (2004) [arXiv:hep-th/0405001].
- [9] N. Beisert and M. Staudacher, *Nucl. Phys. B* **727**, 1 (2005) [arXiv:hep-th/0504190].
- [10] N. Dorey, *J. Phys. A* **39**, 13119 (2006) [arXiv:hep-th/0604175].

- [11] R. A. Janik, *Phys. Rev.* **D73** (2006) 086006 [hep-th/0603038](#)].
- [12] G. Arutyunov, S. Frolov and M. Zamaklar, *JHEP* **0704** (2007) 002 [[arXiv:hep-th/0612229](#)].
- [13] J. Ambjorn, R. A. Janik and C. Kristjansen, *Nucl. Phys.* **B736** (2006) 288–301 [hep-th/0510171](#)].
- [14] G. Arutyunov and S. Frolov, *JHEP* **0712** (2007) 024 [[arXiv:0710.1568 \[hep-th\]](#)].
- [15] Z. Bajnok, "Review of AdS/CFT Integrability, Chapter III.6: Thermodynamic Bethe Ansatz", [arXiv:1012.3985 \[hep-th\]](#).
- [16] N. Dorey, D. M. Hofman and J. M. Maldacena, *Phys. Rev. D* **76** (2007) 025011 [[arXiv:hep-th/0703104](#)].
- [17] G. Arutyunov, S. Frolov and M. Staudacher, *JHEP* **0410**, 016 (2004) [[arXiv:hep-th/0406256](#)].
- [18] N. Beisert and T. Klose, *J. Stat. Mech.* **0607**, P006 (2006) [[arXiv:hep-th/0510124](#)].
- [19] H. Y. Chen, N. Dorey and K. Okamura, *JHEP* **0611**, 035 (2006) [[arXiv:hep-th/0608047](#)].
- [20] D. Volin, *J. Phys. A* **42**, 372001 (2009) [[arXiv:0904.4929 \[hep-th\]](#)].
- [21] I. Kostov, D. Serban and D. Volin, *JHEP* **0808**, 101 (2008) [[arXiv:0801.2542 \[hep-th\]](#)].
- [22] I. Kostov, D. Serban and D. Volin, *Nucl. Phys. B* **789**, 413 (2008) [[arXiv:hep-th/0703031](#)]. • D. Volin, [arXiv:0812.4407 \[hep-th\]](#).
- [23] A. Rej, "Review of AdS/CFT Integrability, Chapter I.3: Long-range spin chains", [arXiv:1012.3985 \[hep-th\]](#).
- [24] A. V. Kotikov and L. N. Lipatov, *Nucl. Phys. B* **661** (2003) 19 [Erratum-ibid. *B* **685** (2004) 405] [[arXiv:hep-ph/0208220](#)].
- [25] G. Arutyunov and S. Frolov, [arXiv:0904.4575 \[hep-th\]](#).
- [26] B. Eden and M. Staudacher, *J. Stat. Mech.* **0611**, P014 (2006) [[arXiv:hep-th/0603157](#)].
- [27] M. K. Benna, S. Benvenuti, I. R. Klebanov and A. Scardicchio, *Phys. Rev. Lett.* **98** (2007) 131603 [[arXiv:hep-th/0611135](#)]. • N. Gromov, V. Kazakov and P. Vieira, [arXiv:0906.4240 \[hep-th\]](#).
- [28] G. P. Korchemsky and A. V. Radyushkin, *Phys. Lett. B* **279**, 359 (1992) [[arXiv:hep-ph/9203222](#)]. • Z. Bern, L. J. Dixon and V. A. Smirnov, *Phys. Rev. D* **72**, 085001 (2005) [[arXiv:hep-th/0505205](#)].

- [29] A. Vogt, S. Moch and J. Vermaseren, Nucl. Phys. Proc. Suppl. **152**, 110 (2006) [arXiv:hep-ph/0407321]. • A. V. Kotikov, L. N. Lipatov, A. I. Onishchenko and V. N. Velizhanin, Phys. Part. Nucl. **36S1**, 28 (2005) [arXiv:hep-th/0502015].
- [30] Z. Bern, M. Czakon, L. J. Dixon, D. A. Kosower and V. A. Smirnov, Phys. Rev. D **75** (2007) 085010 [arXiv:hep-th/0610248]. • F. Cachazo, M. Spradlin and A. Volovich, Phys. Rev. D **75** (2007) 105011 [arXiv:hep-th/0612309].
- [31] J. Minahan, "Review of AdS/CFT Integrability, Chapter I.1: Spin Chain in  $N = 4$  SYM", arXiv:1012.3983 [hep-th].
- [32] N. Beisert, T. McLoughlin and R. Roiban, Phys. Rev. D **76**, 046002 (2007) [arXiv:0705.0321 [hep-th]].
- [33] M. Staudacher, JHEP **0505** (2005) 054; [arXiv:hep-th/0412188]. • C. Sieg and A. Torrielli, Nucl. Phys. B **723** (2005) 3 [arXiv:hep-th/0505071]. • A. V. Kotikov, L. N. Lipatov, A. Rej, M. Staudacher and V. N. Velizhanin, J. Stat. Mech. **0710** (2007) P10003 [arXiv:0704.3586 [hep-th]].
- [34] R. Janik, "Review of AdS/CFT Integrability, Chapter III.5: Luscher corrections", arXiv:1012.3994 [hep-th].
- [35] F. Fiamberti, A. Santambrogio, C. Sieg and D. Zanon, Nucl. Phys. B **805** (2008) 231 • V. N. Velizhanin, JETP Lett. **89**, 6 (2009).
- [36] L. Freyhult, "Review of AdS/CFT Integrability, Chapter III.4: Twist states and the cusp anomalous dimension", arXiv:1012.3993 [hep-th].
- [37] V. A. Kazakov, A. Marshakov, J. A. Minahan and K. Zarembo, JHEP **0405**, 024 (2004) [arXiv:hep-th/0402207].
- [38] N. Mann and J. Polchinski, Phys. Rev. D **72**, 086002 (2005) [arXiv:hep-th/0508232]. • A. Rej, D. Serban and M. Staudacher, JHEP **0603**, 018 (2006) [arXiv:hep-th/0512077]. • N. Gromov, V. Kazakov, K. Sakai and P. Vieira, Nucl. Phys. B **764**, 15 (2007) [arXiv:hep-th/0603043]. • N. Gromov and V. Kazakov, Nucl. Phys. B **780**, 143 (2007) [arXiv:hep-th/0605026]. • A. Rej, M. Staudacher and S. Zieme, J. Stat. Mech. **0708**, P08006 (2007) [arXiv:hep-th/0702151]. • K. Sakai and Y. Satoh, Phys. Lett. B **661** (2008) 216 [arXiv:hep-th/0703177]. • K. Sakai and Y. Satoh, JHEP **0712** (2007) 044 [arXiv:0709.3342 [hep-th]]. • R. A. Janik and T. Lukowski, Phys. Rev. D **78**, 066018 (2008) [arXiv:0804.4295 [hep-th]].
- [39] N. Gromov and P. Vieira, Nucl. Phys. B **790**, 72 (2008) [arXiv:hep-th/0703266].
- [40] R. Hernandez and E. Lopez, JHEP **0607**, 004 (2006) [arXiv:hep-th/0603204].
- [41] G. Arutyunov and S. Frolov, Phys. Lett. B **639** (2006) 378 [arXiv:hep-th/0604043].
- [42] S. Frolov and A. A. Tseytlin, JHEP **0206**, 007 (2002) [arXiv:hep-th/0204226]. • T. McLoughlin, "Review of AdS/CFT Integrability, Chapter II.3: Quantum Strings in  $AdS_5 \times S^5$ ", arXiv:1012.3987 [hep-th].

- [43] N. Beisert and A. A. Tseytlin, Phys. Lett. B **629**, 102 (2005) [arXiv:hep-th/0509084].
- [44] L. Freyhult and C. Kristjansen, Phys. Lett. B **638** (2006) 258 [arXiv:hep-th/0604069].
- [45] N. Gromov and P. Vieira, Nucl. Phys. B **789**, 175 (2008) [arXiv:hep-th/0703191]. • S. Schafer-Nameki, "Review of AdS/CFT Integrability, Chapter II.4: The Spectral Curve", arXiv:1012.3989 [hep-th].
- [46] A. V. Kotikov and L. N. Lipatov, Nucl. Phys. B **769**, 217 (2007) [arXiv:hep-th/0611204]. • Beisert, N., "Strong/Weak Interpolation in the Spectrum of AdS/CFT" <http://www.ift.uam.es/strings07/> • Ferreti, G., "Applying the BES trick to QCD" *Integrability and the Gauge/String Correspondence*, <http://www.newton.ac.uk/programmes/SIS/sisw03.html> • M. Kruczenski and A. Tirziu, Phys. Rev. D **80**, 086002 (2009) [arXiv:0907.4118 [hep-th]].
- [47] T. Klose, T. McLoughlin, J. A. Minahan and K. Zarembo, JHEP **0708** (2007) 051 [arXiv:0704.3891 [hep-th]].
- [48] J. M. Maldacena and I. Swanson, Phys. Rev. D **76** (2007) 026002 [arXiv:hep-th/0612079].
- [49] P. Y. Casteill and C. Kristjansen, Nucl. Phys. B **785** (2007) 1 [arXiv:0705.0890 [hep-th]]. • A. V. Belitsky, Phys. Lett. B **659**, 732 (2008) [arXiv:0710.2294 [hep-th]].
- [50] B. Basso, G. P. Korchemsky and J. Kotanski, Phys. Rev. Lett. **100**, 091601 (2008) [arXiv:0708.3933 [hep-th]].
- [51] R. Roiban and A. A. Tseytlin, JHEP **0711**, 016 (2007) [arXiv:0709.0681 [hep-th]].
- [52] B. Basso and G. P. Korchemsky, Nucl. Phys. B **807** (2009) 397 [arXiv:0805.4194 [hep-th]].
- [53] D. Fioravanti, P. Grinza and M. Rossi, Nucl. Phys. B **810**, 563 (2009) [arXiv:0804.2893 [hep-th]] • D. Fioravanti, P. Grinza and M. Rossi, Nucl. Phys. B **827**, 359 (2010) [arXiv:0805.4407 [hep-th]] • D. Fioravanti, P. Grinza and M. Rossi, JHEP **0911**, 037 (2009) [arXiv:0808.1886 [hep-th]].
- [54] D. Volin, arXiv:1003.4725 [hep-th].
- [55] L. Freyhult, A. Rej and M. Staudacher, J. Stat. Mech. **0807** (2008) P07015 [arXiv:0712.2743 [hep-th]]. • D. Bombardelli, D. Fioravanti and M. Rossi, Nucl. Phys. B **810**, 460 (2009) [arXiv:0802.0027 [hep-th]].
- [56] L. F. Alday and J. M. Maldacena, JHEP **0711** (2007) 019 [arXiv:0708.0672 [hep-th]].
- [57] N. Gromov, JHEP **0811** (2008) 085 [arXiv:0805.4615 [hep-th]]. • Z. Bajnok, J. Balog, B. Basso, G. P. Korchemsky and L. Palla, Nucl. Phys. B **811**, 438 (2009) [arXiv:0809.4952 [hep-th]].

- [58] S. Frolov, A. Tirziu and A. A. Tseytlin, Nucl. Phys. B **766**, 232 (2007) [arXiv:hep-th/0611269].
- [59] S. Giombi, R. Ricci, R. Roiban, A. A. Tseytlin and C. Vergu, arXiv:1002.0018 [hep-th].
- [60] Al. B. Zamolodchikov, Phys. Lett. B **253** (1991) 391.
- [61] N. Gromov, V. Kazakov and P. Vieira, Phys. Rev. Lett. **103** (2009) 131601 [arXiv:0901.3753 [hep-th]]. • V. Kazakov and N. Gromov, "Review of AdS/CFT Integrability, Chapter III.7: Hirota Dynamics for Quantum Integrability", arXiv:1012.3996 [hep-th].
- [62] L. D. Faddeev and N. Y. Reshetikhin, Annals Phys. **167**, 227 (1986).

# Review of AdS/CFT Integrability, Chapter III.4: Twist states and the cusp anomalous dimension

LISA FREYHULT

*Department of Physics and Astronomy, Division for Theoretical Physics, Uppsala University, Box 516, SE-751 20 Uppsala, Sweden*

`lisa.freyhult@physics.uu.se`

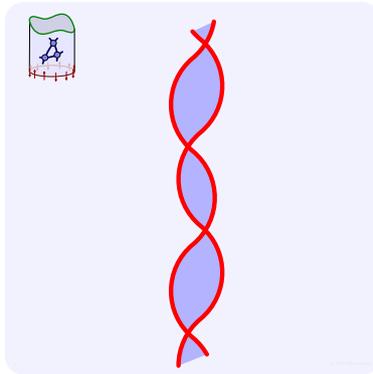

**Abstract:** We review the computation of the anomalous dimension of twist operators in the planar limit of  $\mathcal{N} = 4$  SYM using the asymptotic Bethe ansatz and demonstrate how this quantity is obtained at weak, strong and intermediate values of the coupling constant. The anomalous dimension of twist operators in the limit of large Lorentz spin played a major role in the construction as well as in many tests of the asymptotic Bethe equations, this aspect of the story is emphasised.

# 1 Introduction

One of the best investigated quantities in the subject of integrability in the context of the AdS/CFT correspondence is the anomalous dimension of twist operators<sup>1</sup>. The reasons for this are numerous and range from the interest in these operators due to the role they play in deep inelastic scattering in QCD to the fact that their anomalous dimension provides a quantity ideal for studying the AdS/CFT correspondence, a quantity that interpolate between the weak and strong coupling regimes of the theory.

The construction of the asymptotic Bethe equations that determine the spectrum of planar  $\mathcal{N} = 4$  supersymmetric Yang-Mills theory was based on and inspired by a number of conjectures. The two major ones are the complete, all-loop, integrability of the model and the AdS/CFT correspondence itself. Given the conjectures at the basis of the asymptotic construction it is absolutely necessary to put it to as many tests as possible and for this suitable quantities, amenable for studies, are needed. Twist operators constitute such quantities and played a major role in the developments of the asymptotic system and were also important for understanding its inadequacies. It is now beyond any doubt that the asymptotic equations do not provide the final answer to the spectral problem in the planar limit. A system taking finite size effects into account is being constructed and also for tests of this system twist operators have played and can be expected to play an important role, see [1, 2] for reviews.

The operators in question appear in a wide range of contexts, see also the review [3]. Their anomalous dimensions can be computed from considerations of Wilson loops, gluon scattering amplitudes and they, as mentioned, play an important role in QCD and deep inelastic scattering. Naturally this is a great advantage since this allows for many cross-checks. Furthermore, providing all loop expressions for the scaling dimensions of the operators is not only important to AdS/CFT and the studies of integrability but also for making progress in these other areas.

The simplest representatives of twist operators in  $\mathcal{N} = 4$  SYM are operators in the  $\mathfrak{sl}(2)$  subsector, constructed from complex scalar fields,  $Z$ , and covariant light-cone derivatives,  $D$ ,

$$O(x) = \text{Tr}(D^M Z^L) + \dots \quad (1.1)$$

The abbreviation denotes all possible ways in which the derivatives are distributed on the scalar fields. The length or the twist of the operator is denoted by  $L$  and  $M$  is the number of covariant derivatives or the Lorentz spin.

The asymptotic Bethe equations were derived by assuming all loop integrability and imposing  $PSU(2, 2|4)$  symmetry on the internal S-matrix of the theory, see [4, 5] for a review. This fixes the S-matrix and the Bethe equations up to an overall phase [6]. In analogy with relativistic models the phase obeys crossing symmetry [7], this symmetry however does not completely constrain the phase. The condition of crossing symmetry has to be supplemented by information on the analytical properties of the phase. A

---

<sup>1</sup>This name might be slightly misleading. The twist of an operator is defined as its scaling dimension minus its Lorentz spin. Hence one could refer to any local operator with a definite value of the twist as a twist operator. We will make it explicit below which operators we are considering. In the literature these kind of operators are also referred to as Wilson operators.

proposal for the dressing phase was made based upon the structural properties of the anomalous dimensions of twist operators in the limit of large spin,  $M$  [8,9]. An important clue was provided by the impressive direct field theory computation of the same object to four loops [10,11] which allowed to test the proposed Bethe equations and the dressing phase. Later it was demonstrated that the conjectured phase also constitutes a minimal solution to the crossing equations [12].

In the limit of large spin the anomalous dimension of the operators exhibits logarithmic, Sudakov, scaling [13,14] and all the coupling constant dependence is collected in the so called scaling function. The scaling function was also obtained from considerations of light like Wilson loops with a cusp [15,16], both at weak and strong coupling [17,18], and is therefore also termed the cusp anomalous dimension.

Twist operators in the large spin limit have a universal behavior, their minimal anomalous dimension does not depend on the length of the operator [16,33,8]. It was therefore conjectured that this quantity was not affected by finite-size/wrapping effects (see [19] for a review) and consequently the asymptotic Bethe equations can be used to compute it to any loop order. This is also in line with the identification with cusped Wilson loops which independently implies no wrapping corrections. This allows for the construction of an all loop integral equation [8,9] which, if solved, provides the anomalous dimension as a function of the coupling constant, a quantity that smoothly interpolates between weak and strong coupling. Needless to say such a quantity is of great importance for a better understanding of the AdS/CFT correspondence.

The string duals of twist two operators are folded strings with spin  $S$  on  $AdS_3$ . The string sigma model allows for a semiclassical expansion and the energy of the string states can be obtained to leading orders in the sigma model loop expansion, see the discussion in [20] and [21]. The spin  $S$  is taken large and identified with  $M$  and for the dual operators this provides a prediction of their scaling dimension at strong coupling. The agreement between the string energy [22–24] and the anomalous dimensions of the dual operators found by solving the Bethe equations at strong coupling [25–32] provided a remarkable check of the equations as well as the AdS/CFT correspondence.

Here we will review the developments that led to an integral equation determining the all loop expressions for the scaling dimensions of twist operators in the limit of large Lorentz spin. We will then solve this equation at weak, strong and intermediate values of the coupling constant and relate the results obtained to other, completely independent, computations of the same object. We will further review the anomalous dimensions for finite values of the Lorentz spin as well as their subleading corrections in the large spin expansion and the structural properties of the weak and strong coupling expansions.

## 2 The asymptotic Bethe ansatz for $\mathfrak{sl}(2)$ twist operators

The twist operators (1.1) belong to the  $\mathfrak{sl}(2)$  subsector, a closed subsector of the theory. In the spin chain picture, using  $\text{Tr}(Z^L)$  as the reference state the covariant derivatives are interpreted as excitations on this vacuum. Any number of excitations  $M$  is hence

allowed and this number may exceed the length of the operator. The Bethe equations which determine the asymptotic spectrum of anomalous dimensions in the  $\mathfrak{sl}(2)$  sector are then written, in terms of the rapidities or Bethe roots  $u_i$ , as [4, 5]

$$\left(\frac{x_k^+}{x_k^-}\right)^L = \prod_{j=1}^M \frac{u_k - u_j - i}{u_k - u_j + i} \left(\frac{1 - g^2/x_k^+ x_j^-}{1 - g^2/x_k^- x_j^+}\right)^2 e^{2i\theta(u_k, u_j)} \quad (2.1)$$

where  $g^2 = \frac{\lambda}{16\pi^2}$ ,  $\lambda$  is the 't Hooft coupling,  $u = x(u) + \frac{g^2}{x(u)}$  and  $x^\pm(u) = x(u \pm i/2)$ . Solving the Bethe equations together with the cyclicity constraint  $\prod_{j=1}^L \frac{x_j^+}{x_j^-} = 1$  for the rapidities the anomalous dimension can be computed using

$$\gamma(g) = 2g^2 E = 2g^2 \sum_j \left( \frac{i}{x_j^+} - \frac{i}{x_j^-} \right). \quad (2.2)$$

Here  $E$  denotes the energy of the corresponding spin state. The explicit form of the dressing phase,  $\theta(u, v)$ , can be found in [9, 5]. At leading order in the weak coupling expansion (2.1) and (2.2) give the spectrum of the non-compact  $XXX_{-1/2}$  spin chain with nearest neighbor interactions. In this sector all the Bethe roots are real. In order to study the limit when  $M \rightarrow \infty$  it is useful to first consider the leading order equations, determining the anomalous dimension to one-loop, on the form

$$-iL \log \frac{u_k + i/2}{u_k - i/2} = 2\pi n_k - i \sum_{j \neq k}^M \log \frac{u_k - u_j - i}{u_k - u_j + i}. \quad (2.3)$$

Here  $n_k$  reflects the choice of branch of the logarithm. This choice specifies the state in the spectrum. For generic values of  $L$  the states occupy a band [33, 14, 34] and we will here make the choice to study the lowest state in the band by setting  $n_k = \text{sign}(u_k)$  and consider configurations where the roots are distributed symmetrically around the origin<sup>2</sup>. For  $L = 2$  there is only one state.

In the limit the roots accumulate on a smooth contour with endpoints  $\pm b$  and the discrete roots in (2.3) can be replaced by the continuum parameter  $u$ . Introducing the rescaled roots  $\bar{u} = u/M$ , the one-loop density  $\rho_0(u) = \frac{1}{M} \sum_j \delta(u - u_j)$  and the rescaled density  $\bar{\rho}_0(\bar{u}) = \frac{1}{M} \sum_j \delta(\bar{u} - \frac{u_j}{M})$  with support on the interval  $[-b, b]$  the leading equation can be written as

$$0 = 2\pi \text{sign}(\bar{u}) - 2 \int_{-b}^b \frac{\bar{\rho}_0(\bar{u}') d\bar{u}'}{\bar{u} - \bar{u}'}. \quad (2.4)$$

---

<sup>2</sup>For twist  $L \geq 3$  it is possible to construct several operators with the same  $L$  and  $M$  with different anomalous dimensions. The anomalous dimensions can be labeled by an additional quantum number,  $l$ , as  $\gamma_{L,M}^{(l)}$  and represents the eigenvalues of the mixing matrix associated with the dilatation operator. They can be ordered as  $\gamma_{M,L}^{(0)} < \gamma_{M,L}^{(1)} < \dots$  and are smooth functions of  $M$ . We refer to  $\gamma_{M,L}^{(0)}$  as the lowest state in the band and the others as excited states. The different states are distinguished in the Bethe ansatz by their different the mode numbers. See the references above for a detailed discussion.

The integral with a bar in the above equation is used to denote the principal value integral. A solution is found by standard methods using the inverse Hilbert transform [8]

$$\bar{\rho}_0(\bar{u}) = \frac{1}{\pi} \log \frac{1 + \sqrt{1 - \bar{u}^2/b^2}}{1 - \sqrt{1 - \bar{u}^2/b^2}}. \quad (2.5)$$

This result was initially obtained by an alternative method in [35]. The normalization of the density,

$$\int_{-b}^b \bar{\rho}_0(\bar{u}) d\bar{u} = 1, \quad (2.6)$$

determines the endpoints to  $\pm b = \pm 1/2$ . The one-loop anomalous dimension in the large  $M$  limit is hence

$$\gamma_0 = \frac{2g^2}{M} \int_{-1/2}^{1/2} \frac{\bar{\rho}_0(\bar{u}) d\bar{u}}{\bar{u}^2 + 1/4M^2} = 4g^2 \log \frac{\sqrt{1 + 1/M^2} + 1}{\sqrt{1 + 1/M^2} - 1} = 8g^2 \log M + \mathcal{O}(M^0). \quad (2.7)$$

Having solved the one-loop problem we proceed to all loops. Taking the logarithm of both sides of the equation (2.1) and multiplying by  $i$  we write

$$\begin{aligned} 2L \arctan(2u_k) + iL \log \frac{1 + g^2/(x_k^-)^2}{1 + g^2/(x_k^+)^2} &= 2\pi \tilde{n}_k - 2 \sum_{\substack{j=-M/2 \\ j \neq k}}^{M/2} \arctan(u_k - u_j) \\ + 2i \sum_{j=-M/2}^{M/2} \log \frac{1 - g^2/x_k^+ x_j^-}{1 - g^2/x_k^- x_j^+} - 2 \sum_{j=-M/2}^{M/2} \theta(u_k, u_j), \quad k = \pm 1, \pm 2, \dots, \pm \frac{M}{2} \end{aligned} \quad (2.8)$$

where the shifted mode numbers are

$$\tilde{n}_k = \frac{L-3}{2} \text{sign}(k) + k = \frac{L-2}{2} \text{sign}(k) + k', \quad k' = \pm \frac{1}{2}, \pm \frac{3}{2}, \dots, \pm \frac{M-1}{2}. \quad (2.9)$$

It is convenient to use shifted mode numbers, as opposed to the mode numbers we used at one-loop, as in the limit when  $M$  is taken to infinity  $x = k'/M$  becomes a continuous variable and the density can be obtained from  $\rho(u) = \frac{dx}{du}$ . Note however that this is just a trick used to get the equations on a convenient form, the state and mode numbers specified are identical to the one-loop case studied above. Differentiating we find the leading continuum equation

$$\begin{aligned} 0 &= 2\pi \rho(u) - 2 \int_{-M/2}^{M/2} \frac{\rho(u') du'}{(u-u')^2 + 1} + 2i \int_{-M/2}^{M/2} du' \rho(u') \frac{d}{du} \log \frac{1 - g^2/x^+(u)x^-(u')}{1 - g^2/x^-(u)x^+(u')} \\ &- 2 \int_{-M/2}^{M/2} \frac{d}{du} \theta(u, u') \rho(u') du'. \end{aligned} \quad (2.10)$$

To this leading order all dependence on the twist  $L$  is removed. Twist dependence will however enter as the first subleading corrections are included. By a numerical analysis of this equation [8] one finds that the density with the one-loop part subtracted is localised

close to the origin. Splitting the density  $\rho(u) = \rho_0(u) + \sigma(u)$  the limits of integration in all integrals containing  $\sigma(u)$  can therefore be extended to  $\pm\infty$  as the limit  $M \rightarrow \infty$  is taken. The integrals containing  $\rho_0(u)$  can then be explicitly evaluated using (2.5). Finally rescaling  $\sigma(u) \rightarrow -\frac{\gamma_0}{2M}\sigma(u)$  this leads to the following equation for the Fourier-Laplace transform<sup>3</sup>,  $\hat{\sigma}(t) = e^{-t/2} \int_{-\infty}^{\infty} du e^{-itu} \sigma(u)$ ,

$$\hat{\sigma}(t) = \frac{t}{e^t - 1} \left( K(2gt, 0) - 4g^2 \int_0^{\infty} K(2gt, 2gt') \hat{\sigma}(t') \right). \quad (2.11)$$

The kernel in (2.11) is given by

$$\begin{aligned} K(t, t') &= K_0(t, t') + K_1(t, t') + K_d(t, t') \\ K_0(t, t') &= \frac{tJ_1(t)J_0(t') - t'J_0(t)J_1(t')}{t^2 - t'^2} = \frac{2}{tt'} \sum_{n=1}^{\infty} (2n-1) J_{2n-1}(t) J_{2n-1}(t') \\ K_1(t, t') &= \frac{t'J_1(t)J_0(t') - tJ_0(t)J_1(t')}{t^2 - t'^2} = \frac{2}{tt'} \sum_{n=1}^{\infty} 2n J_{2n}(t) J_{2n}(t') \\ K_d(t, t') &= 8g^2 \int_0^{\infty} dt'' K_1(t, 2gt'') \frac{t''}{e^{t''} - 1} K_0(2gt'', t'), \end{aligned} \quad (2.12)$$

where the kernel  $K_d(t, t')$  has its origin in the dressing phase. From (2.2) we find that it is possible to rewrite the anomalous dimension in terms of the density at zero,

$$\gamma(g) = 16g^2 \sigma(0) \log M = f(g) \log M. \quad (2.13)$$

The function  $f(g)$  is the so called scaling function. We note here that the higher loop density,  $\sigma(u)$ , also gives the one-loop anomalous dimension. Computing the anomalous dimension in this way, as opposed to directly from (2.2), requires information about the density to one loop order higher than the desired anomalous dimension.

The leading integral equation for the density (2.11) is independent of the twist of the operator or the length of the corresponding spin chain. The derivation above is based on the asymptotic Bethe ansatz which is expected to break down at order  $g^{2L}$  due to wrapping effects. For twist two operators the asymptotic equations are, due to superconformal invariance, valid to  $\mathcal{O}(g^6)$  [6]<sup>4</sup>. The fact that the result is independent of the twist lead to the conjecture that the anomalous dimension is universal and that wrapping plays no role for these operators to the leading order in the large spin expansion [8].

In the approach to the study of twist operators discussed above an operator constructed solely from scalar fields was identified with the ground state of the spin chain. The covariant derivatives were viewed as excitations on the chain and we had to solve the Bethe equations for a large number of excitations to be able to describe the states of interest. There is another possible description of the operators that is somewhat more

<sup>3</sup> For details on the Fourier-Laplace transforms see [8].

<sup>4</sup>States in the same supersymmetry multiplet have the same anomalous dimension. In the same multiplet as the operators (1.1) with  $L = 2$  there are also length four operators and therefore wrapping is delayed.

natural in this context. It is possible to let the derivatives act as an effective ground state and instead view the scalar fields as excitations. This reduces the complexity of the problem as in this case the twist two operators can be described by considering the scattering of only 2 excitations, termed holes [14, 36]. In this description the one-loop anomalous dimension for twist  $L$  is written as

$$\begin{aligned} \frac{\gamma_0}{g^2} &= 4\gamma_E L + 2 \sum_{j=1}^L \left( \psi(1/2 + iu_h^{(j)}) + \psi(1/2 - iu_h^{(j)}) \right) \\ &+ 2 \int_{-\infty}^{\infty} \frac{dv}{\pi} i \frac{d^2}{dv^2} \left( \log \frac{\Gamma(1/2 + iv)}{\Gamma(1/2 - iv)} \right) \text{Im} \log [1 + (-1)^\delta e^{iZ(v+i0)}] \end{aligned} \quad (2.14)$$

where  $\delta = L + M \bmod 2$  and  $Z(u)$  denotes the counting function which in turn is determined by a non-linear integral equation. This kind of equations are often referred to as Destri-de Vega equations or, simply, non-linear integral equations, NLIE, and have been discussed in numerous publications, see [37] for a pedagogical introduction and further references. The counting function determines the rapidities of the holes as well as of the Bethe roots. In the limit of large  $M$  one immediately finds two large holes with  $u_h \rightarrow \pm M/\sqrt{2}$  and in addition it is possible to show that the non-linear term in (2.14) go as  $4 \log 2 + \mathcal{O}((\frac{\log M}{M})^2)$ , see [36] for details. The leading anomalous dimension (2.7) is therefore immediately obtained. This analysis extends to include all higher loops and it is also possible to treat general values of the twist. To leading order in the large  $M$  expansion one finds this way the same integral equation as in (2.11). Making use of this method it is however straightforward to continue the expansion and include also subleading corrections, for general  $L$  this allows for a the construction of an integral equation for terms proportional to  $M^0$  [36, 38, 39] and all corrections of the form  $1/(\log M)^k$ , with  $k$  any integer  $\geq 1$  [40]. For general  $L$  the anomalous dimension has the structure

$$\gamma_L(g, M) = f(g) (\log M + \gamma_E + (L - 2) \log 2) + B_L(g) + \sum_{k=1}^{\infty} \frac{C_L^{(k)}(g)}{(\log M)^k} \dots \quad (2.15)$$

For  $L = 2, 3$  one can continue the expansion up to  $\mathcal{O}((\frac{\log M}{M})^2)$  where the non-linear terms start contributing. For  $L = 2$  the result is

$$\gamma_2(g, M) = f(g) \left( \log M + \gamma_E + \frac{f(g) \log M + \gamma_E}{2} \frac{1}{M} + \frac{1 + B_2(g)}{2M} \right) + B_2(g) + \mathcal{O}((\frac{\log M}{M})^2). \quad (2.16)$$

The advantage of this method is that it is completely straightforward. No splitting of densities or input from numerics, as was used to derive (2.11) from (2.10), was needed. On the other hand one here faces the difficulty of treating the non-linear term.

### 3 Weak coupling expansion

The evaluation of the scaling function at weak coupling constitutes an important test of the conjectured asymptotic all loop Bethe equations. This very same function appears

in scattering amplitudes, in light-like Wilson loops with a cusp and is part of a direct Feynman-diagram evaluation of the corresponding QCD result. For this reason there are several ways to compute the quantity and predictions for what the Bethe equations, if correct, should give.

The integral equation (2.11) is a Fredholm equation of the second type and easily expanded to many loop orders at weak coupling,

$$f(g) = 8g^2 - \frac{8\pi^2}{3}g^4 + \frac{88\pi^4}{45}g^6 - 16 \left( \frac{73}{630}\pi^6 + 4\zeta(3)^2 \right) g^8 + \dots \quad (3.1)$$

This expansion, to any loop order, shows an important structure. Assigning *the degree of transcendentality*  $k$  to  $\zeta(k)$  and  $\pi^k$  we find that the  $l$ -loop term has degree of transcendentality  $2l - 2$ <sup>5</sup>. This is a manifestation of the maximal transcendentality principle conjectured in [41]. This principle states that the  $\mathcal{N} = 4$  result can be extracted from the corresponding QCD result by removing all terms that are not of maximal transcendentality. Using this conjecture it was possible to extend the one-loop result, first computed in [42], to two loops by extracting the scaling function from the QCD result [43], obtained by a direct field theory calculation. Further the three loop result was obtained in [44] using the computation of the QCD splitting functions in [45].

This prediction was confirmed using the fact that the scaling function determines the leading  $1/\epsilon^2$  pole of the logarithm of gluon amplitudes computed using dimensional regularisation in  $4 - 2\epsilon$  dimensions. The two and three loop planar four point amplitude in  $\mathcal{N} = 4$  SYM was computed in [10]. Through an impressive effort that computation was also extended to four loops [11].

The anomalous dimension of light-like Wilson loops with a cusp is identified with the anomalous dimension of twist operators and also provide the first orders in the weak coupling expansion [15, 16].

Up to three loops the result (3.1) is not sensitive to the dressing phase, to be able to fix the dressing phase the knowledge of the four loop scaling function therefore played a major role [8, 11, 9]. The scaling dimension, computed from the Bethe equations with the correct dressing phase, is in full agreement with the results of the completely independent calculations mentioned above, providing highly non-trivial evidence that the Bethe equations and the assumptions made to derive them are indeed correct.

In fact the three-loop result extracted from the QCD field theory computation is exact in  $M$  and naturally expressed in terms of harmonic sums

$$\begin{aligned} \gamma(M) = & 8g^2 S_1 - 16g^4 \left( S_3 + S_{-3} - 2S_{-2,1} + 2S_1 (S_2 + S_{-2}) \right) \\ & - 64g^6 \left( 2S_{-3} S_2 - S_5 - 2S_{-2} S_3 - 3S_{-5} + 24S_{-2,1,1,1} + 6(S_{-4,1} + S_{-3,2} + S_{-2,3}) \right. \\ & - 12(S_{-3,1,1} + S_{-2,1,2} + S_{-2,2,1}) - (S_2 + 2S_1^2)(3S_{-3} + S_3 - 2S_{-2,1}) \\ & \left. - S_1(8S_{-4} + S_{-2}^2 4S_2 S_{-2} + 2S_2^2 + 3S_4 - 12S_{-3,1} - 10S_{-2,2} + 16S_{-2,1,1}) \right), \quad (3.2) \end{aligned}$$

---

<sup>5</sup>The transcendentality of a product is given by the sum of the transcendentality of the factors.

where

$$S_a = \sum_{m=1}^M \frac{(\text{sign}(a))^m}{m^a}, \quad S_{a_1, a_2, a_3, \dots} = \sum_{m=1}^M \frac{(\text{sign}(a_1))^m}{m^{a_1}} S_{a_2, a_3, \dots}(m). \quad (3.3)$$

For properties of the generalised harmonic sums see for example [46]. The transcendentality principle for the expression exact in  $M$  states that the degrees of the sums,  $|a_1| + |a_2| + |a_3| + \dots$ , should add up to  $2l - 1$  at  $l$  loops.

The exact expressions (3.2) can also be obtained from the Bethe ansatz. One way to obtain such expressions is to numerically solve the Bethe equations for different values of  $M$  and then fit the obtained result to a linear combination of harmonic sums and products of harmonic sums that obeys the transcendentality principle [47–51]. While there are additional properties that allows to restrict the number of terms in such an ansatz, see [47–51] for more details, the number of terms to be fitted against and the complexity of the result still increase rapidly with the loop order. This method has allowed for the construction of the anomalous dimension for any  $M$  for twist two and three operators up to 5 loops, we refer to the mentioned papers for explicit expressions for the anomalous dimensions as the expressions grow rapidly in length and fill pages. There are also some results for operators with higher twist [52].

Another complementary approach has been to study the so called Baxter equation. This equation is formulated in terms of the Baxter function,  $Q(u) = \prod_{j=1}^M (u - u_j)$ , and the transfer matrix eigenvalue,  $t(u)$ , and reads for the  $\mathfrak{sl}(2)$  sector at one loop

$$t(u)Q(u) = (u + i/2)^L Q(u + i) + (u - i/2)^L Q(u - i), \quad (3.4)$$

$$t(u) = 2u^L + q_{L-2}u^{L-2} + \dots + q_0, \quad (3.5)$$

where  $q_{L-2} = -(M + L/2)(M + L/2 + 1) - L/4$ . The remaining  $q_r$ ,  $r = 0, \dots, L - 3$  specify the state. For  $L = 2$  there is only one state and this equation can be identified with the equation for Wilson or Hahn polynomials and is hence solved by [35, 8]

$$Q(u) = {}_4F_3\left(-\frac{M}{2}, \frac{M+1}{2}, \frac{1}{2} + iu, \frac{1}{2} - iu; 1, 1, \frac{1}{2}; 1\right) = {}_3F_2\left(-M, M + 1, \frac{1}{2} - iu; 1, 1; 1\right). \quad (3.6)$$

The one-loop anomalous dimension is given by

$$\gamma(g, M) = 2g^2 \left. \frac{d}{du} (i \log Q(u + i/2)) \right|_{u=0} = 8g^2 S_1(M) \quad (3.7)$$

which at large  $M$  reduces to (2.13). The analogous result for the ground state with  $L = 3$  was found in [53].

The all loop  $\mathfrak{sl}(2)$  Baxter equation was derived in a series of papers [54] and this construction made it possible to develop methods for finding higher loop solutions exact in the spin  $M$ . By a deformation of the one-loop solution the result for  $L = 2, 3$  was found to three loops [55] and later extended to four loops [56].

The construction of these results exact in spin allowed for another important check of the Bethe equations. The asymptotic equations are supposed to break down due to wrapping effects. As the interaction range is growing with the order in the loop expansion

this happens soon enough for short operators as twist two and three. Nevertheless there are indications that terms up to the order  $\mathcal{O}((\frac{\log M}{M})^2)$  in the large spin expansion are free from corrections. To investigate the supposed breakdown of the Bethe ansatz prediction at higher loop orders the studies of high energy scattering amplitudes in  $\mathcal{N} = 4$  provides important insights. The Balitsky-Fadin-Kuraev-Lipatov (BFKL) equation describes the high energy scattering both in QCD and in  $\mathcal{N} = 4$  and provides the relation between the anomalous dimension and the spin  $M$  near the point  $M = -1$  [57, 41]. With the spin  $M = -1 + \omega$ , and  $\omega$  taken small, the one-loop relation for twist 2 operators reads

$$-\frac{\omega}{4g^2} = \psi\left(-\frac{\gamma}{2}\right) + \psi\left(1 + \frac{\gamma}{2}\right) - 2\psi(1), \quad (3.8)$$

Expanding the  $\psi$ -functions in power series and then inverting the series we find

$$\gamma = 2\left(-\frac{4g^2}{\omega}\right) - 4\zeta(3)\left(-\frac{4g^2}{\omega}\right)^4 + \mathcal{O}(g^{12}). \quad (3.9)$$

Hence the one-loop BFKL equation provides an all-loop prediction for the leading singularities as  $\omega \rightarrow 0$ . The 5-loop result for general values of the spin can now be analytically continued to  $M = -1 + \omega$  and expanded for  $\omega \ll 1$ , the result is

$$\gamma = 2\left(-\frac{4g^2}{\omega}\right) - 2\frac{(-4g^2)^4}{\omega^7} + 2\frac{(-4g^2)^5}{\omega^9} + \mathcal{O}(g^{12}). \quad (3.10)$$

This clearly shows that the Bethe ansatz prediction breaks down at four loops, as was indeed expected from general considerations. It is also possible to check that the results are free from wrapping up to  $\mathcal{O}((\frac{\log M}{M})^2)$ , for  $L = 2$  to four loops this has been demonstrated explicitly [58, 59] and for 5-loops this is very likely to hold [51]. Similar arguments can also be made for  $L = 3$  [50]. Furthermore the BFKL equation has been proposed to two-loop order which by the same arguments as above provides an all-loop prediction for the next to leading singularity, also this prediction disagrees with the result from the Bethe ansatz [48, 51]. Including wrapping corrections restores this agreement, see [1] for a review.

The exact expressions in terms of harmonic sums as well as the integral equations for further subleading terms in the large  $M$  expansion show yet another interesting feature. Continuing the expansion beyond the leading order one finds that the perturbative expressions can be organised as in (2.16)<sup>6</sup>. The structure observed in the expansion is due to a property referred to as reciprocity or parity preservation [60–62], see also [63] for a recent review. The twist operators (1.1) can be classified using representations of the collinear  $SL(2, \mathbb{R})$  subgroup of the conformal group  $SO(2, 4)$  [64, 3]. This suggests the conformal spin,  $m = M + L/2 + \gamma(M)$ , as a natural parameter for the expansion and that the anomalous dimension can be written as

$$\gamma(M, L) = f(M + \gamma(M, L), L). \quad (3.11)$$

---

<sup>6</sup>A similar structure is also present for  $L > 2$  and for the further terms in the large  $M$  expansion.

Reciprocity states that the function  $f(M)$  can be expanded in terms of the quadratic Casimir of the collinear group,  $J^2 = (M + L/2)(M + L/2 - 1)$

$$f(M) = \sum_{n=0}^{\infty} \frac{f_n(\log J)}{J^{2n}}. \quad (3.12)$$

This is fully consistent with the relations between the coefficients in (2.16) and implies relations between further terms in the expansion and hence reduces the number of unknown functions appearing in the expansion, roughly by a factor of two.

Reciprocity also restricts the expressions exact in  $M$  which naturally is helpful for finding them, it can be used to restrict the ansatz in terms of harmonic sums [65,50,56,51]. An interesting thing to note however is that the perturbative expressions found respects reciprocity both when wrapping interactions are included as well as when they are not [59].

Reciprocity in this context is based on an earlier idea that appeared in the context of deep inelastic scattering in QCD, the Gribov-Lipatov one-loop reciprocity [66]. That idea states that the splitting functions  $P(x)$ , related to the twist 2 anomalous dimensions in QCD by Mellin transformation, obeys the relation  $P(x) = -xP(1/x)$ . This leads to relations between coefficients in the large  $M$  expansion of the anomalous dimension as were first observed in [45,67], the so called MVV relations, and extended to higher orders in the expansion in [61].

A complete understanding of the origin of the observed reciprocity property is lacking. It is not a unique feature of  $\mathcal{N} = 4$  SYM, not tied to integrability or even to the planar limit. Indeed it holds in QCD in sectors where integrability is not present and for an arbitrary number of colors [61]. In  $\mathcal{N} = 4$  reciprocity is a feature of other known minimal anomalous dimensions of twist operators [68,49,69,65] while broken for higher states in the band [34,70]. Further it was also observed in  $\mathcal{N} = 6$  Chern-Simons theory [70], see also the review [71].

## 4 Strong coupling expansion

With the equation (2.11) we have the first explicit realisation of a quantity important for the AdS/CFT correspondence that can be computed for all values of the coupling constant. Considering the dual string states we can therefore put both the Bethe equations and the correspondence itself to a test. Studying the dual string states, folded strings with one large angular momentum  $S$  on  $AdS_3$ , the string energy could be computed to first orders in the strong coupling expansion [22,17,23,70,24] (see also [20,21]), this provides the prediction for the scaling function

$$f(g) = 4g - \frac{3 \log 2}{\pi} - \frac{K}{4\pi^2} \frac{1}{g} + \dots, \quad (4.1)$$

where  $K$  is Catalan's constant. It is thus desirable to solve (2.11) at strong coupling. This however turned out to be a lot harder than first expected. The integral equation was shown to reproduce the first two orders in the strong coupling expansion numerically with

high accuracy [72]. Despite this a straightforward expansion gives only the leading term in (4.1) analytically, already the first subleading term could not be obtained analytically this way. With considerable effort the first subleading term was reproduced by solving the Bethe equations [30, 73], however this was done by first expanding the equations at strong coupling and then taking the large spin limit and hence not by solving the integral equation (2.11). This approach can not easily be continued to include higher orders in the expansion. Some important progress towards solving the integral equation, analytical as well as numerical, was made in [26, 27, 74, 28] and the final solution was then presented in [29] and further discussed in [31, 32].

In order to solve (2.11) at strong coupling it proved useful to split the density as

$$\frac{e^t - 1}{t} \hat{\sigma}(t) = \frac{\gamma_+(2gt)}{2gt} + \frac{\gamma_-(2gt)}{2gt} \quad (4.2)$$

and expand the even and odd part in Neumann series [26, 29]

$$\begin{aligned} \gamma_+(t) &= \sum_{k=1}^{\infty} (-1)^{k+1} 2k J_{2k}(t) \gamma_{2k} \\ \gamma_-(t) &= \sum_{k=1}^{\infty} (-1)^{k+1} (2k-1) J_{2k-1}(t) \gamma_{2k-1}. \end{aligned} \quad (4.3)$$

Applying the density split (4.2) in (2.11) the equation can be decomposed into an even and an odd part [74, 75, 29]. Introducing a further change of variables,

$$\Gamma(t) = \left( 1 + i \coth \frac{t}{4g} \right) \gamma(t) \quad (4.4)$$

where  $\Gamma(t) = \Gamma_+(t) + i\Gamma_-(t)$  and  $\gamma(t) = \gamma_+(t) + i\gamma_-(t)$ , it is possible to collect all dependence on the coupling constant in  $\Gamma_{\pm}(t)$  and (2.11) is rewritten as the system

$$\begin{aligned} \int_0^{\infty} \frac{dt}{t} (\Gamma_+(t) + \Gamma_-(t)) J_{2n}(t) &= 0 \\ \int_0^{\infty} \frac{dt}{t} (\Gamma_-(t) - \Gamma_+(t)) J_{2n-1}(t) &= \delta_{n,1}. \end{aligned} \quad (4.5)$$

The coupling constant dependence of the functions  $\Gamma_{\pm}(t)$  is determined by requiring the correct analyticity properties of the functions, which follows from (4.4) and (4.3). (4.4) can be rewritten and expanded as [32]

$$\Gamma(it) = \frac{\sin(\frac{t}{4g} + \frac{\pi}{4})}{\sin(\frac{t}{4g}) \sin(\frac{\pi}{4})} \gamma(it) = \gamma(it) \sqrt{2} \prod_{k=-\infty}^{\infty} \frac{t - 4\pi g(k - 1/4)}{t - 4\pi gk}. \quad (4.6)$$

From this one can conclude [31, 32] that  $\Gamma(it)$  has an infinite set of zeros and poles given by

$$t_{zero} = 4\pi g(l - 1/4), \quad l \in \mathbb{Z} \quad (4.7)$$

$$t_{pole} = 4\pi gl', \quad l' \in \mathbb{Z}, l' \neq 0. \quad (4.8)$$

To construct the general solution to the integral equations we will consider the inverse Fourier transform of  $\Gamma(t)$ ,  $\Gamma(u) = \int_{-\infty}^{\infty} \frac{dt}{2\pi} e^{iut} \Gamma(t)$ . From (4.6) follows

$$\Gamma(u) = \int_{-\infty}^{\infty} \frac{dt}{2\pi} e^{iut} \frac{\sinh(\frac{t}{4g} + i\frac{\pi}{4})}{\sin(\frac{t}{4g}) \sin(\frac{\pi}{4})} \gamma(t). \quad (4.9)$$

This integral can be computed by deforming the contour, picking up the residues of the poles along the imaginary axis. This can however only be done if the integrand vanishes at infinity. Since  $\gamma(t)$  admits a Neumann expansion we can conclude that  $\gamma(u) = 0$  for  $u^2 > 1$ , using the property of the Bessel functions that  $\int_{-\infty}^{\infty} \frac{dt}{2\pi} e^{iut} J_n(t) = 0$  for  $u^2 > 1$ . This means that  $\gamma(t) \sim e^{|t|}$  for large complex  $t$  as  $|t| \rightarrow \infty$  and hence the above integral can be computed by deforming the contour when  $u^2 > 1$ , the result is

$$\Gamma(u) = \theta(u-1) \sum_{n=1}^{\infty} c_+(n, g) e^{-4\pi n g (u-1)} + \theta(-u-1) \sum_{n=1}^{\infty} c_-(n, g) e^{-4\pi n g (-u-1)} \quad (4.10)$$

where  $c_{\pm}(n, g) = \mp 4g\gamma(\pm 4\pi i g n) e^{-4\pi n g}$ . To find  $\Gamma(u)$  for  $-1 \leq u \leq 1$  we will make an attempt to solve the equations (4.5). Before doing that we note that the infinite system in (4.5) can be rewritten as two equations with an additional arbitrary parameter  $\phi$  by applying the relation derived from the Jacobi-Anger identity,

$$e^{it \sin \phi} = \frac{2}{\cos \phi} \sum_{n=1}^{\infty} \left( \frac{J_{2n-1}(t)}{t} (2n-1) \cos((2n-1)\phi) + i \frac{J_{2n}(t)}{t} 2n \sin(2n\phi) \right). \quad (4.11)$$

Using the notation  $u = \sin \phi$  we find for  $-1 \leq u \leq 1$

$$\int_0^{\infty} dt (e^{itu} \Gamma_-(t) - e^{-itu} \Gamma_+(t)) = 2. \quad (4.12)$$

In terms of  $\Gamma(u)$  this equation can be expressed as

$$\Gamma(u) + \frac{1}{\pi} \int_{-1}^1 dv \frac{\Gamma(v)}{v-u} = \Phi(u) \quad (4.13)$$

$$\Phi(u) = -\frac{1}{\pi} \left( 2 + \int_{-\infty}^{-1} dv \frac{\Gamma(v)}{v-u} + \int_1^{\infty} dv \frac{\Gamma(v)}{v-u} \right). \quad (4.14)$$

In  $\Phi(u)$  one can use the solution (4.10) and solving the above equation renders a solution in terms of  $c_{\pm}(n, g)$ , valid in the interval  $-1 \leq u \leq 1$ . Since this solution together with (4.10) determines the function  $\Gamma(u)$  for all values of  $u$  it is now finally possible to go back to the Fourier transform and find an expression for  $\Gamma(it)$ , we refer to [32] for details.

The general solution is expressed in terms of the functions of the coupling constant  $c_{\pm}(n, g)$ . These are completely determined by requiring the correct analyticity properties of the function  $\Gamma(it)$ , requiring that the function has zeros according to (4.7) we find the so called quantisation conditions.

These conditions determine  $c_{\pm}(n, g)$  and the solution for all values of the coupling constant. Expanding the quantization condition at strong coupling one finds, to leading orders,

$$c_+(n, g) = (8\pi gn)^{1/4} \frac{2\Gamma(n+1/4)}{\Gamma(n+1)\Gamma^2(1/4)} \left( 1 - \frac{1}{g} \left( \frac{3 \log 2}{4} + \frac{3}{32n} + \dots \right) \right) \quad (4.15)$$

$$c_-(n, g) = (8\pi gn)^{1/4} \frac{\Gamma(n+3/4)}{2\Gamma(n+1)\Gamma^2(3/4)} \left( 1 + \frac{1}{g} \left( \frac{3 \log 2}{4} + \frac{5}{32n} + \dots \right) \right). \quad (4.16)$$

Finally the scaling function is written in terms of  $c_{\pm}(n, g)$  and from this the strong coupling expansion (4.1) follows.

It is also possible to continue this expansion to many more orders in the coupling constant [29] (see also [76] for a Mathematica code that generates the expansion). The first orders above are the ones that have been checked against the semiclassical quantisation of the string sigma model, comparison of further terms remains a challenge.

Solving the integral equation for subleading corrections in the large spin expansion at strong coupling turns out to be straightforward once the analysis for the leading term is completed. It is possible to write the first subleading terms in terms of the leading solution. The coefficients  $c_{\pm}(n, g)$  determine the anomalous dimension to order  $\mathcal{O}(\frac{1}{(\log M)^k})$ ,  $k \rightarrow \infty$  for general values of  $L$  and up to order  $\mathcal{O}((\frac{\log M}{M})^2)$  for  $L = 2, 3$ . It is interesting to note that when evaluating the subleading terms at strong coupling one finds that the expansion reorganises in terms of the parameter  $M/g$  [39]. This is fully consistent with the computation done in string theory where  $S/g$  is kept fixed expanding for large  $g$  and then subsequently taken large. For twist two the string result [77] is reproduced from the Bethe ansatz, since the computation is done by resumming all orders in the weak coupling expansion this gives a strong indication that wrapping plays no role for these first orders in the large  $M$  expansion.

As for the weak coupling expansion reciprocity is suggested to hold for the all loop anomalous dimension. The energy of the dual string solutions exhibits the same structure as the anomalous dimensions (2.16) and reciprocity is verified at strong coupling [61, 77, 24]. Indeed this is also confirmed by the structure obtained by solving the integral equations that follow from the asymptotic Bethe equations up to  $\mathcal{O}((\frac{\log M}{M})^2)$  [39].

Thanks to the method developed to treat the strong coupling expansion of the BES equation also other closely related integral equations, corresponding to operators belonging to other larger sectors of the theory, could be solved [78] and the anomalous dimensions matched to the corresponding string states [20]. This was possible because the kernels coincided with the BES kernel. In sectors where that is not the case the strong coupling solutions of integral equations derived from the Bethe equations remain a challenge [79].

## 5 Non-perturbative corrections and intermediate values of the coupling constant

The quantization condition as well as the expression for the scaling function in terms of the functions  $c_{\pm}(n, g)$  are valid for all values of the coupling constant. The equations

do not admit a solution on a closed form for arbitrary coupling but numerically it is however possible to find a solution for any value of the coupling constant which indeed demonstrates a smoothly interpolating scaling function [29, 80, 32]. The strong coupling expansion in (4.1) defines an asymptotic series and is non-Borel summable. The reason for this is that when expanding the quantization conditions at strong coupling we have not taken non-perturbative corrections into account. Using the construction in the previous section and expanding the quantisation conditions, retaining the non-perturbative corrections, it is found to leading orders [32]

$$f(g) = 4g - \frac{3 \log 2}{\pi} - \frac{K}{4\pi^2 g} + \mathcal{O}(1/g^2) - \frac{2\Lambda^2}{\pi^2} \left( 1 + \frac{3 - 6 \log 2}{16\pi g} + \mathcal{O}(1/g^2) \right) + \mathcal{O}(\Lambda^4) \quad (5.1)$$

where

$$\Lambda^2 = \sigma \frac{1}{\sqrt{2\pi g}} e^{-2\pi g} \frac{\Gamma(\frac{3}{4})}{\Gamma(\frac{5}{4})} \quad (5.2)$$

defines the non-perturbative scale. The non-perturbative corrections can be organised in terms of the mass of the  $O(6)$ -model

$$m_{O(6)} = \frac{4\sqrt{2}}{\pi\sigma} \Lambda^2 \left( 1 + \frac{3 - 6 \log 2}{16\pi g} + \mathcal{O}(1/g^2) \right) + \mathcal{O}(\Lambda^4). \quad (5.3)$$

Note that the series in  $1/g$  in (5.1) is not Borel summable. It is only the series in  $1/g$  together with the expansion in  $\Lambda^2$  that is Borel summable. The complex parameter  $\sigma$  appearing in the expansion is determined by the way the series in  $1/g$  is regularised, alternatively on the renormalisation scheme used in the  $O(6)$ -model.

The cusp anomalous dimension appears also in the leading order of the large  $M$  expansion of twist operators with  $L = j \log M$ , where  $j$  is some finite number. The leading order is governed by the the so called generalised scaling function of which the scaling function constitutes a part [14, 81, 36, 82, 83],

$$\gamma(g, j, M) = (f(g) + \epsilon(g, j)) \log M. \quad (5.4)$$

The function  $\epsilon(g, j)$  denotes the twist dependent part of the generalised scaling function. The string duals are folded strings spinning with one angular momentum,  $S$  identified with  $M$ , in  $AdS_5$  and one angular momentum,  $J \propto \log S$  identified with  $L$ , on  $S^5$ . The energy of the string solutions was obtained directly from the string sigma model to two-loops in the sigma model loop expansion, see [84] and references therein. The string sigma model with  $J \sim \log S$ ,  $S$  and  $g$  taken large reduces to the  $O(6)$  model [81]. This corresponds to a low energy limit in which only the massless excitations around the classical solution remain. These massless fields describe the  $O(6)$  model and as a result the sigma model can be completely solved in this limit. The limit can also be considered from the gauge theory side using the asymptotic Bethe equations [36] where the relation to the sigma model was explicitly demonstrated in [82] and further studied in [85, 83, 86]. The generalised scaling function is hence associated with the free energy of the  $O(6)$ -sigma model, a quantity that receives non-perturbative corrections in terms of the mass scale of the sigma model  $m_{O(6)}$ .

In [32] it was demonstrated that the non-perturbative scale appearing in the strong coupling expansion of the scaling function is related to the non-perturbative scale, the mass gap, in the  $O(6)$ -model. In fact the mass scale that can be identified in  $f(g)$  is identical to  $m_{O(6)}$  to all orders in the strong coupling expansion.

## References

- [1] R. Janik, “*Review of AdS/CFT Integrability, Chapter III.5: Lüscher corrections*”, [arxiv:1012.3994](#).
- [2] V. Kazakov and N. Gromov, “*Review of AdS/CFT Integrability, Chapter III.7: Hirota Dynamics for Quantum Integrability*”, [arxiv:1012.3996](#). • Z. Bajnok, “*Review of AdS/CFT Integrability, Chapter III.6: Thermodynamic Bethe Ansatz*”, [arxiv:1012.3995](#).
- [3] G. Korchemsky, “*Review of AdS/CFT Integrability, Chapter IV.4: Integrability in QCD and  $\mathcal{N} < 4$  SYM*”, [arxiv:1012.4000](#).
- [4] M. Staudacher, “*Review of AdS/CFT Integrability, Chapter III.1: Bethe Ansätze and the R-Matrix Formalism*”, [arxiv:1012.3990](#). • C. Ahn and R. I. Nepomechie, “*Review of AdS/CFT Integrability, Chapter III.2: Exact world-sheet S-matrix*”, [arxiv:1012.3991](#).
- [5] P. Vieira and D. Volin, “*Review of AdS/CFT Integrability, Chapter III.3: The dressing factor*”, [arxiv:1012.3992](#).
- [6] M. Staudacher, “*The factorized S-matrix of CFT/AdS*”, JHEP 0505, 054 (2005), [hep-th/0412188](#). • N. Beisert and M. Staudacher, “*Long-range PSU(2,2/4) Bethe ansätze for gauge theory and strings*”, Nucl. Phys. B727, 1 (2005), [hep-th/0504190](#).
- [7] R. A. Janik, “*The AdS<sub>5</sub> × S<sup>5</sup> superstring worldsheet S-matrix and crossing symmetry*”, Phys. Rev. D73, 086006 (2006), [hep-th/0603038](#). • C. Gomez and R. Hernandez, “*The magnon kinematics of the AdS/CFT correspondence*”, JHEP 0611, 021 (2006), [hep-th/0608029](#). • J. Plefka, F. Spill and A. Torrielli, “*On the Hopf algebra structure of the AdS/CFT S-matrix*”, Phys. Rev. D74, 066008 (2006), [hep-th/0608038](#).
- [8] B. Eden and M. Staudacher, “*Integrability and transcendentality*”, J. Stat. Mech. 0611, P014 (2006), [hep-th/0603157](#).
- [9] N. Beisert, B. Eden and M. Staudacher, “*Transcendentality and crossing*”, J. Stat. Mech. 0701, P021 (2007), [hep-th/0610251](#).
- [10] C. Anastasiou, Z. Bern, L. J. Dixon and D. A. Kosower, “*Planar amplitudes in maximally supersymmetric Yang-Mills theory*”, Phys. Rev. Lett. 91, 251602 (2003), [hep-th/0309040](#). • Z. Bern, L. J. Dixon and V. A. Smirnov, “*Iteration of planar amplitudes in maximally supersymmetric Yang-Mills theory at three loops and beyond*”, Phys. Rev. D72, 085001 (2005), [hep-th/0505205](#).
- [11] Z. Bern, M. Czakon, L. J. Dixon, D. A. Kosower and V. A. Smirnov, “*The Four-Loop Planar Amplitude and Cusp Anomalous Dimension in Maximally Supersymmetric Yang-Mills Theory*”, Phys. Rev. D75, 085010 (2007), [hep-th/0610248](#).
- [12] D. Volin, “*Minimal solution of the AdS/CFT crossing equation*”, [arxiv:0904.4929](#).

- [13] J. C. Collins, “*Sudakov form factors*”, Adv. Ser. Direct. High Energy Phys. 5, 573 (1989), hep-ph/0312336.
- [14] A. V. Belitsky, A. S. Gorsky and G. P. Korchemsky, “*Logarithmic scaling in gauge / string correspondence*”, Nucl. Phys. B748, 24 (2006), hep-th/0601112.
- [15] G. P. Korchemsky and A. V. Radyushkin, “*Loop space formalism and renormalization group for the infrared asymptotics of QCD*”, Phys. Lett. B171, 459 (1986).
- [16] G. P. Korchemsky, “*Asymptotics of the Altarelli-Parisi-Lipatov Evolution Kernels of Parton Distributions*”, Mod. Phys. Lett. A4, 1257 (1989). • G. P. Korchemsky and G. Marchesini, “*Structure function for large  $x$  and renormalization of Wilson loop*”, Nucl. Phys. B406, 225 (1993), hep-ph/9210281.
- [17] M. Kruczenski, “*A note on twist two operators in  $N = 4$  SYM and Wilson loops in Minkowski signature*”, JHEP 0212, 024 (2002), hep-th/0210115.
- [18] L. F. Alday and J. M. Maldacena, “*Gluon scattering amplitudes at strong coupling*”, JHEP 0706, 064 (2007), arxiv:0705.0303.
- [19] C. Sieg, “*Review of AdS/CFT Integrability, Chapter I.2: The spectrum from perturbative gauge theory*”, arxiv:1012.3984.
- [20] A. Tseytlin, “*Review of AdS/CFT Integrability, Chapter II.1: Classical  $AdS_5 \times S^5$  string solutions*”, arxiv:1012.3986.
- [21] T. McLoughlin, “*Review of AdS/CFT Integrability, Chapter II.2: Quantum Strings in  $AdS_5 \times S^5$* ”, arxiv:1012.3987.
- [22] S. S. Gubser, I. R. Klebanov and A. M. Polyakov, “*A semi-classical limit of the gauge/string correspondence*”, Nucl. Phys. B636, 99 (2002), hep-th/0204051. • S. Frolov and A. A. Tseytlin, “*Semiclassical quantization of rotating superstring in  $AdS(5) \times S(5)$* ”, JHEP 0206, 007 (2002), hep-th/0204226.
- [23] R. Roiban, A. Tirziu and A. A. Tseytlin, “*Two-loop world-sheet corrections in  $AdS_5 \times S^5$  superstring*”, JHEP 0707, 056 (2007), arxiv:0704.3638. • R. Roiban and A. A. Tseytlin, “*Strong-coupling expansion of cusp anomaly from quantum superstring*”, JHEP 0711, 016 (2007), arxiv:0709.0681.
- [24] M. Beccaria, G. V. Dunne, V. Forini, M. Pawellek and A. A. Tseytlin, “*Exact computation of one-loop correction to energy of spinning folded string in  $AdS_5 \times S^5$* ”, arxiv:1001.4018.
- [25] A. V. Kotikov and L. N. Lipatov, “*On the highest transcendentality in  $\mathcal{N} = 4$  SUSY*”, Nucl. Phys. B769, 217 (2007), hep-th/0611204.
- [26] L. F. Alday, G. Arutyunov, M. K. Benna, B. Eden and I. R. Klebanov, “*On the strong coupling scaling dimension of high spin operators*”, JHEP 0704, 082 (2007), hep-th/0702028.
- [27] I. Kostov, D. Serban and D. Volin, “*Strong coupling limit of Bethe ansatz equations*”, Nucl. Phys. B789, 413 (2008), hep-th/0703031.
- [28] M. Beccaria, G. F. De Angelis and V. Forini, “*The scaling function at strong coupling from the quantum string Bethe equations*”, JHEP 0704, 066 (2007), hep-th/0703131.
- [29] B. Basso, G. P. Korchemsky and J. Kotanski, “*Cusp anomalous dimension in maximally supersymmetric Yang-Mills theory at strong coupling*”, Phys. Rev. Lett. 100, 091601 (2008), arxiv:0708.3933.

- [30] P. Y. Casteill and C. Kristjansen, “*The Strong Coupling Limit of the Scaling Function from the Quantum String Bethe Ansatz*”, Nucl. Phys. B785, 1 (2007), arxiv:0705.0890.
- [31] I. Kostov, D. Serban and D. Volin, “*Functional BES equation*”, JHEP 0808, 101 (2008), arxiv:0801.2542.
- [32] B. Basso and G. P. Korchemsky, “*Nonperturbative scales in AdS/CFT*”, J. Phys. A42, 254005 (2009), arxiv:0901.4945.
- [33] A. V. Belitsky, A. S. Gorsky and G. P. Korchemsky, “*Gauge / string duality for QCD conformal operators*”, Nucl. Phys. B667, 3 (2003), hep-th/0304028.
- [34] A. V. Belitsky, G. P. Korchemsky and R. S. Pasechnik, “*Fine structure of anomalous dimensions in  $\mathcal{N} = 4$  super Yang-Mills theory*”, Nucl. Phys. B809, 244 (2009), arxiv:0806.3657.
- [35] G. P. Korchemsky, “*Quasiclassical QCD pomeron*”, Nucl. Phys. B462, 333 (1996), hep-th/9508025.
- [36] L. Freyhult, A. Rej and M. Staudacher, “*A Generalized Scaling Function for AdS/CFT*”, J. Stat. Mech. 0807, P07015 (2008), arxiv:0712.2743.
- [37] G. Feverati, D. Fioravanti, P. Grinza and M. Rossi, “*On the finite size corrections of anti-ferromagnetic anomalous dimensions in  $\mathcal{N} = 4$  SYM*”, JHEP 0605, 068 (2006), hep-th/0602189. • G. Feverati, D. Fioravanti, P. Grinza and M. Rossi, “*Hubbard’s adventures in  $\mathcal{N} = 4$  SYM-land? Some non-perturbative considerations on finite length operators*”, J. Stat. Mech. 0702, P001 (2007), hep-th/0611186. • D. Fioravanti and M. Rossi, “*On the commuting charges for the highest dimension  $SU(2)$  operator in planar  $\mathcal{N} = 4$  SYM*”, JHEP 0708, 089 (2007), arxiv:0706.3936. • D. Bombardelli, D. Fioravanti and M. Rossi, “*Non-linear integral equations in  $\mathcal{N} = 4$  SYM*”, arxiv:0711.2934.
- [38] D. Bombardelli, D. Fioravanti and M. Rossi, “*Large spin corrections in  $\mathcal{N} = 4$  SYM  $sl(2)$ : still a linear integral equation*”, Nucl. Phys. B810, 460 (2009), arxiv:0802.0027.
- [39] L. Freyhult and S. Zieme, “*The virtual scaling function of AdS/CFT*”, Phys. Rev. D79, 105009 (2009), arxiv:0901.2749.
- [40] D. Fioravanti, P. Grinza and M. Rossi, “*On the logarithmic powers of  $sl(2)$   $SYM_4$* ”, arxiv:0911.2425.
- [41] A. V. Kotikov and L. N. Lipatov, “*DGLAP and BFKL evolution equations in the  $N=4$  supersymmetric gauge theory*”, Nucl. Phys. B661, 19 (2003), hep-ph/0208220.
- [42] H. Georgi and H. D. Politzer, “*Electroproduction scaling in an asymptotically free theory of strong interactions*”, Phys. Rev. D9, 416 (1974). • D. J. Gross and F. Wilczek, “*Asymptotically Free Gauge Theories. 1*”, Phys. Rev. D8, 3633 (1973). • F. A. Dolan and H. Osborn, “*Conformal four point functions and the operator product expansion*”, Nucl. Phys. B599, 459 (2001), hep-th/0011040.
- [43] A. V. Kotikov, L. N. Lipatov and V. N. Velizhanin, “*Anomalous dimensions of Wilson operators in  $N = 4$  SYM theory*”, Phys. Lett. B557, 114 (2003), hep-ph/0301021.
- [44] A. V. Kotikov, L. N. Lipatov, A. I. Onishchenko and V. N. Velizhanin, “*Three-loop universal anomalous dimension of the Wilson operators in  $\mathcal{N} = 4$  SUSY Yang-Mills model*”, Phys. Lett. B595, 521 (2004), hep-th/0404092.

- [45] S. Moch, J. A. M. Vermaseren and A. Vogt, “*The three-loop splitting functions in QCD: The non-singlet case*”, Nucl. Phys. B688, 101 (2004), hep-ph/0403192.
- [46] J. Vermaseren, “*Harmonic sums, Mellin transforms and integrals*”, Int.J.Mod.Phys. A14, 2037 (1999), hep-ph/9806280.
- [47] M. Beccaria, “*Anomalous dimensions at twist-3 in the  $sl(2)$  sector of  $\mathcal{N} = 4$  SYM*”, JHEP 0706, 044 (2007), arxiv:0704.3570.
- [48] A. V. Kotikov, L. N. Lipatov, A. Rej, M. Staudacher and V. N. Velizhanin, “*Dressing and Wrapping*”, J. Stat. Mech. 0710, P10003 (2007), arxiv:0704.3586.
- [49] M. Beccaria, Y. L. Dokshitzer and G. Marchesini, “*Twist 3 of the  $sl(2)$  sector of  $\mathcal{N} = 4$  SYM and reciprocity respecting evolution*”, Phys. Lett. B652, 194 (2007), arxiv:0705.2639.
- [50] M. Beccaria, V. Forini, T. Lukowski and S. Zieme, “*Twist-three at five loops, Bethe Ansatz and wrapping*”, JHEP 0903, 129 (2009), arxiv:0901.4864.
- [51] T. Lukowski, A. Rej and V. N. Velizhanin, “*Five-Loop Anomalous Dimension of Twist-Two Operators*”, arxiv:0912.1624.
- [52] M. Beccaria and F. Catino, “*Sum rules for higher twist  $sl(2)$  operators in  $\mathcal{N} = 4$  SYM*”, JHEP 0806, 103 (2008), arxiv:0804.3711.
- [53] S. E. Derkachov, G. P. Korchemsky and A. N. Manashov, “*Evolution equations for quark gluon distributions in multi-color QCD and open spin chains*”, Nucl. Phys. B566, 203 (2000), hep-ph/9909539.
- [54] A. V. Belitsky, G. P. Korchemsky and D. Mueller, “*Towards Baxter equation in supersymmetric Yang-Mills theories*”, Nucl. Phys. B768, 116 (2007), hep-th/0605291. • A. V. Belitsky, “*Long-range  $SL(2)$  Baxter equation in  $\mathcal{N} = 4$  super-Yang-Mills theory*”, Phys. Lett. B643, 354 (2006), hep-th/0609068. • A. V. Belitsky, “*Baxter equation beyond wrapping*”, Phys. Lett. B677, 93 (2009), arxiv:0902.3198.
- [55] A. V. Kotikov, A. Rej and S. Zieme, “*Analytic three-loop Solutions for  $\mathcal{N} = 4$  SYM Twist Operators*”, Nucl. Phys. B813, 460 (2009), arxiv:0810.0691.
- [56] M. Beccaria, A. V. Belitsky, A. V. Kotikov and S. Zieme, “*Analytic solution of the multiloop Baxter equation*”, arxiv:0908.0520.
- [57] E. Kuraev, L. Lipatov and V. S. Fadin, “*The Pomernanchuk Singularity in Nonabelian Gauge Theories*”, Sov.Phys.JETP 45, 199 (1977). • I. Balitsky and L. Lipatov, “*The Pomernanchuk Singularity in Quantum Chromodynamics*”, Sov.J.Nucl.Phys. 28, 822 (1978).
- [58] Z. Bajnok, R. A. Janik and T. Lukowski, “*Four loop twist two, BFKL, wrapping and strings*”, Nucl. Phys. B816, 376 (2009), arxiv:0811.4448.
- [59] M. Beccaria and V. Forini, “*Four loop reciprocity of twist two operators in  $\mathcal{N} = 4$  SYM*”, JHEP 0903, 111 (2009), arxiv:0901.1256.
- [60] Y. L. Dokshitzer, G. Marchesini and G. P. Salam, “*Revisiting parton evolution and the large- $x$  limit*”, Phys. Lett. B634, 504 (2006), hep-ph/0511302.
- [61] B. Basso and G. P. Korchemsky, “*Anomalous dimensions of high-spin operators beyond the leading order*”, Nucl. Phys. B775, 1 (2007), hep-th/0612247.

- [62] Y. L. Dokshitzer and G. Marchesini, “ $\mathcal{N} = 4$  SUSY Yang-Mills: Three loops made simple( $r$ )”, Phys. Lett. B646, 189 (2007), [hep-th/0612248](#).
- [63] M. Beccaria, V. Forini and G. Macorini, “Generalized Gribov-Lipatov Reciprocity and AdS/CFT”, [arxiv:1002.2363](#).
- [64] V. M. Braun, G. P. Korchemsky and D. Mueller, “The uses of conformal symmetry in QCD”, Prog. Part. Nucl. Phys. 51, 311 (2003), [hep-ph/0306057](#).
- [65] M. Beccaria and V. Forini, “Reciprocity of gauge operators in  $\mathcal{N} = 4$  SYM”, JHEP 0806, 077 (2008), [arxiv:0803.3768](#).
- [66] V. N. Gribov and L. N. Lipatov, “ $e^+ e^-$  pair annihilation and deep inelastic  $e p$  scattering in perturbation theory”, Sov. J. Nucl. Phys. 15, 675 (1972).
- [67] A. Vogt, S. Moch and J. A. M. Vermaseren, “The three-loop splitting functions in QCD: The singlet case”, Nucl. Phys. B691, 129 (2004), [hep-ph/0404111](#).
- [68] M. Beccaria, “Universality of three gaugino anomalous dimensions in  $\mathcal{N} = 4$  SYM”, JHEP 0706, 054 (2007), [arxiv:0705.0663](#).
- [69] M. Beccaria, “Three loop anomalous dimensions of twist-3 gauge operators in  $\mathcal{N} = 4$  SYM”, JHEP 0709, 023 (2007), [arxiv:0707.1574](#).
- [70] S. Giombi, R. Ricci, R. Roiban, A. A. Tseytlin and C. Vergu, “Quantum  $AdS_5 \times S^5$  superstring in the AdS light-cone gauge”, [arxiv:0912.5105](#).
- [71] T. Klose, “Review of AdS/CFT Integrability, Chapter IV.3:  $\mathcal{N} = 6$  Chern-Simons and Strings on  $AdS_4 \times CP^3$ ”, [arxiv:1012.3999](#).
- [72] M. K. Benna, S. Benvenuti, I. R. Klebanov and A. Scardicchio, “A test of the AdS/CFT correspondence using high-spin operators”, Phys. Rev. Lett. 98, 131603 (2007), [hep-th/0611135](#).
- [73] A. V. Belitsky, “Strong coupling expansion of Baxter equation in  $\mathcal{N} = 4$  SYM”, Phys. Lett. B659, 732 (2008), [arxiv:0710.2294](#).
- [74] A. V. Kotikov and L. N. Lipatov, “Eden-Staudacher and Beisert-Eden-Staudacher equations in the  $\mathcal{N} = 4$  supersymmetric gauge theory”, Theor. Math. Phys. 155, 606 (2008).
- [75] B. Eden, “The BES equation and its strong coupling limit”, Talk at 12th Itzykson meeting, Saclay/Paris.
- [76] D. Volin, “Quantum integrability and functional equations”, [arxiv:1003.4725](#).
- [77] M. Beccaria, V. Forini, A. Tirziu and A. A. Tseytlin, “Structure of large spin expansion of anomalous dimensions at strong coupling”, Nucl. Phys. B812, 144 (2009), [arxiv:0809.5234](#).
- [78] B. Basso, “Exciting the GKP string at any coupling”, [arxiv:1010.5237](#). • L. Freyhult, A. Rej and S. Zieme, “From weak coupling to spinning strings”, [arxiv:0911.2458](#).
- [79] A. Rej, M. Staudacher and S. Zieme, “Nesting and dressing”, J. Stat. Mech. 0708, P08006 (2007), [hep-th/0702151](#).
- [80] J. Kotanski, “Cusp anomalous dimension in maximally supersymmetric Yang-Mills theory”, Acta Phys. Polon. B39, 3127 (2008), [arxiv:0811.2667](#).

- [81] L. F. Alday and J. M. Maldacena, “*Comments on operators with large spin*”, JHEP 0711, 019 (2007), [arxiv:0708.0672](#).
- [82] B. Basso and G. P. Korchemsky, “*Embedding nonlinear  $O(6)$  sigma model into  $\mathcal{N} = 4$  super-Yang-Mills theory*”, Nucl. Phys. B807, 397 (2009), [arxiv:0805.4194](#).
- [83] Z. Bajnok, J. Balog, B. Basso, G. P. Korchemsky and L. Palla, “*Scaling function in AdS/CFT from the  $O(6)$  sigma model*”, Nucl. Phys. B811, 438 (2009), [arxiv:0809.4952](#).
- [84] S. Giombi, R. Ricci, R. Roiban, A. A. Tseytlin and C. Vergu, “*Generalized scaling function from light-cone gauge  $AdS_5 \times S^5$  superstring*”, [arxiv:1002.0018](#).
- [85] D. Fioravanti, P. Grinza and M. Rossi, “*The generalised scaling function: a note*”, [arxiv:0805.4407](#). • F. Buccheri and D. Fioravanti, “*The integrable  $O(6)$  model and the correspondence: checks and predictions*”, [arxiv:0805.4410](#). • N. Gromov, “*Generalized Scaling Function at Strong Coupling*”, JHEP 0811, 085 (2008), [arxiv:0805.4615](#). • M. Beccaria, “*The generalized scaling function of AdS/CFT and semiclassical string theory*”, JHEP 0807, 082 (2008), [arxiv:0806.3704](#). • D. Fioravanti, P. Grinza and M. Rossi, “*The generalised scaling function: a systematic study*”, [arxiv:0808.1886](#).
- [86] D. Volin, “*The 2-loop generalized scaling function from the BES/FRS equation*”, [arxiv:0812.4407](#).



# Review of AdS/CFT Integrability, Chapter III.5: Lüscher corrections

ROMUALD A. JANIK

*Institute of Physics  
Jagiellonian University  
ul. Reymonta 4  
30-059 Kraków  
Poland*

romuald@th.if.uj.edu.pl

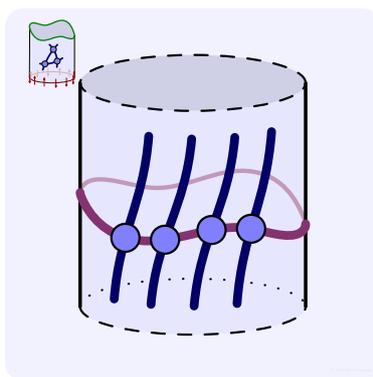

**Abstract:** In integrable quantum field theories the large volume spectrum is given by the Bethe Ansatz. The leading corrections, due to virtual particles circulating around the cylinder, are encoded in so-called Lüscher corrections. In order to apply these techniques to the AdS/CFT correspondence one has to generalize these corrections to the case of generic dispersion relations and to multiparticle states. We review these various generalizations and the applications of Lüscher's corrections to the study of the worldsheet QFT of the superstring in  $AdS_5 \times S^5$  and, consequently, to anomalous dimensions of operators in  $\mathcal{N} = 4$  SYM theory.

# 1 Introduction

For many integrable systems the main question that one is interested in is the understanding of the energy spectrum for the system of a given size  $L$ . The size of the system in question may be discrete, like the number of sites of a spin chain or other kind of lattice system, or continuous, like the circumference of a cylinder on which a given integrable field theory is defined.

The first answer to this question for a wide variety of integrable systems is generically given in terms of Bethe equations. These are equations for a set of (complex) numbers  $p_i$  of the form

$$1 = e^{ip_j L} \prod_{k:k \neq j}^N S(p_j, p_k) \quad (1.1)$$

Once a solution  $\{p_j\}_{j=1..N}$  is found, the energy is obtained through an additive formula

$$E = \sum_{j=1}^N E(p_j) \quad (1.2)$$

where  $E(p)$  and  $S(p, p')$  are (known) functions characterizing the given integrable system. In practice, for generic integrable systems, these equations become the more complicated nested Bethe equations, with a system of equations instead of (1.1), with additional auxiliary unknowns appearing in (1.1) but not in the energy formula (1.2). All this is described in detail in two other chapters of this review [1].

Bethe equations of the type described above appear both in the case of discrete integrable spin chains and continuous two-dimensional integrable quantum field theories. Moreover they also appear as equations for the anomalous dimensions of single trace operators in the  $\mathcal{N} = 4$  four-dimensional SYM theory and in various other contexts.

Now comes the fundamental difference between the various classes of integrable systems. For integrable spin chains, like the Heisenberg XXX, XXZ etc. models, the Bethe ansatz equations are *exact* and the energies given by (1.2) are the exact eigenvalues of the spin chain hamiltonian. On the other hand, for two-dimensional integrable quantum field theories, the answer provided by (1.1) and (1.2) is only valid for asymptotically large sizes of the cylinder  $L$ . There are corrections which arise due to the quantum field theoretical nature of the system, namely virtual particles circulating around the cylinder and their interaction with the physical particles forming a given energy state. For a single particle in a relativistic QFT, Lüscher derived formulas [2] for the leading corrections. The goal of this chapter is to review the subsequent generalizations and applications of Lüscher corrections within the AdS/CFT correspondence. Let us note in passing that there may be also some intermediate cases like the Hubbard model as considered in [3], where the situation is not so clear.

Once one goes beyond these leading corrections by say decreasing the size of the system, one has to include the effects of multiple virtual corrections which becomes quite complicated, and have never been attempted so far. Fortunately, for integrable quantum field theories, there exists a technique of Thermodynamic Bethe Ansatz — TBA [4] (and/or Nonlinear Integral Equations — NLIE [5]), which allows for finding the

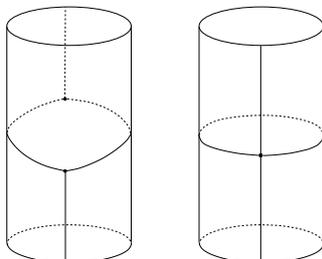

**Figure 1:** Spacetime interpretation of Lüscher's formulas —  $\mu$ -term (left) and F-term (right).

exact energy spectrum and thus effectively resumming all these virtual corrections. This is, however, technically very involved, so even for the cases where it is known, Lüscher corrections remain an efficient calculational tool. These exact treatments are described in the chapters [6] and [7] of this review.

As a final note, let us mention that for anomalous dimensions in the  $\mathcal{N} = 4$  SYM theory, the Bethe equations break down due to so-called wrapping interactions. This will be discussed in more detail in section 3 (see also the chapter [8]). Since according to the AdS/CFT correspondence anomalous dimensions are exactly equal to the energies of string states in  $AdS_5 \times S^5$ , which are just the energy levels of the two-dimensional integrable worldsheet quantum field theory, this violation of Bethe ansatz equations is in fact quite natural and can be quantitatively described using the formalism of Lüscher corrections for two dimensional QFT.

The plan of this chapter is as follows. First, after introducing Lüscher's original formulas, we will describe the various derivations of (generalized versions of) these formulas – a diagrammatic one, through a large volume expansion of TBA equations and through a Poisson resummation of quadratic fluctuations. Then we will review recent applications of generalized Lüscher corrections within the context of the AdS/CFT correspondence.

## 2 Lüscher formulas

Lüscher derived universal formulas for the leading large  $L$  mass shift (w.r.t. the particle mass in infinite volume) of a single particle state when the theory is put on a cylinder of size  $L$ . The universality means that the value of the leading correction is determined completely by the infinite volume S-matrix of the theory. This relation does not depend on integrability at all, and is even valid for arbitrary QFT's in higher number of dimensions, however it is most useful for two dimensional integrable field theories for which we very often know the exact analytical expression for the S-matrix.

The leading mass correction is given as a sum of two terms – the F-term

$$\Delta m_F(L) = -m \int_{-\infty}^{\infty} \frac{d\theta}{2\pi} e^{-mL \cosh \theta} \cosh \theta \sum_b \left( S_{ab}^{ab} \left( \theta + i\frac{\pi}{2} \right) - 1 \right) \quad (2.1)$$

and the  $\mu$ -term

$$\Delta m_\mu(L) = -\frac{\sqrt{3}}{2} m \sum_{b,c} M_{abc}(-i) \operatorname{res}_{\theta=2\pi i/3} S_{ab}^{ab}(\theta) \cdot e^{-\frac{\sqrt{3}}{2} mL} \quad (2.2)$$

quoted here, for simplicity, for a two dimensional theory with particles of the same mass [9].  $S_{ab}^{ab}(\theta)$  is the (infinite volume)  $S$ -matrix element, and  $M_{abc} = 1$  if  $c$  is a bound state of  $a$  and  $b$  and zero otherwise. These two terms have a distinct spacetime interpretation depicted in Figure 1. The F-term corresponds to the interaction of the physical particle with a virtual particle circulating around the cylinder, while the  $\mu$ -term corresponds to the splitting of the particle into two others which will then recombine after circulating around the cylinder.

In order to apply the above formulas to the case of the worldsheet QFT of the superstring in  $AdS_5 \times S^5$  (in generalized light cone gauge – see [10] for a detailed review), one has to generalize Lüscher’s original formulas in two directions.

Firstly, the worldsheet QFT is not relativistic. The dispersion relation for elementary excitations is

$$E(p) = \sqrt{1 + 16g^2 \sin^2 \frac{p}{2}} \quad (2.3)$$

and moreover, there is no analog of a Lorentz symmetry, which brings about the fact that the S-matrix is a nontrivial function of two independent momenta instead of just the rapidity difference  $\theta \equiv \theta_1 - \theta_2$  as in the case of relativistic theories. Secondly, due to the level matching condition of the string, the physical states, corresponding to operators in  $\mathcal{N} = 4$  SYM, have vanishing total momentum (or a multiple of  $2\pi$ ). Since single particle states with  $p = 0$  are protected by supersymmetry, all states interesting from the point of view of gauge theory are necessarily multiparticle states.

Consequently, one has to generalize Lüscher corrections to theories with quite generic dispersion relations and also to multiparticle states.

We will describe these generalizations at the same time showing how Lüscher corrections can be derived in many different and apparently unrelated ways.

## 2.1 Diagrammatic derivation

The diagrammatic derivation was the original one used by Lüscher in [2]. Its advantage is that it is the most general, does not assume integrability and is even valid in any number of dimensions. Its drawback, however, is that it is very difficult to generalize to multiparticle states or higher orders. On the other hand it is easy to extend to theories with generic dispersion relations which was done in [11]. We will present a sketch of this derivation here applicable to a theory with the dispersion relation

$$E^2 = \varepsilon^2(p) \quad (2.4)$$

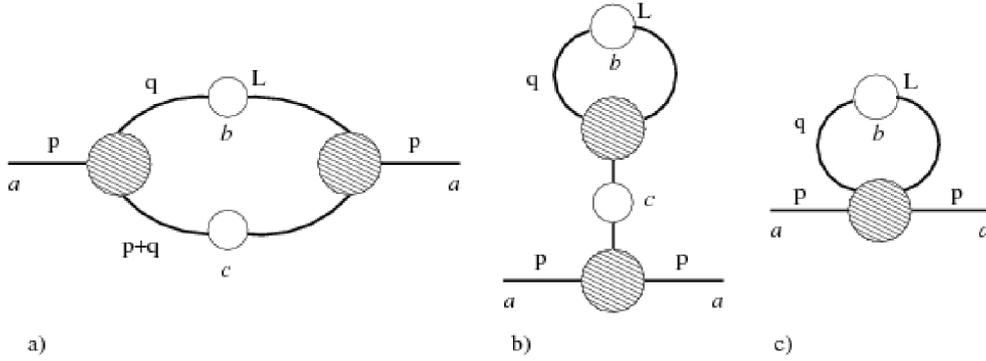

**Figure 2:** The graphs giving a leading finite size correction to the self energy: a)  $I_{abc}$ , b)  $J_{abc}$ , c)  $K_{ab}$ . The filled circles are the vertex functions  $\Gamma$ , empty circles represent the 2-point Green's function. The letter  $L$  represents the factor of  $e^{-iq^1 L}$  and the letters in italics label the type of particles.

which encompasses both the relativistic dispersion relation  $\varepsilon^2(p) = m^2 + p^2$ , as well as the AdS one  $\varepsilon^2(p) = 1 + 16g^2 \sin^2 p/2$ .

The starting point is the observation that the dispersion relation is encoded, as the mass shell condition, in the pole structure of the Green's function. Hence to find the leading large  $L$  corrections, one has to evaluate how the Green's function is modified at finite volume. It is convenient to translate the problem into a modification of the 1PI (1-particle irreducible) self energy defined by

$$G(p)^{-1} = \varepsilon_E^2 + \varepsilon^2(p) - \Sigma_L(p) \quad (2.5)$$

The renormalization scheme is fixed by requiring that the self energy and its first derivatives vanish on-shell (at infinite volume). The shift of the energy, following from (2.5) becomes

$$\delta\varepsilon_L = -\frac{1}{2\varepsilon(p)}\Sigma_L(p) \quad (2.6)$$

The propagator in a theory at fixed circumference can be obtained from the infinite volume one through averaging over translations  $x \rightarrow x + nL$ . In momentum space this will correspond to distributing factors of  $e^{inp^1 L}$  over all lines. In the next step, we assume, following [2, 9], that the dominant corrections at large  $L$  will be those graphs which have only a single such factor with  $n = \pm 1$ . Picking  $n = -1$  for definiteness, any such graph belongs to one of the three classes shown in Figure 2. Thus

$$\Sigma_L = \frac{1}{2} \left( \sum_{bc} I_{abc} + \sum_{bc} J_{abc} + \sum_b K_{ab} \right) \quad (2.7)$$

Now, one has to shift the contour of integration over the loop *spatial* momentum into the complex plane. Due to the exponent  $e^{-ip^1 L}$ , the integral over the shifted contour will be negligible and the main contribution will come from crossing a pole of a Green's function in one of the graphs of Figure 2. This is the crucial point for arriving at Lüscher's corrections. Taking the residue effectively puts the line in question *on-shell*,

thus reducing the two dimensional loop integral to a single dimensional one. It is very convenient to eliminate the spatial momentum using the mass shell condition, and leave the last integral over Euclidean energy which we denote by  $q$ . The on-shell condition becomes

$$q^2 + \varepsilon(p^1)^2 = 0 \quad (2.8)$$

which in the case of the  $AdS_5 \times S^5$  superstring theory leads to

$$p^1 = -i2 \operatorname{arcsinh} \frac{\sqrt{1+q^2}}{4g} \quad (2.9)$$

Plugging this back into the exponential factor  $e^{-ip^1 L}$  leads to the term which governs the overall magnitude of the Lüscher correction

$$e^{-ip^1 L} = e^{-L \cdot E_{TBA}(q)} = e^{-L \cdot 2 \operatorname{arcsinh} \frac{\sqrt{1+q^2}}{4g}} \quad (2.10)$$

We will analyze the physical meaning of this formula in section 3.

The mass shell condition has also another, equally important, consequence. Since the line is on-shell, in the integrand we may cut it open thus effectively transforming the graphs of the 2-point 1PI self energy into those of a 4-point forward Green's function. Keeping track of all the necessary factors gives

$$\Sigma_L = \int \frac{dq}{2\pi} \frac{i}{\varepsilon^2(p^1)'} \cdot e^{-L \cdot E_{TBA}(q)} \cdot \sum_b (-1)^{F_b} G_{abab}(-p, -q, p, q) \quad (2.11)$$

The  $p$  appearing in the argument of  $G_{abab}$  is the spatial momentum of the physical particle, while  $q$  is the Euclidean energy of the virtual one. In the final step, one links the 4-point forward Green's function with the forward S-matrix element arriving at Lüscher's F-term formula generalized to a generic dispersion relation:

$$\delta \varepsilon_a^F = - \int_{-\infty}^{\infty} \frac{dq}{2\pi} \left( 1 - \frac{\varepsilon'(p)}{\varepsilon'(q)} \right) \cdot e^{-iqsL} \cdot \sum_b (-1)^{F_b} (S_{ba}^{ba}(q, p) - 1) \quad (2.12)$$

with the same conventions for the arguments of  $\varepsilon'$  and  $S_{ba}^{ba}$  as described below (2.11). The  $\mu$ -term arises in the process of shifting the contours by localizing on a residue of the above formula. It is thus given just by the residue of (2.12). For further details consult [11]. Let us mention that for relativistic theories one can perform a more detailed analysis concerning the contribution of  $\mu$ -terms [9]. In particular,  $\mu$ -terms are expected to contribute only if, in the spacetime diagram shown in Figure 1, both particles move forward in time (i.e. have positive real part of the energy). This analysis has not been done rigorously for the  $AdS_5 \times S^5$  case.

The diagrammatic derivation presented above is very general and does not require integrability. Moreover the difference between a theory with diagonal and non-diagonal scattering is quite trivial. One can go from the simpler case of a single particle species to the most general case of nondiagonal scattering just by substituting the scalar S-matrix by an appropriate supertrace of the nondiagonal S-matrix. Generalizing this property

to multiparticle states leads to a simple shortcut for obtaining multiparticle Lüscher corrections — one can first obtain the formulas for a simple theory with a single particle in the spectrum, and then generalize to the generic case by trading the product of the scalar S-matrices for a supertrace of the product of the nondiagonal ones. We will present this derivation in the following section.

## 2.2 Multiparticle Lüscher corrections from TBA

In this section we will show how *multiparticle* Lüscher corrections arise from the Thermodynamic Bethe Ansatz. Here, we will be able to obtain these more powerful results using significantly stronger assumptions. In particular we will assume that the theory in question is integrable with diagonal scattering. Then, as explained above, we will use the expected very universal dependence of Lüscher corrections on the S-matrix to conjecture the general versions valid for any integrable theory with a nondiagonal S-matrix (for which TBA equations are much more complicated).

As explained in [6], TBA equations are derived by trading the complicated problem of finding the (ground state) energy of the theory at finite volume for the much simpler one of computing a thermal partition function of the theory with space and time interchanged through a double Wick rotation. In the latter case, since one is dealing with the theory at almost infinite volume, Bethe ansatz is exact and can be used to evaluate the partition function. Hence the energies and momenta in the following are those of the spacetime interchanged one (*aka* mirror theory) related to the energy and momentum of the original theory through

$$\tilde{E} = ip \quad \tilde{p} = iE \quad (2.13)$$

The ground state TBA equation for the theory with a single type of particle takes the form

$$\varepsilon(z) = L\tilde{E}(z) + \int \frac{dw}{2\pi i} (\partial_w \log S(w, z)) \log(1 + e^{-\varepsilon(w)}) \quad (2.14)$$

and the ground state energy is obtained from the solution  $\varepsilon(z)$  through

$$E = - \int \frac{dz}{2\pi} \tilde{p}'(z) \log(1 + e^{-\varepsilon(z)}) \quad (2.15)$$

In order to describe excited states, one uses an analytical continuation trick due to Dorey and Tateo [12] that essentially introduces additional source terms into (2.14). These source terms are generated by singularities of the integrand  $1 + e^{-\varepsilon(z_i)} = 0$ , which, through integration by parts and an evaluation through residues give rise to additional source terms on the r.h.s. of (2.14)

$$\varepsilon(z) = L\tilde{E} + \log S(z_1, z) + \log S(z_2, z) + \int \frac{dw}{2\pi i} (\partial_w \log S(w, z)) \log(1 + e^{-\varepsilon(w)}) \quad (2.16)$$

and additional contributions to the energy

$$E = E(z_1) + E(z_2) - \int \frac{dz}{2\pi} \tilde{p}'(z) \log(1 + e^{-\varepsilon(z)}) \quad (2.17)$$

where we quote the result with just two additional singularities.

It is quite nontrivial what kind of source terms to introduce for the theory at hand. If a theory does not have bound states and  $\mu$ -terms, the rule of thumb is that for each physical particle a single source term has to be included (this happens in the case of e.g. the sinh-Gordon model). On the other hand, for a theory with  $\mu$ -terms, like the SLYM, at least two source terms correspond to a single physical particle (see [12, 13]).

Now in order to obtain the Lüscher corrections, we have to perform a large volume expansion of these equations. Solving (2.16) by iteration, neglecting the integral term and inserting this approximation into the energy formula gives

$$\begin{aligned} E &= E(z_1) + E(z_2) - \int \frac{dz}{2\pi} \tilde{p}' e^{-L\tilde{E}(z)} \frac{1}{S(z_1, z)S(z_2, z)} \\ &= E(z_1) + E(z_2) - \int \frac{dq}{2\pi} e^{-L\tilde{E}(q)} S(z, z_1)S(z, z_2) \end{aligned} \quad (2.18)$$

We recognize at once an integral of the F-term type (with  $q \equiv \tilde{p}$ ) in addition to the sum of energies of the individual particles. There is a subtlety here, namely one has to dynamically impose the equations for the positions of the singularities

$$1 + e^{-\varepsilon(z_i)} = 0 \quad (2.19)$$

If we insert here the same approximation as we have just used in the formula for the energy, we will recover the Bethe equations

$$e^{iLp_1} = S(p_1, p_2) \quad (2.20)$$

However, in Lüscher's corrections we should keep all leading exponential terms. Therefore for the quantization condition (2.19), we have to use also the first nontrivial iteration of (2.16). This will give rise to modifications of the Bethe quantization conditions. The quantization conditions  $\varepsilon(z_i) = i\pi$  becomes

$$0 = \underbrace{\log\{e^{iLp_1} S(z_2, z_1)\}}_{BY_1} + \underbrace{\int \frac{dw}{2\pi i} (\partial_w S(w, z_1)) S(w, z_2) e^{-L\tilde{E}(w)}}_{\Phi_1} \quad (2.21)$$

$$0 = \underbrace{\log\{e^{iLp_2} S(z_1, z_2)\}}_{BY_2} + \underbrace{\int \frac{dw}{2\pi i} S(w, z_1) (\partial_w S(w, z_2)) e^{-L\tilde{E}(w)}}_{\Phi_2} \quad (2.22)$$

Since the integrals are exponentially small we may solve these equations in terms of corrections to the Asymptotic Bethe Ansatz (ABA) giving

$$\frac{\partial BY_1}{\partial p_1} \delta p_1 + \frac{\partial BY_1}{\partial p_2} \delta p_2 + \Phi_1 = 0 \quad (2.23)$$

$$\frac{\partial BY_2}{\partial p_1} \delta p_1 + \frac{\partial BY_2}{\partial p_2} \delta p_2 + \Phi_2 = 0 \quad (2.24)$$

The final formula for the energy thus takes the form

$$E = E(p_1) + E(p_2) + E'(p_1)\delta p_1 + E'(p_2)\delta p_2 - \int \frac{dq}{2\pi} e^{-L\tilde{E}} S(z, z_1)S(z, z_2) \quad (2.25)$$

For nondiagonal scattering, we expect that the above formula will get modified just by exchanging the products of scalar S-matrices by a supertrace of a product of real *matrix* S-matrices. This generalization has been proposed in [30]. In the F-term integrand we will thus get the transfer matrix (c.f. [7]) or more precisely its eigenvalue<sup>1</sup>

$$e^{i\delta(\tilde{p}|p_1, \dots, p_N)} = (-1)^F [S_{a_1 a}^{a_2 a}(\tilde{p}, p_1) S_{a_2 a}^{a_3 a}(\tilde{p}, p_2) \dots S_{a_N a}^{a_1 a}(\tilde{p}, p_N)] \quad (2.26)$$

where we also substituted the complex rapidities used earlier by more physical momenta. The BY condition reads as

$$2n_k \pi = BY_k(p_1, \dots, p_n) + \delta\Phi_k = p_k L - i \log \left[ \prod_{k \neq j} S_{aa}^{aa}(p_k, p_j) \right] + \delta\Phi_k \quad (2.27)$$

with the correction to these equations given by

$$\delta\Phi_k = - \int_{-\infty}^{\infty} \frac{d\tilde{p}}{2\pi} (-1)^F \left[ S_{a_1 a}^{a_2 a}(\tilde{p}, p_1) \dots \frac{\partial S_{a_k a}^{a_{k+1} a}(\tilde{p}, p_k)}{\partial \tilde{p}} \dots S_{a_N a}^{a_1 a}(\tilde{p}, p_N) \right] e^{-\epsilon_{a_1}(\tilde{p})L} \quad (2.28)$$

The final correction then reads as

$$\begin{aligned} E(L) = & \sum_k \epsilon(p_k) - \sum_{j,k} \frac{d\epsilon(p_k)}{dp_k} \left( \frac{\delta BY_k}{\delta p_j} \right)^{-1} \delta\Phi_j \\ & - \int_{-\infty}^{\infty} \frac{d\tilde{p}}{2\pi} \sum_{a_1, \dots, a_N} (-1)^F [S_{a_1 a}^{a_2 a}(\tilde{p}, p_1) S_{a_2 a}^{a_3 a}(\tilde{p}, p_2) \dots S_{a_N a}^{a_1 a}(p, p_N)] e^{-\epsilon_{a_1}(\tilde{p})L} \end{aligned} \quad (2.29)$$

For theories with  $\mu$ -terms, we expect that the corresponding  $\mu$ -terms will be obtained by localizing the integrals on the poles of the S-matrix.

## 2.3 Poisson resummation of fluctuations

In this section we will present a simple, very physical, derivation of Lüscher's F-term formula from a summation over quadratic fluctuations. Although this approach requires the most restrictive assumptions, it is quite intuitive and gives a new perspective on the origin of Lüscher's corrections.

For simplicity we will just present the derivation for a particle with vanishing momentum, analogous to Lüscher's original formulas. A more general case is treated<sup>2</sup> in [14].

Consider a soliton at rest which is put on a very large cylinder, so large that we may neglect the effect of the deformation of the solution. Now a small fluctuation very far from the soliton will just be an excitation of the vacuum, so can be treated as another soliton<sup>3</sup> (more precisely a single particle state). This small 'fluctuation' soliton will scatter on

<sup>1</sup>We present below the case when the physical particles forming the multiparticle state scatter between themselves diagonally

<sup>2</sup>In ref. [14], a minus sign will have to be included in the second term in eq. (13) there.

<sup>3</sup>Here we use 'soliton' as a generic term which includes e.g. 'breathers' in the sine-Gordon model.

the stationary one and will get a phase shift expressible in terms of the S-matrix (which we assume here to be diagonal)

$$S_{ba}^{ba}(k, p) = e^{i\delta_{ba}(k, p)} \quad (2.30)$$

Due to the finite size of the cylinder, the momentum of the ‘fluctuation’ soliton will have to be quantized giving

$$k_n = \frac{2\pi n}{L} + \frac{\delta_b(k_n)}{L} \quad (2.31)$$

We now have to perform a summation over the energies of the fluctuations

$$\delta\varepsilon_{naive} = \frac{1}{2} \sum_b \sum_{n=-\infty}^{\infty} (-1)^{F_b} (\varepsilon(k_n) - \varepsilon(k_n^{(0)})) \quad (2.32)$$

where the energies of fluctuations around the vacuum (with  $k_n^{(0)} = 2\pi n/L$ ) have been subtracted out.

The key result of [14] is that Lüscher’s corrections are exactly the leading exponential terms ( $m = \pm 1$ ) in the Poisson resummation

$$\sum_{n=-\infty}^{\infty} F\left(\frac{2\pi n}{L}\right) = \frac{L}{2\pi} \sum_{m=-\infty}^{\infty} \int_{-\infty}^{+\infty} F(t) e^{-imLt} dt \quad (2.33)$$

of (2.32). The relevant terms will be

$$\delta\varepsilon = \frac{L}{4\pi} \text{Re} \int_{-\infty}^{\infty} e^{iLt} (\epsilon(k(t)) - \epsilon(t)) dt \quad (2.34)$$

where  $k(t) = t + \delta(k(t))/L$  is the quantization condition, the solution of which we do not need explicitly. Now, after a sequence of integration by parts and a simple change of variables (see [14] for details) we can rewrite (2.34) as

$$\delta\varepsilon = \frac{1}{4\pi i} \text{Re} \int_{-\infty}^{+\infty} e^{-iLk} (e^{i\delta(k)} - 1) \epsilon'(k) dk = \frac{1}{4\pi i} \text{Re} \int_{-\infty}^{+\infty} e^{-iLk} (S_{ba}^{ba}(k, p) - 1) \epsilon'(k) dk \quad (2.35)$$

which is essentially Lüscher’s F-term but evaluated on the physical line. We should now shift the contour to ensure that the exponent is strictly real and decreasing at infinity giving rise to Lüscher’s corrections. Here the boundary terms require a case by case analysis. Also  $\mu$ -terms may be generated when in the process of shifting the contour we would encounter bound state poles. The above derivation shows that evaluating Lüscher F-term contributions is equivalent to computing directly 1-loop energy shifts around the corresponding classical solution. Although one has to be careful in this interpretation when one evaluates the phase shifts (2.30) exactly and not only semiclassically.

### 3 Applications of generalized Lüscher's corrections in the AdS/CFT correspondence

In this section we will briefly review various applications of generalized Lüscher's corrections in the context of the integrable worldsheet QFT of the superstring in  $AdS_5 \times S^5$ . Due to the AdS/CFT correspondence, the energy levels of this theory (energies of string states) are identified with the anomalous dimensions of the corresponding gauge theory operators. In this way, the intrinsically two-dimensional methods may be applied to the four-dimensional  $\mathcal{N} = 4$  SYM theory.

Before we review the obtained results let us first discuss the generic magnitude of Lüscher corrections in this context.

As we saw from the derivations, the order of magnitude of the F-term formula is essentially governed by the exponential factor [15]

$$e^{-L\tilde{E}(\tilde{p})} \quad (3.1)$$

where  $\tilde{E}$  and  $\tilde{p} \equiv q$  are the energy and momentum of a theory with a double Wick rotation exchanging space and time – called ‘mirror theory’ [16]. For the case at hand we have

$$e^{-L \cdot 2 \operatorname{arcsinh} \frac{\sqrt{Q^2+q^2}}{4g}} \quad (3.2)$$

where  $Q = 1$  corresponds to the fundamental particle (magnon) and  $Q > 1$  labels the bound states of the theory.

In the strong coupling limit, this expression becomes

$$e^{-Q \frac{L}{2g}} \Big|_{Q=1} = e^{-\frac{2\pi L}{\sqrt{\lambda}}} \quad (3.3)$$

which is the typical finite size fluctuation effect observed for spinning strings [17]. We also see that at strong coupling, the contribution of bound states is exponentially suppressed, so one can just consider the fundamental magnons circulating around the cylinder.

The  $\mu$ -term, which arises from the F-term by taking residues also appears at strong coupling. It's magnitude at strong coupling for a single magnon can be estimated to be

$$e^{-\frac{2\pi J}{\sqrt{\lambda} \sin \frac{p}{2}}} \quad (3.4)$$

where  $p$  is the momentum of the physical magnon. We see that the exponential term gives a stronger suppression than the F-term, however, the terms differ in the scaling of the prefactor with the coupling. The F-term is associated with quantum effects, while the  $\mu$ -term appears already in the classical contribution hence the F-term is suppressed by a factor of  $\sqrt{\lambda}$  w.r.t. the  $\mu$ -term. Let us note that the link between  $\mu$ -terms and classical solutions is still to a large extent not understood. We may get another qualitative estimate from the formula (3.4) for classical finite-gap solutions which may be considered to arise in the worldsheet theory as a state of very many particles, each of which will presumably have a very small momentum. Then (3.4) suggests that the  $\mu$ -term should be completely negligible for such states.

At weak coupling, we obtain a quite different formula

$$\frac{\# g^{2L}}{(Q^2 + q^2)^L} \quad (3.5)$$

Firstly, we see that the effect of the virtual corrections only starts at a certain loop order, from the point of view of gauge theory perturbative expansion. Up to this order the Bethe equations are in fact exact. Such a behaviour is wholly due to the nonstandard AdS dispersion relation (2.3). The loop order at which these corrections start to contribute is related to the size of the gauge theory operator in question. This is very good, as just at that order we expect a new class of Feynman graphs to appear in the perturbative computation. These are the so-called ‘wrapping corrections’ and are given by graphs where, in the computation of a two point function relevant for extracting anomalous dimensions, at least one propagator crosses all vertical legs. From the very start [18] (see also [19]), these graphs were expected not to be described by the Asymptotic Bethe Ansatz. Their identification with (possibly multiple) Lüscher corrections was first proposed in [15].

Secondly, we see that at weak coupling, all bound states contribute at the same order. This makes the computation of wrapping effects at weak coupling more complicated, but at the same time more interesting, as they are sensitive to much finer details of the worldsheet QFT than at strong coupling.

The corrections to Lüscher formulas are very difficult to quantify. Even in the relativistic case there are no formulas for the leading corrections. These would be multiple wrapping graphs and hence a  $0^{th}$  order estimate of their relative magnitude would be another exponential term. At strong coupling we would thus probably see a mixture of the first double wrapping graphs for magnons with ordinary single wrapping graphs for the first  $Q = 2$  bound states. At weak coupling, the next wrapping correction would generically have a relative magnitude of  $g^{2L}$  although there might also be factors of  $g$  coming from the prefactor which we do not control so the loop order for subleading multiple wrapping corrections is not precisely determined.

Let us finish this section with a brief note on the elusive nature of  $\mu$ -terms. Physical arguments based on the relativistic spacetime picture of the  $\mu$ -term diagram, amounting to the requirement that the produced virtual particles propagate forward in time suggests that at weak coupling  $\mu$ -terms should not appear since the bound state is heavier than the fundamental magnon. Explicit computations for the Konishi operator and twist-2 operators (see section 3.2 below) confirm this intuition. Yet, at strong coupling the  $\mu$ -term definitely contributes to the giant magnon finite size dispersion relation. It is still not understood how and when does this occur, especially in terms of the proposed exact TBA formulations.

### 3.1 Strong coupling results

An excitation of the worldsheet theory with momentum  $p \sim \mathcal{O}(1)$  has an energy which scales as  $\sqrt{\lambda}$  characteristic of a classical string solution. Such a solution has been found in [20] and is called the ‘giant magnon’. Subsequently, corrections to its energy were

found when the excitation was considered on a cylinder of finite size  $J$ . The resulting correction was evaluated from the deformed classical solution in [21] to be

$$\delta E_{string} = -\frac{\sqrt{\lambda}}{\pi} \cdot \frac{4}{e^2} \cdot \sin^3 \frac{p}{2} \cdot e^{-\frac{2\pi J}{\sqrt{\lambda} \sin \frac{p}{2}}} \equiv -g \cdot \frac{16}{e^2} \cdot \sin^3 \frac{p}{2} \cdot e^{-\frac{2}{g \sin \frac{p}{2}} J} \quad (3.6)$$

In [11], the above expression was recovered from Lüscher's corrections. The exponential term is different from the one appearing in the F-term formula however it turns out that it is exactly the term appearing in the  $\mu$ -term, when we find the residue of the F-term expression at the bound state pole.

The prefactor comes from evaluating the residue of the (super)trace of the forward S-matrix at the bound state pole. A very curious feature of the above expression is the contribution of the dressing factor, which, at strong coupling, has an expansion (see [22])

$$\sigma^2 = \exp\left(g \chi_{AFS} + \chi_{HL} + \sum_{n=2}^{\infty} \frac{1}{g^{n-1}} \chi_n\right) \quad (3.7)$$

Naively, one may expect that only the first two terms would give a contribution, however it turns out that due to the special kinematics of the bound state pole, *all*  $\chi_{2n}$  contribute. The evaluation of this contribution is quite nontrivial with a divergent series appearing, which can be resummed using Borel resummation. The result exactly reproduces (3.6).

Among further developments, finite size contributions to dyonic giant magnons were analyzed [23], quantum fluctuations were linked with the F-term [24, 14], similar computations were also done for giant magnons and dyonic magnons in the ABJM theory [25]. In addition finite size corrections were evaluated for open strings (which corresponds to Lüscher corrections in a boundary integrable field theory [26]) [27].

One can also analyze Lüscher corrections for classical spinning strings. There the picture is quite different from the giant magnons. The spinning string solutions arise as a superposition of very many excitations, all with very small momenta. So the  $\mu$ -term exponential factor will be very much suppressed and the dominant correction will arise from the F-term. The F-term integrand can be evaluated in terms of the transfer matrix directly in terms of the Bethe root distributions describing the spinning string in question. Alternatively, an analysis of these issues have been done from the algebraic curve perspective in [28].

## 3.2 Weak coupling results

Lüscher's corrections are particularly interesting when applied in the weak coupling regime corresponding to perturbative gauge theory. There, they provide the only calculational method to compute wrapping corrections apart from a direct perturbative computation which usually is prohibitively complicated (see [8]). Calculations based on generalized Lüscher's corrections are typically much simpler and allow to obtain 4- and 5- loop gauge theory results which cannot be obtained using other means.

From a more theoretical perspective, the agreement of Lüscher corrections with perturbative gauge theory results is interesting as it gives a nontrivial quantitative test of the AdS/CFT correspondence, as well as of our understanding of the fine details of the

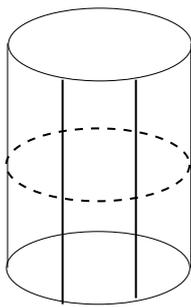

**Figure 3:** The single Lüscher graph entering the computation of the four loop Konishi anomalous dimension.

worldsheet QFT of the  $AdS_5 \times S^5$  superstring. Moreover, it is very interesting to realize that the breakdown of the Asymptotic Bethe Ansatz for anomalous dimensions in the four dimensional gauge theory occurs *exactly* in a way characteristic of a *two dimensional* quantum field theory (and thus characteristic of string theory).

A natural testing ground for these methods is the Konishi operator  $\text{tr } \Phi_i^2$  (or equivalently  $\text{tr } XZXZ - \text{tr } X^2Z^2$ ,  $\text{tr } DZDZ - \text{tr } ZD^2Z$ ), which is the shortest operator not protected by supersymmetry.

From the string perspective, it corresponds to a two particle state in the worldsheet QFT on a cylinder of size  $J = 2$ . Despite the fact that  $J$  is so small, we may expect to get an exact answer from Lüscher corrections at least at 4- and 5- loop level due to the estimate (3.5). Since at weak coupling all bound states contribute at the same order, we have to perform a summation over all bound states and their polarization states and use the bound state-fundamental magnon S-matrix. There is a further subtlety here, which does not appear in relativistic systems. In the physical theory, the bound states discovered in [29] are in the symmetric representation, while states in the antisymmetric representation are unstable. On the other hand, in the mirror theory, the physical bound states are in the antisymmetric representation [16], and in fact it is these antisymmetric bound states which have to be taken into account when computing Lüscher's corrections.

Performing the computation yields the result for the 4-loop wrapping correction to the anomalous dimension of the Konishi operator [30]:

$$\Delta_w^{(8)} = 324 + 864\zeta(3) - 1440\zeta(5) \quad (3.8)$$

which is in exact agreement with direct perturbative computations using both supergraph techniques [31] and component Feynman graphs [32]. The string computation is much simpler as it involves evaluating just the single graph shown in Figure 3.

In another development, wrapping corrections for twist two operators

$$\text{tr } ZD^M Z + \text{permutations} \quad (3.9)$$

were computed. Here, the main motivation for performing this computation was the fact there are stringent analytical constraints on the structure of the anomalous dimensions  $\Delta(M)$  as a function of  $M$ . In fact the disagreement, at 4 loops, between the behaviour of the Bethe Ansatz  $\Delta(M)$  for  $M = -1 + \omega$  and gauge theory constraints from the BFKL

(Balitsky-Fadin-Kuraev-Lipatov) and NLO BFKL equations describing high energy scattering in the Regge limit [33] were the first quantitative indication that the Asymptotic Bethe Ansatz breaks down [34].

In [35], the anomalous dimensions of twist two operators were evaluated at 4 loop level using Lüscher corrections for an  $M$ -particle state. The wrapping correction was found to exactly compensate the mismatch between the Bethe Ansatz and BFKL expectations.

Subsequently, the leading wrapping corrections for the lowest lying twist-three operators were also determined from Lüscher corrections [36]. These occur at 5 loop level. Another class of operators which was considered were single particle states [37] and the Konishi operator [38] in the  $\beta$  deformed theory. These results agree with direct field theoretical computations when available [39].

In all the above computations of the leading wrapping corrections there were significant simplifications. Firstly, the wrapping modifications of the Bethe Ansatz quantization condition did not appear. Secondly, the dressing factor of the S-matrix also did not contribute.

Once one moves to subleading perturbative wrapping order (5-loop for Konishi and twist two, and 6-loop for twist three), both of these effects start to play a role. The modification of the Bethe Ansatz quantization is particularly interesting, as it is only in its derivation that the convolution terms in TBA equations contribute. In contrast to the simple single component TBA equation presented here, the structure of the TBA equations proposed for the  $AdS_5 \times S^5$  system is very complicated [40]. So Lüscher corrections may be a nontrivial cross-check for these proposals. In addition, due to the kinematics of the scattering between the physical particle and the mirror particle, it turns out that already at 5 loops, an infinite set of coefficients of the BES/BHL dressing phase contributes to the answer.

A key difficulty in performing such a computation is the possibility of testing the answer. Fortunately we have at our disposal two independent consistency checks. Firstly, at weak coupling we do not expect the appearance of  $\mu$ -terms which implies that a sum over residues of certain dynamical poles in the integrand has to cancel after summing over all bound states. Secondly, the transcendental structure of the final answer should be quite simple, while the subexpressions involve very complicated expressions which should cancel out in the final answer. In addition, for the case of twist two operators, one can use the numerous stringent constraints on the analytic structure coming from BFKL, NLO BFKL, reciprocity etc.

In [41], the five loop wrapping correction to the Konishi anomalous dimension was derived

$$\Delta_w^{(10)} = -11340 + 2592\zeta(3) - 5184\zeta(3)^2 - 11520\zeta(5) + 30240\zeta(7) \quad (3.10)$$

while in [42] a *tour-de-force* computation was performed for twist two operators at five loops. Subsequently twist three operators were also considered at subleading wrapping order in [43].

Recently, the five loop result coming from Lüscher corrections was confirmed by expanding the exact TBA equations at large volume first numerically [44], and then analytically [45]. Finally, subsubleading (6-loop) wrapping corrections were considered for single impurity operators in the  $\beta$  deformed theory [46].

## 4 Summary and outlook

Lüscher's corrections situate themselves in the middle ground between Bethe Ansatz and a full fledged solution of two dimensional integrable quantum field theories in the guise of Thermodynamic Bethe Ansatz or Nonlinear Integral Equations. They encode effects of an explicitly quantum field theoretical nature, namely virtual corrections associated with the topology of a cylinder. In this way Lüscher's corrections may be seen to differentiate between spin chain like systems, where the Bethe Ansatz is exact and quantum field theories, for which the Bethe Ansatz is only a large volume approximation.

In this review, we have presented various ways of arriving at Lüscher's corrections, some of them more or less rigorous, others more conjectural. The fact that the methods are quite different one from the other serves as an important cross check of these results. It would be, however, quite interesting to extend some of these methods in various directions e.g. the diagrammatic calculations to multiparticle states and subleading wrapping. Recently, the multiparticle Lüscher corrections proposed in [30] were tested in [47, 44, 45]. It would be interesting to obtain some kind of universal understanding how the structure necessary for Lüscher corrections is encoded in the very complicated nondiagonal TBA systems.

With respect to the concrete applications of Lüscher corrections in the AdS/CFT correspondence there are still some loose ends like the rather mysterious formula for the finite size corrections of the giant magnon in the  $\beta$  deformed theory [48]. Apart from that, the agreement between the computations based on Lüscher corrections, which typically involve a single graph, and the very complicated four loop gauge theory computations involving hundreds or even many thousands of graphs suggests that there is some very nontrivial hidden structure in the perturbative expansion. It would be very interesting to understand whether it could be understood in any explicit way.

**Acknowledgments:** This work was supported by Polish science funds as a research project N N202 105136 (2009-2011).

## References

- [1] M. Staudacher, “*Review of AdS/CFT Integrability, Chapter III.1: Bethe Ansätze and the R-Matrix Formalism*”, [arxiv:1012.3990](#). • C. Ahn and R. Nepomechie, “*Review of AdS/CFT Integrability, Chapter III.2: Exact world-sheet S-matrix*”, [arxiv:1012.3991](#).
- [2] M. Luscher, “*Volume Dependence of the Energy Spectrum in Massive Quantum Field Theories. 1. Stable Particle States*”, *Commun. Math. Phys.* 104, 177 (1986).
- [3] A. Rej, D. Serban and M. Staudacher, “*Planar  $\mathcal{N} = 4$  gauge theory and the Hubbard model*”, *JHEP* 0603, 018 (2006), [hep-th/0512077](#).
- [4] A. B. Zamolodchikov, “*THERMODYNAMIC BETHE ANSATZ IN RELATIVISTIC MODELS. SCALING THREE STATE POTTS AND LEE-YANG MODELS*”, *Nucl. Phys.* B342, 695 (1990).
- [5] C. Destri and H. J. De Vega, “*Unified approach to thermodynamic Bethe Ansatz and finite size corrections for lattice models and field theories*”, *Nucl. Phys.* B438, 413 (1995),

- hep-th/9407117. • D. Fioravanti, A. Mariottini, E. Quattrini and F. Ravanini, “*Excited state Destri-De Vega equation for sine-Gordon and restricted sine-Gordon models*”, Phys. Lett. B390, 243 (1997), hep-th/9608091.
- [6] Z. Bajnok, “*Review of AdS/CFT Integrability, Chapter III.6: Thermodynamic Bethe Ansatz*”, arxiv:1012.3995.
- [7] V. Kazakov and N. Gromov, “*Review of AdS/CFT Integrability, Chapter III.7: Hirota Dynamics for Quantum Integrability*”, arxiv:1012.3996.
- [8] C. Sieg, “*Review of AdS/CFT Integrability, Chapter I.2: The spectrum from perturbative gauge theory*”, arxiv:1012.3984.
- [9] T. R. Klassen and E. Melzer, “*On the relation between scattering amplitudes and finite size mass corrections in QFT*”, Nucl. Phys. B362, 329 (1991).
- [10] G. Arutyunov and S. Frolov, “*Foundations of the  $AdS_5 \times S^5$  Superstring. Part I*”, J. Phys. A42, 254003 (2009), arxiv:0901.4937.
- [11] R. A. Janik and T. Lukowski, “*Wrapping interactions at strong coupling – the giant magnon*”, Phys. Rev. D76, 126008 (2007), arxiv:0708.2208.
- [12] P. Dorey and R. Tateo, “*Excited states by analytic continuation of TBA equations*”, Nucl. Phys. B482, 639 (1996), hep-th/9607167.
- [13] P. Dorey and R. Tateo, “*Excited states in some simple perturbed conformal field theories*”, Nucl. Phys. B515, 575 (1998), hep-th/9706140.
- [14] M. P. Heller, R. A. Janik and T. Lukowski, “*A new derivation of Lüscher F-term and fluctuations around the giant magnon*”, JHEP 0806, 036 (2008), arxiv:0801.4463.
- [15] J. Ambjorn, R. A. Janik and C. Kristjansen, “*Wrapping interactions and a new source of corrections to the spin-chain / string duality*”, Nucl. Phys. B736, 288 (2006), hep-th/0510171.
- [16] G. Arutyunov and S. Frolov, “*On String S-matrix, Bound States and TBA*”, JHEP 0712, 024 (2007), arxiv:0710.1568.
- [17] S. Schafer-Nameki, “*Exact expressions for quantum corrections to spinning strings*”, Phys. Lett. B639, 571 (2006), hep-th/0602214. • S. Schafer-Nameki, M. Zamaklar and K. Zarembo, “*How accurate is the quantum string Bethe ansatz?*”, JHEP 0612, 020 (2006), hep-th/0610250.
- [18] N. Beisert, V. Dippel and M. Staudacher, “*A novel long range spin chain and planar  $\mathcal{N} = 4$  super Yang-Mills*”, JHEP 0407, 075 (2004), hep-th/0405001.
- [19] C. Sieg and A. Torrielli, “*Wrapping interactions and the genus expansion of the 2-point function of composite operators*”, Nucl. Phys. B723, 3 (2005), hep-th/0505071.
- [20] D. M. Hofman and J. M. Maldacena, “*Giant magnons*”, J. Phys. A39, 13095 (2006), hep-th/0604135.
- [21] G. Arutyunov, S. Frolov and M. Zamaklar, “*Finite-size effects from giant magnons*”, Nucl. Phys. B778, 1 (2007), hep-th/0606126. • D. Astolfi, V. Forini, G. Grignani and G. W. Semenoff, “*Gauge invariant finite size spectrum of the giant magnon*”, Phys. Lett. B651 329 (2007), hep-th/0702043
- [22] Vieira, P. and Volin, D., “*Review of AdS/CFT Integrability, Chapter III.3: The dressing factor*”, arxiv:1012.3992.

- [23] Y. Hatsuda and R. Suzuki, “*Finite-Size Effects for Dyonics Giant Magnons*”, Nucl. Phys. B800, 349 (2008), [arxiv:0801.0747](#).
- [24] N. Gromov, S. Schafer-Nameki and P. Vieira, “*Quantum Wrapped Giant Magnon*”, Phys. Rev. D78, 026006 (2008), [arxiv:0801.3671](#).
- [25] G. Grignani, T. Harmark, M. Orselli and G. W. Semenoff, “*Finite size Giant Magnons in the string dual of  $N=6$  superconformal Chern-Simons theory*”, JHEP 0812, 008 (2008), [arXiv:0807.0205](#). • D. Bombardelli and D. Fioravanti, “*Finite-Size Corrections of the  $CP^3$  Giant Magnons: the Lüscher terms*”, JHEP 0907, 034 (2009), [arxiv:0810.0704](#). • T. Lukowski and O. O. Sax, “*Finite size giant magnons in the  $SU(2) \times SU(2)$  sector of  $AdS_4 \times CP^3$* ”, JHEP 0812, 073 (2008), [arxiv:0810.1246](#). • C. Ahn and P. Bozhilov, “*Finite-size Effect of the Dyonics Giant Magnons in  $\mathcal{N} = 6$  super Chern-Simons Theory*”, Phys. Rev. D79, 046008 (2009), [arxiv:0810.2079](#). • C. Ahn, M. Kim and B.-H. Lee, “*Quantum finite-size effects for dyonics magnons in the  $AdS_4 \times CP^3$* ”, JHEP 1009, 062 (2010), [arxiv:1007.1598](#).
- [26] Z. Bajnok, L. Palla and G. Takacs, “*Finite size effects in quantum field theories with boundary from scattering data*”, Nucl. Phys. B716, 519 (2005), [hep-th/0412192](#).
- [27] D. H. Correa and C. A. S. Young, “*Finite size corrections for open strings/open chains in planar AdS/CFT*”, JHEP 0908, 097 (2009), [arxiv:0905.1700](#). • Z. Bajnok and L. Palla, “*Boundary finite size corrections for multiparticle states and planar AdS/CFT*”, [arxiv:1010.5617](#).
- [28] N. Gromov, S. Schafer-Nameki and P. Vieira, “*Efficient precision quantization in AdS/CFT*”, JHEP 0812, 013 (2008), [arxiv:0807.4752](#).
- [29] N. Dorey, “*Magnon bound states and the AdS/CFT correspondence*”, J. Phys. A39, 13119 (2006), [hep-th/0604175](#).
- [30] Z. Bajnok and R. A. Janik, “*Four-loop perturbative Konishi from strings and finite size effects for multiparticle states*”, Nucl. Phys. B807, 625 (2009), [arxiv:0807.0399](#).
- [31] F. Fiamberti, A. Santambrogio, C. Sieg and D. Zanon, “*Wrapping at four loops in  $\mathcal{N} = 4$  SYM*”, Phys. Lett. B666, 100 (2008), [arxiv:0712.3522](#). • F. Fiamberti, A. Santambrogio, C. Sieg and D. Zanon, “*Anomalous dimension with wrapping at four loops in  $\mathcal{N} = 4$  SYM*”, Nucl. Phys. B805, 231 (2008), [arxiv:0806.2095](#).
- [32] V. N. Velizhanin, “*The four-loop anomalous dimension of the Konishi operator in  $N=4$  supersymmetric Yang-Mills theory*”, JETP Lett. 89, 6 (2009), [arxiv:0808.3832](#).
- [33] L. N. Lipatov, “*Reggeization of the vector meson and the vacuum singularity in nonabelian gauge theories*,” Sov. J. Nucl. Phys. **23** (1976) 338 [Yad. Fiz. **23** (1976) 642]; E. A. Kuraev, L. N. Lipatov and V. S. Fadin, “*The Pomeranchuk singularity in nonabelian gauge theories*,” Sov. Phys. JETP **45** (1977) 199 [Zh. Eksp. Teor. Fiz. **72** (1977) 377]; I. I. Balitsky and L. N. Lipatov, “*The Pomeranchuk singularity in Quantum Chromodynamics*,” Sov. J. Nucl. Phys. **28** (1978) 822 [Yad. Fiz. **28** (1978) 1597].
- [34] A. V. Kotikov, L. N. Lipatov, A. Rej, M. Staudacher and V. N. Velizhanin, “*Dressing and Wrapping*”, J. Stat. Mech. 0710, P10003 (2007), [arxiv:0704.3586](#).
- [35] Z. Bajnok, R. A. Janik and T. Lukowski, “*Four loop twist two, BFKL, wrapping and strings*”, Nucl. Phys. B816, 376 (2009), [arxiv:0811.4448](#).

- [36] M. Beccaria, V. Forini, T. Lukowski and S. Zieme, “*Twist-three at five loops, Bethe Ansatz and wrapping*”, JHEP 0903, 129 (2009), [arxiv:0901.4864](#).
- [37] M. Beccaria and G. F. De Angelis, “*On the wrapping correction to single magnon energy in twisted  $N=4$  SYM*”, Int. J. Mod. Phys. A24, 5803 (2009), [arxiv:0903.0778](#).
- [38] C. Ahn, Z. Bajnok, D. Bombardelli and R. I. Nepomechie, “*Finite-size effect for four-loop Konishi of the beta- deformed  $N=4$  SYM*”, Phys. Lett. B693, 380 (2010), [arxiv:1006.2209](#).
- [39] F. Fiamberti, A. Santambrogio, C. Sieg and D. Zanon, “*Single impurity operators at critical wrapping order in the beta-deformed  $\mathcal{N} = 4$  SYM*”, JHEP 0908, 034 (2009), [arxiv:0811.4594](#). • F. Fiamberti, A. Santambrogio and C. Sieg, “*Five-loop anomalous dimension at critical wrapping order in  $N=4$  SYM*”, JHEP 1003, 103 (2010), [arxiv:0908.0234](#).
- [40] D. Bombardelli, D. Fioravanti and R. Tateo, “*Thermodynamic Bethe Ansatz for planar AdS/CFT: a proposal*”, J. Phys. A42, 375401 (2009), [arxiv:0902.3930](#). • N. Gromov, V. Kazakov and P. Vieira, “*Exact Spectrum of Anomalous Dimensions of Planar  $N=4$  Supersymmetric Yang-Mills Theory*”, Phys. Rev. Lett. 103, 131601 (2009), [arxiv:0901.3753](#). • N. Gromov, V. Kazakov, A. Kozak and P. Vieira, “*Exact Spectrum of Anomalous Dimensions of Planar  $N = 4$  Supersymmetric Yang-Mills Theory: TBA and excited states*”, Lett. Math. Phys. 91, 265 (2010), [arxiv:0902.4458](#). • G. Arutyunov and S. Frolov, “*Thermodynamic Bethe Ansatz for the  $AdS_5 \times S^5$  Mirror Model*”, JHEP 0905, 068 (2009), [arxiv:0903.0141](#). • G. Arutyunov and S. Frolov, “*Simplified TBA equations of the  $AdS_5 \times S^5$  mirror model*”, JHEP 0911, 019 (2009), [arxiv:0907.2647](#).
- [41] Z. Bajnok, A. Hegedus, R. A. Janik and T. Lukowski, “*Five loop Konishi from AdS/CFT*”, Nucl. Phys. B827, 426 (2010), [arxiv:0906.4062](#).
- [42] T. Lukowski, A. Rej and V. N. Velizhanin, “*Five-Loop Anomalous Dimension of Twist-Two Operators*”, Nucl. Phys. B831, 105 (2010), [arxiv:0912.1624](#).
- [43] V. N. Velizhanin, “*Six-Loop Anomalous Dimension of Twist-Three Operators in  $N=4$  SYM*”, JHEP 1011, 129 (2010), [arxiv:1003.4717](#).
- [44] G. Arutyunov, S. Frolov and R. Suzuki, “*Five-loop Konishi from the Mirror TBA*”, JHEP 1004, 069 (2010), [arxiv:1002.1711](#).
- [45] J. Balog and A. Hegedus, “*5-loop Konishi from linearized TBA and the XXX magnet*”, JHEP 1006, 080 (2010), [arxiv:1002.4142](#). • J. Balog and A. Hegedus, “*The Bajnok-Janik formula and wrapping corrections*”, JHEP 1009, 107 (2010), [arxiv:1003.4303](#).
- [46] Z. Bajnok and O. e. Deeb, “*6-loop anomalous dimension of a single impurity operator from AdS/CFT and multiple zeta values*”, [arxiv:1010.5606](#).
- [47] N. Gromov, V. Kazakov and P. Vieira, “*Finite Volume Spectrum of 2D Field Theories from Hirota Dynamics*”, JHEP 0912, 060 (2009), [arxiv:0812.5091](#). • J. Balog and A. Hegedus, “*The finite size spectrum of the 2-dimensional  $O(3)$  nonlinear sigma-model*”, [arxiv:0907.1759](#).
- [48] D. V. Bykov and S. Frolov, “*Giant magnons in TsT-transformed  $AdS_5 \times S^5$* ”, JHEP 0807, 071 (2008), [arxiv:0805.1070](#).



# Review of AdS/CFT Integrability, Chapter III.6: Thermodynamic Bethe Ansatz

ZOLTÁN BAJNOK

Theoretical Physics Research Group of the  
Hungarian Academy of Sciences,  
H-1117 Pázmány s. 1/A, Budapest, Hungary

bajnok@elte.hu

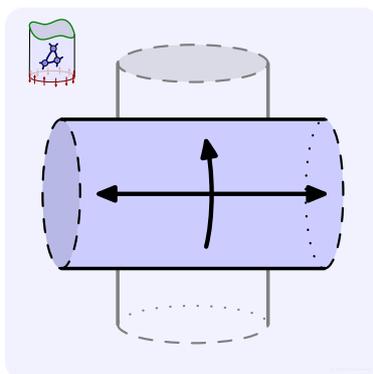

**Abstract:** The aim of the chapter is to introduce in a pedagogical manner the concept of Thermodynamic Bethe Ansatz designed to calculate the energy levels of finite volume integrable systems and to review how it is applied in the planar AdS/CFT setting.

## 1 Introduction

Thermodynamic Bethe Ansatz (TBA) is a method to calculate exactly the groundstate energy of an integrable quantum field theory in finite volume using its infinite volume scattering data [1]<sup>1</sup>. The equations can be extended to excited states as well by analytical continuation [3, 4].

The idea of the TBA is to exploit that the Euclidean partition function is dominated for large imaginary times by the groundstate energy. Calculating the partition function in the doubly Wick rotated (mirror) theory the imaginary time becomes the physical size which is taken to be large. Since the large volume spectrum is under control, the partition function can be evaluated in the saddle point approximation which results in nonlinear integral equation for pseudo energies leading to an exact description of the ground state energy. Excited states on the complex (volume/coupling) plane are connected to the groundstate which enables one to derive nonlinear integral equations for excited states as well.

We start in Section 2 with a toy model containing one single particle with AdS dispersion relation and with scattering matrix which is not a function of the differences of the momenta. Although this is a fictitious system it helps to introduce conceptual notions and steps needed to explain the TBA which is, in analogy, used in Section 3 to present the results for planar AdS/CFT. Finally, we give a guide to the literature in Section 4 and list some open problems.

## 2 The concept of TBA: a toy model

The application of the TBA method to solve completely the finite volume spectral problem is standard by now and follows the following steps. First the scattering theory has to be solved in infinite volume by determining the scattering matrix from its generic properties such as symmetry, unitarity, crossing relation. The poles of the scattering matrix lying in the physical strip are related to bound-states. These bound-states have to be mapped and their scattering matrices have to be determined from the constituents' scattering matrices. Then in the second step these scattering matrices can be used to describe the spectrum for large volume, which amounts to restrict the allowed particles' momenta via phase shifts and periodicity, and use the dispersion relation to express the energy in terms of the quantized momenta. This method sums up all power like corrections in the inverse of the volume and provides an asymptotical spectrum. The very same asymptotic description of the mirror theory is also needed as it can be used to calculate the exponentially small finite energy corrections from the partition function. Evaluating the Euclidean partition function for large imaginary times (large mirror volumes) in the saddle point approximation provides integral equations describing the ground state energy exactly. Finally, these equations can be extended for excited states by analytical continuation. Now let us see how these steps are elaborated in the simplest setting.

---

<sup>1</sup>The method has its origin in the work of Yang and Yang applied for spin chains and for the Bose gas with  $\delta$  interaction [2].

### Infinite volume characteristics of the model

We consider a toy model with one single particle type only. The dispersion relation is supposed to be the same as in the AdS/CFT correspondence <sup>2</sup>:

$$E(p) = \sqrt{1 + 4g^2 \sin^2 \frac{p}{2}}$$

The sine function indicates lattice behavior and restricts the momentum as  $p \in [-\pi, \pi]$ . The square root, however, has a relativistic origin. The theory is supposed to be integrable, thus multiparticle scattering matrices factorize into two particle scatterings. As relativistic invariance is not supposed the two particle S-matrix can depend separately on the two momenta  $S(p_1, p_2)$  and satisfies unitarity  $S(p_1, p_2)S(p_2, p_1) = 1$  and crossing symmetry, which helps to fix it completely. We will not need its explicit form, but will suppose that in the  $p_1 = p_2 = p$  particular case  $S(p, p) = -1$ .

### Infinite volume characteristics of the mirror model

The Euclidean version of the model is defined by analytically continuing in the time variable  $t = iy$  and considering space  $x$  and imaginary time  $y$  on an equal footing. The Euclidean theory so obtained can be considered as an analytical continuation of another theory, in which  $x$  serves as the analytically continued time  $x = i\tau$  and  $y$  is the space coordinate. The theory defined in terms of  $y, \tau$  is called the mirror theory and its dispersion relation can be obtained by the same analytical continuation  $E = i\tilde{E}$  and  $p = i\tilde{p}$  which results in

$$\tilde{E}(\tilde{p}) = 2 \operatorname{arcsinh} \left( \frac{1}{2g} \sqrt{\tilde{p}^2 + 1} \right)$$

Contrary to the original theory the mirror model is not of the lattice type as its momentum can take any real value  $\tilde{p} \in \mathbb{R}$ . As the scattering matrix is related via the reduction formula to the Euclidean correlator the mirror S-matrix is simply the analytical continuation of the original scattering matrix:  $S(\tilde{p}_1, \tilde{p}_2)$ .

### Very large volume solution: asymptotic Bethe Ansatz for the model

Let us put  $N$  particles in a large volume  $L$  subject to periodic boundary condition. Integrability ensures that the particle number is conserved and the particles' momenta are not changed in the consecutive scatterings. The leading effect of the finite volume is the momentum quantization constraint:

$$1 = e^{ip_j L} \prod_{k:k \neq j}^N S(p_j, p_k) \quad (2.1)$$

which is called the Bethe Yang equation or asymptotic Bethe Ansatz (ABA) and follows from the periodicity of the multiparticle wave function. Due to the sine function in the

---

<sup>2</sup>The string tension is related to the 't Hooft coupling as  $2\pi g = \sqrt{\lambda}$

dispersion relation and the periodicity of  $p$  consistency of (2.1) requires  $L$  to take integer values only.

Bound-states of the theory are manifested in the ABA as complex string-like solutions. Indeed, if the scattering matrix has a pole for  $\Im m(p) > 0$ , then complex  $p$  solutions are also allowed in (2.1). If we take  $L$  very large with  $p_1 \approx \frac{p}{2} + iq$  then the rhs. of (2.1) would go to  $\infty$  which should be compensated by another complex momentum,  $p_2 \approx \frac{p}{2} - iq$  say, such that  $S(p_1, p_2)$  exhibits a pole. The two particles with momenta  $p_1$  and  $p_2$  form a bound-state with momentum  $p = p_1 + p_2$ , energy  $E_2(p) = E(p_1) + E(p_2)$  and scattering matrix  $S_{21}(p, p_j) = S(\frac{p}{2} + iq, p_j)S(\frac{p}{2} - iq, p_j)$ . In general complex solutions built up from more particles are also allowed and they usually form a string-like pattern. Their dispersion relation and scattering matrices can be calculated by extending the method above, which is called the S-matrix bootstrap.

### Very large volume solution: ABA for the mirror model

In the mirror model the considerations go along the same line as in the original theory. If we denote the mirror volume by  $R$  the ABA reads as

$$1 = e^{i\tilde{p}_j R} \prod_{k:k \neq j} S(\tilde{p}_j, \tilde{p}_k) \quad (2.2)$$

Since  $S(\tilde{p}_1, \tilde{p}_2)$  lives in a different analytical domain than  $S(p_1, p_2)$  its pole structure can be also different. If it exhibits poles also at the proper location the mirror theory has also bound-states. Once bound-states exist we can calculate their dispersion relation and scattering matrices from the bootstrap method. Suppose that the bound-states can be labeled with some charge  $Q$ , they have energy  $\tilde{E}_Q(\tilde{p})$  and their scattering matrix is  $S_{Q_j Q_k}(\tilde{p}_j, \tilde{p}_k)$ . The generic ABA valid for all the excitations (also for bound-states) will be

$$1 = e^{i\tilde{p}_j R} \prod_{k:k \neq j} S_{Q_j Q_k}(\tilde{p}_j, \tilde{p}_k) \quad (2.3)$$

Once these equations are solved the energy of the multiparticle state is

$$\tilde{E} = \sum_{j=1}^N \tilde{E}_{Q_j}(\tilde{p}_j)$$

which describes the spectrum asymptotically for large volumes  $R$ .

### Groundstate TBA equation from the partition function

Let us come back to the original model and see how the exact groundstate energy can be determined in a finite volume  $L$  from the Euclidean partition function. We exploit the fact that the imaginary time evolution for large times,  $R$ , is dominated by the lowest energy state

$$\lim_{R \rightarrow \infty} Z(L, R) = \lim_{R \rightarrow \infty} \text{Tr}(e^{-RH(L)}) = \lim_{R \rightarrow \infty} e^{-RE_0(L)} + \dots$$

| original model                                                                    | mirror model                                                                       |
|-----------------------------------------------------------------------------------|------------------------------------------------------------------------------------|
| $(t, x) \equiv (y = it, x)$                                                       | $(y, x = i\tau) \equiv (\tau, y)$                                                  |
| 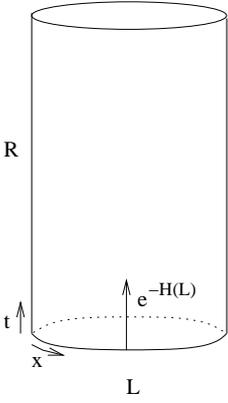 | 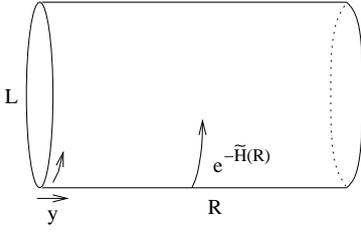 |
| $(E, P) \equiv (P_y = iE, P_x = P)$                                               | $(P_y = \tilde{P}, P_x = i\tilde{E}) \equiv (\tilde{E}, \tilde{P})$                |

**Table 1:** The relation between the original and the mirror model.

where the ellipsis represents terms exponentially suppressed in  $R$ . The same partition function can be determined alternatively, using the time evolution of the mirror theory which is generated by the mirror Hamiltonian  $\tilde{H}$ :

$$Z(L, R) = \tilde{Z}(R, L) = \text{Tr}(e^{-L\tilde{H}(R)}) = \sum_n e^{-L\tilde{E}_n(R)}$$

The relation between the original model and the mirror model is summarized in Table 1. In switching to the mirror model we ensure that the volume goes to infinity (and not the imaginary time) where the spectrum is controlled by the ABA (2.3).

In the large  $R$  limit the sum in the partition function is dominated by finite density particle states. Introducing the density of the particles (and bound-states) in momentum space ( $\rho_Q(\tilde{p}) = \frac{\Delta n_Q}{R\Delta\tilde{p}}$ ) the energy can be expressed as

$$\tilde{E}[\rho] = R \sum_Q \int d\tilde{p} \rho_Q(\tilde{p}) \tilde{E}_Q(\tilde{p}) = R \sum_Q \int du \rho_Q(u) \tilde{E}_Q(u)$$

where for later convenience we reparametrized the momentum as  $\tilde{p}(u)$ , momentum integrations go from  $-\infty$  to  $\infty$ . The quantization condition comes from taking the logarithm of the mirror ABA

$$\tilde{p}_j(u_j) + \sum_{Q'} \int du' (-i \log S_{Q_j Q'}(u_j, u')) \rho_{Q'}(u') = 2\pi \frac{n_j}{R} \quad (2.4)$$

where  $n_j$  labels the quantized momentum  $\tilde{p}_j$  whose charge is  $Q_j$ . For a generic multiparticle state there are momenta  $\tilde{p}_k$  which satisfy the same equation but which are not excited, not present in the system. They are called holes and their densities in the large volume limit is described by  $\bar{\rho}_Q$ . Clearly the densities of particles and holes are not

independent they are connected by the thermodynamical limit of eq. (2.4) as

$$\partial_u \tilde{p} - 2\pi(\rho_Q + \bar{\rho}_Q) = - \sum_{Q'} \int du' K_{QQ'}(u, u') \rho_{Q'}(u') =: -K_{QQ'} \star \rho_{Q'} \quad (2.5)$$

where the kernel is defined as

$$K_{QQ'}(u, u') = -i\partial_u \log S_{QQ'}(u, u')$$

The particle density itself does not characterize properly the states we sum over in the partition function. Indeed in a given interval  $(u, u + du)$  the occupied  $R\rho_Q(u)du$  particles can be distributed  $\binom{R(\rho_Q(u) + \bar{\rho}_Q(u))du}{R\rho_Q(u)du}$  different ways leading to an entropy factor in the sum. Since in the large particle number limit the factorials can be approximated with the Stirling formula the partition function will take the form

$$Z(L, R) = \sum_n e^{-L\tilde{E}_n(R)} = \sum_Q \int d[\rho_Q] e^{-L\tilde{E}[\rho_Q] + S[\rho_Q, \bar{\rho}_Q]}$$

where the entropy factor is

$$S[\rho_Q, \bar{\rho}_Q] = R \int du [(\rho_Q + \bar{\rho}_Q) \log(\rho_Q + \bar{\rho}_Q) - \rho_Q \log \rho_Q - \bar{\rho}_Q \log \bar{\rho}_Q]$$

One can slightly generalize the partition function by adding a chemical potential term to the energy  $-L\tilde{E}_Q[\rho_Q] \rightarrow \mu_Q[\rho_Q] - L\tilde{E}_Q[\rho_Q]$  where  $\mu_Q[\rho_Q] = R\mu_Q \sum_Q \int du \rho_Q(u)$ . For fermions we take  $\mu_Q = i\pi$ , while for bosons  $\mu_Q = 0$ . This extended partition function can be evaluated in the saddle point approximation. Taking into account the relation between  $\delta\rho_Q$  and  $\delta\bar{\rho}_Q$  originating from the variation of (2.5) we obtain the minimizing equation in the so called pseudo energy  $\epsilon_Q = \log \frac{\bar{\rho}_Q}{\rho_Q}$  as

$$\begin{aligned} \epsilon_Q(u) - L\tilde{E}_Q(u) + \mu_Q &= - \sum_{Q'} \int \frac{du'}{2\pi} K_{Q'Q}(u', u) \log(1 + e^{-\epsilon_{Q'}(u')}) \\ &=: -(\log(1 + e^{-\epsilon_{Q'}}) \star K_{Q'Q})(u) \end{aligned}$$

Once the pseudo energies are determined the ground state energy in volume  $L$  can be obtained as

$$E_0(L) = - \sum_Q \int \frac{du}{2\pi} (\partial_u \tilde{p}) \log(1 + e^{-\epsilon_Q(u)}) \quad (2.6)$$

The nonlinear integral equation which determines the pseudo energies is called the thermodynamic Bethe Ansatz (TBA) equation. Although it is not possible to solve it in general it provides an implicit exact description of the groundstate energy. This implicit solution is a starting point of a systematic large and small volume expansion and can be used to derive either functional relations for the pseudo energies or TBA equations for excited states by analytical continuation.

### Excited states by analytical continuation

Here we start with bosonic theories without bound-states and suppose that by analytically continuing in some parameter (say in the volume) we can reach all excited states. The way how excited states appear can be understood by analyzing the energy expression (2.6) integrated by parts

$$E = \int \frac{du}{2\pi} \tilde{p}(u) \partial_u \log(1 + e^{-\epsilon(u)})$$

Let us suppose that in the analytical continuation singularities of type  $1 + e^{-\epsilon(u_i)} = 0$  appear. When we deform the contour their residue contributions give rise to

$$E = \sum_i E(u_i) - \int \frac{du}{2\pi} \partial_u \tilde{p}(u) \log(1 + e^{-\epsilon(u)})$$

where we took into account the relation between the energy and the mirror momentum  $E(u_j) = i\tilde{p}(u_j)$ . Taking the same analytical continuation in the equation for the pseudo energy we obtain

$$\epsilon(u) = L\tilde{E}(u) + \sum_i \log S(u_i, u) - \int \frac{dw}{2\pi} K(w, u) \log(1 + e^{-\epsilon(w)})$$

Solving these equations iteratively for large  $L$  we can recognize that the  $1 + e^{-\epsilon(u_i)} = 0$  equations, which determine the positions of the singularities, coincide at leading order with the ABA equations (2.1). The subleading order calculation provides a universal formula for the leading finite size correction of multiparticle energy levels [5]. Alternatively for doing the analytical continuation one can think of the final result as choosing a different integration contour which surrounds the  $1 + e^{-\epsilon(u_i)} = 0$  singularities, and when we take the integration contour back to the real axis we pick up the above residue contributions.

Finally we note that if we have more species (labeled by  $Q$ ) with diagonal scatterings (like in the previous subsection) then a singularity in  $1 + e^{-\epsilon_{Q_i}(u_i)} = 0$  results in the equations

$$\epsilon_Q(u) = L\tilde{E}_Q(u) + \sum_i \log S_{Q_i Q}(u_i, u) - (\log(1 + e^{-\epsilon_{Q'}}) \star K_{Q'Q})(u)$$

whose solutions  $\epsilon_Q(u)$  and  $\{u_i\}$  have to be plugged into the energy formula

$$E = \sum_i E_{Q_i}(u_i) - \sum_Q \int \frac{du}{2\pi} \partial_u \tilde{p}_Q(u) \log(1 + e^{-\epsilon_Q(u)})$$

One has to be careful with such an analytical continuation in the presence of bound-states. Bound-states require pole singularities of the scattering matrices which usually cross the integration contour in the analytical continuation and result in extra source terms. See the Lee-Yang model in the relativistic case [3, 4] for example.

### 3 TBA for planar AdS/CFT

In this section we push forward the TBA program for planar AdS/CFT. The main difference compared to the previous discussion lies in the nondiagonal nature of the scattering matrix. There is a way, however, how we can profit from the previous diagonal results: the nondiagonal nature of any theory can be encoded into a diagonal theory but with auxiliary degrees of freedom. These auxiliary excitations do not contribute to the energy merely modifies the allowed momenta. Let us now follow the steps of Section 2.

#### 3.1 Infinite volume characteristics of the model

The symmetry algebra of the theory has a factorized form:  $su(2|2) \otimes su(2|2)$ . The fundamental particle called magnon transforms in the bifundamental representation whose S-matrix has the structure

$$\mathbb{S}_{11}(p_1, p_2) = S(p_1, p_2) \hat{S}_{11}(p_1, p_2) \otimes \hat{S}_{11}(p_1, p_2) \quad (3.1)$$

where the matrix part  $\hat{S}$  is fixed from its covariance under one copy of  $su(2|2)$  up to a scalar factor, which is determined from unitarity and crossing symmetry. The scattering matrix has simple poles corresponding to bound-states. There is an infinite tower of bound-states labeled by a positive integer charge  $Q$ . They transform under the tensor product of the atypical totally *symmetric* representations of the algebra and have dispersion relation

$$E_Q(p) = \sqrt{Q^2 + 4g^2 \sin^2 \frac{p}{2}}$$

#### 3.2 Infinite volume characteristics of the mirror model

As the mirror model is derived from the same Euclidean theory the fundamental particles' scattering matrix is the analytical continuation of the scattering matrix (3.1). We are in a different analytical domain, however, and here different poles correspond to bound-states. These bound-states are also labeled by the charge  $Q$  but they transform under the atypical totally *antisymmetric* representations and have dispersion relation:

$$\tilde{E}_Q(\tilde{p}) = 2 \operatorname{arcsinh} \left( \frac{1}{2g} \sqrt{\tilde{p}^2 + Q^2} \right)$$

#### 3.3 Very large volume solution: ABA for the model

If we put  $N$  particles in a finite volume  $L$  the momenta of the particles will be quantized. The multiparticle wave function has to be periodic in each argument, that is when a particle transported along the cylinder it scatters on all other particles before arriving back to its initial position. In a diagonal theory this results in (2.1). In a nondiagonal theory, however, the multiparticle transfer matrix has to be diagonalized. This can be achieved by introducing new type of (magnonic) particles with vanishing dispersion relations and considering the original problem in terms of them as a diagonal scattering theory.

Here we focus only on the charge  $Q = 1$  sector of the theory. We have momentum carrying particles ( $\bullet_1$ ) which scatter on each other as <sup>3</sup>

$$S_{11}^{\bullet\bullet}(p_1, p_2) = S(p_1, p_2) = \frac{x_1^+ - x_2^-}{x_1^- - x_2^+} \frac{1 - \frac{1}{x_1^- x_2^+}}{1 - \frac{1}{x_1^+ x_2^-}} \sigma_{12}^{-2}$$

where  $x^\pm(p) = \frac{(\cot \frac{p}{2} \pm i)}{2g} \left(1 + \sqrt{1 + 4g^2 \sin^2 \frac{p}{2}}\right)$  and  $\sigma$  represents the dressing phase. These particles are extended for each  $su(2|2)$  factor with two types of auxiliary particles ( $y, \circ_1$ ), whose parameters are labeled by  $y \in \mathbb{R}$  and  $w \in \mathbb{R}$ . The auxiliary particles have trivial dispersion relations (their energy and momentum are zero) and scatter with the fundamental, momentum carrying ones as

$$S_{1y}^{\bullet y}(p, y) = \frac{x^- - y}{x^+ - y} \sqrt{\frac{x^+}{x^-}} = S_{y1}^{y\bullet}(y, p)^{-1} \quad ; \quad S_{11}^{\bullet\circ}(p, w) = 1$$

Furthermore, they scatter on each other as

$$S_{11}^{\circ\circ}(w_1, w_2) = S_{-2}(w_1 - w_2) \quad ; \quad S_{y1}^{y\circ}(y, w) = S_1(v(y) - w) \quad ; \quad S_{yy}^{yy}(y_1, y_2) = 1$$

where  $v(y) = y + y^{-1}$  and we introduced a useful function  $S_n(v - w) = \frac{v - w + \frac{in}{g}}{v - w - \frac{in}{g}}$ . Any scattering matrix can be extended by unitarity to the opposite order of their particle types/arguments:  $S(i, j)S(j, i) = 1$ .

In formulating the ABA equations for the full theory we have to take into account the two  $su(2|2)$  factors and that they commute. The ABA equation for the momentum carrying particles reads as

$$1 = e^{ip_j L} \prod_{k:k \neq j}^{N_1^\bullet} S_{11}^{\bullet\bullet}(p_j, p_k) \prod_{\alpha=1,2} \prod_{l=1}^{N_{y\alpha}} S_{1y}^{\bullet y}(p_j, y_l^\alpha)$$

where  $N_1^\bullet$  is the number of fundamental and  $N_{y\alpha}$  the number of  $y$  type particles, while the  $\alpha = 1, 2$  index refers to the two  $su(2|2)$  factors. Since the two factors commute the ABA equations for the auxiliary particles with rapidities  $y^{1,2}$  and  $w^{1,2}$  can be written as

$$\prod_{k:k \neq j}^{N_1^\bullet} S_{y1}^{y\bullet}(y_j^\alpha, p_k) \prod_{l=1}^{N_{1,\alpha}^\circ} S_{y1}^{y\circ}(y_j^\alpha, w_l^\alpha) = 1 = \prod_{k:k \neq j}^{N_{y\alpha}} S_{1y}^{\circ y}(w_j^\alpha, y_k^\alpha) \prod_{l:l \neq k}^{N_{1,\alpha}^\circ} S_{11}^{\circ\circ}(w_j^\alpha, w_l^\alpha)$$

Not all solutions of the ABA equations correspond to single trace operators as the level matching/zero momentum condition has to be fulfilled  $\sum_j p_j = 0$ . The theory contains also bound-states which can be determined from the singularity structure of the scattering matrices. Since from the TBA point of view only the bound-state spectrum of the mirror theory is relevant we will focus only on them.

<sup>3</sup>The index 1 in  $\bullet_1$  refers to the charge of the particle. This particle is a first member of an infinite series of bound-states labeled by  $\bullet_Q$ . Similarly we will meet particles of type  $\circ_N$  and  $\triangleright_M$ .

### 3.4 Very large volume solution: ABA for the mirror model

In the case of the mirror theory the fundamental scattering matrix is the analytical continuation of the original one  $p \rightarrow \tilde{p}$ . As a result the ABA will be the analytical continuation, too

$$1 = e^{i\tilde{p}_j R} \prod_{k:k \neq j}^{N_1^\bullet} S_{11}^{\bullet\bullet}(\tilde{p}_j, \tilde{p}_k) \prod_{\alpha=1,2} \prod_{l=1}^{N_{y^\alpha}} S_{1y}^{\bullet y}(\tilde{p}_j, y_l^\alpha) \quad (3.2)$$

$$-1 = \prod_{k:k \neq j}^{N_1^\bullet} S_{y1}^{y\bullet}(y_j^\alpha, \tilde{p}_k) \prod_{l=1}^{N_{1,\alpha}^\circ} S_{y1}^{y^\circ}(y_j^\alpha, w_l^\alpha) \quad (3.3)$$

$$1 = \prod_{k:k \neq j}^{N_y^\alpha} S_{1y}^{\circ y}(w_j^\alpha, y_k^\alpha) \prod_{l:l \neq k}^{N_w^\alpha} S_{11}^{\circ\circ}(w_j^\alpha, w_l^\alpha) \quad (3.4)$$

There are some differences compared to the original ABA. First the domain of  $\tilde{p} \in \mathbb{R}$  is different compared to  $p \in [-\pi, \pi]$  and the total mirror momentum does not need to vanish. Then, as we are in the mirror theory, the way how  $x^\pm$  is expressed in terms of  $\tilde{p}$  is also different:  $x^\pm = \frac{(\tilde{p}-i)}{2g} \left( \sqrt{1 + \frac{4g^2}{1+\tilde{p}^2}} \mp 1 \right)$ . Additionally, in the calculations of the ground state energy the sectors with antiperiodic fermions are relevant and this is manifested in a minus sign in the middle equation. The possible bound-states and their ABA equations are the subject of the next section. Let us note that usually in the literature instead of (3.4) its inverse is considered as this will lead to positive particle densities in the thermodynamic limit.

### 3.5 Exact groundstate energy: TBA

In this section we derive TBA integral equations for the groundstate energy in finite volume  $R$ . We treat the theory as if it were diagonal with the scattering matrices specified above. First we analyze whether this “diagonal” theory has bound-states by analyzing the thermodynamic behavior of the equations and calculate the scattering matrices of the bound-states, the so called strings. They are special complex solutions of the ABA equations and they all contribute to the partition function which determines the ground state energy. Then we use the canonical procedure to derive coupled integral equations for the pseudo energies in a raw form, finally, using identities between the scattering matrices originating from the symmetry, we rewrite them in a simplified form and analyze simple excited states.

#### 3.5.1 String hypothesis for the mirror model

The string hypothesis is similar to closing the S-matrix bootstrap program, that is to identify all particles (including bound-states) of the theory and to determine their scattering matrices. Let us premise that we will find bound-states of three infinite types  $(\bullet_Q, \triangleright_M, \circ_N)$  for  $Q, M, N \in \mathbb{N}$ , and also of a finite type  $y_\delta$  particle with  $\delta \in \{\pm\}$ . They

can be arranged in the two dimensional lattice shown in Figure 1. Let us see how they arise from the ABA equations.

In the following we put  $R$  and all particle numbers large (keeping their ratio finite) and analyze the ABA one by one. Let us first note the reality properties of the equations. Unitarity of the mirror scattering matrix implies that the  $y$  roots come in complex conjugated pairs  $y_i = (y_j^{-1})^*$  or lie on the unit circle  $y = (y^{-1})^*$ , similarly the roots  $w$  come in complex conjugated pairs  $w_i = w_j^*$  or are real.

### • $Q$ particles

In looking for momentum bound-states we rewrite the scattering matrix in (3.2) as

$$S_{11}^{\bullet\bullet}(\tilde{p}_1, \tilde{p}_2) = \frac{u_1 - u_2 + \frac{2i}{g}}{u_1 - u_2 - \frac{2i}{g}} \Sigma_{11}^{-2} \quad ; \quad \Sigma_{11} = \frac{1 - \frac{1}{x_1^+ x_2^-}}{1 - \frac{1}{x_1^- x_2^+}} \sigma$$

where the rapidity is introduced as  $u \pm \frac{i}{g} = x^\pm + \frac{1}{x^\pm}$ . As  $R$  is very large complex values for  $u_1$  with positive imaginary part are allowed. In this case the lhs. of (3.2) for  $j = 1$  diverges so there should be another  $u$  say  $u_2$  that goes to  $u_1 - \frac{2i}{g}$ . If  $u_2$  still has a positive imaginary part then by the same argument there should be another  $u$  say  $u_3$  which goes to  $u_2 - \frac{2i}{g}$ . Applying this procedure we arrive at a string of  $Q$  roots  $u + (Q-1)\frac{i}{g}, u + (Q-3)\frac{i}{g}, \dots, u - (Q-3)\frac{i}{g}, u - (Q-1)\frac{i}{g}$  or shortly  $u_{Q+1-2j} = u + i(Q+1-2j)\frac{i}{g}$  where  $j = 1, \dots, Q$ . (Clearly the  $Q = 1$  string is the original particle itself.) The scattering of the  $Q$ -string with any other particle of type  $(.)$ , label  $i$  and rapidity  $q$  is

$$S_{Q_i}^{\bullet\bullet}(u, q) = \prod_{j=1}^Q S_{i_1}^{\bullet\bullet}(u_{Q+1-2j}, q) = S_{i_Q}^{\bullet\bullet}(q, u)^{-1}$$

Although naively the scattering matrices seem to depend on the parameters  $x^\pm$  and such a way the bound-state scattering matrix depends on its constituents, this is not the case when we take into account the contributions of the dressing phase as was shown in [6].

The auxiliary particles exist for both  $su(2|2)$  factors. Here we focus only on one of them and omit to write out its index.

### $y_\delta$ particles

Let us analyze (3.3). If we suppose that the number of momentum carrying particles  $N_1^\bullet$  goes to infinity then

$$\prod_{k:k \neq j}^{N_1^\bullet} S_{y_1}^{y_\bullet}(y_j, \tilde{p}_k) \rightarrow \begin{cases} 0 & \text{if } |y_j| < 1 \\ \pm 1 & \text{if } |y_j| = 1 \\ \infty & \text{if } |y_j| > 1 \end{cases} \quad (3.5)$$

In the middle case  $y$  roots lying on the unit circle are allowed. As the scattering matrix  $S_{y_1}^{y_\bullet}(y, w)$  has a difference form in the variable  $v(y) = y + y^{-1}$  we might use the parameter  $v$  instead of  $y$ . The inverse of the relation, however, is not unique. Defining  $y_-(v) =$

$\frac{1}{2}(v - i\sqrt{4 - v^2})$  with the branch cuts running from  $\pm\infty$  to  $\pm 2$  we can describe any  $y$  with  $\Im m(y) < 0$  for  $v \in [-2, 2]$ . Clearly  $y_+(v) = y_-(v)^{-1}$  describes the other  $\Im m(y) > 0$  case and in the scattering matrices  $S_{y_1}^{y_\bullet}$  which depends on  $y$ , and not on  $v$ , we have to specify which root is taken. As a consequence we have two types of  $y$  particles  $y_\delta$  with  $\delta = \pm$  and the scattering matrices split as  $S_{y_1}^{y_\bullet}(y, q) \rightarrow S_{\delta_1}^{y_\bullet}(y_\delta(v), q) =: S_{\delta_1}^{y_\bullet}(v, q)$ .

### $\triangleright_M$ particles

If  $|y_1| < 1$  in (3.5) then the rhs. of (3.3) goes to zero which has to be compensated by a  $w_1$  root which goes to  $v_1 - \frac{i}{g} = y_1 + y_1^{-1} - \frac{i}{g}$ . But then taking the ABA for  $w_1$  means that the rhs. of (3.4) will diverge which has to be compensated by a root  $v_2 = w_1 - \frac{i}{g}$ . If the corresponding  $y_2$  satisfies  $|y_2| > 1$  then (3.3) is consistent with (3.5) and reality requires  $y_1 = (y_2^{-1})^*$ ,  $w_1 = w_1^*$ . The three roots  $y_1 \leftrightarrow v_1 = v + \frac{i}{g}$  and  $w_1 = v$  and  $v - \frac{i}{g} = v_2 \leftrightarrow y_2$  form an  $M = 1$  string which we denote by  $\triangleright_1$ . In the case when  $|y_2| < 1$  then we have to repeat the same arguments for  $y_2$  leading to  $w_2$  and  $y_3$  and so on. Finally we arrive at the notion of a  $\triangleright_M$  string. It consists of  $2M$   $y$  particles with  $y_j = (y_{-j}^{-1})^*$  and  $M$   $o$  particles with synchronized parameters  $w_{M+1-2j} = v + (M+1-2j)\frac{i}{g}$  and  $y_j \rightarrow v_{\text{sign}(j)(M+2-2j)} = v + \text{sign}(j)(M+2-2j)\frac{i}{g}$  for  $j = 1, \dots, M$ . The composite scattering matrix of the  $\triangleright_M$  particle with all other particles is simply the product of the scatterings of its each individual constituents

$$S_{M_i}^{\triangleright}(v, q) = \prod_{j=1}^{M+1} S_{-i}^{y_j}(v_{M+2-2j}, q) \prod_j^M S_{1i}^{o_j}(w_{M+1-2j}, q) \prod_{j=1}^{M-1} S_{+i}^{y_j}(v_{M-2j}, q) = S_{iM}^{\triangleright}(i, v)^{-1}$$

### $\circ_N$ particles

Suppose we have a large number of  $y$  particles and that  $w_1$  has a positive imaginary part. Then the first factor of the rhs. of (3.4) will go to zero which has to be compensated by a root  $w_2 = w_1 - \frac{2i}{g}$ . If  $\Im m(w_2) < 0$  then we obtain a  $\circ_2$  string. In the opposite case we repeat to previous argumentation leading to an  $N$  string  $w_{N+1-2j} = w + (N+1-2j)\frac{i}{g}$ . Clearly a single  $w$  is just a  $\circ_1$  string. The scattering of the  $N$  string with any other particle is

$$S_{N_i}^{\circ}(w, i) = \prod_{j=1}^N S_{wi}^{o_j}(w_{N+1-2j}, i)$$

### Scattering matrices

Summarizing, the mirror AdS theory in the thermodynamic limit could be replaced by a diagonal theory having constituents of infinite type  $(\bullet, \triangleright, \circ)$  and index  $Q, M, N$  for  $Q, M, N \in \mathbb{N}$ , and also of finite type  $y$  particles with  $\delta \in \{\pm\}$ . See also Figure 1.

For the readers convenience we summarize the scattering matrices in Table 2. The

|                    | $\bullet_{Q'}$                    | $\triangleright_{M'}$                    | $\circ_{N'}$             | $y_{\delta'}$                     |
|--------------------|-----------------------------------|------------------------------------------|--------------------------|-----------------------------------|
| $\bullet_Q$        | $S_{QQ'}^{\bullet\bullet}$        | $S_{QM'}^{\bullet\triangleright}$        | 1                        | $S_{Q\delta'}^{\bullet y}$        |
| $\triangleright_M$ | $S_{MQ'}^{\triangleright\bullet}$ | $S_{MM'}^{\triangleright\triangleright}$ | 1                        | $S_{M\delta'}^{\triangleright y}$ |
| $\circ_N$          | 1                                 | 1                                        | $S_{NN'}^{\circ\circ}$   | $S_{N\delta'}^{\circ y}$          |
| $y_\delta$         | $S_{\delta Q'}^{y\bullet}$        | $S_{\delta M'}^{y\triangleright}$        | $S_{\delta N'}^{y\circ}$ | 1                                 |

**Table 2:** Scattering matrices of the various particles

scattering matrices are unitary  $S_{ij}S_{ji} = 1$  and their explicit forms are

$$\begin{aligned}
 S_{QQ'}^{\bullet\bullet}(u, u') &= S_{QQ'}(u - u') \Sigma_{QQ'}(u, u')^{-2} \\
 S_{QQ'}(u - u') &= S_{Q+Q'}(u - u') S_{Q'-Q}(u - u') \prod_{j=1}^{Q-1} S_{Q'-Q+2j}(u - u')^2 \\
 \Sigma_{QQ'}(u, u') &= \prod_{j=1}^Q \prod_{k=1}^{Q'} \sigma(u_{Q+1-2j}, u_{Q'+1-2k}) \frac{1 - \frac{1}{x(u_{Q-2j})x(u_{Q'+2-2k})}}{1 - \frac{1}{x(u_{Q+2-2j})x(u_{Q'-2k})}}
 \end{aligned}$$

where  $u_j = u + j\frac{i}{g}$  and we reparametrized the momentum carrying particles in terms of the rapidity via the function  $x(u) = \frac{1}{2}(u - i\sqrt{4 - u^2})$ . Recall also that  $S_n(u - w) = \frac{u_n - w}{u_n - w}$ . The other matrix elements are

$$\begin{aligned}
 S_{QM}^{\bullet\triangleright}(u, v) &= \frac{x(u_{-Q}) - x(v_M)}{x(u_Q) - x(v_M)} \frac{x(u_{-Q}) - x(v_{-M})}{x(u_Q) - x(v_{-M})} \frac{x(u_Q)}{x(u_{-Q})} \prod_{j=1}^{M-1} S_{M-Q-2j}(u, v) \\
 S_{Q\delta}^{\bullet y}(u, v) &= \frac{x(u_{-Q}) - x(v)^\delta}{x(u_Q) - x(v)^\delta} \sqrt{\frac{x(u_Q)}{x(u_{-Q})}} \\
 S_{MM'}^{\triangleright\triangleright}(u, u) &= S_{MM'}(u - u') = S_{MM'}^{\circ\circ}(u, u')^{-1} \\
 S_{M\delta}^{\triangleright y}(u, v) &= S_M(u - v) = S_{M\delta}^{\circ y}(u, v)
 \end{aligned}$$

The ABA equations then have a generic form

$$(-1)^F = e^{i\tilde{p}\cdot(q_j)R} \prod_k S_{jQ_k}^{\bullet\bullet}(q_j, u_{Q_k}) \prod_{\alpha=1,2} \prod_l S_{j\delta_l}^{\bullet y}(q_j, v_l^\alpha) \prod_m S_{jM_m}^{\bullet\triangleright}(q_j, v_{M_m}^\alpha) \prod_n S_{jN_n}^{\circ\circ}(q_j, w_{N_n})$$

where  $\bullet$  can be any type of  $\bullet, \triangleright, \circ, y$  but only the  $\bullet$  particles have nonvanishing energy  $\tilde{E}_Q$  and momentum  $\tilde{p}_Q(u) = g(x(u_{-Q}) - x(u_Q)) + iQ$ . The parameter  $F$  denotes the fermion number. We also indicated the contributions of the two  $su(2|2)$  factors. The energy of such a multiparticle state having  $N_{Q_k}^\bullet$  of  $Q_k$  particles is

$$\tilde{E}(\tilde{p}_1, \dots, \tilde{p}_k) = \sum_k \tilde{E}_{Q_k}(\tilde{p}_k)$$

Let us note that the ABA equations for the auxiliary particles can be inverted without changing their physical meaning. Taking the inverse of (3.4) is equivalent to redefining simultaneously the scattering matrices  $S_{1\delta}^{\circ y} \rightarrow (S_{1\delta}^{\circ y})^{-1}$  and  $S_{11}^{\circ\circ} \rightarrow (S_{11}^{\circ\circ})^{-1}$ . Actually these are the equations used in the literature as they give positive particle densities in the thermodynamic limit.

### 3.5.2 Raw TBA equations

Suppose now that we would like to describe the groundstate energy in the AdS system in volume  $L$ . In doing so we follow the steps presented in Section 2 to evaluate the partition function for large mirror sizes. We introduce densities of particles (strings)  $\rho_Q^\bullet(u)$ ,  $\rho_M^\triangleright(u)$ ,  $\rho_N^\circ(u)$  for  $u \in \mathbb{R}$  and  $\rho_\delta^y(u)$  for  $u \in [-2, 2]$  and the analogous densities of holes  $\rho \rightarrow \bar{\rho}$ . They are restricted via the logarithm of the ABA which contains the logarithmic derivatives of the scattering matrices

$$K_{jj'}(u, u') = -i\partial_u \log S_{jj'}(u, u')$$

Clearly  $K_{jj'}(u, u') \neq -K_{j'j}(u', u)$  as the scattering matrices are not of the difference type. (Keeping in mind how we obtained the string solutions the densities are naturally ordered  $\rho_Q^\bullet \gg \rho^y \gg \rho_N^\circ, \rho_M^\triangleright$ .) Then we introduce the entropy factors for the densities,  $i\pi$  chemical potential for fermions and calculate the saddle point of the functional integral. This results in integral equations for the pseudo energies  $\epsilon_Q^\bullet, \epsilon_M^\triangleright, \epsilon_N^\circ, \epsilon_\delta^y$  as follows

$$\epsilon_Q^\bullet = L\tilde{E}_Q - \log(1 + e^{-\epsilon_{Q'}}^\bullet) \star K_{Q'Q}^\bullet - \log(1 + e^{-\epsilon_M^\triangleright}) \star K_{MQ}^\triangleright - \log(1 + e^{-\epsilon_\delta^y}) \star K_{\delta Q}^{y\bullet}$$

where in the contributions of the  $\triangleright_M$  and  $y_\delta$  we have to sum for the contributions of the two  $su(2|2)$  factors (which we omitted to write out). The remaining equations are valid separately for the two  $su(2|2)$  factors separately:

$$\begin{aligned} \epsilon_M^\triangleright &= -\log(1 + e^{-\epsilon_Q^\bullet}) \star K_{QM}^\triangleright - \log(1 + e^{-\epsilon_{M'}}^\triangleright) \star K_{M'M}^\triangleright - \log(1 + e^{-\epsilon_\delta^y}) \star K_{\delta M}^{y\triangleright} \\ \epsilon_N^\circ &= \log(1 + e^{-\epsilon_{N'}}^\circ) \star K_{N'N}^\circ + \log(1 + e^{-\epsilon_\delta^y}) \star K_{\delta N}^{y\circ} \\ \epsilon_\delta^y &= -\log(1 + e^{-\epsilon_Q^\bullet}) \star K_{Q\delta}^{y\bullet} - \log(1 + e^{-\epsilon_M^\triangleright}) \star K_{M\delta}^{y\triangleright} - \log(1 + e^{-\epsilon_N^\circ}) \star K_{N\delta}^{y\circ} + i\pi \end{aligned}$$

Once these equations are solved the groundstate energy can be obtained as

$$E_0(L) = -\sum_{Q=1}^{\infty} \int \frac{du}{2\pi} \partial_u \tilde{p}_Q \log(1 + e^{-\epsilon_Q^\bullet})$$

Finally we note that we replaced the magnonic ABA for the particle type  $\circ_N$  with its inverse and made the corresponding change in the scattering matrices to ensure the positivity of the magnonic densities  $\rho_N^\circ$ . It effectively changed the sign of the related kernels.

### 3.5.3 Simplified TBA equations and Y-system

In this subsection using identities among the TBA kernels we bring the equations in to a universal local form. This means that pseudo energies can be drawn in a two dimensional lattice, such that only neighboring sites couple to each other with the following universal kernel

$$s I_{MN} = \delta_{MN} - (K+1)_{MN}^{-1} \quad ; \quad s(u) = \frac{g}{4 \cosh \frac{g\pi u}{2}} \quad (3.6)$$

where  $I_{MN} = \delta_{M+1,N} + \delta_{M-1,N}$  and  $(K+1)_{MN}^{-1} \star (K_{NL} + \delta_{NL}) = \delta_{ML}$ . To simplify the notation let us introduce the following  $Y$  functions

$$Y_Q^\bullet = e^{-\epsilon_Q^\bullet} \quad ; \quad Y_M^\triangleright = e^{-\epsilon_M^\triangleright} \quad ; \quad Y_N^\circ = e^{\epsilon_N^\circ} \quad ; \quad Y_\delta^y = e^{\delta \epsilon_\delta^y}$$

Clearly we have two copies for  $Y_M^{\triangleright,\alpha}, Y_N^{\circ,\alpha}, Y_\delta^{y,\alpha}$ . (To conform with the literature we inverted the ABA equations for  $\triangleright_M$  and  $y_-$ ). Acting with the operator (3.6) on these inverted TBA equations and using kernel identities like  $(K+1)_{MN}^{-1} \star K_N = s \delta_{M,1}$  we arrive at their simplified, universal form

$$\begin{aligned} \log Y_M^\triangleright &= \log(1 + Y_{M+1}^\bullet) \star s - I_{MM'} \log\left(1 + \frac{1}{Y_{M'}^\triangleright}\right) \star s + \delta_{M,1} \log \frac{1 + Y_+^y}{1 + \frac{1}{Y_-^y}} \hat{\star} s \\ \log Y_N^\circ &= I_{NN'} \log(1 + Y_{N'}^\circ) \star s + \delta_{N,1} \log \frac{1 + Y_-^y}{1 + \frac{1}{Y_+^y}} \hat{\star} s \end{aligned}$$

where in the convolution  $\hat{\star}$  we integrate over the interval  $[-2, 2]$  only. The other equations do not behave so nicely.

$$\begin{aligned} \log Y_Q^\bullet &= -I_{QQ'} \log\left(1 + \frac{1}{Y_{Q'}^\bullet}\right) \star s + \log(1 + Y_{Q-1}^{\triangleright,1}) \star s + \log(1 + Y_{Q-1}^{\triangleright,2}) \star s \quad ; \quad Q > 1 \\ \log Y_1^\bullet &= -\log\left(1 + \frac{1}{Y_2^\bullet}\right) \star s + (\log(1 + Y_-^{y,1})(1 + Y_-^{y,2})) \star s - \check{\Delta} \star s \end{aligned}$$

where  $\check{\Delta}$  vanishes on the interval  $[-2, 2]$  whose explicit form can be found in [7]. The equation for the  $y$  particles are simpler in the original form

$$\delta \log Y_\delta^y = -\log(1 + Y_Q^\bullet) \star K_{Q\delta}^{\bullet,y} + \log \frac{1 + Y_M^\triangleright}{1 + \frac{1}{Y_M^\circ}} \star K_M + i\pi$$

These equations for  $Y_\delta^y$  are not in a local form. However, acting with the inverse of  $s$  they can be brought into such form. The operator  $s^{-1}$  acts as  $(f \star s^{-1})(u) = f(u + \frac{i}{g} - i0) + f(u - \frac{i}{g} + i0)$  and involves the analytical continuation of the functions. It has a large null space, thus when acting on the equation information is lost:

$$\log Y_-^y \star s^{-1} = \log(1 + Y_1^\bullet) + \log(1 + Y_1^\circ) - \log\left(1 + \frac{1}{Y_1^\triangleright}\right)$$

The advantage of defining  $s^{-1}$  in the above manner is that it uses the analytically continued values of the  $Y$  functions on the rapidity torus only. If we continue them across the cuts by using  $(f \star s^{-1})(u) = f(u + \frac{i}{g} - i0) + f(u - \frac{i}{g} - i0) = f^+(u) + f^-(u)$  then the term  $\check{\Delta}$  disappears, but the  $Y$  functions have to be extended to an infinite genus Riemann surface. On this surface the  $Y$ -system has the universal form

$$Y_{N,M}^+ Y_{N,M}^- = \frac{(1 + Y_{N,M+1})(1 + Y_{N,M-1})}{(1 + Y_{N-1,M}^{-1})(1 + Y_{N+1,M}^{-1})} \quad (3.7)$$

where the  $N, M$  indices live on a two dimensional integral lattice. In our situation the identification can be drawn on Figure 1, which explicitly reads as  $Y_Q^\bullet = Y_{Q,0}$ ,  $Y_M^{\triangleright,\alpha} = Y_{M+1,\nu_\alpha}$ ,  $Y_N^{\circ,\alpha} = Y_{1,\nu_\alpha(N+1)}$ ,  $Y_-^{y,\alpha} = Y_{1,\nu_\alpha}$  and  $Y_+^{y,\alpha} = Y_{2,\nu_\alpha 2}$  where  $\nu_1 = 1$  and  $\nu_2 = -1$ .

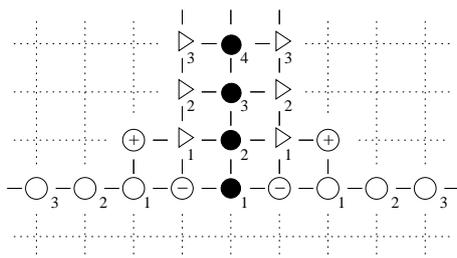

**Figure 1:**  $Y$ - system for planar AdS/CFT.  $Y_-$  is denoted by  $\ominus$  while  $Y_+$  by  $\oplus$ .

### 3.5.4 Excited states by analytical continuation

Here we focus on the TBA equations for excited states in the  $sl_2$  sector for small coupling. This sector contains particles of type  $\bullet_1$  only and have ABA:

$$1 = e^{ip_k L} \prod_{j:j \neq k} S_{11}^{\bullet\bullet}(p_k, p_l)$$

These equations are asymptotic only and the exact system of TBA equations is required to describe the energy of the multiparticle state exactly. As the vacuum is a BPS state it has vanishing energy and its analytical continuation cannot describe excited states. Alternatively we choose an integration contour, such that when it is taken back to the real axis the residue of a singularity of the form  $1 + e^{-\epsilon_1^{\bullet}(p_k)} = 0$  is picked up resulting in additional source terms in the raw equations as:

$$\epsilon_Q^{\bullet} \rightarrow \sum_j \log S_{1Q}^{\bullet\bullet}(p_j, u) \quad ; \quad \epsilon_M^{\triangleright} \rightarrow \sum_j \log S_{1M}^{\triangleright\bullet}(p_j, u) \quad ; \quad \epsilon_\delta^y \rightarrow \sum_j \log S_{1\delta}^{\bullet y}(p_j, u)$$

Once the new system of TBA equations are solved the pseudo energies  $\epsilon_Q^{\bullet}$  have to be plugged into the energy formula:

$$E(L) = \sum_k E_1(p_k) - \sum_{Q=1}^{\infty} \int \frac{du}{2\pi} \partial_u \tilde{p}_Q \log(1 + e^{-\epsilon_Q^{\bullet}})$$

to obtain the energy of the multiparticle system.

We can rewrite the TBA equations in terms of the  $Y$  functions into their simplified form. They satisfy the same  $Y$ -system relations (3.7) but with a different asymptotical behavior. There is a systematical asymptotical expansion of the  $Y$ -system, which reproduces both the ABA and the leading Lüscher correction of these multiparticle states. This is valid for weak coupling  $g \rightarrow 0$  (or large sizes) and it is very nontrivial to follow the analytical behavior of the  $Y$  functions as one increases the coupling. The ABA solution itself suggests, that additional  $1 + Y = 0$  singularities could appear and then the TBA equations have to be modified by additional source terms. These source terms ensure the analytical behavior of the energy around these singular points.

## 4 Guide to the literature

Here we list the representative papers where the various parts of the TBA program were developed.

The idea that the TBA program can be applied in the planar AdS/CFT setting was presented in [9]. The infinite volume scattering description of theory can be found in chapters [10, 11]. The ABA equations for the planar AdS/CFT model was conjectured in [12] (and thoroughly discussed in chapters [13, 14]), while the analogous ABA for the mirror model was described in [15]. As the color structure ( $su(2|2)$ ) of the scattering matrix is the same as that of the Hubbard model, the Hubbard TBA solution can be adopted [16]. This results in the string hypothesis which was formulated explicitly in [17]. The standard procedure leads to raw TBA equations, which were developed in [19, 18, 20]. The simplified form of the TBA equations was presented in [7] and the Y-system relations, presented previously in [21], were derived in [19, 18, 20]. In doing this the analytical properties of the dressing phase [6, 20, 22] had to be investigated. In the AdS/CFT context the volume of the integrable system has to be an integer, which can be seen also on the groundstate TBA [23].

Although we obtained the Y-system from the ground-state TBA equations, in principle, it follows from the hidden  $PSU(2, 2|4)$  symmetry of the model. An independent alternative approach based on this symmetry is the subject of the next Chapter in this volume [24].

The Y-system plays a crucial role in describing excited states. As it is related to the symmetry of the model [24–26] it is the same for each state. What makes the difference is the asymptotical and analytical behavior of the Y-functions. The analytical properties of the Y-functions was thoroughly analyzed in [19, 28, 23, 8]. Based on the solution of the Y-system of the  $O(4)$  model [27] the authors of [21] identified the large volume solution in terms of the transfer matrices of the ABA [14]. This helps to derive excited states TBA equations for the  $sl_2$  sector, which was done in [20, 28]. The excited state TBA equations provide an exact description of the given state and they were used in the Konishi case, [29, 30], to analyze numerically the behavior of the energy for large coupling. The results are summarized in Figure 2<sup>4</sup>, see also [31]. It was further shown in [28] how to modify these excited state TBA equations if a  $1 + Y = 0$  singularity appears in the analytical continuation in  $g$ .

The weak coupling limit of the Y-system equations can be compared to the ABA [14] and Lüscher type correction [32]. The leading order behavior is built in the asymptotic solution [21] of the Y-function, but the next to leading one provides a stringent test of the excited states TBA equations, which was performed numerically for the Konishi operator in [33] and analytically at next to leading order in [34]. Later this analytical calculation was extended to describe the next to leading order Lüscher correction of generic twist two states [35] in [36].

The strong coupling limit of the Y-system for a finite density of string particles was analyzed in [37], where a complete agreement with the one loop string energies including all exponential finite size corrections has been found. The functional Y-system equations were encoded into simpler  $Q$  functions in [38, 25, 31].

Let us mention, how our TBA equations are related to those in the literature. We summarized the relation between the various conventions for half of the Y-system in Table 2 as the other half is trivially related, see also [8]. Under this replacement our simplified

---

<sup>4</sup>We thank the authors of [31] for borrowing their figure.

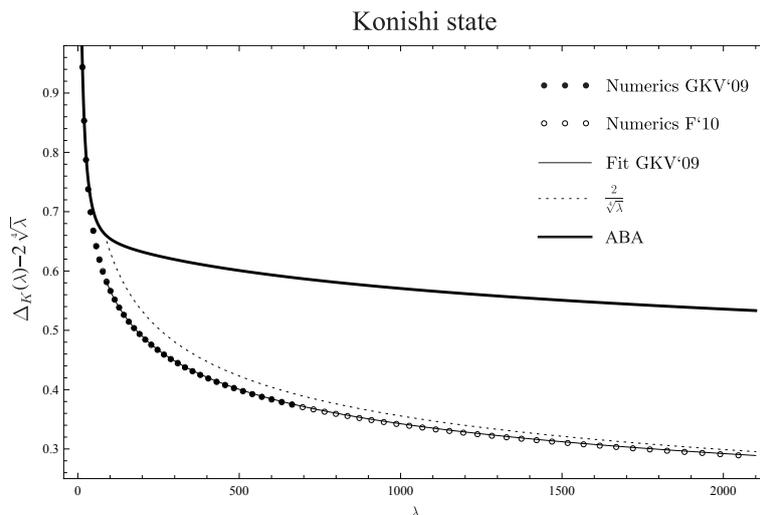

**Figure 2:** Numerical solution of the excited TBA equations for the Konishi state [29, 30].

| $Y_{a,s}$      | This review             | AF                 | BFT          | GKKV                   |
|----------------|-------------------------|--------------------|--------------|------------------------|
| $Y_{Q,0}(u)$   | $Y_Q^\bullet(u)$        | $Y_Q(u)$           | $Y_Q(u)$     | $Y_{\bullet_Q}(u')$    |
| $Y_{M+1,1}(u)$ | $Y_M^\triangleright(u)$ | $Y_{M vw}^{-1}(u)$ | $Y_{v,M}(u)$ | $Y_{\Delta_{M+1}}(u')$ |
| $Y_{1,N+1}(u)$ | $Y_N^\circ(u)$          | $Y_{N v}(u)$       | $Y_{w,N}(u)$ | $Y_{\circ_{N+1}}(u')$  |
| $Y_{2,2}(u)$   | $Y_+^y(u)$              | $-Y_+(u)$ ,        | $Y_y(u)$     | $Y_{\oplus}(u')$       |
| $Y_{1,1}(u)$   | $Y_-^y(u)$              | $-Y_-^{-1}(u)$ ,   | $Y_{y^*}(u)$ | $Y_{\otimes}(u')$      |

**Table 3:** Relating the Y-functions to those in the literature, where  $u' = gu$ .

equations are equivalent to AF [7], while the raw equations to BFT [18], except for the chemical potentials of [18]. In comparing to GKKV [20] the identification is not enough. Comparing our kernel  $K_{QQ'}^{\bullet\bullet}$  to the one  $K_{\bullet_Q\bullet_{Q'}}$  in [20] we observe a slight difference. This is irrelevant, however, for excited states satisfying the level matching/zero momentum condition <sup>5</sup>.

The  $AdS_5/CFT_4$  correspondence has a brother theory, the  $AdS_4/CFT_3$  duality [39], where the TBA program has been developed in an analogous way. The ABA together with the string hypothesis of the mirror theory lead to ground state TBA equations and Y-system relations in [40, 41] and extend the previously conjectured Y-system proposal of [21]. This program is further elaborated in [41] by additionally determining excited states TBA equations and comparing them to the asymptotic solution of the Y functions [21] and to the quasi classical string spectrum.

Finally, let us list some open problems.

There are two disagreeing string theory calculations ([42] and [43]) for the anomalous dimension of the Konishi state. Additionally, the numerical solution of the TBA equations for large couplings [29, 30] provides a third result, and calls for improvements both the string theory and the TBA sides. On the string theory side it could be a pure

<sup>5</sup>We thank the authors of [20] for pointing out this.

spinor calculation, while on the TBA side one should analyze the analytical behavior of the Y-system and check whether, with increasing  $g$ , a singularity of type  $1 + Y = 0$  indeed appears, as the asymptotic solution suggests [28]. In principle the effect of such singularities is to make the coupling dependence of the energies analytical, but it has to be established concretely.

The anomalous dimensions of twist operators in the planar limit can be described by integral equations derived directly from the ABA [44]. It would be nice to see, how the exact excited TBA equations reduce to these equations in the large spin limit.

The analytical comparison of the excited state TBA equations to the next to leading order Lüscher corrections [34, 36] tested explicitly only the  $\triangleright$  part of the Y-system. A next to next to leading order analysis could test the  $\circ$  part as well.

The excited states TBA equations are coupled nonlinear integral equations for infinite unknowns. An ideal system of equations should contain finite unknowns only, and could be developed in analogy to [27, 45] by exploiting the result of [38, 25, 31].

## Acknowledgments

We thank G. Arutyunov, N. Beisert, D. Fioravanti, S. Frolov, N. Gromov, A. Hegedus, V. Kazakov, R. Suzuki and R. Tateo for useful comments on the manuscript. The work was supported by a Bolyai Scholarship, and by OTKA K81461.

## Note added in proof

After this review chapter was finished three string theory calculations based on different methods determined the strong coupling expansion of the anomalous dimension of the Konishi operator [46–48]. All agreed with each other and with the strong coupling expansion of the TBA equation [29, 30]. This gives a strong support not only for the correctness of the TBA equations but also for the integrability approach to planar AdS/CFT.

## References

- [1] A. B. Zamolodchikov, “*Thermodynamic Bethe Ansatz in relativistic models. Scaling three state Potts and Lee-Yang models*”, Nucl. Phys. B342, 695 (1990).
- [2] C.-N. Yang and C. P. Yang, “*Thermodynamics of a one-dimensional system of bosons with repulsive delta-function interaction*”, J. Math. Phys. 10, 1115 (1969).
- [3] P. Dorey and R. Tateo, “*Excited states by analytic continuation of TBA equations*”, Nucl. Phys. B482, 639 (1996), [hep-th/9607167](#).
- [4] P. Dorey and R. Tateo, “*Excited states in some simple perturbed conformal field theories*”, Nucl. Phys. B515, 575 (1998), [hep-th/9706140](#).
- [5] Z. Bajnok, A. Hegedus, R. A. Janik and T. Lukowski, “*Five loop Konishi from AdS/CFT*”, [arxiv:0906.4062](#).
- [6] G. Arutyunov and S. Frolov, “*The Dressing Factor and Crossing Equations*”, [arxiv:0904.4575](#).

- [7] G. Arutyunov and S. Frolov, “*Simplified TBA equations of the  $AdS_5 \times S^5$  mirror model*”, [arxiv:0907.2647](#).
- [8] A. Cavaglia, D. Fioravanti and R. Tateo, “*Extended Y-system for the  $AdS_5/CFT_4$  correspondence*”, [arxiv:1005.3016](#).
- [9] J. Ambjorn, R. A. Janik and C. Kristjansen, “*Wrapping interactions and a new source of corrections to the spin-chain / string duality*”, Nucl. Phys. B736, 288 (2006), [hep-th/0510171](#).
- [10] C. Ahn and R. Nepomechie, “*Review of AdS/CFT Integrability, Chapter III.2: Exact world-sheet S-matrix*”, [arxiv:1012.3991](#).
- [11] P. Vieira and D. Volin, “*Review of AdS/CFT Integrability, Chapter III.3: The dressing factor*”, [arxiv:1012.3992](#).
- [12] N. Beisert and M. Staudacher, “*Long-range  $PSU(2,2/4)$  Bethe ansatzes for gauge theory and strings*”, Nucl. Phys. B727, 1 (2005), [hep-th/0504190](#).
- [13] A. Rej, “*Review of AdS/CFT Integrability, Chapter I.3: Long-range spin chains*”, [arxiv:1012.3985](#).
- [14] M. Staudacher, “*Review of AdS/CFT Integrability, Chapter III.1: Bethe Ansatzes and the R-Matrix Formalism*”, [arxiv:1012.3990](#).
- [15] G. Arutyunov and S. Frolov, “*On String S-matrix, Bound States and TBA*”, JHEP 0712, 024 (2007), [arxiv:0710.1568](#).
- [16] F. H. L. Essler, H. Frahm, F. Goehmann, A. Klumper and V. E. Korepin, “*The One-Dimensional Hubbard Model*, Cambridge University Press”.
- [17] G. Arutyunov and S. Frolov, “*String hypothesis for the  $AdS_5 \times S^5$  mirror*”, JHEP 0903, 152 (2009), [arxiv:0901.1417](#).
- [18] D. Bombardelli, D. Fioravanti and R. Tateo, “*Thermodynamic Bethe Ansatz for planar AdS/CFT: a proposal*”, [arxiv:0902.3930](#).
- [19] G. Arutyunov and S. Frolov, “*Thermodynamic Bethe Ansatz for the  $AdS_5 \times S^5$  Mirror Model*”, JHEP 0905, 068 (2009), [arxiv:0903.0141](#).
- [20] N. Gromov, V. Kazakov, A. Kozak and P. Vieira, “*Integrability for the Full Spectrum of Planar AdS/CFT II*”, [arxiv:0902.4458](#).
- [21] N. Gromov, V. Kazakov and P. Vieira, “*Integrability for the Full Spectrum of Planar AdS/CFT*”, [arxiv:0901.3753](#).
- [22] D. Volin, “*Minimal solution of the AdS/CFT crossing equation*”, [arxiv:0904.4929](#).
- [23] S. Frolov and R. Suzuki, “*Temperature quantization from the TBA equations*”, Phys. Lett. B679, 60 (2009), [arxiv:0906.0499](#).
- [24] V. Kazakov and N. Gromov, “*Review of AdS/CFT Integrability, Chapter III.7: Hirota Dynamics for Quantum Integrability*”, [arxiv:1012.3996](#).
- [25] N. Gromov, V. Kazakov and Z. Tsuboi, “ *$PSU(2,2-4)$  Character of Quasiclassical AdS/CFT*”, JHEP 1007, 097 (2010), [arxiv:1002.3981](#).
- [26] D. Volin, “*String hypothesis for  $gl(n-m)$  spin chains: a particle/hole democracy*”, [arxiv:1012.3454](#).

- [27] N. Gromov, V. Kazakov and P. Vieira, “*Finite Volume Spectrum of 2D Field Theories from Hirota Dynamics*”, [arxiv:0812.5091](#).
- [28] G. Arutyunov, S. Frolov and R. Suzuki, “*Exploring the mirror TBA*”, [arxiv:0911.2224](#).
- [29] N. Gromov, V. Kazakov and P. Vieira, “*Exact AdS/CFT spectrum: Konishi dimension at any coupling*”, [arxiv:0906.4240](#).
- [30] S. Frolov, “*Konishi operator at intermediate coupling*”, [arxiv:1006.5032](#).
- [31] N. Gromov, V. Kazakov, S. Leurent and Z. Tsuboi, “*Wronskian Solution for AdS/CFT Y-system*”, [arxiv:1010.2720](#).
- [32] R. Janik, “*Review of AdS/CFT Integrability, Chapter III.5: Lüscher corrections*”, [arxiv:1012.3994](#).
- [33] G. Arutyunov, S. Frolov and R. Suzuki, “*Five-loop Konishi from the Mirror TBA*”, [arxiv:1002.1711](#).
- [34] J. Balog and A. Hegedus, “*5-loop Konishi from linearized TBA and the XXX magnet*”, [arxiv:1002.4142](#).
- [35] T. Lukowski, A. Rej and V. N. Velizhanin, “*Five-Loop Anomalous Dimension of Twist-Two Operators*”, [arxiv:0912.1624](#).
- [36] J. Balog and A. Hegedus, “*The Bajnok-Janik formula and wrapping corrections*”, [arxiv:1003.4303](#).
- [37] N. Gromov, “*Y-system and Quasi-Classical Strings*”, [arxiv:0910.3608](#).
- [38] A. Hegedus, “*Discrete Hirota dynamics for AdS/CFT*”, [arxiv:0906.2546](#).
- [39] T. Klose, “*Review of AdS/CFT Integrability, Chapter IV.3:  $\mathcal{N} = 6$  Chern-Simons and Strings on  $AdS_4 \times CP^3$* ”, [arxiv:1012.3999](#).
- [40] D. Bombardelli, D. Fioravanti and R. Tateo, “*TBA and Y-system for planar  $AdS_4/CFT_3$* ”, Nucl. Phys. B834, 543 (2010), [arxiv:0912.4715](#).
- [41] N. Gromov and F. Levkovich-Maslyuk, “*Y-system, TBA and Quasi-Classical Strings in  $AdS_4 \times CP^3$* ”, JHEP 1006, 088 (2010), [arxiv:0912.4911](#).
- [42] G. Arutyunov and S. Frolov, “*Uniform light-cone gauge for strings in  $AdS_5 \times S^5$ : Solving  $su(1/1)$  sector*”, JHEP 0601, 055 (2006), [hep-th/0510208](#).
- [43] R. Roiban and A. A. Tseytlin, “*Quantum strings in  $AdS_5 \times S^5$ : strong-coupling corrections to dimension of Konishi operator*”, [arxiv:0906.4294](#).
- [44] L. Freyhult, “*Review of AdS/CFT Integrability, Chapter III.4: Twist states and the cusp anomalous dimension*”, [arxiv:1012.3993](#).
- [45] V. Kazakov and S. Leurent, “*Finite Size Spectrum of  $SU(N)$  Principal Chiral Field from Discrete Hirota Dynamics*”, [arxiv:1007.1770](#).
- [46] N. Gromov, D. Serban, I. Shenderovich and D. Volin, “*Quantum folded string and integrability: from finite size effects to Konishi dimension*”, [arXiv:1102.1040](#).
- [47] R. Roiban and A. A. Tseytlin, “*Semiclassical string computation of strong-coupling corrections to dimensions of operators in Konishi multiplet*”, [arXiv:1102.1209](#).
- [48] B. C. Vallilo and L. Mazzucato, “*The Konishi multiplet at strong coupling*”, [arXiv:1102.1219](#).



# Review of AdS/CFT Integrability, Chapter III.7: Hirota Dynamics for Quantum Integrability

NIKOLAY GROMOV<sup>a</sup>, VLADIMIR KAZAKOV<sup>b</sup>

<sup>a</sup> *King's College, London Department of Mathematics WC2R 2LS, UK  
St.Petersburg INP, St.Petersburg, Russia*

<sup>b</sup> *Ecole Normale Supérieure, LPT, 75231 Paris CEDEX-5, France  
l'Université Paris-VI, Paris, France*

<sup>a</sup>nikolay.gromov@kcl.ac.uk

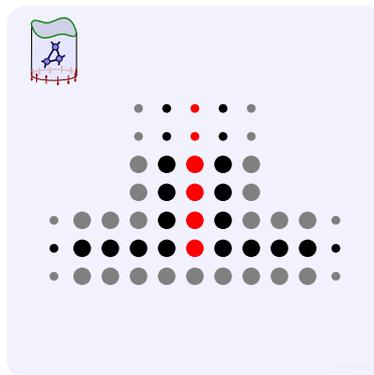

**Abstract:** We review recent applications of the integrable discrete Hirota dynamics (Y-system) in the context of calculation of the planar AdS/CFT spectrum. We start from the description of solution of Hirota equations by the Bäcklund method where the requirement of analyticity results in the nested Bethe ansatz equations. Then we discuss applications of the Hirota dynamics for the analysis of the asymptotic limit of long operators in the AdS/CFT Y-system.

# 1 Introduction

The Hirota integrable hierarchy [1] enables us to take a very general point of view on integrability, in classical systems [2] as well as in 2D statistical mechanical [3] and quantum systems [4–6]. The analytic Bethe ansatz approach based on the Y- and T-systems for the fusion of transfer-matrices in various representations was successfully applied to various spin chains and 2D QFT's [6, 7] and is especially efficient for the supersymmetric systems [8–10]. Being integrable, Hirota equation with specific boundary conditions stemming from the symmetry of the problem, can be often solved explicitly, either by the Bäcklund method [6, 9] or in the determinant (Wronskian) form [6, 11]. Of course to specify completely the physical solutions we have to precise the functional space for the functions of spectral parameter entering Hirota equation, or in other words, we also need to impose certain analyticity conditions on these solutions which is usually the hardest part of the problem. In the spin chains the role of analyticity conditions is usually played by the polynomiality of the transfer-matrices, resulting in supplementary conditions - the Bethe ansatz equations. For the Y-systems of integrable 2D QFT's (sigma models) at a finite volume, the analyticity imposes the absence of singularities on a physical domain of the complex plane of a spectral parameter, except those related to various physical excitations (see [12] for the example of  $O(4)$  sigma model).

These methods, based on the Hirota integrable dynamics, recently have shown again their power in the problem of calculation of the exact conformal dimensions in the planar  $N=4$  SYM theory. The program of integrability for the spectrum in planar AdS/CFT correspondence has lead to the discovery of a system of exact spectral equations — the Y-system — containing an important information about the anomalous dimensions of all local operators at arbitrary 't Hooft coupling. The AdS/CFT Y-system and the underlying integrable Hirota equation were first conjectured in a functional form [13] and later reproduced in the form of an infinite system of non-linear integral equations [14–16] from the TBA approach [4]. It was successfully tested analytically in the weak coupling regime, in particular for Konishi operator and twist-2 operators by the direct 4-loop perturbation theory, and even up to 5 loops, comparing with the BFKL approximation [17], and in the strong coupling for long operators, by comparison with quasi-classical string theory results [18, 19]. The first numerical study of Konishi dimension [20] in a wide range of couplings (see Fig.2 of [21]), showed a perfect interpolation between the  $N = 4$  SYM perturbation theory and the SYM strong coupling asymptotics described by the large radius of the superstring  $AdS_5 \times S^5$  background [22].

In this paper, we will introduce the reader into the basics of Hirota approach to the quantum integrability on the example of  $AdS_5/CFT_4$  duality. But first we will show how to solve, following the methods of [9, 23, 6, 8], Hirota equation for the fusion in the rational supersymmetric spin chains with  $gl(N|M)$  symmetry, in terms of a generating functional (generalized Baxter equations) by means of the Bäcklund method, and to derive the nested Bethe ansatz equations. Then we will follow this logic in the AdS/CFT system and try to show that the worldsheet scattering theory and asymptotic Bethe ansatz ABA for the superstring on  $AdS_5/CFT_4$  background are also tightly related to the analyticity of the Y-system whose form, in its turn, is greatly constrained by the superconformal  $psu(2, 2|4)$  symmetry of the theory.

## 2 Hirota Equations in the $gl(N)$ spin chain

The simplest example where the Hirota equation appears naturally is the generalized Heisenberg  $gl(N)$  spin chain for compact representations. The spin chain Hamiltonian and all other conserved charges can be constructed from the R-matrix [24]. We give in this section the basics of the analytic Bethe ansatz approach to this system following [9,10,23].

Our the explanations (though not the proofs) will be self-contained, all the way from the R-matrix to the Hirota equation. The R-matrix of  $gl(N)$  super-spin chain is

$$R_\lambda(u) = u \mathbb{I} \otimes \mathbb{I}_\lambda + i \sum_{\alpha,\beta=1}^N e_{\beta\alpha} \otimes \pi_\lambda(e_{\alpha\beta}), \quad (2.1)$$

where the generators in the l.h.s.(r.h.s.) of the tensor product in each term correspond

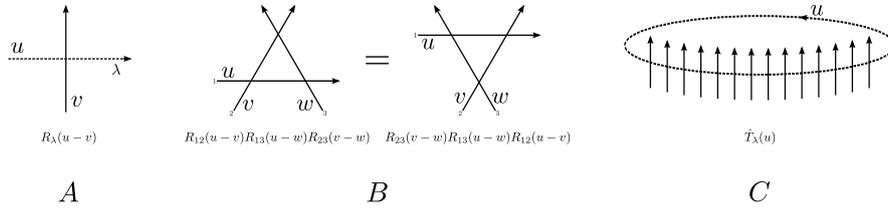

**Figure 1:** A:  $R$ -matrix in pictures; B: Yang-Baxter relation; C: Transfer matrix

to the “physical” (“auxiliary”) space and  $\lambda$  refers to an arbitrary representation in the “auxiliary” space.  $\mathbb{I}$  and  $\mathbb{I}_\lambda$  are the identity elements in fundamental representation and in representation  $\lambda$ , respectively;  $e_{\alpha\beta}$  are the generators of  $u(N)$  algebra acting in the fundamental representation on the basis  $e_\gamma$  as  $e_{\alpha\beta}e_\gamma = e_\alpha\delta_{\beta\gamma}$ , and  $\pi_\lambda(e_{\alpha\beta})$  are the same generators in any irrep  $\lambda$ . In  $\lambda$  fundamental, the second term  $\mathcal{P} \equiv \sum_{\alpha\beta} e_{\beta\alpha} \otimes e_{\alpha\beta}$ , becomes simply the permutation operator and it is easy to check that the R-matrix satisfies the Yang-Baxter equation

$$R_{12}(u)R_{13}(u+v)R_{23}(v) = R_{23}(v)R_{13}(u+v)R_{12}(u) \quad (2.2)$$

where the operators act on the tensor product of 3 fundamental physical states and the lower indexes show on which of the states the action of  $R$  is nontrivial (see Fig.1B).

Next, we introduce the transfer matrix as a trace in the auxiliary space of irrep  $l$  of the monodromy matrix (see the Fig.1C):

$$\hat{T}_\lambda(u, g) \equiv \text{tr}_{\text{aux}} (R_\lambda(u)^{\otimes L} \pi_\lambda(g)),$$

where the tensor products are taken for the physical spaces and the usual matrix product and the trace refers to the the auxiliary space,  $\pi_\lambda(g)$  being a group element  $g$  in the irrep  $l$ . The transfer matrix  $\hat{T}_\lambda(u, g)$  is thus an operator acting on  $L$  copies of the physical space, i.e. on the Hilbert space of the spin chain with  $L$  sites. Notice that for  $L = 0$  the transfer matrix is simply a character  $\chi_\lambda(g)$ .

To relate the transfer matrices to the group characters, we introduce a useful operator called the co-derivative  $\mathcal{D}$  [10] defined by the action on a function of  $g$ :

$$\mathcal{D}f(g) = e_{\beta\alpha} \frac{\partial}{\partial \phi_{\alpha\beta}} f(e^{\phi_{\delta\gamma}} e^{\delta\gamma} g) \Big|_{\phi=0}, \quad \text{where} \quad \frac{\partial}{\partial \phi_{\alpha_1\beta_1}} \phi_{\alpha_2\beta_2} \equiv \delta_{\alpha_1\alpha_2} \delta_{\beta_1\beta_2}. \quad (2.3)$$

In particular, applying it to (2.1), we rewrite the transfer matrix in an instructive way

$$\hat{T}_\lambda(u) = (u + i\mathcal{D})^{\otimes L} \chi_\lambda(g). \quad (2.4)$$

In what follows we consider only the representations  $l = s^a$  with rectangular Young diagrams  $\lambda_i = s$ ,  $i = 1, \dots, a$ . Below we demonstrate that the transfer matrices with different spectral parameters  $u$  and irreps  $\lambda$  commute with each other and thus we can work with their eigenvalues denoted below as  $T_\lambda(u)$ . We denote  $\chi_{a,s} \equiv \chi_{s^a}$  and

$$\hat{T}_{a,s}(u) \equiv \frac{\hat{T}_{s^a}(u + \frac{s-a}{2i})}{(u + \frac{s-a}{2i})^L} \quad (2.5)$$

where we chose the normalization of the eigenvalues

$$T_{a,0} = T_{0,s} = 1. \quad (2.6)$$

The goal of this section is to demonstrate the following Hirota equation [3, 6]:

$$T_{a,s}(u + \frac{i}{2}) T_{a,s}(u - \frac{i}{2}) = T_{a+1,s}(u) T_{a-1,s}(u) + T_{a,s+1}(u) T_{a,s-1}(u) \quad (2.7)$$

Let us demonstrate the validity of (2.7) on the case  $a = 1$ . The symmetric characters  $\chi_{1,s}(g)$  are generated as the Schur polynomials from the generating function

$$w(z) = \det(1 - zg)^{-1} = \sum_{s=0}^{\infty} z^s \chi_{1,s}. \quad (2.8)$$

Acting on  $w(z)$  by the left co-derivative we easily find that

$$\mathcal{D} \log w(z) = \frac{zg}{1 - zg} \quad (2.9)$$

$$(1 + \mathcal{D})w(z_1) \mathcal{D}w(z_2) = \frac{1}{1 - z_1 g} \frac{z_2 g}{1 - z_2 g} = \frac{z_2}{z_1} \frac{z_1 g}{1 - z_1 g} \frac{1}{1 - z_2 g} = \frac{z_2}{z_1} \mathcal{D}w(z_1) (1 + \mathcal{D})w(z_2). \quad (2.10)$$

The last equation in particular implies the following relation among the characters

$$\mathcal{D}\chi_{1,s}(\chi_s + \mathcal{D}\chi_s) = \mathcal{D}\chi_{1,s+1}(\chi_{s-1} + \mathcal{D}\chi_{s-1}) \quad (2.11)$$

which, for the simple one spin chain  $L = 1$ , is equivalent to a particular case of (2.7)

$$\hat{T}_{1,s}(u + \frac{i}{2}) \hat{T}_{1,s}(u - \frac{i}{2}) = \hat{T}_{0,s}(u) \hat{T}_{2,s}(u) + \hat{T}_{1,s-1}(u) \hat{T}_{1,s+1}(u) \quad (2.12)$$

where we had to use that  $\chi_{2,s} = \chi_{1,s}^2 - \chi_{1,s+1} \chi_{1,s-1}$  and  $\chi_{0,s} = 1$ . Moreover, one can see that the one spin transfer matrices are a combinations of only  $g$  and the unit matrix

and thus commute with each other. We send the interested reader to [10] for the general proof of the Hirota relation (2.7) for any irrep and any number of spins. Eq.(2.7) is a generalization of a similar, but simplified, Hirota relation among the characters:  $\chi_{a,s}^2 = \chi_{a+1,s}\chi_{a-1,s} + \chi_{a,s+1}\chi_{a,s-1}$  - following from the multiplication of rectangular irreps.

It is remarkable that the fusion equation (2.7) is the same for all  $gl(N)$  groups. Different  $N$  will correspond however to different boundary conditions. In particular, one has  $T_{N+1,s} = 0$  (as well as  $T_{a<0,s} = T_{a\neq 0,s<0} = 0$ ),  $T_{a<0,s} = T_{a\neq 0,s<0} = 0$  which is clear from the same conditions for the characters:  $\chi_{N+1,s} = 0$ . It turns out that for the super groups  $gl(N|M)$  the Hirota equation is again the same whereas the nonzero  $T_{a,s}$  belong to so called fat-hook [8] (see Fig.2a).

It is easy to check that the ‘‘gauge’’ transformation<sup>I</sup>

$$T_{a,s} \rightarrow g_1^{[a+s]} g_2^{[a-s]} g_3^{[s-a]} g_4^{[-a-s]} T_{a,s} \quad (2.13)$$

where  $g_i$  are arbitrary functions, leaves the form of the Hirota equation unchanged. One may choose certain normalization of the solutions by fixing these functions in one or another way, as we do in (2.6). Notice that (2.6) still leaves one gauge degree of freedom unfixed<sup>II</sup>. We can also introduce the quantities gauge invariant w.r.t. (2.13)

$$Y_{a,s} = \frac{T_{a,s+1}T_{a,s-1}}{T_{a+1,s}T_{a-1,s}} \quad (2.14)$$

As a consequence of Hirota equations (2.7) they satisfy the discrete Y-system equations

$$Y_{a,s}^+ Y_{a,s}^- = \frac{(1 + Y_{a,s+1})(1 + Y_{a,s-1})}{(1 + 1/Y_{a+1,s})(1 + 1/Y_{a-1,s})}. \quad (2.15)$$

There exists a concise solution of Cauchy problem for Hirota equation in the semi- $(a, s)$ -plane, in terms of  $T_{1,s}(u)$  fixed along the boundary (recall that  $T_{0,s}(u) = 1$  in our gauge), the so called Bazhanov-Reshetikhin determinant formula [25, 10] for the fusion in spin chains (valid here in a more general context)<sup>III</sup>

$$T_{a,s} = \det_{1 \leq j, k \leq a} T_{1, s+k-j} \left( u + \frac{k+j-a-1}{2i} \right). \quad (2.16)$$

Our strategy will be to get as much information as possible about the system by solving the Hirota equations. The Bethe ansatz equations naturally appear in this approach as a requirement of analyticity, or, in the case of spin chains, of polynomiality of all transfer-matrices. In the next section we show how the Hirota classical integrable discrete dynamics helps to solve, by means of the Bäcklund transform, the fusion relations (2.7) in terms of a generating functional.

<sup>I</sup>We will often use the notations  $f^\pm = f(\theta \pm \frac{i}{2})$ ,  $f^{\pm\pm} = f(\theta \pm i)$ , and in general  $f^{[\pm k]} = f(\theta \pm \frac{i}{2}k)$ .

<sup>II</sup>Another normalization, more natural for the spin chains, is to require  $T_{a,s}(u)$  to be polynomial. This corresponds to (2.5) without denominator. For the AdS/CFT applications, and for the sigma-models in general, these requirements of polynomiality are too strong

<sup>III</sup>A similar formula expresses  $T_{a,s}$  through the antisymmetric characters  $T_{a,1}$ . There exist also a generalization to the irreps with arbitrary Young tableaux.

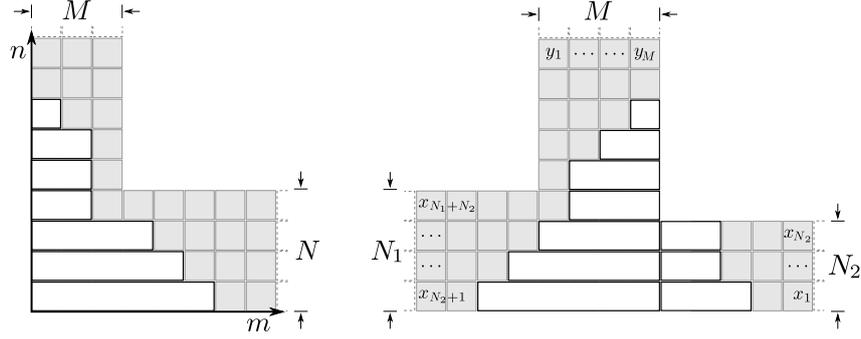

**Figure 2:** The fat-hook for the representations of  $SU(N|M)$  (left) and T-hook for the representations of  $SU(N_1, N_2|M)$  (right). The lengths of horizontal (white) strips forming the Young tableau of an irrep are equal to its highest weight components.

### 3 Integrability of Hirota Equations

In this section we describe the general solution of Hirota equations in the  $(N|M)$  fat hook shown on the Fig.2. We apply for that the Bäcklund transformation technique based on the classical integrability of discrete Hirota dynamics, and show how it helps to solve the problem by gradually reducing the  $(N|M)$  fat hook to a trivial one  $(0|0)$ . As a result we derive the generating functional for the general solution of Hirota equations. In particular, the polynomial solution corresponds to the transfer matrices of the  $SL(N|M)$  rational Heisenberg super-spin chain described above.

#### 3.1 Linear system for Hirota equation

The classical integrability for the Hirota dynamics manifests itself in the existence of an axillary linear problem - a pair of Lax equations

$$\begin{aligned} \text{eq}_{a,s}^I(u) : T_{a+1,s} F_{a,s}^+ &= +x T_{a+1,s-1}^+ F_{a,s+1} + T_{a,s}^+ F_{a+1,s} , \\ \text{eq}_{a,s}^{II}(u) : T_{a,s-1} F_{a,s}^+ &= -x T_{a+1,s-1}^+ F_{a-1,s} + T_{a,s}^+ F_{a,s-1} . \end{aligned} \quad (3.1)$$

Their compatibility condition gives the Hirota equation (2.7). Indeed, we notice that  $F_{a,s}^{++}$  can be expressed through  $F_{a+1,s-1}$ ,  $F_{a,s}$ ,  $F_{a-1,s+1}$  in two different ways: 1) use  $\text{eq}_{a,s}^I(u + \frac{i}{2})$  and then  $\text{eq}_{a,s+1}^{II}(u)$  with  $\text{eq}_{a+1,s}^{II}(u)$  2) use  $\text{eq}_{a,s}^{II}(u + \frac{i}{2})$  and then  $\text{eq}_{a-1,s}^I(u)$  with  $\text{eq}_{a,s-1}^I(u)$ . If we subtract the two results only the term linear in  $x$  survives which implies:

$$\frac{T_{a,s}^+ T_{a+1,s-2}}{T_{a,s-1} T_{a+1,s-1}^-} + \frac{T_{a,s}^+ T_{a+2,s-1}}{T_{a+1,s} T_{a+1,s-1}^-} - \frac{T_{a+1,s-1}^+ T_{a-1,s}}{T_{a,s-1} T_{a,s}^-} - \frac{T_{a+1,s-1}^+ T_{a,s+1}}{T_{a+1,s} T_{a,s}^-} = 0 \quad (3.2)$$

or, to put it differently, the function defined by  $f_{a,s} = \frac{T_{a-1,s} T_{a+1,s} + T_{a,s-1} T_{a,s+1}}{T_{a,s}^+ T_{a,s}^-}$  should be periodic under the shift  $f_{a,s}(u) = f_{a+1,s-1}(u)$ . Since for the transfer matrices  $T_{0,s} = 1$  this implies that  $f_{0,s} = 1$  and thus  $f_{a,s} \equiv 1$ , leading to Hirota eq. (2.7).

Next, noticing that the Hirota equation is invariant under  $(a, s, u) \rightarrow (-a, -s, -u)$  we can easily find another linear system (useful for the next section)

$$\begin{aligned} T_{a-1,s} \tilde{F}_{a,s}^- &= +y T_{a-1,s+1}^- \tilde{F}_{a,s-1} + T_{a,s}^- \tilde{F}_{a-1,s} , \\ T_{a,s+1} \tilde{F}_{a,s}^- &= -y T_{a-1,s+1}^- \tilde{F}_{a+1,s} + T_{a,s}^- \tilde{F}_{a,s+1} . \end{aligned} \quad (3.3)$$

## 3.2 Solution of Hirota fusion equation by the Bäcklund method

As it was announced above the Bäcklund method allows to reduce the Hirota equation in a fat-hook  $(N|M)$  to the same equation in a smaller fat hook  $(n|m)$  with  $n \leq N$ ,  $m \leq M$ . For that we notice that (3.1), after the appropriate shifts in the spectral parameter and in  $a$  and  $s$ , can be written in the form

$$\begin{aligned} F_{a-1,s} T_{a,s}^- &= +x F_{a-1,s+1}^- T_{a,s-1} + F_{a,s}^- T_{a-1,s} , \\ F_{a,s+1} T_{a,s}^- &= -x F_{a-1,s+1}^- T_{a+1,s} + F_{a,s}^- T_{a,s+1} \end{aligned} \quad (3.4)$$

which is precisely the second linear system (3.3) with  $F_{a,s}$  and  $T_{a,s}$  interchanged. In particular, this implies that  $F_{a,s}$  should also satisfy the same Hirota equation. It is always possible to choose  $F_{a,s}$  so that it satisfies Hirota equation in a smaller fat-hook  $(N-1|M)$  i.e. to have  $F_{N,s} = 0$ ,  $s > M$ . One can immediately see from (3.4) that this condition is compatible with the fat hook boundary condition for T-functions  $T_{N+1,s>M} = 0$ . Below we will construct this solution explicitly.

In view of this symmetry between  $F$  and  $T$  we can denote  $T_{a,s}^{N|M} = T_{a,s}$  and  $T_{a,s}^{N-1|M} \propto F_{a,s}$  with a particular normalization (2.13): we normalize them so that  $T_{0,s} = 1$  and  $T_{a,0} = 1$ . From (3.1), this normalization implies for  $F$  the following relations  $F_{0,s+1} = F_{0,s}^-$ ,  $F_{a-1,0} = F_{a,0}^-$  which means that we can express  $F_{0,s}$  or  $F_{a,0}$  in terms of  $F_{0,0}$  with a shifted argument  $F_{0,s} = F_{0,0}(u - i\frac{s}{2})$ ,  $F_{a,0} = F_{0,0}(u + i\frac{a}{2})$ . Thus in our normalization we get  $T_{a,s}^{N-1|M} \equiv \frac{F_{a,s}(u)}{F_{0,0}(u + \frac{s-a}{2i})}$ . It should be also clear that due to the symmetry between  $F$  and  $T$  we can change the logic and tell that (3.1) allows to increase  $M$ . Similarly, the second linear system (3.3) allows to decrease  $M$  (or increase  $N$ ) and we denote  $T_{a,s}^{N|M-1} \equiv \frac{\tilde{F}_{a,s}(u)}{\tilde{F}_{0,0}(u + \frac{s-a}{2i})}$ .

By making an appropriate chain of these two transformations we can always reduce a fat hook  $(N|M)$  to the trivial one  $(0|0)$ , through a set of the intermediate fat hooks  $(n|m)$ ,  $0 < n < N$ ;  $0 < m < M$  (see fig.3). This procedure allows to write the solution quite explicitly.<sup>IV</sup> For the next section we introduce the parameterization

$$\frac{F_{0,0}^{--}}{F_{0,0}} = \frac{\mathcal{Q}_{N|M}^{++} \mathcal{Q}_{N-1|M}^{--}}{\mathcal{Q}_{N|M} \mathcal{Q}_{N-1|M}}, \quad \frac{\tilde{F}_{0,0}^{++}}{\tilde{F}_{0,0}} = \frac{\mathcal{Q}_{N|M}^{--} \mathcal{Q}_{N|M-1}^{++}}{\mathcal{Q}_{N|M} \mathcal{Q}_{N|M-1}} \quad (3.5)$$

The above equations define  $\mathcal{Q}_{N|M-1}$  and  $\mathcal{Q}_{N-1|M}$  in terms of  $\mathcal{Q}_{N|M}$ , for given functions  $F_{0,0}, \tilde{F}_{0,0}$ . Since our normalization (2.6) allows for one more gauge one can set  $\mathcal{Q}_{N|M} = 1$ . This, however, is not the most convenient choice. In the case of spin chains (as in

<sup>IV</sup>This procedure is a “quantum” analogue of the construction of the so called Gelfand-Zeitlin basis.

section 2) a natural choice is  $\mathcal{Q}_{N|M} = \prod_{j=1}^L (u - \theta_j)$ . In this normalization, at an arbitrary step, or nesting level  $(n|m)$  of our Bäcklund procedure,  $\mathcal{Q}_{n|m}$  will be a polynomial, the denominator of the rational functions  $T_{a,s}^{n|m}(u - \frac{s-a}{2i})$  (like in (2.5)).

Furthermore we denote

$$\mathcal{X}_{n|m} = x_n \frac{\mathcal{Q}_{n|m}^{++} \mathcal{Q}_{n-1|m}^{--}}{\mathcal{Q}_{n|m} \mathcal{Q}_{n-1|m}}, \quad \mathcal{Y}_{n|m} = y_m \frac{\mathcal{Q}_{n|m}^{--} \mathcal{Q}_{n|m-1}^{++}}{\mathcal{Q}_{n|m} \mathcal{Q}_{n|m-1}}. \quad (3.6)$$

### 3.3 A recurrent equation for the generating functional

For the quantum generalization of the generating function for the characters (2.8) we introduce an operator valued functional

$$\mathcal{W}^{n|m} = \sum_{s=-\infty}^{\infty} D^s T_{1,s}^{n|m}(u) D^s \quad (3.7)$$

where  $D$  is a shift operator defined by  $Df(u) = f(u - \frac{i}{2})D$ . From (3.1) at  $a = 0$  we get in notations (3.6)

$$T_{1,s}^{n-1|m}(u) = T_{1,s}^{n|m}(u) - \mathcal{X}_{n|m}(u + \frac{s-1}{2i}) T_{1,s-1}^{n|m}(u + \frac{i}{2}) \quad (3.8)$$

where we introduced new  $n|m$  indices for  $F$  characterizing the “level” on which we make this Bäcklund transformation. This implies

$$\mathcal{W}^{n-1|m} = \mathcal{W}^{n|m} (1 - D\mathcal{X}_{n|m}D) \quad (3.9)$$

and similarly

$$\mathcal{W}^{n|m} = \mathcal{W}^{n|m-1} (1 - D\mathcal{Y}_{n|m}D). \quad (3.10)$$

Using the relations (3.9) and (3.10) we can show that any solution of Hirota equation in the  $(N|M)$  fat hook can be explicitly and concisely written in the form of a simple generating functional. For that we have to apply the recursions (3.9) and (3.10) along a path of the length  $N + M$  on the  $(n|m)$  lattice, connecting the upper right and the lower left corners of the  $N \times M$  rectangle on Fig.3. This gives the following formula for the generating functional (3.7) [6, 8, 9]

$$\mathcal{W}^{N|M} = \overleftarrow{\prod}_{\text{path}} \begin{cases} (1 - D\mathcal{X}_{n|m}D)^{-1} & , \text{ vertical} \\ (1 - D\mathcal{Y}_{n|m}D) & , \text{ horizontal} \end{cases} \quad (3.11)$$

where the subset of  $N + M$  functions  $\mathcal{X}_{n|m}$ ,  $\mathcal{Y}_{n|m}$ , chosen out of the whole set of  $N \times M$  such functions, depends on the path (see Fig.3).

$$\mathcal{X}_{n|m} \quad , \quad \text{line from } (n, m) \text{ to } (n - 1, m) \quad (3.12)$$

$$\mathcal{Y}_{n|m} \quad , \quad \text{line from } (n, m) \text{ to } (n, m - 1) \quad (3.13)$$

In the case when  $\mathcal{Q}_{n|m}$  are polynomials the solution of Hirota equation constructed in this way corresponds to the transfer matrices with a twist given by a supergroup element  $g = \text{diag}\{x_1, \dots, x_N | y_1, \dots, y_M\}$ .



We see that we only have to require the cancelation of the poles in the square brackets to ensure that the poles will not appear at any order in  $D$ . Similar relations can be written for a horizontal link following by a vertical one. That gives another pair of the Bethe equations, so that we have

$$\frac{\mathcal{Q}_{n|m-1} \mathcal{Q}_{n+1|m}^{++}}{\mathcal{Q}_{n|m-1}^{++} \mathcal{Q}_{n+1|m}} \Big|_{u_j^{(n|m)}} = \frac{y_m}{x_{n+1}}, \quad \frac{\mathcal{Q}_{n-1|m} \mathcal{Q}_{n|m+1}^{--}}{\mathcal{Q}_{n-1|m}^{--} \mathcal{Q}_{n|m+1}} \Big|_{u_j^{(n|m)}} = \frac{x_n}{y_{m+1}}. \quad (3.17)$$

Notice that this pair of equations is compatible with the first pair (3.15) – their products coincide. This is a consequence of the “zero curvature” equations discussed below. In general, we need only  $N + M - 1$  Bethe equations, written in the interior vertices of a path of Fig.3, to fix completely the full set of  $Q$ -functions with all their zeros.

### 3.5 Self-consistency of the construction and $QQ$ -relations

Once a path on Fig.3 is fixed one can choose an arbitrary set of functions  $\mathcal{Q}_{n|m}$  along this path in order to get some solution of the Hirota equation. If we want now to change the nesting path without changing the solution for  $T$ -functions, it is possible to choose a new subset of  $N + M - 1$   $Q$ -functions entering the generating functional (3.11). Let us consider such an elementary modification of the functional:

$$(1 - D\mathcal{X}_{n|m-1}D)^{-1}(1 - D\mathcal{Y}_{n|m}D) = (1 - D\mathcal{Y}_{n-1|m}D)(1 - D\mathcal{X}_{n|m}D)^{-1} \quad (3.18)$$

The terms quartic in  $D$  cancel automatically and the quadratic terms give

$$\mathcal{X}_{n|m-1} - \mathcal{Y}_{n|m} = \mathcal{X}_{n|m} - \mathcal{Y}_{n-1|m} \quad (3.19)$$

which means that the combination

$$f_{n|m} = \frac{x_n \mathcal{Q}_{n-1|m-1}^- \mathcal{Q}_{n|m}^+ - y_m \mathcal{Q}_{n-1|m-1}^+ \mathcal{Q}_{n|m}^-}{\mathcal{Q}_{n-1|m}^- \mathcal{Q}_{n|m-1}^+} \quad (3.20)$$

is a periodic function with a period  $i$ . In the case when  $\mathcal{Q}_{n|m}$  are polynomials  $f_{n|m}$  should be a constant, which leads to the following  $QQ$  relation [8, 9]

$$f_{n|m} \mathcal{Q}_{n-1|m}^- \mathcal{Q}_{n|m-1}^+ = x_n \mathcal{Q}_{n-1|m-1}^- \mathcal{Q}_{n|m}^+ - y_m \mathcal{Q}_{n-1|m-1}^+ \mathcal{Q}_{n|m}^-. \quad (3.21)$$

In the spin chain case, when  $Q$ 's are polynomials, one can fix their normalization to have the same lading large  $u$  coefficient. In this case, evidently  $f_{n,m} = x_n - y_m$ .

Now we will show how all these rather abstract considerations can help us to attack an important physical problem - the study of the  $Y$ -system for the exact spectrum of an AdS/CFT system.

## 4 Classical transfer matrix of $AdS_5 \times S^5$ superstring

In this section, we remind the results of the finite gap solution of the classical superstring on  $AdS_5 \times S^5$  [26, 27] (see [28] for the details). We will construct in the classical limit

a set of the eigenvalues of transfer matrices in various representations. We demonstrate that, very similarly to transfer matrices of the spin chains, the classical transfer matrices (traces of the monodromy matrix in various irreps) of the Metsaev-Tseytlin sigma model satisfy the Hirota equation. The crucial difference with the previous example is the non-compact symmetry group  $PSU(2, 2|4)$  which implies a different type of boundary conditions for the Hirota equation - the so called  $\mathbb{T}$ -Hook (Fig.2b).

We examine the properties of solutions of Hirota eqs. given by the classical transfer matrices and then in the next section we discuss certain aspects of the generalization to the quantum case.

#### 4.1 Characters of $PSU(2, 2|4)$ and their Hirota dynamics

The monodromy matrix  $\Omega(x)$  is a spectral parameter dependent  $SU(2, 2|4)$  group element. In the fundamental representation it is a  $4|4 \times 4|4$  supermatrix with  $4 + 4$  eigenvalues  $(x_1, \dots, x_4|y_1, \dots, y_4)$  expressed through the quasi-momenta (of  $S^5$  and  $AdS_5$  respectively) as follows:  $x_j = e^{-i\tilde{p}_j(x)}$ ,  $y_j = e^{-i\hat{p}_j(x)}$ ,  $j = 1, 2, 3, 4$ . The dependence of  $\Omega(x)$  on the spectral parameter  $x$  comes from the expression for the Lax pair [27]. Supertrace of the monodromy matrix  $\Omega(x)$  in any unitary highest weight irreducible representation (irrep)  $\lambda$  will be denoted by  $T_\lambda = \text{Str}_\lambda \Omega(x)^V$ .

Such highest weight irreps of  $U(2, 2|4)$  can be parameterized by generalized Young diagrams (see Fig.2b). The rectangular irreps  $\lambda_i = s + 2$ ,  $i = 1, \dots, a$  which we denote as  $[a, s]$  are playing a crucial role since they obey a closed system of relations w.r.t. their tensor product  $[a, s] \otimes [a, s] = [a + 1, s] \otimes [a - 1, s] \oplus [a, s + 1] \otimes [a, s - 1]$ . Tracing out this relation we find that the characters of  $T_{a,s}$  of such irreps again satisfy the Hirota relation, as it was the case for the characters  $\chi_{a,s}$  of the sec.2

$$T_{a,s}T_{a,s} = T_{a+1,s}T_{a-1,s} + T_{a,s+1}T_{a,s-1}. \quad (4.1)$$

As we shall see later, this equation is a special limit of the full quantum Hirota equation (2.7) containing no shift in the spectral parameter, since it is invisible in this system in the strong 't Hooft coupling  $\lambda \rightarrow \infty$  limit where the spectral parameter is parameterized as  $u = \frac{\sqrt{\lambda}}{4\pi}(x + 1/x)$  and scales as  $\sqrt{\lambda}$ .

Let us compare the characters for finite dimensional irreps of  $U(4|4)$  and the characters of non-compact infinite dimensional irreps of  $U(2, 2|4)$ . They satisfy the same Hirota equation (4.1) but with different boundary conditions in the infinite  $(a, s)$  lattice. Both are defined by the same generating function

$$w(z) = \text{SDet} (1 - z\Omega(x))^{-1} = \frac{(1 - y_1z)(1 - y_2z)(1 - y_3z)(1 - y_4z)}{(1 - x_1z)(1 - x_2z)(1 - x_3z)(1 - x_4z)} \quad (4.2)$$

where the characters of irreps  $(1, s)$  are generated by the contour integrals

$$T_{1,s}^{(4|4)} = \frac{1}{2\pi i} \oint_C \frac{dz}{z^{s+1}} w(z), \quad (4.3)$$

---

<sup>V</sup>Since all the unitary representations are indefinite dimensional the supertrace may not be convergent in some special cases. For sufficiently large  $L/\sqrt{\lambda}$  the convergence is guaranteed.

and all the other representations can be generated from there irreps by the Jacobi-Trudi type formula (which is a direct consequence of (4.1)):

$$T_{a,s} = \det_{1 \leq i,j \leq a} T_{1,s+i-j}. \quad (4.4)$$

The two types of characters differ by the definition of the integration contour  $C$ . If the contour encircles the origin, living aside all the poles in the denominator of (4.2), then the corresponding  $T_{a,s}$  (also called the super-Schur polynomials) constructed from  $T_{1,s}$  by means of (4.4) will be non-zero only inside the so called  $4|4$  fat hook on the  $(a,s)$  lattice (see Fig.2). This corresponds to the compact unitary representations of  $U(4|4)$ . But if the contour encircles the origin *together* with the poles  $t = x_3^{-1}, x_4^{-1}$  the corresponding characters generated by (4.4) are non-zero only within the  $\mathbb{T}$ -hook Fig.2b. It is shown in [29,30] that the irreps corresponding to these characters are indeed the unitary infinite dimensional irreps of  $U(2,2|4)$  (see also [19] for some explanations and for the explicit formulas for these characters).

These characters have a few discrete symmetries. They have a specific symmetry w.r.t. to the inversion of the eigenvalues:

$$T_{a,s}(x_1, \dots, x_4 | y_1, \dots, y_4) = T_{a,-s} \left( \frac{1}{x_4}, \dots, \frac{1}{x_1} \middle| \frac{1}{y_4}, \dots, \frac{1}{y_1} \right) \quad (4.5)$$

and instead of the full Weyl symmetry of the compact irreps, they have only a residual permutational symmetry

$$x_1, x_2 \leftrightarrow x_2, x_1 \ ; \ x_3, x_4 \leftrightarrow x_4, x_3 \ ; \ \{y_1, y_2, y_3, y_4\} \leftrightarrow \text{Perm}\{y_1, y_2, y_3, y_4\}. \quad (4.6)$$

They also have some complex conjugation properties described below.

## 4.2 $Z_4$ symmetry and reality

From the unitarity of the classical monodromy matrix, the eigenvalues as functions of  $x$  are unimodular

$$\overline{x_i(x)} = 1/x_i(\bar{x}) \ , \ \overline{y_i(x)} = 1/y_i(\bar{x}). \quad (4.7)$$

The  $Z_4$ -symmetry of this  $AdS_5 \times S^5$  coset model imposes the following monodromy property [27]

$$x_{1,2,3,4}(1/x) = \frac{1}{x_{2,1,4,3}(x)} \ , \ y_{1,2,3,4}(1/x) = \frac{1}{y_{2,1,4,3}(x)}. \quad (4.8)$$

Since on the unit circle  $|x| = 1$  we have  $\bar{x} = 1/x$  and we get

$$\overline{x_{1,2,3,4}(x)} = \frac{1}{x_{1,2,3,4}(1/x)} = x_{2,1,4,3}(x) \ , \ \overline{y_{1,2,3,4}(x)} = y_{2,1,4,3}(x). \quad (4.9)$$

All this, together with (4.6), implies the reality of  $T_{a,s}$  on the unit circle  $|x| = 1$ :

$$\overline{T_{a,s}} = T_{a,s}. \quad (4.10)$$

Then the  $Y$  functions defined by (2.14) are also real:  $\overline{Y_{a,s}} = Y_{a,s}$ . It follows from the definition (2.14) and the explanations below the eq.(4.4) that whereas  $T_{a,s}$  are non-zero in the vertices of the Fig.4(left) the  $Y_{a,s}$  are defined only in the visible nodes on the Fig.4(right). As was explained in [18] eq.(4.1) and the corresponding simplified Y-system describe the quasi-classical limit of the AdS<sub>5</sub>/CFT<sub>4</sub> system.

## 5 Quantum Hirota equation for AdS/CFT

There is no rigorous prove that the Metsaev-Tseytlin (MT) superstring  $\sigma$ -model is a well defined quantum theory, though the explicit perturbative SYM calculations lead to the results consistent up to two loops with the classical limit of MT model [31,32]. We know that this  $\sigma$ -model is classically integrable and that there is also an abundant evidence of its quantum mechanical integrability. The experience from relativistic quantum  $\sigma$ -models with massive spectra shows that the problem of the energy spectrum on a finite space circle, or a finite radius 2D space-time cylinder, always boils down to a very simply looking and universal system of functional Y- and T-systems, or Hirota equations (2.7), the same as for the spin chains considered in the Sec.2. The boundary conditions in  $a, s$  and the analyticity conditions in  $u$  for the Hirota-type system or the corresponding Y-system differ from model to model, but usually their general form (2.7) is tightly related to the underlying symmetry and stays the same for all  $gl(N|M)$  algebras (with only minor modifications for other algebras)<sup>VI</sup>. Unless there exists an integrable lattice version, the only tangible proof of the Y-system for each particular finite size  $\sigma$ -model is based on the TBA approach [33] with the finite temperature interpreted as a finite space circle [4].

The quantum MT  $\sigma$ -model in the light-cone gauge, looking as a massive, though not explicitly relativistic theory, seems to be in the same class of integrable  $\sigma$ -models as the above mentioned relativistic examples. The absence of the worldsheet relativistic invariance, necessary to swap the worldsheet time and space directions, complicates but does not ruin the TBA approach to the finite size problem.

To apply the T-system for a particular  $\sigma$ -model one should identify the boundary conditions on the  $(a, s)$ -lattice. The quasi-classical picture of the previous section suggests that the full quantum Hirota equation should have the same boundary conditions, the T-hook of Fig.4, as the simplified system for characters (4.1), as a consequence of the AdS/CFT superconformal  $PSU(2, 2|4)$  symmetry.

The next step is to identify the spectral parameter  $u$  entering the full quantum Hirota eq.(2.7). In analogy with the integrable sigma-models [34] it can be taken the same as entering the pair  $(p, u)$ , where  $p$  is the quasi-momentum of the classical monodromy matrix, defining the symplectic structure of the algebraic curve and entering the holomorphic integrals  $\oint pdu$  of the Bohr-Sommerfeld quantization. This parameter is related to the one used in the previous section by Zhukovski map [27]

$$u = \frac{\sqrt{\lambda}}{4\pi}(x + 1/x). \quad (5.1)$$

<sup>VI</sup>For an incomplete table of integrable models and their Y-systems see the last page of [12].

We will assume that this spectral parameter  $u$  is the same as in the full quantum AdS/CFT Y-system (2.15). The initial spectral parameter  $x$  is then a double valued function w.r.t. the new parameter  $u$ . As a consequence of these additional analyticity features in this construction we expect that  $Y_{a,s}$  has several cuts parallel to the real axes, with the branchpoints at  $\pm 2g + \frac{in}{2}$ . To fix the cut structure we distinguish two kinematics: the physical and the mirror (where the role of time and space is swapped)

$$x^{\text{ph}}(u) = \frac{1}{2} \left( \frac{u}{g} + \sqrt{\frac{u}{g} - 2} \sqrt{\frac{u}{g} + 2} \right) , \quad x^{\text{mir}}(u) = \frac{1}{2} \left( \frac{u}{g} + i \sqrt{4 - \frac{u^2}{g^2}} \right) , \quad (5.2)$$

having branch cuts at  $(-2g, 2g)$  and  $(-\infty, -2g) \cup (2g, \infty)$ , respectively.<sup>VII</sup>

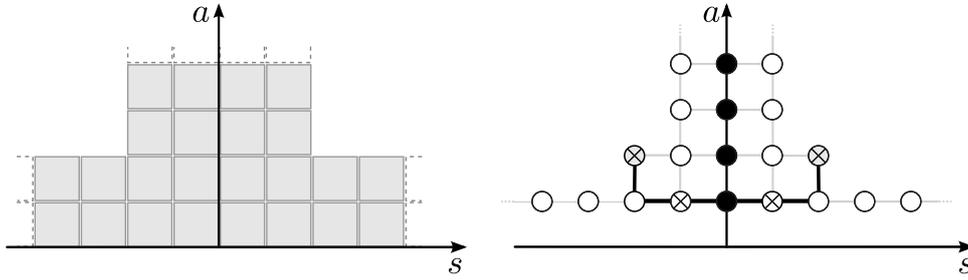

**Figure 4:** T-shaped “fat hook” (T-hook) uniting two  $SU(2|2)$  fat hooks, see [13] for this T-hook and its generalization [35].

In the supersymmetric models the Hirota equation [13] appears to be a little more than the Y-system (2.15) in which two corner equations are missing. When one tries to truncate the Y-system from the full  $(a, s)$  plane lattice to the T-hook one has to put Y-functions to zero on the vertical boundaries, and to  $\infty$  at the horizontal boundaries in the left figure of Fig.4. Then the equation for  $Y_{2,\pm 2}$  contains an uncertainty  $\frac{0}{0}$ . The Y-system has to be supplemented by additional information. In this respect, the T-system, free of that uncertainty, looks more fundamental than the Y-system.

To fix the functions  $Y_{2,\pm 2}(u)$  at the corner nodes we will use a fact noticed from TBA [14–16] (and partially inspired by): in the mirror kinematics,  $Y_{2,\pm 2}(u)$  and  $Y_{1,\pm 1}(u)$  are related on two sides of the cut  $(-\infty, -2g) \cup (2g, \infty)$  on  $\mathbb{R}$  by

$$Y_{2,\pm 2}(u + i0) = \frac{1}{Y_{1,\pm 1}(u - i0)} . \quad (5.3)$$

In the next section we will use (5.3) as a natural analytic input for the asymptotic large  $L$  solution of the quantum Y-system.

Given a particular solution of the Y-system, the corresponding energy of a string

---

<sup>VII</sup> $x(u)$  as analytic function has the following conjugation properties:  $\bar{x}(u) = \frac{1}{x(u)}$  on the mirror sheet and  $\hat{x}(u) = x(u)$  on the physical sheet.

state (or anomalous dimension of a SYM operator) can be obtained from<sup>VIII</sup>

$$E = \sum_j \epsilon_1^{\text{ph}}(u_{4,j}) + \sum_{a=1}^{\infty} \int_{-\infty}^{\infty} \frac{du}{2\pi i} \frac{\partial \epsilon_a^{\text{mir}}}{\partial u} \log(1 + Y_{a,0}(u)), \quad (5.4)$$

whose general form is rather standard in the TBA context. The physical energy  $\epsilon_a^{\text{ph}}$  or the mirror momentum  $\epsilon_a^{\text{mir}}$  are defined by the same formula

$$\epsilon_a(u) = a + \frac{2ig}{x^{[+a]}} - \frac{2ig}{x^{[-a]}}. \quad (5.5)$$

with the corresponding choice of  $x(u)$  from (5.2).

The physical roots  $u_{4,j}$  are subject to the exact, finite size Bethe ansatz equations

$$Y_{1,0}^{\text{ph}}(u_{4,j}) = -1 \quad (5.6)$$

where the  $Y_{1,0}^{\text{ph}}(u)$  was explicitly defined in [20] as an analytic continuation of  $Y_{1,0}(u)$  down through the cut  $(-\infty, -2g + \frac{i}{2}) \cup (+2g + \frac{i}{2}, +\infty)$ . The first term in (5.4) is given by the logarithmic pole contributions from the second one at the points  $u_{4,j}$ .

It is also important to mention that at large  $L$  the Y-functions of the middle (black) nodes are exponentially suppressed on the real axis in the mirror sheet

$$Y_{a,0}(u) \sim e^{-ip_a^{\text{mir}}(u)L}, \quad \text{where } p_a(u) = -i \log \left( \frac{x^{[+a]}}{x^{[-a]}} \right)^L. \quad (5.7)$$

## 5.1 Integrability of AdS/CFT Y-system and large volume limit

To study the AdS/CFT Y-system we need to clarify the analyticity properties of the Y-functions. Most of this information is due to the TBA derivation of the Y-system. The full understanding of these properties still needs additional efforts (see [37] for some advances). We will try to summarize them and demonstrate their naturalness. Ideal would be to postulate these properties from some simple and natural physical principles and then deduce from them the asymptotic Bethe ansatz (ABA) equations, along with the dressing factor (ignoring the standard S-matrix bootstrap procedure) as it can be done for various relativistic sigma-models (see [12, 38] for an inspiring example of the  $SU(N) \times SU(N)$  principal chiral field). On our current level of understanding of the AdS/CFT Y-system, this program can be fulfilled only partially.

This Y-system is equivalent to Hirota eq.(2.7) in the T-hook fig.4(left) with specific analyticity conditions. Fortunately, many of the results for the simplified Hirota eq.(4.1) for quasi-classical AdS/CFT, in particular (4.4) and (4.2), as well as the analyticity (4.7)-(4.10), can be generalized to the full quantum case. We will demonstrate in this section that the asymptotic Bethe ansatz (ABA) of [39] can be explained, and partially derived from the AdS/CFT Y-system (2.15) together with the relation (5.3), providing the reality of Y-functions, the  $s \leftrightarrow -s$  symmetry and certain natural analyticity assumptions, such as the existence of analyticity strips in  $u$ -plane.

<sup>VIII</sup>which can be partially motivated by a similar formula for the wrapping contributions in the quasi-classical quantization from the algebraic curve of the finite gap method, see [36, 19].

## 5.2 Generating functional for $U(2, 2|4)$ T-functions

Since Hirota equation for  $\text{AdS}_5/\text{CFT}_4$  is exactly the same as the one considered in the Sec.2 for spin chains one may try to construct its general solution in terms of only a few functions. But we here we deal with a non-compact symmetry group, and the  $\mathbb{T}$ -hook instead of the usual  $\mathbb{L}$ -shaped fat hook domain for the Y-system as a consequence. In the pervious section, in the strong coupling limit the difference between the  $U(4|4)$  and  $U(2, 2|4)$  generating functions was only in the way we expand various parts of (4.2) w.r.t. the generating parameter  $t$ . A natural generalization of (3.11) for the quantum case or the  $\mathbb{T}$ -hook gives  $T_{1,s}(u)$  in terms of the generating functional [19]

$$W = \left[ (1 - D\mathcal{Y}_1 D) \frac{1}{1 - D\mathcal{X}_1 D} \frac{1}{1 - D\mathcal{X}_2 D} (1 - D\mathcal{Y}_2 D) \right]_+ \times \quad (5.8)$$

$$\left[ (1 - D\mathcal{Y}_3 D) \frac{1}{1 - D\mathcal{X}_3 D} \frac{1}{1 - D\mathcal{X}_4 D} (1 - D\mathcal{Y}_4 D) \right]_- = \sum_{s=-\infty}^{\infty} D^s T_{1,s} D^s$$

Here  $\{\mathcal{Y}_1(u)|\mathcal{X}_1(u), \mathcal{X}_2(u)|\mathcal{Y}_2(u), \mathcal{Y}_3(u)|\mathcal{X}_3(u), \mathcal{X}_4(u)|\mathcal{Y}_4(u)\}$  are 8 arbitrary functions of the spectral parameter  $u$  parameterizing the general solution where, as a convenient choice for the  $\text{AdS}/\text{CFT}$  system, the grading is fixed by the Kac-Dynkin diagram  $\otimes - \circ - \otimes - \circ - \otimes$ . Similarly to the  $U(2, 2|4)$  characters (see after eq. (4.4)), we expand in positive powers of the shift operator  $D$ <sup>IX</sup> (replacing the  $t$  of (4.2)) inside the bracket  $[\dots]_+$  corresponding to the  $u(2|2)_R$  sub-algebra, and in negative powers of  $D$  inside the bracket  $[\dots]_-$  corresponding to the  $u(2|2)_L$  subalgebra<sup>X</sup>. As a result one gets an infinite sum for each  $T_{1,s}$ ,  $-\infty < s < \infty$ . Note also that (5.8) corresponds to a gauge where  $T_{0,s} = 1$  and all other  $T_{a,s}$  can be found from (2.16).

In the asymptotic  $L \rightarrow \infty$  limit the full Y-system in the  $U(2, 2|4)$   $\mathbb{T}$ -hook almost splits into two Y-subsystems of two  $su(2|2)_{L,R}$  fat hooks corresponding to the  $L, R$  wings:  $\mathcal{X}_1, \mathcal{X}_2, \mathcal{Y}_1, \mathcal{Y}_2$  are exponentially small whereas  $\mathcal{X}_3, \mathcal{X}_4, \mathcal{Y}_3, \mathcal{Y}_4$  are exponentially large, thus the terms in the sum over  $s$  are organized in powers of wrapping<sup>XI</sup>.

We can easily find these 8 functions in the  $L \rightarrow \infty$  limit by comparing  $T_{1,1}(u)$  generated from (5.8) with the explicit asymptotic solution of the Y-system with given Bethe roots found in [13] (partially by matching with the known ABA of [39])

$$\mathcal{Y}_1 = H_R F_0^+ \frac{\mathcal{Q}_1^-}{\mathcal{Q}_1^+}, \quad \mathcal{X}_1 = H_R \frac{\mathcal{Q}_1^- \mathcal{Q}_2^{++}}{\mathcal{Q}_1^+ \mathcal{Q}_2}, \quad \mathcal{X}_2 = H_R \frac{\mathcal{Q}_2^{--} \mathcal{Q}_3^+}{\mathcal{Q}_2 \mathcal{Q}_3}, \quad \mathcal{Y}_2 = H_R \frac{\mathcal{Q}_3^+}{\mathcal{Q}_3} F_4^-,$$

$$\mathcal{Y}_4 = H_L \frac{1}{F_0^-} \frac{\mathcal{Q}_7^+}{\mathcal{Q}_7^-}, \quad \mathcal{X}_4 = H_L \frac{\mathcal{Q}_7^+ \mathcal{Q}_6^{--}}{\mathcal{Q}_7^- \mathcal{Q}_6}, \quad \mathcal{X}_3 = H_L \frac{\mathcal{Q}_6^{++} \mathcal{Q}_5^-}{\mathcal{Q}_6 \mathcal{Q}_5^+}, \quad \mathcal{Y}_3 = H_L \frac{\mathcal{Q}_5^-}{\mathcal{Q}_5^+} \frac{1}{F_4^+} \quad (5.9)$$

<sup>IX</sup>We remind that  $D$  is defined by  $Df(u) = f(u - i/2)D$ . Since presently we may expect branch cuts originated from the map  $x(u)$  the shift may be ambiguous, the prescription is to analytically continue along the path going between the branch points without crossing the cuts going to infinity parallel to the real axes.

<sup>X</sup>As was noticed in [40], we can generate symmetric and antisymmetric representations by expanding the generating functional in powers of  $D$  and  $D^{-1}$  respectively. Mixed expansions generate infinite representations for non-compact real forms of  $gl(M|N)$ .

<sup>XI</sup>Wrappings are related to the Feynman graphs wrapped around the ‘‘spin chain’’ representing an operator of a length  $L$ : in weak coupling,  $k$  wrappings occur at the order  $\lambda^{Lk}$

$$\text{where } F_4 = \prod_j \frac{x - x_{4,j}^+}{x - x_{4,j}^-}, \quad H_R = \left(\frac{x^-}{x^+}\right)^{\frac{L}{2}} \prod_j \frac{x^+ - x_{4,j}^-}{x^- - x_{4,j}^-} \sigma(u, x_{4,j}^\pm) \quad (5.10)$$

$$F_0 = \bar{F}_4, \quad H_L = \tilde{H}_R. \quad (5.11)$$

As before, the bar means the complex conjugation in mirror plane whereas the tilde is the complex conjugation in physical plane. The  $\mathcal{Q}_a$  functions generalize the Baxter polynomials - they are generic "polynomials" on the two-sheet Riemann surface<sup>XII</sup>

$$\mathcal{Q}_a = \prod_{j=1}^{K_a} (x(u) - y_{a,j}) \prod_{j=1}^{\bar{K}_a} \left( \frac{1}{x(u)} - y_{\bar{a},j} \right). \quad (5.12)$$

The roots of these polynomials are constrained by the mirror reality condition of the Y functions. Namely, we have, as in the strong coupling limit (4.9)<sup>XIII</sup>

$$\bar{\mathcal{X}}_1 = \mathcal{X}_2, \quad \bar{\mathcal{Y}}_1 = \mathcal{Y}_2. \quad (5.13)$$

This asymptotic solution has a few important symmetries and analytic properties. We will study some of them below. It is very important to find a minimal set of such properties, such as reality and analyticity, which can be used then to constrain the 8 functions parameterizing the general solution, to generate only the physically relevant solutions. We present below a possible list of some of such properties which, in our opinion, should be satisfied by the physical solutions and try to constrain by them the ABA solution (5.9). This program worked well for the principal chiral field model [12,38] but it appears to be more tricky to do it for the AdS/CFT Y-system.

We will show that an essential part of ABA can be derived from these properties.

### 5.3 Minimal analyticity structure of Y-functions

Here we summarize some of the analyticity properties of Y-functions which, by our assumption, are satisfied by the physical solutions of the AdS/CFT Y-system:

*Reality:*

- I) Reality of Y-functions  $\bar{Y}_{a,s} = Y_{a,s}$
- II) Reality of the Bethe roots  $u_{4,j}$ <sup>XIV</sup>

*Analyticity:*

- 1)  $Y_{1,\pm 1}, Y_{2,\pm 2}$  should have a Zhukovski cut on the real axes and be related by (5.3)
- 2)  $Y_{1,s}$  should have no branch cuts inside the strip  $-\frac{s-1}{2} < \text{Im } u < \frac{s-1}{2}$
- 3)  $Y_{a,1}$  should have no branch cuts inside the strip  $-\frac{a-1}{2} < \text{Im } u < \frac{a-1}{2}$

<sup>XII</sup>We allow for some of the Bethe roots  $y_j$  to be at infinity.

<sup>XIII</sup> and similarly for the left wing:  $\bar{\mathcal{X}}_4 = \tilde{\mathcal{X}}_3, \quad \bar{\mathcal{Y}}_4 = \tilde{\mathcal{Y}}_3$

<sup>XIV</sup>We believe that the auxiliary roots should be real or appear in complex conjugated pairs, though this question deserves a better study.

4)  $Y_{a,0}$  should have no branch cuts inside the strip  $-\frac{a}{2} < \text{Im } u < \frac{a}{2}$

This list may be not enough to completely constrain the ABA and the physical meaning of some of them remains to be understood. All this deserves an additional study. But these properties are consistent with the TBA equations for the excited states.

In what follows we consider for simplicity the operators/states obeying the symmetry  $Y_{a,s} = Y_{a,-s}$ . The generalization to the full asymmetric case is almost straightforward. One can see that  $Y_{a,s} = Y_{a,-s}$  implies (which is also true for finite  $L$ )

$$\frac{\mathcal{X}_4^+}{\mathcal{Y}_4^+} = \frac{\mathcal{Y}_1^-}{\mathcal{X}_1^-}, \quad \frac{\mathcal{X}_4}{\mathcal{X}_3} = \frac{\mathcal{X}_2}{\mathcal{X}_1}, \quad \frac{\mathcal{X}_3^-}{\mathcal{Y}_3^-} = \frac{\mathcal{Y}_2^+}{\mathcal{X}_2^+}. \quad (5.14)$$

### 5.3.1 Reality

Reality of  $Y_{a,s>0}$  implies that  $T_{a,s}$  are also real up to a gauge transformation. Here we will examine this condition in the asymptotic large  $L$  limit.

It is easy to see that since the first four functions  $\mathcal{X}_1, \mathcal{Y}_1, \mathcal{Y}_2, \mathcal{X}_2$  are small whereas  $\mathcal{X}_3, \mathcal{Y}_3, \mathcal{Y}_4, \mathcal{X}_4$  are large in the  $L \rightarrow \infty$  limit only a half of the generating functional (5.8) (corresponding to one of the subgroups  $su(2|2)_{L,R}$ ) contributes. For  $s \geq 0$  the full functional reduces to [40]<sup>XV</sup>

$$\mathcal{W}^R \simeq (1 - D\mathcal{Y}_1 D) \frac{1}{1 - D\mathcal{X}_1 D} \frac{1}{1 - D\mathcal{X}_2 D} (1 - D\mathcal{Y}_2 D) \frac{\mathcal{Y}_3^- \mathcal{Y}_4^+}{\mathcal{X}_3^- \mathcal{X}_4^+} = \sum_{s=0}^{\infty} D^s T_{1,s} D^s \quad (5.15)$$

Since we fixed  $T_{0,s} = 1$  we have only two degrees of freedom left: one is a possible redefinition of  $D \rightarrow g(u)D$  which does not change the definition of the shift operator, whereas another corresponds to the transformation  $\mathcal{W} \rightarrow \mathcal{W}g(u)$ . In particular, we can remove the last factor from (5.15) by a desired gauge transformation (2.13) to get

$$\mathcal{W} = (1 - D\mathcal{Y}_1 D) \frac{1}{1 - D\mathcal{X}_1 D} \frac{1}{1 - D\mathcal{X}_2 D} (1 - D\mathcal{Y}_2 D). \quad (5.16)$$

Let us show that the hermiticity of the above generating functional automatically implies the reality of all  $Y_{a,s>0}$ . Indeed since  $D$  is hermitian we have

$$\begin{aligned} \mathcal{W} &= \sum_s D^s T_{1,s} D^s = \sum_s D^s \bar{T}_{1,s} D^s = \mathcal{W}^\dagger \\ &= (1 - D\bar{\mathcal{Y}}_2 D) \frac{1}{1 - D\bar{\mathcal{X}}_2 D} \frac{1}{1 - D\bar{\mathcal{X}}_1 D} (1 - D\bar{\mathcal{Y}}_1 D), \end{aligned} \quad (5.17)$$

which is equivalent to (5.13): since we have to equate the coefficients of infinitely many powers of  $D$  the monomials should coincide. This relation is a quantum analog of (4.8). Notice that (5.13) implies (assuming that  $H_R$  and  $F_4$  do not depend explicitly on the Bethe roots  $y_{a,j}, y_{\bar{a},j}$ ) that

$$\bar{\mathcal{Q}}_1 = \mathcal{Q}_3, \quad \bar{\mathcal{Q}}_2 = \mathcal{Q}_2, \quad \bar{F}_4 = F_0, \quad \bar{H}_R = H_R. \quad (5.18)$$

<sup>XV</sup>For  $s \leq 0$  only the complimentary part of the full generating functional, dropped in (5.16), is relevant.

The first equality implies that  $y_{\bar{1},j} = y_{3,j}$ ,  $y_{1,j} = y_{\bar{3},j}$ . The second equality tells us that  $y_{2,j} = y_{\bar{2},j}$  i.e. that  $\mathcal{Q}_2$  is a usual polynomial of  $u$ . Notice that the combination  $\mathcal{Q}_1\mathcal{Q}_3$  is a polynomial of  $u$ . Finally, the last equality implies for the (unitary) dressing factor

$$\prod_j \frac{\sigma(u, u_{4,j})}{\bar{\sigma}(u, u_{4,j})} = \prod_j \frac{1/x^- - x_{4,j}^+}{1/x^+ - x_{4,j}^+} \frac{x^- - x_{4,j}^-}{x^+ - x_{4,j}^-} \quad (5.19)$$

which is the crossing condition of [41]<sup>XVI</sup> (see [42] for its solution).

### 5.3.2 Analyticity properties 1), 2)

To see the consequences of the analyticity property 1) let us make a simple observation. By a direct calculation of the corresponding T-functions from (5.16) we get

$$Y_{1,+1}Y_{2,+2} \simeq \frac{\mathcal{X}_1^- \mathcal{X}_2^+}{\mathcal{Y}_1^- \mathcal{Y}_2^+} = \frac{1}{F_0 F_4}, \quad (5.20)$$

and hence the property 1) immediately implies  $F_0(u+i0)F_4(u+i0) = \frac{1}{F_0(u-i0)F_4(u-i0)}$ . To arrive to the above conclusion we used a weaker version of the property 1) for the product of two  $Y$  functions. In fact, one can get more from the property 1), namely  $F_4^{[+0]} = 1/F_0^{[-0]}$ , which together with (5.18) gives a powerful constraint on the functions  $F_4$  and  $F_0$ . We will show below that requiring  $F_4$  and  $F_0$  to have only one Zhukovski cut on the real axes leads to the conditions 2) and 3).

Let us study the property 2). Notice that the transformation  $\mathcal{X}_{1,2} \rightarrow g\mathcal{X}_{1,2}$ ,  $\mathcal{Y}_{1,2} \rightarrow g\mathcal{Y}_{1,2}$  where  $g(u)$  is an arbitrary function, does not affect  $Y_{1,s}$  and therefore it is a gauge transformation. If we take  $g = \frac{\mathcal{Q}_1^+}{H_R \mathcal{Q}_1^-}$  we notice that  $\mathcal{Q}_1$  appears only in the combination  $\mathcal{Q}_1\mathcal{Q}_3$ , which does not have branch cuts as we have shown above. This implies that in that gauge  $\mathcal{X}_1$  and  $\mathcal{X}_2$  have no branch cuts any more. Expanding the denominator in (5.16) we get

$$W \simeq \sum_{s=0}^{\infty} D^s (1 - D\mathcal{Y}_1^{[+s]}D) \left( \sum_{n=-s}^s \mathcal{X}_1^{[-s+1]} \dots \mathcal{X}_1^{[n-1]} \mathcal{X}_2^{[n+1]} \dots \mathcal{X}_2^{[+s-1]} \right) (1 - D\mathcal{Y}_2^{[-s]}D) D^s.$$

The cuts in  $T_{1,s}$  come only from  $\mathcal{Y}_1^{[+s-1]}$  and  $\mathcal{Y}_2^{[-s+1]}$ . The analyticity requirement 2) is satisfied since  $T_{1,s} \sim \mathcal{Y}_1^{[+s-1]}\mathcal{Y}_2^{[-s+1]} \sim F_0^{[+s]}F_4^{[-s]}$  have the analyticity strip  $|\text{Im}(u)| < s/2$  because  $F_0, F_4$  have only a single cut on the real axes.

### 5.3.3 Duality transformation and analyticity 3)

Similarly to the Sec.3.5 we can consider a duality transformation as an effect of the commutation of two operatorial factors within the generating functional:

$$(1 - D\mathcal{X}_1 D)^{-1} (1 - D\mathcal{Y}_1 D) = (1 - D\hat{\mathcal{Y}}_1 D) (1 - D\hat{\mathcal{X}}_1 D)^{-1} \quad (5.21)$$

<sup>XVI</sup>The original crossing relation of Janik coincides with (5.19) up to a factor which becomes 1 due to the zero total momentum (level matching) condition on the roots  $u_{4,j}$ .

and a similar equation for the factors with  $\mathcal{X}_2, \mathcal{Y}_2$ . It is convenient to parameterize the new factors as (compare it with (3.6),(3.18))

$$\hat{\mathcal{X}}_1 = \hat{H}_R \frac{\hat{\mathcal{Q}}_1^+}{\hat{\mathcal{Q}}_1^-} \frac{1}{F_0^-} , \quad \hat{\mathcal{Y}}_1 = \hat{H}_R \frac{\mathcal{Q}_2^- \hat{\mathcal{Q}}_1^+}{\mathcal{Q}_2 \hat{\mathcal{Q}}_1^-} , \quad \hat{\mathcal{Y}}_2 = \hat{H}_R \frac{\mathcal{Q}_2^{++} \hat{\mathcal{Q}}_3^-}{\mathcal{Q}_2 \hat{\mathcal{Q}}_3^+} , \quad \hat{\mathcal{X}}_2 = \hat{H}_R \frac{\hat{\mathcal{Q}}_3^-}{\hat{\mathcal{Q}}_3^+} \frac{1}{F_4^+} \quad (5.22)$$

where by definition  $\hat{H}_R$  can only depend on the momentum carrying roots  $u_{4,k}$  whereas  $\hat{\mathcal{Q}}_1$  is a function of the form (5.12). In this parameterization we have  $\hat{\mathcal{X}}_1^+/\hat{\mathcal{Y}}_1^+ = \mathcal{X}_1^-/\mathcal{Y}_1^-$ ,  $\hat{\mathcal{X}}_2^-/\hat{\mathcal{Y}}_2^- = \mathcal{X}_2^+/\mathcal{Y}_2^+$  and to keep (5.16) intact we only have to satisfy compare with (3.19))  $\hat{\mathcal{X}}_1 - \hat{\mathcal{Y}}_1 = \mathcal{X}_1 - \mathcal{Y}_1$ ,  $\hat{\mathcal{X}}_2 - \hat{\mathcal{Y}}_2 = \mathcal{X}_2 - \mathcal{Y}_2$ . Second equation is the complex conjugate of the first one. The first equation gives  $\frac{\hat{\mathcal{Q}}_1^+ \mathcal{Q}_1^+}{\hat{\mathcal{Q}}_1^- \mathcal{Q}_1^-} = F_0^- \frac{H_R}{\hat{H}_R} \frac{F_0^+ \mathcal{Q}_2^- \mathcal{Q}_2^{++}}{F_0^- \mathcal{Q}_2^- - \mathcal{Q}_2^{++}}$  which has the solution  $\hat{\mathcal{Q}}_1 \mathcal{Q}_1 = f(u, x_{4,k})(F_0 \mathcal{Q}_2^- - \mathcal{Q}_2^+)$ . Since the r.h.s. has no poles at  $x = 1/x_{4,k}^+$  and cannot explicitly depend on  $x_{4,k}$  we should take  $f = C \prod_k (1/x - x_{4,k}^+)$  to cancel the poles in  $F_0$ . This leads to the condition  $\hat{\mathcal{Q}}_1 \mathcal{Q}_1 \propto \mathcal{Q}_2^+ \prod_{k=1}^{K_4} (1/x - x_{4,k}^+) - \mathcal{Q}_2^- \prod_{k=1}^{K_4} (1/x - x_{4,k}^-)$  from where we can determine  $\hat{\mathcal{Q}}_1$  and its complex conjugate  $\hat{\mathcal{Q}}_3$ . The resulting formulas are analogous to (3.20).

We demonstrated above that the terms in the generating functional can be reshuffled in such a way that the expression for the new elementary factors (5.22) are very similar to the initial ones (5.9), with the modified Bethe roots.

Now let us use this fact to show that  $Y_{a,1}$  are also analytic in their strips given in the property 3). Indeed, using the Bäcklund relations, in the way similar to the subsection 3.3 where  $T_{a,s}$  was generated from  $\mathcal{W}$ , we can show that  $T_{a,1}$  can be computed from  $\mathcal{W}^{-1}$  as follows [9]

$$\mathcal{W}^{-1} = (1 - D\hat{\mathcal{X}}_2 D) \frac{1}{1 - D\hat{\mathcal{Y}}_2 D} \frac{1}{1 - D\hat{\mathcal{Y}}_1 D} (1 - D\hat{\mathcal{X}}_1 D) \simeq \sum_{a=0}^{\infty} (-1)^a D^a T_{a,1} D^a . \quad (5.23)$$

As we saw in subsection 5.3.2, for the analyticity of T-functions in their physical strips  $F_4$  should have a cut only on the real axes. The arguments given there can be also applied to the functional (5.23) which leads to the proof of the property 3). It also shows that in a certain gauge  $T_{a,1}$  has the analyticity strip  $|\text{Im}(u)| < a/2$ .

Due to (5.7) we can drop the denominator in the r.h.s. of (2.15) at  $s = 0$  and rewrite it, using  $1 + Y_{a,s} = \frac{T_{a,s}^+ T_{a,s}^-}{T_{a+1,s} T_{a-1,s}}$  following from (2.7) and (2.14),  $\frac{Y_{a,0}^+ Y_{a,0}^-}{Y_{a-1,0} Y_{a+1,0}} \simeq \left( \frac{T_{a,1}^+ T_{a,1}^-}{T_{a-1,1} T_{a+1,1}} \right)^2$ , where in the equation for  $a = 1$  one should replace in the l.h.s.  $Y_{0,0}$  by 1. Solving this Y-system equation for  $Y_{a,0}$  we get  $Y_{a,0} = \frac{\phi(u+ia/2)}{\phi(u-ia/2)} T_{a,1}^2$  where the first factor, a zero mode, is easy to calculate since  $\phi(u)$  can be extracted from  $Y_{1,0}$ . Hence the most complicated part of  $Y_{a,0}$  is hidden in  $T_{a,1}$  and has the correct analyticity structure 4). The proof of the correct analyticity of the factor  $\frac{\phi(u+ia/2)}{\phi(u-ia/2)}$  is left to the reader.

### 5.3.4 Reality of $Y_{a,0}$

Finally let us also imply the reality condition to  $Y_{1,0} = \frac{(\mathcal{Y}_1 - \mathcal{X}_1 - \mathcal{X}_2 + \mathcal{Y}_2)^2}{\mathcal{Y}_2 \mathcal{Y}_3}$ . Note that the numerator is real, so for the reality of  $Y_{1,0}$  we only have to require that  $\mathcal{Y}_2 \mathcal{Y}_3 = H_L H_R \frac{F_4^-}{F_4^+}$  is

real. Note that the factors  $H_R$  is a real function as a consequence of the crossing equation in the mirror kinematics stemming from the last of eqs.(5.18). In the physical kinematics  $H_L$  is conjugate to  $H_R$  and naively one would expect it to be also real as well. However the conjugation in the physical sense does not necessarily commute with the mirror conjugation. Explicit calculation shows that  $\mathcal{Y}_2\mathcal{Y}_3 = \frac{Q_4^{++}Q_4^{--}}{Q_4^2}$  ,  $Q_4 = \prod_{k=1}^{K_4}(u - u_{4,k})$  which is indeed real. The reality of all other  $Y_{a,0}$  follows from the Y-system.

Finally, the above expression for  $Y_{1,0}$  simplifies on a Bethe root  $u = u_{4,k}$ : since  $1/F_4^-(u_{4,k}) = 0$  ,  $\mathcal{Y}_2$  dominates the numerator and we get from  $Y_{1,0}(u_{4,k}) = \mathcal{Y}_2/\mathcal{Y}_3 = \frac{H_R}{H_L} F_4^+ F_4^- \frac{Q_3^+ Q_5^+}{Q_3^- Q_5^-} = -1$ . Since  $H_R$  is a complex conjugate of  $H_L$  we see that  $Y_{1,0}(u_{4,k})$  is unimodular in the physical kinematics, ensuring the reality of the Bethe roots  $u_{4,k}$ <sup>XVII</sup>.

## 6 Conclusions and perspectives

Our main purpose in these notes was mainly pedagogical: to show the power of Hirota discrete integrable dynamics (HDID) for the solution of quantum integrable models. The Bäcklund method of solution of Hirota equation for fusion in the supersymmetric generalizations of the Heisenberg spin chain, with the polynomiality condition of the transfer matrix gives a rather direct way of derivation of the final Bethe ansatz equations for the roots of Baxter's Q-polynomials. However, the applications of HDID is not limited to the spin chains and can be quite efficient in the study of integrable CFT's,  $\sigma$ -models at finite volume and, remarkably, in such a complicated problem as the AdS<sub>5</sub>/CFT<sub>4</sub> system.

We demonstrated that the general asymptotic solution of Y-system for AdS/CFT obeys several remarkable analyticity and reality properties. They seem to be rather constraining and could be used at finite volume to single out the physically relevant solutions of this Y-system. It seems possible to reverse the logic and derive the asymptotic Bethe ansatz equations from these equations, as in relativistic  $\sigma$ -models.

We hope that further study of this circle of questions, and in particular of the role and the consequences of the equation (5.3), will lead to the complete understanding of the analyticity structure of the integrable AdS/CFT systems. This understanding, together with the solutions of Y-system stemming from the HDID (in the form the generating functional (5.8) or in the Wronskian form recently obtained in [43]) should allow to reduce the problem to a finite set of integral Destri-DeVega type equations.

### Acknowledgments

The work of VK was partly supported by the ANR grants INT-AdS/CFT (ANR36ADSCSTZ) and GranMA (BLAN-08-1-313695) and the grant RFFI 08-02-00287. V.K. also thanks NORDITA institute in Stockholm, as well as Vladimir Bazhanov and the theoretical physics group of Australian National University (Canberra) for the kind hospitality and interesting discussions. We thank Sebastien Leurent, Zengo Tsuboi, Pedro Vieira and especially Dymitro Volin for useful discussions.

<sup>XVII</sup>This property was also demonstrated in [20] numerically to hold at finite  $L$ .

## References

- [1] R. Hirota, Journal of the Phys. Soc. of Japan, **50** (1981) 3785-3791.
- [2] M. Jimbo and T. Miwa, Publ. Res. Inst. Math. Sci. Kyoto **19** (1983) 943.
- [3] A. Klümper and P. A. Pearce, Physica A **183** (1992) 304. ; A. Kuniba, T. Nakanishi and J. Suzuki, Int. J. Mod. Phys. A **9** (1994) 5215 ; L. Faddeev, A. Volkov, Lett. Math. Phys. **32** (1994) 125
- [4] Al. B. Zamolodchikov, Nuclear Physics B **342**, (1990) 695
- [5] V. V. Bazhanov, S. L. Lukyanov and A. B. Zamolodchikov, Commun. Math. Phys. **177** (1996) 381
- [6] I. Krichever, O. Lipan, P. Wiegmann and A. Zabrodin, Commun. Math. Phys. **188** (1997) 267
- [7] V. V. Bazhanov, S. L. Lukyanov and A. B. Zamolodchikov, Nucl. Phys. B **489**, 487 (1997) ; P. Dorey and R. Tateo, Nucl. Phys. B **482**, 639 (1996) ; G. Juttner, A. Klumper and J. Suzuki, Nucl. Phys. B **512** (1998) 581 ; P. Fendley, Nucl. Phys. B **374**, 667 (1992) ; D. Fioravanti, A. Mariottini, E. Quattrini and F. Ravanini, Phys. Lett. B **390** (1997) 243 [arXiv:hep-th/9608091].
- [8] Z. Tsuboi, J. Phys. A **30**, 7975 (1997) ; Z. Tsuboi, Physica A **252**, 565 (1998)
- [9] V. Kazakov, A. S. Sorin and A. Zabrodin, Nucl. Phys. B **790** (2008) 345
- [10] V. Kazakov and P. Vieira, JHEP **0810** (2008) 050 ; V. Kazakov, S. Leurent, Z. Tsuboi, [arXiv:1010.4022 [math-ph]].
- [11] V. V. Bazhanov and Z. Tsuboi, Nucl. Phys. B **805** (2008) 451 ; Z. Tsuboi, Nucl.Phys.B 826 (2010) 399
- [12] N. Gromov, V. Kazakov and P. Vieira, JHEP **0912** (2009) 060
- [13] N. Gromov, V. Kazakov and P. Vieira, Phys. Rev. Lett. **103** (2009) 131601
- [14] D. Bombardelli, D. Fioravanti and R. Tateo, J. Phys. A **42**, 375401 (2009)
- [15] N. Gromov, V. Kazakov, A. Kozak and P. Vieira, Lett. Math. Phys. **91**(2010)265
- [16] G. Arutyunov and S. Frolov, JHEP **0905** (2009) 068
- [17] R. A. Janik and T. Lukowski, Phys. Rev. D **76**, 126008 (2007) ; M. P. Heller, R. A. Janik and T. Lukowski, JHEP **0806**, 036 (2008) ; Z. Bajnok and R. A. Janik, Nucl. Phys. B **807**, 625 (2009) ; Z. Bajnok, R. A. Janik and T. Lukowski, arXiv:0811.4448 [hep-th]. ; F. Fiamberti, A. Santambrogio, C. Sieg and D. Zanon, Nucl. Phys. B **805** (2008) 231 ; V. N. Velizhanin, arXiv:0811.0607 [hep-th] ; G. Arutyunov, S. Frolov and R. Suzuki, arXiv:1002.1711 [hep-th]. ; T. Lukowski, A. Rej

- and V. N. Velizhanin, Nucl. Phys. B **831** (2010) 105 ; J. Balog and A. Hegedus, JHEP **1006**, 080 (2010) ; V. N. Velizhanin, arXiv:0811.0607 [hep-th].
- [18] N. Gromov, JHEP **1001**, 112 (2010)
- [19] N. Gromov, V. Kazakov and Z. Tsuboi, JHEP **07** (2010) 097
- [20] N. Gromov, V. Kazakov, P. Vieira, Phys. Rev. Lett. **104** (2010) 211601. [arXiv:0906.4240 [hep-th]].
- [21] Z.Bajnok, “*Review of AdS/CFT Integrability, Chapter III.6: Thermodynamic Bethe Ansatz,*” arXiv:1012.3995 [hep-th].
- [22] S. S. Gubser, I. R. Klebanov and A. M. Polyakov, Phys. Lett. B **428** (1998) 105
- [23] A. Zabrodin, arXiv:0705.4006 [hep-th].
- [24] L. D. Faddeev, arXiv:hep-th/9605187.
- [25] V. V. Bazhanov and N. Y. Reshetikhin, Int. J. Mod. Phys. A **4** (1989) 115.
- [26] I. Bena, J. Polchinski and R. Roiban, Phys. Rev. D **69**, 046002 (2004)
- [27] N. Beisert, V. Kazakov, K. Sakai, K. Zarembo, Comm.Math.Phys. **263**, 659 (2006)
- [28] S.Schäfer-Nameki, “*Review of AdS/CFT Integrability, Chapter II.4: The Spectral Curve,*” arXiv:1012.3989 [hep-th].
- [29] S.-J. Cheng, N. Lam and R.B. Zhang, J. Algebra **273**, 780 (2004)
- [30] J.-H. Kwon, Adv. Math. **217** 713 (2008)
- [31] D. Serban and M. Staudacher, JHEP **0406** (2004) 001
- [32] N. Beisert, V. A. Kazakov, K. Sakai and K. Zarembo, JHEP **0507** (2005) 030
- [33] G. Japaridze, A. Nersesian and P.Wiegmann, Nucl. Phys. B **230** (1984) 511. ; E. Ogievetsky and P. Wiegmann, Phys. Lett. B **168** (1986) 360. ; E. Ogievetsky, P. Wiegmann and N. Reshetikhin, Nucl. Phys. B **280** (1987) 45.
- [34] N. Dorey and B. Vicedo, JHEP **0703**, 045 (2007)
- [35] A. Hegedus, Nucl. Phys. B **825**, 341 (2010)
- [36] N. Gromov and P. Vieira, Nucl. Phys. B **789** (2008) 175
- [37] A. Cavaglia, D. Fioravanti and R. Tateo, arXiv:1005.3016 [hep-th].
- [38] V. Kazakov and S. Leurent, arXiv:1007.1770 [hep-th].
- [39] N. Beisert, B. Eden and M. Staudacher, *J. Stat. Mech.* **0701** (2007) P021

- [40] N. Beisert, *J. Stat. Mech.* **0701**, P017 (2007)
- [41] R. A. Janik, *Phys. Rev.* **D73** (2006) 086006
- [42] P.Vieira and D.Volin, “*Review of AdS/CFT Integrability, Chapter III.3: The Dressing Factor,*” arXiv:1012.3992 [hep-th].
- [43] N. Gromov, V. Kazakov, S. Leurent, Z. Tsuboi [arXiv:1010.2720 [hep-th]].

# Review of AdS/CFT Integrability, Chapter IV.1: Aspects of Non-Planarity

C. KRISTJANSEN

*The Niels Bohr Institute, Blegdamsvej 17, DK-2100 Copenhagen Ø, Denmark*

kristjan@nbi.dk

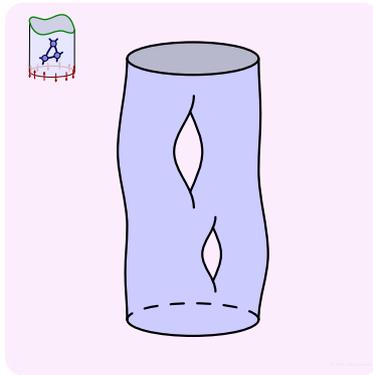

**Abstract:** We review the role of integrability in certain aspects of  $\mathcal{N} = 4$  SYM which go beyond the planar spectrum. In particular, we discuss integrability in relation to non-planar anomalous dimensions, multi-point functions and Maldacena-Wilson loops.

# 1 Introduction

The discovery of the integrability of the planar spectral problem of AdS/CFT [1–3] has provided us with a wealth of new results and tools for the study of gauge and string theory. Given this success it is natural to investigate whether the integrability extends to other aspects of the AdS/CFT correspondence. Here we shall discuss this possibility mainly from the gauge theory perspective and staying entirely within the maximally supersymmetric gauge theory in four dimensions,  $\mathcal{N} = 4$  SYM. The fate of the integrability of the planar spectral problem when reducing or completely removing the supersymmetry is discussed in the chapters [4] and [5]. A natural direction in which to search for integrability is in the non-planar version of the spectral problem. As we will review below, while the non-planar version of the dilatation generator can easily be written down (at least in some sub-sectors and to a certain loop order) attempts to diagonalize it have so far not revealed any traces of integrability. For a conformal field theory like  $\mathcal{N} = 4$  SYM natural observables apart from anomalous dimensions are the structure constants which appear in the three point functions of the theory and govern the theory’s operator product expansion. Three-point functions are of course not unrelated to non-planar anomalous dimensions as correlators of three traces can be seen as building blocks for higher genus two-point functions. As we shall see the calculation of structure constants of  $\mathcal{N} = 4$  SYM is impeded by extensive operator mixing. For a certain subset of operators, this mixing can be handled via the diagonalization of the planar dilatation operator and the structure constants can be calculated using tools pertaining to planar integrability. An integrable structure allowing to treat all types of three-point functions has not been identified.

Anomalous dimensions and structure constants are observables which are associated with local gauge invariant operators but in a gauge theory one of course also has at hand numerous types of non-local observables such as Wilson loops, ’t Hooft loops, surface operators and domain walls. Here we will limit our discussion to Wilson loops, more precisely to locally supersymmetric Maldacena-Wilson loops. Another type of Wilson loops, Alday-Maldacena-Wilson loops and their relation to scattering amplitudes of  $\mathcal{N} = 4$  SYM will be discussed in the chapters [6]. As was known before the discovery of the spin-chain related integrability of the AdS/CFT system, expectation values of Maldacena-Wilson loops can in certain cases be expressed in terms of expectation values of a zero-dimensional integrable matrix model and this connection has provided us with the most successful test of the AdS/CFT correspondence beyond the planar limit to date. The connection of Maldacena-Wilson loops to integrability in the form of spin-chain integrability is so far very limited.

We start by discussing the role of integrability in connection with non-planar anomalous dimensions in section 2 and subsequently treat multi-point functions and Maldacena-Wilson loops in sections 3 and 4.

## 2 Non-planar anomalous dimensions

In a CFT conformal operators,  $\{\mathcal{O}_\alpha\}$ , and their associated conformal dimensions,  $\Delta_\alpha$ , are characterized by being eigenstates and eigenvalues of the dilatation generator,  $\hat{D}$ . As a consequence of this two-point functions of conformal operators upon appropriate normalization take the form

$$\langle \mathcal{O}_\alpha(x) \mathcal{O}_\beta(y) \rangle = \frac{\delta_{\alpha\beta}}{(x-y)^{2\Delta_\alpha}}. \quad (2.1)$$

### 2.1 The non-planar dilatation generator

The dilatation generator,  $\hat{D}$ , of  $\mathcal{N} = 4$  SYM has a double expansion in  $\lambda$  and  $\frac{1}{N}$  where  $\lambda$  is the 't Hooft coupling which we until further notice take to be

$$\lambda = \frac{g_{\text{YM}}^2 N}{8\pi^2}, \quad (2.2)$$

and where  $N$  is the order of the gauge group,  $SU(N)$ . By the planar limit we mean the limit  $N \rightarrow \infty$ ,  $\lambda$  fixed. At a finite order in  $\lambda$  the  $\frac{1}{N}$ -expansion of the dilatation generator starts at order  $N^0$  and terminates after finitely many terms, the number of which increases with the loop order. The planar dilatation generator and its loop expansion is discussed in the chapter [7]. The non-planar part of the dilatation generator was first derived at one loop order in the  $SO(6)$  sector [8, 9], see also [10]. The derivation was based on evaluation of Feynman diagrams and was extended to two-loop order in the  $SU(2)$  sector in [2]. Later a derivation based entirely on algebraic arguments gave the dilatation generator including non-planar parts for all fields at one-loop order [11] and for the fields in the  $SU(1,1|2)$  sector at two-loop order [12]. Recently, the non-planar part of the dilatation generator was written down at order  $\lambda^{3/2}$  in the  $SU(2|3)$  sector [13]. In addition, the non-planar part of the dilatation generator is known in the scalar sector in a certain  $\mathcal{N} = 2$  superconformal gauge theory [14]. In ABJM theory [15] and ABJ theory [16] the non-planar part of the two-loop dilatation generator has been derived in a  $SU(2) \times SU(2)$  sector [17, 18].<sup>1</sup>

The diagonalization problem for the full dilatation generator of  $\mathcal{N} = 4$  SYM has mainly been studied in the  $SU(2)$ -sector which consists of multi-trace operators built from two complex scalar fields, say  $X$  and  $Z$ . For simplicity we shall likewise focus our discussion on this sector. The one-loop dilatation generator including the non-planar parts reads for the  $SU(2)$  sector

$$\hat{D} = -\frac{\lambda}{N} : \text{Tr}[X, Z][\check{X}, \check{Z}] :, \quad \text{where} \quad \check{Z}_{\alpha\beta} = \frac{\delta}{\delta Z_{\beta\alpha}}, \quad (2.3)$$

---

<sup>1</sup>We remark that our  $\hat{D}$  is the dilatation generator describing the asymptotic spectrum. Hence we ignore the wrapping contributions discussed in the chapters [7, 19]. In particular, the splitting of the dilatation operator into planar and non-planar parts that we discuss here pertains to the asymptotic regime. What is here referred to as non-planar parts of the dilatation generator might for short operators give rise to planar wrapping contributions [20].

and similarly for  $\check{X}$ . The normal ordering symbol signifies that the derivatives should not act on the  $X$  and  $Z$  field belonging to the dilatation generator itself. Below we illustrate how the full dilatation generator acts on a double trace operator. Notice that we only consider one out of four terms contributing to the dilatation generator and that we only represent one possible way of applying the derivatives

$$\begin{aligned} \text{Tr}(ZX\check{Z}\check{X}) \cdot \overbrace{\text{Tr}(XZXXZ)}^1 \text{Tr}(XZ) &= \text{Tr}(ZX\check{Z}\check{Z}X\overbrace{XZ}^2) \overbrace{\text{Tr}(XZ)}^3 \\ &= N\text{Tr}(ZXX\check{X}\check{Z}) \text{Tr}(XZ) + \text{Tr}(ZX) \text{Tr}(ZX\check{X}) \text{Tr}(XZ) + \text{Tr}(ZX\check{Z}\check{Z}X\check{X}\check{Z}). \end{aligned}$$

As is evident from this example the full one-loop dilatation generator can be written as follows

$$\hat{D} = \lambda(\hat{D}_0 + \frac{1}{N} \hat{D}_+ + \frac{1}{N} \hat{D}_-), \quad (2.4)$$

where  $\hat{D}_+$  and  $\hat{D}_-$  respectively increases and decreases the trace number by one and where  $\hat{D}_0$  conserves the number of traces. Suggestions for how to write  $\hat{D}_+$  and  $\hat{D}_-$  in a more explicit form can be found in [21, 22]. We notice that for gauge group  $SO(N)$  or  $Sp(N)$  the one-loop dilatation operator will have a term which is of order  $\frac{1}{N}$  but still conserves the number of traces [23]. At  $l$ -loop order the dilatation operator can change the number of traces by at most  $l$ . Notice that since the anomalous dimensions are the *eigenvalues* of the dilatation generator these do not necessarily have a  $\frac{1}{N}$ -expansion which truncates. What is more, some anomalous dimensions do not even have a well-defined double expansion in  $\lambda$  and  $\frac{1}{N}$ . An example of an operator with this property can be found in [2]. Speaking about a one-loop anomalous dimension, however, always makes sense. To calculate the leading  $\frac{1}{N}$ -corrections to one-loop anomalous dimensions one can make use of standard quantum mechanical perturbation theory. Let us assume that we have found an eigenstate of the planar dilatation generator  $\hat{D}_0$ , i.e.

$$\hat{D}_0|\mathcal{O}\rangle = \gamma_{\mathcal{O}}|\mathcal{O}\rangle, \quad (2.5)$$

and let us treat the terms sub-leading in  $\frac{1}{N}$  as a perturbation. First, let us assume that there are no degeneracies between  $n$ -trace states and  $(n+1)$ -trace states in the spectrum. If that is the case we can proceed by using non-degenerate quantum mechanical perturbation theory. Clearly, the  $\frac{1}{N}$  terms in eqn. (2.4) do not have any diagonal components so the correction to the anomalous dimension for the state  $|\mathcal{O}\rangle$  reads

$$\delta\gamma_{\mathcal{O}} = \frac{1}{N^2} \sum_{\mathcal{K} \neq \mathcal{O}} \frac{\langle \mathcal{O} | \hat{D}_+ + \hat{D}_- | \mathcal{K} \rangle \cdot \langle \mathcal{K} | \hat{D}_+ + \hat{D}_- | \mathcal{O} \rangle}{\gamma_{\mathcal{O}} - \gamma_{\mathcal{K}}}, \quad (2.6)$$

and is of order  $\frac{1}{N^2}$ . If there are degeneracies between  $n$ -trace states and  $(n+1)$ -trace states we have to diagonalize the perturbation in the subset of degenerate states and the corrections will typically be of order  $\frac{1}{N}$ . We remark that the dilatation generator is *not* a Hermitian operator but it is related to its Hermitian conjugate by a similarity transformation and therefore its eigenvalues are always real [24, 9].

## 2.2 The non-planar spectrum and integrability

Planar  $\mathcal{N} = 4$  SYM is described in terms of only one parameter,  $\lambda$ , and planar anomalous dimensions have a perturbative expansion in terms of this single parameter. This fact made it possible initially to search for integrability in the planar spectrum order by order in  $\lambda$ . In particular, the concept of perturbative integrability was introduced, meaning that at  $l$  loops the planar spectrum could be described as an integrable system when disregarding terms of order  $\lambda^{l+1}$  [2]. Studying this perturbative form of integrability eventually led to the all loop Bethe equations conjectured to be true perturbatively to any loop order and non-perturbatively as well [25–27]. When going beyond the planar limit it is natural to follow a similar perturbative approach. The question of integrability beyond the planar limit has so far been addressed only perturbatively in  $\frac{1}{N}$  at the one-loop order. The fact that the non-planar part of the dilatation generator introduces splitting and joining of traces enormously enlarges the Hilbert space of states of the system. This complicates the direct search for integrability via the identification of conserved charges or the construction of an asymptotic S-matrix with the appropriate properties. As a simple way of getting an indication of whether integrability persists at the non-planar level one can test for degenerate parity pairs [2]. Parity pairs are operators with the same anomalous dimension but opposite parity where the parity operation on a single trace operator is defined by [28]

$$\hat{P} \cdot \text{Tr}(X_{i_1} X_{i_2} \dots X_{i_n}) = \text{Tr}(X_{i_n} \dots X_{i_2} X_{i_1}). \quad (2.7)$$

(For a multi-trace operator,  $\hat{P}$  must act on each of its single trace components.) At the planar one-loop level one observes a lot of such parity pairs. The presence of these degeneracies has its origin in the integrability of the model.  $\mathcal{N} = 4$  SYM is parity invariant and its dilatation generator commutes with the parity operation, i.e.

$$[\hat{D}, \hat{P}] = 0. \quad (2.8)$$

Notice that this only tells us that eigenstates of the dilatation generator can be organized into eigenstates of the parity operator and nothing about degeneracies in the spectrum. The degeneracies can be explained by the existence of an extra conserved charge,  $\hat{Q}_3$ , which commutes with the dilatation generator but anti-commutes with parity, i.e.

$$[\hat{D}, \hat{Q}_3] = 0, \quad \{\hat{P}, \hat{Q}_3\} = 0. \quad (2.9)$$

Acting on a state with  $\hat{Q}_3$ , one obtains another state with the opposite parity but with the same energy<sup>2</sup>. Taking into account non-planar corrections the degeneracies are lifted. Since parity is still conserved this is taken as an indication (but not a proof, obviously) of the disappearance of the higher conserved charges and thus a breakdown of integrability. Notice that in accordance with this picture, the parity pairs survive the inclusion of planar higher loop corrections. The situation in ABJM theory is the same. Degenerate parity pairs are seen at the planar level but disappear once non-planar corrections are taken into account [17]. (For  $\mathcal{N} = 4$  SYM with gauge group  $SO(N)$  or  $Sp(N)$  parity is

---

<sup>2</sup>There exist states which are unpaired and annihilated by  $\hat{Q}_3$ .

gauged and the concept of planar parity pairs loses its meaning [23]. For ABJ theory parity is broken at the non-planar level [18].) Hence it seems that one can not hope for integrability of the spectrum of AdS/CFT beyond the planar limit, at least not in a simple perturbative sense.<sup>3</sup>

### 2.3 Results on non-planar anomalous dimensions

Prior to the derivation of the dilatation generator of  $\mathcal{N} = 4$  SYM anomalous dimensions were determined through a rather complicated process which involved for each set of operators considered an explicit calculation of their two-point correlation functions through Feynman diagram evaluation. Early results on non-planar anomalous dimensions for short operators obtained by this method can be found in [30, 31].

With the derivation of the dilatation generator the calculation of anomalous dimensions was enormously simplified. At the planar level one now even has at hand the tools of integrability and all information about the (asymptotic) spectrum is encoded in a set of algebraic Bethe equations. As argued above similar tools are not currently available at the non-planar level. Thus to obtain spectral information beyond the planar limit one has to explicitly diagonalize the dilatation generator in each closed subset of states. For the following discussion it is convenient to divide the set of operators into three different types, short operators, BMN type operators and operators dual to spinning strings.

By short operators we mean operators which contain a finite, small number of fields. Such operators only mix with a finite, small number of other operators and the resulting mixing matrix can be calculated and diagonalized by hand (or using Mathematica). Various results on non-planar corrections to anomalous dimensions of short operator in the  $SU(2)$  sector of  $\mathcal{N} = 4$  SYM can be found in [2] and [21]. Reference [21] in addition contains results on the  $SL(2)$ -sector of  $\mathcal{N} = 4$  SYM. Results for the  $SU(2) \times SU(2)$  sector of ABJM and ABJ theory were obtained in [17] and [18].

BMN type operators [32] are operators consisting of many fields of one type and a few excitations in the form of fields of another type (or of derivatives). Two-excitation eigenstates can easily be written down at the planar level. In the  $SU(2)$  sector they read

$$\mathcal{O}_n^{J_0, J_1, \dots, J_k} = \frac{1}{J_0 + 1} \sum_{p=0}^{J_0} \cos\left(\frac{\pi n(2p + 1)}{J_0 + 1}\right) \text{Tr}(X Z^p X Z^{J_0-p}) \text{Tr}(Z^{J_1}) \dots \text{Tr}(Z^{J_k}), \quad (2.10)$$

where  $0 \leq n \leq \lfloor \frac{J_0}{2} \rfloor$  and where the corresponding planar eigenvalues are

$$E_n = 8\lambda \sin^2\left(\frac{\pi n}{J_0 + 1}\right). \quad (2.11)$$

Acting with the non-planar part of the dilatation generator on BMN states only requires a finite and small number of operations and the non-planar part of the mixing matrix for

<sup>3</sup>The paper, [29], entitled “Hints of Integrability Beyond the Planar Limit: Non-trivial Backgrounds” is dealing with anomalous dimensions of operators from the  $SU(2)$ -sector consisting of the factor  $(\det(Z))^M$  multiplying a single trace operator. In the limit  $N, M \rightarrow \infty$  with  $\frac{N}{M} \rightarrow 0$  and  $g_{\text{YM}}^2 M$  fixed the authors find a set of conserved charges commuting with the dilatation generator. We remark, however, that in the limit considered the terms  $\hat{D}_+$  and  $\hat{D}_-$  do not contribute to the dilatation generator.

BMN states can easily be written down [9]. Treating  $\hat{D}_+ + \hat{D}_-$  as a perturbation of  $\hat{D}_0$  one should thus be able to determine the leading non-planar corrections to the anomalous dimensions of BMN operators by standard quantum mechanical perturbation theory, cf. section 2.2. However, degeneracies between single and multiple-trace states require the use of degenerate perturbation theory and due to the complexity of the coupling between degenerate states the mixing problem for BMN states was never resolved. For a discussion of this problem, see [33]. There is one case, however, for which there is no degeneracy issue and that is for states with mode number,  $n = 1$ . Here it is possible to find the leading non-planar correction to the anomalous dimension in the limit  $J_i \rightarrow \infty$ ,  $i = 0, 1, \dots, k$ , and  $\lambda \rightarrow \infty$  with  $\lambda' = \lambda/J^2$  and  $g_2 = J^2/N$  fixed where  $J = \sum_{i=0}^k J_i$ . The result reads [8, 34]

$$\delta E_{n=1} = \lambda' g_2^2 \left( \frac{1}{12} + \frac{35}{32\pi^2} \right). \quad (2.12)$$

There exist similar results for BMN operators belonging to the  $SL(2)$  sector of  $\mathcal{N} = 4$  SYM [35] and for BMN operators in a certain  $\mathcal{N} = 2$  superconformal gauge theory [14]. The result in eqn. (2.12) was extended to two-loop order in [9].

The third class of operators, operators dual to spinning strings, consist of an infinitely large number of background fields and an infinite number of excitations. In the  $SU(2)$  sector they take the form

$$\mathcal{O} = \text{Tr}(Z^{J-M} X^M) + \dots, \quad (2.13)$$

where  $\dots$  denotes similar terms obtained by permuting the fields and where  $J, M \rightarrow \infty$ , but  $M/J$  is kept finite. Acting with the non-planar dilatation generator on such an operator involves an infinite number of operations and becomes unfeasible. In [36], based on a coherent state formalism, matrix elements of the non-planar dilatation generator between operators dual to particular folded spinning strings were calculated but an explicit diagonalization of the non-planar dilatation generator for the situation in question did not seem tractable.

## 2.4 Comparison to string theory

In order to generate string theory data with which to compare non-planar corrections to anomalous dimensions one needs to take into account string loop corrections corresponding to considering string world-sheets of higher genus. For short operators such a comparison is currently out of sight since we do not even have any examples of a successful comparison at the planar level, except for certain BPS states which can be shown to have vanishing anomalous dimensions [37]. Recently, it was shown at one-loop order that certain 1/4 BPS states can be labeled by irreducible representations of the Brauer algebra [38], see also [39].

The situation is slightly more encouraging in the case of BMN operators. Considering the BMN limit on the gauge theory side corresponds on the string theory side to taking the Penrose limit of the  $AdS_5 \times S^5$  background which turns the geometry into a PP-wave. On the PP-wave one can quantize the free IIB string theory in light cone gauge and find the corresponding free spectrum. In addition, considering higher genus effects

is possible by means of light cone string field theory (LCSFT). A review of the PP-wave/BMN correspondence including an introduction to LCSFT can be found in the references [40, 41]. In LCSFT string interactions are described in terms of a three-string vertex which encodes the information about the splitting and joining of strings. There seems to be several ways of consistently defining this three-string vertex and there exist at least three proposals for its exact form. For all proposals, however, it holds that there is a freedom of choosing a certain pre-factor of the vertex. Reference [42] constitutes the most recent review of this topic describing the different possible choices of the three-vertex and containing all the relevant references. Furthermore, the authors of [42] show that the one-loop gauge theory result (2.12) can be obtained from LCSFT provided one chooses one particular of the proposed vertices and chooses its pre-factor in a specific way.<sup>4</sup> It is, however, not possible to recover the two-loop gauge theory result from the LCSFT and generically LCSFT gives rise to half-integer powers of  $\lambda'$  appearing in the expressions for non-planar anomalous dimensions. Such half-integer powers of  $\lambda'$  were also found in the analysis of worldsheet one-loop corrections to the planar energies of spinning strings [43] and eventually led to the recognition that the BMN expansion breaks down not only at strong coupling but also at weak coupling starting at four-loop order [44, 26, 45]. Hence, it appears that in order to obtain complete agreement between gauge and string theory we are forced to consider the full  $AdS_5 \times S^5$  geometry.

Finally, in the case of operators dual to spinning strings no direct comparison between gauge theory and string theory has been possible. In reference [22] the decay of a single folded spinning string into two such strings was studied in a semi-classical approximation and a certain relation between the conserved charges of the decay products was found. If the semi-classical decay channel were the dominant one, as it is known to be in flat space, one could hope that the matrix elements for string splitting and joining found in [36] could encode some similar relation. The analysis of [36], however, did not point towards the semi-classical decay channel being the dominant one.

### 3 Multi-point functions

By multi-point functions we mean correlation functions of the following type

$$\langle \mathcal{O}_{\Delta_1}(x_1) \mathcal{O}_{\Delta_2}(x_2) \dots \mathcal{O}_{\Delta_n}(x_n) \rangle, \quad (3.1)$$

where the operators involved are eigenstates of the dilatation generator and carry the conformal dimensions  $\Delta_1, \Delta_2, \dots, \Delta_n$ . Three-point functions play a particular role since their form is fixed by conformal invariance and since they contain the information about the structure constants  $C_{ijk}$  which appear in the theory's operator product expansion. For appropriately normalized conformal operators the three-point functions take the form

$$\langle \mathcal{O}_{\Delta_1}(x_1) \mathcal{O}_{\Delta_2}(x_2) \mathcal{O}_{\Delta_3}(x_3) \rangle = \frac{C_{\Delta_1 \Delta_2 \Delta_3}}{(x_1 - x_2)^{\Delta - 2\Delta_3} (x_2 - x_3)^{\Delta - 2\Delta_1} (x_3 - x_1)^{\Delta - 2\Delta_2}}, \quad (3.2)$$

---

<sup>4</sup>It should be noticed, though, that the match to the one-loop gauge theory result is obtained after a truncation to the so-called impurity conserving channel while at the same time it is proved that generically all channels would contribute to the result. In addition, it is pointed out that an undetermined supercharge could potentially also contribute to the result.

where  $\Delta = \Delta_1 + \Delta_2 + \Delta_3$ .

### 3.1 Results on multi-point functions

Before the advent of the BMN paper in 2002 [32] results on multi-point functions mostly had to do with protected versions of these. A nice review and a complete list of references can be found in [46]. Here we will only very briefly list the pre-BMN results. First, two- and three- point functions of 1/2 BPS and 1/4 BPS operators do not renormalize. Secondly, a large class of multi-point functions of 1/2 BPS operators have very simple renormalization properties. These are the so-called extremal, next-to-extremal and near extremal correlators. Extremal correlators fulfill that  $\Delta_1 = \Delta_2 + \dots + \Delta_n$  and can always be expressed entirely in terms of two-point functions. Next-to-extremal correlators obey  $\Delta_1 = \Delta_2 + \dots + \Delta_n - 2$  and factorize into a product of  $n - 3$  two-point functions and one three-point function. Finally, near extremal multi-point functions have the property that  $\Delta_1 = \Delta_2 + \dots + \Delta_n - 2m$ , where  $2 \leq m \leq n - 3$  and  $4 \leq \Delta_1 \leq 2n - 2$ . These multi-point functions can all be expressed in terms of lower point functions. The results on multi-point functions, briefly reviewed here, can also be understood from the string theory side [46].

With the advent of the BMN limit [32] the focus was shifted from BPS operators to near BPS operators or BMN operators. As mentioned above these are operators which are created from long BPS operators by the insertion of a few impurities. A much studied set of BMN operators belonging to the  $SO(6)$  sector are the following ones

$$\mathcal{O}_{ij,n}^J = \frac{1}{\sqrt{JN^{J+2}}} \left( \sum_{p=0}^n e^{\frac{2\pi i n p}{J}} \text{Tr}(\Phi_i Z^p \Phi_j Z^{J-p}) - \delta_{ij} \text{Tr}(\bar{Z} Z^{J+1}) \right), \quad (3.3)$$

where  $Z$  is one of the three complex scalars of  $\mathcal{N} = 4$  SYM, say  $Z = \Phi_1 + i\Phi_2$ , and  $i, j \in \{3, 4, 5, 6\}$ . These operators are determined by the requirement that they should be eigenvectors of the one-loop planar dilatation operator [32] in the limit  $J \rightarrow \infty$ . (For the exact finite  $J$  version of (3.3), see [47].) They can be organized into representations of  $SO(6)$  in the obvious way. The calculation of three-point functions of non-protected operators such as BMN operators necessitates a highly non-trivial resolution of operator mixing. First, in the case of extremal correlators, in order to calculate the classical three-point function to leading order in  $1/N$  one needs to take into account mixing between single and double trace states [48]. For BMN operators this calculation was carried out in reference [8, 34] with the following result for the space-time independent part of the three-point functions involving two BMN operators and one 1/2 BPS operator of the form  $\mathcal{O}^J = \frac{1}{\sqrt{JN^J}} \text{Tr}(Z^J)$ .

$$\langle \bar{\mathcal{O}}_{ij,n}^J \mathcal{O}_{kl,m}^{r \cdot J} \mathcal{O}^{(1-r) \cdot J} \rangle = \frac{2 J^{3/2} \sqrt{1-r} \sin^2(\pi n r)}{N \sqrt{r} \pi^2 (n^2 - m^2/r^2)^2} \left( 1 - \frac{\lambda(n^2 - m^2/r^2)}{2J^2} \right) \times \left( \delta_{i(k} \delta_{l)j} n^2 + \delta_{i[k} \delta_{l]j} \frac{nm}{r} + \frac{1}{4} \delta_{ij} \delta_{kl} \frac{m^2}{r^2} \right), \quad (3.4)$$

where it is understood that the operators appearing on the left hand side of (3.4) have

been redefined to take into account the effects of the just mentioned operator mixing.<sup>5</sup> To determine the order  $\lambda$  correction to the structure constants requires a number of considerations. First, one actually has to resolve the operator mixing problem to two loop order [31], see also the discussion in [51] as well as the remarks in [8, 34]. The reason is that whereas the diagonalization of the dilatation generator to one-loop order does not introduce any coupling constant dependent mixing of the states this is not so at two-loop order. At one-loop order one has a set of states  $\{\mathcal{O}_\alpha\}$  which are simultaneously eigenstates at the classical and one-loop level. However, when two-loop corrections are taken into account these eigenstates are changed to  $\{\mathcal{O}_\alpha + \lambda c_{\alpha\beta} \mathcal{O}_\beta\}$ . The coupling constant dependent modification of the states which occur at two-loop level gives contributions to the structure constants of order  $\lambda$ . Finally, one of course has to ensure that the structure constants one reads off from the three-point functions are renormalization scheme independent. This can be achieved by normalizing the two-point functions of the operators involved to unity at order  $\lambda$ , see discussion in [51].

The early papers which dealt with three-point functions ignored either one or both the two complications from operator mixing, i.e. the mixing with multi-trace states and the mixing which naively appears to be of higher order. References [52] dealt with the second type of mixing phenomenon and suggested to solve it using purely algebraic means, hence avoiding the explicit evaluation of higher loop two-point functions. References [53, 54, 51] which studied one-loop properties of structure constants did not take into account any of the two above mentioned mixing issues. However, these references pointed out certain connections of three-point functions to integrable spin chains which we will review below together with some very recent progress along the same lines [55].

### 3.2 Multi-point functions and integrability

As explained above calculating three-point functions involves first dealing with a subtle mixing problem and secondly executing the Wick contractions between the appropriate eigenstates. We will follow the historical development and postpone the discussion of the mixing problem to the end of this section.

For one-loop three-point functions of scalar operators one has tried to derive a kind of effective vertex which when applied to the three operators involved gives the order  $\lambda$  contribution to the structure constant [53, 51]. When evaluating three-point functions (apart from non-extremal ones) one generically encounters two types of Feynman diagrams. One type is two-point-like involving only non-trivial contractions between fields from two of the three operators appearing in the three-point function whereas the other type involves non-trivial contractions between fields from all three operators. The generic term of the effective vertex of [51] correspondingly acts on the indices of three different operators. However, one can show that in a certain renormalization scheme the one-loop correction to the structure constant only obtains contributions from Feynman diagrams which are two-point-like [53] and therefore it is possible to construct an effective vertex whose terms act at most on indices from two different operators at a time [53]. Both

---

<sup>5</sup>Notice that in references [49, 10, 50] where classical three-point functions of BMN operators also appear the contribution to the three-point function from the mixing with double trace states was *not* taken into account.

of the resulting effective vertices have a close resemblance to the Hamiltonian of the integrable  $SO(6)$  spin chain. Notice, however, that both approaches [53, 51] ignore the two particular mixing issues discussed in the previous section.

An approach to the calculation of three-point functions which explicitly exploits the integrability of the planar dilatation generator was presented in reference [54]. Here the field theoretic three-point functions are represented as matrix elements of certain spin operators of the integrable spin chain determining the spectrum and it is shown how these matrix elements can in principle be expressed in terms of the elements of the spin chain's monodromy matrix. The method does not allow one to resolve the mixing between single and multi-trace operators, however.

More recently, it was understood how, for a certain subclass of operators, the mixing due to one-loop corrections and the calculation of tree-level three-point functions could be efficiently dealt with using integrability tools having their origin in the planar integrability of the theory and this led to exact results for a class of tree-level structure constants [55]. Furthermore, combining these tools with the ideas of [54] a wealth of new data on one-loop three-point functions for short operators was obtained [55]. Notice again that these studies are restricted to cases without mixing between single and multi-trace operators. Reference [56] also contains extensive data on one-loop three-point functions for short operators but here even the single trace mixing problem was not fully resolved for all cases.

### 3.3 Comparison to string theory

Given the success of the comparison of the anomalous dimensions of gauge theory operators with the energies of string states it is natural to look for a representation of the structure constants entering the three-point functions of non-protected operators in terms of string theory quantities. With the discovery of the pp-wave limit of the type IIB string theory and the corresponding BMN limit of  $\mathcal{N} = 4$  SYM hope was raised that in this limit the AdS/CFT dictionary could be extended to include the structure constants of the gauge theory and a first proposal for the translation of these into string theory was put forward in [10]. Here some structure constants  $C_{ijk}$  were suggested to be related in a simple way to the matrix elements of the three-string vertex of the light cone string field theory. A lot of debate followed this initial proposal. First of all it was debated whether the  $C_{ijk}$  were supposed to be the true CFT structure constants appearing after taking into account the two types of operator mixing discussed in section 3.1 or if the translation to string theory would not involve this mixing. Secondly, as mentioned in section 2.4 the exact form of the three-string vertex of LCSFT was also a subject of debate. The status of the discussion by the end of 2003 is well summarized in the review [41]. In 2004 reference [57] provided a unifying description of the various earlier approaches. The true LCSFT vertex was argued to be a linear combination of the two earlier proposed ones and the  $C_{ijk}$ 's of relevance for the comparison between gauge and string theory were argued to be the true CFT structure constants. The precise translation of the gauge theory structure constants to the string theory language is well explained in [58]. All this should, however, be taken with some caution, as it has been understood that only for the full AdS/CFT system can one hope for a complete matching of string and gauge

theory, cf. the discussion in section 2.4.

In the past year there has been quite some progress in the calculation of two- and three-point correlation functions of string states in the full  $AdS_5 \times S^5$  geometry using semi-classical methods. First, in [59] (see also [60]) a semi-classical approach was shown to reproduce the characteristic conformal scaling of the two-point function with the energy for spinning strings with large quantum numbers and it was suggested that a similar approach could be applied to three point functions. In [61] the semi-classical calculation of two-point functions was formulated in terms of vertex operators describing classical spinning strings [62]. Subsequently, the semi-classical approach was extended to the calculation of three-point functions involving two heavy states and one BPS state [63] and various cases of this type were considered [64]. Furthermore, using the vertex operator representation of the correlation functions a number of three-point functions between two heavy states and one light non-BPS state was determined [65]. So far an explicit comparison of the string theory three-point functions discussed here and gauge theory three point functions has only been possible for protected correlators. However, very recently it has been suggested that an expansion of the string theory three-point functions in a large angular momentum of the heavy states might allow for a comparison with a gauge theory perturbative expansion of the same quantity, at least for the first few loop orders [66].

## 4 Maldacena-Wilson loops

Wilson loops constitute an important class of gauge invariant non-local observables in any gauge theory. The idea that Wilson loops should have a dual string representation has a long history, see [67] and references therein. A realization of this idea in the context of the AdS/CFT correspondence was obtained by Maldacena who introduced the following special type of locally supersymmetric Wilson loops [68]

$$W[C] = \frac{1}{\dim(\mathcal{R})} \text{Tr}_{\mathcal{R}} \left( \text{P exp} \left[ \oint_C d\tau (iA_\mu(x)\dot{x}^\mu + \Phi_i(x)\theta^i|\dot{x}|) \right] \right). \quad (4.1)$$

Here  $\mathcal{R}$  denotes an irreducible representation of  $SU(N)$ ,  $x^\mu(\tau)$  is a parametrization of the loop  $C$ ,  $\Phi_i(x)$  are the 6 real scalar fields of  $\mathcal{N} = 4$  SYM and  $\theta_i(\tau)$  is a curve on  $S^5$ . In the present section we will use the following definition of the 't Hooft coupling constant

$$\lambda = g_{\text{YM}}^2 N. \quad (4.2)$$

According to Maldacena [68] the expectation value of such a Wilson loop in the fundamental representation should be determined by the action of a string ending at the curve  $C$  at the boundary of  $AdS_5$ , i.e.

$$\langle W[C] \rangle = \int_{\partial X=C} \mathcal{D}X \exp \left( -\sqrt{\lambda} S[X] \right). \quad (4.3)$$

Expectation values of many supersymmetric Wilson loops have turned out to be expressible in terms of expectation values in integrable zero-dimensional matrix models. Furthermore, Wilson loops have provided us with the most promising test of the AdS/CFT

correspondence beyond the planar limit to date. The relation between Maldacena-Wilson loops and spin chain integrability is so far rather sparse, cf. subsection 4.4.

## 4.1 The 1/2 BPS line and circle

A Wilson loop in form of a single straight line, i.e. given by  $x(\tau) = \tau$ ,  $\theta^i(\tau) = \text{const}$ , constitutes a 1/2 BPS object. Its expectation value does not get any quantum corrections and is exactly equal to one. The circular Wilson loop parametrized by

$$x(\tau) = (\cos \tau, \sin \tau, 0, 0), \quad (4.4)$$

and  $\theta^i(\tau) = \text{const}$  can be obtained from the straight line by a conformal transformation and is likewise 1/2 BPS. Its expectation value does get quantum corrections, however. The expectation value of the circular Wilson loop was calculated at the planar level in perturbation theory to two loop order in [69] and it was found that only ladder like diagrams (i.e. diagrams whose vertices all lie on the loop) contributed. The authors of [69] proposed that this could be true to all orders and showed that under that assumption the calculation of the expectation value could be reduced to a combinatorial problem the answer to which was given by an expectation value in a zero-dimensional Gaussian matrix model. Subsequently, it was understood that the reason why the problem was zero-dimensional in nature was that the expectation value of the circular Wilson loop could be understood as an anomaly arising at the point at infinity when conformally mapping the straight line to a circle [70]. In addition, the proposal of [69] was extended to all orders in the  $\frac{1}{N}$ -expansion [70]. Stated precisely, the proposal says that the expectation value of the circular Wilson loop is given to all orders in  $\lambda$  and all orders in  $\frac{1}{N}$  by the following expression <sup>6</sup>

$$\langle W_{circle} \rangle = \left\langle \frac{1}{N} \text{Tr} (\exp(M)) \right\rangle = \frac{1}{Z} \int \mathcal{D}M \frac{1}{N} \text{Tr} (\exp(M)) \exp \left( -\frac{2N}{\lambda} \text{Tr} M^2 \right). \quad (4.5)$$

Using matrix model techniques the expectation value can be calculated *exactly* and yields [70]

$$\langle W_{circle} \rangle = \frac{1}{N} L_{N-1}^1(-\lambda/4N) \exp(\lambda/8N), \quad (4.6)$$

where  $L_{N-1}^1$  is a Laguerre polynomial. One can explicitly write down the genus expansion of (4.6) and then taking the strong coupling,  $\lambda \rightarrow \infty$ , limit of this one gets

$$\langle W_{circle} \rangle = \sum_{p=0}^{\infty} \frac{1}{N^{2p}} \frac{e^{\sqrt{\lambda}}}{p!} \sqrt{\frac{2}{\pi}} \frac{\lambda^{\frac{6p-3}{4}}}{96^p} \left[ 1 - \frac{3(12p^2 + 8p + 5)}{40\sqrt{\lambda}} + \mathcal{O}\left(\frac{1}{\lambda}\right) \right]. \quad (4.7)$$

The possibility of the expectation value getting additional contributions from instantons was investigated in [71]. Recently, however, the proposal of [69, 70] was proved to be true [72].

---

<sup>6</sup>Here the integration is over Hermitian matrices, i.e.  $\mathcal{D}M = \prod_i dM_{ii} \prod_{j>i} d\Re(M_{ij}) d\Im(M_{ij})$  and  $Z$  is the partition function of the model.

The expectation value of the circular Wilson loop can be found from the string theory recipe (4.3) in the strong coupling limit by performing a saddle point analysis. It turns out that the string action is dominated by its bosonic part at the saddle point and the calculation becomes equivalent to determining the area of the minimal area surface ending at the loop  $C$ . The minimal surface area, however, diverges and requires a regularization which results in the saddle point action being negative [68]. The minimal area corresponding to the circle was first determined in [73] and led to the first crude estimate of the expectation value of the planar circular Wilson loop from the string theory side  $\langle W_{circle} \rangle^{string} \sim e^{\sqrt{\lambda}}$ . Later the string analysis was extended to include sub-leading corrections in  $\lambda$  coming from integration over zero-modes and to include higher genus surfaces [70]. This led to the following string theory estimate of the expectation of the circular Wilson loop

$$\langle W_{circle} \rangle^{string} \propto \sum_{p=0}^{\infty} \frac{1}{N^{2p}} \frac{e^{\sqrt{\lambda}}}{p!} \lambda^{\frac{6p-3}{4}} \left[ 1 + \mathcal{O}\left(\frac{1}{\sqrt{\lambda}}\right) \right]. \quad (4.8)$$

The matching between (4.7) and (4.8) provides a piece of evidence in favour of the validity of the AdS/CFT correspondence beyond the planar level. In order to reproduce the additional factor  $\sqrt{\frac{2}{\pi}}$  appearing in (4.7) from string theory one needs to take into account the fluctuations about the minimal surface. The framework for performing this calculation at the planar level was laid out in [74] and recently interesting progress was achieved in the explicit evaluation of the missing sub-leading contribution in the planar case [75].

## 4.2 More supersymmetric Wilson loops

In reference [76] Zarembo found a series of Wilson loops of 1/4, 1/8 and 1/16 BPS type which can be viewed as generalizations of the 1/2 BPS Wilson line living in the higher dimensional subspaces  $\mathbb{R}^2$ ,  $\mathbb{R}^3$  and  $\mathbb{R}^4$ . These Wilson loops all have trivial expectation values. This was argued from the gauge theory side in [76, 77] and an understanding from the string theory perspective was provided in [78]. Finally, it was explained by topological arguments in [79].

The first example of a 1/4 BPS Wilson loop with non-trivial expectation value was found by Drukker [80]. Later a large family of supersymmetric Wilson loops with non-trivial expectation values was identified [81, 82]. This family of loops constitute generalizations of the 1/2 BPS circular loop above. The most generic type is 1/16 BPS and lives on an  $S^3$  sub-manifold of four-dimensional space-time. Loops further restricted to an  $S^2$  are 1/8 BPS and their expectation values were conjectured to be equal to the analogous expectation values in the zero instanton sector of two-dimensional Yang-Mills theory on a sphere [82] which implies that they can again be evaluated using a matrix model. More precisely, for such loops we should have

$$\langle W[C] \rangle = \frac{1}{N} L_{N-1}^1 \left( g_{\text{YM}}^2 \frac{\mathcal{A}_1 \mathcal{A}_2}{\mathcal{A}^2} \right) \exp \left[ -\frac{g_{\text{YM}}^2}{2} \frac{\mathcal{A}_1 \mathcal{A}_2}{\mathcal{A}^2} \right], \quad (4.9)$$

where  $\mathcal{A}_1$  and  $\mathcal{A}_2$  are the two areas of the sphere bounded by the loop and  $\mathcal{A} = \mathcal{A}_1 + \mathcal{A}_2 = 4\pi$ . Perturbative gauge theory arguments supporting the conjecture were presented in [82, 83] and string theoretic arguments in favour of the conjecture appeared in [84]. The conjecture was further supported by studies using localization techniques in [85].

A unifying and exhaustive description of all supersymmetric Wilson loops was given in [86] and it was found that the two classes of Wilson loops described by respective Zarembo and Drukker et al. are indeed the two most natural ones.

Some aspects of the analysis outlined above have been generalized to  $\mathcal{N} = 6$  supersymmetric Chern-Simons matter theory. The 1/2 BPS Wilson loop has been constructed [87] and its expectation value shown to be expressible in terms of an expectation value in a zero-dimensional supermatrix model [88, 87]. In addition, one has identified a 1/6 BPS Wilson loop [89] whose expectation value can likewise be calculated using a matrix model [88, 90].

### 4.3 Higher representations

Having obtained the result (4.5) and using the Schur polynomial formula one has access to the expectation value of the 1/2 BPS circular Wilson loop in any given irreducible representation of  $SU(N)$ . When the rank of the representation,  $k$ , i.e. the number of boxes in the Young tableau, fulfills that  $k \sim \mathcal{O}(N)$  the appropriate string theory description of the Wilson loop is in terms of Dp-branes rather than fundamental strings. Early ideas in this direction were presented in [91, 92]. The precise dictionary between Wilson loops in higher representations and Dp-branes was found in [93]. A Wilson loop operator in a representation given by a Young diagram with  $M$  rows and  $K$  columns with  $n_i$  boxes in the  $i$ 'th row and  $m_j$  boxes in the  $j$ 'th column has two different string realizations. One is in terms of  $K$  D3-branes carrying electric charges  $n_1, \dots, n_K$  and the other is in terms of  $M$  D5-branes carrying electric charges  $m_1, \dots, m_M$ . In both cases, as long as  $k \ll N^2$ , one should be able to determine the expectation value of the Wilson loop by treating the Dp-brane using the probe approximation, i.e. ignoring the back reaction of the  $AdS_5 \times S^5$  geometry.<sup>7</sup>

For the completely symmetric and the completely antisymmetric representation of rank  $k$  the gauge theory expectation value of the 1/2 BPS circular Wilson loop has been extracted from the matrix model in the limit  $N \rightarrow \infty$ ,  $k \rightarrow \infty$  with  $k/N$  fixed using saddle point techniques. In the antisymmetric case the result in the large  $\lambda$  limit reads [96]

$$\langle W_{A_k}(C) \rangle = \exp \left[ \frac{2N}{3\pi} \sqrt{\lambda} \sin^3 \theta_k \right], \quad (4.10)$$

where  $\theta_k$  is given by

$$\pi \left( 1 - \frac{k}{N} \right) = (\theta_k - \sin(\theta_k) \cos(\theta_k)). \quad (4.11)$$

<sup>7</sup> In particular, it is expected that energies of certain spinning D3- and D5-branes correspond to anomalous dimensions of local twist operators (cf. the chapter [94]) carrying higher representations of the gauge group [95].

This result matches the result of a supergravity calculation on the string theory side using D5-brane probes [97]. For the completely symmetric representation the situation is more involved since in the large  $N$  analysis one encounters two different saddle points. Which one dominates depends on the precise values of  $\lambda$  and  $k/N$ . If one considers the limit of large  $\lambda$  and  $N$  with a fixed value of  $\kappa$ , defined by

$$\kappa = \frac{\sqrt{\lambda}k}{4N}, \quad (4.12)$$

one finds [96, 98]

$$\langle W_{S_k}^{(1)}[C] \rangle = \exp \left[ 2N \left( \kappa \sqrt{1 + \kappa^2} + \sinh^{-1}(\kappa) \right) \right]. \quad (4.13)$$

This result matches a supergravity calculation carried out using D3-brane probes [92]. The same saddle point dominates in the limit  $\lambda \rightarrow \infty$ ,  $k \rightarrow \infty$ ,  $N \rightarrow \infty$  with  $k/N$  fixed. In other regions of the parameter space the second saddle point might come into play and in general one has that the expectation value of the Wilson loop in the symmetric representation is a sum of two terms, i.e.  $W_{S_k}[C] = W_{S_k}^{(1)}[C] + W_{S_k}^{(2)}[C]$ .

When the rank of the representation reaches the size  $k \sim \mathcal{O}(N^2)$  the probe approximation breaks down as the back reaction of the  $AdS_5 \times S^5$  geometry can no longer be ignored. In this case the resulting string background can be described as a bubbling geometry [99]. The determination of the bubbling geometry corresponding to 1/2 BPS Wilson loops was initiated in [100] and completed in [101]. The calculation of the expectation value of the Wilson loop from the gauge theory side still proceeds via the matrix model and was carried out in [102].

Like the 1/2 BPS Wilson loop the less supersymmetric Wilson loops can be studied in higher representations of the gauge group. This was done for a number of 1/4 BPS Wilson loops in [103]. There also exist numerous results on correlation functions involving multiple Wilson loops as well as Wilson loops and local operators for loops in various representations.

#### 4.4 Other instances of integrability of Wilson loops

As explained in section 4.1 expectation values of Wilson loops in the strong coupling,  $\lambda \rightarrow \infty$  limit can be evaluated by finding a classical string solution with appropriate boundary conditions. The string sigma model describing type IIB strings on  $AdS_5 \times S^5$  is known to be classically integrable [3] and this fact was exploited in reference [104] to find the strong coupling expectation values of numerous Wilson loops with  $x^\mu(t)$  and  $\theta^i(t)$  periodic. More recently a class of polygonal (non-supersymmetric) Wilson loops built from light like segments have attracted attention due to their relation with gluon scattering amplitudes [105]. The minimal surfaces corresponding to these loops have turned out to be described by integrable systems of Hitchin type. For a discussion of Wilson loops related to scattering amplitudes and the relevant set of references we refer to the chapters [6].

It seems difficult to relate the expectation value of supersymmetric Wilson loops to integrable spin chains but there exists one special construction which exposes such a

relation. In reference [106] the authors studied insertion of composite operators into Wilson loops. The Wilson loop was taken to be a straight line or a circle and  $\theta^i$  to describe a single point on  $S^5$ . Furthermore, the composite operator was assumed to be built from two complex scalars  $Z = (\Phi_1 + i\Phi_2)/\sqrt{2}$  and  $X = (\Phi_3 + i\Phi_4)/\sqrt{2}$ . It is possible to assign a conformal dimension to such an inserted operator and to determine this dimension one has to solve a certain mixing problem involving two-point functions of the type

$$\langle W_{line} [\mathcal{O}_\beta^\dagger(t)\mathcal{O}_\alpha(0)] \rangle = \langle \frac{1}{N} \text{Tr} \left( P \mathcal{O}_\alpha^\dagger(t)\mathcal{O}_\beta(0) \exp \left[ i \int (A_t + i\Phi_6) dt \right] \right) \rangle. \quad (4.14)$$

An operator insertion  $\mathcal{O}_\Delta$  with a well-defined conformal dimension fulfills

$$\langle W_{line} [\mathcal{O}_\Delta^\dagger(t)\mathcal{O}_\Delta(0)] \rangle \sim \frac{1}{t^{2\Delta}}. \quad (4.15)$$

The above mixing problem was studied at the planar one-loop order in [106] and mapped onto the problem of diagonalising the Hamiltonian of an  $SU(2)$  open Heisenberg spin chain with completely reflective boundary conditions. This spin chain is integrable and can be solved by Bethe ansatz. For a description of the Bethe equations associated with integrable open spin chains, we refer to the chapter [4]. The string dual of the inserted operator can be identified and a successful comparison between the gauge theory side and string theory side for inserted operators of BMN type and of the type dual to spinning strings was carried out in [106].

## 5 Conclusion

The search for spin chain like integrable structures in  $\mathcal{N} = 4$  SYM regarding non-planar anomalous dimensions and Maldacena-Wilson loops has so far not provided us with very strong positive results. Maldacena-Wilson loops are more naturally related to zero-dimensional integrable matrix models than to spin chains and non-planar anomalous dimensions have not yet provided us with any traces of integrability. It is possible that one can learn more about non-planar anomalous dimensions by studying the three-point functions or structure constants of the theory. Non-trivial operator mixing issues, however, make the evaluation of structure constants quite involved. For a subset of single trace operators the mixing is an entirely planar effect and can in principle be handled using tools originating from the planar integrability of the theory. In the generic case, however, single trace operators will mix with multi-trace operators and the calculation of structure constants requires a diagonalization of the non-planar dilatation operator. The most naive approach to studying non-planar anomalous dimensions, namely doing perturbation theory in  $\frac{1}{N}$  requires dealing with the splitting and joining of spin-chains and leads to a Hilbert space of states for which the standard concepts of integrability such as the asymptotic S-matrix and two-particle scattering do not immediately apply. Going beyond the planar limit hence seems to require a rethinking of the entire framework of integrability or invoking some non-perturbative way of handling the higher topologies.

**Acknowledgments:** I am grateful to N. Beisert, N. Drukker, C. Sieg, A. Tseytlin, D.

Young and K. Zoubos for useful discussions and comments during the writing of this review. This work was supported by FNU through grant number 272-08-0329.

## References

- [1] J. A. Minahan and K. Zarembo, “*The Bethe-ansatz for  $\mathcal{N} = 4$  super Yang-Mills*”, JHEP 0303, 013 (2003), [hep-th/0212208](#).
- [2] N. Beisert, C. Kristjansen and M. Staudacher, “*The dilatation operator of  $\mathcal{N} = 4$  super Yang-Mills theory*”, Nucl. Phys. B664, 131 (2003), [hep-th/0303060](#).
- [3] G. Mandal, N. V. Suryanarayana and S. R. Wadia, “*Aspects of semiclassical strings in  $AdS_5$* ”, Phys. Lett. B543, 81 (2002), [hep-th/0206103](#). • I. Bena, J. Polchinski and R. Roiban, “*Hidden symmetries of the  $AdS_5 \times S^5$  superstring*”, Phys. Rev. D69, 046002 (2004), [hep-th/0305116](#).
- [4] K. Zoubos, “*Review of AdS/CFT Integrability, Chapter IV.2: Deformations, Orbifolds and Open Boundaries*”, [arxiv:1012.3998](#).
- [5] G. Korchemsky, “*Review of AdS/CFT Integrability, Chapter IV.4: Integrability in QCD and  $\mathcal{N} < 4$  SYM*”, [arxiv:1012.4000](#).
- [6] R. Roiban, “*Review of AdS/CFT Integrability, Chapter V.1: Scattering Amplitudes – a Brief Introduction*”, [arxiv:1012.4001](#). • J. M. Drummond, “*Review of AdS/CFT Integrability, Chapter V.2: Dual Superconformal Symmetry*”, [arxiv:1012.4002](#). • L. F. Alday, “*Review of AdS/CFT Integrability, Chapter V.3: Scattering Amplitudes at Strong Coupling*”, [arxiv:1012.4003](#).
- [7] C. Sieg, “*Review of AdS/CFT Integrability, Chapter I.2: The spectrum from perturbative gauge theory*”, [arxiv:1012.3984](#).
- [8] N. Beisert, C. Kristjansen, J. Plefka, G. W. Semenoff and M. Staudacher, “*BMN correlators and operator mixing in  $\mathcal{N} = 4$  super Yang-Mills theory*”, Nucl. Phys. B650, 125 (2003), [hep-th/0208178](#).
- [9] N. Beisert, C. Kristjansen, J. Plefka and M. Staudacher, “*BMN gauge theory as a quantum mechanical system*”, Phys. Lett. B558, 229 (2003), [hep-th/0212269](#).
- [10] N. R. Constable et al., “*PP-wave string interactions from perturbative Yang-Mills theory*”, JHEP 0207, 017 (2002), [hep-th/0205089](#).
- [11] N. Beisert, “*The complete one-loop dilatation operator of  $\mathcal{N} = 4$  super Yang-Mills theory*”, Nucl. Phys. B676, 3 (2004), [hep-th/0307015](#).
- [12] B. I. Zwiebel, “ *$\mathcal{N} = 4$  SYM to two loops: Compact expressions for the non-compact symmetry algebra of the  $su(1,1/2)$  sector*”, JHEP 0602, 055 (2006), [hep-th/0511109](#).
- [13] Z. Xiao, “*BMN operators with a scalar fermion pair and operator mixing in  $\mathcal{N} = 4$  Super Yang-Mills Theory*”, Phys. Rev. D81, 026004 (2010), [arxiv:0910.3390](#).
- [14] G. De Risi, G. Grignani, M. Orselli and G. W. Semenoff, “*DLCQ string spectrum from  $\mathcal{N} = 2$  SYM theory*”, JHEP 0411, 053 (2004), [hep-th/0409315](#).
- [15] O. Aharony, O. Bergman, D. L. Jafferis and J. Maldacena, “ *$\mathcal{N} = 6$  superconformal Chern-Simons-matter theories, M2-branes and their gravity duals*”, JHEP 0810, 091 (2008), [arxiv:0806.1218](#).

- [16] O. Aharony, O. Bergman and D. L. Jafferis, “*Fractional M2-branes*”, JHEP 0811, 043 (2008), [arxiv:0807.4924](#).
- [17] C. Kristjansen, M. Orselli and K. Zoubos, “*Non-planar ABJM Theory and Integrability*”, JHEP 0903, 037 (2009), [arxiv:0811.2150](#).
- [18] P. Caputa, C. Kristjansen and K. Zoubos, “*Non-planar ABJ Theory and Parity*”, Phys. Lett. B677, 197 (2009), [arxiv:0903.3354](#).
- [19] R. Janik, “*Review of AdS/CFT Integrability, Chapter III.5: Lüscher corrections*”, [arxiv:1012.3994](#). • Z. Bajnok, “*Review of AdS/CFT Integrability, Chapter III.6: Thermodynamic Bethe Ansatz*”, [arxiv:1012.3995](#). • V. Kazakov and N. Gromov, “*Review of AdS/CFT Integrability, Chapter III.7: Hirota Dynamics for Quantum Integrability*”, [arxiv:1012.3996](#).
- [20] C. Sieg and A. Torrielli, “*Wrapping interactions and the genus expansion of the 2-point function of composite operators*”, Nucl. Phys. B723, 3 (2005), [hep-th/0505071](#).
- [21] S. Bellucci, P. Y. Casteill, J. F. Morales and C. Sochichiu, “*Spin bit models from non-planar  $\mathcal{N} = 4$  SYM*”, Nucl. Phys. B699, 151 (2004), [hep-th/0404066](#).
- [22] K. Peeters, J. Plefka and M. Zamaklar, “*Splitting spinning strings in AdS/CFT*”, JHEP 0411, 054 (2004), [hep-th/0410275](#).
- [23] P. Caputa, C. Kristjansen and K. Zoubos, “*On the spectral problem of  $\mathcal{N}=4$  SYM with orthogonal or symplectic gauge group*”, JHEP 1010, 082 (2010), [arxiv:1005.2611](#).
- [24] D. J. Gross, A. Mikhailov and R. Roiban, “*A calculation of the plane wave string Hamiltonian from  $\mathcal{N} = 4$  super-Yang-Mills theory*”, JHEP 0305, 025 (2003), [hep-th/0208231](#). • R. A. Janik, “*BMN operators and string field theory*”, Phys. Lett. B549, 237 (2002), [hep-th/0209263](#).
- [25] N. Beisert and M. Staudacher, “*Long-range PSU(2,2/4) Bethe ansatzes for gauge theory and strings*”, Nucl. Phys. B727, 1 (2005), [hep-th/0504190](#).
- [26] N. Beisert, B. Eden and M. Staudacher, “*Transcendentality and crossing*”, J. Stat. Mech. 0701, P021 (2007), [hep-th/0610251](#).
- [27] N. Beisert, R. Hernandez and E. Lopez, “*A crossing-symmetric phase for  $AdS_5 \times S^5$  strings*”, JHEP 0611, 070 (2006), [hep-th/0609044](#).
- [28] A. Doikou and R. I. Nepomechie, “*Parity and Charge Conjugation Symmetries and S Matrix of the XXZ Chain*”, [hep-th/9810034](#).
- [29] R. de Mello Koch, T. K. Dey, N. Ives and M. Stephanou, “*Hints of Integrability Beyond the Planar Limit*”, JHEP 1001, 014 (2010), [arxiv:0911.0967](#).
- [30] S. Penati and A. Santambrogio, “*Superspace approach to anomalous dimensions in  $\mathcal{N} = 4$  SYM*”, Nucl. Phys. B614, 367 (2001), [hep-th/0107071](#). • A. V. Ryzhov, “*Quarter BPS operators in  $\mathcal{N} = 4$  SYM*”, JHEP 0111, 046 (2001), [hep-th/0109064](#). • M. Bianchi, B. Eden, G. Rossi and Y. S. Stanev, “*On operator mixing in  $\mathcal{N} = 4$  SYM*”, Nucl. Phys. B646, 69 (2002), [hep-th/0205321](#).
- [31] G. Arutyunov, S. Penati, A. C. Petkou, A. Santambrogio and E. Sokatchev, “*Non-protected operators in  $\mathcal{N} = 4$  SYM and multiparticle states of  $AdS_5$  SUGRA*”, Nucl. Phys. B643, 49 (2002), [hep-th/0206020](#).

- [32] D. E. Berenstein, J. M. Maldacena and H. S. Nastase, “*Strings in flat space and pp waves from  $\mathcal{N} = 4$  super Yang Mills*”, JHEP 0204, 013 (2002), [hep-th/0202021](#).
- [33] D. Z. Freedman and U. Gursoy, “*Instability and degeneracy in the BMN correspondence*”, JHEP 0308, 027 (2003), [hep-th/0305016](#). • C. Kristjansen, “*Quantum mechanics, random matrices and BMN gauge theory*”, Acta Phys. Polon. B34, 4949 (2003), [hep-th/0307204](#). • P. Gutjahr and J. Plefka, “*Decay widths of three-impurity states in the BMN correspondence*”, Nucl. Phys. B692, 110 (2004), [hep-th/0402211](#).
- [34] N. R. Constable, D. Z. Freedman, M. Headrick and S. Minwalla, “*Operator mixing and the BMN correspondence*”, JHEP 0210, 068 (2002), [hep-th/0209002](#).
- [35] U. Gursoy, “*Vector operators in the BMN correspondence*”, JHEP 0307, 048 (2003), [hep-th/0208041](#).
- [36] P. Y. Casteill, R. A. Janik, A. Jarosz and C. Kristjansen, “*Quasilocality of joining/splitting strings from coherent states*”, JHEP 0712, 069 (2007), [arxiv:0710.4166](#).
- [37] E. D’Hoker, D. Z. Freedman and W. Skiba, “*Field theory tests for correlators in the AdS/CFT correspondence*”, Phys. Rev. D59, 045008 (1999), [hep-th/9807098](#).
- [38] Y. Kimura, “*Quarter BPS classified by Brauer algebra*”, JHEP 1005, 103 (2010), [arxiv:1002.2424](#).
- [39] T. W. Brown, “*Cut-and-join operators and  $\mathcal{N}=4$  super Yang-Mills*”, JHEP 1005, 058 (2010), [arxiv:1002.2099](#).
- [40] A. Pankiewicz, “*Strings in plane wave backgrounds*”, Fortsch. Phys. 51, 1139 (2003), [hep-th/0307027](#). • J. C. Plefka, “*Lectures on the plane-wave string / gauge theory duality*”, Fortsch. Phys. 52, 264 (2004), [hep-th/0307101](#). • M. Spradlin and A. Volovich, “*Light-cone string field theory in a plane wave*”, [hep-th/0310033](#). • D. Sadri and M. M. Sheikh-Jabbari, “*The plane-wave / super Yang-Mills duality*”, Rev. Mod. Phys. 76, 853 (2004), [hep-th/0310119](#).
- [41] R. Russo and A. Tanzini, “*The duality between IIB string theory on pp-wave and  $\mathcal{N} = 4$  SYM: A status report*”, Class. Quant. Grav. 21, S1265 (2004), [hep-th/0401155](#).
- [42] G. Grignani, M. Orselli, B. Ramadanovic, G. W. Semenoff and D. Young, “*AdS/CFT vs. string loops*”, JHEP 0606, 040 (2006), [hep-th/0605080](#).
- [43] N. Beisert and A. A. Tseytlin, “*On quantum corrections to spinning strings and Bethe equations*”, Phys. Lett. B629, 102 (2005), [hep-th/0509084](#).
- [44] B. Eden and M. Staudacher, “*Integrability and transcendentality*”, J. Stat. Mech. 0611, P014 (2006), [hep-th/0603157](#).
- [45] Z. Bern, M. Czakon, L. J. Dixon, D. A. Kosower and V. A. Smirnov, “*The Four-Loop Planar Amplitude and Cusp Anomalous Dimension in Maximally Supersymmetric Yang-Mills Theory*”, Phys. Rev. D75, 085010 (2007), [hep-th/0610248](#).
- [46] E. D’Hoker and D. Z. Freedman, “*Supersymmetric gauge theories and the AdS/CFT correspondence*”, [hep-th/0201253](#).
- [47] N. Beisert, “*BMN operators and superconformal symmetry*”, Nucl. Phys. B659, 79 (2003), [hep-th/0211032](#).

- [48] E. D'Hoker, D. Z. Freedman, S. D. Mathur, A. Matusis and L. Rastelli, “*Extremal correlators in the AdS/CFT correspondence*”, hep-th/9908160.
- [49] C. Kristjansen, J. Plefka, G. W. Semenoff and M. Staudacher, “*A new double-scaling limit of  $\mathcal{N} = 4$  super Yang-Mills theory and PP-wave strings*”, Nucl. Phys. B643, 3 (2002), hep-th/0205033.
- [50] C.-S. Chu, V. V. Khoze and G. Travaglini, “*Three-point functions in  $\mathcal{N} = 4$  Yang-Mills theory and pp-waves*”, JHEP 0206, 011 (2002), hep-th/0206005.
- [51] L. F. Alday, J. R. David, E. Gava and K. S. Narain, “*Structure constants of planar  $\mathcal{N} = 4$  Yang Mills at one loop*”, JHEP 0509, 070 (2005), hep-th/0502186.
- [52] G. Georgiou, V. L. Gili and R. Russo, “*Operator Mixing and the AdS/CFT correspondence*”, JHEP 0901, 082 (2009), arxiv:0810.0499. • G. Georgiou, V. L. Gili and R. Russo, “*Operator mixing and three-point functions in  $\mathcal{N} = 4$  SYM*”, JHEP 0910, 009 (2009), arxiv:0907.1567.
- [53] K. Okuyama and L.-S. Tseng, “*Three-point functions in  $\mathcal{N} = 4$  SYM theory at one-loop*”, JHEP 0408, 055 (2004), hep-th/0404190.
- [54] R. Roiban and A. Volovich, “*Yang-Mills correlation functions from integrable spin chains*”, JHEP 0409, 032 (2004), hep-th/0407140.
- [55] J. Escobedo, N. Gromov, A. Sever and P. Vieira, “*Tailoring Three-Point Functions and Integrability*”, arxiv:1012.2475.
- [56] A. Grossardt and J. Plefka, “*One-Loop Spectroscopy of Scalar Three-Point Functions in planar  $N=4$  super Yang-Mills Theory*”, arxiv:1007.2356.
- [57] S. Dobashi and T. Yoneya, “*Resolving the holography in the plane-wave limit of AdS/CFT correspondence*”, Nucl. Phys. B711, 3 (2005), hep-th/0406225.
- [58] S. Dobashi and T. Yoneya, “*Impurity non-preserving 3-point correlators of BMN operators from pp-wave holography. I: Bosonic excitations*”, Nucl. Phys. B711, 54 (2005), hep-th/0409058.
- [59] R. A. Janik, P. Surowka and A. Wereszczynski, “*On correlation functions of operators dual to classical spinning string states*”, JHEP 1005, 030 (2010), arxiv:1002.4613.
- [60] S. Dobashi, H. Shimada and T. Yoneya, “*Holographic reformulation of string theory on  $AdS_5 \times S^5$  background in the PP-wave limit*”, Nucl. Phys. B665, 94 (2003), hep-th/0209251. • T. Yoneya, “*Holography in the large  $J$  limit of AdS/CFT correspondence and its applications*”, Prog. Theor. Phys. Suppl. 164, 82 (2007), hep-th/0607046. • A. Tsuji, “*Holography of Wilson loop correlator and spinning strings*”, Prog. Theor. Phys. 117, 557 (2007), hep-th/0606030.
- [61] E. I. Buchbinder and A. A. Tseytlin, “*On semiclassical approximation for correlators of closed string vertex operators in AdS/CFT*”, JHEP 1008, 057 (2010), arxiv:1005.4516.
- [62] A. A. Tseytlin, “*On semiclassical approximation and spinning string vertex operators in  $AdS_5 \times S^5$* ”, Nucl. Phys. B664, 247 (2003), hep-th/0304139. • E. I. Buchbinder, “*Energy-Spin Trajectories in  $AdS_5 \times S^5$  from Semiclassical Vertex Operators*”, JHEP 1004, 107 (2010), arxiv:1002.1716.
- [63] K. Zarembo, “*Holographic three-point functions of semiclassical states*”, JHEP 1009, 030 (2010), arxiv:1008.1059. • M. S. Costa, R. Monteiro, J. E. Santos

- and D. Zoakos, “On three-point correlation functions in the gauge/gravity duality”, JHEP 1011, 141 (2010), [arxiv:1008.1070](#).
- [64] R. Hernandez, “Three-point correlation functions from semiclassical circular strings”, [arxiv:1011.0408](#). • S. Ryang, “Correlators of Vertex Operators for Circular Strings with Winding Numbers in  $AdS_5 \times S^5$ ”, [arxiv:1011.3573](#). • G. Georgiou, “Two and three-point correlators of operators dual to folded string solutions at strong coupling”, [arxiv:1011.5181](#).
- [65] R. Roiban and A. A. Tseytlin, “On semiclassical computation of 3-point functions of closed string vertex operators in  $AdS_5 \times S^5$ ”, [arxiv:1008.4921](#).
- [66] J. G. Russo and A. A. Tseytlin, “Large spin expansion of semiclassical 3-point correlators in  $AdS_5 \times S^5$ ”, [arxiv:1012.2760](#).
- [67] A. M. Polyakov, “String theory and quark confinement”, Nucl. Phys. Proc. Suppl. 68, 1 (1998), [hep-th/9711002](#).
- [68] J. M. Maldacena, “Wilson loops in large  $N$  field theories”, Phys. Rev. Lett. 80, 4859 (1998), [hep-th/9803002](#).
- [69] J. K. Erickson, G. W. Semenoff and K. Zarembo, “Wilson loops in  $\mathcal{N} = 4$  supersymmetric Yang-Mills theory”, Nucl. Phys. B582, 155 (2000), [hep-th/0003055](#).
- [70] N. Drukker and D. J. Gross, “An exact prediction of  $\mathcal{N} = 4$  SUSYM theory for string theory”, J. Math. Phys. 42, 2896 (2001), [hep-th/0010274](#).
- [71] M. Bianchi, M. B. Green and S. Kovacs, “Instantons and BPS Wilson loops”, [hep-th/0107028](#). • M. Bianchi, M. B. Green and S. Kovacs, “Instanton corrections to circular Wilson loops in  $\mathcal{N} = 4$  supersymmetric Yang-Mills”, JHEP 0204, 040 (2002), [hep-th/0202003](#).
- [72] V. Pestun, “Localization of gauge theory on a four-sphere and supersymmetric Wilson loops”, [arxiv:0712.2824](#).
- [73] D. E. Berenstein, R. Corrado, W. Fischler and J. M. Maldacena, “The operator product expansion for Wilson loops and surfaces in the large  $N$  limit”, Phys. Rev. D59, 105023 (1999), [hep-th/9809188](#). • N. Drukker, D. J. Gross and H. Ooguri, “Wilson loops and minimal surfaces”, Phys. Rev. D60, 125006 (1999), [hep-th/9904191](#).
- [74] N. Drukker, D. J. Gross and A. A. Tseytlin, “Green-Schwarz string in  $AdS_5 \times S^5$ : Semiclassical partition function”, JHEP 0004, 021 (2000), [hep-th/0001204](#).
- [75] M. Kruczenski and A. Tirziu, “Matching the circular Wilson loop with dual open string solution at 1-loop in strong coupling”, JHEP 0805, 064 (2008), [arxiv:0803.0315](#).
- [76] K. Zarembo, “Supersymmetric Wilson loops”, Nucl. Phys. B643, 157 (2002), [hep-th/0205160](#).
- [77] Z. Guralnik and B. Kulik, “Properties of chiral Wilson loops”, JHEP 0401, 065 (2004), [hep-th/0309118](#).
- [78] A. Dymarsky, S. S. Gubser, Z. Guralnik and J. M. Maldacena, “Calibrated surfaces and supersymmetric Wilson loops”, JHEP 0609, 057 (2006), [hep-th/0604058](#).
- [79] A. Kapustin and E. Witten, “Electric-magnetic duality and the geometric Langlands program”, [hep-th/0604151](#).

- [80] N. Drukker, “*1/4 BPS circular loops, unstable world-sheet instantons and the matrix model*”, JHEP 0609, 004 (2006), [hep-th/0605151](#).
- [81] N. Drukker, S. Giombi, R. Ricci and D. Trancanelli, “*More supersymmetric Wilson loops*”, Phys. Rev. D76, 107703 (2007), [arxiv:0704.2237](#).
- [82] N. Drukker, S. Giombi, R. Ricci and D. Trancanelli, “*Wilson loops: From four-dimensional SYM to two-dimensional YM*”, Phys. Rev. D77, 047901 (2008), [arxiv:0707.2699](#). • N. Drukker, S. Giombi, R. Ricci and D. Trancanelli, “*Supersymmetric Wilson loops on  $S^3$* ”, JHEP 0805, 017 (2008), [arxiv:0711.3226](#).
- [83] A. Bassetto, L. Griguolo, F. Pucci and D. Seminara, “*Supersymmetric Wilson loops at two loops*”, JHEP 0806, 083 (2008), [arxiv:0804.3973](#). • D. Young, “*BPS Wilson Loops on  $S^2$  at Higher Loops*”, JHEP 0805, 077 (2008), [arxiv:0804.4098](#).
- [84] S. Giombi, V. Pestun and R. Ricci, “*Notes on supersymmetric Wilson loops on a two-sphere*”, JHEP 1007, 088 (2010), [arxiv:0905.0665](#).
- [85] V. Pestun, “*Localization of the four-dimensional  $N=4$  SYM to a two-sphere and 1/8 BPS Wilson loops*”, [arxiv:0906.0638](#).
- [86] A. Dymarsky and V. Pestun, “*Supersymmetric Wilson loops in  $N=4$  SYM and pure spinors*”, JHEP 1004, 115 (2010), [arxiv:0911.1841](#).
- [87] N. Drukker and D. Trancanelli, “*A supermatrix model for  $\mathcal{N}=6$  super Chern-Simons-matter theory*”, JHEP 1002, 058 (2010), [arxiv:0912.3006](#).
- [88] A. Kapustin, B. Willett and I. Yaakov, “*Exact Results for Wilson Loops in Superconformal Chern-Simons Theories with Matter*”, JHEP 1003, 089 (2010), [arxiv:0909.4559](#).
- [89] N. Drukker, J. Plefka and D. Young, “*Wilson loops in 3-dimensional  $\mathcal{N}=6$  supersymmetric Chern-Simons Theory and their string theory duals*”, JHEP 0811, 019 (2008), [arxiv:0809.2787](#). • B. Chen and J.-B. Wu, “*Supersymmetric Wilson Loops in  $\mathcal{N}=6$  Super Chern-Simons-matter theory*”, Nucl. Phys. B825, 38 (2010), [arxiv:0809.2863](#). • S.-J. Rey, T. Suyama and S. Yamaguchi, “*Wilson Loops in Superconformal Chern-Simons Theory and Fundamental Strings in Anti-de Sitter Supergravity Dual*”, JHEP 0903, 127 (2009), [arxiv:0809.3786](#).
- [90] M. Marino and P. Putrov, “*Exact Results in ABJM Theory from Topological Strings*”, JHEP 1006, 011 (2010), [arxiv:0912.3074](#).
- [91] C. G. Callan and J. M. Maldacena, “*Brane dynamics from the Born-Infeld action*”, Nucl. Phys. B513, 198 (1998), [hep-th/9708147](#). • S.-J. Rey and J.-T. Yee, “*Macroscopic strings as heavy quarks in large  $N$  gauge theory and anti-de Sitter supergravity*”, Eur. Phys. J. C22, 379 (2001), [hep-th/9803001](#).
- [92] N. Drukker and B. Fiol, “*All-genus calculation of Wilson loops using D-branes*”, JHEP 0502, 010 (2005), [hep-th/0501109](#).
- [93] J. Gomis and F. Passerini, “*Holographic Wilson loops*”, JHEP 0608, 074 (2006), [hep-th/0604007](#).
- [94] L. Freyhult, “*Review of AdS/CFT Integrability, Chapter III.4: Twist states and the cusp anomalous dimension*”, [arxiv:1012.3993](#).

- [95] A. Armoni, “*Anomalous dimensions from a spinning D5-brane*”, JHEP 0611, 009 (2006), [hep-th/0608026](#). • D. Gang, J.-S. Park and S. Yamaguchi, “*Operator with large spin and spinning D3-brane*”, JHEP 0911, 024 (2009), [arxiv:0908.3938](#).
- [96] S. A. Hartnoll and S. P. Kumar, “*Higher rank Wilson loops from a matrix model*”, JHEP 0608, 026 (2006), [hep-th/0605027](#).
- [97] S. Yamaguchi, “*Wilson loops of anti-symmetric representation and D5- branes*”, JHEP 0605, 037 (2006), [hep-th/0603208](#).
- [98] K. Okuyama and G. W. Semenoff, “*Wilson loops in  $\mathcal{N} = 4$  SYM and fermion droplets*”, JHEP 0606, 057 (2006), [hep-th/0604209](#).
- [99] H. Lin, O. Lunin and J. M. Maldacena, “*Bubbling AdS space and 1/2 BPS geometries*”, JHEP 0410, 025 (2004), [hep-th/0409174](#).
- [100] S. Yamaguchi, “*Bubbling geometries for half BPS Wilson lines*”, Int. J. Mod. Phys. A22, 1353 (2007), [hep-th/0601089](#). • O. Lunin, “*On gravitational description of Wilson lines*”, JHEP 0606, 026 (2006), [hep-th/0604133](#).
- [101] E. D’Hoker, J. Estes and M. Gutperle, “*Gravity duals of half-BPS Wilson loops*”, JHEP 0706, 063 (2007), [arxiv:0705.1004](#).
- [102] T. Okuda, “*A prediction for bubbling geometries*”, JHEP 0801, 003 (2008), [arxiv:0708.3393](#). • T. Okuda and D. Trancanelli, “*Spectral curves, emergent geometry, and bubbling solutions for Wilson loops*”, JHEP 0809, 050 (2008), [arxiv:0806.4191](#).
- [103] N. Drukker, S. Giombi, R. Ricci and D. Trancanelli, “*On the D3-brane description of some 1/4 BPS Wilson loops*”, JHEP 0704, 008 (2007), [hep-th/0612168](#).
- [104] N. Drukker and B. Fiol, “*On the integrability of Wilson loops in  $AdS_5 \times S^5$ : Some periodic ansatze*”, JHEP 0601, 056 (2006), [hep-th/0506058](#).
- [105] L. F. Alday and J. M. Maldacena, “*Gluon scattering amplitudes at strong coupling*”, JHEP 0706, 064 (2007), [arxiv:0705.0303](#).
- [106] N. Drukker and S. Kawamoto, “*Small deformations of supersymmetric Wilson loops and open spin-chains*”, JHEP 0607, 024 (2006), [hep-th/0604124](#).

# Review of AdS/CFT Integrability, Chapter IV.2: Deformations, Orbifolds and Open Boundaries

KONSTANTINOS ZOUBOS

*Niels Bohr Institute, Blegdamsvej 17, DK-2100 Copenhagen Ø, Denmark*

kzoubos@nbi.dk

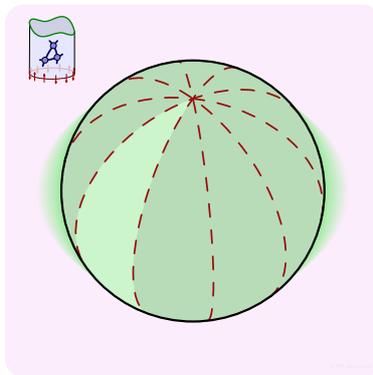

**Abstract:** We review the role of integrability in the planar spectral problem of four-dimensional superconformal gauge theories besides  $\mathcal{N} = 4$  SYM. The cases considered include the Leigh–Strassler marginal deformations of  $\mathcal{N} = 4$  SYM, quiver theories which arise as orbifolds of  $\text{AdS}_5 \times \text{S}^5$  on the dual gravity side, as well as various theories involving open spin chains.

## 1 Introduction

The fascinating integrable structures of the  $\mathcal{N} = 4$  SYM theory, reviewed in other contributions to this collection, highlight the unique position that this theory occupies among quantum field theories in four dimensions. Planar integrability is just the latest addition to a long list of remarkable properties, such as exact (perturbative and non-perturbative) conformal invariance, Montonen–Olive S-duality, as well as the celebrated AdS/CFT correspondence, stating its equivalence to IIB string theory on the  $\text{AdS}_5 \times S^5$  background.

The price to pay for these unique features is that the theory is highly unrealistic, and arguably very far removed from QCD, the theory of the strong interactions. It is thus natural to wonder whether the recent great advances in the understanding of  $\mathcal{N} = 4$  SYM are of any use when studying less supersymmetric theories. In the specific context of AdS/CFT integrability, one can ask whether there exist other four-dimensional field theories with similar integrability structures, where the techniques developed in the  $\mathcal{N} = 4$  SYM context can also be applied.

In this short review we will attempt to provide a guide to the current state of affairs regarding AdS/CFT integrability in less supersymmetric situations. We will restrict ourselves to the very special class of four-dimensional supersymmetric field theories with similar finiteness properties to  $\mathcal{N} = 4$  SYM, which are therefore also superconformal.<sup>1</sup> We will see that, despite many similarities to the  $\mathcal{N} = 4$  SYM case, there also appear significant differences in the way integrability is manifested. Therefore, although there still is quite a long way to go from these theories to QCD, their study is worthwhile and can be expected to provide a useful stepping-stone towards unraveling the implications of integrability in more realistic field theories.

## 2 The Marginal Deformations of $\mathcal{N} = 4$ SYM

For any conformal field theory, it is interesting to study its space of *exactly marginal deformations*, all the ways to deform the theory preserving quantum conformal invariance. It has been known since the early eighties that  $\mathcal{N} = 4$  SYM admits  $\mathcal{N} = 1$  supersymmetric marginal deformations, with a non-perturbative proof given by Leigh and Strassler in 1995 [3] (where references to the earlier literature can also be found).

In  $\mathcal{N} = 1$  superspace language, the Leigh–Strassler deformations can be obtained purely by deforming the superpotential of the  $\mathcal{N} = 4$  SYM theory. The relevant part of the  $\mathcal{N} = 4$  SYM lagrangian is (with  $g$  being the gauge coupling)

$$\mathcal{L}_{\text{sup}} = \int d^2\theta \mathcal{W}_{\mathcal{N}=4}, \quad \text{where} \quad \mathcal{W}_{\mathcal{N}=4} = g\text{Tr}(X[Y, Z]). \quad (2.1)$$

Here  $X, Y$  and  $Z$  are the three adjoint chiral superfields of the  $\mathcal{N} = 4$  theory. It is not hard to see that  $\mathcal{W}_{\mathcal{N}=4}$  possesses an  $\text{SU}(3) \times \text{U}(1)_R$  global invariance, the maximal part

---

<sup>1</sup>We will thus not touch the topic of integrability in QCD, which is covered in [1] in this collection. Neither will we discuss integrability in the 3-dimensional ABJM theory, referring instead to [2].

of the SU(4) R-symmetry of the theory which can be made explicit in  $\mathcal{N} = 1$  superspace. Now consider the following more general  $\mathcal{N} = 1$  superpotential:

$$\mathcal{W}_{LS} = \kappa \text{Tr} \left( X[Y, Z]_q + \frac{h}{3} (X^3 + Y^3 + Z^3) \right) \quad (2.2)$$

where  $\kappa, q$  and  $h$  are a priori complex parameters and the  $q$ -commutator is defined as  $[X, Y]_q = XY - qYX$ . The  $\mathcal{N} = 4$  SYM theory can be recovered by the choice  $(\kappa, q, h) = (g, 1, 0)$ . Generically, the only continuous symmetry of  $\mathcal{W}_{LS}$  is the  $U(1)_R$  which is always present in an  $\mathcal{N} = 1$  superconformal theory. When  $h = 0$ , it is standard to express  $q = \exp(2\pi i\beta)$  and call this case the  $\beta$ -deformation.<sup>2</sup> Here, apart from  $U(1)_R$ ,  $\mathcal{W}_{LS}$  has an extra  $U(1) \times U(1)$  symmetry acting by phase rotations on the scalars. The  $\beta$ -deformation with  $\beta$  real (i.e.  $q$  a phase) is variously known as the real- $\beta$  or the  $\gamma$ -deformation.

There are several more marginal terms one could add to the superpotential, however (2.2) is special in that it preserves an important set of discrete symmetries:

$$\begin{aligned} \text{(a)} \quad & X \rightarrow Y, \quad Y \rightarrow Z, \quad Z \rightarrow X, \\ \text{(b)} \quad & X \rightarrow X, \quad Y \rightarrow \omega Y, \quad Z \rightarrow \omega^2 Z \end{aligned} \quad (2.3)$$

with  $\omega$  a third root of unity. The first of these symmetries is particularly crucial, because it ensures that all scalar anomalous dimensions are equal. This observation allowed Leigh and Strassler to argue that finiteness imposes a *single* complex constraint on the four couplings  $(g, \kappa, q, h)$ , implying the existence of a three-dimensional parameter space of finite gauge theories. On this space, the superpotential (2.2) is thus *exactly* marginal. The finiteness constraint can be calculated at low loop orders, but its exact form is unknown, and its determination, even in the planar limit, would be a major step in our understanding of superconformal gauge theory. Here we give it at one loop (see e.g. [4] for a derivation):

$$2g^2 = \kappa \bar{\kappa} \left[ \frac{2}{N^2} (1+q)(1+\bar{q}) + \left( 1 - \frac{4}{N^2} \right) (1 + q\bar{q} + h\bar{h}) \right]. \quad (2.4)$$

Note that the constraint simplifies considerably in the planar ( $N \rightarrow \infty$ ) limit, and that for the real  $\beta$ -deformation it reduces to  $g^2 = \kappa \bar{\kappa}$ , precisely the same as that for  $\mathcal{N} = 4$  SYM. It has been shown [5] that in this real- $\beta$  case the one-loop constraint is not modified at any higher order in the perturbative expansion. This is a first indication that, in the planar limit, the theory will share many of the properties of  $\mathcal{N} = 4$  SYM, including, as we will see, integrability.

## 2.1 The gravity dual of the $\beta$ -deformation

If the  $\mathcal{N} = 4$  SYM theory admits exactly marginal deformations, the same must be true for its dual gravity background. Since the deformations preserve the conformal group, the AdS<sub>5</sub> factor of the geometry will not be affected, but we expect the S<sup>5</sup> part

<sup>2</sup>There exist several other conventions in the literature, related by relabellings of  $\beta$  and  $\kappa$ .

to be deformed, reflecting the reduction of the R-symmetry group to a subgroup of  $SU(4)_R \simeq SO(6)$ . For the  $\beta$ -deformation, the metric of this deformed  $S^5$  was found by Lunin and Maldacena in 2005 [6]. Focusing first on the *real*- $\beta$  deformation, these authors showed that it can be obtained from  $S^5$  by a sequence of T-duality, angle shift and T-duality, called a *TsT* transformation. To make this a bit more explicit, let us start with the 5-sphere embedded in  $\mathbb{R}^6$  as  $\bar{X}X + \bar{Y}Y + \bar{Z}Z = 1$ , and parametrise

$$X = \cos \gamma e^{i\varphi_1}, \quad Y = \sin \gamma \cos \psi e^{i\varphi_2}, \quad Z = \sin \gamma \sin \psi e^{i\varphi_3} \quad (2.5)$$

to obtain the five-sphere metric in terms of angle coordinates

$$ds^2 = d\gamma^2 + \cos^2 \gamma d\varphi_1^2 + \sin^2 \gamma (d\psi^2 + \cos^2 \psi d\varphi_2^2 + \sin^2 \psi d\varphi_3^2). \quad (2.6)$$

There are three explicit  $U(1)$  isometries related to the angles  $\varphi_i$ , with the diagonal shift  $\varphi_i \rightarrow \varphi_i + a$  corresponding to the  $U(1)_R$  which is required by  $\mathcal{N} = 1$  superconformal invariance. The *TsT* procedure starts by T-dualising along the other two isometry directions, then shifting the dual angles as  $\tilde{\varphi}_2 \rightarrow \tilde{\varphi}_2 + \beta \tilde{\varphi}_3$ , and finally T-dualising back. This breaks the  $SO(6)$  implicit in (2.6) and results in a geometry preserving just a  $U(1)^3$  isometry group, the right amount of symmetry for the dual to the  $\beta$ -deformation. We refer to [6, 7] for more details and for the explicit IIB solution.<sup>3</sup> Starting from the real- $\beta$  background, a sequence of S-dualities leads to the dual of the complex- $\beta$  deformation [6]. However, the geometry dual to the most general deformation (with  $h \neq 0$ ) is still unknown.

## 2.2 The real- $\beta$ deformation and integrability

In this section we focus on the real- $\beta$  deformation, which has received the most attention in the literature. The integrability properties of this theory were first investigated in [9], where it was shown that the one-loop planar dilatation generator in the two-scalar  $SU(2)_\beta$  sector corresponds to the hamiltonian of the integrable XXX  $SU(2)_\beta$  spin chain. This was extended to the  $SU(3)_\beta$  sector in [10]. In the latter work it was also noted that a suitable site-dependent transformation can map the hamiltonian of the deformed theory to that of the undeformed one (i.e.  $\mathcal{N} = 4$  SYM) but with *twisted* boundary conditions. Building on [6], where a simple star-product was introduced to keep track of the additional phases appearing in the real- $\beta$  theory compared to the undeformed case, the work [11] showed that given an undeformed  $R$ -matrix satisfying the Yang–Baxter equation, the twisted one will do so as well.<sup>4</sup>

The conclusion is that the real- $\beta$  deformation is just as integrable as  $\mathcal{N} = 4$  SYM. It should thus be possible to find a Bethe ansatz encoding the spectrum of the theory. This can indeed be done by introducing appropriate phases (“twisting”) in the  $\mathcal{N} = 4$  SYM Bethe ansatz. In the  $SU(2)_\beta$  sector, this was performed at one loop in [10], at

<sup>3</sup>It should also be noted that for  $\beta = 1/k$  (i.e.  $q$  being a  $k$ -th root of unity) the dual background is actually an  $AdS_5 \times S^5/\mathbb{Z}_k \times \mathbb{Z}_k$  orbifold [8].

<sup>4</sup>The effect of the twist on other algebraic structures of the theory, such as the Yangian (reviewed in [12]), was considered in [13].

higher loops in [14], while the higher-loop twist for all sectors was obtained in [11]. For simplicity, here we display just the one-loop,  $SU(2)_\beta$  sector case:

$$e^{-2\pi i\beta L} \left( \frac{u_k + i/2}{u_k - i/2} \right)^L = \prod_{j=1, j \neq k}^M \frac{u_k - u_j + i}{u_k - u_j - i}, \quad \prod_{k=1}^M \frac{u_k + i/2}{u_k - i/2} = e^{2\pi i\beta M} \quad (2.7)$$

where the second equation is the cyclicity condition. Very recently, [15] provided a deeper understanding of the all-loop-twisted Bethe equations by deriving them from a suitable *Drinfeld-twisted* S-matrix combined with a twist of the boundary conditions.

### Integrability and the LM background

Integrability of the IIB Green–Schwarz sigma model in the real- $\beta$  deformed case was demonstrated in [7] by explicit construction of a Lax pair for the LM background. A Lax pair was also constructed for the pure-spinor sigma-model in [16]. Therefore, just as in the undeformed case (reviewed in [17]) one can attempt to compare gauge theory results with strong coupling ones by considering semiclassical strings moving on the LM background. This was done in [18], with the construction of several semiclassical string solutions, which were matched to specific configurations of roots of the twisted Bethe ansatz. Their energies precisely agree with the gauge theory anomalous dimensions.

Giant magnons [19] on the LM background were constructed in [20] and [21], with the latter considering multispin configurations, while [22] considered more general rigid string solutions on the  $S_\gamma^3$  subspace, with the giant magnons and spiky strings as special cases. The first finite-size correction to the giant magnon energy was computed in [23] and takes the following form:<sup>5</sup>

$$E - J = 2g \sin \frac{p}{2} \left( 1 - \frac{4}{e^2} \sin^2 \frac{p}{2} \cos \left[ \frac{2\pi(n - \beta J)}{2^{3/2} \cos^3 \frac{p}{4}} \right] e^{-\frac{J}{g \sin p/2}} + \dots \right) \quad (2.8)$$

where  $n$  is the unique integer for which  $|n - \beta J| \leq \frac{1}{2}$ . This expression exhibits the expected exponential falloff, but the momentum dependence is highly unusual, and indeed reproducing it from the Lüscher correction techniques discussed in [25] is still an open problem.

### Wrapping corrections

In order to calculate wrapping corrections to the spectrum (due to interactions whose span is greater than the length of the spin chain), one needs to go beyond the asymptotic Bethe ansatz. It turns out that the techniques developed for  $\mathcal{N} = 4$  SYM (reviewed in [25–27] in this collection) can be applied with relative ease to the  $\beta$ -deformed theory. In particular, it was argued in [28] that the  $\beta$ -deformation is described by the *same* Y-system as  $\mathcal{N} = 4$  SYM. The  $\beta$  parameter arises by appropriately modifying the asymptotic (large  $L$ ) solution, exploiting the freedom to twist it by certain complex numbers. The authors of [28] showed that this procedure correctly reproduces the higher-loop asymptotic Bethe

<sup>5</sup>Recently, this result was extended to the case of dyonic, or two-spin, giant magnons [24].

ansatz of [11] (for all sectors, and more general twists) and derived generalised Lüscher formulae for generic operators in the  $\beta$ -deformed theory.

Turning to results for specific operators, an interesting feature of the  $\beta$ -deformed theory compared to  $\mathcal{N} = 4$  SYM (first noted in [29]) is that one-impurity operators

$$O_{1,L} = \text{Tr} \phi Z^{L-1}, \quad \phi \in \{X, Y\} \quad (2.9)$$

are not protected by supersymmetry and thus acquire anomalous dimensions. Because of this, the real- $\beta$  theory provides an excellent setting for the perturbative study of wrapping effects for short operators (reviewed in [30] and also in [31]): Apart from the calculations being simpler (compared to two-impurity cases like the Konishi operator), it also allows for a clean separation of the effects of wrapping from those due to the dressing factor, since the latter does not contribute at all for these states. Wrapping effects for such states, at critical wrapping (where the loop level equals the length of the operator) have been computed up to 11 loops in [32,33] (who also provided a recursive formula for calculating them at higher loop orders), and have recently been reproduced in [28] via the twisted solution to the Y-system and in [34] using generalised Lüscher formulae.<sup>6</sup>

A very special case arises when  $\beta = \frac{1}{2}$  and one considers even length operators. Then the (higher-loop version of the) Bethe ansatz (2.7) becomes the same as that for  $\mathcal{N} = 4$  SYM, apart from a sign in the cyclicity constraint. In this case, a closed (instead of iterative) form for the critical wrapping correction at any  $L$  was found in [35]. Also working at  $\beta = \frac{1}{2}$ , and using the Lüscher techniques reviewed in [25], the work [36] calculated the wrapping corrections to the single-impurity operator with  $L = 4$  up to five loops, i.e. the first two nontrivial orders:<sup>7</sup>

$$\begin{aligned} \Delta_w^{4\text{-loop}} &= 128(4\zeta(3) - 5\zeta(5)), \\ \Delta_w^{5\text{-loop}} &= -128(12\zeta(3)^2 + 32\zeta(3) + 40\zeta(5) - 105\zeta(7)). \end{aligned} \quad (2.10)$$

The four-loop result agrees with the perturbative calculations in [32], while at the time of writing there does not exist a perturbative result for the five-loop (subleading wrapping) correction. In [37], the wrapping corrections at  $\beta = \frac{1}{2}$  were used to argue for the equivalence (suggested by (2.7) for the asymptotic spectrum) of the full (non-asymptotic) spectra of the  $\beta$ -deformed theory at  $\beta$  and  $\beta + 1/L$ , with the recent leading-finite-size results of [34] in complete agreement with this.

Moving on to the two  $L = 4$  two-impurity operators ( $\text{Tr}(XYXY)$  and  $\text{Tr}(XXYY)$ ), their anomalous dimensions were found to four-loop order through explicit calculation in [32, 33].<sup>8</sup> They were also computed and matched (for arbitrary  $\beta$ ) using Lüscher methods in [38] as well as through the Y-system in [28]. Essentially the same calculation (starting from a slightly different perspective) was performed in [34].

Finally, there exists at the moment a prediction [34], coming from Lüscher methods, for the leading finite-size correction to the energy for one- and two-impurity  $sl(2)$ -sector

<sup>6</sup>Note that no TBA equations (see [26]) have yet been constructed for the  $\beta$ -deformed theory.

<sup>7</sup>Here  $\Delta_w$  denotes the wrapping contribution to the anomalous dimension, i.e. the difference of the exact result from the asymptotic one.

<sup>8</sup>Note that in  $\mathcal{N} = 4$  SYM one linear combination of these operators is BPS, while the other is a descendant of the Konishi operator. However, in the deformed theory there is no BPS combination.

operators, which has yet to be checked by explicit perturbative calculations.<sup>9</sup>

### Amplitudes

As reviewed in [40], one manifestation of integrability in the  $\mathcal{N} = 4$  SYM context is the appearance of iterative structures (which go by the name of the *BDS conjecture*) expressing multiloop amplitudes in terms of one-loop ones. One might therefore expect that amplitudes in the real- $\beta$  theory satisfy such relations as well. It has indeed been shown [41] that all (MHV and non-MHV) planar amplitudes in the real- $\beta$  theory are proportional to the corresponding  $\mathcal{N} = 4$  SYM ones, differing only in phases affecting the tree-level part of the amplitude. Thus the BDS conjecture for  $\mathcal{N} = 4$  SYM extends straightforwardly to the real- $\beta$  deformation. At strong coupling (where the tree-level part is not visible), gluon amplitudes in the real- $\beta$  theory have been shown to equal those for  $\mathcal{N} = 4$  SYM [42].

### 2.3 Integrability beyond the real- $\beta$ deformation?

In the above we focused on a very special subset of the marginal deformations, those where  $h = 0$ , while  $q$  is just a phase. One can ask whether there exist other integrable values of the parameters  $(q, h)$ . Keeping  $h = 0$  but passing to complex  $\beta$ , the hamiltonian in the two-holomorphic-scalar sector is that of the  $SU(2)_q$  XXZ model and is thus integrable [9]. However, this generically ceases to be the case beyond this simple sector [10]: Contrary to initial expectations, the one-loop hamiltonian in the *full* scalar sector is not that of the integrable  $SO(6)_q$  XXZ spin chain, but of a type not matching any known integrable hamiltonians. It was also shown in [10] that, unlike the real- $\beta$  case, it is not possible to transfer the deformation to the boundary conditions by site-dependent redefinitions.<sup>10</sup> The conclusion was that the one-loop hamiltonian for the *generic* LS deformation is not integrable.<sup>11</sup>

Nevertheless, as demonstrated in [44], there *do* exist certain special choices of parameters for which the one-loop hamiltonian is integrable:

$$(q, h) = \left\{ (0, 1/\bar{h}), \left( (1 + \rho) e^{\frac{2\pi im}{3}}, \rho e^{\frac{2\pi in}{3}} \right), \left( -e^{\frac{2\pi im}{3}}, e^{\frac{2\pi in}{3}} \right) \right\}. \quad (2.11)$$

Some of these choices were also discovered via the study of amplitudes in [45]: They correspond to special cases where the 1-loop planar finiteness condition (2.4) does not receive corrections at higher loops, similarly to the real- $\beta$  deformation.

In [46], a unifying framework for all these integrable cases was proposed: Their corresponding one-loop hamiltonians can be related to the real- $\beta$  case by *Hopf twists*. These are a way of modifying the underlying  $R$ -matrix, leaving the integrability properties unaffected. Since (as shown in [11]) the real- $\beta$  hamiltonian is itself related to the undeformed hamiltonian by such a twist, all these integrable cases can be seen to be nothing but Hopf-twisted  $\mathcal{N} = 4$  SYM.

<sup>9</sup>See also [39] for more recent results on wrapping for twist operators in the  $\beta$ -deformed theory.

<sup>10</sup>Note, furthermore, that the star-product techniques of [6] do not apply beyond real  $\beta$ , their naive extension giving rise to a non-associative product.

<sup>11</sup>The question of whether higher-loop integrability persists in the (all-loop closed)  $SU(2)_q$  sector remains open, with some progress towards constructing the required higher charges reported in [43].

Another special (one-loop) integrable sector beyond real  $\beta$  was found in [47]: It is an  $SU(3)$  sector composed of two holomorphic and one antiholomorphic scalar, for instance  $\{X, Y, \bar{Z}\}$ . The hamiltonian in this sector actually turns out to be XXZ  $SU(3)_q$ , the standard (integrable)  $q$ -deformation of  $SU(3)$ . However, this sector is not closed beyond one loop, complicating the discussion of higher-loop integrability.

Apart from these special cases, the deformed hamiltonian is not integrable. An intuitive explanation for this [14] is that the construction of the dual gravity background for the complex  $\beta$  deformation involves a sequence of S-duality transformations on the LM background [6]. The strong-weak nature of S-duality means that the intermediate stages involve interacting strings, which (as reviewed in [48]) are unlikely to preserve integrability.

A more direct argument for this lack of integrability was recently given in [46], who noticed that there exists a Hopf algebraic deformation of the global  $SU(3)$  R-symmetry group of the  $\mathcal{N} = 4$  theory under which the full LS superpotential (2.2) is invariant. However, this symmetry, defined through a suitable  $R$ -matrix depending on the deformation parameters  $q$  and  $h$ , is not a “standard” quantum-group deformation of  $SU(3)$ . In particular, apart from the special cases discussed above, the  $(q, h)$ - $R$ -matrix does *not* respect the Yang–Baxter equation, and consequently the corresponding Hopf algebra is not quasitriangular. Thus the construction (reviewed in [49]) of the transfer matrices and eventually of the integrable S-matrix of the theory would not be expected to go through.

### 2.3.1 More general TsT transformations

A different way of generalising the Lunin–Maldacena solution is by performing TsT transformations along all three available  $U(1)$ ’s within the  $S^5$  [7]. Since one of these corresponds to the R-symmetry, this procedure will completely break the superconformal symmetry. However it can be shown that these  $\gamma_i$ -*deformations* preserve integrability: The Lax pair construction goes through in this case as well [7] and in [50] it was argued that the Green–Schwarz action on TsT-deformed backgrounds is the same as the undeformed one, but with twisted boundary conditions. In [51], string energies were shown to match anomalous dimensions coming from the corresponding three-phase deformed spin chain. In addition, [52] showed that the action for three-spin strings in the “fast string” limit admits a Lax pair and thus that string motion is integrable. The integrability properties of the  $\gamma_i$  theories are thus very similar to the real- $\beta$  case.<sup>12</sup>

One can also perform integrability-preserving  $TsT$  transformations along one  $AdS_5$  and one  $S^5$  direction, leading to dipole-type deformations in the gauge theory [54], as well as purely along the  $AdS_5$  directions, leading to a noncommutative deformation on the gauge theory side [55] (see [56] for a review of the latter case).

---

<sup>12</sup>As was the case for the  $\beta$  deformation, it is possible to generalise the  $\gamma_i$ -deformations to complex values of  $\gamma_i$  while preserving integrability, but only for very special values, similar to (2.11) [53].

### 2.3.2 Non-field theory deformations

As was first noted in [10], there exist integrable deformations of the algebraic structures at the  $\mathcal{N} = 4$  SYM point which do not have a good field theory interpretation, in the sense of arising as the one-loop hamiltonian of a deformed field theory. A large class of such deformations was presented in [11]. More recently,  $q$ -deformations of the  $\mathfrak{psu}(2|2) \times \mathbb{R}^3$  algebra were considered in [57]. The role of such deformations in the AdS/CFT correspondence is not well understood, but their further study can be expected to provide a deeper understanding of the  $\mathcal{N} = 4$  integrable structures by embedding them in a larger framework.<sup>13</sup>

## 3 Integrability and orbifolds of $\mathcal{N} = 4$ SYM

Besides adding marginal operators, another way of obtaining CFT's with less supersymmetry from  $\mathcal{N} = 4$  SYM is by orbifolding [58]. On the gauge theory side, this involves picking a discrete subgroup  $\Gamma$  of the  $R$ -symmetry group and performing the following projection on the fields (here for  $\Gamma = \mathbb{Z}_M$ ):

$$\phi \rightarrow \omega^{s_\phi} \gamma \phi \gamma^{-1}, \quad \text{where } \gamma = \text{diag}(1, \omega, \omega^2, \dots, \omega^{M-1}), \quad \omega = e^{\frac{2\pi i}{M}}. \quad (3.1)$$

The integer  $s_\phi$  is related to the  $SU(4)_R$  charge of the field  $\phi$ . The resulting theories have a quiver structure: Starting with an  $U(MN)$  theory, one obtains a product gauge group  $U(N)_1 \times \dots \times U(N)_M$  with matter fields in bifundamental representations. The amount of supersymmetry preserved can be  $\mathcal{N} = 2, 1$  or  $0$ , depending on the subgroup of  $SU(4)_R$  on which  $\Gamma$  acts:  $SU(2)$ ,  $SU(3)$  or the whole  $SU(4)_R$  respectively. For instance, a choice of  $s_\phi$  resulting in an  $\mathcal{N} = 2$  theory is  $(s_X, s_Y, s_Z) = (1, -1, 0)$ .

One can easily keep track of gauge invariant operators by writing them in terms of the unorbifolded fields but with suitable phases inserted in the trace:

$$\text{Tr}(\gamma_m X Y X Z \dots), \quad \text{where } \gamma_m = \text{diag}(1, \omega^m, \dots, \omega^{(M-1)m}), \quad m = 1, \dots, M-1. \quad (3.2)$$

Operators for different choices of  $m$  do not mix with each other and correspond to different *twisted sectors* on the string side ( $m = 0$  being the untwisted sector). It is easy to see that the parent and orbifolded theory will only differ by additional phases in the Bethe equations, as well as a modification of the cyclicity condition. The one-loop Bethe equations in various  $SU(2)$  sectors were considered in [59], while their structure for the full scalar sector was derived in [60], who also argued that the higher-loop  $\mathcal{N} = 4$  SYM equations can easily be adapted to the orbifold case.<sup>14</sup> For the  $(X, Y)$   $m$ -twisted  $SU(2)$  sector, the one-loop equations take the form

$$e^{-\frac{4\pi i m}{M}} \left( \frac{u_k + \frac{i}{2}}{u_k - \frac{i}{2}} \right)^J = \prod_{j \neq k}^K \frac{u_k - u_j + i}{u_k - u_j - i}, \quad \prod_{k=1}^K \left( \frac{u_k + \frac{i}{2}}{u_k - \frac{i}{2}} \right) = e^{\frac{2\pi i m}{M}}. \quad (3.3)$$

<sup>13</sup>For a simple illustrative example of how considering a deformed theory can nicely clarify aspects of the undeformed one, the reader is referred to section 1.2 of [49] in this collection.

<sup>14</sup>These authors also exhibited the Bethe equations for a *combination* of orbifolding and twisting.

Note the strong similarity to the Bethe ansatz (2.7) for the  $\beta$ -deformation. The Bethe ansatz for more general (e.g. non-abelian) orbifolds was presented in [61].

On the string side, one considers an  $\text{AdS}_5 \times \text{S}^5/\mathbb{Z}_M$  background<sup>15</sup>, constructed via the following identifications (here for an  $\mathcal{N} = 2$  orbifold):

$$(X, Y, Z) \sim (e^{\frac{2\pi i}{M}} X, e^{-\frac{2\pi i}{M}} Y, Z) . \quad (3.4)$$

An analysis of two-spin semiclassical strings on this and more general backgrounds was performed in [59] and their energies were successfully compared to the corresponding solutions of the orbifolded Bethe ansatz above.

An advantage of the orbifold theory compared to the parent one is that a *single* giant magnon is a physical state. This was used in [63] to settle an issue of gauge non-invariance (dependence of the magnon energy on the light-cone gauge fixing parameter, once finite-size effects are considered) which had previously arisen in the  $\text{AdS}_5 \times \text{S}^5$  case [64]. It was later argued that single magnons in  $\mathcal{N} = 4$  SYM can always be thought of as living on the orbifolded theory [65]. Recently, TBA equations and wrapping effects (up to next-to-leading order) were considered for a particular orbifold theory in [34].

Another interesting application of orbifold theories is that, having a new parameter  $M$ , one can consider novel scaling limits. One such limit produces the “winding state” [66], where one starts with a string winding around an  $\text{S}^3/\mathbb{Z}_M$  in an  $\mathcal{N} = 2$  orbifold and takes  $M \rightarrow \infty$  while also taking  $J$  large, keeping  $M^2/J$  finite. In [67], finite-size corrections to this state, as well as to orbifolded circular strings, were calculated up to order  $1/J^2$  and shown to match with Bethe ansatz results. In a related  $M \rightarrow \infty$ , BMN-type limit [68], the first finite-size corrections to two-impurity operators in the  $\mathcal{N} = 2$  theory were computed in [69], both directly using the dilatation operator (to two loops) and using the higher-loop version of the twisted Bethe ansatz 3.3. They were shown to agree with each other and, given the appropriate choice of dressing factor, with the dual pp-wave string result, calculated using DLCQ methods (see [70] for related earlier work).

Starting from the  $\mathcal{N} = 2$   $\text{U}(N) \times \text{U}(N)$  quiver theory, one can move away from the orbifold point by varying the two gauge couplings independently, while preserving superconformal invariance. In [71] this was shown to break integrability, but in the extremal case where one of the two couplings vanishes (and we obtain an  $\text{SU}(N)$  gauge theory with  $N_f = 2N$  flavors) it appeared that integrability might be recovered. This result, if confirmed, would provide a first example of an integrable theory in the Veneziano limit ( $N, N_f \rightarrow \infty$  with  $N/N_f$  constant) instead of the usual ’t Hooft limit. Recently, [72] considered magnon propagation on such interpolating non-integrable chains.

On the amplitude side, it is known that orbifold theories are planar equivalent to the parent theory to all orders in perturbation theory [73]. Thus the BDS iterative conjecture is expected to immediately transfer to the orbifold theories.

### 3.1 Other backgrounds

Apart from the orbifold theories discussed above, there exist several AdS/CFT setups with reduced supersymmetry in the literature, and one can ask whether integrability

<sup>15</sup>Integrability for  $\text{AdS}_5 \times \text{S}^5/\mathbb{Z}_p \times \mathbb{Z}_q$  orbifolds has been considered in [62].

appears in those cases as well. Perhaps the best-known example of this kind [74] is constructed by taking the near horizon limit of a stack of D-branes situated at the tip of the *conifold*, a noncompact 6-dimensional Calabi–Yau manifold which can be written as a cone over the 5-dimensional *Sasaki–Einstein* manifold known as  $T^{1,1}$ . The near horizon geometry of this system is  $\text{AdS}_5 \times T^{1,1}$  and corresponds to an  $\mathcal{N} = 1$  superconformal  $U(N) \times U(N)$  gauge theory with bifundamentals, which is an infrared limit of a  $\mathbb{Z}_2$  orbifold theory of the type discussed above.

There has been intense activity in constructing semiclassical string solutions on  $T^{1,1}$ , as well as generalisations known as  $T^{p,q}$ ,  $Y^{p,q}$  and  $L^{p,q,r}$  [75–77]. However, these conformal fixed points only appear at strong coupling, and thus do not correspond to perturbatively finite field theories. It is therefore far from obvious that one should expect to find integrability. Indeed, no Lax pair construction is known for these backgrounds. Furthermore, as observed in [76] for  $T^{1,1}$  and its  $\beta$ -deformed analogue, the dispersion relation for magnons and spiky strings is transcendental, in stark contrast to the  $\text{AdS}_5 \times S^5$  case. This is a clear indication that integrability, if it appears at all, would have to do so in a much more complicated way than in  $\mathcal{N} = 4$  SYM. On the other hand, it was shown in [78] that, for the cases mentioned above, the bosonic sector in the near-flat-space limit [79] is the same as for  $S^5$ . Thus the full sigma models do at least possess an integrable subsector.

## 4 Open spin chain boundary conditions

One can also investigate integrability in a less supersymmetric setting by considering systems involving spin chains with *open* boundary conditions. This clearly signals the presence of open strings, and therefore D-branes, on the dual string side. After reviewing some universal aspects of open spin chains, we will proceed to discuss several different situations where they make an appearance in the AdS/CFT context.

As reviewed in [49] in this collection, in the algebraic approach to integrability for closed spin chains one begins by considering the RTT relations for the monodromy matrix, defined in terms of an  $R$ -matrix satisfying the Yang–Baxter equation:

$$R_{12}(u, v)R_{13}(u, w)R_{23}(v, w) = R_{23}(v, w)R_{13}(u, w)R_{12}(u, v) . \quad (4.1)$$

For open chains, these equations still hold, but have to be supplemented (at each boundary) with the *reflection*, or *boundary Yang–Baxter* equation [80]:

$$R_{12}(u, v)K_1(u)R_{21}(v, -u)K_2(v) = K_2(v)R_{12}(u, -v)K_1(u)R_{21}(-u, -v) . \quad (4.2)$$

Here the  $K_{1,2}(u)$  are known as the boundary reflection matrices. See e.g. [81] for a discussion of various boundary conditions, and the corresponding reflection matrices, for  $\mathfrak{sl}(n)$  and  $\mathfrak{sl}(m|n)$  spin chains, as well as further references to the open-chain literature. In the special case where the boundary conditions preserve the same  $\mathfrak{gl}(n)$  symmetry as the bulk chain (which is often not the case in the setups to be considered below), the general form of a perturbatively long-range integrable  $\mathfrak{gl}(n)$  spin chain with open boundary conditions was given in [82].

The generic structure of any putative open string Bethe ansatz is

$$e^{2ip_k L} = B_1(p_k) B_2(p_k) \prod_{j=1, j \neq k}^M S_{jk}(p_j, p_k) S_{kj}(-p_j, p_k) \quad (4.3)$$

where the  $S_{jk}$  are the bulk S-matrices, and  $B_{1,2}$  are the boundary reflection matrices. To understand the above structure (see also [82] for a nice exposition), note that a given excitation moving with momentum  $p_i$  will scatter with a number of other excitations, reflect from the boundary, scatter with the other excitations again (but with opposite momentum) and reflect from the second boundary before finally returning to its original position. Assuming that the bulk theory is integrable, the question of integrability hinges on the precise form of the boundary matrices  $B_{1,2}$ .

In the closed-chain case the Bethe ansatz is normally accompanied by a cyclicity condition (which on the string side arises from the closed-string level-matching condition). However, this is absent for the open-chain case. An immediate consequence of this is that single-impurity states are physical, even for non-zero momentum.

As in the closed spin-chain case, new effects arise when considering long-range *short* open spin chains, in particular *spanning* terms, which are the analogues of the closed-chain wrapping interactions for finite-length open spin chains. Little is known at present about their structure from the field theory side, though a study of such terms in [82] suggests that they are not strongly constrained by integrability, which would therefore appear to lose some of its predictive power for short chains.

## 4.1 Open spin chains within $\mathcal{N} = 4$ SYM

Although this review is mainly concerned with integrable theories beyond  $\mathcal{N} = 4$  SYM, there exist several interesting cases where integrable open spin chains arise *within* the  $\mathcal{N} = 4$  theory itself. We will thus first discuss this class of theories, which arise through the consideration of non-trivial backgrounds within  $\mathcal{N} = 4$  SYM.

### 4.1.1 Open strings on giant gravitons

The first case of this type is that of open strings ending on maximal giant gravitons [83] in  $\text{AdS}_5 \times S^5$ . These are  $D3$ -branes wrapping 3-cycles inside the 5-sphere. The gauge theory picture is that of an open-spin chain word attached to a baryon-like (determinant) operator in  $\mathcal{N} = 4$  SYM, formed out of one of the scalars in the theory, here denoted  $\Phi_B$ :

$$\epsilon_{i_1 \dots i_N} \epsilon^{j_1 \dots j_N} (\Phi_B)_{j_1}^{i_1} \dots (\Phi_B)_{j_{N-1}}^{i_{N-1}} (\Phi_{k_1} \Phi_{k_2} \dots \Phi_{k_L})_{j_N}^{i_N}. \quad (4.4)$$

In the large- $N$  limit the determinant part becomes very heavy and has no dynamics of its own, so this system behaves as a spin chain with open boundary conditions.

The one-loop hamiltonian for this type of chain was considered in [84] and shown to be integrable. It was further investigated at two-loops in [85], with the final two-loop result, in the  $\text{SU}(2)$  sector, given in [86]:

$$H = (2g^2 - 8g^4) \sum_{i=1}^{\infty} (I - P_{i,i+1}) + 2g^4 \sum_{i=1}^{\infty} (I - P_{i,i+2}) + (2g^2 - 4g^4) q_1^{\Phi_B} + 2g^4 q_2^{\Phi_B} \quad (4.5)$$

with  $q_i^{\Phi_B} = 1$  if  $\Phi_i = \Phi_B$  and 0 otherwise. The first two terms are the same as the bulk hamiltonian, the third is the naive boundary contribution coming from all the derivatives in the dilatation operator acting outside the determinant, while the last term comes from one of the derivatives acting *on* the determinant. This term is naively  $1/N$  suppressed, but survives in the planar limit, the suppression being compensated by the fact that it can act on any of the  $N - 1$  terms in the determinant. As shown in [19], the hamiltonian (4.5) is consistent with integrability. On the string side, [87] constructed non-local conserved sigma-model charges for classical open strings ending on maximal giant gravitons in the full bosonic sector, thus providing strong supporting evidence for all-loop integrability of the maximal graviton system.

For non-maximal giant gravitons (which correspond to sub-determinant-type operators in the gauge theory) the open spin chain becomes dynamical, in the sense that the number of sites can vary, even at one-loop level. This case was investigated in [88], where it was argued that the formalism of *Cuntz chains* provides a better description than the standard spin chain, and some (numerical) evidence for integrability was provided. However, on the string side, the appearance of extra conditions hinders the construction of non-local sigma model charges [87]. Thus the prospects for integrability in this case do not look particularly good.<sup>16</sup>

### Reflecting magnons

Giant magnons ending on maximal giant gravitons were considered in [86]. One can, without loss of generality, choose to consider open chains made up of a large number of  $Z$  fields, which, on the string side, correspond to semiclassical strings with a large angular momentum along the 5 – 6 plane within  $S^5$ . One can then consider two different orientations of the giant magnon relative to this plane.

*The  $Y = 0$  magnon:* In this case we choose the  $D3$ -brane to wrap the 3-sphere defined by  $Y = 0$ , which corresponds to the operator  $\det Y$  in the gauge theory. Attaching an open spin chain to this determinant, we are led to an operator of the form:

$$\epsilon_{i_1 \dots i_N} \epsilon^{j_1 \dots j_N} Y_{j_1}^{i_1} \dots Y_{j_{N-1}}^{i_{N-1}} (Z \dots Z \chi Z \dots Z)_{j_N}^{i_N} . \quad (4.6)$$

Here  $\chi$  stands for any impurity, though it will need to be a  $Y$  field if we wish to stay within the  $SU(2)$  sector. As explained in [86], this configuration has no boundary degrees of freedom, and there is a unique vacuum state. The boundary preserves an  $SU(1|2)^2$  out of the bulk  $SU(2|2)$  symmetry. The boundary scattering phase was found in [90], while commuting open-chain transfer matrices, necessary for the construction of the Bethe ansatz, were derived in [91].<sup>17</sup> In [93] it was shown that part of the bulk Yangian symmetry persists for boundary scattering and can be used to determine the bound-state reflection matrices. This boundary Yangian was further discussed in [94]. The higher-loop Bethe ansatz for this class of operators was proposed in [95], see also [96] for an earlier discussion. A different derivation, which agrees with the one above, is in [97].

<sup>16</sup>Nevertheless, integrability was recently demonstrated for giant magnons scattering off  $Y = 0$  non-maximal gravitons [89], indicating that integrable subcases do exist.

<sup>17</sup>The works [92] generalised the  $q$ -deformed S-matrix of [57] to the  $Y = 0$  and  $Z = 0$  magnon context, and studied open-chain transfer matrices for these cases.

*The  $Z = 0$  magnon:* Here we consider a  $D3$ -brane wrapping the 3-sphere defined by  $Z = 0$ , which is dual to the gauge theory operator  $\det Z$ . The open chain is still made up mainly of  $Z$ 's, but it is easy to see that they cannot be attached directly to the determinant: Such a configuration would factorise into a determinant plus a trace. To obtain a nontrivial open spin chain, there need to be impurities (fields other than  $Z$ ) stuck to the boundary:<sup>18</sup>

$$\epsilon_{i_1 \dots i_N} \epsilon^{j_1 \dots j_N} Z_{j_1}^{i_1} \dots Z_{j_{N-1}}^{i_{N-1}} (\chi Z \dots Z \chi'' Z \dots Z \chi')_{j_N}^{i_N} . \quad (4.7)$$

In this case there *are* boundary degrees of freedom, which (like the bulk magnon) fall into representations of  $SU(2|2)^2$  [86]. There are thus 16 states living on each boundary, which were identified on the string side in [98], by considering fermionic zero modes around the finite-size string solution for an open string ending on the  $Z = 0$  graviton.<sup>19</sup> The boundary scattering phase was found in [99]. One notable feature of the  $Z = 0$  case is the presence of poles in the reflection amplitude not corresponding to bound states, whose origin was explained in [100]. As for  $Y = 0$ , a boundary  $R$ -matrix was proposed in [86], however it did not directly satisfy the BYBE. This was reconsidered in [101], who found a suitable basis where the boundary  $R$  matrix does satisfy the BYBE. The higher-loop nested Bethe ansatz in this case was constructed in [102].

### Finite-size effects

Considerable recent activity in the  $\mathcal{N} = 4$  SYM context has centered around understanding finite-size effects, or wrapping interactions on the gauge theory side (see the reviews [25, 30, 27, 26] in this collection). There is an analogous formalism for the open-chain case, which was used in [103] to compute Lüscher-type corrections to open strings ending on giant gravitons (for vacuum states) and compare with explicit gauge theory results. The anomalous dimension of the  $Y = 0$  vacuum chain was shown to vanish (a result expected by supersymmetry) while in the  $Z = 0$  case it was non-trivial. The Lüscher formulae of [103] were extended to the multiparticle case in [104], allowing the computation of finite-size corrections to one-excitation states in the  $Y = 0$  case and leading to an explicit prediction to be checked by future gauge theory perturbative calculations. The analogous computation for the (more challenging)  $Z = 0$  brane has not yet been performed. Furthermore, no TBA or Y-system equations are available at present for the boundary case.

Classical solutions for finite-size magnons on  $Z = 0$  gravitons (generalising those in [98]) can be found in [105].

### Other graviton-magnon combinations

The work [106] studied open strings ending on giant gravitons in the AdS part of the geometry and, on the gauge side, identified the planar dilatation operator as the hamiltonian of an open  $sl(2)$  spin chain. However, novel features such as a variable occupation number and continuous bands in the spectrum prevented a clear understanding

<sup>18</sup>In the  $SU(2)$  sector, all the  $\chi$ 's will have to be of the same type, e.g.  $Y$  fields.

<sup>19</sup>The string solution itself was previously found in unpublished work by C. Ahn, D. Bak and S.J. Rey.

of integrability in this case. Other configurations of strings on giant gravitons have been considered in [107] (in the BMN limit), as well as in [108], where gauge theory operators dual to a giant graviton/magnon bound state are proposed.

#### 4.1.2 Operators with very large R-charge

Giant gravitons are dual to baryonic operators in  $\mathcal{N} = 4$  SYM whose dimensions grow linearly with  $N$ . One can consider other types of operators whose dimension grows as  $N^2$ , which in the simplest case are of the form  $(\det Z)^M$  (with  $M \sim N$ ) but more generally are described by Schur polynomial operators related to the Young diagram encoding their symmetries. On the dual gravity side the number of  $D3$ -branes is so large that it is no longer possible to ignore backreaction, and this modifies the AdS geometry into an LLM-type background. Strings “attached” to the above operators<sup>20</sup> have recently been considered from the gauge theory side in [109]. It is possible to integrate out the effect of the background and construct an effective dilatation operator, which is integrable in a certain limit. Interestingly, this limit includes non-planar diagrams between the trace operator and the background. Although, as reviewed in [48], truly non-planar contributions (acting on the trace operator by splitting and joining) are still expected to spoil integrability, this novel integrable limit of  $\mathcal{N} = 4$  SYM is still interesting and deserves further exploration.

#### 4.1.3 Open string insertions on Wilson loops

In the absence of nontrivial background operators for the spin chain to end on, open string boundary conditions would not be gauge invariant. A way to avoid this problem is to consider open chain insertions on Wilson loops [110]. As shown in that work, which considered such operators in the  $SU(2)$  sector at one loop, the boundary conditions turn out to be purely reflective (Neumann). Thus the Bethe ansatz can be related to a closed-chain one by the method of images. The dual description of the Wilson loop (which has angular momenta on  $S^5$  to account for the scalar insertions) was shown to reduce to “half” the standard closed folded string solution, whose energy precisely matches the Bethe ansatz computation. This setup is thus at least one-loop integrable (no higher-loop checks have been performed at present).

## 4.2 Theories with fundamental flavor

One can also obtain open spin chains by extending the field content of  $\mathcal{N} = 4$  SYM by adding flavors, i.e. fields in the fundamental representation of the gauge group. Introducing such fields in the spectrum means that, apart from trace operators, one can construct gauge-invariant operators of the generic form:

$$\bar{Q}\Phi_{i_1}\Phi_{i_2}\cdots\Phi_{i_L}Q \quad (4.8)$$

---

<sup>20</sup>Note that these are actually closed strings, since after the  $D3$ -branes have backreacted there are no explicit open strings on the background.

where  $Q$  is one of the fundamental fields. This operator, having no cyclicity properties, will behave as an open chain. We will now review three distinct settings where these types of operators have been studied in an integrability context.

#### 4.2.1 The orientifold theory

In this setup, one considers a D3–O7–D7 system, where one first performs an orientifold projection and then adds the required number of D7 branes (four, plus their mirrors) to cancel the orientifold charge. The result is  $\mathcal{N} = 2$  SYM with gauge group  $\mathrm{Sp}(N)$ , one hypermultiplet in the antisymmetric representation and four in the fundamental, which is known to be a finite theory.<sup>21</sup> The  $\mathcal{N} = 2$  vector multiplet contains an adjoint chiral multiplet  $W$ , while the antisymmetric hypermultiplet two chiral multiplets  $Z, Z'$ . The near-horizon geometry is that of an  $\mathrm{AdS}_5 \times S^5/\mathbb{Z}_2$  orientifold. Here the  $\mathbb{Z}_2$  acts as  $Z \rightarrow -Z$  (or  $\varphi_3 \rightarrow \varphi_3 + \pi$ ), leaving a fixed plane at  $Z = 0$ . The worldsheet coordinate is also identified as  $\sigma \rightarrow \pi - \sigma$ .

Relatively few studies of integrability have been undertaken for this theory. The pp-wave spectrum was discussed in [112]. Several open spinning string solutions on the dual orientifold were considered in [113]. In [114], the one-loop hamiltonian for the  $\mathrm{SU}(3)$  sector comprised of  $W, Z, Z'$  was shown to be integrable and the corresponding one-loop Bethe ansatz constructed. In the  $(Z, Z')$   $\mathrm{SU}(2)$  sector, it is:

$$\left( \frac{u_k + \frac{i}{2}}{u_k - \frac{i}{2}} \right)^{2L} = \prod_{j \neq k}^K \frac{u_k - u_j + i}{u_k - u_j - i} \frac{u_k + u_j + i}{u_k + u_j - i} \quad (4.9)$$

Notice that it is of the form (4.3). Applying the doubling trick, by means of which this Bethe ansatz can be related to a closed string one with the extra condition that the set of roots is symmetric under  $u_j \rightarrow -u_j$ , energies of two-spin open strings were successfully compared to gauge theory in [115]. At the time of writing three-spin strings have not been compared, while the question of higher-loop integrability is still open.

#### 4.2.2 The D3–D7–brane system

Here one considers  $\mathrm{AdS}_5 \times S^5$ , with a D7-brane filling  $\mathrm{AdS}_5$  and wrapping an  $S^3$  in  $S^5$ . Unlike the case above, this theory is conformal only in the strict large- $N$  limit, where the backreaction of the D7 brane can be ignored. On the gauge theory side, this corresponds to ignoring  $1/N$ -suppressed processes with virtual fundamental flavors between bulk states (which would provide a non-zero contribution to the  $\beta$ -function).

The bulk hamiltonian is the same as for  $\mathcal{N} = 4$  SYM, so closed spin chains in this setup are automatically integrable. The one-loop open-chain hamiltonian is integrable as well, with trivial boundary terms [116]. The one-loop,  $\mathrm{SU}(2)$ -sector Bethe ansatz is precisely the same as (4.9). The higher-loop reflection matrices for this case were studied in [117], where it was shown that integrability survives, largely thanks to the fact that

---

<sup>21</sup>A different type of orientifold which preserves  $\mathcal{N} = 4$  SYM but leads to gauge group  $\mathrm{SO}(N)$  or  $\mathrm{Sp}(N)$  was recently considered in [111], though in that case the focus was on non-planar corrections, the differences to  $\mathrm{SU}(N)$  being relatively minor at planar level.

the boundary respects the  $\mathfrak{psl}(2|2) \times \overline{\mathfrak{psl}(2|2)}$  factorisation of the bulk theory. More recently, the work [118] extended these results by constructing the reflection matrices for boundary scattering of *bound states*.

On the gravity side, [87] showed integrability for the full bosonic sector by observing that the equations governing open string motion are practically the same as in the maximal giant graviton case discussed above. It is thus expected that this system exhibits higher-loop integrability.

### 4.2.3 Defect theories

A different setup with fundamentals can be obtained by considering a D3–D5 system, with a single D5 sharing only three directions (say  $x^0, x^1$  and  $x^2$ ) with the stack of  $N$  D3 branes. The configuration thus has four Neumann–Dirichlet directions and preserves supersymmetry. Taking the D3-brane near-horizon limit, we obtain the usual  $\text{AdS}_5 \times S^5$  geometry, but now the D5 brane wraps an  $\text{AdS}_4 \times S^2$  in  $\text{AdS}_5 \times S^5$ . On the gauge theory side, we obtain  $\mathcal{N} = 4$  SYM coupled to a *defect* located at  $x^3 = 0$ . The matter content on the defect is a 3d  $\text{SU}(N)$  vector multiplet plus a 3d fundamental hypermultiplet (containing two chiral multiplets  $q_{1,2}$ ).

As shown in [119], starting from a ground state of the form  $\bar{q}_1 Z \cdots Z q_1$  there are two types of excitations one can consider: If the excitations are along the D5 brane, the boundary conditions are Dirichlet, which on the gauge theory translates to the boundary term being fixed. Otherwise, the string satisfies Neumann boundary conditions, which for the spin chain means that the boundary excitations are dynamical: The boundary state can flip from  $q_1$  to  $q_2$ , which effectively increases the length of the chain by 1. In both cases the boundary matrix is trivial and the full bosonic sector is integrable at one loop. As before, there is no boundary phase in the  $\text{SU}(2)$  sector, though it does make an appearance in the  $\text{SL}(2)$  sector [120]. Spinning string solutions in this setup were considered in [121].

However, it was eventually understood that this one-loop integrability is an accident. The first indication came from the gravity side, when [87] showed that nonlocal charges could only be constructed in the  $\text{SU}(2)$  sector. Finally, by careful analysis of the symmetries, [117] constructed the all-loop reflection matrices (aspects of which were previously considered in [96]) with the result that they do *not* satisfy the BYBE.

## 5 Outlook

In this short review we gave an overview of several different known ways of pushing integrability beyond the highly symmetric case of  $\mathcal{N} = 4$  SYM. As we have seen, it is relatively easy to maintain integrability at the one-loop level in less supersymmetric (but still superconformal) situations, but all-loop integrability is a much more stringent requirement. Indeed, it appears that all non- $\mathcal{N} = 4$  SYM models where higher-loop integrability persists are really just  $\mathcal{N} = 4$  SYM in disguise, in the sense that the bulk spin chain is undeformed, with differences arising only in the boundary conditions: Twisted ones for the real- $\beta$  deformations, orbifold ones for the quiver theories, and open

ones for giant gravitons and theories with fundamentals.

This observation seems to reaffirm how special the  $\mathcal{N} = 4$  SYM theory is, even within the already very restricted class of superconformal quantum field theories. On the other hand, the rich pattern of integrability breaking in the theories discussed above should help us better appreciate the implications (and limitations) of integrability for more realistic theories, in a more controllable setting than that of QCD. Even in those cases which *are* believed to be higher-loop integrable, there remain numerous open questions whose resolution can be expected to contribute to a deeper understanding of AdS/CFT integrability, and ultimately of the AdS/CFT correspondence itself.

**Acknowledgments** I am grateful to N. Beisert, R. Janik, C. Kristjansen, T. Månsson, C. Sieg and A. Torrielli for useful discussions, comments and clarifications during the writing of this review. This work was supported by FNU through grant number 272-08-0329.

## References

- [1] G. Korchemsky, “*Review of AdS/CFT Integrability, Chapter IV.4: Integrability in QCD and  $\mathcal{N} < 4$  SYM*”, arxiv:1012.4000.
- [2] T. Klose, “*Review of AdS/CFT Integrability, Chapter IV.3:  $\mathcal{N} = 6$  Chern-Simons and Strings on  $AdS_4 \times CP^3$* ”, arxiv:1012.3999.
- [3] R. G. Leigh and M. J. Strassler, “*Exactly marginal operators and duality in four-dimensional  $N=1$  supersymmetric gauge theory*”, Nucl. Phys. B447, 95 (1995), hep-th/9503121.
- [4] O. Aharony and S. S. Razamat, “*Exactly marginal deformations of  $N = 4$  SYM and of its supersymmetric orbifold descendants*”, JHEP 0205, 029 (2002), hep-th/0204045.
- [5] A. Mauri, S. Penati, A. Santambrogio and D. Zanon, “*Exact results in planar  $N = 1$  superconformal Yang-Mills theory*”, JHEP 0511, 024 (2005), hep-th/0507282.
- [6] O. Lunin and J. M. Maldacena, “*Deforming field theories with  $U(1) \times U(1)$  global symmetry and their gravity duals*”, JHEP 0505, 033 (2005), hep-th/0502086.
- [7] S. Frolov, “*Lax pair for strings in Lunin-Maldacena background*”, JHEP 0505, 069 (2005), hep-th/0503201.
- [8] D. Berenstein, V. Jejjala and R. G. Leigh, “*Marginal and relevant deformations of  $N = 4$  field theories and non-commutative moduli spaces of vacua*”, Nucl. Phys. B589, 196 (2000), hep-th/0005087.
- [9] R. Roiban, “*On spin chains and field theories*”, JHEP 0409, 023 (2004), hep-th/0312218.
- [10] D. Berenstein and S. A. Cherkis, “*Deformations of  $N = 4$  SYM and integrable spin chain models*”, Nucl. Phys. B702, 49 (2004), hep-th/0405215.
- [11] N. Beisert and R. Roiban, “*Beauty and the twist: The Bethe ansatz for twisted  $N = 4$  SYM*”, JHEP 0508, 039 (2005), hep-th/0505187.

- [12] A. Torrielli, “Review of AdS/CFT Integrability, Chapter VI.2: Yangian Algebra”, arxiv:1012.4005.
- [13] J. N. Ihry, “Yangians in Deformed Super Yang-Mills Theories”, JHEP 0804, 051 (2008), arxiv:0802.3644.
- [14] S. A. Frolov, R. Roiban and A. A. Tseytlin, “Gauge - string duality for superconformal deformations of  $N = 4$  super Yang-Mills theory”, JHEP 0507, 045 (2005), hep-th/0503192.
- [15] C. Ahn, Z. Bajnok, D. Bombardelli and R. I. Nepomechie, “Twisted Bethe equations from a twisted  $S$ -matrix”, JHEP 1102, 027 (2011), arxiv:1010.3229.
- [16] P. A. Grassi and J. Kluson, “Pure spinor strings in TsT deformed background”, JHEP 0703, 033 (2007), hep-th/0611151.
- [17] A. Tseytlin, “Review of AdS/CFT Integrability, Chapter II.1: Classical  $AdS_5 \times S^5$  string solutions”, arxiv:1012.3986. • T. McLoughlin, “Review of AdS/CFT Integrability, Chapter II.2: Quantum Strings in  $AdS_5 \times S^5$ ”, arxiv:1012.3987.
- [18] H.-Y. Chen and S. Prem Kumar, “Precision test of AdS/CFT in Lunin-Maldacena background”, JHEP 0603, 051 (2006), hep-th/0511164. • H.-Y. Chen and K. Okamura, “The anatomy of gauge / string duality in Lunin-Maldacena background”, JHEP 0602, 054 (2006), hep-th/0601109.
- [19] D. M. Hofman and J. M. Maldacena, “Giant magnons”, J. Phys. A39, 13095 (2006), hep-th/0604135.
- [20] C.-S. Chu, G. Georgiou and V. V. Khoze, “Magnons, classical strings and beta-deformations”, JHEP 0611, 093 (2006), hep-th/0606220.
- [21] N. P. Bobev, H. Dimov and R. C. Rashkov, “Semiclassical strings in Lunin-Maldacena background”, hep-th/0506063.
- [22] N. P. Bobev and R. C. Rashkov, “Spiky Strings, Giant Magnons and beta-deformations”, Phys. Rev. D76, 046008 (2007), arxiv:0706.0442.
- [23] D. V. Bykov and S. Frolov, “Giant magnons in TsT-transformed  $AdS_5 \times S^5$ ”, JHEP 0807, 071 (2008), arxiv:0805.1070.
- [24] C. Ahn and P. Bozhilov, “Finite-Size Dyonic Giant Magnons in TsT-transformed  $AdS_5 \times S^5$ ”, JHEP 1007, 048 (2010), arxiv:1005.2508.
- [25] R. Janik, “Review of AdS/CFT Integrability, Chapter III.5: Lüscher corrections”, arxiv:1012.3994.
- [26] Z. Bajnok, “Review of AdS/CFT Integrability, Chapter III.6: Thermodynamic Bethe Ansatz”, arxiv:1012.3995.
- [27] V. Kazakov and N. Gromov, “Review of AdS/CFT Integrability, Chapter III.7: Hirota Dynamics for Quantum Integrability”, arxiv:1012.3996.
- [28] N. Gromov and F. Levkovich-Maslyuk, “Y-system and beta-deformed  $N=4$  Super-Yang-Mills”, J. Phys. A44, 015402 (2011), arxiv:1006.5438.
- [29] D. Z. Freedman and U. Gursoy, “Comments on the beta-deformed  $N = 4$  SYM theory”, JHEP 0511, 042 (2005), hep-th/0506128.
- [30] C. Sieg, “Review of AdS/CFT Integrability, Chapter I.2: The spectrum from perturbative gauge theory”, arxiv:1012.3984.

- [31] F. Fiamberti, A. Santambrogio and C. Sieg, “*Superspace methods for the computation of wrapping effects in the standard and beta-deformed  $N=4$  SYM*”, arxiv:1006.3475.
- [32] F. Fiamberti, A. Santambrogio, C. Sieg and D. Zanon, “*Finite-size effects in the superconformal beta-deformed  $N=4$  SYM*”, JHEP 0808, 057 (2008), arxiv:0806.2103.
- [33] F. Fiamberti, A. Santambrogio, C. Sieg and D. Zanon, “*Single impurity operators at critical wrapping order in the beta-deformed  $N=4$  SYM*”, JHEP 0908, 034 (2009), arxiv:0811.4594.
- [34] G. Arutyunov, M. de Leeuw and S. J. van Tongeren, “*Twisting the Mirror TBA*”, JHEP 1102, 025 (2011), arxiv:1009.4118.
- [35] M. Beccaria and G. F. De Angelis, “*On the wrapping correction to single magnon energy in twisted  $N=4$  SYM*”, Int. J. Mod. Phys. A24, 5803 (2009), arxiv:0903.0778.
- [36] Z. Bajnok, A. Hegedus, R. A. Janik and T. Lukowski, “*Five loop Konishi from AdS/CFT*”, Nucl. Phys. B827, 426 (2010), arxiv:0906.4062.
- [37] J. Gunnesson, “*Wrapping in maximally supersymmetric and marginally deformed  $N=4$  Yang-Mills*”, JHEP 0904, 130 (2009), arxiv:0902.1427.
- [38] C. Ahn, Z. Bajnok, D. Bombardelli and R. I. Nepomechie, “*Finite-size effect for four-loop Konishi of the beta-deformed  $N=4$  SYM*”, Phys. Lett. B693, 380 (2010), arxiv:1006.2209.
- [39] M. Beccaria, F. Levkovich-Maslyuk and G. Macorini, “*On wrapping corrections to GKP-like operators*”, JHEP 1103, 001 (2011), arxiv:1012.2054. • M. de Leeuw and T. Lukowski, “*Twist operators in  $N=4$  beta-deformed theory*”, arxiv:1012.3725.
- [40] R. Roiban, “*Review of AdS/CFT Integrability, Chapter V.1: Scattering Amplitudes – a Brief Introduction*”, arxiv:1012.4001.
- [41] V. V. Khoze, “*Amplitudes in the beta-deformed conformal Yang-Mills*”, JHEP 0602, 040 (2006), hep-th/0512194.
- [42] Y. Oz, S. Theisen and S. Yankielowicz, “*Gluon Scattering in Deformed  $N=4$  SYM*”, Phys. Lett. B662, 297 (2008), arxiv:0712.3491.
- [43] T. Mansson, “*Is there a tower of charges to be discovered?*”, J. Phys. A41, 194014 (2008), arxiv:0711.0931.
- [44] D. Bundzik and T. Mansson, “*The general Leigh-Strassler deformation and integrability*”, JHEP 0601, 116 (2006), hep-th/0512093.
- [45] L. V. Bork, D. I. Kazakov, G. S. Vartanov and A. V. Zhiboedov, “*Conformal Invariance in the Leigh-Strassler deformed  $N=4$  SYM Theory*”, JHEP 0804, 003 (2008), arxiv:0712.4132.
- [46] T. Mansson and K. Zoubos, “*Quantum Symmetries and Marginal Deformations*”, JHEP 1010, 043 (2010), arxiv:0811.3755.
- [47] T. Mansson, “*The Leigh-Strassler Deformation and the Quest for Integrability*”, JHEP 0706, 010 (2007), hep-th/0703150.
- [48] C. Kristjansen, “*Review of AdS/CFT Integrability, Chapter IV.1: Aspects of Non-planarity*”, arxiv:1012.3997.
- [49] M. Staudacher, “*Review of AdS/CFT Integrability, Chapter III.1: Bethe Ansätze and the R-Matrix Formalism*”, arxiv:1012.3990.

- [50] L. F. Alday, G. Arutyunov and S. Frolov, “*Green-Schwarz strings in TsT-transformed backgrounds*”, JHEP 0606, 018 (2006), [hep-th/0512253](#).
- [51] S. A. Frolov, R. Roiban and A. A. Tseytlin, “*Gauge-string duality for (non)supersymmetric deformations of  $N = 4$  super Yang-Mills theory*”, Nucl. Phys. B731, 1 (2005), [hep-th/0507021](#).
- [52] A. H. Prinsloo, “*gamma(i) deformed Lax pair for rotating strings in the fast motion limit*”, JHEP 0601, 050 (2006), [hep-th/0510095](#).
- [53] L. Freyhult, C. Kristjansen and T. Mansson, “*Integrable spin chains with  $U(1)^{*3}$  symmetry and generalized Lunin-Maldacena backgrounds*”, JHEP 0512, 008 (2005), [hep-th/0510221](#).
- [54] N. P. Bobev, H. Dimov and R. C. Rashkov, “*Semiclassical strings, dipole deformations of  $N = 1$  SYM and decoupling of KK modes*”, JHEP 0602, 064 (2006), [hep-th/0511216](#).
- [55] T. McLoughlin and I. Swanson, “*Integrable twists in AdS/CFT*”, JHEP 0608, 084 (2006), [hep-th/0605018](#).
- [56] I. Swanson, “*A review of integrable deformations in AdS/CFT*”, Mod. Phys. Lett. A22, 915 (2007), [arxiv:0705.2844](#).
- [57] N. Beisert and P. Koroteev, “*Quantum Deformations of the One-Dimensional Hubbard Model*”, J. Phys. A41, 255204 (2008), [arxiv:0802.0777](#).
- [58] S. Kachru and E. Silverstein, “*4d conformal theories and strings on orbifolds*”, Phys. Rev. Lett. 80, 4855 (1998), [hep-th/9802183](#). • A. E. Lawrence, N. Nekrasov and C. Vafa, “*On conformal field theories in four dimensions*”, Nucl. Phys. B533, 199 (1998), [hep-th/9803015](#).
- [59] K. Ideguchi, “*Semiclassical strings on  $AdS(5) \times S^{*5}/Z(M)$  and operators in orbifold field theories*”, JHEP 0409, 008 (2004), [hep-th/0408014](#).
- [60] N. Beisert and R. Roiban, “*The Bethe ansatz for  $Z(S)$  orbifolds of  $N = 4$  super Yang-Mills theory*”, JHEP 0511, 037 (2005), [hep-th/0510209](#).
- [61] A. Solovoyov, “*Bethe Ansatz Equations for General Orbifolds of  $N=4$  SYM*”, JHEP 0804, 013 (2008), [arxiv:0711.1697](#).
- [62] D. Sadri and M. M. Sheikh-Jabbari, “*Integrable spin chains on the conformal moose*”, JHEP 0603, 024 (2006), [hep-th/0510189](#).
- [63] D. Astolfi, V. Forini, G. Grignani and G. W. Semenoff, “*Gauge invariant finite size spectrum of the giant magnon*”, Phys. Lett. B651, 329 (2007), [hep-th/0702043](#).
- [64] G. Arutyunov, S. Frolov and M. Zamaklar, “*Finite-size effects from giant magnons*”, Nucl. Phys. B778, 1 (2007), [hep-th/0606126](#).
- [65] B. Ramadanovic and G. W. Semenoff, “*Finite Size Giant Magnon*”, Phys. Rev. D79, 126006 (2009), [arxiv:0803.4028](#).
- [66] M. Bertolini, J. de Boer, T. Harmark, E. Imeroni and N. A. Obers, “*Gauge theory description of compactified pp-waves*”, JHEP 0301, 016 (2003), [hep-th/0209201](#).
- [67] D. Astolfi, G. Grignani, T. Harmark and M. Orselli, “*Finite-size corrections to the rotating string and the winding state*”, JHEP 0808, 099 (2008), [arxiv:0804.3301](#).
- [68] S. Mukhi, M. Rangamani and E. P. Verlinde, “*Strings from quivers, membranes from moose*”, JHEP 0205, 023 (2002), [hep-th/0204147](#).

- [69] D. Astolfi, V. Forini, G. Grignani and G. W. Semenoff, “*Finite size corrections and integrability of  $N = 2$  SYM and DLCQ strings on a pp-wave*”, JHEP 0609, 056 (2006), hep-th/0606193.
- [70] G. De Risi, G. Grignani, M. Orselli and G. W. Semenoff, “*DLCQ string spectrum from  $N = 2$  SYM theory*”, JHEP 0411, 053 (2004), hep-th/0409315.
- [71] A. Gadde, E. Pomoni and L. Rastelli, “*Spin Chains in  $N=2$  Superconformal Theories: from the  $Z_2$  Quiver to Superconformal QCD*”, arxiv:1006.0015.
- [72] A. Gadde and L. Rastelli, “*Twisted Magnons*”, arxiv:1012.2097.
- [73] M. Bershadsky and A. Johansen, “*Large  $N$  limit of orbifold field theories*”, Nucl. Phys. B536, 141 (1998), hep-th/9803249.
- [74] I. R. Klebanov and E. Witten, “*Superconformal field theory on threebranes at a Calabi-Yau singularity*”, Nucl. Phys. B536, 199 (1998), hep-th/9807080.
- [75] M. Schvellinger, “*Spinning and rotating strings for  $N = 1$  SYM theory and brane constructions*”, JHEP 0402, 066 (2004), hep-th/0309161. • N. Kim, “*Multi-spin strings on  $AdS(5) \times T(1,1)$  and operators of  $N = 1$  superconformal theory*”, Phys. Rev. D69, 126002 (2004), hep-th/0312113. • X.-J. Wang, “*Spinning strings on deformed  $AdS(5) \times T(1,1)$  with NS  $B$ - fields*”, Phys. Rev. D72, 086006 (2005), hep-th/0501029. • S. Benvenuti and M. Kruczenski, “*Semiclassical strings in Sasaki-Einstein manifolds and long operators in  $N = 1$  gauge theories*”, JHEP 0610, 051 (2006), hep-th/0505046. • S. Benvenuti and E. Tonni, “*Giant magnons and spiky strings on the conifold*”, JHEP 0902, 041 (2009), arxiv:0811.0145. • D. Giataganas, “*Semi-classical Strings in Sasaki-Einstein Manifolds*”, JHEP 0910, 087 (2009), arxiv:0904.3125.
- [76] H. Dimov, M. Michalcik and R. C. Rashkov, “*Strings on the deformed  $T^{1,1}$ : giant magnon and single spike solutions*”, JHEP 0910, 019 (2009), arxiv:0908.3065.
- [77] D. Giataganas, “*Semiclassical strings in marginally deformed toric  $AdS/CFT$* ”, arxiv:1010.1502.
- [78] S. Benvenuti and E. Tonni, “*Near-flat space limit and Einstein manifolds*”, JHEP 0802, 022 (2008), arxiv:0707.1676.
- [79] J. M. Maldacena and I. Swanson, “*Connecting giant magnons to the pp-wave: An interpolating limit of  $AdS_5 \times S^5$* ”, Phys. Rev. D76, 026002 (2007), hep-th/0612079.
- [80] E. K. Sklyanin, “*Boundary Conditions for Integrable Quantum Systems*”, J. Phys. A21, 2375 (1988).
- [81] D. Arnaudon, J. Avan, N. Crampe, A. Doikou, L. Frappat and E. Ragoucy, “*General boundary conditions for the  $sl(N)$  and  $sl(M|N)$  open spin chains*”, J. Stat. Mech. 0408, P005 (2004), math-ph/0406021.
- [82] N. Beisert and F. Loebbert, “*Open Perturbatively Long-Range Integrable  $gl(N)$  Spin Chains*”, Adv. Sci. Lett. 2, 261 (2009), arxiv:0805.3260.
- [83] J. McGreevy, L. Susskind and N. Toumbas, “*Invasion of the giant gravitons from anti-de Sitter space*”, JHEP 0006, 008 (2000), hep-th/0003075.
- [84] D. Berenstein and S. E. Vazquez, “*Integrable open spin chains from giant gravitons*”, JHEP 0506, 059 (2005), hep-th/0501078.

- [85] A. Agarwal, “*Open spin chains in super Yang-Mills at higher loops: Some potential problems with integrability*”, JHEP 0608, 027 (2006), [hep-th/0603067](#).
- [86] D. M. Hofman and J. M. Maldacena, “*Reflecting magnons*”, JHEP 0711, 063 (2007), [arxiv:0708.2272](#).
- [87] N. Mann and S. E. Vazquez, “*Classical open string integrability*”, JHEP 0704, 065 (2007), [hep-th/0612038](#).
- [88] D. Berenstein, D. H. Correa and S. E. Vazquez, “*Quantizing open spin chains with variable length: An example from giant gravitons*”, Phys. Rev. Lett. 95, 191601 (2005), [hep-th/0502172](#). • D. Berenstein, D. H. Correa and S. E. Vazquez, “*A study of open strings ending on giant gravitons, spin chains and integrability*”, JHEP 0609, 065 (2006), [hep-th/0604123](#).
- [89] A. Ciavarella, “*Giant magnons and non-maximal giant gravitons*”, JHEP 1101, 040 (2011), [arxiv:1011.1440](#).
- [90] H.-Y. Chen and D. H. Correa, “*Comments on the Boundary Scattering Phase*”, JHEP 0802, 028 (2008), [arxiv:0712.1361](#).
- [91] R. Murgan and R. I. Nepomechie, “*Open-chain transfer matrices for AdS/CFT*”, JHEP 0809, 085 (2008), [arxiv:0808.2629](#).
- [92] R. Murgan and R. I. Nepomechie, “*q-deformed su(2|2) boundary S-matrices via the ZF algebra*”, JHEP 0806, 096 (2008), [arxiv:0805.3142](#). • R. Murgan, “*A note on open-chain transfer matrices from q-deformed su(2|2) S-matrices*”, Fortschr. Phys. 57, 895 (2009), [arxiv:0906.4361](#).
- [93] C. Ahn and R. I. Nepomechie, “*Yangian symmetry and bound states in AdS/CFT boundary scattering*”, JHEP 1005, 016 (2010), [arxiv:1003.3361](#).
- [94] N. MacKay and V. Regelskis, “*Yangian symmetry of the Y=0 maximal giant graviton*”, JHEP 1012, 076 (2010), [arxiv:1010.3761](#).
- [95] W. Galleas, “*The Bethe Ansatz Equations for Reflecting Magnons*”, Nucl. Phys. B820, 664 (2009), [arxiv:0902.1681](#).
- [96] K. Okamura and K. Yoshida, “*Higher loop Bethe ansatz for open spin-chains in AdS/CFT*”, JHEP 0609, 081 (2006), [hep-th/0604100](#).
- [97] R. I. Nepomechie, “*Bethe ansatz equations for open spin chains from giant gravitons*”, JHEP 0905, 100 (2009), [arxiv:0903.1646](#).
- [98] D. Bak, “*Zero Modes for the Boundary Giant Magnons*”, Phys. Lett. B672, 284 (2009), [arxiv:0812.2645](#).
- [99] C. Ahn, D. Bak and S.-J. Rey, “*Reflecting Magnon Bound States*”, JHEP 0804, 050 (2008), [arxiv:0712.4144](#).
- [100] L. Palla, “*Issues on magnon reflection*”, Nucl. Phys. B808, 205 (2009), [arxiv:0807.3646](#).
- [101] C. Ahn and R. I. Nepomechie, “*The Zamolodchikov-Faddeev algebra for open strings attached to giant gravitons*”, JHEP 0805, 059 (2008), [arxiv:0804.4036](#).
- [102] D. H. Correa and C. A. S. Young, “*Asymptotic Bethe equations for open boundaries in planar AdS/CFT*”, [arxiv:0912.0627](#).

- [103] D. H. Correa and C. A. S. Young, “*Finite size corrections for open strings/open chains in planar AdS/CFT*”, JHEP 0908, 097 (2009), [arxiv:0905.1700](#).
- [104] Z. Bajnok and L. Palla, “*Boundary finite size corrections for multiparticle states and planar AdS/CFT*”, JHEP 1101, 011 (2011), [arxiv:1010.5617](#).
- [105] A. Ciavarella and P. Bowcock, “*Boundary Giant Magnons and Giant Gravitons*”, JHEP 1009, 072 (2010), [arxiv:1007.1674](#).
- [106] D. H. Correa and G. A. Silva, “*Dilatation operator and the super Yang-Mills duals of open strings on AdS giant gravitons*”, JHEP 0611, 059 (2006), [hep-th/0608128](#).
- [107] D. Sadri and M. M. Sheikh-Jabbari, “*Giant hedge-hogs: Spikes on giant gravitons*”, Nucl. Phys. B687, 161 (2004), [hep-th/0312155](#).
- [108] S. Hirano, “*Fat magnon*”, JHEP 0704, 010 (2007), [hep-th/0610027](#).
- [109] R. de Mello Koch, T. K. Dey, N. Ives and M. Stephanou, “*Hints of Integrability Beyond the Planar Limit*”, JHEP 1001, 014 (2010), [arxiv:0911.0967](#).
- [110] N. Drukker and S. Kawamoto, “*Small deformations of supersymmetric Wilson loops and open spin-chains*”, JHEP 0607, 024 (2006), [hep-th/0604124](#).
- [111] P. Caputa, C. Kristjansen and K. Zoubos, “*On the spectral problem of  $N=4$  SYM with orthogonal or symplectic gauge group*”, JHEP 1010, 082 (2010), [arxiv:1005.2611](#).
- [112] D. E. Berenstein, E. Gava, J. M. Maldacena, K. S. Narain and H. S. Nastase, “*Open strings on plane waves and their Yang-Mills duals*”, [hep-th/0203249](#).
- [113] B. Stefanski, Jr., “*Open spinning strings*”, JHEP 0403, 057 (2004), [hep-th/0312091](#).
- [114] B. Chen, X.-J. Wang and Y.-S. Wu, “*Integrable open spin chain in super Yang-Mills and the plane-wave / SYM duality*”, JHEP 0402, 029 (2004), [hep-th/0401016](#).
- [115] B. Chen, X.-J. Wang and Y.-S. Wu, “*Open spin chain and open spinning string*”, Phys. Lett. B591, 170 (2004), [hep-th/0403004](#).
- [116] T. Erler and N. Mann, “*Integrable open spin chains and the doubling trick in  $N = 2$  SYM with fundamental matter*”, JHEP 0601, 131 (2006), [hep-th/0508064](#).
- [117] D. H. Correa and C. A. S. Young, “*Reflecting magnons from  $D7$  and  $D5$  branes*”, J. Phys. A41, 455401 (2008), [arxiv:0808.0452](#).
- [118] N. MacKay and V. Regelskis, “*On the reflection of magnon bound states*”, JHEP 1008, 055 (2010), [arxiv:1006.4102](#).
- [119] O. DeWolfe and N. Mann, “*Integrable open spin chains in defect conformal field theory*”, JHEP 0404, 035 (2004), [hep-th/0401041](#).
- [120] T. McLoughlin and I. Swanson, “*Open string integrability and AdS/CFT*”, Nucl. Phys. B723, 132 (2005), [hep-th/0504203](#).
- [121] Y. Susaki, Y. Takayama and K. Yoshida, “*Open semiclassical strings and long defect operators in AdS/dCFT correspondence*”, Phys. Rev. D71, 126006 (2005), [hep-th/0410139](#). • Y. Susaki, Y. Takayama and K. Yoshida, “*Integrability and higher loops in AdS/dCFT correspondence*”, Phys. Lett. B624, 115 (2005), [hep-th/0504209](#). • K. Okamura, Y. Takayama and K. Yoshida, “*Open spinning strings and AdS/dCFT duality*”, JHEP 0601, 112 (2006), [hep-th/0511139](#).

# Review of AdS/CFT Integrability, Chapter IV.3: $\mathcal{N} = 6$ Chern-Simons and Strings on $AdS_4 \times CP^3$

THOMAS KLOSE

*Department of Physics and Astronomy, Uppsala University  
SE-751 08 Uppsala, Sweden*

thomas.klose@fysast.uu.se

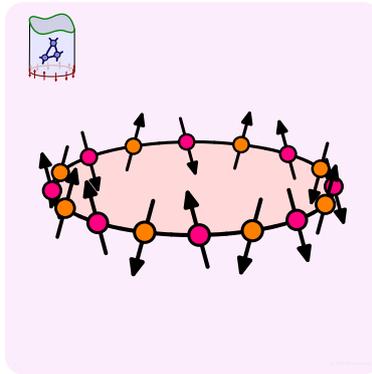

**Abstract:** We review the duality and integrability of  $\mathcal{N} = 6$  superconformal Chern-Simons theory in three dimensions and IIA superstring theory on the background  $AdS_4 \times CP^3$ . We introduce both of these models and describe how their degrees of freedom are mapped to excitations of a long-range integrable spin-chain. Finally, we discuss the properties of the Bethe equations, the S-matrix and the algebraic curve that are special to this correspondence and differ from the case of  $\mathcal{N} = 4$  SYM theory and strings on  $AdS_5 \times S^5$ .

# 1 Introduction

Almost all statements that have been made in the other chapters of this review [1] about the duality and integrability of string theory on  $AdS_5 \times S^5$  and  $\mathcal{N} = 4$  Yang-Mills theory in four dimensions, also hold in an appropriately adopted form for a second example of the AdS/CFT correspondence. This example has been known since June 2008 [2], and it is as concrete as the “old” one. Because the involved space-times are of one less dimension, this correspondence is often referred to as  $AdS_4/CFT_3$  to distinguish it from the more established  $AdS_5/CFT_4$ .<sup>1</sup>

In the  $AdS_5/CFT_4$  case, we had IIB superstring theory on  $AdS_5 \times S^5$  with self-dual RR 5-form flux  $F^{(5)} \sim N$  through  $AdS_5$  and  $S^5$ . This is now replaced by:

$$\begin{aligned} &\text{IIA superstring theory on } AdS_4 \times CP^3 \\ &\text{with RR four-form flux } F^{(4)} \sim N \text{ through } AdS_4 \\ &\text{and RR two-form flux } F^{(2)} \sim k \text{ through a } CP^1 \subset CP^3. \end{aligned} \quad (1.1)$$

On the gauge theory side, we had  $\mathcal{N} = 4$  superconformal Yang-Mills theory with coupling  $g_{YM}$  and gauge group  $U(N)$  on  $\mathbb{R}^{1,3}$ . Now this is replaced by ABJM theory:

$$\begin{aligned} &\mathcal{N} = 6 \text{ superconformal Chern-Simons-matter theory} \\ &\text{with gauge group } U(N) \times U(N) \text{ on } \mathbb{R}^{1,2} \\ &\text{and Chern-Simons levels } k \text{ and } -k. \end{aligned} \quad (1.2)$$

Both theories are controlled by two and only two parameters,  $k$  and  $N$ , which take integer values. These parameters determine all other quantities like coupling constants and the effective string tension. In ABJM theory, the Chern-Simons level  $k$  acts like a coupling constant. The fields can be rescaled in such a way that all interactions are suppressed by powers of  $\frac{1}{k}$ , i.e. large  $k$  is the weak coupling regime. One can take a planar, or ’t Hooft, limit which is given by

$$k, N \rightarrow \infty \quad , \quad \lambda \equiv \frac{N}{k} = \text{fixed} . \quad (1.3)$$

It is in this limit where integrability shows up and which is therefore the focus of this review. On the gravity side, the string coupling constant and effective tension are given by<sup>2</sup>

$$g_s \sim \left( \frac{N}{k^5} \right)^{1/4} = \frac{\lambda^{5/4}}{N} \quad , \quad \frac{R^2}{\alpha'} = 4\pi\sqrt{2\lambda} , \quad (1.4)$$

where  $R$  is the radius of  $CP^3$  and *twice* the radius of  $AdS_4$ . These relations are qualitatively the same as in the  $AdS_5/CFT_4$  context. In the planar limit  $g_s$  goes to zero and thus the strings do not split or join. At small ’t Hooft coupling, the background is highly curved and the string is subject to large quantum fluctuations. At large ’t

<sup>1</sup>Since December 2009, also an  $AdS_3/CFT_2$  correspondence has been discussed in the context of integrability [3].

<sup>2</sup>There are corrections to the second relation at two loops in the sigma model [4].

Hooft coupling, the background is weakly curved which renders the sigma-model weakly coupled and the string behaves classically.

The first equation in (1.4) contains a hint that the duality is about more than the relationship between (1.1) and (1.2). If we are not in the 't Hooft limit but if we let  $N \gg k^5$ , then the string coupling  $g_s$  becomes large. However, strongly coupled IIA string theory is M-theory. Indeed, ABJM theory (1.2) at arbitrary value of  $k$  and  $N$  is dual to [2]

$$\begin{aligned} &\text{M-theory on } AdS_4 \times S^7/\mathbb{Z}_k \\ &\text{with four-form flux } F^{(4)} \sim N \text{ through } AdS_4. \end{aligned} \tag{1.5}$$

In other words, ABJM theory is the world-volume theory of a stack of  $N$  M2 branes moving on  $\mathbb{C}^4/\mathbb{Z}_k$  [2]. The duality of (1.1) and (1.2) is really only a corollary of this more general M/ABJM duality in the limit where  $k^5 \gg N$  and where therefore M-theory is well approximated by weakly coupled IIA string theory on a  $AdS_4 \times CP^3$  background<sup>3</sup>. The lecture notes [5] discuss the general M/ABJM correspondence. However, in the planar limit (1.3), where  $k$  and  $N$  grow large with equal powers, we are always in the IIA regime. Thus, by concentrating on the question of integrability we are only concerned with IIA/ABJM. An extended and largely self-contained review of the  $AdS_4/CFT_3$  correspondence is forthcoming [6].

**Overview.** In a nutshell, the differences between  $AdS_5/CFT_4$  and  $AdS_4/CFT_3$ , see Tab. 1, are: The first duality involves theories that are invariant under the supergroup  $PSU(2, 2|4)$  and therefore are maximally supersymmetric (32 supercharges), while the theories in the second duality are  $OSp(6|4)$ -symmetric, a group which contains “only” 24 supercharges. After gauge fixing, the symmetry groups reduce to two and one copy of  $SU(2|2)$ , respectively. The *sixteen* elementary excitations in the 5/4d case transform in the representation  $(2|2)_L \otimes (2|2)_R$  of the residual symmetry group, while there are only *eight* elementary excitations in the 4/3d case which transform in the representation

$$(2|2)_{A\text{-particles}} \oplus (2|2)_{B\text{-particles}} . \tag{1.6}$$

In Sec. 3 and Sec. 5 we will show how these two types of particles arise from the gauge and string theory degrees of freedom, respectively.

Another difference between the two dualities is that the interpolation between weak and strong coupling in  $AdS_4/CFT_3$  is much more intricate. Take e.g. the magnon dispersion relation, which due to the underlying  $SU(2|2)$  symmetry is fixed in either duality to be of the form [7] (see also [8])

$$E(p) = \sqrt{Q^2 + 4h^2(\lambda) \sin^2 \frac{p}{2}} , \tag{1.7}$$

where  $Q$  is the magnon R-charge and where the function  $h(\lambda)$  is *not* fixed by symmetry. The fundamental magnon in  $AdS_5/CFT_4$  has charge  $Q = 1$ , while in  $AdS_4/CFT_3$  it has

---

<sup>3</sup> $CP^3$  arises from writing  $S^7$  as  $S^1$  fibered over  $CP^3$  and by identifying the circle as the M-theory direction which shrinks to zero size by the orbifold action of  $\mathbb{Z}_k$  in the large  $k$  limit.

|                   | $AdS_5/CFT_4$                                                                     | $AdS_4/CFT_3$                                                                       |
|-------------------|-----------------------------------------------------------------------------------|-------------------------------------------------------------------------------------|
| Global symmetry   | $PSU(2, 2 4)$                                                                     | $OSp(6 4)$                                                                          |
| Dynkin diagram    | 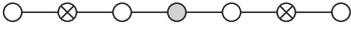 | 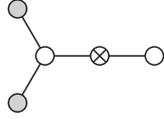 |
| Residual symmetry | $SU(2 2)_L \times SU(2 2)_R$                                                      | $SU(2 2)$                                                                           |
| Representations   | $(2 2)_L \otimes (2 2)_R = 16 \text{ d.o.f}$                                      | $(2 2)_A \oplus (2 2)_B = 8 \text{ d.o.f}$                                          |

**Table 1: Comparison of symmetries.** The Dynkin diagram of  $PSU(2, 2|4)$  contains two  $SU(2|2)$  branches which represent the residual symmetries, and exactly one momentum carrying root which we marked by shading it gray. This indicates that all 16 elementary excitations transform in a single irreducible representation with one fundamental index in each  $SU(2|2)$ . The Dynkin diagram of  $OSp(6|4)$  contains only one  $SU(2|2)$  branch, but two momentum carrying roots. Correspondingly, the 8 elementary excitations transform in two copies of the fundamental representation of  $SU(2|2)$ .

$Q = \frac{1}{2}$ . In the  $AdS_5/CFT_4$  case the function  $h(\lambda)$  turned out to be simply  $\sqrt{\lambda}/4\pi$ , which can be argued to arise from S-duality [9]. In the present case there is no such argument and indeed the function  $h$  happens to be quite non-trivial. The weak and strong coupling asymptotics are given by

$$h(\lambda) = \begin{cases} \lambda \left[ 1 + c_1 \lambda^2 + c_2 \lambda^4 + \dots \right] & \text{for } \lambda \ll 1, \\ \sqrt{\frac{\lambda}{2}} + a_1 + \frac{a_2}{\sqrt{\lambda}} + \dots & \text{for } \lambda \gg 1, \end{cases} \quad (1.8)$$

where the leading terms were deduced in [10, 11] and [11, 12], respectively. In fact, the  $\lambda$ -dependence of many other quantities like the S-matrix, the Bethe ansatz, the Zhukowsky map, the universal scaling function, etc., are also related between the  $AdS_5/CFT_4$  and the  $AdS_4/CFT_3$  correspondence by appropriately replacing  $\lambda$  by  $h(\lambda)$ . Despite this fact, the subleading terms seem to be scheme dependent. E.g. a worldsheet computation yields a non-zero  $a_1$  [13] while the algebraic curve computation produces  $a_1 = 0$  [14] which is also what is used in the Bethe ansatz proposal [15]. In order to unambiguously compare different approaches, one should therefore express all results in terms of a physical reference observable, and neither in terms of  $\lambda$  nor  $h(\lambda)$ .

## 2 $\mathcal{N} = 6$ Chern-Simons matter theory

**Field content.** ABJM theory is a three-dimensional superconformal Chern-Simons theory with product gauge group  $U(N) \times \hat{U}(N)$  at levels  $\pm k$  and specific matter content. The quiver diagram visualizing the fields of the theory and their gauge representations is drawn in Fig. 1. The entire field content is given by two gauge fields  $A_\mu$  and  $\hat{A}_\mu$ ,

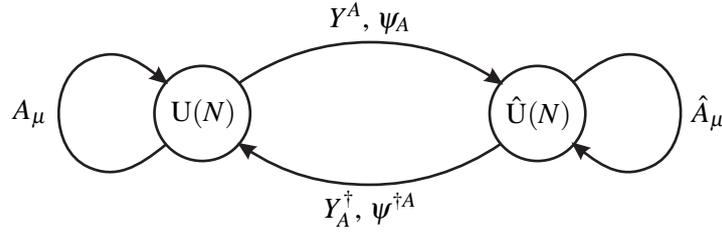

**Figure 1: Quiver diagram of ABJM theory.** The arrows indicate the representations of the fields under the gauge groups. The arrows are drawn from a fundamental to an anti-fundamental representation.

|               | $U(N)$         | $\hat{U}(N)$       | $SU(4)_R$          | $SU(2)_r$    | $U(1)_\Delta$ | $U(1)_b$ |
|---------------|----------------|--------------------|--------------------|--------------|---------------|----------|
| $A_\mu$       | $\mathbf{N}^2$ | $\mathbf{1}$       | $\mathbf{1}$       | $\mathbf{3}$ | 1             | 0        |
| $\hat{A}_\mu$ | $\mathbf{1}$   | $\mathbf{N}^2$     | $\mathbf{1}$       | $\mathbf{3}$ | 1             | 0        |
| $Y^A$         | $\mathbf{N}$   | $\bar{\mathbf{N}}$ | $\mathbf{4}$       | $\mathbf{1}$ | $\frac{1}{2}$ | 1        |
| $\psi_A$      | $\mathbf{N}$   | $\bar{\mathbf{N}}$ | $\bar{\mathbf{4}}$ | $\mathbf{2}$ | 1             | 1        |

**Table 2: Representations of ABJM fields.**

four complex scalar fields  $Y^A$ , and four Weyl-spinors  $\psi_A$ . The matter fields are  $N \times N$  matrices transforming in the bi-fundamental representation of the gauge group.

**Global symmetries.** The global symmetry group of ABJM theory, for Chern-Simons level<sup>4</sup>  $k > 2$ , is given by the orthosymplectic supergroup  $OSp(6|4)$  [2, 16] and the “baryonic”  $U(1)_b$  [2]. The bosonic components of  $OSp(6|4)$  are the R-symmetry group  $SO(6)_R \cong SU(4)_R$  and the 3d conformal group  $Sp(4) \cong SO(2, 3)$ . The conformal group contains the spacetime rotations  $SO(3)_r \cong SU(2)_r$  and dilatations  $SO(2)_\Delta \cong U(1)_\Delta$ . The fermionic part of  $OSp(6|4)$  generates the  $\mathcal{N} = 6$  supersymmetry transformations. The baryonic charge  $U(1)_b$  is +1 for bi-fundamental fields,  $-1$  for anti-bi-fundamental fields, and 0 for adjoint fields. The representations in which the fields transform under these symmetries are listed in Tab. 2. For more details about the  $OSp(6|4)$  group theory in this context see [17]. Finally, the model also possesses a discrete, parity-like symmetry. This might be surprising since the Chern-Simons action is not invariant but changes sign under a canonical parity transformation. The trick to make the model parity invariant is to accompany the “naive” parity transformation by the exchange of the two gauge group factors. The total transformation is a symmetry because the Chern-Simons terms for the two gauge group factors have opposite signs.

**Action.** The ABJM action was first spelled out in all detail in [18] in  $\mathcal{N} = 2$  superspace and in component form. An  $\mathcal{N} = 3$  [19], an  $\mathcal{N} = 1$  [20], and an  $\mathcal{N} = 6$  [21] superspace

<sup>4</sup>We are ignoring the symmetry enhancement to  $OSp(8|4)$  at  $k = 1$  and  $k = 2$ , because for the purpose of discussing integrability we have to work in the ’t Hooft limit where  $k$  is large.

version is also known. The component action using the conventions of [18] reads

$$\mathcal{S} = \frac{k}{4\pi} \int d^3x \left[ \epsilon^{\mu\nu\lambda} \text{tr} \left( A_\mu \partial_\nu A_\lambda + \frac{2i}{3} A_\mu A_\nu A_\lambda - \hat{A}_\mu \partial_\nu \hat{A}_\lambda - \frac{2i}{3} \hat{A}_\mu \hat{A}_\nu \hat{A}_\lambda \right) - \text{tr} (D_\mu Y)^\dagger D^\mu Y - i \text{tr} \psi^\dagger \not{D} \psi - V_{\text{ferm}} - V_{\text{bos}} \right], \quad (2.1)$$

where the sextic bosonic and quartic mixed potentials are

$$V^{\text{bos}} = -\frac{1}{12} \text{tr} \left[ Y^A Y_A^\dagger Y^B Y_B^\dagger Y^C Y_C^\dagger + Y_A^\dagger Y^A Y_B^\dagger Y^B Y_C^\dagger Y^C + 4Y^A Y_B^\dagger Y^C Y_A^\dagger Y^B Y_C^\dagger - 6Y^A Y_B^\dagger Y^B Y_A^\dagger Y^C Y_C^\dagger \right]. \quad (2.2)$$

$$V^{\text{ferm}} = \frac{i}{2} \text{tr} \left[ Y_A^\dagger Y^A \psi^{\dagger B} \psi_B - Y^A Y_A^\dagger \psi_B \psi^{\dagger B} + 2Y^A Y_B^\dagger \psi_A \psi^{\dagger B} - 2Y_A^\dagger Y^B \psi^{\dagger A} \psi_B - \epsilon^{ABCD} Y_A^\dagger \psi_B Y_C^\dagger \psi_D + \epsilon_{ABCD} Y^A \psi^{\dagger B} Y^C \psi^{\dagger D} \right]. \quad (2.3)$$

The covariant derivative acts on bi-fundamental fields as

$$D_\mu Y = \partial_\mu Y + i A_\mu Y - i Y \hat{A}_\mu, \quad (2.4)$$

while on anti-bi-fundamental fields it acts with  $A_\mu$  and  $\hat{A}_\mu$  interchanged. According to the M-theory interpretation, this theory describes the low-energy limit of  $N$  M2 branes probing a  $\mathbb{C}^4/\mathbb{Z}_k$  singularity. The three-dimensional spacetime of ABJM theory is the world-volume of those M2 branes. For conventions and further details we refer to [18].

**Perturbation theory and 't Hooft limit.** Note that the Chern-Simons level occurs in (2.1) as an overall factor of the entire action. Alternatively, one can rescale the fields in such a way that all quadratic terms come without any factors of  $k$  and interactions of order  $n$  come with  $\frac{1}{k^{n/2-1}}$ . Either way, this shows that  $g_{\text{CS}}^2 \equiv \frac{1}{k}$  acts like a coupling constant of ABJM theory, quite similar to  $g_{\text{YM}}^2$  in  $\mathcal{N} = 4$  SYM, though of course  $k$  has to be an integer to preserve non-abelian gauge symmetry. As announced in the introduction, the theory can be restricted to the planar sector by taking the 't Hooft limit (1.3) which introduces the effective coupling

$$\lambda \equiv g_{\text{CS}}^2 N = \frac{N}{k}. \quad (2.5)$$

In this limit the theory becomes integrable [10] (see also [11, 22]) in the same sense as we are used to in planar  $\mathcal{N} = 4$  SYM theory and as we will discuss below.

**Gauge group.** The model can be generalized to have gauge group  $U(M)_k \times U(N)_{-k}$  [23]. This generalization goes by the name ABJ theory. The M-theory interpretation is given by  $\min(M, N)$  M2 branes allowed to move freely on  $\mathbb{C}^4/\mathbb{Z}_k$  and  $|M - N|$  fractional M2 branes stuck to the singularity. The gauge theory action is formally the same as in (2.1), except that the matter fields are now given by rectangular matrices. Thus two 't Hooft couplings can be defined by

$$\lambda = \frac{M}{k}, \quad \hat{\lambda} = \frac{N}{k}, \quad (2.6)$$

and it becomes possible to take different planar limits depending on the ratio of  $\lambda$  and  $\hat{\lambda}$ . On the other hand, the generalized parity invariance of the ABJM theory is explicitly broken, because now the two gauge group factors cannot be exchanged anymore.

**Deformation.** It is possible to introduce independent Chern-Simons levels  $k$  and  $\hat{k}$  for the two gauge groups  $U(N)$  and  $\hat{U}(N)$  that do not sum to zero. This generalized theory possesses less supersymmetry and less global symmetry. It is proposed to be dual to a type IIA background with the Romans mass  $F_0 = k + \hat{k}$  turned on [24]. This modification, however, seems to break integrability [25].

### 3 From ABJM theory to the integrable model

**Spin-chain picture.** The integrability of the planar ABJM theory is best described in terms of an integrable  $OSp(6|4)$  spin-chain which represents single trace operators [10]. A qualitative difference between the case at hand and the case of  $\mathcal{N} = 4$  SYM is that the ABJM spin-chain is an “alternating spin-chain.” Because the matter fields are in bi-fundamental representations of the product gauge group  $U(N) \times \hat{U}(N)$ , gauge invariant operators need to be built from products of fields that transform alternatingly in the representations  $(\mathbf{N}, \bar{\mathbf{N}})$  and  $(\bar{\mathbf{N}}, \mathbf{N})$ , e.g.

$$\text{tr}(Y^1 Y_4^\dagger Y^1 Y_4^\dagger \dots). \quad (3.1)$$

Thus, the spin-chain has even length and the fields on the odd sites are distinct from the ones on the even sites. On the odd sites, we can have any of the  $4_B + 8_F$  fields  $Y^A$ ,  $\psi_{A\alpha}$ , and on the even sites, we can have any of the  $4_B + 8_F$  fields  $Y_A^\dagger$ ,  $\psi_\alpha^{\dagger A}$ . We can also act with an arbitrary number of derivatives  $D_\mu = D_{\alpha\beta}$  onto the fields, but derivatives do not introduce extra sites. Also field strength insertions do not count as extra sites as they can be written as anti-symmetrized derivatives.

**Spin-chain excitations.** In the spin-chain description, the ABJM fields are distinguished according to whether they represent the vacuum (or “down spin”), or elementary or multiple excitations. A convenient and common choice for the vacuum spin-chain is the BPS operator (3.1), i.e.  $Y^1$  is the vacuum on the odd sites, and  $Y_4^\dagger$  is the vacuum on the even sites.

Selecting a vacuum breaks the  $OSp(6|4)$  symmetry group of ABJM theory down to  $SU(2|2) \times U(1)_{\text{extra}}$  which becomes the symmetry group of the spin-chain model [10, 11]. The bosonic components of this  $SU(2|2)$  are  $SU(2)_G \times SU(2)_r \times U(1)_E$ , where  $SU(2)_G$  is the unbroken part of  $SU(4)_R$ ,  $SU(2)_r \cong SO(1, 2)_r$  is the Lorentz group, and  $U(1)_E$  is the spin-chain energy  $E = \Delta - J$  which itself is a combination of the conformal dimension  $\Delta$  and a broken  $SU(4)_R$  generator  $J$ . The charges of the fields under these groups are listed and explained in Tab. 3.

By construction, the ground state spin-chain (3.1) has energy  $E = \Delta - J = 0$ . This spin-chain can be excited by replacing one of the vacuum fields by a different field or by acting with a covariant derivative. This procedure increases the energy in quanta of

|                       | $SU(4)_R$<br>[ $p_1, q, p_2$ ] | $SU(2)_{G'}$<br>$J$ | $SU(2)_G$ | $U(1)_{\text{extra}}$ | $U(1)_\Delta$<br>$\Delta$ | $SU(2)_r$<br>$s$ | $U(1)_E$<br>$E = \Delta - J$ |
|-----------------------|--------------------------------|---------------------|-----------|-----------------------|---------------------------|------------------|------------------------------|
| $Y^1$                 | [1, 0, 0]                      | +1/2                | 0         | +1                    | 1/2                       | 0                | 0                            |
| $Y^2$                 | [-1, 1, 0]                     | 0                   | +1/2      | -1                    | 1/2                       | 0                | 1/2                          |
| $Y^3$                 | [0, -1, 1]                     | 0                   | -1/2      | -1                    | 1/2                       | 0                | 1/2                          |
| $Y^4$                 | [0, 0, -1]                     | -1/2                | 0         | +1                    | 1/2                       | 0                | 1                            |
| $\psi_{1\pm}$         | [-1, 0, 0]                     | -1/2                | 0         | -1                    | 1                         | $\pm 1/2$        | 3/2                          |
| $\psi_{2\pm}$         | [1, -1, 0]                     | 0                   | -1/2      | +1                    | 1                         | $\pm 1/2$        | 1                            |
| $\psi_{3\pm}$         | [0, 1, -1]                     | 0                   | +1/2      | +1                    | 1                         | $\pm 1/2$        | 1                            |
| $\psi_{4\pm}$         | [0, 0, 1]                      | +1/2                | 0         | -1                    | 1                         | $\pm 1/2$        | 1/2                          |
| $D_0$                 | [0, 0, 0]                      | 0                   | 0         | 0                     | 1                         | 0                | 1                            |
| $D_\pm$               | [0, 0, 0]                      | 0                   | 0         | 0                     | 1                         | $\pm 1$          | 1                            |
| $Y_1^\dagger$         | [-1, 0, 0]                     | -1/2                | 0         | -1                    | 1/2                       | 0                | 1                            |
| $Y_2^\dagger$         | [1, -1, 0]                     | 0                   | -1/2      | +1                    | 1/2                       | 0                | 1/2                          |
| $Y_3^\dagger$         | [0, 1, -1]                     | 0                   | +1/2      | +1                    | 1/2                       | 0                | 1/2                          |
| $Y_4^\dagger$         | [0, 0, 1]                      | +1/2                | 0         | -1                    | 1/2                       | 0                | 0                            |
| $\psi^{\dagger 1\pm}$ | [1, 0, 0]                      | +1/2                | 0         | +1                    | 1                         | $\pm 1/2$        | 1/2                          |
| $\psi^{\dagger 2\pm}$ | [-1, 1, 0]                     | 0                   | +1/2      | -1                    | 1                         | $\pm 1/2$        | 1                            |
| $\psi^{\dagger 3\pm}$ | [0, -1, 1]                     | 0                   | -1/2      | -1                    | 1                         | $\pm 1/2$        | 1                            |
| $\psi^{\dagger 4\pm}$ | [0, 0, -1]                     | -1/2                | 0         | +1                    | 1                         | $\pm 1/2$        | 3/2                          |

**Table 3: Charges of fields.** The R-symmetry group  $SO(6)_R \cong SU(4)_R$  splits up into  $SU(2)_{G'} \times SU(2)_G \times U(1)_{\text{extra}}$ , and the conformal group  $Sp(2, 2) \cong SO(2, 3)$  splits up into  $U(1)_\Delta \times SU(2)_r$ . The symmetry group of the spin-chain is  $SU(2|2) \times U(1)_{\text{extra}} \supset SU(2)_G \times SU(2)_r \times U(1)_E \times U(1)_{\text{extra}}$ . The  $U(1)_J$  generator  $J = \frac{p_1 + q + p_2}{2}$  is the Cartan generator of  $SU(2)_{G'}$ , and the  $U(1)_E$  generator  $E$  is given by the difference  $\Delta - J$ .

$\delta E = 1/2$  by a total amount that can be read off from the last column in Tab. 3. If the energy increases by 1/2, then the excitation is an elementary one. We find that the elementary excitations on the odd and even sites are given by

$$\text{“A”-particles: } (Y^2, Y^3 | \psi_{4+}, \psi_{4-}), \quad (3.2a)$$

$$\text{“B”-particles: } (Y_3^\dagger, Y_2^\dagger | \psi_+^{\dagger 1}, \psi_-^{\dagger 1}), \quad (3.2b)$$

respectively [11]. These are the two multiplets anticipated in (1.6). All other fields correspond to composite excitations and are listed in Tab. 4.

**Subsectors.** A subsector is a set of fields which is closed under the action of the spin-chain Hamiltonian, i.e. there is no overlap between spin-chains from within a subsector with spin-chains from outside. The subsectors of ABJM theory above the vacuum (3.1) are listed in Tab. 5. To prove that these sectors are closed to all orders in perturbation theory, one defines a positive semi-definite charge  $P = n_1 p_1 + n_2 q + n_3 p_2 + n_4 \Delta + n_5 s + n_6 b \geq 0$  from the eigenvalues of all operators that commute with the spin-chain Hamiltonian  $E = \Delta - J$ . These are the 5 Cartan generators of  $OSp(6|4)$  and the baryonic charge  $U(1)_b$ . The set of fields with  $P = 0$  constitute a closed subsector. Different subsectors are obtained by different choices for the numbers  $n_i$ .

**Spin-chain Hamiltonian.** Various works have computed the spin-chain Hamiltonian for different subsectors to different loop orders with different methods in different ap-

|                    | Multi-excitation                                                                                                               | made of                                                                                                                                 |
|--------------------|--------------------------------------------------------------------------------------------------------------------------------|-----------------------------------------------------------------------------------------------------------------------------------------|
| Double excitations | $Y_1^\dagger Y^1, Y^4 Y_4^\dagger$<br>$\psi_2 Y_4^\dagger, \psi^{\dagger 3} Y^1$<br>$\psi_3 Y_4^\dagger, \psi^{\dagger 2} Y^1$ | $Y^2 Y_2^\dagger \pm Y^3 Y_3^\dagger$<br>$\psi_4 Y_2^\dagger \pm Y^3 \psi^{\dagger 1}$<br>$\psi_4 Y_3^\dagger \pm Y^2 \psi^{\dagger 1}$ |
| Triple excitations | $\psi_1 Y_4^\dagger Y^1$<br>$\psi^{\dagger 4} Y^1 Y_4^\dagger$<br>$D_\mu Y^1 Y_4^\dagger$                                      | $Y^2 \psi^{\dagger 1} Y^3$<br>$Y_2^\dagger \psi_4 Y_3^\dagger$<br>$\psi_4 \gamma_\mu \psi^{\dagger 1}$                                  |

**Table 4: Multi-excitations.** In order to determine which elementary excitations a composite is made out of, one needs to compare their  $SU(2|2) \times U(1)_{\text{extra}}$  charges. E.g. for the triple excitation  $\psi_1$  one can check that the charges of  $\psi_1$  together with the two background fields  $Y^1 Y_4^\dagger$  coincide with the charges of the three elementary excitations  $Y^2 \psi^{\dagger 1} Y^3$ .

| Subsector            | Vacuum            | Single                                         | Double                             |
|----------------------|-------------------|------------------------------------------------|------------------------------------|
| Vacuum               | $Y^1 Y_4^\dagger$ |                                                |                                    |
| $SU(2) \times SU(2)$ | $Y^1 Y_4^\dagger$ | $Y^2 Y_3^\dagger$                              |                                    |
| $OSp(2 2)$           | $Y^1 Y_4^\dagger$ | $\psi_{4+} \psi_+^{\dagger 1}$                 | $D_+$                              |
| $OSp(4 2)$           | $Y^1 Y_4^\dagger$ | $Y^2 \psi_{4+} Y_3^\dagger \psi_+^{\dagger 1}$ | $D_+ \psi_{3+} \psi_+^{\dagger 2}$ |
| $SU(2)$              | $Y^1 Y_4^\dagger$ | $Y^2$                                          |                                    |
| $SU(1 1)$            | $Y^1 Y_4^\dagger$ | $\psi_{4+}$                                    |                                    |
| $SU(2 1)$            | $Y^1 Y_4^\dagger$ | $Y^2 \psi_{4+}$                                |                                    |
| $SU(3 2)$            | $Y^1 Y_4^\dagger$ | $Y^2 Y^3 \psi_{4+} \psi_{4-}$                  |                                    |

**Table 5: Subsectors.** This list of closed subsectors above the vacuum  $\text{tr}(Y^1 Y_4^\dagger Y^1 Y_4^\dagger \dots)$  is complete, although a specific subsector can be realized also by other fields. That would correspond to a different embedding of the sector into the full theory. Note that there is no closed  $SL(2)$  sector that is made only out of derivatives as we had in  $\mathcal{N} = 4$  SYM. This is because derivatives are double excitations of fermions with the above choice of vacuum. However, it is also possible to consider closed subsectors based on a different vacuum. There is, for instance, an  $SL(2)$  sector built from derivatives onto the vacuum  $\text{tr}(Y^1 \psi^{\dagger 1})^L$  [26], which was studied e.g. in [27].

proximations. The first results were obtained in the  $SU(4)$  sector<sup>5</sup> at two<sup>6</sup> loops [10, 22] where the spin-chain Hamiltonian reads

$$H = \frac{\lambda^2}{2} \sum_{l=1}^{2L} (2 - 2P_{l,l+2} + P_{l,l+2}K_{l,l+1} + K_{l,l+1}P_{l,l+2}). \quad (3.3)$$

with  $P_{l,m}$  and  $K_{l,m}$  being the permutation and the trace operator, respectively, and  $2L$  being the length of the spin-chain. This Hamiltonian has been proven to be integrable by means of an algebraic Bethe ansatz [10, 22]. In the  $SU(2) \times SU(2)$  sector, independently studied in [11], the trace operators annihilate the states and the Hamiltonian reduces to the sum of two decoupled Heisenberg  $XXX_{1/2}$  Hamiltonians, one acting onto the even sites and one acting onto the odd sites. The only coupling between these two sublattices comes from the cyclicity condition which says that the *total* momentum of all excitations has to be zero (mod  $2\pi$ ), not individually for the even and odd sites. Nevertheless, the Hamiltonians will continue to be decoupled up to six loop order [15].

The extension of the two-loop Hamiltonian to the full theory was derived in [26] and [28]. The integrability in the  $OSp(4|2)$  sector was proved by means of a Yangian construction [26]. The generalization to ABJ theory at two loops was studied in the scalar sector [29] and the full theory [28], which at this perturbative order amounts to replacing  $\lambda^2$  in the ABJM result by  $\lambda\hat{\lambda}$ , cf. (2.6). That means that the absence of parity in ABJ theory is not visible at two loop order.

Beyond two loops only the dispersion relation, i.e. the eigenvalue of the Hamiltonian on spin-chains with a single excitation, is known to date. It is of the general form (1.7). The expansion of the interpolating function  $h$  to four-loop order was computed for the ABJM and the ABJ theory in [30–32] with the result

$$h^2(\lambda, \hat{\lambda}) = \lambda\hat{\lambda} - (\lambda\hat{\lambda})^2 \left[ \frac{2\pi^2}{3} + \frac{\pi^2}{6} \left( \frac{\lambda - \hat{\lambda}}{\sqrt{\lambda\hat{\lambda}}} \right)^2 \right], \quad (3.4)$$

where the ABJM expression is obtained from this by setting the two 't Hooft couplings equal to each other. We see that  $h(\lambda, \lambda)$  is for the form (1.8) with  $c_1 = -\pi^2/3$ . Note that (3.4) is invariant under the exchange of  $\lambda$  and  $\hat{\lambda}$ , even though ABJ theory lacks manifest parity invariance. The fact that parity is not broken in the spin-chain picture is *not* a consequence of integrability, because as shown in [29] there are integrable but parity breaking spin-chain Hamiltonians already at two loops. Alternative explanations for the non-visibility of parity breaking were proposed [29]. In ABJ theory one can also study the limit  $\lambda \gg \hat{\lambda}$  [30]. In this limit, the Hamiltonian of the  $SU(2) \times SU(2)$  sector is, at any loop order, proportional to two decoupled Heisenberg spin-chain Hamiltonians [30]. An exact expression for the  $\lambda$ -dependent prefactor, which gives a prediction for the function  $h(\lambda, \hat{\lambda})$  in the limit  $\hat{\lambda} \ll \lambda$ , has been conjectured in [33]. Very recently, even for the case when  $\lambda = \hat{\lambda}$  an all-order guess for  $h^2(\lambda)$  was made [32], that is in line with the weak and strong coupling data.

<sup>5</sup>This sector is closed at two-loop order but not beyond.

<sup>6</sup>There is no contribution to the Hamiltonian at an odd number of loops as in three dimensions no such Feynman diagram is logarithmically divergent.

At six loops only a subset of Feynman diagrams have been evaluated, namely those which move the impurities along the spin-chain by the maximal amount that is possible at this loop order [34]. The contributions from this subset to the dilatation operator are consistent with the corresponding spin-chain being integrable [34].

Also non-planar contributions to the two-loop dilatation operator have been computed in the  $SU(2) \times SU(2)$  sector [35]. The degeneracy of the dimensions of parity pairs at the planar level, which is a signature of integrability, is lifted by the non-planar contributions [35]. At the non-planar level, one can also observe the breaking of parity in the ABJ theory already at two loops [36].

## 4 Superstrings on $AdS_4 \times CP^3$

**String background.**  $AdS_4 \times CP^3$  with two- and four-form fluxes turned on is a solution to IIA supergravity that preserves 24 out of 32 supersymmetries [37], i.e. unlike  $AdS_5 \times S^5$  it is not maximally supersymmetric. The  $AdS_4 \times CP^3$  superspace geometry has been constructed in [38]. The fermionic coordinates  $\Theta^{1..32} = (\vartheta^{1..24}, \nu^{1..8})$  split into 24 coordinates  $\vartheta$ , which correspond to the unbroken supersymmetries of the background, and eight coordinates  $\nu$  corresponding to the broken supersymmetries.

**Green-Schwarz action.** Although formal expressions for the Green-Schwarz superstring action exist for any type II supergravity background [39], in practice it is generically hopeless to find exact expressions for the supervielbeins. Nevertheless, utilizing the connection to M-theory on  $AdS_4 \times S^7$ , all functions that are required to write down the Nambu-Goto form of the action, in particular the supervielbeins and the NS-NS two-form superfield, were explicitly spelled out in [38], and the simpler  $\kappa$ -gauge-fixed version was given in [40]. However, it is probably fair to say that working with this action is still quite cumbersome as the explicit expressions are rather involved.

**Coset action.** A more pragmatic approach to strings on  $AdS_4 \times CP^3$  has been taken in [41] and [42]. The observation is that  $AdS_4$  is the coset  $SO(2, 3)/SO(1, 3)$  and  $CP^3$  is the coset  $SO(6)/U(3)$ , and that  $SO(2, 3) \times SO(6)$  is the bosonic subgroup of  $O\text{Sp}(6|4)$ . Thus the idea is to write the superstrings action as a sigma-model on the supercoset

$$\frac{O\text{Sp}(6|4)}{SO(1, 3) \times U(3)}, \quad (4.1)$$

analogously to the  $PSU(2, 2|4)/SO(1, 4) \times SO(5)$  coset model for superstrings on  $AdS_5 \times S^5$  [43], which itself was inspired by the WZW-type action for strings in flat space [44]. Again it is possible to define a  $\mathbb{Z}_4$  grading [45] of the (complexified) algebra [41, 42], and when this grading is used to split up the current one-form  $A = -g^{-1}dg = A^{(0)} + A^{(1)} + A^{(2)} + A^{(3)}$ , constructed from a parametrization of the coset representatives  $g$ , then the coset action is given by

$$\mathcal{S} = -\frac{R^2}{4\pi\alpha'} \int d\sigma d\tau \text{str} \left[ \sqrt{-h} h^{\alpha\beta} A_\alpha^{(2)} A_\beta^{(2)} + \kappa \epsilon^{\alpha\beta} A_\alpha^{(1)} A_\beta^{(3)} \right]. \quad (4.2)$$

The explicit form of this sigma-model action can look quite differently depending on the choice of coset representative and the choice of gauge [41, 42, 46, 47].

**Fermions,  $\kappa$ -symmetry and singular configurations.** There is a subtle problem with the coset action (4.2). The supercoset (4.1) has only 24 fermionic directions, which is the number of supersymmetries preserved by the background. However, independent of how many supersymmetries are preserved, the Green-Schwarz superstring always requires two Majorana-Weyl fermions with a total number of 32 degrees of freedom. Thus the coset model misses 8 fermions and can therefore not be equivalent to the GS string! This problem did not exist in the case of  $AdS_5 \times S^5$  because that background is maximally supersymmetric and the corresponding supercoset has 32 fermionic directions.

It has been argued that the eight missing fermions  $\nu$  are part of the 16 fermionic degrees of freedom that due to  $\kappa$ -gauge symmetry are unphysical anyway, i.e. to think of the coset action on (4.1) as an action with  $\kappa$ -symmetry partially gauge-fixed. Of the remaining 24 fermions  $\vartheta$ , further 8 should then be unphysical. For this interpretation to be correct, the rank of  $\kappa$ -symmetry of the coset action must be 8. This is in fact true for generic bosonic configurations [41, 42], unfortunately however not for strings that move only in the AdS part of the background, in which case the rank of  $\kappa$ -symmetry is 12 [41]. This means that on such a “singular configuration” the coset model is a truncation of the GS string where instead of removing 8 unphysical fermions (from 32 to 24), 4 physical fermions have been put to zero, while 4 unphysical fermions have been retained.

The upshot is that the coset model is generically equivalent to the GS string, but *not* on singular backgrounds. The consequence is that these singular backgrounds cannot be quantized semi-classically within the coset description.

**Near plane-wave expansion.** One method for dealing with a curved RR-background at the quantum level is to take a Penrose limit of the geometry which leads to a solvable plane-wave background and then to include curvature corrections perturbatively. Penrose limits of the  $AdS_4 \times CP^3$  background were studied in [48, 11, 12, 49, 50]. The near plane-wave Hamiltonian was derived in a truncation<sup>7</sup> to the bosonic sector in [51], for a sector including fermions in [52], and for the full theory in [49].

**Alternative approaches.** The pure spinor formulation of the superstring on  $AdS_4 \times CP^3$  was developed in [53]. This approach is suitable for the covariant quantization of the string. Another possibility to obtain an action for the  $AdS_4 \times CP^3$  string is to start from the supermembrane on  $AdS_4 \times S^7$  and perform a double dimensional reduction [54].

## 5 From $AdS_4 \times CP^3$ to the integrable model

**Evidence for integrability.** The purely bosonic sigma-model on  $AdS_4 \times CP^3$  is integrable at the classical level, though quantum corrections spoil the integrability [55]. For

---

<sup>7</sup>This truncation is not consistent and the absence of the fermions yields divergences, which were regularized using  $\zeta$ -function regularization. Up to so-called “non-analytic” terms, the result is correct.

| field                         | mass       | dispersion relation                                 |
|-------------------------------|------------|-----------------------------------------------------|
| $t, \psi$                     | 0          | $\omega_n = n$                                      |
| $x_{1,2,3}, \xi$              | $\kappa$   | $\omega_n = \sqrt{\kappa^2 + n^2}$                  |
| $\theta_{1,2}, \varphi_{1,2}$ | $\kappa/2$ | $\omega_n = \sqrt{(\kappa/2)^2 + n^2} \pm \kappa/2$ |

**Table 6: Spectrum of fluctuations about the point-like string.** Two linear combinations of  $\theta_{1,2}$  and  $\varphi_{1,2}$  possess the dispersion relation with  $+\kappa/2$ , and two other linear combinations the one with  $-\kappa/2$ .

the super-coset model, classical integrability is also proven [41, 42]. The Lax connection found in [56] for the  $AdS_5 \times S^5$  case as a means of writing the equations of motion in a manifestly integrable form is directly applicable here. Moreover, the absence of particle production in the coset sigma-model has been shown explicitly for bosonic amplitudes at tree-level [57]. However, we know that the full GS string is more than the coset model. Therefore, although there are generic arguments in favor of the integrability of the whole theory, the direct proof of the integrability of the complete  $AdS_4 \times CP^3$  superstring still remains an open problem [40]. Different integrable reductions of the sigma model have also been studied [58, 59].

**Matching  $AdS_4 \times CP^3$  to ABJM theory.** The metric on  $AdS_4 \times CP^3$  has the two factors

$$ds^2 = R^2 \left[ \frac{1}{4} ds_{AdS_4}^2 + ds_{CP^3}^2 \right], \quad (5.1)$$

where  $R$  is the radius of  $CP^3$  which is twice the radius of  $AdS_4$ . This relative size is demanded by supersymmetry and comes out automatically when one starts from the coset action (4.2). The radius  $R$  is related to the 't Hooft coupling  $\lambda$  of ABJM theory by (1.4). In global coordinates the metric for  $AdS_4$  reads

$$ds_{AdS_4}^2 = -\cosh^2 \rho dt^2 + d\rho^2 + \sinh^2 \rho (d\theta^2 + \sin^2 \theta d\varphi^2) \quad (5.2)$$

with coordinate ranges  $\rho = 0 \dots \infty$ ,  $t = -\infty \dots \infty$ ,  $\theta = 0 \dots \pi$ , and  $\varphi = 0 \dots 2\pi$ . The metric on  $CP^3$  is the standard Fubini-Study metric and can be written as

$$ds_{CP^3}^2 = d\xi^2 + \cos^2 \xi \sin^2 \xi \left[ d\psi + \frac{1}{2} \cos \theta_1 d\varphi_1 - \frac{1}{2} \cos \theta_2 d\varphi_2 \right]^2 + \frac{1}{4} \cos^2 \xi \left[ d\theta_1^2 + \sin^2 \theta_1 d\varphi_1^2 \right] + \frac{1}{4} \sin^2 \xi \left[ d\theta_2^2 + \sin^2 \theta_2 d\varphi_2^2 \right]. \quad (5.3)$$

The coordinates  $(\theta_1, \varphi_1)$  and  $(\theta_2, \varphi_2)$  parameterize two two-spheres, the angle  $\xi = 0 \dots \frac{\pi}{2}$  determines their radii, and the angle  $\psi = 0 \dots 2\pi$  corresponds to the  $U(1)_R$  isometry.

The background admits five Killing vectors

$$E = -i\partial_t \quad , \quad S = -i\partial_\varphi \quad , \quad J_{\varphi_1} = -i\partial_{\varphi_1} \quad , \quad J_{\varphi_2} = -i\partial_{\varphi_2} \quad , \quad J_\psi = -i\partial_\psi \quad (5.4)$$

leading to the five conserved charges: the worldsheet energy  $E$ , the AdS-spin  $S$  and the  $CP^3$  momenta  $J_{\varphi_1}$ ,  $J_{\varphi_2}$ , and  $J_\psi$ . Note that this is one conserved charge less than in the

$AdS_5 \times S^5$  case where there are two AdS-spins. This shows that  $AdS_4 \times CP^3$  is less symmetric. The charges (5.4) are one choice of Cartan generators of  $SO(3, 2) \times SU(4)$ . The angular momenta  $J_{\varphi_1}$  and  $J_{\varphi_2}$  correspond to the Cartan generators of two  $SU(2)$  subgroups that on the gauge theory side transform  $(Y^1, Y^2)$  and  $(Y^3, Y^4)$ , respectively. The angular momentum  $J_\psi$  is the  $U(1)_R$  generator. Thus, the angular momenta are related to the charges in Tab. 3 according to

$$J_{\varphi_1} = \frac{1}{2}p_1 \quad , \quad J_{\varphi_2} = \frac{1}{2}p_2 \quad , \quad J_\psi = q + \frac{1}{2}(p_1 + p_2) . \quad (5.5)$$

These relations are important for identifying classical strings with gauge theory operators. It also suggests a parametrization of  $CP^3$  inside  $\mathbb{C}^4$  in terms of the embedding coordinates

$$\begin{aligned} y^1 &= \cos \xi \cos \frac{\theta_1}{2} e^{i(+\varphi_1+\psi)/2} & y^3 &= \sin \xi \cos \frac{\theta_2}{2} e^{i(+\varphi_2-\psi)/2} \\ y^2 &= \cos \xi \sin \frac{\theta_1}{2} e^{i(-\varphi_1+\psi)/2} & y^4 &= \sin \xi \sin \frac{\theta_2}{2} e^{i(-\varphi_2-\psi)/2} \end{aligned} \quad (5.6)$$

which can be identified one-to-one with the scalar fields  $Y^A$  of ABJM theory.

**Worldsheet spectrum.** In order to relate the string description to the spin-chain picture, we need to quantize the worldsheet theory. It is only known how to do this by semiclassical means, i.e. by expanding the string about a classical solution and quantizing the fluctuations. As can be seen from the charges, the classical string solution that corresponds to the vacuum spin-chain, or in other words to the gauge theory operator  $\text{tr}(Y^1 Y_4^\dagger)^L$  (with  $L$  large so that the string becomes classical), is a point-like string that moves along the geodesic parametrized by  $t = \kappa\tau$ ,  $\psi = \kappa\tau$ , located at the center of  $AdS_4$  ( $\rho = 0$ ) and the equator of  $CP^3$  ( $\xi = \pi/4$ ), and furthermore sitting at the north pole of the first sphere ( $\theta_1 = 0$ ) and at the south pole of the other sphere ( $\theta_2 = \pi$ ). Expanding the fields in fluctuations of order  $\lambda^{-1/4}$  yields the mass spectrum given in Tab. 6.

The massless fluctuations  $\tilde{t}$  and  $\tilde{\psi}$  can be gauged away, i.e. set to zero. This is the usual light-cone gauge,  $t + \psi \sim \tau$ , with one light-cone direction in  $AdS_4$  and one in  $CP^3$ . We are left with 4 light excitations  $(\theta_{1,2}, \varphi_{1,2})$  from  $CP^3$  and 4 heavy excitations of which one ( $\xi$ ) comes from  $CP^3$  and the other three  $(x_{1,2,3})$  from  $AdS_4$ . For the eight physical fermions the same pattern is found: 4 light excitations of mass  $\kappa/2$  and 4 heavy excitations of mass  $\kappa$ .

These worldsheet modes transform in definite representations of the residual symmetry group  $SU(2|2) \times U(1)_{\text{extra}}$  that is left after fixing the light-cone gauge [60]. The light fields form two  $(2|2)$ -dimensional supermultiplets [47]

$$\text{“A”-particles:} \quad (X^a, \psi_\alpha) , \quad (5.7a)$$

$$\text{“B”-particles:} \quad (X_a^\dagger, \psi^{\dagger\alpha}) , \quad (5.7b)$$

where  $a = 1, 2$  and  $\alpha = 1, 2$  are  $SU(2)_G \times SU(2)_r$  indices. The doublet of complex scalars  $X^a$  is a combination of  $\theta_{1,2}$  and  $\varphi_{1,2}$ , and the fermions are written in terms of a complex spinor  $\psi_\alpha$ . These two supermultiplets correspond precisely to the  $A$ - and  $B$ -particles (3.2) in the spin-chain picture, respectively!

The heavy fields form one (1|4|3)-dimensional supermultiplet  $(\xi, \chi_\alpha^a, x_{1,2,3})$  [47]. The bosonic components are literally the coordinates used above, and the fermionic component is a doublet of Majorana spinors. These heavy fields, however, do not count as independent excitations in the spin-chain description, they are rather an artifact of the above analysis which is done at infinite coupling  $\lambda$ . When going to finite coupling they “dissolve” into two light particles [47]. At the technical level this is seen by looking at which particle poles appear in Green’s functions at *not* strictly infinite coupling [47, 52]. The first observation is that in the free theory the pole for the heavy particles with mass  $\kappa$  coincides with the branch point of the branch cut that accounts for the pair production of two light modes with mass  $\frac{\kappa}{2}$  each. When interactions are turned on, i.e. when  $1/\sqrt{\lambda}$  corrections are considered, the pole moves into the branch cut, and the statement is that the exact propagator has a branch cut only.

**Giant magnons.** As we have just seen, the worldsheet fluctuations match the spin-chain excitations, but only as far as their charges are concerned. The dispersion relation of the worldsheet excitations is relativistic rather than periodic as in (1.7). In order to see the periodic dispersion relation also on the string theory side, macroscopically many quanta must be excited. The result are classical string solutions known as giant magnons [61], or dyonic giant magnons [62, 63] if they have at least two non-zero angular momenta. The dispersion relation of all dyonic giant magnons are of the form (1.7) for appropriate values for  $Q$ .

The variety of giant magnons in  $CP^3$  is somewhat larger than in  $S^5$ . The simplest types are obtained by embedding the HM giant magnon [61] into subspaces of  $CP^3$  [11] (see also [64]). There are two essentially different choices: one may either pick a proper two-sphere inside  $CP^3$  or a two-sphere with antipodes identified. According to these subspaces the former choice leads to what is called the  $CP^1$  ( $\cong S^2$ ) giant magnon [11] and the latter choice to the so-called  $RP^2$  ( $\cong S^2/\mathbb{Z}_2$ ) giant magnon [11, 12].

The  $RP^2$  giant magnon is in fact a threshold bound state of two HM giant magnons, one inside each of the  $S^2$ s parametrized by  $(\theta_1, \varphi_1)$  and  $(\theta_2, \varphi_2)$  in (5.3) [12]. Therefore this kind of giant magnon is sometimes referred to as the  $S^2 \times S^2$  magnon or as the  $SU(2) \times SU(2)$  magnon. This is, however, somewhat misleading as the two constituent magnons do not move independently.

The dyonic generalization of the  $CP^1$  giant magnon moves in a  $CP^2$  subspace of  $CP^3$  and was found for momentum  $p = \pi$  in [65] and for general momenta in [66]. This giant magnon does not have an analogue in  $AdS_5 \times S^5$ . The  $CP^2$  dyonic giant magnons are in one-to-one correspondence with the elementary spin chain excitations (3.2): the polarizations of the giant magnons match the flavors of the excitations [67]. In [67] it has also been shown, that the classical phase shifts in the scattering of these dyonic giant magnons are consistent with the S-matrix proposed by [68]. The general scattering solutions of  $N$  giant magnons have also been known since very recently [69], in fact for the much wider context of giant magnons on  $CP^n$ ,  $SU(n)$  and  $S^n$  [70].

The dyonic generalization of the  $RP^2$  giant magnon moves in a  $RP^3$  subspace of  $CP^3$  and was found in [58]. This giant magnon is the CDO dyonic giant magnon on  $S^3$  [63] embedded into  $RP^3$ . It can be regarded as a composite of two  $CP^2$  dyonic magnons with

equal momenta [67]. Finally, by the dressing method one can also find a two-parameter one-charge solution [66, 71].

## 6 Solving $AdS_4/CFT_3$ using integrability

In this section, we will briefly discuss those aspects of the methods employed to solve the  $AdS_4/CFT_3$  model that differ from the ones in the  $AdS_5/CFT_4$  case. For an introduction to these tools, we refer to the other chapters of this review. For the Bethe ansatz see [72], for the S-matrix see [73], for the algebraic curve see [74], and for the thermodynamic Bethe ansatz and the Y-system see [75].

**Asymptotic Bethe equations.** The Bethe equations for the two-loop  $SU(4)$  sector were derived within the algebraic Bethe ansatz scheme in [10], where also the extension of the Bethe equations to the full theory, though still at one loop, were conjectured. The form of these equations is quite canonical and the couplings between the Bethe roots is encoded in the Dynkin diagram of  $OSp(6|4)$ , see Tab. 1. The all-loop extension of the Bethe equations was conjectured in [15].

The fact that we now have two types of momentum carrying roots—call them  $u$  and  $v$ —means that the conserved charges are given by sums over all roots of both of these kinds

$$Q_n = \sum_{j=1}^{K_u} q_n(u_j) + \sum_{j=1}^{K_v} q_n(v_j), \quad (6.1)$$

where  $q_n$  is the charge carried by a single root. The spin-chain energy, or anomalous dimension, or string light-cone energy, is the second charge  $E = h(\lambda)Q_2$ . The other Bethe roots—call them  $r$ ,  $s$ , and  $w$ —are auxiliary roots and influence the spectrum only indirectly through their presence in the Bethe equations.

The  $SU(2) \times SU(2)$  sector is given by only exciting the momentum carrying roots. The  $SU(4)$  sector uses the roots  $u$ ,  $v$ ,  $r$ , though this sector is only closed at two loops. The four components of an  $A$ -particle, cf. (3.2) and (5.7), correspond to the states with one  $u$  root and excitation numbers  $\{K_r, K_s, K_w\} = \{0, 0, 0\}$ , or  $\{1, 0, 0\}$ , or  $\{1, 1, 0\}$ , or  $\{1, 1, 1\}$  for the auxiliary roots. The same holds for the  $B$ -particle if the  $u$ -root is replaced by one of type  $v$ . This accounts for all light excitations. The heavy excitations are given by a stack of one of each kind of the momentum carrying roots. This is the Bethe ansatz way of seeing that the heavy excitations are compounds.

This Bethe ansatz has been put to a systematic test by comparing the predicted eigenvalues to the direct diagonalization of the spin-chain Hamiltonian for various length-4 and length-6 states at two loops [76].

**S-Matrix.** It has been shown that the proposed all-loop Bethe ansatz can be derived from an exact two-particle S-matrix [68]. The alternating nature of the spin-chain, naturally breaks the S-matrix up into pieces: interactions between two  $A$ -particles, between two  $B$ -particles, and between one of each kind [68], where each piece is proportional

to the old and famous  $SU(2|2)$  S-matrix [7, 77] from  $AdS_5/CFT_4$ . Crossing symmetry relates  $AA$ - and  $BB$ - to  $AB$ -scattering and therefore does not fix the overall scalar factor for any of them uniquely. A solution that is consistent with the Bethe equations was made in [68] and uses the BES dressing phase [78].

This S-matrix does not have poles that correspond to the heavy particles, which is in line with them not being asymptotic states. The heavy particles occur, however, as intermediate states. That is seen from the fact that they appear as internal lines in the Feynman diagrams that are used to derive the worldsheet S-matrix from scattering amplitudes [47].

The S-matrix has the peculiarity that the scattering of  $A$ - and  $B$ -particles is reflectionless [79]. Though at first unexpected, this property has been confirmed perturbatively at weak [80] and at strong coupling [47]. This reflectionlessness would follow straightforwardly if one assumes that the two terms in (6.1) were individually conserved [81].

**Algebraic curve.** The algebraic curve for the  $AdS_4/CFT_3$  duality was constructed from the string coset sigma-model in [82]. It is a ten-sheeted Riemann surface  $q(x)$  whose branches—or quasi-momenta—are pairwise related  $q_{1,2,3,4,5} = -q_{10,9,8,7,6}$ . The physical domain is defined for spectral parameter  $|x| > 1$ . The values of the quasi momenta within the unit circle are related to their values outside it by an inversion rule [82]. Branch cut and pole conditions are identical to the ones in the  $AdS_5/CFT_4$  case. The Virasoro constraints demand that the quasi momenta  $q_1, \dots, q_4$  all have a pole with the same residue at  $x = 1$  and another one at  $x = -1$ , while the quasi momentum  $q_5$  cannot have a pole at  $x = \pm 1$ .

For a given algebraic curve, the charges of the corresponding string solution are encoded in the large  $x$  asymptotics. E.g. the curve

$$q_1(x) = \dots = q_4(x) = \frac{L}{2g} \frac{x}{x^2 - 1} \quad , \quad q_5(x) = 0 \quad . \quad (6.2)$$

carries the charges  $(\Delta_0, S, J_{\varphi_1}, J_{\varphi_2}, J_\psi) = (L, 0, \frac{L}{2}, \frac{L}{2}, L)$  and  $\delta\Delta = 0$  of  $\text{tr}(Y^1 Y_4^\dagger)^L$  and thus corresponds to the vacuum. String excitations are represented by additional poles that connect the various branches. A dictionary between the polarizations of the excitations and the different branch connections is given in [82]. The light modes can be recognized as those which connect a non-trivial sheet with a trivial sheet in (6.2), and the heavy modes are those which connect two non-trivial sheets.

**Thermodynamic Bethe ansatz and Y-system.** The Y-system for the  $OSp(6|4)$  spin-chain was conjectured along with the corresponding equations for  $AdS_5/CFT_4$  in [83]. A derivation of the Y-system, i.e. writing down the asymptotic Bethe ansatz at finite temperature for the mirror theory, formulating the string hypothesis, and Wick rotating back to the original theory, was performed in [84] and [85], and a modification of the original conjecture was found.

## Acknowledgements

I am very happy to thank T. McLoughlin and O. Ohlsson Sax for numerous very helpful discussions. Part of this review was written while I was still affiliated with the Princeton Center for Theoretical Science whom I thank for their support.

## References

- [1] N. Beisert et al., “*Review of AdS/CFT Integrability: An Overview*”, [arxiv:1012.3982](#).
- [2] O. Aharony, O. Bergman, D. L. Jafferis and J. Maldacena, “ *$\mathcal{N} = 6$  superconformal Chern-Simons-matter theories, M2-branes and their gravity duals*”, JHEP 0810, 091 (2008), [arxiv:0806.1218](#).
- [3] A. Babichenko, B. Stefański, Jr. and K. Zarembo, “*Integrability and the AdS(3)/CFT(2) correspondence*”, JHEP 1003, 058 (2010), [arxiv:0912.1723](#).
- [4] O. Bergman and S. Hirano, “*Anomalous radius shift in AdS<sub>4</sub>/CFT<sub>3</sub>*”, JHEP 0907, 016 (2009), [arxiv:0902.1743](#).
- [5] I. R. Klebanov and G. Torri, “*M2-branes and AdS/CFT*”, Int. J. Mod. Phys. A25, 332 (2010), [arxiv:0909.1580](#).
- [6] T. Klose and T. McLoughlin, “*Integrability in AdS<sub>4</sub>/CFT<sub>3</sub>*”, in preparation.
- [7] N. Beisert, “*The su(2/2) dynamic S-matrix*”, Adv. Theor. Math. Phys. 12, 945 (2008), [hep-th/0511082](#).
- [8] D. Berenstein and D. Trancanelli, “*Three-dimensional  $\mathcal{N} = 6$  SCFT’s and their membrane dynamics*”, Phys. Rev. D78, 106009 (2008), [arxiv:0808.2503](#).
- [9] D. Berenstein and D. Trancanelli, “*S-duality and the giant magnon dispersion relation*”, [arxiv:0904.0444](#).
- [10] J. A. Minahan and K. Zarembo, “*The Bethe ansatz for superconformal Chern-Simons*”, JHEP 0809, 040 (2008), [arxiv:0806.3951](#).
- [11] D. Gaiotto, S. Giombi and X. Yin, “*Spin Chains in  $\mathcal{N} = 6$  Superconformal Chern-Simons-Matter Theory*”, JHEP 0904, 066 (2009), [arxiv:0806.4589](#).
- [12] G. Grignani, T. Harmark and M. Orselli, “*The SU(2) × SU(2) sector in the string dual of  $\mathcal{N} = 6$  superconformal Chern-Simons theory*”, Nucl. Phys. B810, 115 (2009), [arxiv:0806.4959](#).
- [13] T. McLoughlin, R. Roiban and A. A. Tseytlin, “*Quantum spinning strings in AdS<sub>4</sub> × CP<sup>3</sup>: testing the Bethe Ansatz proposal*”, JHEP 0811, 069 (2008), [arxiv:0809.4038](#).
- [14] I. Shenderovich, “*Giant magnons in AdS<sub>4</sub>/CFT<sub>3</sub>: dispersion, quantization and finite-size corrections*”, [arxiv:0807.2861](#).
- [15] N. Gromov and P. Vieira, “*The all loop AdS<sub>4</sub>/CFT<sub>3</sub> Bethe ansatz*”, JHEP 0901, 016 (2009), [arxiv:0807.0777](#).
- [16] M. A. Bandres, A. E. Lipstein and J. H. Schwarz, “*Studies of the ABJM Theory in a Formulation with Manifest SU(4) R-Symmetry*”, JHEP 0809, 027 (2008), [arxiv:0807.0880](#).

- [17] G. Papathanasiou and M. Spradlin, “*The Morphology of  $\mathcal{N} = 6$  Chern-Simons Theory*”, JHEP 0907, 036 (2009), [arxiv:0903.2548](#).
- [18] M. Benna, I. Klebanov, T. Klose and M. Smedback, “*Superconformal Chern-Simons Theories and  $AdS_4/CFT_3$  Correspondence*”, JHEP 0809, 072 (2008), [arxiv:0806.1519](#).
- [19] I. L. Buchbinder et al., “*ABJM models in  $\mathcal{N} = 3$  harmonic superspace*”, JHEP 0903, 096 (2009), [arxiv:0811.4774](#).
- [20] A. Mauri and A. C. Petkou, “*An  $N=1$  Superfield Action for  $M2$  branes*”, Phys. Lett. B666, 527 (2008), [arxiv:0806.2270](#).
- [21] M. Cederwall, “*Superfield actions for  $\mathcal{N} = 8$  and  $\mathcal{N} = 6$  conformal theories in three dimensions*”, JHEP 0810, 070 (2008), [arxiv:0809.0318](#).
- [22] D. Bak and S.-J. Rey, “*Integrable Spin Chain in Superconformal Chern-Simons Theory*”, JHEP 0810, 053 (2008), [arxiv:0807.2063](#).
- [23] O. Aharony, O. Bergman and D. L. Jafferis, “*Fractional  $M2$ -branes*”, JHEP 0811, 043 (2008), [arxiv:0807.4924](#).
- [24] D. Gaiotto and A. Tomasiello, “*The gauge dual of Romans mass*”, JHEP 1001, 015 (2010), [arxiv:0901.0969](#).
- [25] D. Forcella and W. Schulgin, “*Spin chain for the deformed ABJM theory*”, [arxiv:0906.3301](#).
- [26] B. I. Zwiebel, “*Two-loop Integrability of Planar  $\mathcal{N} = 6$  Superconformal Chern-Simons Theory*”, [arxiv:0901.0411](#).
- [27] M. Beccaria and G. Macorini, “*QCD properties of twist operators in the  $\mathcal{N} = 6$  Chern-Simons theory*”, JHEP 0906, 008 (2009), [arxiv:0904.2463](#). • M. Beccaria and G. Macorini, “*The virtual scaling function of twist operators in the  $\mathcal{N} = 6$  Chern-Simons theory*”, [arxiv:0905.1030](#).
- [28] J. A. Minahan, W. Schulgin and K. Zarembo, “*Two loop integrability for Chern-Simons theories with  $\mathcal{N} = 6$  supersymmetry*”, JHEP 0903, 057 (2009), [arxiv:0901.1142](#).
- [29] D. Bak, D. Gang and S.-J. Rey, “*Integrable Spin Chain of Superconformal  $U(M) \times U(N)$  Chern-Simons Theory*”, JHEP 0810, 038 (2008), [arxiv:0808.0170](#).
- [30] J. A. Minahan, O. Ohlsson Sax and C. Sieg, “*Magnon dispersion to four loops in the ABJM and ABJ models*”, J. Phys. A43, 275402 (2010), [arxiv:0908.2463](#).
- [31] J. A. Minahan, O. Ohlsson Sax and C. Sieg, “*Anomalous dimensions at four loops in  $N=6$  superconformal Chern-Simons theories*”, [arxiv:0912.3460](#).
- [32] M. Leoni, A. Mauri, J. Minahan, O. Ohlsson Sax, A. Santambrogio, C. Sieg and G. Tartaglino-Mazzucchelli, “*Superspace calculation of the four-loop spectrum in  $N=6$  supersymmetric Chern-Simons theories*”, JHEP 1012, 074 (2010), [arxiv:1010.1756](#).
- [33] J. A. Minahan, O. Ohlsson Sax and C. Sieg, “*A limit on the ABJ model*”, [arxiv:1005.1786](#).
- [34] D. Bak, H. Min and S.-J. Rey, “*Integrability of  $N=6$  Chern-Simons Theory at Six Loops and Beyond*”, [arxiv:0911.0689](#).
- [35] C. Kristjansen, M. Orselli and K. Zoubos, “*Non-planar ABJM Theory and Integrability*”, JHEP 0903, 037 (2009), [arxiv:0811.2150](#).

- [36] P. Caputa, C. Kristjansen and K. Zoubos, “Non-planar ABJ Theory and Parity”, Phys. Lett. B677, 197 (2009), [arxiv:0903.3354](#).
- [37] B. E. W. Nilsson and C. N. Pope, “Hopf fibration of eleven-dimensional supergravity”, Class. Quant. Grav. 1, 499 (1984).
- [38] J. Gomis, D. Sorokin and L. Wulff, “The complete  $AdS_4 \times CP^3$  superspace for the type IIA superstring and D-branes”, JHEP 0903, 015 (2009), [arxiv:0811.1566](#).
- [39] M. T. Grisaru, P. S. Howe, L. Mezincescu, B. Nilsson and P. K. Townsend, “ $N=2$  Superstrings in a Supergravity Background”, Phys. Lett. B162, 116 (1985).
- [40] P. A. Grassi, D. Sorokin and L. Wulff, “Simplifying superstring and D-brane actions in  $AdS_4 \times CP^3$  superbackground”, JHEP 0908, 060 (2009), [arxiv:0903.5407](#).
- [41] G. Arutyunov and S. Frolov, “Superstrings on  $AdS_4 \times CP^3$  as a Coset Sigma-model”, JHEP 0809, 129 (2008), [arxiv:0806.4940](#).
- [42] B. Stefański, Jr., “Green-Schwarz action for Type IIA strings on  $AdS_4 \times CP^3$ ”, Nucl. Phys. B808, 80 (2009), [arxiv:0806.4948](#).
- [43] R. R. Metsaev and A. A. Tseytlin, “Type IIB superstring action in  $AdS_5 \times S^5$  background”, Nucl. Phys. B533, 109 (1998), [hep-th/9805028](#).
- [44] M. Henneaux and L. Mezincescu, “A Sigma Model Interpretation of Green-Schwarz Covariant Superstring Action”, Phys.Lett. B152, 340 (1985).
- [45] N. Berkovits, M. Bershadsky, T. Hauer, S. Zhukov and B. Zwiebach, “Superstring theory on  $AdS_2 \times S^2$  as a coset supermanifold”, Nucl.Phys. B567, 61 (2000), [hep-th/9907200](#).
- [46] D. V. Uvarov, “ $AdS_4 \times CP^3$  superstring and  $D=3$   $\mathcal{N} = 6$  superconformal symmetry”, Phys. Rev. D79, 106007 (2009), [arxiv:0811.2813](#).
- [47] K. Zarembo, “Worldsheet spectrum in  $AdS_4/CFT_3$  correspondence”, [arxiv:0903.1747](#).
- [48] T. Nishioka and T. Takayanagi, “On Type IIA Penrose Limit and  $\mathcal{N} = 6$  Chern-Simons Theories”, JHEP 0808, 001 (2008), [arxiv:0806.3391](#).
- [49] D. Astolfi, V. G. M. Puletti, G. Grignani, T. Harmark and M. Orselli, “Full Lagrangian and Hamiltonian for quantum strings on  $AdS_4 \times CP^3$  in a near plane wave limit”, [arxiv:0912.2257](#).
- [50] G. Grignani, T. Harmark, A. Marini and M. Orselli, “New Penrose Limits and  $AdS/CFT$ ”, [arxiv:0912.5522](#).
- [51] D. Astolfi, V. G. M. Puletti, G. Grignani, T. Harmark and M. Orselli, “Finite-size corrections in the  $SU(2) \times SU(2)$  sector of type IIA string theory on  $AdS_4 \times CP^3$ ”, Nucl. Phys. B810, 150 (2009), [arxiv:0807.1527](#). • P. Sundin, “The  $AdS_4 \times CP^3$  string and its Bethe equations in the near plane wave limit”, JHEP 0902, 046 (2009), [arxiv:0811.2775](#).
- [52] P. Sundin, “On the worldsheet theory of the type IIA  $AdS_4 \times CP^3$  superstring”, [arxiv:0909.0697](#).
- [53] P. Fre and P. A. Grassi, “Pure Spinor Formalism for  $Osp(N/4)$  backgrounds”, [arxiv:0807.0044](#). • G. Bonelli, P. A. Grassi and H. Safaai, “Exploring Pure Spinor String Theory on  $AdS_4 \times CP^3$ ”, JHEP 0810, 085 (2008), [arxiv:0808.1051](#). • R. D’Auria, P. Fre, P. A. Grassi and M. Trigiante, “Superstrings on  $AdS_4 \times CP^3$  from Supergravity”, Phys. Rev. D79, 086001 (2009), [arxiv:0808.1282](#).

- [54] D. V. Uvarov, “*AdS<sub>4</sub> × CP<sup>3</sup> superstring in the light-cone gauge*”, Nucl. Phys. B826, 294 (2010), [arxiv:0906.4699](#).
- [55] E. Abdalla, M. Forger and M. Gomes, “*On the origin of anomalies in the quantum non-local charge for the generalized non-linear sigma models*”, Nucl. Phys. B210, 181 (1982). • E. Abdalla, M. Forger and A. Lima Santos, “*Non-local charges for non-linear sigma models on Grassmann manifolds*”, Nucl. Phys. B256, 145 (1985).
- [56] I. Bena, J. Polchinski and R. Roiban, “*Hidden symmetries of the AdS<sub>5</sub> × S<sup>5</sup> superstring*”, Phys. Rev. D69, 046002 (2004), [hep-th/0305116](#).
- [57] C. Kalousios, C. Vergu and A. Volovich, “*Factorized Tree-level Scattering in AdS<sub>4</sub> × CP<sup>3</sup>*”, [arxiv:0905.4702](#).
- [58] C. Ahn, P. Bozhilov and R. C. Rashkov, “*Neumann-Rosochatius integrable system for strings on AdS<sub>4</sub> × CP<sup>3</sup>*”, JHEP 0809, 017 (2008), [arxiv:0807.3134](#).
- [59] R. C. Rashkov, “*A note on the reduction of the AdS<sub>4</sub> × CP<sup>3</sup> string sigma model*”, Phys. Rev. D78, 106012 (2008), [arxiv:0808.3057](#). • M. Dukalski and S. J. van Tongeren, “*On fermionic reductions of the AdS<sub>4</sub> × CP<sup>3</sup> superstring*”, Phys. Rev. D80, 046005 (2009), [arxiv:0906.0706](#).
- [60] D. Bykov, “*Off-shell symmetry algebra of the AdS<sub>4</sub> × CP<sup>3</sup> superstring*”, [arxiv:0904.0208](#).
- [61] D. M. Hofman and J. M. Maldacena, “*Giant magnons*”, J. Phys. A39, 13095 (2006), [hep-th/0604135](#).
- [62] N. Dorey, “*Magnon bound states and the AdS/CFT correspondence*”, J. Phys. A39, 13119 (2006), [hep-th/0604175](#).
- [63] H.-Y. Chen, N. Dorey and K. Okamura, “*Dyonic giant magnons*”, JHEP 0609, 024 (2006), [hep-th/0605155](#).
- [64] M. C. Abbott and I. Aniceto, “*Giant Magnons in AdS<sub>4</sub> × CP<sup>3</sup>: Embeddings, Charges and a Hamiltonian*”, [arxiv:0811.2423](#).
- [65] M. C. Abbott, I. Aniceto and O. Ohlsson Sax, “*Dyonic Giant Magnons in CP<sup>3</sup>: Strings and Curves at Finite J*”, Phys. Rev. D80, 026005 (2009), [arxiv:0903.3365](#).
- [66] T. J. Hollowood and J. L. Miramontes, “*A New and Elementary CP<sup>n</sup> Dyonic Magnon*”, [arxiv:0905.2534](#).
- [67] Y. Hatsuda and H. Tanaka, “*Scattering of Giant Magnons in CP<sup>3</sup>*”, JHEP 1002, 085 (2010), [arxiv:0910.5315](#).
- [68] C. Ahn and R. I. Nepomechie, “ *$\mathcal{N} = 6$  super Chern-Simons theory S-matrix and all-loop Bethe ansatz equations*”, JHEP 0809, 010 (2008), [arxiv:0807.1924](#).
- [69] C. Kalousios and G. Papanastasiou, “*Giant Magnons in Symmetric Spaces: Explicit N-soliton solutions for CP<sup>n</sup>, SU(n) and S<sup>n</sup>*”, [arxiv:1005.1066](#).
- [70] T. J. Hollowood and J. L. Miramontes, “*Magnons, their Solitonic Avatars and the Pohlmeyer Reduction*”, JHEP 0904, 060 (2009), [arxiv:0902.2405](#).
- [71] C. Kalousios, M. Spradlin and A. Volovich, “*Dyonic Giant Magnons on CP<sup>3</sup>*”, JHEP 0907, 006 (2009), [arxiv:0902.3179](#). • R. Suzuki, “*Giant Magnons on CP<sup>3</sup> by Dressing Method*”, JHEP 0905, 079 (2009), [arxiv:0902.3368](#).

- [72] M. Staudacher, “*Review of AdS/CFT Integrability, Chapter III.1: Bethe Ansatz and the R-Matrix Formalism*”, [arxiv:1012.3990](#).
- [73] C. Ahn and R. I. Nepomechie, “*Review of AdS/CFT Integrability, Chapter III.2: Exact world-sheet S-matrix*”, [arxiv:1012.3991](#).
- [74] S. Schäfer-Nameki, “*Review of AdS/CFT Integrability, Chapter II.4: The Spectral Curve*”, [arxiv:1012.3989](#).
- [75] Z. Bajnok, “*Review of AdS/CFT Integrability, Chapter III.6: Thermodynamic Bethe Ansatz*”, [arxiv:1012.3995](#). • V. Kazakov and N. Gromov, “*Review of AdS/CFT Integrability, Chapter III.7: Hirota Dynamics for Quantum Integrability*”, [arxiv:1012.3996](#).
- [76] G. Papathanasiou and M. Spradlin, “*Two-Loop Spectroscopy of Short ABJM Operators*”, JHEP 1002, 072 (2010), [arxiv:0911.2220](#).
- [77] G. Arutyunov, S. Frolov and M. Zamaklar, “*The Zamolodchikov-Faddeev algebra for  $AdS_5 \times S^5$  superstring*”, JHEP 0704, 002 (2007), [hep-th/0612229](#).
- [78] N. Beisert, B. Eden and M. Staudacher, “*Transcendentality and crossing*”, J. Stat. Mech. 0701, P021 (2007), [hep-th/0610251](#).
- [79] C. Ahn and R. I. Nepomechie, “*An alternative S-matrix for  $\mathcal{N} = 6$  Chern-Simons theory?*”, JHEP 0903, 068 (2009), [arxiv:0810.1915](#).
- [80] C. Ahn and R. I. Nepomechie, “*Two-loop test of the  $\mathcal{N} = 6$  Chern-Simons theory S-matrix*”, JHEP 0903, 144 (2009), [arxiv:0901.3334](#).
- [81] C. Ahn, P. Dorey and R. I. Nepomechie, “*On the absence of reflection in  $AdS_4/CFT_3$* ”, [arxiv:0910.5584](#).
- [82] N. Gromov and P. Vieira, “*The  $AdS_4/CFT_3$  algebraic curve*”, JHEP 0902, 040 (2009), [arxiv:0807.0437](#).
- [83] N. Gromov, V. Kazakov and P. Vieira, “*Integrability for the Full Spectrum of Planar AdS/CFT*”, [arxiv:0901.3753](#).
- [84] D. Bombardelli, D. Fioravanti and R. Tateo, “*TBA and Y-system for planar  $AdS_4/CFT_3$* ”, Nucl. Phys. B834, 543 (2010), [arxiv:0912.4715](#).
- [85] N. Gromov and F. Levkovich-Maslyuk, “*Y-system, TBA and Quasi-Classical Strings in  $AdS_4 \times CP^3$* ”, [arxiv:0912.4911](#).

# Review of AdS/CFT Integrability, Chapter IV.4: Integrability in QCD and $\mathcal{N} < 4$ SYM

G.P. KORCHEMSKY

*Institut de Physique Théorique<sup>1</sup>, CEA Saclay,  
91191 Gif-sur-Yvette Cedex, France*

Gregory.Korchinsky@cea.fr

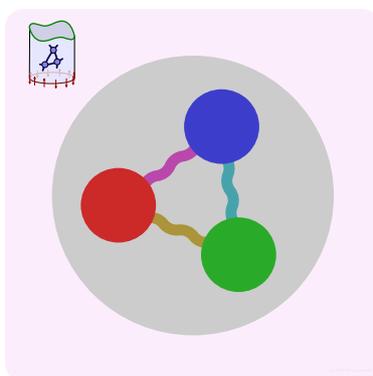

**Abstract:** There is a growing amount of evidence that QCD (and four-dimensional gauge theories in general) possess a hidden symmetry which does not exhibit itself as a symmetry of classical Lagrangians but is only revealed on the quantum level. In this review we consider the scale dependence of local gauge invariant operators and high-energy (Regge) behavior of scattering amplitudes to explain that the effective QCD dynamics in both cases is described by completely integrable systems that prove to be related to the celebrated Heisenberg spin chain and its generalizations.

---

<sup>1</sup>Unité de Recherche Associée au CNRS URA 2306

# 1 Introduction

QCD is a four-dimensional gauge theory describing strong interaction of quarks and gluons. There is a growing amount of evidence that QCD (and Yang-Mills theories in general) possess a hidden symmetry. This symmetry has a dynamical origin in the sense that it is not seen at the level of classical Lagrangian and manifests itself at quantum level through remarkable integrability properties of effective dynamics.

The simplest example which allows us to explain integrability phenomenon is a process of deeply inelastic scattering (DIS) of an energetic hadron off virtual photon,  $\gamma^*(q) + h(p) \rightarrow \text{everything}$ . This process played a distinguished rôle in early days of QCD development and it led, in particular, to important discoveries such as QCD factorization and formulation of parton model for hard processes (see e.g. [1]). The total cross-section of DIS process is related by the optical theorem to imaginary part of the forward scattering amplitude  $\gamma^*(q) + h(p) \rightarrow \gamma^*(q) + h(p)$  (see Fig. 1). It is parameterized by the so-called structure functions  $F(x, q^2)$  depending on the photon virtuality  $q^2 < 0$  and dimensionless Bjorken variable  $0 < x < 1$ . The latter is related to the total center-of-mass energy of the process as  $s = (p + q)^2 = -q^2(1 - x)/x$ .

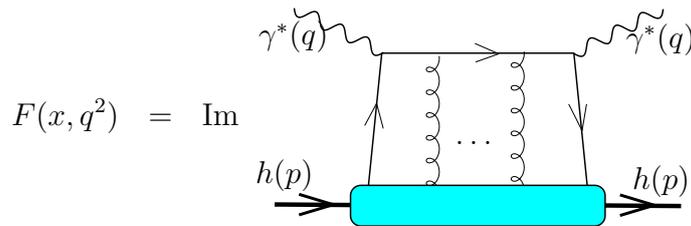

**Figure 1:** The total cross-section of deep inelastic scattering  $\gamma^*(q) + h(p) \rightarrow \text{everything}$  is related by the optical theorem to imaginary part of the forward scattering amplitude. Solid and wavy lines denote quarks and gluons, respectively.

The integrability has been first discovered in Refs. [2–4] in the study of high-energy,  $s \gg -q^2$  (or equivalently  $x \rightarrow 0$ ) asymptotics of  $F(x, q^2)$ . Experimental data indicate that the structure functions increase in this limit as a power of the energy,  $F(x, q^2) \sim (1/x)^\omega$ , in a quantitative agreement with the Regge theory prediction. At weak coupling, the same behavior can be obtained through resummation of perturbative corrections to the structure functions enhanced by logarithm of the energy [5]. The structure functions obtained in this way satisfy nontrivial multi-particle Bethe-Salpeter like evolution equations [6, 7]. These equations have resisted analytical solution but a breakthrough occurred after it was found [2–4] that, in multi-color limit, these equations can be mapped into a Schrödinger equation for a completely integrable quantum (non-compact) Heisenberg  $SL(2, \mathbb{C})$  spin chain. This opened up the possibility of applying the quantum inverse scattering methods for the construction of the exact solution to the evolution equation in planar QCD.

Later, similar integrable structures have been found in Refs. [8–10] in the study of dependence of the structure functions  $F(x, q^2)$  on the momentum transferred  $q^2$ . At large  $Q^2 = -q^2$ , the operator product expansion can be applied to expand the moments of the

structure functions in powers of a hard scale  $1/Q$

$$\int_0^1 dx x^{N-1} F(x, q^2) = \sum_{L \geq 2} \frac{c_{N,L}(\alpha_s(Q^2))}{Q^L} \langle p | O_{N,L} | p \rangle_{\mu^2=Q^2}. \quad (1.1)$$

Here the expansion runs over local composite gauge invariant operators (*Wilson operators*) of Lorentz spin  $N$  and twist  $L$ . The corresponding coefficient functions  $c_{N,L}(\alpha_s(Q^2))$  can be computed at weak coupling as a series in the QCD coupling constant  $\alpha_s(\mu^2) = g^2/(4\pi)$  normalized at  $\mu^2 = Q^2$ . At the same time, the matrix element of the Wilson operator with respect to hadron state  $\langle p | O_{N,L} | p \rangle_{\mu^2=Q^2}$  is a nonperturbative quantity. Its absolute value can not be computed perturbatively whereas its dependence on the hard scale  $Q^2$  is governed by the renormalization group (Callan-Symanzik) equations

$$\mu^2 \frac{d}{d\mu^2} \langle p | O_{N,L}^{(\alpha)} | p \rangle = -\gamma_{N,L}^{(\alpha)}(\alpha_s) \langle p | O_{N,L}^{(\alpha)} | p \rangle. \quad (1.2)$$

Here we introduced the superscript  $(\alpha)$  to indicate that for given  $N$  and  $L$  there are a few Wilson operators parameterized by the index  $\alpha$ . The Callan-Symanzik equation (1.2) has the meaning of a conformal Ward identity for the Wilson operators with the anomalous dimension  $\gamma_{N,L}^{(\alpha)}(\alpha_s)$  being the eigenvalue of the QCD dilatation operator (see e.g. review [11]).

The Wilson operators are built in QCD from elementary quark and gluon fields and from an arbitrary number of covariant derivatives. In general, such operators mix under renormalization with other operators carrying the same Lorentz spin and twist. Diagonalizing the corresponding mixing matrix we can find the spectrum of the anomalous dimensions  $\gamma_{N,L}^{(\alpha)}(\alpha_s)$ . For the Wilson operators of the lowest twist,  $L = 2$ , the anomalous dimensions can be obtained in the closed form [12], whereas for higher twist operators the problem becomes extremely nontrivial already at one loop due to a complicated form of the mixing matrix [13]. Quite remarkably, the spectrum of the anomalous dimensions can be found exactly in QCD in the sector of the so-called maximal-helicity Wilson operators. The reason for this is that the one-loop mixing matrix in QCD in this sector can be mapped in the multi-color limit into a Hamiltonian of the Heisenberg  $SL(2, \mathbb{R})$  spin chain [8–10]. The twist of the Wilson operator  $L$  determines the length of the spin chain while the spin operators in the each site are defined by the generators of the ‘collinear’  $SL(2, \mathbb{R})$  subgroup of the full conformal group [14, 15]. As a result, the exact spectrum of one-loop anomalous dimensions can be computed with a help of Bethe Ansatz [16].

Let us now examine the relation (1.1) for large Lorentz spin,  $N \gg 1$ . This limit has important phenomenological applications in QCD [17, 18]. It is known [12] that the anomalous dimensions of Wilson operators grow as their Lorentz spin increases. As a consequence, the dominant contribution to (1.1) only comes from the operators with the minimal anomalous dimension  $\gamma_{N,L}^{(0)} = \min_{\alpha} \gamma_{N,L}^{(\alpha)}$ . Quite remarkably, this anomalous dimension has a universal (twist  $L$  independent) logarithmic scaling behavior at large  $N$  to all loops [19, 20]

$$\gamma_{N,L}^{(0)} = 2\Gamma_{\text{cusp}}(\alpha_s) \ln N + O(N^0), \quad (1.3)$$

where  $\Gamma_{\text{cusp}}(\alpha_s)$  is the *cusp anomalous dimension* [21].

By definition,  $\Gamma_{\text{cusp}}(\alpha_s)$  governs the scale dependence of Wilson lines with light-like cusps [22, 23] and its relation to anomalous dimensions of large spin Wilson operators is by no means obvious. It can be understood [19] by invoking the physical picture of deep inelastic scattering at large  $N$ . In terms of the moments (1.1), large  $N$  corresponds to the region of  $x \rightarrow 1$ . For  $x \rightarrow 1$  the final state in the deep inelastic scattering has a small invariant mass,  $s = Q^2(1-x)/x \ll Q^2$ , and it consists of a collimated jet of energetic particles accompanying by soft gluon radiation. Interacting with soft gluons, the particles inside the jet acquire the eikonal phases given by Wilson line operators  $P \exp(i \int_0^\infty dt p \cdot A(pt))$  evaluated along semi-infinite line in the direction of the particle momenta. In this way, for  $x \rightarrow 1$ , complicated QCD dynamics in deep inelastic scattering admits an effective description in terms of Wilson lines [24]. The relation (1.3) between anomalous dimensions and cusp singularities of light-like Wilson lines is just one of the application of this formalism. Another examples include the relation between light-like Wilson loops with on-shell scattering amplitudes, Sudakov form factors, gluon Regge trajectories etc (see Ref. [25] and references therein).

At present, integrability of the dilatation operator in planar QCD has been verified to two loops in the  $SL(2; \mathbb{R})$  sector of maximal helicity operators [26]. In other sectors, the dilatation operator receives additional contribution that breaks integrability already to one loop. This contribution vanishes however for large values of the Lorentz spin  $N \gg 1$  thus suggesting that integrability in planar QCD gets restored to all loops in the leading large  $N$  limit [27]. Indeed, as was shown in Ref. [20], the all-loop dilatation operator in QCD in the  $SL(2; \mathbb{R})$  sector can be mapped in the large  $N$  limit into a Hamiltonian of a *classical* Heisenberg  $SL(2; \mathbb{R})$  spin chain. In this manner, the Wilson operators with large  $N$  are described by the so-called finite-gap solutions and the spectrum of anomalous dimension can be found through their semiclassical quantization. In particular, the relation (1.3) naturally appears as describing the ground state energy of the classical  $SL(2; \mathbb{R})$  spin chain of an arbitrary length  $L$  and total spin  $N$ .

The above mentioned integrability structures (those of the scattering amplitudes in the Regge limit and of the dilatation operator) are not specific to QCD. They are also present in generic four-dimensional gauge theories including supersymmetric Yang-Mills models with  $\mathcal{N} = 1, 2, 4$  supercharges. Supersymmetry enhances the phenomenon by extending integrability to a larger class of observables. In this context, the maximally supersymmetric  $\mathcal{N} = 4$  Yang-Mills theory is of a special interest with regards to the AdS/CFT correspondence [28]. The gauge/string duality hints that these structures should manifest themselves through hidden symmetries of the scattering amplitudes and of anomalous dimensions in dual gauge theories to all loops.

## 2 Integrability of dilatation operator in QCD

In this section, we review a hidden integrability of the dilatation operator in a generic four-dimensional Yang-Mills theory describing the coupling of gauge fields to fermions and scalars. Depending on the representation in which the latter fields are defined, we can distinguish two different types of the gauge theories: QCD and supersymmetric

extensions of Yang-Mills theory (SYM).

In QCD, the gauge fields are coupled to quarks in the fundamental representation of the  $SU(N_c)$  gauge group. The quarks are described by four-component Dirac fermions  $\psi$  and the gauge field strength  $F_{\mu\nu} = \frac{i}{g}[D_\mu, D_\nu]$  is determined in terms of the covariant derivatives  $D_\mu = \partial_\mu - igA_\mu^a t^a$  with generators  $t^a$  in the fundamental representation of the  $SU(N_c)$  normalized conventionally as  $\text{tr}(t^a t^b) = \frac{1}{2}\delta^{ab}$ . In SYM theory, the gauge fields are coupled to fermions (gauginos) and scalars belonging to the adjoint representation of the  $SU(N_c)$  group. The supersymmetric Yang-Mills theories with  $\mathcal{N} = 1, 2$  and 4 supercharges are obtained from the Lagrangian of generic Yang-Mills theory by adjusting the number of gaugino and scalar species. The gauginos are described by the Weyl fermion  $\lambda^A$  which belongs to the fundamental representation of an internal  $SU(\mathcal{N})$  symmetry group with its complex conjugate  $\bar{\lambda}_A = (\lambda^A)^*$ . The scalars are assembled into the antisymmetric tensor  $\phi^{AB} = -\phi^{BA}$ , with its complex conjugate  $(\phi^{AB})^* = \bar{\phi}_{AB}$ . As we explain below, integrability is not tied to supersymmetry and the phenomenon persists in the generic Yang-Mills theory for arbitrary  $\mathcal{N}$ , to two loop order at least.

## 2.1 Light-ray operators

Let us first consider renormalization of local gauge invariant operators in QCD. As the simplest example, we examine the following twist-two operator contributing to the moments of DIS structure function (1.1)

$$\langle p | O_{N,L=2}(0) | p \rangle = \langle p | \bar{\psi} \gamma_+ D_+^{N-1} \psi(0) | p \rangle. \quad (2.1)$$

It is built from two quark fields and  $(N - 1)$  covariant derivatives  $D_+ = (n \cdot D)$  projected onto light-like vector  $n_\mu = q_\mu - p_\mu q^2 / (2pq)$  and  $\gamma_+ = (n \cdot \gamma)$  being the projected Dirac matrix. Discussing renormalization properties of Wilson operators like (2.1) it is convenient to switch from infinite set of local operators (2.1) parameterized by positive integer  $N$  to a single nonlocal *light-ray operator*

$$\mathbb{O}(z_1, z_2) = \bar{\psi}(z_1 n) \gamma_+ [nz_1, nz_2] \psi(z_2 n) = \sum_{N \geq 1} [\bar{\psi} \gamma_+ D_+^{N-1} \psi] \frac{(z_1 - z_2)^{N-1}}{(N-1)!} + \dots \quad (2.2)$$

Here  $z_1$  and  $z_2$  are scalar variables defining the position of quark fields on the light-cone and the gauge link  $[nz_1, nz_2] \equiv P \exp(ig \int_{z_1}^{z_2} dt A_+(nt))$  is inserted to ensure gauge invariance of  $\mathbb{O}(z_1, z_2)$ . Also, ellipses in the right-hand side of (2.2) stand for terms involving total derivatives of the twist-two operators and, therefore, providing vanishing contribution to the forward matrix element  $\langle p | \mathbb{O}(z_1, z_2) | p \rangle$ .

We recall that local gauge invariant operators satisfy the evolution equation (1.2). The same is true for the light-ray operators (2.2) although the explicit form of the evolution equation is different due to nonlocal form of the light-ray operators. In particular, for the operators (2.2) the evolution equation takes the following form [29, 13, 30, 31]

$$\left( \mu \frac{\partial}{\partial \mu} + \beta(g^2) \frac{\partial}{\partial g^2} \right) \mathbb{O}(z_1, z_2) = -[\mathbb{H}_2(g^2) \cdot \mathbb{O}](z_1, z_2), \quad (2.3)$$

with the evolution kernel  $\mathbb{H}_2$  to be specified below. The evolution equation (2.3) expresses the conformal Ward identity in QCD and the beta-function term takes into account conformal symmetry breaking contribution. The evolution operator  $\mathbb{H}_2$  in the right-hand side of (2.3) defines a representation of the dilatation operator on the space spanned by nonlocal light-ray operators (2.2). In general,  $\mathbb{H}_2$  has a matrix form as the light-ray operators with different partonic content could mix with each other.

The evolution kernel  $\mathbb{H}_2$  has a perturbative expansion in powers of the coupling constant and admits a representation in the form of an integral operator acting on light-cone coordinates  $z_1$  and  $z_2$  of  $\mathbb{O}(z_1, z_2)$ . To the lowest order in the coupling, its explicit form has been found in QCD in Ref. [30] and its generalization to Yang-Mills theories with an arbitrary number of supercharges has been derived in Ref. [32]. The corresponding expressions for  $\mathbb{H}_2$  are given below in Eq. (2.11). The main advantage of (2.3) compared with the conventional approach based on explicit diagonalization of the mixing matrix for local Wilson operators is that the problem of finding the spectrum of anomalous dimensions can be mapped into spectral problem for one-dimensional quantum mechanical Hamiltonian  $\mathbb{H}_2$ . As we will see in a moment, the same happens in QCD for Wilson operators of high twist  $L \geq 3$ , in which case the corresponding evolution operator  $\mathbb{H}_L$  in the sector of maximal helicity operators turns out to be equivalent for a Hamiltonian of Heisenberg  $SL(2; \mathbb{R})$  spin chain of length  $L$ .

## 2.2 Light-cone formalism

Discussing integrability of the dilatation operator in QCD and in SYM theories, it is convenient to employ the “light-cone formalism” [33–35]. In this formalism one integrates out non-propagating components of fields and formulates the (super) Yang-Mills action in terms of “physical” degrees of freedom. Although the resulting action is not manifestly covariant under the Poincaré transformations, the main advantage of the light-cone formalism for SYM theories is that the  $\mathcal{N}$ -extended supersymmetric algebra is closed off-shell for the propagating fields and there is no need to introduce auxiliary fields. This allows us to design a unifying light-cone superspace formulation of various  $\mathcal{N}$ -extended SYM, including the  $\mathcal{N} = 4$  theory for which a covariant superspace formulation does not exist.

In the light-cone formalism, one quantizes the Yang-Mills theory in a noncovariant, light-cone gauge  $(n \cdot A) \equiv A_+(x) = 0$ . Introducing an auxiliary complementary light-like vector  $\bar{n}_\mu$ , such that  $\bar{n}^2 = 0$  and  $(n \cdot \bar{n}) = 1$ , we split three remaining components of the gauge field into longitudinal,  $A_-(x)$ , and two transverse holomorphic and antiholomorphic components,  $A(x)$  and  $\bar{A}(x)$ , respectively,

$$A_- \equiv (\bar{n} \cdot A), \quad A \equiv \frac{1}{\sqrt{2}}(A_1 + iA_2), \quad \bar{A} \equiv A^* = \frac{1}{\sqrt{2}}(A_1 - iA_2). \quad (2.4)$$

In the similar manner, the fermion field  $\psi(x)$  can be decomposed with a help of projectors  $\Pi_\pm = \frac{1}{2}\gamma_\pm\gamma_\mp$  as

$$\psi = \Pi_+\psi + \Pi_-\psi \equiv \psi_+ + \psi_-, \quad (2.5)$$

where the fermion field  $\psi_+$  has two nonzero components

$$q_\uparrow = \frac{1}{2}(1 - \gamma_5)\psi_+, \quad q_\downarrow = \frac{1}{2}(1 + \gamma_5)\psi_+. \quad (2.6)$$

Then, one finds that the fields  $\psi_-(x)$  and  $A_-(x)$  can be integrated out and the resulting action of the Yang-Mills theory is expressed in terms of “physical” fields: complex gauge field,  $A(x)$  and  $\bar{A}(x)$ , two components of fermion fields,  $q_\uparrow(x)$  and  $q_\downarrow(x)$ , and, in the case of supersymmetric gauge theory, complex scalar fields  $\phi(x)$ . When applied to the vacuum states, the fields  $(A, q_\downarrow, \phi, q_\uparrow, \bar{A})$  create massless particles of helicity  $(-1, -\frac{1}{2}, 0, \frac{1}{2}, 1)$ , respectively.

Taking the product of ‘physical’ fields and light-cone derivatives  $D_+ = \partial_+$ , we can construct the set of local gauge invariant operators. Such operators define the representation of the so-called collinear  $SL(2; \mathbb{R})$  subgroup of the conformal group and they are known in QCD literature as *quasipartonic operators*. A distinguished feature of these operators is that their twist equals the number of constituent physical fields [13]. In analogy with (2.2), we can replace an infinite number of Wilson operators of a given twist  $L$  with a few nonlocal light-ray operators  $\mathbb{O}(z_1, \dots, z_L)$ . The latter can be thought of as generating functions for the former. Due to different  $SU(N_c)$  representation of fermions (fundamental in QCD and adjoint in SYM), the definition of such operators is slightly different in the two theories.

In QCD, in the simplest case of twist two, we can distinguish four different light-ray operators (plus complex conjugated operators)

$$\begin{aligned} \mathbb{O}_{qq}^{(0)}(z_1, z_2) &= \bar{q}_\uparrow(nz_1)q_\uparrow(nz_2), & \mathbb{O}_{gg}^{(0)}(z_1, z_2) &= \text{tr} [\partial_+ \bar{A}(nz_1)\partial_+ A(nz_2)], \\ \mathbb{O}_{qq}^{(1)}(z_1, z_2) &= \bar{q}_\downarrow(nz_1)q_\uparrow(nz_2), & \mathbb{O}_{gg}^{(2)}(z_1, z_2) &= \text{tr} [\partial_+ A(nz_1)\partial_+ A(nz_2)], \end{aligned} \quad (2.7)$$

where the subscript ( $qq$  and  $gg$ ) indicates particle content of the operator and the superscript defines the total helicity. In this basis, the operator (2.2) is given by a linear combination of  $\mathbb{O}_{qq}^{(0)}(z_1, z_2)$  and complex conjugated operator. The operators  $\mathbb{O}_{qq}^{(0)}$  and  $\mathbb{O}_{gg}^{(0)}$  have the same quantum numbers and mix under renormalization. At the same time, the operators  $\mathbb{O}_{qq}^{(1)}$  and  $\mathbb{O}_{gg}^{(2)}$  carry different helicity and have an autonomous scale dependence. In what follows we shall refer to them as maximal helicity operators. The reason why we distinguish such operators is that the one-loop dilatation operator in QCD is integrable in the sector of maximal helicity operators only.

For higher twist  $L \geq 3$  we can define three different types of maximal helicity operators in QCD:

$$\mathbb{O}_{qqq}^{(3/2)}(z_1, z_2, z_3) = \varepsilon_{ijk} q_\uparrow^i(z_1n)q_\uparrow^j(z_2n)q_\uparrow^k(z_3n), \quad (2.8)$$

$$\mathbb{O}_{qq\dots qq}^{(L-1)}(z_1, \dots, z_L) = \bar{q}_\downarrow(nz_1)\partial_+ A(nz_2) \dots \partial_+ A(nz_{L-1})q_\uparrow(nz_L), \quad (2.9)$$

$$\mathbb{O}_{g\dots g}^{(L)}(z_1, \dots, z_L) = \text{tr} [\partial_+ A(nz_1) \dots \partial_+ A(nz_L)], \quad (2.10)$$

to which we shall refer as baryonic ( $L = 3$ ) operators, mixed quark-gluon operators and gluon operators, respectively. We remind that since quark fields belong to the fundamental representation of the  $SU(N_c)$  group, the length of the operator (2.8) ought to be  $N_c = 3$ . At the same time, gluon fields are in the adjoint representation and the single trace operator (2.10) is well-defined for arbitrary  $N_c$  and twist  $L$ . The same applies to the mixed quark-gluon operators (2.9). The operators (2.8) and (2.9) have a direct

phenomenological significance: their matrix elements determine the distribution amplitude of the delta-isobar [36] and higher twist contribution to spin structure functions, respectively.

### 2.3 Evolution kernels

The light-ray operators (2.7) – (2.10) satisfy the evolution equation (2.3). Let us first examine twist-two quark operators  $\mathbb{O}_{qq}^{(0)}$  and  $\mathbb{O}_{qq}^{(1)}$  defined in (2.7). The operator  $\mathbb{O}_{qq}^{(0)}$  can mix with the gluon operator  $\mathbb{O}_{gg}^{(0)}$ . To simplify the situation, we can suppress the mixing by choosing the two quark fields inside  $\mathbb{O}_{qq}^{(0)}$  to have different flavor. To one-loop order, the evolution kernel receives the contribution from one-gluon exchange between two quark fields and from self-energy corrections. The latter one is the same for the two operators while the former one is different

$$\begin{aligned}\mathbb{H}_{qq}^{(1)} &= \frac{g^2 C_F}{8\pi^2} [H_{12} + 2\gamma_q] , \\ \mathbb{H}_{qq}^{(0)} &= \frac{g^2 C_F}{8\pi^2} [H_{12} + V_{12} + 2\gamma_q] .\end{aligned}\tag{2.11}$$

Here  $C_F = t^a t^a = (N_c^2 - 1)/(2N_c)$  is the quadratic Casimir of the  $SU(N_c)$  in the fundamental representation,  $\gamma_q = 1$  is one-loop anomalous dimension of quark field in the axial gauge  $A_+ = 0$  and  $H_{12}$  and  $V_{12}$  are integral operators

$$\begin{aligned}[H_{12} \cdot \mathbb{O}](z_1, z_2) &= \int_0^1 \frac{d\alpha}{\alpha} \bar{\alpha} \left[ 2\mathbb{O}(z_1, z_2) - \mathbb{O}(\bar{\alpha}z_1 + \alpha z_2, z_2) - \mathbb{O}(z_1, \alpha z_1 + \bar{\alpha}z_2) \right], \\ [V_{12} \cdot \mathbb{O}](z_1, z_2) &= \int_0^1 d\alpha_1 \int_0^{\bar{\alpha}_1} d\alpha_2 \mathbb{O}(\alpha_1 z_1 + \bar{\alpha}_1 z_2, \alpha_2 z_2 + \bar{\alpha}_2 z_1),\end{aligned}\tag{2.12}$$

where  $\bar{\alpha}_i \equiv 1 - \alpha_i$ . These operators have a transparent physical interpretation: they displace two particles along the light-cone in the direction of each other.

To find the spectrum of anomalous dimensions of twist-two quark operators generated by light-ray operators (2.7), we have to diagonalize the operators  $\mathbb{H}_{qq}^{(1)}$  and  $\mathbb{H}_{qq}^{(0)}$ . This can be done with a help of conformal symmetry. We recall that the conformal symmetry is broken in QCD at loop level. However the dilatation operator receives conformal symmetry breaking contribution only starting from two loops and, as a consequence, the one-loop evolution kernels in QCD have to respect conformal symmetry of QCD Lagrangian. For nonlocal light-ray operators built from fields  $X(nz)$ , the full  $SO(2, 4)$  conformal symmetry reduces to its collinear  $SL(2; \mathbb{R})$  subgroup acting on one-dimensional light-cone coordinates of fields [14, 15]

$$z \rightarrow \frac{az + b}{cz + d}, \quad X(zn) \rightarrow (cz + d)^{-2j} X\left(\frac{az + b}{cz + d}n\right)\tag{2.13}$$

with  $ad - bc = 1$ . The generators of these transformations are

$$L^- = -\partial_z, \quad L^+ = 2jz + z^2\partial_z, \quad L^0 = j + z\partial_z.\tag{2.14}$$

Here  $j$  is the conformal weight of the field. For ‘physical’ components of fermions,  $\psi_+$ , it equals  $j_q = 1$ , for transverse components of gauge field,  $\partial_+ A$  and  $\partial_+ \bar{A}$ , it is  $j_g = 3/2$  and for scalars  $j_s = 1/2$ .

In application to light-ray quark operators,  $\mathbb{O}_{qq}^{(0)}(z_1, z_2)$  and  $\mathbb{O}_{qq}^{(1)}(z_1, z_2)$ , the conformal symmetry dictates that the one-loop evolution kernels (2.11) have to commute with the two particle conformal spin  $L_1^\alpha + L_2^\alpha$  (with  $\alpha = -, +, 0$ ). As a consequence,  $\mathbb{H}_{qq}^{(h=0,1)}$  is a function of the corresponding two-particle Casimir operator

$$L_{12}^2 = \sum_{\alpha=+,-,0} (L_1^\alpha + L_2^\alpha)^2 = J_{12}(J_{12} - 1). \quad (2.15)$$

To find the explicit form of this dependence, it suffices to examine the action of the two operators,  $\mathbb{H}_{qq}^{(h)}$  and  $L_{12}^2$ , on the same test function  $(z_1 - z_2)^n$ , which is just the lowest weight in the tensor product of two  $SL(2; \mathbb{R})$  representations carrying the spin  $J_{12} = n + 2$ . Replacing  $\mathbb{O}(z_1, z_2) \rightarrow (z_1 - z_2)^{J_{12}-2}$  in (2.12) we find

$$H_{12} = 2[\psi(J_{12}) - \psi(2)], \quad V_{12} = 1/(J_{12}(J_{12} - 1)), \quad (2.16)$$

where  $\psi(x) = d \ln \Gamma(x)/dx$  is Euler psi-function. Together with (2.11) these relations determine the spectrum of anomalous dimensions of twist-two quark operators.

## 2.4 Relation to Heisenberg $SL(2; \mathbb{R})$ spin chain

As the first sign of integrability, we notice that  $H_{12}$  coincides with the known expression for two-particle Hamiltonian of Heisenberg spin chain [37, 38]

$$H_L = H_{12} + \dots + H_{L1}, \quad H_{i,i+1} = \psi(J_{i,i+1}) - \psi(2j), \quad (2.17)$$

where the spin operators are identified as  $SL(2; \mathbb{R})$  conformal generators (2.14). As follows from (2.11), the one-loop dilatation operator  $\mathbb{H}_{qq}^{(1)}$  depends on  $H_{12}$  and, therefore, it is mapped into Heisenberg  $SL(2; \mathbb{R})$  spin chain of length 2. At the same time, the dilatation operator  $\mathbb{H}_{qq}^{(0)}$  receives the additional contribution  $V_{12}$ . It preserves the conformal symmetry but breaks integrability. Notice that  $V_{12}$  vanishes for large values of the conformal spin  $J_{12} \gg 1$  so that the two evolution kernels,  $\mathbb{H}_{qq}^{(0)}$  and  $\mathbb{H}_{qq}^{(1)}$ , have the same asymptotic behavior at large  $J_{12}$ . This suggests that for the operator  $\mathbb{H}_{qq}^{(0)}$  integrability is restored in the limit of large conformal spin only.

For twist-two operators, the anomalous dimensions are uniquely determined by their conformal spin. To appreciate the power of integrability, we have to consider Wilson operators of high twist  $L \geq 3$ . For example, for the maximal helicity baryonic operators (2.8) the one-loop dilatation operator has the form [10]

$$\mathbb{H}_{qqq}^{(3/2)} = \frac{\alpha_s}{2\pi} \left[ (1 + 1/N_c)(H_{12} + H_{23} + H_{31}) + \frac{3}{2}C_F \right] \quad (2.18)$$

with  $N_c = 3$  and  $H_{12}$  given by (2.16). Comparing this relation with (2.17) we recognize that  $\mathbb{H}_{qqq}^{(3/2)}$  can be mapped into Heisenberg spin chain of length  $L = 3$ . The spin at each site  $j = 1$  is determined by the conformal spin of quark field.

For gluon operators of the maximal helicity (2.10) the dilatation operator receives contribution from self-energy corrections to gluon fields and from one-gluon exchange between any pair of gluons. The latter produces both planar and nonplanar corrections (for  $L > 3$ ). In the planar limit, the one-loop dilatation operator has the following form [39]

$$\mathbb{H}_{g\dots g}^{(L)} = \frac{g^2 N_c}{8\pi^2} (H_{12} + \dots + H_{L1}), \quad (2.19)$$

where two-particle kernel  $H_{i,i+1}$  acts locally on light-cone coordinates of gluons with indices  $i$  and  $i+1$ . The conformal symmetry implies that  $H_{i,i+1}$  is a function of the conformal spin of two gluons  $J_{i,i+1}$ . Quite remarkably, the dependence of  $H_{i,i+1}$  on  $J_{i,i+1}$  has the same form as in (2.17). As a consequence, the one-loop planar dilatation operator for maximal helicity gluon operator (2.10) coincides with the Hamiltonian of the Heisenberg  $SL(2; \mathbb{R})$  spin chain. The length of the spin chain equals the twist of the operator  $L$  and the spin in each site  $j = 3/2$  coincides with the conformal spin of the gluon field.

For mixed quark-gluon operators of the maximal helicity (2.9), the quark fields can interact in the planar limit with the adjacent gluon fields only while quark-quark interaction is suppressed in this limit. As a consequence, the one-loop dilatation operator has the following form in the planar limit

$$\mathbb{H}_{qg\dots gq}^{(L-1)} = \frac{g^2 N_c}{8\pi^2} (U_{12} + H_{23} + \dots + H_{L-1,L} + U_{L-1,L}). \quad (2.20)$$

Here  $H_{i,i+1}$  describes the interaction of two gluons with aligned helicities and it is the same as in (2.17). The kernels  $U_{12}$  and  $U_{L-1,L}$  describes quark-gluon interaction and their explicit form can be found in Ref. [40, 41]. Notice that the operator  $\mathbb{H}_{qg\dots gq}^{(L-1)}$  has the form of a Hamiltonian of *open spin chain* of length  $L$ . The spin in sites 1 and  $L$  coincides with the conformal spin of quark  $j_q = 1$  and the spin in all remaining sites is given by gluon conformal spin  $j_g = 3/2$ . As was shown in Ref. [40, 41], the open spin chain (2.20) is integrable.

## 2.5 Exact solution

Integrability of the one-loop dilatation operator allows us to find the exact spectrum of anomalous dimensions with a help of the Bethe Ansatz [8–10]

$$\begin{aligned} \gamma_{N,L} &= \frac{g^2 N_c}{8\pi^2} \mathcal{E}_{N,L} + O(g^4), \\ \mathcal{E}_{N,L} &= \sum_{k=1}^N \frac{2j}{u_k^2 + j^2} = i \frac{d}{du} \ln \frac{Q(u + ij)}{Q(u - ij)} \Big|_{u=0}. \end{aligned} \quad (2.21)$$

Here  $j$  is the conformal spin in each site ( $j = 1$  for quark operators and  $j = 3/2$  for gluon operators),  $u_k$  are Bethe roots and  $Q(u)$  is a polynomial of degree  $N$  of the form

$$Q(u) = \prod_{j=1}^N (u - u_j). \quad (2.22)$$

The function  $Q(u)$  defined in this way has the meaning of the eigenvalue of the Baxter operator for the  $SL(2, \mathbb{R})$  magnet [4, 42]. It satisfies the finite-difference Baxter equation

$$t_L(u)Q(u) = (u + ij)^L Q(u + i) + (u - ij)^L Q(u - i), \quad (2.23)$$

where  $t_L(u)$  is the transfer matrix of the spin chain

$$t_L(u) = 2u^L + q_2 u^{L-2} + \dots + q_L \quad (2.24)$$

and  $q_2, \dots, q_L$  are the conserved charges.

The Baxter equation (2.23) alone does not specify  $Q(u)$  uniquely and it has to be supplemented by additional condition for analytical properties of  $Q(u)$ . For the  $SL(2; \mathbb{R})$  spin chains describing the anomalous dimensions,  $Q(u)$  has to be a polynomial in the spectral parameter. Being combined with the Baxter equation (2.23), this condition determines  $Q(u)$  up to an overall normalization and, as a consequence, allows us to establish the quantization conditions for the  $q$ -charges and to compute the exact energy  $\mathcal{E}_{N,L}$ .

Solving the Baxter equation (2.23) for  $N = 0, 1, \dots$  one finds the eigenspectrum of the Hamiltonian  $\mathbb{H}_L$  and, as a consequence, determines the exact spectrum of the anomalous dimensions of the maximal helicity baryon operators (for  $j = 1$  and  $L = 3$ ) and of maximal helicity gluon operators (for  $j = 3/2$  and  $L \geq 2$ ). The spectrum obtained in this way exhibits remarkable regularity: almost all eigenvalues are double degenerate and for large  $N$  they belong to the set of trajectories [4, 43]. Both properties are ultimately related to integrability of the dilatation operators and can be served to test integrability at high loops.

For the  $SL(2; \mathbb{R})$  spin chains under consideration, the Baxter equation approach and conventional Bethe Ansatz are equivalent. Indeed, substituting (2.22) into the Baxter equation (2.23), one finds that the roots  $u_j$  satisfy the conventional  $SU(2)$  Bethe equations for spin  $(-j)$ . The fact that the spin is negative leads to a number of important differences as compared to “compact”  $SU(2)$  magnets. In particular, the Bethe roots take real values only and the number of solutions is infinite [4, 43].

## 2.6 Semiclassical limit

The Baxter operator approach becomes advantageous when one studies the properties of anomalous dimensions at large spin  $N$  and/or twist  $L$ . The reason for this is that the Baxter equation (2.23) takes the form of discretized Schrödinger equation. After rescaling of the spectral parameter,  $u \rightarrow (N + Lj)x$ , we can seek for solution to (2.23) in the WKB form [44, 45, 43]

$$Q(Nx) = \exp\left(\frac{i}{\hbar} S(x)\right), \quad \hbar = 1/(N + Lj), \quad (2.25)$$

where the action function  $S(x)$  admits an expansion in powers of  $\hbar$ . Substitution of (2.25) into the Baxter equation (2.23) yields the equation for  $S(x)$  which can be solved as a series in  $\hbar$ . To leading order we have

$$S(x) = \int_{x_0}^x dx p(x) + O(\hbar), \quad (2.26)$$

where the momentum  $p(x)$  is defined on the spectral curve (“equal energy” condition) of the classical  $SL(2; \mathbb{R})$  magnet  $y(x) = 2x^L \sinh p(x)$  with [46]

$$\Gamma_L : \quad y^2 = (t_L(x))^2 - 4x^{2L}. \quad (2.27)$$

The classical dynamics on this spectral curve has been studied in detail in Refs. [47, 27]. Using (2.25) we can compute the asymptotic behavior of the energy as [43, 48]

$$\mathcal{E}_{N,L}^{(\text{as})} = 2 \ln 2 + \sum_{n=1}^L [\psi(j + i\delta_n) + \psi(j - i\delta_n) - \psi(2j)] + \dots, \quad (2.28)$$

where ellipses denote terms subleading at large  $(N + jL)$ . Here  $\delta_n$  are roots of the transfer matrix defined in (2.24),  $t_L(\delta_n) = 0$ . They depend on the conserved charges  $q_2, \dots, q_L$  whose values satisfy the WKB quantization conditions

$$\oint_{\alpha_k} dx p(x) = 2\pi\hbar(\ell_k + \frac{1}{2}), \quad (\text{for } k = 1, \dots, L-1). \quad (2.29)$$

Here integration goes over the cycles  $\alpha_k$  on the complex curve (2.27) encircling intervals on the real axis satisfying  $y^2(x) > 0$  and integers  $\ell_k$  enumerate the quantized values of the charges  $q_2, \dots, q_L$  and the energy  $\mathcal{E}_{N,L} = \mathcal{E}_{N,L}(\ell_1, \dots, \ell_{L-2})$ . For large spin  $N$  and twist  $L$ , the minimal energy  $\mathcal{E}_{N,L}^{(0)} = \min_{\ell_k} \mathcal{E}_{N,L}$  has the following scaling behavior [48]

$$\mathcal{E}_{N,L}^{(0)} = f(\rho) \ln N + O(N^0), \quad \rho = \frac{L}{\ln N} = \text{fixed}, \quad N, L \gg 1 \quad (2.30)$$

where  $f(\rho)$  is the so-called generalized scaling function. Detailed analysis of the relations (2.28) and (2.29) can be found in Refs. [43, 10, 39, 27, 48]. For recent development in the generalized scaling function in  $\mathcal{N} = 4$  SYM see review Ref. [49].

So far we have discussed the exact solution for the one-loop anomalous dimensions of quark and gluon maximal helicity operators. For the anomalous dimensions of mixed quark-gluon operators (2.9), similar analysis of the spin chain (2.20) can be carried out using Bethe Ansatz for open  $SL(2; \mathbb{R})$  spin chains [39, 40].

## 2.7 Integrability of dilatation operators in SYM theories

In this subsection, we extend consideration to supersymmetric Yang-Mills theories. Discussing integrability of dilatation operator in these theories, it is convenient to employ supersymmetric version of light-cone formalism due to Mandelstam [35] and Brink *et al.* [34]. In this formalism, all symmetries of SYM theory become manifest and calculations can be performed in a unified manner for different numbers of supercharges  $\mathcal{N} = 0, 1, 2, 4$ . The maximally-supersymmetric  $\mathcal{N} = 4$  SYM theory is a finite, four-dimensional conformal field theory [35, 34, 50, 51], while the  $\mathcal{N} = 0$  theory corresponds to pure gluodynamics.

Defining a SYM theory on the light-cone, one starts with the component form of the action, fixes the light-cone gauge  $A_+(x) = 0$ , decompose all propagating, “physical” fields

into definite helicity components. In the case of  $\mathcal{N} = 4$  SYM, they include helicity ( $\pm 1$ ) fields,  $A(x)$  and  $\bar{A}(x)$ , built from two-dimensional transverse components of the gauge field, complex scalar fields  $\phi^{AB}$  of helicity 0 and helicity  $\pm 1/2$  components of Majorana–Weyl fermions,  $\lambda^A$  and  $\bar{\lambda}_A$ , all in the adjoint representation of the  $SU(N_c)$  gauge group. An important property of the light-cone formalism, which makes it advantageous over the covariant one, is that the latter fields have only one non-vanishing component. As a consequence, one can describe helicity ( $\pm 1/2$ ) fermions by Grassmann-valued complex fields without any Lorentz index. Introducing four fermionic coordinates  $\theta^A$  (with  $A = 1, \dots, 4$ ) possessing the helicity ( $-\frac{1}{2}$ ) and their conjugates  $\bar{\theta}_A$  with helicity  $\frac{1}{2}$ , we can assemble the above fields into a single, complex chiral  $\mathcal{N} = 4$  superfield [34]

$$\begin{aligned} \Phi(x, \theta^A) &= \partial_+^{-1} A(x) + \theta^A \partial_+^{-1} \bar{\lambda}_A(x) + \frac{i}{2!} \theta^A \theta^B \bar{\phi}_{AB}(x) \\ &\quad - \frac{1}{3!} \varepsilon_{ABCD} \theta^A \theta^B \theta^C \lambda^D(x) - \frac{1}{4!} \varepsilon_{ABCD} \theta^A \theta^B \theta^C \theta^D \partial_+ \bar{A}(x). \end{aligned} \quad (2.31)$$

It embraces all particle helicities, from  $-1$  to  $1$  with half-integer step, and, therefore,  $\Phi(x, \theta^A)$  describes a CPT self-conjugate supermultiplet.

Gauge theories on the light-cone with less or no supersymmetry can be deduced from the maximally supersymmetric  $\mathcal{N} = 4$  theory by removing “unwanted” physical fields. In the superfield formulation this amounts to a truncation of the  $\mathcal{N} = 4$  superfield, or equivalently, reduction of the number of fermionic directions in the superspace [52]. For instance, to get the  $\mathcal{N} = 1$  superfields one removes three odd coordinates  $\theta^2 = \theta^3 = \theta^4 = 0$ , whereas for  $\mathcal{N} = 0$  all  $\theta$ 's in (2.31) have to be set to zero. Notice that under this procedure the truncated  $\mathcal{N} = 2$ ,  $\mathcal{N} = 1$  and  $\mathcal{N} = 0$  theories involve only half of the fields described by the  $\mathcal{N}$ -extended SYM theory and the other half of the needed particle content arises from the complex conjugated superfields  $\bar{\Phi} \equiv \Phi^*$ . Explicit expressions for the action of the SYM theory in terms of the light-cone superfields can be found in Ref. [32].

In a close analogy with (2.10), we can introduce multiparticle single-trace operators built from light-cone superfields

$$\mathbb{O}(Z_1, \dots, Z_L) = \text{tr} \{ \Phi(Z_1) \Phi(Z_2) \cdots \Phi(Z_L) \}, \quad (2.32)$$

where  $\Phi(Z) \equiv \Phi^a(Z) t^a$  is a matrix ( $SU(N_c)$ ) valued superfield and  $Z = (x, \theta^A)$  denotes its position in the superspace with four even coordinates,  $x_\mu$ , and  $\mathcal{N}$  odd coordinates,  $\theta^A$  with  $A = 1, \dots, \mathcal{N}$ . In addition, we choose all superfields to be located along the light-cone direction in the four-dimensional Minkowski space defined by the light-like vector  $n_\mu$  (with  $n^2 = 0$ ), so that  $n \cdot A = A_+ = 0$ . Similarly to the QCD case, the positions of the superfields on the light-cone are parameterized by real numbers  $x_\mu = z n_\mu$ ,  $\Phi(Z_k) \equiv \Phi(z_k n, \theta_k^A)$ . The single-trace operators (2.32) represent a natural generalization of nonlocal light-ray operators in QCD, cf. Eq. (2.10). To obtain the latter it is sufficient to expand  $\mathbb{O}(Z_1, \dots, Z_L)$  in powers of odd variables  $\theta_1^{A_1} \dots \theta_L^{A_L}$ . As in QCD, nonlocal operators (2.32) serve as generating functions for Wilson operators with the maximal Lorentz spin and minimal twist equal to the number of constituent fields  $L$ . Such operators define a representation of the  $SL(2|\mathcal{N})$  subgroup of the full superconformal group.

Examining light-ray operators (2.32) in SYM theories with different number of supercharges, we find that  $\mathcal{N} = 4$  case is special. In  $\mathcal{N} = 4$  SYM theory there is only one independent chiral superfield  $\Phi(Z)$  and, as a consequence, the operators (2.32) generate *all* Wilson operators of twist  $-L$  built from  $L$  fundamental fields. For  $\mathcal{N} \leq 2$ , the superfield  $\Phi(Z)$  and its conjugate  $\bar{\Phi}(Z)$  are independent of each other and, in addition to the operators in (2.32), one can introduce “mixed” operators built from both superfields. This means that in the  $\mathcal{N} = 0, 1$  and  $2$  SYM theories, the operators (2.32) only generate a certain subset of the existing Wilson operators in the  $SL(2|\mathcal{N})$  subsector.

The light-ray operators (2.32) play a special role as far as integrability is concerned. Namely, as was shown in Refs. [32], the one-loop dilatation operator acting on the space of single-trace operators (2.32) can be mapped in the multicolor limit into a Hamiltonian of a completely integrable Heisenberg  $SL(2|\mathcal{N})$  spin chain. As before, the length of the spin chain coincides with the number of superfields in (2.32) and spin operators are generators of a collinear  $SL(2|\mathcal{N})$  subgroup of the full superconformal group [32].

We recall that in SYM theories with  $\mathcal{N} \leq 2$  supercharges the operators (2.32) only generate a subsector of Wilson operators of twist  $L$ . To describe the remaining operators, one has to consider single-trace operators built from both superfields, like  $\text{tr} \{ \Phi(Z_1) \bar{\Phi}(Z_2) \cdots \Phi(Z_L) \}$ . For such operators, the one-loop dilatation operator involves the additional term describing the exchange interaction between superfields on the light-cone  $\Phi \bar{\Phi} \rightarrow \bar{\Phi} \Phi$ . It breaks integrability symmetry and generates a mass gap in the spectrum of the anomalous dimensions [10]. At the same time, for large values of the superconformal spin the exchange interaction vanishes and integrability gets restored in the leading large spin asymptotics of the anomalous dimensions.

## 2.8 Integrability in QCD and SYM beyond one loop

It is well-known that the conformal symmetry is broken in QCD and SYM theories with  $\mathcal{N} < 4$  supercharges while in the maximally supersymmetric  $\mathcal{N} = 4$  model it survives on the quantum level. However the conformal anomaly modifies anomalous dimensions starting from two loops only and, therefore, the one-loop dilatation operator inherits the conformal symmetry of the classical theory [11, 53].

Starting from two-loop order, the dilatation operator in the  $SL(2)$  sector acquires several new features. First, it receives conformal symmetry breaking corrections arising both due to a nonzero beta-function and a subtle symmetry-violating effect induced by the regularization procedure [54]. Second, the form of the dilatation operator starts to depend on the representation of the fermion fields, i.e., fundamental  $SU(3)$  in QCD and adjoint  $SU(N_c)$  in SYM theories. The difference between the two is that it is only in the latter case that one can select planar diagrams by going over to the multi-color limit, while in the former case the large- $N_c$  counting is inapplicable and the two-loop dilatation operator receives equally important contributions from both planar and nonplanar Feynman graphs. Thus, by studying the two-loop dilatation operator in the  $SL(2)$  sector we can identify what intrinsic properties of gauge theories (conformal symmetry, supersymmetry and/or planar limit) are responsible for the existence of the integrability phenomenon per se.

For an all-loop dilatation operator  $\mathbb{H}(\lambda)$ , depending on 't Hooft coupling constant

$\lambda = g^2 N_c / (8\pi^2)$  and acting on a Wilson operator built from  $L$  constituent fields and an arbitrary number of covariant derivatives, integrability would require, in general, the existence of  $L$  conserved charges. Two of the charges—the light-cone component of the total momentum of  $L$  fields and the scaling dimension of the operator—follow immediately from Lorentz covariance of the gauge theory. However, the identification of the remaining charges  $q_k(\lambda)$  with  $k = 3, \dots, L$  is an extremely nontrivial task. The eigenvalues of the charges  $q_k$  define the complete set of quantum numbers parameterizing the eigenspectrum of the dilatation operator. Integrability imposes a nontrivial analytical structure of anomalous dimensions of Wilson operators and implies the double degeneracy of eigenvalues with the opposite parity [4, 55, 10]. At the same time, breaking of integrability leads to lifting of the degeneracy in the eigenspectrum of the one-loop dilatation operator.

Explicit two-loop calculation of the anomalous dimensions of the aforementioned aligned-helicity fermionic operators in all SYM theories showed that the same relation between integrability and degeneracy of the eigenstates holds true to two loops. Namely, as was found in Refs. [26], the desired pairing of eigenvalues occurs for three-gaugino operators in SYM theories with  $\mathcal{N} = 1, 2$  supercharges and the  $SU(N_c)$  gauge group.

The two-loops dilatation operator in SYM theories receives conformal symmetry breaking contribution and, in addition, it depends on the number of supercharges  $\mathcal{N}$ . The latter dependence comes about through the contribution of  $2(\mathcal{N} - 1)$  real scalars and  $\mathcal{N}$  gaugino fields propagating inside loops. Both contributions to two-loop dilatation operator can be factored out (modulo an additive normalization factor) into a multiplicative c-number. This property makes the eigenspectrum of the two-loop dilatation operator alike in all gauge theories including the  $\mathcal{N} = 4$  SYM in which case the dilatation operator is believed to be integrable to all loops [56]. Summarizing the results of two-loop calculations of the anomalous dimension in QCD and in SYM theories, integrability of the dilatation operator only requires the planar limit but it is sensitive neither to conformal symmetry, nor to supersymmetry [26]. For recent discussion of integrability in relation to non-planar corrections to the anomalous dimensions in  $\mathcal{N} = 4$  SYM see review Ref. [57].

In this section, discussing the properties of anomalous dimensions we restricted ourselves to the  $SL(2)$  sector. There have been several developments that we cannot address here in detail. In particular, an important observation was made in Ref. [58], where it was shown that the diagonal part of one-loop QCD evolution kernels governing the scale dependence of Wilson operators of arbitrary twist, can be written in a Hamiltonian form in terms of quadratic Casimir operators of the full conformal  $SO(2, 4)$  group. This observation was used in Ref. [59] to work out the non-diagonal parts of the evolution kernels for generic twist-four operators.

### 3 Integrability in high energy scattering

In the previous section, we described how integrability emerges in the problem of finding the dependence of the structure functions  $F(x, Q^2)$  on the hard scale  $Q^2$ . In this section, we explain that yet another integrability symmetry arises in the high-energy limit.

In application to the structure function  $F(x, Q^2)$  this limit corresponds to  $x \rightarrow 0$  for

fixed  $Q^2$ . At small  $x$ , the invariant energy  $s = Q^2(1-x)/x$  of colliding virtual photon and hadron becomes large and the structure function is expected to have Regge-like scaling behavior  $F(x, Q^2) \sim (1/x)^\omega$ . In terms of moments (1.1), this corresponds to appearance of the Regge pole at  $N = \omega$

$$\tilde{F}_N(q^2) = \int_0^1 dx x^{N-1} F(x, q^2) \sim \frac{1}{N - \omega}. \quad (3.1)$$

It is well-known [5] that perturbative corrections to  $F(x, q^2)$  are enhanced at small  $x$  by large logarithms  $\sim (\alpha_s \ln(1/x))^p$ . This raised the hope that the Regge behavior (3.1) can be derived in QCD from resummation of such corrections to all loops. Going to moments, the expansion over  $(\alpha_s \ln s)^p$  is traded for the expansion of  $\tilde{F}_N(q^2)$  over  $(\alpha_s/N)^p$ .

### 3.1 Evolution equation

Careful study of asymptotic behavior of Feynman diagrams describing interaction between virtual photon and hadron shows that the dominant contribution to  $F(x, q^2)$  only comes  $t$ -channel exchange of particles of maximal spin, i.e. gluons (see Fig. 2). Moreover, in the center-of-mass frame of  $\gamma^*(q)$  and  $h(p)$ , due to hierarchy of the scales,  $s \gg Q^2$ , interaction takes place in the two-dimensional plane orthogonal to the plane defined by the momenta of scattered particles,  $p_\mu$  and  $q_\mu$ . This implies that in generic Yang-Mills theory the leading high-energy asymptotic behavior of the scattering amplitudes is driven by  $t$ -channel exchange of an arbitrary number of gluons. In the so-called generalized leading logarithmic approximation, their contribution to the moments (3.1) takes the form

$$\tilde{F}_N(q^2) = \sum_{L \geq 2} \int [d^2k] \int [d^2k'] \Phi_{\gamma^*}(\{k\}) T_L(\{k\}, \{k'\}; N) \Phi_h(\{k'\}), \quad (3.2)$$

where integration goes over two-dimensional momenta of  $L$  gluons propagating in the  $t$ -channel,  $[d^2k] = \prod_1^L d^2k_i$  and similarly for  $[d^2k']$ . Here, the wave functions  $\Phi_{\gamma^*}(\{k\})$  and  $\Phi_h(\{k'\})$  describe the coupling of  $L$  gluons to virtual photon and hadron, respectively. Also,  $T_L(\{k\}, \{k'\}; N)$  describes elastic scattering of  $L$  gluons in the  $t$ -channel (see Fig. 2) and is the main object of our consideration.

It is convenient to rewrite (3.2) as the following matrix element

$$\tilde{F}_N(q^2) = \sum_{L \geq 2} \langle \Phi_{\gamma^*} | T_L(N) | \Phi_h \rangle, \quad (3.3)$$

where the minimum number of two gluons,  $L = 2$ , is required in order to get a colorless exchange. The transition operator  $T_L(N)$  describes the elastic scattering of  $L$  gluons. In the generalized leading logarithmic approximation, the Feynman diagrams contribution to  $T_L(N)$  have ladder structure as shown in Fig 2. They can be resummed leading to the following Bethe-Salpeter equation [6, 7]

$$NT_L(N) = T_L^{(0)} + \frac{\alpha_s}{2\pi} \mathbb{H}_L T_L(N), \quad (3.4)$$

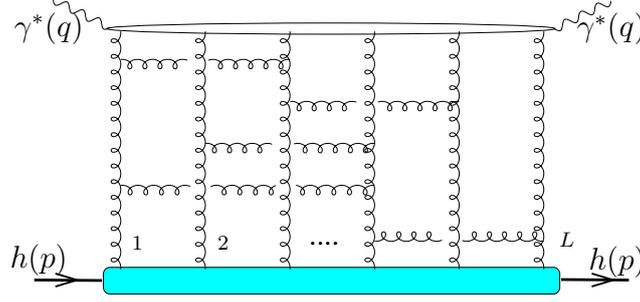

**Figure 2:** The Feynman diagrams contributing to the deep inelastic scattering in the generalized leading logarithmic approximation. Wavy lines denote (reggeized) gluons. They couple to virtual photons through a quark loop.

where  $T_L^{(0)}$  corresponds to the free propagation of  $L$  gluons in the  $t$ -channel and the evolution operator  $\mathbb{H}_L$  describes their pair-wise interaction. The operator  $\mathbb{H}_L$  acts both on two-dimensional momenta and on colors of  $L$  gluons and has the following two-particle form

$$\mathbb{H}_L = \sum_{1 \leq i < j \leq L} H_{ij} t_i^a t_j^a. \quad (3.5)$$

Each term in this sum is given by the product of the color factor involving color charges of two gluons and two-particle kernel  $H_{ij}$  acting locally on the transverse momenta of gluons with indices  $i$  and  $j$ . The kernel  $H_{ij}$  is known as BFKL operator [5] and it is defined below in (3.19).

Combining together (3.4) and (3.3) we obtain the following expression for  $\tilde{F}_N(q^2)$

$$\tilde{F}_N(q^2) = \sum_{L \geq 2} \langle \Phi_{\gamma^*} | \left( N - \frac{\alpha_s}{2\pi} \mathbb{H}_L \right)^{-1} T_L^{(0)} | \Phi_h \rangle. \quad (3.6)$$

We observe that  $\tilde{F}_N(q^2)$  has (Regge) singularities in  $N$  which are determined by the eigenspectrum of the operator  $\mathbb{H}_n$ , the so-called BKP equation [6, 7],

$$\mathbb{H}_L \Psi_{L,\{q\}}(k_1, \dots, k_L) = E_{L,\{q\}} \Psi_{L,\{q\}}(k_1, \dots, k_L). \quad (3.7)$$

The solutions to (3.7) define color singlet compound states of  $L$  gluons and we introduced  $\{q\}$  to denote the set of quantum numbers parameterizing all solutions. Having solved Schrödinger like equation (3.7), we can compute the moments of the structure function as [4]

$$\tilde{F}_N(q^2) = \sum_{L \geq 2} \sum_{\{q\}} \left( N - \frac{\alpha_s}{2\pi} E_{L,\{q\}} \right)^{-1} \beta_{L,\{q\}}. \quad (3.8)$$

Here the impact factor  $\beta_{L,\{q\}} = \langle \Phi_{\gamma^*} | \Psi_{L,\{q\}} \rangle \langle \Psi_{L,\{q\}} | T_L^{(0)} | \Phi_h \rangle$  measures the projection of the eigenstates onto the wave functions of scattered particles. The double sum in (3.8) runs over the possible number of gluons  $L \geq 2$  and over all eigenstates of the

BKP Hamiltonian (3.7) parameterized by the conserved charges  $q$ . We observe that this relation has an expected Regge form (3.1). Moreover, the leading Regge behavior of the structure function is controlled by right-most singularity of  $\tilde{F}_N(q^2)$  in complex  $N$  plane. According to (3.8), it corresponds to the *maximal* value of the ‘energy’  $E_{L,\{q\}}$ .

### 3.2 Conformal $SL(2; \mathbb{C})$ symmetry

We recall that  $k_i$  in the BKP equation (3.7) describe two-dimensional transverse momenta of  $i$ th gluon and the relation (3.7) can be interpreted as two-dimensional Schrödinger equation for  $n$  particles carrying  $SU(N_c)$  color charges.

As was found in [60, 2, 3], the BKP equation (3.7) becomes integrable in the multi-color limit. In this limit, the relevant ladder Feynman diagrams contributing to  $\tilde{F}_N(q^2)$  have the topology of a cylinder and, as a consequence, the evolution operator  $\mathbb{H}_L$  reduces to the sum of terms corresponding to pairwise nearest-neighbor BFKL interactions:

$$\mathbb{H}_L = \frac{1}{2} \sum_{k=1}^L H_{k,k+1} + O(1/N_c^2) \quad (3.9)$$

with periodic boundary conditions  $H_{L,L+1} = H_{L,1}$ . Notice that this relation is exact for  $L = 2$ .

The BFKL operator  $H_{k,k+1}$  has a number of remarkable properties which allow us to solve the Schrödinger equation (3.7) exactly [61, 60]. To elucidate these properties it is convenient to switch from two-dimensional momenta  $k_i$  to two-dimensional coordinates  $b_i$  via Fourier transform and, then, introduce complex holomorphic and the antiholomorphic coordinates

$$\vec{k}_i \mapsto \vec{b}_i = \{x_i, y_i\} \mapsto (z_i = x_i + iy_i, \quad \bar{z}_i = x_i - iy_i). \quad (3.10)$$

Quite remarkably,  $H_{12}$  is invariant under the conformal  $SL(2; \mathbb{C})$  transformations of the gluon coordinates on the plane [61, 60]

$$z_k \rightarrow \frac{az_k + b}{cz_k + d}, \quad (ad - bc = 1), \quad (3.11)$$

and similarly for antiholomorphic coordinates  $\bar{z}_k$ . The generators of these transformations are

$$L_{k,-} = -\partial_{z_k}, \quad L_{k,0} = z_k \partial_{z_k}, \quad L_{k,+} = z_k^2 \partial_{z_k}, \quad (3.12)$$

and the corresponding antiholomorphic generators  $\bar{L}_{k,-}$ ,  $\bar{L}_{k,0}$  and  $\bar{L}_{k,+}$  are given by similar expressions with  $z_k$  replaced by  $\bar{z}_k$ , with  $k = 1, 2$  enumerating particles. Then,  $H_{12}$  commutes with all two-particle generators

$$[H_{12}, L_{1,a} + L_{2,a}] = [H_{12}, \bar{L}_{1,a} + \bar{L}_{2,a}] = 0 \quad (3.13)$$

with  $a = +, -, 0$ . This implies that, firstly,  $H_{12}$  only depends on the two-particle Casimir operators of the  $SL(2, \mathbb{C})$  group

$$L_{12}^2 = -(z_1 - z_2)^2 \partial_{z_1} \partial_{z_2}, \quad \bar{L}_{12}^2 = -(\bar{z}_1 - \bar{z}_2)^2 \partial_{\bar{z}_1} \partial_{\bar{z}_2}, \quad (3.14)$$

and, secondly, the eigenstates of  $H_{12}$  have to diagonalize the Casimir operators

$$L_{12}^2 \Psi_{n,\nu} = h(h-1) \Psi_{n,\nu}, \quad \bar{L}_{12}^2 \Psi_{n,\nu} = \bar{h}(\bar{h}-1) \Psi_{n,\nu}. \quad (3.15)$$

Here a pair of complex conformal spins is introduced

$$h = \frac{1+n}{2} + i\nu, \quad \bar{h} = \frac{1-n}{2} + i\nu \quad (3.16)$$

with a non-negative integer  $n$  and real  $\nu$  that specify the irreducible (principal series) representation of the  $SL(2, \mathbb{C})$  group to which  $\Psi_{n,\nu}$  belongs. The solutions to Eqs. (3.15) are [61]

$$\Psi_{n,\nu}(b_1, b_2) = \left( \frac{z_{12}}{z_{10}z_{20}} \right)^{(1+n)/2+i\nu} \left( \frac{\bar{z}_{12}}{\bar{z}_{10}\bar{z}_{20}} \right)^{(1-n)/2+i\nu}, \quad (3.17)$$

where  $z_{jk} = z_j - z_k$  and  $b_0 = (z_0, \bar{z}_0)$  is the collective coordinate, reflecting the invariance of  $H_{12}$  under translations. The corresponding eigenvalue of  $H_{12}$  reads [5, 61]

$$E_{n,\nu} = 2\psi(1) - \psi\left(\frac{n+1}{2} + i\nu\right) - \psi\left(\frac{n+1}{2} - i\nu\right). \quad (3.18)$$

Its maximal value,  $\max E_{n,\nu} = 4 \ln 2$ , corresponds to  $n = \nu = 0$ , or equivalently  $h = \bar{h} = 1/2$ . It defines the position of the right-most singularity  $\omega = 4 \ln 2 \alpha_s N_c / \pi$  in (3.1) known as the BFKL pomeron [5]. The relations (3.17) and (3.18) define the exact solution to the Schrödinger equation (3.7) for  $n = 2$ , that is for the color-singlet compound state built from two reggeized gluons.

### 3.3 Heisenberg $SL(2; \mathbb{C})$ spin chain

Using (3.18) one can reconstruct the operator form of the BFKL kernel  $H_{12}$  on the representation space of the principal series of the  $SL(2, \mathbb{C})$  group

$$H_{12} = \frac{1}{2} [H(J_{12}) + H(\bar{J}_{12})], \quad H(J) = 2\psi(1) - \psi(J) - \psi(1-J), \quad (3.19)$$

where, as before, the two-particle spins are defined as  $L_{12}^2 = J_{12}(J_{12} - 1)$  and  $\bar{L}_{12}^2 = \bar{J}_{12}(\bar{J}_{12} - 1)$ . Notice that we already encountered the similar Hamiltonian in Sect. 2 (see Eq. (2.17)) and found that it gives rise to integrability for the dilatation operator.

Most remarkably, the Hamiltonian (3.9) has the same hidden integrability as the dilatation operator (2.17) and it coincides in fact with the Hamiltonian of the  $SL(2, \mathbb{C})$  Heisenberg magnet [2, 3]. The important difference between the two operators is that they are defined on the different space of functions: the operator (2.17) acts on the nonlocal light-ray operators (2.2) which are polynomials in the light-cone coordinates while the eigenfunctions of the operator (3.19) are single-valued functions on the two-dimensional plane, Eq. (3.17). This leads to a dramatic change in the properties of the two evolution kernels.

The number of sites in the Heisenberg  $SL(2, \mathbb{C})$  spin chain (3.9) equals the number of particles and the corresponding spin operators are identified as six generators,  $L_k^\pm, L_k^0$  and

$\bar{L}_k^\pm, \bar{L}_k^0$ , of the  $SL(2, \mathbb{C})$  group. It possesses a large-enough set of mutually commuting conserved charges  $q_n$  and  $\bar{q}_n$  ( $n = 2, \dots, L$ ) such that  $\bar{q}_n = q_n^\dagger$  and  $[\mathbb{H}_L, q_n] = [\mathbb{H}_L, \bar{q}_n] = 0$ . The charges  $q_n$  are polynomials of degree  $n$  in the holomorphic spin operators. They have the following form [2, 3]

$$q_n = \sum_{1 \leq j_1 < j_2 < \dots < j_n \leq L} z_{j_1 j_2} z_{j_2 j_3} \dots z_{j_n j_1} p_{j_1} p_{j_2} \dots p_{j_n} \quad (3.20)$$

with  $z_{jk} = z_j - z_k$  and  $p_j = i\partial_{z_j}$ . The “lowest” charge  $q_2$  is related to the total spin of the system  $h$ . For the principal series of the  $SL(2, \mathbb{C})$  it takes the following values

$$q_2 = -h(h-1), \quad h = \frac{1+n_h}{2} + i\nu_h, \quad (3.21)$$

with  $n_h$  integer and  $\nu_h$  real. The eigenvalues of the integrals of motion,  $q_2, \dots, q_L$ , form the complete set of quantum numbers parameterizing the  $L$ -gluon states (3.7).

Identification of (3.9) as the Hamiltonian of the  $SL(2, \mathbb{C})$  Heisenberg magnet allows us to map the  $L$ -gluon states into the eigenstates of this lattice model. In spite of the fact that the Heisenberg  $SL(2, \mathbb{C})$  magnet represents a generalization of the  $SL(2, \mathbb{R})$  spin chain, finding its exact solution is a much more complicated task. The principal difficulty is that, in distinction with  $SL(2, \mathbb{R})$  magnet, the quantum space of the  $SL(2, \mathbb{C})$  magnet does not possess a highest weight – the so-called “pseudo-vacuum state” – and, as a consequence, conventional methods like the Algebraic Bethe Ansatz method [16] are not applicable. The eigenproblem (3.9) has been solved exactly in Refs. [62–64] using the method of the Baxter  $Q$ -operator [65, 45, 66, 44] which does not rely on the existence of a highest weight. In this approach, it becomes possible to establish the quantization conditions for the integrals of motion  $q_3, \dots, q_L$  and to obtain an explicit form for the dependence of the energy  $E_L$  on the integrals of motion.

In this manner, the spectrum of the  $L$ -gluon state has been calculated for  $L \geq 3$  particles: For  $L = 3$  few low-lying states have been found in [67, 68] and the complete spectrum of states for  $3 \leq L \leq 8$  was determined in [63, 64] (see also [69]). The obtained eigenspectrum has a very rich structure. The quantized values of the conserved  $q$ -charges and the energy  $E_L$  depend on the integer  $n_h$  and the real number  $\nu_h$  defining the total  $SL(2, \mathbb{C})$  spin of the state, Eq. (3.16). In addition, they also depend on the “hidden” set of integers  $\ell = (\ell_1, \ell_2, \dots, \ell_{2(L-2)})$ . As a function of  $\nu_h$ , the charges form a family of trajectories in the moduli space  $\mathbf{q} = (q_2, q_3, \dots, q_L)$  labelled by integers  $n_h$  and  $\ell$ . Each trajectory in the  $q$ -space induces a corresponding trajectory for the energy  $E_L = E_L(\nu_h; n_h, \ell)$ . The origin of these trajectories and the physical interpretation of the integers  $\ell$  can be understood by solving the Schrödinger equation (3.7) within the semiclassical approach described in the next subsection.

### 3.4 Semiclassical limit

In the semiclassical approach [70], we assume that the  $SL(2; \mathbb{C})$  spins  $h$  and  $\bar{h}$  are large and apply the WKB methods to construct the asymptotic solution to (3.7). One might expect a priori that this approach could be applicable only for highly-excited states.

Nevertheless, as was demonstrated in [70], the semi-classical formulae work with good accuracy throughout the whole spectrum.

From the viewpoint of classical dynamics, the multi-gluon states (3.7) are describe by a chain of interacting particles ‘living’ on the two-dimensional  $\vec{b}$ -plane [47, 27]. The classical model inherits the complete integrability of the quantum noncompact spin magnet. Its Hamiltonian and the integrals of motion are obtained from (3.9), (3.19) and (3.20) by replacing the momentum operators by the corresponding classical functions. Since the Hamiltonian (3.9) is given by the sum of holomorphic and antiholomorphic functions, from point of view of classical dynamics the model describes two copies of one-dimensional systems defined on the complex  $z$ - and  $\bar{z}$ -lines. The solutions to the classical equations of motion have a rich structure and turn out to be intrinsically related to the finite-gap solutions to the nonlinear equations [71, 72]; namely, the classical trajectories have the form of plane waves propagating in the chain of  $L$  particles. Their explicit form in terms of the Riemann  $\theta$ -functions was established in [47] by the methods of finite-gap theory [71, 72].

In the semiclassical approach, the eigenfunctions in (3.9) have the standard WKB form,  $\Psi_{\text{WKB}}(\vec{z}_1, \dots, \vec{z}_L) \sim \exp(iS_0/\hbar)$  where the Planck constant  $\hbar = |q_2|^{-1/2}$  is related to the lowest charge (3.21) and the action function  $S_0$  satisfies the Hamilton-Jacobi equations in the classical  $SL(2; \mathbb{C})$  spin chain. It turns out that the solutions to these equations are determined by the same spectral curve (2.27) as for the  $SL(2; \mathbb{R})$  spin chain. The charges  $\mathbf{q}$  define the moduli of this curve and take arbitrary complex values in the classical model. Going over to the quantum model, we find that charges  $\mathbf{q}$  are quantized.

The quantization conditions for the charges  $\mathbf{q}$  follow from the requirement that  $\Psi_{\text{WKB}}(\vec{z}_1, \dots, \vec{z}_L)$  has to be a single-valued function of  $\vec{z}_i$ . As was shown in Refs. [27, 70], these conditions can be expressed in terms of the periods of the ‘‘action’’ differential over the canonical set of the  $\alpha$ - and  $\beta$ -cycles on the Riemann surface corresponding to the complex curve (2.27)

$$\operatorname{Re} \oint_{\alpha_k} dx p(x) = \pi \ell_{2k-1}, \quad \operatorname{Re} \oint_{\beta_k} dx p(x) = \pi \ell_{2k}, \quad (3.22)$$

with  $k = 1, \dots, L-2$  and  $\boldsymbol{\ell} = (\ell_1, \dots, \ell_{2L-4})$  being the set of integers. The relations (3.22) define the system of  $2(L-2)$  real equations for  $(L-2)$  complex charges  $q_3, \dots, q_L$  (we recall that the eigenvalues of the ‘‘lowest’’ charge  $q_2$  are given by (3.21)). Their solution leads to the semiclassical expression for the eigenvalues of the conserved charges. In turn, the energy of the  $L$ -gluon states  $E_{L, \mathbf{q}}$  can be expressed as a function of  $q_3, \dots, q_L$ . In the semiclassical approach, the corresponding expression is

$$\begin{aligned} E_L^{(\text{as})} &= 4 \ln 2 \\ &+ 2 \operatorname{Re} \sum_{k=0}^L \left[ \psi(1 + i \operatorname{Re} \delta_k + |\operatorname{Im} \delta_k|) + \psi(i \operatorname{Re} \delta_k + |\operatorname{Im} \delta_k|) - 2\psi(1) \right], \end{aligned} \quad (3.23)$$

where  $\delta_k$  are roots of the polynomial  $t_L(u)$  defined in (2.24).

The expression in Eq. (3.23) is similar to the energy of the  $SL(2, \mathbb{R})$  magnet in Eq. (2.28) although the properties of the two models are different. As was demonstrated

in [70], the resulting semiclassical expressions for  $q_3, \dots, q_L$  and  $E_L$  are in good agreement with exact results [63, 64]. A novel feature of the quantization conditions (3.22) is that they involve *both* the  $\alpha$ - and  $\beta$ -periods on the Riemann surface. This should be compared with the situation in the Heisenberg  $SL(2, \mathbb{R})$  magnet discussed in Section 2.6. There, the WKB quantization conditions involve only the  $\alpha$ -cycles, Eq. (2.29), since the  $\beta$ -cycles correspond to classically forbidden zones. For the  $SL(2, \mathbb{C})$  magnet, the classical trajectories wrap over an arbitrary closed contour on the spectral curve (2.27) leading to (3.22). This fact allows us to explore the full modular group [73] of the complex curve (2.27) and explain the fine structure of the exact eigenspectrum of the  $SL(2; \mathbb{C})$  magnet. More details can be found in Ref. [70].

## 4 Concluding remarks

In this review, we have described integrability symmetry in application to the deeply inelastic scattering in QCD. Due to space limitations, we did not review various important topics and we refer the interested reader to Ref. [53] for a comprehensive review on the subject. We would like to emphasize that integrability is not of a mere academic interest in QCD as it offers a powerful technique for solving important phenomenological problems such as finding the scale dependence of hadronic structure functions of higher twist and describing their high-energy (Regge) asymptotic behaviour. On theory side, the very fact that QCD evolution equations exhibit integrability property provides yet another indication that QCD possesses some hidden (integrable) structures waiting to be uncovered.

## Acknowledgements

It is a pleasure to thank A. Belitsky, V. Braun, S. Derkachov, A. Gorsky, A. Manashov and D. Müller for an enjoyable collaboration on the topics reviewed above.

## References

- [1] R.K. Ellis, W.J. Stirling, B. Webber, *QCD and Collider Physics, Cambridge Monographs on Particle Physics, Nuclear Physics and Cosmology (No. 8), 2003.*
- [2] L.N. Lipatov, “*High Energy Asymptotics of Multi-Colour QCD and Exactly Solvable Lattice Models*”, JETP Lett. **59**, 596 (1994) [hep-th/9311037].
- [3] L.D. Faddeev, G.P. Korchemsky, “*High energy QCD as a completely integrable model*”, Phys. Lett. B **342**, 311 (1995) [hep-th/9404173].
- [4] G.P. Korchemsky, “*Bethe Ansatz for QCD Pomeron*,” Nucl. Phys. B **443**, 255 (1995) [hep-ph/9501232].

- [5] E.A. Kuraev, L.N. Lipatov, V.S. Fadin, “*The Pommeranchuk singularity in nonabelian gauge theories*,” Sov. Phys. JETP **45**, 199 (1977); I.I. Balitsky, L.N. Lipatov, “*The Pommeranchuk singularity in Quantum Chromodynamics*,” Sov. J. Nucl. Phys. **28**, 822 (1978).
- [6] J. Bartels, “*High-Energy Behavior In A Nonabelian Gauge Theory. 2. First Corrections To  $T(N \rightarrow M)$  Beyond The Leading Lns Approximation*,” Nucl. Phys. B **175**, 365 (1980).
- [7] J. Kwiecinski, M. Praszalowicz, “*Three Gluon Integral Equation And Odd C Singlet Regge Singularities In QCD*,” Phys. Lett. B **94**, 413 (1980).
- [8] V.M. Braun, S.E. Derkachov, A.N. Manashov, “*Integrability of three-particle evolution equations in QCD*,” Phys. Rev. Lett. **81**, 2020 (1998) [hep-ph/9805225].
- [9] A.V. Belitsky, “*Fine structure of spectrum of twist-three operators in QCD*,” Phys. Lett. B **453**, 59 (1999) [hep-ph/9902361]; “*Integrability and WKB solution of twist-three evolution equations*,” Nucl. Phys. B **558**, 259 (1999) [hep-ph/9903512].
- [10] V.M. Braun, S.E. Derkachov, G.P. Korchemsky, A.N. Manashov, “*Baryon distribution amplitudes in QCD*,” Nucl. Phys. B **553**, 355 (1999) [hep-ph/9902375].
- [11] V.M. Braun, G.P. Korchemsky, D. Müller, “*The Uses of Conformal Symmetry in QCD*” Prog. Part. Nucl. Phys. **51**, 311 (2003) [hep-ph/0306057].
- [12] D.J. Gross, F. Wilczek, “*Asymptotically Free Gauge Theories*,” Phys. Rev. D **8**, 3633 (1973); H. Georgi, H.D. Politzer, “*Electroproduction scaling in an asymptotically free theory of strong interactions*,” Phys. Rev. D **9**, 416 (1974).
- [13] A.P. Bukhvostov, G.V. Frolov, L.N. Lipatov, E.A. Kuraev, “*Evolution equations for quasi-partonic operators*,” Nucl. Phys. B **258**, 601 (1985).
- [14] Y.M. Makeenko, “*Conformal operators in quantum chromodynamics*,” Sov. J. Nucl. Phys. **33**, 440 (1981).
- [15] T. Ohrndorf, “*Constraints from conformal covariance on the mixing of operators of lowest twist*,” Nucl. Phys. B **198**, 26 (1982).
- [16] L.A. Takhtajan, L.D. Faddeev, “*The Quantum method of the inverse problem and the Heisenberg XYZ model*,” Russ. Math. Survey **34**, 11 (1979); E.K. Sklyanin, L.A. Takhtajan, L.D. Faddeev, “*Quantum Inverse Problem. Method.I.*,” Theor. Math. Phys. **40**, 688 (1980); V.E. Korepin, N.M. Bogoliubov, A.G. Izergin, *Quantum inverse scattering method and correlation functions*, (Cambridge Univ. Press, 1993).
- [17] S. Simula, “*Soft gluon effects in the extraction of higher twists at large Bjorken  $x$* ,” Phys. Lett. B **493** (2000) 325 [hep-ph/0005315].

- [18] E. Gardi, R. G. Roberts, “*The interplay between Sudakov resummation, renormalons and higher twist in deep inelastic scattering*,” Nucl. Phys. B **653** (2003) 227 [hep-ph/0210429]; E. Gardi, G. P. Korchemsky, D. A. Ross, S. Tafat, “*Power corrections in deep inelastic structure functions at large Bjorken  $x$* ,” Nucl. Phys. B **636** (2002) 385 [hep-ph/0203161].
- [19] G. P. Korchemsky, “*Asymptotics of the Altarelli-Parisi-Lipatov Evolution Kernels of Parton Distributions*,” Mod. Phys. Lett. A **4**, 1257 (1989); G.P. Korchemsky, G. Marchesini, “*Structure function for large  $x$  and renormalization of Wilson loop*,” Nucl. Phys. B **406**, 225 (1993).
- [20] A.V. Belitsky, A.S. Gorsky, G.P. Korchemsky, “*Gauge/string duality for QCD conformal operators*,” Nucl. Phys. B **667**, 3 (2003) [hep-th/0304028].
- [21] G. P. Korchemsky, A. V. Radyushkin, “*Renormalization of the Wilson Loops Beyond the Leading Order*,” Nucl. Phys. B **283**, 342 (1987).
- [22] A.M. Polyakov, “*Gauge fields as rings of glue*,” Nucl. Phys. B **164**, 171 (1980).
- [23] I. A. Korchemskaya, G. P. Korchemsky, “*On lightlike Wilson loops*,” Phys. Lett. B **287**, 169 (1992); A. Bassetto, I. A. Korchemskaya, G. P. Korchemsky, G. Nardelli, “*Gauge invariance and anomalous dimensions of a light cone Wilson loop in lightlike axial gauge*,” Nucl. Phys. B **408**, 62 (1993) [hep-ph/9303314].
- [24] S. V. Ivanov, G. P. Korchemsky, A. V. Radyushkin, “*Infrared Asymptotics Of Perturbative QCD: Contour Gauges*,” Yad. Fiz. **44**, 230 (1986) [Sov. J. Nucl. Phys. **44** (1986) 145]; G. P. Korchemsky, A. V. Radyushkin, “*Loop Space Formalism And Renormalization Group For The Infrared Asymptotics Of QCD*,” Phys. Lett. B **171**, 459 (1986); “*Infrared factorization, Wilson lines and the heavy quark limit*,” Phys. Lett. B **279**, 359 (1992) [hep-ph/9203222].
- [25] J. M. Drummond, G. P. Korchemsky, E. Sokatchev, “*Conformal properties of four-gluon planar amplitudes and Wilson loops*,” Nucl. Phys. **B795**, 385 (2008) [0707.0243 [hep-th]].
- [26] A.V. Belitsky, G.P. Korchemsky, D. Mueller, “*Integrability in Yang-Mills theory on the light cone beyond leading order*,” Phys. Rev. Lett. **94** (2005) 151603 [hep-th/0412054]; “*Integrability of two-loop dilatation operator in gauge theories*,” Nucl. Phys. B **735** (2006) 17 [hep-th/0509121]; “*Towards Baxter equation in supersymmetric Yang-Mills theories*,” Nucl. Phys. B **768** (2007) 116 [hep-th/0605291];
- [27] A. Gorsky, I.I. Kogan, G.P. Korchemsky, “*High Energy QCD: Stringy Picture from Hidden Integrability*,” JHEP **0205**, 053 (2002) [hep-th/0204183].
- [28] J.M. Maldacena, “*The Large  $N$  Limit of Superconformal Field Theories and Supergravity*,” Adv. Theor. Math. Phys. **2**, 231 (1998) [hep-th/9711200]; S.S. Gubser, I.R. Klebanov, A.M. Polyakov, “*Gauge theory correlators from non-critical string theory*,” Phys. Lett. B **428**, 105 (1998) [hep-th/9802109]; E. Witten, “*Anti De Sitter Space And Holography*,” Adv. Theor. Math. Phys. **2**, 253 (1998) [hep-th/9802150].

- [29] S.A. Anikin, O.I. Zavyalov, “*Short Distance and Light Cone Expansions for Products of Currents*,” *Annals Phys.* **116**, 135 (1978).
- [30] I.I. Balitsky, V.M. Braun, “*Evolution equations for QCD string operators*,” *Nucl. Phys. B* **311**, 541 (1989).
- [31] D. Müller, D. Robaschik, B. Geyer, F. M. Dittes, J. Horejsi, “*The Altarelli-Parisi kernel as asymptotic limit of an extended Brodsky-Lepage kernel*,” *Phys. Lett. B* **209**, 325 (1988); “*Wave Functions, Evolution Equations and Evolution Kernels from Light-Ray Operators of QCD*,” *Fortsch. Phys.* **42**, 101 (1994) [hep-ph/9812448].
- [32] A.V. Belitsky, S.E. Derkachov, G.P. Korchemsky, A.N. Manashov, “*Quantum integrability in (super) Yang-Mills theory on the light-cone*,” *Phys. Lett. B* **594**, 385 (2004) [hep-th/0403085]; “*Dilatation operator in (super-)Yang-Mills theories on the light-cone*,” *Nucl. Phys. B* **708** (2005) 115 [hep-th/0409120].
- [33] J.B. Kogut, D.E. Soper, “*Quantum Electrodynamics in the Infinite-Momentum Frame*,” *Phys. Rev. D* **1** (1970) 2901.
- [34] L. Brink, O. Lindgren, B.E. Nilsson, “ *$N = 4$  Yang-Mills theory on the light cone*,” *Nucl. Phys. B* **212**, 401 (1983); “*The ultra-violet finiteness of the  $N=4$  Yang-Mills theory*,” *Phys. Lett. B* **123**, 323 (1983).
- [35] S. Mandelstam, “*Light Cone Superspace And The Ultraviolet Finiteness Of The  $N=4$  Model*,” *Nucl. Phys. B* **213**, 149 (1983).
- [36] S.J. Brodsky, G.P. Lepage, “*Exclusive processes in perturbative quantum chromodynamics*,” *Phys. Rev. D* **22** (1980) 2157.
- [37] P.P. Kulish, N.Yu. Reshetikhin, E.K. Sklyanin, “*Yang-Baxter equations and representation theory*,” *Lett. Math. Phys.* **5**, 393 (1981).
- [38] V.O. Tarasov, L.A. Takhtajan, L.D. Faddeev, “*Local Hamiltonians for integrable quantum models on a lattice*,” *Theor. Math. Phys.* **57**, 1059 (1983).
- [39] A.V. Belitsky, “*Renormalization of twist-three operators and integrable lattice models*,” *Nucl. Phys. B* **574**, 407 (2000) [hep-ph/9907420].
- [40] S.E. Derkachov, G.P. Korchemsky, A.N. Manashov, *Nucl. Phys. B* **566**, 203 (2000) [hep-ph/9909539].
- [41] A.V. Belitsky, “*Renormalization of twist-three operators and integrable lattice models*,” *Nucl. Phys. B* **574** (2000) 407 [hep-ph/9907420].
- [42] S.E. Derkachov, “*Baxter’s Q-operator for the homogeneous XXX spin chain*,” *J. Phys. A: Math. Gen.* **32**, 5299 (1999).
- [43] G. P. Korchemsky, “*Quasiclassical QCD pomeron*,” *Nucl. Phys. B* **462** (1996) 333 [hep-th/9508025].

- [44] V. Pasquier, M. Gaudin, “*The periodic Toda chain and a matrix generalization of the Bessel function’s recursion relations*,” J. Phys. A: Math. Gen. **25**, 5243 (1992).
- [45] E.K. Sklyanin, Lecture Notes in Physics, vol. 226, Springer, 1985, pp. 196–233; *Functional Bethe ansatz*, in *Integrable and superintegrable systems*, ed. B.A. Kupershmidt, (World Scientific, 1990), pp. 8–33; Progr. Theor. Phys. Suppl. **118**, 35 (1995) [solv-int/9504001].
- [46] G. P. Korchemsky, “*Integrable structures and duality in high-energy QCD*,” Nucl. Phys. B **498** (1997) 68 [hep-th/9609123].
- [47] G. P. Korchemsky, I. M. Krichever, “*Solitons in high-energy QCD*,” Nucl. Phys. B **505** (1997) 387 [hep-th/9704079].
- [48] A. V. Belitsky, A. S. Gorsky, G. P. Korchemsky, “*Logarithmic scaling in gauge/string correspondence*,” Nucl. Phys. B **748** (2006) 24 [hep-th/0601112].
- [49] L. Freyhult, “*Review of AdS/CFT Integrability, Chapter III.4: Twist states and the cusp anomalous dimension*,” arXiv:1012.3993 [hep-th].
- [50] M.F. Sohnius, P.C. West, “*Conformal invariance in  $N = 4$  supersymmetric Yang-Mills theory*,” Phys. Lett. B **100**, 245 (1981).
- [51] P.S. Howe, K.S. Stelle, P.K. Townsend, “*Miraculous ultraviolet cancellations in supersymmetry made manifest*,” Nucl. Phys. B **236**, 125 (1984).
- [52] L. Brink, A. Tollstén, “ *$N = 4$  Yang-Mills theory in terms of  $N = 3$  and  $N = 2$  light-cone superfields*,” Nucl. Phys. B **249**, 244 (1985).
- [53] A. V. Belitsky, V. M. Braun, A. S. Gorsky, G. P. Korchemsky, “*Integrability in QCD and beyond*,” Int. J. Mod. Phys. A **19** (2004) 4715 [hep-th/0407232].
- [54] D. Müller, “*Conformal constraints and the evolution of the nonsinglet meson distribution amplitude*,” Phys. Rev. D **49**, 2525 (1994); A.V. Belitsky, D. Müller, “*Broken conformal invariance and spectrum of anomalous dimensions in QCD*,” Nucl. Phys. B **537**, 397 (1999) [hep-ph/9804379].
- [55] M. Grabowski, P. Mathieu, “*Quantum integrals of motion for the Heisenberg spin chain*,” Mod. Phys. Lett. A **9** (1994) 2197.
- [56] N. Beisert et al., “*Review of AdS/CFT Integrability, An Overview*,” arXiv:1012.3982 [hep-th].
- [57] C. Kristjansen, “*Review of AdS/CFT Integrability, Chapter IV.1: Aspects of Non-planarity*,” arXiv:1012.3997 [hep-th].
- [58] G. Ferretti, R. Heise, K. Zarembo, “*New integrable structures in large- $N$  QCD*,” Phys. Rev. D **70** (2004) 074024 [hep-th/0404187]; N. Beisert, G. Ferretti, R. Heise, K. Zarembo, “*One-loop QCD spin chain and its spectrum*,” Nucl. Phys. B **717** (2005) 137 [hep-th/0412029].

- [59] V. M. Braun, A. N. Manashov, J. Rohrwild, “*Renormalization of Twist-Four Operators in QCD*,” Nucl. Phys. B **826**, 235 (2010) [0908.1684 [hep-ph]].
- [60] L.N. Lipatov, “*Pomeron and odderon in QCD and a two dimensional conformal field theory*,” Phys. Lett. B **251**, 284 (1990); “*High energy asymptotics of multi-colour QCD and two-dimensional conformal field theories*,” Phys. Lett. B **309**, 394 (1993).
- [61] L.N. Lipatov, “*The bare pomeron in Quantum Chromodynamics*,” Sov. Phys. JETP **63**, 904 (1986)
- [62] S.E. Derkachov, G.P. Korchemsky, A.N. Manashov, “*Noncompact Heisenberg spin magnets from high-energy QCD: I. Baxter Q-operator and Separation of Variables*,” Nucl. Phys. B **617**, 375 (2001) [hep-th/0107193].
- [63] G.P. Korchemsky, J. Kotanski, A.N. Manashov, “*Solution of the multi-reggeon compound state problem in multi-colour QCD*,” Phys. Rev. Lett. **88**, 122002 (2002) [hep-ph/0111185].
- [64] S.E. Derkachov, G.P. Korchemsky, J. Kotanski, A.N. Manashov, “*Noncompact Heisenberg spin magnets from high-energy QCD: II. Quantization conditions and energy spectrum*,” Nucl. Phys. B **645**, 237 (2002) [hep-th/0204124].
- [65] R.J. Baxter, *Exactly Solved Models in Statistical Mechanics*, (Academic Press, London, 1982).
- [66] V. V. Bazhanov, Yu. G. Stroganov, “*Chiral Potts model as a descendant of the six vertex model*,” J. Stat. Phys. **59** (1990) 799.
- [67] R.A. Janik, J. Wosiek, “*Solution of the odderon problem for arbitrary conformal weights*,” Phys. Rev. Lett. **79**, 2935 (1997) [hep-th/9610208]; “*Solution of the odderon problem*,” Phys. Rev. Lett. **82**, 1092 (1999) [hep-th/9802100].
- [68] J. Bartels, L. N. Lipatov, G. P. Vacca, “*A new odderon solution in perturbative QCD*,” Phys. Lett. B **477**, 178 (2000) [hep-ph/9912423].
- [69] H. J. De Vega, L. N. Lipatov, “*Interaction of Reggeized gluons in the Baxter-Sklyanin representation*,” Phys. Rev. D **64**, 114019 (2001) [hep-ph/0107225]; “*Exact resolution of the Baxter equation for reggeized gluon interactions*,” Phys. Rev. D **66**, 074013 (2002) [hep-ph/0204245].
- [70] S.E. Derkachov, G.P. Korchemsky, A.N. Manashov, “*Noncompact Heisenberg spin magnets from high-energy QCD: III. Quasiclassical approach*,” Nucl. Phys. B **661**, 533 (2003) [hep-th/0212169].
- [71] S.P. Novikov, S.V. Manakov, L.P. Pitaevskii, V.E. Zakharov, *Theory of Solitons: The Inverse Scattering Method*, (Consultants Bureau, New York, 1984); B.A. Dubrovin, V.B. Matveev, S.P. Novikov, “*Non-linear Equations of Korteweg-de Vries Type, Finite-Zone Linear Operators, and Abelian Varieties*,” Russ. Math. Surv. **31**, 59 (1976).

- [72] I.M. Krichever, “*Methods of algebraic geometry in the theory of non-linear equations,*” Russ. Math. Surv. **32**, 185 (1977); “*Integration of nonlinear equations by the methods of algebraic geometry,*” Func. Anal. Appl. **14**, 531 (1980); **11**, 12 (1977).
- [73] B.A. Dubrovin, “*Theta functions and non-linear equations,*” Russ. Math. Surv. **36**, 11 (1981).

# Review of AdS/CFT Integrability, Chapter V.1: Scattering Amplitudes – a Brief Introduction

R. ROIBAN

*Department of Physics, The Pennsylvania State University  
University Park, PA 16802, USA*

radu@phys.psu.edu

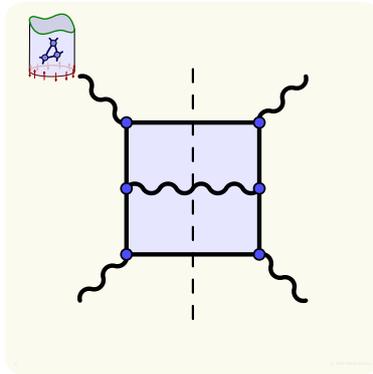

**Abstract:** We review current efficient techniques for the construction of multi-leg and multi-loop on-shell scattering amplitudes in supersymmetric gauge theories. Examples in the maximally supersymmetric Yang-Mills theory in four dimensions are included.

## 1 Introduction

The scattering amplitudes of on-shell excitations are perhaps the most basic quantities in any quantum field theory. They provide the only link between models of Nature and experimental data, being thus an indispensable tool for testing theoretical ideas about high energy physics. They also contain a wealth of off-shell information, such as certain anomalous dimensions of composite operators, making their evaluation an important alternative approach to direct off-shell calculations.

Scattering amplitudes may exhibit larger symmetries than the Lagrangian<sup>1</sup>. For example, as reviewed in [1] in this volume, it was shown that the tree-level S-matrix of the  $\mathcal{N} = 4$  super-Yang-Mills theory (sYM) is invariant [2] under the Yangian of the four-dimensional superconformal group, even though this is not a symmetry of the Lagrangian. Part of this invariance was initially observed as symmetries of higher-loop amplitudes [3]. Thus, in this theory, (tree-level) scattering amplitudes realize the symmetries responsible for the integrability of its dilatation operator and of the worldsheet theory of its string theory dual. With more symmetry, one may hope that scattering amplitudes have simpler structure than one may naively expect.

Textbook approaches to scattering amplitude calculations make use of Feynman diagrams. Symmetries, however, even those of the Lagrangian, are obscured in this approach, re-emerging only after all Feynman diagrams are assembled. For this reason, even at tree level, the evaluation of multi-leg amplitudes can become quite involved. Multi-loop amplitudes have similar features. Nevertheless, the fact that scattering amplitudes to any loop order are computable in terms of Feynman diagrams is an invaluable guide for identifying new techniques bypassing their difficulties.

Here we review the basics of modern on-shell methods for the evaluation of scattering amplitudes – the (super)MHV vertex expansion, on-shell recursion relations and the generalized unitarity-based method. Other methods and developments are briefly mentioned in the concluding section.

## 2 Organization, presentation, relations between amplitudes

Whether carried out in terms of Feynman diagrams or by other means, a good notation and a transparent organization of the calculation and results are indispensable ingredients of an efficient calculation of scattering amplitudes. Color ordering separates the color flow from momentum flow and thus separates amplitudes into smaller gauge-invariant parts – the color-ordered amplitudes. Projection of these parts onto definite helicity configurations leads to partial amplitudes with useful properties and simple structure. An enlightening discussion of these topics may be found in [4]. Here we briefly summarize the salient points.

---

<sup>1</sup>At tree-level it is possible to argue that they have the same symmetries as the equations of motion.

## 2.1 Spinor helicity and color ordering

In a massless theory, solutions of the chiral Dirac equation provide an parametrization of momenta and polarization vectors [5] which allows *e.g.* the construction of physical polarization vectors without fixing noncovariant gauges. At the basis of this parametrization lies the well-known relation

$$(k_\mu \bar{\sigma}^\mu)^{\dot{\alpha}\alpha} u_{-\alpha}(k) = 0 \quad ; \quad u_-(k) \bar{u}_-(k) = -k_\mu \sigma^\mu \quad , \quad (2.1)$$

where as usual  $\sigma = (\mathbf{1}, \boldsymbol{\sigma})$  and  $\bar{\sigma} = (\mathbf{1}, -\boldsymbol{\sigma})$  are the Pauli matrices . This factorization also follows more formally from the fact that the matrix on the right-hand-side of equation (2.1) has unit rank if the momentum  $k$  is null. It is common<sup>2</sup> to denote  $u_-(k)$  and  $\bar{u}_-(k)$  by  $\lambda$  and  $\tilde{\lambda}$ , respectively. Multiplication of spinors is dictated by Lorentz invariance:

$$\langle ij \rangle = \epsilon^{\alpha\beta} \lambda_{i\alpha} \lambda_{j\beta} \quad [ij] = -\epsilon^{\dot{\alpha}\dot{\beta}} \tilde{\lambda}_{i\dot{\alpha}} \tilde{\lambda}_{j\dot{\beta}} \quad . \quad (2.2)$$

Gauge invariance constrains the physical polarization vectors; they must also be transverse and take the standard form of circular polarization vectors in the relevant frame. They can be constructed in terms of  $\lambda$ ,  $\tilde{\lambda}$  and arbitrary fixed spinors  $\xi$  and  $\tilde{\xi}$ :

$$\epsilon_{\alpha\dot{\alpha}}^-(k, \xi) = -\sqrt{2} \frac{\lambda_\alpha \tilde{\xi}_{\dot{\alpha}}}{[\xi k]} \quad \epsilon_{\alpha\dot{\alpha}}^+(k, \xi) = \sqrt{2} \frac{\xi_\alpha \tilde{\lambda}_{\dot{\alpha}}}{\langle \xi k \rangle} \quad . \quad (2.3)$$

The freedom of choosing independently reference spinors for each of the gluons participating in the scattering process makes it easy to prove that tree-level gluon amplitudes with less than two gluons of the same helicity vanish identically. The first nonvanishing tree-level amplitudes have two gluons of the same helicity opposite from the other ones; they are known as maximally helicity-violating (MHV) amplitudes. In supersymmetric theories this pattern holds to all orders in perturbation theory.

A clean organization of scattering amplitudes is a second useful ingredient in the construction of scattering amplitudes at any fixed loop order  $L$ . Besides the organization following the helicity of external states, at each loop order an organization following the color structure is also possible and desirable, if only because, for  $n$ -point amplitudes, there are at most  $(n-1)!$  gauge invariant components. For an  $SU(N)$  gauge theory with gauge group generators denoted by  $T^a$ , any  $L$ -loop amplitude may be decomposed as follows [6]:

$$\mathcal{A}_n^{(L)} = N^L \sum_{\rho \in S_n / \mathbb{Z}_n} \text{Tr}[T^{a_{\rho(1)}} \dots T^{a_{\rho(n)}}] A_n^{(L)}(k_{\rho(1)} \dots k_{\rho(n)}, N^{-1}) + \text{multi-traces} \quad , \quad (2.4)$$

where the sum extends over all non-cyclic permutations  $\rho$  of  $(1 \dots n)$ . The coefficients  $A(k_{\rho(1)} \dots k_{\rho(n)}, N^{-1})$  are called color-ordered amplitudes. The  $(n-1)!$  color-ordered

---

<sup>2</sup>In Minkowski signature  $\lambda$  and  $\tilde{\lambda}$  are complex conjugate of each other and the factorization (2.1) exhibits a rephasing invariance  $\lambda \mapsto S\lambda$ ,  $\tilde{\lambda} \mapsto S^{-1}\tilde{\lambda}$  with  $S^* = S^{-1}$ . It is useful to promote momenta to (holomorphic) complex variables and the Lorentz group to  $SL(2, \mathbb{C}) \times SL(2, \mathbb{C})$ . Then,  $\lambda$  and  $\tilde{\lambda}$  become independent complex variables and rephasing by  $S$  becomes rescaling by an arbitrary complex number. Scattering amplitudes have definite scaling properties under this transformation.

amplitudes in (2.4) are not independent; in [7] and [8] it was shown how to express them in terms of  $(n-2)!$  and  $(n-3)!$  basic amplitudes, respectively.

In the limit of large number of colors,  $N \rightarrow \infty$ , the multi-trace terms left unspecified in the equation above drop out. The same is true for all  $N$ -dependent terms in  $A_n(k_{\rho(1)} \dots k_{\rho(n)}, N^{-1})$ , reducing them to planar partial amplitudes  $A_n(k_{\rho(1)} \dots k_{\rho(n)})$ . In this limit we will normalize the loop expansion parameter as

$$a = \frac{g^2 N}{8\pi^2} \quad (2.5)$$

Color ordered scattering amplitudes have definite transformation properties under cyclic permutation of (subsets of) external legs. They also have definite factorization properties in limits in which external momenta reach certain singular configurations. *E.g.* the tree-level collinear and multi-particle factorization formulae are

$$A_n^{(0)}(1 \dots (n-1)^{h_{n-1}}, n^{h_n}) \xrightarrow{k_{n-1} || k_n} \sum_h A_{n-1}^{(0)}(1 \dots k^h) \text{Split}_{-h}^{(0)}((n-1)^{h_{n-1}}, n^{h_n}) \quad , \quad (2.6)$$

$$A_n^{(0)}(1, \dots, n) \xrightarrow{k_{1,m}^2 \rightarrow 0} \sum_{h=\pm} A_{m+1}^{(0)}(1, \dots, m, k_{1,m}^h) \frac{i}{k_{1,m}^2} A_{n-m+1}^{(0)}(-k_{1,m}^{-h}, m+1, \dots, n) \quad (2.7)$$

where  $\text{Split}^{(0)}$  is a universal function known as the tree-level splitting amplitude. These properties, and their higher-loop generalizations, provide stringent tests on the direct evaluation of higher-loop amplitudes and the validity of new methods proposed for this purpose. For a thorough discussion we refer the reader to the original literature [9–11].

## 2.2 Superspace and supersymmetry relations

Supersymmetric field theories are more constrained than their non-supersymmetric counterparts. Through supersymmetric Ward identities [12], supersymmetry implies nontrivial relations between scattering amplitudes to all orders in perturbation theory. For example, the vanishing of all gluon amplitudes with less than two gluons of helicity different from the rest may be understood as a consequence of supersymmetry. Tree-level supersymmetry relations between gluon scattering amplitudes hold in all theories, regardless of their amount of supersymmetry or of their field content.

Supersymmetric Ward identities imply that not all amplitudes are independent; rather, most of them are generated from certain "basic" amplitudes by repeated application of supersymmetry transformations. *E.g.*, MHV amplitudes, differing by the position of the negative helicity gluons, are all related by supersymmetry transformations. The next-to-MHV amplitudes (involving three negative helicity gluons) and their superpartners, are generated by three independent amplitudes [13, 14]. A general solution to the relations imposed by supersymmetry Ward identities in  $\mathcal{N} = 4$  sYM theory and in  $\mathcal{N} = 8$  supergravity was discussed in [14].

Chiral superspace provides an efficient organization of the scattering amplitudes of the  $\mathcal{N} = 4$  sYM theory. The physical states are assembled into a single superfield

$$\Phi(x, \eta) = \frac{1}{4!} g_{abcd}^+ \eta^a \eta^b \eta^c \eta^d + \frac{1}{3!} f_{abc}^+ \eta^a \eta^b \eta^c + \frac{1}{2!} s_{ab} \eta^a \eta^b + f_a^- \eta^a + g^- \quad , \quad (2.8)$$

where  $\eta$  denote the anticommuting superspace coordinates, transforming in the fundamental representation of the R-symmetry group  $SU(4)$ ;  $g_{\pm}$  and  $f_{\pm}$  are, respectively, the positive and negative helicity gluons and gluinos and  $s_{ab}$  are scalars. Component amplitudes are repackaged into superamplitudes and can be extracted by multiplication with a superfield containing only the desired component field for each external leg and integration over all anticommuting superspace coordinates.

The fact that all MHV amplitudes are related by a suitable chain of supersymmetry transformations is reflected by the fact that all MHV amplitudes may be assembled into a single-term superamplitude proportional to the conservation constraint for the chiral supercharge  $Q^{\alpha\alpha} = \sum_i \lambda_i^{\alpha} \eta_i^{\alpha}$ :

$$\mathcal{A}_n^{(0),\text{MHV}}(1, 2, \dots, n) \equiv \frac{i}{\prod_{j=1}^n \langle j (j+1) \rangle} \delta^{(8)} \left( \sum_{j=1}^n \lambda_{\alpha}^j \eta_j^{\alpha} \right). \quad (2.9)$$

The  $\overline{\text{MHV}}$  superamplitudes in chiral superspace is more complicated [15, 16]:

$$\mathcal{A}_n^{(0),\overline{\text{MHV}}}(1, 2, \dots, n) = \frac{i}{\prod_{j=1}^n [j (j+1)]} \int \prod_{a=1}^4 d^8 \omega^a \prod_{i=1}^n \delta^{(4)}(\eta_i^{\alpha} - \tilde{\lambda}_i^{\dot{\alpha}} \omega_{\dot{\alpha}}^a). \quad (2.10)$$

Supersymmetric Ward identities imply that, to all orders in perturbation theory, MHV and  $\overline{\text{MHV}}$  superamplitudes are proportional to the corresponding tree-level superamplitude. The proportionality coefficient, henceforth called scalar factor and denoted by  $M_n^{(l)}$  where  $n$  is the number of external legs and  $l$  is the loop order, is a completely symmetric scalar function of momentum invariants which naturally splits into parity-even and a parity-odd components. The superamplitude containing the gluon amplitudes with  $(k+2)$  negative helicity gluons (the so-called  $N^k\text{MHV}$  amplitudes) contains  $4(k+2)$  delta functions whose arguments are linear combinations of anticommuting coordinates. Examples for  $k=1$  may be found in [17].

The dual superspace, in which the superfield is related to (2.8) by a fermionic Fourier transform is also extensively used [17, 18]. While the superamplitude is unchanged, one extracts component amplitudes by applying suitable fermionic differential operators. For example, to extract a gluon amplitude one differentiates solely with respect to the  $\eta$  parameters corresponding to the negative helicity gluons.

### 2.3 Factorization of infrared divergences

A general feature of on-shell scattering amplitudes in massless theories is the presence of infrared divergences.<sup>3</sup> Unlike ultraviolet divergences they cannot be renormalized away; rather, they cancel in infrared-safe quantities, such as cross sections of color-singlet states, anomalous dimensions, etc.

There are two sources of infrared divergences in a massless theory: the small energy region of some virtual particle and the region in which some virtual particle is collinear

<sup>3</sup>While absent in the  $\mathcal{N}=4$  sYM theory, in general massless theories ultraviolet divergences are, of course, present as well.

with some external particle, respectively:

$$\int \frac{d\omega}{\omega^{1+\epsilon}} \propto \frac{1}{\epsilon} \quad \int \frac{dk_T}{k_T^{1+\epsilon}} \propto \frac{1}{\epsilon} . \quad (2.11)$$

Since they can occur simultaneously, the leading infrared singularity at  $L$ -loops is an  $1/\epsilon^{2L}$  pole in dimensional regularization.

The structure of soft and collinear singularities in a massless gauge theory in four dimensions has been extensively studied and understood [19–22]. The realization that soft and virtual collinear effects can be factorized in a universal way, together with the fact [23] that the soft radiation can be further factorized from the (harder) collinear one, led to a three-factor structure for gauge theory scattering amplitudes [22, 24]:

$$\mathcal{M}_n = \left[ \prod_{i=1}^n J_i \left( \frac{Q}{\mu}, \alpha_s(\mu), \epsilon \right) \right] \times S \left( k, \frac{Q}{\mu}, \alpha_s(\mu), \epsilon \right) \times h_n \left( k, \frac{Q}{\mu}, \alpha_s(\mu), \epsilon \right) . \quad (2.12)$$

Here the product runs over all the external lines,  $Q$  is the factorization scale, separating soft and collinear momenta,  $\mu$  is the renormalization scale and  $\alpha_s(\mu) = \frac{g(\mu)^2}{4\pi}$  is the running coupling at scale  $\mu$ . Both  $h_n(k, Q/\mu, \alpha_s(\mu), \epsilon)$  and the amplitude  $\mathcal{M}_n$  are vectors in the space of color configurations available for the scattering process. The soft function  $S(k, Q/\mu, \alpha_s(\mu), \epsilon)$  is a matrix acting on this space; it is defined up to a multiple of the identity matrix. It captures the soft gluon radiation, it is responsible for the purely infrared poles and it can be computed in the eikonal approximation in which the hard partonic lines are replaced by Wilson lines. The “jet” functions  $J_i(Q/\mu, \alpha_s(\mu), \epsilon)$  are color-singlets and contain the complete information on collinear dynamics of virtual particles. Finally,  $h_n(k, Q/\mu, \alpha_s(\mu), \epsilon)$  contains the effects of highly virtual fields and is finite as  $\epsilon \rightarrow 0$ . The jet and soft functions can be independently defined and evaluated in terms of specific matrix elements.

In the planar limit all except one color structure are subdominant; the soft function is then proportional to the identity matrix and may be absorbed into the definition of the jet functions reducing equation (2.12) to a two-factor expression. In this limit, the jet function may be given a physical interpretation by using the factorized form of the amplitude for the decay of a color-singlet state into two gluons of momenta  $k_i$  and  $k_{i+1}$ . This is, by definition, the Sudakov form factor  $\mathcal{M}^{[gg \rightarrow 1]}(s_{i,i+1}/\mu, \lambda(\mu), \epsilon)$ . With this information the factorized form of a general planar amplitude is

$$\mathcal{M}_n = \left[ \prod_{i=1}^n \mathcal{M}^{[gg \rightarrow 1]} \left( \frac{Q}{\mu}, \lambda(\mu), \epsilon \right) \right]^{1/2} \times h_n \left( k, \frac{Q}{\mu}, \lambda(\mu), \epsilon \right) , \quad (2.13)$$

where  $\lambda(\mu) = g(\mu)^2 N$  is the 't Hooft coupling. Here  $\mathcal{M}_n$  denotes the unique single-trace structure relevant in the planar limit.

Independence on the factorization scale  $Q$  implies that the Sudakov form factor obeys certain renormalization group type equations which relate it to the cusp anomalous dimension as well as to another function — the “collinear anomalous dimension” — whose physical interpretation is less transparent (see however [25]). For their derivation

and analysis we shall refer the reader to the original literature [20, 26]. Their solution for  $\mathcal{N} = 4$  sYM is [27]:

$$\mathcal{M}_n = \exp \left[ -\frac{1}{8} \sum_{l=1}^{\infty} a^l \left( \frac{\gamma_K^{(l)}}{(l\epsilon)^2} + \frac{2\mathcal{G}_0^{(l)}}{l\epsilon} \right) \sum_{i=1}^n \left( \frac{\mu^2}{-s_{i,i+1}} \right)^{l\epsilon} \right] \times h_n \quad , \quad (2.14)$$

where the cusp anomaly (universal scaling function) and the collinear anomalous dimension are constructed from the coefficients  $\gamma_K^{(l)}$  and  $\mathcal{G}_0^{(l)}$  as:

$$f(\lambda) \equiv \gamma_K(\lambda) = \sum_l a^l \gamma_K^{(l)} \quad G_0 = \sum_l \mathcal{G}_0^{(l)} a^l \quad . \quad (2.15)$$

In writing (2.14) it was assumed that the factorization scale of IR divergences associated to the external legs carrying momenta  $k_i$  and  $k_{i+1}$  is  $Q = s_{i,i+1}$ .

The detailed structure of IR divergences of scattering amplitudes described above used to great effect [28] for the evaluation of the 4-loop cusp anomaly which tests the detailed structure of the BES equation [29] and thus of integrability for  $\mathcal{N} = 4$  sYM theory. The BES equation provides all-order results for  $\gamma_K$ ; no such all-order determination of the collinear anomalous dimension is available, though its relation to other anomalous dimensions [25] may remedy this situation.

### 3 Tree level amplitudes

All symmetries of the Lagrangian of a quantum field theory are visible in its on-shell scattering amplitudes. Scattering amplitudes may however have more symmetries than the Lagrangian. New presentations of scattering amplitudes may thus expose hitherto unsuspected hidden properties of the theory.

An enigmatic presentation of tree-level scattering superamplitudes of  $\mathcal{N} = 4$  sYM followed [30] from Witten's interpretation of the theory as a topological string theory in the super-twistor space of super-Minkowski space. The generating function of tree-level amplitudes with  $n$  external legs is

$$A_n = \sum_{d=2}^{n-3} \int d\mathcal{M}_{1,d} \langle J_1 \dots J_n \rangle \quad (3.1)$$

where  $d\mathcal{M}_{1,d}$  is the integration measure over the moduli space of maps of degree  $d$  from  $S^2$  to  $CP^{3|4}$  and  $J_i$  are certain free fermion currents. Recently, the properties of this presentation of amplitudes started being understood [31] through the Grassmannian interpretation of the tree-level amplitudes.

Witten's interpretation of  $\mathcal{N} = 4$  sYM theory as a topological string theory also led to the MHV vertex rules [32] subsequently generalized to the super-MHV vertex rules.<sup>4</sup> They are effective rules expressing general amplitudes as sums of products of MHV superamplitudes. The following (super)steps generate the  $n$ -point  $N^k$ MHV gauge theory superamplitude:

<sup>4</sup>The MHV (super)vertex rules were proven from a Lagrangian standpoint in [33].

- draw all tree graphs with  $(k + 1)$  vertices, on which the  $n$  external legs are distributed in all possible inequivalent ways while maintaining the color order.
- to each vertex associate an MHV superamplitude (2.9). The holomorphic spinor  $\lambda_P$  of an internal line is constructed from the off-shell momentum  $P$  of that line using a fixed arbitrary reference anti-holomorphic spinor  $\zeta^{\dot{\alpha}}$ :

$$\lambda_{P\alpha} \equiv P_{\alpha\dot{\alpha}}\zeta^{\dot{\alpha}}. \quad (3.2)$$

Alternatively, the holomorphic spinor  $\lambda_P = |P^b\rangle$  is constructed from the null projection of the off-shell momentum  $P$  along a reference null vector  $\zeta^\mu$  common for all legs [34]:

$$P^b = P - \frac{P^2}{2\zeta \cdot P}\zeta. \quad (3.3)$$

- to each internal line associate a super-propagator, *i.e.* a standard scalar Feynman propagator  $i/P^2$  and a factor which equates the fermionic coordinates  $\eta$  of the internal line in the two vertices connected by it.<sup>5</sup>
- integrate over all the anticommuting coordinates associated to internal lines.

Upon application of these rules, the  $N^k$ MHV superamplitude is given by

$$\mathcal{A}_n^{N^k\text{MHV}} = i^m \sum_{\text{all graphs}} \int \left[ \prod_{j=1}^k \frac{d^4\eta_j}{P_j^2} \right] \mathcal{A}_{(1)}^{\text{MHV}} \mathcal{A}_{(2)}^{\text{MHV}} \dots \mathcal{A}_{(k)}^{\text{MHV}} \mathcal{A}_{(k+1)}^{\text{MHV}}, \quad (3.4)$$

where the integral is over the  $4k$  internal Grassmann parameters ( $d^4\eta_j \equiv \prod_{a=1}^4 d\eta_j^a$ ) and each  $P_j$  is the off-shell momentum of the  $j$ 'th internal leg of the graph.

Each integration  $\int d^4\eta_i$  in (3.4) selects the configurations with exactly four distinct  $\eta$ -variables  $\eta_i^1\eta_i^2\eta_i^3\eta_i^4$  on each of the internal lines. Since a particular  $\eta_i^a$  can originate from either of two MHV amplitudes connected by the internal line  $i$ , there are  $2^4$  possibilities that may give non-vanishing contributions. However, for a given choice of external states, each term corresponding to a distinct graph in (3.4) receives nonzero contributions from exactly one state for each internal leg.

The observation that integrating over the common  $\eta$  variables yields a sum over the 16 states in the  $N = 4$  multiplet will be important also in the following sections in evaluating similar sums (called "supersums") appearing in generalized unitarity cuts.

The simplest example illustrating the MHV (super)vertex rules is the construction of the MHV gluon amplitude; its split helicity configuration is simply:

$$\begin{aligned} A_5^{(0)}(1^-, 2^-, 3^-, 4^+, 5^+) = & \quad (3.5) \\ & \frac{\langle 23 \rangle^4}{\langle 23 \rangle \langle 34 \rangle \langle 4P_1 \rangle \langle P_1 2 \rangle} \frac{1}{P_1^2} \frac{\langle 1P_1 \rangle^4}{\langle 51 \rangle \langle 1P_1 \rangle \langle P_1 5 \rangle} + \frac{\langle 3P_2 \rangle^4}{\langle P_2 3 \rangle \langle 34 \rangle \langle 4P_2 \rangle} \frac{1}{P_2^2} \frac{\langle 12 \rangle^4}{\langle 2P_2 \rangle \langle P_2 5 \rangle \langle 51 \rangle \langle 12 \rangle} \\ & + \frac{\langle 3P_3 \rangle^4}{\langle 34 \rangle \langle 45 \rangle \langle 5P_3 \rangle \langle P_3 3 \rangle} \frac{1}{P_3^2} \frac{\langle 12 \rangle^4}{\langle P_3 1 \rangle \langle 12 \rangle \langle 2P_3 \rangle} + \frac{\langle 23 \rangle^4}{\langle 23 \rangle \langle 3P_4 \rangle \langle P_4 2 \rangle} \frac{1}{P_4^2} \frac{\langle 1P_4 \rangle^4}{\langle 1P_4 \rangle \langle P_4 4 \rangle \langle 45 \rangle \langle 51 \rangle} \end{aligned}$$

<sup>5</sup>For the superfields (2.8) this factor is just  $\int d^4\eta' \delta^{(4)}(\eta - \eta')$ .

The momenta  $P_i$  follow from momentum conservation at each MHV vertex; their null components assumed above are obtained as in (3.3).

While much more efficient than Feynman diagrams, the MHV supervertex expansion is not recursive and the number of contributing graphs grows quite fast with the number of external legs; it also exhibits an artificial lack of covariance at intermediate stages due to the presence of the fixed spinors  $\zeta$ . The BCFW recursion relation [35] reconstruct covariantly tree-level amplitudes from this pole structure and their multi-particle factorization properties.

Their direct derivation [35] uses only complex analysis. One singles out two momenta  $p_i$  and  $p_j$  (the choice of momenta is, to a large extent, arbitrary; we will discuss shortly the origin of constraints on the choice of  $i$  and  $j$ ) and shifts them as

$$p_i \rightarrow \hat{p}_i = p_i + z\zeta_{ij} \quad p_j \rightarrow \hat{p}_j = p_j - z\zeta_{ij} \quad (\zeta_{ij})_{\alpha\dot{\alpha}} = \lambda_{i\alpha}\tilde{\lambda}_{j\dot{\alpha}} \quad (3.6)$$

where the vector  $(\zeta_{ij})$  is chosen such that the shifted momenta are still null. More elaborate shifts have also been discussed. By tuning the parameter  $z$  it is possible to expose one by one all poles of the amplitude. As the relevant values of  $z$  are complex, equation (3.6) is interpreted as an analytic continuation to complex momenta.

The fact that the only poles of the shifted amplitude arise from the  $z$  dependence of propagators implies that none of them is at  $z = 0$ .<sup>6</sup> The original (unshifted) amplitude may then be recovered by integrating the shifted amplitude on a small contour  $C_0$  around  $z = 0$ . Reinterpreting it as a contour around  $z = \infty$  implies that the amplitude may be rewritten in terms of the residues of the shifted amplitude. Since the corresponding poles are in one to one correspondence with multi-particle factorization limits of the shifted amplitude, it follows from eq. (2.7) that their residues are themselves products of amplitudes. We are finally led to [35]

$$\begin{aligned} A_{(1\dots n)} &= \frac{1}{2\pi i} \oint_{C_0} \frac{dz}{z} A_{(\hat{1}, 2\dots \hat{n}; z)} = -\frac{1}{2\pi i} \oint_{C_\infty} \frac{dz}{z} A_{(\hat{1}, 2\dots \hat{n}; z)} \\ &= \sum_{l, h} A_L(\hat{1}, 2\dots l, \hat{q}^h; z_{0l}) \frac{1}{P_{1, \dots, l}^2} A_R(-\hat{q}^{-h}, (l+1), \dots, \hat{n}; z_{0l}) + \mathcal{C}_\infty \quad , \end{aligned} \quad (3.7)$$

where  $h$  denotes the helicity of the intermediate leg. For definiteness and ease of notation we chose to shift the external momenta  $p_1$  and  $p_n$ ; the momentum  $\hat{q}$  of the internal line is determined by momentum conservation and depends on  $z$ . The value of  $z_{0l}$  is determined from the on-shell condition for the intermediate line:

$$z_{0l} = \frac{P_{1, \dots, l}^2}{2 \zeta_{1n} \cdot P_{1, \dots, l}} \quad . \quad (3.8)$$

The term denoted by  $\mathcal{C}_\infty$  represents the contribution of the pole at  $z = \infty$ . It is possible to argue [35] using either Feynman diagrammatics or the MHV vertex rules that this contribution is absent for the shift (3.6) for all choices of helicity for the legs  $(i, j)$  except  $(h_i, h_j) = (+, -)$ .

---

<sup>6</sup>Poles on the  $z$ -plane may drift close to the origin only in multi-particle factorization limits of the *unshifted* amplitude.

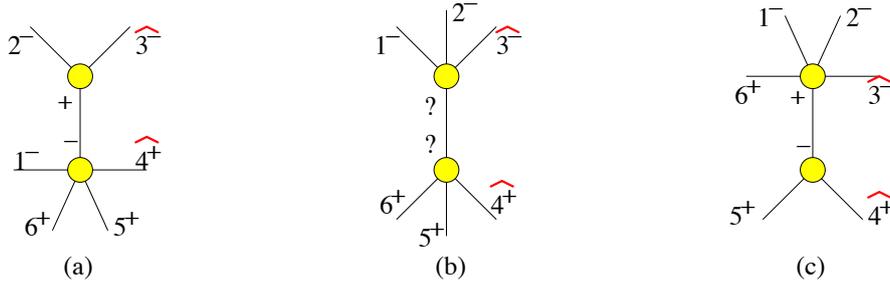

**Figure 1:** The diagrammatic presentation of the terms in equation (3.7) for  $A_{(1^-2^-3^-4^+5^+6^+)}$ .

Some of the terms in the sum in equation (3.7) contain three-particle amplitudes. The analytic continuation to complex momenta (*i.e.*  $\lambda \neq (\tilde{\lambda})^*$ ) makes these terms nonvanishing.<sup>7</sup>

The six-point amplitude in split helicity configuration  $A_{(1^-2^-3^-4^+5^+6^+)}$  provides a simple illustration of the BCFW recursion relations. Choosing to shift the momenta  $p_3$  and  $p_4$ , the diagrams representing the terms in equation (3.7) are shown in figure 1. Diagram (b) vanishes identically; the other two contribute as follows:

$$\begin{aligned}
 T_a &= \frac{\langle 2\hat{3} \rangle^3}{\langle \hat{3}p_{23} \rangle \langle p_{23}2 \rangle} \frac{1}{p_{23}^2} \frac{\langle 1p_{23} \rangle^3}{\langle p_{23}4 \rangle \langle \hat{4}5 \rangle \langle 56 \rangle \langle 61 \rangle} & z_{01} &= \frac{p_{23}^2}{\langle 4|P_{23}|3 \rangle} \\
 T_c &= \frac{[p_{45}6]^3}{[\hat{p}_{23}6][61][12][2\hat{3}][\hat{3}p_{23}]} \frac{1}{p_{45}^2} \frac{[\hat{4}5]^3}{[5p_{45}][\hat{p}_{45}4]} & z_{03} &= \frac{p_{45}^2}{\langle 4|p_{45}|3 \rangle} \quad (3.9)
 \end{aligned}$$

Combining them and making use of the corresponding shifts leads to

$$A_{(1^-2^-3^-4^+5^+6^+)} = \frac{1}{\langle 5|p_{34}|2 \rangle} \left[ \frac{\langle 1|p_{23}|4 \rangle^3}{[23][34]\langle 56 \rangle \langle 61 \rangle p_{234}^2} + \frac{\langle 3|p_{45}|6 \rangle^3}{[61][12]\langle 34 \rangle \langle 45 \rangle p_{345}^2} \right]. \quad (3.10)$$

This is indeed the correct answer for the six-point split-helicity tree-level gluon amplitude, as may be verified by direct comparison with the classic results of [9].

BCFW recursion relations have been generalized [36, 37, 18] to chiral on-shell superspace. By solving them explicit expressions for all tree-level amplitudes of  $\mathcal{N} = 4$  sYM have been obtained in [38].

## 4 Generalized unitarity and loop amplitudes

As explained in the previous section, the MHV vertex rules and the on-shell recursion relations may be understood as procedures for reconstructing a function of many variables from its singularities and behavior at infinity.

Historically, through the optical theorem, such a strategy was first used to construct loop amplitudes. Unitarity of the scattering matrix implies that its interaction part

<sup>7</sup> Either the MHV or the  $\overline{\text{MHV}}$  three-particle amplitude may be chosen nonvanishing, but not both.

$S = \mathbf{1} + iT$  obeys the equation:

$$i(T^\dagger - T) = T^\dagger T \quad . \quad (4.1)$$

Expanding both sides in the coupling constant implies that, at loop order  $L$ , the discontinuity<sup>8</sup> – or cut – of  $T$  in some multi-particle invariant is given by the product of lower order terms in the perturbative expansion of the  $T$  matrix, i.e. lower order on-shell amplitudes.

For bookkeeping purposes it is useful to separate cuts in two classes: singlet and non-singlet. In the former only one type of field crosses the cut. In the latter several types of particles – complete multiplets in a supersymmetric theory – cross the cut. The summation over all such states can be tedious; at low orders it may be explicitly carried out using the component version of the supersymmetric Ward identities. General procedures, based on chiral superspace, for effortlessly carrying out such sums – called supersums – have been described in detail in [18, 16].

Reconstructing an amplitude from its unitarity cuts is not completely straightforward. One of the main difficulties is that the emerging integrals – dispersion integrals – are *not* of the type usually found in Feynman diagram calculations. A reinterpretation of the equation (4.1) bypasses this issue, expresses the result in terms of Feynman integrals and allows use of the recent sophisticated techniques for their evaluation: integral identities, modern reduction techniques, differential equations, reduction to master integrals, etc.

To reinterpret the  $L$ -loop component of eq. (4.1) we notice that, due to the Feynman diagrammatics underlying the amplitude calculation, it is possible to identify on the left-hand side of this equation all the terms with a prescribed set of cut propagators. Equation (4.1) expresses the sum of these terms as a product of lower-loop amplitudes. Thus, at the level of the amplitudes' integrand, a unitarity cut may be interpreted as isolating the terms containing a prescribed set of (cut) propagators.

These observations, originally due to Bern, Dixon, Dunbar and Kosower [10] and improved at one-loop level by Britto, Cachazo and Feng [39], allow “cutting” more than  $(L + 1)$  propagators for an  $L$ -loop amplitude, generalizing the unitarity relation (4.1). These generalized cuts<sup>9</sup> do not have the interpretation of the imaginary part of some higher-loop amplitude. Rather, they should be interpreted as isolating the terms that contain a prescribed set of propagators. The Feynman rules underlying the calculation guarantee that the totality of generalized cuts contains the complete information necessary to reconstruct the amplitude to any order in perturbation theory. Indeed, each term in the integrand of the amplitude contains (perhaps after integral reduction) some subset of the propagators required by Feynman rules and each such term is captured by at least one generalized cut.

These arguments assume that the generalized cuts are constructed in the regularized theory. In the following dimensional regularization with  $d = 4 - 2\epsilon$  is assumed.<sup>10</sup> In practice it is convenient to start by analyzing four-dimensional cuts, as one can saturate

<sup>8</sup>This interpretation is a consequence of the  $i\epsilon$  prescription:  $\frac{1}{l^2+i\epsilon} - \frac{1}{l^2-i\epsilon} = -2\pi i\theta(l^0)\delta(l^2)$ .

<sup>9</sup>Similarly to regular cuts, generalized cuts can be either of singlet and non-singlet types.

<sup>10</sup>In planar  $\mathcal{N} = 4$  sYM specific patterns of breaking of gauge symmetry also provide successful IR regularization [40]. We will comment on their features in the concluding section.

them with four-dimensional helicity states and also make use of the supersymmetric Ward identities. The terms arising from the  $(-2\epsilon)$ -dimensional components of the momenta in momentum-dependent vertices that are potentially missed by four-dimensional cuts are separately found either by a comparison with  $d$ -dimensional cuts or by other means. In supersymmetric theories it can be argued [41] based on the improved power-counting of the theory that, through  $\mathcal{O}(\epsilon^0)$ , one-loop amplitudes follow from four-dimensional cuts.

In [42] a generalized unitarity approach was proposed for theories that may be continued to six dimensions. This construction, which is based on a six-dimensional version of spinor helicity [43], provides a natural context for the  $\mathcal{O}(\epsilon)$  components of momenta and allows a Coulomb-branch regularization of IR divergences.

An  $L$ -loop  $n$ -point amplitude has (very) many generalized cuts; it is important to evaluate them such that the maximum number of terms is determined with the least amount of effort. A strategy initially advocated in [44] and extensively used in [45, 46] is to begin with the generalized cuts imposing  $4L$  cut conditions (maximal cuts) and then proceed by releasing the on-shell condition for one propagator at a time (near-maximal cuts). This is known as "the method of maximal cuts".

## 5 One loop amplitudes

Quite generally in four dimensions, such one-loop scattering amplitudes in a massless supersymmetric theory may be shown to be a linear combination of scalar box, triangle and bubble integrals (see Figure 2) with coefficients depending on the external momenta.

<sup>11</sup> In  $\mathcal{N} = 4$  sYM it is possible to argue [10] that amplitudes with external states belong to the same  $\mathcal{N} = 1$  vector multiplet may be written as a sum of box integrals:<sup>12</sup>

$$A_n^{(1)} = \sum_{ijk} c_{ijkl} I_{ijkl} \quad . \quad (5.1)$$

Experience shows that the same holds for other external states as well. In eq. (5.1)  $(i, j, k, l)$  are cyclic labels of the first external leg at each corner of the box (counting clockwise),  $I_{ijkl}$  is the corresponding integral and the sum runs over all ways of choosing the labels  $(i, j, k, l)$ . These integrals are linearly independent (over rational, momentum dependent coefficients) so this decomposition is unique.

Since each box integral has an unique set of four propagators, a quadruple cut (i.e. the result of eliminating four propagators and using the on-shell condition for their momenta) isolates an unique box integral and its coefficient [39]. Following the previous discussion, the quadruple cut of the amplitude is simply given by the product of four tree amplitudes evaluated on the solution of the on-shell conditions for the four propagators:

$$c_{ijkl} = \frac{1}{2} \sum_{h_{q_i}} A(q_1, i \dots j-1, -q_2) A(q_2, j \dots k-1, -q_3) A(q_3, k \dots l-1, -q_4) A(q_4, l \dots i-1, -q_1) \Big|_{q_i^2=0} \quad (5.2)$$

<sup>11</sup>Non-supersymmetric theories contain additional rational terms. Their determination is beyond the scope of this review. See however [47] and references therein.

<sup>12</sup> The box integrals, represented graphically in Figure 2(a), are defined and given in reference [48] (with the four-mass boxes from ref. [49]).

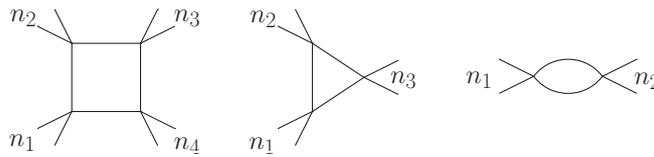

**Figure 2:** Box, triangle and bubble integrals with arbitrary numbers of external legs  $n_{1,2,3,4}$  at each vertex.

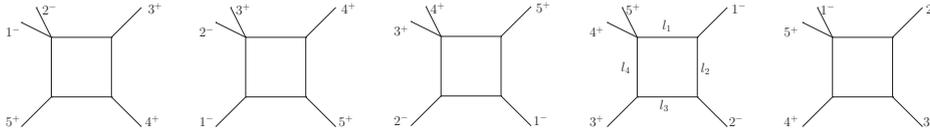

**Figure 3:** Contributions to the one-loop five-point MHV amplitude.

The sum runs over all possible helicity assignments on the internal lines. The factor of  $1/2$  above is due to the four on-shell conditions having two solutions with equal values of the quadruple-cut box integrals. The sum over these solutions is implicit in the sum in equation (5.2). It is important to realize that any amplitude contains at least one box integral with one three-point corner. To construct its coefficient through this method it is necessary to analytically continue momenta to complex values.

The calculation of the five-point amplitude, initially computed by other means [50] in both in  $\mathcal{N} = 4$  sYM and QCD, is a simple illustration of the quadruple cut approach. The five possible integral contributions are shown in Figure 3. Let us comment on the fourth one. Of the two possible helicity assignments to the cut propagators, one does not have solutions for the on shell conditions. The other yields the coefficient of the fourth box integral in Figure 3:

$$\frac{[l_2 l_1]^3}{[1l_2][l_1 1]} \times \frac{\langle 2l_2 \rangle^3}{\langle 2l_3 \rangle \langle l_3 l_2 \rangle} \times \frac{[3l_4]^3}{[l_4 l_3][l_3 3]} \times \frac{\langle l_1 l_4 \rangle^3}{\langle l_4 4 \rangle \langle 4 5 \rangle \langle 5 l_1 \rangle} = -\frac{s_{12} s_{23} \langle 12 \rangle^3}{\langle 23 \rangle \langle 34 \rangle \langle 45 \rangle \langle 51 \rangle} \quad (5.3)$$

The coefficients of the other integrals may be computed in a similar fashion. They are related to the coefficient evaluated here by the obvious relabeling the factor  $s_{12} s_{23}$ .

The quadruple cut technique described and illustrated above may equally well be used to construct non-planar one-loop amplitudes. Alternatively and perhaps less calculationally intensive, in theories with only adjoint fields and only antisymmetric structure constant couplings one-loop leading and subleading color contributions are algebraically related [6] by  $U(1)$  decoupling identities.

## 6 Higher loops

Higher loop calculations in  $\mathcal{N} = 4$  sYM enjoy similar simplifications, though to a lesser extent. An important difference from one-loop calculations within the generalized unitarity method is that the natural integrals form only an over-complete basis. Complete bases may be identified on a case by case basis<sup>13</sup>. Since, in general, not all higher loop in-

<sup>13</sup>See the two-loop examples [51] and [52] and the general strategy [53].

tegrals can be frozen by cutting all their propagators, a naive higher-loop generalization of the quadruple cuts is problematic. The leading singularity method [54] bypasses the latter difficulty by making use of additional propagator-like singularities in the remaining variables, which are specific to four dimensions.

Generalized cuts can nevertheless be used to great effect to isolate parts of the full amplitude containing some prescribed set of propagators. The previous arguments continue to hold and imply that the complete amplitude can be reconstructed from its  $d$ -dimensional generalized cuts. A detailed, general algorithm for assembling the amplitude was described in [55]. In a nutshell, starting from one (generalized) cut, one corrects it iteratively such that all the other cuts are correctly reproduced.

While fundamentally all cuts are equally important, some of them exhibit more structure than other, which makes them useful starting points for the reconstruction of the amplitude. In some cases they also have a simple iterative structure and thus lead to effective rules for determining their contribution to the full amplitude.

## 6.1 Effective rules

Two-particle cuts are the simplest to analyze as they involve cutting the smallest number of propagators. For MHV amplitudes they exhibit special properties. As mentioned in section 2.2, to all loop orders MHV amplitudes are proportional in a natural way to the tree-level amplitude. At the level of generalized cuts this translates into the observation [56, 57] that sewing two tree-level MHV amplitudes leads in a natural way to another tree-level MHV amplitude factor:

$$A_{n_1}^{(0),\text{MHV}} \times A_{n_2}^{(0),\text{MHV}} \propto A_{n_1+n_2-4}^{(0),\text{MHV}} \quad . \quad (6.1)$$

The operation may be repeated, leading to what is known as "iterated two-particle cuts". For four-particle amplitudes, the higher-loop terms detected by iterated two-particle cuts are effectively given by the rung-rule [56]. It states that the  $L$ -loop integrals which follow from iterated two-particle cuts can be obtained from the  $(L-1)$ -loop amplitudes by adding a rung in all possible (planar) ways while in each instance also inserting the numerator factor

$$i(l_1 + l_2)^2 \quad (6.2)$$

where  $l_1$  and  $l_2$  are the momenta of the lines connected by the rung.<sup>14</sup> For higher-point amplitudes the rung rule is less effective and a direct evaluation of generalized cuts is typically necessary.

The box substitution identity [44] and its generalizations [46] relate further terms in higher-loop amplitudes to terms in lower loop amplitudes. The idea is to organize terms in an  $L$ -loop amplitude to expose an  $L'$ -loop four-point sub-amplitude. A contribution to the  $(L+\ell)$ -loop amplitude is then obtained by literally replacing this  $L'$ -loop four-point sub-amplitude with its  $(L'+\ell)$ -loop counterpart.

---

<sup>14</sup> The rung rule can generate integrals which do not exhibit any two-particle cuts. Such contributions must be checked by a direct evaluation of other cuts. Examples in this direction first appear in the planar four-loop four-gluon amplitude [28].

Certain non-planar contributions to scattering amplitudes turn out to be related to planar ones at the same loop order by a Jacobi-like identities [46,58]. Such manipulations can be carried out pictorially. We will not describe them in detail here, but refer the reader to the original literature for a detailed discussion (see also [59] for a string theory based argument for these relations).

Quite generally, effective rules do not yield all contributions to amplitudes. Their usefulness should not, however, be underestimated: it is easier to correct an existing ansatz rather than construct it from scratch starting from generalized cuts. To determine the missing terms and confirm the ones obtained through effective rules it is necessary to directly evaluate certain judiciously chosen set of the generalized cuts.

## 6.2 An example: two-loop four-point amplitude in $\mathcal{N} = 4$ sYM theory

Perhaps the simplest example that illustrates the higher-loop discussion in the previous subsections is the calculation [56] of the two-loop four-point amplitude. Direct evaluation of the  $s$ -channel iterated 2-particle cut (the  $t$ -channel cut may be obtained by simple relabeling) leads to:

$$\begin{aligned}
 & A_4^{(0)}(l_2, k_1^-, k_2^-, l_1) A_4^{(0)}(-l_1, -l_4, -l_3, -l_2) A_4^{(0)}(l_4, k_3^+, k_4^+, l_3) \\
 &= i s_{12} (k_2 - l_4)^2 \frac{1}{(l_2 - k_1)^2 (l_2 + l_3)^2} A_4^{(0)}(-l_3, 1^-, 2^-, -l_4) A_4^{(0)}(l_4, k_3^+, k_4^+, l_3) \\
 &= A_4^{(0)}(k_1^-, k_2^-, k_3^+, k_4^+) \left[ i s_{12} (k_2 - l_4)^2 \frac{1}{(l_2 - k_1)^2 (l_2 + l_3)^2} \right] \left[ i s_{12} s_{23} \frac{1}{(l_3 - k_1)^2 (l_3 + k_4)^2} \right] \\
 &= -s_{12}^2 s_{23} A_4^{(0)}(k_1^-, k_2^-, k_3^+, k_4^+) \cdot \text{Diagram} \quad (6.3)
 \end{aligned}$$
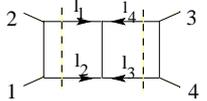

Together with the loop expansion parameter (2.5), this leads to the following ansatz:

$$\frac{A_4^{(2)}(k_1, k_2, k_3, k_4)}{A_4^{(0)}(k_1, k_2, k_3, k_4)} = -\frac{1}{4} s_{12} s_{23} \left\{ s_{12} \text{Diagram}_1 + s_{23} \text{Diagram}_2 \right\} \quad (6.4)$$
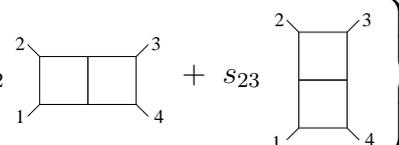

This ansatz turns out to be complete, as can be verified by evaluating the three-particle cut [56]. In less supersymmetric theories additional contributions are necessary.

The same ansatz (6.4), to be checked through a three-particle cut calculation, may be obtained either through the rung rule (by inserting a rung in the  $s$ - and the  $t$ -channel in a one-loop box integral) and the box insertion identity.

In general, the evaluation of a complete (spanning) set of cuts is always necessary. The power of effective rules lies in that they provide a fast and rather effortless way of obtaining a large number of terms (and sometimes all terms) in the amplitude. It is technically much more convenient to test and complete an existing ansatz than to construct it starting from the expressions of generalized unitarity cuts.

### 6.3 An interesting integral basis; dual conformal invariance

An interesting over-complete basis (at least for MHV amplitudes) may be conjectured based on the observation [3] that the integrals appearing in the two- and three-loop four-gluon planar amplitudes exhibit a momentum space conformal symmetry known as dual conformal symmetry.<sup>15</sup> Curiously, this symmetry is exhibited separately by each integral appearing in the amplitude, when regularized in a specific way. In dimensional regularization they are known as pseudo-conformal integrals. Dual conformal symmetry was shown to also be present in certain higher-loops and for higher-point amplitudes; it has been conjectured [28, 3] that, to all orders in perturbation theory, planar scattering amplitudes exhibit this symmetry and that each integral in their expressions is pseudo-conformal. Since only the infrared regulator breaks dual conformal invariance, extraction of the known infrared divergences (2.14) should lead yield a dual conformally invariant quantity. For MHV amplitudes this conjecture applies to the parity-even part of the scalar factor. For non-MHV amplitude it has been proposed [17] that the ratio between the resummed amplitude and the MHV amplitude with the same number of external legs is invariant under dual conformal transformations. This conjecture was successfully tested for the (appropriately defined) even part of the six-point NMHV amplitude at two loops [60].

The even part of planar MHV amplitudes is expected to be a sum of pseudo-conformal integrals with constant coefficients:

$$\mathcal{M}_n^{(L)} = \sum_i c_i I_i \quad ; \quad (6.5)$$

the coefficients  $c_i$  may be determined by comparing cuts of this ansatz to direct evaluation of generalized cuts of the amplitude. In certain cases maximal cuts are sufficient. This strategy was used to determine the five-loop four-point amplitude [44] as well as the two-loop MHV amplitudes with any number of external legs [61].

## 7 Comments on other methods and outlook

Other methods have been put forward for the construction of scattering amplitudes in  $\mathcal{N} = 4$  sYM theory and, more generally, in maximally-supersymmetric theories. A notable one, which captures the spirit of the complete localization of one-loop integrals under quadruple cuts, is the so-called leading singularity conjecture [37]. As previously discussed, evaluating the maximal cuts of an amplitude does not lead to a complete localization of integrals. In certain cases the result however exhibits further propagator-like singularities which may also be cut. The result is known as the "leading singularity". The conjecture states that scattering amplitudes in maximally supersymmetric theories are completely determined by their leading singularities. Two-loop results based on this conjecture agree with the results of the unitarity method calculation. It was also used to construct [62] the odd part of the six-point MHV amplitude at two-loops as well as [63]

---

<sup>15</sup>This symmetry, which appears to be related to the higher nonlocal symmetries of the dilatation operator of  $\mathcal{N} = 4$  sYM is reviewed in detail in [1].

the three-loop five-gluon amplitude. Together with the assumption that the superconformal and dual superconformal symmetries are realized to all orders in perturbation theory, it led to a proposal [64] for the all-loop all-point planar scattering amplitudes of the  $\mathcal{N} = 4$  sYM theory; a specific regularization prescription is required. The six-point MHV amplitude is correctly reproduced by this proposal [65]; this calculation also emphasizes that, in this proposal, the natural integrals are technically simpler than standard Feynman integrals. It has been suggested that this is related to them having *only* unit leading singularities.

All-order expressions of scattering amplitudes are in general hard to construct. Based on explicit two-loop [66] and three-loop calculations [27] as well as on the collinear properties of amplitudes it was conjectured that the scalar factor of  $n$ -point MHV amplitudes has, to all loop orders, a simple iterative structure in terms of the corresponding one-loop amplitude [27] to all orders in  $d = 4 - 2\epsilon$  dimensions:

$$\mathcal{M}_n = \exp \left[ \sum_{l=1}^{\infty} a^l f^{(l)}(\epsilon) \mathcal{M}_n^{(1)}(l\epsilon) + C^{(l)} + \mathcal{O}(\epsilon) \right] \quad (7.1)$$

where  $f^{(l)}(\epsilon) = f_0^{(l)} + \epsilon f_1^{(l)} + \epsilon^2 f_2^{(l)}$  with  $f_0^{(l)}$  and  $f_1^{(l)}$  determined in terms of the similar coefficients appearing in the Sudakov form factor (2.14), (2.15).

For  $n = 4, 5$  this expression appears to hold [67] if dual conformal invariance is present to all orders in perturbation theory. At higher-points dual conformal invariance is no longer sufficient to fix the expression of the amplitude. Direct calculations [68] of the six-point amplitudes show a departure from this expression, initially anticipated from a strong coupling analysis [69] based on the proposed relation between planar MHV scattering amplitudes and certain null polygonal Wilson loops [70] in this regime (see also [71]). The so-called “remainder function” quantifies this difference; its analytic form was found in [72] and simplified in [73].

The proposed relation between planar MHV scattering amplitudes and Wilson loops [70] led to the conjecture [67, 74] that a similar relation may hold order by order in weak coupling perturbation theory. This topic is reviewed in detail in [1]. The comparison of the six-point MHV amplitude at two loops with the relevant Wilson loop was discussed in [68, 75]. Expectation values of Wilson loops relevant for higher-point amplitudes have been computed in [76]; comparison with the corresponding scattering amplitude calculations [61, 77] awaits further developments in the calculation of higher-loop higher-point Feynman integrals.

Throughout our discussion we assumed that IR divergences are regularized in dimensional regularization. Ultraviolet divergences not being an issue in  $\mathcal{N} = 4$  sYM, infrared divergences may also be regularized by letting fields acquire masses through spontaneous breaking of the gauge symmetry [40] (Higgs regularization). Much like the original (all-massive) regularization of [3], this regularization has the advantage of preserving dual conformal invariance up to transformation of the mass parameter(s). This regularization was used to great effect to test the exponentiation (7.1) of the four-point amplitude at two- and three-loops [40, 78]. Diagrammatic rules, based on the color flow, may be devised to avoid repeating the unitarity-based construction in the presence of mass parameters.

The Higgs-regularized amplitude may also be obtained from the dimensionally regularized one by simply treating as mass parameters the  $(-2\epsilon)$ -dimensional components of loop momenta. A calculation is necessary to ascertain whether the Higgs-regularized amplitude contains terms proportional to the regulator which yield non-vanishing contributions upon integration.

Being somewhat outside the main theme of the collection, we glossed over the very important techniques developed specifically for the calculation of nonplanar scattering amplitudes, in particular the Bern-Carrasco-Johansson relations [58] and the connection between  $\mathcal{N} = 4$  sYM theory and  $\mathcal{N} = 8$  supergravity.

The full consequences and implications of the developments outlined in this review (as well as of those that were not) are yet to emerge and many questions, which will undoubtedly contribute in this direction, remain to be addressed. Despite substantial progress in the calculation of multi-loop and multi-leg amplitudes there is room for improvement. It is clear that further structure is present in  $\mathcal{N} = 4$  sYM theory and that it may be sufficiently powerful to completely determine, at least in some sectors, the kinematic dependence of the scattering matrix of the theory.

## Acknowledgements

I would like to thank Z. Bern, J.J.M. Carrasco, L. Dixon, H. Johansson, D. Kosower, M. Spradlin, A. Tseytlin, C. Vergu and A. Volovich for many useful discussions and collaboration on the topics reviewed here. This work was supported by the US DoE under contract DE-FG02-201390ER40577 (OJI), the US NSF under grants PHY-0608114 and PHY-0855356 and the A. P. Sloan Foundation.

## References

- [1] J. M. Drummond, “*Review of AdS/CFT Integrability, Chapter V.2: Dual Superconformal Symmetry*”, [arxiv:1012.4002](#).
- [2] J. M. Drummond, J. M. Henn and J. Plefka, “*Yangian symmetry of scattering amplitudes in  $\mathcal{N} = 4$  super Yang-Mills theory*”, JHEP 0905, 046 (2009), [arxiv:0902.2987](#).
- [3] J. M. Drummond, J. Henn, V. A. Smirnov and E. Sokatchev, “*Magic identities for conformal four-point integrals*”, JHEP 0701, 064 (2007), [hep-th/0607160](#).
- [4] L. J. Dixon, “*Calculating scattering amplitudes efficiently*”, [hep-ph/9601359](#).
- [5] F. A. Berends, R. Kleiss, P. De Causmaecker, R. Gastmans and T. T. Wu, “*Single Bremsstrahlung Processes in Gauge Theories*”, Phys. Lett. B103, 124 (1981). • P. De Causmaecker, R. Gastmans, W. Troost and T. T. Wu, “*Multiple Bremsstrahlung in Gauge Theories at High-Energies. 1. General Formalism for Quantum Electrodynamics*”, Nucl. Phys. B206, 53 (1982). • Z. Xu, D.-H. Zhang and L. Chang, “*Helicity Amplitudes for Multiple Bremsstrahlung in Massless Nonabelian Gauge Theories. 1. New Definition of Polarization Vector and Formulation of Amplitudes in Grassmann Algebra*”, TUTP-84/3-TSINGHUA. • R. Kleiss and W. J. Stirling, “*Spinor*”

- Techniques for Calculating  $p$  anti- $p \rightarrow W^{+-} / Z^0 + \text{Jets}$* , Nucl. Phys. B262, 235 (1985). • J. F. Gunion and Z. Kunszt, “*Improved Analytic Techniques for Tree Graph Calculations and the  $G g q$  anti- $q$  Lepton anti-Lepton Subprocess*”, Phys. Lett. B161, 333 (1985). • Z. Xu, D.-H. Zhang and L. Chang, “*Helicity Amplitudes for Multiple Bremsstrahlung in Massless Nonabelian Gauge Theories*”, Nucl. Phys. B291, 392 (1987).
- [6] Z. Bern and D. A. Kosower, “*Color decomposition of one loop amplitudes in gauge theories*”, Nucl. Phys. B362, 389 (1991).
- [7] V. Del Duca, L. J. Dixon and F. Maltoni, “*New color decompositions for gauge amplitudes at tree and loop level*”, Nucl. Phys. B571, 51 (2000), hep-ph/9910563.
- [8] N. E. J. Bjerrum-Bohr, P. H. Damgaard and P. Vanhove, “*Minimal Basis for Gauge Theory Amplitudes*”, Phys. Rev. Lett. 103, 161602 (2009), arxiv:0907.1425.
- [9] M. L. Mangano, S. J. Parke and Z. Xu, “*Duality and Multi - Gluon Scattering*”, Nucl. Phys. B298, 653 (1988).
- [10] Z. Bern, L. J. Dixon, D. C. Dunbar and D. A. Kosower, “*One-Loop  $n$ -Point Gauge Theory Amplitudes, Unitarity and Collinear Limits*”, Nucl. Phys. B425, 217 (1994), hep-ph/9403226.
- [11] D. A. Kosower, “*All-order collinear behavior in gauge theories*”, Nucl. Phys. B552, 319 (1999), hep-ph/9901201.
- [12] M. T. Grisaru and H. N. Pendleton, “*Some Properties of Scattering Amplitudes in Supersymmetric Theories*”, Nucl. Phys. B124, 81 (1977).
- [13] J. Broedel and L. J. Dixon, “ *$R^4$  counterterm and  $E7(\gamma)$  symmetry in maximal supergravity*”, arxiv:0911.5704.
- [14] H. Elvang, D. Z. Freedman and M. Kiermaier, “*Solution to the Ward Identities for Superamplitudes*”, arxiv:0911.3169.
- [15] J. M. Drummond, J. Henn, G. P. Korchemsky and E. Sokatchev, “*Generalized unitarity for  $\mathcal{N} = 4$  super-amplitudes*”, arxiv:0808.0491.
- [16] Z. Bern, J. J. M. Carrasco, H. Ita, H. Johansson and R. Roiban, “*On the Structure of Supersymmetric Sums in Multi-Loop Unitarity Cuts*”, arxiv:0903.5348.
- [17] J. M. Drummond, J. Henn, G. P. Korchemsky and E. Sokatchev, “*Dual superconformal symmetry of scattering amplitudes in  $\mathcal{N} = 4$  super-Yang-Mills theory*”, arxiv:0807.1095.
- [18] H. Elvang, D. Z. Freedman and M. Kiermaier, “*Recursion Relations, Generating Functions, and Unitarity Sums in  $N=4$  SYM Theory*”, JHEP 0904, 009 (2009), arxiv:0808.1720.
- [19] R. Akhoury, “*Mass Divergence of Wide Angle Scattering Amplitudes*”, Phys. Rev. D19, 1250 (1979).
- [20] A. H. Mueller, “*On the Asymptotic Behavior of the Sudakov Form-factor*”, Phys. Rev. D20, 2037 (1979). • J. C. Collins, “*Algorithm to Compute Corrections to the Sudakov Form-factor*”, Phys. Rev. D22, 1478 (1980). • A. Sen, “*Asymptotic Behavior of the Sudakov Form-Factor in QCD*”, Phys. Rev. D24, 3281 (1981).

- [21] G. Sterman, “*Summation of Large Corrections to Short Distance Hadronic Cross-Sections*”, Nucl. Phys. B281, 310 (1987). • J. Botts and G. Sterman, “*Sudakov Effects in Hadron Hadron Elastic Scattering*”, Phys. Lett. B224, 201 (1989). • S. Catani and L. Trentadue, “*Resummation of the QCD Perturbative Series for Hard Processes*”, Nucl. Phys. B327, 323 (1989). • G. P. Korchemsky, “*Sudakov Form-factor in QCD*”, Phys. Lett. B220, 629 (1989). • L. Magnea and G. Sterman, “*Analytic continuation of the Sudakov form-factor in QCD*”, Phys. Rev. D42, 4222 (1990). • G. P. Korchemsky and G. Marchesini, “*Resummation of large infrared corrections using Wilson loops*”, Phys. Lett. B313, 433 (1993). • S. Catani, “*The singular behaviour of QCD amplitudes at two-loop order*”, Phys. Lett. B427, 161 (1998), hep-ph/9802439.
- [22] G. Sterman and M. E. Tejeda-Yeomans, “*Multi-loop amplitudes and resummation*”, Phys. Lett. B552, 48 (2003), hep-ph/0210130.
- [23] J. C. Collins, D. E. Soper and G. Sterman, “*Factorization of Hard Processes in QCD*”, Adv. Ser. Direct. High Energy Phys. 5, 1 (1988), hep-ph/0409313.
- [24] A. Sen, “*Asymptotic Behavior of the Wide Angle On-Shell Quark Scattering Amplitudes in Nonabelian Gauge Theories*”, Phys. Rev. D28, 860 (1983). • S. M. Aybat, L. J. Dixon and G. Sterman, “*The two-loop soft anomalous dimension matrix and resummation at next-to-next-to leading pole*”, Phys. Rev. D74, 074004 (2006), hep-ph/0607309.
- [25] L. J. Dixon, L. Magnea and G. Sterman, “*Universal structure of subleading infrared poles in gauge theory amplitudes*”, JHEP 0808, 022 (2008), arxiv:0805.3515.
- [26] S. V. Ivanov, G. P. Korchemsky and A. V. Radyushkin, “*Infrared Asymptotics of Perturbative QCD: Contour Gauges*”, Yad. Fiz. 44, 230 (1986). • G. P. Korchemsky and A. V. Radyushkin, “*Loop Space Formalism and Renormalization Group for the Infrared Asymptotics of QCD*”, Phys. Lett. B171, 459 (1986).
- [27] Z. Bern, L. J. Dixon and V. A. Smirnov, “*Iteration of planar amplitudes in maximally supersymmetric Yang-Mills theory at three loops and beyond*”, Phys. Rev. D72, 085001 (2005), hep-th/0505205.
- [28] Z. Bern, M. Czakon, L. J. Dixon, D. A. Kosower and V. A. Smirnov, “*The Four-Loop Planar Amplitude and Cusp Anomalous Dimension in Maximally Supersymmetric Yang-Mills Theory*”, Phys. Rev. D75, 085010 (2007), hep-th/0610248.
- [29] N. Beisert, B. Eden and M. Staudacher, “*Transcendentality and crossing*”, J. Stat. Mech. 0701, P021 (2007), hep-th/0610251.
- [30] R. Roiban, M. Spradlin and A. Volovich, “*On the tree-level S-matrix of Yang-Mills theory*”, Phys. Rev. D70, 026009 (2004), hep-th/0403190.
- [31] N. Arkani-Hamed, F. Cachazo, C. Cheung and J. Kaplan, “*A Duality For The S Matrix*”, arxiv:0907.5418. • N. Arkani-Hamed, F. Cachazo and C. Cheung, “*The Grassmannian Origin Of Dual Superconformal Invariance*”, arxiv:0909.0483. • L. Mason and D. Skinner, “*Dual Superconformal Invariance, Momentum Twistors and Grassmannians*”, arxiv:0909.0250. • M. Spradlin and A. Volovich, “*From Twistor String Theory To Recursion Relations*”, arxiv:0909.0229. • D. Nandan, A. Volovich and C. Wen, “*A Grassmannian Etude in NMHV Minors*”, arxiv:0912.3705.
- [32] F. Cachazo, P. Svrcek and E. Witten, “*MHV vertices and tree amplitudes in gauge theory*”, JHEP 0409, 006 (2004), hep-th/0403047.

- [33] A. Gorsky and A. Rosly, “*From Yang-Mills Lagrangian to MHV diagrams*”, JHEP 0601, 101 (2006), [hep-th/0510111](#). • P. Mansfield, “*The Lagrangian origin of MHV rules*”, JHEP 0603, 037 (2006), [hep-th/0511264](#). • J. H. Eittle, T. R. Morris and Z. Xiao, “*The MHV QCD Lagrangian*”, JHEP 0808, 103 (2008), [arxiv:0805.0239](#). • H. Elvang, D. Z. Freedman and M. Kiermaier, “*Proof of the MHV vertex expansion for all tree amplitudes in  $\mathcal{N} = 4$  SYM theory*”, JHEP 0906, 068 (2009), [arxiv:0811.3624](#). • R. Boels, L. Mason and D. Skinner, “*Supersymmetric gauge theories in twistor space*”, JHEP 0702, 014 (2007), [hep-th/0604040](#). • H. Feng and Y.-t. Huang, “*MHV lagrangian for  $N = 4$  super Yang-Mills*”, JHEP 0904, 047 (2009), [hep-th/0611164](#).
- [34] D. A. Kosower, “*Next-to-maximal helicity violating amplitudes in gauge theory*”, Phys. Rev. D71, 045007 (2005), [hep-th/0406175](#). • I. Bena, Z. Bern and D. A. Kosower, “*Twistor-space recursive formulation of gauge theory amplitudes*”, Phys. Rev. D71, 045008 (2005), [hep-th/0406133](#).
- [35] R. Britto, F. Cachazo, B. Feng and E. Witten, “*Direct Proof Of Tree-Level Recursion Relation In Yang-Mills Theory*”, Phys. Rev. Lett. 94, 181602 (2005), [hep-th/0501052](#).
- [36] A. Brandhuber, P. Heslop and G. Travaglini, “*A note on dual superconformal symmetry of the  $\mathcal{N} = 4$  super Yang-Mills S-matrix*”, Phys. Rev. D78, 125005 (2008), [arxiv:0807.4097](#).
- [37] N. Arkani-Hamed, F. Cachazo and J. Kaplan, “*What is the Simplest Quantum Field Theory?*”, [arxiv:0808.1446](#).
- [38] J. M. Drummond and J. M. Henn, “*All tree-level amplitudes in  $\mathcal{N} = 4$  SYM*”, JHEP 0904, 018 (2009), [arxiv:0808.2475](#).
- [39] R. Britto, F. Cachazo and B. Feng, “*Generalized unitarity and one-loop amplitudes in  $\mathcal{N} = 4$  super-Yang-Mills*”, Nucl. Phys. B725, 275 (2005), [hep-th/0412103](#).
- [40] L. F. Alday, J. M. Henn, J. Plefka and T. Schuster, “*Scattering into the fifth dimension of  $\mathcal{N} = 4$  super Yang-Mills*”, [arxiv:0908.0684](#).
- [41] Z. Bern, L. J. Dixon, D. C. Dunbar and D. A. Kosower, “*Fusing gauge theory tree amplitudes into loop amplitudes*”, Nucl. Phys. B435, 59 (1995), [hep-ph/9409265](#).
- [42] Z. Bern, J. J. Carrasco, T. Dennen, Y.-t. Huang and H. Ita, “*Generalized Unitarity and Six-Dimensional Helicity*”, [arxiv:1010.0494](#).
- [43] C. Cheung and D. O’Connell, “*Amplitudes and Spinor-Helicity in Six Dimensions*”, JHEP 0907, 075 (2009), [arxiv:0902.0981](#). • T. Dennen, Y.-t. Huang and W. Siegel, “*Supertwistor space for 6D maximal super Yang-Mills*”, JHEP 1004, 127 (2010), [arxiv:0910.2688](#).
- [44] Z. Bern, J. J. M. Carrasco, H. Johansson and D. A. Kosower, “*Maximally supersymmetric planar Yang-Mills amplitudes at five loops*”, Phys. Rev. D76, 125020 (2007), [arxiv:0705.1864](#).
- [45] Z. Bern, J. J. M. Carrasco, L. J. Dixon, H. Johansson and R. Roiban, “*Manifest Ultraviolet Behavior for the Three-Loop Four-Point Amplitude of  $\mathcal{N} = 8$  Supergravity*”, Phys. Rev. D78, 105019 (2008), [arxiv:0808.4112](#).
- [46] Z. Bern, J. J. M. Carrasco, L. J. Dixon, H. Johansson and R. Roiban, “*The Complete Four-Loop Four-Point Amplitude in  $N=4$  Super-Yang-Mills Theory*”, [arxiv:1008.3327](#).

- [47] C. F. Berger and D. Forde, “*Multi-Parton Scattering Amplitudes via On-Shell Methods*”, *Ann. Rev. Nucl. Part. Sci.* 60, 181 (2010), [arxiv:0912.3534](#).
- [48] Z. Bern, L. J. Dixon and D. A. Kosower, “*Dimensionally Regulated One-Loop Integrals*”, *Phys. Lett.* B302, 299 (1993), [hep-ph/9212308](#). • Z. Bern, L. J. Dixon and D. A. Kosower, “*Dimensionally regulated pentagon integrals*”, *Nucl. Phys.* B412, 751 (1994), [hep-ph/9306240](#).
- [49] A. Denner, U. Nierste and R. Scharf, “*A Compact expression for the scalar one loop four point function*”, *Nucl. Phys.* B367, 637 (1991). • N. I. Usyukina and A. I. Davydychev, “*An Approach to the evaluation of three and four point ladder diagrams*”, *Phys. Lett.* B298, 363 (1993). • N. I. Usyukina and A. I. Davydychev, “*Exact results for three and four point ladder diagrams with an arbitrary number of rungs*”, *Phys. Lett.* B305, 136 (1993).
- [50] Z. Bern, L. J. Dixon and D. A. Kosower, “*One loop corrections to five gluon amplitudes*”, *Phys. Rev. Lett.* 70, 2677 (1993), [hep-ph/9302280](#).
- [51] V. A. Smirnov and O. L. Veretin, “*Analytical results for dimensionally regularized massless on-shell double boxes with arbitrary indices and numerators*”, *Nucl. Phys.* B566, 469 (2000), [hep-ph/9907385](#).
- [52] T. Gehrmann and E. Remiddi, “*Two-Loop Master Integrals for  $\gamma^* \rightarrow 3$  Jets: The planar topologies*”, *Nucl. Phys.* B601, 248 (2001), [hep-ph/0008287](#).
- [53] J. Gluza, K. Kajda and D. A. Kosower, “*Towards a Basis for Planar Two-Loop Integrals*”, [arxiv:1009.0472](#).
- [54] F. Cachazo, “*Sharpening The Leading Singularity*”, [arxiv:0803.1988](#).
- [55] Z. Bern, L. J. Dixon and D. A. Kosower, “*Two-Loop  $g - \bar{g}$   $gg$  Splitting Amplitudes in QCD*”, *JHEP* 0408, 012 (2004), [hep-ph/0404293](#).
- [56] Z. Bern, J. S. Rozowsky and B. Yan, “*Two-loop four-gluon amplitudes in  $N = 4$  super-Yang-Mills*”, *Phys. Lett.* B401, 273 (1997), [hep-ph/9702424](#).
- [57] Z. Bern, L. J. Dixon, D. C. Dunbar, M. Perelstein and J. S. Rozowsky, “*On the relationship between Yang-Mills theory and gravity and its implication for ultraviolet divergences*”, *Nucl. Phys.* B530, 401 (1998), [hep-th/9802162](#).
- [58] Z. Bern, J. J. M. Carrasco and H. Johansson, “*New Relations for Gauge-Theory Amplitudes*”, *Phys. Rev.* D78, 085011 (2008), [arxiv:0805.3993](#). • Z. Bern, J. J. M. Carrasco and H. Johansson, “*Perturbative Quantum Gravity as a Double Copy of Gauge Theory*”, *Phys. Rev. Lett.* 105, 061602 (2010), [arxiv:1004.0476](#).
- [59] N. E. J. Bjerrum-Bohr, P. H. Damgaard, T. Sondergaard and P. Vanhove, “*Monodromy and Jacobi-like Relations for Color-Ordered Amplitudes*”, [arxiv:1003.2403](#).
- [60] D. A. Kosower, R. Roiban and C. Vergu, “*The Six-Point NMHV amplitude in Maximally Supersymmetric Yang-Mills Theory*”, [arxiv:1009.1376](#).
- [61] C. Vergu, “*The two-loop MHV amplitudes in  $\mathcal{N} = 4$  supersymmetric Yang-Mills theory*”, [arxiv:0908.2394](#).
- [62] F. Cachazo, M. Spradlin and A. Volovich, “*Leading Singularities of the Two-Loop Six-Particle MHV Amplitude*”, *Phys. Rev.* D78, 105022 (2008), [arxiv:0805.4832](#).

- [63] M. Spradlin, A. Volovich and C. Wen, “*Three-Loop Leading Singularities and BDS Ansatz for Five Particles*”, Phys. Rev. D78, 085025 (2008), arxiv:0808.1054.
- [64] N. Arkani-Hamed, J. L. Bourjaily, F. Cachazo, S. Caron-Huot and J. Trnka, “*The All-Loop Integrand For Scattering Amplitudes in Planar  $N=4$  SYM*”, arxiv:1008.2958.
- [65] J. M. Drummond and J. M. Henn, “*Simple loop integrals and amplitudes in  $N=4$  SYM*”, arxiv:1008.2965.
- [66] C. Anastasiou, Z. Bern, L. J. Dixon and D. A. Kosower, “*Planar amplitudes in maximally supersymmetric Yang-Mills theory*”, Phys. Rev. Lett. 91, 251602 (2003), hep-th/0309040.
- [67] J. M. Drummond, J. Henn, G. P. Korchemsky and E. Sokatchev, “*On planar gluon amplitudes/Wilson loops duality*”, Nucl. Phys. B795, 52 (2008), arxiv:0709.2368.
- [68] Z. Bern, L. Dixon, D. Kosower, R. Roiban, M. Spradlin, C. Vergu and A. Volovich, “*The Two-Loop Six-Gluon MHV Amplitude in Maximally Supersymmetric Yang-Mills Theory*”, Phys. Rev. D78, 045007 (2008), arxiv:0803.1465.
- [69] L. F. Alday and J. Maldacena, “*Comments on gluon scattering amplitudes via AdS/CFT*”, JHEP 0711, 068 (2007), arxiv:0710.1060.
- [70] L. F. Alday and J. M. Maldacena, “*Gluon scattering amplitudes at strong coupling*”, JHEP 0706, 064 (2007), arxiv:0705.0303.
- [71] L. F. Alday, “*Review of AdS/CFT Integrability, Chapter V.3: Scattering Amplitudes at Strong Coupling*”, arxiv:1012.4003.
- [72] V. Del Duca, C. Duhr and V. A. Smirnov, “*An Analytic Result for the Two-Loop Hexagon Wilson Loop in  $N = 4$  SYM*”, arxiv:0911.5332.
- [73] A. B. Goncharov, M. Spradlin, C. Vergu and A. Volovich, “*Classical Polylogarithms for Amplitudes and Wilson Loops*”, arxiv:1006.5703.
- [74] J. M. Drummond, G. P. Korchemsky and E. Sokatchev, “*Conformal properties of four-gluon planar amplitudes and Wilson loops*”, Nucl. Phys. B795, 385 (2008), arxiv:0707.0243. • A. Brandhuber, P. Heslop and G. Travaglini, “*MHV Amplitudes in  $\mathcal{N} = 4$  Super Yang-Mills and Wilson Loops*”, Nucl. Phys. B794, 231 (2008), arxiv:0707.1153.
- [75] J. M. Drummond, J. Henn, G. P. Korchemsky and E. Sokatchev, “*Hexagon Wilson loop = six-gluon MHV amplitude*”, Nucl. Phys. B815, 142 (2009), arxiv:0803.1466.
- [76] C. Anastasiou, A. Brandhuber, P. Heslop, V. V. Khoze, B. Spence and G. Travaglini, “*Two-Loop Polygon Wilson Loops in  $\mathcal{N} = 4$  SYM*”, JHEP 0905, 115 (2009), arxiv:0902.2245.
- [77] C. Vergu, “*Higher point MHV amplitudes in  $\mathcal{N} = 4$  Supersymmetric Yang-Mills Theory*”, Phys. Rev. D79, 125005 (2009), arxiv:0903.3526.
- [78] J. M. Henn, S. G. Naculich, H. J. Schnitzer and M. Spradlin, “*Higgs-regularized three-loop four-gluon amplitude in  $N=4$  SYM: exponentiation and Regge limits*”, arxiv:1001.1358.



# Review of AdS/CFT Integrability, Chapter V.2: Dual Superconformal Symmetry

J. M. DRUMMOND

*PH-TH Division, CERN, 1211 Geneva 23, Switzerland*

*LAPTH, Université de Savoie, CNRS, B.P. 110, F-74941 Annecy-le-Vieux Cedex, France*

drummond@lapp.in2p3.fr

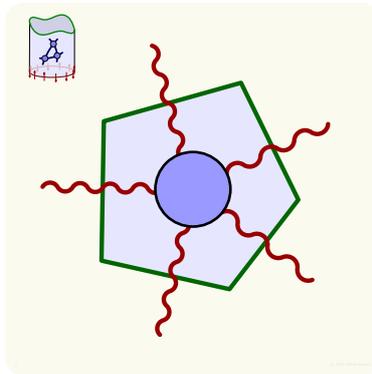

**Abstract:** Scattering amplitudes in planar  $\mathcal{N} = 4$  super Yang-Mills theory reveal a remarkable symmetry structure. In addition to the superconformal symmetry of the Lagrangian of the theory, the planar amplitudes exhibit a dual superconformal symmetry. The presence of this additional symmetry imposes strong restrictions on the amplitudes and is connected to a duality relating scattering amplitudes to Wilson loops defined on polygonal light-like contours. The combination of the superconformal and dual superconformal symmetries gives rise to a Yangian, an algebraic structure which is known to be related to the appearance of integrability in other regimes of the theory. We discuss two dual formulations of the symmetry and address the classification of its invariants.

## 1 Introduction

The aim of this article is to give an overview of the role of extended symmetries in the context of scattering amplitudes in  $\mathcal{N} = 4$  super Yang-Mills. We will begin by examining the structure of the loop corrections in perturbation theory. The scattering amplitudes are typically described in terms of scalar loop integrals. The integrals contributing in the planar limit turn out to reveal a remarkable property, namely that when exchanged for their dual graphs they exhibit a new conformal symmetry, dual conformal symmetry.

This symmetry of scattering amplitudes is also revealed if one considers the strong coupling description which is given in terms of minimal surfaces in  $\text{AdS}_5$ . More detail on this subject can be found in [V.3]. A T-duality transformation of the classical string equations of motion then relates scattering amplitudes to Wilson loops defined on polygonal light-like contour. The T-dual space where the Wilson loop is defined is related to the momenta of the particles in the scattering amplitude. The relation to Wilson loops has been observed for certain amplitudes also in the perturbative regime. From the symmetry point of view the most important consequence of this is that the conformal symmetry naturally associated to the Wilson loop also acts as a new symmetry of the amplitudes. Thus the dual conformal symmetry is at least partially explained by the duality between amplitudes and Wilson loops. The explanation is by no means complete as the dual description only applies to the special class of maximally-helicity-violating (MHV) amplitudes. However it turns out that the notion of dual conformal symmetry seems to apply to all amplitudes and furthermore naturally extends to a full dual superconformal symmetry. In particular tree-level amplitudes of all helicity types are covariant under dual superconformal symmetry. We will describe the formulation of these symmetries and discuss to what extent the symmetry is controlled beyond tree-level.

The combination of the original Lagrangian superconformal symmetry and the dual superconformal symmetry yields a Yangian structure. This structure arises in many regimes of the planar AdS/CFT system and can be thought of as the indicator of the integrability of the model. A natural question which arises with such an infinite-dimensional symmetry to hand is whether one can classify all of its invariants. It turns out that a remarkable integral formula which gives all possible leading singularities of the perturbative scattering amplitudes also fills the role of providing all possible Yangian invariants. In some sense this indicates that the planar amplitude is being determined by its symmetry at the level of its leading singularities. More concretely one can say that the integrand of the amplitude is Yangian invariant up to a total derivative. It remains to be seen to what extent these ideas can be extended to determine the loop corrections themselves, i.e. after doing the loop integrations.

## 2 Amplitudes at weak coupling

We will begin our discussion by examining perturbative scattering amplitudes in  $\mathcal{N} = 4$  super Yang-Mills theory in the planar limit. Further details on scattering amplitudes in perturbation theory can be found in [V.1]. A lot can be learned from the simplest

case of the four-gluon scattering amplitudes. Due to supersymmetry, the only non-zero amplitudes are those for two gluons of each helicity type. These amplitudes are examples of the so-called maximally-helicity-violating or MHV amplitudes which have a total helicity of  $(n - 4)$ . For four particles this quantity vanishes and so by applying a parity transformation one can see that the amplitudes are also anti-MHV or  $\overline{\text{MHV}}$  amplitudes. MHV amplitudes are particularly simple in that they can naturally be written as a product of the rational tree-level amplitude and a loop-correction function which is a series in the 't Hooft coupling  $a$ ,

$$\mathcal{A}_n^{\text{MHV}} = \mathcal{A}_{n,\text{tree}}^{\text{MHV}} M_n(p_1, \dots, p_n; a). \quad (2.1)$$

One can write any amplitude in this form of course, but the special property of MHV amplitudes is that the function  $M_n$  is a function which produces a constant after taking  $2l$  successive discontinuities at  $l$  loops. In other words, all leading singularities of MHV amplitudes are proportional to the MHV tree-level amplitude. Strictly speaking the amplitude is infrared divergent and the function  $M_n$  also depends on the regularisation parameters. The operation of taking  $2l$  discontinuities at  $l$  loops yields an infrared finite quantity however and the regulator can therefore then be set to zero.

The function  $M_n$  is given by a perturbative expansion in terms of scalar loop integrals. If we consider the four-particle case then the relevant planar loop integral topologies appearing up to three-loop order are of the form shown in Fig. 1 [1, 4] The integrals

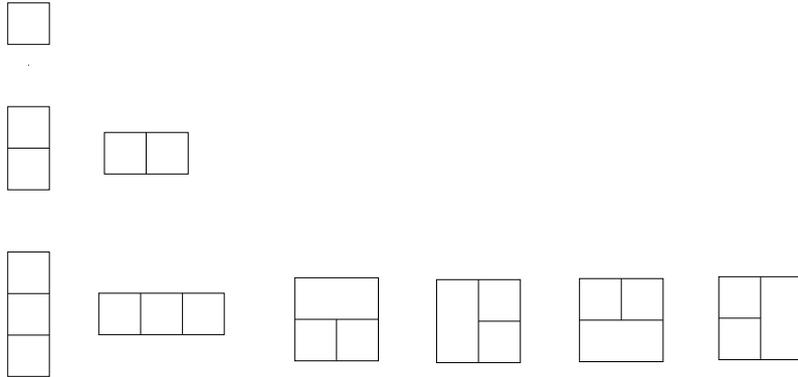

**Figure 1:** Integral topologies up to three loops. The external momenta flow in at the four corners in each topology.

contributing to  $M_4$  all have a remarkable property - they exhibit an unexpected conformal symmetry called ‘dual conformal symmetry’ [8]. The way to make this symmetry obvious is to make a change of variables from momentum parametrisation of such integrals to a dual coordinate representation,

$$p_i^\mu = x_i^\mu - x_{i+1}^\mu \equiv x_{i,i+1}^\mu, \quad x_{n+1}^\mu \equiv x_1^\mu. \quad (2.2)$$

We will illustrate this here on the example of the one-loop scalar box integral which is the one-loop contribution to  $M_4$ ,

$$I^{(1)} = \int \frac{d^4 k}{k^2(k-p_1)^2(k-p_1-p_2)^2(k+p_4)^2}. \quad (2.3)$$

In this case the change of variables takes the form,

$$p_1 = x_{12}, \quad p_2 = x_{23}, \quad p_3 = x_{34}, \quad p_4 = x_{41}. \quad (2.4)$$

The integral can then be written as a four-point star diagram (the dual graph for the one-loop box) with the loop integration replaced by an integration over the internal vertex  $x_5$  as illustrated in Fig. 2. In the new variables a new symmetry is manifest. If

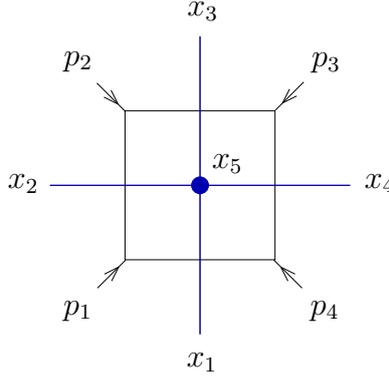

**Figure 2:** Dual diagram for the one-loop box. The black lines denote the original momentum space loop integral. The propagators can equivalently be represented as scalar propagators in the dual space, denoted by the blue lines.

we consider conformal inversions of the dual coordinates,

$$x_i^\mu \longrightarrow -\frac{x_i^\mu}{x_i^2}, \quad (2.5)$$

then we see that the integrand, including the measure factor  $d^4x_5$ , is actually covariant,

$$\frac{d^4x_5}{x_{15}^2 x_{25}^2 x_{35}^2 x_{45}^2} \longrightarrow (x_1^2 x_2^2 x_3^2 x_4^2) \frac{d^4x_5}{x_{15}^2 x_{25}^2 x_{35}^2 x_{45}^2}. \quad (2.6)$$

The property of dual conformal covariance of the integral form is not restricted to one loop but continues to all loop orders so far explored [18, 26]. For example, at three loops one of the relevant integrals requires a precise numerator factor to remain dual conformally covariant (see Fig. 3). Note that the operation of drawing the dual graph is only possible for planar diagrams. This is the first indication that the dual conformal property is something associated with the integrability of the planar theory.

Beyond tree-level the scattering amplitudes are infrared divergent. This can be seen at the level of the integrals, e.g. as defined in (2.3). We therefore need to introduce an infrared regulator. One choice is to use dimensional regularisation. This breaks the dual conformal symmetry slightly since the integration measure is then no longer four-dimensional,

$$d^4x_5 \longrightarrow d^{4-2\epsilon}x_5. \quad (2.7)$$

Alternatively one can regularise by introducing expectation values for the scalar fields [35]. The mass parameters then play the role of radial coordinates in  $AdS_5$ . This

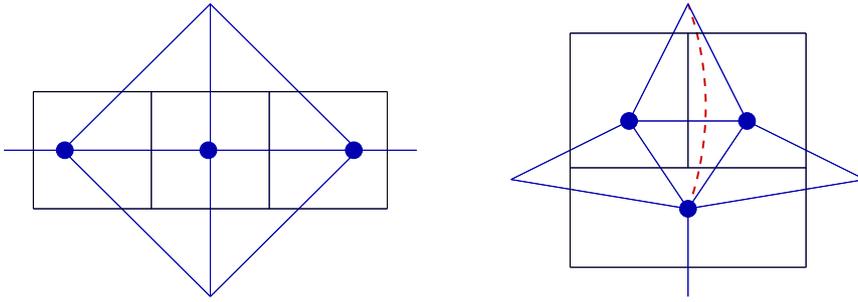

**Figure 3:** Dual diagrams for the three-loop box and for the ‘tennis court’ with its numerator denoted by the dashed line corresponding to a factor in the numerator of the square distance between the two points.

Coulomb branch approach has the advantage that the corresponding action of dual conformal symmetry transforms the regularised integral covariantly. If all the integrals appearing in the amplitude are dual conformal it implies that amplitudes on the Coulomb branch of  $\mathcal{N} = 4$  super Yang-Mills in the planar limit exhibit an unbroken dual conformal symmetry. For further details on this idea see [43, 53, 56] and for work relating it to higher dimensional theories see [2].

To discuss the consequences of dual conformal symmetry further it is very convenient to introduce a dual description for the scattering amplitudes. In the dual description planar amplitudes are related to Wilson loops defined on a piecewise light-like contour in the dual coordinate space. The dual conformal symmetry of the amplitude is simply the ordinary conformal symmetry of the Wilson loop. Since the conformal symmetry of a Wilson loop has a Lagrangian origin, it is possible to derive a Ward identity for it. This will show us more precisely the constraints that dual conformal symmetry places on the form of the scattering amplitudes.

### 3 Amplitudes and Wilson loops

Let us consider the general structure of a planar MHV amplitude in perturbation theory. As we have discussed we can naturally factorise MHV amplitudes into a tree-level factor and a loop-correction factor  $M_n$ . The factor  $M_n$  contains the dependence of the amplitude on the regularisation needed to deal with the infrared divergences. Here we will use dimensional regularisation. the amplitudes will therefore depend on the regulator  $\epsilon$  and some associated scale  $\mu$ .

Since we are discussing planar colour-ordered amplitudes it is clear that the infrared divergences will involve only a very limited dependence on the kinematical variables. Specifically, the exchange of soft or collinear gluons is limited to sectors between two adjacent incoming particles and thus the infrared divergences will factorise into pieces which depend only on a single Mandelstam variable  $s_{i,i+1} = (p_i + p_{i+1})^2$ .

Moreover the dependence of each of these factors is known to be of a particular exponentiated form [3, 5] where there is at most a double pole in the regulator in the exponent. Combining these two facts together it is most natural to write the logarithm

of the loop corrections  $M_n$ ,

$$\log M_n = \sum_{l=1}^{\infty} a^l \left[ \frac{\Gamma_{\text{cusp}}^{(l)}}{(l\epsilon)^2} + \frac{\Gamma_{\text{col}}^{(l)}}{l\epsilon} \right] \sum_i \left( \frac{\mu_{IR}^2}{-s_{i,i+1}} \right)^{l\epsilon} + F_n^{\text{MHV}}(p_1, \dots, p_n; a) + O(\epsilon). \quad (3.1)$$

The leading infrared divergence is known to be governed by  $\Gamma_{\text{cusp}}(a) = \sum a^l \Gamma_{\text{cusp}}^{(l)}$ , the cusp anomalous dimension [6], a quantity which is so-called because it arises as the leading ultraviolet divergence of Wilson loops with light-like cusps. This is the first connection between scattering amplitudes and Wilson loops.

In [4] Bern, Dixon and Smirnov (BDS) made an all order ansatz for the form of the finite part of the  $n$ -point MHV scattering amplitude in the planar limit. Their ansatz had the following form,

$$F_n^{\text{BDS}}(p_1, \dots, p_n; a) = \Gamma_{\text{cusp}}(a) \mathcal{F}_n(p_1, \dots, p_n) + c_n(a). \quad (3.2)$$

The notable feature of this ansatz is that the dependence on the coupling factorises into a single function, the cusp anomalous dimension, while the momentum dependence is contained in the coupling-independent function  $\mathcal{F}_n$ . The latter could therefore be defined by the one-loop amplitude, making the ansatz true by definition at one loop. The formula (3.2) was conjectured after direct calculations of the four-point amplitude to two loops [1] and three loops [4]. It was found to be consistent with the five-point amplitude at two loops [7] and three loops [9]. As we will see the results for four and five points can be explained by dual conformal symmetry, which also permits for a deviation from the form (3.2) starting from six points. Indeed the ansatz breaks down at six points and as we will see this is in agreement with dual conformal symmetry and the relation between amplitudes and Wilson loops.

In planar  $\mathcal{N} = 4$  super Yang-Mills theory the connection between amplitudes and Wilson loops runs deeper than just the leading infrared divergence. As we have seen one can naturally associate a collection of dual coordinates  $x_i$  with a gluon scattering amplitude. Each dual coordinate is light-like separated from its neighbours,

$$(x_i - x_{i+1})^2 = 0 \quad (3.3)$$

as the difference  $x_i - x_{i+1}$  is the momentum  $p_i$  of an on-shell massless particle. The collection of points  $\{x_i\}$  therefore naturally defines a piecewise light-like polygonal contour  $C_n$  in the dual space. A natural object that one can associate with such a contour in gauge theory is the Wilson loop,

$$W_n = \langle \mathcal{P} \exp \oint_{C_n} A \rangle. \quad (3.4)$$

Here, in contrast to the situation for the scattering amplitude, the dual space is being treated as the actual configuration space of the gauge theory, i.e. the theory in which we compute the Wilson loop is local in this space.

A lot is known about the structure of such Wilson loops. In particular, due to the cusps on the contour at the points  $x_i$  the Wilson loop is ultraviolet divergent. The

divergences of such Wilson loops are intimately related to the infrared divergences of scattering amplitudes [6, 10]. Indeed the leading ultraviolet divergence is again the cusp anomalous dimension and one can write an equation very similar to that for the loop corrections to the MHV amplitude,

$$\log W_n = \sum_{l=1}^{\infty} a^l \left[ \frac{\Gamma_{\text{cusp}}^{(l)}}{(l\epsilon)^2} + \frac{\Gamma^{(l)}}{l\epsilon} \right] \sum_i (-\mu_{UV}^2 x_{i,i+2}^2)^{l\epsilon} + F_n^{\text{WL}}(x_1, \dots, x_n; a) + O(\epsilon). \quad (3.5)$$

The objects of most interest to us here are the two functions  $F_n^{\text{MHV}}$  from (3.1) and  $F_n^{\text{WL}}$  from (3.5) describing the finite parts of the amplitude and Wilson loop respectively. In fact there is by now a lot of evidence that in the planar theory, the two functions are identical up to an additive constant,

$$F_n^{\text{MHV}}(p_1, \dots, p_n; a) = F_n^{\text{WL}}(x_1, \dots, x_n; a) + d_n(a) \quad (3.6)$$

upon using the change of variables (2.2).

The identification of the two finite parts was first made at strong coupling [11] where the AdS/CFT correspondence can be used to study the theory. In this regime the identification is a consequence of a particular T-duality transformation of the string sigma model which maps the AdS background into a dual AdS space. Shortly afterwards the identification was made in perturbation theory, suggesting that such a phenomenon is actually a non-perturbative feature. The matching was first observed at four points and one loop [12] and generalised to  $n$  points in [13]. Two loop calculations then followed [14–17]. In each case the duality relation (3.6) was indeed verified.

An important point is that dual conformal symmetry finds a natural home within the duality between amplitudes and Wilson loops. It is simply the ordinary conformal symmetry of the Wilson loop defined in the dual space. Moreover, since this symmetry is a Lagrangian symmetry from the point of view of the Wilson loop, its consequences can be derived in the form of Ward identities [14, 15]. Importantly, conformal transformations preserve the form of the contour, i.e. light-like polygons map to light-like polygons. Thus the conformal transformations effectively act only on a finite number of points (the cusp points  $x_i$ ) defining the contour. The generator of special conformal transformations relevant to the class of light-like polygonal Wilson loops is therefore

$$K_\mu = \sum_i \left[ x_{i\mu} x_i \cdot \frac{\partial}{\partial x_i} - \frac{1}{2} x_i^2 \frac{\partial}{\partial x_i^\mu} \right]. \quad (3.7)$$

Indeed the analysis of [15] shows that the ultraviolet divergences induce an anomalous behaviour for the finite part  $F_n^{\text{WL}}$  which is entirely captured by the following conformal Ward identity

$$K^\mu F_n^{\text{WL}} = \frac{1}{2} \Gamma_{\text{cusp}}(a) \sum_i (2x_i^\mu - x_{i-1}^\mu - x_{i+1}^\mu) \log x_{i-1,i+1}^2. \quad (3.8)$$

A very important consequence of the conformal Ward identity is that the finite part of the Wilson loop is fixed up to a function of conformally invariant cross-ratios,

$$u_{ijkl} = \frac{x_{ij}^2 x_{kl}^2}{x_{ik}^2 x_{jl}^2}. \quad (3.9)$$

In the cases of four and five edges, there are no such cross-ratios available due to the light-like separations of the cusp points (3.3). This means that the conformal Ward identity (3.8) has a unique solution up to an additive constant. Remarkably, the solution coincides with the Bern-Dixon-Smirnov all-order ansatz for the corresponding scattering amplitudes,

$$F_4^{(\text{BDS})} = \frac{1}{4} \Gamma_{\text{cusp}}(a) \log^2\left(\frac{x_{13}^2}{x_{24}^2}\right) + \text{const} , \quad (3.10)$$

$$F_5^{(\text{BDS})} = -\frac{1}{8} \Gamma_{\text{cusp}}(a) \sum_{i=1}^5 \log\left(\frac{x_{i,i+2}^2}{x_{i,i+3}^2}\right) \log\left(\frac{x_{i+1,i+3}^2}{x_{i+2,i+4}^2}\right) + \text{const} . \quad (3.11)$$

In fact the BDS ansatz provides a particular solution to the conformal Ward identity for any number of points. From six points onwards however the functional form is not uniquely fixed as there are conformal cross-ratios available. At six points, for example there are three of them,

$$u_1 = \frac{x_{13}^2 x_{46}^2}{x_{14}^2 x_{36}^2}, \quad u_2 = \frac{x_{24}^2 x_{51}^2}{x_{25}^2 x_{41}^2}, \quad u_3 = \frac{x_{35}^2 x_{62}^2}{x_{36}^2 x_{41}^2}. \quad (3.12)$$

The solution to the Ward identity is therefore

$$F_6^{(\text{WL})} = F_6^{(\text{BDS})} + f(u_1, u_2, u_3; a) . \quad (3.13)$$

Here, upon the identification  $p_i = x_i - x_{i+1}$ ,

$$F_6^{(\text{BDS})} = \frac{1}{4} \Gamma_{\text{cusp}}(a) \sum_{i=1}^6 \left[ -\log\left(\frac{x_{i,i+2}^2}{x_{i,i+3}^2}\right) \log\left(\frac{x_{i+1,i+3}^2}{x_{i,i+3}^2}\right) + \frac{1}{4} \log^2\left(\frac{x_{i,i+3}^2}{x_{i+1,i+4}^2}\right) - \frac{1}{2} \text{Li}_2\left(1 - \frac{x_{i,i+2}^2 x_{i+3,i+5}^2}{x_{i,i+3}^2 x_{i+2,i+5}^2}\right) \right] + \text{const} , \quad (3.14)$$

while  $f(u_1, u_2, u_3; a)$  is some function of the three cross-ratios and the coupling. As we have discussed the function  $f$  is not fixed by the Ward identity and has to be determined by explicit calculation of the Wilson loop. The calculation of [13] shows that at one loop  $f$  vanishes (recall that at one loop the BDS ansatz is true by definition and the Wilson loop and MHV amplitude are known to agree for an arbitrary number of points). At two loops, direct calculation shows that  $f$  is non-zero [16]. Moreover the calculation [17] of the six-particle MHV amplitude shows explicitly that the BDS ansatz breaks down at two loops and the same function appears there,

$$F_6^{\text{MHV}} = F_6^{\text{WL}} + \text{const}, \quad F_6^{\text{MHV}} \neq F_6^{\text{BDS}}. \quad (3.15)$$

The agreement between the two functions  $F_6^{\text{MHV}}$  and  $F_6^{\text{WL}}$  was verified numerically to within the available accuracy. Subsequently the integrals appearing in the calculation of the finite part of the of the hexagonal Wilson loop have been evaluated analytically in terms of multiple polylogarithms [19].

Further calculations of polygonal Wilson loops have been performed. The two-loop diagrams appearing for an arbitrary number of points have been described in [20] where numerical evaluations of the seven-sided and eight-sided light-like Wilson loops were made. These functions have not yet been compared with the corresponding MHV amplitude calculations [21] due to the difficulty of numerically evaluating the relevant integrals. However given the above evidence it seems very likely that the agreement between MHV amplitudes and light-like polygonal Wilson loops will continue to an arbitrary number of points, to all orders in the coupling.

While the agreement between Wilson loops is fascinating it is clearly not the end of the story. Firstly the duality as we have described it applies only to the MHV amplitudes. In the strict strong coupling limit this does not matter since all amplitudes are dominated by the minimal surface in AdS, independently of the helicity configuration [11]. At weak coupling that is certainly not the case and non-MHV amplitudes reveal a much richer structure than their MHV counterparts. Recently the duality has been extended to take into account non-MHV amplitudes [22] by introducing an appropriate supersymmetrisation of the Wilson loop.

Even without regard to a dual Wilson loop, one may still ask what happens to dual conformal symmetry for non-MHV amplitudes. To properly ask this question one must first deal with the notion of helicity since non-MHV amplitudes are not naturally written as a product of tree-level and loop-correction contributions. In considering different helicity configurations we are led to the notion of dual superconformal symmetry.

## 4 Superconformal and dual superconformal symmetry

The on-shell supermultiplet of  $\mathcal{N} = 4$  super Yang-Mills theory is conveniently described by a superfield  $\Phi$ , dependent on Grassmann parameters  $\eta^A$  which transform in the fundamental representation of  $su(4)$ . The on-shell superfield can be expanded as follows

$$\Phi = G^+ + \eta^A \Gamma_A + \frac{1}{2!} \eta^A \eta^B S_{AB} + \frac{1}{3!} \eta^A \eta^B \eta^C \epsilon_{ABCD} \bar{\Gamma}^D + \frac{1}{4!} \eta^A \eta^B \eta^C \eta^D \epsilon_{ABCD} G^-. \quad (4.1)$$

Here  $G^+, \Gamma_A, S_{AB} = \frac{1}{2} \epsilon_{ABCD} \bar{S}^{CD}, \bar{\Gamma}^A, G^-$  are the positive helicity gluon, gluino, scalar, anti-gluino and negative helicity gluon states respectively. Each of the possible states  $\phi \in \{G^+, \Gamma_A, S_{AB}, \bar{\Gamma}^A, G^-\}$  carries a definite on-shell momentum

$$p^{\alpha\dot{\alpha}} = \lambda^\alpha \tilde{\lambda}^{\dot{\alpha}}, \quad (4.2)$$

and a definite weight  $h$  (called helicity) under the rescaling

$$\lambda \longrightarrow \alpha \lambda, \quad \tilde{\lambda} \longrightarrow \alpha^{-1} \tilde{\lambda}, \quad \phi(\lambda, \tilde{\lambda}) \longrightarrow \alpha^{-2h} \phi(\lambda, \tilde{\lambda}). \quad (4.3)$$

The helicities of the states appearing in (4.1) are  $\{+1, +\frac{1}{2}, 0, -\frac{1}{2}, -1\}$  respectively. If, in addition, we assign  $\eta$  to transform in the same way as  $\tilde{\lambda}$ ,

$$\eta^A \longrightarrow \alpha^{-1} \eta^A, \quad (4.4)$$

then the whole superfield  $\Phi$  has helicity 1. In other words the helicity generator<sup>1</sup>,

$$h = -\frac{1}{2}\lambda^\alpha \frac{\partial}{\partial \lambda^\alpha} + \frac{1}{2}\tilde{\lambda}^{\dot{\alpha}} \frac{\partial}{\partial \tilde{\lambda}^{\dot{\alpha}}} + \frac{1}{2}\eta^A \frac{\partial}{\partial \eta^A}, \quad (4.5)$$

acts on  $\Phi$  in the following way,

$$h\Phi = \Phi. \quad (4.6)$$

When we consider superamplitudes, i.e. colour-ordered scattering amplitudes of the on-shell superfields, then the helicity condition (or ‘homogeneity condition’) is satisfied for each particle,

$$h_i \mathcal{A}(\Phi_1, \dots, \Phi_n) = \mathcal{A}(\Phi_1, \dots, \Phi_n), \quad i = 1, \dots, n. \quad (4.7)$$

The tree-level amplitudes in  $\mathcal{N} = 4$  super Yang-Mills theory can be written as follows,

$$\mathcal{A}(\Phi_1, \dots, \Phi_n) = \mathcal{A}_n = \frac{\delta^4(p)\delta^8(q)}{\langle 12 \rangle \dots \langle n1 \rangle} \mathcal{P}_n(\lambda_i, \tilde{\lambda}_i, \eta_i) = \mathcal{A}_n^{\text{MHV}} \mathcal{P}_n. \quad (4.8)$$

The MHV tree-level amplitude,

$$\mathcal{A}_n^{\text{MHV}} = \frac{\delta^4(p)\delta^8(q)}{\langle 12 \rangle \dots \langle n1 \rangle}, \quad (4.9)$$

contains the delta functions  $\delta^4(p)\delta^8(q)$  which are a consequence of translation invariance and supersymmetry and it can be factored out leaving behind a function with no helicity,

$$h_i \mathcal{P}_n = 0, \quad i = 1, \dots, n. \quad (4.10)$$

The function  $\mathcal{P}_n$  can be expanded in terms of increasing Grassmann degree (the Grassmann degree always comes in multiples of 4 due to invariance under  $su(4)$ ),

$$\mathcal{P}_n = 1 + \mathcal{P}_n^{\text{NMHV}} + \mathcal{P}_n^{\text{NNMHV}} + \dots + \mathcal{P}_n^{\overline{\text{MHV}}}. \quad (4.11)$$

The explicit form of the function  $\mathcal{P}_n$  which encodes all tree-level amplitudes was found in [23] by solving a supersymmetrised version [24, 25] of the BCFW recursion relations [27].

Maximally supersymmetric Yang-Mills is a superconformal field theory so we should expect that this is reflected in the structure of the scattering amplitudes. Indeed the space of functions of the variables  $\{\lambda_i, \tilde{\lambda}_i, \eta_i\}$  admits a representation of the superconformal algebra. The explicit form of the representation acting on the on-shell superspace

---

<sup>1</sup>In terms of the superconformal algebra  $su(2, 2|4)$ , the operator  $h$  is the central charge.

coordinates  $(\lambda_i, \tilde{\lambda}_i, \eta_i)$  is essentially the oscillator representation [28].

$$\begin{aligned}
 p^{\dot{\alpha}\alpha} &= \sum_i \tilde{\lambda}_i^{\dot{\alpha}} \lambda_i^\alpha, & k_{\alpha\dot{\alpha}} &= \sum_i \partial_{i\alpha} \partial_{i\dot{\alpha}}, \\
 \bar{m}_{\dot{\alpha}\dot{\beta}} &= \sum_i \tilde{\lambda}_{i(\dot{\alpha}} \partial_{i\dot{\beta})}, & m_{\alpha\beta} &= \sum_i \lambda_{i(\alpha} \partial_{i\beta)}, \\
 d &= \sum_i \left[ \frac{1}{2} \lambda_i^\alpha \partial_{i\alpha} + \frac{1}{2} \tilde{\lambda}_i^{\dot{\alpha}} \partial_{i\dot{\alpha}} + 1 \right], & r^A{}_B &= \sum_i \left[ -\eta_i^A \partial_{iB} + \frac{1}{4} \delta_B^A \eta_i^C \partial_{iC} \right], \\
 q^{\alpha A} &= \sum_i \lambda_i^\alpha \eta_i^A, & \bar{q}_A^{\dot{\alpha}} &= \sum_i \tilde{\lambda}_i^{\dot{\alpha}} \partial_{iA}, \\
 s_{\alpha A} &= \sum_i \partial_{i\alpha} \partial_{iA}, & \bar{s}_A^{\dot{\alpha}} &= \sum_i \eta_i^A \partial_{i\dot{\alpha}}, \\
 c &= \sum_i \left[ 1 + \frac{1}{2} \lambda_i^\alpha \partial_{i\alpha} - \frac{1}{2} \tilde{\lambda}_i^{\dot{\alpha}} \partial_{i\dot{\alpha}} - \frac{1}{2} \eta_i^A \partial_{iA} \right]. & & (4.12)
 \end{aligned}$$

This realisation of the superconformal algebra also appears in the discussion of gauge-invariant operators [VI.1]. From the commutation relations of the superconformal algebra one finds that the algebra is generically  $su(2, 2|4)$  with central charge  $c = \sum_i (1 - h_i)$ . Amplitudes are in the space of functions with helicity 1 for each particle so we have that  $c = 0$  after imposing the helicity conditions (4.7) and the algebra acting on the space of homogeneous functions is  $psu(2, 2|4)$ .

At tree-level there are no infrared divergences and amplitudes are annihilated by the generators of the standard superconformal symmetry (up to contact terms which vanish for generic configurations of the external momenta, see [29, 30]),

$$j_a \mathcal{A}_n = 0. \quad (4.13)$$

Here we use the notation  $j_a$  for any generator of the superconformal algebra  $psu(2, 2|4)$ ,

$$j_a \in \{p^{\alpha\dot{\alpha}}, q^{\alpha A}, \bar{q}_A^{\dot{\alpha}}, m_{\alpha\beta}, \bar{m}_{\dot{\alpha}\dot{\beta}}, r^A{}_B, d, s_A^\alpha, \bar{s}_\alpha^A, k_{\alpha\dot{\alpha}}\}. \quad (4.14)$$

As well as superconformal symmetry one can naturally define the action of dual superconformal symmetry [31] on colour-ordered amplitudes. We have already seen that one can define dual coordinates  $x_i$  related to the particle momenta. These variables implicitly solve the momentum conservation condition imposed by the delta function  $\delta^4(p)$ . The presence of a corresponding  $\delta^8(q)$  due to supersymmetry suggests defining new fermionic dual variables  $\theta_i$  related to the supercharges. Together these variables parametrise a chiral dual superspace,

$$x_i^{\alpha\dot{\alpha}} - x_{i+1}^{\alpha\dot{\alpha}} = \lambda_i^\alpha \tilde{\lambda}_i^{\dot{\alpha}} = p_i^{\alpha\dot{\alpha}}, \quad \theta_i^{\alpha A} - \theta_{i+1}^{\alpha A} = \lambda_i^\alpha \eta_i^A = q_i^{\alpha A}. \quad (4.15)$$

Dual superconformal symmetry acts canonically on the dual superspace variables  $x_i, \theta_i$ . It also acts on the on-shell superspace variables  $\{\lambda_i, \tilde{\lambda}_i, \eta_i\}$  in order to be compatible with the defining relations (4.15). In particular one can deduce an action of dual conformal inversions on  $\lambda_i, \tilde{\lambda}_i$  compatible with (4.15),

$$I[\lambda_i^\alpha] = \frac{(\lambda_i x_i)^\alpha}{x_i^2}, \quad I[\tilde{\lambda}_i^{\dot{\alpha}}] = \frac{(\tilde{\lambda}_i x_i)^{\dot{\alpha}}}{x_{i+1}^2}. \quad (4.16)$$

Alternatively one may think about infinitesimal dual superconformal transformations. In this case one should extend the canonical generators on the chiral superspace variables  $x_i$  and  $\theta_i$  to act on the on-shell superspace variables  $\lambda_i, \tilde{\lambda}_i$  and  $\eta_i$  so that they commute with the constraints (4.15) modulo the constraints themselves. We give explicitly the form of the dual conformal generator,

$$K_{\alpha\dot{\alpha}} = \sum_i [x_{i\dot{\alpha}}^{\dot{\beta}} x_{i\dot{\alpha}}^{\beta} \partial_{i\beta\dot{\beta}} + x_{i\dot{\alpha}}^{\beta} \theta_{i\dot{\alpha}}^B \partial_{i\beta B} + x_{i\dot{\alpha}}^{\beta} \lambda_{i\dot{\alpha}} \partial_{i\beta} + x_{i+1\alpha}^{\dot{\beta}} \tilde{\lambda}_{i\dot{\alpha}} \partial_{i\dot{\beta}} + \tilde{\lambda}_{i\dot{\alpha}} \theta_{i+1\alpha}^B \partial_{iB}]. \quad (4.17)$$

The anti-chiral fermionic generators are also of interest,

$$\bar{Q}_{\dot{\alpha}}^A = \sum_i [\theta_i^{\alpha A} \partial_{i\alpha\dot{\alpha}} + \eta_i^A \partial_{i\dot{\alpha}}], \quad \bar{S}_{\dot{\alpha}A} = \sum_i [x_{i\dot{\alpha}}^{\beta} \partial_{i\beta A} + \tilde{\lambda}_{i\dot{\alpha}} \partial_{iA}]. \quad (4.18)$$

The remaining generators can be found in [31]. Note that when restricted to the on-shell superspace, the generators  $\bar{Q}_{\dot{\alpha}}^A$  and  $\bar{S}_{\dot{\alpha}A}$  coincide with the generators  $\bar{s}_{\dot{\alpha}}^A$  and  $\bar{q}_{\dot{\alpha}A}$  respectively from the original superconformal algebra.

Now that the symmetry has been defined we must also specify how the amplitudes transform. In [31] it was conjectured, based on the supersymmetric forms of the MHV and next-to-MHV (NMHV) tree-level amplitudes, that the full tree-level superamplitude  $\mathcal{A}_{n,\text{tree}}$  is covariant under dual superconformal symmetry. Explicitly, it was conjectured that the tree-level amplitudes obey

$$K^{\alpha\dot{\alpha}} \mathcal{A}_n = - \sum_i x_i^{\alpha\dot{\alpha}} \mathcal{A}_n, \quad (4.19)$$

$$S^{\alpha A} \mathcal{A}_n = - \sum_i \theta_i^{\alpha A} \mathcal{A}_n, \quad (4.20)$$

together with the obvious properties  $D\mathcal{A}_n = n\mathcal{A}_n$  and  $C\mathcal{A}_n = n\mathcal{A}_n$ . The remaining generators of the dual superconformal algebra annihilate the amplitudes.

The amplitudes can be expressed in the dual variables by eliminating  $(\tilde{\lambda}_i, \eta_i)$  in favour of  $(x_i, \theta_i)$ . If we relax the cyclicity condition on the dual points so that  $x_1 \neq x_{n+1}$  and  $\theta_1 \neq \theta_{n+1}$  then we have

$$\mathcal{A}_n = \frac{\delta^4(x_1 - x_{n+1}) \delta^8(\theta_1 - \theta_{n+1})}{\langle 12 \rangle \dots \langle n1 \rangle} \mathcal{P}_n(x_i, \theta_i). \quad (4.21)$$

From the dual conformal transformations described earlier we can see that the MHV prefactor itself satisfies the covariance conditions (4.19,4.20). The function  $\mathcal{P}_n$  must therefore be dual superconformally invariant. At the MHV level the function  $\mathcal{P}_n$  is simply 1 while at NMHV level it is given by [31,32,23]

$$\mathcal{P}_n^{\text{NMHV}} = \sum_{a,b} R_{n,ab} \quad (4.22)$$

where the sum runs over the range  $2 \leq a < b \leq n-1$  (with  $a$  and  $b$  separated by at least two) and

$$R_{n,ab} = \frac{\langle a a - 1 \rangle \langle b b - 1 \rangle \delta^4(\langle n | x_{na} x_{ab} | \theta_{bn} \rangle + \langle n | x_{nb} x_{ba} | \theta_{an} \rangle)}{x_{ab}^2 \langle n | x_{na} x_{ab} | b \rangle \langle n | x_{na} x_{ab} | b - 1 \rangle \langle n | x_{nb} x_{ba} | a \rangle \langle n | x_{nb} x_{ba} | a - 1 \rangle}. \quad (4.23)$$

This formula was originally constructed in [31] by supersymmetrising the three-mass coefficients of NMHV gluon scattering amplitudes at one loop in [33]. It was then derived from supersymmetric generalised unitarity [32] as the general form of the one-loop three-mass box coefficient. One can see from the transformations described earlier that each  $R_{n,ab}$  is by itself a dual superconformal invariant.

The pattern of invariance continues for all tree-level amplitudes. Indeed the conjecture (4.19,4.20) was shown to hold recursively in [24], using the supersymmetric BCFW recursion relations. Indeed the BCFW recursion relations admit a closed form solution for all tree-level amplitudes in  $\mathcal{N} = 4$  super Yang-Mills theory [23] with each term being a dual superconformal invariant by itself.

What happens to the symmetry of scattering amplitudes beyond tree-level? Firstly we expect a breakdown of the original conformal symmetry due to infrared divergences. One might also expect a breakdown of the dual superconformal symmetry in the same way. However, at least for the MHV amplitudes we have already seen that the dual conformal symmetry is broken only mildly in that it is controlled by the anomalous Ward identity (3.8). Based on analysis of the one-loop NMHV amplitudes it was conjectured in [31] that the same anomaly controls the breakdown for all amplitudes, irrespective of the MHV degree. Specifically if one writes the all-order superamplitude as a product of the MHV superamplitude and an infrared finite ratio function<sup>2</sup>,

$$\mathcal{A}_n = \mathcal{A}_n^{\text{MHV}} R_n, \quad (4.24)$$

then the conjecture states that, setting the regulator to zero,  $R_n$  is dual conformally invariant,

$$K^\mu R_n = 0. \quad (4.25)$$

In [32] it was argued that this conjecture holds for NMHV amplitudes at one loop, based on explicit calculations up to nine points using supersymmetric generalised unitarity. Subsequently [34] it has been argued to hold for all one-loop amplitudes by analysing the dual conformal anomaly arising from infrared divergent two-particle cuts.

Note that the conjecture (4.25) makes reference only to the dual conformal generator  $K$  and not to the full set of dual superconformal transformations. The reason is that some of these transformations overlap with the broken part of the original superconformal symmetry. In particular the generator  $\bar{Q}$  is not a symmetry of the ratio function  $R_n$ . This fact is related to the breaking of the original superconformal invariance by loop corrections since  $\bar{Q}$  is really the same symmetry as  $\bar{s}$ . Indeed, even at tree-level  $\bar{s}$  is subtly broken by contact term contributions [29, 30]. At one loop unitarity relates the discontinuity of the amplitude in a particular channel to the product of two tree-level amplitudes integrated over the allowed phase space of the exchanged particles. The subtle non-invariance of the trees therefore translates into non-invariance of the discontinuity and therefore of the loop amplitude itself [30, 36]. In [36] a deformation of the ordinary and dual superconformal generators is presented which takes into account the one-loop corrections to the amplitudes. The existence of Wilson loops which take into account the

---

<sup>2</sup>The ratio function  $R_n$  is infrared finite because the infrared divergences of all planar amplitudes are independent of the helicity configuration and are thus contained entirely in the factor  $\mathcal{A}_n^{\text{MHV}}$ .

non-MHV amplitudes [22] suggests that the universality of the dual conformal anomaly is very natural from the dual perspective.

## 5 Yangian symmetry

In order to put the dual superconformal symmetry on the same footing as invariance under the standard superconformal algebra (4.13), the covariance (4.19,4.20) can be rephrased as an invariance of  $\mathcal{A}_n$  by a simple redefinition of the generators [37],

$$K'^{\alpha\dot{\alpha}} = K^{\alpha\dot{\alpha}} + \sum_i x_i^{\alpha\dot{\alpha}}, \quad (5.1)$$

$$S'^{\alpha A} = S^{\alpha A} + \sum_i \theta_i^{\alpha A}, \quad (5.2)$$

$$D' = D - n. \quad (5.3)$$

The redefined generators still satisfy the commutation relations of the superconformal algebra, but now with vanishing central charge,  $C' = 0$ . Then dual superconformal symmetry is simply

$$J'_a \mathcal{A}_n = 0. \quad (5.4)$$

Here we use the notation  $J'_a$  for any generator of the *dual* copy of  $psu(2, 2|4)$ ,

$$J'_a \in \{P_{\alpha\dot{\alpha}}, Q_{\alpha A}, \bar{Q}_{\dot{\alpha}}^A, M_{\alpha\beta}, \bar{M}_{\dot{\alpha}\dot{\beta}}, R^A_B, D', S'^A, \bar{S}'^{\dot{\alpha}}, K'^{\alpha\dot{\alpha}}\}. \quad (5.5)$$

In order to have both symmetries acting on the same space it is useful to restrict the dual superconformal generators to act only on the on-shell superspace variables  $(\lambda_i, \tilde{\lambda}_i, \eta_i)$ . Then one finds that the generators  $P_{\alpha\dot{\alpha}}, Q_{\alpha A}$  become trivial while the generators  $\{\bar{Q}, M, \bar{M}, R, D', \bar{S}'\}$  coincide (up to signs) with generators of the standard superconformal symmetry. The non-trivial generators which are not part of the  $j_a$  are  $K'$  and  $S'$ . In [37] it was shown that the generators  $j_a$  and  $S'$  (or  $K'$ ) together generate the Yangian of the superconformal algebra,  $Y(psu(2, 2|4))$ . The generators  $j_a$  form the level-zero  $psu(2, 2|4)$  subalgebra<sup>3</sup>,

$$[j_a, j_b] = f_{ab}^c j_c. \quad (5.6)$$

In addition there are level-one generators  $j_a^{(1)}$  which transform in the adjoint under the level-zero generators,

$$[j_a, j_b^{(1)}] = f_{ab}^c j_c^{(1)}. \quad (5.7)$$

Higher commutators among the generators are constrained by the Serre relation<sup>4</sup>,

$$\begin{aligned} & [j_a^{(1)}, [j_b^{(1)}, j_c]] + (-1)^{|a|(|b|+|c|)} [j_b^{(1)}, [j_c^{(1)}, j_a]] + (-1)^{|c|(|a|+|b|)} [j_c^{(1)}, [j_a^{(1)}, j_b]] \\ & = h^2 (-1)^{|r||m|+|t||n|} \{j_l, j_m, j_n\} f_{ar}^l f_{bs}^m f_{ct}^n f^{rst}. \end{aligned} \quad (5.8)$$

<sup>3</sup>We use the symbol  $[O_1, O_2]$  to denote the bracket of the Lie superalgebra,  $[O_2, O_1] = (-1)^{1+|O_1||O_2|} [O_1, O_2]$ .

<sup>4</sup>The symbol  $\{\cdot, \cdot, \cdot\}$  denotes the graded symmetriser.

The level-zero generators are represented by a sum over single particle generators,

$$j_a = \sum_{k=1}^n j_{ka}. \quad (5.9)$$

The level-one generators are represented by the bilocal formula [38],

$$j_a^{(1)} = f_a^{cb} \sum_{k < k'} j_{kb} j_{k'c}. \quad (5.10)$$

Thus finally the full symmetry of the tree-level amplitudes can be rephrased as

$$y \mathcal{A}_n = 0, \quad (5.11)$$

for any  $y \in Y(psu(2, 2|4))$ .

It is particularly simple to describe the symmetry in terms of twistor variables. These variables will become especially relevant in the next section where we relate the symmetry to a conjectured formula for all leading singularities of planar  $\mathcal{N} = 4$  SYM amplitudes. In  $(2, 2)$  signature the twistor variables are simply related to the on-shell superspace variables  $(\lambda, \tilde{\lambda}, \eta)$  by a Fourier transformation  $\lambda \rightarrow \tilde{\mu}$ . Expressed in terms of the twistor space variables  $\mathcal{Z}^A = (\tilde{\mu}^\alpha, \tilde{\lambda}^{\dot{\alpha}}, \eta^A)$ , the level-zero and level-one generators of the Yangian symmetry assume a simple form

$$j^A_{\mathcal{B}} = \sum_i \mathcal{Z}_i^A \frac{\partial}{\partial \mathcal{Z}_i^{\mathcal{B}}}, \quad (5.12)$$

$$j^{(1)A}_{\mathcal{B}} = \sum_{i < j} (-1)^c \left[ \mathcal{Z}_i^A \frac{\partial}{\partial \mathcal{Z}_i^c} \mathcal{Z}_j^c \frac{\partial}{\partial \mathcal{Z}_j^{\mathcal{B}}} - (i, j) \right]. \quad (5.13)$$

Both of the formulas (5.12) and (5.13) are understood to have the supertrace proportional to  $(-1)^A \delta_{\mathcal{B}}^A$  removed<sup>5</sup>. In this representation the generators of superconformal symmetry are first-order operators while the level-one Yangian generators are second order.

In [39] it was demonstrated that there exists an alternative T-dual representation of the symmetry. The dual superconformal symmetries  $J_a$  which play the role of the level-zero generators, while some of the level-one generators are induced by the ordinary superconformal symmetries. In this case, the generators act on the function  $\mathcal{P}_n$ , where the MHV tree-level amplitude is factored out.

$$J_a \mathcal{P}_n = 0, \quad J_a^{(1)} \mathcal{P}_n = 0. \quad (5.14)$$

It is possible to rewrite the generators in the momentum (super)twistor representation defined in [40]  $\mathcal{W}_i^A = (\lambda_i^\alpha, \mu_i^{\dot{\alpha}}, \chi_i^A)$ . These variables are algebraically related to the on-shell superspace variables  $(\lambda, \tilde{\lambda}, \eta)$  via the introduction of dual coordinates (4.15) and are the twistors associated to this dual coordinate space,

$$\mu_i^{\dot{\alpha}} = x_i^{\alpha\dot{\alpha}} \lambda_{i\alpha}, \quad \chi_i^A = \theta_i^{\alpha A} \lambda_{i\alpha}. \quad (5.15)$$

<sup>5</sup>One removes the supertrace of an  $(m|m) \times (m|m)$  matrix  $M^A_{\mathcal{B}}$  by forming the combination  $M^A_{\mathcal{B}} - \frac{1}{2m} (-1)^{A+C} \delta_{\mathcal{B}}^A M^C_{\mathcal{C}}$ . In addition to the supertrace  $gl(m|m)$  also has a central element proportional to the identity  $\delta_{\mathcal{B}}^A$ . In the present context the trace of (5.12) vanishes due to the homogeneity conditions while (5.13) is traceless due to the antisymmetrisation in  $i$  and  $j$ .

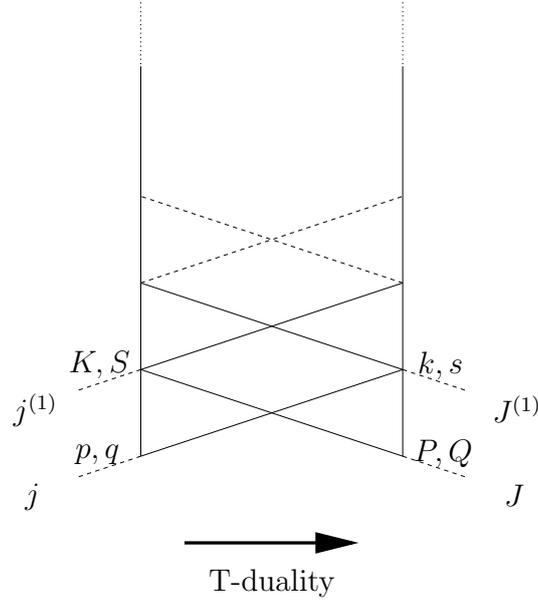

**Figure 4:** The tower of symmetries acting on scattering amplitudes in  $\mathcal{N} = 4$  super Yang-Mills theory. The original superconformal charges are denoted by  $j$  and the dual ones by  $J$ . Each can be thought of as the level-zero part of the Yangian  $Y(psu(2, 2|4))$ . The dual superconformal charges  $K$  and  $S$  form part of the level-one  $j^{(1)}$  while the original superconformal charges  $k$  and  $s$  form part of the level one charges  $J^{(1)}$ . In each representation the ‘negative’ level ( $P$  and  $Q$  or  $p$  and  $q$ ) is trivialised. T-duality maps  $j$  to  $J$  and  $j^{(1)}$  to  $J^{(1)}$ .

These variables linearise dual superconformal symmetry in complete analogy with the twistor variables  $\mathcal{Z}_i$  and the original superconformal symmetry,

$$J^A_{\mathcal{B}} = \sum_i \mathcal{W}_i^A \frac{\partial}{\partial \mathcal{W}_i^{\mathcal{B}}}. \quad (5.16)$$

The original conformal invariance of the amplitude  $k_{\alpha\dot{\alpha}}\mathcal{A}_n = 0$  induces a second-order operator which annihilates  $\mathcal{P}_n$ . When combined with the dual superconformal symmetry one finds that the following second-order operators annihilate  $\mathcal{P}_n$ ,

$$J^{(1)\mathcal{A}}_{\mathcal{B}} = \sum_{i < j} (-1)^c \left[ \mathcal{W}_i^{\mathcal{A}} \frac{\partial}{\partial \mathcal{W}_i^{\mathcal{C}}} \mathcal{W}_j^{\mathcal{C}} \frac{\partial}{\partial \mathcal{W}_j^{\mathcal{B}}} - (i, j) \right]. \quad (5.17)$$

As in the case of the original superconformal symmetry, both formulas (5.16) and (5.17) are understood to have the supertrace removed.

The operation we have performed is summarised in Fig. 4. A very similar picture also arises in considering the combined action of bosonic and fermionic T-duality in the AdS sigma model [41]. It can be thought of as the algebraic expression of T-duality in the perturbative regime of the theory.

Having described the symmetry of the theory, one might naturally ask how one can produce invariants. This question has been addressed in various papers [42, 39, 44]. It

turns out to be intimately connected to another conjecture about the leading singularities of the scattering amplitudes of  $\mathcal{N} = 4$  super Yang-Mills theory.

## 6 Grassmannian formulas

In [45] a remarkable formula was proposed which computes leading singularities of scattering amplitudes in  $\mathcal{N} = 4$  super Yang-Mills theory. The formula takes the form of an integral over the Grassmannian  $G(k, n)$ , the space of complex  $k$ -planes in  $\mathbb{C}^n$ . The integrand is a specific  $k(n - k)$ -form  $K$  to be integrated over cycles  $C$  of the corresponding dimension, with the integral being treated as a multi-dimensional contour integral. The result obtained depends on the choice of contour and is non-vanishing for closed contours because the form has poles located on certain hyperplanes in the Grassmannian,

$$\mathcal{L} = \int_C K. \quad (6.1)$$

The form  $K$  is constructed from a product of superconformally-invariant delta functions of linear combinations of twistor variables. It is through this factor that the integral depends on the kinematic data of the  $n$ -point scattering amplitude of the gauge theory. The delta functions are multiplied by a cyclically invariant function on the Grassmannian which has poles. Specifically the formula takes the following form in twistor space

$$\mathcal{L}_{\text{ACCK}}(\mathcal{Z}) = \int \frac{D^{k(n-k)}_c}{\mathcal{M}_1 \dots \mathcal{M}_n} \prod_{a=1}^k \delta^{4|4} \left( \sum_{i=1}^n c_{ai} \mathcal{Z}_i \right), \quad (6.2)$$

where the  $c_{ai}$  are complex parameters which are integrated choosing a specific contour. The form  $D^{k(n-k)}_c$  is the natural holomorphic globally  $gl(n)$ -invariant and locally  $sl(k)$ -invariant  $(k(n - k), 0)$ -form given explicitly in [46]. The denominator is the cyclic product of consecutive  $(k \times k)$  minors  $\mathcal{M}_p$  made from the columns  $p, \dots, p + k - 1$  of the  $(k \times n)$  matrix of the  $c_{ai}$

$$\mathcal{M}_p \equiv (p \ p + 1 \ p + 2 \ \dots \ p + k - 1). \quad (6.3)$$

As described in [45] the formula (6.2) has a  $GL(k)$  gauge symmetry which implies that  $k^2$  of the  $c_{ai}$  are gauge degrees of freedom and therefore should not be integrated over. The remaining  $k(n - k)$  are the true coordinates on the Grassmannian. This formula (6.2) produces leading singularities of  $N^{k-2}$ MHV scattering amplitudes when suitable closed integration contours are chosen. This fact was explicitly verified up to eight points in [45] and it was conjectured that the formula produces all possible leading singularities at all orders in the perturbative expansion.

The formula (6.2) has a T-dual version [46], expressed in terms of momentum twistors. The momentum twistor Grassmannian formula takes the same form as the original

$$\mathcal{L}_{\text{MS}}(\mathcal{W}) = \int \frac{D^{k(n-k)}_t}{\mathcal{M}_1 \dots \mathcal{M}_n} \prod_{a=1}^k \delta^{4|4} \left( \sum_{i=1}^n t_{ai} \mathcal{W}_i \right), \quad (6.4)$$

but now it is the dual superconformal symmetry that is manifest. The integration variables  $t_{ai}$  are again a  $(k \times n)$  matrix of complex parameters and we use the notation  $\mathcal{M}_p$

to refer to  $(k \times k)$  minors made from the matrix of the  $t_{ai}$ . The formula (6.4) produces the same objects as (6.2) but now with the MHV tree-level amplitude factored out. They therefore contribute to  $N^k$ MHV amplitudes.

The equivalence of the two formulations (6.2) and (6.4) was shown in [47] via a change of variables. Therefore, since each of the formulas has a different superconformal symmetry manifest, they both possess an invariance under the Yangian  $Y(\mathfrak{psl}(4|4))$ . The Yangian symmetry of these formulas was explicitly demonstrated in [39] by directly applying the Yangian level-one generators to the Grassmannian integral itself.

In [39] it was found that applying the level-one generator to the form  $K$  yields a total derivative,

$$J^{(1)\mathcal{A}}{}_{\mathcal{B}}K = d\Omega^{\mathcal{A}}{}_{\mathcal{B}}. \quad (6.5)$$

This property guarantees that  $\mathcal{L}$  is invariant for every choice of closed contour. Moreover it has been shown [44] that the form  $K$  is unique after imposing the condition (6.5). In this sense the Grassmannian integral is the most general form of Yangian invariant. Moreover, replacing  $\delta^{4|4} \rightarrow \delta^{m|m}$ , the formulas (6.2,6.4) are equally valid for generating invariants of the symmetry  $Y(\mathfrak{psl}(m|m))$  where one no longer has the interpretation of the symmetry as superconformal symmetry. Thus the Grassmannian integral formula is really naturally associated to the series of Yangians  $Y(\mathfrak{psl}(m|m))$ .

It is very striking that the leading singularities seem to be all given by Yangian invariants and even more striking that they seem to exhaust all such possibilities. The first of these statements follows from the analysis of leading singularities in [48, 49]. The second still requires rigorous proof but is consistent with all investigations so far conducted of leading singularities and residues in the Grassmannian. In some sense one can say that the leading singularity part of the amplitude is being determined by its symmetry. In fact the invariance of the leading singularities follows from the fact that the all-loop planar integrand is Yangian invariant up to a total derivative. This was shown by constructing it via a BCFW type recursion relation in a way which respects the Yangian symmetry [48].

It is not yet clear if the full Yangian invariance  $Y(\mathfrak{psl}(4|4))$  exhibits itself on the actual amplitudes themselves (i.e. after the loop integrations have been performed). As we have discussed the problem lies in the breakdown of the original (super)conformal symmetry. At one loop for MHV amplitudes (or Wilson loops) a  $Y(\mathfrak{sl}(2)) \oplus Y(\mathfrak{sl}(2))$  subalgebra of the full symmetry is present [50] for a special restricted two-dimensional kinematical setup [51]. It is possible to consider a particular finite, conformally invariant ratio of light-like Wilson loops, introduced in [52, 54] in order to understand the OPE properties of light-like Wilson loops. The conformal symmetry of this setup is  $\mathfrak{sl}(2) \oplus \mathfrak{sl}(2)$  and on the finite ratio the two commuting symmetries each extend to their Yangians in a natural way. This is equivalent to the effects of the original conformal symmetry in the two-dimensional kinematics. It remains to be seen to what extent this statement can be extended beyond the restricted kinematics and beyond one loop. Since the symmetry manifests itself as certain second-order differential equations it is possible that the differential equations found in [55] for certain momentum twistor loop integrals will be important in understanding whether this can be implemented. If the Yangian structure does manifest itself on all the loop corrections this would in some sense amount to the

integrability of the S-matrix of planar  $\mathcal{N} = 4$  super Yang-Mills theory.

## Acknowledgements

It is a pleasure to thank Livia Ferro, Johannes Henn, Gregory Korchemsky, Jan Plefka, Vladimir Smirnov and Emery Sokatchev for collaboration on the topics presented in this review.

## References

- [V.1] R. Roiban, “*Review of AdS/CFT Integrability, Chapter V.1: Scattering Amplitudes – Formalism, Recursion and Unitarity*”.
- [V.3] L. F. Alday, “*Review of AdS/CFT Integrability, Chapter V.3: Scattering Amplitudes at Strong Coupling*”.
- [VI.1] N. Beisert, “*Review of AdS/CFT Integrability, Chapter VI.1: Superconformal Algebra*”.
- [1] C. Anastasiou, Z. Bern, L. J. Dixon and D. A. Kosower, “*Planar amplitudes in maximally supersymmetric Yang-Mills theory*”, Phys. Rev. Lett. 91, 251602 (2003), hep-th/0309040.
- [2] Z. Bern, J. J. Carrasco, T. Dennen, Y.-t. Huang and H. Ita, “*Generalized Unitarity and Six-Dimensional Helicity*”, arxiv:1010.0494. • S. Caron-Huot and D. O’Connell, “*Spinor Helicity and Dual Conformal Symmetry in Ten Dimensions*”, arxiv:1010.5487. • T. Dennen and Y.-t. Huang, “*Dual Conformal Properties of Six-Dimensional Maximal Super Yang-Mills Amplitudes*”, arxiv:1010.5874.
- [3] R. Akhoury, “*MASS DIVERGENCES OF WIDE ANGLE SCATTERING AMPLITUDES*”, Phys. Rev. D19, 1250 (1979). • A. H. Mueller, “*ON THE ASYMPTOTIC BEHAVIOR OF THE SUDAKOV FORM-FACTOR*”, Phys. Rev. D20, 2037 (1979). • J. C. Collins, “*ALGORITHM TO COMPUTE CORRECTIONS TO THE SUDAKOV FORM-FACTOR*”, Phys. Rev. D22, 1478 (1980). • A. Sen, “*Asymptotic Behavior of the Sudakov Form-Factor in QCD*”, Phys. Rev. D24, 3281 (1981). • G. Sterman, “*Summation of Large Corrections to Short Distance Hadronic Cross-Sections*”, Nucl. Phys. B281, 310 (1987). • J. Botts and G. Sterman, “*Hard Elastic Scattering in QCD: Leading Behavior*”, Nucl. Phys. B325, 62 (1989). • S. Catani and L. Trentadue, “*Resummation of the QCD Perturbative Series for Hard Processes*”, Nucl. Phys. B327, 323 (1989).
- [4] Z. Bern, L. J. Dixon and V. A. Smirnov, “*Iteration of planar amplitudes in maximally supersymmetric Yang-Mills theory at three loops and beyond*”, Phys. Rev. D72, 085001 (2005), hep-th/0505205.
- [5] G. P. Korchemsky, “*SUDAKOV FORM-FACTOR IN QCD*”, Phys. Lett. B220, 629 (1989). • G. P. Korchemsky, “*DOUBLE LOGARITHMIC ASYMPTOTICS IN QCD*”, Phys. Lett. B217, 330 (1989). • L. Magnea and G. Sterman, “*Analytic continuation of the Sudakov form-factor in QCD*”,

- Phys. Rev. D42, 4222 (1990). • G. P. Korchemsky and G. Marchesini, “*Resummation of large infrared corrections using Wilson loops*”, Phys. Lett. B313, 433 (1993). • S. Catani, “*The singular behaviour of QCD amplitudes at two-loop order*”, Phys. Lett. B427, 161 (1998), hep-ph/9802439. • G. Sterman and M. E. Tejeda-Yeomans, “*Multi-loop amplitudes and resummation*”, Phys. Lett. B552, 48 (2003), hep-ph/0210130.
- [6] S. V. Ivanov, G. P. Korchemsky and A. V. Radyushkin, “*INFRARED ASYMPTOTICS OF PERTURBATIVE QCD: CONTOUR GAUGES*”, Yad. Fiz. 44, 230 (1986). • G. P. Korchemsky and G. Marchesini, “*Structure function for large  $x$  and renormalization of Wilson loop*”, Nucl. Phys. B406, 225 (1993), hep-ph/9210281.
- [7] F. Cachazo, M. Spradlin and A. Volovich, “*Iterative structure within the five-particle two-loop amplitude*”, Phys. Rev. D74, 045020 (2006), hep-th/0602228. • Z. Bern, M. Czakon, D. A. Kosower, R. Roiban and V. A. Smirnov, “*Two-loop iteration of five-point  $\mathcal{N} = 4$  super-Yang-Mills amplitudes*”, Phys. Rev. Lett. 97, 181601 (2006), hep-th/0604074.
- [8] J. M. Drummond, J. Henn, V. A. Smirnov and E. Sokatchev, “*Magic identities for conformal four-point integrals*”, JHEP 0701, 064 (2007), hep-th/0607160.
- [9] M. Spradlin, A. Volovich and C. Wen, “*Three-Loop Leading Singularities and BDS Ansatz for Five Particles*”, Phys. Rev. D78, 085025 (2008), arxiv:0808.1054.
- [10] I. A. Korchemskaya and G. P. Korchemsky, “*Evolution equation for gluon Regge trajectory*”, Phys. Lett. B387, 346 (1996), hep-ph/9607229.
- [11] L. F. Alday and J. M. Maldacena, “*Gluon scattering amplitudes at strong coupling*”, JHEP 0706, 064 (2007), arxiv:0705.0303.
- [12] J. M. Drummond, G. P. Korchemsky and E. Sokatchev, “*Conformal properties of four-gluon planar amplitudes and Wilson loops*”, Nucl. Phys. B795, 385 (2008), arxiv:0707.0243.
- [13] A. Brandhuber, P. Heslop and G. Travaglini, “*MHV Amplitudes in  $\mathcal{N} = 4$  Super Yang-Mills and Wilson Loops*”, Nucl. Phys. B794, 231 (2008), arxiv:0707.1153.
- [14] J. M. Drummond, J. Henn, G. P. Korchemsky and E. Sokatchev, “*On planar gluon amplitudes/Wilson loops duality*”, Nucl. Phys. B795, 52 (2008), arxiv:0709.2368.
- [15] J. M. Drummond, J. Henn, G. P. Korchemsky and E. Sokatchev, “*Conformal Ward identities for Wilson loops and a test of the duality with gluon amplitudes*”, arxiv:0712.1223.
- [16] J. M. Drummond, J. Henn, G. P. Korchemsky and E. Sokatchev, “*The hexagon Wilson loop and the BDS ansatz for the six-gluon amplitude*”, Phys. Lett. B662, 456 (2008), arxiv:0712.4138. • J. M. Drummond, J. Henn, G. P. Korchemsky and E. Sokatchev, “*Hexagon Wilson loop = six-gluon MHV amplitude*”, Nucl. Phys. B815, 142 (2009), arxiv:0803.1466.
- [17] Z. Bern, L. Dixon, D. Kosower, R. Roiban, M. Spradlin, C. Vergu and A. Volovich, “*The Two-Loop Six-Gluon MHV Amplitude in Maximally Supersymmetric Yang-Mills Theory*”, Phys. Rev. D78, 045007 (2008), arxiv:0803.1465.

- [18] Z. Bern, M. Czakon, L. J. Dixon, D. A. Kosower and V. A. Smirnov, “*The Four-Loop Planar Amplitude and Cusp Anomalous Dimension in Maximally Supersymmetric Yang-Mills Theory*”, Phys. Rev. D75, 085010 (2007), [hep-th/0610248](#).
- [19] V. Del Duca, C. Duhr and V. A. Smirnov, “*The Two-Loop Hexagon Wilson Loop in  $\mathcal{N} = 4$  SYM*”, [arxiv:1003.1702](#).
- [20] C. Anastasiou, A. Brandhuber, P. Heslop, V. V. Khoze, B. Spence and G. Travaglini, “*Two-Loop Polygon Wilson Loops in  $\mathcal{N} = 4$  SYM*”, JHEP 0905, 115 (2009), [arxiv:0902.2245](#).
- [21] C. Vergu, “*Higher point MHV amplitudes in  $\mathcal{N} = 4$  Supersymmetric Yang-Mills Theory*”, Phys. Rev. D79, 125005 (2009), [arxiv:0903.3526](#). • C. Vergu, “*The two-loop MHV amplitudes in  $\mathcal{N} = 4$  supersymmetric Yang-Mills theory*”, [arxiv:0908.2394](#).
- [22] L. Mason and D. Skinner, “*The Complete Planar S-matrix of  $\mathcal{N}=4$  SYM as a Wilson Loop in Twistor Space*”, JHEP 1012, 018 (2010), [arxiv:1009.2225](#). • S. Caron-Huot, “*Notes on the scattering amplitude / Wilson loop duality*”, [arxiv:1010.1167](#).
- [23] J. M. Drummond and J. M. Henn, “*All tree-level amplitudes in  $\mathcal{N} = 4$  SYM*”, JHEP 0904, 018 (2009), [arxiv:0808.2475](#).
- [24] A. Brandhuber, P. Heslop and G. Travaglini, “*A note on dual superconformal symmetry of the  $\mathcal{N} = 4$  super Yang-Mills S-matrix*”, Phys. Rev. D78, 125005 (2008), [arxiv:0807.4097](#).
- [25] N. Arkani-Hamed, F. Cachazo and J. Kaplan, “*What is the Simplest Quantum Field Theory?*”, [arxiv:0808.1446](#). • H. Elvang, D. Z. Freedman and M. Kiermaier, “*Recursion Relations, Generating Functions, and Unitarity Sums in  $\mathcal{N}=4$  SYM Theory*”, JHEP 0904, 009 (2009), [arxiv:0808.1720](#).
- [26] Z. Bern, J. J. M. Carrasco, H. Johansson and D. A. Kosower, “*Maximally supersymmetric planar Yang-Mills amplitudes at five loops*”, Phys. Rev. D76, 125020 (2007), [arxiv:0705.1864](#).
- [27] R. Britto, F. Cachazo and B. Feng, “*New Recursion Relations for Tree Amplitudes of Gluons*”, Nucl. Phys. B715, 499 (2005), [hep-th/0412308](#). • R. Britto, F. Cachazo, B. Feng and E. Witten, “*Direct Proof Of Tree-Level Recursion Relation In Yang- Mills Theory*”, Phys. Rev. Lett. 94, 181602 (2005), [hep-th/0501052](#).
- [28] E. Witten, “*Perturbative gauge theory as a string theory in twistor space*”, Commun. Math. Phys. 252, 189 (2004), [hep-th/0312171](#).
- [29] T. Bargheer, N. Beisert, W. Galleas, F. Loebbert and T. McLoughlin, “*Exacting  $\mathcal{N} = 4$  Superconformal Symmetry*”, [arxiv:0905.3738](#).
- [30] G. P. Korchemsky and E. Sokatchev, “*Symmetries and analytic properties of scattering amplitudes in  $\mathcal{N} = 4$  SYM theory*”, [arxiv:0906.1737](#). • A. Sever and P. Vieira, “*Symmetries of the  $\mathcal{N} = 4$  SYM S-matrix*”, [arxiv:0908.2437](#).
- [31] J. M. Drummond, J. Henn, G. P. Korchemsky and E. Sokatchev, “*Dual superconformal symmetry of scattering amplitudes in  $\mathcal{N} = 4$  super-Yang-Mills theory*”, [arxiv:0807.1095](#).
- [32] J. M. Drummond, J. Henn, G. P. Korchemsky and E. Sokatchev, “*Generalized unitarity for  $\mathcal{N} = 4$  super-amplitudes*”, [arxiv:0808.0491](#).

- [33] Z. Bern, L. J. Dixon and D. A. Kosower, “*All next-to-maximally helicity-violating one-loop gluon amplitudes in  $\mathcal{N} = 4$  super-Yang-Mills theory*”, Phys. Rev. D72, 045014 (2005), [hep-th/0412210](#).
- [34] A. Brandhuber, P. Heslop and G. Travaglini, “*Proof of the Dual Conformal Anomaly of One-Loop Amplitudes in  $\mathcal{N} = 4$  SYM*”, [arxiv:0906.3552](#).
- [35] L. F. Alday, J. M. Henn, J. Plefka and T. Schuster, “*Scattering into the fifth dimension of  $\mathcal{N} = 4$  super Yang-Mills*”, [arxiv:0908.0684](#).
- [36] N. Beisert, J. Henn, T. McLoughlin and J. Plefka, “*One-Loop Superconformal and Yangian Symmetries of Scattering Amplitudes in  $N=4$  Super Yang-Mills*”, JHEP 1004, 085 (2010), [arxiv:1002.1733](#).
- [37] J. M. Drummond, J. M. Henn and J. Plefka, “*Yangian symmetry of scattering amplitudes in  $\mathcal{N} = 4$  super Yang-Mills theory*”, JHEP 0905, 046 (2009), [arxiv:0902.2987](#).
- [38] L. Dolan, C. R. Nappi and E. Witten, “*A relation between approaches to integrability in superconformal Yang-Mills theory*”, JHEP 0310, 017 (2003), [hep-th/0308089](#). • L. Dolan, C. R. Nappi and E. Witten, “*Yangian symmetry in  $D=4$  superconformal Yang-Mills theory*”, [hep-th/0401243](#).
- [39] J. M. Drummond and L. Ferro, “*Yangians, Grassmannians and T-duality*”, [arxiv:1001.3348](#).
- [40] A. Hodges, “*Eliminating spurious poles from gauge-theoretic amplitudes*”, [arxiv:0905.1473](#).
- [41] N. Berkovits and J. Maldacena, “*Fermionic T-Duality, Dual Superconformal Symmetry, and the Amplitude/Wilson Loop Connection*”, JHEP 0809, 062 (2008), [arxiv:0807.3196](#). • N. Beisert, R. Ricci, A. A. Tseytlin and M. Wolf, “*Dual Superconformal Symmetry from  $AdS_5 \times S^5$  Superstring Integrability*”, Phys. Rev. D78, 126004 (2008), [arxiv:0807.3228](#). • N. Beisert, “*T-Duality, Dual Conformal Symmetry and Integrability for Strings on  $AdS_5 \times S^5$* ”, Fortschr. Phys. 57, 329 (2009), [arxiv:0903.0609](#).
- [42] G. P. Korchemsky and E. Sokatchev, “*Twistor transform of all tree amplitudes in  $\mathcal{N} = 4$  SYM theory*”, [arxiv:0907.4107](#).
- [43] J. M. Henn, S. G. Naculich, H. J. Schnitzer and M. Spradlin, “*Higgs-regularized three-loop four-gluon amplitude in  $N=4$  SYM: exponentiation and Regge limits*”, JHEP 1004, 038 (2010), [arxiv:1001.1358](#).
- [44] J. M. Drummond and L. Ferro, “*The Yangian origin of the Grassmannian integral*”, [arxiv:1002.4622](#). • G. P. Korchemsky and E. Sokatchev, “*Superconformal invariants for scattering amplitudes in  $N=4$  SYM theory*”, [arxiv:1002.4625](#).
- [45] N. Arkani-Hamed, F. Cachazo, C. Cheung and J. Kaplan, “*A Duality For The S Matrix*”, [arxiv:0907.5418](#).
- [46] L. Mason and D. Skinner, “*Dual Superconformal Invariance, Momentum Twistors and Grassmannians*”, [arxiv:0909.0250](#).
- [47] N. Arkani-Hamed, F. Cachazo and C. Cheung, “*The Grassmannian Origin Of Dual Superconformal Invariance*”, JHEP 1003, 036 (2010), [arxiv:0909.0483](#).

- [48] N. Arkani-Hamed, J. L. Bourjaily, F. Cachazo, S. Caron-Huot and J. Trnka, “*The All-Loop Integrand For Scattering Amplitudes in Planar  $N=4$  SYM*”, arxiv:1008.2958.
- [49] J. M. Drummond and J. M. Henn, “*Simple loop integrals and amplitudes in  $N=4$  SYM*”, arxiv:1008.2965.
- [50] J. M. Drummond, L. Ferro and E. Ragoucy, “*Yangian symmetry of light-like Wilson loops*”, arxiv:1011.4264.
- [51] L. F. Alday and J. Maldacena, “*Null polygonal Wilson loops and minimal surfaces in Anti-de-Sitter space*”, arxiv:0904.0663.
- [52] L. F. Alday, D. Gaiotto, J. Maldacena, A. Sever and P. Vieira, “*An Operator Product Expansion for Polygonal null Wilson Loops*”, arxiv:1006.2788.
- [53] R. H. Boels, “*No triangles on the moduli space of maximally supersymmetric gauge theory*”, JHEP 1005, 046 (2010), arxiv:1003.2989.
- [54] D. Gaiotto, J. Maldacena, A. Sever and P. Vieira, “*Bootstrapping Null Polygon Wilson Loops*”, arxiv:1010.5009.
- [55] J. M. Drummond, J. M. Henn and J. Trnka, “*New differential equations for on-shell loop integrals*”, arxiv:1010.3679.
- [56] J. M. Henn, S. G. Naculich, H. J. Schnitzer and M. Spradlin, “*More loops and legs in Higgs-regulated  $N=4$  SYM amplitudes*”, JHEP 1008, 002 (2010), arxiv:1004.5381.



# Review of AdS/CFT Integrability, Chapter V.3: Scattering Amplitudes at Strong Coupling

LUIS F. ALDAY

*Mathematical Institute, University of Oxford  
24–29 St. Giles', Oxford OX1 3LB, UK.*

*School of Natural Sciences, Institute for Advanced Study,  
Princeton, NJ 08540, USA*

alday@maths.ox.ac.uk

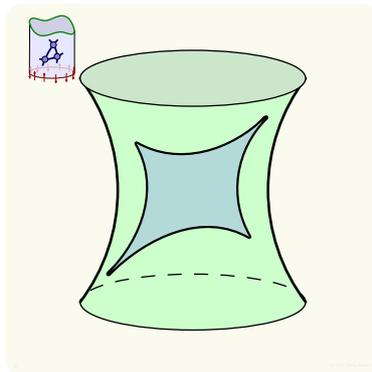

**Abstract:** We review the computation of scattering amplitudes of planar maximally super-symmetric Yang-Mills at strong coupling. By using the *AdS/CFT* duality the problem boils down to the computation of the area of certain minimal surfaces on *AdS*. The integrability of the model can then be efficiently used in order to give an answer for the problem in terms of a set of integral equations.

## 1 Introduction

The aim of this review is to study gluon scattering amplitudes of four dimensional planar maximally super-symmetric Yang-Mills (MSYM). We hope that the study of such amplitudes would teach us something about scattering amplitudes of QCD, but at the same time they are much more tractable. The reason for such tractability is twofold. On one hand, perturbative computations are much simpler than in QCD, due to the high degree of symmetry. In fact enormous progress has been made in the last few years. On the other hand, the strong coupling regime of the theory can be studied by means of the AdS/CFT duality, by studying a weakly coupled string sigma-model.

In this review we focus on how to use the AdS/CFT duality in order to compute gluon scattering amplitudes of planar MSYM at strong coupling, referring the reader to [V.1, V.2] for details on the perturbative side of the computation. In section two we set up the problem of computing scattering amplitudes at strong coupling. The problem boils down to the computation of the area of certain minimal surfaces in  $AdS$ . For the particular case of four gluons, such surface, and its area, can be explicitly computed. Furthermore, the strong coupling computation hints at some symmetries that actually appear to be symmetries at all values of the coupling. This is briefly reviewed at the end of section two. In section three we focus on the mathematical problem of computing the area of minimal surfaces in  $AdS$ . The integrability of the model allows the introduction of a spectral parameter. By studying the problem as a function of the spectral parameter we are able to give a solution in the form of a set of integral equations. These equations have the precise form of thermodynamic Bethe ansatz (TBA) equations. The area turns out to coincide with the free energy of such TBA system. Finally, In section four, we end up with some conclusions and a list of open problems.

## 2 Gluon scattering amplitudes at strong coupling

Four dimensional MSYM, the theory whose amplitudes we want to consider, turns out to be dual to type IIB string theory on  $AdS_5 \times S^5$ . This duality receives the name of *AdS/CFT* duality [1] and is the main focus of this review. A remarkable feature of this duality is that it allows to compute certain observables of MSYM at strong coupling by doing geometrical computations on  $AdS$ . A well known example is the computation of the expectation value of super-symmetric Wilson loops, which reduces to a minimal area problem [2]. In this section we will show that this is also the case for the computation of scattering amplitudes at strong coupling! <sup>1</sup>

As in the gauge theory, we will need to introduce a regulator in order to define properly scattering amplitudes. In order to set-up our computation we introduce a D-brane as IR regulator, as we explain in detail below. Another convenient regulator is the strong coupling/super-gravity analog of dimensional regularization. This regulator will be used in order to compare our results with expectations from the perturbative side.

---

<sup>1</sup>In this section, we follow closely [3], to which we refer the reader for the details.

## 2.1 Set-up of the computation

In order to set up the computation at strong coupling, it is convenient to introduce a regularization as follows. We start from a  $U(N+k)$  theory, with  $k \ll N$ , and then consider a vacuum breaking the symmetry to  $U(N) \times U(k)$  by giving to a scalar field a vacuum expectation value  $m_{IR}$  which plays the role of an infrared cut-off.<sup>2</sup> When we take the 't Hooft limit we keep  $k$  fixed, so that the low energy  $U(k)$  theory becomes free. We then scatter gluons of this  $U(k)$  theory. We are interested in the regime where all kinematic invariants are much larger than the IR cut-off,  $s_{ij} \gg m_{IR}^2$ . It turns out that the leading exponential behavior at strong coupling can be captured simply by considering  $k=1$ . At strong coupling this corresponds to consider a  $D3$ -brane localized in the radial direction. More precisely, we start with the  $AdS_5$  metric written in Poincare coordinates

$$ds^2 = R^2 \frac{dx_{3+1}^2 + dz^2}{z^2} \quad (2.1)$$

and place a  $D3$ -brane at some fixed large value of  $z = z_{IR}$  and extending along the  $x_{3+1}$  coordinates. The asymptotic states are open strings that end on that D-brane. We then consider the scattering of these open strings, that will have the interpretation of the gluons that we are scattering.

The proper momentum of the strings is  $k_{pr} = kz_{IR}/R$ , where  $k$  is the momentum conjugate to  $x_{3+1}$ , plays the role of gauge theory momentum and will be kept fixed as we take away the IR cut-off,  $z_{IR} \rightarrow \infty$ . Therefore, due to the warping of the metric, the proper momentum is very large, so we are considering the scattering of strings at fixed angle and with very large momentum.

Amplitudes in such regime were studied in flat space by Gross and Mende [5]. The key feature of their computation is that the amplitude is dominated by a saddle point of the classical action. In our case we need to consider classical strings on  $AdS$ . Hence, we need to consider a world-sheet with the topology of a disk with vertex operator insertions on its boundary, which correspond to the external states (see fig. 1). A disk amplitude with a fixed ordering of the open string vertex operators corresponds to a given color ordered amplitude.

What are the boundary conditions for such world-sheet? since the open strings are attached to the D-brane,  $z = z_{IR}$  at the boundary. Furthermore, in the vicinity of a vertex operator, the momentum of the external state should fix the form of the solution.

In order to state more simply the boundary conditions for the world-sheet, it is convenient to describe the solution in terms of T-dual coordinates  $y^\mu$ , defined as follows

$$ds^2 = w^2(z) dx_\mu dx^\mu + \dots \quad \rightarrow \quad \partial_\alpha y^\mu = iw^2(z) \epsilon_{\alpha\beta} \partial_\beta x^\mu \quad (2.2)$$

The presence of the  $i$  is due to the fact that we are considering a Euclidean world-sheet in Minkowski space-time. Note that we do not T-dualize along the radial direction. After defining  $r = R^2/z$  the dual metric takes the form

$$ds^2 = R^2 \frac{dy_\mu dy^\mu + dr^2}{r^2} \quad (2.3)$$

---

<sup>2</sup>See [4] for perturbative computations using this regulator.

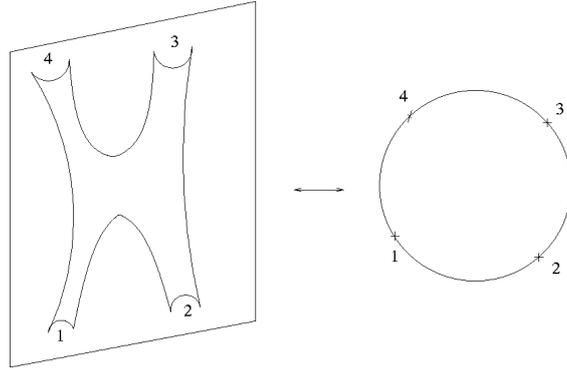

**Figure 1:** World-sheet corresponding to the scattering of four open strings. In the figure on the left we see four open strings ending on the IR D-brane, the world-sheet has then the topology of a disk, shown on the right, with four vertex operator insertions.

Note that this metric is equivalent to the same  $AdS_5$  metric we started with! A crucial difference is that now, in terms of the dual coordinates, the boundary of the world-sheet is located at  $r = R^2/z_{IR}$ , which is very small. Furthermore, the  $T$ -duality we performed interchanges Neumann by Dirichlet boundary conditions. This means that the boundary of the world-sheet sits at a fixed point in the space of the dual coordinates. When a vertex operator with momentum  $k^\mu$  is inserted, the location of such point gets shifted by an amount proportional to  $\Delta y^\mu = 2\pi k^\mu$ .

Summarizing, the boundary of the world-sheet is located at  $r = R^2/z_{IR}$  and is a particular line constructed as follows

- For each particle of momentum  $k^\mu$ , draw a segment joining two points separated by  $\Delta y^\mu = 2\pi k^\mu$ .
- Concatenate the segments according to the insertions on the disk.

Since gluons are massless, the segments are light-like. Furthermore, due to momentum conservation, the segments form a closed polygon. The world-sheet, when expressed in T-dual coordinates, will then end in such sequence of light-like segments (see fig. 2) located at  $r = R^2/z_{IR}$ .

As we take away the IR cut-off,  $z_{IR} \rightarrow \infty$ , the boundary of the world-sheet moves towards the boundary of the T-dual metric, at  $r = 0$ . This computation would then be formally equivalent to the computation of the expectation value of a Wilson loop given by a sequence of light-like segments at strong coupling [2].<sup>3</sup>

Our prescription is that the leading exponential behavior of the  $N$ -point scattering amplitude is given by the area  $A$  of the minimal surface that ends on a sequence of light-like segments on the boundary

$$\mathcal{A}_N \sim e^{-\frac{\sqrt{\lambda}}{2\pi} A(k_1, \dots, k_N)} \quad (2.4)$$

<sup>3</sup>As explained in detail in [V.2], this remarkable duality between Wilson loops and scattering amplitudes was also observed in perturbative computations.

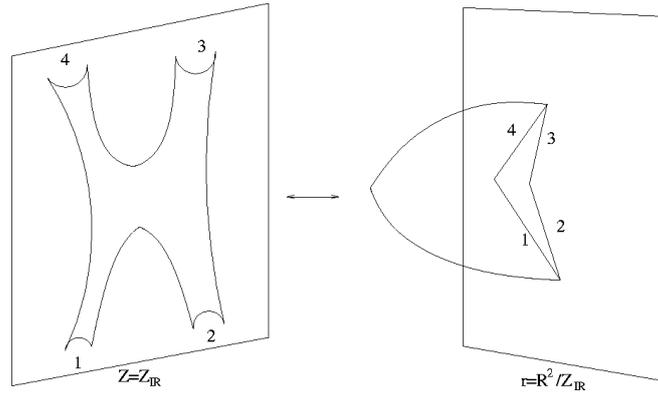

**Figure 2:** Comparison of the world sheet in original and T-dual coordinates. The hyperplane on the picture to the right should not be interpreted as a D-brane, but rather as a radial slice where the boundary of the world-sheet it located.

An important comment is in order. Note that the strong coupling computation is blind to the type or polarization of the external particles. Such information will contribute to prefactors in (2.4) and will be subleading in a  $1/\sqrt{\lambda}$  expansion, relative to the leading exponential term<sup>4</sup>. These differences should be visible once we consider quantum corrections to the classical area. This is still an open problem.

Some generalizations to the above picture were developed. In [7] finite temperature was introduced while in [8] the authors considered solutions with non trivial motion on the  $S^5$ . Finally, in [9], the scattering of quarks at strong coupling was considered. Unfortunately, due to space limitations, we wont discuss these interesting developments here, but refer the reader to the original literature.

We have then reduced the problem of computing scattering amplitudes at strong coupling to the problem of finding minimal surfaces in  $AdS$ . In the following we will show that such surface can be found for the particular case of the scattering of four gluons. To find and understand this solution in detail will be quite instructive. Then, in the next section, we will use the integrability of the problem in order to give a general solution, for any number of gluons, in the form of a set of integral equations.

## 2.2 Scattering of four gluons

Consider the scattering of two particles into two particles,  $k_1 + k_3 \rightarrow k_2 + k_4$  and define the usual Mandelstam variables

$$s = -(k_1 + k_2)^2, \quad t = -(k_2 + k_3)^2 \quad (2.5)$$

According to our prescription we need to find the minimal surface ending in the following light-like polygon

In order to write the Nambu-Goto action it is convenient to use Poincare coordinates  $(r, y_0, y_1, y_2)$ , setting  $y_3 = 0$  and parametrize the surface by its projection to the  $(y_1, y_2)$

<sup>4</sup>As discussed in more detail in [6], when computing the disk amplitude in the saddle point approximation, one can neglect the polarization of the gluon vertex operators.

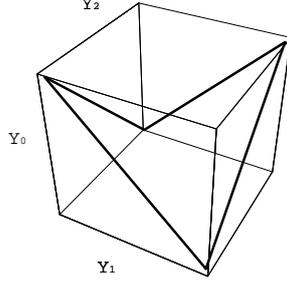

**Figure 3:** Polygon corresponding to the scattering of four gluons

plane. In this case we obtain an action for two fields,  $r$  and  $t$ , living in the space parametrized by  $y_1$  and  $y_2$

$$S = \frac{R^2}{2\pi} \int dy_1 dy_2 \frac{\sqrt{1 + (\partial_i r)^2 - (\partial_i y_0)^2 - (\partial_1 r \partial_2 y_0 - \partial_2 r \partial_1 y_0)^2}}{r^2} \quad (2.6)$$

where  $r = r(y_1, y_2)$  and  $\partial_i r = \partial_{y_i} r$ , etc. Our aim is to find a solution to the classical equations of motion with the appropriate boundary conditions. Let us consider first the case  $s = t$ , where the projection of the polygon lines to the  $(y_1, y_2)$  plane is a square. By scale invariance we can choose the edges of the square to lie at  $y_1, y_2 = \pm 1$ . The boundary conditions are then given by

$$r(\pm 1, y_2) = r(y_1, \pm 1) = 0, \quad y_0(\pm 1, y_2) = \pm y_2, \quad y_0(y_1, \pm 1) = \pm y_1 \quad (2.7)$$

In [10] the solution corresponding to a single cusp was considered. One can make educated guesses using such solution as a guidance and propose

$$y_0(y_1, y_2) = y_1 y_2, \quad r(y_1, y_2) = \sqrt{(1 - y_1^2)(1 - y_2^2)} \quad (2.8)$$

Remarkably this turns out to be a solution of the equations of motion! This is the solution for the case  $s = t$ , how can we obtain the most general solution?

The dual  $AdS_5$  space has a  $SO(2, 4)$  group of isometries. This symmetry is sometimes referred to as "dual conformal symmetry" and should not be confused with the original  $SO(2, 4)$  symmetry associated to the original  $AdS$  space. This dual symmetry can be used in order to map the particular solution we have just found to the most general solution with four edges, in particular with  $s \neq t$ . The general solution can be conveniently written as

$$r = \frac{a}{\cosh u_1 \cosh u_2 + b \sinh u_1 \sinh u_2}, \quad y_0 = \frac{a \sqrt{1 + b^2} \sinh u_1 \sinh u_2}{\cosh u_1 \cosh u_2 + b \sinh u_1 \sinh u_2} \quad (2.9)$$

$$y_1 = \frac{a \sinh u_1 \cosh u_2}{\cosh u_1 \cosh u_2 + b \sinh u_1 \sinh u_2}, \quad y_2 = \frac{a \cosh u_1 \sinh u_2}{\cosh u_1 \cosh u_2 + b \sinh u_1 \sinh u_2} \quad (2.10)$$

where  $u_{1,2}$  parametrize the world-sheet and we have written the surface as a solution to the equations of motion in conformal gauge.  $a$  and  $b$  encode the kinematical information of the scattering as follows

$$-s(2\pi)^2 = \frac{8a^2}{(1-b)^2}, \quad -t(2\pi)^2 = \frac{8a^2}{(1+b)^2}, \quad \frac{s}{t} = \frac{(1+b)^2}{(1-b)^2} \quad (2.11)$$

According to the prescription, we should now plug the classical solution into the classical action to compute the area and obtain the four point scattering amplitude at strong coupling. However, in doing so, we obtain a divergent answer. That is of course the case, since we have taken the IR regulator away. In order to obtain a finite answer we need to reintroduce a regulator. Since we want to compare our results to field theory expectations, it is convenient to introduce the strong coupling analog of dimensional regularization.

Gauge theory amplitudes are regularized by considering the theory in  $D = 4 - 2\epsilon$  dimensions. More precisely, one starts with  $\mathcal{N} = 1$  in ten dimensions and then dimensionally reduce to  $4 - 2\epsilon$  dimensions. For integer  $2\epsilon$  this is precisely the low energy theory living on a  $Dp$ -brane, where  $p = 3 - 2\epsilon$ . We regularize the amplitudes at strong coupling by considering the gravity dual of these theories and then analytically continuing in  $\epsilon$ . The string frame metric is

$$ds^2 = f^{-1/2} dx_{4-2\epsilon}^2 + f^{1/2} [dr^2 + r^2 d\Omega_{5+2\epsilon}^2], \quad f = (4\pi^2 e^\gamma)^\epsilon \Gamma(2 + \epsilon) \mu^{2\epsilon} \frac{\lambda}{r^{4+2\epsilon}} \quad (2.12)$$

Following the steps described above, we are led to the following action

$$S = \frac{\sqrt{c_\epsilon \lambda} \mu^\epsilon}{2\pi} \int \frac{\mathcal{L}_{\epsilon=0}}{r^\epsilon} \quad (2.13)$$

Where  $\mathcal{L}_{\epsilon=0}$  is the Lagrangian density for  $AdS_5$ . The presence of the factor  $r^\epsilon$  will have two important effects. On one hand, previously divergent integrals will now converge (if  $\epsilon < 0$ ). On the other hand, the equations of motion will now depend on  $\epsilon$  and we were not able to compute the full solution for arbitrary  $\epsilon$ . However, we are interested in computing the amplitude only up to finite terms as we take  $\epsilon \rightarrow 0$ . In that case, it turns out to be sufficient to plug the original solution into the  $\epsilon$ -deformed action<sup>5</sup>. After performing the integrals and expanding in powers of  $\epsilon$  we get the final answer

$$\begin{aligned} \mathcal{A} = e^{-\frac{\sqrt{\lambda}}{2\pi} A}, \quad , -\frac{\sqrt{\lambda}}{2\pi} A = iS_{div} + \frac{\sqrt{\lambda}}{8\pi} \left( \log \frac{s}{t} \right)^2 + \tilde{C} \\ S_{div} = 2S_{div,s} + 2S_{div,t} \\ iS_{div,s} = -\frac{1}{\epsilon^2} \frac{1}{2\pi} \sqrt{\frac{\lambda \mu^{2\epsilon}}{(-s)^\epsilon}} - \frac{1}{\epsilon} \frac{1}{4\pi} (1 - \log 2) \sqrt{\frac{\lambda \mu^{2\epsilon}}{(-s)^\epsilon}} \end{aligned} \quad (2.14)$$

This answer has the correct general structure (see *e.g.* [V.1, V.2]) from field theory expectations. Furthermore, once we use the strong coupling behavior for the cusp anomalous dimension [11],  $f(\lambda) = \frac{\sqrt{\lambda}}{\pi} + \dots$  we see that the leading divergence, as well as the finite piece, have not only the correct kinematical dependence but also the correct overall coefficient in order to match the BDS ansatz [V.2, 12]. As we will see shortly, this result is actually a consequence of the symmetries of the problem!

<sup>5</sup>Up to a contribution from the regions close to the cusps that adds an unimportant additional constant term.

## 2.3 $T$ -duality and dual conformal symmetry at strong coupling

An important ingredient of the previous computation was the existence of a dual  $SO(2, 4)$  symmetry <sup>6</sup>, associated to the isometry group of the dual  $AdS_5$  space. This symmetry allowed the construction of new solutions and fixed somehow the finite piece of the scattering amplitude. <sup>7</sup>

To a symmetry we associate a Ward identity and in particular dual conformal symmetry will impose some constraints on the amplitudes. Quite remarkably, this duality was also (actually before!) observed at weak coupling and is by now believed to be a duality of scattering amplitudes at all values of the coupling. You can see [V.2] for a detailed account of this symmetry and the constraints it imposes on the amplitudes.<sup>8</sup> Here we will just mention that dual conformal symmetry fixes the answer for the four-point function to have the form (2.14), actually, to all values of the coupling! and hence its agreement with the BDS ansatz. Furthermore, dual conformal symmetry does not fix the answer for the scattering of more than six gluons, hence, in general, the answer deviates from the BDS ansatz. The need for such a deviation, usually called remainder function, was established in [15, 16]. See [V.2] for more details.

In the last section we have seen that existence of a dual  $AdS$  space, is related to the fact that  $AdS_5$  goes to itself after a sequence of four  $T$ -dualities, followed by the inversion of the radial coordinate, see (2.1) vs (2.3). This set of  $T$ -dualities, however, does not leave the full  $AdS_5 \times S^5$  sigma model invariant. For instance, Buscher rules for  $T$ -dualities [17] imply a shift on the dilaton of the form

$$\phi \rightarrow \phi + 4 \times \log z \quad (2.15)$$

where  $z$  is the radial coordinate of the original metric (2.1). The factor of 4 is due to the fact that we are making four  $T$ -dualities. In addition to the usual, "bosonic",  $T$ -dualities, one can introduce a fermionic  $T$ -duality [18]. This duality is a non local redefinition of the fermionic world-sheet fields, very much like the bosonic  $T$ -duality is a redefinition of the bosonic fields. These  $T$ -dualities change the fields of the sigma model according to precise rules. For instance, each fermionic  $T$ -duality shifts the dilaton by an amount

$$\phi \rightarrow \phi - \frac{1}{2} \times \log z \quad (2.16)$$

We see that by doing eight fermionic  $T$ -dualities we can undo the shift (2.15) on the dilaton. Actually, one can check that a combination of the four bosonic  $T$ -dualities plus eight fermionic  $T$ -dualities maps the full sigma model to itself! Note also that

---

<sup>6</sup>Actually, this symmetry was first noticed in perturbative computations [13] and then independently in the strong coupling computation described here.

<sup>7</sup>Naively, this conformal symmetry would imply that the amplitude is independent of  $s$  and  $t$ , since they can be sent to arbitrary values by a dual conformal transformation. The whole dependence on  $s$  and  $t$  arises due to the necessity of introducing an IR regulator. However after keeping track of the dependence on the IR regulator, the amplitude is still determined by the dual conformal symmetry. Hence, this regulator breaks the dual conformal symmetry, but in a controlled way!

<sup>8</sup>These constraints have also been derived at strong coupling [14].

this argument does not depend on the value of the coupling. One of the implications is that the dual model has the same conformal symmetry group as the original, helping to understand the origin of dual conformal symmetry. Actually, as the construction suggests, dual conformal symmetry extends to a full dual super conformal symmetry. In addition, one has a map between the full set of conserved charges of the two models, in such a way that some of the local charge of one model are mapped to non local charges of the dual model, and viceversa, see for instance [18].

The structure of dual super conformal symmetry was also seen at weak coupling and is explained in detail in [V.2], for which we refer the reader for more details.

### 3 Minimal surfaces on $AdS$

In the previous section we have seen how the problem of computing gluon scattering amplitudes at strong coupling reduces to the computation of the area of certain minimal surfaces in  $AdS$ . In this section we show how the integrability of the system can be used in order to give a solution to the problem, in the form of a set of integral equations. We will follow closely [19–21], see also [22], to which we refer the readers for the details.<sup>9</sup> For this review, we will focus mostly on a particular kinematic configuration, in which the minimal surfaces are actually embedded into an  $AdS_3$  subspace of the full  $AdS_5$ . However, the full problem has been solved and it will be briefly mentioned at the end of the section.

The mathematical problem is to find the area of the minimal surface ending on the boundary of  $AdS$  at a given polygon of light-like edges. The polygon is parametrized by the location of its cusps  $x_i$ , which are null separated, namely  $x_{i,i+1}^2 = 0$ .

We will focus on certain regularized area that is invariant under conformal transformations. As such, it will depend only on cross-ratios, of the form  $\chi_{ijkl} = \frac{x_{ij}^2 x_{kl}^2}{x_{ik}^2 x_{jl}^2}$ . Given the cross-ratios, we want to compute the area as a function of those. The full problem involves minimal surfaces on  $AdS_5$ , in which case there are  $3N - 15$  independent cross-ratios, where  $N$  is the number of cusps/gluons. We will restrict to special kinematical configurations in which the minimal surfaces involved are embedded in  $AdS_3$ . In this case, we have  $N - 6$  independent cross-ratios<sup>10</sup> and the polygon is a zig-zaged polygon living in one plus one dimensions, which correspond to the boundary of  $AdS_3$ , see figure 4.

Since we want a closed contour, and we are in  $1 + 1$  dimensions, we can consider only polygons with an even number of sides, hence  $N = 2n$ . As one can see in figure 4, the contour is parametrized by  $n$  coordinates  $x_i^+$  and  $n$  coordinates  $x_i^-$ . With each set of coordinates we can form  $n - 3$  invariant cross-ratios, of the form  $\chi_{ijkl}^\pm = \frac{x_{ij}^\pm x_{kl}^\pm}{x_{ik}^\pm x_{jl}^\pm}$ .

<sup>9</sup>Some of the key ideas used below may be found in relation to the study of wall crossing [23]. Actually, the method of the first paper in [23] where instrumental in deriving the expression for the eight gluon amplitude at strong coupling in [19].

<sup>10</sup>For the general scattering in four dimensions we have  $4N$  coordinates, minus  $N$ , since the distance between consecutive points has to be light-like, minus 15, that is the dimension of the conformal group  $SO(2, 4)$ . In the case of  $AdS_3$ , we have  $2N - N$  minus 6, which is the dimension of  $SO(2, 2)$ .

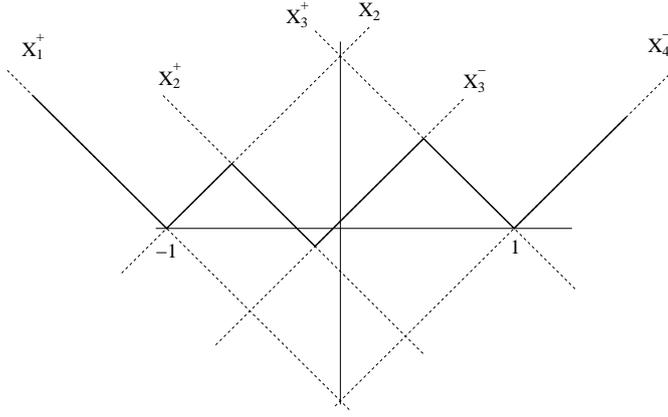

**Figure 4:** A zig-zaged null polygon in 1 + 1 dimensions is parametrized by  $n x_i^+$  coordinates and  $n x_i^-$  coordinates. If you want a closed polygon, you can fold the figure in a cylinder.

In order to consider minimal surfaces in  $AdS_3$  we need to consider the world-sheet of classical strings on  $AdS_3$ . This is the subject of the following subsection.

### 3.1 Strings on $AdS_3$

Classical strings on  $AdS_3$  can be described in terms of embedding coordinates, where  $AdS_3$  is the following surface embedded in  $R^{2,2}$

$$Y \cdot Y \equiv -Y_{-1}^2 - Y_0^2 + Y_1^2 + Y_2^2 = -1 \quad (3.1)$$

we take the world-sheet to be the whole complex plane. Since we are interested in classical solutions, the fields have to satisfy the conformal gauge equations of motion and the Virasoro constraints

$$\partial \bar{\partial} Y - (\partial Y \cdot \bar{\partial} Y) Y = 0, \quad \partial Y \cdot \partial Y = \bar{\partial} Y \cdot \bar{\partial} Y = 0 \quad (3.2)$$

where  $\partial Y = \partial_z Y$ , etc. An efficient way to focus only in the physical degrees of freedom, similar to fixing light-cone gauge, is by performing the so-called Pohlmeyer kind of reduction, see for instance [24], and consider the "reduced" fields

$$\alpha = \log \partial Y \cdot \bar{\partial} Y, \quad p^2 = \partial^2 Y \cdot \partial^2 Y \quad (3.3)$$

As a consequence of the equations of motion and Virasoro constraints,  $p$  can be seen to be a holomorphic function,  $p = p(z)$  while  $\alpha(z, \bar{z})$  can be seen to satisfy a generalized version of the Sinh-Gordon equation

$$\partial \bar{\partial} \alpha - e^\alpha + p(z) \bar{p}(\bar{z}) e^{-\alpha} = 0 \quad (3.4)$$

From the definition of the reduced fields, it is clear that they are invariant under space-time conformal transformation. This means that they describe only the essential part of the problem, without redundancies.

Before proceeding, let us make the following remark. Since  $p(z)$  is a holomorphic function, it is possible to make a change of coordinates from the  $z$ -plane to the  $w$ -plane, where  $dw = \sqrt{p(z)}dz$ . In the  $w$ -plane, after a simple field redefinition, the generalized Sinh-Gordon equation takes the usual form

$$\alpha = \hat{\alpha} + \frac{1}{2} \log p\bar{p} \rightarrow \partial_w \bar{\partial}_w \hat{\alpha} = 2 \sinh \hat{\alpha} \quad (3.5)$$

It would seem that we got rid of all the information on  $p(z)$ . However, this is not the case, since the  $w$ -plane will have in general a complicated structure (for instance, it will have a branch cuts, etc, depending on  $p(z)$ ). So, we can choose between a complicated equation on the complex plane, or a simple equation on a more complicated space. Depending which questions we want to answer, one description may be more convenient than another. Finally, we are interested in the area of the classical World-sheet. Written in terms of the reduced fields it becomes

$$\mathcal{A} = \int e^\alpha d^2 z = \int e^{\hat{\alpha}} d^2 w \quad (3.6)$$

### 3.2 Classical solutions corresponding to minimal surfaces ending on null polygons

What are the properties of the holomorphic function  $p(z)$  and  $\alpha(z, \bar{z})$  for solutions corresponding to minimal surfaces ending on null polygons? In order to answer this question we can start by considering the four cusps solution found in the previous section and perform the Pohlmeyer reduction. We find

$$p(z) = 1, \quad \alpha = \hat{\alpha} = 0 \quad (3.7)$$

Hence, the four cusps solution simply correspond to the vacuum solution of the Sinh-Gordon equation! What about solutions with a higher number of cusps? First of all we propose that the field  $\alpha$  is regular everywhere, since we are looking for smooth space-like solutions. Second, we expect a general solution to be similar to the four cusps solution when approaching the boundary, so we expect that  $\hat{\alpha} \rightarrow 0$  as  $|z|$  becomes large.

Finally, if we are interested on a minimal surface ending on a polygon with  $2n$  cusps, we propose  $p(z)$  to be a polynomial of degree  $n - 2$ <sup>11</sup>

$$p(z) = z^{n-2} + c_{n-4}z^{n-4} + \dots + c_1z + c_0 \quad (3.8)$$

we have used rescalings and translations in order to set the coefficients of  $z^{n-2}$  and  $z^{n-3}$  to one and zero respectively. Such polynomial contains  $n - 3$  complex coefficients, or  $2n - 6$  real coefficients, which exactly agrees with the amount of expected independent cross ratios for a polygon with  $2n$  cusps!

Summarizing: minimal surfaces ending on a light-like polygon with  $2n$  cusps correspond to a holomorphic polynomial of degree  $n - 2$  and a field  $\hat{\alpha}$  satisfying the Sinh-Gordon equations and with boundary conditions such that it decays at infinity and

<sup>11</sup>The motivation for this proposal, comes from the fact that an homogeneous polynomial of degree  $n - 2$  possesses all the symmetries to correspond to a symmetric polygon of  $n$  edges.

diverges logarithmically at the zeroes of  $p(z)$ , which amounts to say that  $\alpha$  is regular everywhere.

Since  $\hat{\alpha}$  decays at infinity, the integral defining the area (3.6) diverges. We define a regularized area by subtracting the behavior at infinity

$$A_{reg} = \int (e^{\hat{\alpha}} - 1) d^2w \quad (3.9)$$

As the reduced fields are invariant under space-time conformal transformations, the regularized area will be a function of the cross-ratios only.<sup>12</sup> The computation of this regularized area is the main focus of the remaining of this review.

### 3.2.1 Reconstructing the space-time solution and its behavior at infinity

In the following we would to check that the world-sheet we are considering has the desired form. In particular, we would like to understand the shape, in space-time, of the boundary of our world-sheet. For that, we first review a general procedure to reconstruct the world-sheet from the reduced fields, and then study its boundary.

Given an holomorphic function  $p(z)$  and a field  $\alpha$  satisfying (3.4) it is possible to reconstruct a space-time solution satisfying (3.2), and (3.1). The procedure amounts to solve two auxiliary linear problems, which we denote as left and right

$$(d + B^L)\psi_a^L = 0, \quad (d + B^R)\psi_{\dot{a}}^R = 0 \quad (3.10)$$

where the flat connections  $B^{L,R}$  are two by two matrices constructed from  $p(z)$  and  $\alpha(z, \bar{z})$ . For instance

$$B_z^L = \begin{pmatrix} \partial\alpha/4 & \frac{1}{\sqrt{2}}e^{\alpha/2} \\ \frac{1}{\sqrt{2}}pe^{-\alpha/2} & -\partial\alpha/4 \end{pmatrix} \quad (3.11)$$

we denote different components of the connections by  $B_{\alpha\beta}^L$  and  $B_{\dot{\alpha}\dot{\beta}}^R$ . On the other hand, the indices  $a$  and  $\dot{a}$  in (3.10) denote independent solutions of the auxiliary linear problems. Each  $\psi_a^L$  or  $\psi_{\dot{a}}^R$  is then a doublet. We denote the components of this doublet by  $\psi_{\alpha,a}^L$ , etc.

Given the solutions of these two auxiliary linear problems, one can show that the space-time coordinates are simply given by

$$Y_{a,\dot{a}} = \begin{pmatrix} Y_{-1} + Y_2 & Y_1 - Y_0 \\ Y_1 + Y_0 & Y_{-1} + Y_2 \end{pmatrix}_{a,\dot{a}} = \psi_{\alpha,a}^L \delta^{\alpha\dot{\beta}} \psi_{\dot{\beta},\dot{a}}^R \quad (3.12)$$

One can show that  $Y$  constructed this way satisfies all the required properties. If we see  $\psi^L$  and  $\psi^R$  as two by two matrices, then the space-time coordinates would be given by  $Y = (\psi^L)^T \psi^R$ . On the other hand, note that given a solution to the left problem,  $\psi^L$ , then  $\psi^L U^T$  is an equally good solution, and the same happens with the right problem.

<sup>12</sup>The full answer would include also the integral of the one we have subtracted. In order to compute it one would need to introduce a physical regulator and this part of the answer will not be conformal invariant. Anyway, its explicitly form can be worked out and turns out to be quite universal. In this review we will focus on the "interesting" part of the answer  $A_{reg}$ .

Hence, given  $Y$ , we obtain a family of space-time solutions  $UYV$ . These are nothing but the space-time conformal transformations.

Now we would like to understand the behavior of the solutions of the linear auxiliary problems for very large values of  $|z|$ , or  $|w|$ . This will tell us the behavior of the world-sheet near its boundary. Let us start, by simplicity, with the case of a homogeneous polynomial,  $p(z) = z^{n-2}$ . Hence  $w \approx z^{n/2}$ . As a result, as we go once around the  $z$ -plane, we go around the  $w$ -plane  $n/2$  times.

Due to the boundary conditions for the reduced fields, the flat connections  $B^{L,R}$  drastically simplify at infinity and we can solve the auxiliary linear problems. A general solution will be of the form

$$\begin{aligned} \psi_a^L &\approx c_a^+ \begin{pmatrix} 1 \\ 0 \end{pmatrix} e^{w+\bar{w}} + c_a^- \begin{pmatrix} 0 \\ 1 \end{pmatrix} e^{-(w+\bar{w})} \\ \psi_a^R &\approx d_a^+ \begin{pmatrix} 1 \\ 0 \end{pmatrix} e^{\frac{w-\bar{w}}{i}} + d_a^- \begin{pmatrix} 0 \\ 1 \end{pmatrix} e^{-\frac{w-\bar{w}}{i}} \end{aligned} \quad (3.13)$$

The  $w$ -plane is naturally divided into quadrants, see figure 5. In each quadrant one of

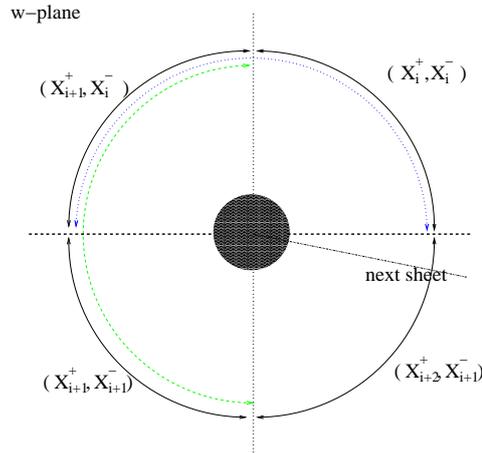

**Figure 5:** When looking at the left problem, (each sheet of) the  $w$ -plane is naturally divided into two parts, according to the sign of  $Re(w)$ . In the same way, when looking at the right problem, the  $w$ -plane is naturally divided into two parts, according to the sign of  $Im(w)$ . Hence, the  $w$ -plane is naturally divided into four quadrants. Large values of  $|w|$  in each of these angular sectors correspond to a cusp.

the two solutions of each problem (left and right) dominates. For instance, in the upper right quadrant, the solution proportional to  $c_a^+$  dominates in the left problem, while the solution proportional to  $d_a^+$  dominates in the right problem. This means that for large values of  $|w|$ , the whole quadrant corresponds to a single point in the boundary, given by  $Y_{a\dot{a}} \approx (Large) \times c_a^+ d_{\dot{a}}^+$ .

As we change quadrant, one and only one of the two dominant solutions change and we jump a light-like distance to the next cusp. In each quadrant/cusp we can write

$$Y_{a,\dot{a}} \approx \lambda_a \tilde{\lambda}_{\dot{a}} \quad (3.14)$$

where  $\lambda$  is given by the leading contribution to the left problem and  $\tilde{\lambda}$  by the leading contribution to the right problem. As we change quadrant, one of the two solutions,  $\lambda$  or  $\tilde{\lambda}$ , changes. As we go around the  $w$ -plane  $n/2$  times, we get the expected  $2n$  cusps!

In the general case in which the polynomial is not homogeneous, the picture is very much the same. In general, the degree of the polynomial determines the number of cusps, while the coefficients on the polynomial determine the shape of the polygon.

Let us finish this section with a very important observation. Since we know that the classical equations describing strings on  $AdS_5 \times S^5$  are integrable, see for instance [26], we expect the present problem to be integrable as well. Indeed, it is possible to introduce a spectral parameter  $\zeta$

$$B_z \rightarrow B_z(\zeta) = \frac{1}{4} \begin{pmatrix} \partial\alpha & 0 \\ 0 & -\partial\alpha \end{pmatrix} + \frac{1}{\zeta} \frac{1}{\sqrt{2}} \begin{pmatrix} 0 & e^{\alpha/2} \\ pe^{-\alpha/2} & 0 \end{pmatrix} \quad (3.15)$$

$$B_{\bar{z}} \rightarrow B_{\bar{z}}(\zeta) = \frac{1}{4} \begin{pmatrix} -\bar{\partial}\alpha & 0 \\ 0 & \bar{\partial}\alpha \end{pmatrix} + \zeta \frac{1}{\sqrt{2}} \begin{pmatrix} 0 & \bar{p}e^{-\alpha/2} \\ e^{\alpha/2} & 0 \end{pmatrix} \quad (3.16)$$

such that the flat connections are still flat, namely they satisfy  $\partial B_{\bar{z}} - \bar{\partial} B_z + [B_z, B_{\bar{z}}] = 0$ , for all values of  $\zeta$ . The introduction of the spectral parameter, also allows to study both linear problems in a unified manner. The left and right connections are just particular cases of the above flat connection, more precisely

$$B(\zeta = 1) = B^L, \quad B(\zeta = i) = B^R \quad (3.17)$$

The existence of the spectral parameter played a key role in the spectrum problem, see for instance [27]. In that context, the key objects are the eigenvalues of the monodromy matrix constructed out of the flat connection. In the present case the key objects are certain cross-ratios constructed from the holonomy of the connections.

### 3.3 Y-system for minimal surfaces

Let us focus on the left problem. We see that each sheet on the  $w$ -plane is naturally divided into two sectors, one with  $Re(w) > 0$  and the other with  $Re(w) < 0$ . In each sector the small solution is well defined (up to a normalization constant). On the other hand, the large solution is not, as we can add to it a part of the small solution. Let us then introduce the following terminology:

- The  $w$ -plane is divided into  $n$  sectors, since each sheet contains two sectors. We label these sectors by  $i = 0, \dots, n-1$ .
- We call  $s_i^L$  the small solution at the  $i$ -th sector. This is the solution with the fastest decay along the line in the center of the  $i$ -th sector, for increasing  $|w|$ .

In order to understand why these small solutions are important, we need to introduce a new element. Given that our connections are  $SL(2)$  matrices, we can introduce a  $SL(2)$  invariant product

$$\psi_a^L \wedge \psi_b^L \equiv \epsilon^{\alpha\beta} \psi_{\alpha,a}^L \psi_{\beta,b}^L = \epsilon_{ab} \quad (3.18)$$

The second equality corresponds to setting a normalization factor for our solutions. This can be done since one can check the above product is independent on the world-sheet coordinate  $z$ .

As already seen, the location of the cusps is determined by the large solutions. The large component of a solution, on a given sector, can be extracted by using the small solution on such sector and the  $SL(2)$  invariant product just introduced, more precisely

$$\psi_a^L \wedge s_i^L \approx \lambda_a^i \quad (3.19)$$

where the symbol  $\approx$  means up to factors that will cancel out in the final expression for the cross-ratios. How do we construct space-time cross-ratios? we have seen that the location of the cusps is given by  $Y_{a\dot{a}}^i = \lambda_a^i \tilde{\lambda}_{\dot{a}}^i$ . The space time cross-ratios involve distances like

$$Y^i \cdot Y^j = \epsilon^{ab} \epsilon^{\dot{a}\dot{b}} Y_{a\dot{a}}^i Y_{b\dot{b}}^j = \langle \lambda^i \lambda^j \rangle \langle \tilde{\lambda}^i \tilde{\lambda}^j \rangle, \quad \langle \lambda^i \lambda^j \rangle = \epsilon^{ab} \lambda_a^i \lambda_b^j \quad (3.20)$$

Given the normalization condition (3.18), one can easily show

$$\langle \lambda^i \lambda^j \rangle \approx \langle (\psi_a^L \wedge s_i^L)(\psi_a^L \wedge s_j^L) \rangle = s_i^L \wedge s_j^L \quad (3.21)$$

Which means that space-time cross-ratios can be constructed from inner products of the small solutions in the corresponding sectors! more precisely

$$\frac{x_{ij}^+ x_{kl}^+}{x_{ik}^+ x_{jl}^+} = \frac{(s_i^L \wedge s_j^L)(s_k^L \wedge s_l^L)}{(s_i^L \wedge s_k^L)(s_j^L \wedge s_l^L)} \quad (3.22)$$

Small solutions are defined up to a normalization constant. Note that such normalization constants cancel out when computing cross-ratios.

The strategy we will follow is to introduce the spectral parameter  $\zeta$  as shown in the previous section and study the small solutions of the corresponding connection

$$(d + B(\zeta))s_i(\zeta) = 0 \quad (3.23)$$

then, we can consider the cross-ratios as a function of such spectral parameter

$$\chi_{ijkl}(\zeta) = \frac{(s_i \wedge s_j)(s_k \wedge s_l)}{(s_i \wedge s_k)(s_j \wedge s_l)} \quad (3.24)$$

The physical cross-ratios are then obtained by setting the spectral parameter to appropriate values

$$\chi_{ijkl}(\zeta = 1) = \chi_{ijkl}^+, \quad \chi_{ijkl}(\zeta = i) = \chi_{ijkl}^- \quad (3.25)$$

A very important property of the flat connection  $B(\zeta)$  is that it possesses a  $Z_2$  symmetry:  $B(e^{i\pi}\zeta) = \sigma_3 B(\zeta) \sigma_3$ , where  $\sigma_3$  is the usual Pauli matrix. This symmetry allows to relate small solutions at different values of the spectral parameter, for instance  $s_{i+1}(\zeta) = \sigma_3 s_i(e^{i\pi}\zeta)$ , and in particular, it implies

$$s_i \wedge s_j(e^{i\pi}\zeta) = s_{i+1} \wedge s_{j+1}(\zeta) \quad (3.26)$$

This identity is crucial in deriving the equations below. Besides, in order to simplify subsequent expressions, we will assume  $s_i \wedge s_{i+1} = 1$ .

Now we have all the elements to derive the so called Hirota equations and the  $Y$ -system equations. The trick is to choose  $s_0$  and  $s_1$  as a complete basis of flat sections, and express two arbitrary consecutive small solutions  $s_k$  and  $s_{k+1}$  in terms of these

$$s_k = (s_k \wedge s_1)s_0 - (s_k \wedge s_0)s_1 \quad (3.27)$$

$$s_{k+1} = (s_{k+1} \wedge s_1)s_0 - (s_{k+1} \wedge s_0)s_1 \quad (3.28)$$

Next, use (3.26) in order to express every wedge as a wedge involving  $s_0$  and consider  $1 = s_k \wedge s_{k+1}$ , we obtain

$$-(s_{k-1} \wedge s_0)^{++}(s_{k+1} \wedge s_0) + (s_k \wedge s_0)^{++}(s_k \wedge s_0) = 1 \quad (3.29)$$

where we have introduced the notation  $f^\pm = f(e^{\pm i\pi/2}\zeta)$ ,  $f^{++} = f(e^{i\pi}\zeta)$ , etc. Let us introduce  $T_k = s_0 \wedge s_{k+1}(e^{-i(k+1)\pi/2}\zeta)$ . In terms of these we obtain

$$T_s^+ T_s^- = T_{s+1} T_{s-1} + 1 \quad (3.30)$$

which has the form of the so called Hirota equations! from the definition of  $T_s$ , we see that it is non trivial for  $s = 0, \dots, n-2$ . The  $Y$ -system equations can be obtained by introducing  $Y_s \equiv T_{s-1} T_{s+1}$

$$Y_s^+ Y_s^- = (1 + Y_{s+1})(1 + Y_{s-1}) \quad (3.31)$$

$Y_s$  is non trivial for  $s = 1, \dots, n-3$ . Note that this agrees with the amount of (complex) cross-ratios of our scattering problem. These are functional equations for  $Y_s(\zeta)$  and are valid for any value of  $\zeta$ . Note that they followed from a chain of rather trivial facts!

One could reintroduce the normalized factors  $s_i \wedge s_{i+1}$  and check that the  $Y$ -functions are given by the usual cross-ratios introduced above. The physical cross-ratios, are then obtained by evaluating  $Y_s(\zeta)$  at  $\zeta = 1$  and  $\zeta = i$ .

Such equations are not the whole story. In particular, note that that the holomorphic function  $p(z)$  does not enter at all in such equations! The point is the following. There are many solutions to such equations. The correct solution is then picked by specifying the analytic properties and boundary conditions of  $Y_s(\zeta)$  as we move on the  $\zeta$ -plane. This is how the information about the holomorphic polynomial enters and will be the subject of the following section.

### 3.4 Integral equations

In order to pick the appropriate solution to the  $Y$ -system equations (3.31) we need to specify the analytic properties of  $Y_s(\zeta)$ . By analyzing the auxiliary linear problems and the definition of  $Y_s(\zeta)$  one can show that  $Y_s(\zeta)$  are analytic away from  $\zeta = 0, \infty$ . On the other hand, As  $\zeta \rightarrow 0, \infty$ , the flat connection simplifies and the inverse problem can be solved by using a *WKB* approximation, where the role of  $\hbar$  is played by  $\zeta$  or  $1/\zeta$ . By calling  $\zeta = e^\theta$ , one can show that for large  $\theta$  the solution behaves as <sup>13</sup>

$$\log Y_s \approx -m_s \cosh \theta + \dots \quad (3.32)$$

<sup>13</sup>Note that even though we used the WKB approximation, this is the behavior of the exact solution.

where  $m_a$  is given by the periods of  $p(z)^{1/2}$  along the cycles  $\gamma_a$ , namely  $m_a \approx -\oint_{\gamma_a} \sqrt{p(z)} dz$ . This is how the information of the polynomial  $p(z)$  enters into the problem. These periods are usually complex, and there are  $n - 3$  of them, which exactly agrees with the quantity of expected cross-ratios. These  $m_a$  should be seen as the boundary conditions for the above equations.

The strategy now is well known from the study of integrable systems. We can combine the  $Y$ -system equations with the analytic properties and boundary conditions for the  $Y$ -functions, in order to write a system of integral equations for them. The solutions to these integral equations will automatically satisfy the  $Y$ -system equations and have the required boundary conditions. The system of integral equations is given by <sup>14</sup>

$$\log Y_s = -m_s \cosh \theta + \frac{1}{2\pi} \int_{-\infty}^{\infty} \frac{1}{\cosh(\theta - \theta')} \log(1 + Y_{s+1}(\theta'))(1 + Y_{s-1}(\theta')) \quad (3.33)$$

The system of equations (3.33) has the form of TBA equations, that arise when studying integrable models in finite volume, see *e.g.* [25]. Even though, for the sake of clarity, some overall coefficients have been suppressed in the derivation of these equations, the final form of the equations is given with all the correct coefficients. From the TBA point of view, the parameters  $m_a$  enter as masses. Once the masses are given, the solution of the above system is unique. The physical cross-ratios can be read off by looking at  $Y_s(\theta)$  for appropriate values of  $\theta$ .

These integral equations can also be written in terms of the physical cross-ratios  $y_s^+ = Y_s(\zeta = 1)$  and  $y_s^- = Y_s(\zeta = i)$  only, without resorting to the auxiliary parameters  $m_s$ . In order to achieve that, one simply evaluates (3.33) at the physical values of the spectral parameter in order to eliminate the masses, see [29]. We obtain

$$\log Y_s = \cosh \theta \log y_s^+ - i \sinh \theta \log y_s^- + \int d\theta' \frac{\sinh 2\theta}{\cosh(\theta' - \theta) \sinh 2\theta'} \log(1 + Y_{s+1}(\theta'))(1 + Y_{s-1}(\theta')) \quad (3.34)$$

Note that having solved (3.34), we could read off the masses from the asymptotic behavior of the solutions.

How do we compute the regularized area, once we have solved the above system of integral equations? It turns out that the area can be written in terms of the  $Y$ -functions in a very simple form

$$A_{reg} = \sum_s \int d\theta \frac{m_s}{2\pi} \cosh \theta \log(1 + Y_s(\theta)) \quad (3.35)$$

In order to derive this expression, one expands the  $Y$  functions a few orders for small and for large values of  $\zeta$ . The expansion coefficients are written in terms of period integrals that also appear in the expression for the area, see [21] for details. This expression has exactly the form of the free energy of the TBA system. <sup>15</sup>

<sup>14</sup>Considering  $l_s \equiv \log(Y_s/e^{-m_s \cosh \theta})$ , which is analytic in the strip  $Im(\theta) < \pi/2$  and vanishes as  $\theta$  approaches infinite. The integral equations can be obtained by convoluting the equation  $l_s^+ + l_s^- = \log(1 + Y_{s+1})(1 + Y_{s-1})$  with the kernel in (3.33).

<sup>15</sup>It can be shown [29] that actually this area coincides with the extremum of the Yang-Yang functional for the modified TBA equations (3.34)

The strategy to solve the full problem is then clear. For a choice of the cross-ratios we solve the integral equations (3.34), and from their solution we compute the area (3.35). Hence, we have the area for these values of the cross-ratios.

In this review we have treated in detail the case of minimal surfaces in  $AdS_3$ . However, the general case of minimal surfaces in  $AdS_5$  can also be solved [21]. Much of what we have said can be carried out for the general case. In this case we get a bigger system of  $Y$ -functions, denoted by  $Y_{a,s}$ , where  $a = 1, 2, 3$  and  $s = 1, \dots, N - 5$ . Note that their number equals the number of independent cross-ratios. Very much as before, one can obtain  $Y$ -system equations, which supplemented with the appropriate boundary conditions can be written as a system of integral equations. Again, this system of equations has the form of a TBA system, and the regularized area coincides with the free energy of such system.

These equations can be solved numerically, see for instance [21]. On the other hand, it is very hard to find analytical solutions. However, some limits, for instance the so called small masses/CFT limit and the large masses limit, are more tractable, see [28].

## 4 Conclusions

We reviewed the computation of scattering amplitudes of planar maximally super-symmetric Yang-Mills at strong coupling. By using the  $AdS/CFT$  duality the problem boils down to the computation of the area of certain minimal surfaces on  $AdS$ .

Then we showed how the integrability of the model can be efficiently used in order to give an answer for the problem in terms of a set of integral equations. Integrability allows to introduce a one parameter deformation (the spectral parameter  $\zeta$ ) and study such deformed problem. One can then write down a system of functional equations, or  $Y$ -system, valid for any value of  $\zeta$ . One can combine these functional equations with the knowledge of the analytic behavior of the  $Y$ -functions in the  $\zeta$ -plane, in order to write a set of integral equations which can be solved iteratively, and give the desired answer. There are many directions one could try to follow, some of the most interesting are the following

- It would be nice to find a physical connection between the integrable system that the TBA equations describe and the original integrable system.
- It would be very interesting to extend the present construction to the full quantum problem. As a first step, one could try to compute one loop (from the strong coupling point of view) corrections to the above picture. This would allow, for instance, to distinguish between different amplitudes.
- It would also be interesting to look for similar structures (for instance, the analogous of the spectral parameter, etc) in perturbative computations. Related to this, in [29] and subsequent papers, an operator product expansion for Wilson loops have been developed. This allows to use certain tools of integrability [30] in order to make predictions at all values of the coupling.

- One could hope that similar technology can be applied to related problems. One such problem is the computation of form factors, in which progress have been made recently, see [15] [31] [32].

### Acknowledgments

We would like to thank Davide Gaiotto, Amit Sever, Pedro Vieira and specially Juan Maldacena for collaboration on the material exposed in this review.

## References

- [V.1] R. Roiban, “Review of AdS/CFT Integrability, Chapter V.1: Scattering Amplitudes – a Brief Introduction,” arXiv:1012.4001 [hep-th].
- [V.2] J. Drummond, “Review of AdS/CFT Integrability, Chapter V.2: Dual Superconformal Symmetry,” arXiv:1012.4002 [hep-th].
- [1] J. M. Maldacena, “The large N limit of superconformal field theories and supergravity,” *Adv. Theor. Math. Phys.* **2** (1998) 231 [*Int. J. Theor. Phys.* **38** (1999) 1113] [arXiv:hep-th/9711200].
- [2] S. J. Rey and J. T. Yee, “Macroscopic strings as heavy quarks in large N gauge theory and anti-de Sitter supergravity,” *Eur. Phys. J. C* **22** (2001) 379 [arXiv:hep-th/9803001]. • J. M. Maldacena, “Wilson loops in large N field theories,” *Phys. Rev. Lett.* **80** (1998) 4859 [arXiv:hep-th/9803002].
- [3] L. F. Alday and J. M. Maldacena, “Gluon scattering amplitudes at strong coupling,” *JHEP* **0706** (2007) 064 [arXiv:0705.0303 [hep-th]].
- [4] L. F. Alday, J. M. Henn, J. Plefka and T. Schuster, “Scattering into the fifth dimension of N=4 super Yang-Mills,” *JHEP* **1001** (2010) 077 [arXiv:0908.0684 [hep-th]].
- [5] D. J. Gross and P. F. Mende, “String Theory Beyond the Planck Scale,” *Nucl. Phys. B* **303** (1988) 407.
- [6] J. McGreevy and A. Sever, “Planar scattering amplitudes from Wilson loops,” *JHEP* **0808** (2008) 078 [arXiv:0806.0668 [hep-th]].
- [7] K. Ito, H. Nastase and K. Iwasaki, “Gluon scattering in N = 4 super Yang-Mills at finite temperature,” *Prog. Theor. Phys.* **120** (2008) 99 [arXiv:0711.3532 [hep-th]]. • G. Georgiou and D. Giataganas, “Gluon Scattering Amplitudes in Finite Temperature Gauge/Gravity Dualities,” arXiv:1011.6339 [hep-th].
- [8] H. Dorn, N. Drukker, G. Jorjadze and C. Kalousios, “Space-like minimal surfaces in AdS x S,” *JHEP* **1004** (2010) 004 [arXiv:0912.3829 [hep-th]].

- [9] J. McGreevy and A. Sever, “Quark scattering amplitudes at strong coupling,” JHEP **0802** (2008) 015 [arXiv:0710.0393 [hep-th]]. • Z. Komargodski and S. S. Razamat, JHEP **0801** (2008) 044 [arXiv:0707.4367 [hep-th]]. • E. Barnes and D. Vaman, “Massive quark scattering at strong coupling from AdS/CFT,” Phys. Rev. D **81** (2010) 126007 [arXiv:0911.0010 [hep-th]].
- [10] M. Kruczenski, “A note on twist two operators in  $N = 4$  SYM and Wilson loops in Minkowski signature,” JHEP **0212** (2002) 024 [arXiv:hep-th/0210115].
- [11] S. S. Gubser, I. R. Klebanov and A. M. Polyakov, “A semi-classical limit of the gauge/string correspondence,” Nucl. Phys. B **636** (2002) 99 [arXiv:hep-th/0204051].
- [12] Z. Bern, L. J. Dixon and V. A. Smirnov, “Iteration of planar amplitudes in maximally supersymmetric Yang-Mills theory at three loops and beyond,” Phys. Rev. D **72**, 085001 (2005) [arXiv:hep-th/0505205].
- [13] J. M. Drummond, J. Henn, V. A. Smirnov and E. Sokatchev, “Magic identities for conformal four-point integrals,” JHEP **0701** (2007) 064 [arXiv:hep-th/0607160].
- [14] Z. Komargodski, “On collinear factorization of Wilson loops and MHV amplitudes in  $N=4$  SYM,” JHEP **0805** (2008) 019 [arXiv:0801.3274 [hep-th]]. • L. F. Alday, “Lectures on Scattering Amplitudes via AdS/CFT,” Fortsch. Phys. **56** (2008) 816 [arXiv:0804.0951 [hep-th]].
- [15] L. F. Alday and J. Maldacena, “Comments on gluon scattering amplitudes via AdS/CFT,” JHEP **0711** (2007) 068 [arXiv:0710.1060 [hep-th]].
- [16] Z. Bern, L. J. Dixon, D. A. Kosower, R. Roiban, M. Spradlin, C. Vergu and A. Volovich, “The Two-Loop Six-Gluon MHV Amplitude in Maximally Supersymmetric Yang-Mills Theory,” Phys. Rev. D **78** (2008) 045007 [arXiv:0803.1465 [hep-th]].
- [17] T. H. Buscher, “Path Integral Derivation of Quantum Duality in Nonlinear Sigma Models,” Phys. Lett. B **201**, 466 (1988).
- [18] N. Berkovits and J. Maldacena, “Fermionic T-Duality, Dual Superconformal Symmetry, and the Amplitude/Wilson Loop Connection,” JHEP **0809**, 062 (2008) [arXiv:0807.3196 [hep-th]]. • N. Beisert, R. Ricci, A. A. Tseytlin and M. Wolf, “Dual Superconformal Symmetry from AdS<sub>5</sub> x S<sup>5</sup> Superstring Integrability,” Phys. Rev. D **78**, 126004 (2008) [arXiv:0807.3228 [hep-th]].
- [19] L. F. Alday and J. Maldacena, “Minimal surfaces in AdS and the eight-gluon scattering amplitude at strong coupling,” arXiv:0903.4707 [hep-th].
- [20] L. F. Alday and J. Maldacena, “Null polygonal Wilson loops and minimal surfaces in Anti-de-Sitter space,” JHEP **0911**, 082 (2009) [arXiv:0904.0663 [hep-th]]. • L. F. Alday, D. Gaiotto and J. Maldacena, “Thermodynamic Bubble Ansatz,” arXiv:0911.4708 [hep-th].

- [21] L. F. Alday, J. Maldacena, A. Sever and P. Vieira, “Y-system for Scattering Amplitudes,” arXiv:1002.2459 [hep-th].
- [22] B. A. Burrington and P. Gao, “Minimal surfaces in AdS space and Integrable systems,” JHEP **1004** (2010) 060 [arXiv:0911.4551 [hep-th]]. • Y. Hatsuda, K. Ito, K. Sakai, Y. Satoh, “Thermodynamic Bethe Ansatz Equations for Minimal Surfaces in AdS(3),” JHEP **1004**, 108 (2010). [arXiv:1002.2941 [hep-th]].
- [23] D. Gaiotto, G. W. Moore and A. Neitzke, “Four-dimensional wall-crossing via three-dimensional field theory,” Commun. Math. Phys. **299** (2010) 163 [arXiv:0807.4723 [hep-th]]. • D. Gaiotto, G. W. Moore and A. Neitzke, “Wall-crossing, Hitchin Systems, and the WKB Approximation,” arXiv:0907.3987 [hep-th].
- [24] H. J. De Vega and N. G. Sanchez, “Exact Integrability Of Strings In D-Dimensional De Sitter Space-Time,” Phys. Rev. D **47**, 3394 (1993). • A. Jevicki, K. Jin, C. Kalousios and A. Volovich, “Generating AdS String Solutions,” JHEP **0803**, 032 (2008) [arXiv:0712.1193 [hep-th]]. • H. Dorn, “Some comments on spacelike minimal surfaces with null polygonal boundaries in  $AdS_m$ ,” JHEP **1002**, 013 (2010) [arXiv:0910.0934 [hep-th]].
- [25] A. B. Zamolodchikov, “Thermodynamic Bethe Ansatz In Relativistic Models. Scaling Three State Potts And Lee-Yang Models,” Nucl. Phys. B **342**, 695 (1990).
- [26] I. Bena, J. Polchinski and R. Roiban, “Hidden symmetries of the AdS(5) x S\*\*5 superstring,” Phys. Rev. D **69** (2004) 046002 [arXiv:hep-th/0305116].
- [27] S. Schafer-Nameki, “Review of AdS/CFT Integrability, Chapter II.4: The Spectral Curve,” arXiv:1012.3989 [hep-th].
- [28] Y. Hatsuda, K. Ito, K. Sakai, Y. Satoh, “Six-point gluon scattering amplitudes from Z4-symmetric integrable model,” JHEP **1009**, 064 (2010). [arXiv:1005.4487 [hep-th]]. • Y. Hatsuda, K. Ito, K. Sakai, Y. Satoh, “g-functions and gluon scattering amplitudes at strong coupling,” [arXiv:1102.2477 [hep-th]]. • J. Bartels, J. Kotanski, V. Schomerus, “Excited Hexagon Wilson Loops for Strongly Coupled N=4 SYM,” JHEP **1101**, 096 (2011). [arXiv:1009.3938 [hep-th]].
- [29] L. F. Alday, D. Gaiotto, J. Maldacena, A. Sever and P. Vieira, “An Operator Product Expansion for Polygonal null Wilson Loops,” arXiv:1006.2788 [hep-th].
- [30] B. Basso, “Exciting the GKP string at any coupling,” arXiv:1010.5237 [hep-th].
- [31] J. Maldacena and A. Zhiboedov, “Form factors at strong coupling via a Y-system,” JHEP **1011** (2010) 104 [arXiv:1009.1139 [hep-th]].
- [32] A. Brandhuber, B. Spence, G. Travaglini and G. Yang, “Form Factors in N=4 Super Yang-Mills and Periodic Wilson Loops,” JHEP **1101** (2011) 134 [arXiv:1011.1899 [hep-th]].



# Review of AdS/CFT Integrability, Chapter VI.1: Superconformal Symmetry

NIKLAS BEISERT

*Max-Planck-Institut für Gravitationsphysik, Albert-Einstein-Institut  
Am Mühlenberg 1, 14476 Potsdam, Germany*

nbeisert@aei.mpg.de

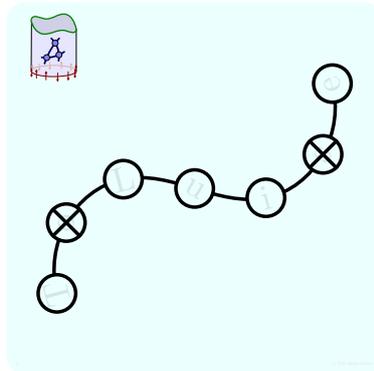

**Abstract:** Aspects of the  $D = 4$ ,  $\mathcal{N} = 4$  superconformal symmetry relevant to the AdS/CFT duality and integrability are reviewed. These include the Lie superalgebra  $\mathfrak{psu}(2, 2|4)$ , its representations, conformal transformations and correlation functions in  $\mathcal{N} = 4$  super Yang–Mills theory as well as an illustration of the  $AdS_5 \times S^5$  superspace on which the dual string theory is formulated.

## 1 Introduction

The AdS/CFT correspondence predicts the exact equivalence of  $\mathcal{N} = 4$  super Yang–Mills (SYM) theory with IIB superstrings propagating on the  $AdS_5 \times S^5$  background. One of the immediate checks is that the two models have coincident global symmetries:  $\mathcal{N} = 4$  superconformal symmetry on the one hand and the isometries of the  $AdS_5 \times S^5$  superspace on the other are both given by the Lie supergroup  $\widetilde{\text{PSU}}(2, 2|4)$  or its algebra  $\mathfrak{psu}(2, 2|4)$ .

Symmetry serves as an important organising principle — e.g. for objects with similar properties — and leads to structural constraints — e.g. for correlation functions. Furthermore, supersymmetry often implies that selected quantities are protected from receiving quantum corrections. Two famous examples are the exact quantum conformal symmetry of  $\mathcal{N} = 4$  SYM due to absence of a beta-function [1] and the exactness of correlators for certain BPS operators in agreement with a prediction of the AdS/CFT duality, see the review [2]. Nevertheless, agreement of the symmetry groups is far from sufficient to prove an exact duality.<sup>1</sup> To verify the AdS/CFT conjecture one therefore needs tests involving dynamical quantities which are not protected by the symmetry. Much of the activity concerning AdS/CFT integrability is devoted to such tests. Making use of superconformal symmetry has helped the progress at various stages.

The present paper reviews some aspects of the Lie superalgebra  $\mathfrak{psu}(2, 2|4)$  relevant to AdS/CFT integrability. The presented facts are by no means restricted to integrability; they were known long before AdS/CFT integrability was discovered, and little progress was made in connection with the latter. Nevertheless, many results in AdS/CFT integrability are based on a good knowledge of  $\mathfrak{psu}(2, 2|4)$ . This paper therefore serves a different purpose than the other chapters of the review collection [3]: It is not so much a review of one particular aspect of AdS/CFT integrability, but should be viewed as a reference guide to key concepts concerning the underlying global symmetry.

This paper is split into three parts: In Sec. 2 we shall review purely algebraic aspects of  $\mathfrak{psu}(2, 2|4)$  such as the algebra itself as well as some essential representation theory. In Sec. 3 we apply it to local operators in  $\mathcal{N} = 4$  SYM and their correlation functions. In Sec. 4 we discuss the  $AdS_5 \times S^5$  background on which superstrings can propagate and which is a particular coset of  $\widetilde{\text{PSU}}(2, 2|4)$ .

## 2 The $\mathfrak{psu}(2, 2|4)$ Algebra

**Definition.** The algebra  $\mathfrak{psu}(2, 2|4)$  is a real Lie superalgebra of (even|odd) dimension  $30|32$ , see e.g. [4]. In order to define it, it is convenient to start with complex  $4|4$ -dimensional square supermatrices

$$X = \left( \begin{array}{c|c} A & B \\ \hline C & D \end{array} \right). \quad (2.1)$$

---

<sup>1</sup>In this case the large amount of (super)symmetry at least makes both constituent models essentially unique and exceptional, which may be viewed as a hint towards the validity of the correspondence.

Each block  $A, B, C, D$  is a  $4 \times 4$  matrix of (non-Graßmannian) complex numbers. The blocks  $A, D$  are considered *even* and  $B, C$  *odd*. The Lie superalgebra  $\mathfrak{gl}(4|4, \mathbb{C})$  is the  $32|32$ -dimensional vector space of these supermatrices. Its graded Lie bracket  $[\cdot, \cdot]$  is defined as the graded commutator of supermatrices (in the following  $Y$  is the analog of  $X$  in (2.1) with blocks  $E, F, G, H$ )

$$[X, Y] = XY - (-1)^{XY} YX := \left( \begin{array}{c|c} AE + BG - EA + FC & AF + BH - EB - FD \\ \hline CE + DG - GA - HC & CF + DH + GB - HD \end{array} \right). \quad (2.2)$$

It differs from a conventional commutator through the signs for the odd-odd products  $FC$  and  $GB$ . It also satisfies a graded Jacobi-identity

$$(-1)^{XZ} [[X, Y], Z] + (-1)^{YX} [[Y, Z], X] + (-1)^{ZY} [[Z, X], Y] = 0. \quad (2.3)$$

This algebra is not simple, it has non-trivial ideals: One is related to the supertrace  $\text{STr } X := \text{Tr } A - \text{Tr } D$  which is zero for graded commutators  $\text{STr}[X, Y] = 0$ . Demanding that  $\text{STr } X = 0$  thus removes a derivation from  $\mathfrak{gl}(4|4, \mathbb{C})$ , and restricts it to the subalgebra  $\mathfrak{sl}(4|4, \mathbb{C})$ . Furthermore, the identity supermatrix 1 commutes with all other matrices,  $[1, X] = 0$ . Hence it generates the centre and can be projected out from  $\mathfrak{gl}(4|4, \mathbb{C})$  yielding  $\mathfrak{pgl}(4|4, \mathbb{C})$ . The combination of restriction and projection is the  $30|32$ -dimensional complex Lie superalgebra  $\mathfrak{psl}(4|4, \mathbb{C})$ .<sup>2</sup>

**Real Form.** To restrict to the real form  $\mathfrak{psu}(2, 2|4)$  one imposes a hermiticity condition on the supermatrices

$$\left( \begin{array}{c|c} A & B \\ \hline C & D \end{array} \right) = \left( \begin{array}{c|c} HA^\dagger H^{-1} & -iHC^\dagger \\ \hline -iB^\dagger H^{-1} & D^\dagger \end{array} \right), \quad (2.4)$$

where  $H$  is a hermitian matrix of signature  $(2, 2)$ . There are two natural choices for  $H$ : In the first,  $H$  is diagonal, written in terms of  $2 \times 2$  blocks ('+'/'-' denotes the  $2 \times 2$  positive/negative identity matrix;  $X'$  is a reordering of rows and columns to be explained)

$$H = \left( \begin{array}{cc} + & 0 \\ 0 & - \end{array} \right), \quad X = \left( \begin{array}{cc|c} M_1 & iN & -iQ_1 \\ iN & M_2 & +iQ_2 \\ \hline \bar{Q}_1 & \bar{Q}_2 & R \end{array} \right), \quad X' = \left( \begin{array}{c|c|c} M_1 & -iQ_1 & iN \\ \hline \bar{Q}_1 & R & \bar{Q}_2 \\ \hline iN & +iQ_2 & M_2 \end{array} \right). \quad (2.5)$$

Here the hermitian blocks  $M_1$  and  $M_2$  generate the maximal compact subalgebra  $\mathfrak{su}(2) \oplus \mathfrak{su}(2) \oplus \mathfrak{u}(1) = \mathfrak{so}(4) \oplus \mathfrak{so}(2)$  of  $\mathfrak{su}(2, 2) = \mathfrak{so}(4, 2)$ . This choice is useful in the context of the  $AdS_5$  spacetime, cf. Sec. 4, and for unitary representations. Equivalently one can choose an off-diagonal  $H$

$$H = \left( \begin{array}{cc} 0 & + \\ + & 0 \end{array} \right), \quad X = \left( \begin{array}{cc|c} L & P & -iQ \\ K & \bar{L} & -i\bar{S} \\ \hline S & \bar{Q} & R \end{array} \right), \quad X' = \left( \begin{array}{c|c|c} L & -iQ & P \\ \hline S & R & \bar{Q} \\ \hline K & -i\bar{S} & \bar{L} \end{array} \right). \quad (2.6)$$

<sup>2</sup>It is not possible to restrict to  $\text{Tr } A = \text{Tr } D = 0$  because the graded commutator does *not close* onto such supermatrices; The centre proportional to the unit supermatrix can only be *projected* out or removed by redefining the graded commutator accordingly.

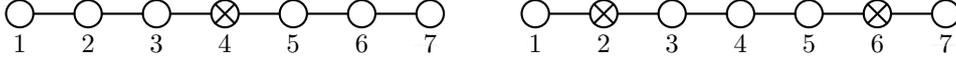

**Figure 1:** Two Dynkin diagrams for  $\mathfrak{sl}(4|4) = \mathfrak{sl}(2|4|2)$ .

Now the hermitian conjugate blocks  $L, \bar{L}$  in  $X$  generate the Lorentz and scaling transformations in  $\mathfrak{sl}(2, \mathbb{C}) \oplus \mathfrak{gl}(1) = \mathfrak{so}(3, 1) \oplus \mathfrak{so}(1, 1)$ . Obviously, this choice is adapted to four-dimensional Minkowski space, see Sec. 3. In the context of the real form  $\mathfrak{psu}(2, 2|4)$  it is often convenient to reorder the 2, 2|4 rows and columns, and move one of the 2's past the 4. The supermatrix  $X$  reordered in 2|4|2-block form is displayed in (2.5, 2.6) as  $X'$ . From now on we shall use exclusively the 2|4|2-grading.

**Simple Generators.** A useful presentation of Lie algebras, which is frequently encountered in the solution of integrable systems, is through  $r$  triplets of *simple* (raising, Cartan and lowering) generators  $E_k, H_k, F_k$ , ( $r$  is the rank of the algebra), see e.g. [5]. For the Lie algebras  $\mathfrak{sl}(n)$  the elements  $E_k, H_k, F_k$  with  $k = 1, \dots, n - 1$ , generate the three main diagonals  $X_{k,k+1}, X_{k,k} - X_{k+1,k+1}, X_{k+1,k}$ . The remaining elements are obtained by repeated Lie brackets, e.g.  $[E_k, E_{k+1}]$  generates  $X_{k,k+2}$ . Evidently, the algebra generated by arbitrary repeated brackets is enormous and needs to be reduced by certain relations. To that end, the simple generators satisfy a set of Chevalley–Serre relations which encode all the information on the specific Lie algebra,  $\mathfrak{sl}(n)$ , in a condensed form

$$\begin{aligned} [H_j, E_k] &= +A_{jk}E_k, & [H_j, F_k] &= -A_{jk}F_k, & [E_j, F_k] &= \delta_{jk}H_k, \\ [[E_k, E_{k\pm 1}], E_{k\pm 1}] &= [[F_k, F_{k\pm 1}], F_{k\pm 1}] = 0, \\ [E_j, E_k] &= [F_j, F_k] = 0 \text{ for } |j - k| > 1. \end{aligned} \quad (2.7)$$

Here  $A_{j,k}$  is the Cartan matrix; for  $\mathfrak{sl}(n)$  the three main diagonals take the values  $-1, +2, -1$  while the other elements are zero. For a superalgebra  $\mathfrak{sl}(n|m)$  the definition is similar; the main difference is that some of the raising and lowering elements are odd. For an odd  $E_k$  ( $k = 2, 6$  in our case) one has to replace the relation  $[[E_{k\pm 1}, E_k], E_k] = 0$  by two new ones<sup>3</sup>

$$[E_k, E_k] = 0, \quad [[E_{k-1}, E_k], [E_{k+1}, E_k]] = 0, \quad (2.8)$$

and similarly for  $F_k$ . Furthermore for this  $k$  two Cartan matrix elements are modified:  $A_{k,k} = 0$  and  $A_{k,k+1} = +1$ . Cartan matrices and Chevalley–Serre relations are often displayed in the form of Dynkin diagrams. Two Dynkin diagrams for  $\mathfrak{su}(2, 2|4)$  are displayed in Fig. 1: Dots correspond to simple generators  $E_k, H_k, F_k$ ; crossed dots indicate odd generators  $E_k, F_k$ . Links stand for non-trivial relations between the corresponding simple generators and non-trivial Cartan matrix elements. If two dots  $j$  and  $k$  are unlinked, the generators  $E_k, F_k, H_k$  and  $E_j, F_j, H_j$  commute and  $A_{jk} = 0$ . Although the two Dynkin diagrams lead to quite different relations, they describe the same algebra.

<sup>3</sup>It turns out that in gauge/string applications the latter relations are dropped, see e.g. [6]. The new generators  $G_k \sim [[E_{k-1}, E_k], [E_{k+1}, E_k]]$  (similarly for  $F_k$ ) are part of an ideal of a substantially bigger algebra. The ideal generates gauge transformations acting as the constraint  $G_k \simeq 0$  for physical states.

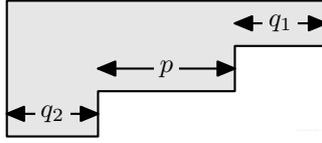

**Figure 2:** Young diagram corresponding to  $\mathfrak{sl}(4)$  representation with Dynkin labels  $[q_1, p, q_2]$ : A single block corresponds to a fundamental representation, rows and columns correspond to symmetrisation and antisymmetrisation.

The point is that for Lie superalgebras there commonly exist inequivalent choices for the set of simple generators. The two diagrams correspond to the two grading assignments  $4|4$  and  $2|4|2$  for the rows and columns of a supermatrix, cf.  $X$  vs.  $X'$  in (2.5,2.6).

**Unitary Representations.** In physical models, multiplets of states transform under *unitary* representations of the symmetry algebra. Let us therefore review unitary representations of  $\mathfrak{psu}(2, 2|4)$  [7]. As the (bosonic part of the) superalgebra is non-compact, unitary representations are necessarily infinite-dimensional. An important class of unitary representations are the *lowest-weight* (equivalently highest-weight) representations. Under the maximal compact subalgebra  $\mathfrak{su}(2) \oplus \mathfrak{su}(2) \oplus \mathfrak{su}(4) \oplus \mathfrak{u}(1)$  such representations decompose into (infinitely many) finite-dimensional irreps, one of which is defined as the lowest. All states corresponding to this lowest irrep are annihilated by the lowering generators associated to the lower triangular blocks  $\bar{Q}_1, Q_2, \bar{N}$  of  $X'$  in (2.5). The states of the higher irreps arise from the repeated action of the raising generators associated to the upper triangular blocks  $Q_1, \bar{Q}_2, N$  of  $X'$ .

Lowest-weight unitary representations of  $\mathfrak{psu}(2, 2|4)$  are thus specified by an irrep under the maximal compact subalgebra  $\mathfrak{su}(2) \oplus \mathfrak{su}(2) \oplus \mathfrak{su}(4) \oplus \mathfrak{u}(1)$ . Irreps of the two  $\mathfrak{su}(2)$ 's are specified by their non-negative half-integer spin  $\frac{1}{2}s_{1,2}$  or equivalently by the non-negative integer *Dynkin labels*  $[s_1]$  and  $[s_2]$ . Analogously, irreps of  $\mathfrak{su}(4)$  are specified through three non-negative integer Dynkin labels  $[q_1, p, q_2]$ . An alternative description uses a Young diagram with no more than three rows, see Fig. 2, cf. [8] Finally, a  $\mathfrak{u}(1)$  irrep is specified through a number  $E$ . Here there is a subtlety: The abelian algebra  $\mathfrak{u}(1) = \mathbb{R}$  can either generate the compact group  $U(1)$  or the non-compact additive group  $\mathbb{R}$ . For a compact group  $E$  is restricted to an integer whereas a non-compact group merely requires  $E$  to be real. The supergroup  $PSU(2, 2|4)$  contains the compact version and hence the spectrum of  $E$  is discrete. However,  $PSU(2, 2|4)$  has a non-trivial *universal cover*  $\widetilde{PSU}(2, 2|4)$  where the abelian subgroup becomes non-compact. It is this universal cover which has applications to physics, and consequently we shall allow continuous values for  $E$ .

Altogether, a unitary representation is specified by the Dynkin labels  $[s_1], [s_2], [q_1, p, q_2]$  and the number  $E$ . These combine into  $\mathfrak{su}(2, 2|4)$  Dynkin labels:

$$[s_1; r_1; q_1, p, q_2; r_2; s_2], \quad r_k = \frac{1}{2}E + \frac{1}{2}s_k - \frac{3}{4}q_k - \frac{1}{2}p - \frac{1}{4}q_{3-k}. \quad (2.9)$$

Finally, we should note that the value of  $E$  must be above a certain bound which is most conveniently expressed in terms of the  $r_k$

$$r_k \geq 1 + s_k \quad \text{or} \quad r_k = s_k = 0. \quad (2.10)$$

If one of the bounds for the first condition is saturated or one of the second conditions is satisfied, the representation is called *atypical* or short. In this case certain combinations of the raising generators annihilate the lowest-weight state. Otherwise there are no additional restrictions on the representation of the raising generators, and the representation is called *typical* or long.

### 3 Superconformal Symmetry in $\mathcal{N} = 4$ SYM

For  $\mathcal{N} = 4$  supersymmetric gauge theory on four-dimensional Minkowski space the super-Poincaré algebra extends to the superconformal algebra  $\mathfrak{psu}(2, 2|4)$ . In the following we shall discuss the representation theory of  $\mathfrak{psu}(2, 2|4)$  related to this gauge theory, see also [2] for an extended review.

**Conformal Transformations.** Conformal transformations preserve the metric up to a local rescaling of distances. In four-dimensional Minkowski space conformal symmetry is based on the Lie algebra  $\mathfrak{so}(4, 2) = \mathfrak{su}(2, 2)$ . It contains the  $\mathfrak{sl}(2, \mathbb{C})$  Lorentz rotations  $L, \bar{L}$  and translations  $P$  which form the Poincaré algebra. In addition, there are the dilatation  $D$  and the conformal boosts  $K$ . The extension to the superconformal algebra consists of the internal  $\mathfrak{su}(4)$  rotations  $R$ , the supertranslations  $Q, \bar{Q}$  as well as the superconformal boosts  $S, \bar{S}$ . These generators correspond to the submatrices in (2.6).

The conformal generators  $P, D, K$  act on the coordinates  $x^\mu$  of Minkowski space with metric  $\eta^{\mu\nu}$  as

$$P_\mu x^\nu = i\delta_\mu^\nu, \quad Dx^\mu = ix^\mu, \quad K^\mu x^\nu = ix^\mu x^\nu - \frac{i}{2}\eta^{\mu\nu} x \cdot x. \quad (3.1)$$

The action of the odd generators is rather complicated and requires the introduction of fermionic coordinates; we refrain from spelling out the explicit form. Fields on Minkowski space transform according to the above rules, but in addition they have intrinsic transformation properties such as *spin* and *conformal dimension*. For example, the conformal representation on a scalar primary field  $\Phi(x)$  of dimension  $d$  reads

$$P_\mu \Phi = i\partial_\mu \Phi, \quad D\Phi = id\Phi + ix \cdot \partial \Phi, \quad K^\mu \Phi = id x^\mu \Phi + ix^\mu x \cdot \partial \Phi - \frac{i}{2} x \cdot x \partial^\mu \Phi. \quad (3.2)$$

Representations for fields with spin are slightly more complicated, and representations of the complete superconformal algebra suggest the use of fields on superspace. Both of these aspects will not be considered explicitly.

**Correlators.** The power of conformal symmetry is that it constrains correlation functions in a conformal quantum field theory, see e.g. [9]. In particular, the spacetime dependence of two- and three-point functions is fully determined

$$\begin{aligned} \langle \Phi_1(x) \Phi_2(y) \rangle &= \frac{N}{|x - y|^{2d}}, \quad (\text{requires } d_1 = d_2 = d), \\ \langle \Phi_1(x) \Phi_2(y) \Phi_3(z) \rangle &= \frac{C_{123}}{|x - y|^{d_1+d_2-d_3} |y - z|^{d_2+d_3-d_1} |z - x|^{d_3+d_1-d_2}}. \end{aligned} \quad (3.3)$$

Indices for fields with spin are typically contracted with suitable tensors, e.g.  $I^{\mu\nu} = \eta^{\mu\nu} - 2(x-y)^\mu(x-y)^\nu/(x-y)^2$ . The reason for complete determination is that any three points can be mapped to any other three points by conformal transformations. The value of the correlator at one configuration of three points thus determines the value of the correlator at any other configuration. For four or more points there exist conformally invariant cross ratios, e.g.  $|x_{12}||x_{34}|/|x_{13}||x_{24}|$ , on which the correlation functions can depend without constraints. Note that there exist superconformal cross ratios of the fermionic coordinates already for three points in superspace.<sup>4</sup>

The above constraints on correlators hold for all fields which have well-defined transformation properties under superconformal symmetry. This includes the fundamental fields (to some extent), but more importantly also *composite local operators*. The latter are local products of the fundamental fields and their derivatives. In the free field theory, they transform in tensor products of the fundamental field representation. Let us therefore discuss the superconformal representations that come to use.

**Fundamental Field Representation.** Consider first a scalar field  $\Phi$  in four dimensions. In the free theory  $\Phi$  obeys the conformal transformation rules (3.2) with  $d = 1$ . For a local operator we shall need  $\Phi$  and its derivatives at the point  $x$  which for convenience we assume to be the origin of spacetime  $x = 0$ . In other words, we represent  $\Phi(x)$  through its Taylor series around  $x = 0$

$$\Phi(x) = \Phi(0) + x^\mu \partial_\mu \Phi(0) + \frac{1}{2} x^\mu x^\nu \partial_\mu \partial_\nu \Phi(0) + \dots \quad (3.4)$$

We can now see that the conformal representation (3.2) acts on these Taylor components (we drop the argument  $x = 0$ ):

$$\begin{aligned} P_\mu \Phi &= i \partial_\mu \Phi, & D\Phi &= i d \Phi, & K^\mu \Phi &= 0, \\ P_\mu \partial_\rho \Phi &= i \partial_\rho \partial_\mu \Phi, & D\partial_\rho \Phi &= i(d+1) \partial_\rho \Phi, & K^\mu \partial_\rho \Phi &= i d \delta_\rho^\mu \Phi, \\ & & \dots & & \dots & \end{aligned} \quad (3.5)$$

This is a lowest-weight representation, where  $K$  serves as the lowering generator to annihilate the primary field  $\Phi$ . The raising generator  $P$  is used to access the descendants  $\partial_\mu \Phi$ ,  $\partial_\mu \partial_\nu \Phi$ ,  $\dots$ , while  $D$  essentially measures the number of derivatives.

There is one noteworthy peculiarity of the boost acting on  $\partial_\rho \partial_\sigma \Phi$

$$K^\mu \partial_\rho \partial_\sigma \Phi = i(d+1) \delta_\sigma^\mu \partial_\rho \Phi + i(d+1) \delta_\rho^\mu \partial_\sigma \Phi - i \eta_{\rho\sigma} \partial^\mu \Phi. \quad (3.6)$$

When acting on the D'Alembertian derivative  $\partial \cdot \partial \Phi$  one obtains  $2i(d-1) \partial^\mu \Phi$  which vanishes precisely for the physical scaling dimension  $d = 1$ . This means that the lowest-weight representation is reducible, and we should divide out a subrepresentation by imposing the free equation of motion  $\partial \cdot \partial \Phi = 0$ .

The equation of motion implies the absence of certain components in the Taylor expansion. The enumeration of non-trivial components is most transparent when using

<sup>4</sup>The number of invariants is related to the dimension of the group, the dimension of the stabiliser and the number of coordinates. E.g., three points in superspace have 48 fermionic coordinates, but the group has only 32. Hence there should be 16 invariant combinations of fermionic coordinates.

pairs of spinor indices  $\beta\dot{\alpha}$  instead of the vector indices  $\mu$ . Now a trace  $\eta^{\mu\nu}$  is replaced by a pair of antisymmetric  $\mathfrak{sl}(2, \mathbb{C})$  invariants  $\varepsilon^{\beta\dot{\delta}}\varepsilon^{\dot{\alpha}\dot{\gamma}}$ . For any pair of derivatives we can thus exclude antisymmetrisation in both pairs of spinor indices by virtue of the equations of motion. Furthermore, due to the commutative nature of derivatives, antisymmetrisation in just one pair of spinor indices is also zero. Effectively it means that all spinor indices of either kind must be fully symmetrised. Such symmetrisation is automatic for states of a four-dimensional *harmonic oscillator*: We can replace

$$\partial_{\beta\dot{\alpha}}\partial_{\delta\dot{\gamma}}\dots\Phi \simeq \bar{\mathbf{a}}_{\beta}\bar{\mathbf{a}}_{\dot{\delta}}\dots\bar{\mathbf{b}}_{\dot{\alpha}}\bar{\mathbf{b}}_{\dot{\gamma}}\dots|0\rangle, \quad (3.7)$$

where the algebra of creation and annihilation operators is defined through the non-trivial commutation relations

$$[\mathbf{a}^{\alpha}, \bar{\mathbf{a}}_{\gamma}] = i\delta_{\gamma}^{\alpha}, \quad [\mathbf{b}^{\dot{\alpha}}, \bar{\mathbf{b}}_{\dot{\gamma}}] = i\delta_{\dot{\gamma}}^{\dot{\alpha}}, \quad \{\mathbf{c}^a, \bar{\mathbf{c}}_c\} = \delta_c^a. \quad (3.8)$$

Here we have added a set of four fermionic oscillators  $\mathbf{c}$  which make the generalisation to all fields of  $\mathcal{N} = 4$  straight-forward: States have up to four excitations of  $\bar{\mathbf{c}}$  transforming in the  $\mathfrak{su}(4)$  representations  $\mathbf{1}, \mathbf{4}, \mathbf{6}, \bar{\mathbf{4}}, \mathbf{1}$ , respectively. This matches precisely with the representations of the chiral part of the gauge field strength  $\Gamma_{\alpha\gamma}$ , the chiral fermions  $\Psi_{ac}$ , the scalars  $\Phi_{ac}$ , the antichiral fermions  $\bar{\Psi}_{\dot{\alpha}}^c$  and the antichiral field strength  $\bar{\Gamma}_{\dot{\alpha}\dot{\gamma}}$ .<sup>5</sup> Altogether, for every state of the supersymmetric oscillator, subject to the constraint

$$\mathbf{N}_{\mathbf{a}} - \mathbf{N}_{\mathbf{b}} + \mathbf{N}_{\mathbf{c}} \simeq 2, \quad (3.9)$$

there is exactly one Taylor component of the on-shell fundamental fields of  $\mathcal{N} = 4$  SYM [10]. The excitation number operators are defined as  $\mathbf{N}_{\mathbf{a}} := -i\bar{\mathbf{a}}_{\alpha}\mathbf{a}^{\alpha}$ ,  $\mathbf{N}_{\mathbf{b}} := -i\bar{\mathbf{b}}_{\dot{\alpha}}\mathbf{b}^{\dot{\alpha}}$ ,  $\mathbf{N}_{\mathbf{c}} := \bar{\mathbf{c}}_a\mathbf{c}^a$ .

The oscillator basis is also particularly convenient for the superconformal algebra: All the generators are represented through bilinears in the oscillators:

$$\begin{aligned} \mathbf{L}^{\alpha}_{\gamma} &\simeq \bar{\mathbf{a}}_{\gamma}\mathbf{a}^{\alpha} - \frac{1}{2}\delta_{\gamma}^{\alpha}\bar{\mathbf{a}}_{\epsilon}\mathbf{a}^{\epsilon}, & \mathbf{R}^a_c &\simeq \bar{\mathbf{c}}_c\mathbf{c}^a - \frac{1}{4}\delta_c^a\bar{\mathbf{c}}_e\mathbf{c}^e, \\ \bar{\mathbf{L}}^{\dot{\alpha}}_{\dot{\gamma}} &\simeq \mathbf{b}^{\dot{\alpha}}\bar{\mathbf{b}}_{\dot{\gamma}} - \frac{1}{2}\delta_{\dot{\gamma}}^{\dot{\alpha}}\mathbf{b}^{\dot{\epsilon}}\bar{\mathbf{b}}_{\dot{\epsilon}}, & \mathbf{D} &\simeq \frac{1}{2}\bar{\mathbf{a}}_{\alpha}\mathbf{a}^{\alpha} + \frac{1}{2}\mathbf{b}^{\dot{\alpha}}\bar{\mathbf{b}}_{\dot{\alpha}}, \\ \mathbf{P}_{\gamma\dot{\alpha}} &\simeq \bar{\mathbf{a}}_{\gamma}\bar{\mathbf{b}}_{\dot{\alpha}}, & \mathbf{K}^{\gamma\dot{\alpha}} &\simeq \mathbf{b}^{\dot{\alpha}}\mathbf{a}^{\gamma}, \\ \mathbf{Q}_{\gamma}^a &\simeq \bar{\mathbf{a}}_{\gamma}\mathbf{c}^a, & \mathbf{S}_a^{\gamma} &\simeq \bar{\mathbf{c}}_a\mathbf{a}^{\gamma}, \\ \bar{\mathbf{Q}}_{\dot{\gamma}a} &\simeq \bar{\mathbf{c}}_a\bar{\mathbf{b}}_{\dot{\gamma}}, & \bar{\mathbf{S}}^{\dot{\gamma}a} &\simeq \mathbf{b}^{\dot{\gamma}}\mathbf{c}^a. \end{aligned} \quad (3.10)$$

These satisfy the  $\mathfrak{psu}(2, 2|4)$  algebra along with its reality conditions provided that

$$(\bar{\mathbf{a}}_{\alpha})^{\dagger} = \bar{\mathbf{b}}_{\dot{\alpha}}, \quad (\mathbf{a}^{\alpha})^{\dagger} = \mathbf{b}^{\dot{\alpha}}, \quad (\bar{\mathbf{c}}_a)^{\dagger} = \mathbf{c}^a. \quad (3.11)$$

The algebra extends to  $\mathfrak{u}(2, 2|4)$  by introducing a derivation  $\mathbf{B} \simeq \bar{\mathbf{c}}_a\mathbf{c}^a$  and a central charge  $\mathbf{C} \simeq -i\bar{\mathbf{a}}_{\alpha}\mathbf{a}^{\alpha} + i\mathbf{b}^{\dot{\alpha}}\bar{\mathbf{b}}_{\dot{\alpha}} + \bar{\mathbf{c}}_a\mathbf{c}^a$ . The constraint (3.9) is equivalent to the vanishing of the central charge, hence the above form a consistent representation of  $\mathfrak{psu}(2, 2|4)$ .

<sup>5</sup> The field strength  $\Gamma_{\mu\nu}$  with antisymmetric vector indices decomposes into two complex conjugate fields  $\Gamma_{\alpha\gamma}$  and  $\bar{\Gamma}_{\dot{\alpha}\dot{\gamma}}$  with symmetric spinor indices. Similarly, a real  $\mathfrak{so}(6)$  vector of fields  $\Phi_m$  is equivalent to a field  $\Phi_{ac}$  with antisymmetric  $\mathfrak{su}(4)$  indices and reality condition  $\Phi_{ac} = \frac{1}{2}\varepsilon_{abcd}\bar{\Phi}^{bd}$ .

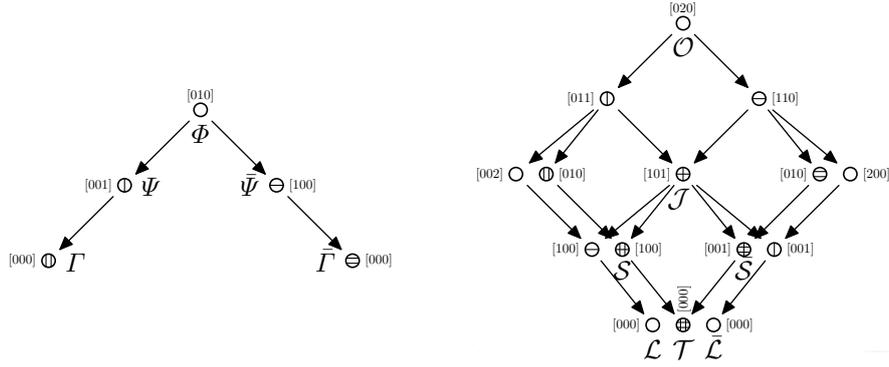

**Figure 3:** Field multiplet  $[0; 0; 0, 1, 0; 0; 0]$  (top component  $\Phi$  at  $d = 1$ ) and current multiplet  $[0; 0; 0, 2, 0; 0; 0]$  (top component  $\mathcal{O}$  at  $d = 2$ ). Each dot corresponds to a field of  $\mathfrak{su}(2, 2) \oplus \mathfrak{su}(4)$ : The two  $\mathfrak{su}(2)$  spins are indicated by horizontal/vertical bars, while the  $\mathfrak{su}(4)$  representation is indicated through Dynkin labels. SW/SE arrows correspond to the action of the Poincaré supercharges  $Q/\bar{Q}$ .

Note that the above construction remains applicable to the interacting theory for the sake of enumerating local composite operators: The r.h.s. of the equation of motion  $\partial \cdot \partial \Phi = \dots$  is not zero, but it is a product of fields which is already accounted for in the basis of local operators. Furthermore, to maintain proper gauge transformation properties, partial derivatives should be replaced by their covariant counterparts. Consequently, antisymmetries of derivatives are no longer excluded. They lead to commutators with the field strength, which are again accounted for in the basis of local operators. The only change in the quantum theory is that the representation on composite operators is deformed in a specific way, see the chapters [11]. For example, the scaling dimensions of composite operators generically receive continuous quantum corrections.

**Composite Operator Multiplets.** Composite operators are local products of the fundamental fields and hence they transform in tensor products of the above representation. Tensor products of lowest-weight representations typically decompose into sums of lowest-weight representations. Thus composite operators form multiplets each of which has a primary field.

The simplest non-trivial local operator is a traceless combination of two scalars<sup>6</sup>  $\mathcal{O}_{mn} = \Phi_m \Phi_n - \frac{1}{6} \delta_{mn} \Phi_p \Phi_p$  transforming as  $(\mathbf{1}, \mathbf{1}; \mathbf{20}; d = 2)$  under  $\mathfrak{sl}(2, \mathbb{C})$ ,  $\mathfrak{su}(4)$  and dilatations. It is annihilated by  $K, S, \bar{S}$  and hence it is the primary field for a multiplet of local operators, cf. Fig. 3. This multiplet is very important because it contains all the conserved currents for  $\mathcal{N} = 4$  SYM: the  $\mathfrak{su}(4)$  Noether current  $\mathcal{J}_{\mu n}^m$  transforming as  $(\mathbf{2}, \mathbf{2}; \mathbf{15}; d = 3)$ , the supersymmetry currents  $\mathcal{S}_{\mu\gamma}^a, \bar{\mathcal{S}}_{\mu b\gamma}$  transforming as  $(\mathbf{3}, \mathbf{2}; \mathbf{4}; d = 3.5)$  and  $(\mathbf{2}, \mathbf{3}; \bar{\mathbf{4}}; d = 3.5)$  and the energy-momentum tensor  $\mathcal{T}_{\mu\nu}$  transforming as  $(\mathbf{3}, \mathbf{3}; \mathbf{1}; d = 4)$ . The currents define all Noether charges for  $\mathfrak{psu}(2, 2|4)$ , e.g.

$$R^a{}_b \sim \int d^3x \mathcal{J}_{0n}^m, \quad Q^a{}_\gamma \sim \int d^3x \mathcal{S}_{0\gamma}^a, \quad P_\mu \sim \int d^3x \mathcal{T}_{0\mu}. \quad (3.12)$$

<sup>6</sup>In a gauge theory one should pick a gauge-invariant combination.

Moreover, the multiplet contains two scalars  $\mathcal{L}_{\text{kin}}, \mathcal{L}_{\text{top}}$  of dimension  $d = 4$ . These are exactly the parity-even kinetic and parity-odd topological parts of the Lagrangian density

$$\mathcal{L}_{\text{kin}} = -\frac{1}{4}\Gamma^{\mu\nu}\Gamma_{\mu\nu} + \frac{1}{2}\partial^\mu\Phi_m\partial_\mu\Phi_m + \dots, \quad \mathcal{L}_{\text{top}} = \frac{1}{8}\varepsilon^{\mu\nu\rho\sigma}\Gamma_{\mu\nu}\Gamma_{\rho\sigma}. \quad (3.13)$$

Next let us consider the labelling of representations for local operators. A lowest-weight representation is characterised by its primary field. The latter is characterised by the  $\mathfrak{sl}(2, \mathbb{C})$  spin, the  $\mathfrak{su}(4)$  representation and the conformal dimension  $d$ . For instance the primary field  $\Phi_m$  of the fundamental field representation transforms as  $(\mathbf{1}, \mathbf{1}; \mathbf{6}; d = 1)$  while the primary field  $\mathcal{O}_{mn}$  of the energy-momentum representation transforms as  $(\mathbf{1}, \mathbf{1}; \mathbf{20}; d = 2)$ . This characterisation is analogous to the discussion of unitary representations of  $\mathfrak{su}(4)$  in Sec. 2. The only difference is that the representation on the Taylor expansion of local operators is *not unitary*:<sup>7</sup> Surely  $\mathfrak{sl}(2, \mathbb{C})$  has no finite-dimensional unitary representations and also the dilatation generator  $D$  has *imaginary eigenvalues*, cf. (3.5). The point is that the Taylor components are not normalisable in the scalar product defining unitarity. Nevertheless, there is a one-to-one map between representations for local operators and unitary representations. It uses the following *complex* conformal transformation of Minkowski space

$$(t, x, y, z) \mapsto 2r^{-1}(iw, x, y, z) \text{ with } w = 1 - \frac{1}{4}x \cdot x \text{ and } r = 1 - it + \frac{1}{4}x \cdot x. \quad (3.14)$$

It maps the dilatation generator to  $D \mapsto iH$  where  $H$  is the generator of the decompactified  $\mathfrak{u}(1)$  discussed in Sec. 2, so the scaling dimension  $d$  maps to the energy eigenvalue  $E$ . Also the Lorentz algebra  $\mathfrak{sl}(2, \mathbb{C})$  is mapped to  $\mathfrak{su}(2) \oplus \mathfrak{su}(2)$  which is commonly used to classify the spin of fields in four dimensions. For all practical purposes the complex nature of the above conformal transformation is harmless in a perturbative quantum field theory where one commonly continues into complex time directions anyway. Therefore one often works with a dilatation generator  $D' = -iD$  whose spectrum is real and with  $\mathfrak{su}(2) \oplus \mathfrak{su}(2)$  Lorentz generators  $L'$  and  $\bar{L}'$ . Hence one can classify multiplets of local operators through unitary representation of  $\mathfrak{psu}(2, 2|4)$ . For instance the fundamental field and energy-momentum multiplets have Dynkin labels  $[0; 0; 0, 1, 0; 0; 0]$  and  $[0; 0; 0, 2, 0; 0; 0]$ , respectively. Note that, the representations  $[0; 0; 0, p, 0; 0; 0]$  are exceptionally short; the lowest state is annihilated by (at least) half of the supertranslations and hence the multiplet is called *half-BPS*.

**Multiplet Splitting.** Scaling dimensions  $d$  for unitary representations can take arbitrary real values above a certain unitarity bound, cf. (2.10). Therefore, the scaling dimension typically varies smoothly with the coupling constant of the quantum theory. However, representations at the lower bounds (2.10) have fewer components in general. For example, the scaling dimension for half-BPS representations  $[0; 0; 0, p, 0; 0; 0]$  is fixed to  $d = p$  and cannot depend on the coupling.

Nevertheless, there is an option to combine two or more short representations at the lower bound into a long representation whose scaling dimension can then be increased

---

<sup>7</sup>Thanks to Gleb Arutyunov and Stefan Fredenhagen for helpful discussions regarding this issue. See also [12] for implications on local operators, correlation functions, string states and their duality.

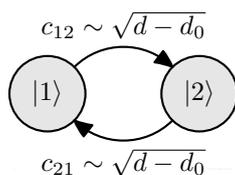

**Figure 4:** Multiplet splitting at the unitarity bound.

smoothly. This process called *multiplet joining* (or *multiplet splitting* in reverse) is an analog of the Higgs effect where a massless vector particle combines with a massless scalar particle to form a massive vector. The set of local operators in  $\mathcal{N} = 4$  SYM has the exceptional feature that almost all short multiplets of the classical theory can be combined into long multiplets in the quantum theory. Only few short multiplets have no partner (such as all half-BPS multiplets  $[0; 0; 0, p, 0; 0; 0]$ ) and their scaling dimensions are therefore protected from quantum corrections.

Multiplet splitting takes place at the unitarity bound, cf. Fig. 4: Consider a long multiplet which decomposes into two short multiplets at  $d = d_0$ . The representation of some generator  $J$  acts on states  $|1\rangle, |2\rangle$  of the submultiplets qualitatively as follows

$$J|1\rangle = c_{12}|2\rangle + \dots, \quad J|2\rangle = c_{21}|1\rangle + \dots \quad (3.15)$$

The algebra relations imply that  $c_{12}c_{21} \sim (d - d_0)$  because splitting at  $d = d_0$  requires  $c_{12} = 0$  or  $c_{21} = 0$ . Unitarity furthermore implies  $c_{12} \sim c_{21}^*$  hence  $c_{12} \sim c_{21} \sim \sqrt{d - d_0}$ . Therefore at  $d = d_0$  the reality properties of the representation necessarily change, i.e.  $d \geq d_0$  is a unitarity bound.

## 4 Isometries of the $AdS_5 \times S^5$ Superspace

Supersymmetric strings require a ten-dimensional supergravity background as the space on which they can consistently propagate. Next to a flat spacetime there exist two more maximal supersymmetric backgrounds. One of them is the  $AdS_5 \times S^5$  superspace. According to the AdS/CFT correspondence this string theory is exactly dual to conformal  $\mathcal{N} = 4$  SYM on Minkowski space being the boundary of  $AdS_5 \times S^5$ , see [13] for an extended review. In the following we shall discuss this superspace, its boundary and its isometries which are generated by the algebra  $\mathfrak{psu}(2, 2|4)$ .

**AdS Spacetime.** We start by defining the anti de Sitter spacetime  $AdS_{n+1}$  leaving  $n$  generic for the time being. This  $(n + 1)$ -dimensional spacetime has homogeneous negative curvature in close analogy to hyperbolic space  $H^{n+1}$ . Similar space(time)s with homogeneous positive curvature are the de Sitter spacetime  $dS_{n+1}$  and the sphere  $S^{n+1}$  (to which we shall frequently contrast  $AdS_{n+1}$ ). There are several equivalent constructions which we shall now review. One can embed it into  $\mathbb{R}^{n,2}$  as single-shell hyperboloid specified by

$$AdS_{n+1} = \{X \in \mathbb{R}^{n,2} | X \cdot X = -1\}, \quad S^{n+1} = \{Y \in \mathbb{R}^{n+2} | Y \cdot Y = +1\}. \quad (4.1)$$

The metric is induced from the flat metric on  $\mathbb{R}^{n,2}$  losing one time-like direction due to the condition  $X \cdot X = -1$ . An obvious alternative description uses time-like rays  $[X]$  in  $\mathbb{R}^{n,2}$

$$AdS_{n+1} = \{[X] \mid X \in \mathbb{R}^{n,2}, X \cdot X < 0\}, \quad \text{where } [X] = [Y] \text{ iff } X = zY \text{ with } z \in \mathbb{R}^+. \quad (4.2)$$

The points  $X$  or rays  $[X]$  transform canonically under  $SO(n, 2)$  and they are stabilised by a  $SO(n, 1)$  subgroup. Consequently,  $AdS_{n+1}$  can be viewed as the coset space

$$AdS_{n+1} = SO(n, 2)/SO(n, 1), \quad S^{n+1} = SO(n + 2)/SO(n + 1). \quad (4.3)$$

Thus the group of isometries of  $AdS_5$  is  $SO(4, 2)$ . Due to the presence of fermions, one should promote the orthogonal to spin groups. For  $n = 4$  the group identities  $Spin(4, 2) = SU(2, 2)$  and  $Spin(4, 1) = Sp(1, 1)$  furthermore allow to write

$$AdS_5 = SU(2, 2)/Sp(1, 1), \quad S^5 = SU(4)/Sp(2). \quad (4.4)$$

**Coordinates.** There exist several choices of coordinates on  $AdS_{n+1}$  which are useful in different situations. One is an analog of angle coordinates on the sphere: Using trigonometric functions it is straight-forward to construct a vector  $X \in \mathbb{R}^{n,2}$  with  $X \cdot X = -1$  (we shall use the signature  $- - + \dots +$ )

$$X = (\sec \sigma \cos \tau, \sec \sigma \sin \tau, \tan \sigma \Omega), \quad (4.5)$$

where  $\Omega \in S^{n-1} \subset \mathbb{R}^n$  is a unit vector and  $\rho \in [0, \frac{1}{2}\pi)$ ,  $\tau \in [0, 2\pi)$ . The induced metric reads

$$ds^2 = \sec^2 \sigma (d\sigma^2 - d\tau^2) + \tan^2 \sigma d\Omega^2. \quad (4.6)$$

On the coordinates  $\Omega$  and  $\tau$  the maximal compact subgroup  $SO(n) \times SO(2)$  acts canonically. The remaining  $2n$  directions of  $SO(n, 2)$  act non-trivially.

A useful alternative is Poincaré-type coordinates  $x \in \mathbb{R}^{n-1,1}$ ,  $y \in \mathbb{R}^+$  with the  $\mathbb{R}^{n,2}$  embedding

$$X = y^{-1} \left( \frac{1}{2}(x \cdot x + y^2 + 1), x, \frac{1}{2}(x \cdot x + y^2 - 1) \right). \quad (4.7)$$

These coordinates reveal the conformally flat nature of the  $AdS_{n+1}$  metric

$$ds^2 = y^{-2}(dx \cdot dx + dy^2). \quad (4.8)$$

A Poincaré subgroup of  $SO(n, 2)$  acts on the  $x$  while the corresponding dilatations act as simultaneous scaling of  $x$  and  $y$  by the same factor. Special conformal transformations mix up  $x$  and  $y$  non-trivially

$$\delta x \sim x(\epsilon \cdot x) - \frac{1}{2}\epsilon(x \cdot x + y^2), \quad \delta y \sim y(\epsilon \cdot x). \quad (4.9)$$

Finally we note that isometries of  $AdS_{n+1}$  also include reflections in  $\mathbb{R}^{n,2}$ . For example, a reflection in the first component of the above  $X$  corresponds to an inversion of time  $\tau$  or a conformal inversion of the coordinates  $(x, y) \in \mathbb{R}^{n,1}$

$$\tau \mapsto \pi - \tau, \quad (x, y) \mapsto -\frac{(x, y)}{x \cdot x + y^2}. \quad (4.10)$$

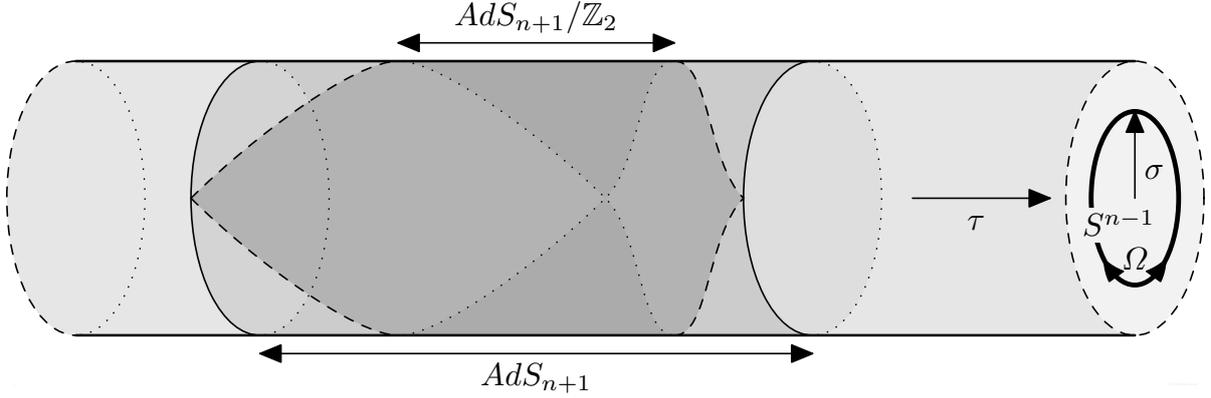

**Figure 5:** Anti de Sitter space. The infinitely extended solid cylinder represents the universal cover  $\widetilde{AdS}_{n+1}$  (light grey).  $AdS_{n+1}$  is obtained by identifying segments of time  $\Delta\tau = 2\pi$  (medium grey). The Poincaré patch  $AdS_{n+1}/\mathbb{Z}_2$  covers half of  $AdS_{n+1}$  (dark grey). The boundary  $\partial\widetilde{AdS}_{n+1} = \mathbb{R} \times S^{n-1}$  is the outer shell of the cylinder.

**Universal Cover.** In (4.5) it is clear that the time coordinate  $\tau$  is periodic:  $\tau \equiv \tau + 2\pi$ . Closed time-like curves are inconvenient for physical applications, but luckily they can be removed by lifting to the *universal cover*  $\widetilde{AdS}_{n+1}$  on which a physical model can be defined. Hence the coordinates  $(\tau, \sigma, \Omega)$  with non-periodic  $\tau \in \mathbb{R}$  define a global chart for  $\widetilde{AdS}_{n+1}$  which has the topology of an infinitely extended solid cylinder, see Fig. 5. The natural embedding into  $\mathbb{R}^{n,2}$  identifies  $\tau$  with  $\tau + 2\pi\mathbb{Z}$  and leads to  $AdS_{n+1}$ . Moreover, the Poincaré-type coordinates in (4.7) cover only half of  $AdS_{n+1}$ . More precisely, if  $\theta$  is the angle between  $\Omega$  and  $\Omega_0 = (0, \dots, 0, 1)$ , then the Poincaré patch is a wedge of the cylinder around  $\tau = 0$  defined by the inequality  $\cos\tau > \sin\sigma \cos\theta$ , cf. Fig. 5.

The universal cover  $\widetilde{AdS}_{n+1}$  also has a direct formulation as a coset: The groups  $SO(n, 2)$  and  $SU(2, 2)$  have non-trivial coverings because their maximal compact subgroups contain the non-simply connected factors  $SO(2)$  and  $U(1)$ , respectively. The covering of  $AdS_{n+1}$  is thus defined as

$$\widetilde{AdS}_{n+1} = \widetilde{SO}(n, 2)/\text{Spin}(n, 1), \quad \widetilde{AdS}_5 = \widetilde{SU}(2, 2)/\text{Sp}(1, 1). \quad (4.11)$$

The universal covers  $\widetilde{SO}(n, 2)$  and  $\widetilde{SU}(2, 2)$  are physically relevant because they allow representations with arbitrary real energies as compared to integer values for  $SO(n, 2)$  and  $SU(2, 2)$ .

**Boundary of  $AdS$ .** The boundary  $\partial AdS_{n+1}$  of  $AdS_{n+1}$  is a  $n$ -dimensional spacetime. It can be viewed as the space of light-like rays  $[X]$  in  $\mathbb{R}^{n,2}$ , cf. (4.2)

$$\partial AdS_{n+1} = \{[X] \mid X \in \mathbb{R}^{n,2}, X \cdot X = 0\}, \quad \text{where } [X] = [Y] \text{ iff } X = zY \text{ with } z \in \mathbb{R}^+. \quad (4.12)$$

In the above coordinates of  $AdS_{n+1}$  it is located at  $\sigma = \frac{1}{2}\pi$  or at  $y = 0$ . From (4.12) the topology of the  $AdS_{n+1}$  boundary follows

$$\partial AdS_{n+1} = S^1 \times S^{n-1}, \quad \partial\widetilde{AdS}_{n+1} = \mathbb{R} \times S^{n-1}. \quad (4.13)$$

While the topology  $S^1$  of time in  $\partial AdS_{n+1}$  is periodic, the boundary of the universal cover  $\widetilde{AdS}_{n+1}$  has no closed time-like curves. Consequently it is the outer shell of the solid cylinder  $\widetilde{AdS}_{n+1}$ . The metric of  $\mathbb{R}^{n,2}$  can be used to measure angles, but not distances on the boundary, hence it merely induces a *conformal* metric on  $\partial AdS_{n+1}$

$$ds^2 \simeq -d\tau^2 + d\Omega^2 \simeq dx \cdot dx. \quad (4.14)$$

In other words the boundary is conformally flat. This is manifest in the Poincaré coordinates (4.7)  $x \in \mathbb{R}^{n-1,1}$  (with  $y = 0$ ) on which  $\text{SO}(n, 2)$  acts by conformal transformations (3.1).

Note that the boundary is at infinite distance to all points of  $AdS_{n+1}$  (similarly to hyperbolic space  $H^{n+1}$  and its boundary  $\partial H^{n+1} = S^n$ ). Nevertheless the boundary can interact with the bulk at finite times: A light ray originating from  $\sigma = \tau = 0$  reaches the boundary  $\sigma = \frac{1}{2}\pi$  at  $\tau = \frac{1}{2}\pi$ , cf. (4.6). From there it travels back to the point  $\sigma = 0$  at time  $\tau = \pi$ .

**$AdS_5 \times S^5$  Superspace.** The  $AdS_5 \times S^5$  superspace is an extension of  $\widetilde{AdS}_5$  and  $S^5$  by 32 fermionic directions. It is very conveniently expressed as a coset space: The groups  $\text{SU}(2, 2)$  and  $\text{SU}(4)$  for the definition  $AdS_5$  and  $S^5$  in (4.4) combine into the supergroup  $\text{PSU}(2, 2|4)$  which has 32 fermionic directions. Dividing by the bosonic denominator groups in (4.4) one obtains the full superspace

$$\widetilde{AdS}_5 \times S^5 \times \mathbb{C}^{0|16} = \frac{\widetilde{\text{PSU}}(2, 2|4)}{\text{Sp}(1, 1) \times \text{Sp}(2)}. \quad (4.15)$$

The curvature radii of the  $\widetilde{AdS}_5$  and  $S^5$  subspaces are equal but opposite, such that the overall scalar curvature vanishes.

In view of the AdS/CFT correspondence, we shall consider the boundary of this superspace. The sphere  $S^5$  is closed and the fermionic space  $\mathbb{C}^{0|16}$  has trivial topology such that the overall boundary originates from the  $\widetilde{AdS}_5$  factor alone. In the spherical coordinates (4.5), it resides at  $\sigma = \frac{1}{2}\pi$ . Let us approach the boundary with a codimension-one surface at a fixed  $\sigma$  near  $\sigma = \frac{1}{2}\pi$ . This surface has the topology  $\mathbb{R} \times S^3 \times S^5 \times \mathbb{C}^{0|16}$ . According to (4.6) the radius of the  $S^3$  is  $\tan \sigma$  while the radius of the  $S^5$  factor is constantly 1. Hence at the boundary the  $S^5$  shrinks to a point in comparison to the  $S^3$ . This means that, for some physical purposes, the boundary of the  $AdS_5 \times S^5$  spacetime is effectively the boundary of  $\widetilde{AdS}_5$  alone, i.e.  $\mathbb{R} \times S^3$ . (A patch of) this spacetime is conformally equivalent to Minkowski space  $\mathbb{R}^{3,1}$ . The boundary of the  $AdS_5 \times S^5$  superspace has additional fermionic coordinates to make up a conformally flat  $\mathcal{N} = 4$  superspace.

**Coset Space Sigma Model.** In string theory isometries of the background spacetime become conserved Noether charges. This becomes obvious in the construction of a coset space sigma model, see the chapter [14]. Thus the group of global symmetries of superstrings on  $AdS_5 \times S^5$  is  $\widetilde{\text{PSU}}(2, 2|4)$ . It should be noted that the coset space sigma model construction not only provides the correct target space metric, but also a non-trivial superspace torsion and five-form supergravity flux coupling to the string worldsheet.

The  $AdS_5 \times S^5$  coset has a couple of exceptional features which make it a suitable background for a consistent quantum string theory: First of all, it has 10 bosonic and 32 fermionic coordinates. Furthermore the worldsheet theory on this coset has 16 kappa symmetries to reduce the effective number of fermionic coordinates to 16. Finally, the Killing form for  $PSU(2, 2|4)$  vanishes identically as required for conformal symmetry on the worldsheet. Only few cosets share these features, cf. [15].

## References

- [1] M. F. Sohnius and P. C. West, “*Conformal Invariance in  $\mathcal{N} = 4$  Supersymmetric Yang-Mills Theory*”, Phys. Lett. B100, 245 (1981). • S. Mandelstam, “*Light Cone Superspace and the Ultraviolet Finiteness of the  $\mathcal{N} = 4$  Model*”, Nucl. Phys. B213, 149 (1983). • L. Brink, O. Lindgren and B. E. W. Nilsson, “ *$\mathcal{N} = 4$  Yang-Mills Theory on the Light Cone*”, Nucl. Phys. B212, 401 (1983). • P. S. Howe, K. S. Stelle and P. K. Townsend, “*Miraculous Ultraviolet Cancellations in Supersymmetry Made Manifest*”, Nucl. Phys. B236, 125 (1984).
- [2] E. D’Hoker and D. Z. Freedman, “*Supersymmetric gauge theories and the AdS/CFT correspondence*”, hep-th/0201253.
- [3] N. Beisert et al., “*Review of AdS/CFT Integrability: An Overview*”, arxiv:1012.3982.
- [4] J. F. Cornwell, “*Group Theory in Physics, Volume III: Supersymmetries and Infinite-Dimensional Algebras*”, Academic Press (1989), London, UK, Techniques of Physics 10. • L. Frappat, P. Sorba and A. Sciarrino, “*Dictionary on Lie Algebras and Superalgebras*”, Academic Press (2000), London, UK. • L. Frappat, P. Sorba and A. Sciarrino, “*Dictionary on Lie Superalgebras*”, hep-th/9607161.
- [5] J. F. Cornwell, “*Group Theory in Physics: An Introduction*”, Academic Press (1997), London, UK.
- [6] N. Beisert, “*The  $su(2/3)$  dynamic spin chain*”, Nucl. Phys. B682, 487 (2004), hep-th/0310252.
- [7] V. K. Dobrev and V. B. Petkova, “*All Positive Energy Unitary Irreducible Representations of Extended Conformal Supersymmetry*”, Phys. Lett. B162, 127 (1985).
- [8] S. Sternberg, “*Group theory and physics*”, Cambridge University Press (1994), Cambridge, UK.
- [9] G. Mack and A. Salam, “*Finite component field representations of the conformal group*”, Ann. Phys. 53, 174 (1969).
- [10] M. Günaydin and N. Marcus, “*The Spectrum of the  $S^5$  Compactification of the Chiral  $\mathcal{N} = 2$ ,  $D = 10$  Supergravity and the Unitary Supermultiplets of  $U(2,2/4)$* ”, Class. Quant. Grav. 2, L11 (1985).
- [11] J. A. Minahan, “*Review of AdS/CFT Integrability, Chapter I.1: Spin Chains in  $\mathcal{N} = 4$  SYM*”, arxiv:1012.3983. • C. Sieg, “*Review of AdS/CFT Integrability, Chapter I.2: The spectrum from perturbative gauge theory*”, arxiv:1012.3984. • A. Rej, “*Review of AdS/CFT Integrability, Chapter I.3: Long-range spin chains*”, arxiv:1012.3985.
- [12] R. A. Janik, P. Surowka and A. Wereszczynski, “*On correlation functions of operators dual to classical spinning string states*”, JHEP 1005, 030 (2010), arxiv:1002.4613.

## Chapter VI.1: Superconformal Symmetry

- [13] O. Aharony, S. S. Gubser, J. M. Maldacena, H. Ooguri and Y. Oz, “*Large N field theories, string theory and gravity*”, Phys. Rept. 323, 183 (2000), [hep-th/9905111](#).
- [14] M. Magro, “*Review of AdS/CFT Integrability, Chapter II.3: Sigma Model, Gauge Fixing*”, [arxiv:1012.3988](#).
- [15] K. Zarembo, “*Strings on Semisymmetric Superspaces*”, JHEP 1005, 002 (2010), [arxiv:1003.0465](#).

# Review of AdS/CFT Integrability, Chapter VI.2: Yangian Algebra

ALESSANDRO TORRIELLI

*Institute for Theoretical Physics and Spinoza Institute,  
Utrecht University, 3508 TD Utrecht, The Netherlands*

*and*

*Department of Mathematics, University of York  
Heslington, York, YO10 5DD, U.K.*

alessandro.torrielli@york.ac.uk

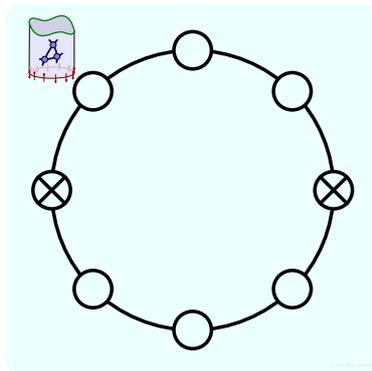

**Abstract:** We review the study of Hopf algebras, classical and quantum R-matrices, infinite-dimensional Yangian symmetries and their representations in the context of integrability for the  $\mathcal{N} = 4$  vs  $AdS_5 \times S^5$  correspondence.

## 1 Introduction

Despite the success obtained so far by the integrability program, many questions are left unanswered. Most notably, the problem remains of understanding what is the non-perturbative definition of the model that seems to reproduce so well all the available data [1]. Answering this question may also be important for a deeper understanding of the finite-size problem and its solution. An essential role in this respect is played by the symmetries of the factorized S-matrix. A clear sign is the presence of a Hopf algebra [2, 3], then promoted to a Yangian [4]. In relativistic integrable quantum field theories, symmetries like the Yangian or quantum affine algebras completely determine the tensorial part of the S-matrix, up to an overall scalar factor. They also entail important consequences for the transfer matrices and for the Bethe equations [5]. This happens also in the AdS/CFT case [6, 7]. However, the AdS/CFT Yangian has very distinctive features still preventing a full mathematical understanding. For instance, there exists an additional Yangian symmetry of the S-matrix [8, 9] with properties not yet entirely understood, pointing to a new type of quantum group<sup>1</sup>. In order to give an ultimate solution of the AdS/CFT integrable system, one needs to understand the features of this novel quantum group, and of the associated quantum integrable model. The scope of this review is illustrating such group-theory aspects.

## 2 Hopf Algebras

Let us begin by recalling a few concepts in the theory of Hopf algebras, as these are very important algebraic structures appearing in the context of integrable models. We will attempt to motivate these concepts mostly from the physical viewpoint, and refer the reader to standard textbooks, such as [11], for a thorough treatment.

The starting point is the algebra of symmetries of a system. Let us consider the case when this algebra is a Lie (super)algebra  $\mathfrak{g}$ , and let us also consider its universal enveloping algebra  $A \equiv U(\mathfrak{g})$ . This step allows us to ‘multiply’ generators, besides taking the Lie bracket. In such universal enveloping algebra there is a *unit element*  $\mathbb{1}$  with respect to the *multiplication map*  $\mu$ . We think about multiplication as  $\mu : A \otimes A \rightarrow A$ , and we introduce a *unit map*  $\eta : \mathbb{C} \rightarrow A$ . A few compatibility conditions on these maps guarantee that we are dealing with the physical symmetries of, say, a single-particle system.

In order to treat multiparticle states, we equip our algebra with two more maps, and obtain a *bialgebra* structure. One map is the *coproduct*  $\Delta : A \rightarrow A \otimes A$ , which tells us how symmetry generators act on two-particle states. The other map is the *counit*  $\epsilon : A \rightarrow \mathbb{C}$ . A list of compatibility axioms ensures that these maps are consistent with the (Lie) (super)algebra structure, so we can safely think of them as the symmetries we started with, just acting on a Fock space. In fact, for a generic  $n$ -particle state, we can generalize the action of the coproduct as the composition  $\Delta^n = \dots(\Delta \otimes \mathbb{1} \otimes \mathbb{1})(\Delta \otimes \mathbb{1})\Delta$ . The *coassociativity* axiom

$$(\Delta \otimes \mathbb{1})\Delta = (\mathbb{1} \otimes \Delta)\Delta \tag{2.1}$$

---

<sup>1</sup>The relation with Yangian symmetry in  $n$ -p.t amplitudes [10] is also a fascinating problem.

guarantees that a change in the positions of the  $\Delta$ 's in the sequence  $\Delta^n$  is immaterial.

One more map turns our structure into a *Hopf algebra*. This map is the *antipode*  $\Sigma : A \rightarrow A$ , which is needed to define antiparticles (conjugated representations of the symmetry algebra). Therefore, the antipode should also be consistent with the (Lie) (super)algebra structure<sup>2</sup>, and be compatible with the coproduct action. If a bialgebra admits an antipode, it is unique.

In the scattering theory of integrable models, the fundamental object encoding the dynamics is the two-particle S-matrix, which exchanges the momenta of the two particles, and reshuffles their colors. One has therefore the possibility of defining the coproduct action as acting on, say, *in* states. Likewise, the composed map  $P\Delta \equiv \Delta^{op}$ , with  $P$  the permutation map, will act on *out* states. The discovery of quantum groups revealed that these two actions need not be the same. They are the same only for *cocommutative* Hopf algebras, one example being the Leibniz rule  $\Delta(a) = a \otimes \mathbb{1} + \mathbb{1} \otimes a$  one normally associates with local actions. In general, coproducts can be more complicated, as we will amply see in what follows<sup>3</sup>.

However, as  $\Delta$  and  $\Delta^{op}$  produce tensor product representations of the same dimensions, they may be related by conjugation *via* an invertible element (the S-matrix itself). The Hopf-algebra is then said to be *quasi-cocommutative*, and, if the S-matrix satisfies an additional condition ('bootstrap' [12]), it is called *quasi-triangular*. The S-matrix must also be compatible with the antipode map, a condition that in physical terms goes under the name of *crossing* symmetry. One can prove that bootstrap implies that the S-matrix satisfies the Yang-Baxter equation and the crossing condition.

As one can easily realize, the framework of Hopf algebras is particularly suitable for dealing with integrable scattering. Integrability reduces the scattering problem to an algebraic procedure, and the axioms we have been discussing just formalize that procedure. However, instead of being a mere translation, the mathematical framework of Hopf algebras provides a set of powerful theorems that unify the treatment of arbitrary representations. To this purpose, the notion of *universal R-matrix* is very important. This is an abstract solution to the quasi-cocommutativity condition, purely expressed in terms of algebra generators. This solution gives an expression for the S-matrix which is therefore free from a particular representation, at the same time being valid in any of them upon plug-in. As we will explicitly see in what follows, the study of the properties of the universal R-matrix reveals a big deal about the structure of the (hidden) symmetry algebra of the integrable system.

### 3 Yangians

Let  $\mathfrak{g}$  be a finite dimensional simple Lie algebra with generators  $\mathfrak{J}^A$ , structure constants  $f_C^{AB}$  defined by  $[\mathfrak{J}^A, \mathfrak{J}^B] = f_C^{AB} \mathfrak{J}^C$  and a non-degenerate invariant bilinear form  $\kappa^{AB}$ . The Yangian  $\mathcal{Y}(\mathfrak{g})$  of  $\mathfrak{g}$  is a deformation of the universal enveloping algebra of half of the loop

<sup>2</sup>Being the antipode connected to conjugation, one imposes  $\Sigma(ab) = (-)^{ab} \Sigma(b) \Sigma(a)$ , where multiplication is *via* the map  $\mu$ .

<sup>3</sup>This is another reason why the Coleman-Mandula theorem does not apply to the S-matrices we will be discussing (besides being in 1 + 1 dimensions).

algebra of  $\mathfrak{g}$ . The loop algebra is defined by (4.5), "half" meaning non-negative indices  $m, n$ . Drinfeld gave two isomorphic realizations of the Yangian<sup>4</sup>. The first realization [18] is as follows.  $\mathcal{Y}(g)$  is defined by relations between level zero generators  $\mathfrak{J}^A$  and level one generators  $\widehat{\mathfrak{J}}^A$ :

$$[\mathfrak{J}^A, \mathfrak{J}^B] = f_C^{AB} \mathfrak{J}^C, \quad [\mathfrak{J}^A, \widehat{\mathfrak{J}}^B] = f_C^{AB} \widehat{\mathfrak{J}}^C. \quad (3.1)$$

The generators of higher levels are derived recursively by computing the commutant, subject to the following Serre relations (for  $\mathfrak{g} \neq \mathfrak{su}(2)$ ):

$$[\widehat{\mathfrak{J}}^A, [\widehat{\mathfrak{J}}^B, \mathfrak{J}^C]] + [\widehat{\mathfrak{J}}^B, [\widehat{\mathfrak{J}}^C, \mathfrak{J}^A]] + [\widehat{\mathfrak{J}}^C, [\widehat{\mathfrak{J}}^A, \mathfrak{J}^B]] = \frac{1}{4} f_D^{AG} f_E^{BH} f_F^{CK} f_{GHK} \mathfrak{J}^{\{D} \mathfrak{J}^E \mathfrak{J}^F\}}. \quad (3.2)$$

Indices are raised (lowered) with  $\kappa^{AB}$  (its inverse). The Yangian is equipped with a Hopf algebra structure. The coproduct is uniquely determined for all generators by specifying it on the level zero and one generators as follows:

$$\Delta(\mathfrak{J}^A) = \mathfrak{J}^A \otimes \mathbb{1} + \mathbb{1} \otimes \mathfrak{J}^A, \quad \Delta(\widehat{\mathfrak{J}}^A) = \widehat{\mathfrak{J}}^A \otimes \mathbb{1} + \mathbb{1} \otimes \widehat{\mathfrak{J}}^A + \frac{1}{2} f_{BC}^A \mathfrak{J}^B \otimes \mathfrak{J}^C. \quad (3.3)$$

Antipode and counit are easily obtained from the Hopf algebra definitions<sup>5</sup>. We will not present here Drinfeld's second realization of the Yangian [19], which is suitable for constructing the universal R-matrix [20]. It suffices to say that it explicitly solves the recursion implicit in the first realization.

### 3.1 The $\mathfrak{psu}(2, 2|4)$ Yangian

Generically, the level zero local generators are realized on spin-chains as

$$\mathfrak{J}^A = \sum_k \mathfrak{J}^A(k), \quad k \in \{\text{spin-chain sites}\}. \quad (3.4)$$

For infinite length, the level one Yangian generators are bilocal combinations

$$\widehat{\mathfrak{J}}^A = \sum_{k < n} f_{BC}^A \mathfrak{J}^B(k) \mathfrak{J}^C(n). \quad (3.5)$$

The relationship with the coproduct (3.3) will be clear later when discussing the Principal Chiral Model. Level  $n$  generators are  $n + 1$ -local expressions. At finite length, boundary effects usually prevent from having conserved charges such as (3.5), while Casimirs of the Yangian may still be well-defined. We refer to [21] for a review.

The  $\mathcal{N} = 4$  SYM spin-chain is based on the superconformal symmetry algebra  $\mathfrak{psu}(2, 2|4)$ . The Yangian charges for infinite length have been constructed, at leading

<sup>4</sup>The reader is referred to *e.g.* [11, 13–15] for a thorough treatment. We will not discuss the 'RTT' realization, see *e.g.* [16, 15]. For generalizations to Lie superalgebras, see *e.g.* [17].

<sup>5</sup>*Via* a rescaling of the algebra generators, one can make a parameter (say,  $\hbar$ ) appear in front of the mixed term  $\frac{1}{2} f_{BC}^A \mathfrak{J}^B \otimes \mathfrak{J}^C$  in the Yangian coproduct (3.3). This parameter is sometimes useful as it can be made small, as in the classical limit, cf. section 3.

order in the 't Hooft coupling, in [22]. The Serre relations for the relevant representations have been proved in [23]. In [24] the first two Casimirs of the Yangian are computed and identified with the first two local abelian Hamiltonians of the spin-chain with periodic boundary conditions.

Perturbative corrections to the Yangian charges in subsectors have been studied in [25–27]. The integrable structure of spin-chains with long-range (LR) interactions, like the one emerging from gauge perturbation theory, lies outside the established picture [28], but a large class of LR spin-chains has been shown to display Yangian symmetries, see also [29]. In absence of other standard tools, Yangian symmetry provides a formal proof of integrability order by order in perturbation theory. The two-loop expression of the Yangian (3.5) for the  $\mathfrak{su}(2|1)$  sector has been derived in [26]. In [27], a large degeneracy of states in the  $\mathfrak{psu}(1,1|2)$  sector is explained *via* nonlocal charges related to the loop-algebra of the  $\mathfrak{su}(2)$  automorphism of  $\mathfrak{psu}(1,1|2)$ . Further references include [30]. For a recent review we recommend [31].

Higher non-local charges analogous to (3.5) emerge in 2D classically integrable field theories [32]. If not anomalous, their quantum versions [33] form a Yangian. *E.g.*, for the Principal Chiral Model

$$\frac{d}{dt} \widehat{\mathfrak{J}}^A = \frac{d}{dt} \int_{-\infty}^{\infty} dx \left[ \epsilon_{\mu\nu} J^{\nu,A} + \frac{1}{2} f_{BC}^A J_{\mu}^B \int_{-\infty}^x dx' J_0^C(x') \right] = 0, \quad (3.6)$$

where  $\mathfrak{J}^A$  are Noether currents for the global (left or right) group multiplication.

The classical integrability of the Green-Schwarz superstring sigma model in the  $\text{AdS}_5 \times \text{S}^5$  background has been established in [34]. The corresponding infinite set of nonlocal classically-conserved charges is found according to a logic very close to the one described above (similar observations for the bosonic part of the action were made in [35]). Further work can be found in [36].

We conclude with a remark on the Hopf algebra structure of the nonlocal charges. How charges (3.6) can give rise to the coproduct (3.3) is shown in [37]. A semiclassical treatment [38] is as follows. One imagines two well-separated solitonic excitations as the classical version of a scattering state. Soliton 1 is localized in the region  $(-\infty, 0)$ , soliton 2 in  $(0, \infty)$ . Defining the *semiclassical action* of a charge on such solution as evaluation on the profile, one splits the current-integration in individual domains relevant for each of the two solitons, respectively:

$$\begin{aligned} \widehat{\mathfrak{J}}_{|profile}^A &= \int_{-\infty}^{\infty} dx J_0^A|_{profile} = \int_{-\infty}^0 dx J_0^A + \int_0^{\infty} dx J_0^A \longrightarrow \Delta(\mathfrak{J}^A) = \mathfrak{J}^A \otimes \mathbb{1} + \mathbb{1} \otimes \mathfrak{J}^A, \\ \widehat{\mathfrak{J}}_{|profile}^A &= \left[ \int_{-\infty}^0 dx J_1^A + \frac{1}{2} f_{BC}^A \int_{-\infty}^0 dx J_0^B(x) \int_{-\infty}^x dy J_0^C(y) \right] \\ &\quad + \left[ \int_0^{\infty} dx J_1^A + \frac{1}{2} f_{BC}^A \int_0^{\infty} dx J_0^B(x) \int_0^x dy J_0^C(y) \right] \\ &\quad + \frac{1}{2} f_{BC}^A \int_0^{\infty} dx J_0^B(x) \int_{-\infty}^0 dy J_0^C(y). \end{aligned} \quad (3.7)$$

Upon quantization in absence of anomalies this gives (3.3) on the Hilbert space.

## 3.2 The centrally-extended $\mathfrak{psu}(2|2)$ Yangian

In the previous section, we have described how algebraic structures related to integrability arise at the two perturbative ends of the AdS/CFT correspondence. To fully exploit these powerful symmetries one needs to take a further step, which allows to go beyond the perturbative regimes. One introduces the choice of a vacuum state, and considers

excitations upon this vacuum. This choice breaks the full  $\mathfrak{psu}(2, 2|4)$  symmetry down to a subalgebra. The excitations carry the quantum numbers of the unbroken symmetry, and they scatter *via* an integrable S-matrix.

The choice that is normally made is, for instance, to consider a string (composite operator) of  $Z$  fields (one of the three complex combinations of the six scalar fields of  $\mathcal{N} = 4$  SYM) as the vacuum state. The unbroken symmetry consists then of two copies of the  $\mathfrak{psu}(2|2)$  Lie superalgebra, which receive central extensions through quantum corrections. The same algebra appears on the string theory side. The excitations carrying the unbroken quantum numbers are called *magnons*, in analogy to the theory of spin-chains and magnetism.

### 3.2.1 The Hopf algebra of the S-matrix

Upon choosing a vacuum, the residual symmetry carried by the magnon excitations is (two copies of) the centrally extended  $\mathfrak{psu}(2|2)$  Lie superalgebra (or  $\mathfrak{psu}(2|2)_c$ ):

$$\begin{aligned}
 [\mathbb{L}_a^b, \mathbb{J}_c] &= \delta_c^b \mathbb{J}_a - \frac{1}{2} \delta_a^b \mathbb{J}_c, & [\mathbb{R}_\alpha^\beta, \mathbb{J}_\gamma] &= \delta_\gamma^\beta \mathbb{J}_\alpha - \frac{1}{2} \delta_\alpha^\beta \mathbb{J}_\gamma, \\
 [\mathbb{L}_a^b, \mathbb{J}^c] &= -\delta_a^c \mathbb{J}^b + \frac{1}{2} \delta_a^b \mathbb{J}^c, & [\mathbb{R}_\alpha^\beta, \mathbb{J}^\gamma] &= -\delta_\alpha^\gamma \mathbb{J}^\beta + \frac{1}{2} \delta_\alpha^\beta \mathbb{J}^\gamma, \\
 \{\mathbb{Q}_\alpha^a, \mathbb{Q}_\beta^b\} &= \epsilon_{\alpha\beta} \epsilon^{ab} \mathbb{C}, & \{\mathbb{S}_\alpha^a, \mathbb{S}_b^\beta\} &= \epsilon^{\alpha\beta} \epsilon_{ab} \mathbb{C}^\dagger, \\
 \{\mathbb{Q}_\alpha^a, \mathbb{S}_b^\beta\} &= \delta_b^a \mathbb{R}_\alpha^\beta + \delta_\alpha^\beta \mathbb{L}_b^a + \frac{1}{2} \delta_b^a \delta_\alpha^\beta \mathbb{H}.
 \end{aligned} \tag{3.8}$$

The generators  $\mathbb{R}_\alpha^\beta$  and  $\mathbb{L}_a^b$  form the two  $\mathfrak{su}(2)$  subalgebras which, together with the central elements  $\{\mathbb{H}, \mathbb{C}, \mathbb{C}^\dagger\}$ , form the bosonic part of  $\mathfrak{psu}(2|2)_c$ . The names are reminiscent of the unbroken  $R$ - and Lorentz symmetry of the model. The fermionic part is generated by the supercharges  $\mathbb{Q}_\alpha^a$  and  $\mathbb{S}_b^\beta$ . The ‘dagger’ symbol is to remember that, in unitary representations, the two charges are indeed conjugate of each other, and a similar conjugation condition holds for the supercharges.

The representation of [39] gives a *dynamical* spin-chain, *i.e.* sites can be created/destroyed by the action of the generators. The central charges act as

$$\mathbb{H} |p\rangle = \epsilon(p) |p\rangle, \quad \mathbb{C} |p\rangle = c(p) |p Z^-\rangle, \quad \mathbb{C}^\dagger |p\rangle = \bar{c}(p) |p Z^+\rangle, \tag{3.9}$$

where  $Z^{+(-)}$  adds (removes) one ‘site’ (*i.e.*, one of the scalar fields  $Z$  in the infinite string that constitutes the vacuum state) to (from) the chain. We denote as  $|p\rangle$  the one-magnon state of momentum  $p$ . This state is given by  $|p\rangle = \sum_n e^{ipn} |\dots Z Z \phi(n) Z \dots\rangle$ ,  $\phi$  being one of the 4 possible orientations of the ‘spin’ in the fundamental representation of  $\mathfrak{psu}(2|2)_c$ . The eigenvalue  $\epsilon(p)$  is the energy (dispersion relation) of the magnon excitation. As we will shortly see,  $c(p)$  contains the exponential of the momentum  $p$  itself. So does  $\bar{c}(p)$ , which in unitary (*alias*, real-momentum) representations is just the conjugate of  $c(p)$ .

The length-changing property can be interpreted, at the Hopf algebra level, as a nonlocal modification of the (otherwise trivial) coproduct [3]. Let us spell out the case

of the central charges. When acting on a two-particle state, one computes

$$\begin{aligned} \mathbb{C} \otimes \mathbb{1} |p_1\rangle \otimes |p_2\rangle &= \\ \mathbb{C} \otimes \mathbb{1} \sum_{n_1 \ll n_2} e^{i p_1 n_1 + i p_2 n_2} | \dots Z Z \phi_1 \underbrace{Z \dots Z}_{n_2 - n_1 - 1} \phi_2 Z \dots \rangle &= \\ (\text{rescaling } n_2) &= c(p_1) e^{i p_2} |p_1\rangle \otimes |p_2\rangle. \end{aligned} \quad (3.10)$$

This action is non-local, since acting on the first magnon (with momentum  $p_1$ ) produces a result which also depends on the momentum  $p_2$  of the second magnon.

We must now impose compatibility of the S-matrix with the symmetry algebra carried by the excitations. Imposing such S-matrix invariance condition  $\Delta(\mathbb{C})S = S\Delta(\mathbb{C})$  implies computing

$$S \Delta(\mathbb{C}) = S [\mathbb{C} \otimes \mathbb{1} + \mathbb{1} \otimes \mathbb{C}] = S [e^{i p_2} \mathbb{C}_{local} \otimes \mathbb{1} + \mathbb{1} \otimes \mathbb{C}_{local}], \quad (3.11)$$

where  $\mathbb{C}_{local}$  is the *local* part of  $\mathbb{C}$ , acting as  $\mathbb{C}_{local}|p\rangle = c(p)|p\rangle$ . An analogous argument works for  $\Delta(\mathbb{C})S$ . One can rewrite (3.11) as

$$\Delta(\mathbb{C}_{local}) = \mathbb{C}_{local} \otimes e^{i p} + \mathbb{1} \otimes \mathbb{C}_{local}. \quad (3.12)$$

Formula (3.12) is the manifestation of a non-trivial Hopf-algebra coproduct<sup>6</sup>. Similarly, to all (super)charges of  $\mathfrak{psu}(2|2)_c$ , one assigns an additive quantum number  $[[A]]$  s.t.

$$\Delta(\mathfrak{J}^A) = \mathfrak{J}^A \otimes e^{i[[A]]p} + \mathbb{1} \otimes \mathfrak{J}^A, \quad (3.13)$$

which gives a (Lie) superalgebra homomorphism. Coint and antipode are derived from the Hopf algebra axioms, and the whole structure defines a consistent Hopf algebra. The S-matrix invariance should be written as

$$\Delta^{op} R = R \Delta \quad (3.14)$$

(quasi-cocommutativity), where the invertible  $R$ -matrix is defined as  $R = PS$ ,  $P$  being the graded permutation. There is a consistency requirement: since  $\Delta(\mathbb{C})$  is central,

$$\Delta^{op}(\mathbb{C}) R = R \Delta(\mathbb{C}) = \Delta(\mathbb{C}) R \quad \implies \quad \Delta^{op}(\mathbb{C}) = \Delta(\mathbb{C}). \quad (3.15)$$

This is guaranteed by interpreting as algebraic condition the physical requirement

$$U \equiv e^{i p} \mathbb{1} = \kappa \mathbb{C} + \mathbb{1} \quad (3.16)$$

for a constant  $\kappa$  related to the coupling  $g$  [39].

A version of the coproduct (3.13) was shown to emerge from the dual worldsheet string-theory. In [40], the result was reproduced by applying the standard Bernard-LeClair procedure [37] to the light-cone worldsheet Noether charges obtained in [41].

---

<sup>6</sup>We remark that a (nonlocal) basis change for spin-chain states can produce  $e^{i p}$  factors in different places in the coproduct (possibly with a different power), with no deep consequences.

## Chapter VI.2: Yangian Algebra

A semi-classical argument, based on the same reasoning presented at the end of section 3, is as follows. The light-cone worldsheet Noether supercharges have nonlocal contributions in the physical fields:

$$\mathfrak{J}^A = \int_{-\infty}^{\infty} d\sigma J_0^A(\sigma) e^{i[[A]] \int_{-\infty}^{\sigma} d\sigma' \partial x^-(\sigma')}. \quad (3.17)$$

If we consider, as before, two well-separated soliton excitations, the *semiclassical action* of these charges on such a scattering state is again obtained by splitting the integrals:

$$\begin{aligned} \mathfrak{J}^A|_{profile} &= \int_{-\infty}^{\infty} d\sigma J_0^A(\sigma)|_{profile} e^{i[[A]] \int_{-\infty}^{\sigma} d\sigma' \partial x^-(\sigma')|_{profile}} \\ &= \int_{-\infty}^0 d\sigma J_0^A(\sigma) e^{i[[A]] \int_{-\infty}^{\sigma} d\sigma' \partial x^-(\sigma')} + \int_0^{\infty} d\sigma J_0^A(\sigma) e^{i[[A]] \int_{-\infty}^{\sigma} d\sigma' \partial x^-(\sigma')} e^{i[[A]] \int_0^{\sigma} d\sigma' \partial x^-(\sigma')} \\ &\sim \mathfrak{J}_1^A + e^{i[[A]] p_1} \mathfrak{J}_2^A \quad \longrightarrow \quad \Delta(\mathfrak{J}^A) = \mathfrak{J}^A \otimes \mathbb{1} + e^{i[[A]] p} \otimes \mathfrak{J}^A, \end{aligned} \quad (3.18)$$

where one has used the definition of the worldsheet momentum for the first excitation.

From the Hopf-algebra antipode  $\Sigma$  one derives the so-called ‘antiparticle’ representation  $\tilde{\mathfrak{J}}^A$  and the corresponding charge-conjugation matrix  $C$ :

$$\Sigma(\mathfrak{J}^A) = C^{-1} [\tilde{\mathfrak{J}}^A]^{st} C, \quad (3.19)$$

where  $M^{st}$  is the supertranspose of  $M$ . These are the ingredients entering the crossing-symmetry relations originally written down in [2], where the existence of an underlying Hopf-algebra of the S-matrix was conjectured. The antiparticle representation and the constraints on the overall scalar factor of the S-matrix as found in [2], naturally follow from (3.19) combined with the general formulas

$$(\Sigma \otimes \mathbb{1}) R = (\mathbb{1} \otimes \Sigma^{-1}) R = R^{-1}, \quad (3.20)$$

where the antipode is derived from the coproduct (3.13).

A reformulation in terms of a Zamolodchikov-Faddeev (ZF) algebra has been given in [42]. There, the basic objects are creation and annihilation operators, with commutation relations given in terms of the S-matrix. Also, a  $q$ -deformation of this structure and of the one-dimensional Hubbard model is studied in [43].

### 3.2.2 The Yangian of the S-matrix

The S-matrix in the fundamental representation has been shown to possess  $\mathfrak{psu}(2|2)_c$  Yangian symmetry [4]. In order to be a Lie superalgebra homomorphism, the coproduct should respect (3.1). Therefore, the structure of the Yangian coproduct has to take into account the deformation in (3.13):

$$\Delta(\widehat{\mathfrak{J}}^A) = \widehat{\mathfrak{J}}^A \otimes \mathbb{1} + U^{[[A]]} \otimes \widehat{\mathfrak{J}}^A + \frac{1}{2} f_{BC}^A \mathfrak{J}^B U^{[[C]]} \otimes \mathfrak{J}^C. \quad (3.21)$$

The representation for  $\widehat{\mathfrak{J}}^A$  is the so-called *evaluation* representation, typically obtained by multiplying level-zero generators by a ‘spectral’ parameter. Here

$$\widehat{\mathfrak{J}}^A = u \mathfrak{J}^A = ig \left( x^+ + \frac{1}{x^+} - \frac{i}{2g} \right) \mathfrak{J}^A. \quad (3.22)$$

The variables  $x^{\pm}$  parameterize the fundamental representation (conventions as in [7]).

A special remark concerns the dual structure constants  $f_{BC}^A$ . They should reproduce the general form (3.3), and analogous ones with all indices lowered should be used to prove the Serre relations (3.2). However, since the Killing form of  $\mathfrak{psu}(2|2)_c$  is zero, one has a problem in defining these structure constants. In [4], the quantities  $f_{BC}^A$  are explicitly given as a list of numbers, without necessarily referring to an index-lowering procedure<sup>7</sup>. The table of coproducts is in this way fully determined.

Another remark concerns the dependence of the spectral parameter  $u$  on the representation variables  $x^\pm$ , or, equivalently, on the eigenvalues of the central charges of  $\mathfrak{psu}(2|2)_c$ . For simple Lie algebras, the spectral parameter is typically an additional variable attached to the evaluation representation. Together with the existence of a *shift*-automorphism  $u \rightarrow u + \text{const}$  of the Yangian in evaluation representations, this implies that the Yangian-invariant S-matrix is of difference-form  $S = S(u_1 - u_2)$ . The dependence of  $u$  on the central charges alters this property, and one does not have a difference form in the fundamental S-matrix (see [48] and section 3.1.1).

The full quantum S-matrix is also invariant under the following exact symmetry, found in [8] and shortly afterwards confirmed in [9]:

$$\begin{aligned} \Delta(\widehat{\mathbb{B}}') &= \widehat{\mathbb{B}}' \otimes \mathbb{1} + \mathbb{1} \otimes \widehat{\mathbb{B}}' + \frac{i}{2g}(\mathbb{S}_\alpha^\alpha \otimes \mathbb{Q}_\alpha^a + \mathbb{Q}_\alpha^a \otimes \mathbb{S}_\alpha^\alpha), \\ \Sigma(\widehat{\mathbb{B}}') &= -\widehat{\mathbb{B}}' + \frac{2i}{g}\mathbb{H}, \\ \widehat{\mathbb{B}}' &= \frac{1}{4}(x^+ + x^- - 1/x^+ - 1/x^-) \text{diag}(1, 1, -1, -1). \end{aligned} \quad (3.23)$$

This coproduct is reminiscent of a level one Yangian symmetry (cf. (3.3)). We will see in the next section the relevance of this generator for the classical  $r$ -matrix. Commuting this symmetry with the (level zero) generators, one obtains novel exact Yangian (super)symmetries of S [8]. The latter act on bosons and fermions with two *different* spectral parameters, reducing in the classical limit to the supercharges of [49].

## 4 The classical $r$ -matrix

The form of the Yangian we discussed resembles the standard one while simultaneously showing some unexpected features. In order to gain a deeper understanding it is commonly advantageous to study certain limits. One important instance is the *classical* limit, *i.e.* one studies perturbations of the  $R$ -matrix around the identity:

$$R = \mathbb{1} \otimes \mathbb{1} + \hbar r + \mathcal{O}(\hbar^2), \quad (4.1)$$

$\hbar$  being a small parameter. The first-order term  $r$  is called the *classical*  $r$ -matrix<sup>8</sup>. One can easily prove that, if  $R$  satisfies the Yang-Baxter equation (YBE),  $r$  satisfies the

<sup>7</sup>An argument in [4] suggests interpreting these quantities as dual structure constants in an enlarged algebra with invertible Killing form, see also [44]. This algebra is obtained by adjoining the  $\mathfrak{sl}(2)$  automorphism of  $\mathfrak{psu}(2|2)_c$  [45,46]. Apart from allowing inversion of the Killing form and determination of  $f_{BC}^A$ , these extra generators would drop out of the final form of the Yangian coproduct (3.21). We also refer to [47] for a derivation of the Yangian coproducts using the exceptional Lie superalgebra  $\mathfrak{D}(2, 1; \alpha)$ .

<sup>8</sup> $r$  lives in  $\mathfrak{g} \otimes \mathfrak{g}$ , for  $\mathfrak{g}$  an algebra,  $R$  in  $U(\mathfrak{g}) \otimes U(\mathfrak{g})$ ,  $U(\mathfrak{g})$  the universal enveloping algebra of  $\mathfrak{g}$ .

classical YBE (CYBE):

$$[r_{12}, r_{13}] + [r_{12}, r_{23}] + [r_{13}, r_{23}] = 0. \quad (4.2)$$

In known cases, studying (4.2) one can classify the solutions of the YBE itself, and the possible quantum group structures underlying such solutions (Belavin-Drinfeld theorem [50]). We will not reproduce here the details. Knowing the  $r$ -matrix, there is a standard procedure for constructing an associate Lie bialgebra, and *quantizing* it<sup>9</sup> in terms of so-called ‘Manin triples’ (see *e.g.* [13]). The quantum structures for simple Lie algebras are elliptic quantum groups, (trigonometric) quantum groups and Yangians. Analogous theorems for superalgebras are investigated in [51]. An illuminating example is Yang’s  $r$ -matrix ( $C_2$  is the quadratic Casimir)

$$r = \frac{C_2}{u_2 - u_1}. \quad (4.3)$$

This is the prototypical rational solution of the CYBE<sup>10</sup>. The geometric series gives

$$r = \frac{C_2}{u_2 - u_1} = \frac{\mathfrak{J}^A \otimes \mathfrak{J}_A}{u_2 - u_1} = \sum_{n \geq 0} \mathfrak{J}^A u_1^n \otimes \mathfrak{J}_A u_2^{-n-1} = \sum_{n \geq 0} \mathfrak{J}_n^A \otimes \mathfrak{J}_{A, -n-1}, \quad (4.4)$$

for  $|u_1/u_2| < 1$ . Such rewriting attributes dependence on the  $u_1$  ( $u_2$ ) to operators in the first (second) space (*factorization*). This gives  $r$  the form of tensor product of algebra representations. Assigning  $\mathfrak{J}_n^A = u^n \mathfrak{J}^A$  in (4.4) gives loop-algebra relations

$$[\mathfrak{J}_m^A, \mathfrak{J}_n^B] = f_C^{AB} \mathfrak{J}_{m+n}^C. \quad (4.5)$$

The loop algebra is precisely the ‘classical’ limit of the Yangian  $\mathcal{Y}(\mathfrak{g})$  (see section 3). With this example one realizes how *rational* solutions of the CYBE, such as (4.3), starting as not-better specified elements of  $\mathfrak{g} \otimes \mathfrak{g}$  for a Lie algebra  $\mathfrak{g}$ , give rise to Yangians upon quantization (namely, their quantized version takes values in  $\mathcal{Y}(\mathfrak{g}) \otimes \mathcal{Y}(\mathfrak{g})$ ). For related aspects concerning the classical  $r$ -matrix, see [32].

## 4.1 $\mathfrak{psu}(2|2)_c$

In the case of the S-matrix found in [39], the parameter controlling the classical expansion is naturally the inverse of the coupling constant  $g$  (near-BMN limit [52]):

$$R = \mathbb{1} \otimes \mathbb{1} + \frac{1}{g} r + \mathcal{O}\left(\frac{1}{g^2}\right). \quad (4.6)$$

The classical  $r$ -matrix  $r$  is identified with the tree-level string scattering matrix computed in [40]. In the parameterization of [53] one has

$$x^\pm(x) = x \sqrt{1 - \frac{1}{g^2(x - \frac{1}{x})^2}} \pm \frac{ix}{g(x - \frac{1}{x})} \rightarrow x. \quad (4.7)$$

<sup>9</sup>Meaning completing the Lie bialgebra to a quantum group (classical  $r$ - to quantum R-matrix).

<sup>10</sup>Since by definition  $[C_2, \mathfrak{J}^A \otimes \mathbb{1} + \mathbb{1} \otimes \mathfrak{J}^A] = 0 \forall A$ , the CYBE is easily proven for (4.3).

One sends  $g$  to  $\infty$  with  $x$  fixed.  $x$  is interpreted as an unconstrained ‘classical’ variable. This classical limit was studied in [54]. The target is finding the complete algebra the  $r$ -matrix takes values in, whose quantization can reveal the full quantum symmetry of the S-matrix. The fundamental representation tends to a limiting centrally-extended  $\mathfrak{psu}(2|2)$ , with generators parameterized by  $x$ . The classical  $r$ -matrix  $r = r(x_1, x_2)$  is not of difference form. The Lie superalgebra is not simple and has zero dual Coxeter number. This prevents applying Belavin-Drinfeld type of theorems. Nevertheless,  $r$  has a simple pole at  $x_1 - x_2 = 0$  with residue<sup>11</sup> the Casimir  $C_2$  of  $\mathfrak{gl}(2|2)$ :

$$C_2 = \sum_{i,j=1}^4 (-)^{[j]} E_{ij} \otimes E_{ji}, \quad (4.8)$$

with  $E_{ij}$  matrices with all zeros but 1 in position  $(i, j)$ , and  $[j]$  the fermionic grading of the index  $j$ . In the absence of a quadratic Casimir for  $\mathfrak{psu}(2|2)_c$ , the classical  $r$ -matrix displays on the pole (it ‘borrows’) the Casimir of a bigger algebra<sup>12</sup> for which a non-degenerate form exists and the quadratic Casimir can be constructed. This ‘borrowing’ reminds a mathematical prescription due to Khoroshkin and Tolstoy [55,20]. One expects that, if a universal  $R$ -matrix exists and if it has to be of Khoroshkin-Tolstoy type, an additional Cartan element of type  $\mathbb{B}$  has to appear.

Type- $\mathbb{B}$  generators play an important role in factorizing  $r$ . The present  $r$  is more complicated than Yang’s one, and it is harder to find a suitable geometric-like series expansion. A first proposal for the fundamental representation was given [49], with a Yangian tower of  $\mathbb{B}$ ’s coupled to a tower of  $\mathbb{H}$ ’s to achieve factorization. This proposal fails to reproduce the bound-state classical  $r$ -matrix [56].

A universal formula was advanced in [9]. It has been shown to reproduce also the classical limit of the bound-state S-matrix [57, 7], and it reads

$$r = \frac{\mathcal{T} - \tilde{\mathbb{B}} \otimes \mathbb{H} - \mathbb{H} \otimes \tilde{\mathbb{B}}}{i(u_1 - u_2)} - \frac{\tilde{\mathbb{B}} \otimes \mathbb{H}}{iu_2} + \frac{\mathbb{H} \otimes \tilde{\mathbb{B}}}{iu_1} - \frac{\mathbb{H} \otimes \mathbb{H}}{\frac{2iu_1u_2}{u_1 - u_2}}, \quad (4.9)$$

$$\begin{aligned} \mathcal{T} &= 2 (\mathbb{R}_\beta^\alpha \otimes \mathbb{R}_\alpha^\beta - \mathbb{L}_b^a \otimes \mathbb{L}_a^b + \mathbb{S}_a^\alpha \otimes \mathbb{Q}_\alpha^a - \mathbb{Q}_\alpha^a \otimes \mathbb{S}_a^\alpha), \\ \tilde{\mathbb{B}} &= \frac{1}{4\epsilon(p)} \text{diag}(1, 1, -1, -1). \end{aligned} \quad (4.10)$$

In this formula, the generators are in their classical limit, the variable  $u$  is the classical limit of (3.22), and  $\epsilon(p)$  is the classical energy (cf. section 4.1). All classical Yangian generators are obtained as  $\tilde{\mathfrak{J}}_n = u^n \mathfrak{J}$  after factorizing *via* the geometric series expansion. Quantization of this formula is an open problem. The classical analysis seems to suggest that the triple central extension may have to merge into some sort of deformation of the loop algebra of  $\mathfrak{gl}(2|2)$ , where the additional generator  $\mathbb{B}$  is sitting. Another open question is how to relate the results described here to the  $r, s$  non-ultralocal structure of the  $\mathfrak{psu}(2, 2|4)$  sigma-model [32, 58].

<sup>11</sup>As a consequence of the CYBE, such residue must be a Casimir.

<sup>12</sup> $\mathfrak{gl}(2|2)$  is obtained by adjoining to  $\mathfrak{su}(2|2)$  the non-supertraceless element  $\mathbb{B} = \text{diag}(1, 1, -1, -1)$ .

### 4.1.1 Difference Form

Formula (4.9) displays an interesting structure where the dependence on the spectral parameter  $u$  is (almost purely) of difference form. The non-difference form is encoded in the representation labels  $x^\pm(u)$  appearing in the symmetry generators, and in the last three terms of formula (4.9). Moreover, Drinfeld's second realization for the  $\mathfrak{psu}(2|2)_c$  Yangian has been obtained in [59], together with the suitable evaluation representation. The Yangian Serre relations, which were left as an open question in [4], are proven to be satisfied in the second realization (see also [60].) The representation of [59] possesses a shift-automorphism  $u \rightarrow u + \text{const}$ , which normally guarantees the difference form of the S-matrix. All this suggests the following, provided an algebraic interpretation of the last three terms in formula (4.9) can be found that generalizes to the full quantum case (possibly along the case of the ideas reported in [9] in terms of twists). Modulo this interpretation, one might hope to achieve a rewriting of the quantum S-matrix such that the dependence on  $u_1$  and  $u_2$  is (almost purely) of difference form, the rest being taken care of by suitable combinations of algebra generators<sup>13</sup>. One would expect this as the result of evaluating a hypothetical Yangian universal  $R$ -matrix in this particular representation. This expectation seems to be consistent with recent studies of the exceptional Lie superalgebra  $\mathfrak{D}(2, 1; \alpha)$  [39, 47, 60]<sup>14</sup>, and with the explicit form of the bound state S-matrix (see next section).

## 5 The bound state S-matrix

The previous discussion highlights the importance of investigating the structure of the S-matrix for generic representations of  $\mathfrak{psu}(2|2)_c$ . One motivation is obtaining the universal  $R$ -matrix and understanding the role of the  $\mathbb{B}'$  symmetry. There is also a more stringent need related to finite-size corrections to the energies according to the TBA approach [63]. According to this philosophy, it becomes crucial to have a concrete realization of the (mirror) bound state S-matrices. Usually, these can be *bootstrapped* once the S-matrix of fundamental constituents is known [12]. However, the present case is more complicated. The fundamental S-matrix does not reduce to a projector on the bound state pole, related to the fact that the tensor product of two short representations (generically irreducible) becomes reducible but indecomposable on the pole. The only way to construct the S-matrix for bound states seems to be a direct derivation from the Lie superalgebra invariance in each bound state representation. This becomes rapidly cumbersome [64]. Moreover, this does not uniquely fix the S-matrix when the bound state number increases, and one needs to resort to YBE, or, as shown in [57], to Yangian invariance. The Yangian eventually provides an efficient solution to this problem and it allows to uniquely determine the S-matrix for arbitrary bound state numbers [7].

The bound state representations are atypical (short) completely symmetric repre-

---

<sup>13</sup>In the fundamental representation, such a rewriting has been shown to be possible in [61]. The resulting form is reminiscent of what a Khoroshkin-Tolstoy type of formula (or some natural quantization of the classical  $r$ -matrix (4.9)) would look like in this representation.

<sup>14</sup> $\mathfrak{psu}(2|2)_c$  can be obtained by suitable contraction of  $\mathfrak{D}(2, 1; \alpha)$ . See also [62].

representations of dimension  $4\ell$ ,  $\ell = 1, 2, \dots$ . They all extend to evaluation representations of the Yangian, with appropriate evaluation parameter  $u$  [57]. A convenient realization is given in terms of differential operators acting on the space of degree  $M$  polynomials (superfields) in two bosonic ( $w_a$ ,  $a = 1, 2$ ) and two fermionic ( $\theta_\alpha$ ,  $\alpha = 1, 2$ ) variables. All details can be found in [7]. The essence of the construction consists in finding a closed subset of states  $|x_i\rangle$  for which the S-matrix can be computed exactly in terms of a definite matrix  $M$ . One then generates all other states  $|y_A\rangle$  by acting with (Yangian) coproducts on this closed subsector, and using quasi-cocommutativity:

$$R|y_A\rangle = R\Delta(\mathbb{J})_A^i|x_i\rangle = \Delta^{op}(\mathbb{J})_A^i R|x_i\rangle = \Delta^{op}(\mathbb{J})_A^i M_i^j|x_j\rangle. \quad (5.1)$$

On the other hand,  $R|y_A\rangle = R_A^B|y_A\rangle = R_A^B\Delta(\mathbb{J})_B^i|x_i\rangle$ . The task is to find as many states as needed to invert the above relation, namely  $R_A^B = \Delta^{op}(\mathbb{J})_A^i M_i^j [\Delta(\mathbb{J})^{-1}]_j^B$ .

The construction automatically provides a *factorizing twist* [65] for the R-matrix in the bound state representations (hence also for the fundamental representation):

$$R = F_{21} \times F_{12}^{-1}. \quad (5.2)$$

However, we remark that the coproduct twisted with  $F_{12}$  is by construction cocommutative, but, as expected, not at all trivial. Furthermore, apart perhaps from the overall factor, the bound state S-matrix depends only on  $u_1 - u_2$ , on combinatorial factors involving the integer bound-state components, and on specific combination of algebra labels  $a_i, b_i, c_i, d_i$ . These combinations are the same noticed in [61]. It remains hard to figure out a universal formula reproducing this S-matrix. Nevertheless, it looks like such a universal object would treat the evaluation parameters of the Yangian as truly independent variables, the latter appearing only in difference-form due to the Yangian shift-automorphism. The rest of the labels would appear because of the presence in the universal R-matrix of the (super)charges in the typical ‘positive  $\otimes$  negative’-roots combinations, breaking the difference-form due to the constraint that links the evaluation parameter to the central charges. This is consistent with the findings of [66], where one of the blocks of the S-matrix has been related to the universal R-matrix of the Yangian of  $\mathfrak{sl}(2)$  in arbitrary bound state representations.

The bound state S-matrix have been utilized in [67] to verify certain conjectures appeared in the literature, concerning the eigenvalues of the transfer matrix in specific short representations [46]. Long representations have been studied in [68].

## 6 Acknowledgments

I would like to warmly thank C. Sieg, J. Plefka, F. Spill, H. Yamane, I. Heckenberger, S. Moriyama, T. Matsumoto, G. Arutyunov, M. de Leeuw and R. Suzuki for the most enjoyable collaborations on the topic of this review, and all the people I had the privilege to share discussions with. I would like to especially thank N. Beisert for carefully reading the manuscript and suggesting several improvements. This work has been partially supported by EPSRC through the grant no. EP/H000054/1.

## References

- [1] M. Staudacher, “Talk at “Strings 2008”, CERN, Geneva, 18 – 23 August 2008”, <http://ph-dep-th.web.cern.ch/ph-dep-th/content2/workshops/strings2008/>.
- [2] R. A. Janik, “The  $AdS_5 \times S^5$  superstring worldsheet  $S$ -matrix and crossing symmetry”, Phys. Rev. D73, 086006 (2006), [hep-th/0603038](#).
- [3] C. Gomez and R. Hernandez, “The magnon kinematics of the  $AdS/CFT$  correspondence”, JHEP 0611, 021 (2006), [hep-th/0608029](#). • J. Plefka, F. Spill and A. Torrielli, “On the Hopf algebra structure of the  $AdS/CFT$   $S$ -matrix”, Phys. Rev. D74, 066008 (2006), [hep-th/0608038](#).
- [4] N. Beisert, “The  $S$ -Matrix of  $AdS/CFT$  and Yangian Symmetry”, PoS SOLVAY, 002 (2006), [arxiv:0704.0400](#).
- [5] A. N. Kirillov and N. Y. Reshetikhin, “The Yangians, Bethe Ansatz and combinatorics”, Lett. Math. Phys. 12, 199 (1986).
- [6] M. de Leeuw, “The Bethe Ansatz for  $AdS_5 \times S^5$  Bound States”, JHEP 0901, 005 (2009), [arxiv:0809.0783](#).
- [7] G. Arutyunov, M. de Leeuw and A. Torrielli, “The Bound State  $S$ -Matrix for  $AdS_5 \times S^5$  Superstring”, Nucl. Phys. B819, 319 (2009), [arxiv:0902.0183](#).
- [8] T. Matsumoto, S. Moriyama and A. Torrielli, “A Secret Symmetry of the  $AdS/CFT$   $S$ -matrix”, JHEP 0709, 099 (2007), [arxiv:0708.1285](#).
- [9] N. Beisert and F. Spill, “The Classical  $r$ -matrix of  $AdS/CFT$  and its Lie Bialgebra Structure”, Commun. Math. Phys. 285, 537 (2009), [arxiv:0708.1762](#).
- [10] J. M. Drummond, “Review of  $AdS/CFT$  Integrability, Chapter V.2: Dual Superconformal Symmetry”, [arxiv:1012.4002](#).
- [11] V. Chari and A. Pressley, “A guide to quantum groups”, Cambridge University Press (1994), Cambridge, UK.
- [12] A. B. Zamolodchikov and A. B. Zamolodchikov, “Factorized  $S$ -matrices in two dimensions as the exact solutions of certain relativistic quantum field models”, Annals Phys. 120, 253 (1979). • P. Dorey, “Exact  $S$  matrices”, [hep-th/9810026](#).
- [13] P. Etingof and O. Schiffman, “Lectures on Quantum Groups”, International Press (1998), Boston, USA.
- [14] N. J. MacKay, “Introduction to Yangian symmetry in integrable field theory”, Int. J. Mod. Phys. A20, 7189 (2005), [hep-th/0409183](#).
- [15] A. Molev, “Yangians and Classical Lie Algebras”, AMS (2007), Providence, RI, USA.
- [16] L. D. Faddeev and L. A. Takhtajan, “Hamiltonian Methods in the Theory of Solitons”, Springer (1987), Berlin, Germany.
- [17] T. Curtright and C. K. Zachos, “Supersymmetry and the nonlocal Yangian deformation symmetry”, Nucl. Phys. B402, 604 (1993), [hep-th/9210060](#). • Y.-Z. Zhang, “Super-Yangian double and its central extension”, Phys. Lett. A234, 20 (1997). • V. Stukopin, “Yangians of classical Lie superalgebras: Basic constructions, quantum double and universal  $R$ -matrix”, Proceedings of the Institute of Math. of NAS of Ukraine 50, 1195 (2004). • L. Gow, “Gauss

- Decomposition of the Yangian  $Y(\mathfrak{gl}(m|n))$* ”, Commun. Math. Phys. 276, 799 (2007), math/0605219. • F. Spill, “*Weakly coupled  $\mathcal{N} = 4$  Super Yang-Mills and  $\mathcal{N} = 6$  Chern-Simons theories from  $u(2/2)$  Yangian symmetry*”, JHEP 0903, 014 (2009), arxiv:0810.3897. • A. Rej and F. Spill, “*The Yangian of  $sl(n/m)$  and the universal  $R$ -matrix*”, arxiv:1008.0872.
- [18] V. G. Drinfel’d, “*Quantum groups*”, J. Math. Sci. 41, 898 (1988).
- [19] V. G. Drinfeld, “*A new realization of Yangians and quantum affine algebras*”, Soviet Math. Dokl. 36, 212 (1988).
- [20] S. M. Khoroshkin and V. N. Tolstoy, “*Yangian double*”, Lett. Math. Phys. 36, 373 (1996), hep-th/9406194.
- [21] D. Bernard, “*An Introduction to Yangian Symmetries*”, Int. J. Mod. Phys. B7, 3517 (1993), hep-th/9211133.
- [22] L. Dolan, C. R. Nappi and E. Witten, “*A relation between approaches to integrability in superconformal Yang-Mills theory*”, JHEP 0310, 017 (2003), hep-th/0308089.
- [23] L. Dolan, C. R. Nappi and E. Witten, “*Yangian symmetry in  $D = 4$  superconformal Yang-Mills theory*”, hep-th/0401243.
- [24] L. Dolan and C. R. Nappi, “*Spin models and superconformal Yang-Mills theory*”, Nucl. Phys. B717, 361 (2005), hep-th/0411020.
- [25] D. Serban and M. Staudacher, “*Planar  $\mathcal{N} = 4$  gauge theory and the Inozemtsev long range spin chain*”, JHEP 0406, 001 (2004), hep-th/0401057. • A. Agarwal and S. G. Rajeev, “*Yangian symmetries of matrix models and spin chains: The dilatation operator of  $\mathcal{N} = 4$  SYM*”, Int. J. Mod. Phys. A20, 5453 (2005), hep-th/0409180. • A. Agarwal, “*Comments on higher loop integrability in the  $su(1/1)$  sector of  $\mathcal{N} = 4$  SYM: Lessons from the  $su(2)$  sector*”, hep-th/0506095.
- [26] B. I. Zwiebel, “*Yangian symmetry at two-loops for the  $su(2/1)$  sector of  $\mathcal{N} = 4$  SYM*”, J. Phys. A40, 1141 (2007), hep-th/0610283.
- [27] N. Beisert and B. I. Zwiebel, “*On Symmetry Enhancement in the  $psu(1,1/2)$  Sector of  $\mathcal{N} = 4$  SYM*”, JHEP 0710, 031 (2007), arxiv:0707.1031.
- [28] A. Rej, “*Review of AdS/CFT Integrability, Chapter I.3: Long-range spin chains*”, arxiv:1012.3985.
- [29] N. Beisert, C. Kristjansen and M. Staudacher, “*The dilatation operator of  $\mathcal{N} = 4$  super Yang-Mills theory*”, Nucl. Phys. B664, 131 (2003), hep-th/0303060. • N. Beisert and T. Klose, “*Long-range  $gl(n)$  integrable spin chains and plane-wave matrix theory*”, J. Stat. Mech. 0607, P006 (2006), hep-th/0510124. • N. Beisert and D. Erkal, “*Yangian Symmetry of Long-Range  $gl(N)$  Integrable Spin Chains*”, J. Stat. Mech. 0803, P03001 (2008), arxiv:0711.4813. • B. I. Zwiebel, “*Iterative Structure of the  $\mathcal{N} = 4$  SYM Spin Chain*”, JHEP 0807, 114 (2008), arxiv:0806.1786.
- [30] A. Agarwal and S. G. Rajeev, “*The dilatation operator of  $\mathcal{N} = 4$  SYM and classical limits of spin chains and matrix models*”, Mod. Phys. Lett. A19, 2549 (2004), hep-th/0405116. • A. Agarwal and A. P. Polychronakos, “*BPS operators in  $\mathcal{N} = 4$  SYM: Calogero models and 2D fermions*”, JHEP 0608, 034 (2006), hep-th/0602049.
- [31] N. Beisert, “*On Yangian Symmetry in Planar  $\mathcal{N} = 4$  SYM*”, arxiv:1004.5423.

- [32] M. Magro, “*Review of AdS/CFT Integrability, Chapter II.3: Sigma Model, Gauge Fixing*”, [arxiv:1012.3988](#). • S. Schafer-Nameki, “*Review of AdS/CFT Integrability, Chapter II.4: The Spectral Curve*”, [arxiv:1012.3989](#).
- [33] M. Lüscher, “*Quantum Nonlocal Charges and Absence of Particle Production in the Two-Dimensional Nonlinear Sigma Model*”, Nucl. Phys. B135, 1 (1978).
- [34] I. Bena, J. Polchinski and R. Roiban, “*Hidden symmetries of the  $AdS_5 \times S^5$  superstring*”, Phys. Rev. D69, 046002 (2004), [hep-th/0305116](#).
- [35] G. Mandal, N. V. Suryanarayana and S. R. Wadia, “*Aspects of semiclassical strings in  $AdS(5)$* ”, Phys. Lett. B543, 81 (2002), [hep-th/0206103](#).
- [36] L. F. Alday, “*Non-local charges on  $AdS_5 \times S^5$  and pp-waves*”, JHEP 0312, 033 (2003), [hep-th/0310146](#). • G. Arutyunov and M. Staudacher, “*Matching higher conserved charges for strings and spins*”, JHEP 0403, 004 (2004), [hep-th/0310182](#). • M. Hatsuda and K. Yoshida, “*Classical integrability and super Yangian of superstring on  $AdS_5 \times S^5$* ”, Adv. Theor. Math. Phys. 9, 703 (2005), [hep-th/0407044](#). • A. K. Das, J. Maharana, A. Melikyan and M. Sato, “*The algebra of transition matrices for the  $AdS_5 \times S^5$  superstring*”, JHEP 0412, 055 (2004), [hep-th/0411200](#). • L. F. Alday, G. Arutyunov and A. A. Tseytlin, “*On integrability of classical superstrings in  $AdS_5 \times S^5$* ”, JHEP 0507, 002 (2005), [hep-th/0502240](#). • S. Frolov, “*Lax pair for strings in Lunin-Maldacena background*”, JHEP 0505, 069 (2005), [hep-th/0503201](#). • A. K. Das, A. Melikyan and M. Sato, “*The algebra of flat currents for the string on  $AdS_5 \times S^5$  in the light-cone gauge*”, JHEP 0511, 015 (2005), [hep-th/0508183](#). • B. Vicedo, “*Hamiltonian dynamics and the hidden symmetries of the  $AdS_5 \times S^5$  superstring*”, JHEP 1001, 102 (2010), [arxiv:0910.0221](#).
- [37] D. Bernard and A. Leclair, “*The Quantum double in integrable quantum field theory*”, Nucl. Phys. B399, 709 (1993), [hep-th/9205064](#).
- [38] M. Lüscher and K. Pohlmeyer, “*Scattering of Massless Lumps and Nonlocal Charges in the Two-Dimensional Classical Nonlinear Sigma Model*”, Nucl. Phys. B137, 46 (1978). • N. J. MacKay, “*On the classical origins of Yangian symmetry in integrable field theory*”, Phys. Lett. B281, 90 (1992).
- [39] N. Beisert, “*The  $su(2/2)$  dynamic S-matrix*”, Adv. Theor. Math. Phys. 12, 945 (2008), [hep-th/0511082](#).
- [40] T. Klose, T. McLoughlin, R. Roiban and K. Zarembo, “*Worldsheet scattering in  $AdS_5 \times S^5$* ”, JHEP 0703, 094 (2007), [hep-th/0611169](#).
- [41] G. Arutyunov, S. Frolov, J. Plefka and M. Zamaklar, “*The off-shell symmetry algebra of the light-cone  $AdS_5 \times S^5$  superstring*”, J. Phys. A40, 3583 (2007), [hep-th/0609157](#).
- [42] G. Arutyunov, S. Frolov and M. Zamaklar, “*The Zamolodchikov-Faddeev algebra for  $AdS_5 \times S^5$  superstring*”, JHEP 0704, 002 (2007), [hep-th/0612229](#).
- [43] N. Beisert and P. Koroteev, “*Quantum Deformations of the One-Dimensional Hubbard Model*”, J. Phys. A41, 255204 (2008), [arxiv:0802.0777](#). • N. Beisert, “*The Classical Trigonometric r-Matrix for the Quantum-Deformed Hubbard Chain*”, [arxiv:1002.1097](#).
- [44] F. Spill, “*Hopf Algebras in the AdS/CFT Correspondence*”, Diploma Thesis - Humboldt University of Berlin. • F. Spill, “*Symmetries of the AdS/CFT S-matrix*”, Acta Phys. Polon. B39, 3135 (2008).

- [45] V. V. Serganova, “Automorphisms of Simple Lie Superalgebras”, *Math. USSR Izv.* 24, 539 (1985).
- [46] N. Beisert, “The Analytic Bethe Ansatz for a Chain with Centrally Extended  $su(2/2)$  Symmetry”, *J. Stat. Mech.* 0701, P017 (2007), [nlin/0610017](https://arxiv.org/abs/nlin/0610017).
- [47] T. Matsumoto and S. Moriyama, “An Exceptional Algebraic Origin of the AdS/CFT Yangian Symmetry”, *JHEP* 0804, 022 (2008), [arxiv:0803.1212](https://arxiv.org/abs/0803.1212).
- [48] V. Bazhanov, “Talk at the Conference on “Integrability in Gauge and String Theory”, Max Planck Institute for Gravitational Physics (Albert Einstein Institute), Potsdam, 29 June – 3 July 2009”, <http://int09.aei.mpg.de/talks/Bazhanov.pdf>.
- [49] S. Moriyama and A. Torrielli, “A Yangian Double for the AdS/CFT Classical  $r$ -matrix”, *JHEP* 0706, 083 (2007), [arxiv:0706.0884](https://arxiv.org/abs/0706.0884).
- [50] A. A. Belavin and V. G. Drinfeld, “Solutions of the classical Yang-Baxter equation for simple Lie algebras”, *Funct. Anal. Appl* 16, 159 (1982). • A. A. Belavin and V. G. Drinfeld, “Triangle equation for simple Lie algebras”, *Math. Phys. Rev.* 4, 93 (1984).
- [51] D. A. Leites and V. V. Serganova, “Solutions of the Classical Yang-Baxter Equation for Simple Superalgebras”, *Theor. Math. Phys.* 58, 16 (1984). • G. Karaali, “Constructing  $r$ -matrices on simple Lie superalgebras”, *J. Algebra* 282, 83 (2004), [math/0303246](https://arxiv.org/abs/math/0303246). • G. Karaali, “A New Lie Bialgebra Structure on  $sl(2,1)$ ”, *Contemp. Math.* 413, 101 (2006), [math/0410473](https://arxiv.org/abs/math/0410473).
- [52] D. Berenstein, J. M. Maldacena and H. Nastase, “Strings in flat space and pp waves from  $\mathcal{N} = 4$  Super Yang Mills”, *JHEP* 0204, 013 (2002), [hep-th/0202021](https://arxiv.org/abs/hep-th/0202021).
- [53] G. Arutyunov and S. Frolov, “On  $AdS_5 \times S^5$  string  $S$ -matrix”, *Phys. Lett.* B639, 378 (2006), [hep-th/0604043](https://arxiv.org/abs/hep-th/0604043).
- [54] A. Torrielli, “Classical  $r$ -matrix of the  $su(2/2)$  SYM spin-chain”, *Phys. Rev.* D75, 105020 (2007), [hep-th/0701281](https://arxiv.org/abs/hep-th/0701281).
- [55] S. M. Khoroshkin and V. N. Tolstoy, “Universal  $R$ -matrix for quantized (super)algebras”, *Commun. Math. Phys.* 141, 599 (1991).
- [56] M. de Leeuw, “The  $S$ -matrix of the  $AdS_5 \times S^5$  superstring”, [arxiv:1007.4931](https://arxiv.org/abs/1007.4931).
- [57] M. de Leeuw, “Bound States, Yangian Symmetry and Classical  $r$ -matrix for the  $AdS_5 \times S^5$  Superstring”, *JHEP* 0806, 085 (2008), [arxiv:0804.1047](https://arxiv.org/abs/0804.1047).
- [58] B. Vicedo, “The classical  $R$ -matrix of AdS/CFT and its Lie dialgebra structure”, [arxiv:1003.1192](https://arxiv.org/abs/1003.1192).
- [59] F. Spill and A. Torrielli, “On Drinfeld’s second realization of the AdS/CFT  $su(2/2)$  Yangian”, *J. Geom. Phys.* 59, 489 (2009), [arxiv:0803.3194](https://arxiv.org/abs/0803.3194).
- [60] T. Matsumoto and S. Moriyama, “Serre Relation and Higher Grade Generators of the AdS/CFT Yangian Symmetry”, *JHEP* 0909, 097 (2009), [arxiv:0902.3299](https://arxiv.org/abs/0902.3299).
- [61] A. Torrielli, “Structure of the string  $R$ -matrix”, *J. Phys.* A42, 055204 (2009), [arxiv:0806.1299](https://arxiv.org/abs/0806.1299).
- [62] I. Heckenberger, F. Spill, A. Torrielli and H. Yamane, “Drinfeld second realization of the quantum affine superalgebras of  $D^{(1)}(2,1/x)$  via the Weyl groupoid”, *Publ. Res. Inst. Math. Sci. Kyoto B8*, 171 (2008), [arxiv:0705.1071](https://arxiv.org/abs/0705.1071).

- [63] Z. Bajnok, “*Review of AdS/CFT Integrability, Chapter III.6: Thermodynamic Bethe Ansatz*”, [arxiv:1012.3995](#).
- [64] G. Arutyunov and S. Frolov, “*The S-matrix of String Bound States*”, Nucl. Phys. B804, 90 (2008), [arxiv:0803.4323](#).
- [65] V. G. Drinfeld, “*Quasi-Hopf algebras*”, Leningrad Math. J. 1, 1419 (1990).
- [66] G. Arutyunov, M. de Leeuw and A. Torrielli, “*Universal blocks of the AdS/CFT Scattering Matrix*”, JHEP 0905, 086 (2009), [arxiv:0903.1833](#).
- [67] G. Arutyunov, M. de Leeuw, R. Suzuki and A. Torrielli, “*Bound State Transfer Matrix for  $AdS_5 \times S^5$  Superstring*”, JHEP 0910, 025 (2009), [arxiv:0906.4783](#).
- [68] G. Arutyunov, M. de Leeuw and A. Torrielli, “*On Yangian and Long Representations of the Centrally Extended  $su(2/2)$  Superalgebra*”, JHEP 1006, 033 (2010), [arxiv:0912.0209](#).
